# Supplementary material for: Thurston's sphere packings on 3-dimensional manifolds, I
Source: arXiv:1904.11122 ancillary file (2023-05-09)
Supplement: Supplementary file 1 [file determinant1.pdf]

(\*Matrix U\* have been checked\*)

$$U = \begin{pmatrix} - (U_{ij} + U_{ik} + U_{il}) & U_{ij} & U_{ik} & U_{il} \\ U_{ij} & - (U_{ij} + U_{jk} + U_{jl}) & U_{jk} & U_{jl} \\ U_{ik} & U_{jk} & - (U_{ik} + U_{jk} + U_{kl}) & U_{kl} \\ U_{il} & U_{jl} & U_{kl} & - (U_{il} + U_{jl} + U_{kl}) \end{pmatrix};$$

(\*3-rank Minors\*)

子式

$$AA_{11} = \begin{pmatrix} - (U_{ij} + U_{jk} + U_{jl}) & U_{jk} & U_{jl} \\ U_{jk} & - (U_{ik} + U_{jk} + U_{kl}) & U_{kl} \\ U_{jl} & U_{kl} & - (U_{il} + U_{jl} + U_{kl}) \end{pmatrix};$$

Ms11 = Det [AA11];

行列式

$$AA_{12} = \begin{pmatrix} U_{ij} & U_{jk} & U_{jl} \\ U_{ik} & - (U_{ik} + U_{jk} + U_{kl}) & U_{kl} \\ U_{il} & U_{kl} & - (U_{il} + U_{jl} + U_{kl}) \end{pmatrix};$$

Ms12 = Det [AA12];

行列式

Expand [Ms12]

展开

$$U_{ij} U_{ik} U_{il} + U_{ij} U_{il} U_{jk} + U_{ik} U_{il} U_{jk} + U_{ij} U_{ik} U_{jl} + U_{ik} U_{il} U_{jl} + \\ U_{ij} U_{jk} U_{jl} + U_{ik} U_{jk} U_{jl} + U_{il} U_{jk} U_{jl} + U_{ij} U_{ik} U_{kl} + U_{ij} U_{il} U_{kl} + \\ U_{ij} U_{jk} U_{kl} + U_{ik} U_{jk} U_{kl} + U_{il} U_{jk} U_{kl} + U_{ij} U_{jl} U_{kl} + U_{ik} U_{jl} U_{kl} + U_{il} U_{jl} U_{kl}$$

$$\begin{aligned} U_{t1} &= U_{ij} U_{ik} U_{il}; & U_{t2} &= U_{ij} U_{il} U_{jk}; \\ U_{t3} &= U_{ik} U_{il} U_{jk}; & U_{t4} &= U_{ij} U_{ik} U_{jl}; \\ U_{t5} &= U_{ik} U_{il} U_{jl}; & U_{t6} &= U_{ij} U_{jk} U_{jl}; \\ U_{t7} &= U_{ik} U_{jk} U_{jl}; & U_{t8} &= U_{il} U_{jk} U_{jl}; \\ U_{t9} &= U_{ij} U_{ik} U_{kl}; & U_{t10} &= U_{ij} U_{il} U_{kl}; \\ U_{t11} &= U_{ij} U_{jk} U_{kl}; & U_{t12} &= U_{ik} U_{jk} U_{kl}; \\ U_{t13} &= U_{il} U_{jk} U_{kl}; & U_{t14} &= U_{ij} U_{jl} U_{kl}; \\ U_{t15} &= U_{ik} U_{jl} U_{kl}; & U_{t16} &= U_{il} U_{jl} U_{kl}; \end{aligned}$$

(\*Our goal is to show Ms12 is nonzero\*)

```

(*Uij=UijVijk1*)
Uij = -2 *  $\frac{Iijk * Cijkl * Aijl2 + Iijl * Cijlk * Aijk2}{192 * (lij2)^2 * Aijk2 * Aijl2}$ ; (*been checked*)
Uik = -2 *  $\frac{Iikj * Cikjl * Aikl2 + Iikl * Ciklj * Aikj2}{192 * (lik2)^2 * Aikj2 * Aikl2}$ ; (*been checked*)
Uil = -2 *  $\frac{Iilk * Ciljk * Ailj2 + Iilj * Ciljk * Ailk2}{192 * (lil2)^2 * Ailk2 * Ailj2}$ ; (*been checked*)
Ujk = -2 *  $\frac{Ijki * Cjkil * Ajkl2 + Ijkl * Cjkli * Ajki2}{192 * (ljk2)^2 * Ajki2 * Ajkl2}$ ; (*been checked*)
Ujl = -2 *  $\frac{Ijli * Cjlik * Ajlk2 + Ijlk * Cjli * Ajli2}{192 * (ljl2)^2 * Ajli2 * Ajlk2}$ ; (*been checked*)
Ukl = -2 *  $\frac{Ikli * Cklij * Aklj2 + Iklj * Cklji * Akli2}{192 * (lk12)^2 * Akli2 * Aklj2}$ ; (*been checked*)

(*Aijk2=Aijk2, (*have been checked*) *)
Aikj2 = Aijk2;
Ajki2 = Aijk2;
Ailj2 = Aijl2;
Ajli2 = Aijl2;
Ailk2 = Aikl2;
Akli2 = Aikl2;
Ajlk2 = Ajkl2;
Aklj2 = Ajkl2;

Simplify[Ut1]

$$- \left( \left( (Aijl2 Cijkl Iijk + Aijk2 Cijlk Iijl) (Aikl2 Cikjl Iikj + Aijk2 Ciklj Iikl) \right. \right. \\ \left. \left. (Aikl2 Ciljk Iilj + Aijl2 Ciljk Iilk) \right) / (884736 Aijk2^2 Aijl2^2 Aikl2^2 lij2^2 lik2^2 lil2^2) \right)$$


(*Ut1new=Simplify[Ut1*884736 Aijk22Aijl22Aikl22Ajk122lij22lik22lil22ljk22ljl22lk122]*)

```

```

Ms12tilde =
  Simplify[Ms12 * (884 736 Aijk22 Aijl22 Aikl22 Ajkl22 lij22 lik22 lil22 ljk22 ljl22 lkl22)];
  化简
Ut1new = Simplify[
  化简
  Ut1 * (884 736 Aijk22 Aijl22 Aikl22 Ajkl22 lij22 lik22 lil22 ljk22 ljl22 lkl22)];
Ut2new = Simplify[Ut2 * (884 736 Aijk22 Aijl22 Aikl22
  化简
  Ajkl22 lij22 lik22 lil22 ljk22 ljl22 lkl22)];
Ut3new = Simplify[Ut3 * (884 736 Aijk22 Aijl22 Aikl22 Ajkl22
  化简
  lij22 lik22 lil22 ljk22 ljl22 lkl22)];
Ut4new = Simplify[Ut4 * (884 736 Aijk22 Aijl22 Aikl22 Ajkl22
  化简
  lij22 lik22 lil22 ljk22 ljl22 lkl22)];
Ut5new = Simplify[Ut5 * (884 736 Aijk22 Aijl22 Aikl22 Ajkl22
  化简
  lij22 lik22 lil22 ljk22 ljl22 lkl22)];
Ut6new = Simplify[Ut6 * (884 736 Aijk22 Aijl22 Aikl22 Ajkl22
  化简
  lij22 lik22 lil22 ljk22 ljl22 lkl22)];
Ut7new = Simplify[Ut7 * (884 736 Aijk22 Aijl22 Aikl22 Ajkl22
  化简
  lij22 lik22 lil22 ljk22 ljl22 lkl22)];
Ut8new = Simplify[Ut8 * (884 736 Aijk22 Aijl22 Aikl22 Ajkl22
  化简
  lij22 lik22 lil22 ljk22 ljl22 lkl22)];
Ut9new = Simplify[Ut9 * (884 736 Aijk22 Aijl22 Aikl22 Ajkl22
  化简
  lij22 lik22 lil22 ljk22 ljl22 lkl22)];
Ut10new = Simplify[Ut10 * (884 736 Aijk22 Aijl22 Aikl22 Ajkl22
  化简
  lij22 lik22 lil22 ljk22 ljl22 lkl22)];
Ut11new = Simplify[Ut11 * (884 736 Aijk22 Aijl22 Aikl22 Ajkl22
  化简
  lij22 lik22 lil22 ljk22 ljl22 lkl22)];
Ut12new = Simplify[Ut12 * (884 736 Aijk22 Aijl22 Aikl22 Ajkl22
  化简
  lij22 lik22 lil22 ljk22 ljl22 lkl22)];
Ut13new = Simplify[Ut13 * (884 736 Aijk22 Aijl22 Aikl22 Ajkl22
  化简
  lij22 lik22 lil22 ljk22 ljl22 lkl22)];
Ut14new = Simplify[Ut14 * (884 736 Aijk22 Aijl22 Aikl22 Ajkl22
  化简
  lij22 lik22 lil22 ljk22 ljl22 lkl22)];
Ut15new = Simplify[Ut15 * (884 736 Aijk22 Aijl22 Aikl22 Ajkl22
  化简
  lij22 lik22 lil22 ljk22 ljl22 lkl22)];
Ut16new = Simplify[Ut16 * (884 736 Aijk22 Aijl22 Aikl22 Ajkl22
  化简
  lij22 lik22 lil22 ljk22 ljl22 lkl22)];

```

```

(* $\eta_{ij}=\eta_{ji}$ , have been checked*)
 $\eta_{ji} = \eta_{ij}$ ;  $\eta_{ki} = \eta_{ik}$ ;  $\eta_{li} = \eta_{il}$ ;  $\eta_{kj} = \eta_{jk}$ ;  $\eta_{lj} = \eta_{jl}$ ;  $\eta_{lk} = \eta_{kl}$ ;
 $\eta_{ij} = \eta_{ik} = \eta_{il} = \eta_{jk} = \eta_{jl} = \eta_{kl} = x$ ;

(* $C_{ijkl}=C_{ijk1}$ *)
Cijk1 = 16 * Iij1 * Aijk2 - Iijk * Bij; (*been checked*)
Cijlk = 16 * Iijk * Aijl2 - Iijl * Bij; (*been checked*)
Cikjl = 16 * Iikl * Aikj2 - Iikj * Bik; (*been checked*)
Cjkil = 16 * Ijkl * Ajki2 - Ijki * Bjk; (*been checked*)
Cjlik = 16 * Ijlk * Ajli2 - Ijli * Bjl; (*been checked*)
Cklij = 16 * Ikli * Akli2 - Ikli * Bkl; (*been checked*)
Cklji = 16 * Ikli * Aklj2 - Iklj * Bkl; (*been checked*)
Cjlkj = 16 * Ijli * Ajlk2 - Ijlk * Bjl; (*been checked*)
Cjklj = 16 * Ijki * Ajkl2 - Ijkl * Bjk; (*been checked*)
Ciklj = 16 * Iikj * Aikl2 - Iikl * Bik; (*been checked*)
Cilkj = 16 * Iilj * Ailk2 - Iilk * Bil; (*been checked*)
Ciljk = 16 * Iilk * Ailj2 - Iilj * Bil; (*been checked*)

(* $B_{ij}=B_{ij}$ *)
Bij = 2 * lij2 * (lik2 + lil2 - lk12) - (lij2 + lik2 - ljk2) * (lij2 + lil2 - lj12);
(*been checked*)
Bil = 2 * lil2 * (lik2 + lij2 - lkj2) - (lil2 + lik2 - llk2) * (lil2 + lij2 - llj2);
(*been checked*)
Bjl = 2 * lj12 * (ljk2 + lji2 - lki2) - (lj12 + ljk2 - llk2) * (lj12 + lji2 - lli2);
(*been checked*)
Bkl = 2 * lk12 * (lkj2 + lki2 - lji2) - (lk12 + lkj2 - llj2) * (lk12 + lki2 - lli2);
(*been checked*)
Bji = Bij; (*been checked*)
Bik = 2 * lik2 * (lij2 + lil2 - lj12) - (lik2 + lij2 - lkj2) * (lik2 + lil2 - lk12);
(*been checked*)
Bjk = 2 * ljk2 * (lji2 + lj12 - lli2) - (ljk2 + lji2 - lki2) * (ljk2 + lj12 - lk12);
(*been checked*)

```

```

(*Iijk=Iijk*)
Iijk = (ri)2 * (rj)2 * (1 - (ηij)2) + (ri)2 * rj * rk * γijk + ri * (rj)2 * rk * γjik;
(*been checked*)
Iilk = (ri)2 * (rl)2 * (1 - (ηil)2) + (ri)2 * rl * rk * γilk + ri * (rl)2 * rk * γlik;
(*been checked*)
Iilj = (ri)2 * (rl)2 * (1 - (ηil)2) + (ri)2 * rl * rj * γilj + ri * (rl)2 * rj * γlij;
(*been checked*)
Iklj = (rk)2 * (rl)2 * (1 - (ηkl)2) + (rk)2 * rl * rj * γklj + rk * (rl)2 * rj * γlkj;
(*been checked*)
Iikj = (ri)2 * (rk)2 * (1 - (ηik)2) + (ri)2 * rk * rj * γikj + ri * (rk)2 * rj * γkij;
(*been checked*)
Iijl = (ri)2 * (rj)2 * (1 - (ηij)2) + (ri)2 * rj * rl * γijl + ri * (rj)2 * rl * γjil;
(*been checked*)
Iikl = (ri)2 * (rk)2 * (1 - (ηik)2) + (ri)2 * rk * rl * γikl + ri * (rk)2 * rl * γkil;
(*been checked*)
Ijkl = (rj)2 * (rk)2 * (1 - (ηjk)2) + (rj)2 * rk * rl * γjkl + rj * (rk)2 * rl * γkjl;
(*been checked*)
Ijki = (rj)2 * (rk)2 * (1 - (ηjk)2) + (rj)2 * rk * ri * γjki + rj * (rk)2 * ri * γkji;
(*been checked*)
Ijlk = (rj)2 * (rl)2 * (1 - (ηjl)2) + (rj)2 * rl * rk * γjlk + rj * (rl)2 * rk * γljk;
(*been checked*)
Ijli = (rj)2 * (rl)2 * (1 - (ηjl)2) + (rj)2 * rl * ri * γjli + rj * (rl)2 * ri * γlji;
(*been checked*)
Ikli = (rk)2 * (rl)2 * (1 - (ηkl)2) + (rk)2 * rl * ri * γkli + rk * (rl)2 * ri * γlki;
(*been checked*)

(*γijk=Γijk*)
γijk = ηjk + ηij * ηik; (*been checked*)
γikj = γijk; (*been checked*)
γjik = ηik + ηji * ηjk; (*been checked*)
γlik = ηik + ηli * ηlk; γlki = γlik; (*been checked*)
γlij = ηij + ηli * ηlj; γlji = γlij; (*been checked*)
γlkj = ηkj + ηlk * ηlj; γljk = γlkj; (*been checked*)
γijl = ηjl + ηij * ηil; (*been checked*)
γilj = γijl; (*been checked*)
γikl = ηkl + ηik * ηil; (*been checked*)
γjkl = ηkl + ηjk * ηjl; (*been checked*)
γjlk = γjkl; (*been checked*)
γjki = ηki + ηjk * ηji; (*been checked*)
γilk = γikl; (*been checked*)
γkij = ηij + ηki * ηkj; γkji = γkij; (*been checked*)
γklj = ηlj + ηkl * ηkj; (*been checked*)
γkjl = γklj; (*been checked*)
γkli = ηli + ηkl * ηki; (*been checked*)
γkil = γkli; (*been checked*)
γjil = ηil + ηji * ηjl; (*been checked*)
γjli = γjil; (*been checked*)

```

```

(*Aijk2=Aijk2*)
Aijk2 =  $\frac{1}{16} * (4 * lij2 * (lik2) - ((lij2) + (lik2) - (ljk2))^2)$ ; (*been checked*)
Aikj2 = Aijk2; Ajki2 = Aijk2;
Aijl2 =  $\frac{1}{16} * (4 * (lij2) * (lil2) - ((lij2) + (lil2) - (lj12))^2)$ ;
(*been checked*)
Ailj2 = Aijl2; Ajli2 = Aijl2;
Aikl2 =  $\frac{1}{16} * (4 * (lik2) * (lil2) - ((lik2) + (lil2) - (lkl2))^2)$ ; (*been checked*)
Ailk2 = Aikl2; Akli2 = Aikl2;
Ajk12 =  $\frac{1}{16} * (4 * (ljk2) * (lj12) - ((ljk2) + (lj12) - (lkl2))^2)$ ; (*been checked*)
Ajl12 = Ajk12;
Aklj2 = Ajk12;

(*lij2=lij2*)
lij2 =  $(ri)^2 + (rj)^2 + 2 * ri * rj * \eta_{ij}$ ;
lji2 = lij2;
lik2 =  $(ri)^2 + (rk)^2 + 2 * ri * rk * \eta_{ik}$ ;
lki2 = lik2;
lil2 =  $(ri)^2 + (rl)^2 + 2 * ri * rl * \eta_{il}$ ;
lli2 = lil2;
lkl2 =  $(rk)^2 + (rl)^2 + 2 * rk * rl * \eta_{kl}$ ;
llk2 = lkl2;
ljk2 =  $(rj)^2 + (rk)^2 + 2 * rj * rk * \eta_{jk}$ ;
lkj2 = ljk2;
lj12 =  $(rj)^2 + (rl)^2 + 2 * rj * rl * \eta_{jl}$ ;
llj2 = lj12;

```

Simplify[Ut1new]

[化简]

$$\begin{aligned}
& -\frac{1}{16384} r_i^6 r_j^2 r_k^2 r_l^2 (1+x)^9 (r_i^2 + r_j^2 + 2 r_i r_j x) (r_i^2 + r_k^2 + 2 r_i r_k x) \\
& (r_j^2 + r_k^2 + 2 r_j r_k x)^2 (r_i^2 + r_l^2 + 2 r_i r_l x) (r_j^2 + r_l^2 + 2 r_j r_l x)^2 (r_k^2 + r_l^2 + 2 r_k r_l x)^2 \\
& (4 (r_j^2 + r_k^2 + 2 r_j r_k x) (r_j^2 + r_l^2 + 2 r_j r_l x) - 4 (r_j^2 - r_k r_l x + r_j (r_k + r_l) x)^2)^2 \\
& (-r_j (r_i r_l (-1+x) - r_i r_j x - r_j r_l x) (r_i r_k r_l x + r_j r_k r_l x + r_i r_j (r_l + r_k x - 2 r_l x)) \\
& (4 (r_i^2 + r_k^2 + 2 r_i r_k x) (r_i^2 + r_l^2 + 2 r_i r_l x) - 4 (r_i^2 - r_k r_l x + r_i (r_k + r_l) x)^2) + \\
& r_k (r_i r_l (-1+x) - r_i r_k x - r_k r_l x) (4 (r_i^2 + r_j^2 + 2 r_i r_j x) (r_i^2 + r_l^2 + 2 r_i r_l x) - \\
& 4 (r_i^2 - r_j r_l x + r_i (r_j + r_l) x)^2) (-r_j r_k r_l x - r_i (r_j r_l x + r_k (r_l + r_j x - 2 r_l x))) \\
& (r_l (r_i r_j (-1+x) - r_i r_l x - r_j r_l x) (4 (r_i^2 + r_j^2 + 2 r_i r_j x) (r_i^2 + r_k^2 + 2 r_i r_k x) - \\
& 4 (r_i^2 - r_j r_k x + r_i (r_j + r_k) x)^2) (-r_j r_k r_l x - r_i (r_k r_l x + r_j (r_l + r_k x - 2 r_l x))) + \\
& r_k (r_i r_j (-1+x) - r_i r_k x - r_j r_k x) (4 (r_i^2 + r_j^2 + 2 r_i r_j x) (r_i^2 + r_l^2 + 2 r_i r_l x) - \\
& 4 (r_i^2 - r_j r_l x + r_i (r_j + r_l) x)^2) (-r_j r_k r_l x - r_i (r_k r_l x + r_j (r_k - 2 r_k x + r_l x))) \\
& (r_l (r_i r_k (-1+x) - r_i r_l x - r_k r_l x) (4 (r_i^2 + r_j^2 + 2 r_i r_j x) (r_i^2 + r_k^2 + 2 r_i r_k x) - \\
& 4 (r_i^2 - r_j r_k x + r_i (r_j + r_k) x)^2) (-r_j r_k r_l x - r_i (r_j r_l x + r_k (r_l + r_j x - 2 r_l x))) + \\
& r_j (r_i r_k (-1+x) - r_i r_j x - r_j r_k x) (4 (r_i^2 + r_k^2 + 2 r_i r_k x) (r_i^2 + r_l^2 + 2 r_i r_l x) - \\
& 4 (r_i^2 - r_k r_l x + r_i (r_k + r_l) x)^2) (-r_j r_k r_l x - r_i (r_k r_l x + r_j (r_k - 2 r_k x + r_l x)))
\end{aligned}$$

$$\text{qq1} = \text{Simplify}\left[\frac{\text{Ut1new}}{r_i^2 r_j^2 r_k^2 r_l^2 (1+x)^9} * 16384 * (1 / (l_{ij}^2 * l_{ik}^2 * l_{il}^2 * l_{jk}^2 * l_{jl}^2 * l_{kl}^2))\right]$$

[化简]

$$\begin{aligned}
& -r_i^4 (r_j^2 + r_k^2 + 2 r_j r_k x) (r_j^2 + r_l^2 + 2 r_j r_l x) (r_k^2 + r_l^2 + 2 r_k r_l x) \\
& (4 (r_j^2 + r_k^2 + 2 r_j r_k x) (r_j^2 + r_l^2 + 2 r_j r_l x) - 4 (r_j^2 - r_k r_l x + r_j (r_k + r_l) x)^2)^2 \\
& (-r_j (r_i r_l (-1+x) - r_i r_j x - r_j r_l x) (r_i r_k r_l x + r_j r_k r_l x + r_i r_j (r_l + r_k x - 2 r_l x)) \\
& (4 (r_i^2 + r_k^2 + 2 r_i r_k x) (r_i^2 + r_l^2 + 2 r_i r_l x) - 4 (r_i^2 - r_k r_l x + r_i (r_k + r_l) x)^2) + \\
& r_k (r_i r_l (-1+x) - r_i r_k x - r_k r_l x) \\
& (4 (r_i^2 + r_j^2 + 2 r_i r_j x) (r_i^2 + r_l^2 + 2 r_i r_l x) - 4 (r_i^2 - r_j r_l x + r_i (r_j + r_l) x)^2) \\
& (-r_j r_k r_l x - r_i (r_j r_l x + r_k (r_l + r_j x - 2 r_l x)))) (r_l (r_i r_j (-1+x) - r_i r_l x - r_j r_l x) \\
& (4 (r_i^2 + r_j^2 + 2 r_i r_j x) (r_i^2 + r_k^2 + 2 r_i r_k x) - 4 (r_i^2 - r_j r_k x + r_i (r_j + r_k) x)^2) \\
& (-r_j r_k r_l x - r_i (r_k r_l x + r_j (r_l + r_k x - 2 r_l x))) + r_k (r_i r_j (-1+x) - r_i r_k x - r_j r_k x) \\
& (4 (r_i^2 + r_j^2 + 2 r_i r_j x) (r_i^2 + r_l^2 + 2 r_i r_l x) - 4 (r_i^2 - r_j r_l x + r_i (r_j + r_l) x)^2) \\
& (-r_j r_k r_l x - r_i (r_k r_l x + r_j (r_k - 2 r_k x + r_l x)))) (r_l (r_i r_k (-1+x) - r_i r_l x - r_k r_l x) \\
& (4 (r_i^2 + r_j^2 + 2 r_i r_j x) (r_i^2 + r_k^2 + 2 r_i r_k x) - 4 (r_i^2 - r_j r_k x + r_i (r_j + r_k) x)^2) \\
& (-r_j r_k r_l x - r_i (r_j r_l x + r_k (r_l + r_j x - 2 r_l x))) + r_j (r_i r_k (-1+x) - r_i r_j x - r_j r_k x) \\
& (4 (r_i^2 + r_k^2 + 2 r_i r_k x) (r_i^2 + r_l^2 + 2 r_i r_l x) - 4 (r_i^2 - r_k r_l x + r_i (r_k + r_l) x)^2) \\
& (-r_j r_k r_l x - r_i (r_k r_l x + r_j (r_k - 2 r_k x + r_l x))))
\end{aligned}$$

Ut2new;

$$\text{qq2} = \text{Simplify}\left[\frac{\text{Ut2new}}{\text{ri}^2 \text{rj}^2 \text{rk}^2 \text{rl}^2 (1+x)^9} * 16384 * \left(\frac{1}{(\text{lij}^2 * \text{lik}^2 * \text{lil}^2 * \text{lj}^2 * \text{lk}^2 * \text{ll}^2)}\right)\right]$$

[化简]

$$\begin{aligned} & -\text{ri}^2 \text{rj}^2 (\text{ri}^2 + \text{rk}^2 + 2 \text{ri rk x}) (\text{rj}^2 + \text{rl}^2 + 2 \text{rj rl x}) (\text{rk}^2 + \text{rl}^2 + 2 \text{rk rl x}) \\ & \left(4 (\text{ri}^2 + \text{rk}^2 + 2 \text{ri rk x}) (\text{ri}^2 + \text{rl}^2 + 2 \text{ri rl x}) - 4 (\text{ri}^2 - \text{rk rl x} + \text{ri} (\text{rk} + \text{rl}) x)^2\right) \\ & \left(4 (\text{rj}^2 + \text{rk}^2 + 2 \text{rj rk x}) (\text{rj}^2 + \text{rl}^2 + 2 \text{rj rl x}) - 4 (\text{rj}^2 - \text{rk rl x} + \text{rj} (\text{rk} + \text{rl}) x)^2\right) \\ & (-\text{rj} (\text{ri rl} (-1+x) - \text{ri rj x} - \text{rj rl x}) (\text{ri rk rl x} + \text{rj rk rl x} + \text{ri rj} (\text{rl} + \text{rk x} - 2 \text{rl x})) \\ & \left(4 (\text{ri}^2 + \text{rk}^2 + 2 \text{ri rk x}) (\text{ri}^2 + \text{rl}^2 + 2 \text{ri rl x}) - 4 (\text{ri}^2 - \text{rk rl x} + \text{ri} (\text{rk} + \text{rl}) x)^2\right) + \\ & \text{rk} (\text{ri rl} (-1+x) - \text{ri rk x} - \text{rk rl x}) \\ & \left(4 (\text{ri}^2 + \text{rj}^2 + 2 \text{ri rj x}) (\text{ri}^2 + \text{rl}^2 + 2 \text{ri rl x}) - 4 (\text{ri}^2 - \text{rj rl x} + \text{ri} (\text{rj} + \text{rl}) x)^2\right) \\ & (-\text{rj rk rl x} - \text{ri} (\text{rj rl x} + \text{rk} (\text{rl} + \text{rj x} - 2 \text{rl x}))) \left(\text{rl} (\text{ri rj} (-1+x) - \text{ri rl x} - \text{rj rl x})\right) \\ & \left(4 (\text{ri}^2 + \text{rj}^2 + 2 \text{ri rj x}) (\text{ri}^2 + \text{rk}^2 + 2 \text{ri rk x}) - 4 (\text{ri}^2 - \text{rj rk x} + \text{ri} (\text{rj} + \text{rk}) x)^2\right) \\ & (-\text{rj rk rl x} - \text{ri} (\text{rk rl x} + \text{rj} (\text{rl} + \text{rk x} - 2 \text{rl x}))) + \text{rk} (\text{ri rj} (-1+x) - \text{ri rk x} - \text{rj rk x}) \\ & \left(4 (\text{ri}^2 + \text{rj}^2 + 2 \text{ri rj x}) (\text{ri}^2 + \text{rl}^2 + 2 \text{ri rl x}) - 4 (\text{ri}^2 - \text{rj rl x} + \text{ri} (\text{rj} + \text{rl}) x)^2\right) \\ & (-\text{rj rk rl x} - \text{ri} (\text{rk rl x} + \text{rj} (\text{rk} - 2 \text{rk x} + \text{rl x}))) \left(\text{rl} (\text{rj rk} (-1+x) - \text{rj rl x} - \text{rk rl x})\right) \\ & \left(4 (\text{ri}^2 + \text{rj}^2 + 2 \text{ri rj x}) (\text{ri}^2 + \text{rk}^2 + 2 \text{ri rk x}) - 4 (\text{ri}^2 - \text{rj rk x} + \text{ri} (\text{rj} + \text{rk}) x)^2\right) \\ & (-\text{ri rk rl x} - \text{rj} (\text{ri rl x} + \text{rk} (\text{rl} + \text{ri x} - 2 \text{rl x}))) + \text{ri} (\text{rj rk} (-1+x) - \text{ri rj x} - \text{ri rk x}) \\ & \left(4 (\text{rj}^2 + \text{rk}^2 + 2 \text{rj rk x}) (\text{rj}^2 + \text{rl}^2 + 2 \text{rj rl x}) - 4 (\text{rj}^2 - \text{rk rl x} + \text{rj} (\text{rk} + \text{rl}) x)^2\right) \\ & (-\text{rj rk rl x} - \text{ri} (\text{rk rl x} + \text{rj} (\text{rk} - 2 \text{rk x} + \text{rl x}))) \end{aligned}$$

Ut3new;

Ut4new;

Ut5new;

Ut6new;

Ut7new;

Ut8new;

Ut9new;

Ut10new;

Ut11new;

Ut12new;

Ut13new;

Ut14new;

Ut15new;

Ut16new;



$$\text{qq3} = \text{Simplify}\left[\frac{\text{Ut3new}}{\text{ri}^2 \text{rj}^2 \text{rk}^2 \text{rl}^2 (1+x)^9} * 16384 * \left(1 / \left(\text{lij}^2 * \text{lik}^2 * \text{lil}^2 * \text{lj}^2 * \text{lk}^2 * \text{ll}^2\right)\right)\right]$$

$$\begin{aligned}
& -r_i^2 r_k^2 (r_i^2 + r_j^2 + 2 r_i r_j x) (r_j^2 + r_l^2 + 2 r_j r_l x) (r_k^2 + r_l^2 + 2 r_k r_l x) \\
& \left( 4 (r_i^2 + r_j^2 + 2 r_i r_j x) (r_i^2 + r_l^2 + 2 r_i r_l x) - 4 (r_i^2 - r_j r_l x + r_i (r_j + r_l) x)^2 \right) \\
& \left( 4 (r_j^2 + r_k^2 + 2 r_j r_k x) (r_j^2 + r_l^2 + 2 r_j r_l x) - 4 (r_j^2 - r_k r_l x + r_j (r_k + r_l) x)^2 \right) \\
& \left( -r_j (r_i r_l (-1 + x) - r_i r_j x - r_j r_l x) (r_i r_k r_l x + r_j r_k r_l x + r_i r_j (r_l + r_k x - 2 r_l x)) \right. \\
& \quad \left. \left( 4 (r_i^2 + r_k^2 + 2 r_i r_k x) (r_i^2 + r_l^2 + 2 r_i r_l x) - 4 (r_i^2 - r_k r_l x + r_i (r_k + r_l) x)^2 \right) + \right. \\
& \quad r_k (r_i r_l (-1 + x) - r_i r_k x - r_k r_l x) \\
& \quad \left. \left( 4 (r_i^2 + r_j^2 + 2 r_i r_j x) (r_i^2 + r_l^2 + 2 r_i r_l x) - 4 (r_i^2 - r_j r_l x + r_i (r_j + r_l) x)^2 \right) \right. \\
& \quad \left. \left( -r_j r_k r_l x - r_i (r_j r_l x + r_k (r_l + r_j x - 2 r_l x)) \right) \right) \left( r_l (r_i r_k (-1 + x) - r_i r_l x - r_k r_l x) \right. \\
& \quad \left. \left( 4 (r_i^2 + r_j^2 + 2 r_i r_j x) (r_i^2 + r_k^2 + 2 r_i r_k x) - 4 (r_i^2 - r_j r_k x + r_i (r_j + r_k) x)^2 \right) \right. \\
& \quad \left. \left( -r_j r_k r_l x - r_i (r_j r_l x + r_k (r_l + r_j x - 2 r_l x)) \right) + r_j (r_i r_k (-1 + x) - r_i r_j x - r_j r_k x) \right. \\
& \quad \left. \left( 4 (r_i^2 + r_k^2 + 2 r_i r_k x) (r_i^2 + r_l^2 + 2 r_i r_l x) - 4 (r_i^2 - r_k r_l x + r_i (r_k + r_l) x)^2 \right) \right. \\
& \quad \left. \left( -r_j r_k r_l x - r_i (r_k r_l x + r_j (r_k - 2 r_k x + r_l x)) \right) \right) \left( r_l (r_j r_k (-1 + x) - r_j r_l x - r_k r_l x) \right. \\
& \quad \left. \left( 4 (r_i^2 + r_j^2 + 2 r_i r_j x) (r_i^2 + r_k^2 + 2 r_i r_k x) - 4 (r_i^2 - r_j r_k x + r_i (r_j + r_k) x)^2 \right) \right. \\
& \quad \left. \left( -r_i r_k r_l x - r_j (r_i r_l x + r_k (r_l + r_i x - 2 r_l x)) \right) + r_i (r_j r_k (-1 + x) - r_i r_j x - r_i r_k x) \right. \\
& \quad \left. \left( 4 (r_j^2 + r_k^2 + 2 r_j r_k x) (r_j^2 + r_l^2 + 2 r_j r_l x) - 4 (r_j^2 - r_k r_l x + r_j (r_k + r_l) x)^2 \right) \right. \\
& \quad \left. \left( -r_j r_k r_l x - r_i (r_k r_l x + r_j (r_k - 2 r_k x + r_l x)) \right) \right) \Big)
\end{aligned}$$

$$\text{qq4} = \text{Simplify}\left[\frac{\text{Ut4new}}{\text{ri}^2 \text{rj}^2 \text{rk}^2 \text{rl}^2 (1+x)^9} * 16384 * \left(1 / (\text{li} \text{j}^2 * \text{li} \text{k}^2 * \text{li} \text{l}^2 * \text{li} \text{j} \text{k}^2 * \text{li} \text{j} \text{l}^2 * \text{li} \text{k} \text{l}^2)\right)\right]$$

$$\begin{aligned}
& -r_i^2 r_j^2 (r_j^2 + r_k^2 + 2 r_j r_k x) (r_i^2 + r_l^2 + 2 r_i r_l x) (r_k^2 + r_l^2 + 2 r_k r_l x) \\
& \left( 4 (r_i^2 + r_k^2 + 2 r_i r_k x) (r_i^2 + r_l^2 + 2 r_i r_l x) - 4 (r_i^2 - r_k r_l x + r_i (r_k + r_l) x)^2 \right) \\
& \left( 4 (r_j^2 + r_k^2 + 2 r_j r_k x) (r_j^2 + r_l^2 + 2 r_j r_l x) - 4 (r_j^2 - r_k r_l x + r_j (r_k + r_l) x)^2 \right) \\
& \left( -r_i (r_j r_l (-1 + x) - r_i r_j x - r_i r_l x) (r_i r_k r_l x + r_j r_k r_l x + r_i r_j (r_l + r_k x - 2 r_l x)) \right. \\
& \quad \left( 4 (r_j^2 + r_k^2 + 2 r_j r_k x) (r_j^2 + r_l^2 + 2 r_j r_l x) - 4 (r_j^2 - r_k r_l x + r_j (r_k + r_l) x)^2 \right) + \\
& \quad r_k (r_j r_l (-1 + x) - r_j r_k x - r_k r_l x) \\
& \quad \left( 4 (r_i^2 + r_j^2 + 2 r_i r_j x) (r_i^2 + r_l^2 + 2 r_i r_l x) - 4 (r_i^2 - r_j r_l x + r_i (r_j + r_l) x)^2 \right) \\
& \quad \left. (-r_i r_k r_l x - r_j (r_i r_l x + r_k (r_l + r_i x - 2 r_l x))) \right) \left( r_l (r_i r_j (-1 + x) - r_i r_l x - r_j r_l x) \right. \\
& \quad \left( 4 (r_i^2 + r_j^2 + 2 r_i r_j x) (r_i^2 + r_k^2 + 2 r_i r_k x) - 4 (r_i^2 - r_j r_k x + r_i (r_j + r_k) x)^2 \right) \\
& \quad \left. (-r_j r_k r_l x - r_i (r_k r_l x + r_j (r_l + r_k x - 2 r_l x))) \right) + r_k (r_i r_j (-1 + x) - r_i r_k x - r_j r_k x) \\
& \quad \left( 4 (r_i^2 + r_j^2 + 2 r_i r_j x) (r_i^2 + r_l^2 + 2 r_i r_l x) - 4 (r_i^2 - r_j r_l x + r_i (r_j + r_l) x)^2 \right) \\
& \quad \left. (-r_j r_k r_l x - r_i (r_k r_l x + r_j (r_k - 2 r_k x + r_l x))) \right) \left( r_l (r_i r_k (-1 + x) - r_i r_l x - r_k r_l x) \right. \\
& \quad \left( 4 (r_i^2 + r_j^2 + 2 r_i r_j x) (r_i^2 + r_k^2 + 2 r_i r_k x) - 4 (r_i^2 - r_j r_k x + r_i (r_j + r_k) x)^2 \right) \\
& \quad \left. (-r_j r_k r_l x - r_i (r_j r_l x + r_k (r_l + r_j x - 2 r_l x))) \right) + r_j (r_i r_k (-1 + x) - r_i r_j x - r_j r_k x) \\
& \quad \left( 4 (r_i^2 + r_k^2 + 2 r_i r_k x) (r_i^2 + r_l^2 + 2 r_i r_l x) - 4 (r_i^2 - r_k r_l x + r_i (r_k + r_l) x)^2 \right) \\
& \quad \left. (-r_j r_k r_l x - r_i (r_k r_l x + r_j (r_k - 2 r_k x + r_l x))) \right) \left. \right)
\end{aligned}$$

$$\text{qq5} = \text{Simplify}\left[\frac{\text{Ut5new}}{\text{ri}^2 \text{rj}^2 \text{rk}^2 \text{r1}^2 (1+x)^9} * 16384 * \left(\frac{1}{(\text{lij}^2 * \text{lik}^2 * \text{li1}^2 * \text{lj}^2 * \text{lj1}^2 * \text{lk}^2)}\right)\right]$$

$$\begin{aligned}
& -r_i^2 r_l^2 (r_i^2 + r_j^2 + 2 r_i r_j x) (r_j^2 + r_k^2 + 2 r_j r_k x) (r_k^2 + r_l^2 + 2 r_k r_l x) \\
& \left( 4 (r_i^2 + r_j^2 + 2 r_i r_j x) (r_i^2 + r_k^2 + 2 r_i r_k x) - 4 (r_i^2 - r_j r_k x + r_i (r_j + r_k) x)^2 \right) \\
& \left( 4 (r_j^2 + r_k^2 + 2 r_j r_k x) (r_j^2 + r_l^2 + 2 r_j r_l x) - 4 (r_j^2 - r_k r_l x + r_j (r_k + r_l) x)^2 \right) \\
& \left( -r_i (r_j r_l (-1 + x) - r_i r_j x - r_i r_l x) (r_i r_k r_l x + r_j r_k r_l x + r_i r_j (r_l + r_k x - 2 r_l x)) \right. \\
& \quad \left( 4 (r_j^2 + r_k^2 + 2 r_j r_k x) (r_j^2 + r_l^2 + 2 r_j r_l x) - 4 (r_j^2 - r_k r_l x + r_j (r_k + r_l) x)^2 \right) + \\
& \quad r_k (r_j r_l (-1 + x) - r_j r_k x - r_k r_l x) \left( 4 (r_i^2 + r_j^2 + 2 r_i r_j x) (r_i^2 + r_l^2 + 2 r_i r_l x) - \right. \\
& \quad \left. 4 (r_i^2 - r_j r_l x + r_i (r_j + r_l) x)^2 \right) \left. \left( -r_i r_k r_l x - r_j (r_i r_l x + r_k (r_l + r_i x - 2 r_l x)) \right) \right) \\
& \left( -r_j (r_i r_l (-1 + x) - r_i r_j x - r_j r_l x) (r_i r_k r_l x + r_j r_k r_l x + r_i r_j (r_l + r_k x - 2 r_l x)) \right. \\
& \quad \left( 4 (r_i^2 + r_k^2 + 2 r_i r_k x) (r_i^2 + r_l^2 + 2 r_i r_l x) - 4 (r_i^2 - r_k r_l x + r_i (r_k + r_l) x)^2 \right) + \\
& \quad r_k (r_i r_l (-1 + x) - r_i r_k x - r_k r_l x) \\
& \quad \left( 4 (r_i^2 + r_j^2 + 2 r_i r_j x) (r_i^2 + r_l^2 + 2 r_i r_l x) - 4 (r_i^2 - r_j r_l x + r_i (r_j + r_l) x)^2 \right) \\
& \quad \left. \left( -r_j r_k r_l x - r_i (r_j r_l x + r_k (r_l + r_j x - 2 r_l x)) \right) \right) \left( r_l (r_i r_k (-1 + x) - r_i r_l x - r_k r_l x) \right. \\
& \quad \left( 4 (r_i^2 + r_j^2 + 2 r_i r_j x) (r_i^2 + r_k^2 + 2 r_i r_k x) - 4 (r_i^2 - r_j r_k x + r_i (r_j + r_k) x)^2 \right) \\
& \quad \left. \left( -r_j r_k r_l x - r_i (r_j r_l x + r_k (r_l + r_j x - 2 r_l x)) \right) + r_j (r_i r_k (-1 + x) - r_i r_j x - r_j r_k x) \right) \\
& \quad \left( 4 (r_i^2 + r_k^2 + 2 r_i r_k x) (r_i^2 + r_l^2 + 2 r_i r_l x) - 4 (r_i^2 - r_k r_l x + r_i (r_k + r_l) x)^2 \right) \\
& \quad \left. \left( -r_j r_k r_l x - r_i (r_k r_l x + r_j (r_k - 2 r_k x + r_l x)) \right) \right)
\end{aligned}$$

$$\text{qq6} = \text{Simplify}\left[\frac{\text{Ut6new}}{\text{ri}^2 \text{rj}^2 \text{rk}^2 \text{r1}^2 (1+x)^9} * 16384 * \left(\frac{1}{(\text{lij}^2 * \text{lik}^2 * \text{lil}^2 * \text{lj}^2 * \text{lk}^2 * \text{ll}^2)}\right)\right]$$

$$\begin{aligned}
& -rj^4 (ri^2 + rk^2 + 2ri rk x) (ri^2 + rl^2 + 2ri rl x) (rk^2 + rl^2 + 2rk rl x) \\
& \left( 4 (ri^2 + rk^2 + 2ri rk x) (ri^2 + rl^2 + 2ri rl x) - 4 (ri^2 - rk rl x + ri (rk + rl) x)^2 \right)^2 \\
& \left( -ri (rj rl (-1 + x) - ri rj x - ri rl x) (ri rk rl x + rj rk rl x + ri rj (rl + rk x - 2rl x)) \right. \\
& \quad \left. \left( 4 (rj^2 + rk^2 + 2rj rk x) (rj^2 + rl^2 + 2rj rl x) - 4 (rj^2 - rk rl x + rj (rk + rl) x)^2 \right) + \right. \\
& \quad \left. rk (rj rl (-1 + x) - rj rk x - rk rl x) \right. \\
& \quad \left. \left( 4 (ri^2 + rj^2 + 2ri rj x) (ri^2 + rl^2 + 2ri rl x) - 4 (ri^2 - rj rl x + ri (rj + rl) x)^2 \right) \right. \\
& \quad \left. (-ri rk rl x - rj (ri rl x + rk (rl + ri x - 2rl x))) \right) \left( rl (ri rj (-1 + x) - ri rl x - rj rl x) \right) \\
& \quad \left( 4 (ri^2 + rj^2 + 2ri rj x) (ri^2 + rk^2 + 2ri rk x) - 4 (ri^2 - rj rk x + ri (rj + rk) x)^2 \right) \\
& \quad \left( -rj rk rl x - ri (rk rl x + rj (rl + rk x - 2rl x)) \right) + rk (ri rj (-1 + x) - ri rk x - rj rk x) \\
& \quad \left( 4 (ri^2 + rj^2 + 2ri rj x) (ri^2 + rl^2 + 2ri rl x) - 4 (ri^2 - rj rl x + ri (rj + rl) x)^2 \right) \\
& \quad \left( -rj rk rl x - ri (rk rl x + rj (rk - 2rk x + rl x)) \right) \left( rl (rj rk (-1 + x) - rj rl x - rk rl x) \right) \\
& \quad \left( 4 (ri^2 + rj^2 + 2ri rj x) (ri^2 + rk^2 + 2ri rk x) - 4 (ri^2 - rj rk x + ri (rj + rk) x)^2 \right) \\
& \quad \left( -ri rk rl x - rj (ri rl x + rk (rl + ri x - 2rl x)) \right) + ri (rj rk (-1 + x) - ri rj x - ri rk x) \\
& \quad \left( 4 (rj^2 + rk^2 + 2rj rk x) (rj^2 + rl^2 + 2rj rl x) - 4 (rj^2 - rk rl x + rj (rk + rl) x)^2 \right) \\
& \quad \left( -rj rk rl x - ri (rk rl x + rj (rk - 2rk x + rl x)) \right) \left. \right)
\end{aligned}$$

$$\text{qq7} = \text{Simplify}\left[\frac{\text{Ut7new}}{\text{ri}^2 \text{rj}^2 \text{rk}^2 \text{rl}^2 (1+x)^9} * 16384 * (1 / (\text{lij}^2 * \text{lik}^2 * \text{lil}^2 * \text{lkj}^2 * \text{ljl}^2 * \text{lk}^2))\right]$$

$$\begin{aligned}
& -rj^2rk^2(r_i^2+rj^2+2r_iri jx)(r_i^2+r_l^2+2r_iri lx)(rk^2+r_l^2+2rkrlx) \\
& (4(r_i^2+rj^2+2r_iri jx)(r_i^2+r_l^2+2r_iri lx)-4(r_i^2-rjrlx+ri(rj+rl)x)^2) \\
& (4(r_i^2+rk^2+2r_iri kx)(r_i^2+r_l^2+2r_iri lx)-4(r_i^2-rkrlx+ri(rk+rl)x)^2) \\
& (-ri(rjrl(-1+x)-ri rjx-ri rlx)(ri rkrlx+rjrkrlx+ri rj(rl+rkx-2rlx)) \\
& (4(rj^2+rk^2+2rjrkx)(rj^2+r_l^2+2rjrlx)-4(rj^2-rkrlx+rj(rk+rl)x)^2)+ \\
& rk(rjrl(-1+x)-rj rkx-rkrlx) \\
& (4(r_i^2+rj^2+2r_iri jx)(r_i^2+r_l^2+2r_iri lx)-4(r_i^2-rjrlx+ri(rj+rl)x)^2) \\
& (-ri rkrlx-rj(ri rlx+rk(rl+rix-2rlx))))(rl(ri rk(-1+x)-ri rlx-rkrlx) \\
& (4(r_i^2+rj^2+2r_iri jx)(r_i^2+rk^2+2r_iri kx)-4(r_i^2-rjrkx+ri(rj+rk)x)^2) \\
& (-rjrkrlx-ri(rjrlx+rk(rl+rjx-2rlx))))+rj(ri rk(-1+x)-ri rjx-rj rkx) \\
& (4(r_i^2+rk^2+2r_iri kx)(r_i^2+r_l^2+2r_iri lx)-4(r_i^2-rkrlx+ri(rk+rl)x)^2) \\
& (-rjrkrlx-ri(rkrlx+rj(rk-2rkx+rlx))))(rl(rjrk(-1+x)-rjrlx-rkrlx) \\
& (4(r_i^2+rj^2+2r_iri jx)(r_i^2+rk^2+2r_iri kx)-4(r_i^2-rjrkx+ri(rj+rk)x)^2) \\
& (-ri rkrlx-rj(ri rlx+rk(rl+rix-2rlx))))+ri(rjrk(-1+x)-ri rjx-ri rkx) \\
& (4(rj^2+rk^2+2rjrkx)(rj^2+r_l^2+2rjrlx)-4(rj^2-rkrlx+rj(rk+rl)x)^2) \\
& (-rjrkrlx-ri(rkrlx+rj(rk-2rkx+rlx))))))
\end{aligned}$$

$$\text{qq8} = \text{Simplify}\left[\frac{\text{Ut8new}}{\text{ri}^2 \text{rj}^2 \text{rk}^2 \text{rl}^2 (1+x)^9} * 16384 * (1 / (\text{li} \text{j}^2 * \text{li} \text{k}^2 * \text{li} \text{l}^2 * \text{lj} \text{k}^2 * \text{lj} \text{l}^2 * \text{lk} \text{l}^2))\right]$$

$$\begin{aligned}
& -rj^2 r l^2 (ri^2 + rj^2 + 2ri rj x) (ri^2 + rk^2 + 2ri rk x) (rk^2 + r l^2 + 2rk r l x) \\
& \left( 4 (ri^2 + rj^2 + 2ri rj x) (ri^2 + rk^2 + 2ri rk x) - 4 (ri^2 - rj rk x + ri (rj + rk) x)^2 \right) \\
& \left( 4 (ri^2 + rk^2 + 2ri rk x) (ri^2 + r l^2 + 2ri r l x) - 4 (ri^2 - rk r l x + ri (rk + r l) x)^2 \right) \\
& \left( -ri (rj r l (-1 + x) - ri rj x - ri r l x) (ri rk r l x + rj rk r l x + ri rj (r l + rk x - 2 r l x)) \right. \\
& \quad \left( 4 (rj^2 + rk^2 + 2rj rk x) (rj^2 + r l^2 + 2rj r l x) - 4 (rj^2 - rk r l x + rj (rk + r l) x)^2 \right) + \\
& \quad rk (rj r l (-1 + x) - rj rk x - rk r l x) \left( 4 (ri^2 + rj^2 + 2ri rj x) (ri^2 + r l^2 + 2ri r l x) - \right. \\
& \quad \left. 4 (ri^2 - rj r l x + ri (rj + r l) x)^2 \right) \left. \left( -ri rk r l x - rj (ri r l x + rk (r l + ri x - 2 r l x)) \right) \right) \\
& \left( -rj (ri r l (-1 + x) - ri rj x - rj r l x) (ri rk r l x + rj rk r l x + ri rj (r l + rk x - 2 r l x)) \right. \\
& \quad \left( 4 (ri^2 + rk^2 + 2ri rk x) (ri^2 + r l^2 + 2ri r l x) - 4 (ri^2 - rk r l x + ri (rk + r l) x)^2 \right) + \\
& \quad rk (ri r l (-1 + x) - ri rk x - rk r l x) \\
& \quad \left( 4 (ri^2 + rj^2 + 2ri rj x) (ri^2 + r l^2 + 2ri r l x) - 4 (ri^2 - rj r l x + ri (rj + r l) x)^2 \right) \\
& \quad \left. \left( -rj rk r l x - ri (rj r l x + rk (r l + rj x - 2 r l x)) \right) \right) \left( r l (rj rk (-1 + x) - rj r l x - rk r l x) \right) \\
& \left( 4 (ri^2 + rj^2 + 2ri rj x) (ri^2 + rk^2 + 2ri rk x) - 4 (ri^2 - rj rk x + ri (rj + rk) x)^2 \right) \\
& \left( -ri rk r l x - rj (ri r l x + rk (r l + ri x - 2 r l x)) \right) + ri (rj rk (-1 + x) - ri rj x - ri rk x) \\
& \left( 4 (rj^2 + rk^2 + 2rj rk x) (rj^2 + r l^2 + 2rj r l x) - 4 (rj^2 - rk r l x + rj (rk + r l) x)^2 \right) \\
& \left. \left( -rj rk r l x - ri (rk r l x + rj (rk - 2 rk x + r l x)) \right) \right)
\end{aligned}$$

$$\text{qq9} = \text{Simplify}\left[\frac{\text{Ut9new}}{\text{ri}^2 \text{rj}^2 \text{rk}^2 \text{r1}^2 (1+x)^9} * 16384 * \left(\frac{1}{(\text{lij}^2 * \text{lik}^2 * \text{li1}^2 * \text{lj}^2 * \text{lj1}^2 * \text{lk}^2)}\right)\right]$$

$$\begin{aligned}
& -r_i^2 r_k^2 (r_j^2 + r_k^2 + 2 r_i r_k x) (r_i^2 + r_l^2 + 2 r_i r_l x) (r_j^2 + r_l^2 + 2 r_j r_l x) \\
& \left( 4 (r_i^2 + r_j^2 + 2 r_i r_j x) (r_i^2 + r_l^2 + 2 r_i r_l x) - 4 (r_i^2 - r_j r_l x + r_i (r_j + r_l) x)^2 \right) \\
& \left( 4 (r_j^2 + r_k^2 + 2 r_j r_k x) (r_j^2 + r_l^2 + 2 r_j r_l x) - 4 (r_j^2 - r_k r_l x + r_j (r_k + r_l) x)^2 \right) \\
& \left( -r_i (r_k r_l (-1 + x) - r_i r_k x - r_i r_l x) (r_i r_j r_l x + r_j r_k r_l x + r_i r_k (r_l + r_j x - 2 r_l x)) \right. \\
& \quad \left. \left( 4 (r_j^2 + r_k^2 + 2 r_j r_k x) (r_j^2 + r_l^2 + 2 r_j r_l x) - 4 (r_j^2 - r_k r_l x + r_j (r_k + r_l) x)^2 \right) + \right. \\
& \quad \left. r_j (r_k r_l (-1 + x) - r_j r_k x - r_j r_l x) \right. \\
& \quad \left( 4 (r_i^2 + r_k^2 + 2 r_i r_k x) (r_i^2 + r_l^2 + 2 r_i r_l x) - 4 (r_i^2 - r_k r_l x + r_i (r_k + r_l) x)^2 \right) \\
& \quad \left. (-r_i r_k r_l x - r_j (r_i r_l x + r_k (r_l + r_i x - 2 r_l x))) \right) \left( r_l (r_i r_j (-1 + x) - r_i r_l x - r_j r_l x) \right) \\
& \left( 4 (r_i^2 + r_j^2 + 2 r_i r_j x) (r_i^2 + r_k^2 + 2 r_i r_k x) - 4 (r_i^2 - r_j r_k x + r_i (r_j + r_k) x)^2 \right) \\
& \quad \left( -r_j r_k r_l x - r_i (r_k r_l x + r_j (r_l + r_k x - 2 r_l x)) \right) + r_k (r_i r_j (-1 + x) - r_i r_k x - r_j r_k x) \\
& \left( 4 (r_i^2 + r_j^2 + 2 r_i r_j x) (r_i^2 + r_l^2 + 2 r_i r_l x) - 4 (r_i^2 - r_j r_l x + r_i (r_j + r_l) x)^2 \right) \\
& \quad \left( -r_j r_k r_l x - r_i (r_k r_l x + r_j (r_k - 2 r_k x + r_l x)) \right) \left( r_l (r_i r_k (-1 + x) - r_i r_l x - r_k r_l x) \right) \\
& \left( 4 (r_i^2 + r_j^2 + 2 r_i r_j x) (r_i^2 + r_k^2 + 2 r_i r_k x) - 4 (r_i^2 - r_j r_k x + r_i (r_j + r_k) x)^2 \right) \\
& \quad \left( -r_j r_k r_l x - r_i (r_j r_l x + r_k (r_l + r_j x - 2 r_l x)) \right) + r_j (r_i r_k (-1 + x) - r_i r_j x - r_j r_k x) \\
& \left( 4 (r_i^2 + r_k^2 + 2 r_i r_k x) (r_i^2 + r_l^2 + 2 r_i r_l x) - 4 (r_i^2 - r_k r_l x + r_i (r_k + r_l) x)^2 \right) \\
& \quad \left( -r_j r_k r_l x - r_i (r_k r_l x + r_j (r_k - 2 r_k x + r_l x)) \right) \left. \right)
\end{aligned}$$

$$\text{qq10} = \text{Simplify}\left[\frac{\text{Ut10new}}{\text{ri}^2 \text{rj}^2 \text{rk}^2 \text{rl}^2 (1+x)^9} * 16384 * (1 / (\text{lij}^2 * \text{lik}^2 * \text{lil}^2 * \text{lj}^2 * \text{lk}^2 * \text{ll}^2))\right]$$

$$\begin{aligned}
& -ri^2rl^2 (ri^2 + rk^2 + 2ri rk x) (rj^2 + rk^2 + 2rj rk x) (rj^2 + rl^2 + 2rj rl x) \\
& \left( 4 (ri^2 + rj^2 + 2ri rj x) (ri^2 + rk^2 + 2ri rk x) - 4 (ri^2 - rj rk x + ri (rj + rk) x)^2 \right) \\
& \left( 4 (rj^2 + rk^2 + 2rj rk x) (rj^2 + rl^2 + 2rj rl x) - 4 (rj^2 - rk rl x + rj (rk + rl) x)^2 \right) \\
& \left( -ri (rk rl (-1 + x) - ri rk x - ri rl x) (ri rj rl x + rj rk rl x + ri rk (rl + rj x - 2rl x)) \right. \\
& \quad \left. \left( 4 (rj^2 + rk^2 + 2rj rk x) (rj^2 + rl^2 + 2rj rl x) - 4 (rj^2 - rk rl x + rj (rk + rl) x)^2 \right) + \right. \\
& \quad \left. rj (rk rl (-1 + x) - rj rk x - rj rl x) \left( 4 (ri^2 + rk^2 + 2ri rk x) (ri^2 + rl^2 + 2ri rl x) - \right. \right. \\
& \quad \left. \left. 4 (ri^2 - rk rl x + ri (rk + rl) x)^2 \right) (-ri rk rl x - rj (ri rl x + rk (rl + ri x - 2rl x))) \right) \\
& \left( -rj (ri rl (-1 + x) - ri rj x - rj rl x) (ri rk rl x + rj rk rl x + ri rj (rl + rk x - 2rl x)) \right. \\
& \quad \left. \left( 4 (ri^2 + rk^2 + 2ri rk x) (ri^2 + rl^2 + 2ri rl x) - 4 (ri^2 - rk rl x + ri (rk + rl) x)^2 \right) + \right. \\
& \quad \left. rk (ri rl (-1 + x) - ri rk x - rk rl x) \right. \\
& \quad \left. \left( 4 (ri^2 + rj^2 + 2ri rj x) (ri^2 + rl^2 + 2ri rl x) - 4 (ri^2 - rj rl x + ri (rj + rl) x)^2 \right) \right. \\
& \quad \left. (-rj rk rl x - ri (rj rl x + rk (rl + rj x - 2rl x))) \right) (rl (ri rj (-1 + x) - ri rl x - rj rl x) \\
& \quad \left( 4 (ri^2 + rj^2 + 2ri rj x) (ri^2 + rk^2 + 2ri rk x) - 4 (ri^2 - rj rk x + ri (rj + rk) x)^2 \right) \\
& \quad \left( -rj rk rl x - ri (rk rl x + rj (rl + rk x - 2rl x)) \right) + rk (ri rj (-1 + x) - ri rk x - rj rk x) \\
& \quad \left( 4 (ri^2 + rj^2 + 2ri rj x) (ri^2 + rl^2 + 2ri rl x) - 4 (ri^2 - rj rl x + ri (rj + rl) x)^2 \right) \\
& \quad \left. (-rj rk rl x - ri (rk rl x + rj (rk - 2rk x + rl x))) \right)
\end{aligned}$$

qq11 =

$$\text{Simplify}\left[\frac{\text{Ut11new}}{r_i^2 r_j^2 r_k^2 r_l^2 (1+x)^9} * 16384 * \left(1 / \left(l_{ij}^2 * l_{ik}^2 * l_{il}^2 * l_{jk}^2 * l_{jl}^2 * l_{kl}^2\right)\right)\right]$$

化简

$$\begin{aligned} & -r_j^2 r_k^2 (r_i^2 + r_k^2 + 2 r_i r_k x) (r_i^2 + r_l^2 + 2 r_i r_l x) (r_j^2 + r_l^2 + 2 r_j r_l x) \\ & \left(4 (r_i^2 + r_j^2 + 2 r_i r_j x) (r_i^2 + r_l^2 + 2 r_i r_l x) - 4 (r_i^2 - r_j r_l x + r_i (r_j + r_l) x)^2\right) \\ & \left(4 (r_i^2 + r_k^2 + 2 r_i r_k x) (r_i^2 + r_l^2 + 2 r_i r_l x) - 4 (r_i^2 - r_k r_l x + r_i (r_k + r_l) x)^2\right) \\ & (-r_i (r_k r_l (-1+x) - r_i r_k x - r_i r_l x) (r_i r_j r_l x + r_j r_k r_l x + r_i r_k (r_l + r_j x - 2 r_l x)) \\ & \left(4 (r_j^2 + r_k^2 + 2 r_j r_k x) (r_j^2 + r_l^2 + 2 r_j r_l x) - 4 (r_j^2 - r_k r_l x + r_j (r_k + r_l) x)^2\right) + \\ & r_j (r_k r_l (-1+x) - r_j r_k x - r_j r_l x) \\ & \left(4 (r_i^2 + r_k^2 + 2 r_i r_k x) (r_i^2 + r_l^2 + 2 r_i r_l x) - 4 (r_i^2 - r_k r_l x + r_i (r_k + r_l) x)^2\right) \\ & (-r_i r_k r_l x - r_j (r_i r_l x + r_k (r_l + r_i x - 2 r_l x))) \left(r_l (r_i r_j (-1+x) - r_i r_l x - r_j r_l x)\right) \\ & \left(4 (r_i^2 + r_j^2 + 2 r_i r_j x) (r_i^2 + r_k^2 + 2 r_i r_k x) - 4 (r_i^2 - r_j r_k x + r_i (r_j + r_k) x)^2\right) \\ & (-r_j r_k r_l x - r_i (r_k r_l x + r_j (r_l + r_k x - 2 r_l x))) + r_k (r_i r_j (-1+x) - r_i r_k x - r_j r_k x) \\ & \left(4 (r_i^2 + r_j^2 + 2 r_i r_j x) (r_i^2 + r_l^2 + 2 r_i r_l x) - 4 (r_i^2 - r_j r_l x + r_i (r_j + r_l) x)^2\right) \\ & (-r_j r_k r_l x - r_i (r_k r_l x + r_j (r_k - 2 r_k x + r_l x))) \left(r_l (r_j r_k (-1+x) - r_j r_l x - r_k r_l x)\right) \\ & \left(4 (r_i^2 + r_j^2 + 2 r_i r_j x) (r_i^2 + r_k^2 + 2 r_i r_k x) - 4 (r_i^2 - r_j r_k x + r_i (r_j + r_k) x)^2\right) \\ & (-r_i r_k r_l x - r_j (r_i r_l x + r_k (r_l + r_i x - 2 r_l x))) + r_i (r_j r_k (-1+x) - r_i r_j x - r_i r_k x) \\ & \left(4 (r_j^2 + r_k^2 + 2 r_j r_k x) (r_j^2 + r_l^2 + 2 r_j r_l x) - 4 (r_j^2 - r_k r_l x + r_j (r_k + r_l) x)^2\right) \\ & (-r_j r_k r_l x - r_i (r_k r_l x + r_j (r_k - 2 r_k x + r_l x))) \end{aligned}$$

qq12 =

$$\text{Simplify}\left[\frac{\text{Ut12new}}{r_i^2 r_j^2 r_k^2 r_l^2 (1+x)^9} * 16384 * \left(1 / \left(l_{ij}^2 * l_{ik}^2 * l_{il}^2 * l_{jk}^2 * l_{jl}^2 * l_{kl}^2\right)\right)\right]$$

化简

$$\begin{aligned} & -r_k^4 (r_i^2 + r_j^2 + 2 r_i r_j x) (r_i^2 + r_l^2 + 2 r_i r_l x) (r_j^2 + r_l^2 + 2 r_j r_l x) \\ & \left(4 (r_i^2 + r_j^2 + 2 r_i r_j x) (r_i^2 + r_l^2 + 2 r_i r_l x) - 4 (r_i^2 - r_j r_l x + r_i (r_j + r_l) x)^2\right)^2 \\ & (-r_i (r_k r_l (-1+x) - r_i r_k x - r_i r_l x) (r_i r_j r_l x + r_j r_k r_l x + r_i r_k (r_l + r_j x - 2 r_l x)) \\ & \left(4 (r_j^2 + r_k^2 + 2 r_j r_k x) (r_j^2 + r_l^2 + 2 r_j r_l x) - 4 (r_j^2 - r_k r_l x + r_j (r_k + r_l) x)^2\right) + \\ & r_j (r_k r_l (-1+x) - r_j r_k x - r_j r_l x) \\ & \left(4 (r_i^2 + r_k^2 + 2 r_i r_k x) (r_i^2 + r_l^2 + 2 r_i r_l x) - 4 (r_i^2 - r_k r_l x + r_i (r_k + r_l) x)^2\right) \\ & (-r_i r_k r_l x - r_j (r_i r_l x + r_k (r_l + r_i x - 2 r_l x))) \left(r_l (r_i r_k (-1+x) - r_i r_l x - r_k r_l x)\right) \\ & \left(4 (r_i^2 + r_j^2 + 2 r_i r_j x) (r_i^2 + r_k^2 + 2 r_i r_k x) - 4 (r_i^2 - r_j r_k x + r_i (r_j + r_k) x)^2\right) \\ & (-r_j r_k r_l x - r_i (r_j r_l x + r_k (r_l + r_j x - 2 r_l x))) + r_j (r_i r_k (-1+x) - r_i r_j x - r_j r_k x) \\ & \left(4 (r_i^2 + r_k^2 + 2 r_i r_k x) (r_i^2 + r_l^2 + 2 r_i r_l x) - 4 (r_i^2 - r_k r_l x + r_i (r_k + r_l) x)^2\right) \\ & (-r_j r_k r_l x - r_i (r_k r_l x + r_j (r_k - 2 r_k x + r_l x))) \left(r_l (r_j r_k (-1+x) - r_j r_l x - r_k r_l x)\right) \\ & \left(4 (r_i^2 + r_j^2 + 2 r_i r_j x) (r_i^2 + r_k^2 + 2 r_i r_k x) - 4 (r_i^2 - r_j r_k x + r_i (r_j + r_k) x)^2\right) \\ & (-r_i r_k r_l x - r_j (r_i r_l x + r_k (r_l + r_i x - 2 r_l x))) + r_i (r_j r_k (-1+x) - r_i r_j x - r_i r_k x) \\ & \left(4 (r_j^2 + r_k^2 + 2 r_j r_k x) (r_j^2 + r_l^2 + 2 r_j r_l x) - 4 (r_j^2 - r_k r_l x + r_j (r_k + r_l) x)^2\right) \\ & (-r_j r_k r_l x - r_i (r_k r_l x + r_j (r_k - 2 r_k x + r_l x))) \end{aligned}$$

qq13 =

$$\text{Simplify}\left[\frac{\text{Ut13new}}{r_i^2 r_j^2 r_k^2 r_l^2 (1+x)^9} * 16384 * \left(1 / (l_{ij}^2 * l_{ik}^2 * l_{il}^2 * l_{jk}^2 * l_{jl}^2 * l_{kl}^2)\right)\right]$$

化简

$$\begin{aligned} & -rk^2 r_l^2 (r_i^2 + r_j^2 + 2 r_i r_j x) (r_i^2 + rk^2 + 2 r_i rk x) (r_j^2 + r_l^2 + 2 r_j r_l x) \\ & \left(4 (r_i^2 + r_j^2 + 2 r_i r_j x) (r_i^2 + rk^2 + 2 r_i rk x) - 4 (r_i^2 - r_j rk x + r_i (r_j + rk) x)^2\right) \\ & \left(4 (r_i^2 + r_j^2 + 2 r_i r_j x) (r_i^2 + r_l^2 + 2 r_i r_l x) - 4 (r_i^2 - r_j r_l x + r_i (r_j + r_l) x)^2\right) \\ & (-r_i (rk r_l (-1+x) - r_i rk x - r_i r_l x) (r_i r_j r_l x + r_j rk r_l x + r_i rk (r_l + r_j x - 2 r_l x)) \\ & \left(4 (r_j^2 + rk^2 + 2 r_j rk x) (r_j^2 + r_l^2 + 2 r_j r_l x) - 4 (r_j^2 - rk r_l x + r_j (rk + r_l) x)^2\right) + \\ & r_j (rk r_l (-1+x) - r_j rk x - r_j r_l x) \left(4 (r_i^2 + rk^2 + 2 r_i rk x) (r_i^2 + r_l^2 + 2 r_i r_l x) - \right. \\ & \left. 4 (r_i^2 - rk r_l x + r_i (rk + r_l) x)^2\right) (-r_i rk r_l x - r_j (r_i r_l x + rk (r_l + r_i x - 2 r_l x))) \\ & (-r_j (r_i r_l (-1+x) - r_i r_j x - r_j r_l x) (r_i rk r_l x + r_j rk r_l x + r_i r_j (r_l + rk x - 2 r_l x)) \\ & \left(4 (r_i^2 + rk^2 + 2 r_i rk x) (r_i^2 + r_l^2 + 2 r_i r_l x) - 4 (r_i^2 - rk r_l x + r_i (rk + r_l) x)^2\right) + \\ & rk (r_i r_l (-1+x) - r_i rk x - rk r_l x) \\ & \left(4 (r_i^2 + r_j^2 + 2 r_i r_j x) (r_i^2 + r_l^2 + 2 r_i r_l x) - 4 (r_i^2 - r_j r_l x + r_i (r_j + r_l) x)^2\right) \\ & (-r_j rk r_l x - r_i (r_j r_l x + rk (r_l + r_j x - 2 r_l x))) \left(r_l (r_j rk (-1+x) - r_j r_l x - rk r_l x) \right. \\ & \left. \left(4 (r_i^2 + r_j^2 + 2 r_i r_j x) (r_i^2 + rk^2 + 2 r_i rk x) - 4 (r_i^2 - r_j rk x + r_i (r_j + rk) x)^2\right) \right. \\ & \left. (-r_i rk r_l x - r_j (r_i r_l x + rk (r_l + r_i x - 2 r_l x))) + r_i (r_j rk (-1+x) - r_i r_j x - r_i rk x) \right. \\ & \left. \left(4 (r_j^2 + rk^2 + 2 r_j rk x) (r_j^2 + r_l^2 + 2 r_j r_l x) - 4 (r_j^2 - rk r_l x + r_j (rk + r_l) x)^2\right) \right. \\ & \left. (-r_j rk r_l x - r_i (rk r_l x + r_j (rk - 2 rk x + r_l x))) \right) \end{aligned}$$

qq14 =

$$\text{Simplify}\left[\frac{\text{Ut14new}}{r_i^2 r_j^2 r_k^2 r_l^2 (1+x)^9} * 16384 * \left(1 / (l_{ij}^2 * l_{ik}^2 * l_{il}^2 * l_{jk}^2 * l_{jl}^2 * l_{kl}^2)\right)\right]$$

化简

$$\begin{aligned} & -r_j^2 r_l^2 (r_i^2 + rk^2 + 2 r_i rk x) (r_j^2 + rk^2 + 2 r_j rk x) (r_i^2 + r_l^2 + 2 r_i r_l x) \\ & \left(4 (r_i^2 + r_j^2 + 2 r_i r_j x) (r_i^2 + rk^2 + 2 r_i rk x) - 4 (r_i^2 - r_j rk x + r_i (r_j + rk) x)^2\right) \\ & \left(4 (r_i^2 + rk^2 + 2 r_i rk x) (r_i^2 + r_l^2 + 2 r_i r_l x) - 4 (r_i^2 - rk r_l x + r_i (rk + r_l) x)^2\right) \\ & (-r_i (r_j r_l (-1+x) - r_i r_j x - r_i r_l x) (r_i rk r_l x + r_j rk r_l x + r_i r_j (r_l + rk x - 2 r_l x)) \\ & \left(4 (r_j^2 + rk^2 + 2 r_j rk x) (r_j^2 + r_l^2 + 2 r_j r_l x) - 4 (r_j^2 - rk r_l x + r_j (rk + r_l) x)^2\right) + \\ & rk (r_j r_l (-1+x) - r_j rk x - rk r_l x) \left(4 (r_i^2 + r_j^2 + 2 r_i r_j x) (r_i^2 + r_l^2 + 2 r_i r_l x) - \right. \\ & \left. 4 (r_i^2 - r_j r_l x + r_i (r_j + r_l) x)^2\right) (-r_i rk r_l x - r_j (r_i r_l x + rk (r_l + r_i x - 2 r_l x))) \\ & (-r_i (rk r_l (-1+x) - r_i rk x - r_i r_l x) (r_i r_j r_l x + r_j rk r_l x + r_i rk (r_l + r_j x - 2 r_l x)) \\ & \left(4 (r_j^2 + rk^2 + 2 r_j rk x) (r_j^2 + r_l^2 + 2 r_j r_l x) - 4 (r_j^2 - rk r_l x + r_j (rk + r_l) x)^2\right) + \\ & r_j (rk r_l (-1+x) - r_j rk x - r_j r_l x) \\ & \left(4 (r_i^2 + rk^2 + 2 r_i rk x) (r_i^2 + r_l^2 + 2 r_i r_l x) - 4 (r_i^2 - rk r_l x + r_i (rk + r_l) x)^2\right) \\ & (-r_i rk r_l x - r_j (r_i r_l x + rk (r_l + r_i x - 2 r_l x))) \left(r_l (r_i r_j (-1+x) - r_i r_l x - r_j r_l x) \right. \\ & \left(4 (r_i^2 + r_j^2 + 2 r_i r_j x) (r_i^2 + rk^2 + 2 r_i rk x) - 4 (r_i^2 - r_j rk x + r_i (r_j + rk) x)^2\right) \\ & (-r_j rk r_l x - r_i (rk r_l x + r_j (r_l + rk x - 2 r_l x))) + rk (r_i r_j (-1+x) - r_i rk x - r_j rk x) \\ & \left(4 (r_i^2 + r_j^2 + 2 r_i r_j x) (r_i^2 + r_l^2 + 2 r_i r_l x) - 4 (r_i^2 - r_j r_l x + r_i (r_j + r_l) x)^2\right) \\ & (-r_j rk r_l x - r_i (rk r_l x + r_j (rk - 2 rk x + r_l x))) \end{aligned}$$

qq15 =

$$\text{Simplify}\left[\frac{\text{Ut15new}}{r_i^2 r_j^2 r_k^2 r_l^2 (1+x)^9} * 16384 * \left(1 / (l_{ij}^2 * l_{ik}^2 * l_{il}^2 * l_{jk}^2 * l_{jl}^2 * l_{kl}^2)\right)\right]$$

化简

$$\begin{aligned} & -r_k^2 r_l^2 (r_i^2 + r_j^2 + 2 r_i r_j x) (r_j^2 + r_k^2 + 2 r_j r_k x) (r_i^2 + r_l^2 + 2 r_i r_l x) \\ & \left(4 (r_i^2 + r_j^2 + 2 r_i r_j x) (r_i^2 + r_k^2 + 2 r_i r_k x) - 4 (r_i^2 - r_j r_k x + r_i (r_j + r_k) x)^2\right) \\ & \left(4 (r_i^2 + r_j^2 + 2 r_i r_j x) (r_i^2 + r_l^2 + 2 r_i r_l x) - 4 (r_i^2 - r_j r_l x + r_i (r_j + r_l) x)^2\right) \\ & \left(-r_i (r_j r_l (-1+x) - r_i r_j x - r_i r_l x) (r_i r_k r_l x + r_j r_k r_l x + r_i r_j (r_l + r_k x - 2 r_l x))\right. \\ & \quad \left.(4 (r_j^2 + r_k^2 + 2 r_j r_k x) (r_j^2 + r_l^2 + 2 r_j r_l x) - 4 (r_j^2 - r_k r_l x + r_j (r_k + r_l) x)^2\right) + \\ & \quad r_k (r_j r_l (-1+x) - r_j r_k x - r_k r_l x) \left(4 (r_i^2 + r_j^2 + 2 r_i r_j x) (r_i^2 + r_l^2 + 2 r_i r_l x) - \right. \\ & \quad \left.4 (r_i^2 - r_j r_l x + r_i (r_j + r_l) x)^2\right) (-r_i r_k r_l x - r_j (r_i r_l x + r_k (r_l + r_i x - 2 r_l x))) \Big) \\ & \left(-r_i (r_k r_l (-1+x) - r_i r_k x - r_i r_l x) (r_i r_j r_l x + r_j r_k r_l x + r_i r_k (r_l + r_j x - 2 r_l x))\right. \\ & \quad \left.(4 (r_j^2 + r_k^2 + 2 r_j r_k x) (r_j^2 + r_l^2 + 2 r_j r_l x) - 4 (r_j^2 - r_k r_l x + r_j (r_k + r_l) x)^2\right) + \\ & \quad r_j (r_k r_l (-1+x) - r_j r_k x - r_j r_l x) \\ & \quad \left(4 (r_i^2 + r_k^2 + 2 r_i r_k x) (r_i^2 + r_l^2 + 2 r_i r_l x) - 4 (r_i^2 - r_k r_l x + r_i (r_k + r_l) x)^2\right) \\ & \quad \left.(-r_i r_k r_l x - r_j (r_i r_l x + r_k (r_l + r_i x - 2 r_l x)))\right) (r_l (r_i r_k (-1+x) - r_i r_l x - r_k r_l x) \\ & \quad \left(4 (r_i^2 + r_j^2 + 2 r_i r_j x) (r_i^2 + r_k^2 + 2 r_i r_k x) - 4 (r_i^2 - r_j r_k x + r_i (r_j + r_k) x)^2\right) \\ & \quad \left.(-r_j r_k r_l x - r_i (r_j r_l x + r_k (r_l + r_j x - 2 r_l x))) + r_j (r_i r_k (-1+x) - r_i r_j x - r_j r_k x)\right) \\ & \quad \left(4 (r_i^2 + r_k^2 + 2 r_i r_k x) (r_i^2 + r_l^2 + 2 r_i r_l x) - 4 (r_i^2 - r_k r_l x + r_i (r_k + r_l) x)^2\right) \\ & \quad \left.(-r_j r_k r_l x - r_i (r_k r_l x + r_j (r_k - 2 r_k x + r_l x)))\right) \Big) \end{aligned}$$

qq16 =

$$\text{Simplify}\left[\frac{\text{Ut16new}}{r_i^2 r_j^2 r_k^2 r_l^2 (1+x)^9} * 16384 * \left(1 / (l_{ij}^2 * l_{ik}^2 * l_{il}^2 * l_{jk}^2 * l_{jl}^2 * l_{kl}^2)\right)\right]$$

化简

$$\begin{aligned} & -r_l^4 (r_i^2 + r_j^2 + 2 r_i r_j x) (r_i^2 + r_k^2 + 2 r_i r_k x) (r_j^2 + r_k^2 + 2 r_j r_k x) \\ & \left(4 (r_i^2 + r_j^2 + 2 r_i r_j x) (r_i^2 + r_k^2 + 2 r_i r_k x) - 4 (r_i^2 - r_j r_k x + r_i (r_j + r_k) x)^2\right)^2 \\ & \left(-r_i (r_j r_l (-1+x) - r_i r_j x - r_i r_l x) (r_i r_k r_l x + r_j r_k r_l x + r_i r_j (r_l + r_k x - 2 r_l x))\right. \\ & \quad \left.(4 (r_j^2 + r_k^2 + 2 r_j r_k x) (r_j^2 + r_l^2 + 2 r_j r_l x) - 4 (r_j^2 - r_k r_l x + r_j (r_k + r_l) x)^2\right) + \\ & \quad r_k (r_j r_l (-1+x) - r_j r_k x - r_k r_l x) \left(4 (r_i^2 + r_j^2 + 2 r_i r_j x) (r_i^2 + r_l^2 + 2 r_i r_l x) - \right. \\ & \quad \left.4 (r_i^2 - r_j r_l x + r_i (r_j + r_l) x)^2\right) (-r_i r_k r_l x - r_j (r_i r_l x + r_k (r_l + r_i x - 2 r_l x))) \Big) \\ & \left(-r_i (r_k r_l (-1+x) - r_i r_k x - r_i r_l x) (r_i r_j r_l x + r_j r_k r_l x + r_i r_k (r_l + r_j x - 2 r_l x))\right. \\ & \quad \left.(4 (r_j^2 + r_k^2 + 2 r_j r_k x) (r_j^2 + r_l^2 + 2 r_j r_l x) - 4 (r_j^2 - r_k r_l x + r_j (r_k + r_l) x)^2\right) + \\ & \quad r_j (r_k r_l (-1+x) - r_j r_k x - r_j r_l x) \left(4 (r_i^2 + r_k^2 + 2 r_i r_k x) (r_i^2 + r_l^2 + 2 r_i r_l x) - \right. \\ & \quad \left.4 (r_i^2 - r_k r_l x + r_i (r_k + r_l) x)^2\right) (-r_i r_k r_l x - r_j (r_i r_l x + r_k (r_l + r_i x - 2 r_l x))) \Big) \\ & \left(-r_j (r_i r_l (-1+x) - r_i r_j x - r_j r_l x) (r_i r_k r_l x + r_j r_k r_l x + r_i r_j (r_l + r_k x - 2 r_l x))\right. \\ & \quad \left.(4 (r_i^2 + r_k^2 + 2 r_i r_k x) (r_i^2 + r_l^2 + 2 r_i r_l x) - 4 (r_i^2 - r_k r_l x + r_i (r_k + r_l) x)^2\right) + \\ & \quad r_k (r_i r_l (-1+x) - r_i r_k x - r_k r_l x) \left(4 (r_i^2 + r_j^2 + 2 r_i r_j x) (r_i^2 + r_l^2 + 2 r_i r_l x) - \right. \\ & \quad \left.4 (r_i^2 - r_j r_l x + r_i (r_j + r_l) x)^2\right) (-r_j r_k r_l x - r_i (r_j r_l x + r_k (r_l + r_j x - 2 r_l x))) \Big) \end{aligned}$$

**Aik12**

$$\frac{1}{16} \left( 4 \left( r_i^2 + r_k^2 + 2 r_i r_k x \right) \left( r_i^2 + r_l^2 + 2 r_i r_l x \right) - \left( 2 r_i^2 + 2 r_i r_k x + 2 r_i r_l x - 2 r_k r_l x \right)^2 \right)$$

$$q_{12} = q_{q1} + q_{q2} + q_{q3} + q_{q4} + q_{q5} + q_{q6} + q_{q7} + q_{q8} + q_{q9} + q_{q10} + q_{q11} + q_{q12} + q_{q13} + q_{q14} + q_{q15} + q_{q16};$$

(\*Non degenerate condition\*)

$$G_0 = \begin{pmatrix} 0 & 1 & 1 & 1 & 1 \\ 1 & 0 & l_{ij2} & l_{ik2} & l_{il2} \\ 1 & l_{ij2} & 0 & l_{jk2} & l_{jl2} \\ 1 & l_{ik2} & l_{jk2} & 0 & l_{kl2} \\ 1 & l_{il2} & l_{jl2} & l_{kl2} & 0 \end{pmatrix};$$

**Simplify[Det[G0]]**

[\[化简\]](#) [\[行列式\]](#)

$$-8 (1+x)^2 \left( -2 r_i r_j r_k r_l (r_k r_l + r_j (r_k + r_l)) x + r_j^2 r_k^2 r_l^2 (-1+2x) + r_i^2 (-2 r_j r_k r_l (r_k + r_l) x + r_k^2 r_l^2 (-1+2x) + r_j^2 (-2 r_k r_l x + r_k^2 (-1+2x) + r_l^2 (-1+2x))) \right)$$

$$M1 = \text{Simplify}\left[\text{Det}[G_0] * \frac{1}{8 (1+x)^2}\right]$$

[\[化简\]](#) [\[行列式\]](#)

$$r_j^2 r_k^2 r_l^2 (1-2x) + 2 r_i r_j r_k r_l (r_k r_l + r_j (r_k + r_l)) x + r_i^2 (r_k^2 r_l^2 (1-2x) + 2 r_j r_k r_l (r_k + r_l) x + r_j^2 (r_k^2 + r_l^2 - 2 r_k^2 x + 2 r_k r_l x - 2 r_l^2 x))$$

(\*Nondegeneracy guarantee M1>0\*)

(\*In determinant2.nb, we will show that q12<0 under the condition M1>0\*)

[\[输入行\]](#)
