# Supplementary material for: Thurston's sphere packings on 3-dimensional manifolds, I
Source: arXiv:1904.11122 ancillary file (2023-05-09)
Supplement: Supplementary file 2 [file determinant2.pdf]

[illegible]



$$\begin{aligned}
& 4 (rj^2 - rk r1 x + rj (rk + r1) x)^2) (rj rk r1 x + ri (rk r1 x + rj (r1 + rk x - 2 r1 x))) \\
& (-r1 (4 (ri^2 + rj^2 + 2 ri rj x) (ri^2 + rk^2 + 2 ri rk x) - 4 (ri^2 - rj rk x + ri (rj + rk) x)^2) \\
& (rj r1 x + ri (rj - rj x + r1 x)) (-rj rk r1 x - ri (rk r1 x + rj (r1 + rk x - 2 r1 x))) - \\
& rk (rj rk x + ri (rj - rj x + rk x)) (4 (ri^2 + rj^2 + 2 ri rj x) (ri^2 + r1^2 + 2 ri r1 x) - \\
& 4 (ri^2 - rj r1 x + ri (rj + r1) x)^2) (-rj rk r1 x - ri (rk r1 x + rj (rk - 2 rk x + r1 x))))); \\
& (-r1 (4 (ri^2 + rj^2 + 2 ri rj x) (ri^2 + rk^2 + 2 ri rk x) - 4 (ri^2 - rj rk x + ri (rj + rk) x)^2) \\
& (rk r1 x + rj (rk - rk x + r1 x)) (-ri rk r1 x - rj (ri r1 x + rk (r1 + ri x - 2 r1 x))) - \\
& ri (ri rk x + rj (rk + ri x - rk x)) (4 (rj^2 + rk^2 + 2 rj rk x) (rj^2 + r1^2 + 2 rj r1 x) - \\
& 4 (rj^2 - rk r1 x + rj (rk + r1) x)^2) (-rj rk r1 x - ri (rk r1 x + rj (rk - 2 rk x + r1 x))))); \\
qq7 = & -rj^2 rk^2 (ri^2 + rj^2 + 2 ri rj x) (ri^2 + r1^2 + 2 ri r1 x) (rk^2 + r1^2 + 2 rk r1 x) \\
& (4 (ri^2 + rj^2 + 2 ri rj x) (ri^2 + r1^2 + 2 ri r1 x) - 4 (ri^2 - rj r1 x + ri (rj + r1) x)^2) \\
& (4 (ri^2 + rk^2 + 2 ri rk x) (ri^2 + r1^2 + 2 ri r1 x) - 4 (ri^2 - rk r1 x + ri (rk + r1) x)^2) \\
& (-rk (rk r1 x + rj (r1 + rk x - r1 x)) (4 (ri^2 + rj^2 + 2 ri rj x) (ri^2 + r1^2 + 2 ri r1 x) - \\
& 4 (ri^2 - rj r1 x + ri (rj + r1) x)^2) (-ri rk r1 x - rj (ri r1 x + rk (r1 + ri x - 2 r1 x))) + \\
& ri (ri r1 x + rj (r1 + ri x - r1 x)) (4 (rj^2 + rk^2 + 2 rj rk x) (rj^2 + r1^2 + 2 rj r1 x) - \\
& 4 (rj^2 - rk r1 x + rj (rk + r1) x)^2) (rj rk r1 x + ri (rk r1 x + rj (r1 + rk x - 2 r1 x)))) \\
& (-r1 (4 (ri^2 + rj^2 + 2 ri rj x) (ri^2 + rk^2 + 2 ri rk x) - 4 (ri^2 - rj rk x + ri (rj + rk) x)^2) \\
& (rk r1 x + ri (rk - rk x + r1 x)) (-rj rk r1 x - ri (rj r1 x + rk (r1 + rj x - 2 r1 x))) - \\
& rj (rj rk x + ri (rk + rj x - rk x)) (4 (ri^2 + rk^2 + 2 ri rk x) (ri^2 + r1^2 + 2 ri r1 x) - \\
& 4 (ri^2 - rk r1 x + ri (rk + r1) x)^2) (-rj rk r1 x - ri (rk r1 x + rj (rk - 2 rk x + r1 x)))) \\
& (-r1 (4 (ri^2 + rj^2 + 2 ri rj x) (ri^2 + rk^2 + 2 ri rk x) - 4 (ri^2 - rj rk x + ri (rj + rk) x)^2) \\
& (rk r1 x + rj (rk - rk x + r1 x)) (-ri rk r1 x - rj (ri r1 x + rk (r1 + ri x - 2 r1 x))) - \\
& ri (ri rk x + rj (rk + ri x - rk x)) (4 (rj^2 + rk^2 + 2 rj rk x) (rj^2 + r1^2 + 2 rj r1 x) - \\
& 4 (rj^2 - rk r1 x + rj (rk + r1) x)^2) (-rj rk r1 x - ri (rk r1 x + rj (rk - 2 rk x + r1 x))))); \\
qq8 = & -rj^2 r1^2 (ri^2 + rj^2 + 2 ri rj x) (ri^2 + rk^2 + 2 ri rk x) (rk^2 + r1^2 + 2 rk r1 x) \\
& (4 (ri^2 + rj^2 + 2 ri rj x) (ri^2 + rk^2 + 2 ri rk x) - 4 (ri^2 - rj rk x + ri (rj + rk) x)^2) \\
& (4 (ri^2 + rk^2 + 2 ri rk x) (ri^2 + r1^2 + 2 ri r1 x) - 4 (ri^2 - rk r1 x + ri (rk + r1) x)^2) \\
& (-rk (rk r1 x + ri (r1 + rk x - r1 x)) (4 (ri^2 + rj^2 + 2 ri rj x) (ri^2 + r1^2 + 2 ri r1 x) - \\
& 4 (ri^2 - rj r1 x + ri (rj + r1) x)^2) (-rj rk r1 x - ri (rj r1 x + rk (r1 + rj x - 2 r1 x))) + \\
& rj (rj r1 x + ri (r1 + rj x - r1 x)) (4 (ri^2 + rk^2 + 2 ri rk x) (ri^2 + r1^2 + 2 ri r1 x) - \\
& 4 (ri^2 - rk r1 x + ri (rk + r1) x)^2) (rj rk r1 x + ri (rk r1 x + rj (r1 + rk x - 2 r1 x)))) \\
& (-rk (rk r1 x + rj (r1 + rk x - r1 x)) (4 (ri^2 + rj^2 + 2 ri rj x) (ri^2 + r1^2 + 2 ri r1 x) - \\
& 4 (ri^2 - rj r1 x + ri (rj + r1) x)^2) (-ri rk r1 x - rj (ri r1 x + rk (r1 + ri x - 2 r1 x))) + \\
& ri (ri r1 x + rj (r1 + ri x - r1 x)) (4 (rj^2 + rk^2 + 2 rj rk x) (rj^2 + r1^2 + 2 rj r1 x) - \\
& 4 (rj^2 - rk r1 x + rj (rk + r1) x)^2) (rj rk r1 x + ri (rk r1 x + rj (r1 + rk x - 2 r1 x)))) \\
& (-r1 (4 (ri^2 + rj^2 + 2 ri rj x) (ri^2 + rk^2 + 2 ri rk x) - 4 (ri^2 - rj rk x + ri (rj + rk) x)^2) \\
& (rk r1 x + rj (rk - rk x + r1 x)) (-ri rk r1 x - rj (ri r1 x + rk (r1 + ri x - 2 r1 x))) - \\
& ri (ri rk x + rj (rk + ri x - rk x)) (4 (rj^2 + rk^2 + 2 rj rk x) (rj^2 + r1^2 + 2 rj r1 x) - \\
& 4 (rj^2 - rk r1 x + rj (rk + r1) x)^2) (-rj rk r1 x - ri (rk r1 x + rj (rk - 2 rk x + r1 x))))); \\
qq9 = & -ri^2 rk^2 (rj^2 + rk^2 + 2 rj rk x) (ri^2 + r1^2 + 2 ri r1 x) (rj^2 + r1^2 + 2 rj r1 x) \\
& (4 (ri^2 + rj^2 + 2 ri rj x) (ri^2 + r1^2 + 2 ri r1 x) - 4 (ri^2 - rj r1 x + ri (rj + r1) x)^2)
\end{aligned}$$





```

4 (rj2 - rk r1 x + rj (rk + r1) x)2) (rj rk r1 x + ri (rk r1 x + rj (r1 + rk x - 2 r1 x)))
(- r1 (4 (ri2 + rj2 + 2 ri rj x) (ri2 + rk2 + 2 ri rk x) - 4 (ri2 - rj rk x + ri (rj + rk) x)2)
(rj r1 x + ri (rj - rj x + r1 x)) (- rj rk r1 x - ri (rk r1 x + rj (r1 + rk x - 2 r1 x))) -
rk (rj rk x + ri (rj - rj x + rk x)) (4 (ri2 + rj2 + 2 ri rj x) (ri2 + r12 + 2 ri r1 x) -
4 (ri2 - rj r1 x + ri (rj + r1) x)2) (- rj rk r1 x - ri (rk r1 x + rj (rk - 2 rk x + r1 x)))));
qq15 = -rk2 r12 (ri2 + rj2 + 2 ri rj x) (rj2 + rk2 + 2 rj rk x) (ri2 + r12 + 2 ri r1 x)
(4 (ri2 + rj2 + 2 ri rj x) (ri2 + rk2 + 2 ri rk x) - 4 (ri2 - rj rk x + ri (rj + rk) x)2)
(4 (ri2 + rj2 + 2 ri rj x) (ri2 + r12 + 2 ri r1 x) - 4 (ri2 - rj r1 x + ri (rj + r1) x)2)
(- rj (rj r1 x + rk (r1 + rj x - r1 x)) (4 (ri2 + rk2 + 2 ri rk x) (ri2 + r12 + 2 ri r1 x) -
4 (ri2 - rk r1 x + ri (rk + r1) x)2) (- ri rk r1 x - rj (ri r1 x + rk (r1 + ri x - 2 r1 x))) +
ri (ri r1 x + rk (r1 + ri x - r1 x)) (4 (rj2 + rk2 + 2 rj rk x) (rj2 + r12 + 2 rj r1 x) -
4 (rj2 - rk r1 x + rj (rk + r1) x)2) (rj rk r1 x + ri (rj r1 x + rk (r1 + rj x - 2 r1 x))))
(- rk (rk r1 x + rj (r1 + rk x - r1 x)) (4 (ri2 + rj2 + 2 ri rj x) (ri2 + r12 + 2 ri r1 x) -
4 (ri2 - rj r1 x + ri (rj + r1) x)2) (- ri rk r1 x - rj (ri r1 x + rk (r1 + ri x - 2 r1 x))) +
ri (ri r1 x + rj (r1 + ri x - r1 x)) (4 (rj2 + rk2 + 2 rj rk x) (rj2 + r12 + 2 rj r1 x) -
4 (rj2 - rk r1 x + rj (rk + r1) x)2) (rj rk r1 x + ri (rk r1 x + rj (r1 + rk x - 2 r1 x))))
(- r1 (4 (ri2 + rj2 + 2 ri rj x) (ri2 + rk2 + 2 ri rk x) - 4 (ri2 - rj rk x + ri (rj + rk) x)2)
(rk r1 x + ri (rk - rk x + r1 x)) (- rj rk r1 x - ri (rj r1 x + rk (r1 + rj x - 2 r1 x))) -
rj (rj rk x + ri (rk + rj x - rk x)) (4 (ri2 + rk2 + 2 ri rk x) (ri2 + r12 + 2 ri r1 x) -
4 (ri2 - rk r1 x + ri (rk + r1) x)2) (- rj rk r1 x - ri (rk r1 x + rj (rk - 2 rk x + r1 x)))));
qq16 = -r14 (ri2 + rj2 + 2 ri rj x) (ri2 + rk2 + 2 ri rk x) (rj2 + rk2 + 2 rj rk x)
(4 (ri2 + rj2 + 2 ri rj x) (ri2 + rk2 + 2 ri rk x) - 4 (ri2 - rj rk x + ri (rj + rk) x)2)2
(- rj (rj r1 x + rk (r1 + rj x - r1 x)) (4 (ri2 + rk2 + 2 ri rk x) (ri2 + r12 + 2 ri r1 x) -
4 (ri2 - rk r1 x + ri (rk + r1) x)2) (- ri rk r1 x - rj (ri r1 x + rk (r1 + ri x - 2 r1 x))) +
ri (ri r1 x + rk (r1 + ri x - r1 x)) (4 (rj2 + rk2 + 2 rj rk x) (rj2 + r12 + 2 rj r1 x) -
4 (rj2 - rk r1 x + rj (rk + r1) x)2) (rj rk r1 x + ri (rj r1 x + rk (r1 + rj x - 2 r1 x))))
(- rk (rk r1 x + ri (r1 + rk x - r1 x)) (4 (ri2 + rj2 + 2 ri rj x) (ri2 + r12 + 2 ri r1 x) -
4 (ri2 - rj r1 x + ri (rj + r1) x)2) (- rj rk r1 x - ri (rj r1 x + rk (r1 + rj x - 2 r1 x))) +
rj (rj r1 x + ri (r1 + rj x - r1 x)) (4 (ri2 + rk2 + 2 ri rk x) (ri2 + r12 + 2 ri r1 x) -
4 (ri2 - rk r1 x + ri (rk + r1) x)2) (rj rk r1 x + ri (rk r1 x + rj (r1 + rk x - 2 r1 x))))
(- rk (rk r1 x + rj (r1 + rk x - r1 x)) (4 (ri2 + rj2 + 2 ri rj x) (ri2 + r12 + 2 ri r1 x) -
4 (ri2 - rj r1 x + ri (rj + r1) x)2) (- ri rk r1 x - rj (ri r1 x + rk (r1 + ri x - 2 r1 x))) +
ri (ri r1 x + rj (r1 + ri x - r1 x)) (4 (rj2 + rk2 + 2 rj rk x) (rj2 + r12 + 2 rj r1 x) -
4 (rj2 - rk r1 x + rj (rk + r1) x)2) (rj rk r1 x + ri (rk r1 x + rj (r1 + rk x - 2 r1 x)))));
q12 = qq1 + qq2 + qq3 + qq4 + qq5 + qq6 + qq7 + qq8 + qq9 + qq10 + qq11 +
qq12 + qq13 + qq14 + qq15 + qq16;

```

```

In[5]:= M1 = rj2 rk2 r12 (1 - 2 x) + 2 ri rj rk r1 (rk r1 + rj (rk + r1)) x +
ri2 (rk2 r12 (1 - 2 x) + 2 rj rk r1 (rk + r1) x + rj2 (rk2 + r12 - 2 rk2 x + 2 rk r1 x - 2 r12 x));

```

(\*Goal: Show that Q12 is non-zero under the condition M1>0. \*)

[显示](#)

(\*without loss of generality, one can set ri=1 \*)

```
In[6]:= ri = 1; rj = r2; rk = r3; rl = r4;
```

```
In[7]:= Simplify[M1]
```

化简

```
Out[7]:= r3^2 r4^2 (1 - 2 x) + 2 r2 r3 r4 (r3 + r4 + r3 r4) x +  
r2^2 (r4^2 (1 - 2 x) + 2 r3 r4 (1 + r4) x + r3^2 (1 + r4^2 - 2 x + 2 r4 x - 2 r4^2 x))
```

```
q12;
```

```
Simplify[PolynomialRemainder[q12, M1, x], TimeConstraint -> 500]
```

化简

多项式余式

时间花费限制

```
(*this step takes 11 hours*)
```

```
0
```

```
(*quotient of qq1*)
```

```
qq1quotient = PolynomialQuotient[qq1, M1, x];
```

多项式的商

```
(*this step takes 10 mins*)
```

```
In[9]:= (*quotient of qq2*)
```

```
qq2quotient = PolynomialQuotient[qq2, M1, x];
```

多项式的商

```
In[10]:= (*quotient of qq3*)
```

```
qq3quotient = PolynomialQuotient[qq3, M1, x];
```

多项式的商

```
In[11]:= (*quotient of qq4*)
```

```
qq4quotient = PolynomialQuotient[qq4, M1, x];
```

多项式的商

```
In[12]:= (*quotient of qq5*)
```

```
qq5quotient = PolynomialQuotient[qq5, M1, x];
```

多项式的商

```
In[13]:= (*quotient of qq6*)
```

```
qq6quotient = PolynomialQuotient[qq6, M1, x];
```

多项式的商

```
In[14]:= (*quotient of qq7*)
```

```
qq7quotient = PolynomialQuotient[qq7, M1, x];
```

多项式的商

```
In[15]:= (*quotient of qq8*)
```

```
qq8quotient = PolynomialQuotient[qq8, M1, x];
```

多项式的商

```
In[16]:= (*quotient of qq9*)
```

```
qq9quotient = PolynomialQuotient[qq9, M1, x];
```

多项式的商

```
In[17]:= (*quotient of qq10*)
```

```
qq10quotient = PolynomialQuotient[qq10, M1, x];
```

多项式的商

```
In[18]:= (*quotient of qq11*)
```

```
qq11quotient = PolynomialQuotient[qq11, M1, x];
```

多项式的商

```

In[19]:= (*quotient of qq12*)
qq12quotient = PolynomialQuotient[qq12, M1, x];
           | 多项式的商

In[20]:= (*quotient of qq13*)
qq13quotient = PolynomialQuotient[qq13, M1, x];
           | 多项式的商

In[21]:= (*quotient of qq14*)
qq14quotient = PolynomialQuotient[qq14, M1, x];
           | 多项式的商

In[22]:= (*quotient of qq15*)
qq15quotient = PolynomialQuotient[qq15, M1, x];
           | 多项式的商

In[23]:= (*quotient of qq16*)
qq16quotient = PolynomialQuotient[qq16, M1, x];
           | 多项式的商

(*q12new=quotient of q12*)

In[24]:= q12new = qq1quotient + qq2quotient + qq3quotient + qq4quotient + qq5quotient + qq6quotient +
          qq7quotient + qq8quotient + qq9quotient + qq10quotient + qq11quotient +
          qq12quotient + qq13quotient + qq14quotient + qq15quotient + qq16quotient;

In[25]:= Simplify[PolynomialRemainder[q12new, M1, x]]
           | 化简 | 多项式余式

Out[25]= 0

In[26]:= q12new1 = PolynomialQuotient[q12new, M1, x]
           | 多项式的商

```

$$\begin{aligned}
& \dots 384\,290 \dots + \left( \dots 1 \dots \right) x^{16} + \\
& \left( - \left( \left( 196\,608\,r_2^{16}\,r_3^{14}\,r_4^2 \right) / \left( -2\,r_2^2\,r_3^2 + 2\,r_2^2\,r_3\,r_4 - 2\,r_2^2\,r_4^2 - 2\,r_3^2\,r_4^2 - \right. \right. \right. \\
& \quad \left. \left. \left. 2\,r_2^2\,r_3^2\,r_4^2 + 2\,r_2\,r_3\,r_4\,(r_3 + r_4) + 2\,r_2\,r_3\,r_4\,(r_3\,r_4 + r_2\,(r_3 + r_4)) \right) \right)^2 + \right. \\
& \quad \left( 393\,216\,r_2^{15}\,r_3^{15}\,r_4^2 \right) / \left( -2\,r_2^2\,r_3^2 + 2\,r_2^2\,r_3\,r_4 - 2\,r_2^2\,r_4^2 - 2\,r_3^2\,r_4^2 - \right. \\
& \quad \left. \left. 2\,r_2^2\,r_3^2\,r_4^2 + 2\,r_2\,r_3\,r_4\,(r_3 + r_4) + 2\,r_2\,r_3\,r_4\,(r_3\,r_4 + r_2\,(r_3 + r_4)) \right) \right)^2 + \\
& \quad \frac{393\,216\,r_2^{16}\,r_3^{15}\,r_4^2}{\left( -2\,r_2^2\,r_3^2 + \dots 8 \dots + 2\,r_2\,r_3\,r_4\,(r_3\,r_4 + r_2\,( \dots 1 \dots )) \right)^2} - \frac{196\,608\,r_2^{14}\,r_3^{16}\,r_4^2}{\left( -2\,r_2^2\,r_3^2 + \dots 8 \dots + \dots 1 \dots \right)^2} + \\
& \quad \dots 1410 \dots + \frac{15\,335\,424\,r_2^{11}\,r_3^{16}\,r_4^{16}}{\left( \dots 1 \dots \right)^2} - \frac{6\,094\,848\,r_2^{12}\,r_3^{16}\,r_4^{16}}{\left( -2\,r_2^2\,r_3^2 + \dots 8 \dots + 2\,r_2\,r_3\,r_4\,( \dots 1 \dots ) \right)^2} + \\
& \quad \left( 1\,572\,864\,r_2^{13}\,r_3^{16}\,r_4^{16} \right) / \left( -2\,r_2^2\,r_3^2 + 2\,r_2^2\,r_3\,r_4 - 2\,r_2^2\,r_4^2 - \dots 1 \dots - \right. \\
& \quad \left. \dots 1 \dots + 2\,r_2\,r_3\,r_4\,(r_3 + r_4) + 2\,r_2\,r_3\,r_4\,(r_3\,r_4 + r_2\,(r_3 + r_4)) \right)^2 - \\
& \quad \left( 196\,608\,r_2^{14}\,r_3^{16}\,r_4^{16} \right) / \left( -2\,r_2^2\,r_3^2 + 2\,r_2^2\,r_3\,r_4 - 2\,r_2^2\,r_4^2 - 2\,r_3^2\,r_4^2 - \right. \\
& \quad \left. \left. 2\,r_2^2\,r_3^2\,r_4^2 + 2\,r_2\,r_3\,r_4\,(r_3 + r_4) + 2\,r_2\,r_3\,r_4\,(r_3\,r_4 + r_2\,(r_3 + r_4)) \right) \right)^2 \Big) x^{17}
\end{aligned}$$

大型输出

显示更少

显示更多

显示全部

设定大小限制...

```
(*Simplify[q12new1]*)
```

| 化简



In[27]:= **q12new11 = Simplify[q12new1, TimeConstraint → 500]**

化简

时间花费限制

Out[27]=

$$\begin{aligned}
 & -1024 (1+x)^5 (r^4 (-1+x) - 2 r^3 r^4 (1+r^4) x + r^3^2 (-1+r^4^2 (-1+x) + x - 2 r^4 x)) \\
 & ( \dots 22 \dots + r^2^6 r^3^3 r^4^3 ( \dots 14 \dots + \\
 & \quad r^3^5 r^4^3 (x^2 (-85 - 43 x - 1254 x^2 + 2254 x^3 - 3777 x^4 + 3345 x^5 - 1812 x^6 + 508 x^7) + \\
 & \quad r^4^6 x^2 (-85 - 43 x - 1254 x^2 + 2254 x^3 - 3777 x^4 + 3345 x^5 - 1812 x^6 + 508 x^7) + \\
 & \quad 2 r^4 x (-72 + 79 x - 1979 x^2 + 4155 x^3 - 14134 x^4 + 19571 x^5 - 21841 x^6 + \\
 & \quad 15219 x^7 - 6638 x^8 + 1752 x^9) + 2 r^4^5 x (-72 + 79 x - 1979 x^2 + 4155 x^3 - \\
 & \quad 14134 x^4 + 19571 x^5 - 21841 x^6 + 15219 x^7 - 6638 x^8 + 1752 x^9) + \\
 & \quad 2 r^4^3 x (-240 - 121 x - 5167 x^2 + 9058 x^3 - 38028 x^4 + 48471 x^5 - 56291 x^6 + 30976 x^7 - \\
 & \quad 7354 x^8 + 864 x^9 + 1128 x^{10}) + 2 r^4^2 (-78 + 702 x - 4951 x^2 + 13963 x^3 - 39952 x^4 + \\
 & \quad 61090 x^5 - 85743 x^6 + 74207 x^7 - 50356 x^8 + 24670 x^9 - 7064 x^{10} + 1704 x^{11}) + \\
 & \quad 2 r^4^4 (-78 + 702 x - 4951 x^2 + 13963 x^3 - 39952 x^4 + 61090 x^5 - 85743 x^6 + \\
 & \quad 74207 x^7 - 50356 x^8 + 24670 x^9 - 7064 x^{10} + 1704 x^{11})) ) ) )
 \end{aligned}$$

大型输出

显示更少

显示更多

显示全部

设定大小限制...

In[28]:= **Simplify[Coefficient[q12new11, r2, 15]]**

化简

系数

Out[28]= 0

In[29]:= **Simplify[Coefficient[q12new11, r3, 15]]**

化简

系数

Out[29]= 0

In[30]:= **Simplify[Coefficient[q12new11, r4, 15]]**

化简

系数

Out[30]= 0

In[31]:= **Cf[i\_, j\_, k\_] := Coefficient[Coefficient[Coefficient[q12new11, r2, i], r3, j], r4, k];**

系数

系数

系数

(\*i,j,k=0,...,14\*)

(\* Now we will give the graph of C[i,j,k] of x on [0,1] \*)

此刻

常量

In[32]:= **(\*first group coefficients r2^14r3^14\*)**

**Plot[Cf[14, 14, 14], {x, 0, 1}]**

绘图

Out[32]=

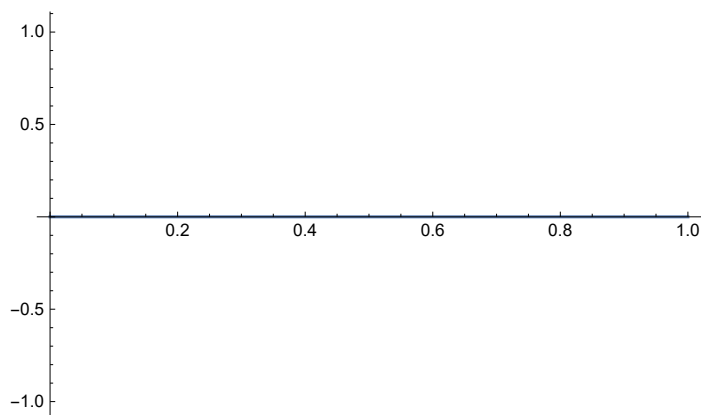

```
Plot[Cf[14, 14, 13], {x, 0, 1}]
```

[绘图](#)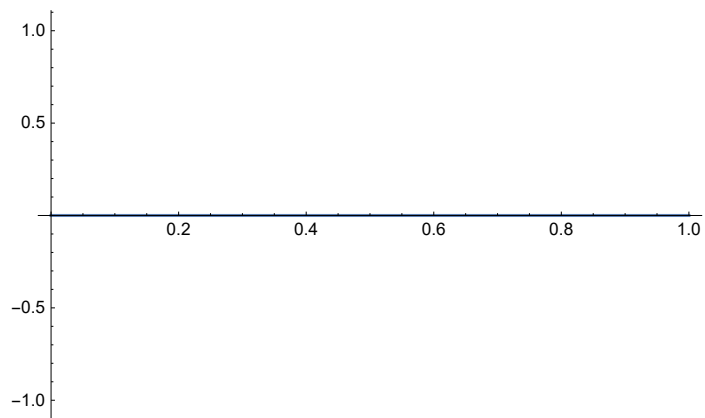

```
Plot[Cf[14, 14, 12], {x, 0, 1}]
```

[绘图](#)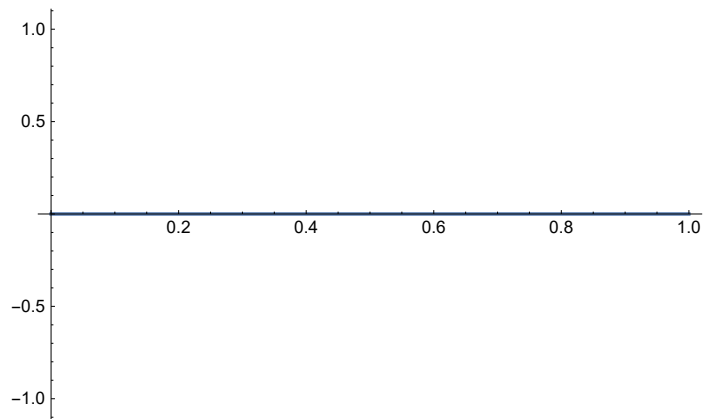

```
Plot[Cf[14, 14, 11], {x, 0, 1}]
```

[绘图](#)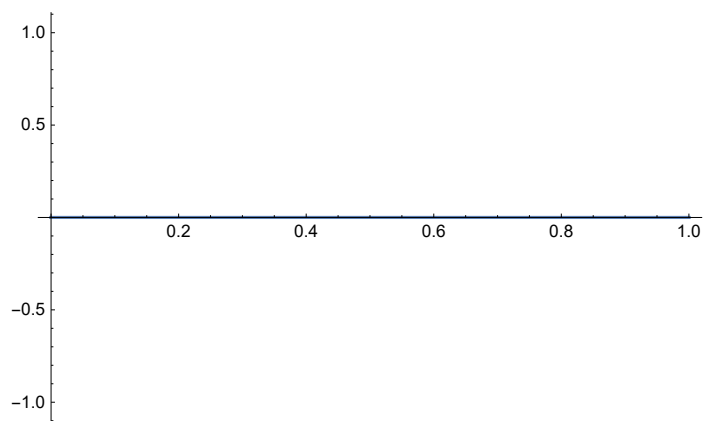

**Plot[Cf[14, 14, 10], {x, 0, 1}]**

[绘图](#)

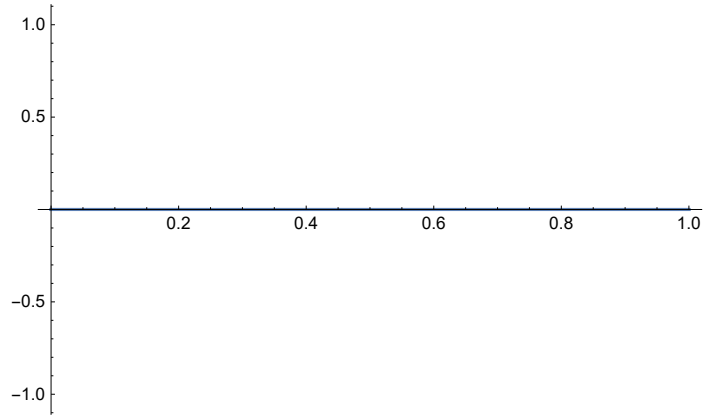

**Plot[Cf[14, 14, 9], {x, 0, 1}]**

[绘图](#)

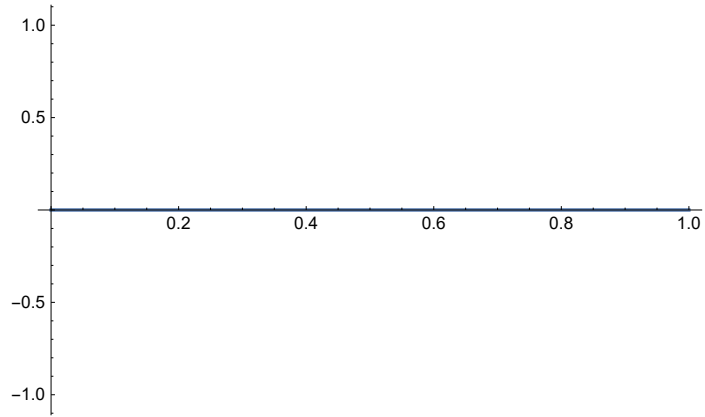

**Plot[Cf[14, 14, 8], {x, 0, 1}]**

[绘图](#)

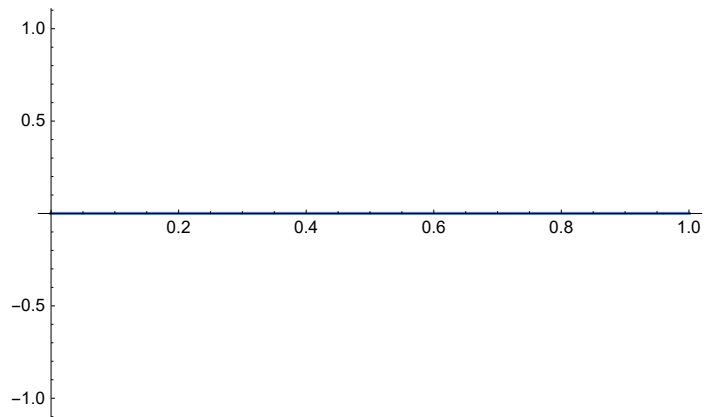

```
Plot[Cf[14, 14, 7], {x, 0, 1}]
```

[绘图](#)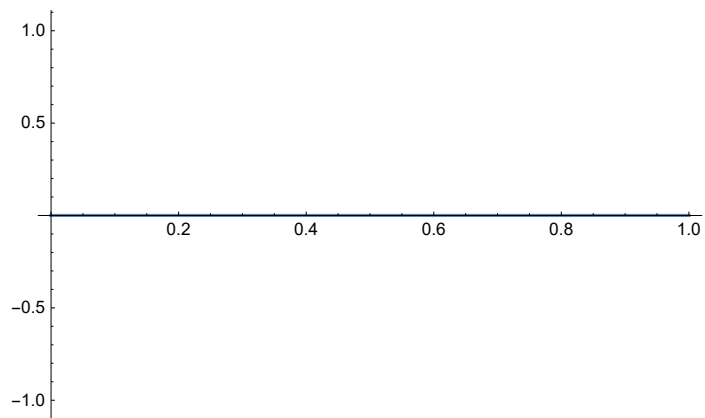

```
Plot[Cf[14, 14, 6], {x, 0, 1}]
```

[绘图](#)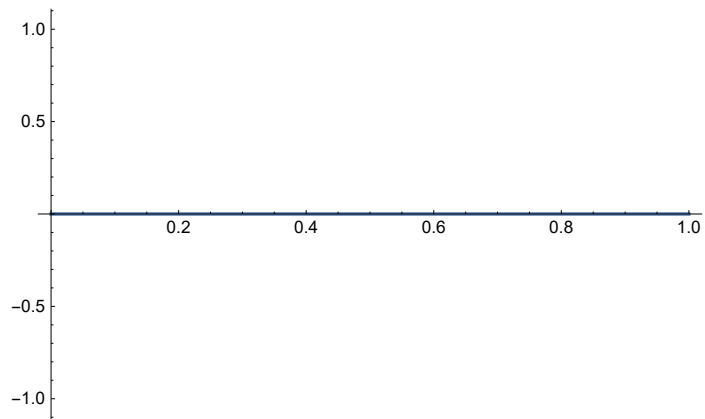

```
Plot[Cf[14, 14, 5], {x, 0, 1}]
```

[绘图](#)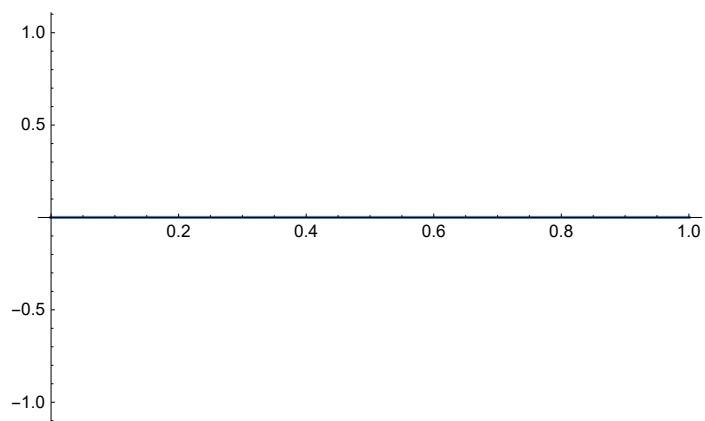

**Plot[Cf[14, 14, 4], {x, 0, 1}]**

[绘图](#)

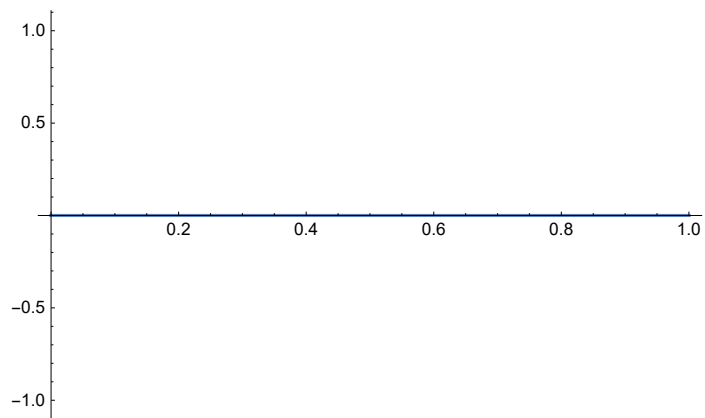

**Plot[Cf[14, 14, 3], {x, 0, 1}]**

[绘图](#)

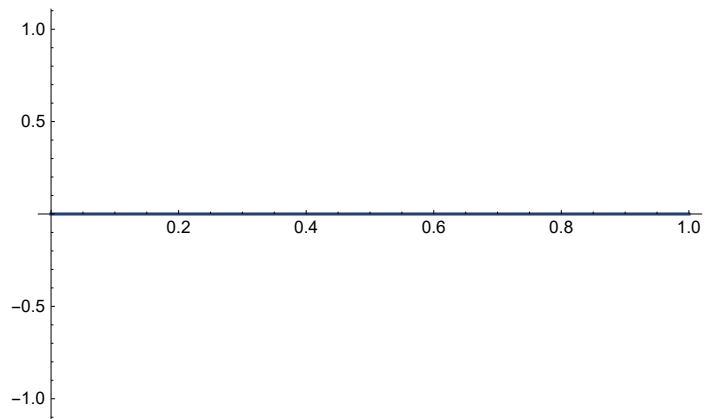

**Plot[Cf[14, 14, 2], {x, 0, 1}]**

[绘图](#)

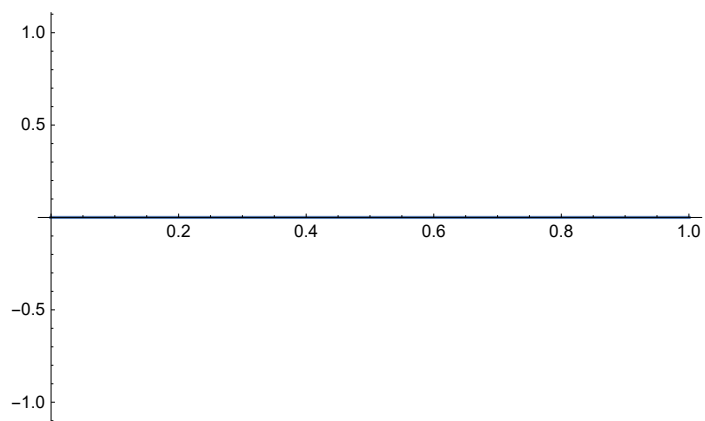

```
Plot[Cf[14, 14, 1], {x, 0, 1}]
```

[绘图](#)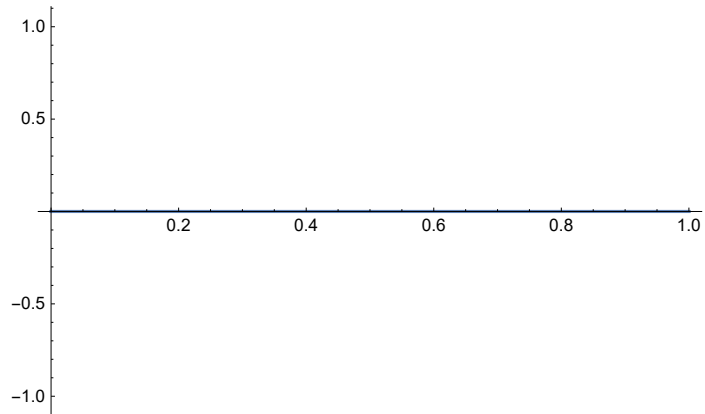

```
Plot[Cf[14, 14, 0], {x, 0, 1}]
```

[绘图](#)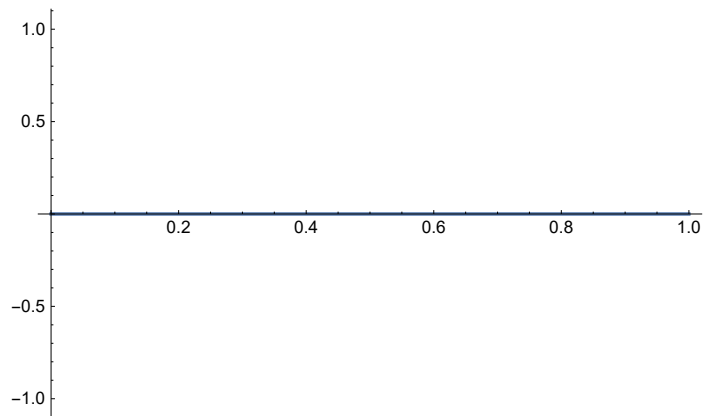

```
(* (2nd group coefficients r2^14r3^13*) *)
```

```
Plot[Cf[14, 13, 14], {x, 0, 1}]
```

[绘图](#)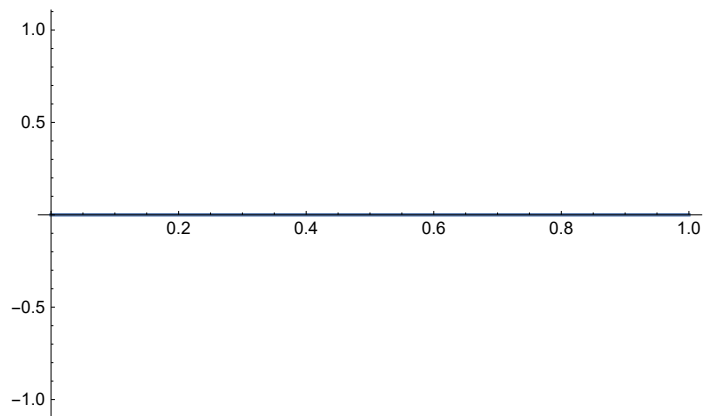

**Plot[Cf[14, 13, 13], {x, 0, 1}]**

[绘图](#)

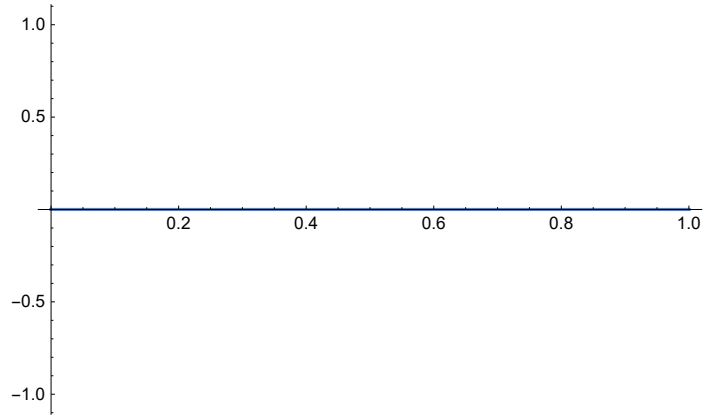

**Plot[Cf[14, 13, 12], {x, 0, 1}]**

[绘图](#)

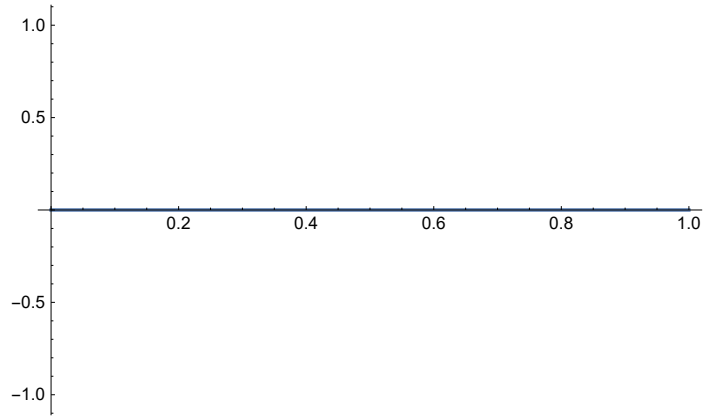

**Plot[Cf[14, 13, 11], {x, 0, 1}]**

[绘图](#)

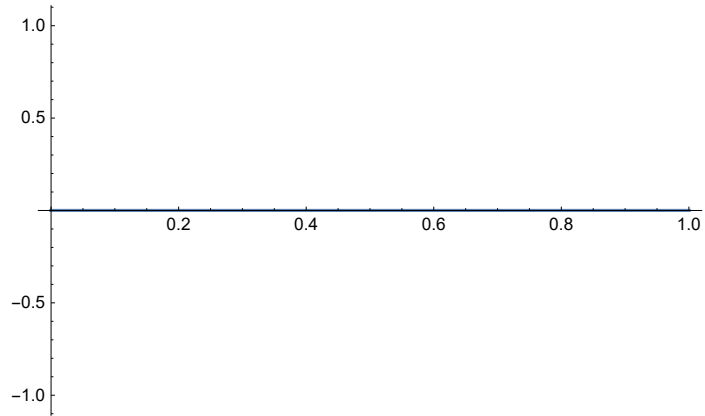

**Plot[Cf[14, 13, 10], {x, 0, 1}]**

[绘图](#)

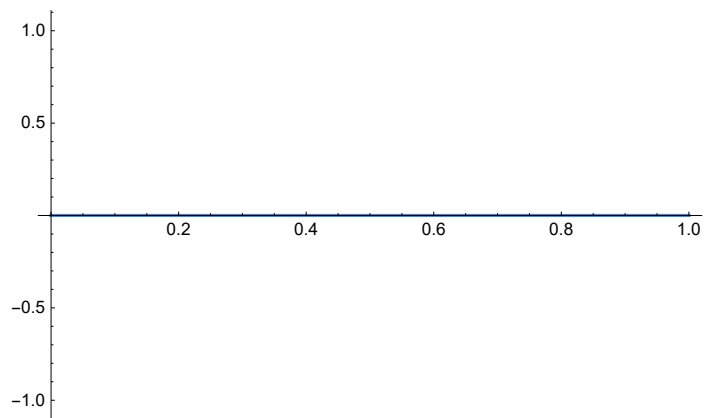

In[33]:= **Plot[Cf[14, 13, 9], {x, 0, 1}]**

[绘图](#)

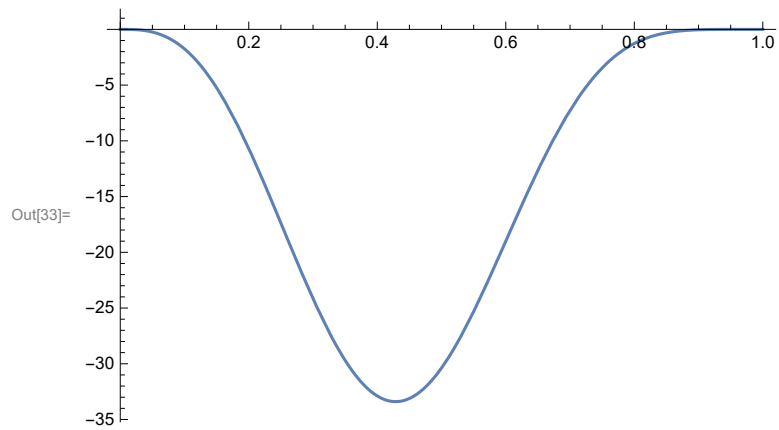

In[38]:= **Plot[Cf[14, 13, 8], {x, 0, 1}]**

[绘图](#)

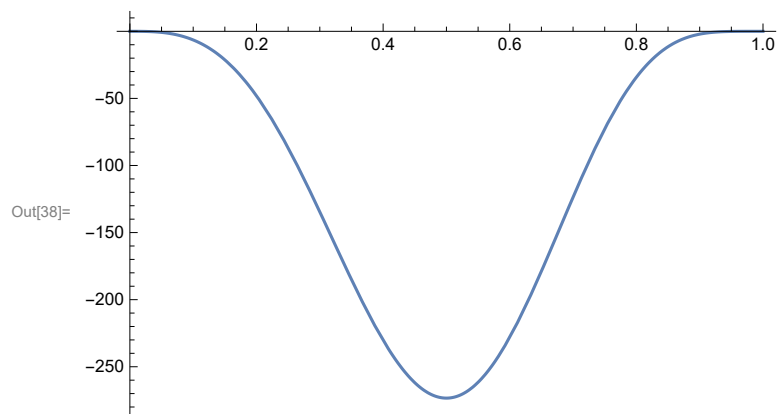



In[39]:= **Plot[Cf[14, 13, 7], {x, 0, 1}]**

[绘图](#)

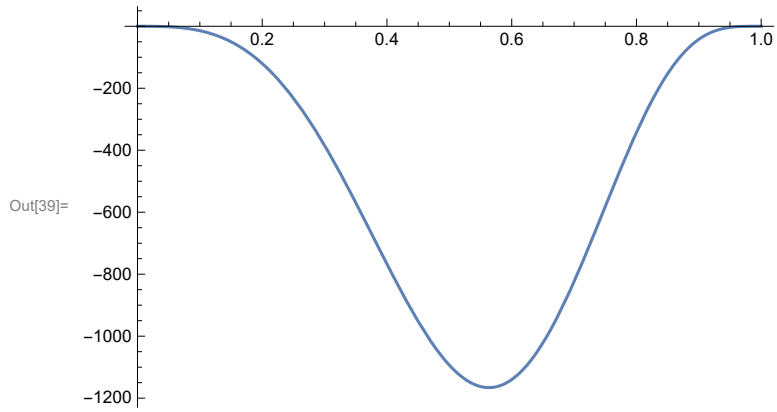

In[37]:= **Plot[Cf[14, 13, 6], {x, 0, 1}]**

[绘图](#)

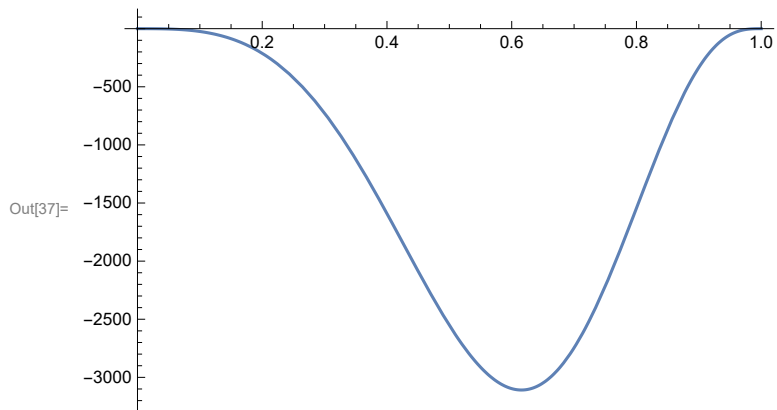

In[36]:= **Plot[Cf[14, 13, 5], {x, 0, 1}]**

[绘图](#)

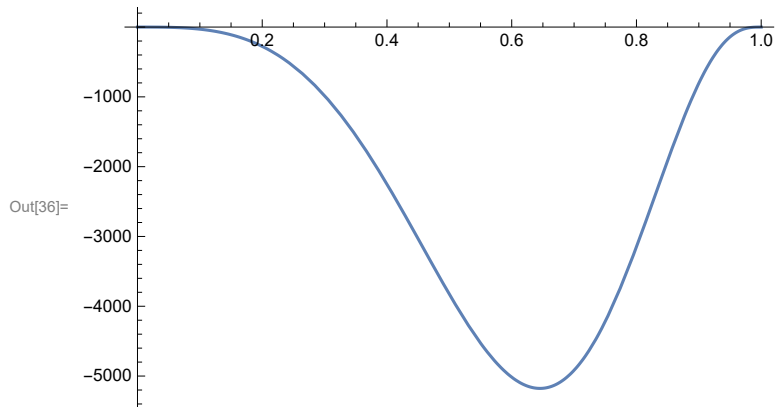

In[35]:= **Plot[Cf[14, 13, 4], {x, 0, 1}]**

[绘图](#)

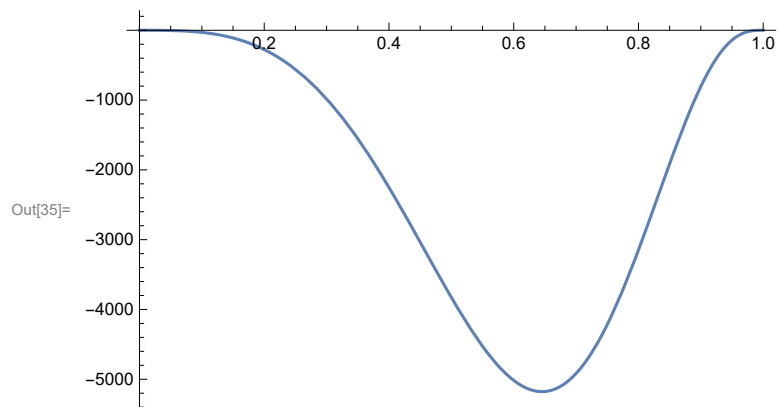

In[43]:= **Plot[Cf[14, 13, 3], {x, 0, 1}]**

[绘图](#)

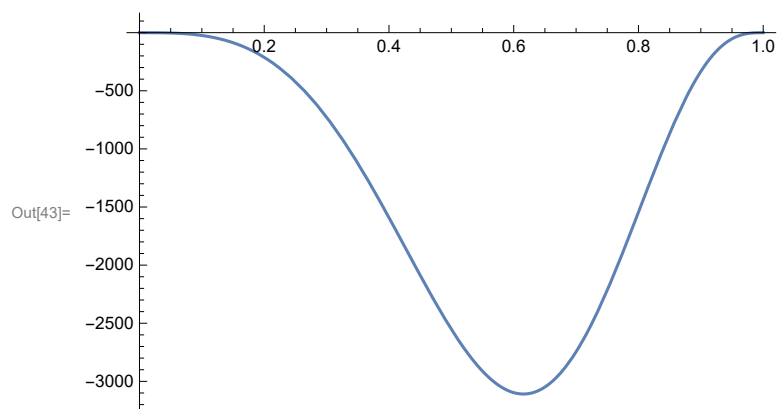

In[42]:= **Plot[Cf[14, 13, 2], {x, 0, 1}]**

[绘图](#)

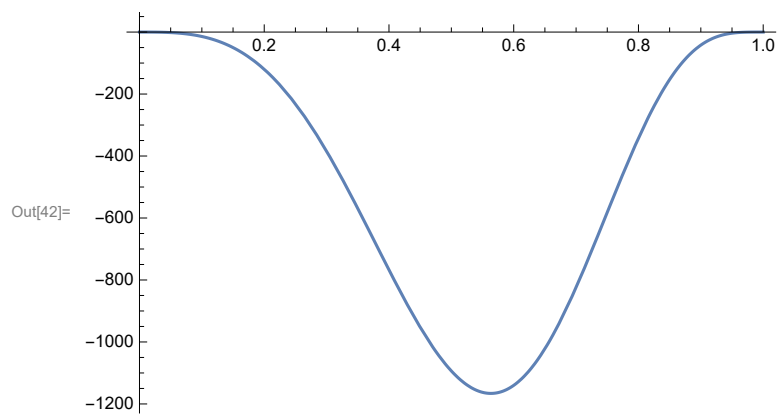

In[41]:= **Plot[Cf[14, 13, 1], {x, 0, 1}]**

[绘图](#)

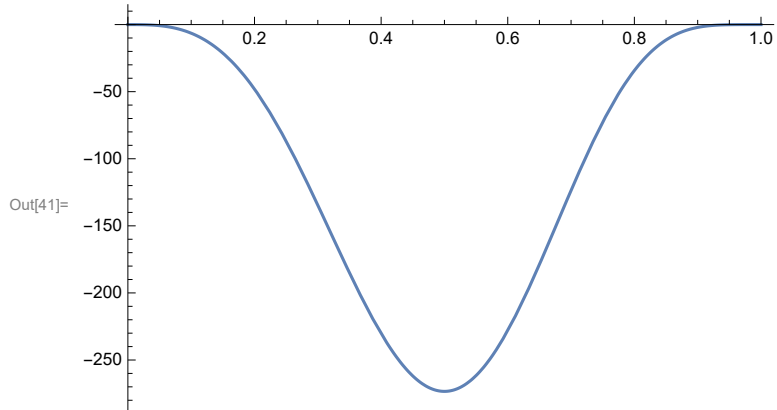

In[40]:= **Plot[Cf[14, 13, 0], {x, 0, 1}]**

[绘图](#)

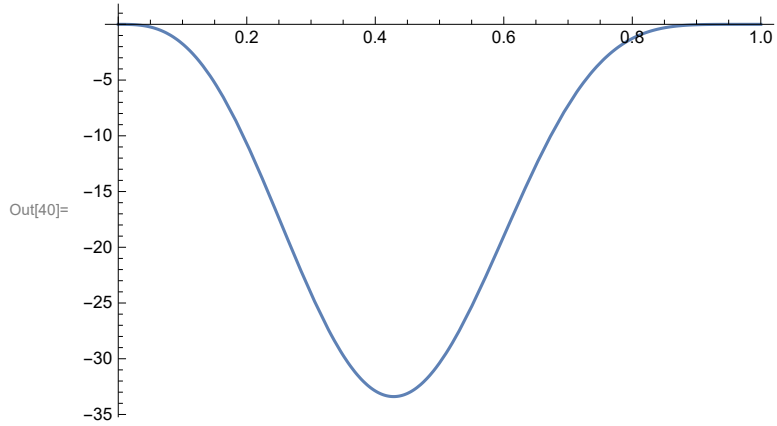

**(\*(3rd group coefficients r2^14r3^12\*))**

**Plot[Cf[14, 12, 14], {x, 0, 1}]**

[绘图](#)

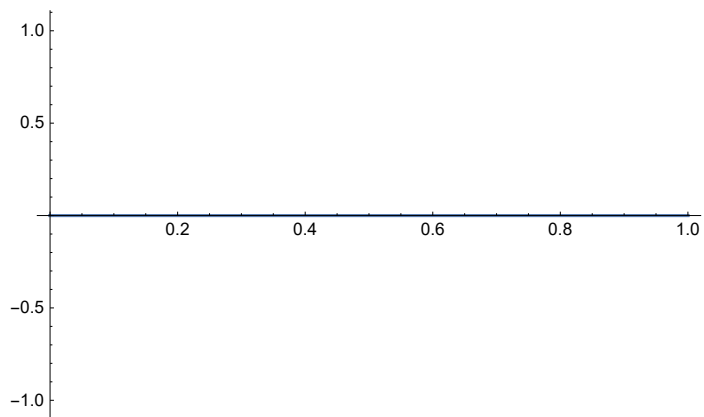

```
Plot[Cf[14, 12, 13], {x, 0, 1}]
```

[绘图](#)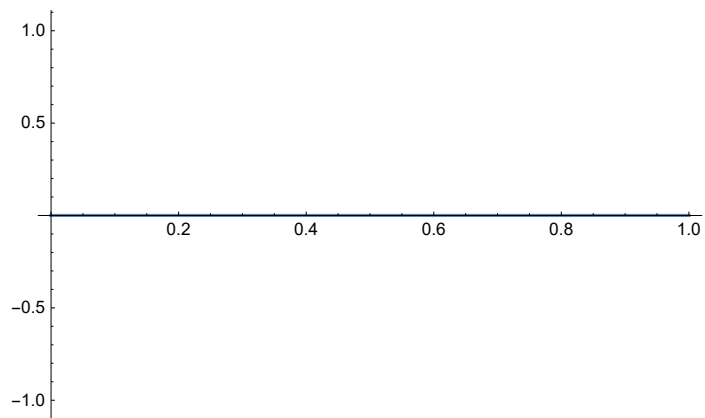

```
Plot[Cf[14, 12, 12], {x, 0, 1}]
```

[绘图](#)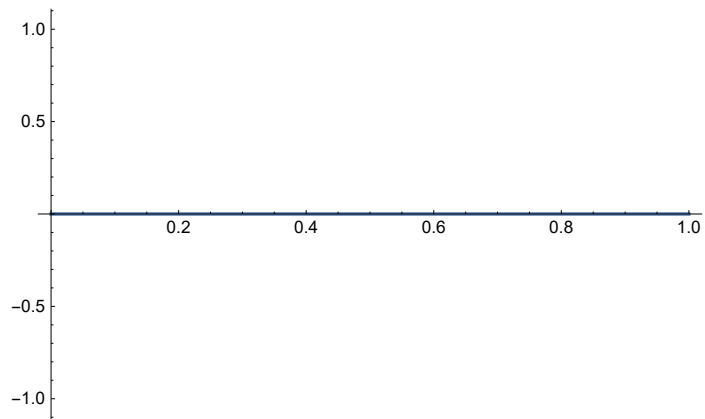

```
Plot[Cf[14, 12, 11], {x, 0, 1}]
```

[绘图](#)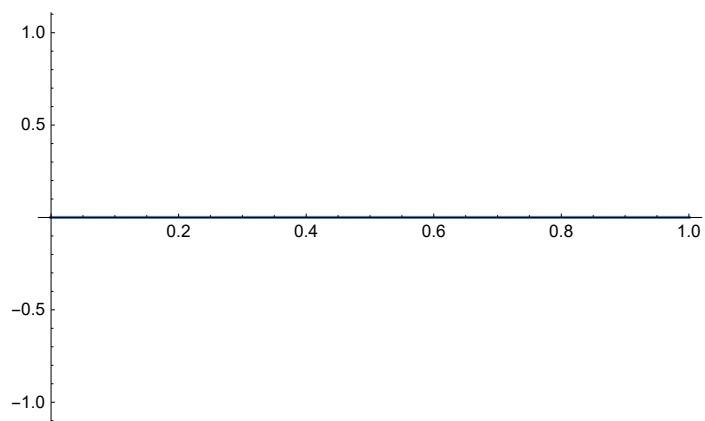

In[44]:= **Plot[Cf[14, 12, 10], {x, 0, 1}]**

[绘图](#)

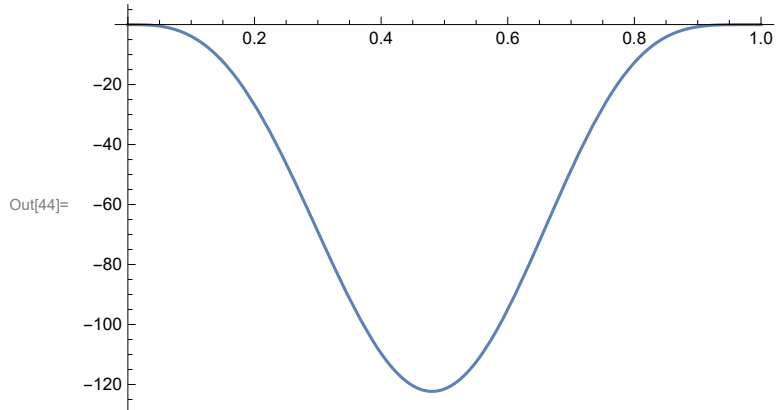

In[45]:= **Plot[Cf[14, 12, 9], {x, 0, 1}]**

[绘图](#)

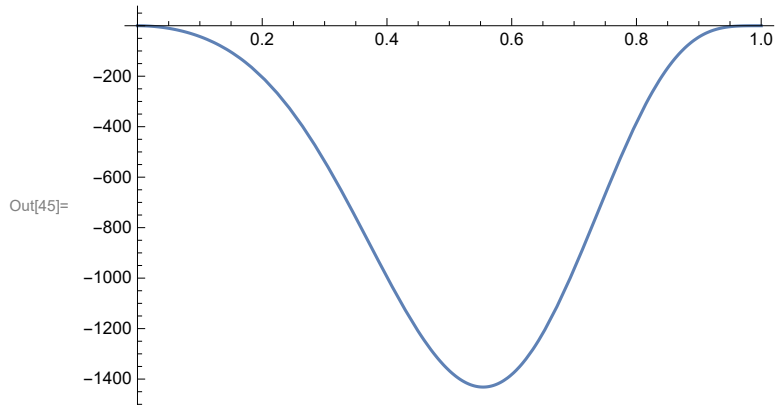

In[46]:= **Plot[Cf[14, 12, 8], {x, 0, 1}]**

[绘图](#)

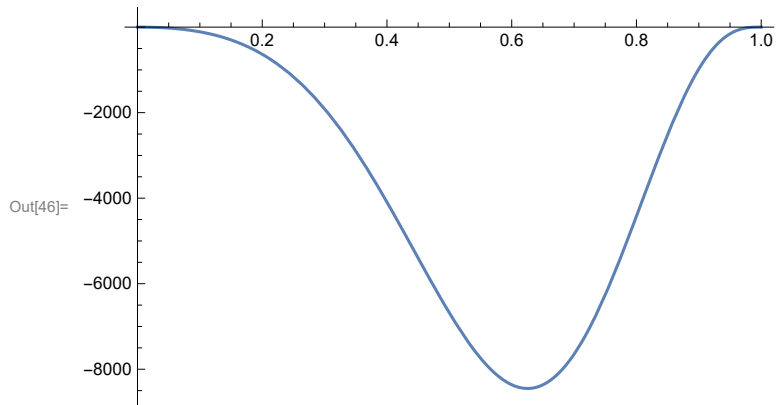

In[47]:= **Plot[Cf[14, 12, 7], {x, 0, 1}]**

[绘图](#)

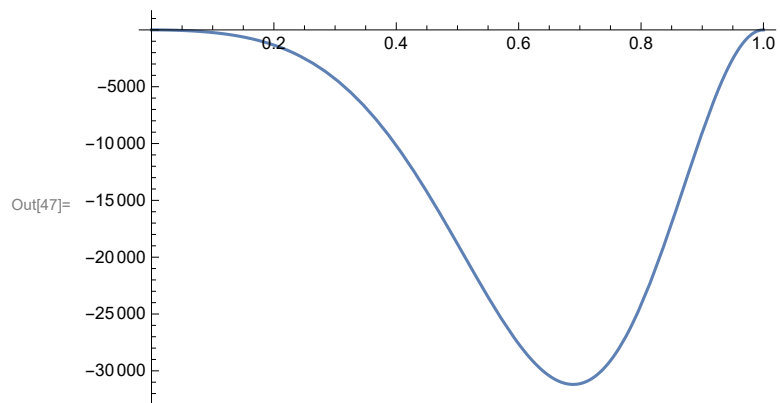

In[48]:= **Plot[Cf[14, 12, 6], {x, 0, 1}]**

[绘图](#)

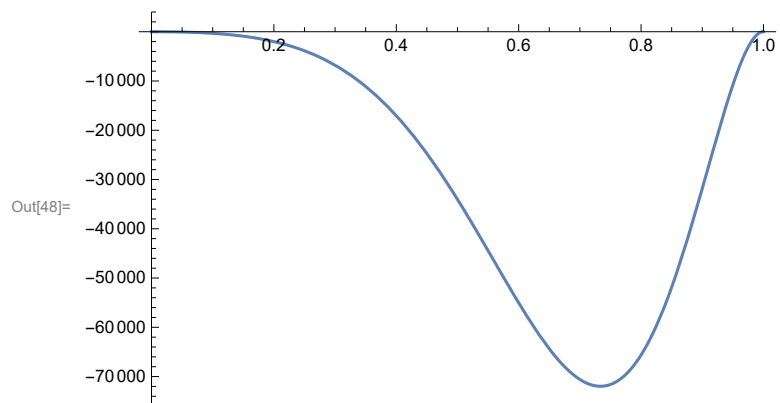

In[49]:= **Plot[Cf[14, 12, 5], {x, 0, 1}]**

[绘图](#)

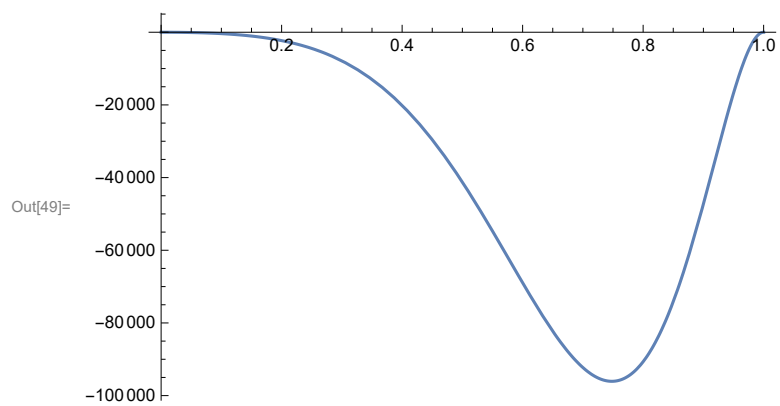

In[50]:= **Plot[Cf[14, 12, 4], {x, 0, 1}]**

[绘图](#)

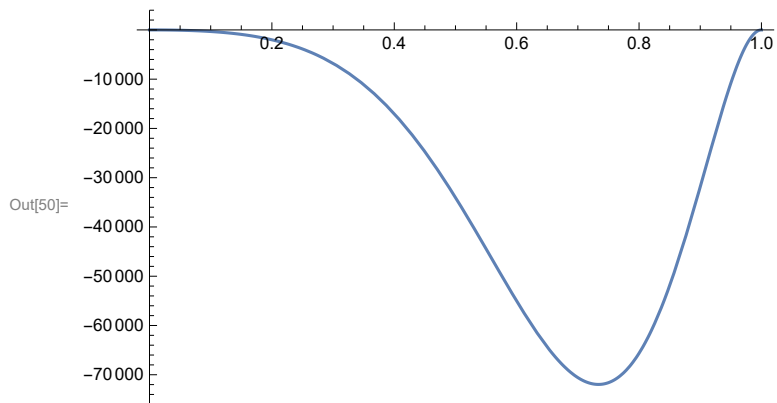

In[51]:= **Plot[Cf[14, 12, 3], {x, 0, 1}]**

[绘图](#)

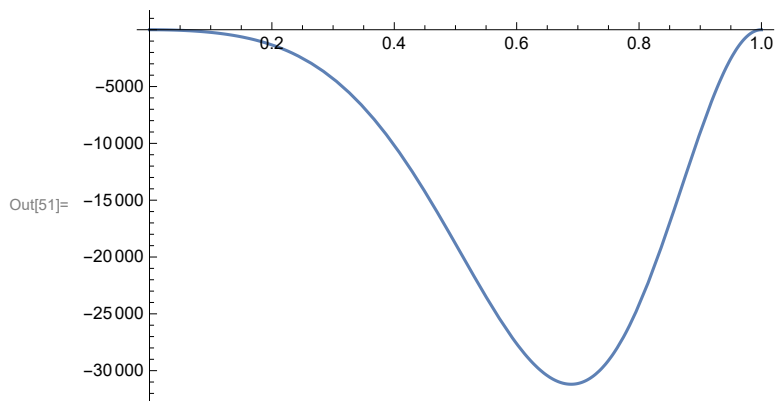

In[52]:= **Plot[Cf[14, 12, 2], {x, 0, 1}]**

[绘图](#)

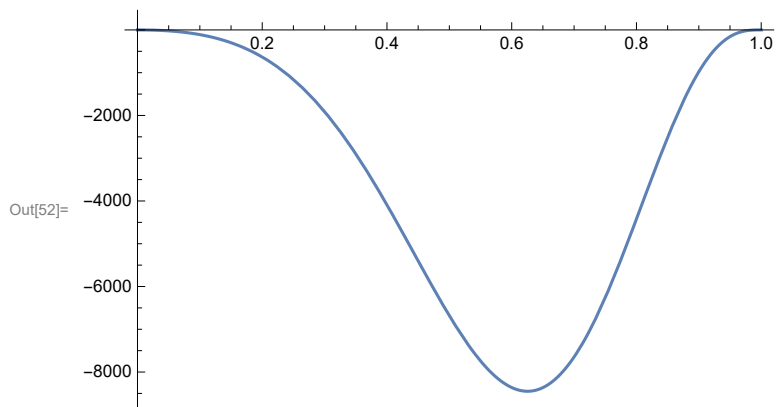

In[53]:= **Plot[Cf[14, 12, 1], {x, 0, 1}]**

[绘图](#)

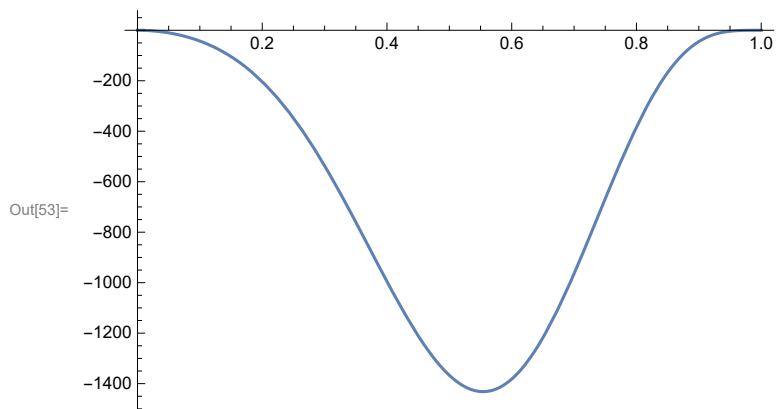

In[54]:= **Plot[Cf[14, 12, 0], {x, 0, 1}]**

[绘图](#)

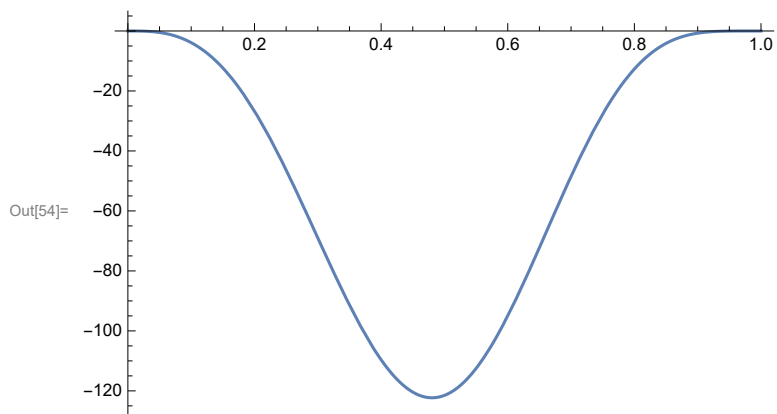

(\*4th group coefficients  $r^2^{14}r^3^{11}$ \*)

**Plot[Cf[14, 11, 14], {x, 0, 1}]**

[绘图](#)

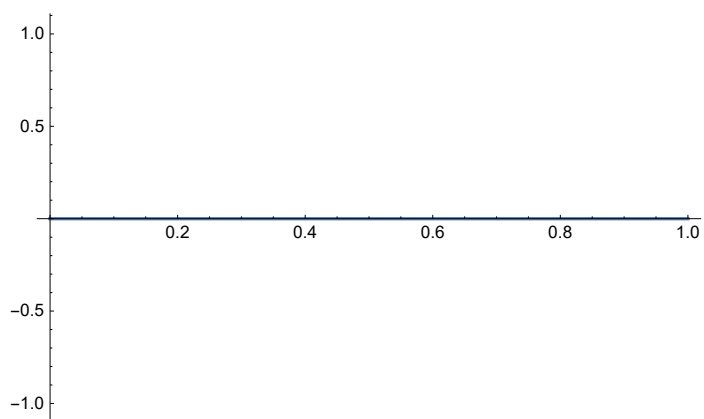



**Plot[Cf[14, 11, 13], {x, 0, 1}]**

[绘图](#)

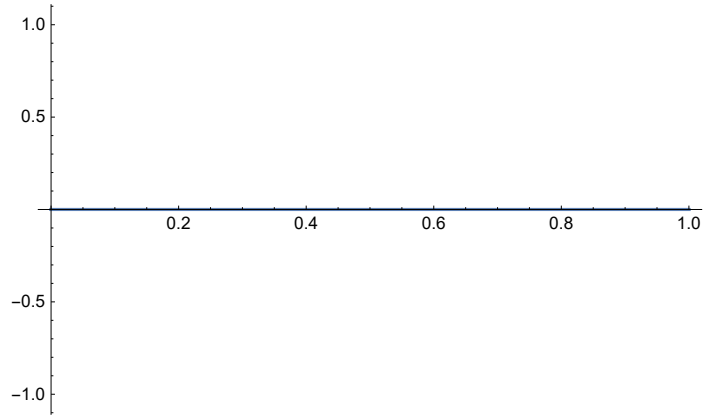

**Plot[Cf[14, 11, 12], {x, 0, 1}]**

[绘图](#)

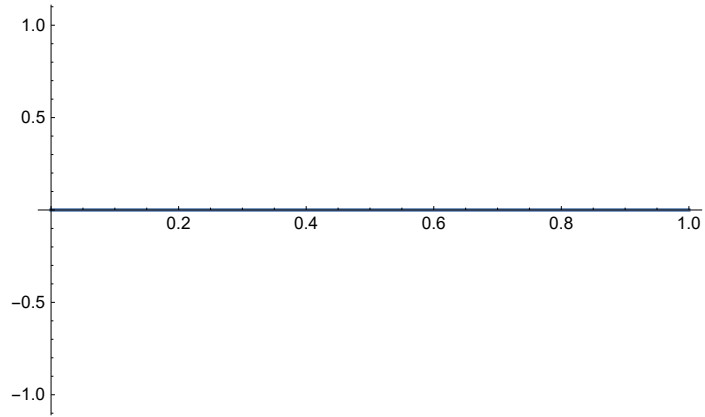

In[55]:= **Plot[Cf[14, 11, 11], {x, 0, 1}]**

[绘图](#)

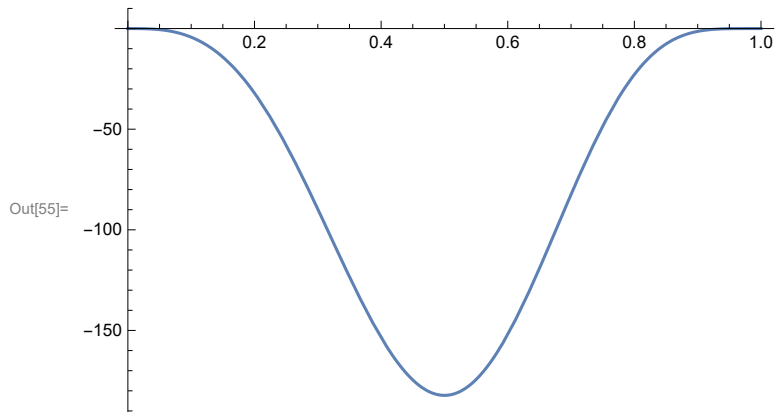

In[56]:= **Plot[Cf[14, 11, 10], {x, 0, 1}]**

[绘图](#)

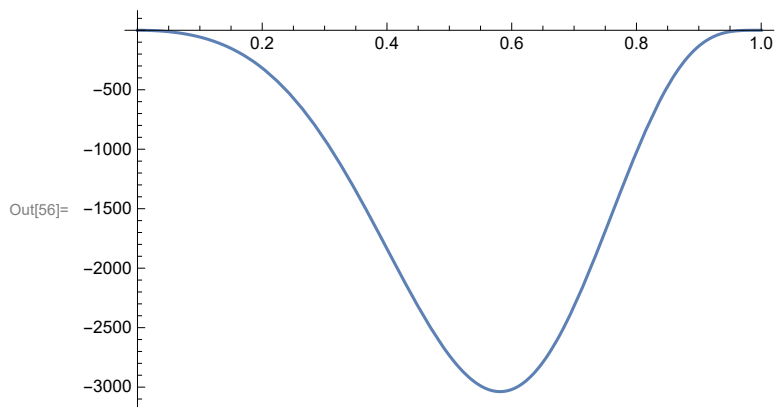

In[57]:= **Plot[Cf[14, 11, 9], {x, 0, 1}]**

[绘图](#)

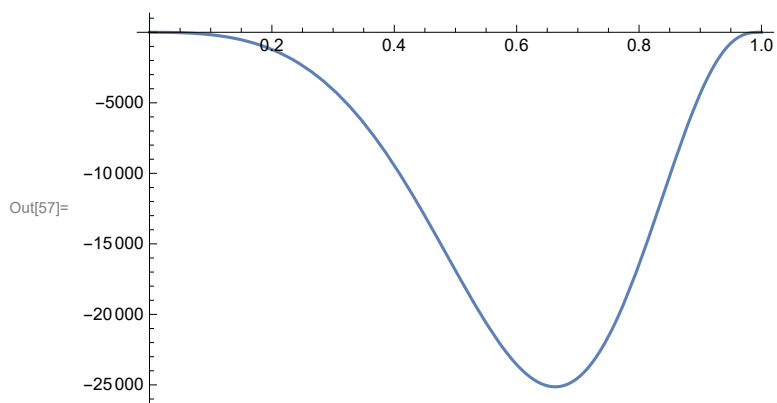

In[58]:= **Plot[Cf[14, 11, 8], {x, 0, 1}]**

[绘图](#)

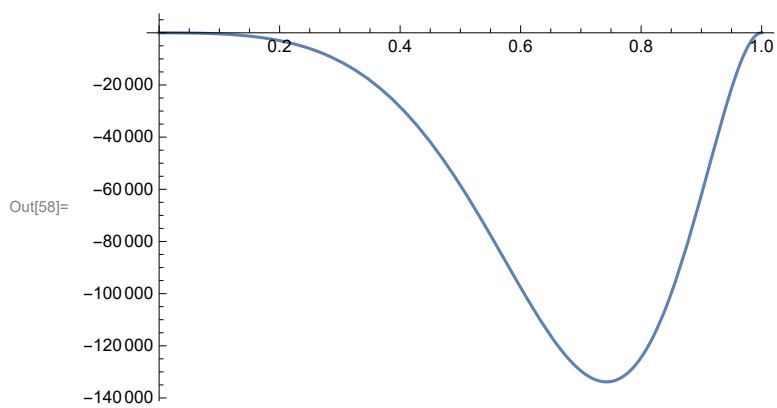

In[59]:= **Plot[Cf[14, 11, 7], {x, 0, 1}]**

[绘图](#)

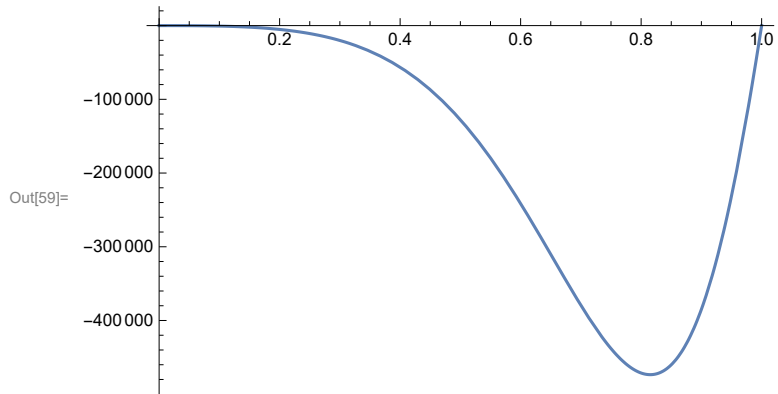

In[60]:= **Plot[Cf[14, 11, 6], {x, 0, 1}]**

[绘图](#)

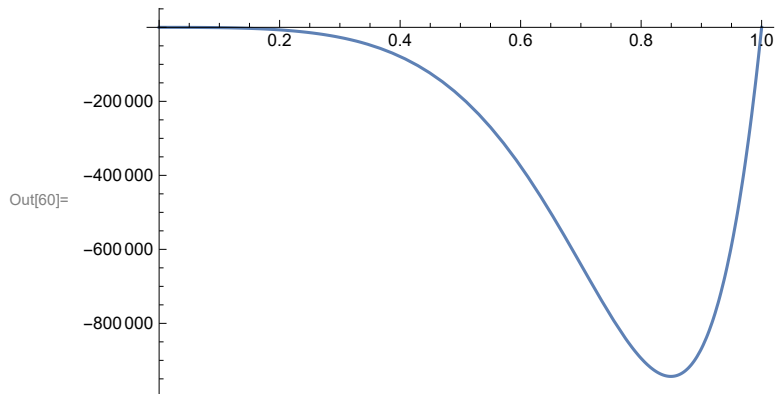

In[61]:= **Plot[Cf[14, 11, 5], {x, 0, 1}]**

[绘图](#)

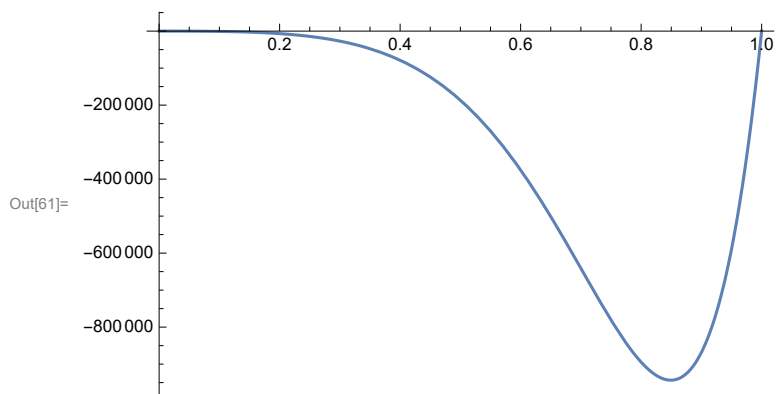

In[62]:= **Plot[Cf[14, 11, 4], {x, 0, 1}]**

[绘图](#)

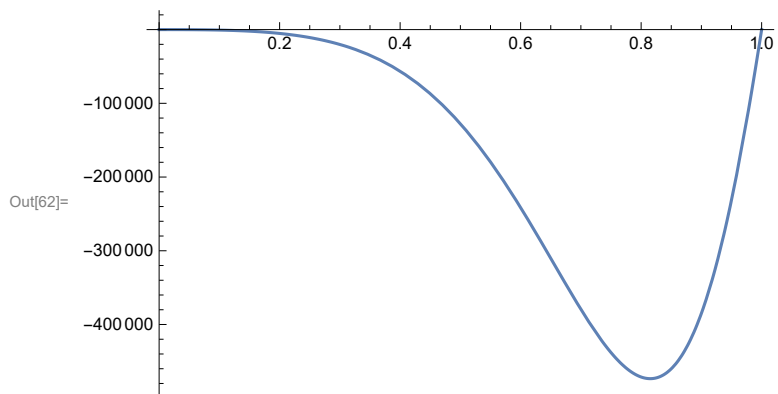

In[63]:= **Plot[Cf[14, 11, 3], {x, 0, 1}]**

[绘图](#)

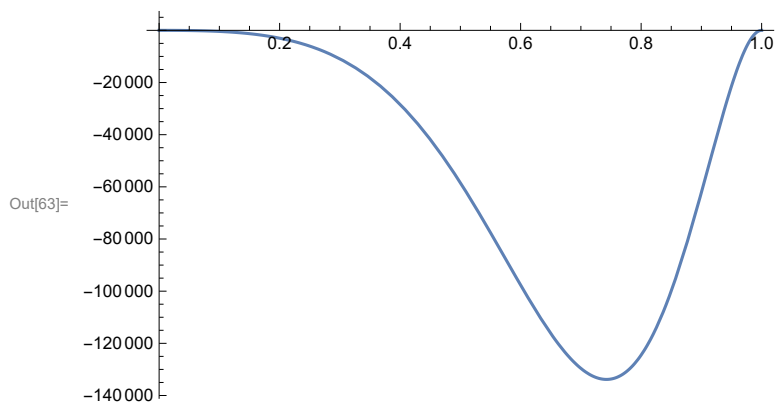

In[65]:= **Plot[Cf[14, 11, 2], {x, 0, 1}]**

[绘图](#)

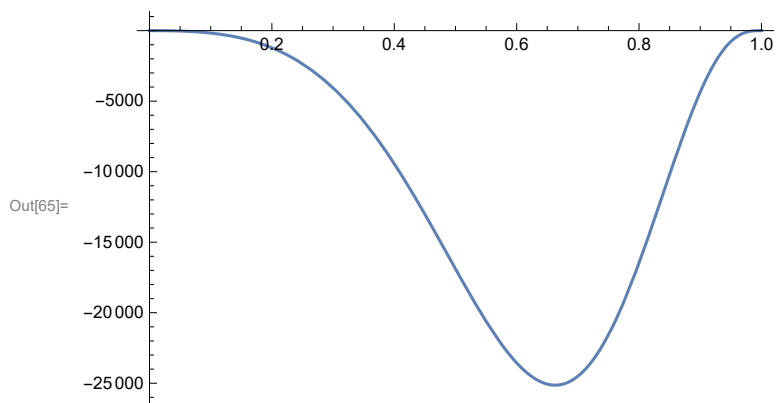

In[66]:= **Plot[Cf[14, 11, 1], {x, 0, 1}]**

[绘图](#)

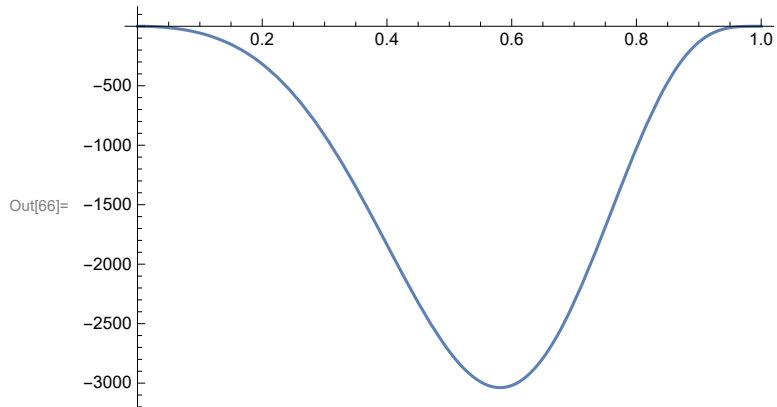

In[67]:= **Plot[Cf[14, 11, 0], {x, 0, 1}]**

[绘图](#)

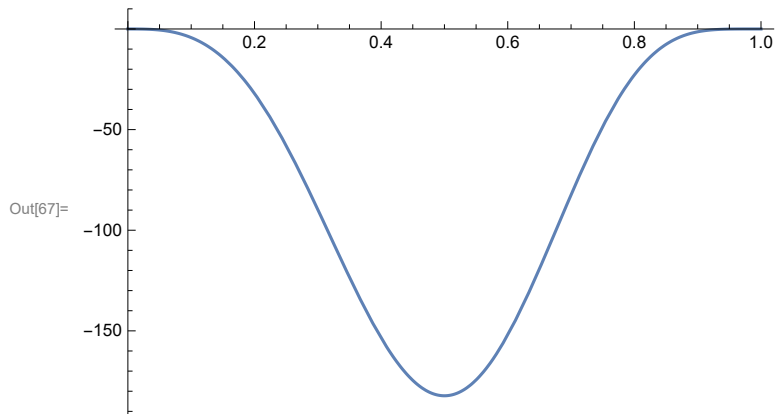

(\*5th group coefficients  $r^2^{14}r^3^{10}$ \*)

**Plot[Cf[14, 10, 14], {x, 0, 1}]**

[绘图](#)

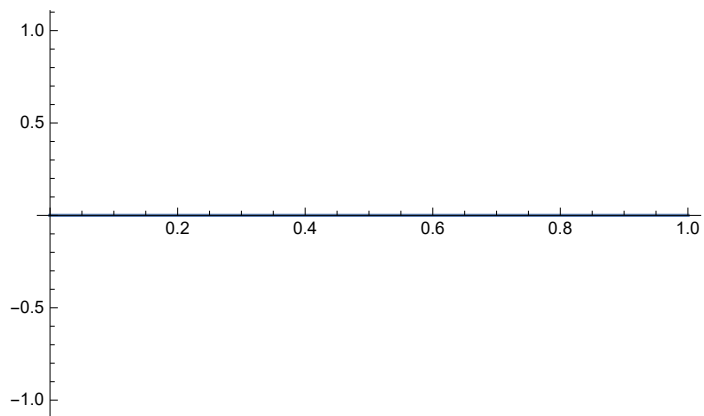

```
Plot[Cf[14, 10, 13], {x, 0, 1}]
```

[绘图](#)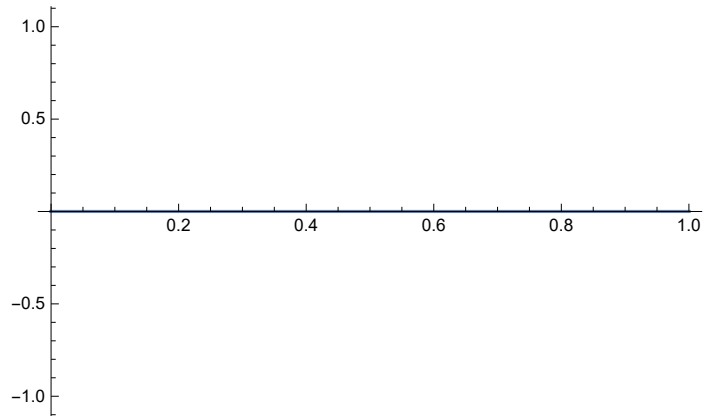

```
In[69]:= Plot[Cf[14, 10, 12], {x, 0, 1}]
```

[绘图](#)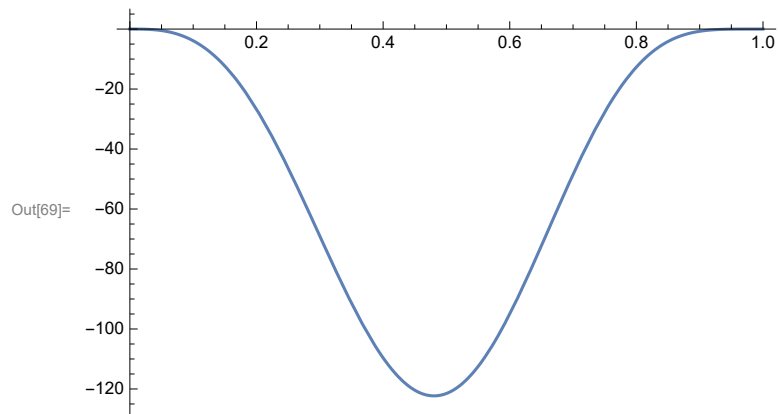

```
In[68]:= Plot[Cf[14, 10, 11], {x, 0, 1}]
```

[绘图](#)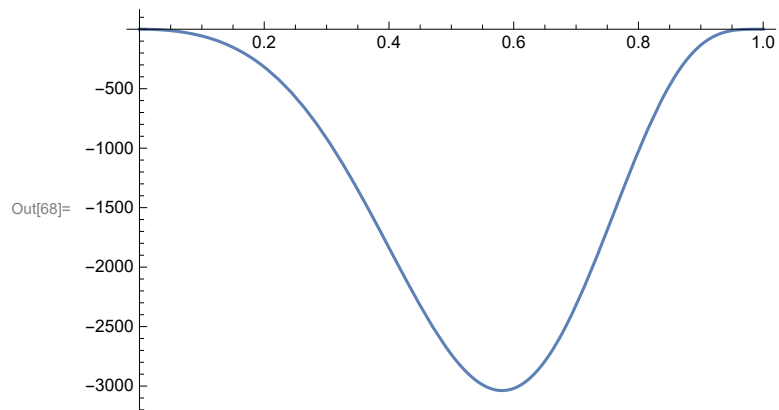

In[70]:= **Plot[Cf[14, 10, 10], {x, 0, 1}]**

[绘图](#)

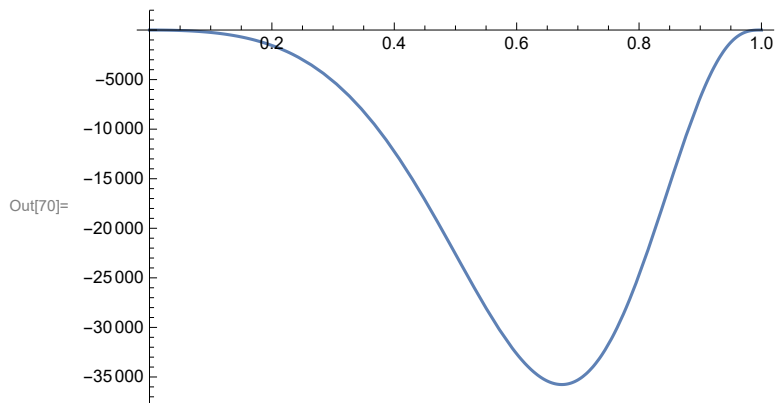

In[71]:= **Plot[Cf[14, 10, 9], {x, 0, 1}]**

[绘图](#)

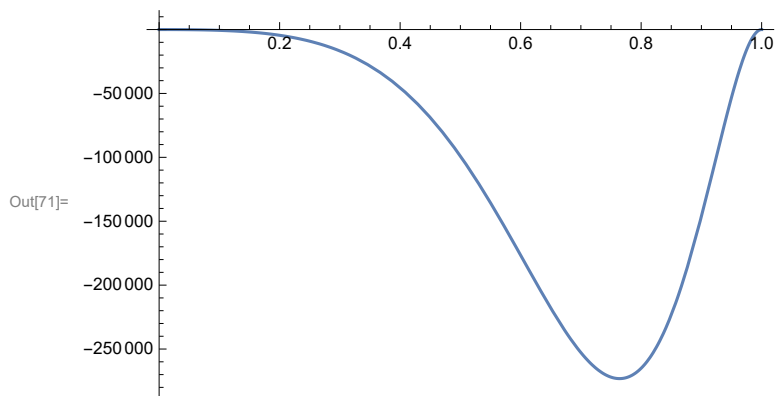

In[72]:= **Plot[Cf[14, 10, 8], {x, 0, 1}]**

[绘图](#)

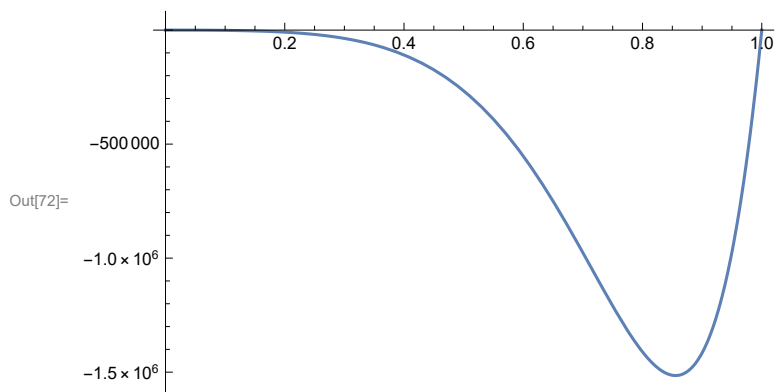

In[73]:= **Plot[Cf[14, 10, 7], {x, 0, 1}]**

[绘图](#)

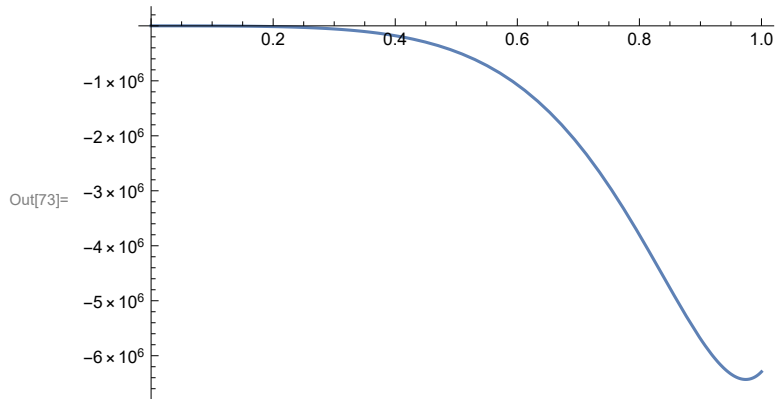

In[74]:= **Plot[Cf[14, 10, 6], {x, 0, 1}]**

[绘图](#)

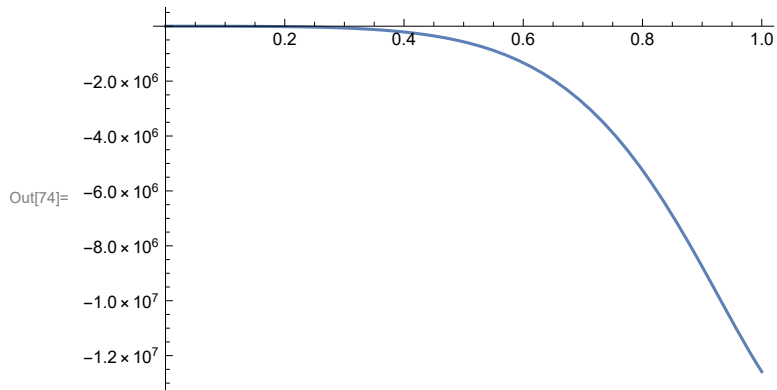

In[75]:= **Plot[Cf[14, 10, 5], {x, 0, 1}]**

[绘图](#)

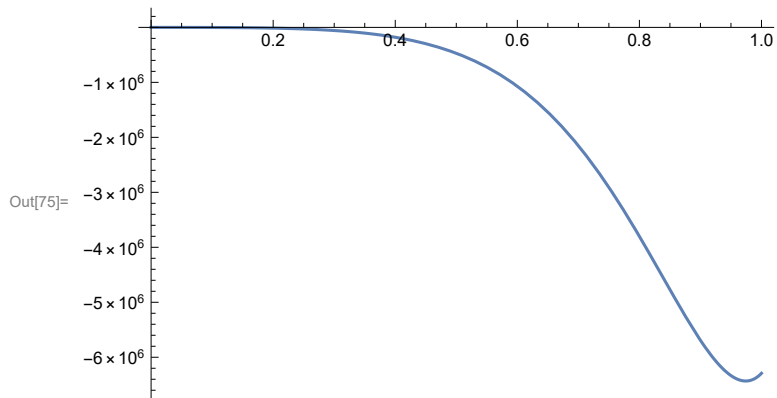



In[76]:= **Plot[Cf[14, 10, 4], {x, 0, 1}]**

[绘图](#)

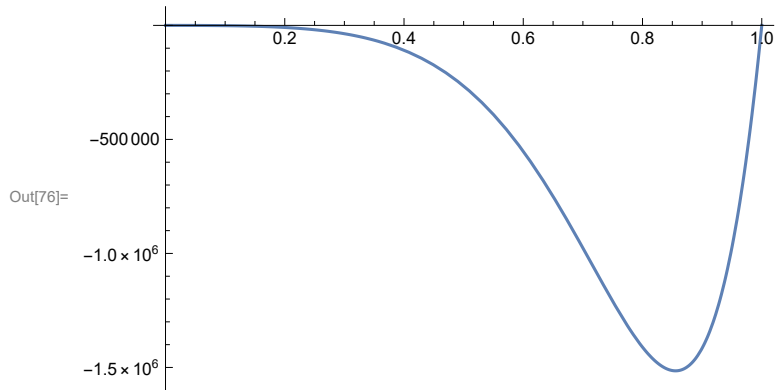

In[77]:= **Plot[Cf[14, 10, 3], {x, 0, 1}]**

[绘图](#)

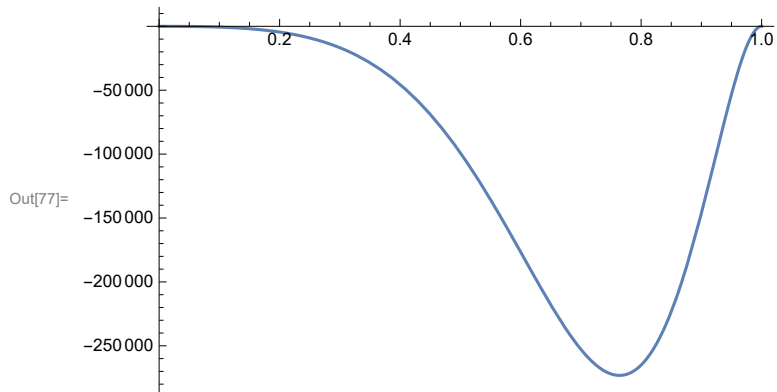

In[78]:= **Plot[Cf[14, 10, 2], {x, 0, 1}]**

[绘图](#)

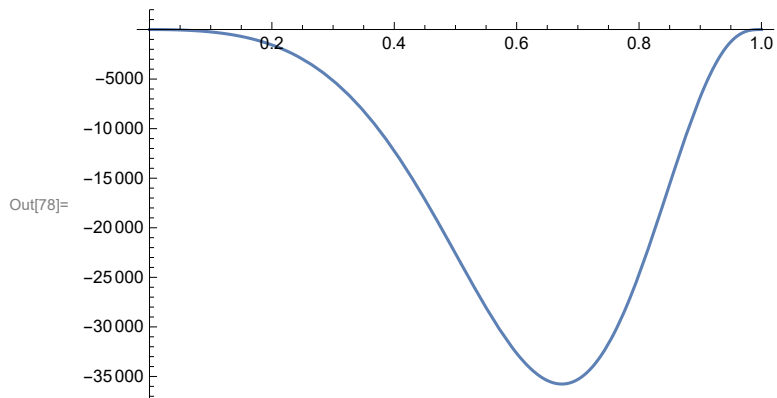

In[79]:= **Plot[Cf[14, 10, 1], {x, 0, 1}]**

[绘图](#)

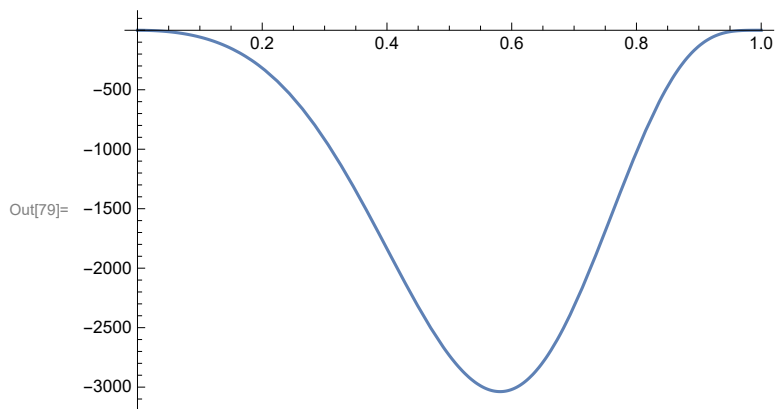

In[80]:= **Plot[Cf[14, 10, 0], {x, 0, 1}]**

[绘图](#)

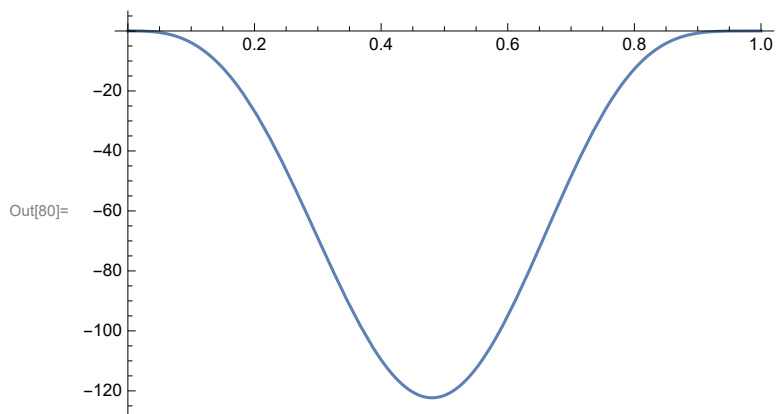

(\*6th group coefficients r2^14r3^9\*)

**Plot[Cf[14, 9, 14], {x, 0, 1}]**

[绘图](#)

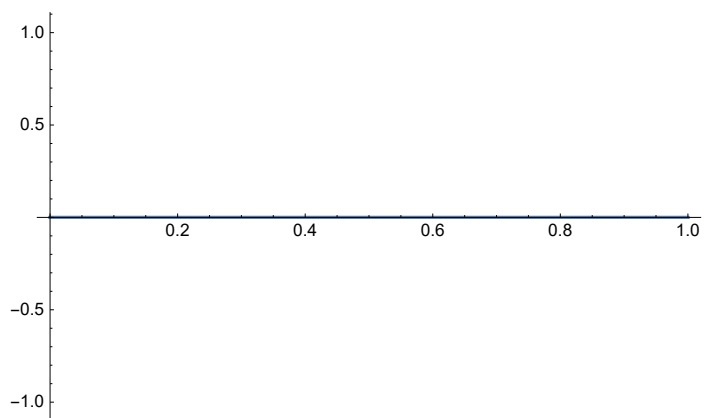

In[81]:= **Plot[Cf[14, 9, 13], {x, 0, 1}]**

[绘图](#)

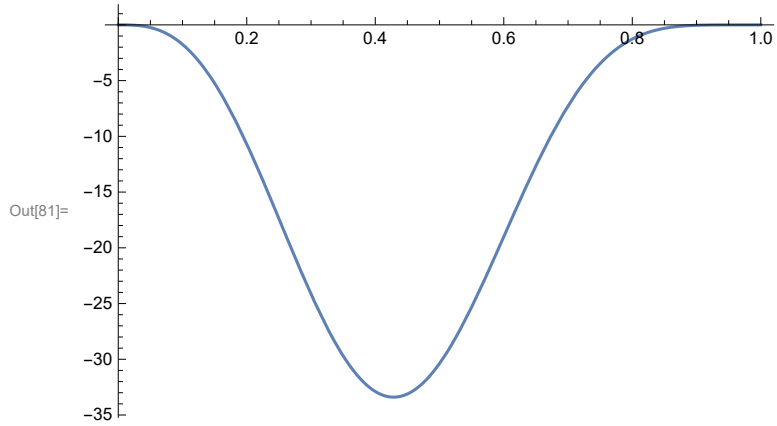

In[84]:= **Plot[Cf[14, 9, 12], {x, 0, 1}]**

[绘图](#)

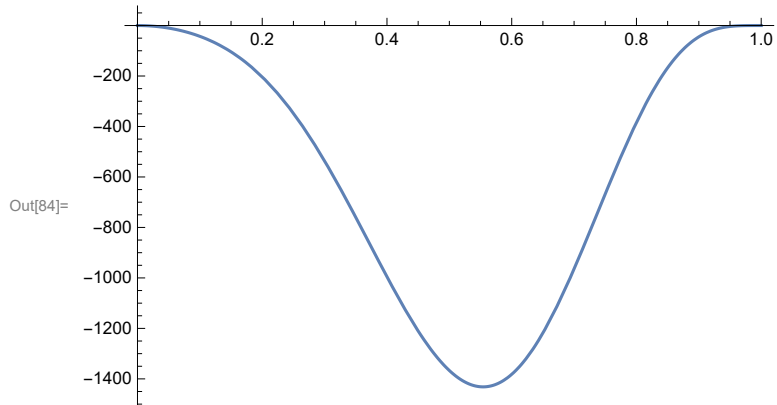

In[82]:= **Plot[Cf[14, 9, 11], {x, 0, 1}]**

[绘图](#)

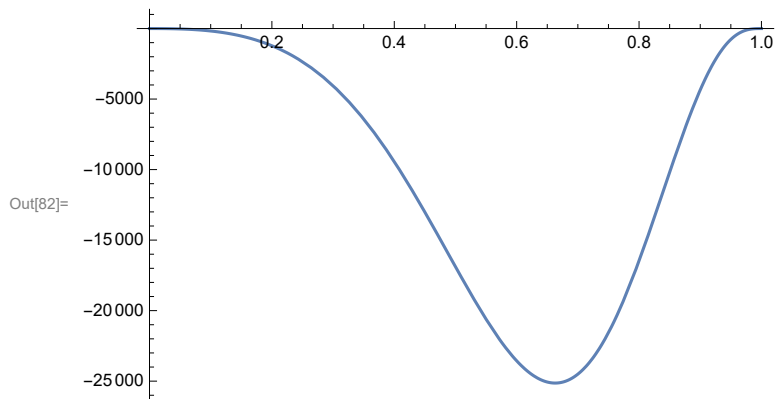

In[83]:= **Plot[Cf[14, 9, 10], {x, 0, 1}]**

[绘图](#)

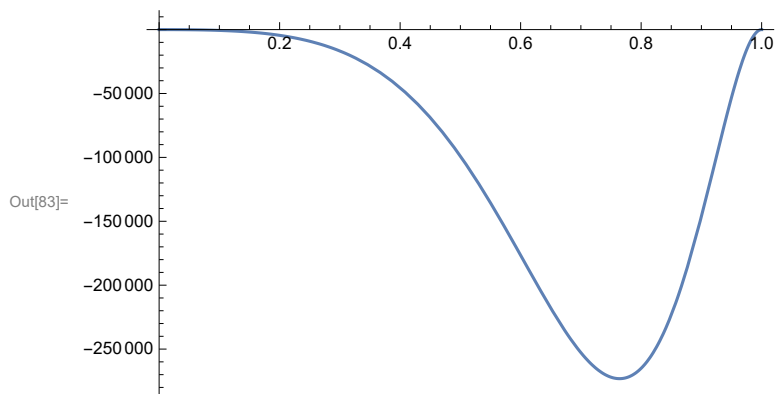

In[85]:= **Plot[Cf[14, 9, 9], {x, 0, 1}]**

[绘图](#)

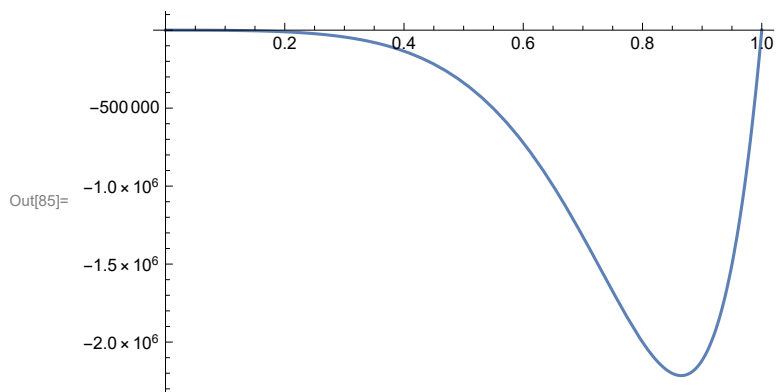

In[87]:= **Plot[Cf[14, 9, 8], {x, 0, 1}]**

[绘图](#)

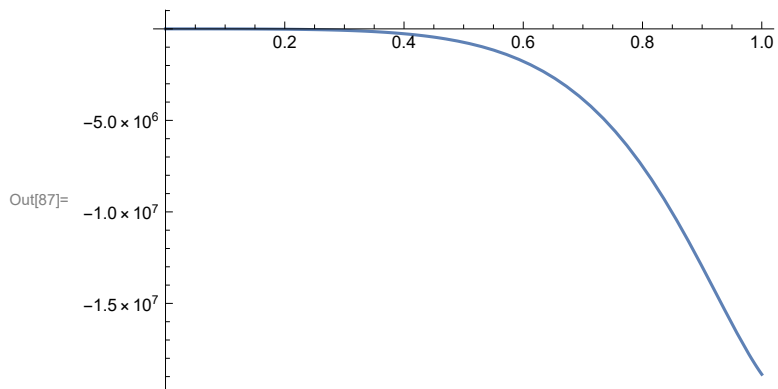

In[88]:= **Plot[Cf[14, 9, 7], {x, 0, 1}]**

[绘图](#)

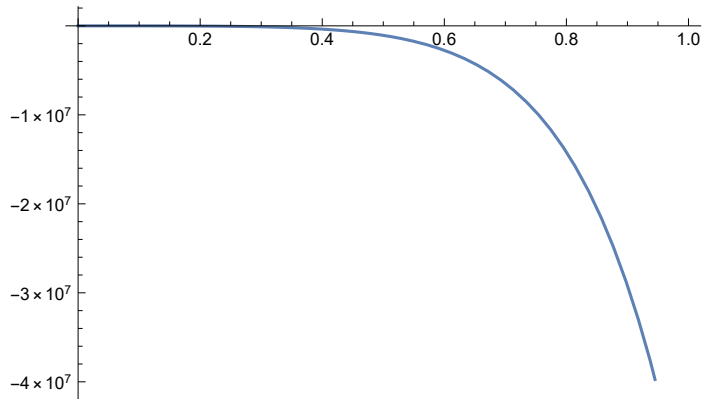

In[89]:= **Plot[Cf[14, 9, 6], {x, 0, 1}]**

[绘图](#)

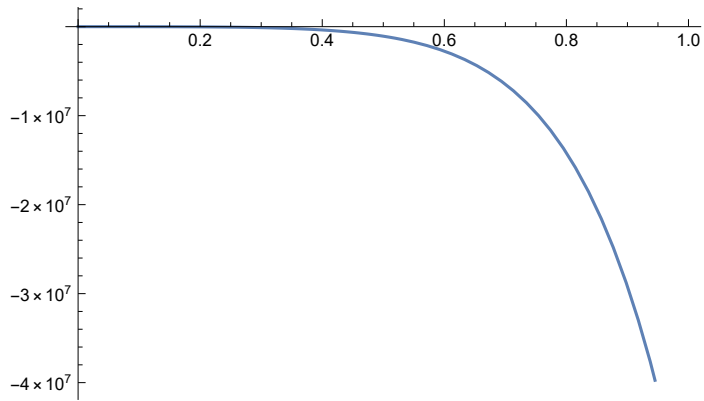

In[90]:= **Plot[Cf[14, 9, 5], {x, 0, 1}]**

[绘图](#)

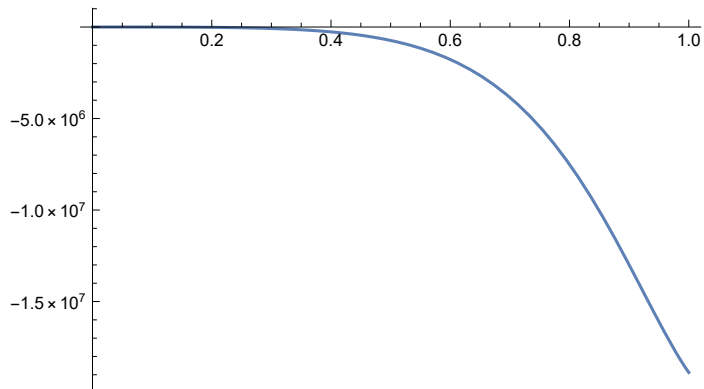

In[91]:= **Plot[Cf[14, 9, 4], {x, 0, 1}]**

[绘图](#)

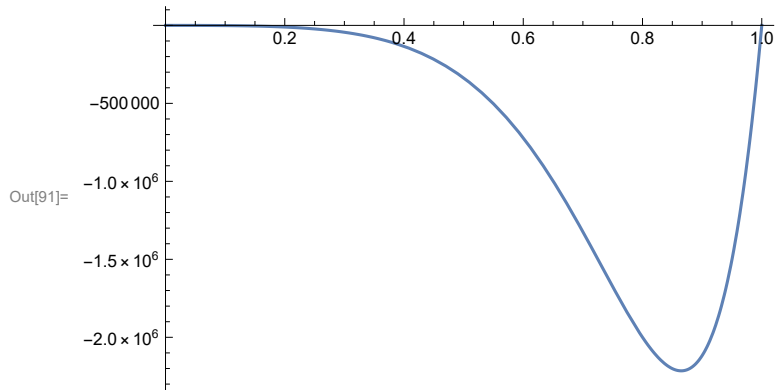

In[92]:= **Plot[Cf[14, 9, 3], {x, 0, 1}]**

[绘图](#)

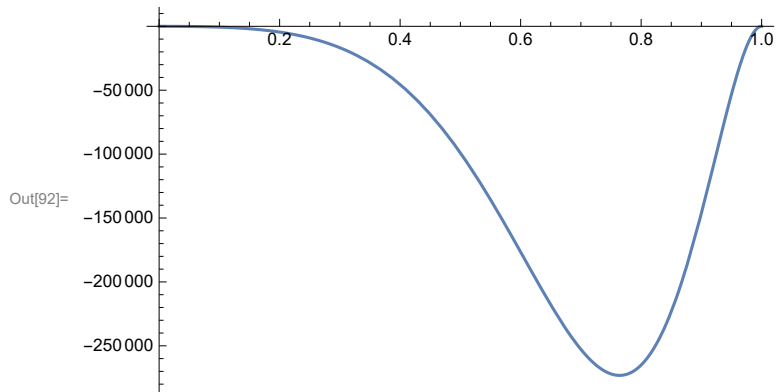

In[93]:= **Plot[Cf[14, 9, 2], {x, 0, 1}]**

[绘图](#)

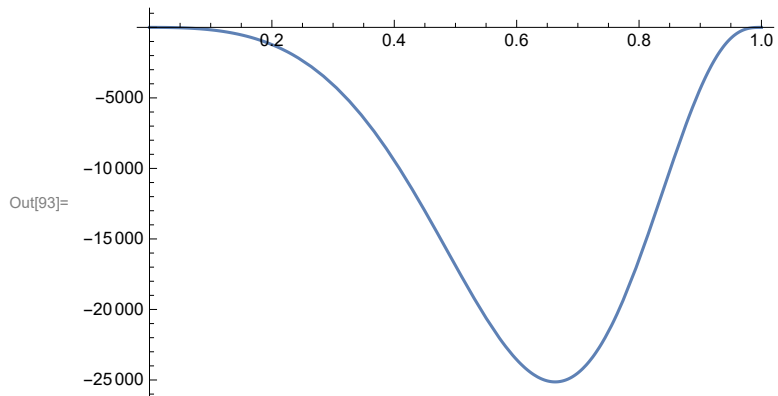

In[94]:= **Plot[Cf[14, 9, 1], {x, 0, 1}]**

[绘图](#)

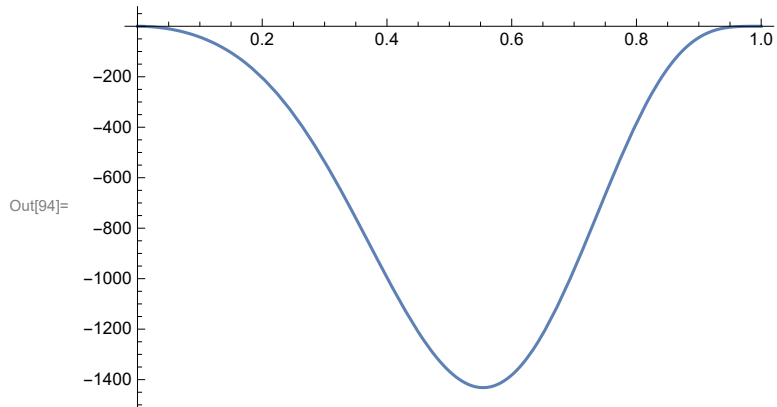

In[95]:= **Plot[Cf[14, 9, 0], {x, 0, 1}]**

[绘图](#)

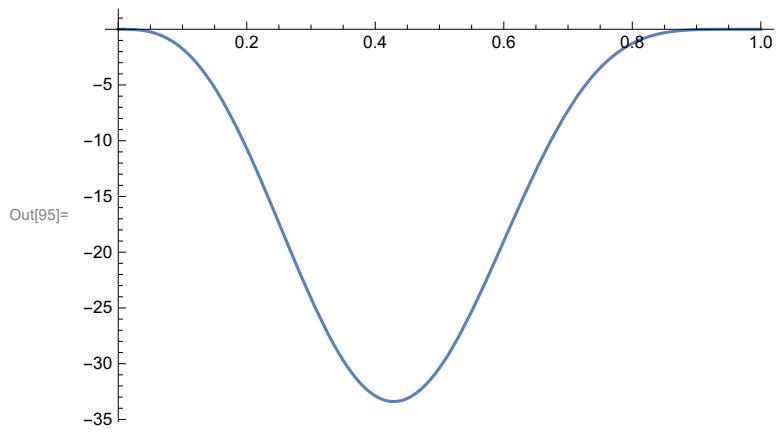

(\*7th group coefficients  $r_2^{14}r_3^8$ \*)

**Plot[Cf[14, 8, 14], {x, 0, 1}]**

[绘图](#)

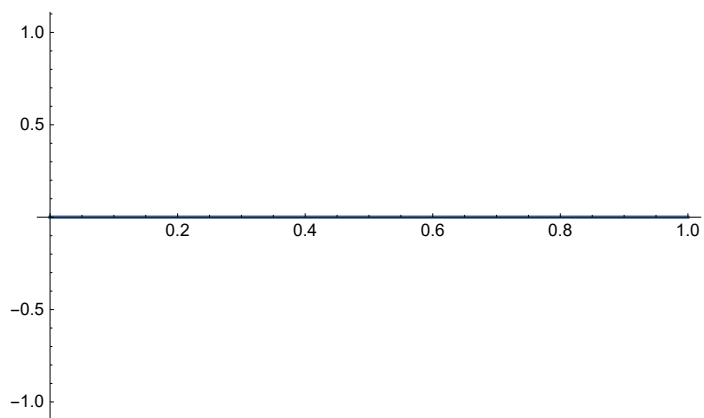

In[96]:= **Plot[Cf[14, 8, 13], {x, 0, 1}]**

[绘图](#)

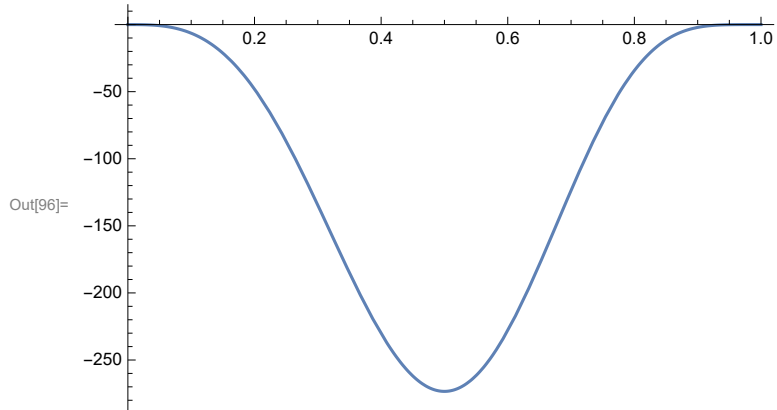

In[97]:= **Plot[Cf[14, 8, 12], {x, 0, 1}]**

[绘图](#)

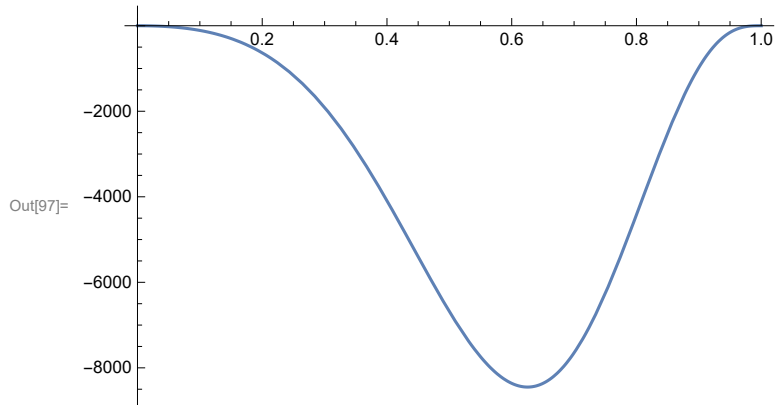

In[98]:= **Plot[Cf[14, 8, 11], {x, 0, 1}]**

[绘图](#)

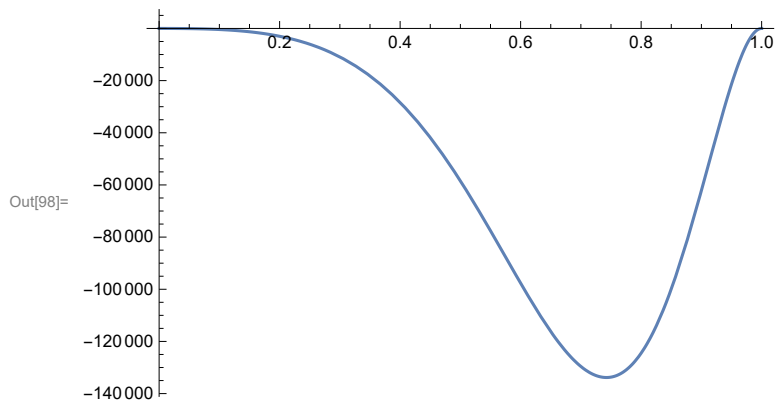



In[99]:= **Plot[Cf[14, 8, 10], {x, 0, 1}]**

[绘图](#)

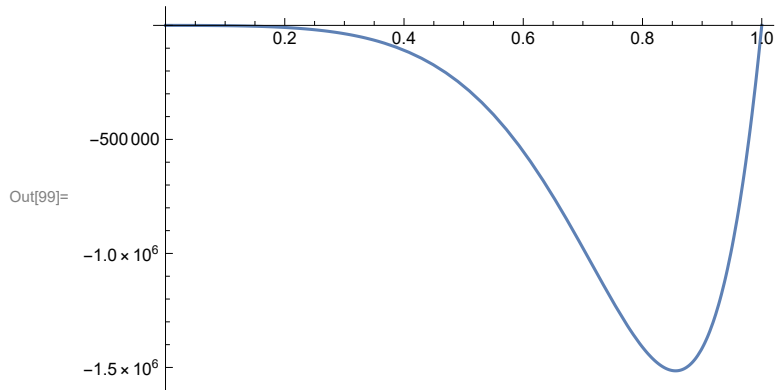

In[100]:= **Plot[Cf[14, 8, 9], {x, 0, 1}]**

[绘图](#)

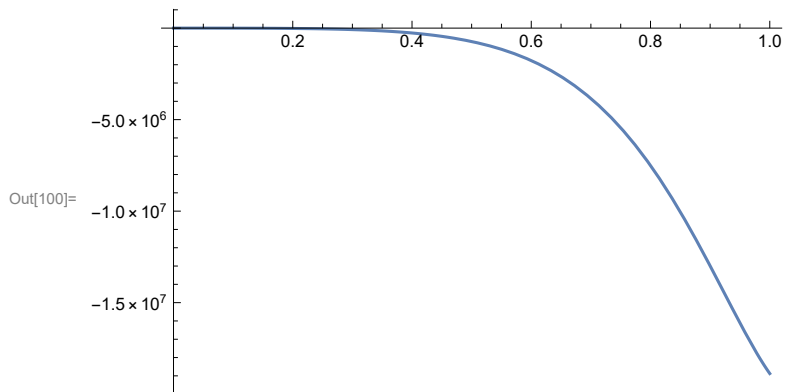

In[101]:= **Plot[Cf[14, 8, 8], {x, 0, 1}]**

[绘图](#)

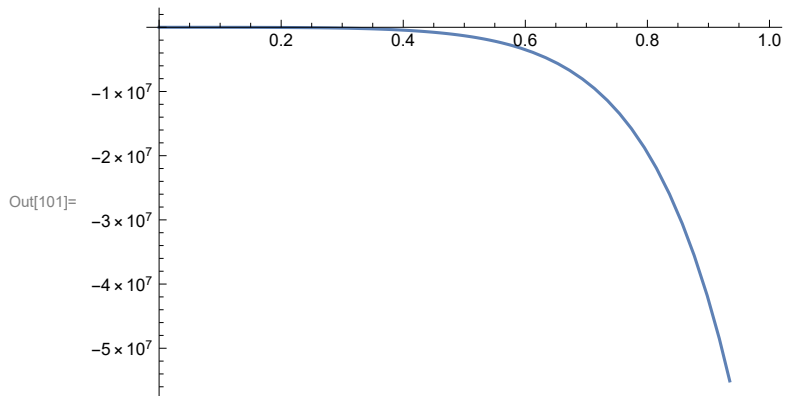

In[102]:= **Plot[Cf[14, 8, 7], {x, 0, 1}]**

[绘图](#)

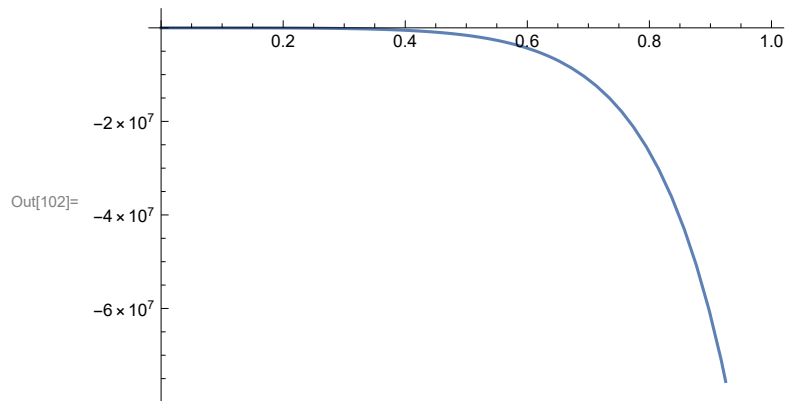

In[103]:= **Plot[Cf[14, 8, 6], {x, 0, 1}]**

[绘图](#)

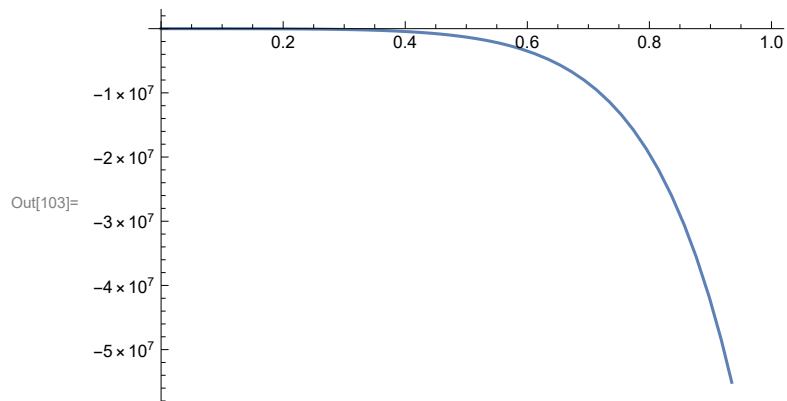

In[104]:= **Plot[Cf[14, 8, 5], {x, 0, 1}]**

[绘图](#)

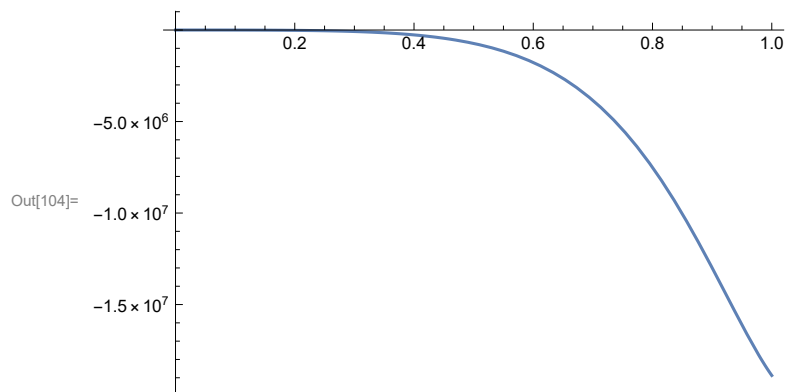

In[105]:= **Plot[Cf[14, 8, 4], {x, 0, 1}]**

[绘图](#)

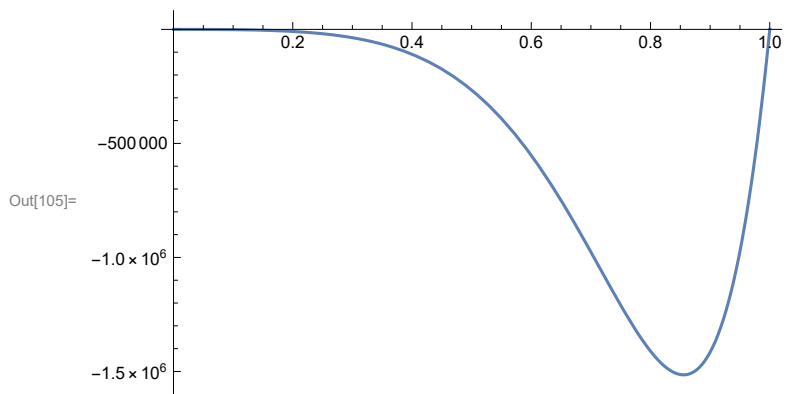

In[106]:= **Plot[Cf[14, 8, 3], {x, 0, 1}]**

[绘图](#)

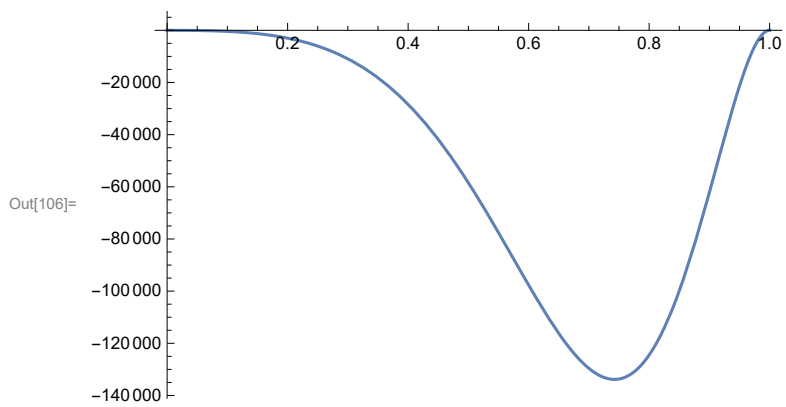

In[108]:= **Plot[Cf[14, 8, 2], {x, 0, 1}]**

[绘图](#)

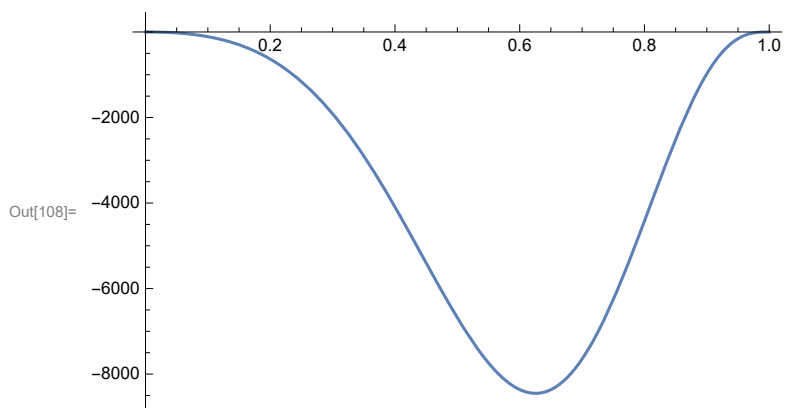

```
In[107]:= Plot[Cf[14, 8, 1], {x, 0, 1}]
```

[绘图](#)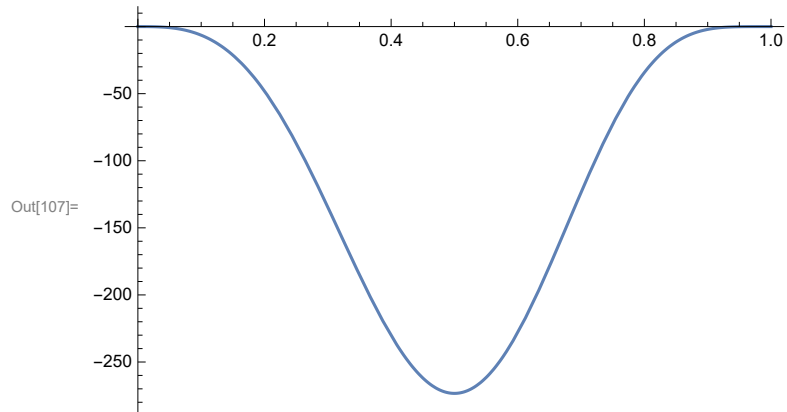

```
Plot[Cf[14, 8, 0], {x, 0, 1}]
```

[绘图](#)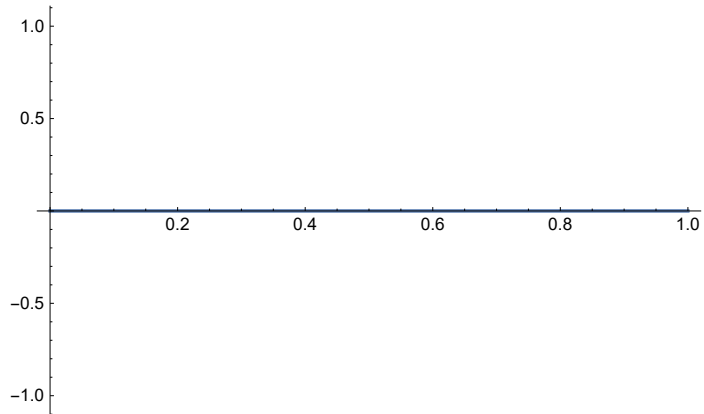

(\*8th group coefficients  $r^2{}^{14}r^3{}^7$ \*)

```
Plot[Cf[14, 7, 14], {x, 0, 1}]
```

[绘图](#)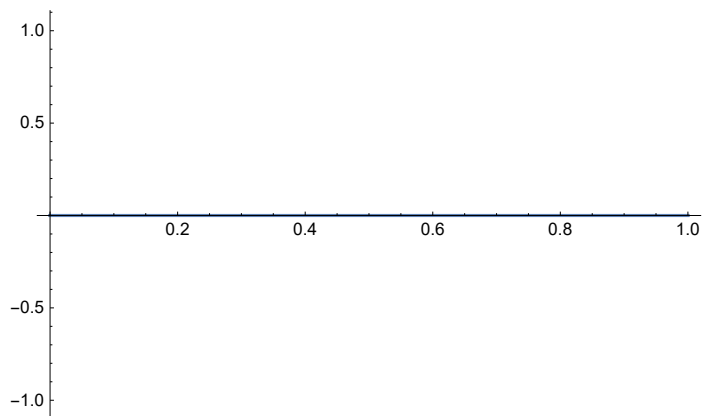

In[109]:= **Plot[Cf[14, 7, 13], {x, 0, 1}]**

[绘图](#)

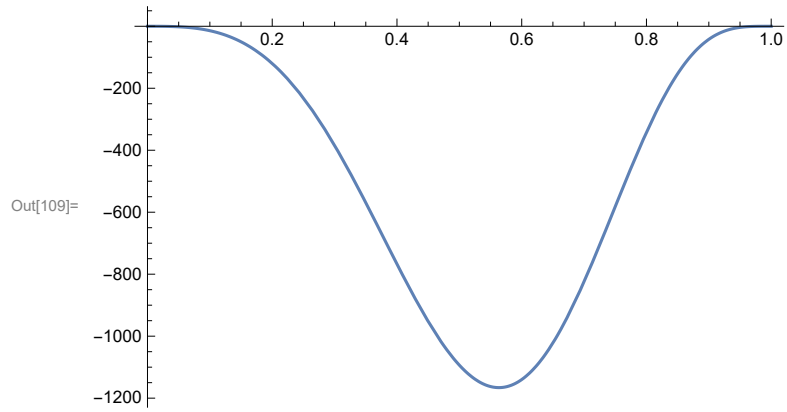

In[110]:= **Plot[Cf[14, 7, 12], {x, 0, 1}]**

[绘图](#)

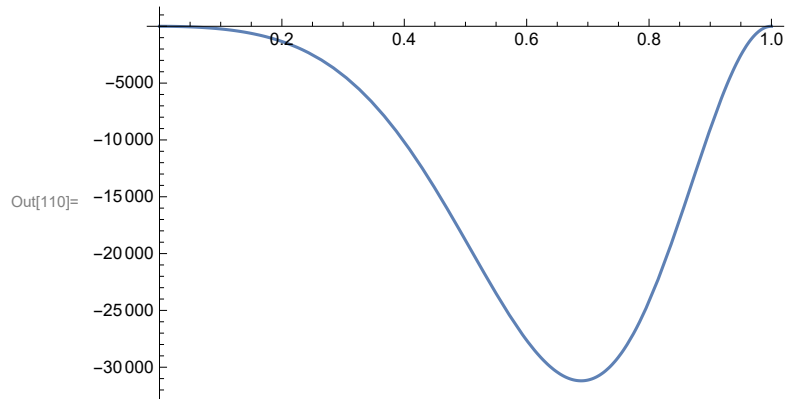

In[111]:= **Plot[Cf[14, 7, 11], {x, 0, 1}]**

[绘图](#)

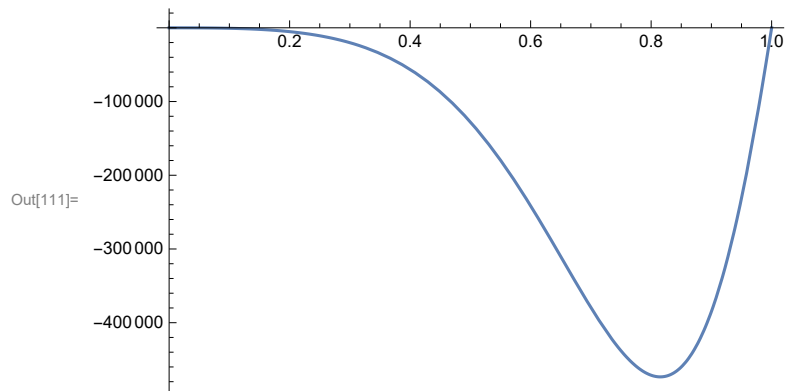

In[112]:= **Plot[Cf[14, 7, 10], {x, 0, 1}]**

[绘图](#)

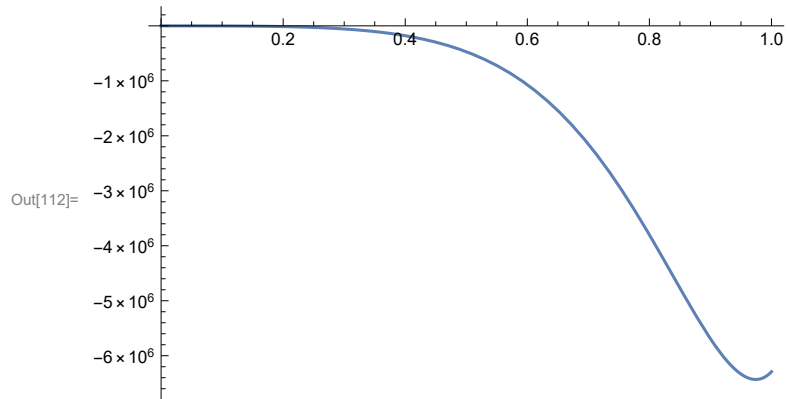

In[113]:= **Plot[Cf[14, 7, 9], {x, 0, 1}]**

[绘图](#)

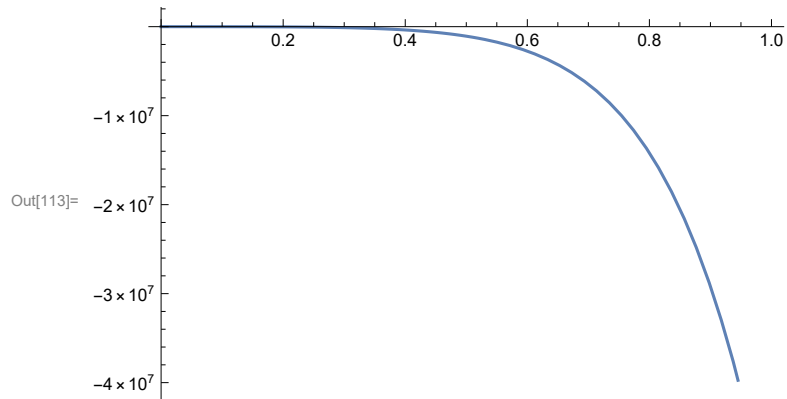

In[114]:= **Plot[Cf[14, 7, 8], {x, 0, 1}]**

[绘图](#)

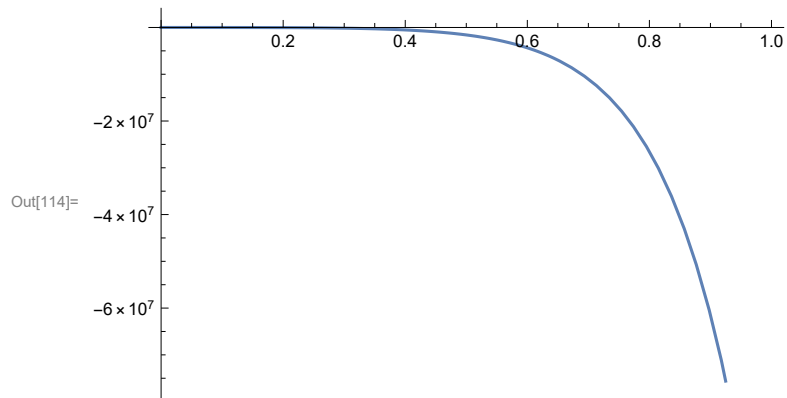

In[115]:= **Plot[Cf[14, 7, 7], {x, 0, 1}]**

[绘图](#)

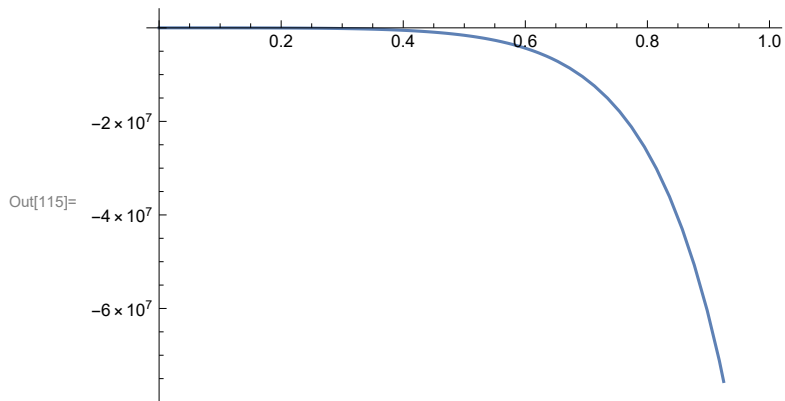

In[116]:= **Plot[Cf[14, 7, 6], {x, 0, 1}]**

[绘图](#)

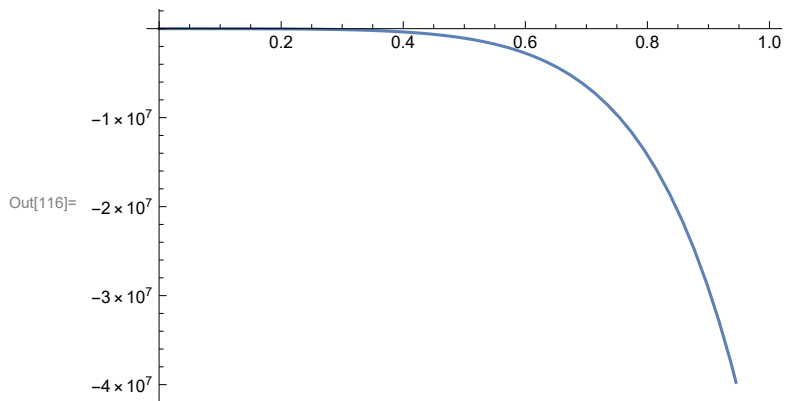

**Plot[Cf[14, 7, 5], {x, 0, 1}]**

[绘图](#)

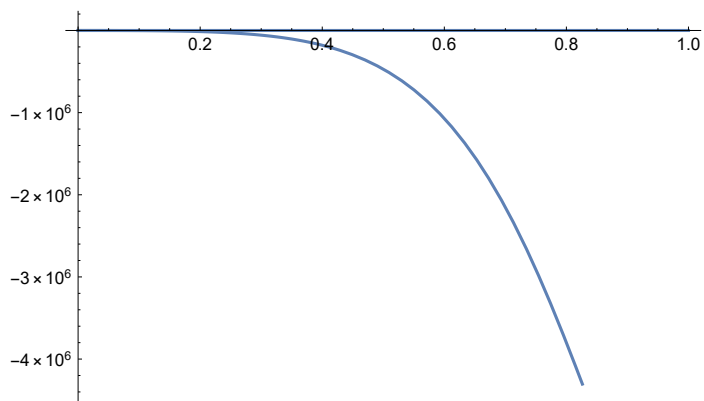

In[117]:= **Plot[Cf[14, 7, 4], {x, 0, 1}]**

[绘图](#)

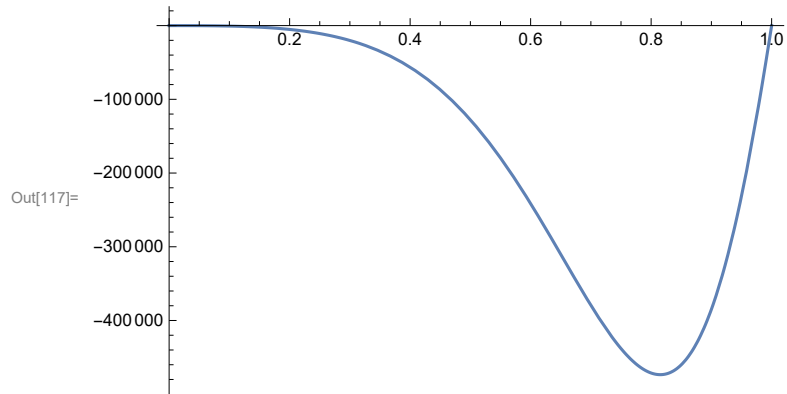

In[118]:= **Plot[Cf[14, 7, 3], {x, 0, 1}]**

[绘图](#)

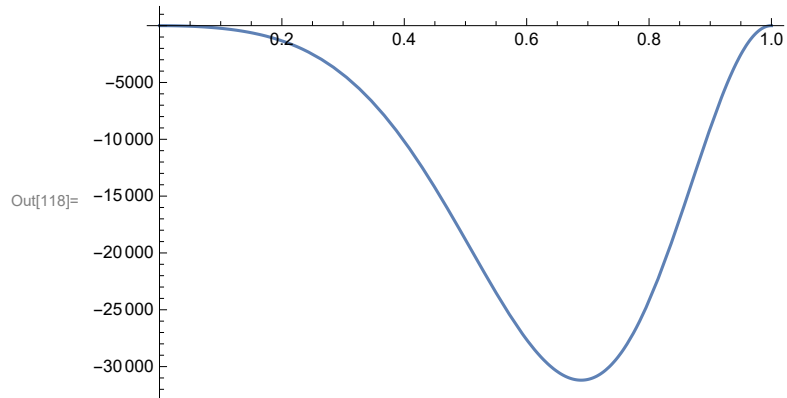

**Plot[Cf[14, 7, 2], {x, 0, 1}]**

[绘图](#)

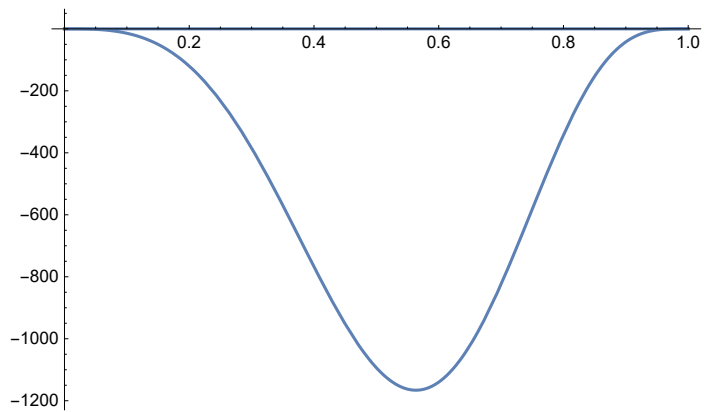



**Plot[Cf[14, 7, 1], {x, 0, 1}]**

[绘图](#)

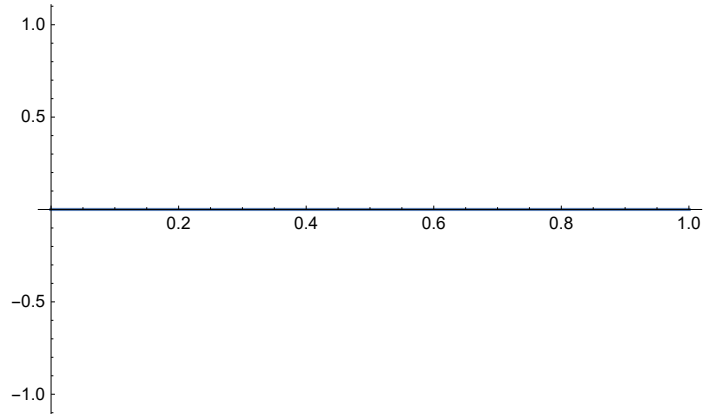

**Plot[Cf[14, 7, 0], {x, 0, 1}]**

[绘图](#)

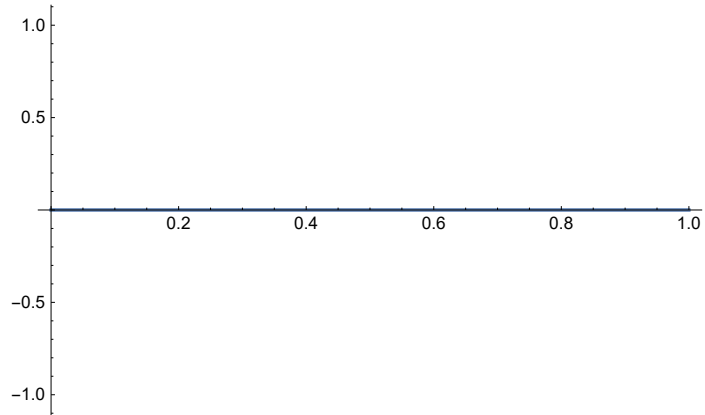

**(\*9th group coefficients r2^14r3^6\*)**

**Plot[Cf[14, 6, 14], {x, 0, 1}]**

[绘图](#)

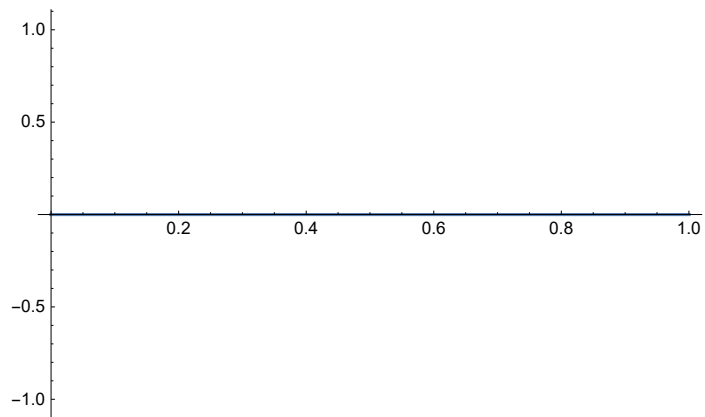

In[119]:= **Plot[Cf[14, 6, 13], {x, 0, 1}]**

[绘图](#)

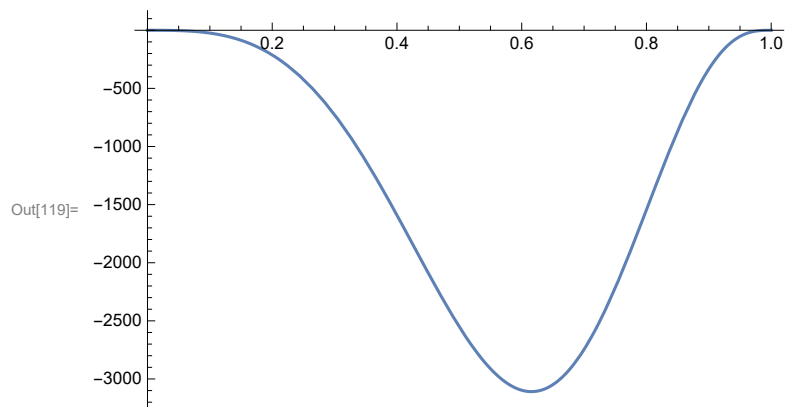

In[120]:= **Plot[Cf[14, 6, 12], {x, 0, 1}]**

[绘图](#)

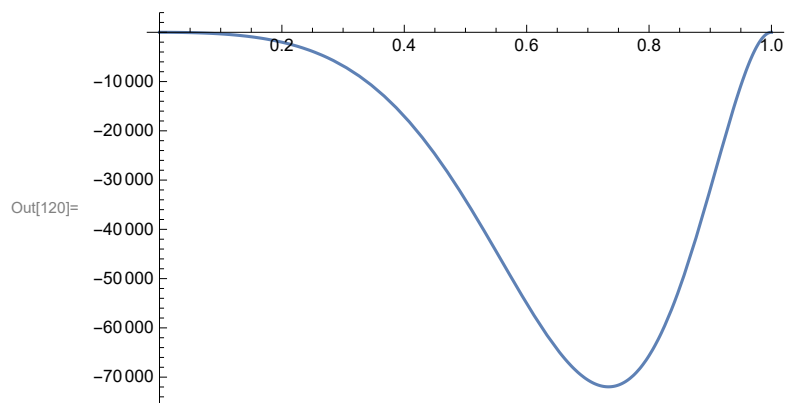

In[121]:= **Plot[Cf[14, 6, 11], {x, 0, 1}]**

[绘图](#)

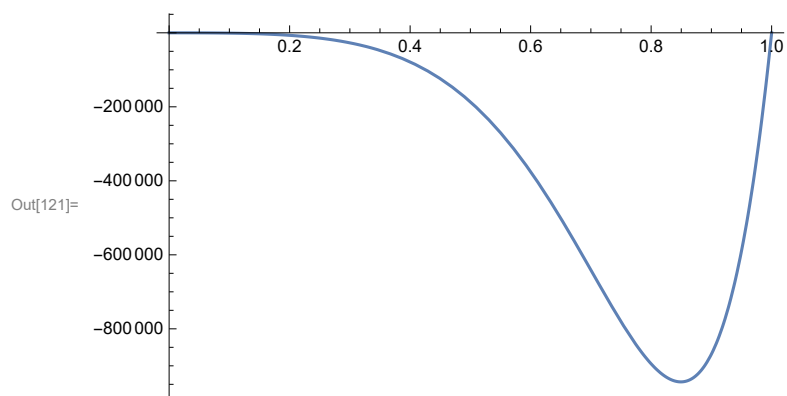

In[122]:= **Plot[Cf[14, 6, 10], {x, 0, 1}]**

[绘图](#)

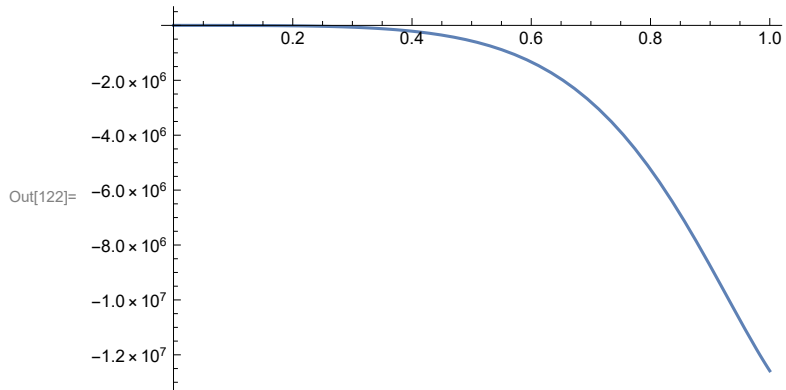

In[123]:= **Plot[Cf[14, 6, 9], {x, 0, 1}]**

[绘图](#)

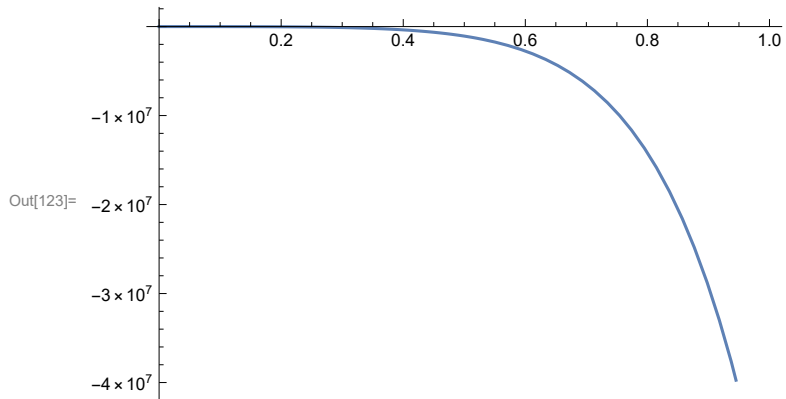

In[124]:= **Plot[Cf[14, 6, 8], {x, 0, 1}]**

[绘图](#)

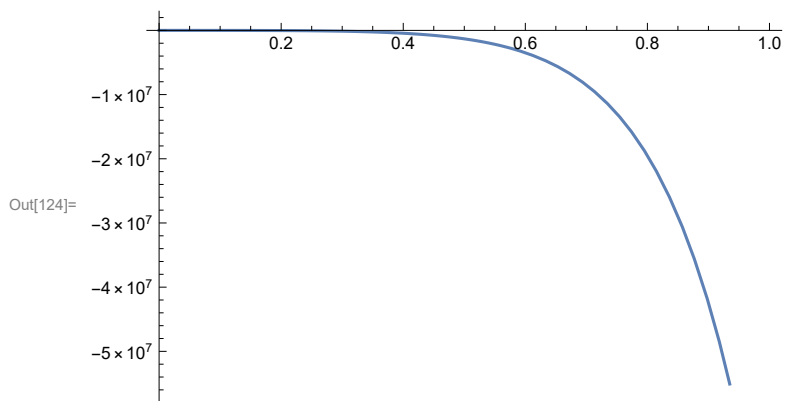

In[125]:= **Plot[Cf[14, 6, 7], {x, 0, 1}]**

[绘图](#)

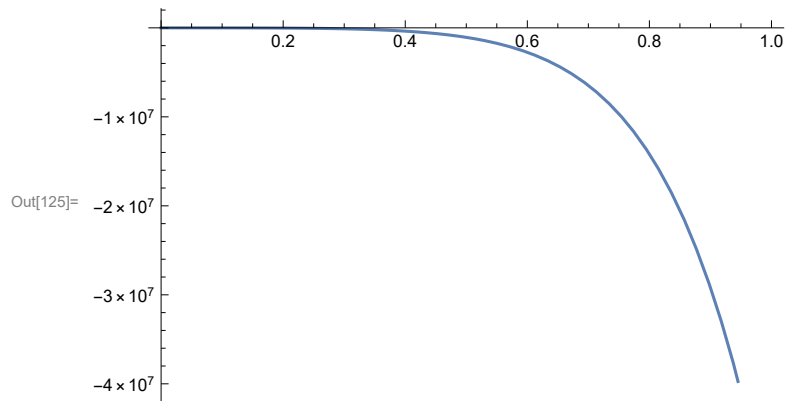

In[126]:= **Plot[Cf[14, 6, 6], {x, 0, 1}]**

[绘图](#)

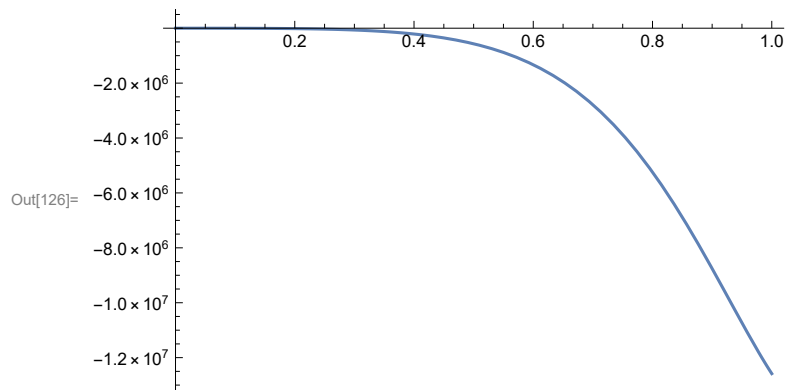

In[127]:= **Plot[Cf[14, 6, 5], {x, 0, 1}]**

[绘图](#)

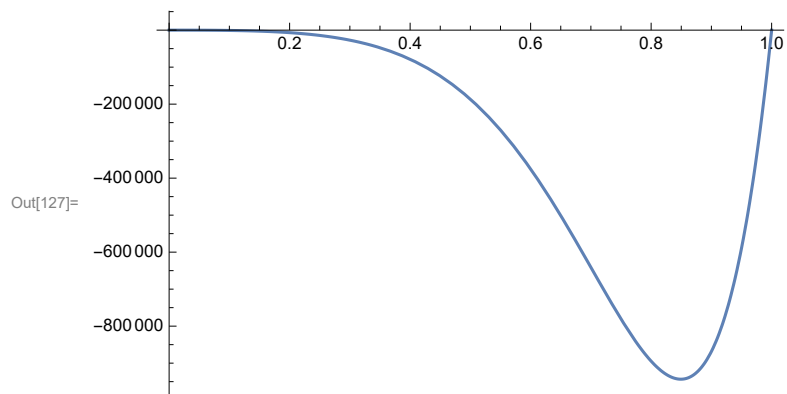

In[128]:= **Plot[Cf[14, 6, 4], {x, 0, 1}]**

[绘图](#)

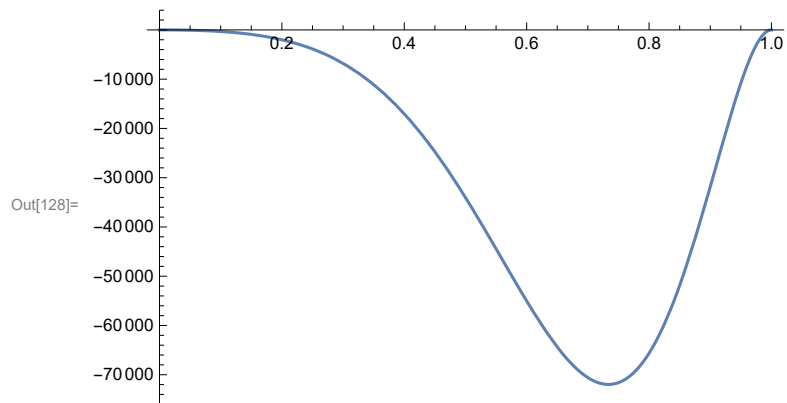

In[129]:= **Plot[Cf[14, 6, 3], {x, 0, 1}]**

[绘图](#)

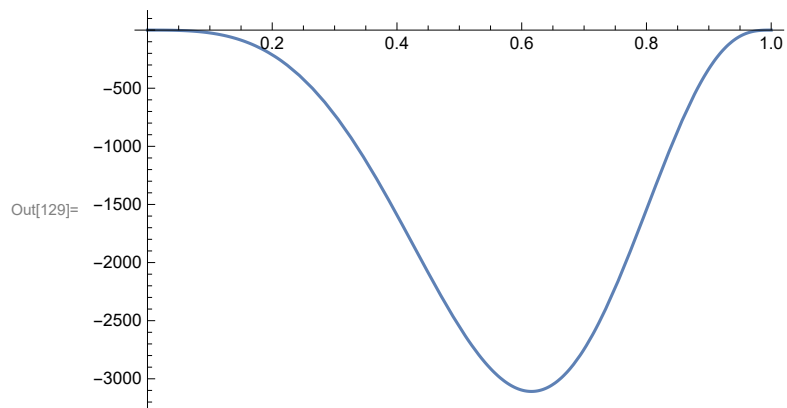

**Plot[Cf[14, 6, 2], {x, 0, 1}]**

[绘图](#)

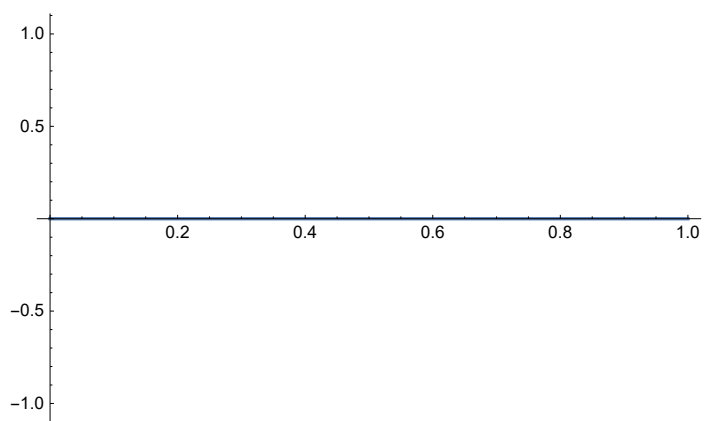

```
Plot[Cf[14, 6, 1], {x, 0, 1}]
```

[绘图](#)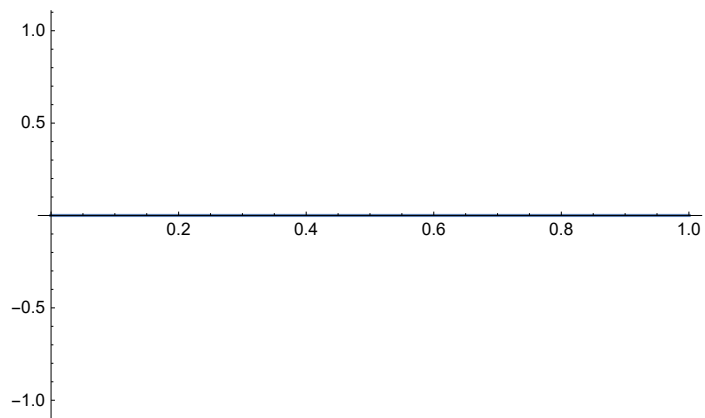

```
Plot[Cf[14, 6, 0], {x, 0, 1}]
```

[绘图](#)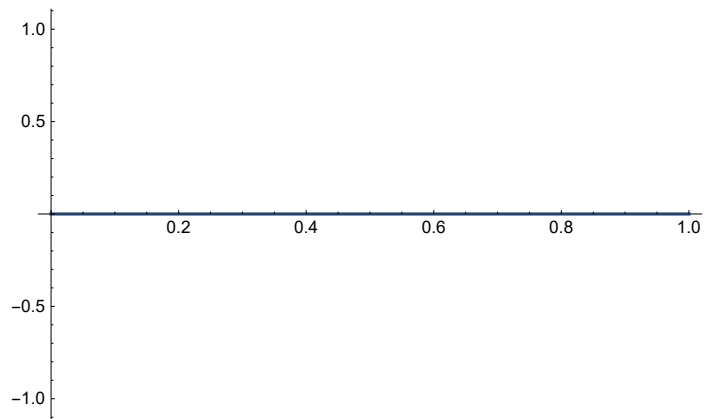

```
(*10th group coefficients r2^14r3^5*)
```

```
Plot[Cf[14, 5, 14], {x, 0, 1}]
```

[绘图](#)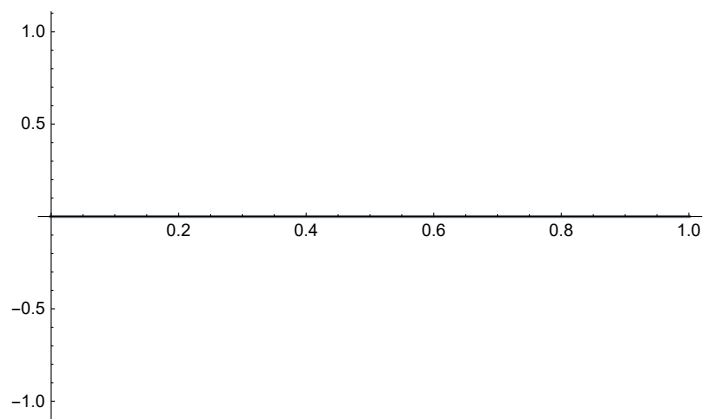

In[130]:= **Plot[Cf[14, 5, 13], {x, 0, 1}]**

[绘图](#)

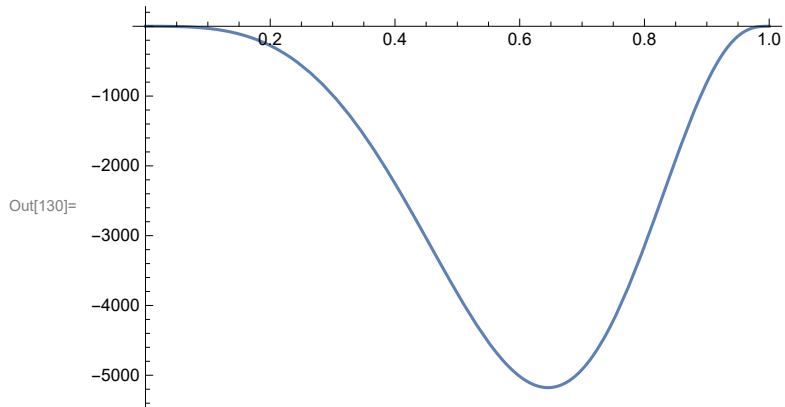

In[132]:= **Plot[Cf[14, 5, 12], {x, 0, 1}]**

[绘图](#)

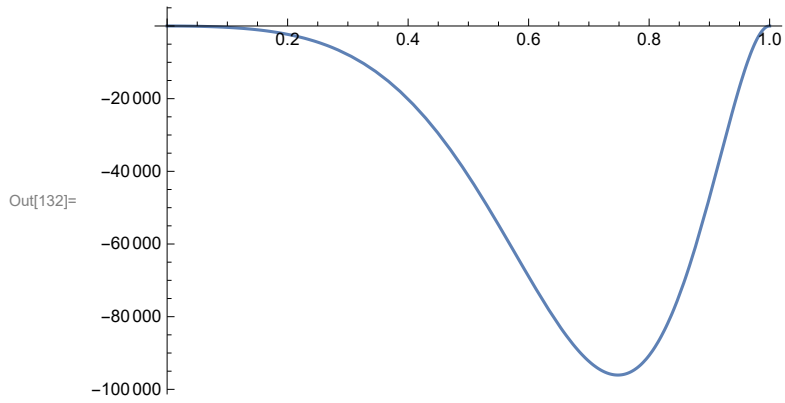

In[131]:= **Plot[Cf[14, 5, 11], {x, 0, 1}]**

[绘图](#)

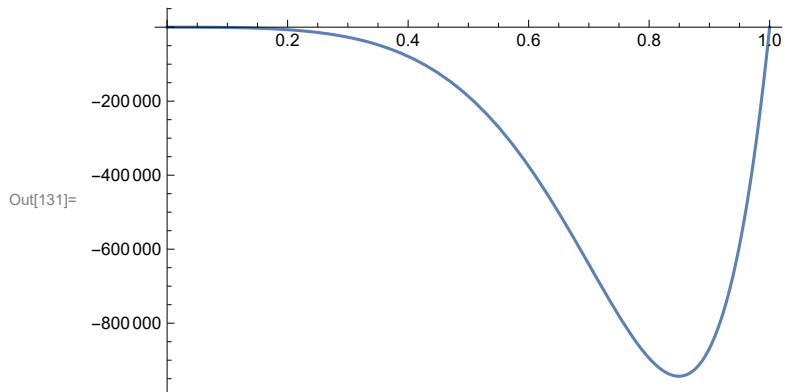

In[133]:= **Plot[Cf[14, 5, 10], {x, 0, 1}]**

[绘图](#)

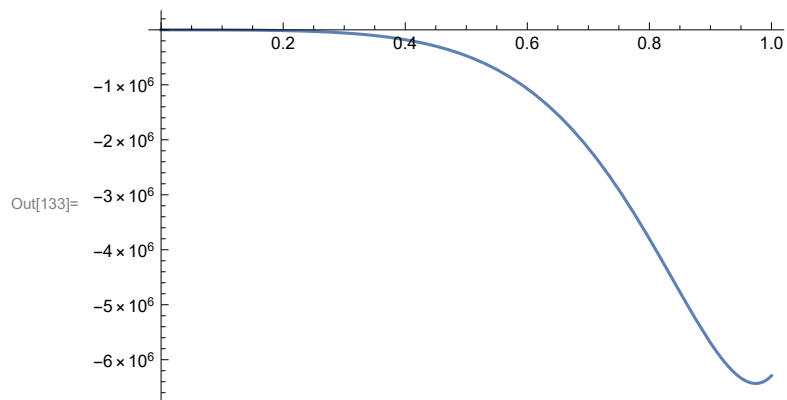

In[134]:= **Plot[Cf[14, 5, 9], {x, 0, 1}]**

[绘图](#)

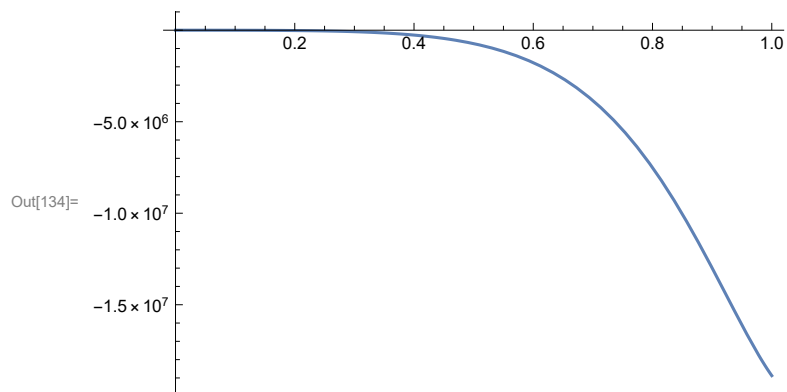

In[135]:= **Plot[Cf[14, 5, 8], {x, 0, 1}]**

[绘图](#)

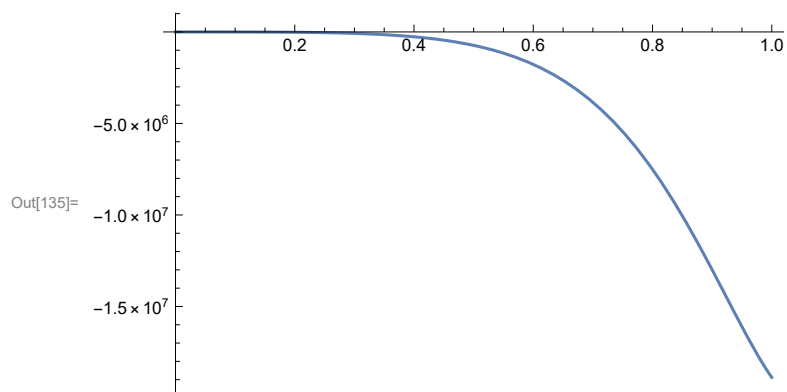



In[136]:= **Plot[Cf[14, 5, 7], {x, 0, 1}]**

[绘图](#)

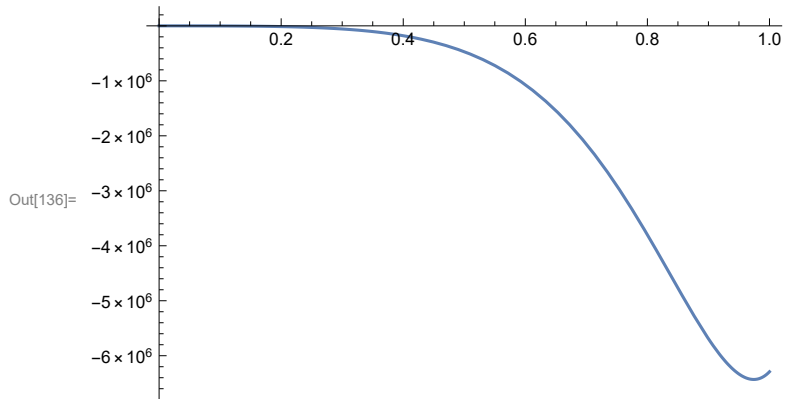

In[137]:= **Plot[Cf[14, 5, 6], {x, 0, 1}]**

[绘图](#)

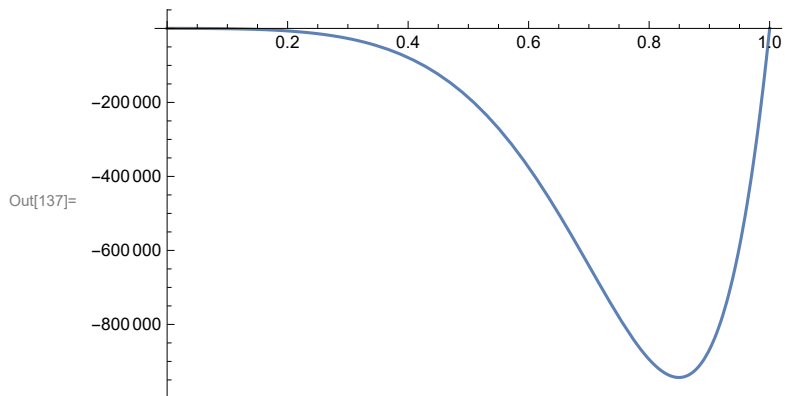

In[138]:= **Plot[Cf[14, 5, 5], {x, 0, 1}]**

[绘图](#)

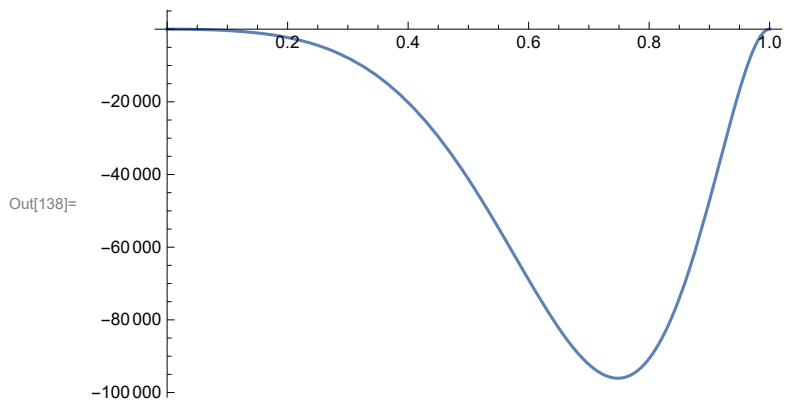

In[139]:= **Plot[Cf[14, 5, 4], {x, 0, 1}]**

[绘图](#)

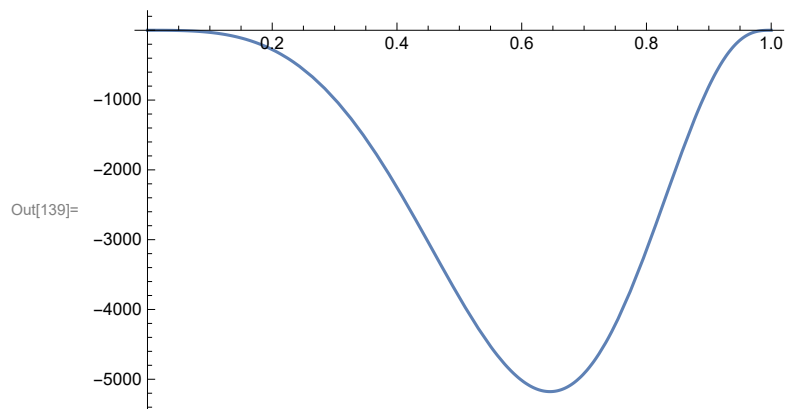

**Plot[Cf[14, 5, 3], {x, 0, 1}]**

[绘图](#)

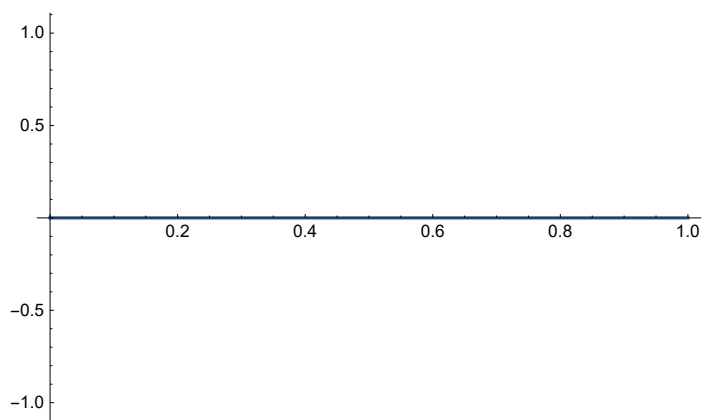

**Plot[Cf[14, 5, 2], {x, 0, 1}]**

[绘图](#)

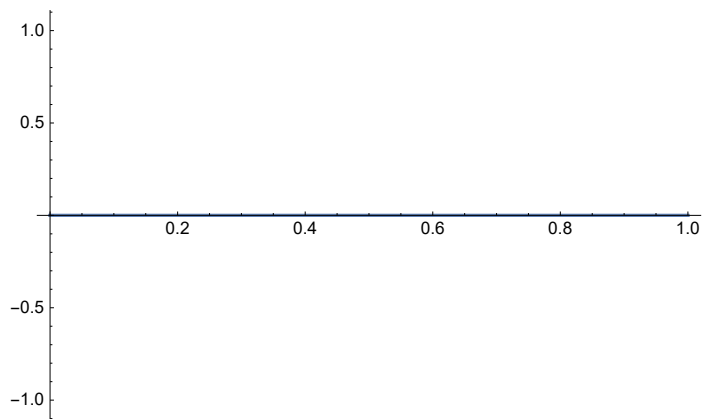

**Plot[Cf[14, 5, 1], {x, 0, 1}]**

[绘图](#)

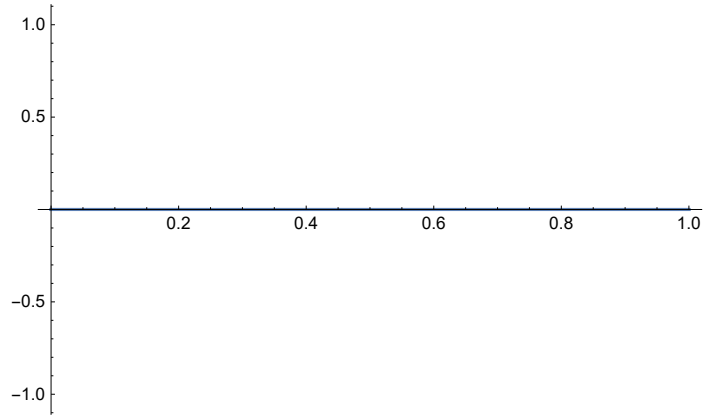

**Plot[Cf[14, 5, 0], {x, 0, 1}]**

[绘图](#)

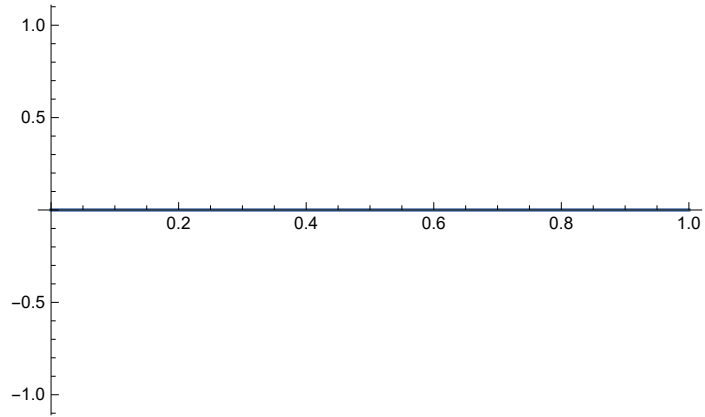

**(\*11th group coefficients r2^14r3^4\*)**

**Plot[Cf[14, 4, 14], {x, 0, 1}]**

[绘图](#)

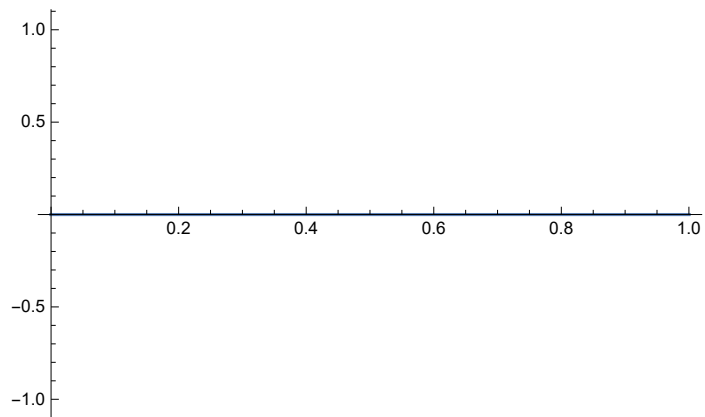

In[140]:= **Plot[Cf[14, 4, 13], {x, 0, 1}]**

[绘图](#)

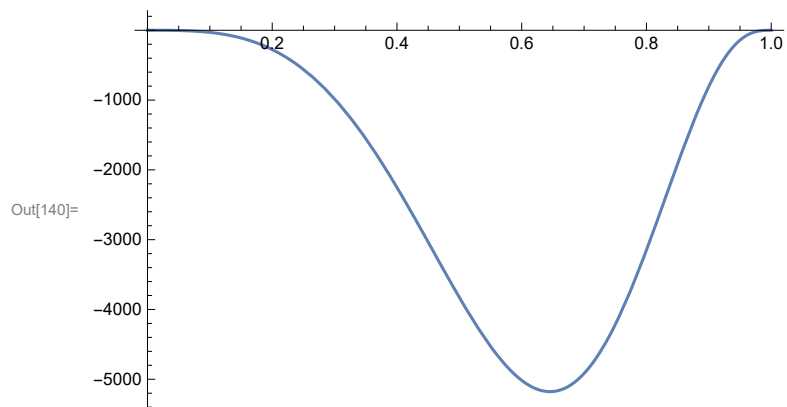

In[141]:= **Plot[Cf[14, 4, 12], {x, 0, 1}]**

[绘图](#)

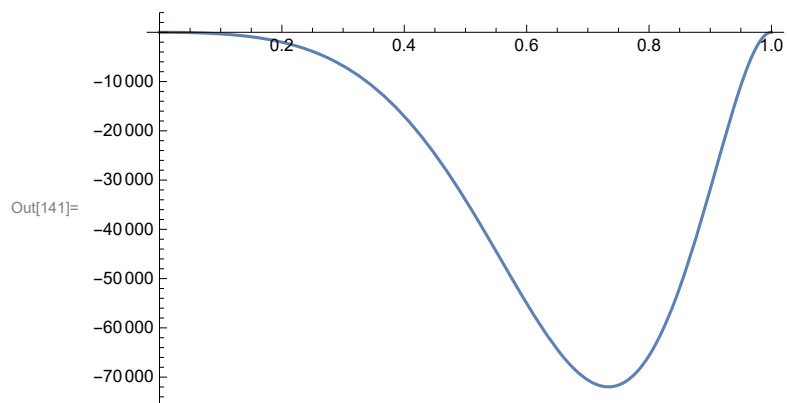

In[142]:= **Plot[Cf[14, 4, 11], {x, 0, 1}]**

[绘图](#)

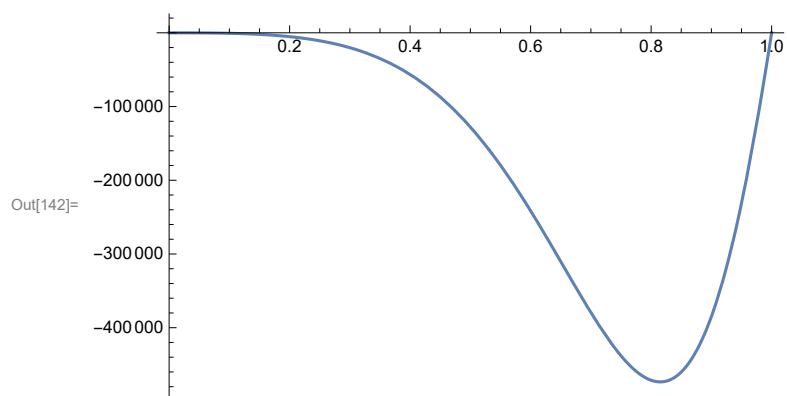

In[143]:= **Plot[Cf[14, 4, 10], {x, 0, 1}]**

[绘图](#)

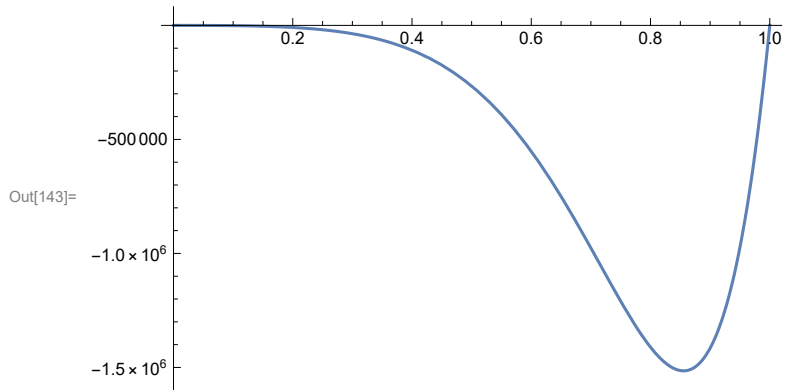

In[144]:= **Plot[Cf[14, 4, 9], {x, 0, 1}]**

[绘图](#)

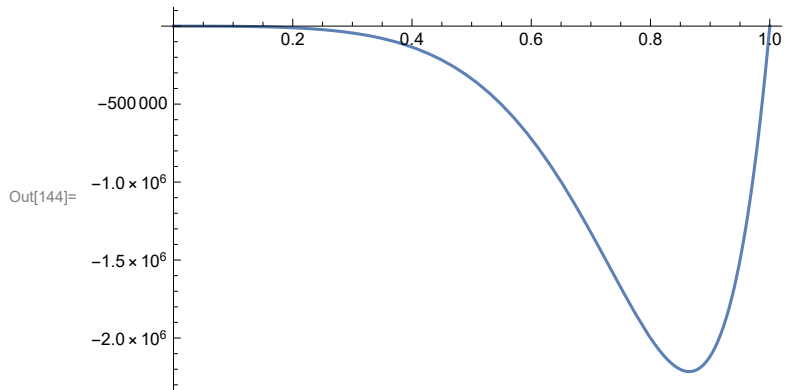

In[145]:= **Plot[Cf[14, 4, 8], {x, 0, 1}]**

[绘图](#)

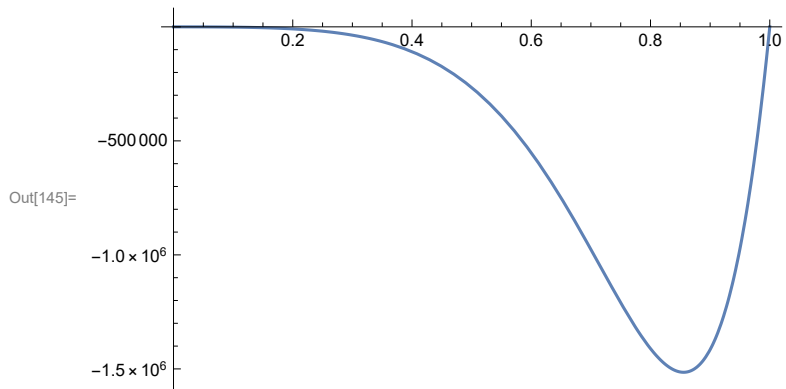

In[146]:= **Plot[Cf[14, 4, 7], {x, 0, 1}]**

[绘图](#)

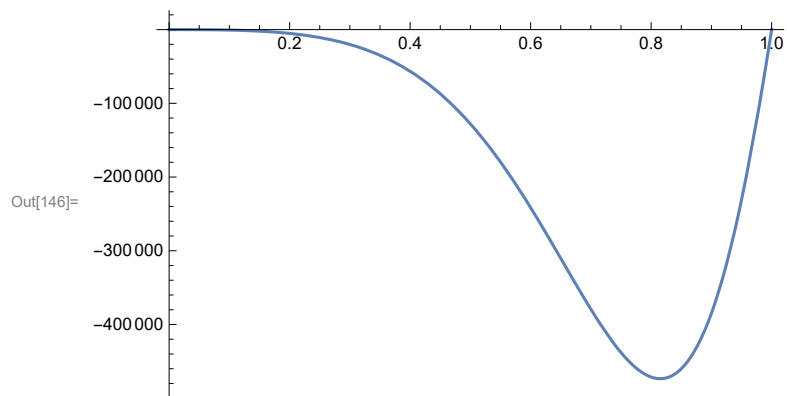

In[147]:= **Plot[Cf[14, 4, 6], {x, 0, 1}]**

[绘图](#)

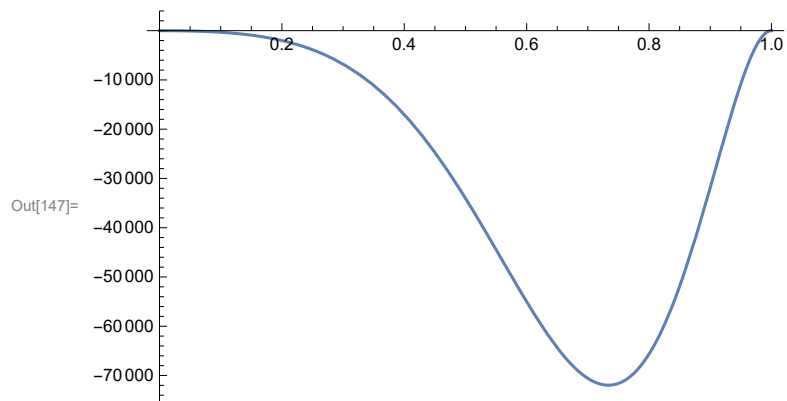

In[148]:= **Plot[Cf[14, 4, 5], {x, 0, 1}]**

[绘图](#)

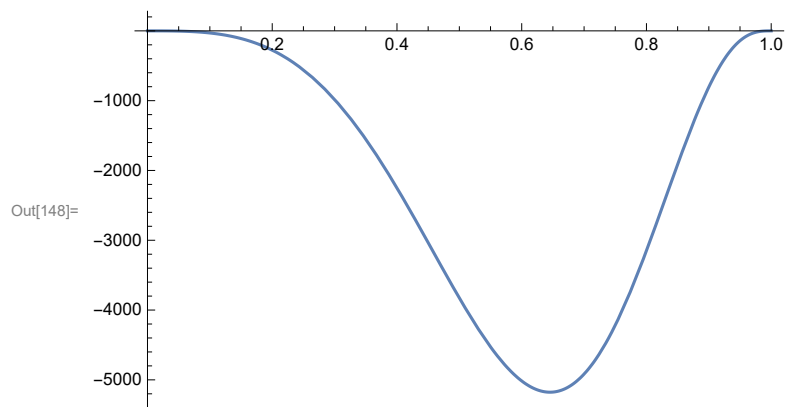

**Plot[Cf[14, 4, 4], {x, 0, 1}]**

[绘图](#)

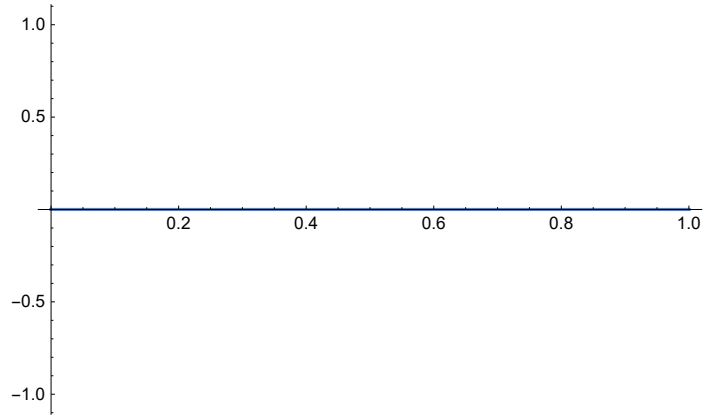

**Plot[Cf[14, 4, 3], {x, 0, 1}]**

[绘图](#)

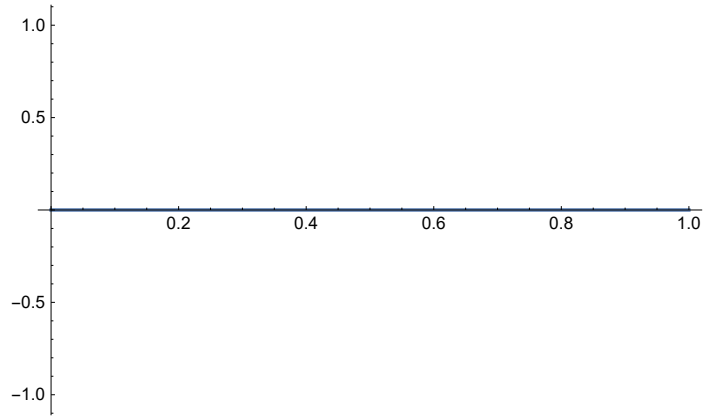

**Plot[Cf[14, 4, 2], {x, 0, 1}]**

[绘图](#)

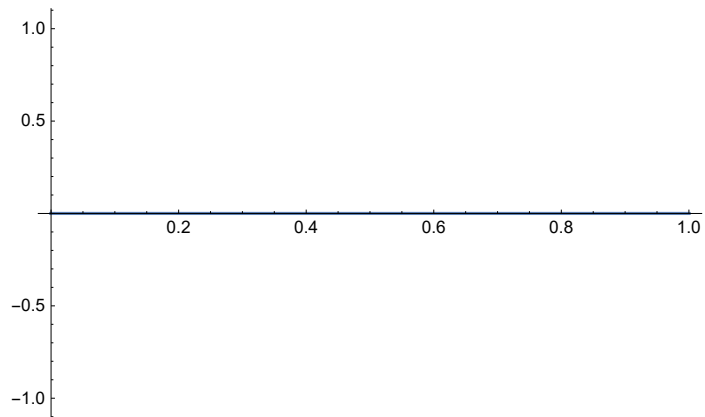

```
Plot[Cf[14, 4, 1], {x, 0, 1}]
```

[绘图](#)

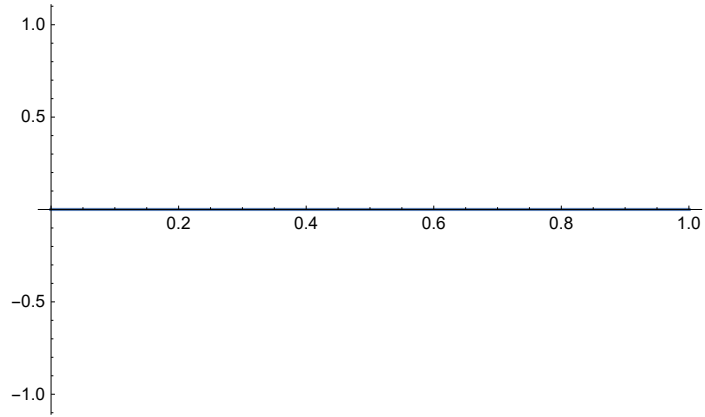

```
Plot[Cf[14, 4, 0], {x, 0, 1}]
```

[绘图](#)

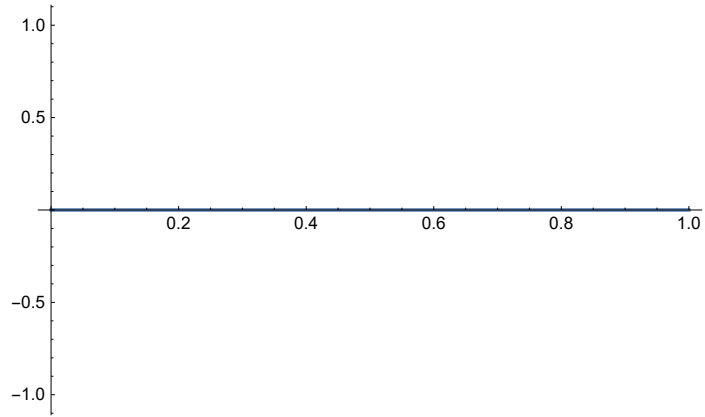

(\*12th group coefficients  $r^2 r^{14} r^3$ \*)

```
Plot[Cf[14, 3, 14], {x, 0, 1}]
```

[绘图](#)

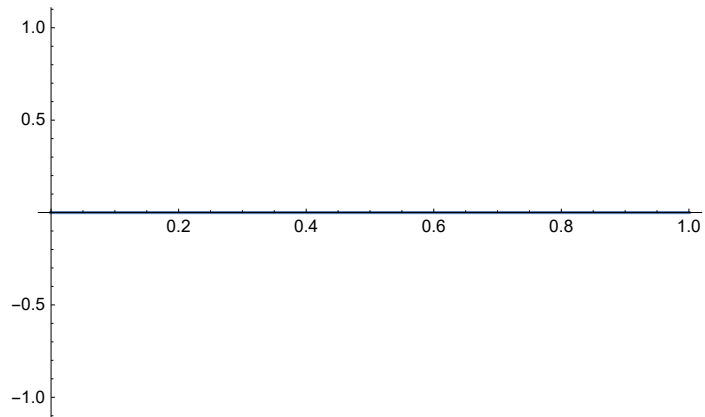



In[149]:= **Plot[Cf[14, 3, 13], {x, 0, 1}]**

[绘图](#)

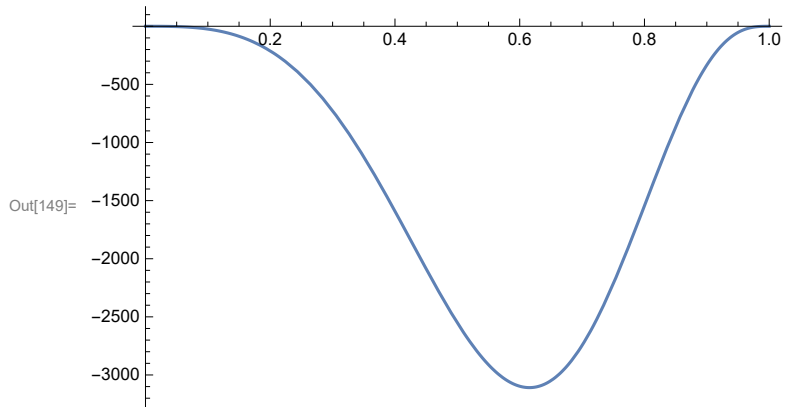

In[150]:= **Plot[Cf[14, 3, 12], {x, 0, 1}]**

[绘图](#)

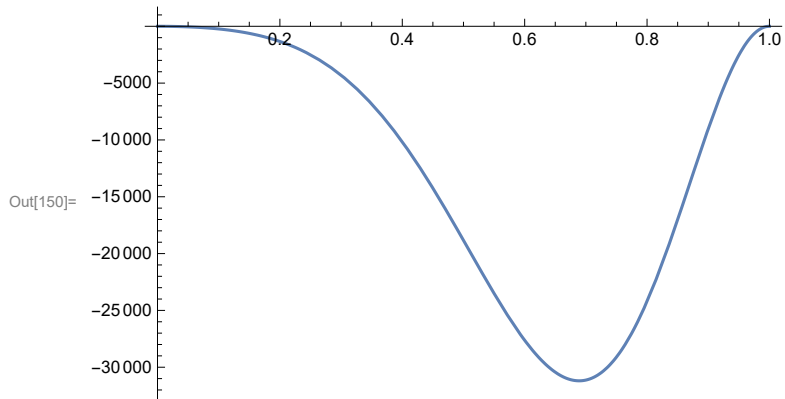

In[151]:= **Plot[Cf[14, 3, 11], {x, 0, 1}]**

[绘图](#)

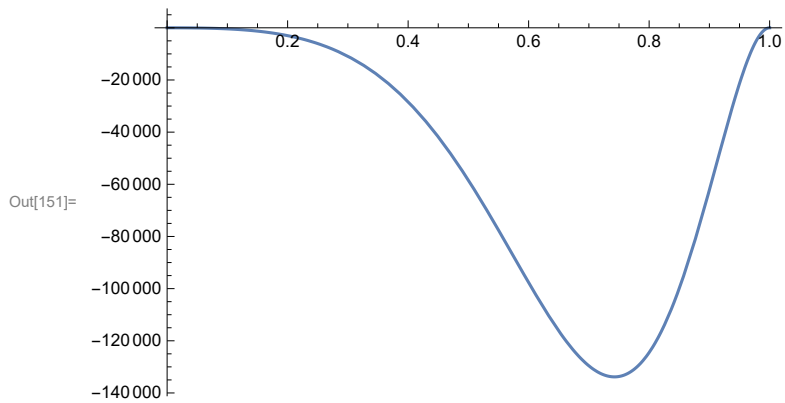

In[152]:= **Plot**[**Cf**[14, 3, 10], {x, 0, 1}]

[绘图](#)

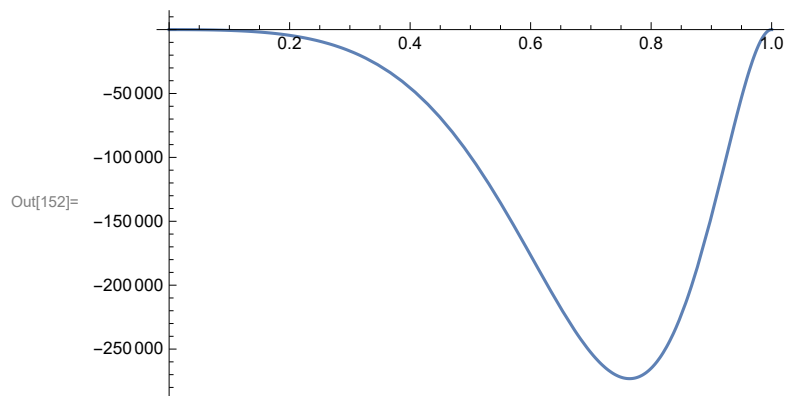

In[153]:= **Plot**[**Cf**[14, 3, 9], {x, 0, 1}]

[绘图](#)

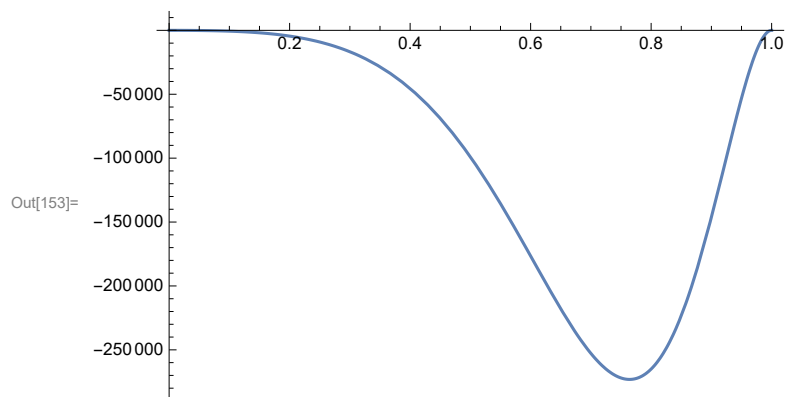

In[154]:= **Plot**[**Cf**[14, 3, 8], {x, 0, 1}]

[绘图](#)

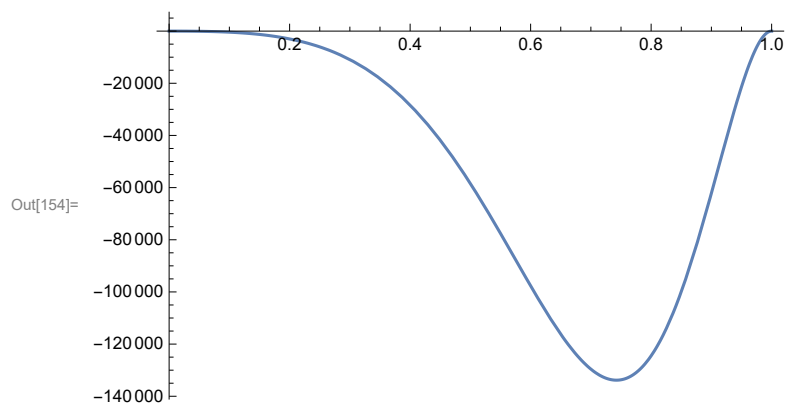

In[155]:= **Plot[Cf[14, 3, 7], {x, 0, 1}]**

[绘图](#)

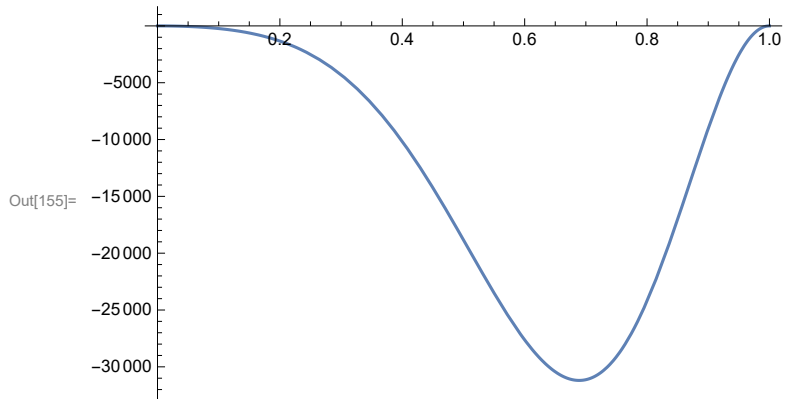

In[156]:= **Plot[Cf[14, 3, 6], {x, 0, 1}]**

[绘图](#)

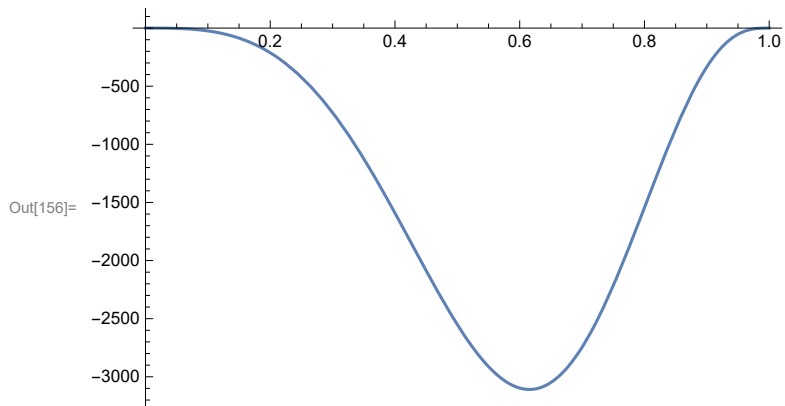

**Plot[Cf[14, 3, 5], {x, 0, 1}]**

[绘图](#)

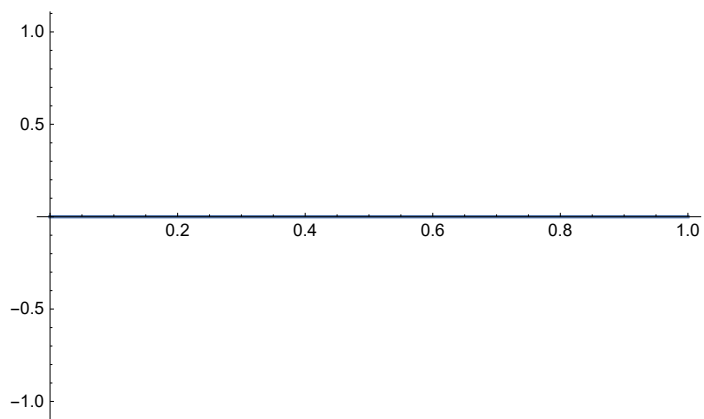

```
Plot[Cf[14, 3, 4], {x, 0, 1}]
```

[绘图](#)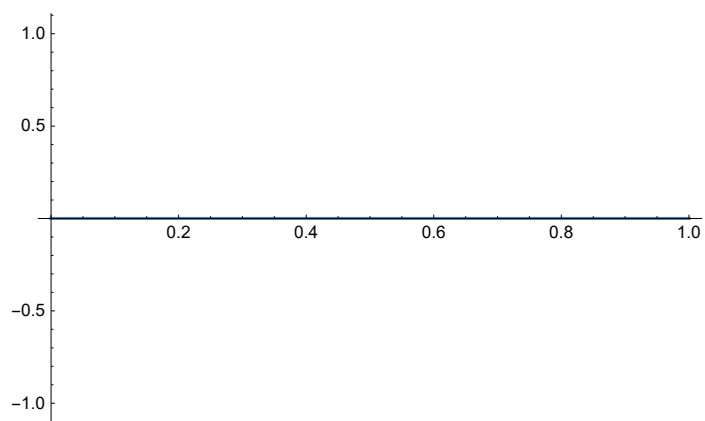

```
Plot[Cf[14, 3, 3], {x, 0, 1}]
```

[绘图](#)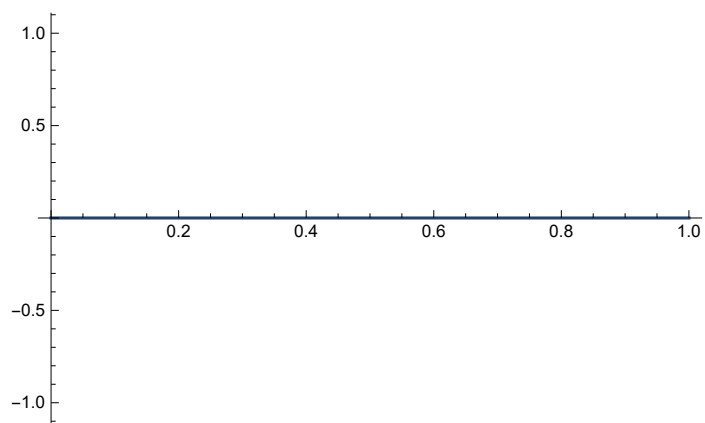

```
Plot[Cf[14, 3, 2], {x, 0, 1}]
```

[绘图](#)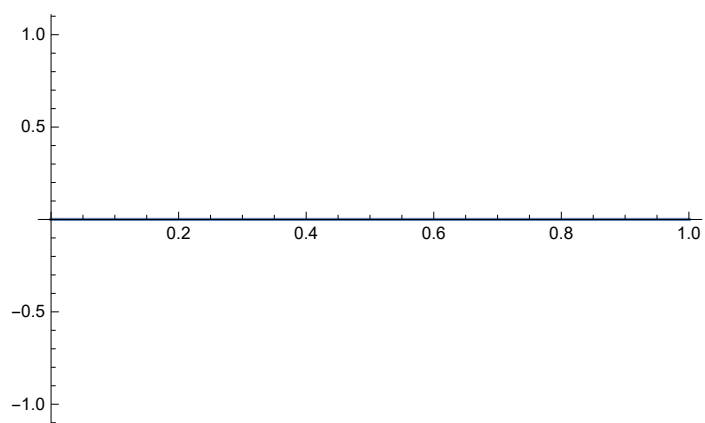

**Plot[Cf[14, 3, 1], {x, 0, 1}]**

[绘图](#)

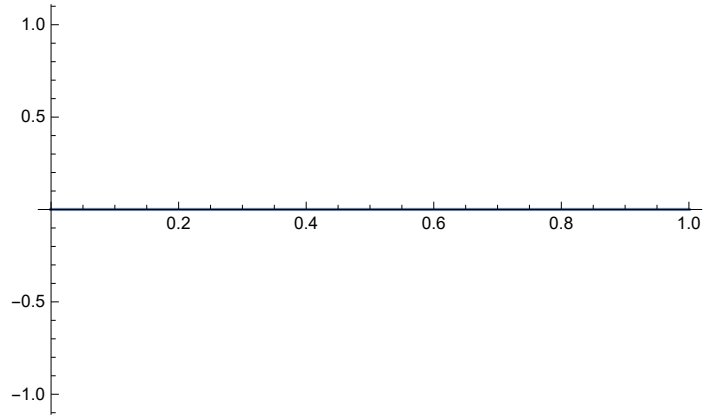

**Plot[Cf[14, 3, 0], {x, 0, 1}]**

[绘图](#)

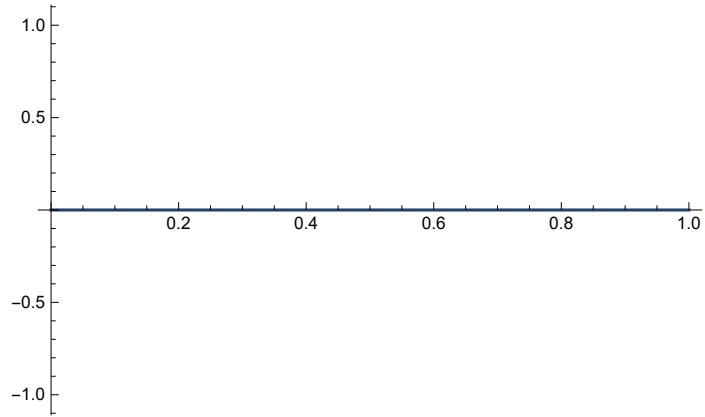

**(\*13th group coefficients r2^14r3^2\*)**

**Plot[Cf[14, 2, 14], {x, 0, 1}]**

[绘图](#)

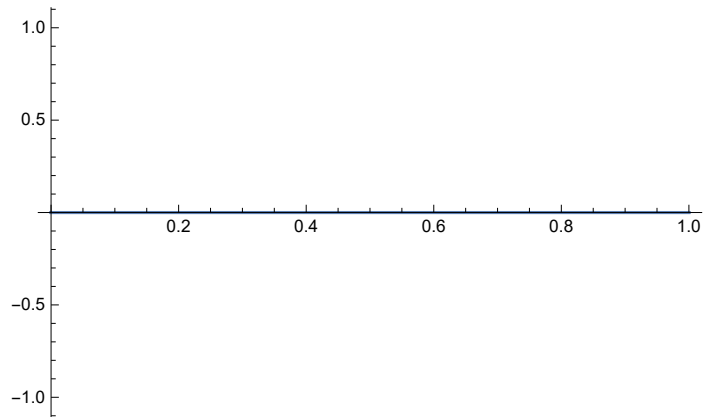

In[157]:= **Plot[Cf[14, 2, 13], {x, 0, 1}]**

[绘图](#)

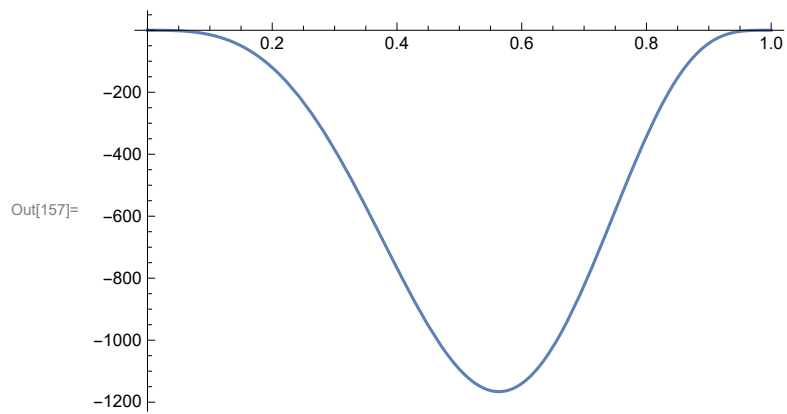

In[158]:= **Plot[Cf[14, 2, 12], {x, 0, 1}]**

[绘图](#)

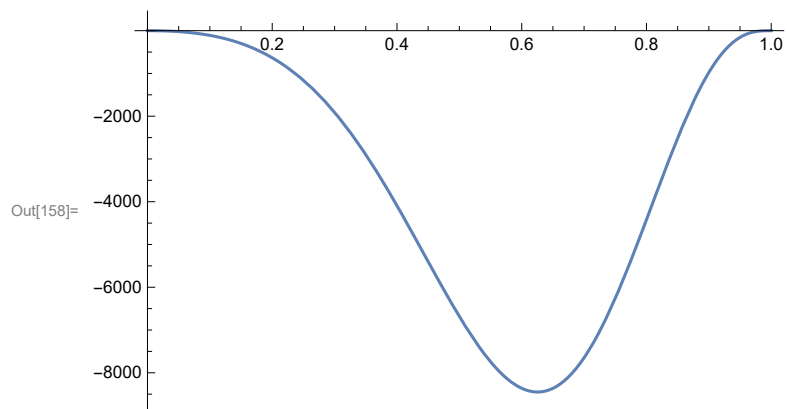

In[159]:= **Plot[Cf[14, 2, 11], {x, 0, 1}]**

[绘图](#)

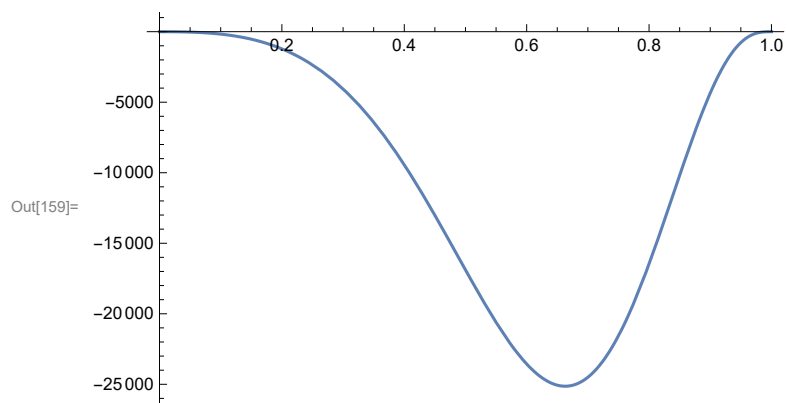

In[160]:= **Plot[Cf[14, 2, 10], {x, 0, 1}]**

[绘图](#)

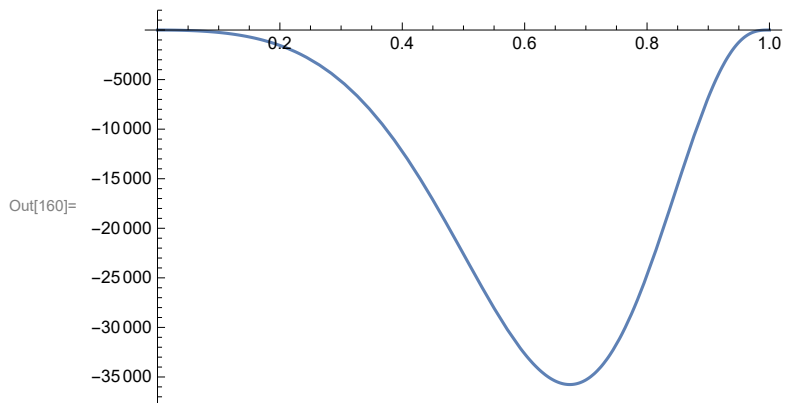

In[161]:= **Plot[Cf[14, 2, 9], {x, 0, 1}]**

[绘图](#)

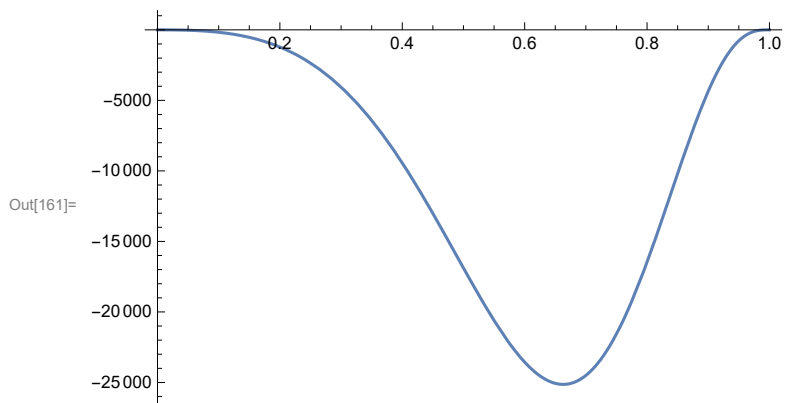

In[162]:= **Plot[Cf[14, 2, 8], {x, 0, 1}]**

[绘图](#)

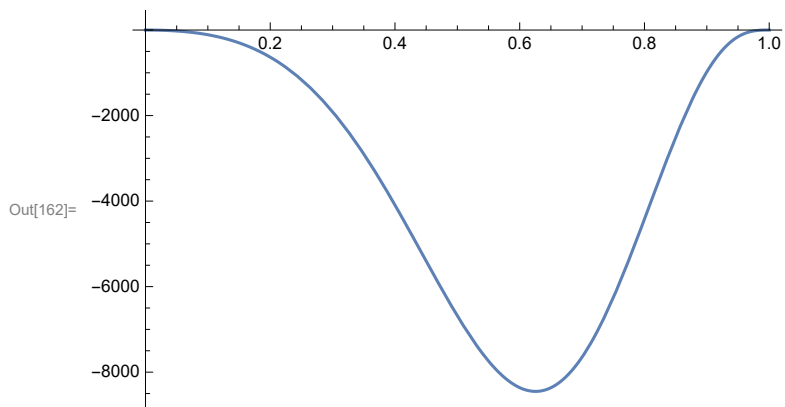

In[163]:= **Plot[Cf[14, 2, 7], {x, 0, 1}]**

[绘图](#)

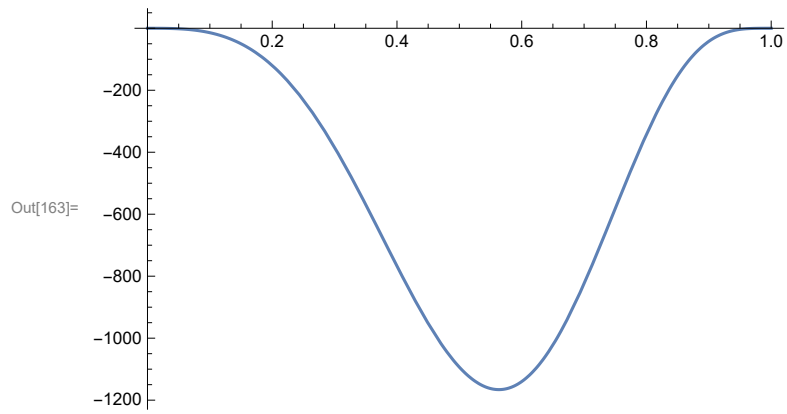

**Plot[Cf[14, 2, 6], {x, 0, 1}]**

[绘图](#)

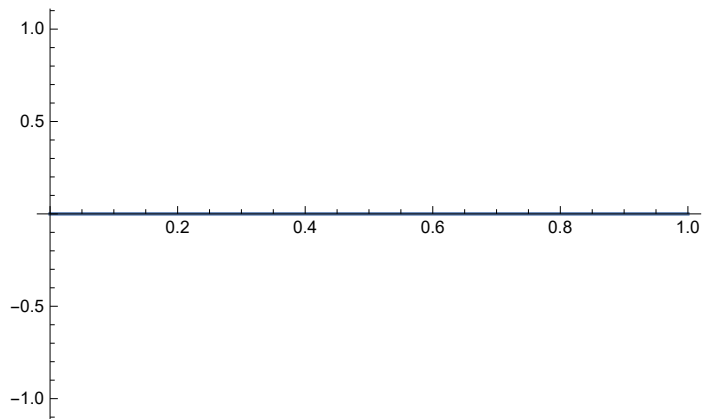

**Plot[Cf[14, 2, 5], {x, 0, 1}]**

[绘图](#)

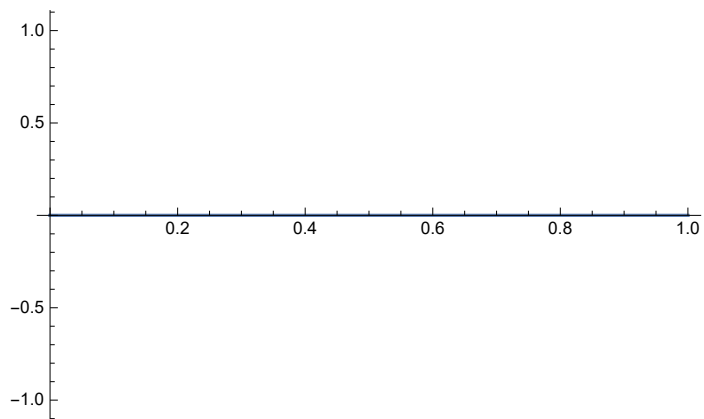



**Plot[Cf[14, 2, 4], {x, 0, 1}]**

[绘图](#)

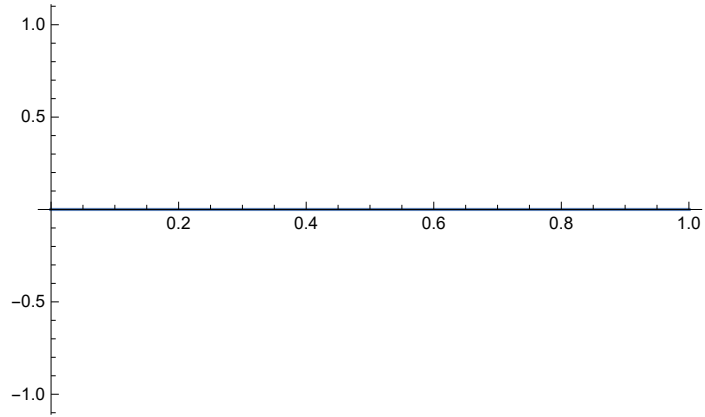

**Plot[Cf[14, 2, 3], {x, 0, 1}]**

[绘图](#)

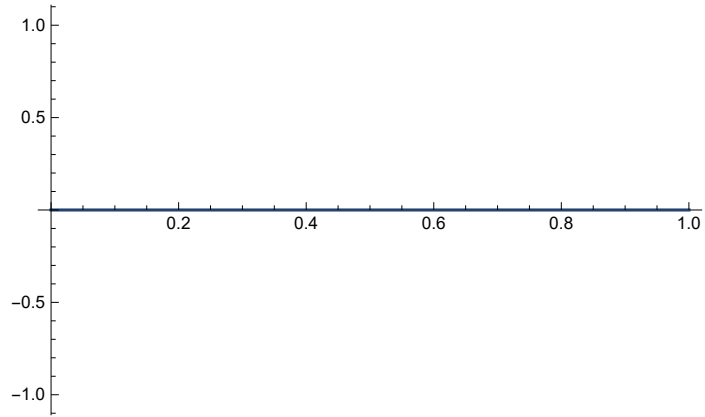

**Plot[Cf[14, 2, 2], {x, 0, 1}]**

[绘图](#)

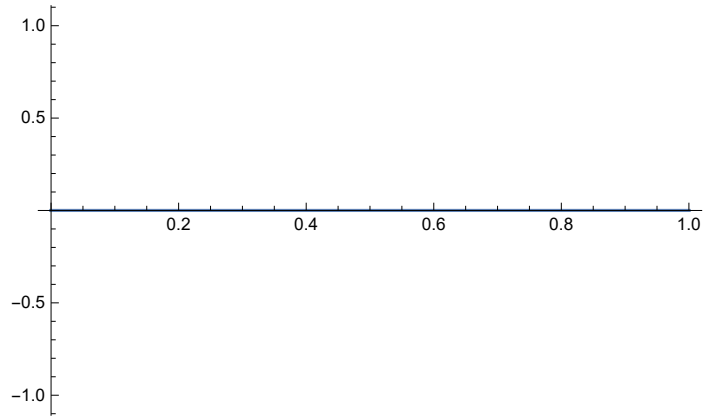

**Plot[Cf[14, 2, 1], {x, 0, 1}]**

[绘图](#)

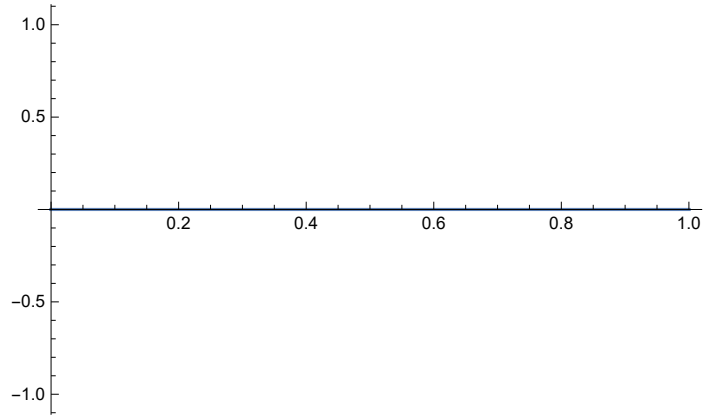

**Plot[Cf[14, 2, 0], {x, 0, 1}]**

[绘图](#)

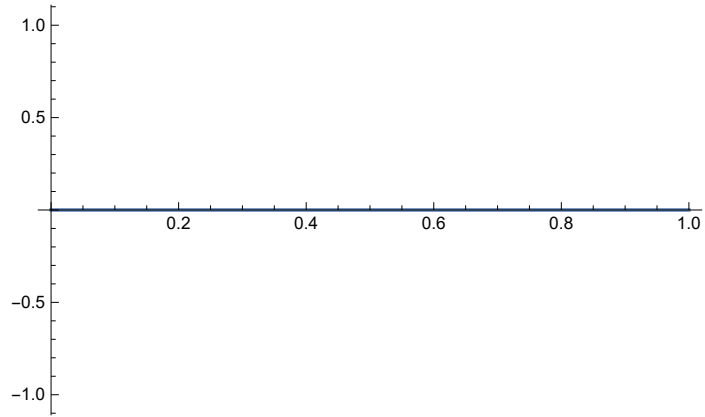

**(\*14th group coefficients r2^14r3^1\*)**

**Plot[Cf[14, 1, 14], {x, 0, 1}]**

[绘图](#)

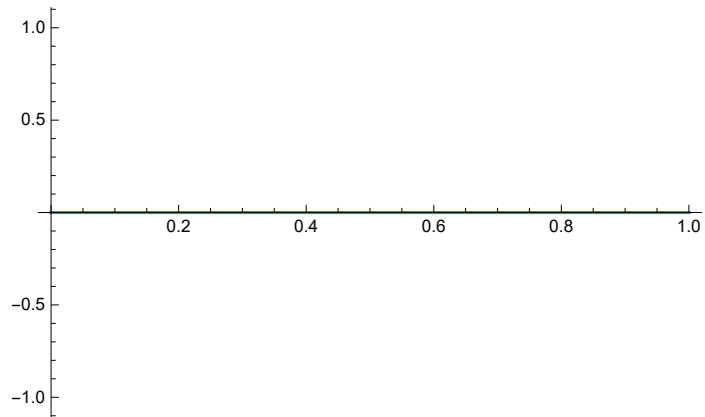

In[164]:= **Plot**[**Cf**[14, 1, 13], {x, 0, 1}]

[绘图](#)

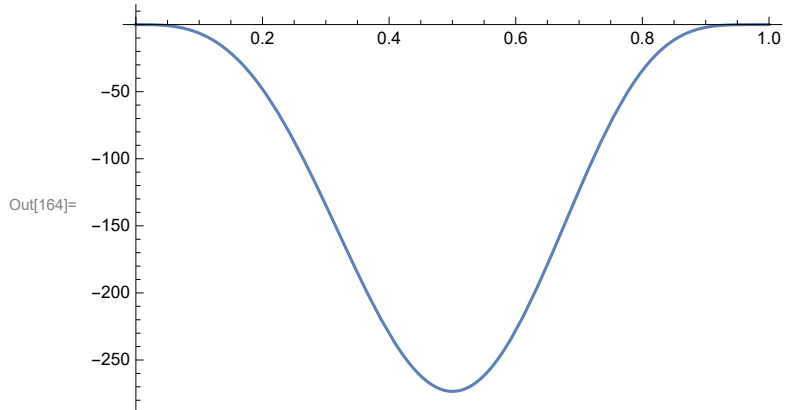

In[165]:= **Plot**[**Cf**[14, 1, 12], {x, 0, 1}]

[绘图](#)

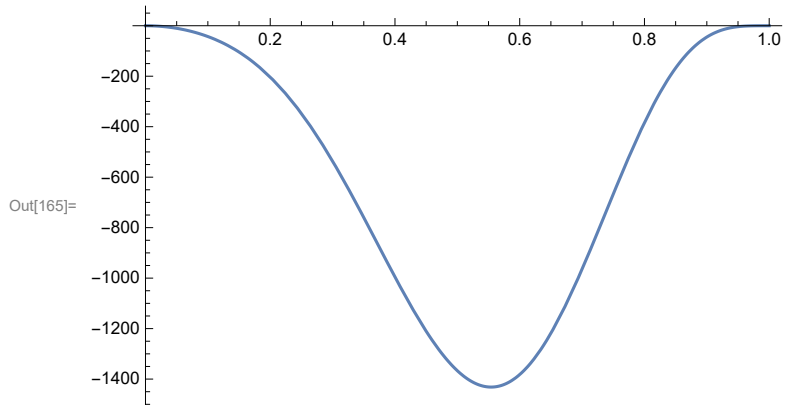

In[166]:= **Plot**[**Cf**[14, 1, 11], {x, 0, 1}]

[绘图](#)

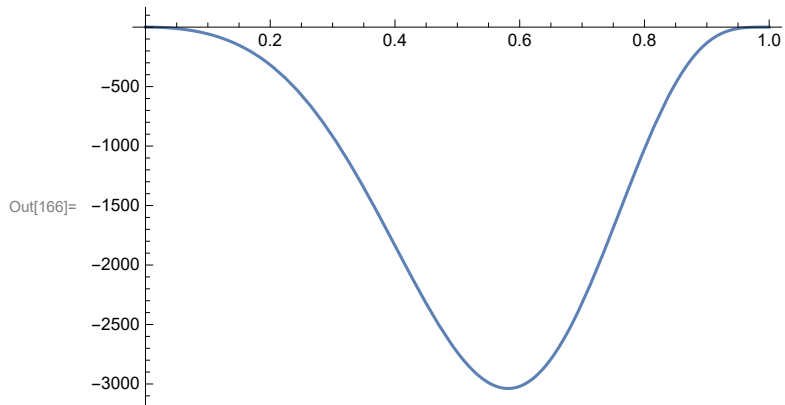

In[167]:= **Plot**[**Cf**[14, 1, 10], {x, 0, 1}]

[绘图](#)

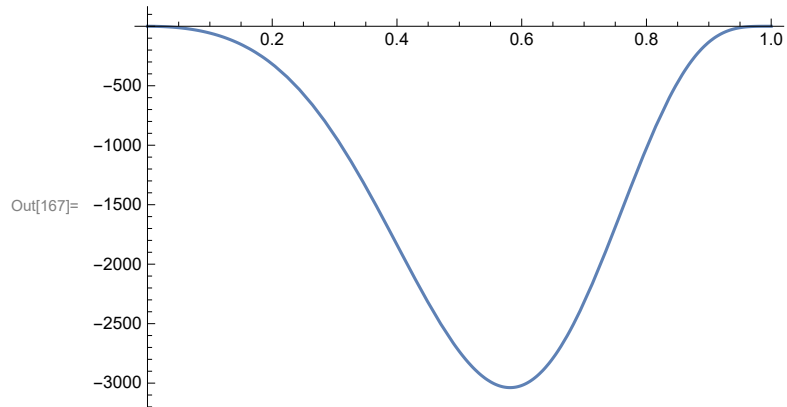

In[168]:= **Plot**[**Cf**[14, 1, 9], {x, 0, 1}]

[绘图](#)

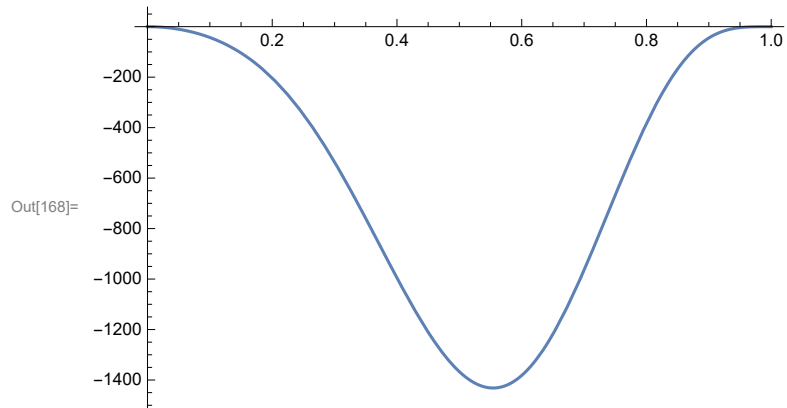

In[169]:= **Plot**[**Cf**[14, 1, 8], {x, 0, 1}]

[绘图](#)

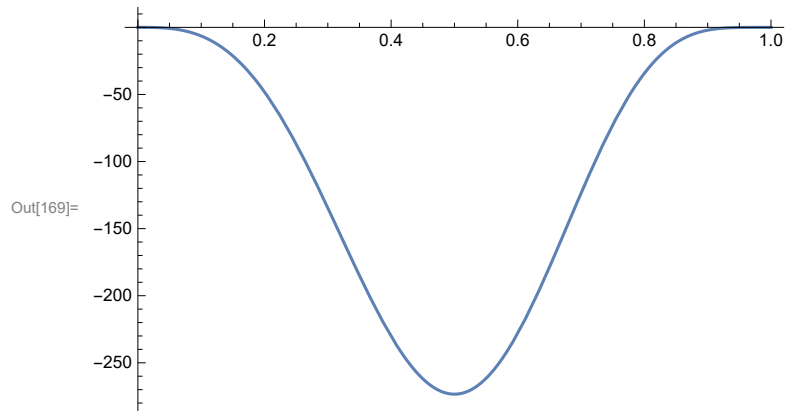

**Plot[Cf[14, 1, 7], {x, 0, 1}]**

[绘图](#)

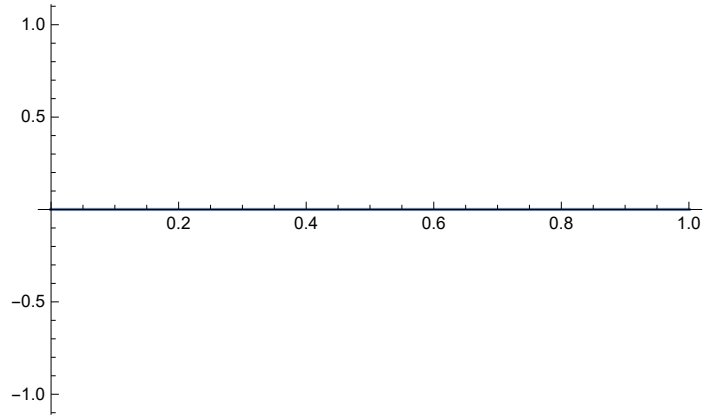

**Plot[Cf[14, 1, 6], {x, 0, 1}]**

[绘图](#)

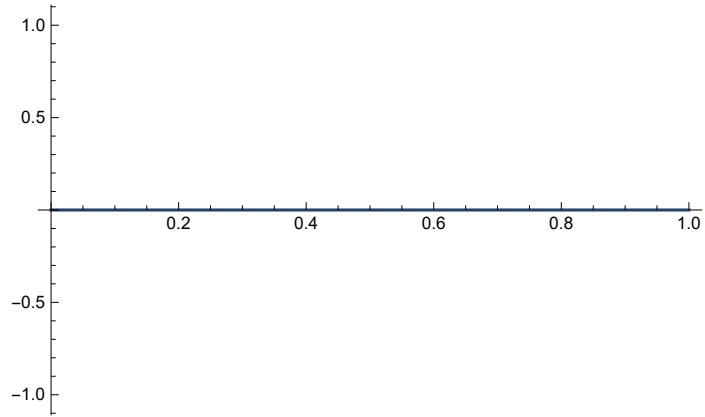

**Plot[Cf[14, 1, 5], {x, 0, 1}]**

[绘图](#)

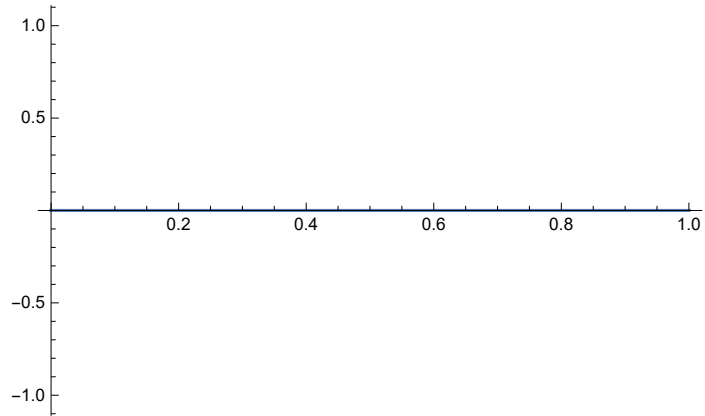

**Plot[Cf[14, 1, 4], {x, 0, 1}]**

[绘图](#)

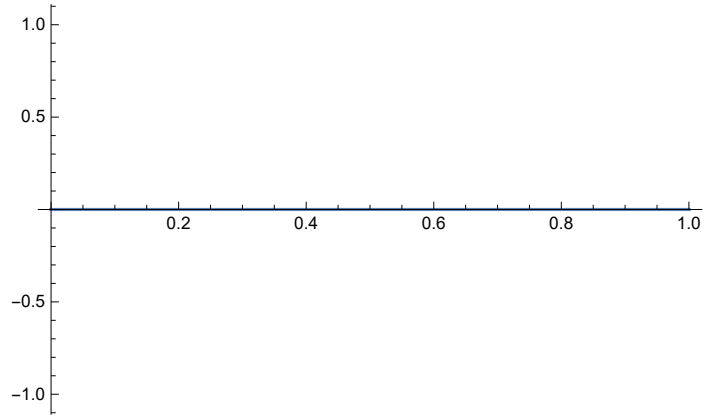

**Plot[Cf[14, 1, 3], {x, 0, 1}]**

[绘图](#)

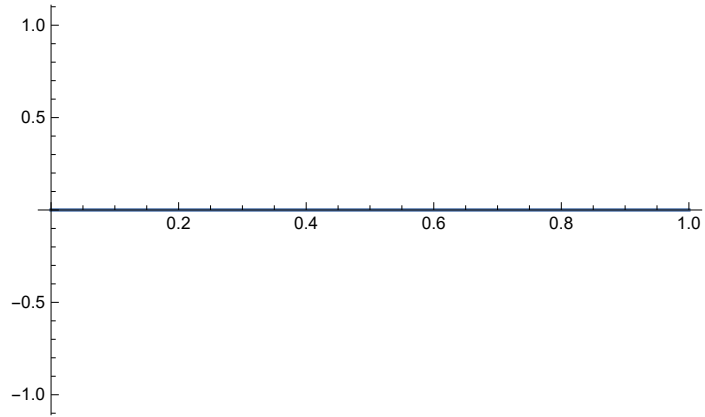

**Plot[Cf[14, 1, 2], {x, 0, 1}]**

[绘图](#)

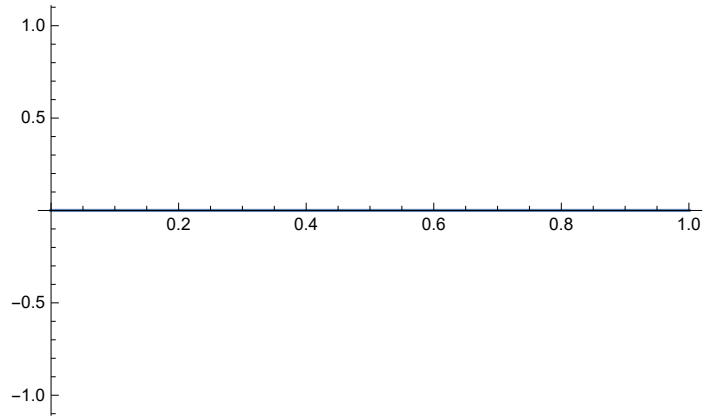

**Plot[Cf[14, 1, 1], {x, 0, 1}]**

[绘图](#)

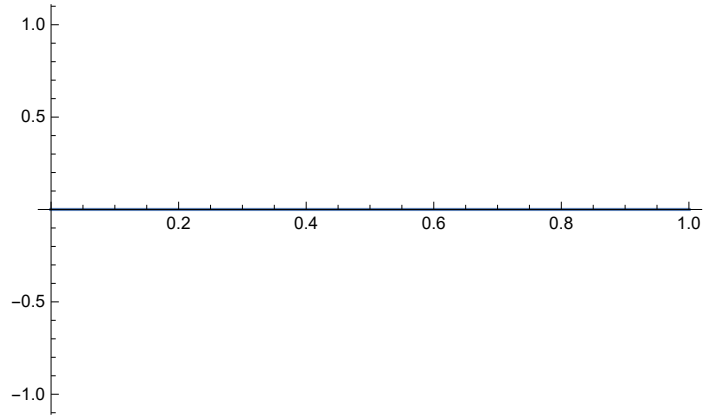

**Plot[Cf[14, 1, 0], {x, 0, 1}]**

[绘图](#)

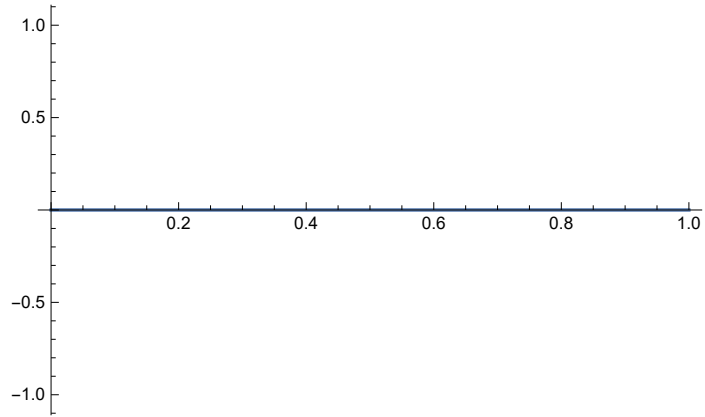

**(\*15th group coefficients r2^14r3^0\*)**

**Plot[Cf[14, 0, 14], {x, 0, 1}]**

[绘图](#)

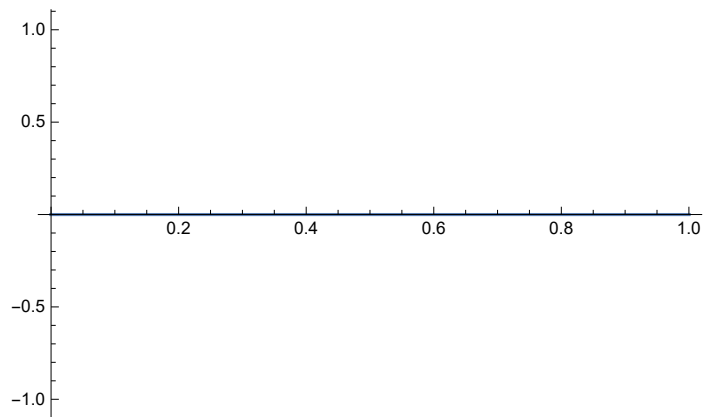

In[170]:= **Plot**[**Cf**[14, 0, 13], {x, 0, 1}]

[绘图](#)

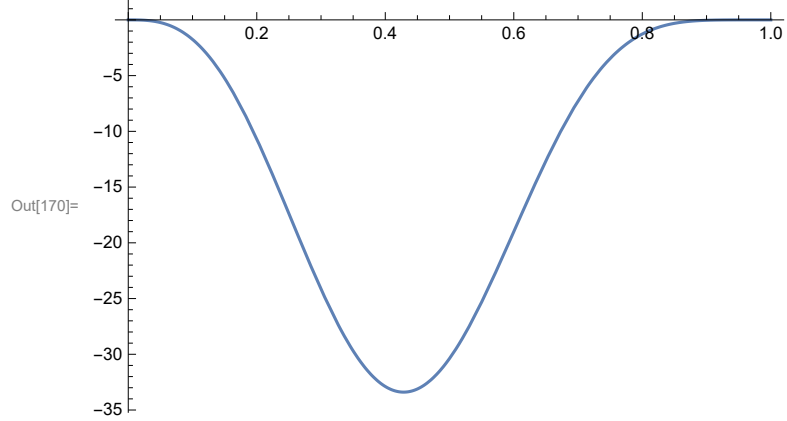

In[171]:= **Plot**[**Cf**[14, 0, 12], {x, 0, 1}]

[绘图](#)

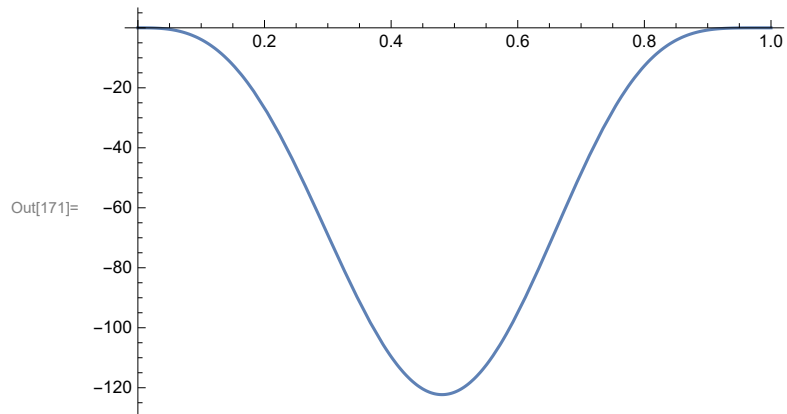

In[173]:= **Plot**[**Cf**[14, 0, 11], {x, 0, 1}]

[绘图](#)

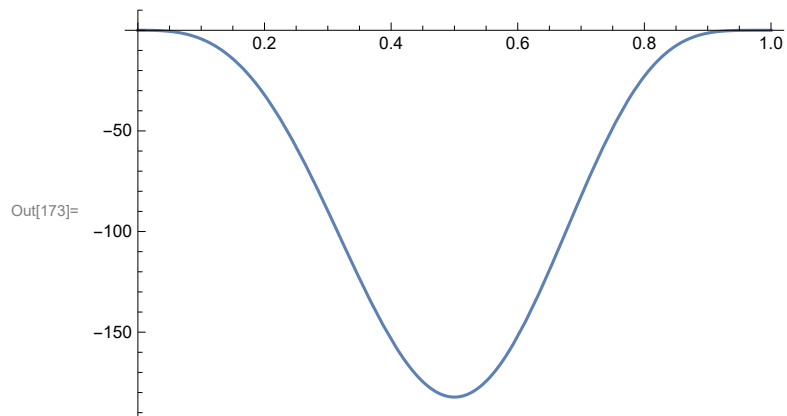



In[174]:= **Plot[Cf[14, 0, 10], {x, 0, 1}]**

[绘图](#)

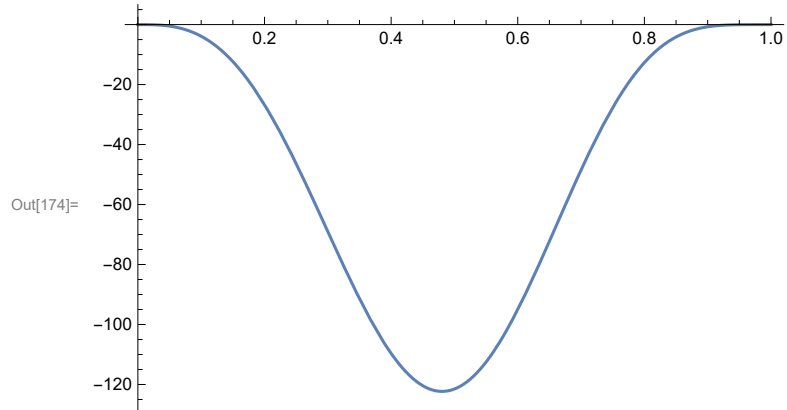

In[175]:= **Plot[Cf[14, 0, 9], {x, 0, 1}]**

[绘图](#)

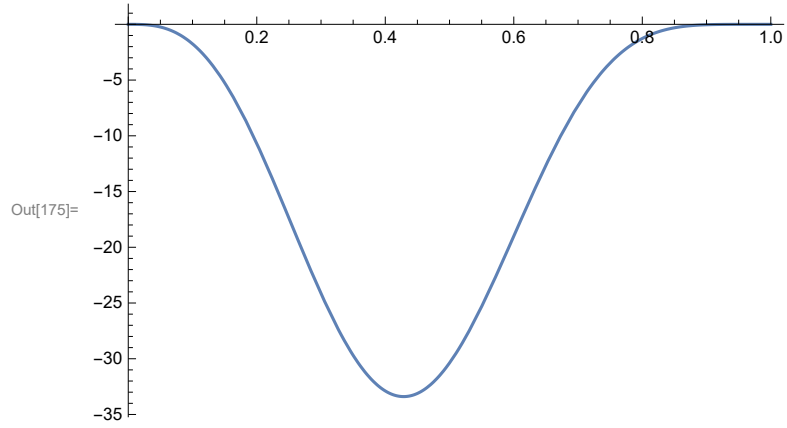

**Plot[Cf[14, 0, 8], {x, 0, 1}]**

[绘图](#)

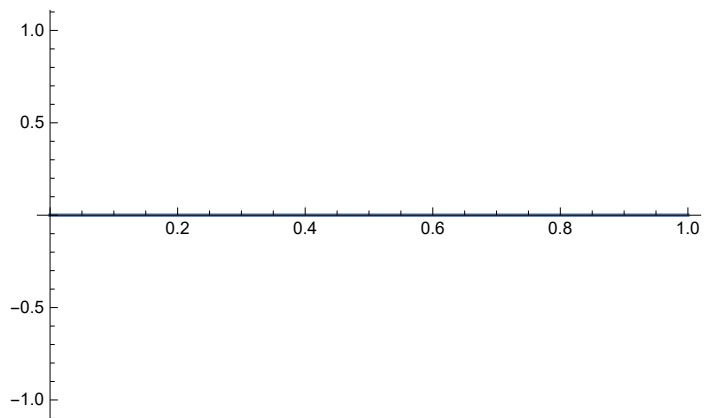

```
Plot[Cf[14, 0, 7], {x, 0, 1}]
```

[绘图](#)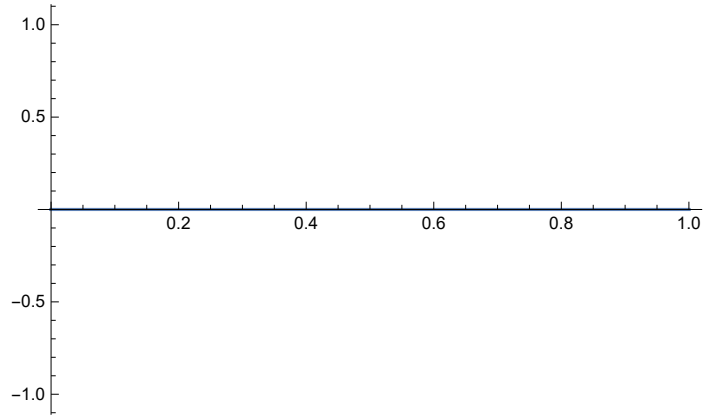

```
Plot[Cf[14, 0, 6], {x, 0, 1}]
```

[绘图](#)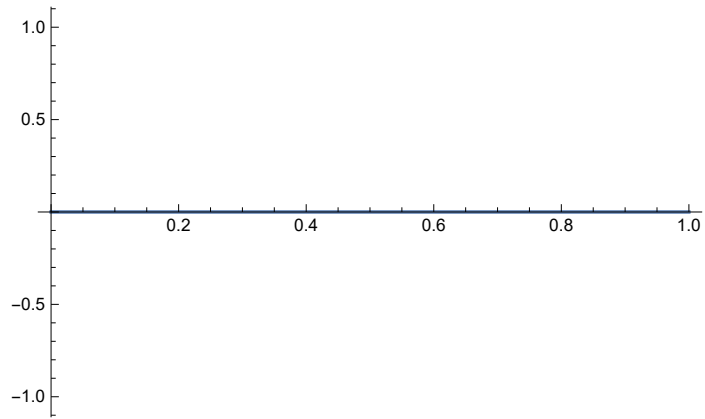

```
Plot[Cf[14, 0, 5], {x, 0, 1}]
```

[绘图](#)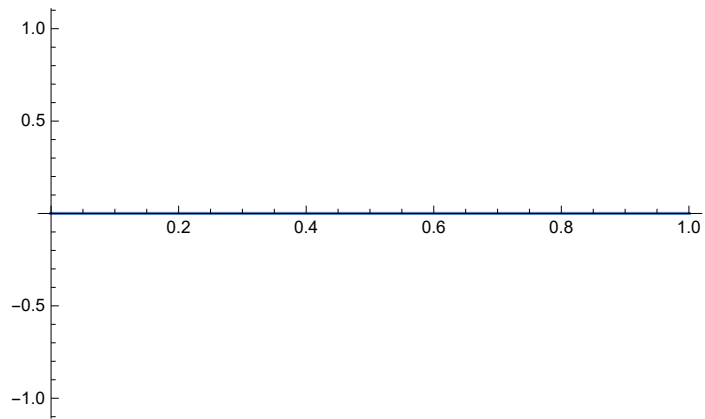

**Plot[Cf[14, 0, 4], {x, 0, 1}]**

[绘图](#)

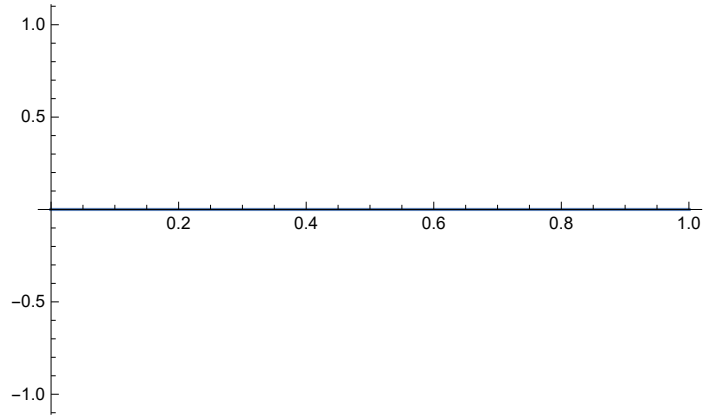

**Plot[Cf[14, 0, 3], {x, 0, 1}]**

[绘图](#)

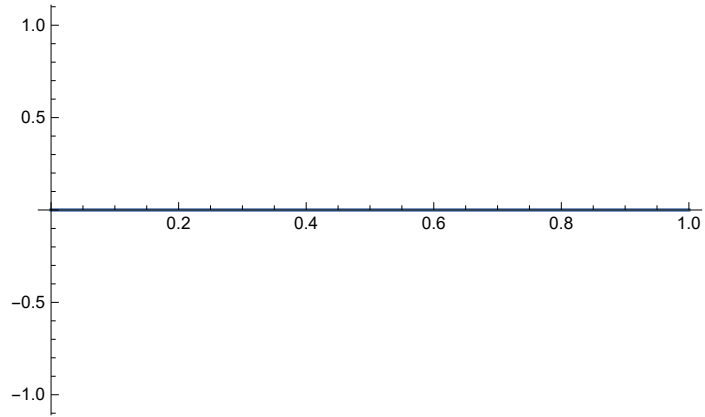

**Plot[Cf[14, 0, 2], {x, 0, 1}]**

[绘图](#)

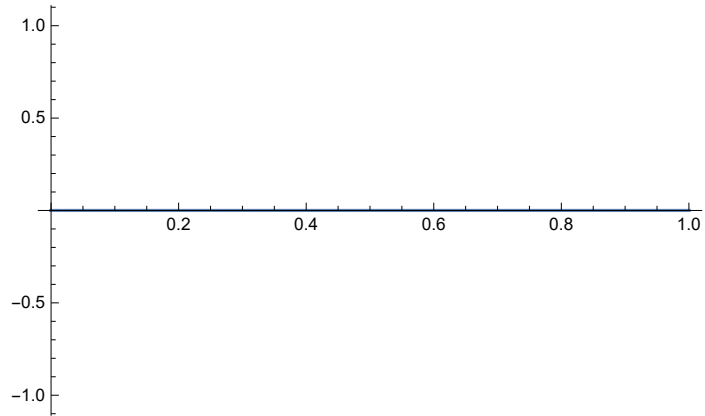

`Plot[Cf[14, 0, 1], {x, 0, 1}]`

[绘图](#)

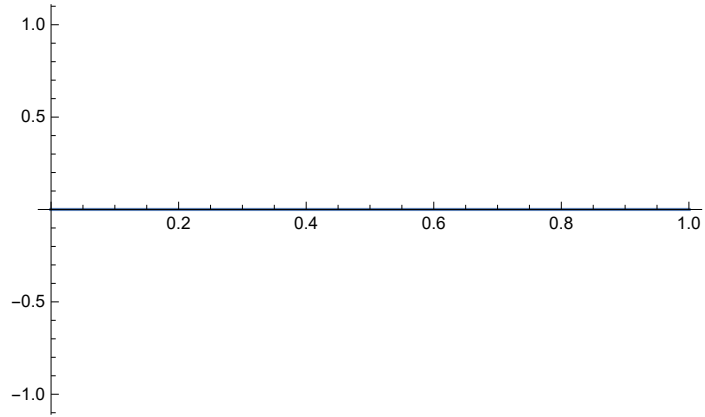

`Plot[Cf[14, 0, 0], {x, 0, 1}]`

[绘图](#)

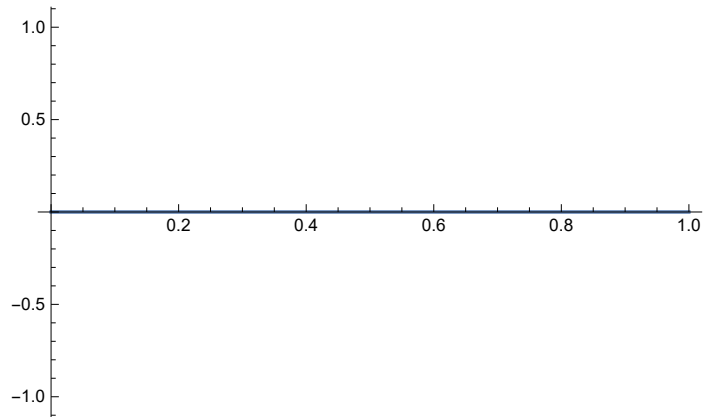

(\*16th group coefficients  $r^2 r^3 r^{14}$ \*)

`Plot[Cf[13, 14, 14], {x, 0, 1}]`

[绘图](#)

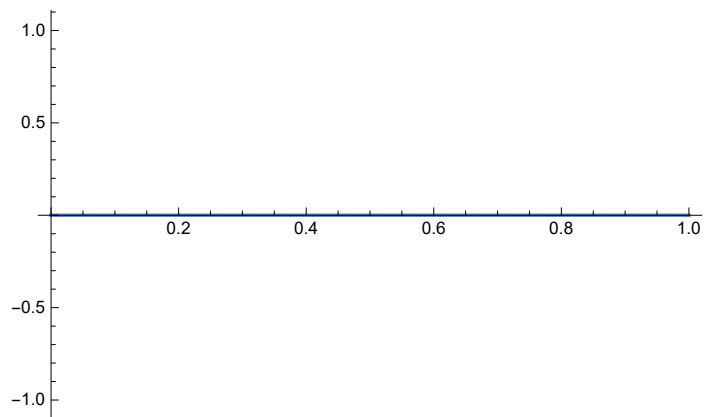

**Plot[Cf[13, 14, 13], {x, 0, 1}]**

[绘图](#)

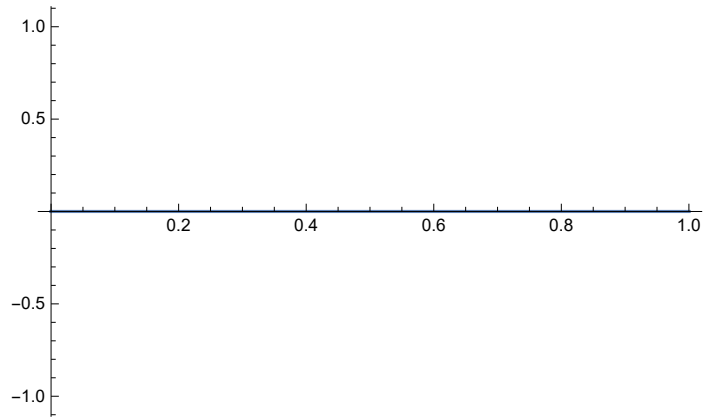

**Plot[Cf[13, 14, 13], {x, 0, 1}]**

[绘图](#)

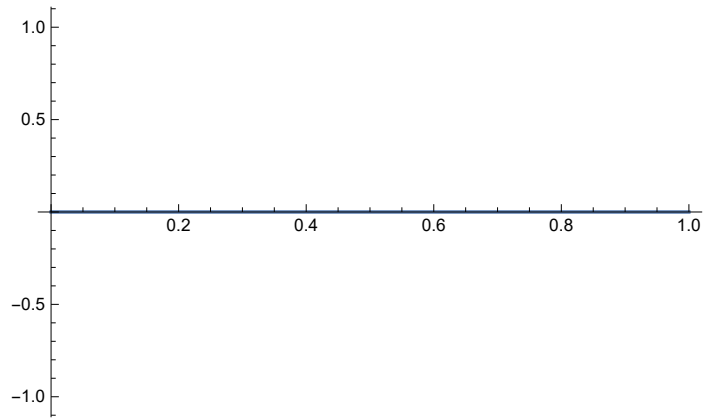

**Plot[Cf[13, 14, 12], {x, 0, 1}]**

[绘图](#)

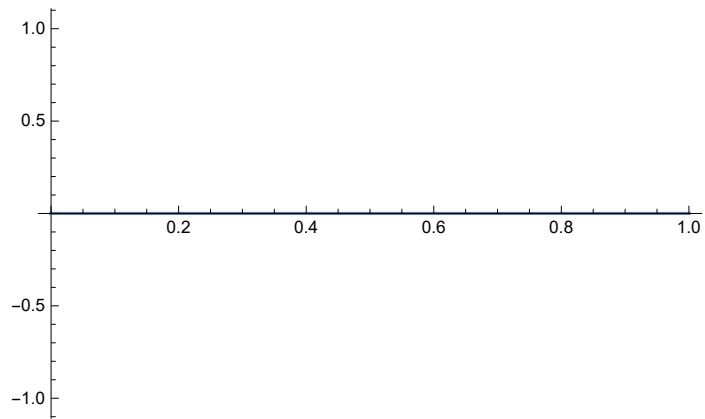

```
Plot[Cf[13, 14, 11], {x, 0, 1}]
```

[绘图](#)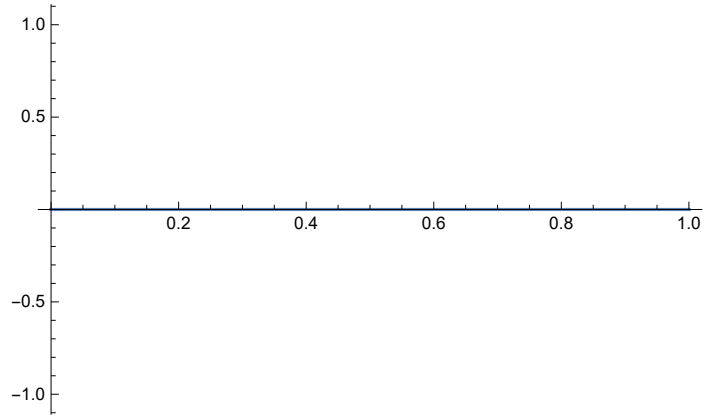

```
Plot[Cf[13, 14, 10], {x, 0, 1}]
```

[绘图](#)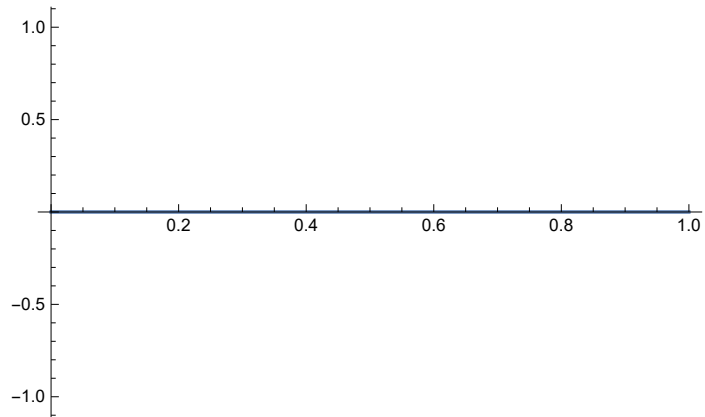

```
In[176]:= Plot[Cf[13, 14, 9], {x, 0, 1}]
```

[绘图](#)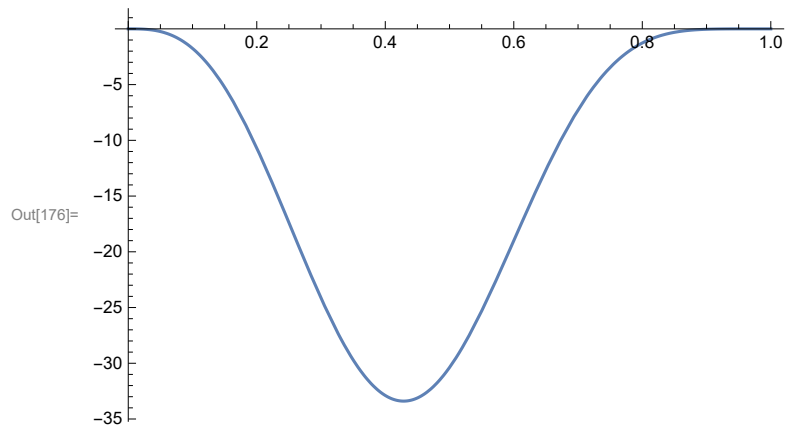

In[177]:= **Plot**[**Cf**[13, 14, 8], {x, 0, 1}]

[绘图](#)

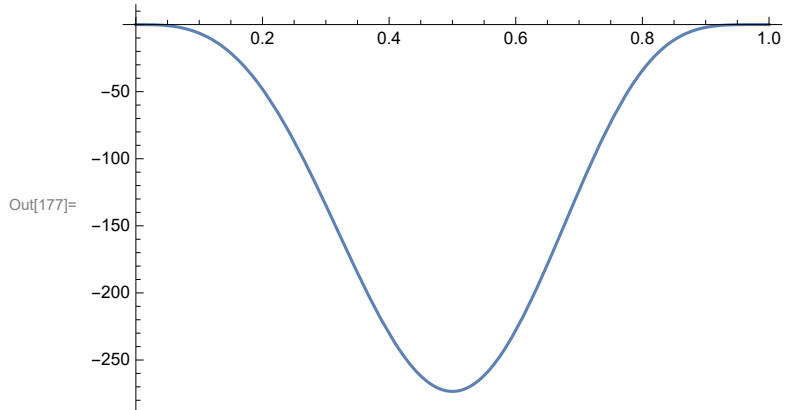

In[178]:= **Plot**[**Cf**[13, 14, 7], {x, 0, 1}]

[绘图](#)

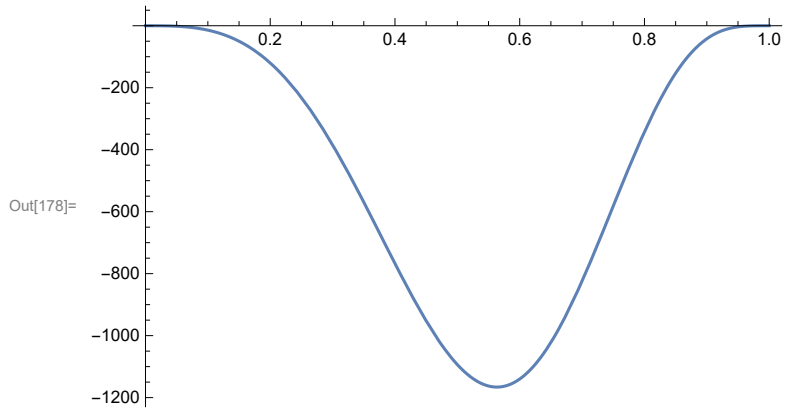

In[179]:= **Plot**[**Cf**[13, 14, 6], {x, 0, 1}]

[绘图](#)

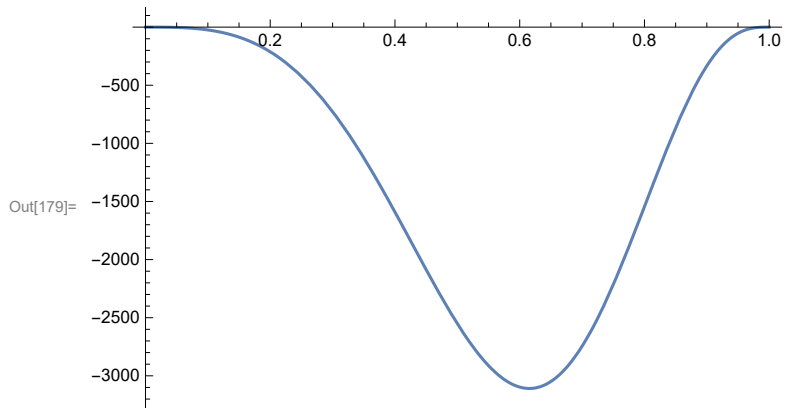

In[180]:= **Plot[Cf[13, 14, 5], {x, 0, 1}]**

[绘图](#)

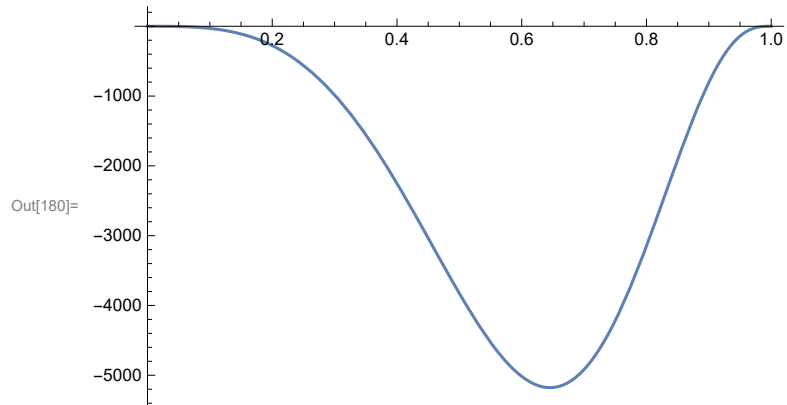

In[181]:= **Plot[Cf[13, 14, 4], {x, 0, 1}]**

[绘图](#)

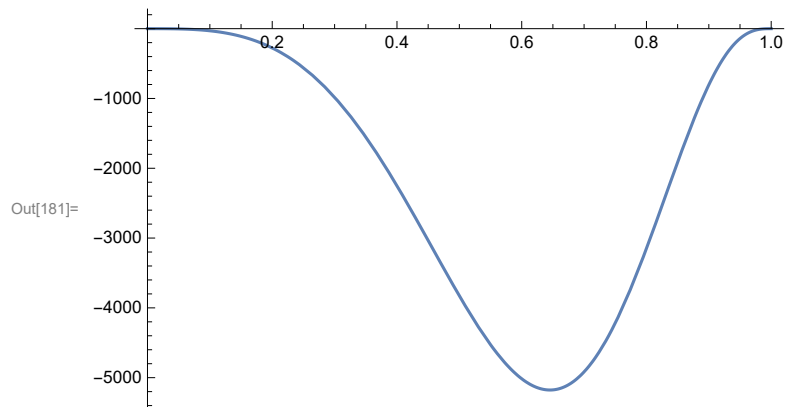

In[182]:= **Plot[Cf[13, 14, 3], {x, 0, 1}]**

[绘图](#)

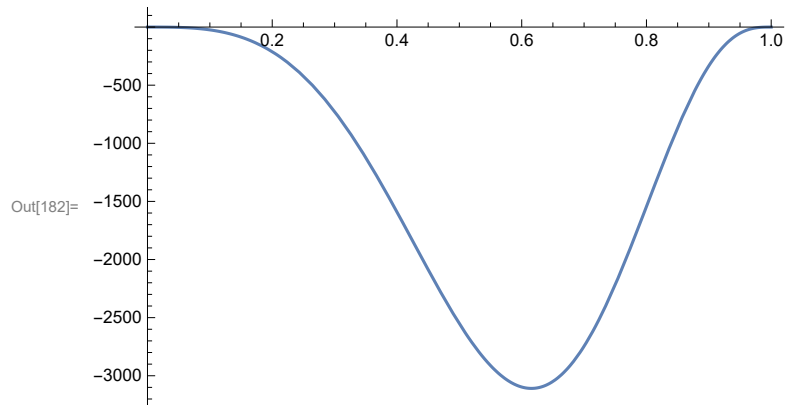



In[183]:= **Plot[Cf[13, 14, 2], {x, 0, 1}]**

[绘图](#)

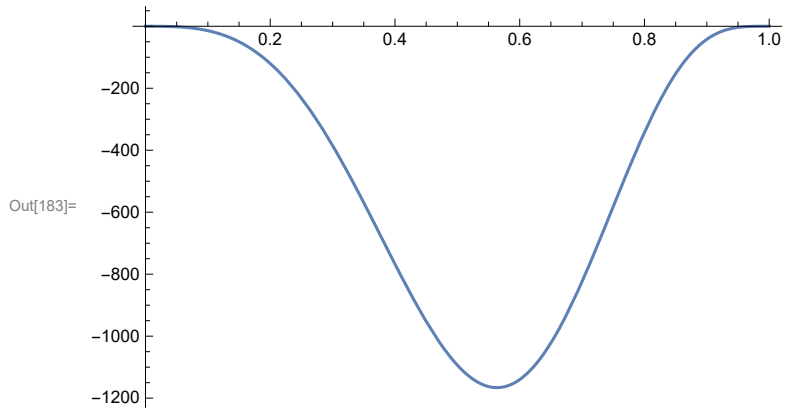

In[184]:= **Plot[Cf[13, 14, 1], {x, 0, 1}]**

[绘图](#)

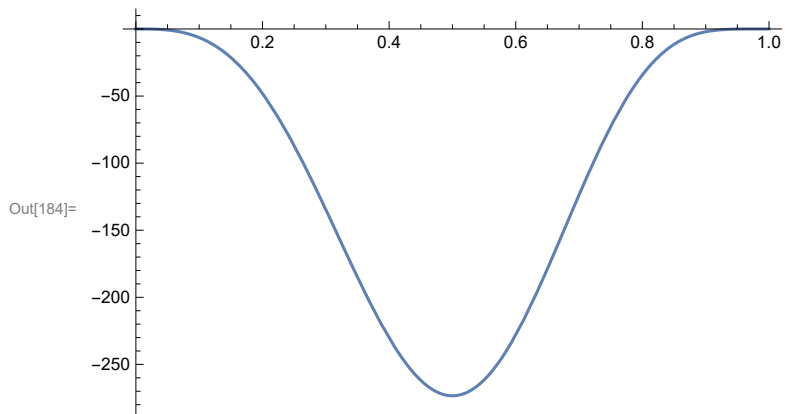

In[185]:= **Plot[Cf[13, 14, 0], {x, 0, 1}]**

[绘图](#)

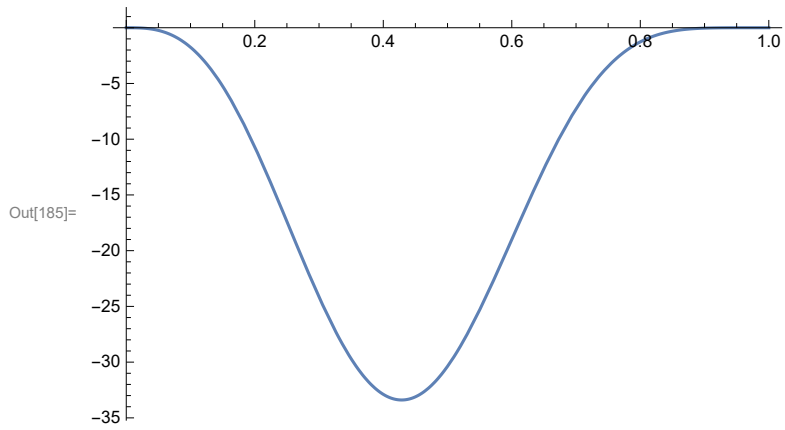

(\*17th group coefficients r2^13r3^13\*)

**Plot[Cf[13, 13, 14], {x, 0, 1}]**

[绘图](#)

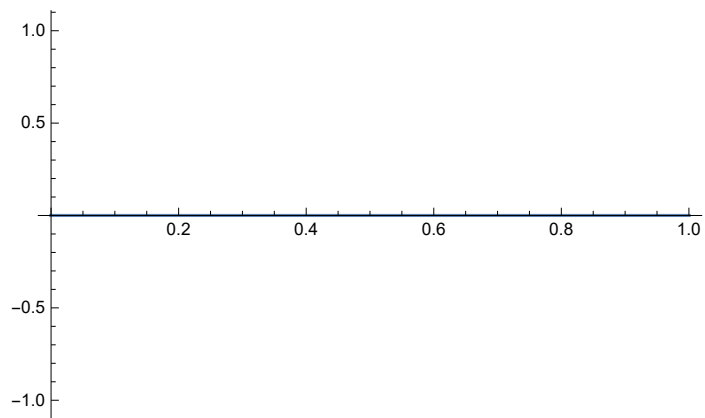

**Plot[Cf[13, 13, 13], {x, 0, 1}]**

[绘图](#)

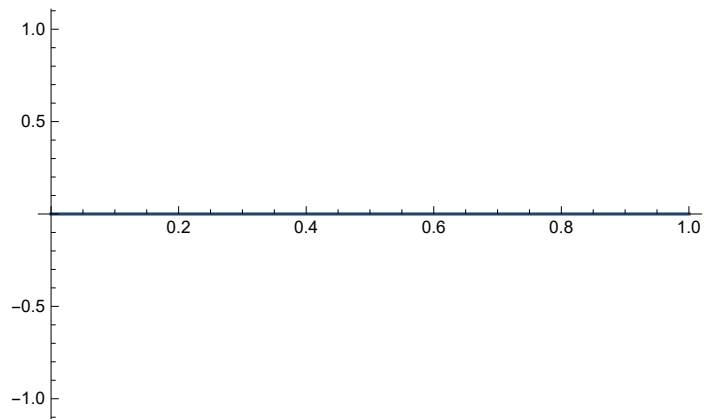

**Plot[Cf[13, 13, 12], {x, 0, 1}]**

[绘图](#)

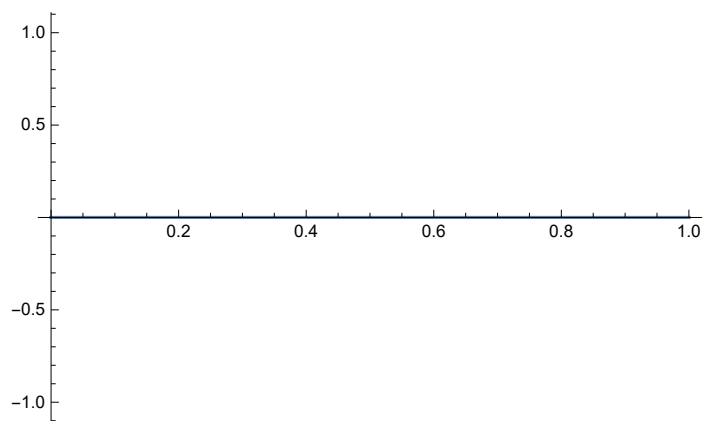

**Plot[Cf[13, 13, 11], {x, 0, 1}]**

[绘图](#)

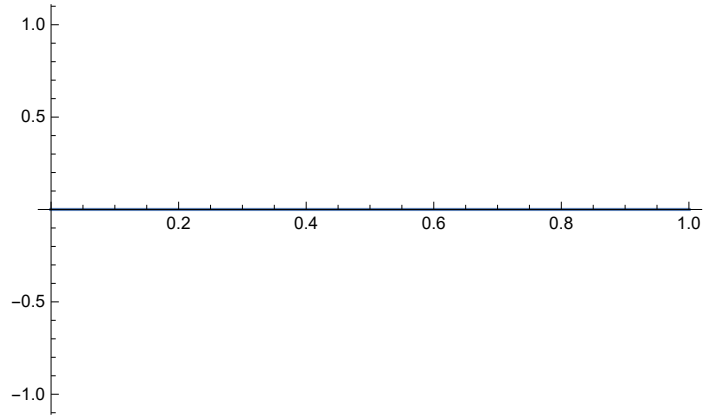

In[186]:= **Plot[Cf[13, 13, 10], {x, 0, 1}]**

[绘图](#)

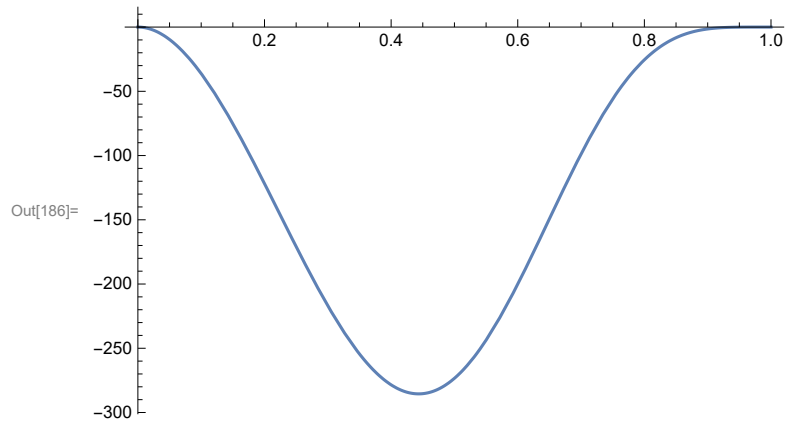

In[187]:= **Plot[Cf[13, 13, 9], {x, 0, 1}]**

[绘图](#)

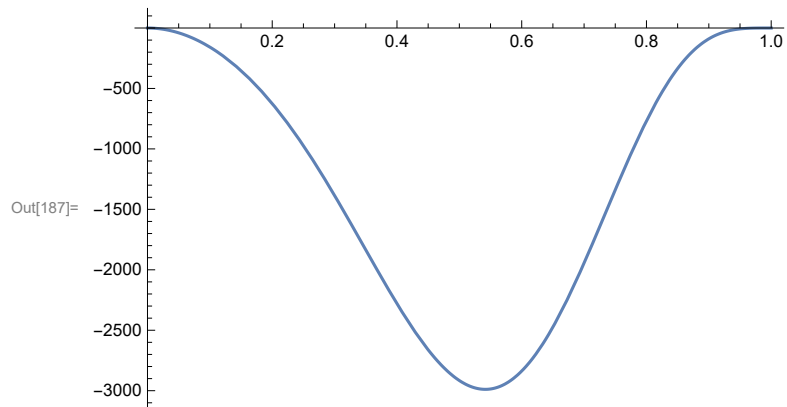

In[188]:= **Plot[Cf[13, 13, 8], {x, 0, 1}]**

[绘图](#)

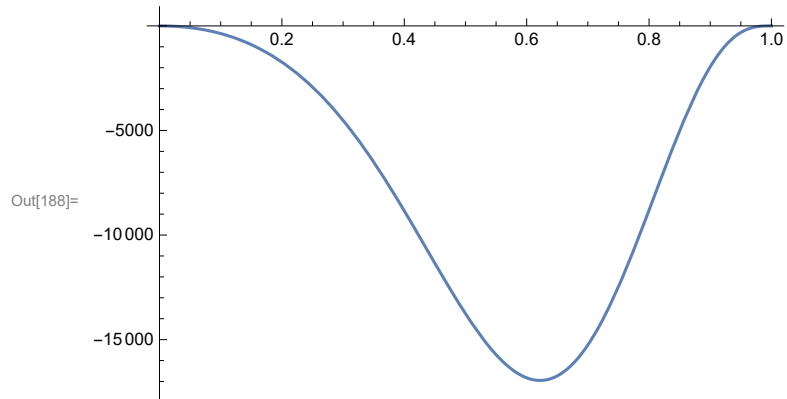

In[189]:= **Plot[Cf[13, 13, 7], {x, 0, 1}]**

[绘图](#)

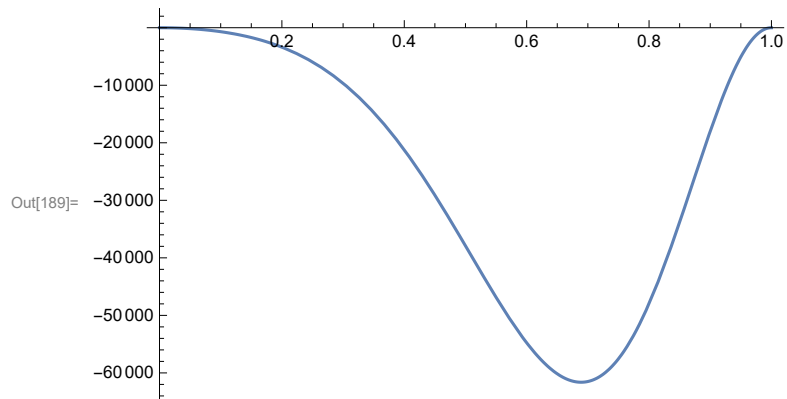

In[190]:= **Plot[Cf[13, 13, 6], {x, 0, 1}]**

[绘图](#)

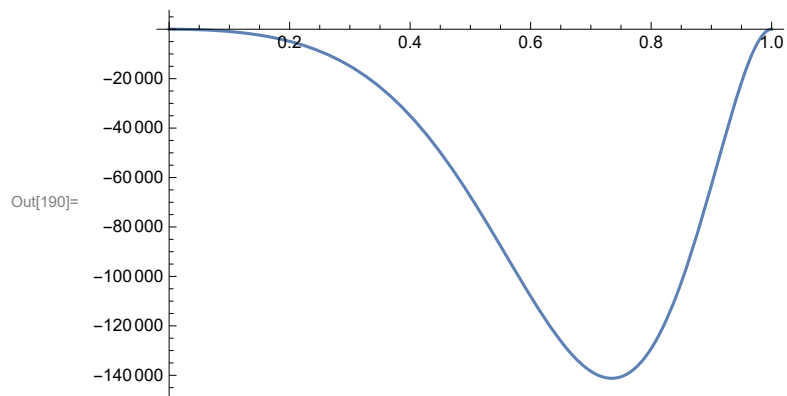

In[191]:= **Plot**[**Cf**[13, 13, 5], {x, 0, 1}]

[绘图](#)

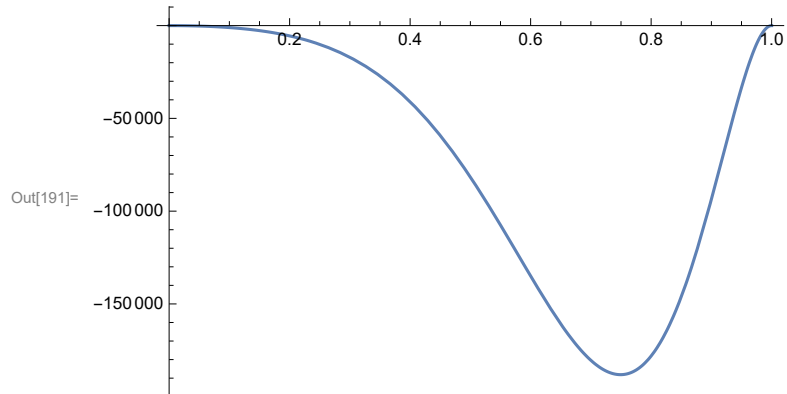

In[192]:= **Plot**[**Cf**[13, 13, 4], {x, 0, 1}]

[绘图](#)

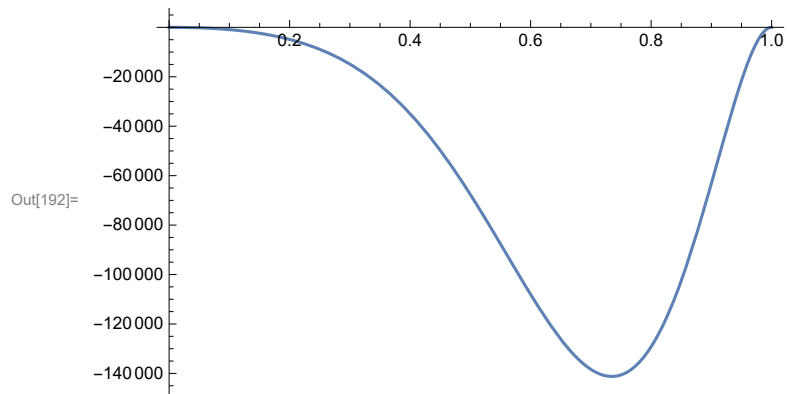

In[193]:= **Plot**[**Cf**[13, 13, 3], {x, 0, 1}]

[绘图](#)

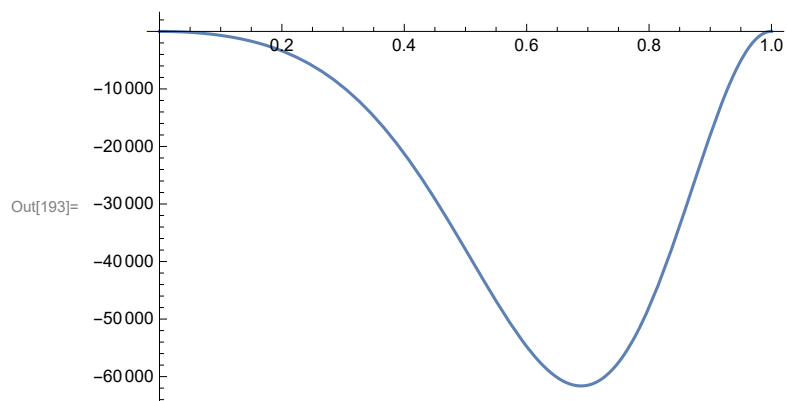

In[194]:= **Plot[Cf[13, 13, 2], {x, 0, 1}]**

[绘图](#)

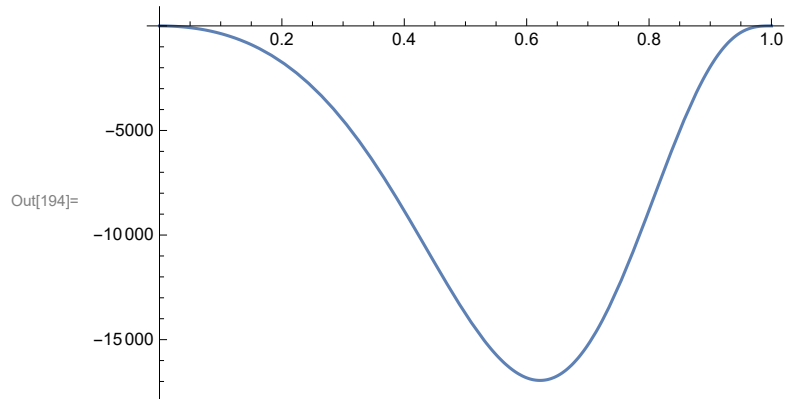

In[195]:= **Plot[Cf[13, 13, 1], {x, 0, 1}]**

[绘图](#)

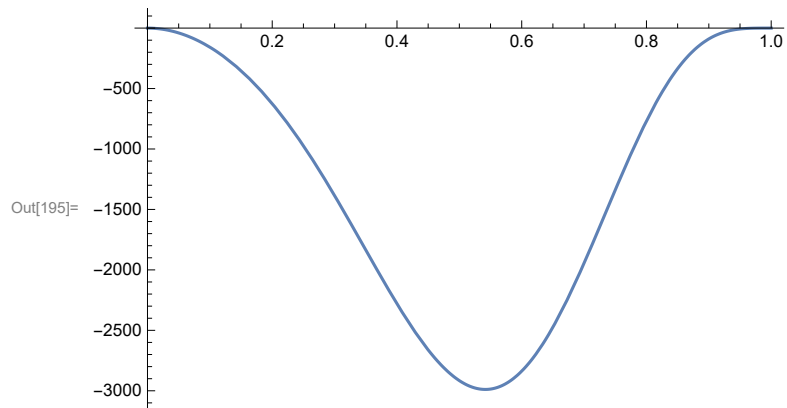

In[196]:= **Plot[Cf[13, 13, 0], {x, 0, 1}]**

[绘图](#)

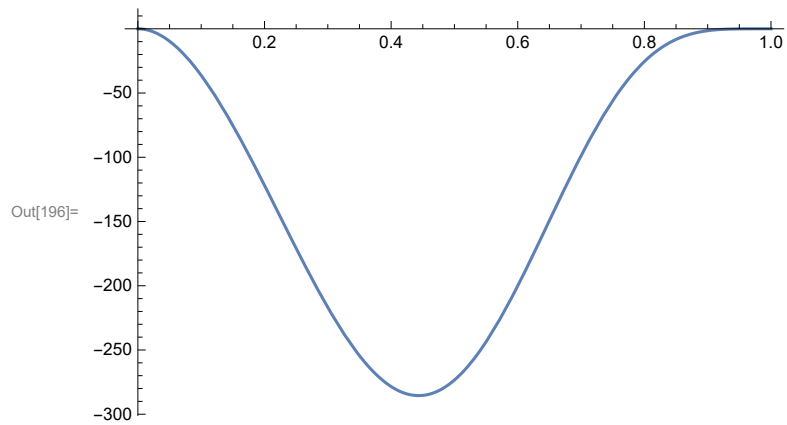

(\*18th group coefficients r2^13r3^12\*)

**Plot[Cf[13, 12, 14], {x, 0, 1}]**

[绘图](#)

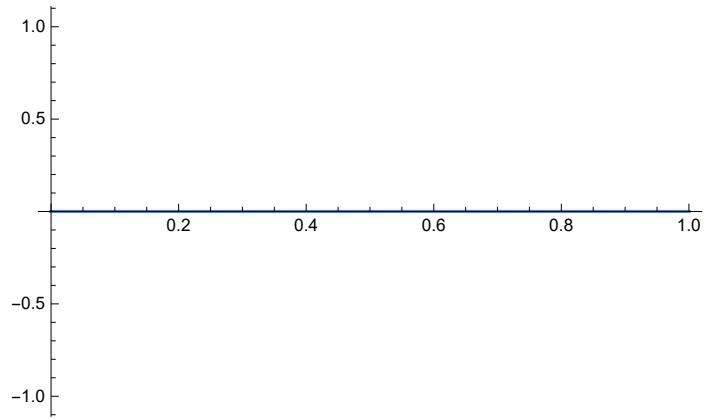

**Plot[Cf[13, 12, 13], {x, 0, 1}]**

[绘图](#)

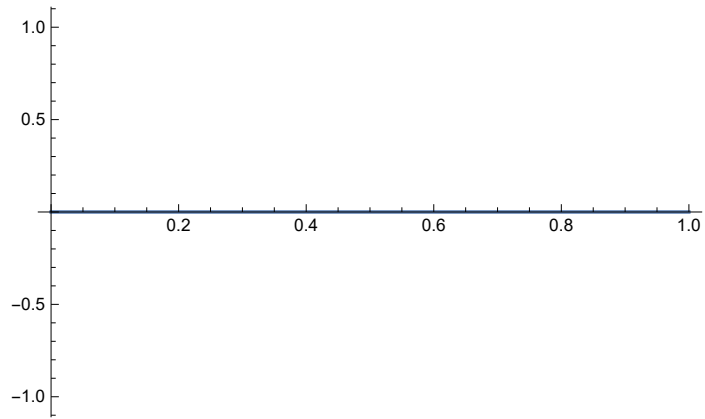

**Plot[Cf[13, 12, 12], {x, 0, 1}]**

[绘图](#)

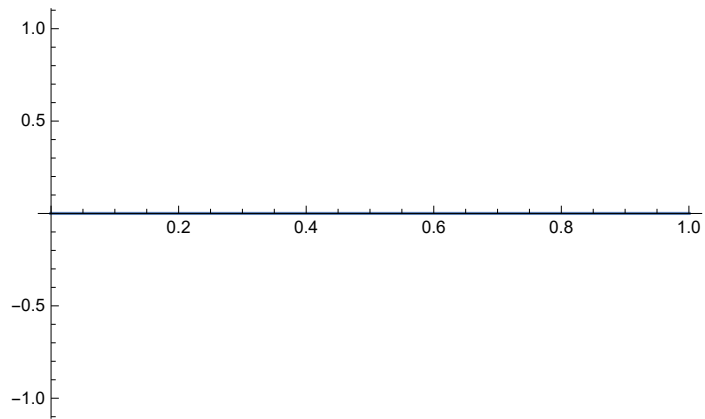

In[197]:= **Plot**[**Cf**[13, 12, 11], {x, 0, 1}]

[绘图](#)

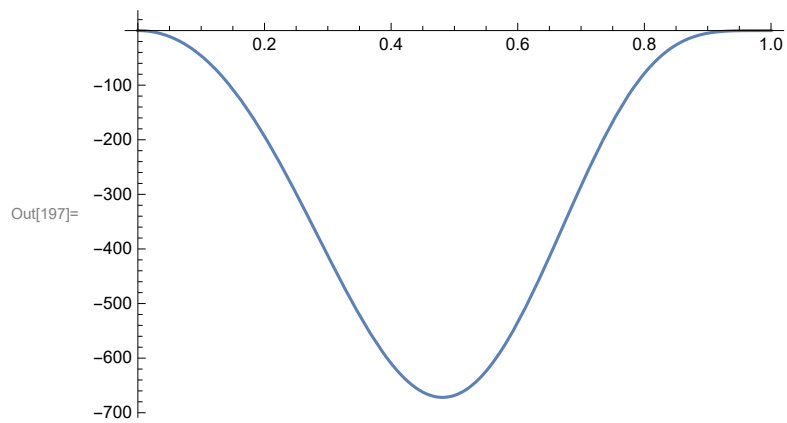

In[199]:= **Plot**[**Cf**[13, 12, 10], {x, 0, 1}]

[绘图](#)

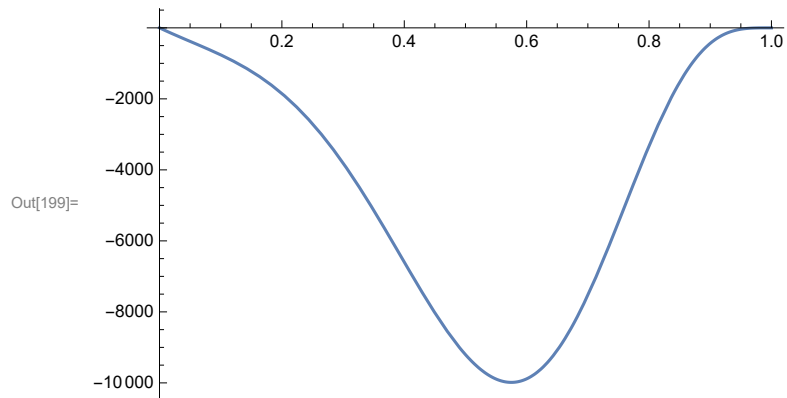

In[200]:= **Plot**[**Cf**[13, 12, 9], {x, 0, 1}]

[绘图](#)

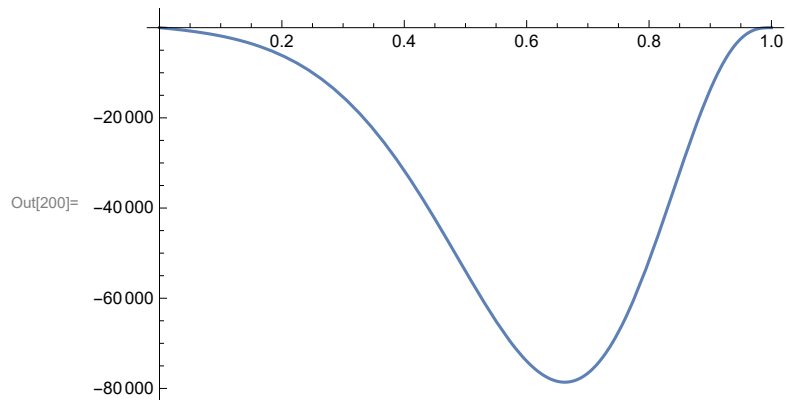



In[202]:= **Plot[Cf[13, 12, 8], {x, 0, 1}]**

[绘图](#)

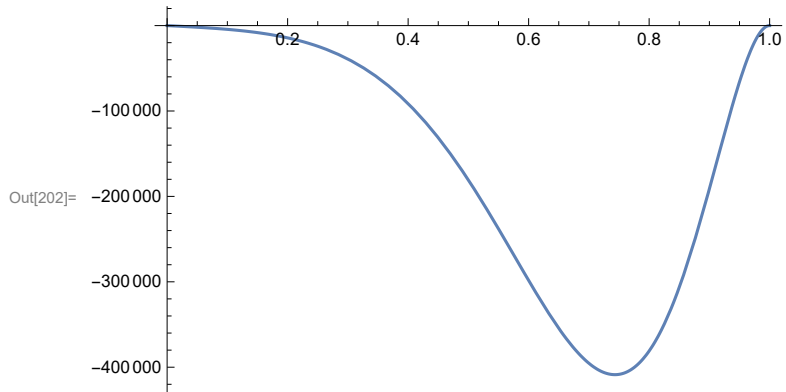

In[203]:= **Plot[Cf[13, 12, 7], {x, 0, 1}]**

[绘图](#)

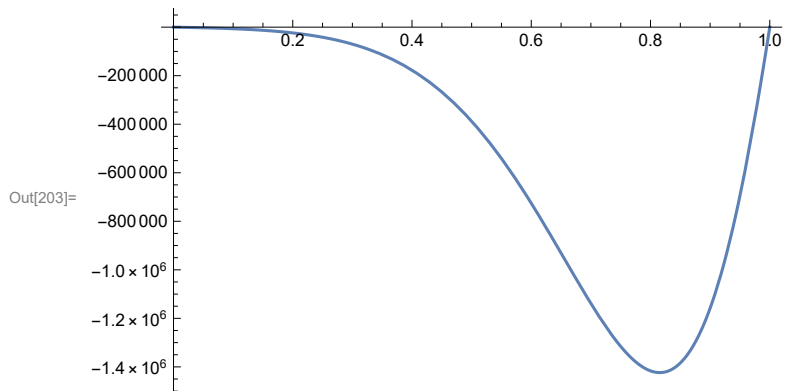

In[205]:= **Plot[Cf[13, 12, 6], {x, 0, 1}]**

[绘图](#)

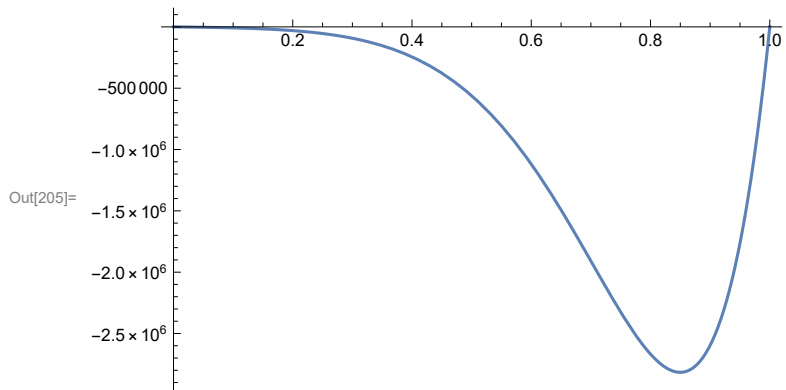

In[206]:= **Plot[Cf[13, 12, 5], {x, 0, 1}]**

[绘图](#)

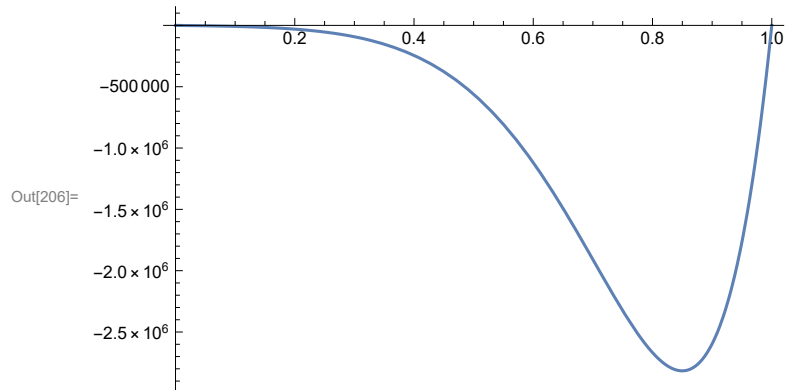

In[207]:= **Plot[Cf[13, 12, 4], {x, 0, 1}]**

[绘图](#)

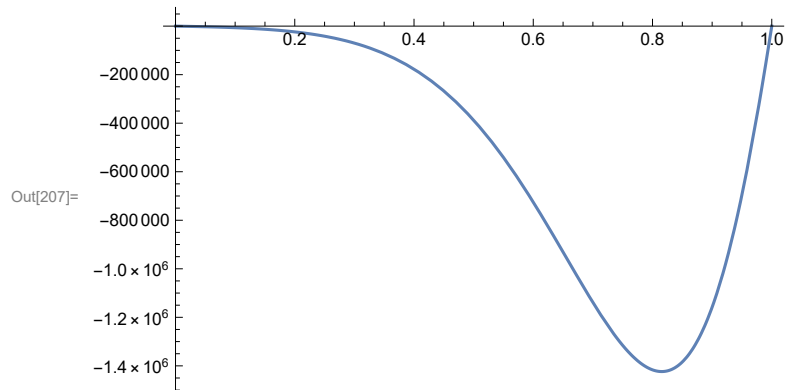

In[208]:= **Plot[Cf[13, 12, 3], {x, 0, 1}]**

[绘图](#)

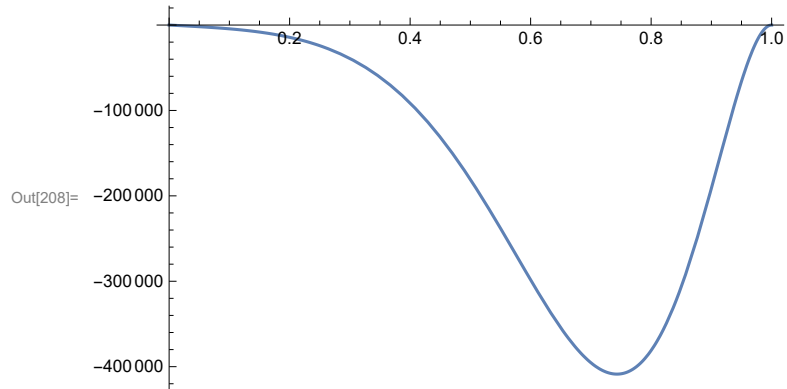

In[209]:= **Plot[Cf[13, 12, 2], {x, 0, 1}]**

[绘图](#)

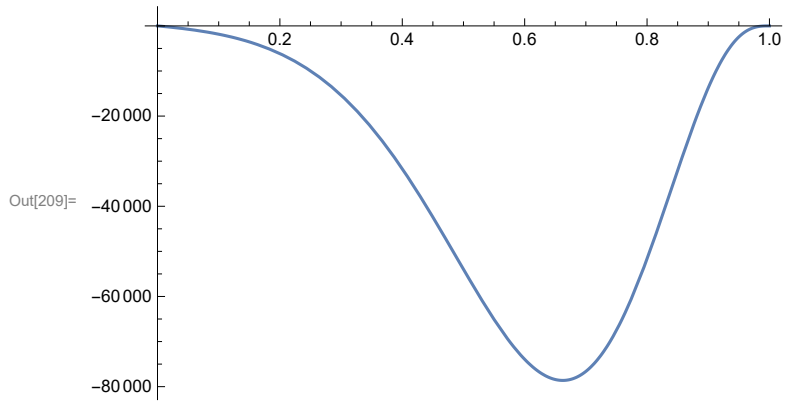

In[210]:= **Plot[Cf[13, 12, 1], {x, 0, 1}]**

[绘图](#)

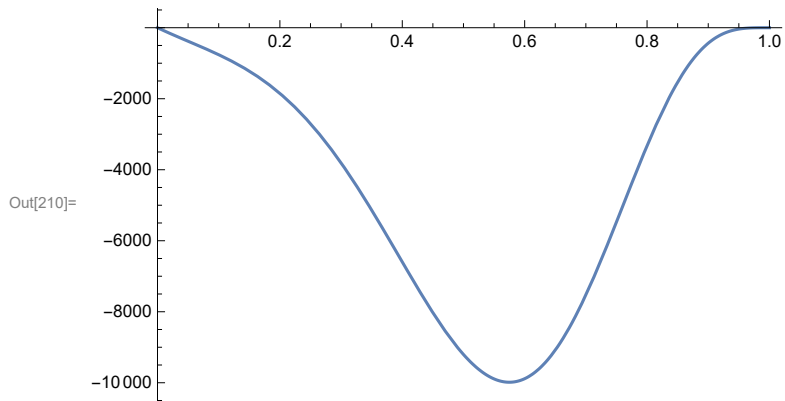

In[211]:= **Plot[Cf[13, 12, 0], {x, 0, 1}]**

[绘图](#)

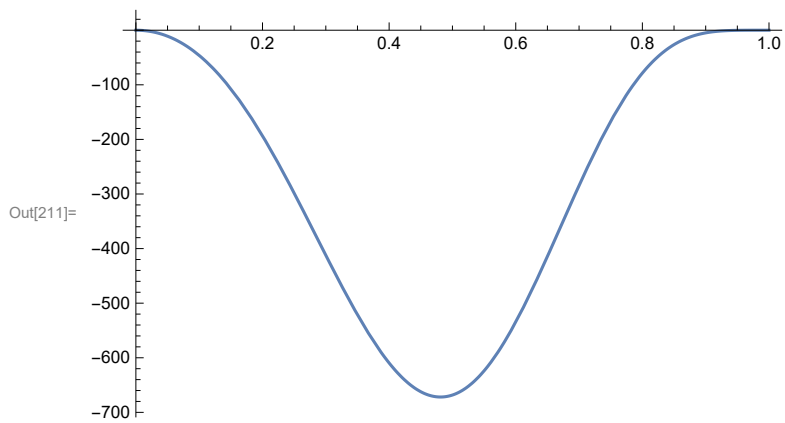

(\*19th group coefficients r2^13r3^11\*)

In[212]:= **Plot**[**Cf**[13, 11, 14], {x, 0, 1}]

[绘图](#)

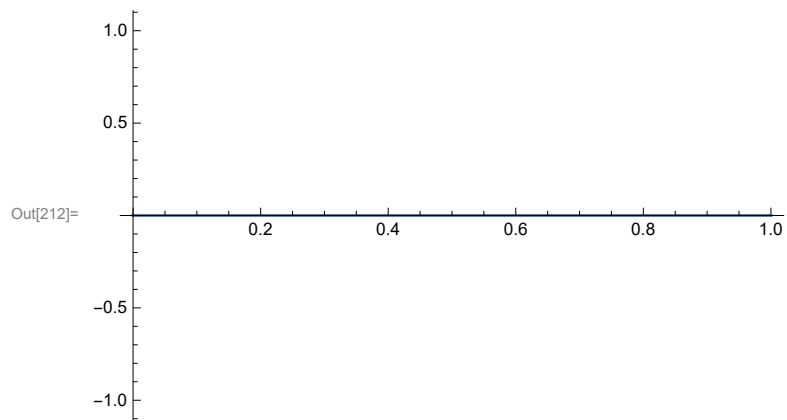

**Plot**[**Cf**[13, 11, 13], {x, 0, 1}]

[绘图](#)

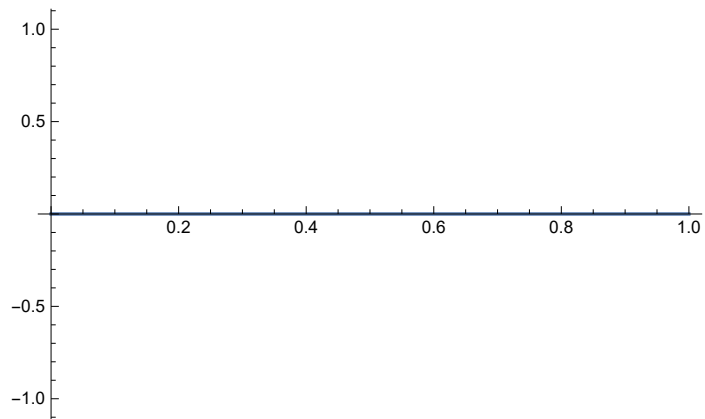

In[213]:= **Plot**[**Cf**[13, 11, 12], {x, 0, 1}]

[绘图](#)

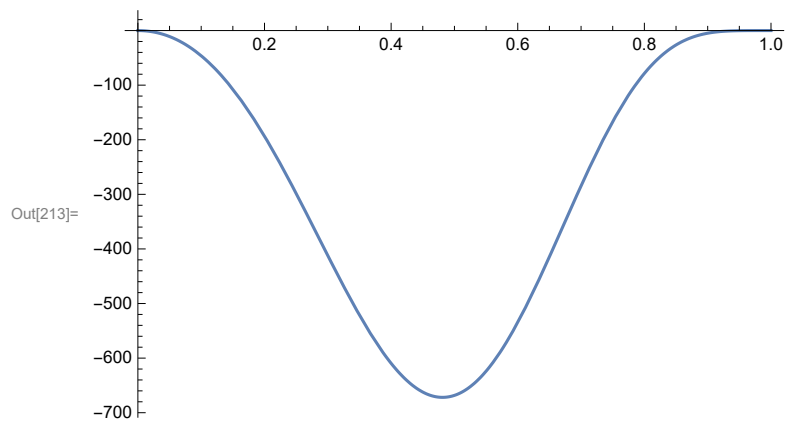

In[214]:= **Plot[Cf[13, 11, 11], {x, 0, 1}]**

[绘图](#)

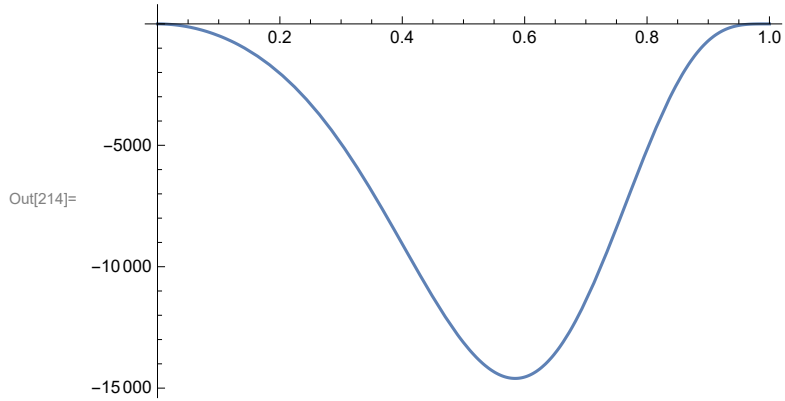

In[215]:= **Plot[Cf[13, 11, 10], {x, 0, 1}]**

[绘图](#)

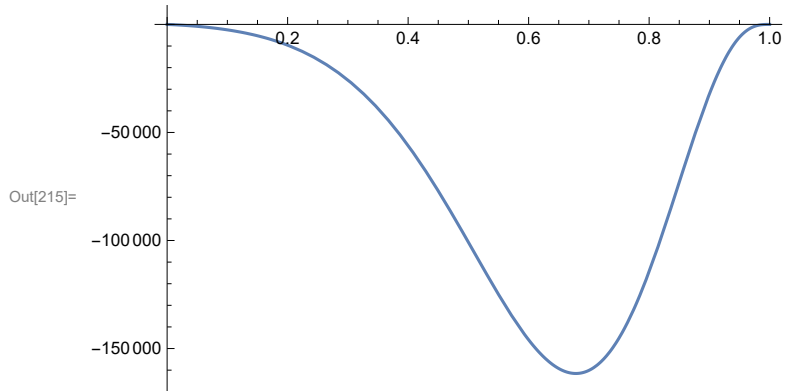

In[216]:= **Plot[Cf[13, 11, 9], {x, 0, 1}]**

[绘图](#)

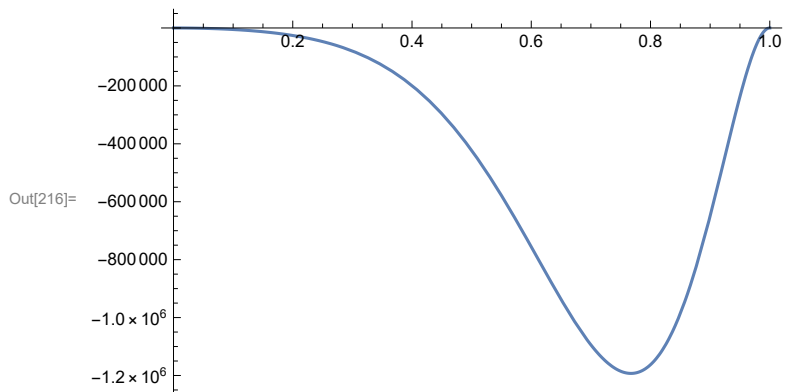

In[217]:= **Plot[Cf[13, 11, 8], {x, 0, 1}]**

[绘图](#)

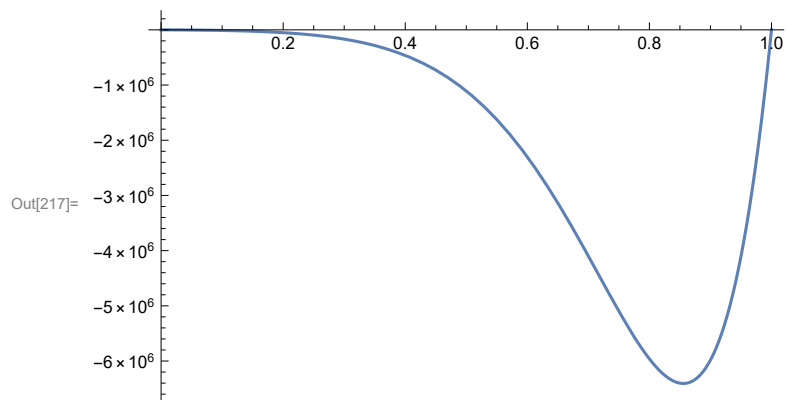

In[218]:= **Plot[Cf[13, 11, 7], {x, 0, 1}]**

[绘图](#)

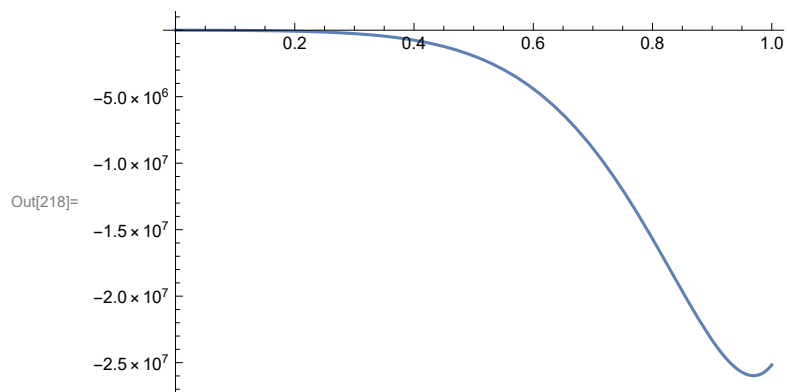

In[219]:= **Plot[Cf[13, 11, 6], {x, 0, 1}]**

[绘图](#)

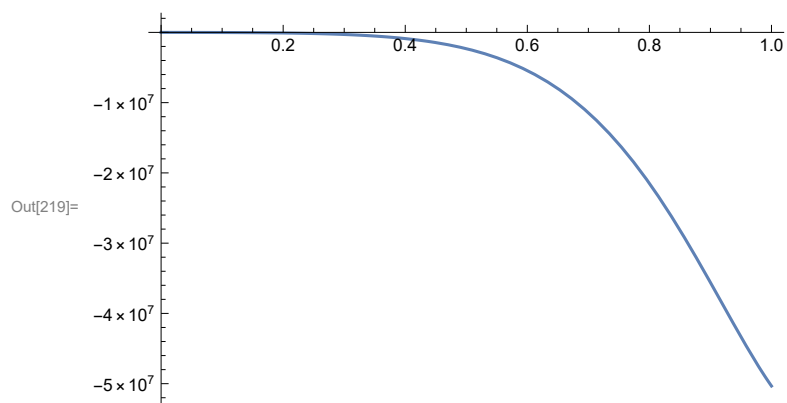

In[220]:= **Plot[Cf[13, 11, 5], {x, 0, 1}]**

[绘图](#)

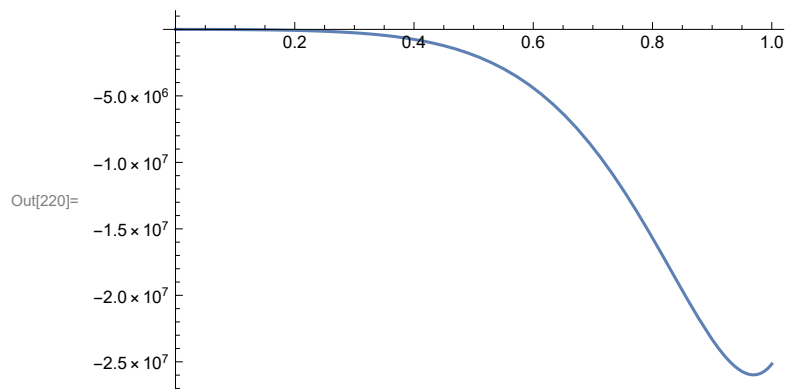

In[221]:= **Plot[Cf[13, 11, 4], {x, 0, 1}]**

[绘图](#)

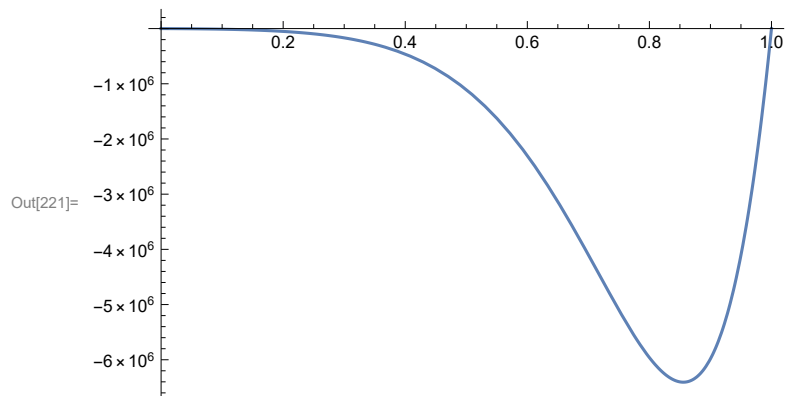

In[222]:= **Plot[Cf[13, 11, 3], {x, 0, 1}]**

[绘图](#)

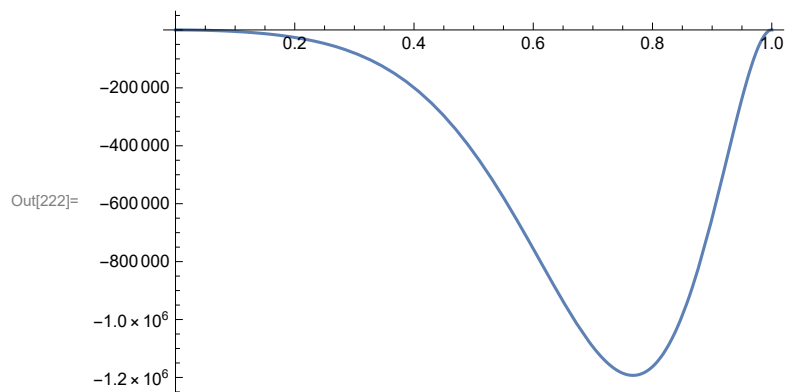

In[223]:= **Plot[Cf[13, 11, 2], {x, 0, 1}]**

[绘图](#)

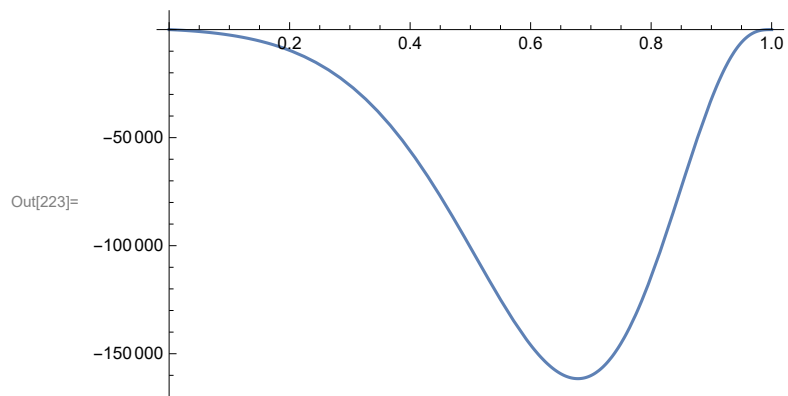

In[224]:= **Plot[Cf[13, 11, 1], {x, 0, 1}]**

[绘图](#)

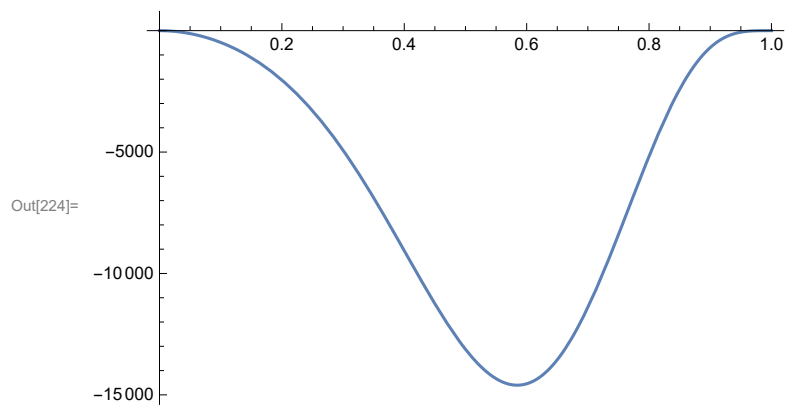

In[225]:= **Plot[Cf[13, 11, 0], {x, 0, 1}]**

[绘图](#)

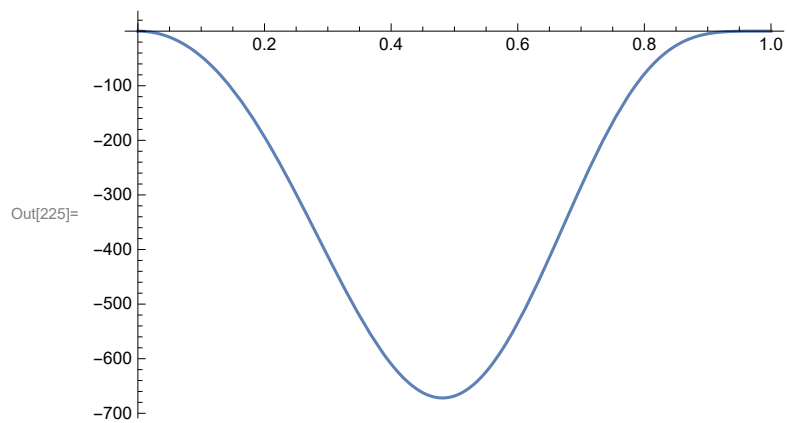

(\*20th group coefficients  $r^2 r^3$ \*)



**Plot[Cf[13, 10, 14], {x, 0, 1}]**

[绘图](#)

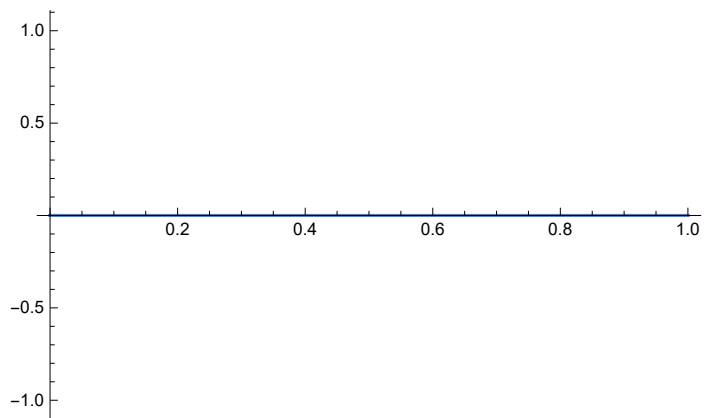

In[226]:= **Plot[Cf[13, 10, 13], {x, 0, 1}]**

[绘图](#)

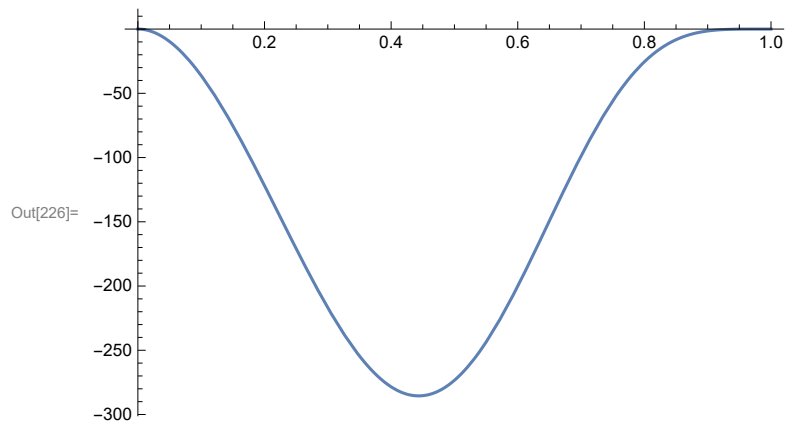

In[227]:= **Plot[Cf[13, 10, 12], {x, 0, 1}]**

[绘图](#)

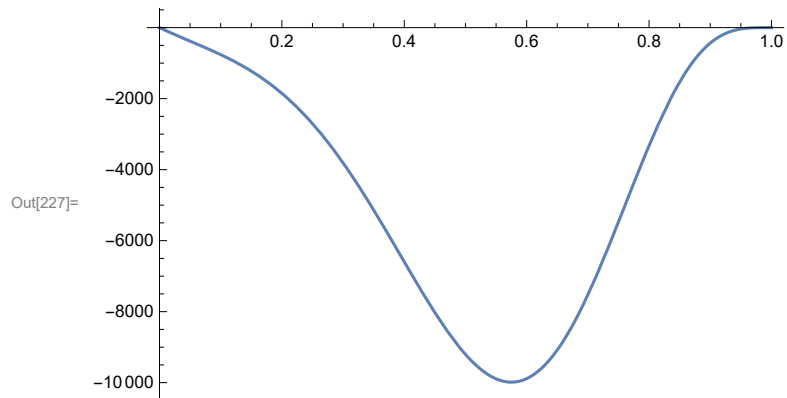

In[228]:= **Plot[Cf[13, 10, 11], {x, 0, 1}]**

[绘图](#)

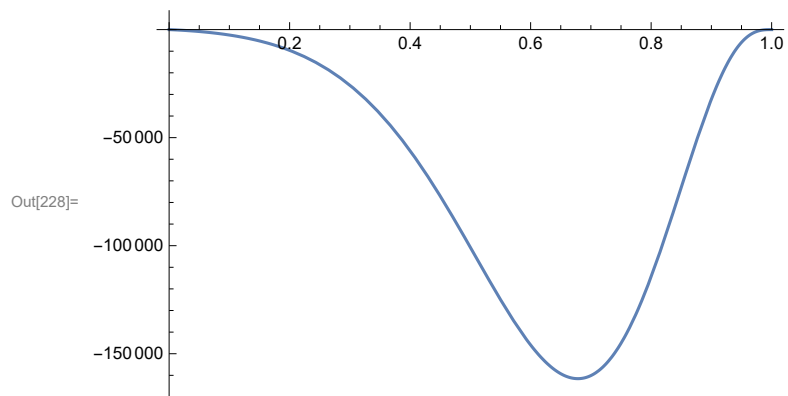

In[229]:= **Plot[Cf[13, 10, 10], {x, 0, 1}]**

[绘图](#)

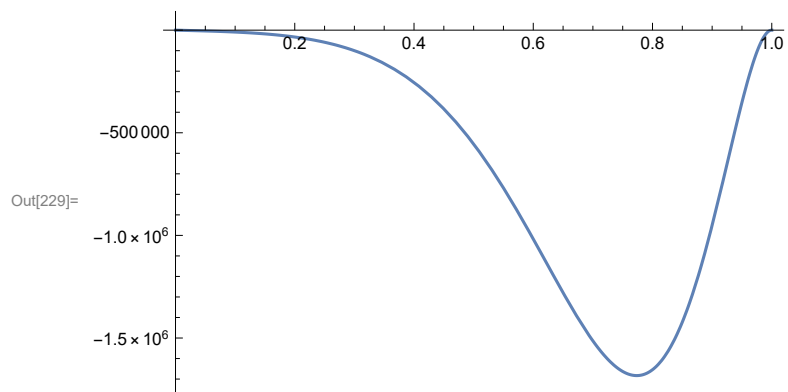

In[230]:= **Plot[Cf[13, 10, 9], {x, 0, 1}]**

[绘图](#)

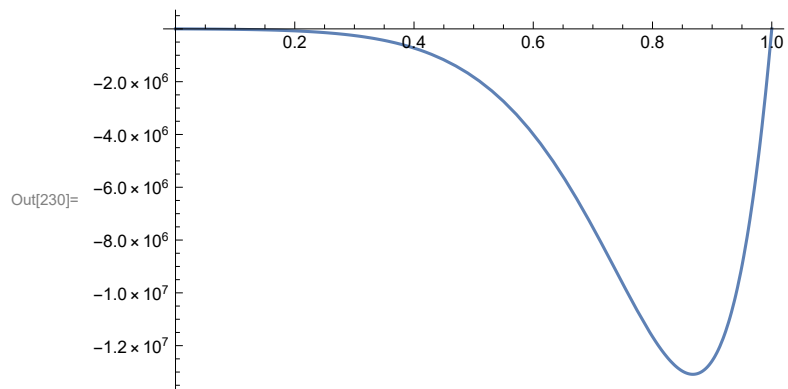

In[231]:= **Plot[Cf[13, 10, 8], {x, 0, 1}]**

[绘图](#)

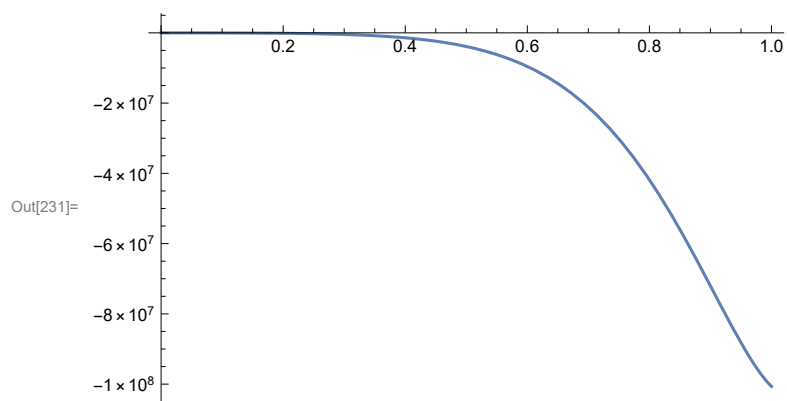

In[232]:= **Plot[Cf[13, 10, 7], {x, 0, 1}]**

[绘图](#)

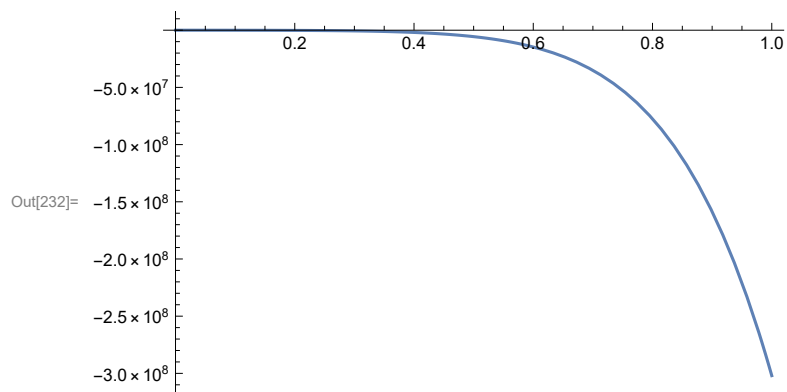

In[233]:= **Plot[Cf[13, 10, 6], {x, 0, 1}]**

[绘图](#)

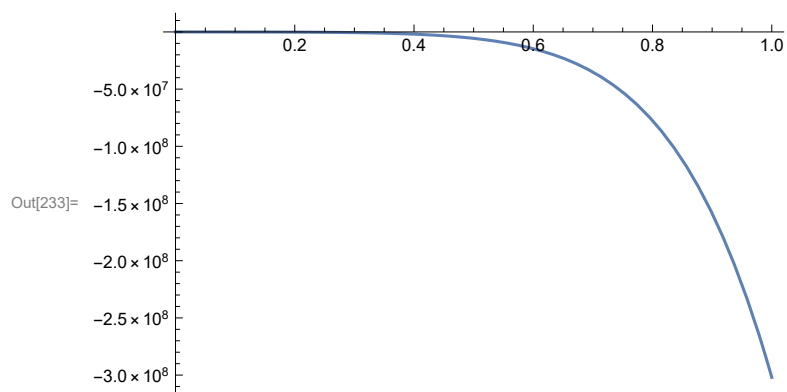

In[234]:= **Plot[Cf[13, 10, 5], {x, 0, 1}]**

[绘图](#)

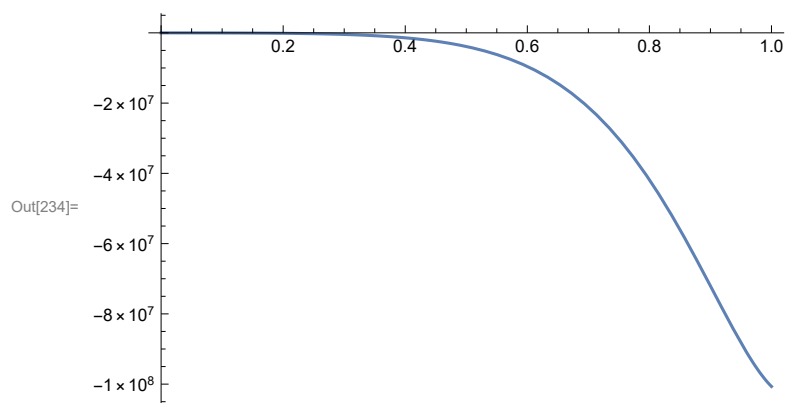

In[235]:= **Plot[Cf[13, 10, 4], {x, 0, 1}]**

[绘图](#)

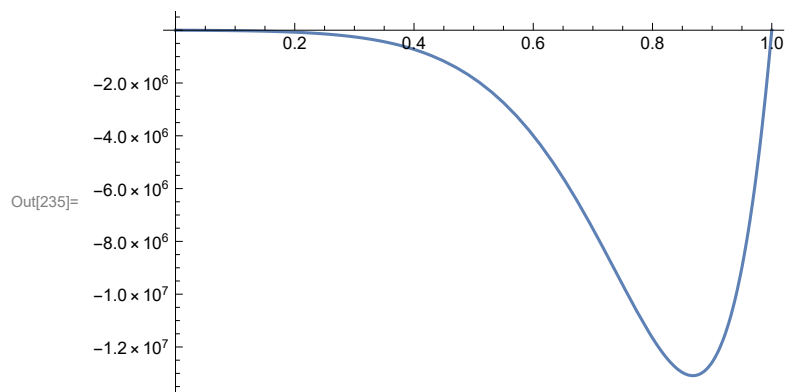

In[236]:= **Plot[Cf[13, 10, 3], {x, 0, 1}]**

[绘图](#)

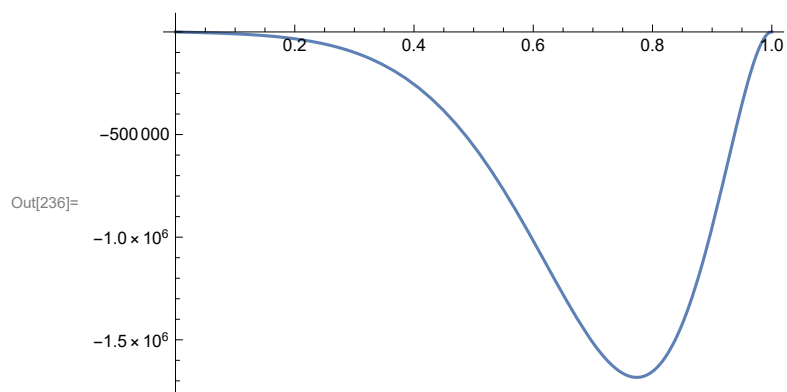

In[237]:= **Plot[Cf[13, 10, 2], {x, 0, 1}]**

[绘图](#)

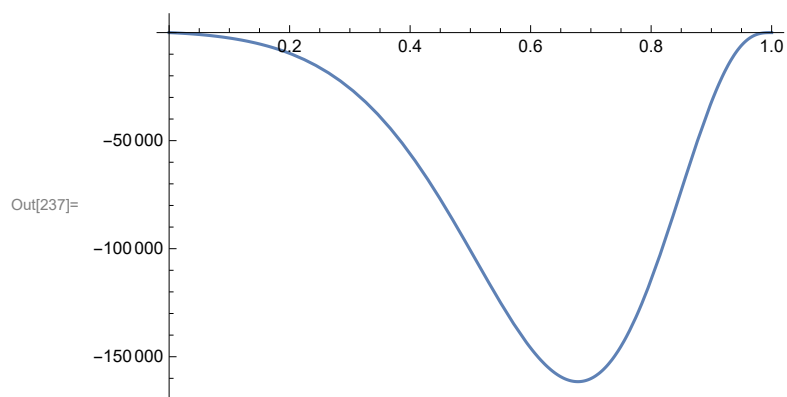

In[238]:= **Plot[Cf[13, 10, 1], {x, 0, 1}]**

[绘图](#)

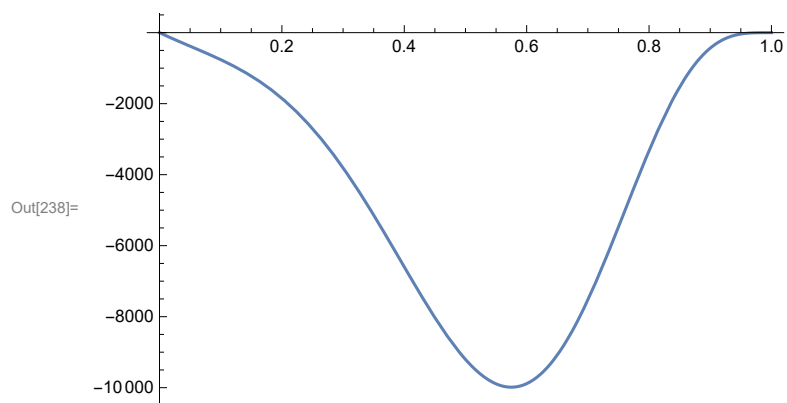

In[239]:= **Plot[Cf[13, 10, 0], {x, 0, 1}]**

[绘图](#)

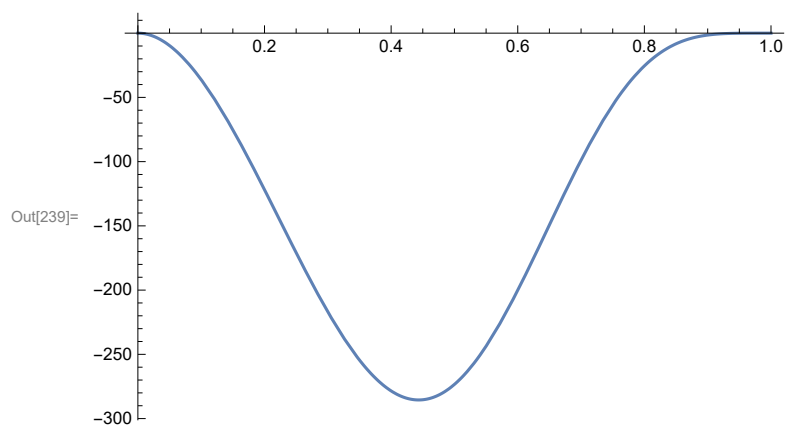

(\*21th group coefficients r2^13r3^9\*)

In[240]:= **Plot[Cf[13, 9, 14], {x, 0, 1}]**

[绘图](#)

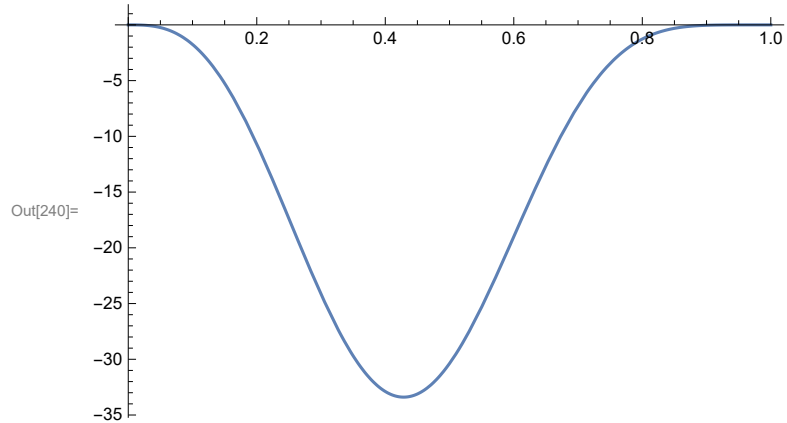

In[241]:= **Plot[Cf[13, 9, 13], {x, 0, 1}]**

[绘图](#)

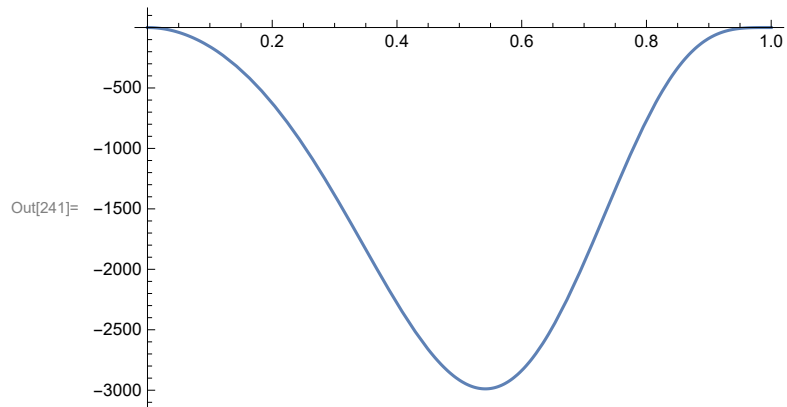

In[242]:= **Plot[Cf[13, 9, 12], {x, 0, 1}]**

[绘图](#)

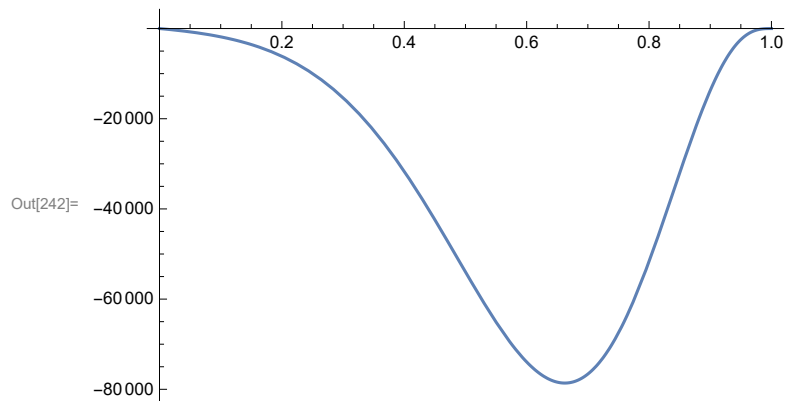

In[243]:= **Plot[Cf[13, 9, 11], {x, 0, 1}]**

[绘图](#)

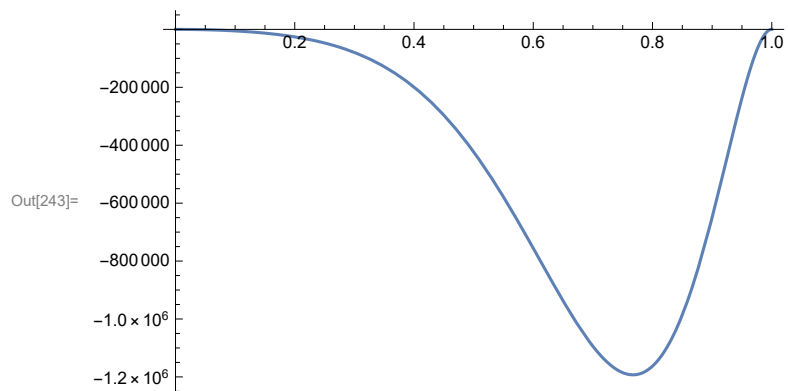

In[244]:= **Plot[Cf[13, 9, 10], {x, 0, 1}]**

[绘图](#)

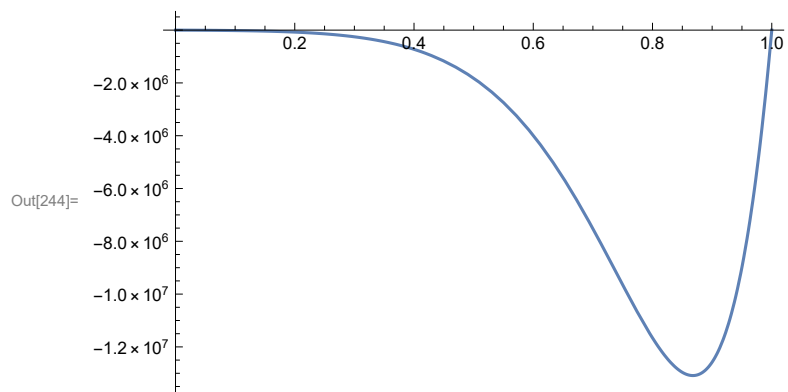

In[245]:= **Plot[Cf[13, 9, 9], {x, 0, 1}]**

[绘图](#)

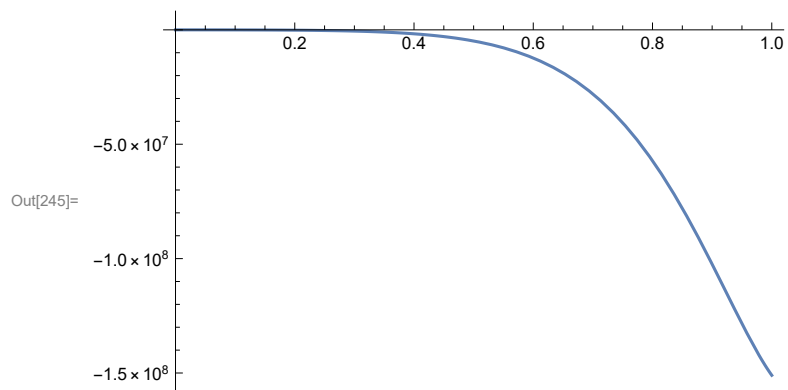

In[246]:= **Plot[Cf[13, 9, 8], {x, 0, 1}]**

[绘图](#)

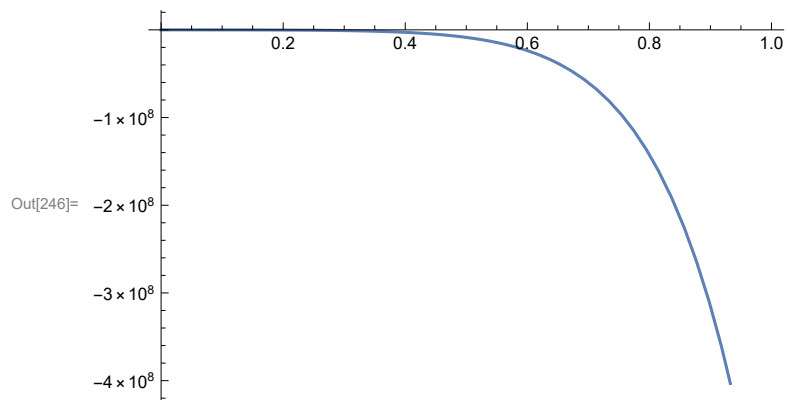

In[247]:= **Plot[Cf[13, 9, 7], {x, 0, 1}]**

[绘图](#)

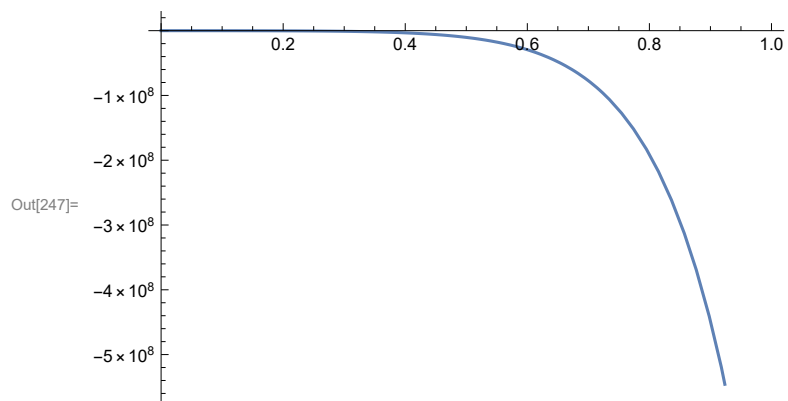

In[248]:= **Plot[Cf[13, 9, 6], {x, 0, 1}]**

[绘图](#)

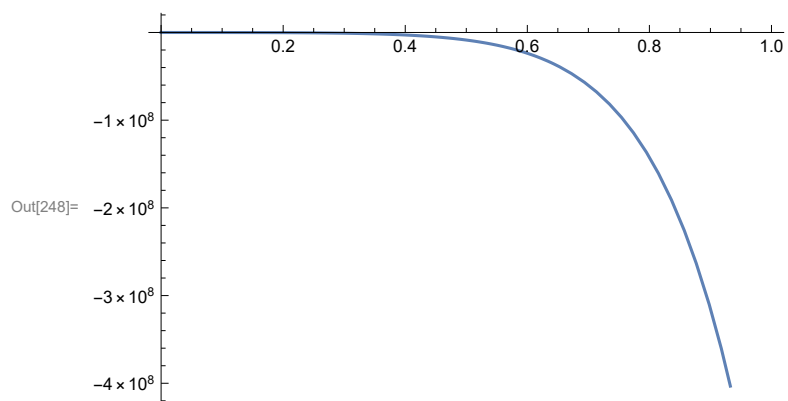



In[249]:= **Plot[Cf[13, 9, 5], {x, 0, 1}]**

[绘图](#)

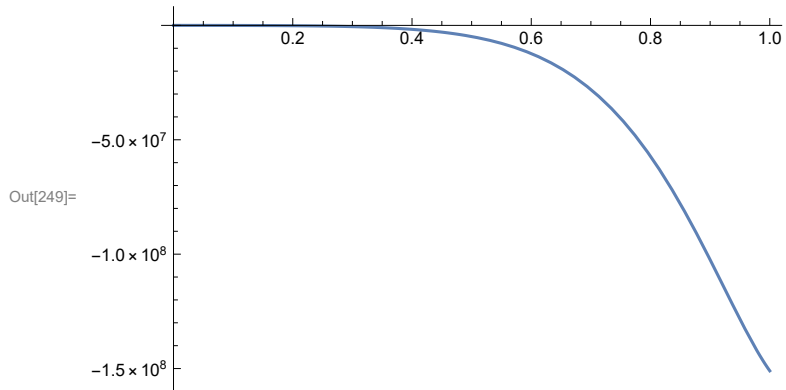

In[250]:= **Plot[Cf[13, 9, 4], {x, 0, 1}]**

[绘图](#)

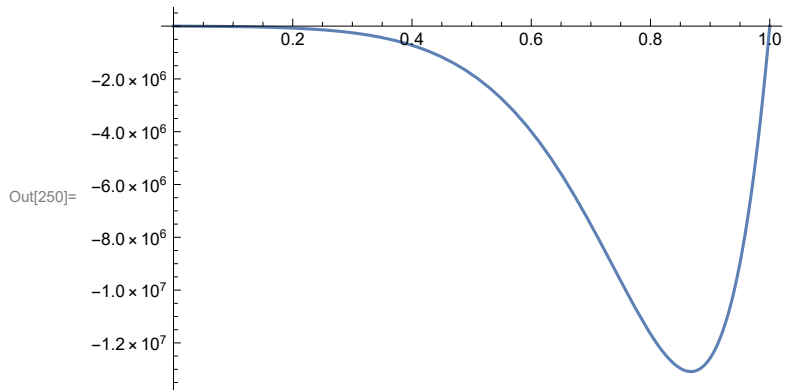

In[251]:= **Plot[Cf[13, 9, 3], {x, 0, 1}]**

[绘图](#)

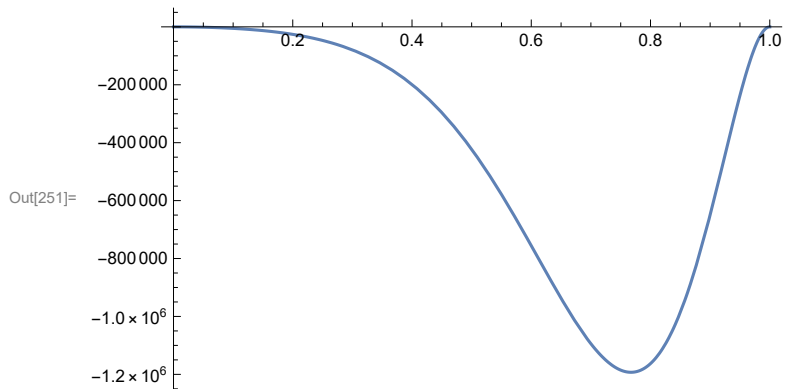

In[252]:= **Plot[Cf[13, 9, 2], {x, 0, 1}]**

[绘图](#)

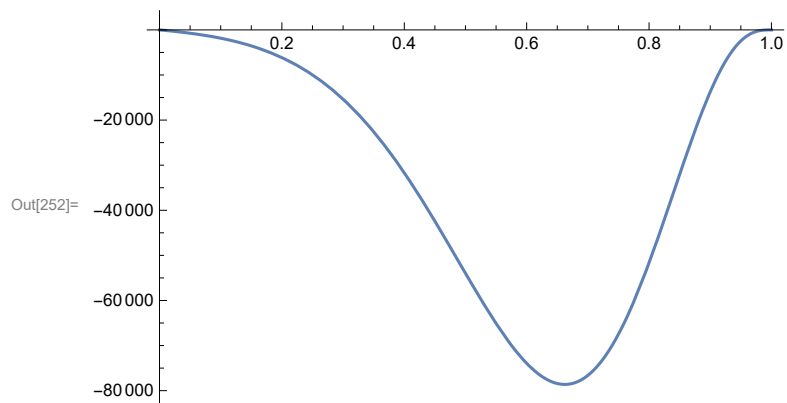

In[253]:= **Plot[Cf[13, 9, 1], {x, 0, 1}]**

[绘图](#)

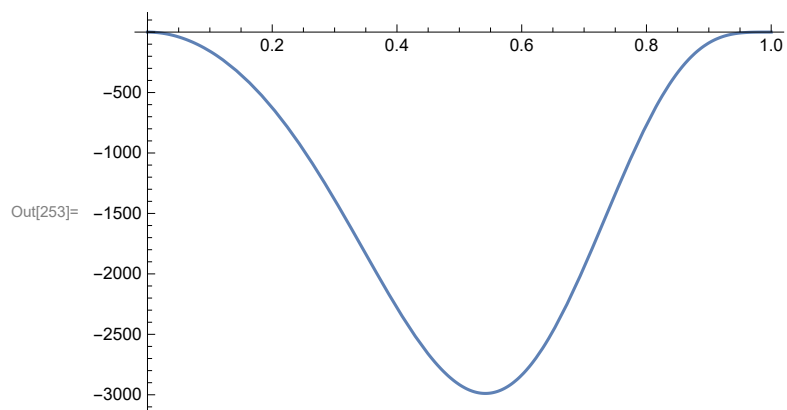

In[254]:= **Plot[Cf[13, 9, 0], {x, 0, 1}]**

[绘图](#)

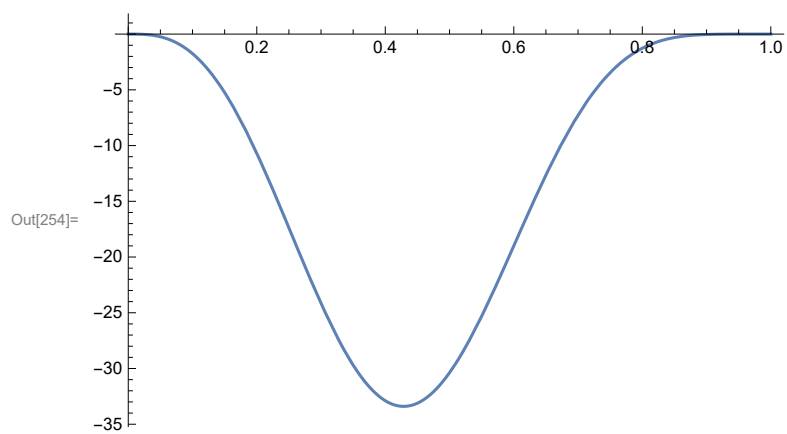

(\*22th group coefficients r2^13r3^8\*)

In[255]:= **Plot**[**Cf**[13, 8, 14], {x, 0, 1}]

[绘图](#)

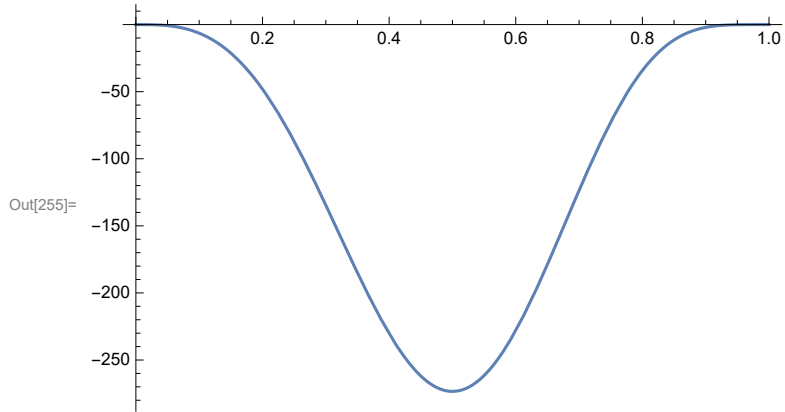

In[256]:= **Plot**[**Cf**[13, 8, 13], {x, 0, 1}]

[绘图](#)

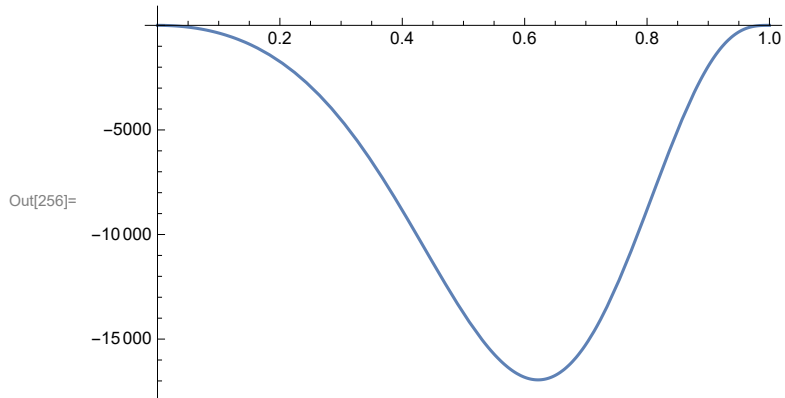

In[257]:= **Plot**[**Cf**[13, 8, 12], {x, 0, 1}]

[绘图](#)

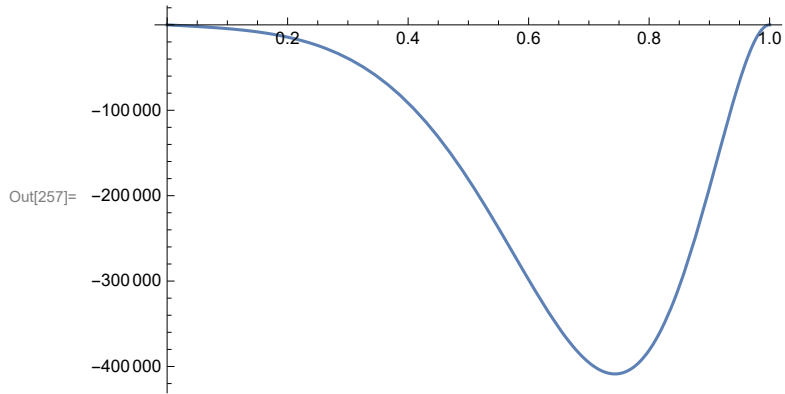

In[258]:= **Plot[Cf[13, 8, 11], {x, 0, 1}]**

[绘图](#)

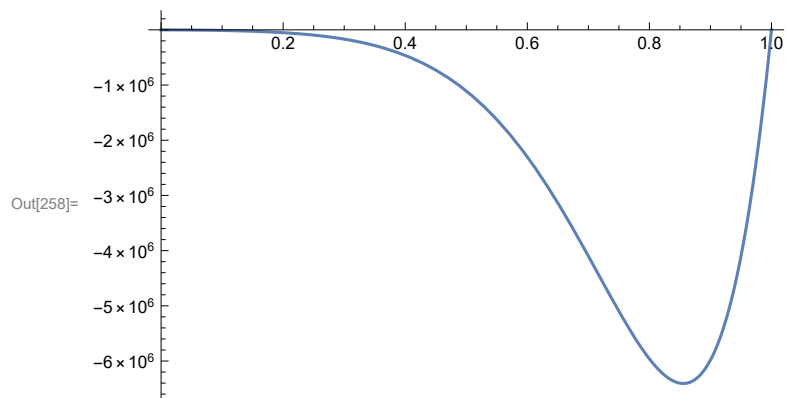

In[259]:= **Plot[Cf[13, 8, 10], {x, 0, 1}]**

[绘图](#)

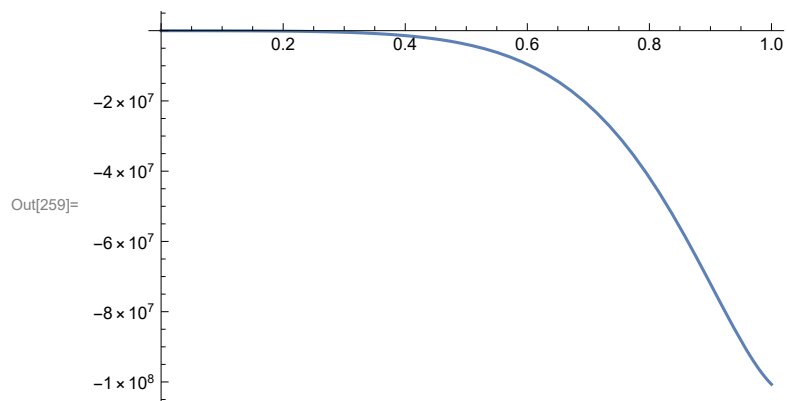

In[260]:= **Plot[Cf[13, 8, 9], {x, 0, 1}]**

[绘图](#)

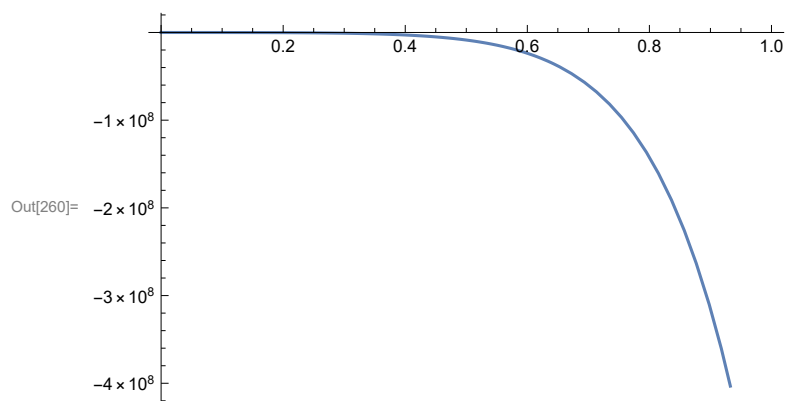

In[261]:= **Plot[Cf[13, 8, 8], {x, 0, 1}]**

[绘图](#)

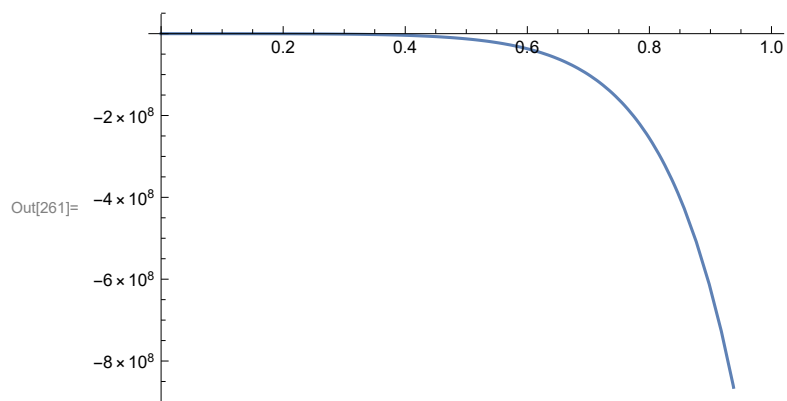

In[262]:= **Plot[Cf[13, 8, 7], {x, 0, 1}]**

[绘图](#)

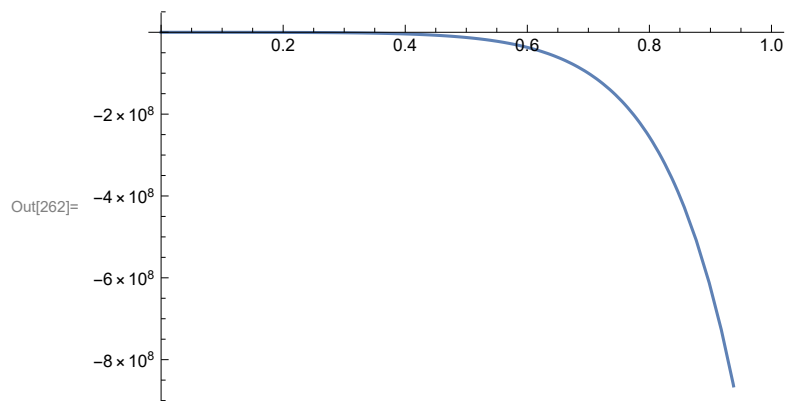

In[263]:= **Plot[Cf[13, 8, 6], {x, 0, 1}]**

[绘图](#)

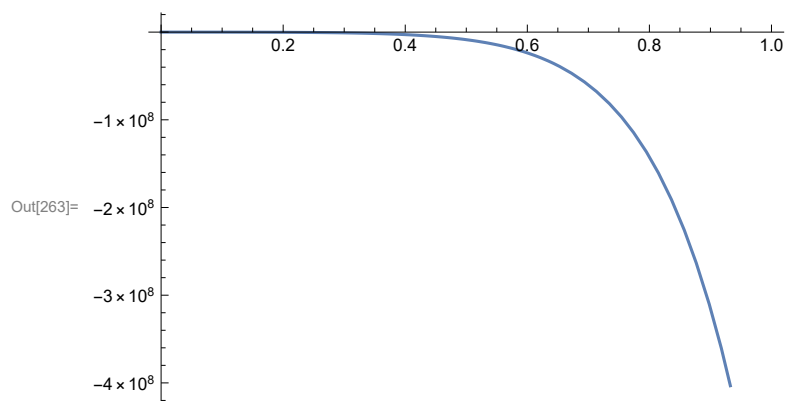

In[264]:= **Plot[Cf[13, 8, 5], {x, 0, 1}]**

[绘图](#)

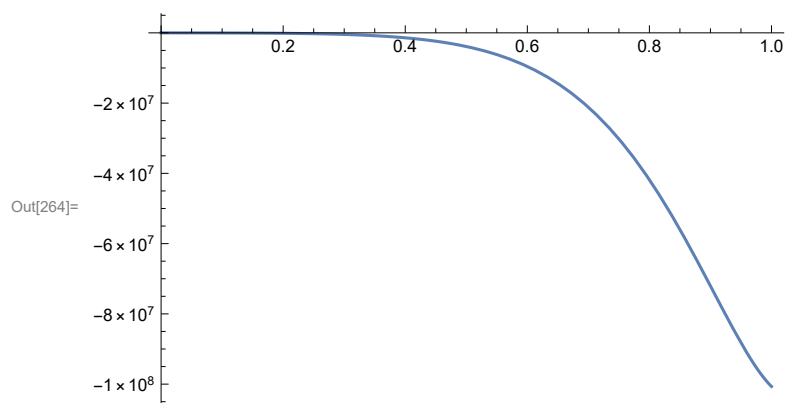

In[265]:= **Plot[Cf[13, 8, 4], {x, 0, 1}]**

[绘图](#)

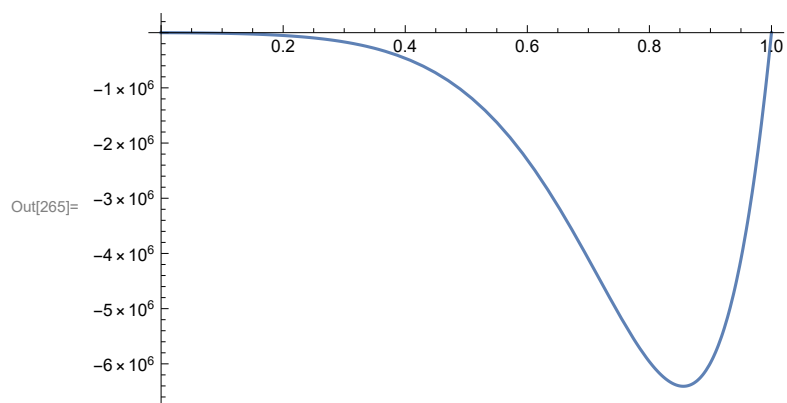

In[266]:= **Plot[Cf[13, 8, 3], {x, 0, 1}]**

[绘图](#)

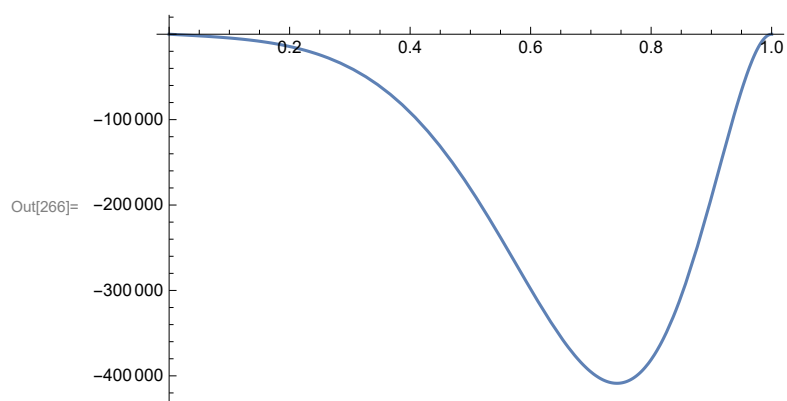

In[267]:= **Plot[Cf[13, 8, 2], {x, 0, 1}]**

[绘图](#)

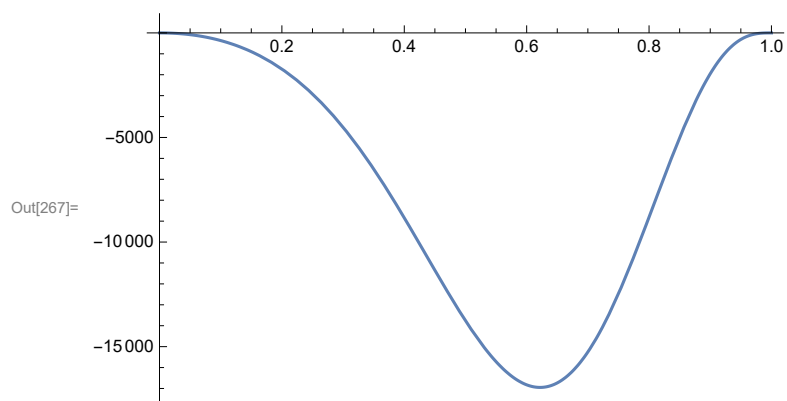

In[268]:= **Plot[Cf[13, 8, 1], {x, 0, 1}]**

[绘图](#)

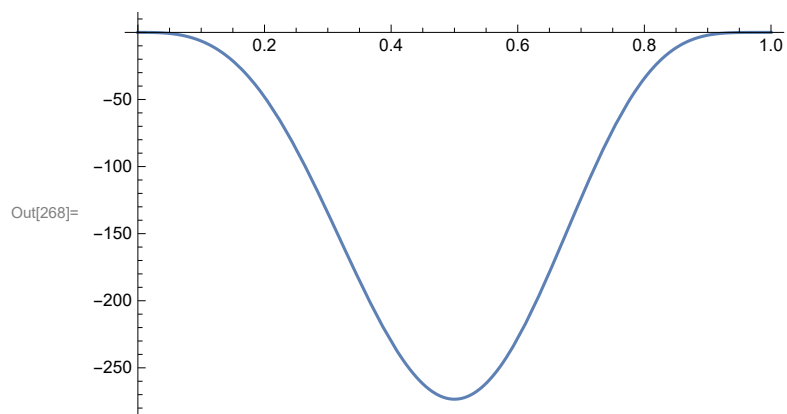

**Plot[Cf[13, 8, 0], {x, 0, 1}]**

[绘图](#)

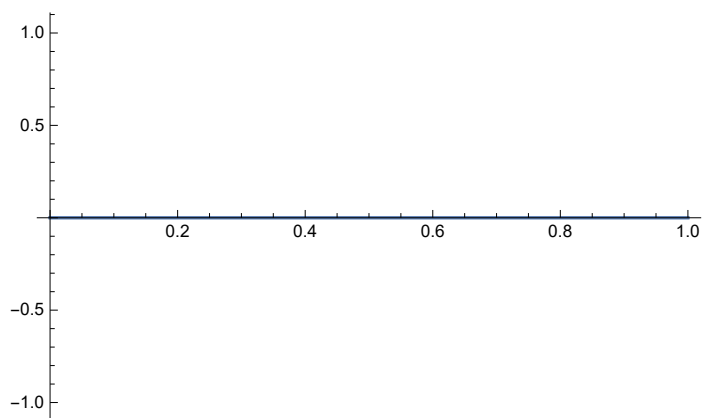

(\*23th group coefficients r2^13r3^7\*)

In[269]:= **Plot[Cf[13, 7, 14], {x, 0, 1}]**

[绘图](#)

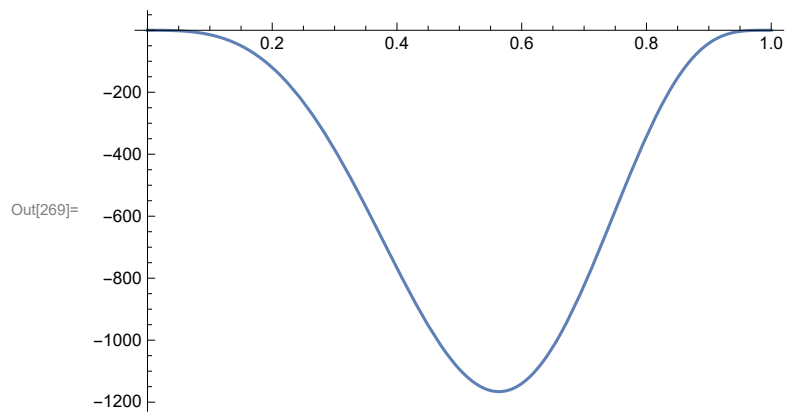

In[270]:= **Plot[Cf[13, 7, 13], {x, 0, 1}]**

[绘图](#)

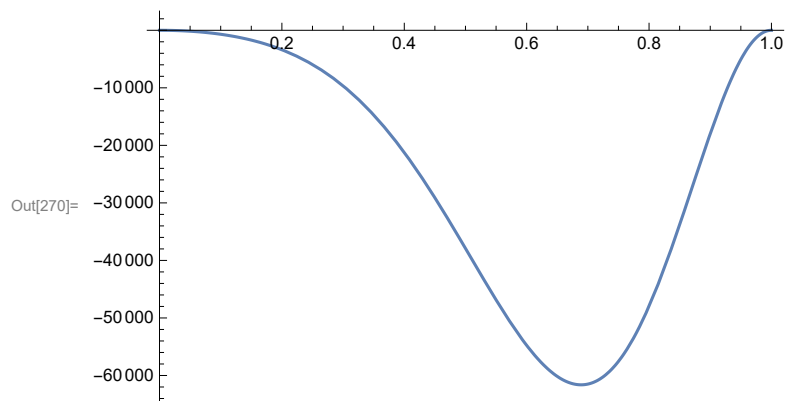

In[271]:= **Plot[Cf[13, 7, 12], {x, 0, 1}]**

[绘图](#)

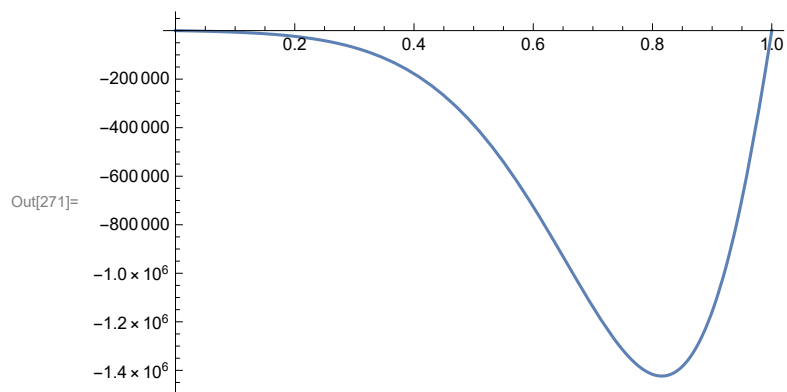



In[272]:= **Plot[Cf[13, 7, 11], {x, 0, 1}]**

[绘图](#)

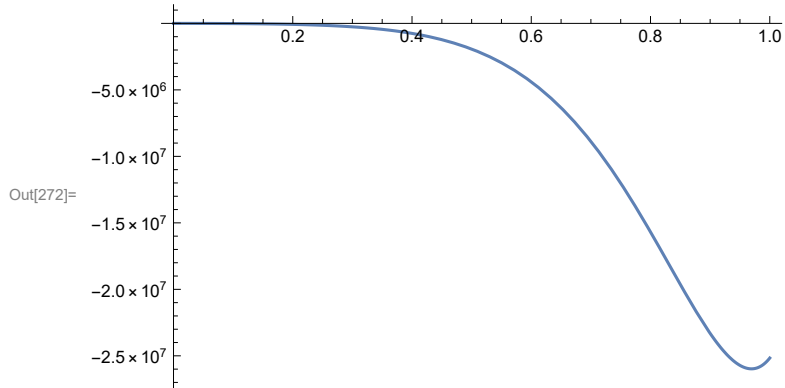

In[273]:= **Plot[Cf[13, 7, 10], {x, 0, 1}]**

[绘图](#)

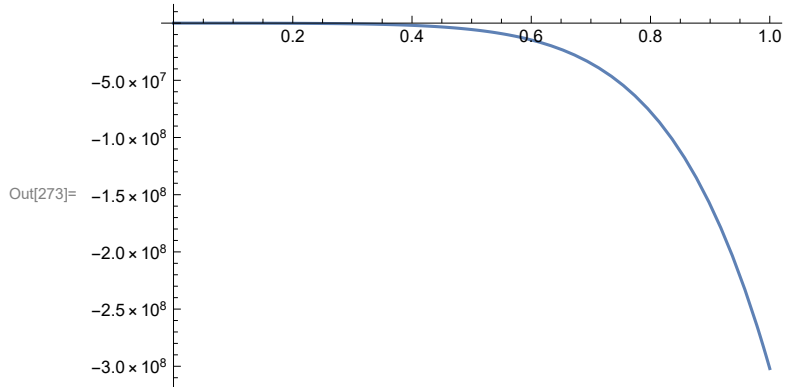

In[274]:= **Plot[Cf[13, 7, 9], {x, 0, 1}]**

[绘图](#)

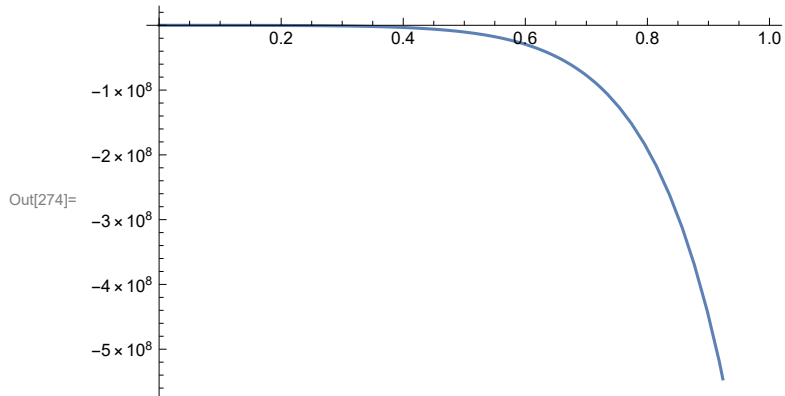

In[275]:= **Plot[Cf[13, 7, 8], {x, 0, 1}]**

[绘图](#)

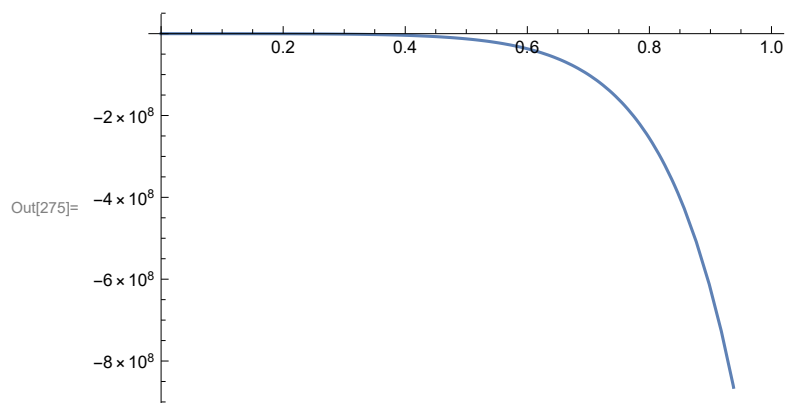

In[276]:= **Plot[Cf[13, 7, 7], {x, 0, 1}]**

[绘图](#)

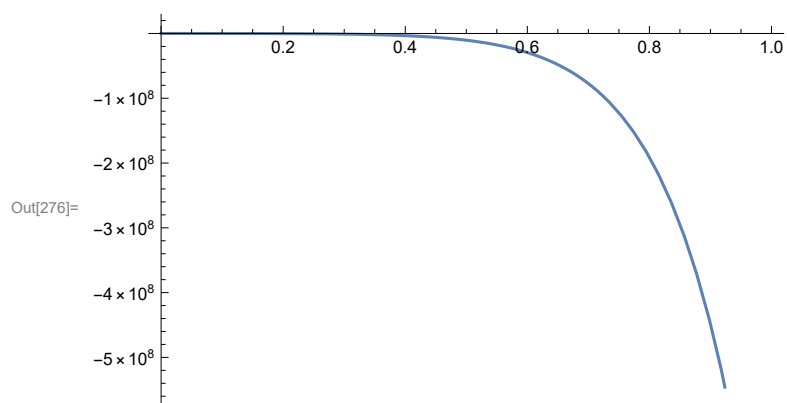

In[277]:= **Plot[Cf[13, 7, 6], {x, 0, 1}]**

[绘图](#)

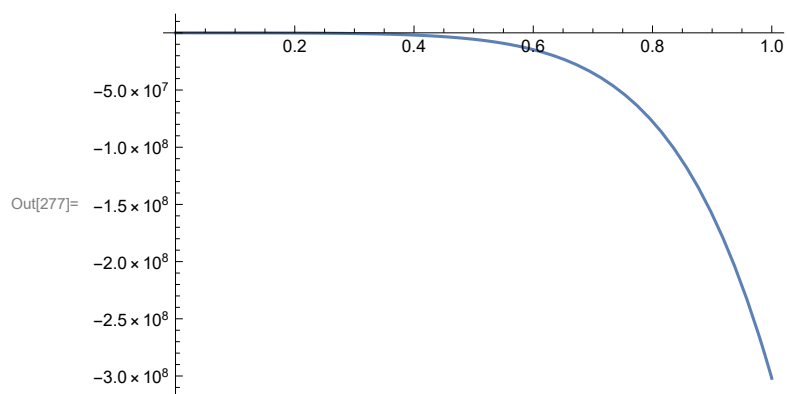

In[278]:= **Plot[Cf[13, 7, 5], {x, 0, 1}]**

[绘图](#)

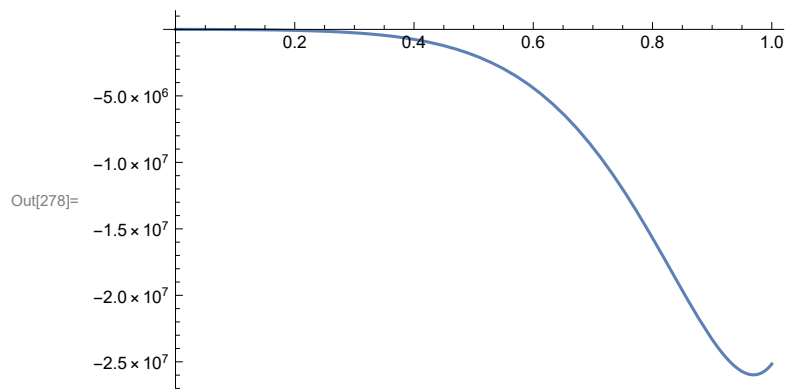

In[279]:= **Plot[Cf[13, 7, 4], {x, 0, 1}]**

[绘图](#)

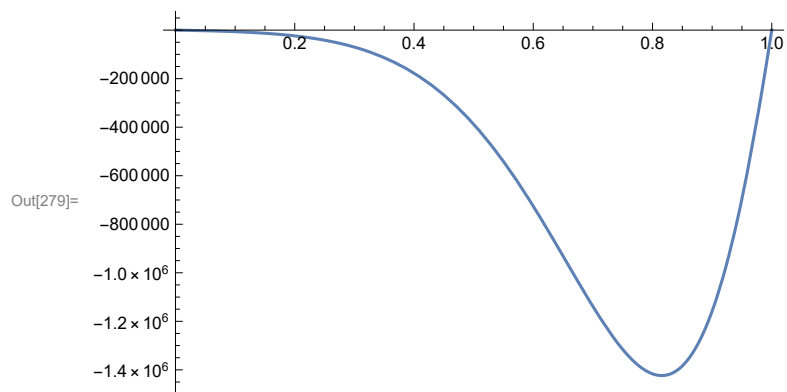

In[280]:= **Plot[Cf[13, 7, 3], {x, 0, 1}]**

[绘图](#)

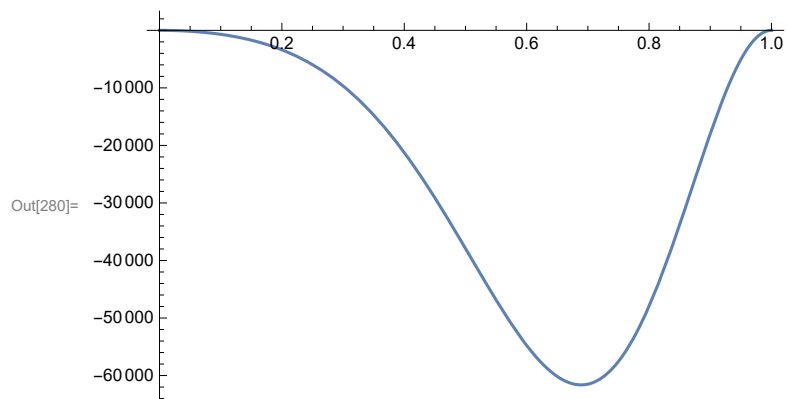

In[281]:= **Plot[Cf[13, 7, 2], {x, 0, 1}]**

[绘图](#)

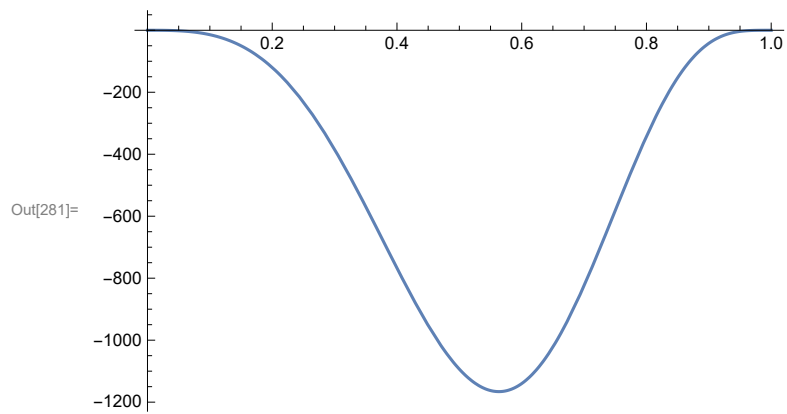

**Plot[Cf[13, 7, 1], {x, 0, 1}]**

[绘图](#)

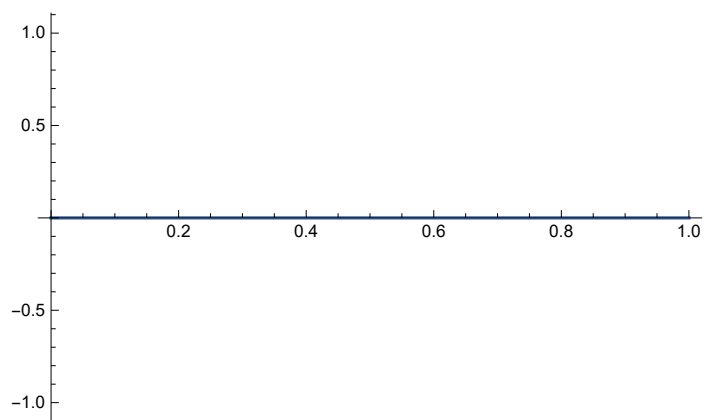

**Plot[Cf[13, 7, 0], {x, 0, 1}]**

[绘图](#)

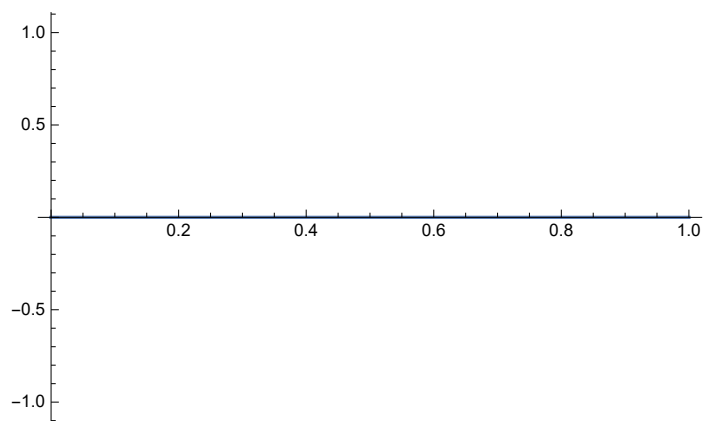

(\*24th group coefficients r2^13r3^6\*)

In[282]:= **Plot[Cf[13, 6, 14], {x, 0, 1}]**

[绘图](#)

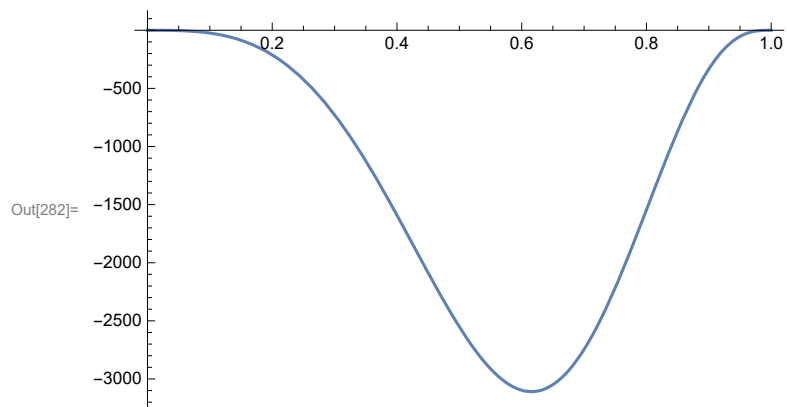

In[283]:= **Plot[Cf[13, 6, 13], {x, 0, 1}]**

[绘图](#)

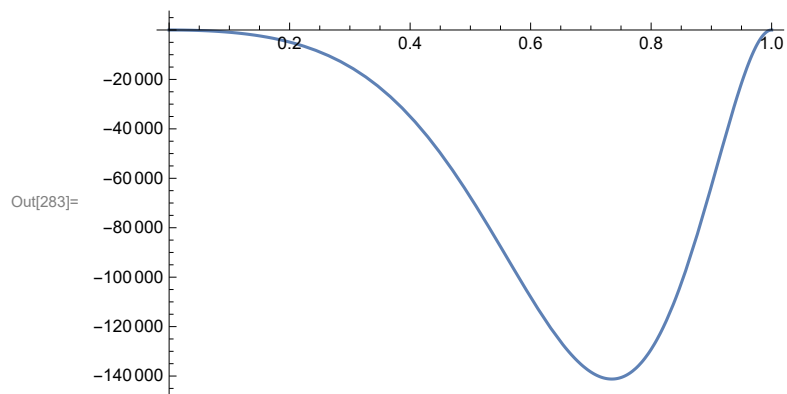

In[284]:= **Plot[Cf[13, 6, 12], {x, 0, 1}]**

[绘图](#)

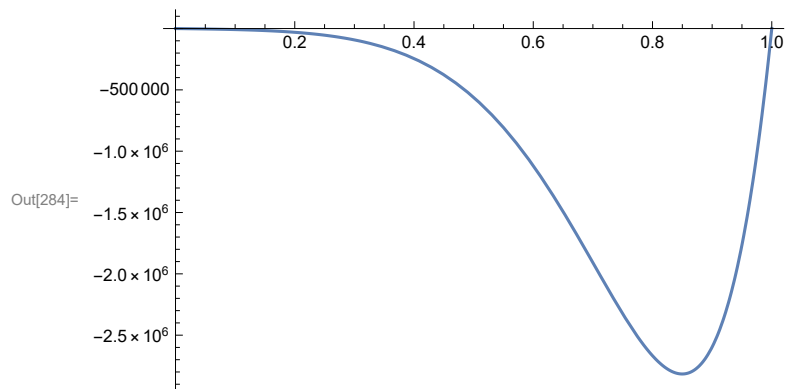

In[285]:= **Plot[Cf[13, 6, 11], {x, 0, 1}]**

[绘图](#)

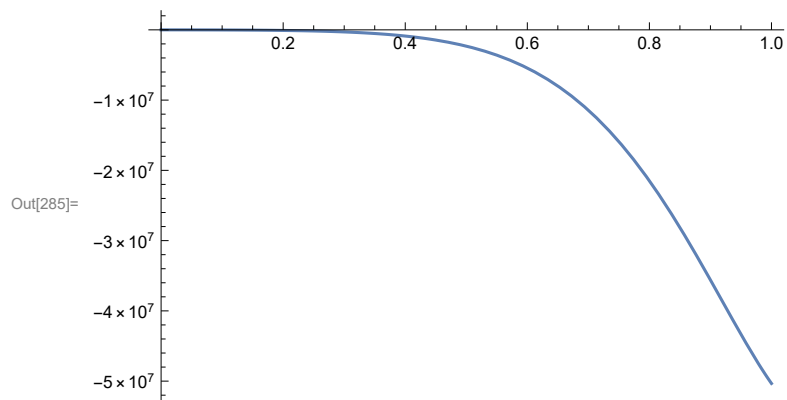

In[286]:= **Plot[Cf[13, 6, 10], {x, 0, 1}]**

[绘图](#)

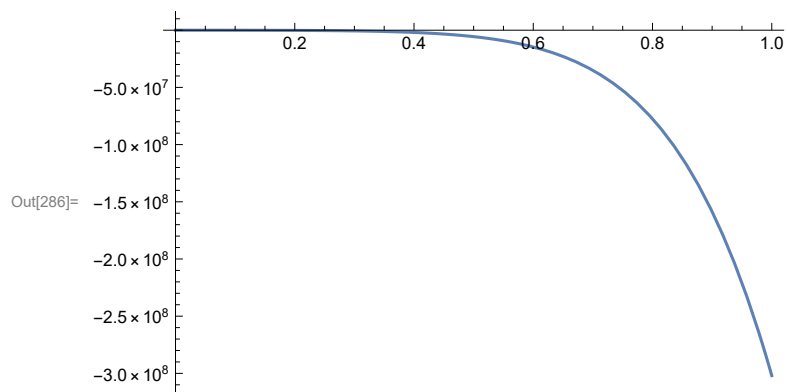

In[287]:= **Plot[Cf[13, 6, 9], {x, 0, 1}]**

[绘图](#)

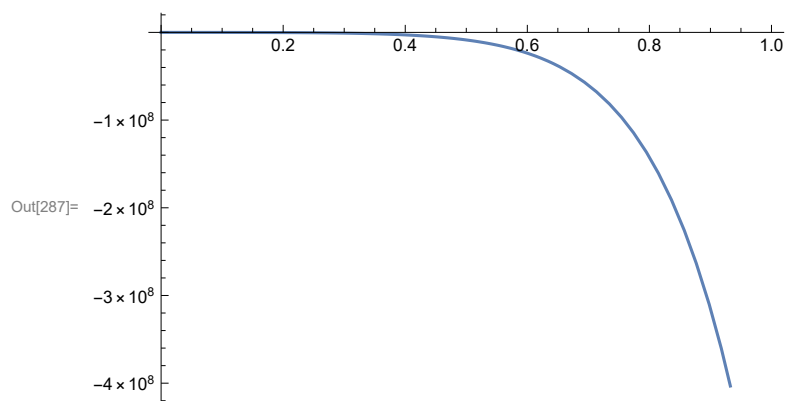

In[288]:= **Plot[Cf[13, 6, 8], {x, 0, 1}]**

[绘图](#)

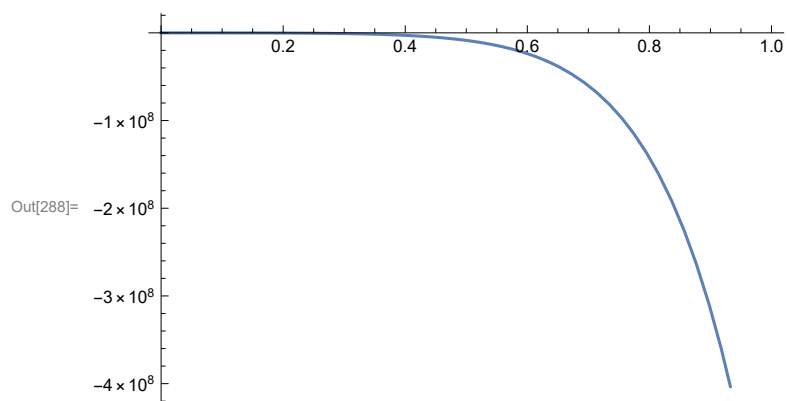

In[289]:= **Plot[Cf[13, 6, 7], {x, 0, 1}]**

[绘图](#)

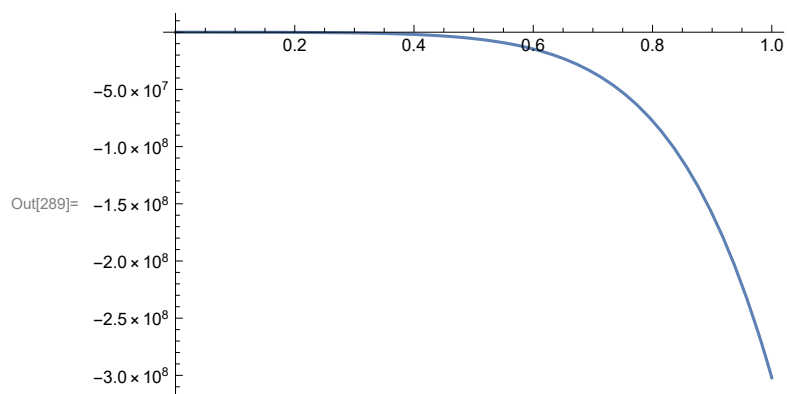

In[290]:= **Plot[Cf[13, 6, 6], {x, 0, 1}]**

[绘图](#)

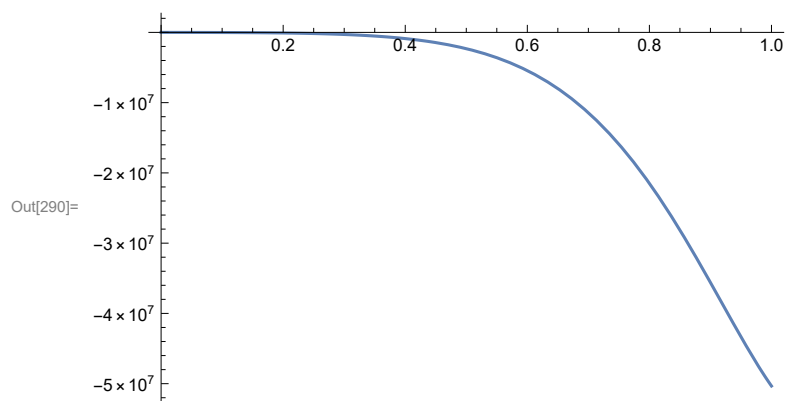

In[291]:= **Plot[Cf[13, 6, 5], {x, 0, 1}]**

[绘图](#)

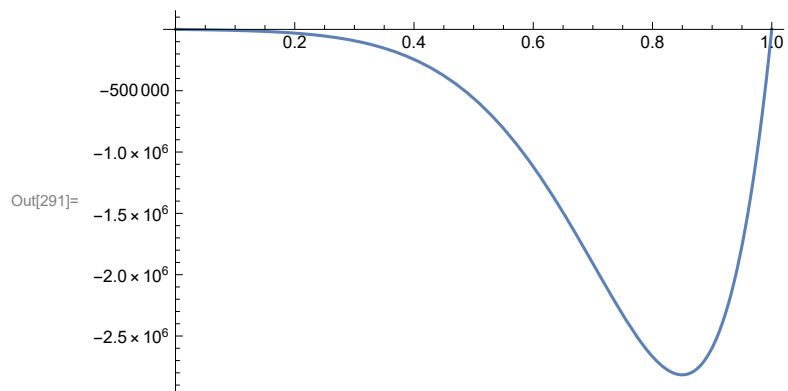

In[292]:= **Plot[Cf[13, 6, 4], {x, 0, 1}]**

[绘图](#)

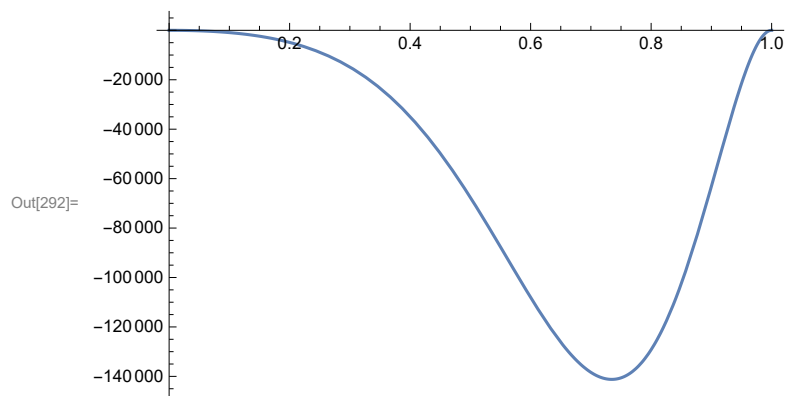

In[293]:= **Plot[Cf[13, 6, 3], {x, 0, 1}]**

[绘图](#)

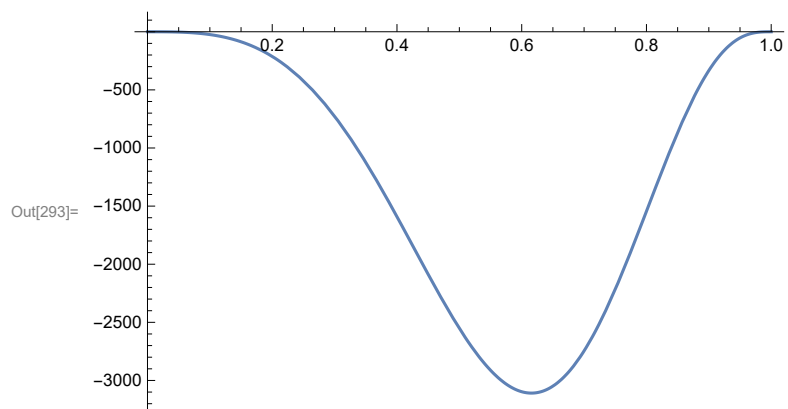



**Plot[Cf[13, 6, 2], {x, 0, 1}]**

[绘图](#)

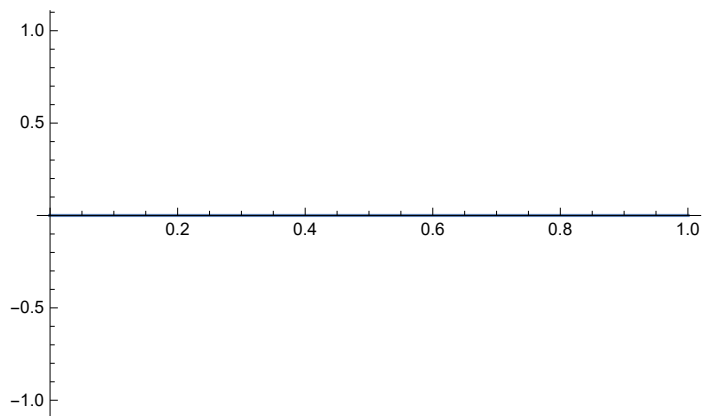

**Plot[Cf[13, 6, 1], {x, 0, 1}]**

[绘图](#)

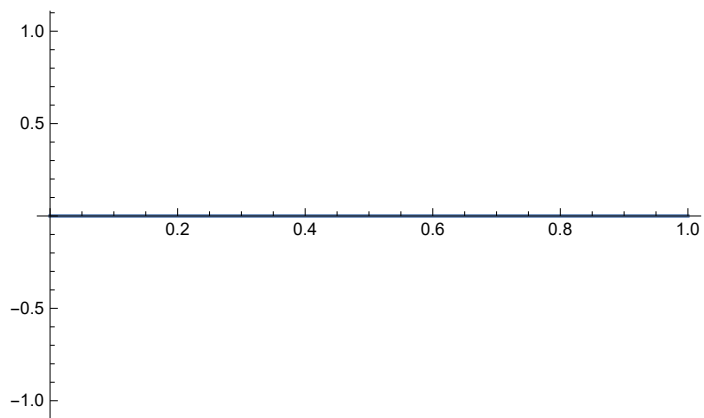

**Plot[Cf[13, 6, 0], {x, 0, 1}]**

[绘图](#)

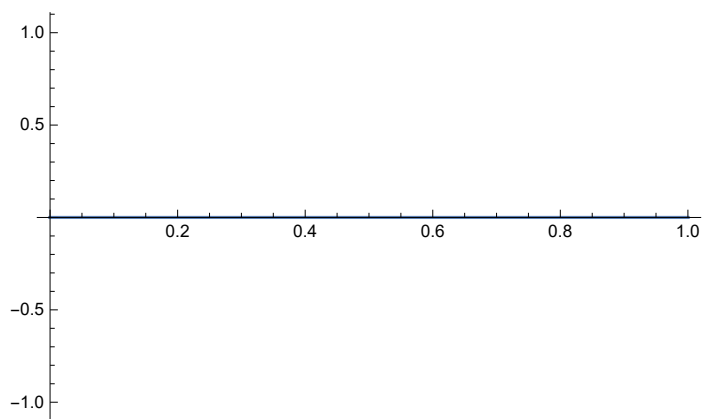

**(\*25th group coefficients r2^13r3^5\*)**

In[294]:= **Plot**[**Cf**[13, 5, 14], {x, 0, 1}]

[绘图](#)

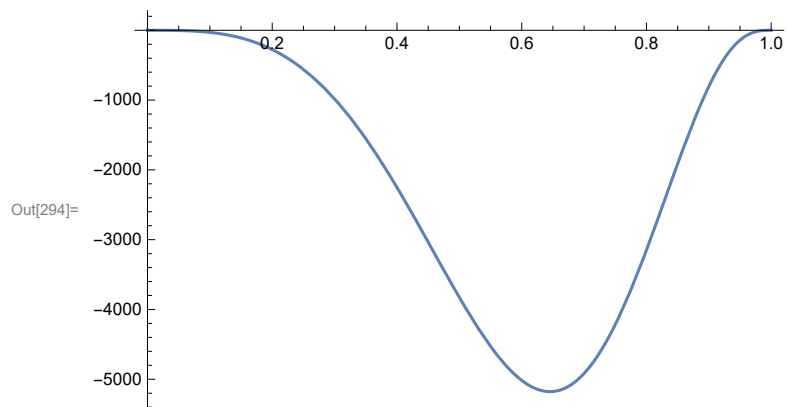

In[295]:= **Plot**[**Cf**[13, 5, 13], {x, 0, 1}]

[绘图](#)

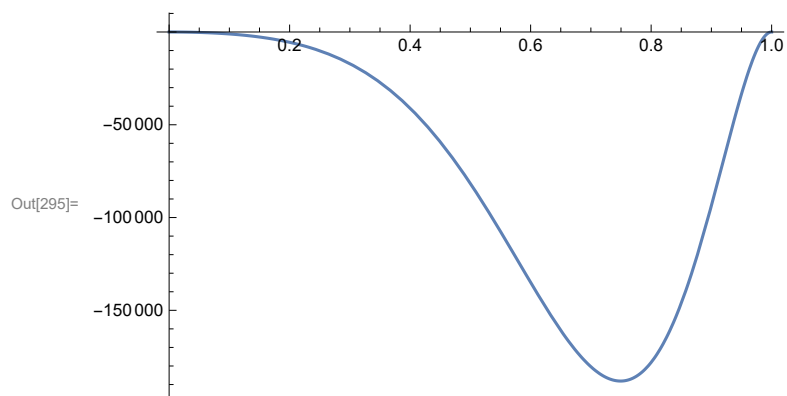

In[296]:= **Plot**[**Cf**[13, 5, 12], {x, 0, 1}]

[绘图](#)

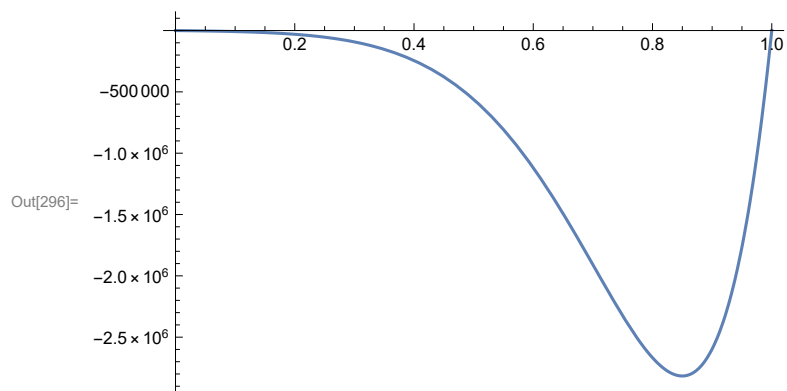

In[297]:= **Plot[Cf[13, 5, 11], {x, 0, 1}]**

[绘图](#)

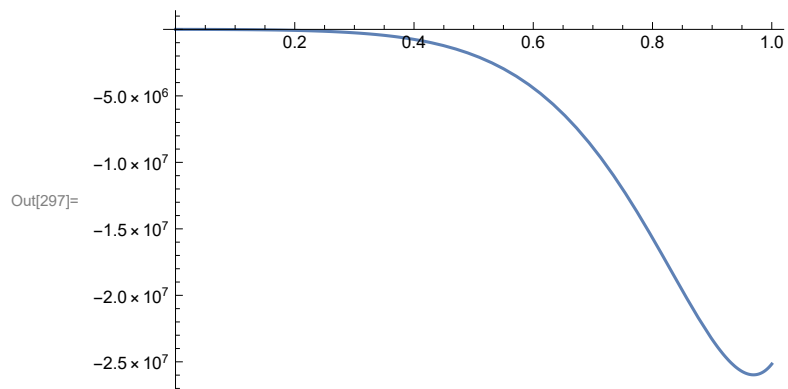

In[298]:= **Plot[Cf[13, 5, 10], {x, 0, 1}]**

[绘图](#)

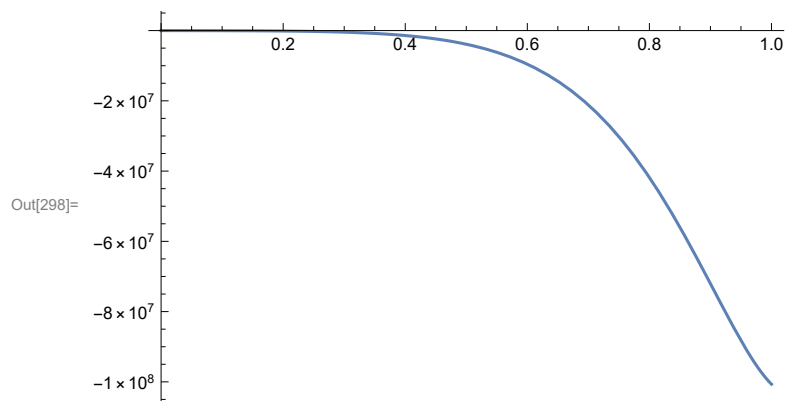

In[299]:= **Plot[Cf[13, 5, 9], {x, 0, 1}]**

[绘图](#)

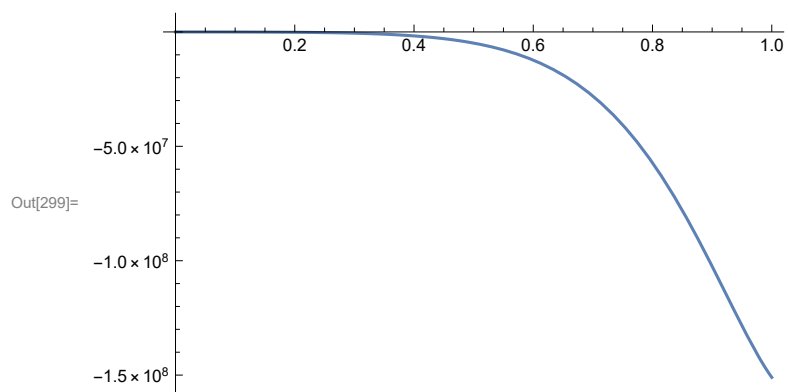

In[300]:= **Plot[Cf[13, 5, 8], {x, 0, 1}]**

[绘图](#)

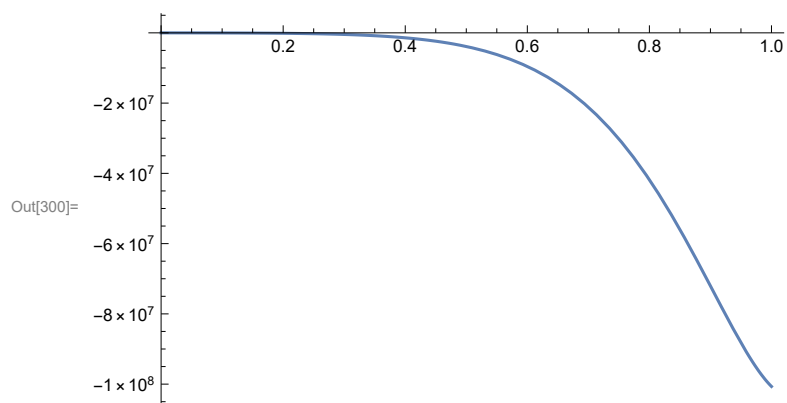

In[301]:= **Plot[Cf[13, 5, 7], {x, 0, 1}]**

[绘图](#)

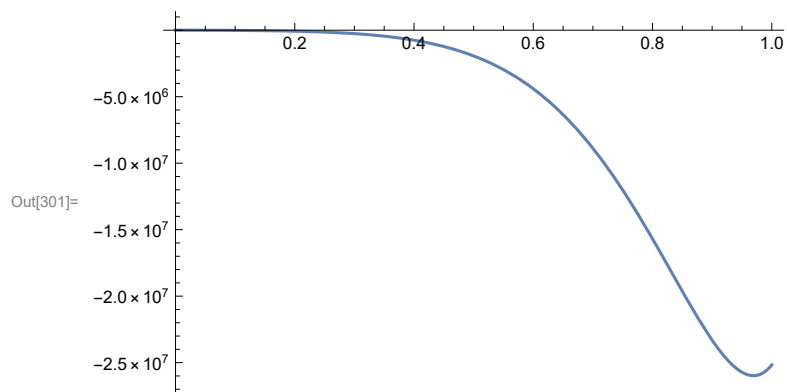

In[302]:= **Plot[Cf[13, 5, 6], {x, 0, 1}]**

[绘图](#)

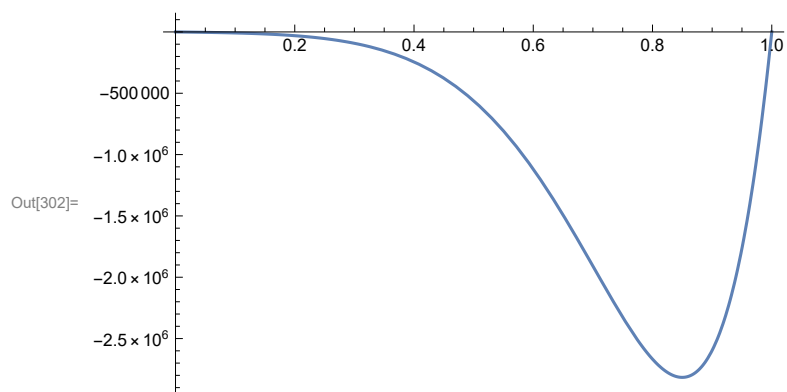

In[303]:= **Plot[Cf[13, 5, 5], {x, 0, 1}]**

[绘图](#)

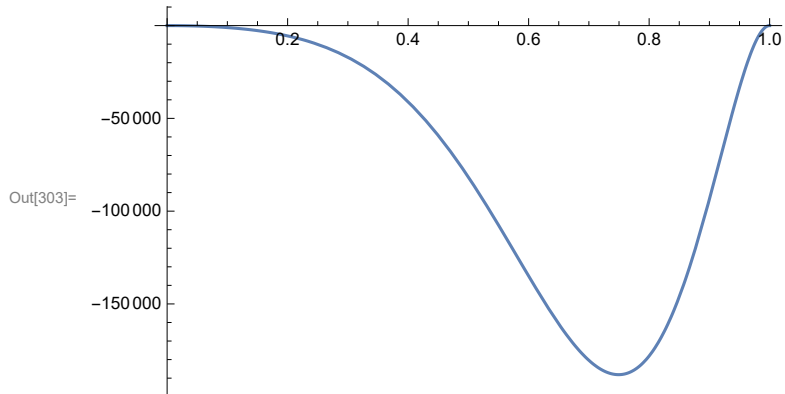

In[304]:= **Plot[Cf[13, 5, 4], {x, 0, 1}]**

[绘图](#)

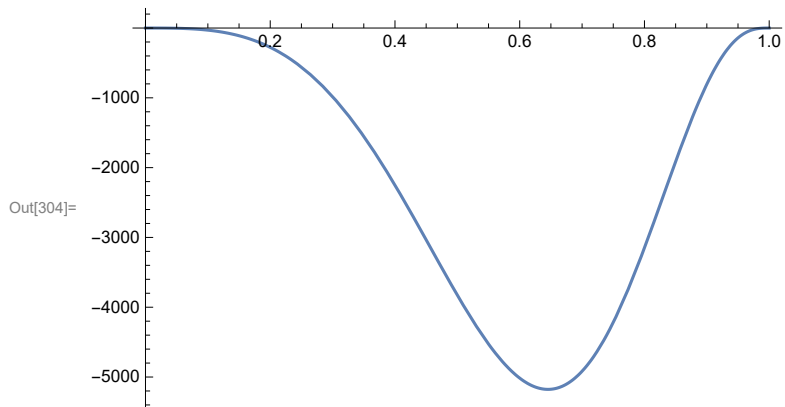

**Plot[Cf[13, 5, 3], {x, 0, 1}]**

[绘图](#)

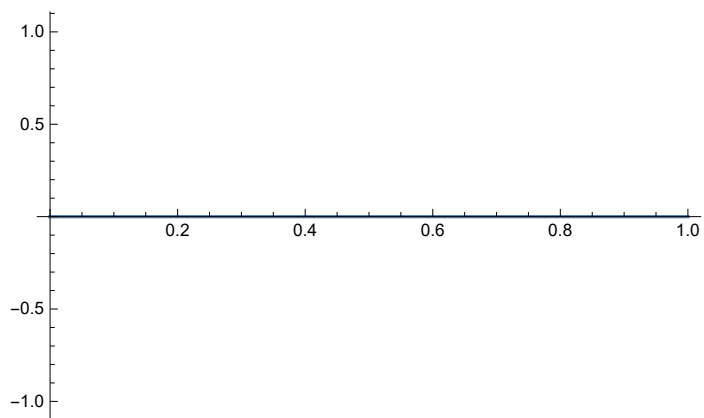

`Plot[Cf[13, 5, 2], {x, 0, 1}]`

[绘图](#)

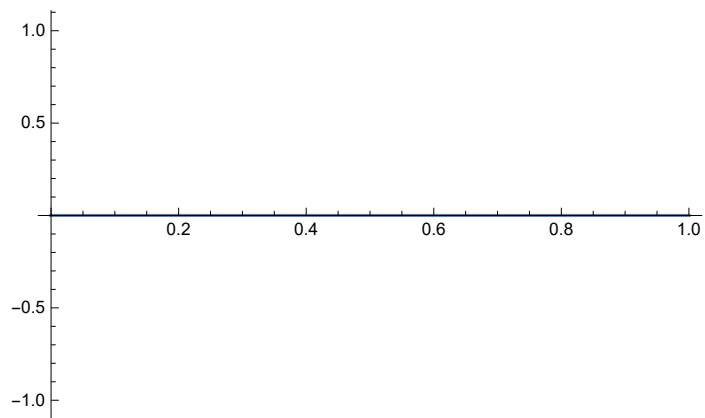

`Plot[Cf[13, 5, 1], {x, 0, 1}]`

[绘图](#)

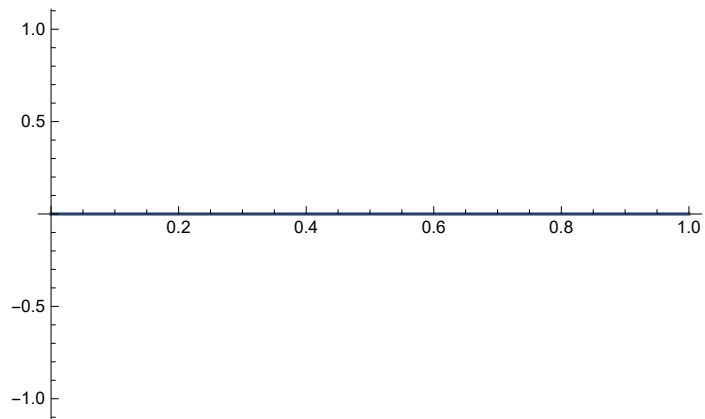

`Plot[Cf[13, 5, 0], {x, 0, 1}]`

[绘图](#)

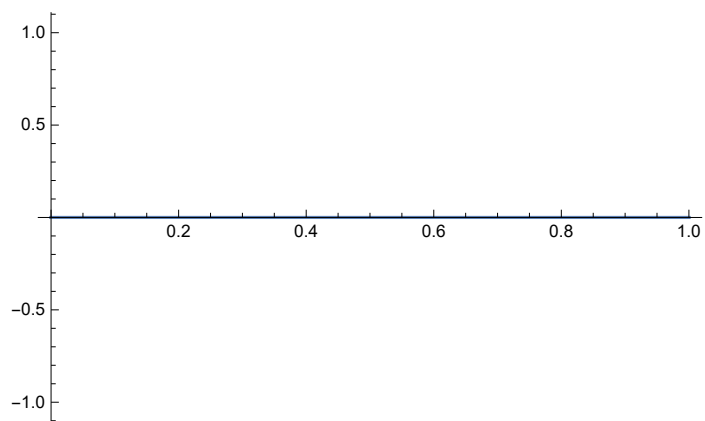

`(*26th group coefficients r2^13r3^4*)`

In[305]:= **Plot**[**Cf**[13, 4, 14], {x, 0, 1}]

[绘图](#)

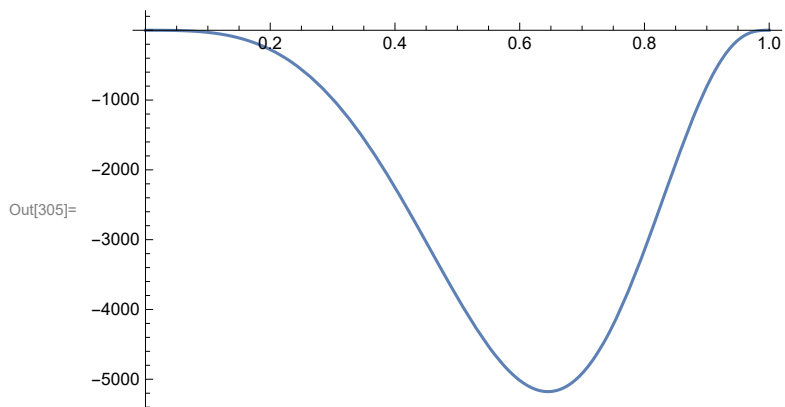

In[306]:= **Plot**[**Cf**[13, 4, 13], {x, 0, 1}]

[绘图](#)

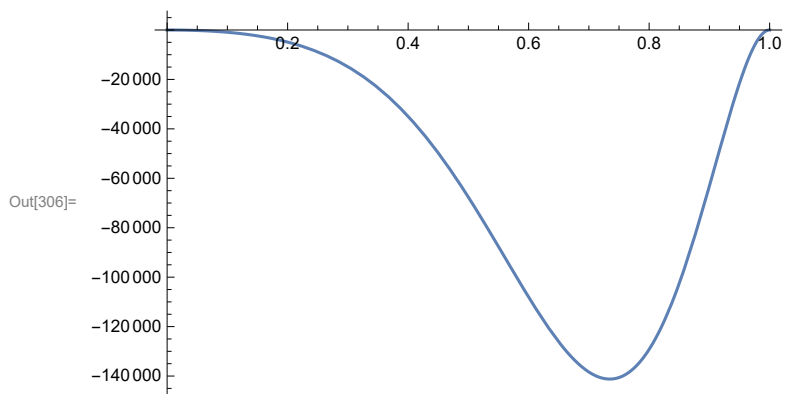

In[307]:= **Plot**[**Cf**[13, 4, 12], {x, 0, 1}]

[绘图](#)

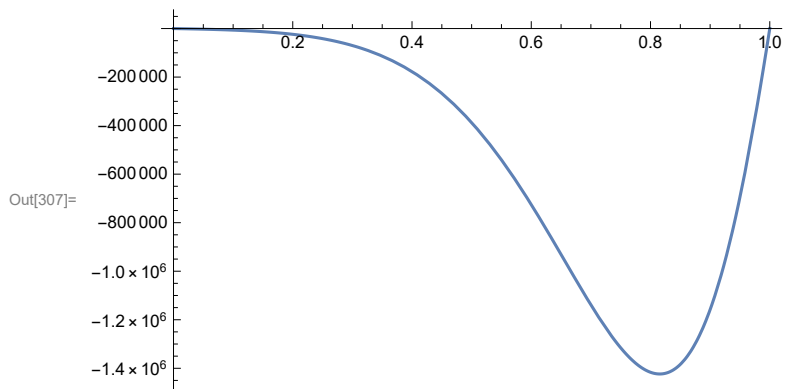

In[308]:= **Plot[Cf[13, 4, 11], {x, 0, 1}]**

[绘图](#)

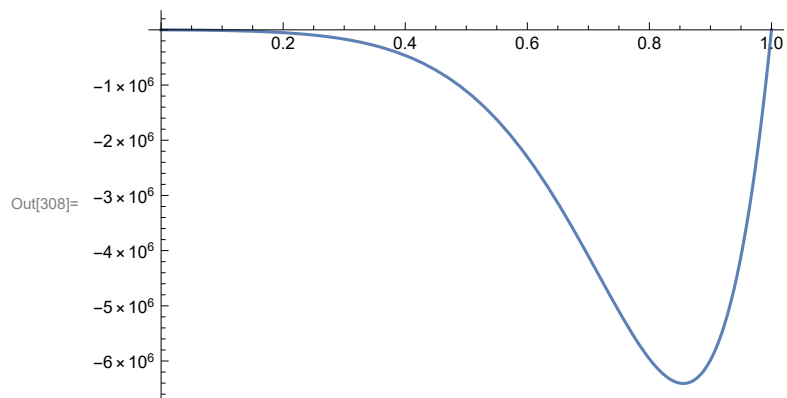

In[309]:= **Plot[Cf[13, 4, 10], {x, 0, 1}]**

[绘图](#)

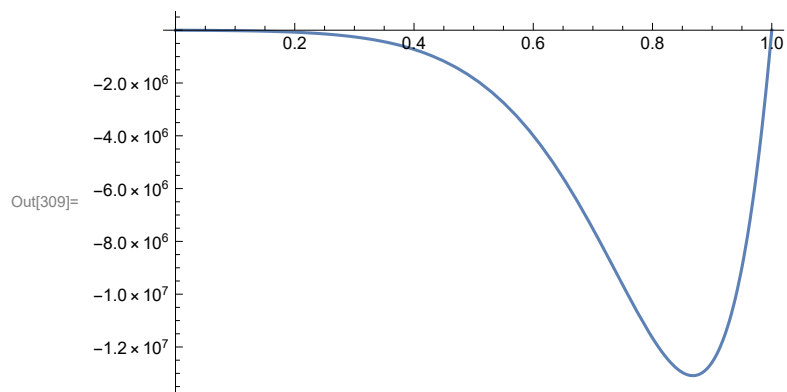

In[310]:= **Plot[Cf[13, 4, 9], {x, 0, 1}]**

[绘图](#)

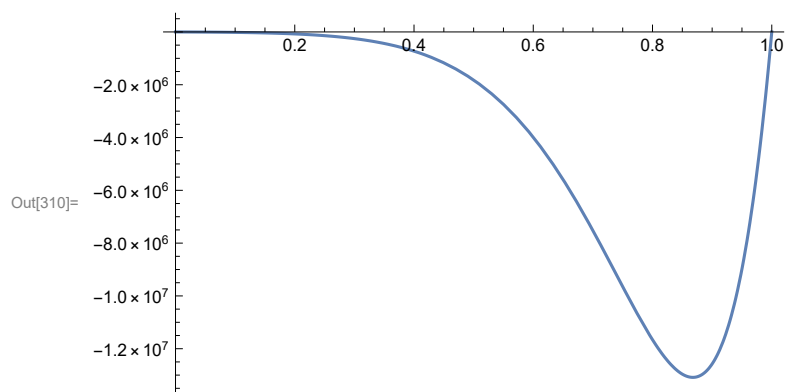



In[311]:= **Plot[Cf[13, 4, 8], {x, 0, 1}]**

[绘图](#)

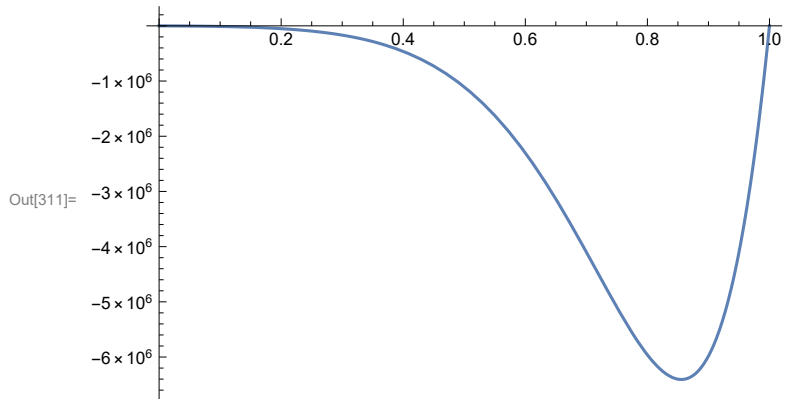

In[312]:= **Plot[Cf[13, 4, 7], {x, 0, 1}]**

[绘图](#)

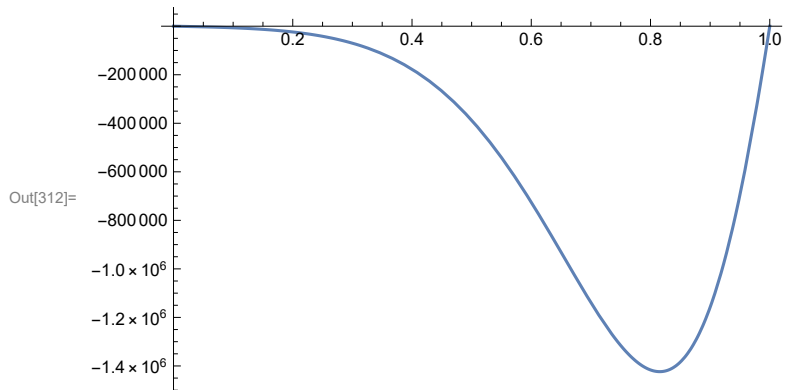

In[313]:= **Plot[Cf[13, 4, 6], {x, 0, 1}]**

[绘图](#)

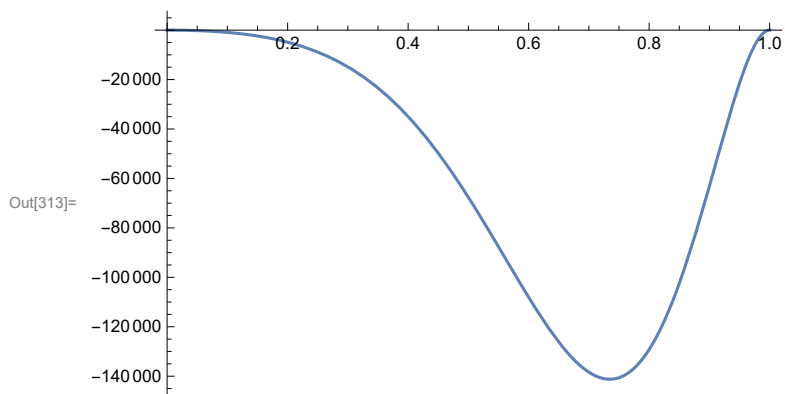

In[314]:= **Plot[Cf[13, 4, 5], {x, 0, 1}]**

[绘图](#)

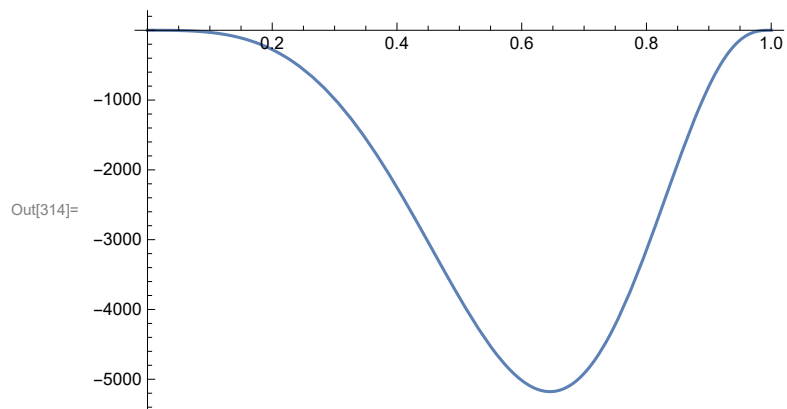

**Plot[Cf[13, 4, 4], {x, 0, 1}]**

[绘图](#)

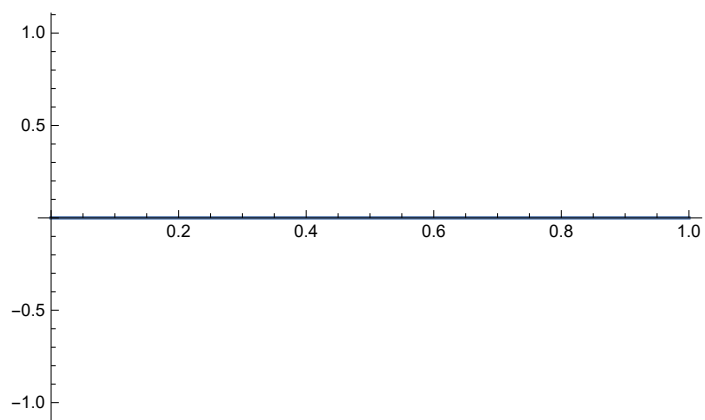

**Plot[Cf[13, 4, 3], {x, 0, 1}]**

[绘图](#)

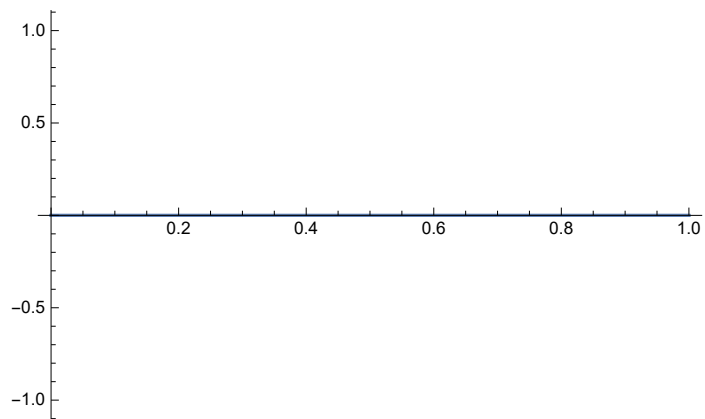

**Plot[Cf[13, 4, 2], {x, 0, 1}]**

[绘图](#)

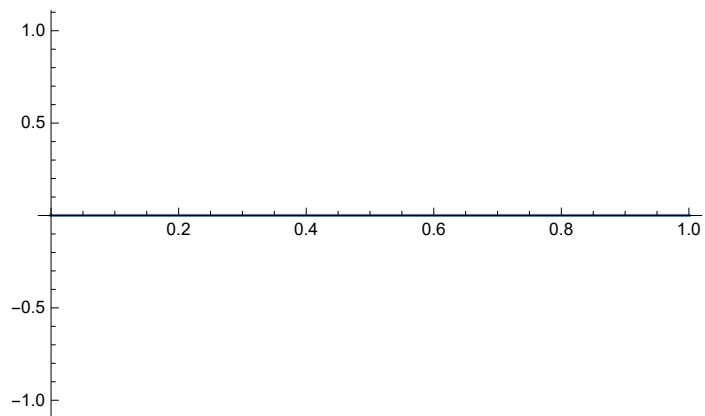

**Plot[Cf[13, 4, 1], {x, 0, 1}]**

[绘图](#)

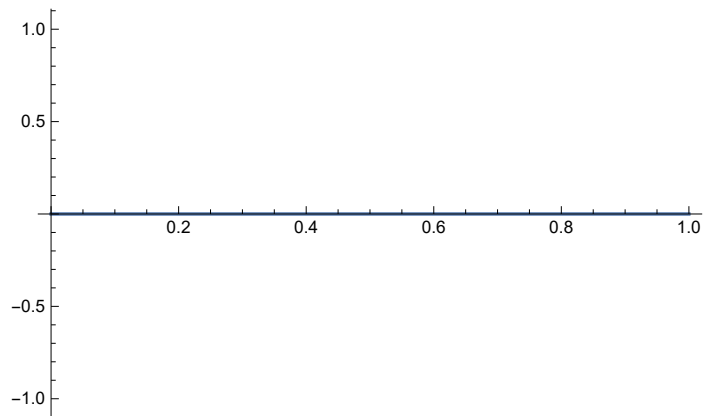

**Plot[Cf[13, 4, 0], {x, 0, 1}]**

[绘图](#)

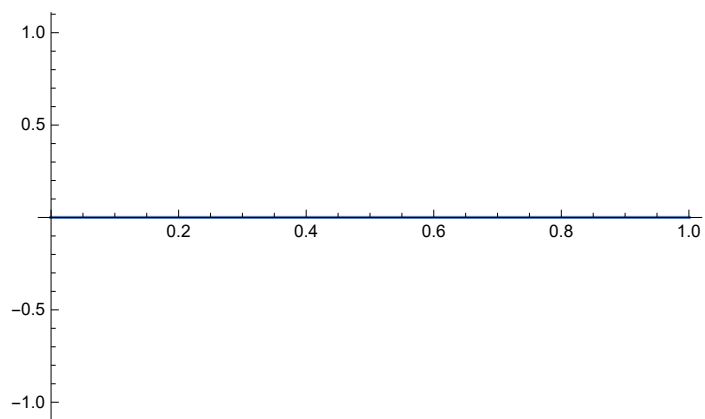

**(\*27th group coefficients r2^13r3^3\*)**

In[315]:= **Plot[Cf[13, 3, 14], {x, 0, 1}]**

[绘图](#)

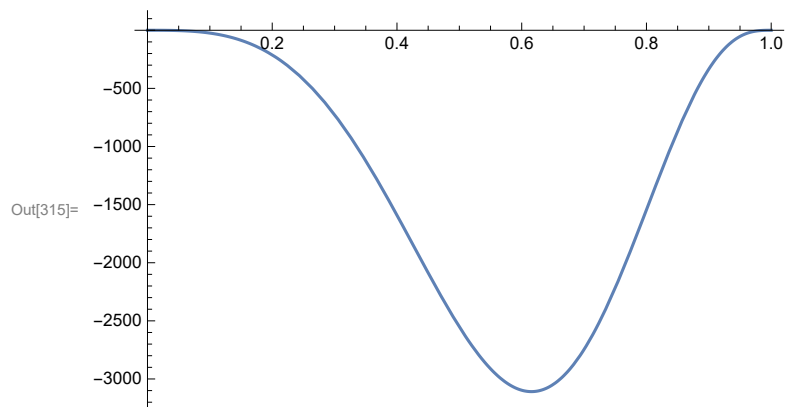

In[316]:= **Plot[Cf[13, 3, 13], {x, 0, 1}]**

[绘图](#)

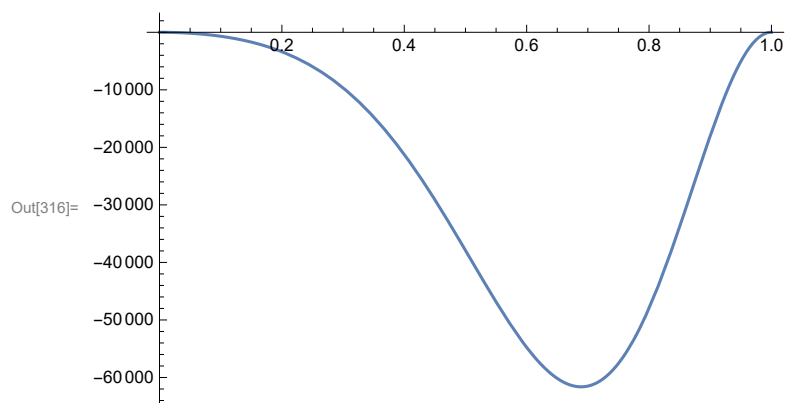

In[317]:= **Plot[Cf[13, 3, 12], {x, 0, 1}]**

[绘图](#)

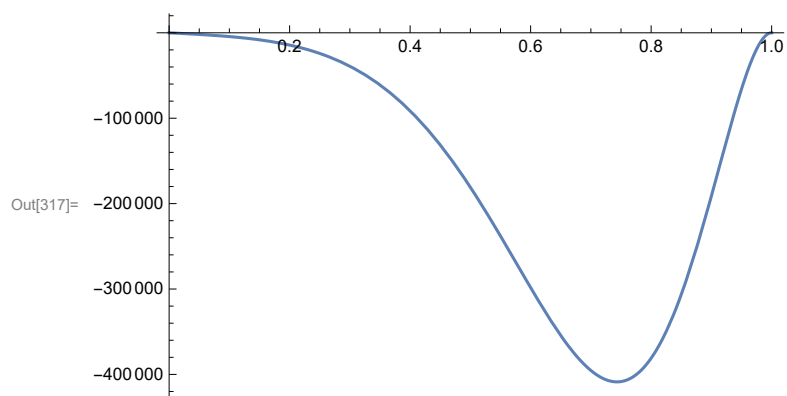

In[318]:= **Plot[Cf[13, 3, 11], {x, 0, 1}]**

[绘图](#)

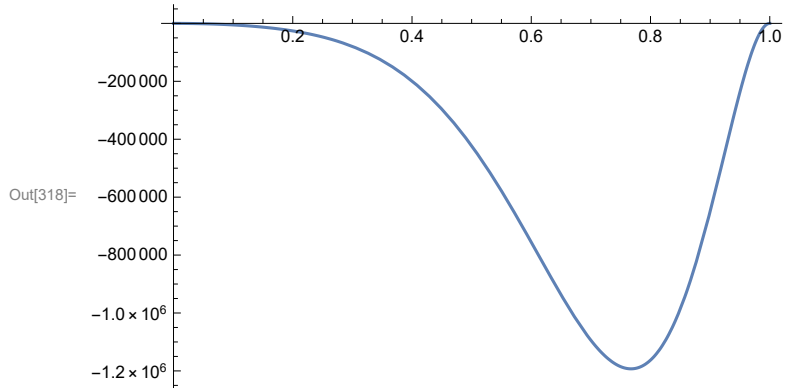

In[319]:= **Plot[Cf[13, 3, 10], {x, 0, 1}]**

[绘图](#)

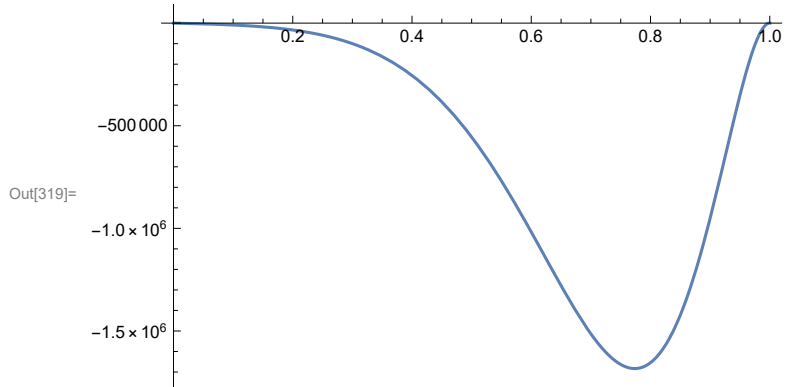

In[320]:= **Plot[Cf[13, 3, 9], {x, 0, 1}]**

[绘图](#)

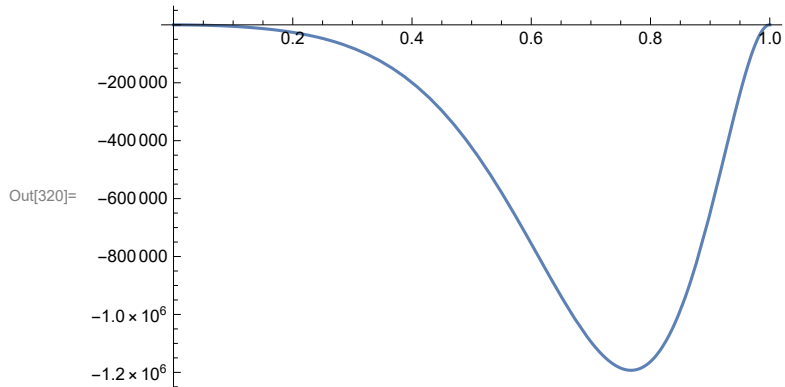

In[321]:= **Plot[Cf[13, 3, 8], {x, 0, 1}]**

[绘图](#)

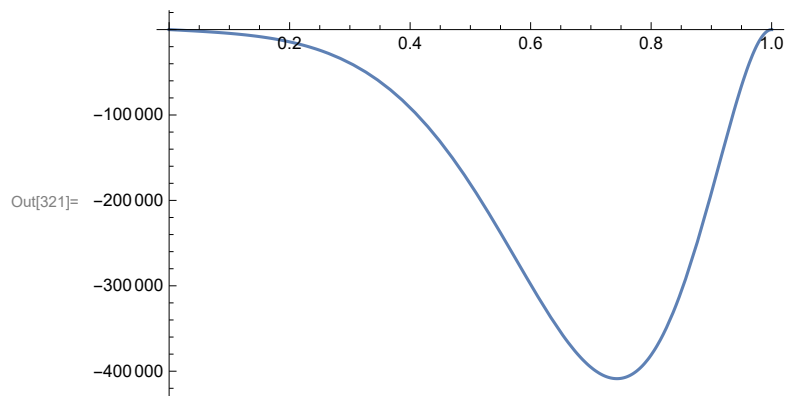

In[322]:= **Plot[Cf[13, 3, 7], {x, 0, 1}]**

[绘图](#)

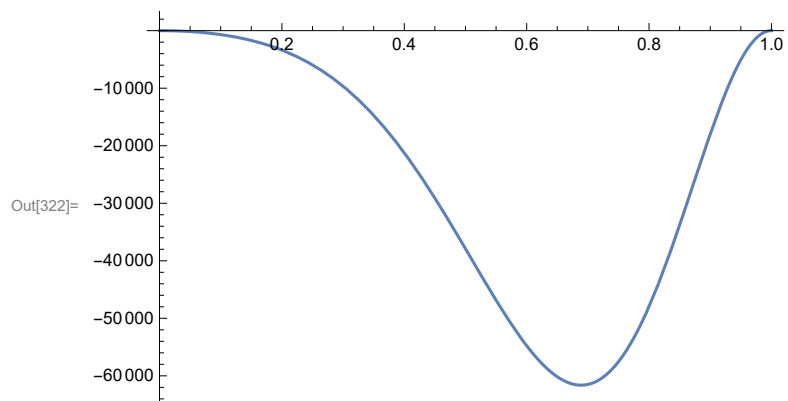

In[323]:= **Plot[Cf[13, 3, 6], {x, 0, 1}]**

[绘图](#)

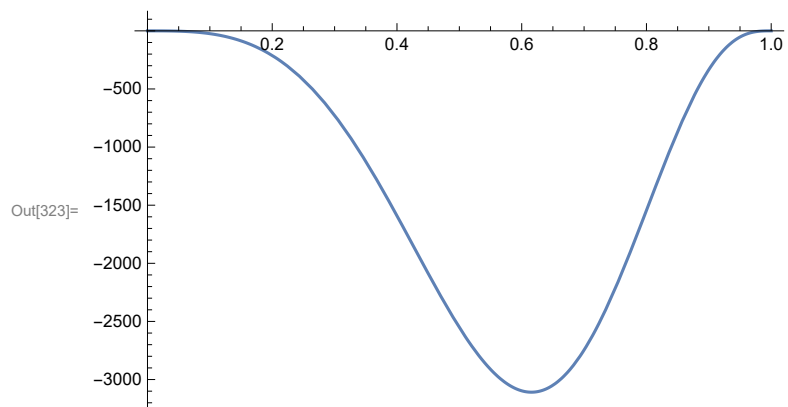

**Plot[Cf[13, 3, 5], {x, 0, 1}]**

[绘图](#)

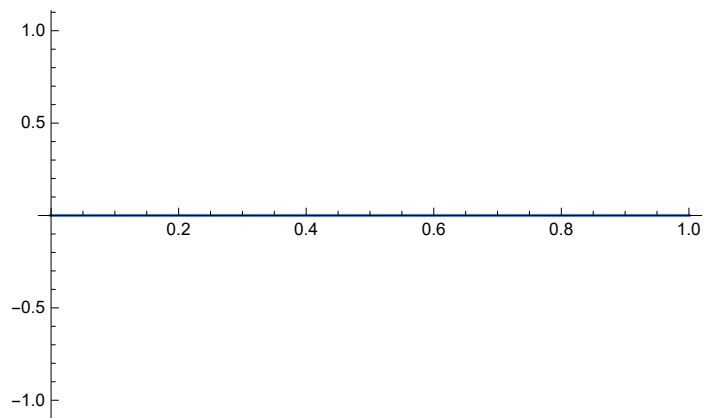

**Plot[Cf[13, 3, 4], {x, 0, 1}]**

[绘图](#)

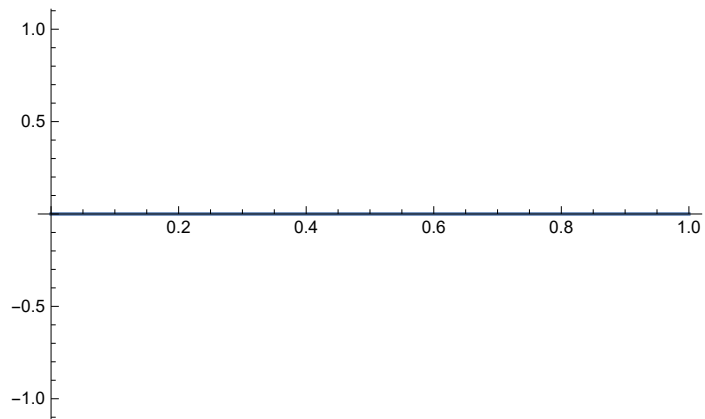

**Plot[Cf[13, 3, 3], {x, 0, 1}]**

[绘图](#)

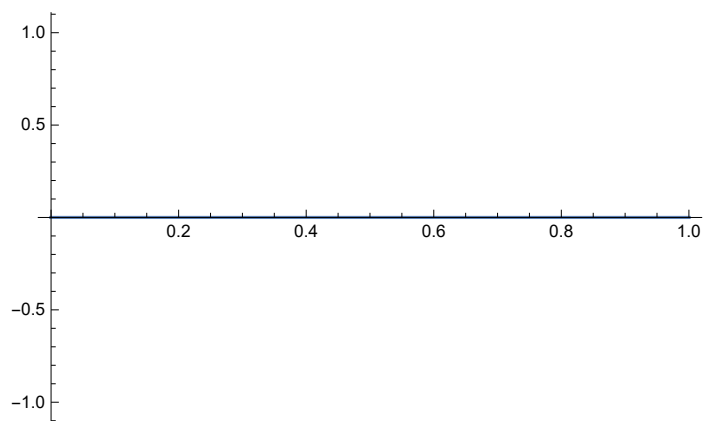

**Plot[Cf[13, 3, 2], {x, 0, 1}]**

[绘图](#)

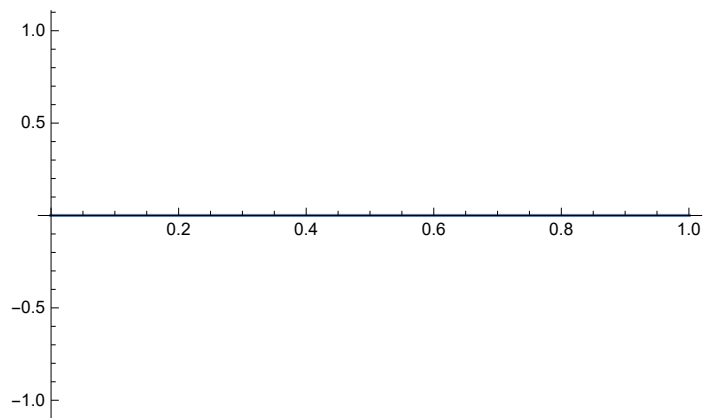

**Plot[Cf[13, 3, 1], {x, 0, 1}]**

[绘图](#)

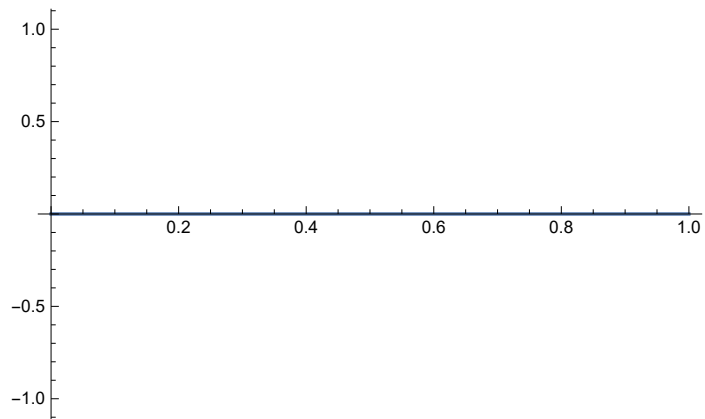

**Plot[Cf[13, 3, 0], {x, 0, 1}]**

[绘图](#)

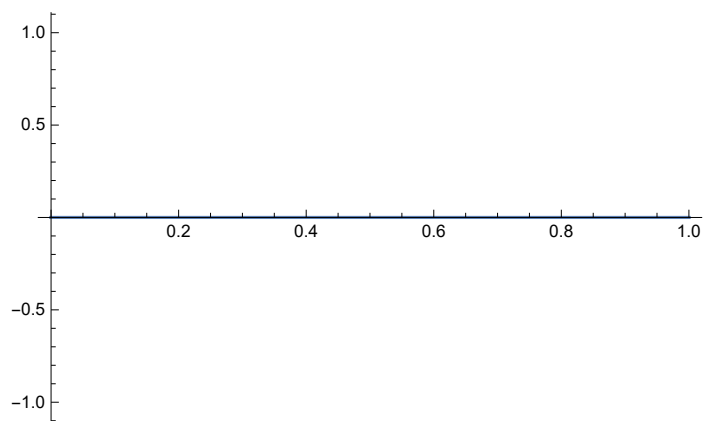

**(\*28th group coefficients r2^13r3^2\*)**



In[324]:= **Plot[Cf[13, 2, 14], {x, 0, 1}]**

[绘图](#)

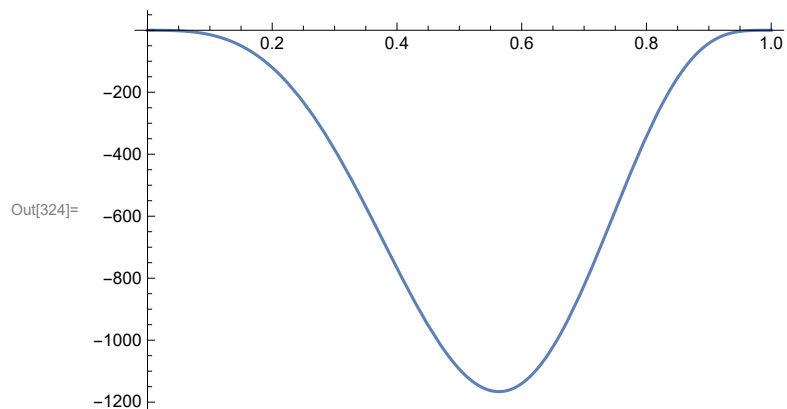

In[325]:= **Plot[Cf[13, 2, 13], {x, 0, 1}]**

[绘图](#)

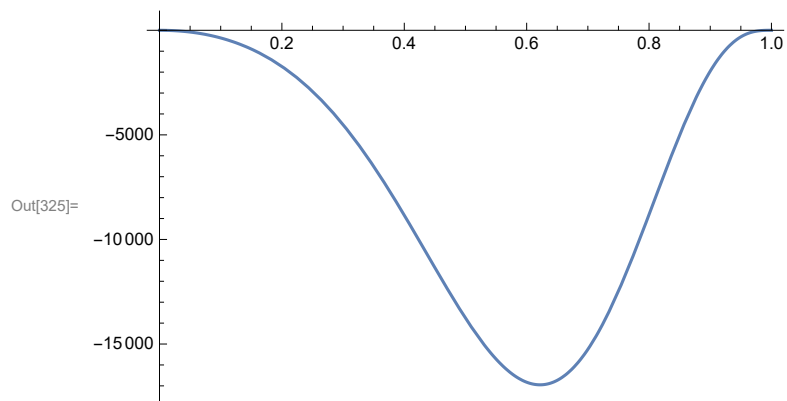

In[326]:= **Plot[Cf[13, 2, 12], {x, 0, 1}]**

[绘图](#)

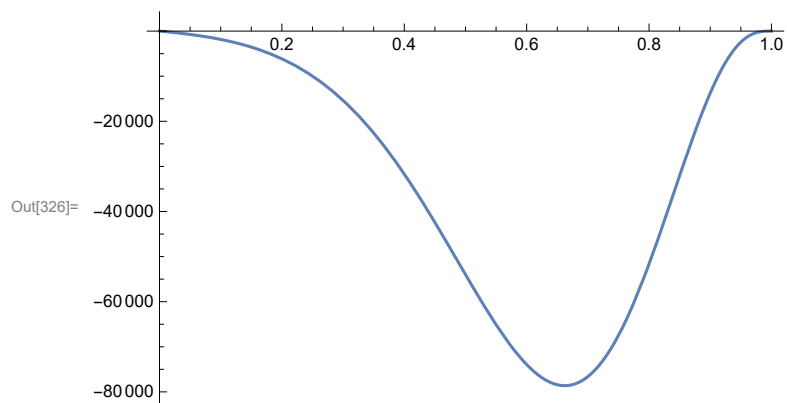

In[327]:= **Plot[Cf[13, 2, 11], {x, 0, 1}]**

[绘图](#)

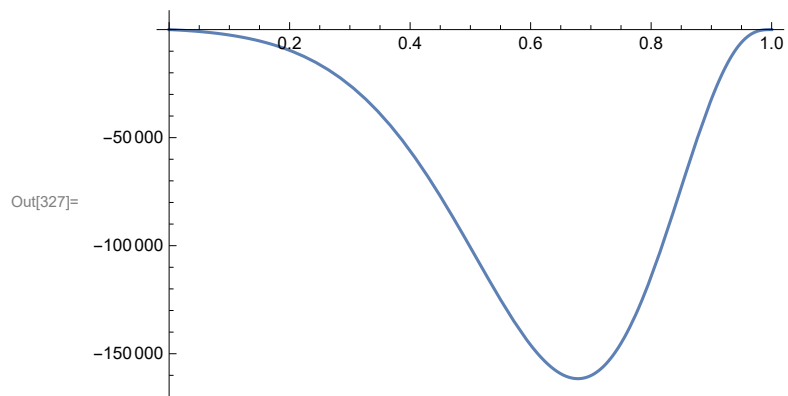

In[328]:= **Plot[Cf[13, 2, 10], {x, 0, 1}]**

[绘图](#)

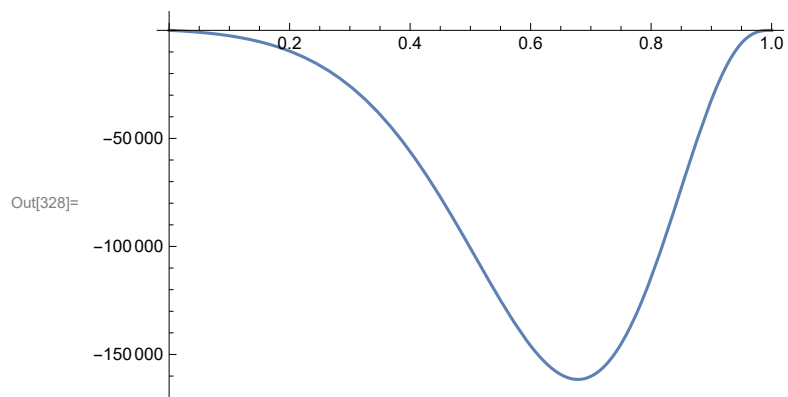

In[329]:= **Plot[Cf[13, 2, 9], {x, 0, 1}]**

[绘图](#)

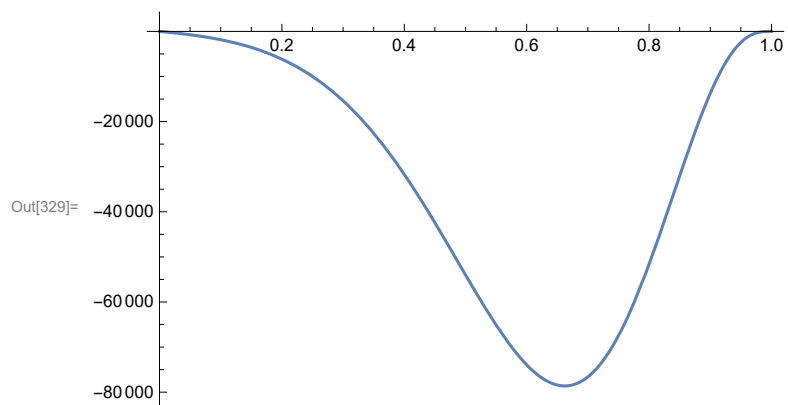

In[330]:= **Plot**[**Cf**[13, 2, 8], {x, 0, 1}]

[绘图](#)

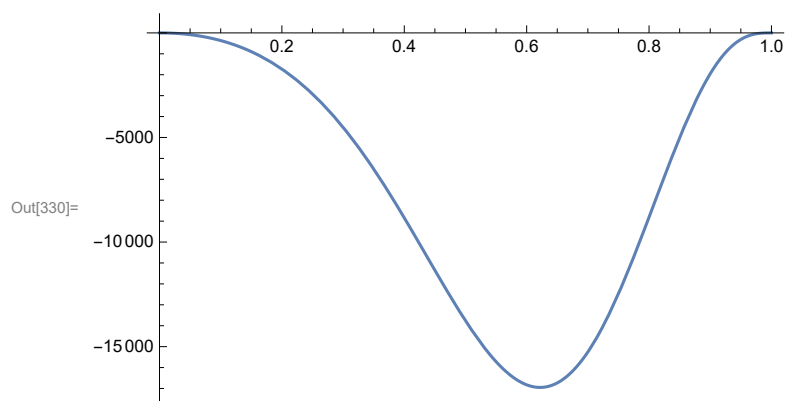

In[331]:= **Plot**[**Cf**[13, 2, 7], {x, 0, 1}]

[绘图](#)

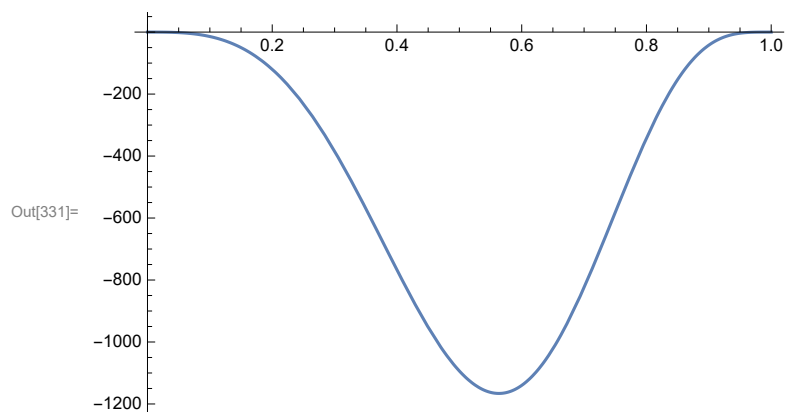

In[332]:= **Plot**[**Cf**[13, 2, 6], {x, 0, 1}]

[绘图](#)

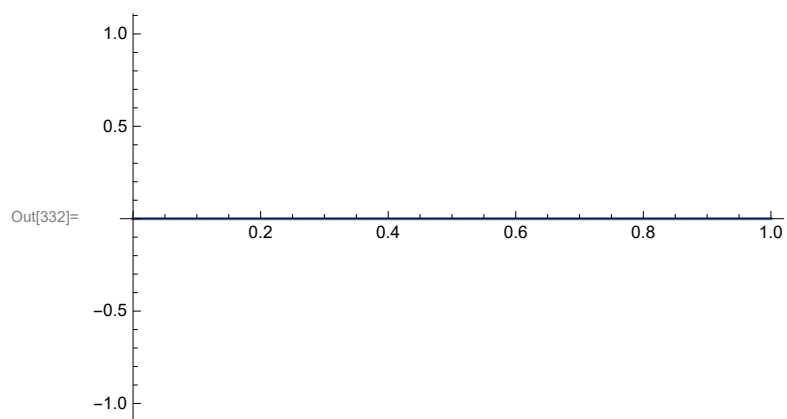

```
Plot[Cf[13, 2, 5], {x, 0, 1}]
```

[绘图](#)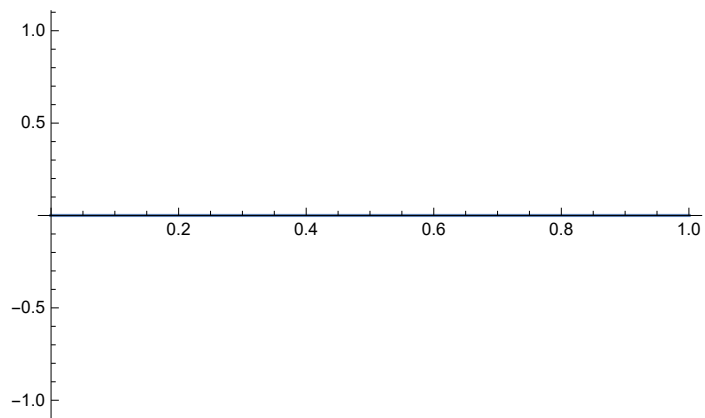

```
Plot[Cf[13, 2, 4], {x, 0, 1}]
```

[绘图](#)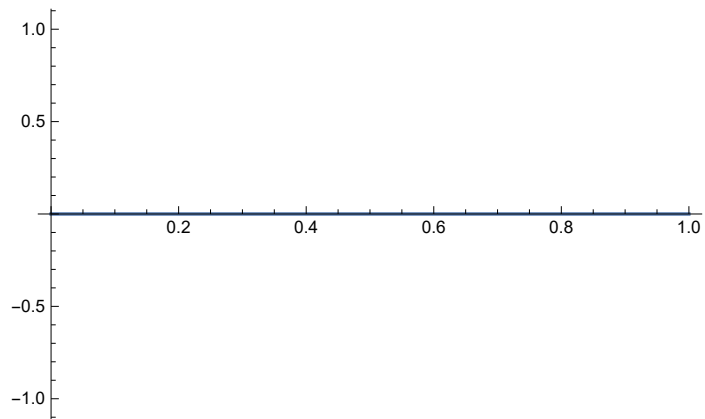

```
Plot[Cf[13, 2, 3], {x, 0, 1}]
```

[绘图](#)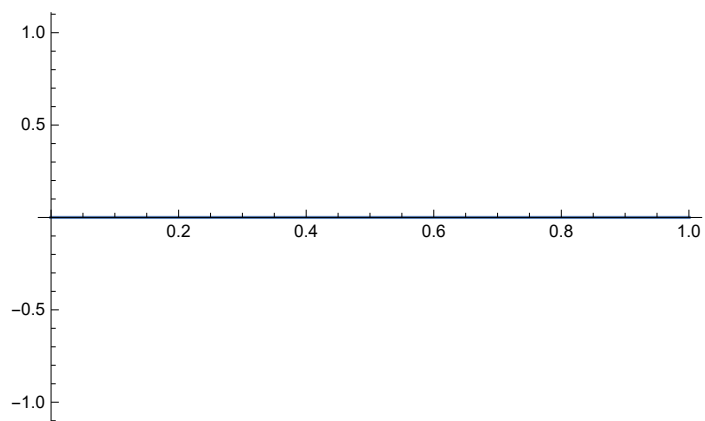

**Plot[Cf[13, 2, 2], {x, 0, 1}]**

[绘图](#)

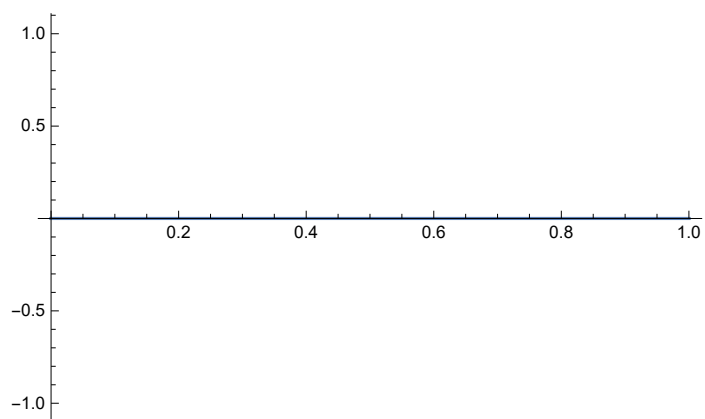

**Plot[Cf[13, 2, 1], {x, 0, 1}]**

[绘图](#)

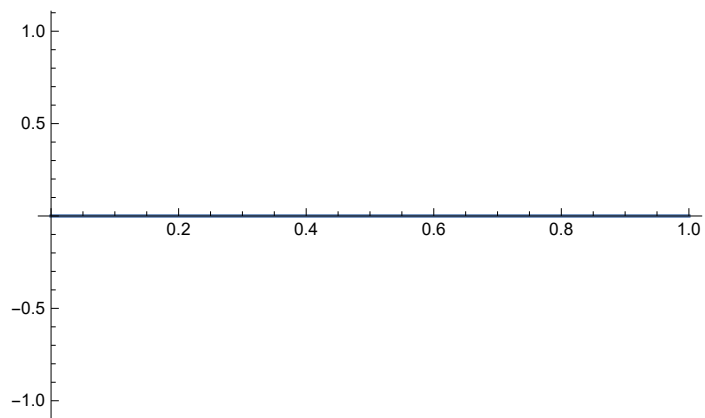

**Plot[Cf[13, 2, 0], {x, 0, 1}]**

[绘图](#)

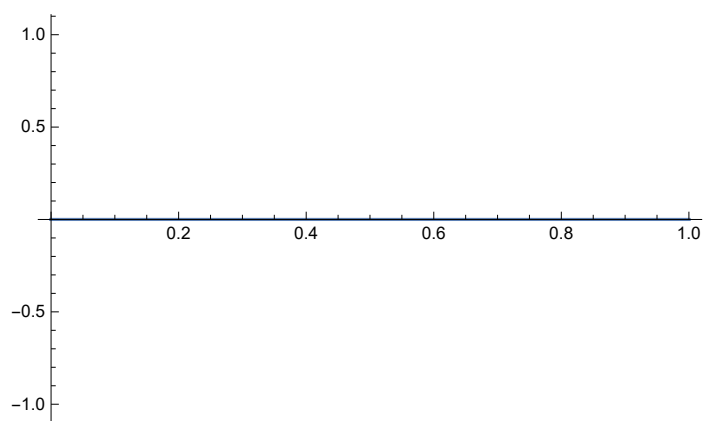

**(\*29th group coefficients r2^13r3^1\*)**

In[333]:= **Plot**[**Cf**[13, 1, 14], {x, 0, 1}]

[绘图](#)

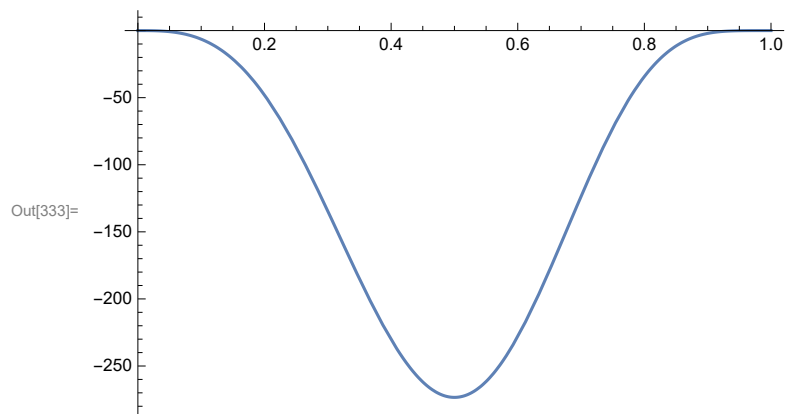

In[334]:= **Plot**[**Cf**[13, 1, 13], {x, 0, 1}]

[绘图](#)

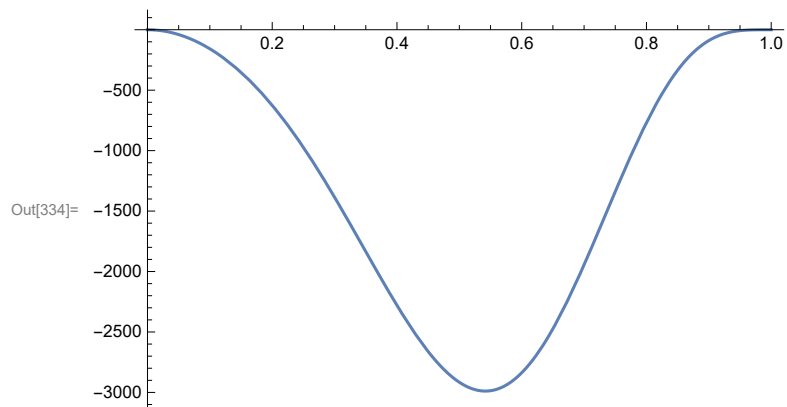

In[335]:= **Plot**[**Cf**[13, 1, 12], {x, 0, 1}]

[绘图](#)

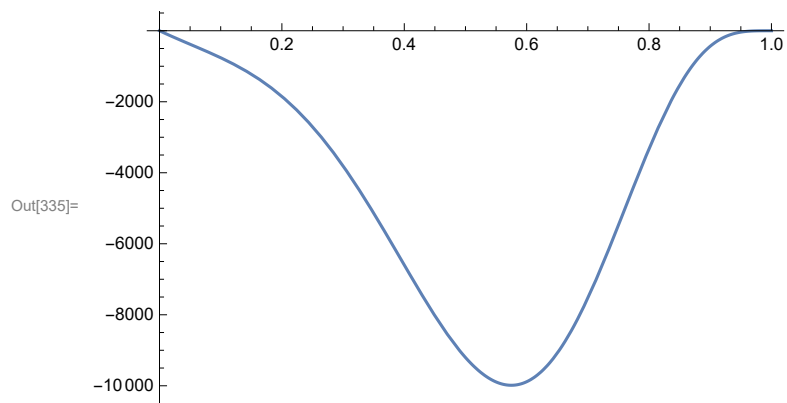

In[336]:= **Plot**[**Cf**[13, 1, 11], {x, 0, 1}]

[绘图](#)

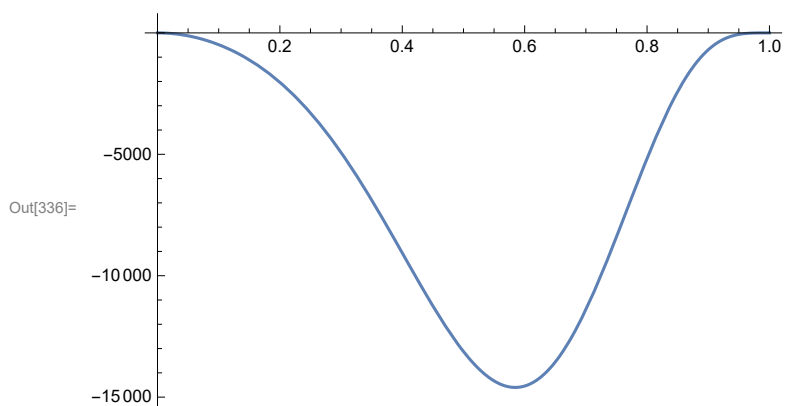

In[337]:= **Plot**[**Cf**[13, 1, 10], {x, 0, 1}]

[绘图](#)

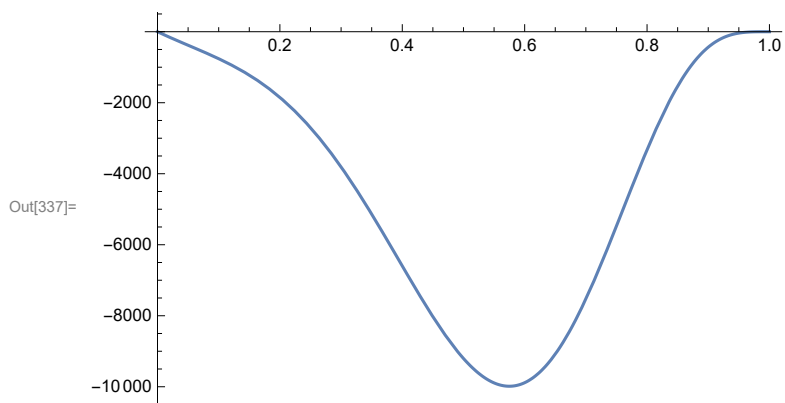

In[338]:= **Plot**[**Cf**[13, 1, 9], {x, 0, 1}]

[绘图](#)

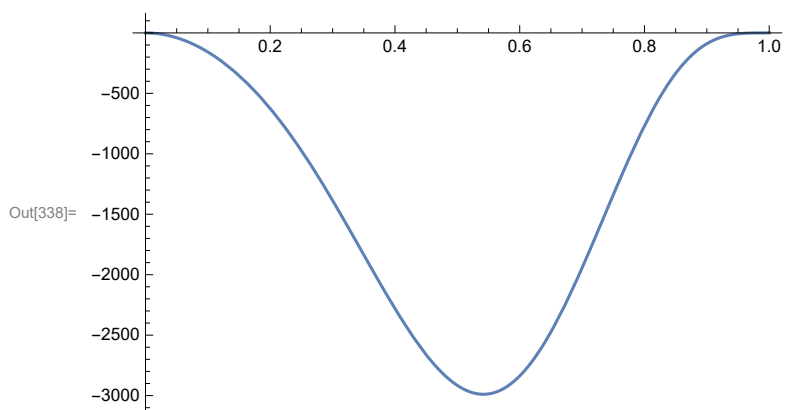

In[339]:= **Plot[Cf[13, 1, 8], {x, 0, 1}]**

[绘图](#)

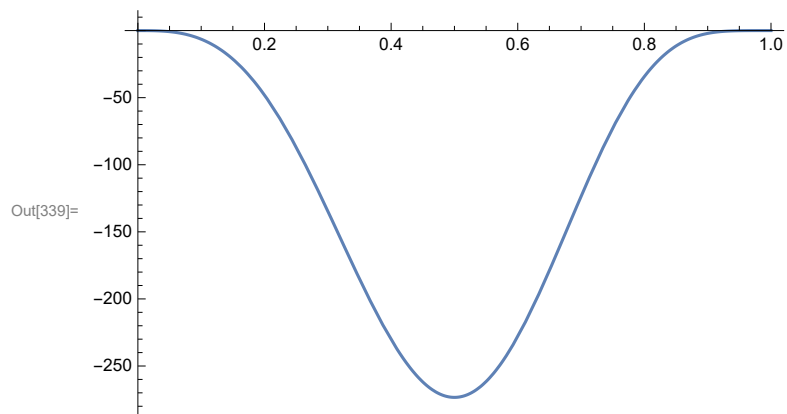

**Plot[Cf[13, 1, 7], {x, 0, 1}]**

[绘图](#)

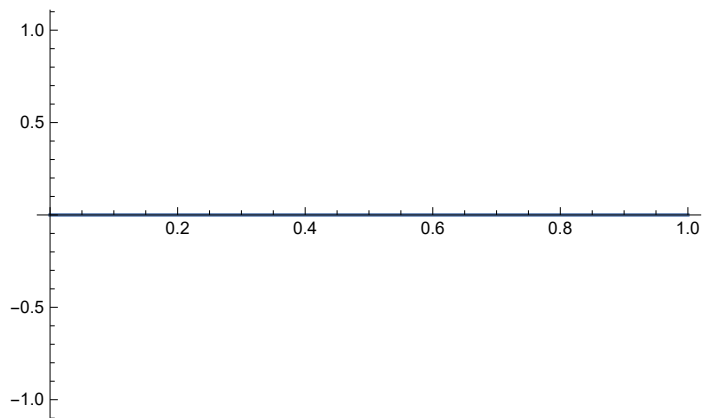

**Plot[Cf[13, 1, 6], {x, 0, 1}]**

[绘图](#)

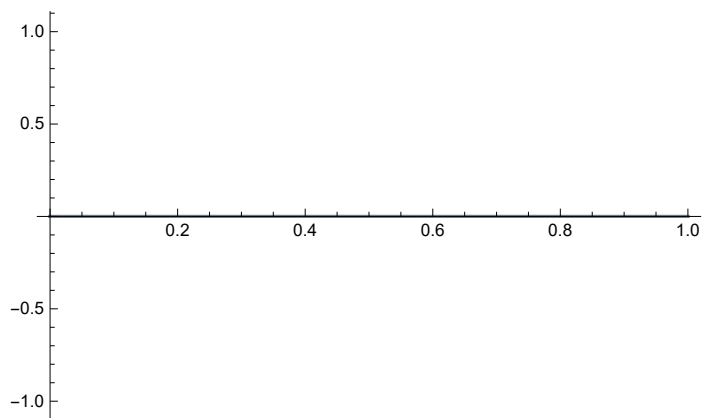



```
Plot[Cf[13, 1, 5], {x, 0, 1}]
```

[绘图](#)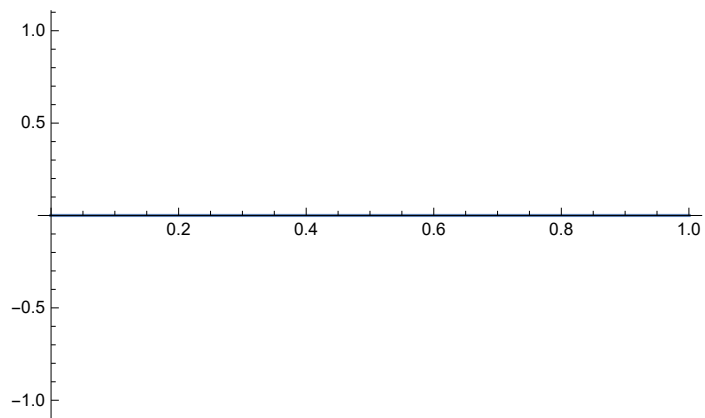

```
Plot[Cf[13, 1, 4], {x, 0, 1}]
```

[绘图](#)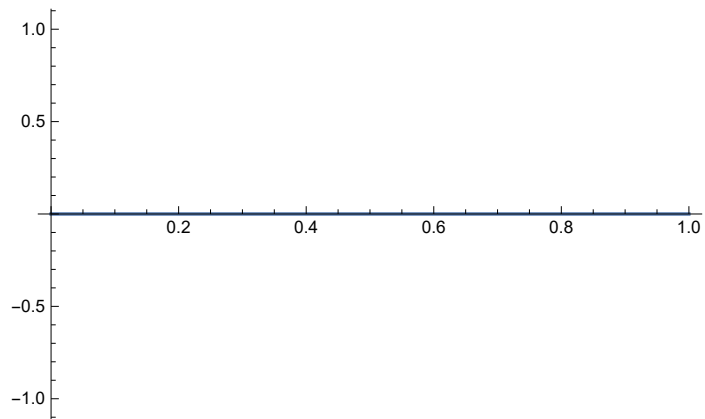

```
Plot[Cf[13, 1, 3], {x, 0, 1}]
```

[绘图](#)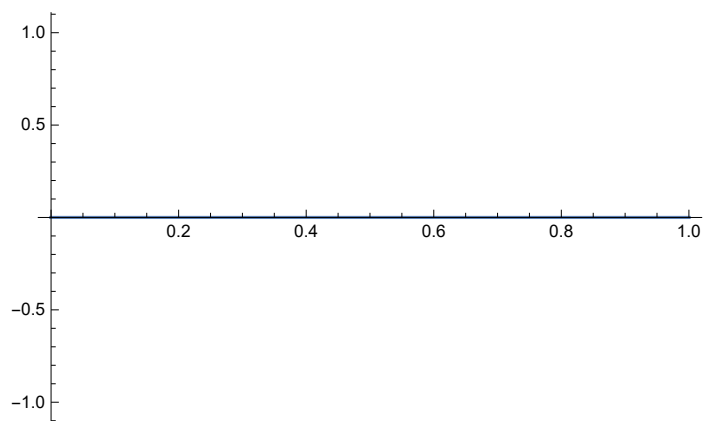

**Plot[Cf[13, 1, 2], {x, 0, 1}]**

[绘图](#)

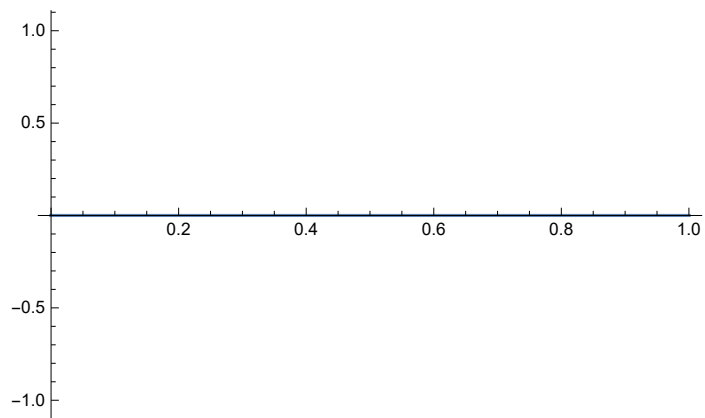

**Plot[Cf[13, 1, 1], {x, 0, 1}]**

[绘图](#)

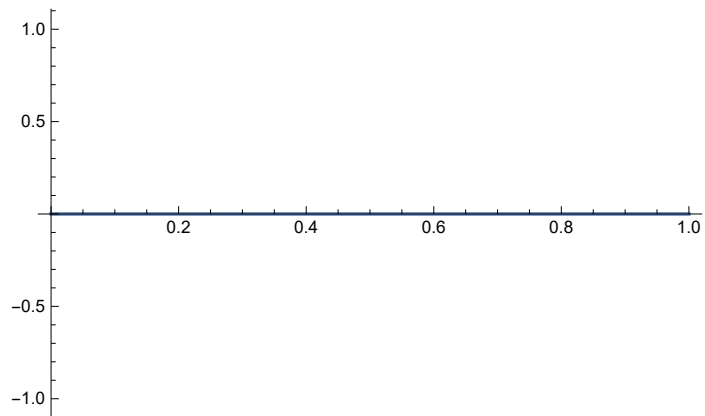

**(\*30th group coefficients r2^13r3^0\*)**

In[340]:= **Plot[Cf[13, 0, 14], {x, 0, 1}]**

[绘图](#)

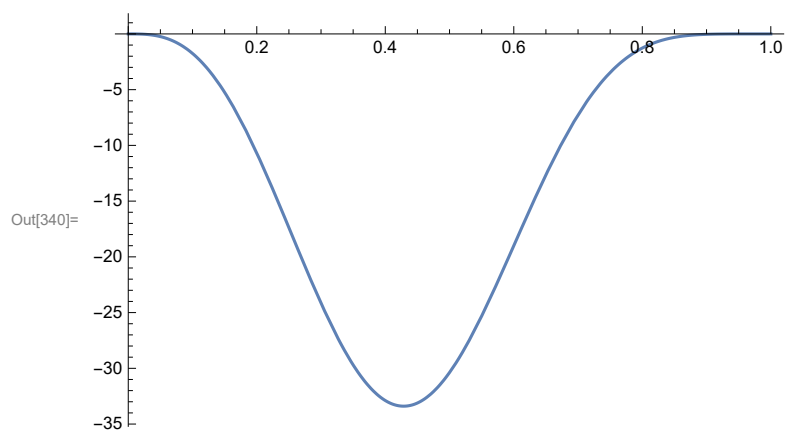

In[341]:= **Plot**[**Cf**[13, 0, 13], {x, 0, 1}]

[绘图](#)

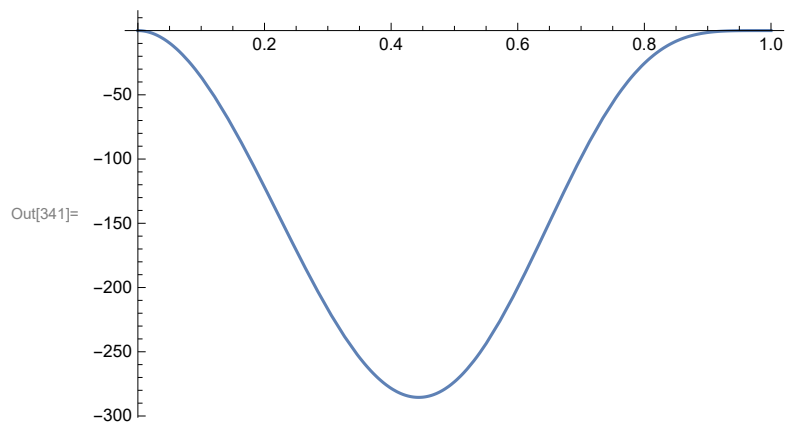

In[342]:= **Plot**[**Cf**[13, 0, 12], {x, 0, 1}]

[绘图](#)

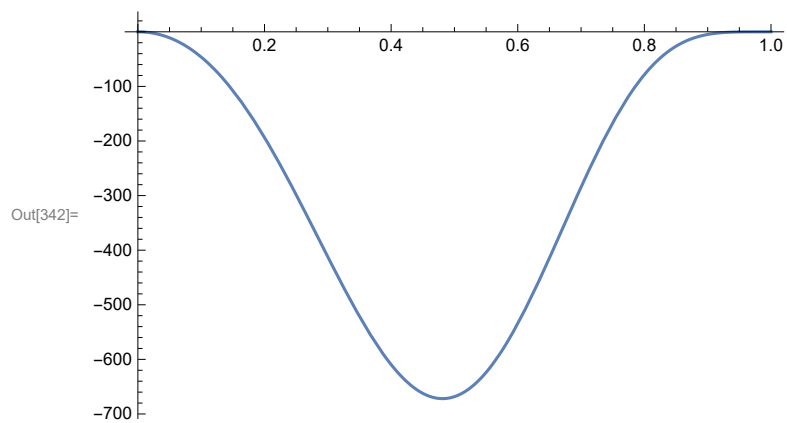

In[343]:= **Plot**[**Cf**[13, 0, 11], {x, 0, 1}]

[绘图](#)

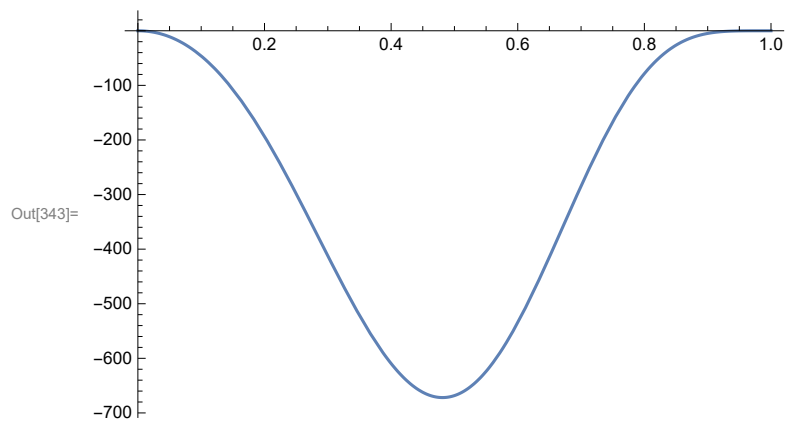

In[344]:= **Plot[Cf[13, 0, 10], {x, 0, 1}]**

[绘图](#)

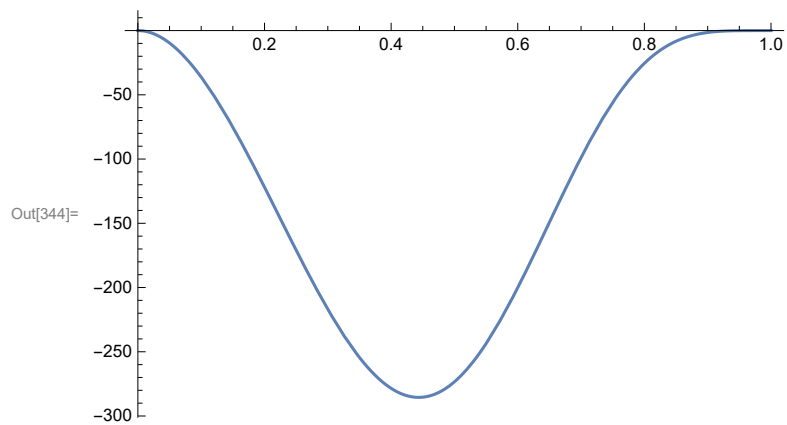

In[345]:= **Plot[Cf[13, 0, 9], {x, 0, 1}]**

[绘图](#)

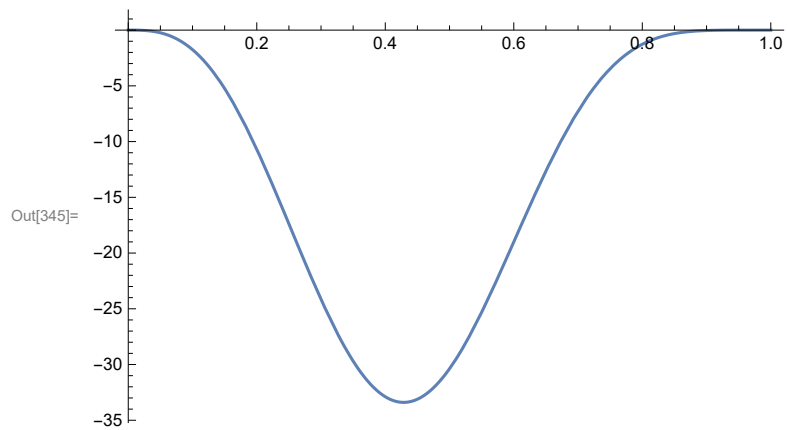

**Plot[Cf[13, 0, 8], {x, 0, 1}]**

[绘图](#)

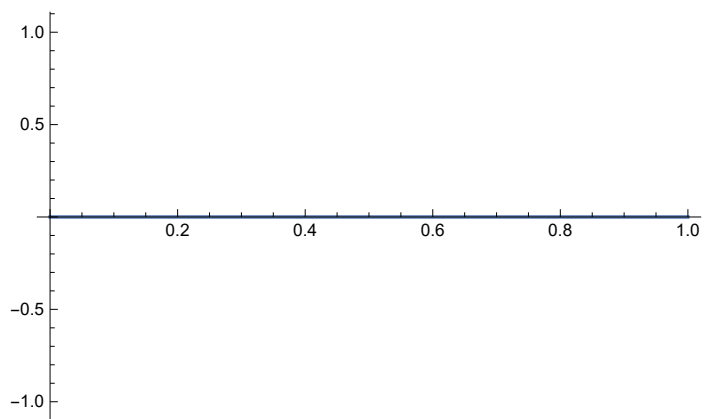

```
Plot[Cf[13, 0, 7], {x, 0, 1}]
```

[绘图](#)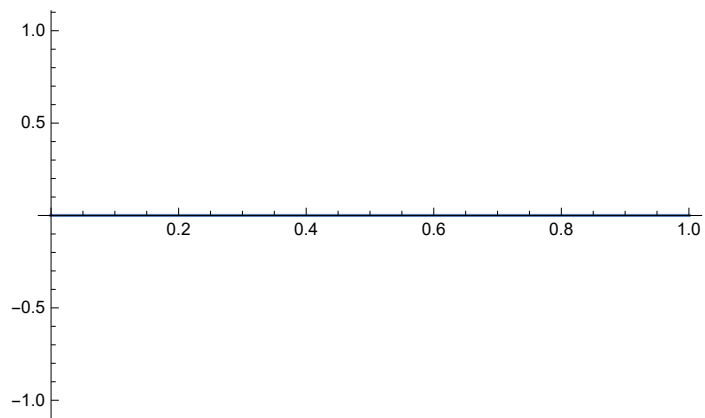

```
Plot[Cf[13, 0, 6], {x, 0, 1}]
```

[绘图](#)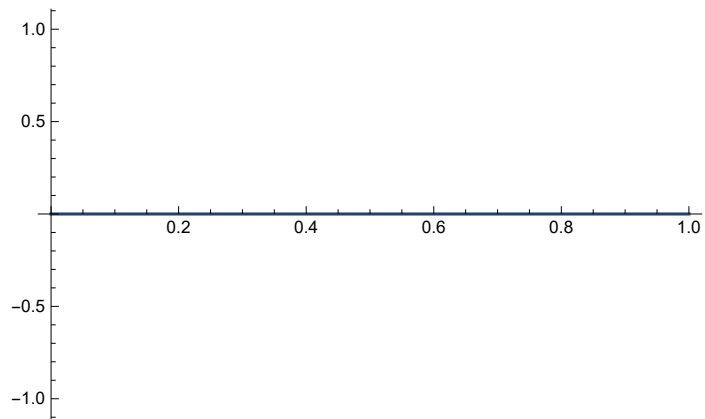

```
Plot[Cf[13, 0, 5], {x, 0, 1}]
```

[绘图](#)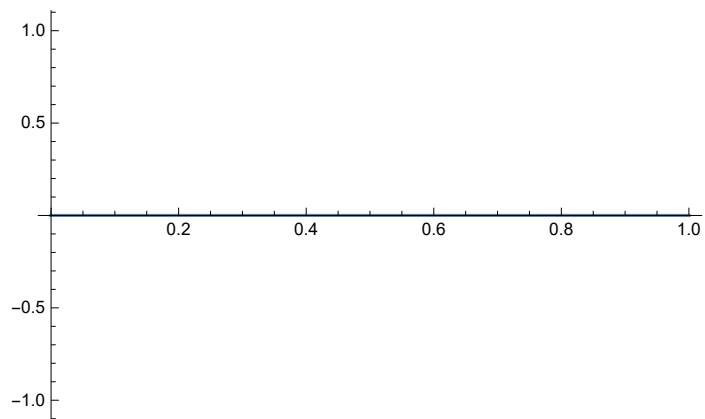

```
Plot[Cf[13, 0, 4], {x, 0, 1}]
```

[绘图](#)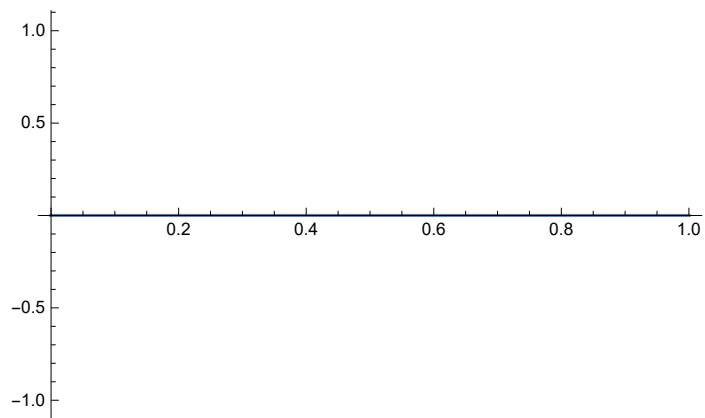

```
Plot[Cf[13, 0, 3], {x, 0, 1}]
```

[绘图](#)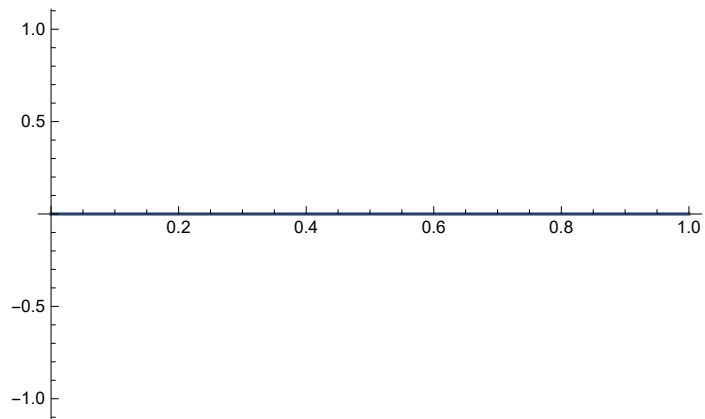

```
Plot[Cf[13, 0, 2], {x, 0, 1}]
```

[绘图](#)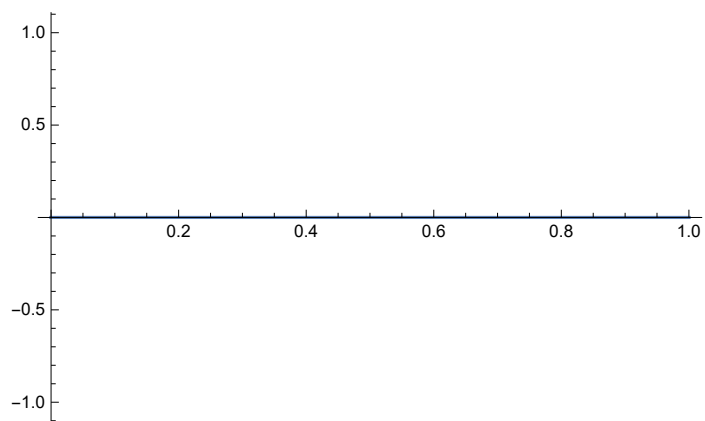

**Plot[Cf[13, 0, 1], {x, 0, 1}]**

[绘图](#)

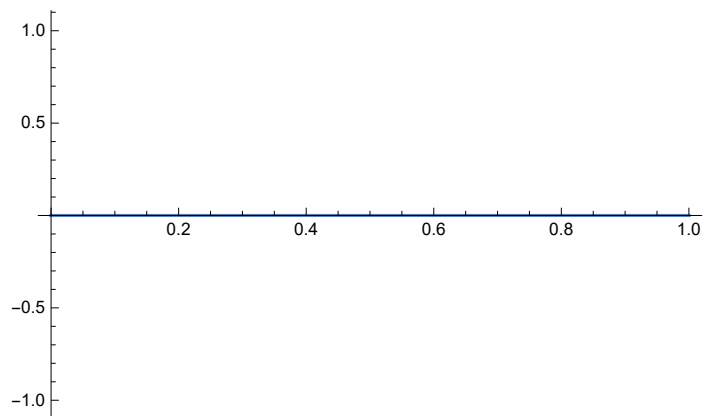

**Plot[Cf[13, 0, 0], {x, 0, 1}]**

[绘图](#)

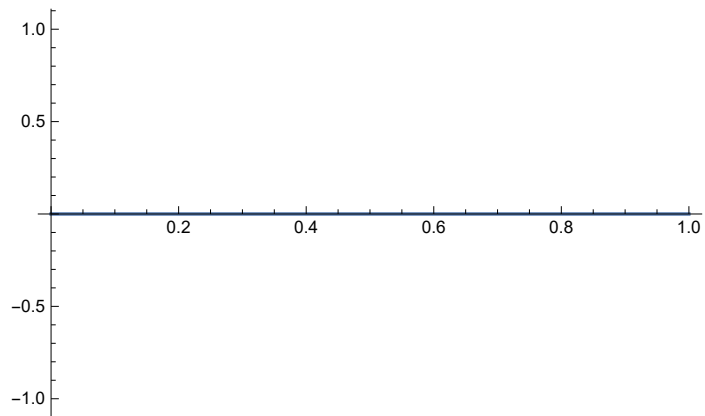

**(\*31th group coefficients r2^12r3^14\*)**

**Plot[Cf[12, 14, 14], {x, 0, 1}]**

[绘图](#)

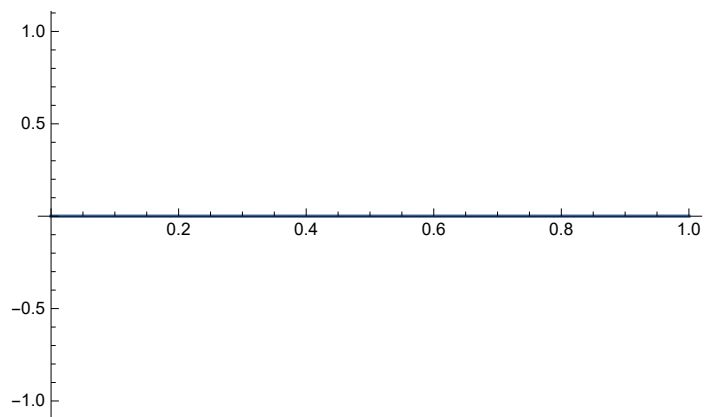

**Plot[Cf[12, 14, 13], {x, 0, 1}]**

[绘图](#)

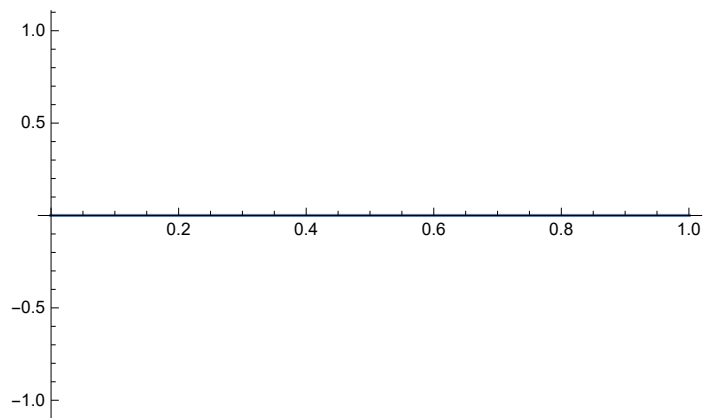

**Plot[Cf[12, 14, 12], {x, 0, 1}]**

[绘图](#)

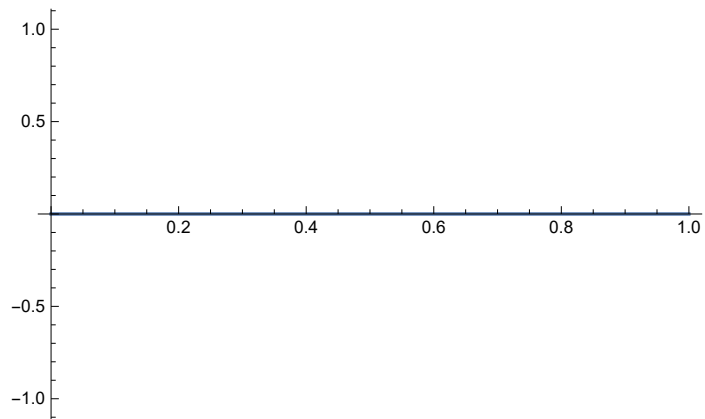

**Plot[Cf[12, 14, 11], {x, 0, 1}]**

[绘图](#)

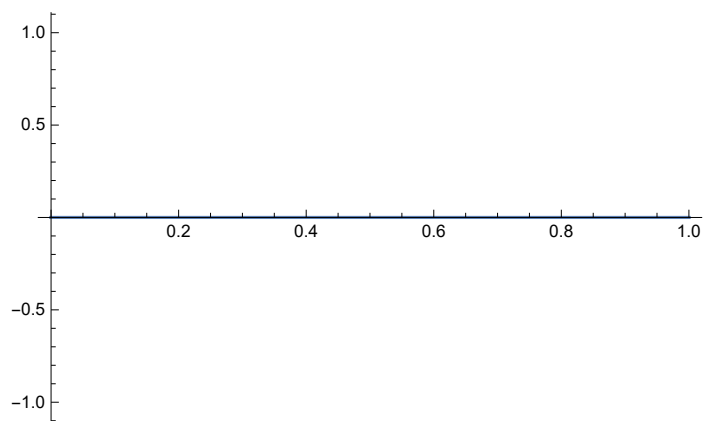



In[346]:= **Plot[Cf[12, 14, 10], {x, 0, 1}]**

[绘图](#)

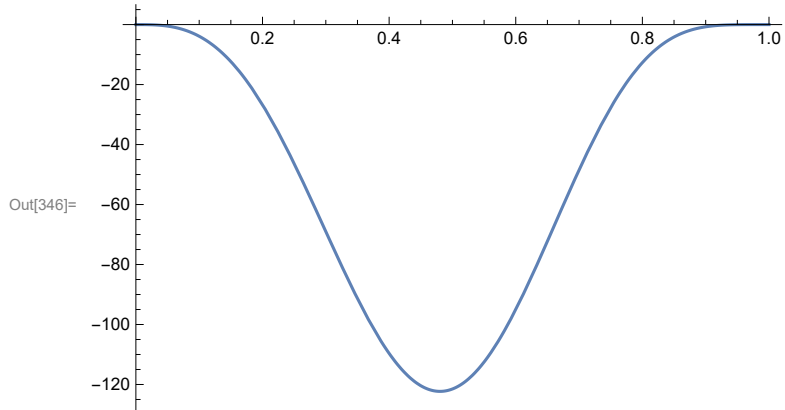

In[347]:= **Plot[Cf[12, 14, 9], {x, 0, 1}]**

[绘图](#)

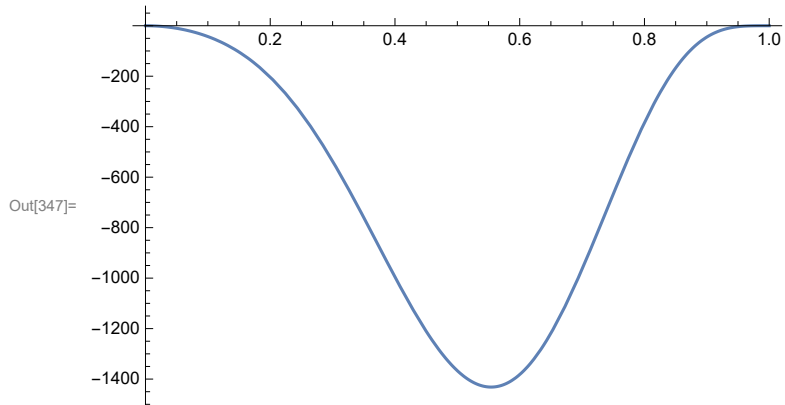

In[348]:= **Plot[Cf[12, 14, 8], {x, 0, 1}]**

[绘图](#)

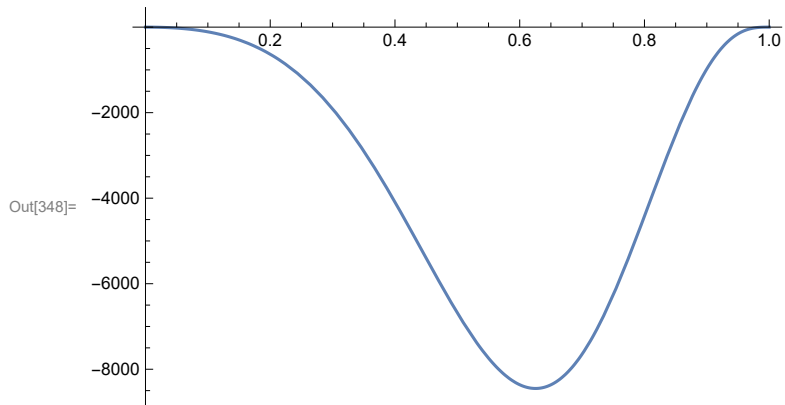

In[349]:= **Plot[Cf[12, 14, 7], {x, 0, 1}]**

[绘图](#)

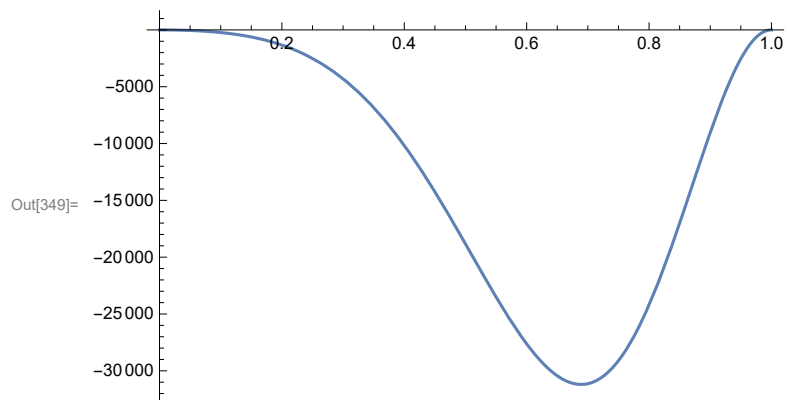

In[350]:= **Plot[Cf[12, 14, 6], {x, 0, 1}]**

[绘图](#)

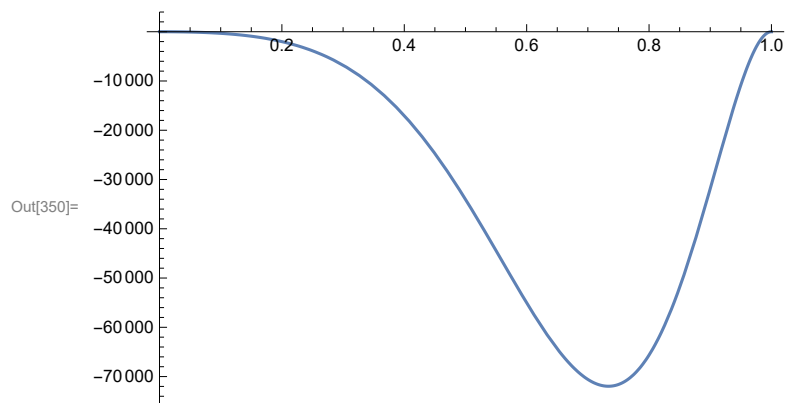

In[351]:= **Plot[Cf[12, 14, 5], {x, 0, 1}]**

[绘图](#)

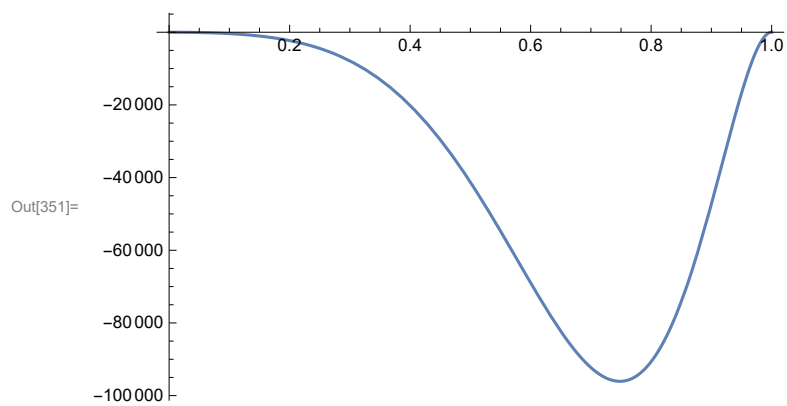

In[352]:= **Plot[Cf[12, 14, 4], {x, 0, 1}]**

[绘图](#)

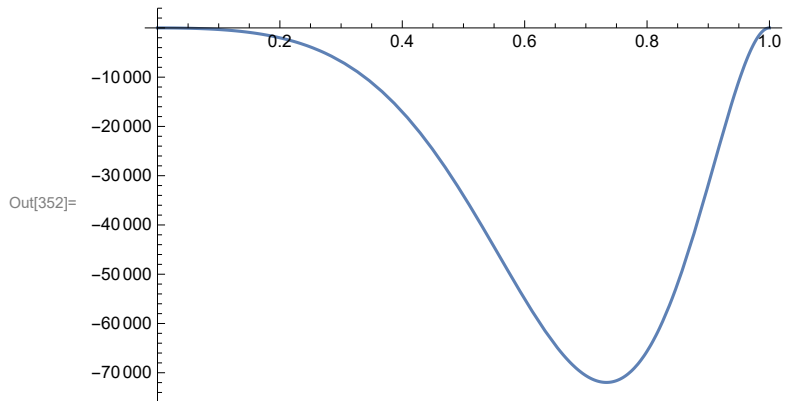

In[353]:= **Plot[Cf[12, 14, 3], {x, 0, 1}]**

[绘图](#)

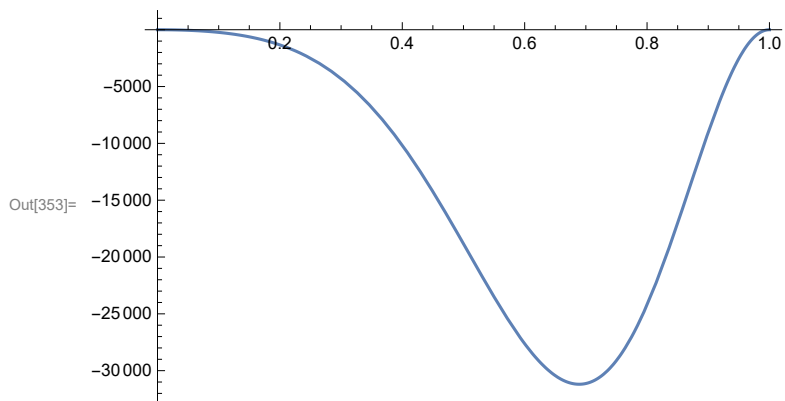

In[354]:= **Plot[Cf[12, 14, 2], {x, 0, 1}]**

[绘图](#)

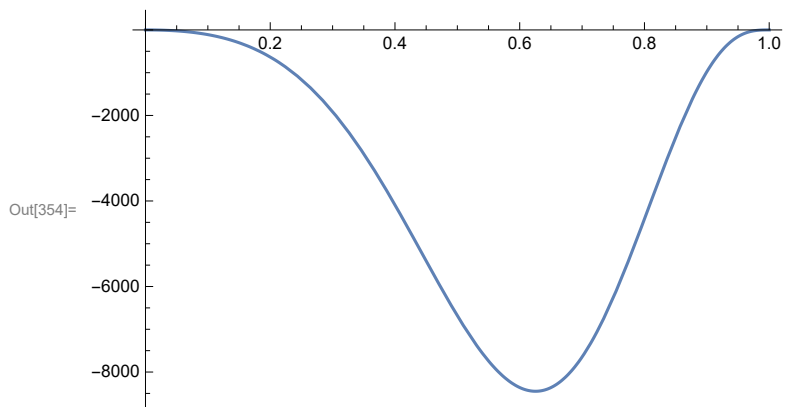

In[355]:= **Plot[Cf[12, 14, 1], {x, 0, 1}]**

[绘图](#)

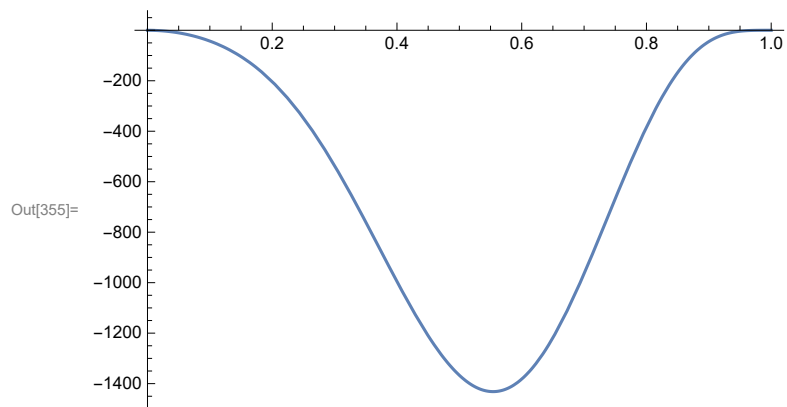

In[356]:= **Plot[Cf[12, 14, 0], {x, 0, 1}]**

[绘图](#)

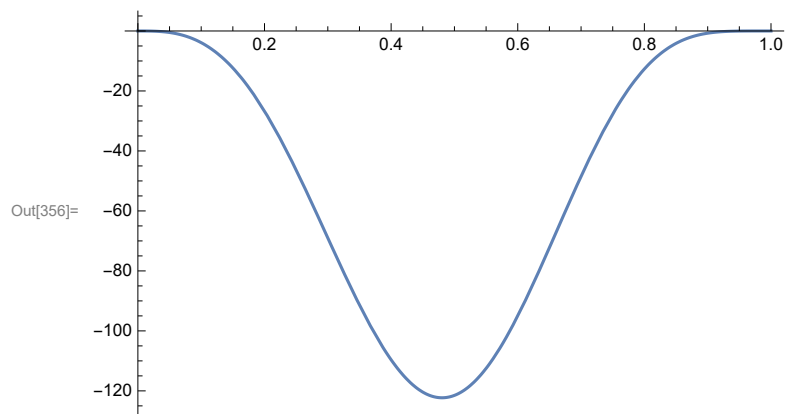

(\*32th group coefficients  $r_2^{12}r_3^{13}$ \*)

**Plot[Cf[12, 13, 14], {x, 0, 1}]**

[绘图](#)

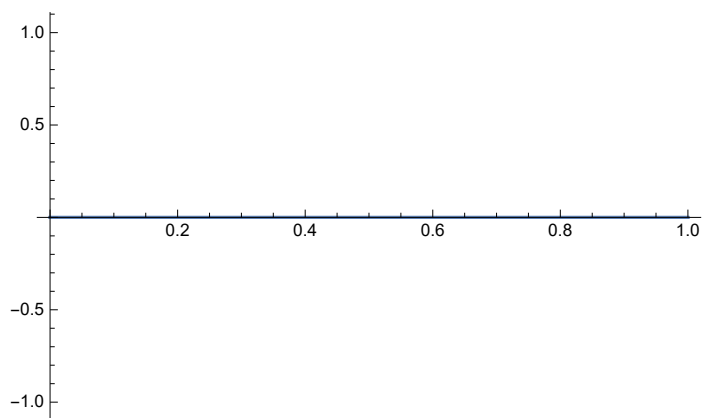

**Plot[Cf[12, 13, 13], {x, 0, 1}]**

[绘图](#)

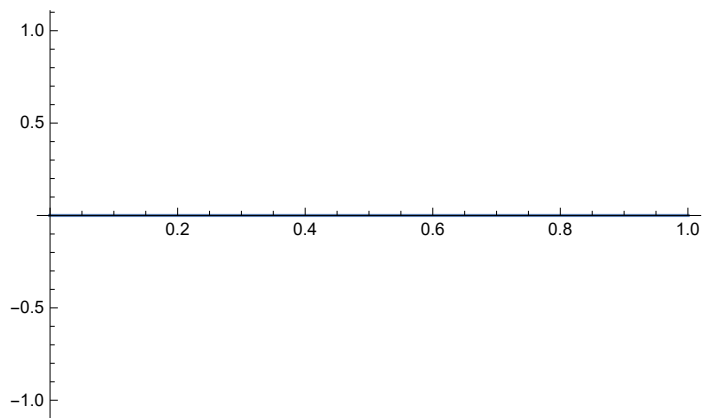

**Plot[Cf[12, 13, 12], {x, 0, 1}]**

[绘图](#)

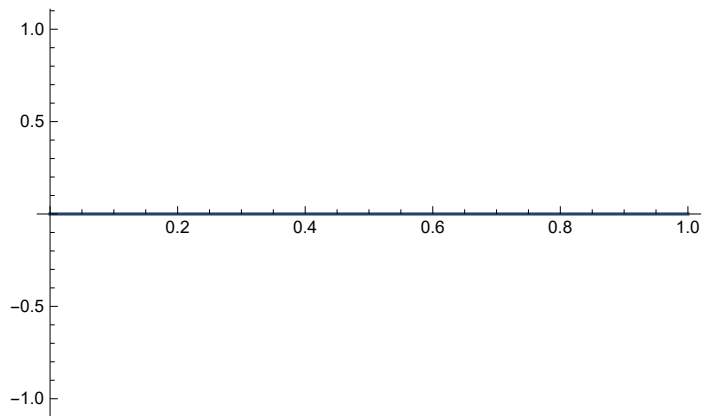

In[357]:= **Plot[Cf[12, 13, 11], {x, 0, 1}]**

[绘图](#)

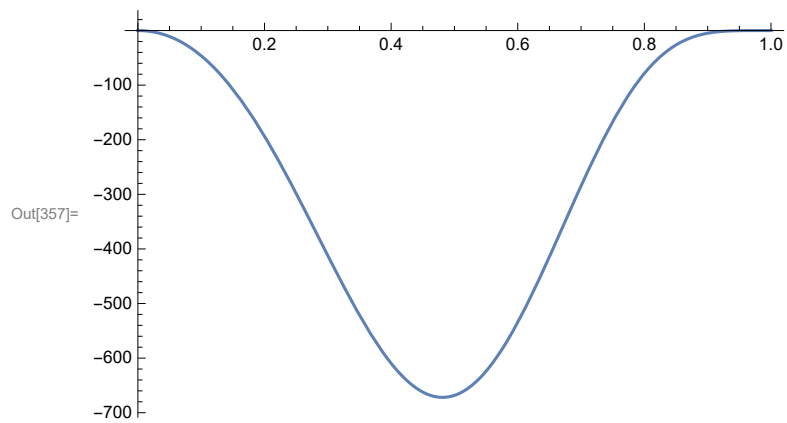

In[358]:= **Plot[Cf[12, 13, 10], {x, 0, 1}]**

[绘图](#)

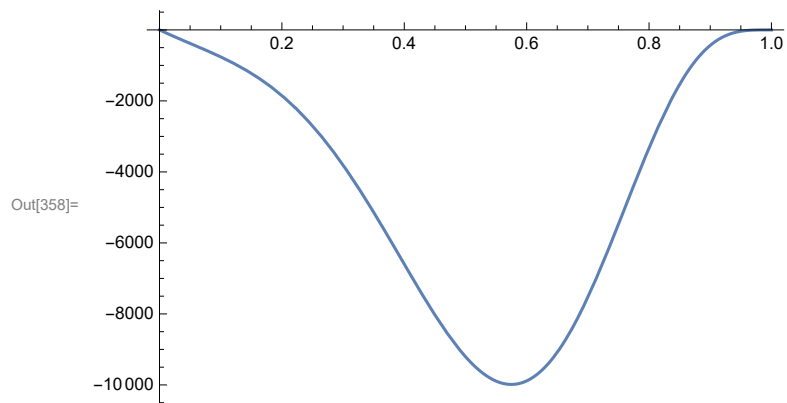

In[359]:= **Plot[Cf[12, 13, 9], {x, 0, 1}]**

[绘图](#)

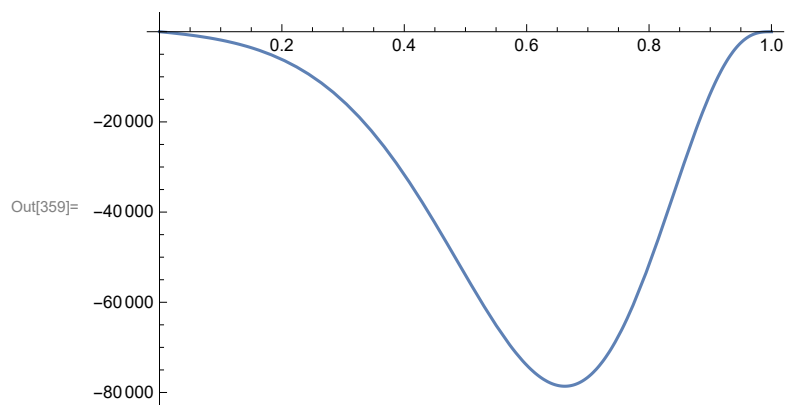

In[360]:= **Plot[Cf[12, 13, 8], {x, 0, 1}]**

[绘图](#)

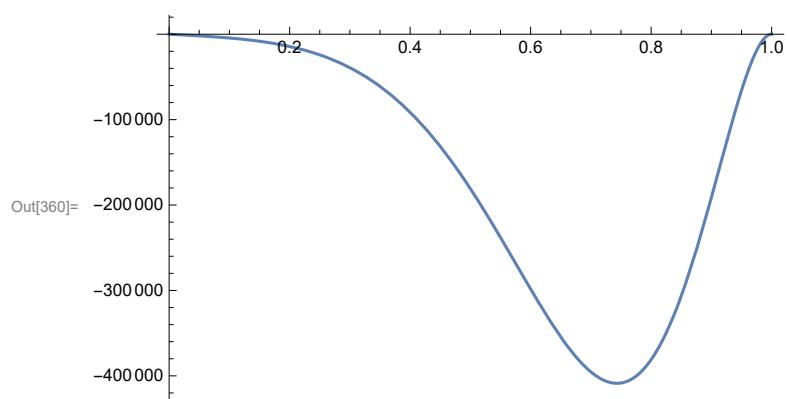

In[361]:= **Plot[Cf[12, 13, 7], {x, 0, 1}]**

[绘图](#)

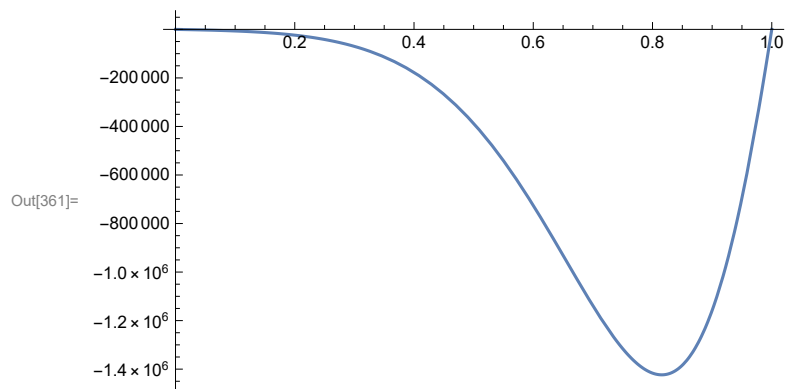

In[362]:= **Plot[Cf[12, 13, 6], {x, 0, 1}]**

[绘图](#)

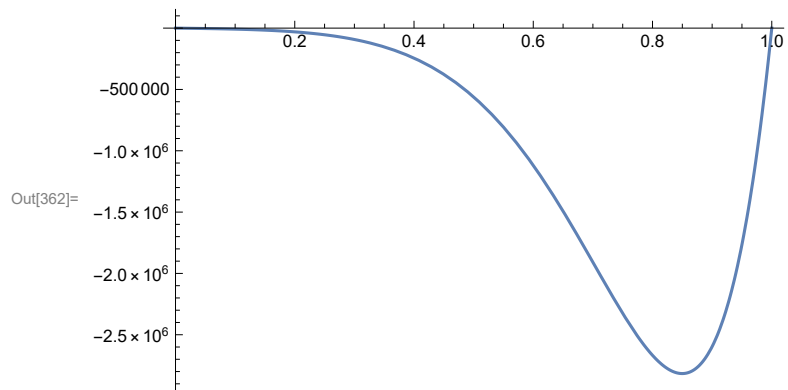

In[363]:= **Plot[Cf[12, 13, 5], {x, 0, 1}]**

[绘图](#)

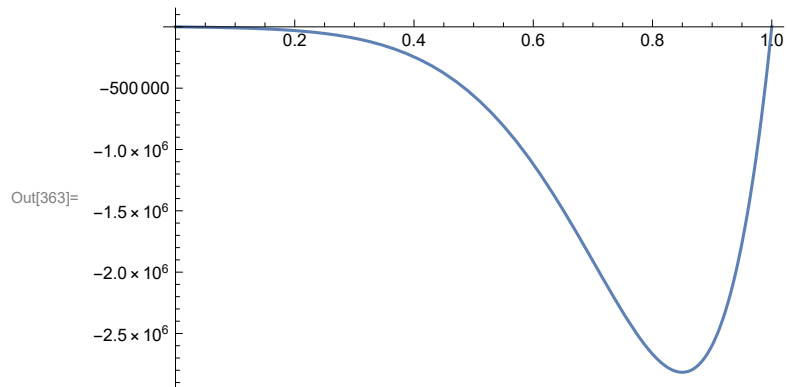

In[364]:= **Plot[Cf[12, 13, 4], {x, 0, 1}]**

[绘图](#)

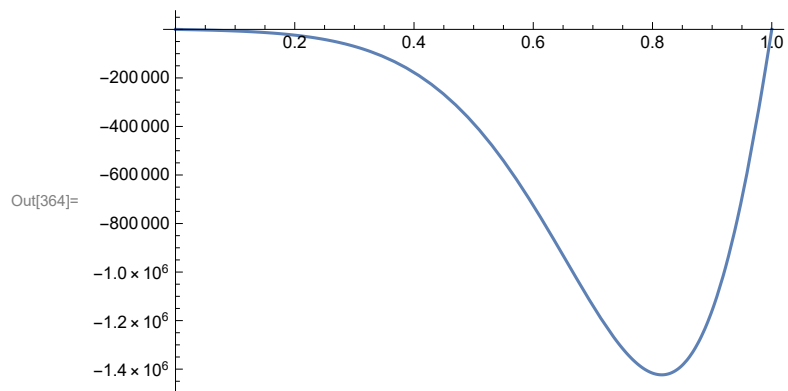

In[365]:= **Plot[Cf[12, 13, 3], {x, 0, 1}]**

[绘图](#)

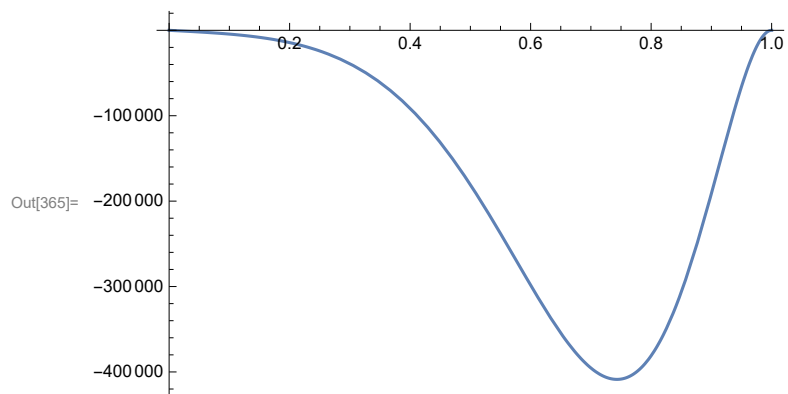

In[366]:= **Plot[Cf[12, 13, 2], {x, 0, 1}]**

[绘图](#)

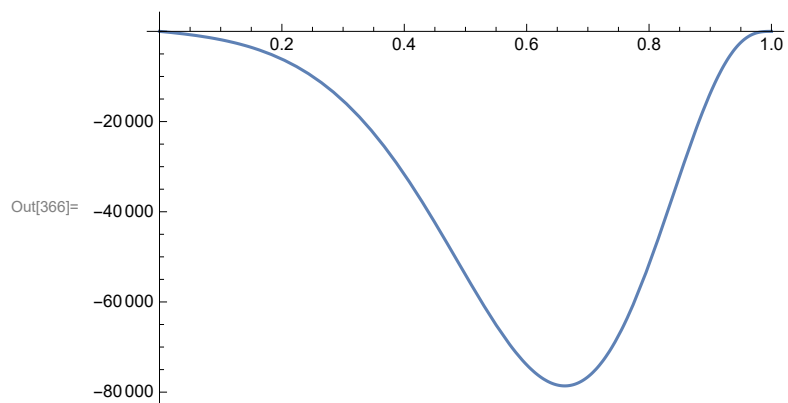



In[367]:= **Plot[Cf[12, 13, 1], {x, 0, 1}]**

[绘图](#)

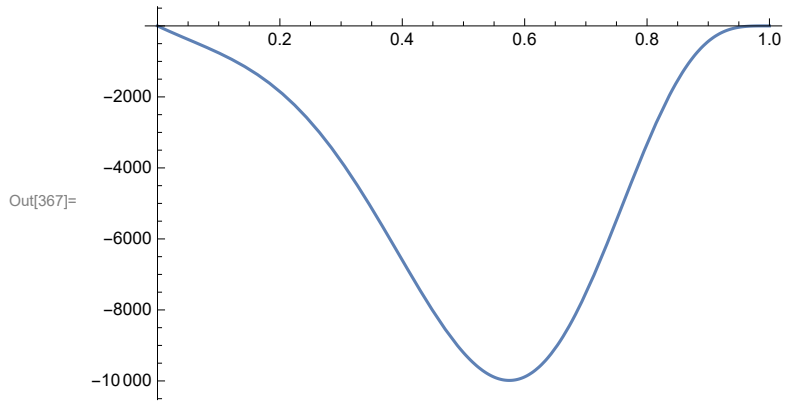

In[368]:= **Plot[Cf[12, 13, 0], {x, 0, 1}]**

[绘图](#)

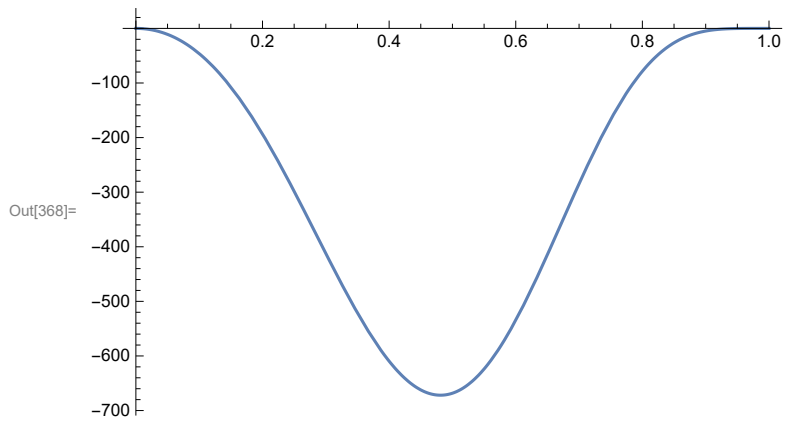

(\*33th group coefficients  $r_2^{12}r_3^{12}$ \*)

**Plot[Cf[12, 12, 14], {x, 0, 1}]**

[绘图](#)

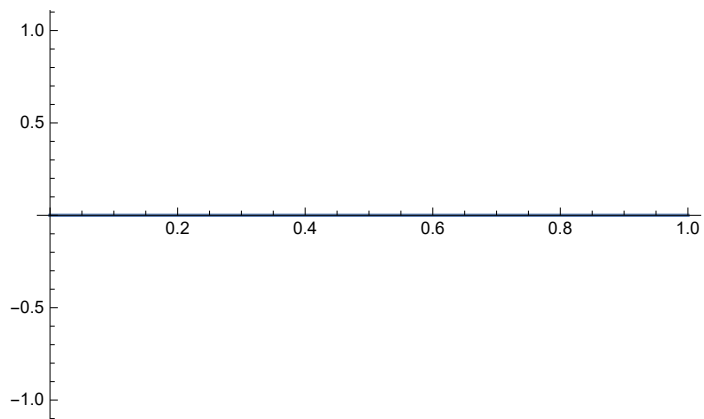

**Plot[Cf[12, 12, 13], {x, 0, 1}]**

[绘图](#)

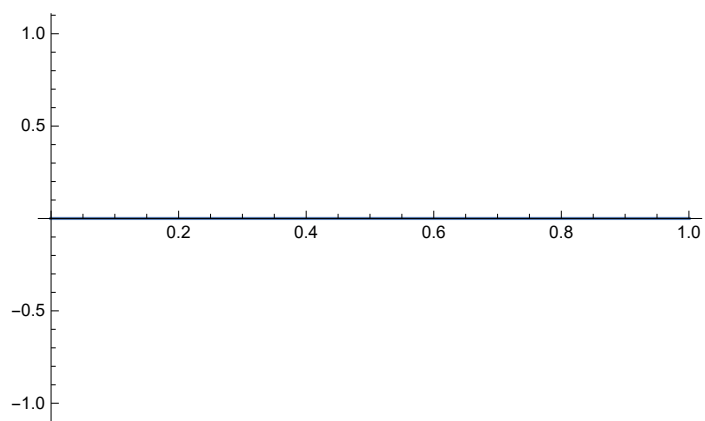

In[369]:= **Plot[Cf[12, 12, 12], {x, 0, 1}]**

[绘图](#)

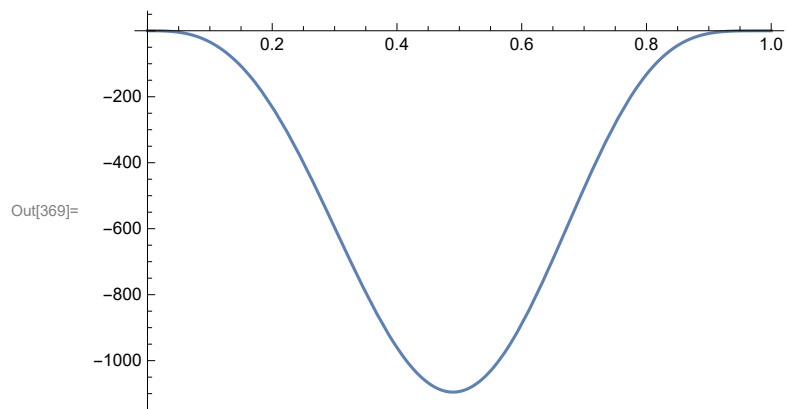

In[370]:= **Plot[Cf[12, 12, 11], {x, 0, 1}]**

[绘图](#)

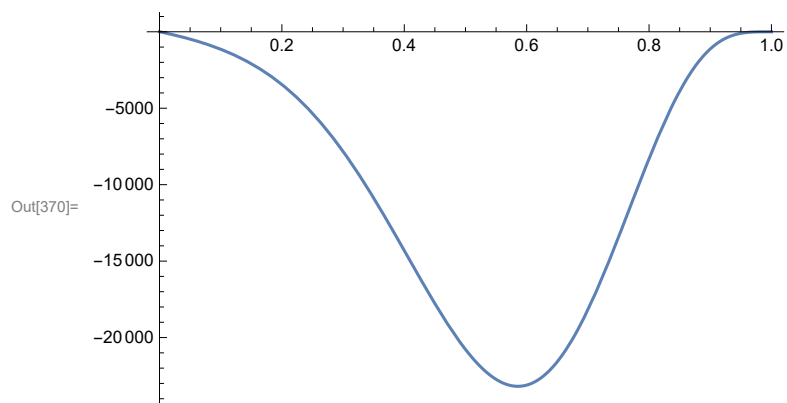

In[371]:= **Plot[Cf[12, 12, 10], {x, 0, 1}]**

[绘图](#)

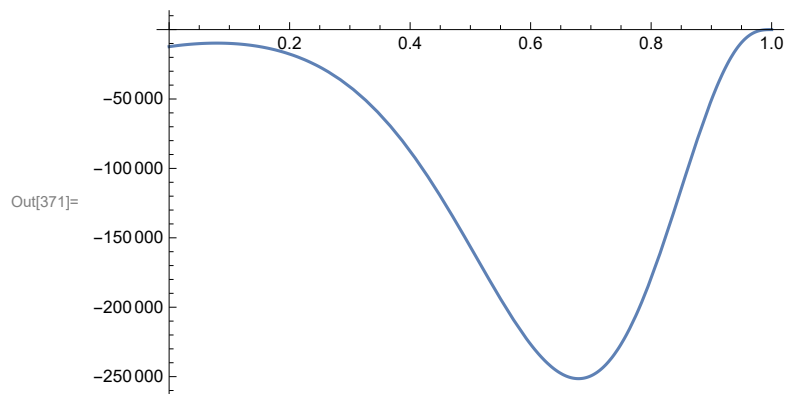

In[372]:= **Plot[Cf[12, 12, 9], {x, 0, 1}]**

[绘图](#)

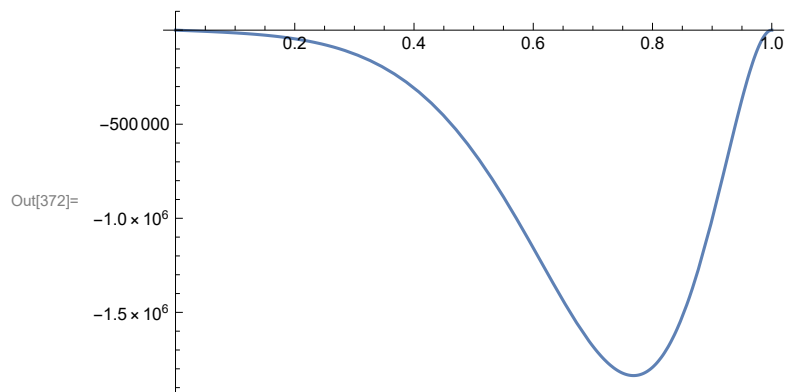

In[373]:= **Plot[Cf[12, 12, 8], {x, 0, 1}]**

[绘图](#)

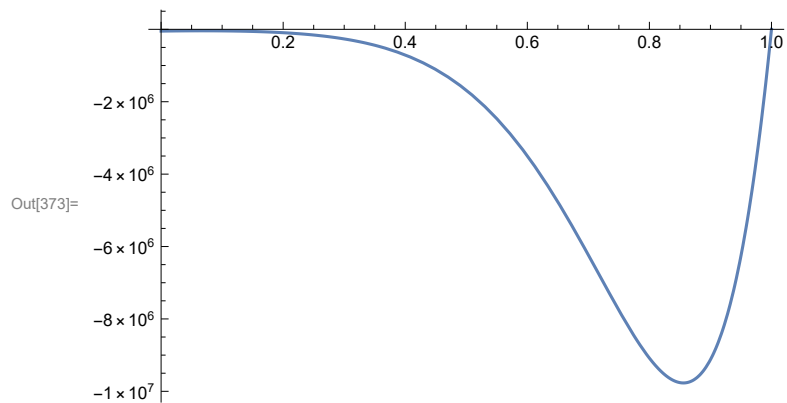

In[374]:= **Plot[Cf[12, 12, 7], {x, 0, 1}]**

[绘图](#)

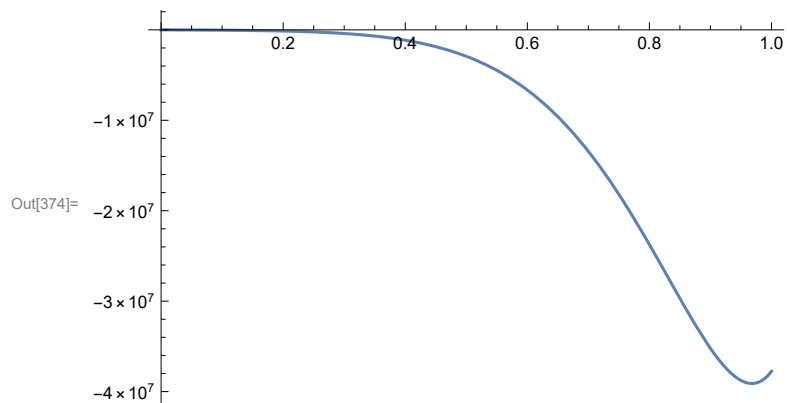

In[375]:= **Plot[Cf[12, 12, 6], {x, 0, 1}]**

[绘图](#)

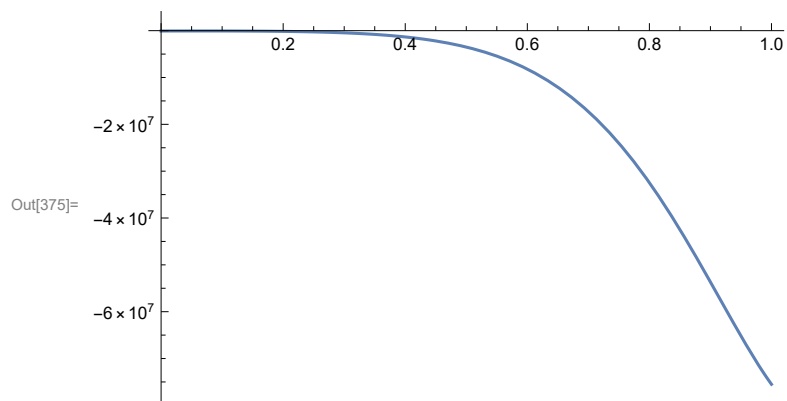

In[376]:= **Plot[Cf[12, 12, 5], {x, 0, 1}]**

[绘图](#)

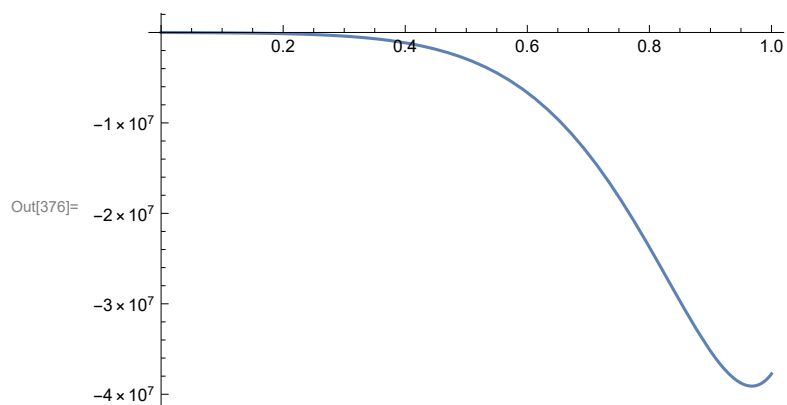

In[377]:= **Plot[Cf[12, 12, 4], {x, 0, 1}]**

[绘图](#)

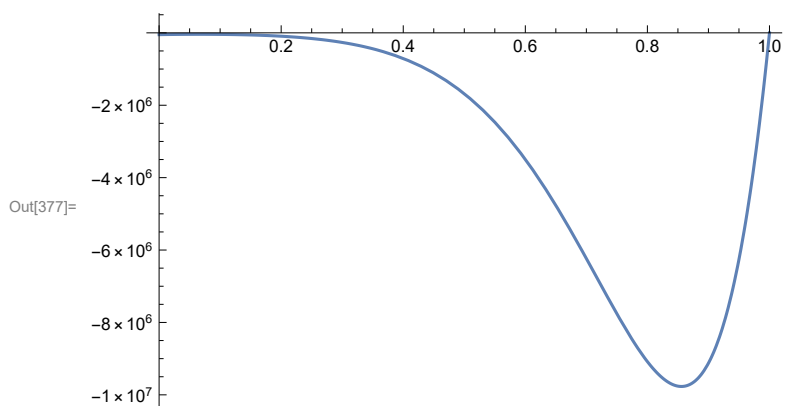

In[378]:= **Plot[Cf[12, 12, 3], {x, 0, 1}]**

[绘图](#)

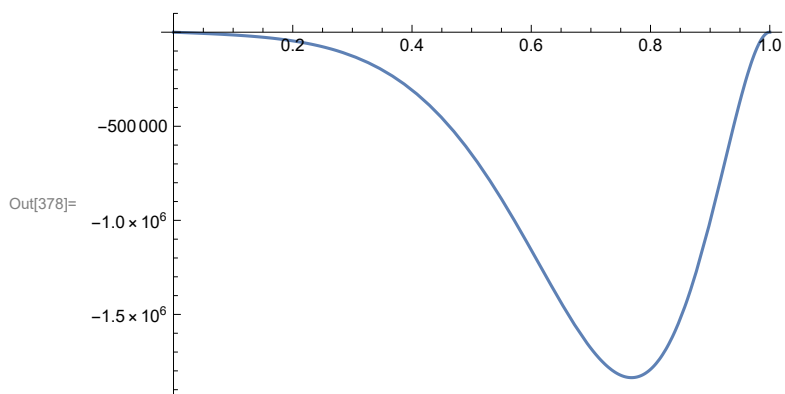

In[379]:= **Plot[Cf[12, 12, 2], {x, 0, 1}]**

[绘图](#)

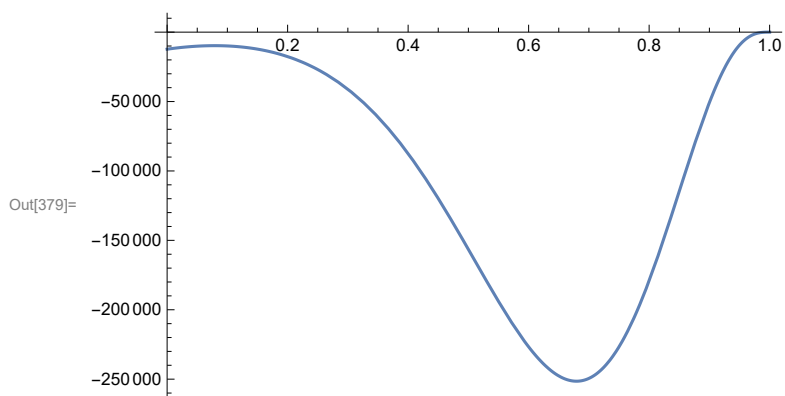

In[380]:= **Plot[Cf[12, 12, 1], {x, 0, 1}]**

[绘图](#)

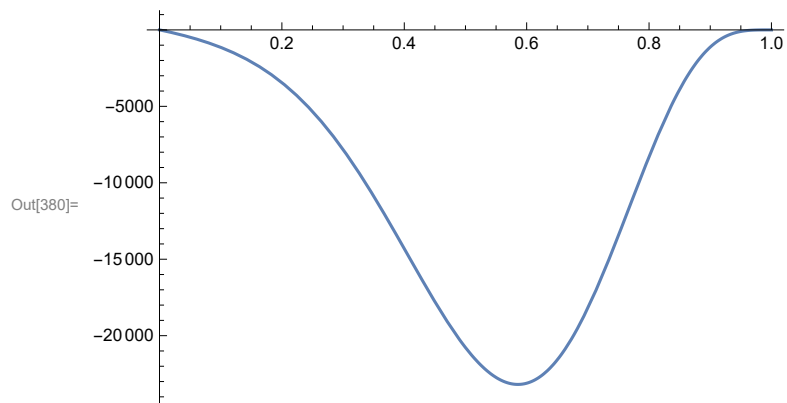

In[381]:= **Plot[Cf[12, 12, 0], {x, 0, 1}]**

[绘图](#)

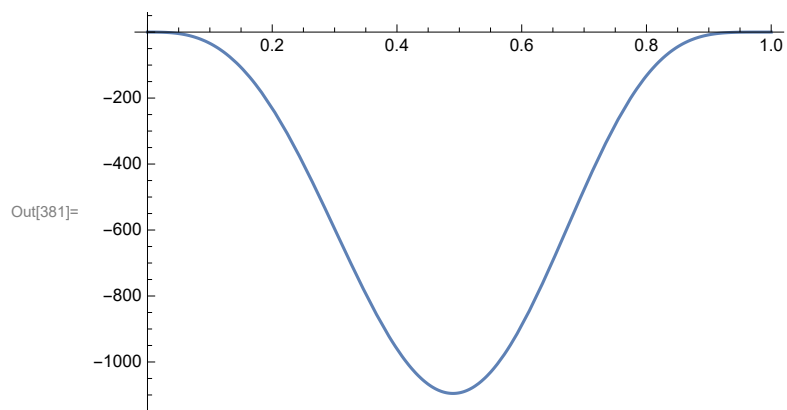

(\*34th group coefficients  $r_2^{12}r_3^{11}$ \*)

**Plot[Cf[12, 11, 14], {x, 0, 1}]**

[绘图](#)

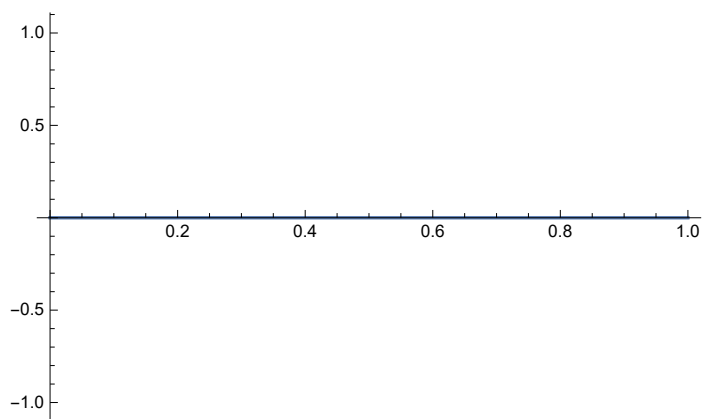

In[382]:= **Plot**[**Cf**[12, 11, 13], {x, 0, 1}]

[绘图](#)

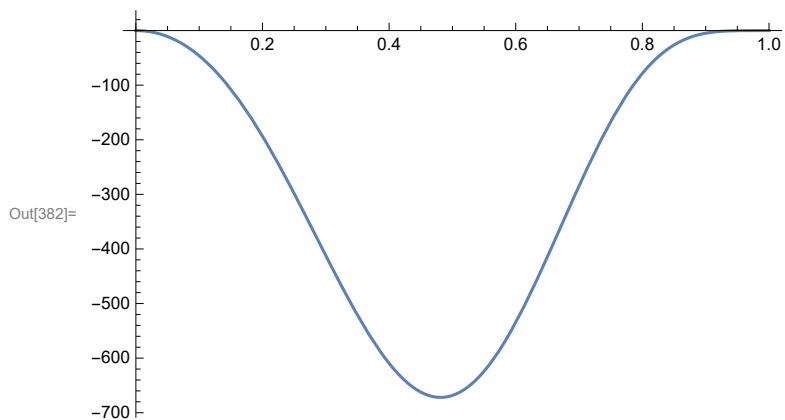

In[383]:= **Plot**[**Cf**[12, 11, 12], {x, 0, 1}]

[绘图](#)

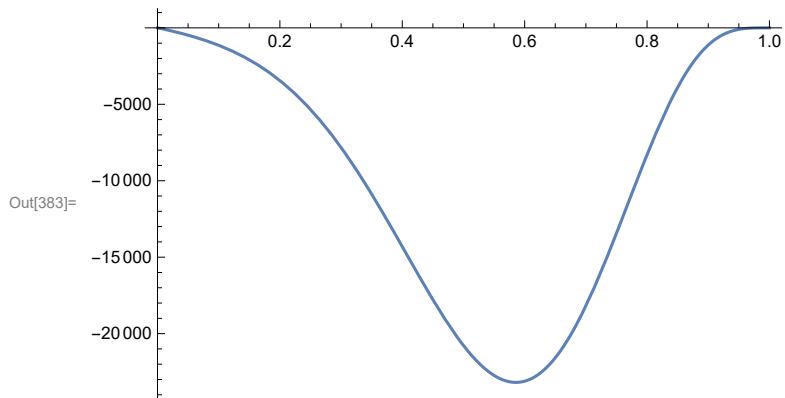

In[384]:= **Plot**[**Cf**[12, 11, 11], {x, 0, 1}]

[绘图](#)

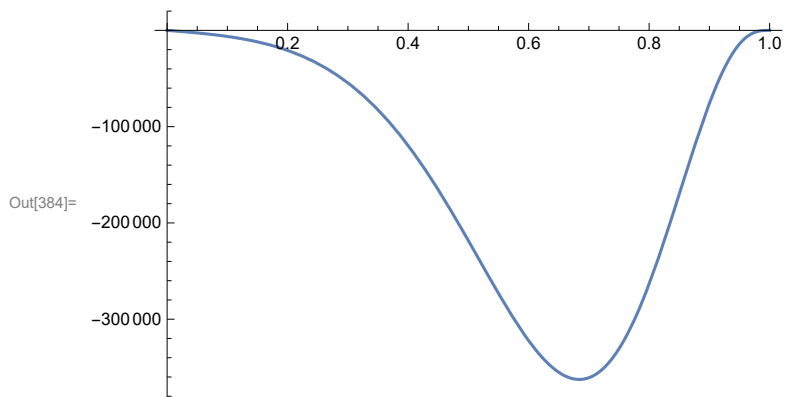

In[385]:= **Plot[Cf[12, 11, 10], {x, 0, 1}]**

[绘图](#)

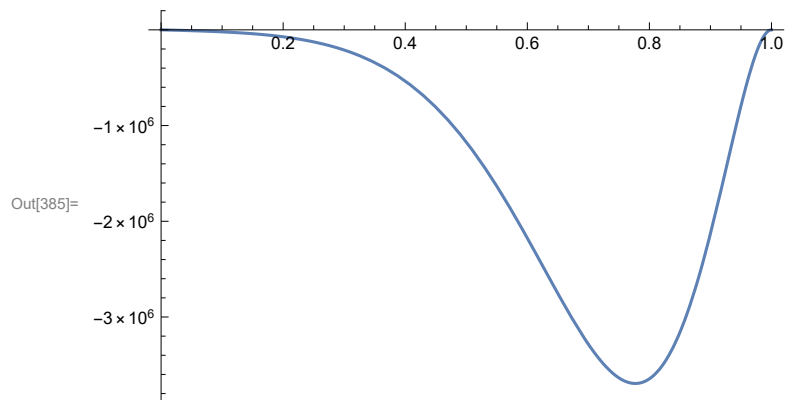

In[386]:= **Plot[Cf[12, 11, 9], {x, 0, 1}]**

[绘图](#)

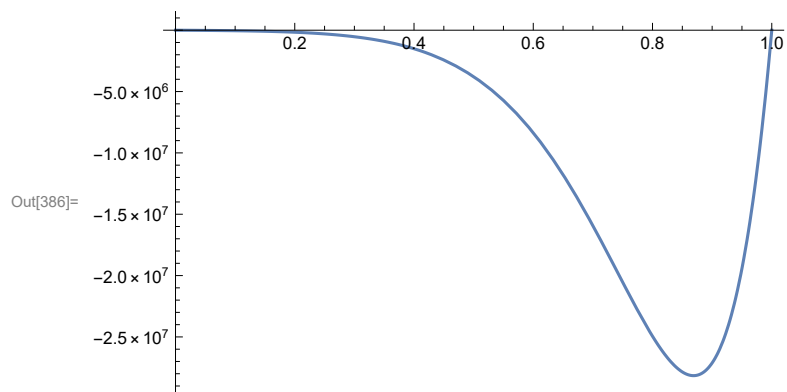

In[387]:= **Plot[Cf[12, 11, 8], {x, 0, 1}]**

[绘图](#)

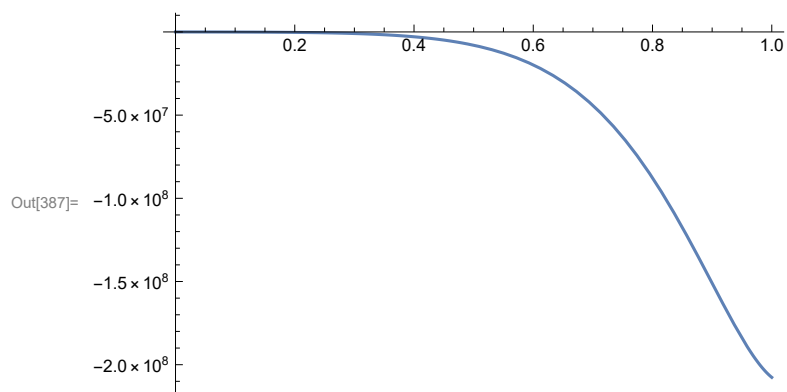



In[388]:= **Plot[Cf[12, 11, 7], {x, 0, 1}]**

[绘图](#)

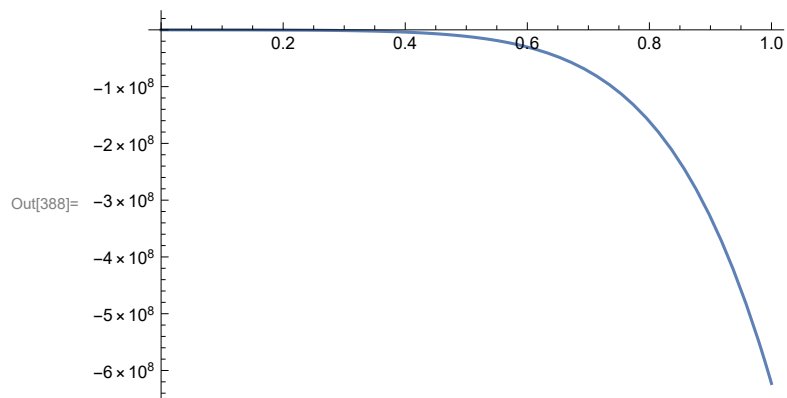

In[389]:= **Plot[Cf[12, 11, 6], {x, 0, 1}]**

[绘图](#)

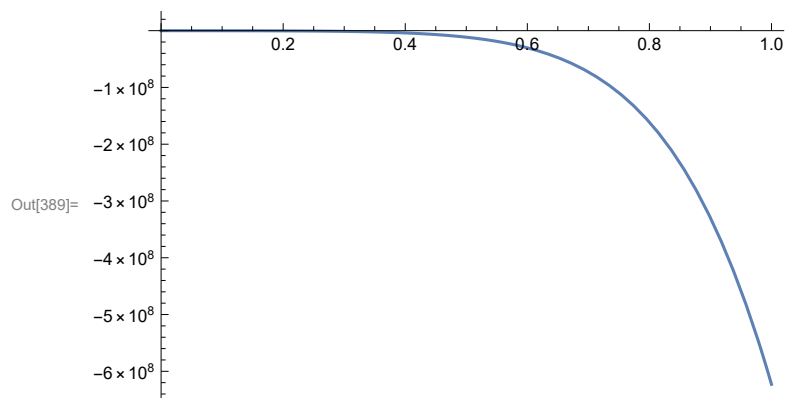

In[390]:= **Plot[Cf[12, 11, 5], {x, 0, 1}]**

[绘图](#)

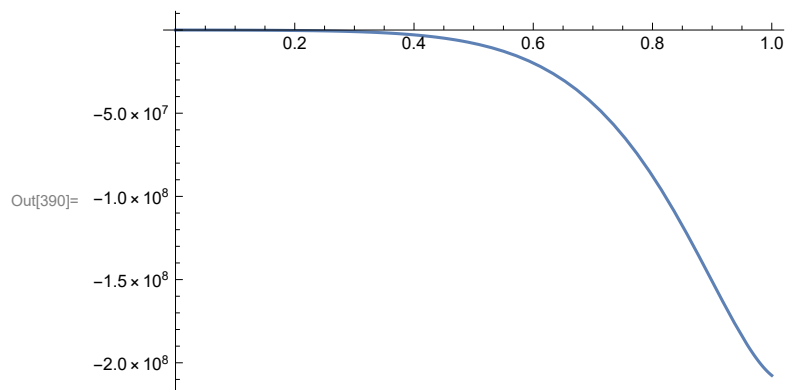

In[391]:= **Plot[Cf[12, 11, 4], {x, 0, 1}]**

[绘图](#)

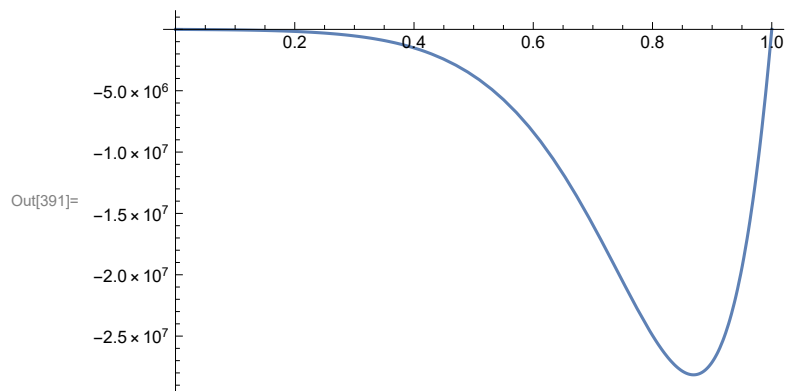

In[392]:= **Plot[Cf[12, 11, 3], {x, 0, 1}]**

[绘图](#)

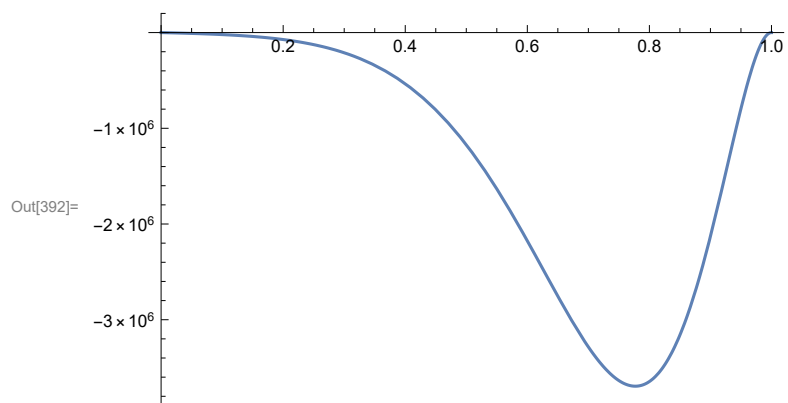

In[393]:= **Plot[Cf[12, 11, 2], {x, 0, 1}]**

[绘图](#)

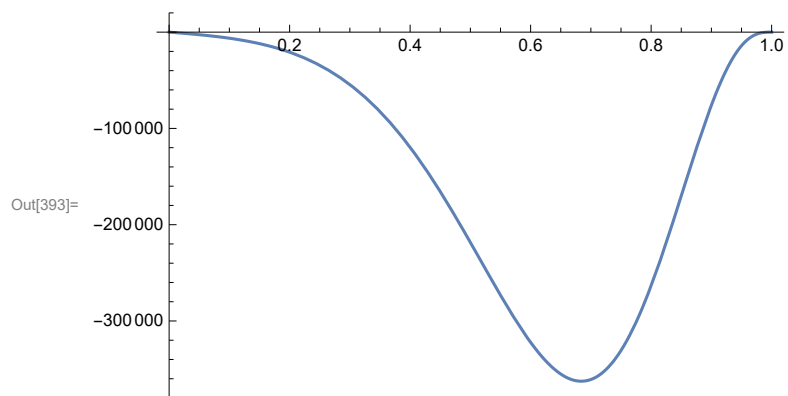

In[394]:= **Plot[Cf[12, 11, 1], {x, 0, 1}]**

[绘图](#)

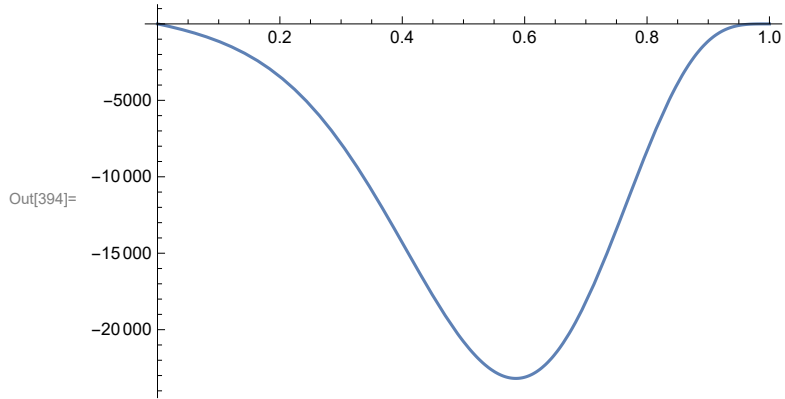

In[395]:= **Plot[Cf[12, 11, 0], {x, 0, 1}]**

[绘图](#)

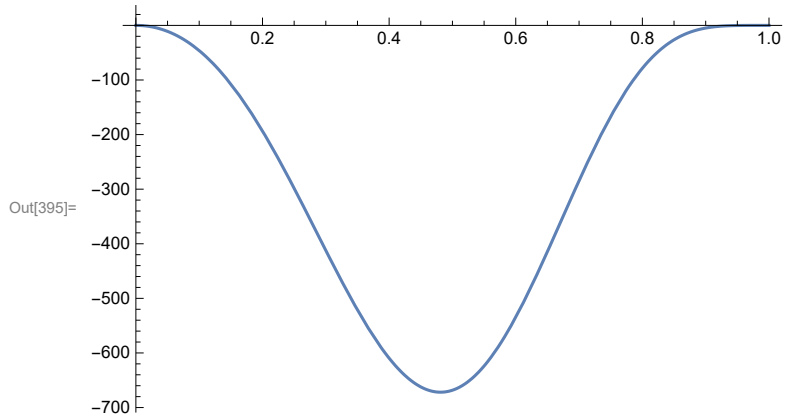

(\*35th group coefficients  $r^2 r^3$ \*)

In[396]:= **Plot[Cf[12, 10, 14], {x, 0, 1}]**

[绘图](#)

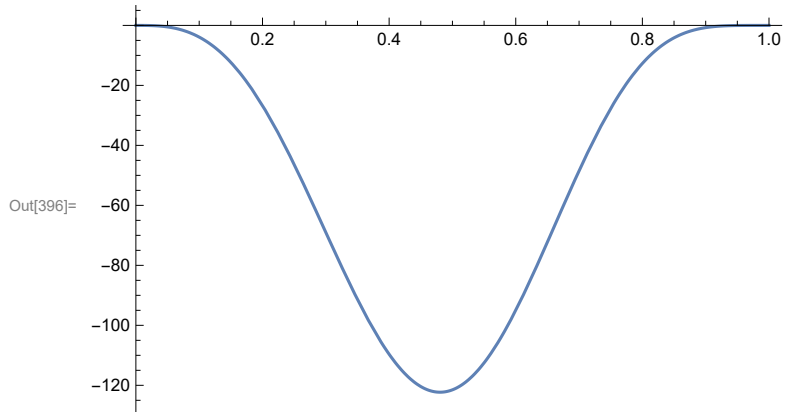

In[397]:= **Plot[Cf[12, 10, 13], {x, 0, 1}]**

[绘图](#)

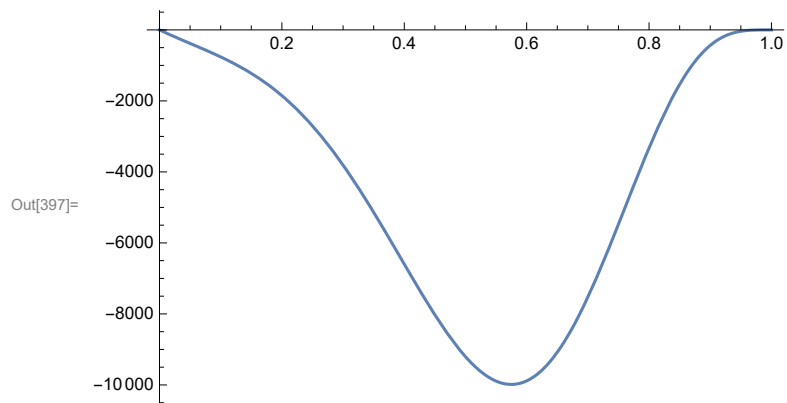

In[398]:= **Plot[Cf[12, 10, 12], {x, 0, 1}]**

[绘图](#)

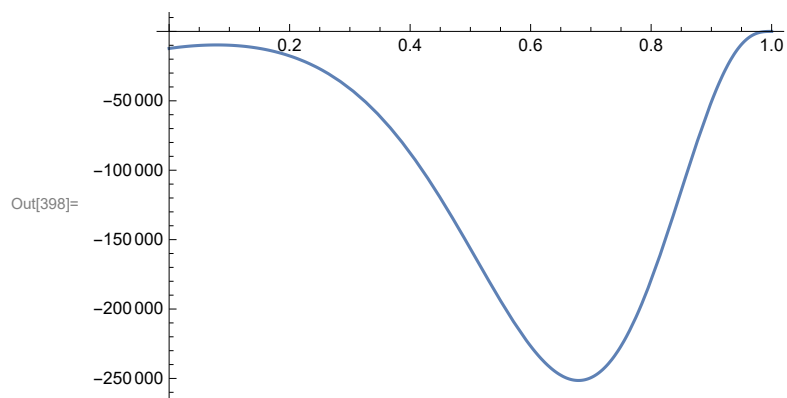

In[399]:= **Plot[Cf[12, 10, 11], {x, 0, 1}]**

[绘图](#)

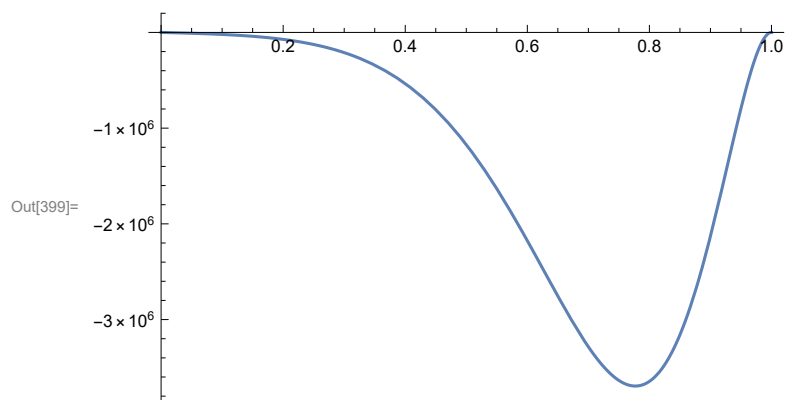

In[400]:= **Plot[Cf[12, 10, 10], {x, 0, 1}]**

[绘图](#)

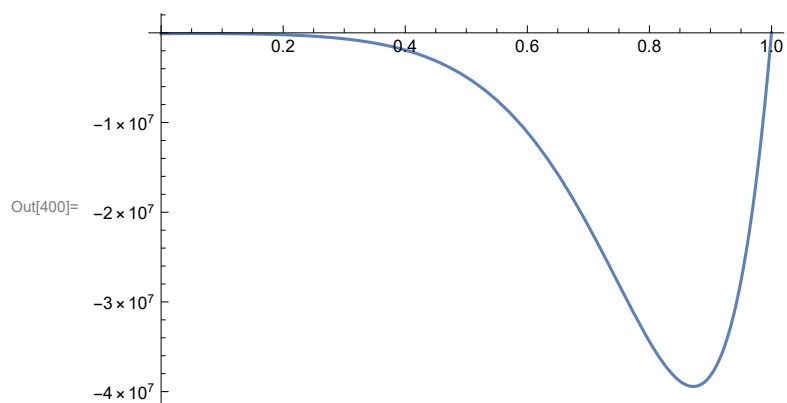

In[401]:= **Plot[Cf[12, 10, 9], {x, 0, 1}]**

[绘图](#)

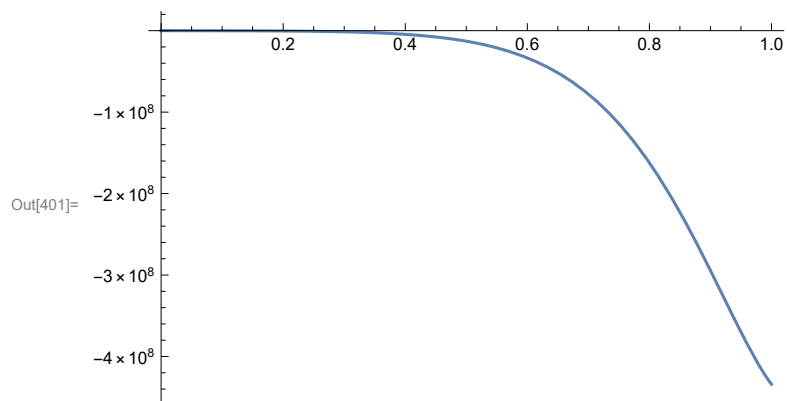

In[402]:= **Plot[Cf[12, 10, 8], {x, 0, 1}]**

[绘图](#)

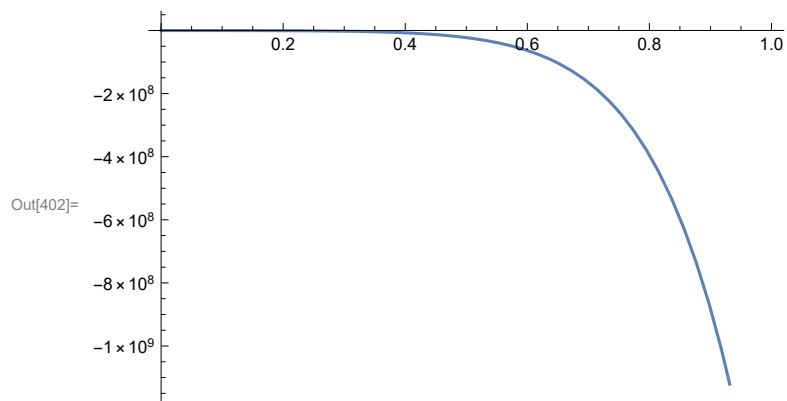

In[403]:= **Plot[Cf[12, 10, 7], {x, 0, 1}]**

[绘图](#)

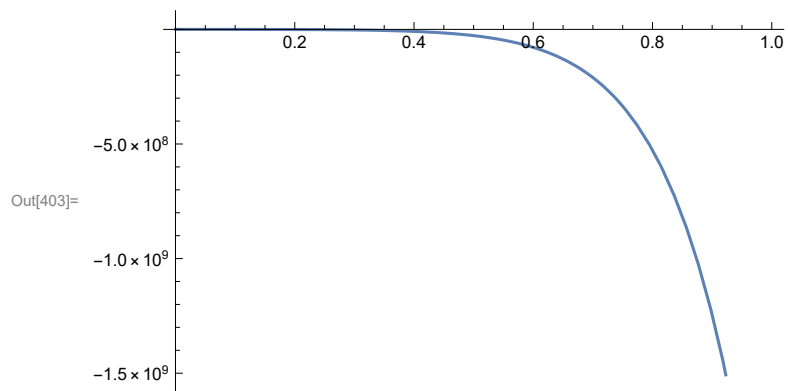

In[404]:= **Plot[Cf[12, 10, 6], {x, 0, 1}]**

[绘图](#)

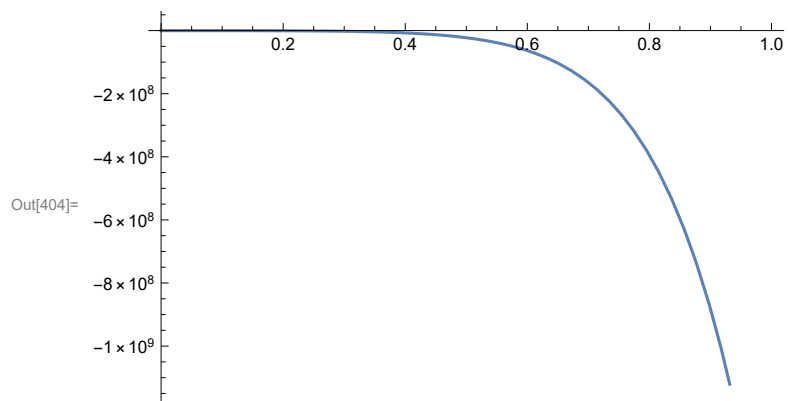

In[405]:= **Plot[Cf[12, 10, 5], {x, 0, 1}]**

[绘图](#)

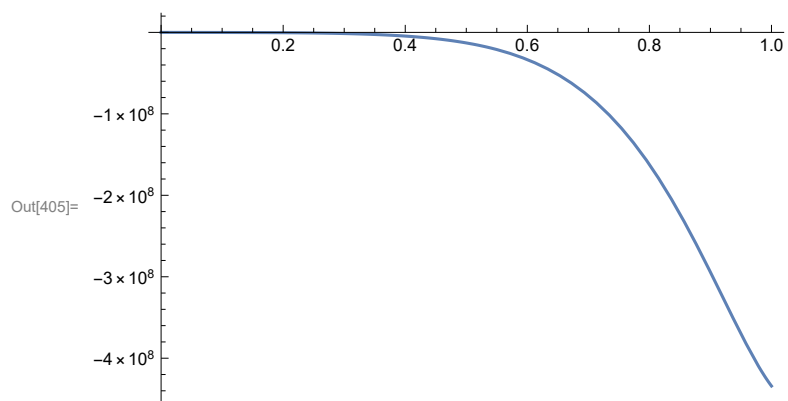

In[406]:= **Plot[Cf[12, 10, 4], {x, 0, 1}]**

[绘图](#)

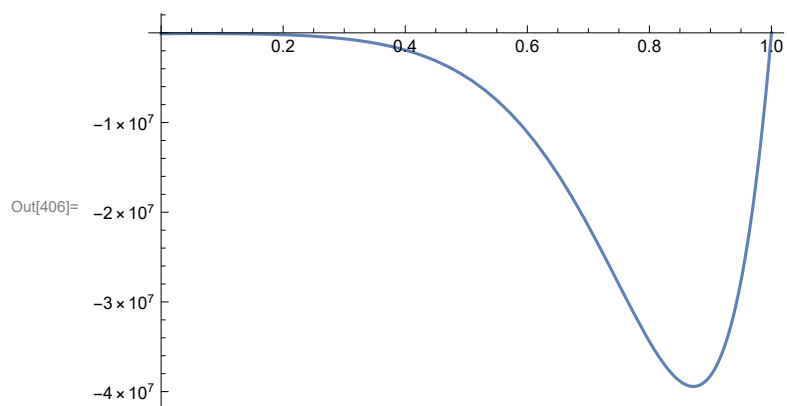

In[407]:= **Plot[Cf[12, 10, 3], {x, 0, 1}]**

[绘图](#)

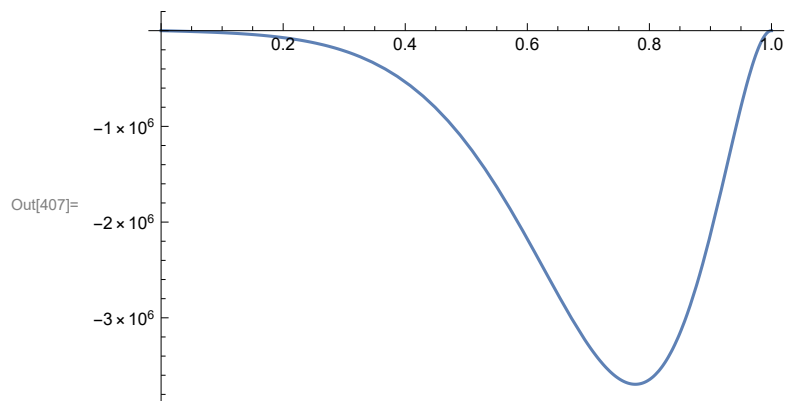

In[408]:= **Plot[Cf[12, 10, 2], {x, 0, 1}]**

[绘图](#)

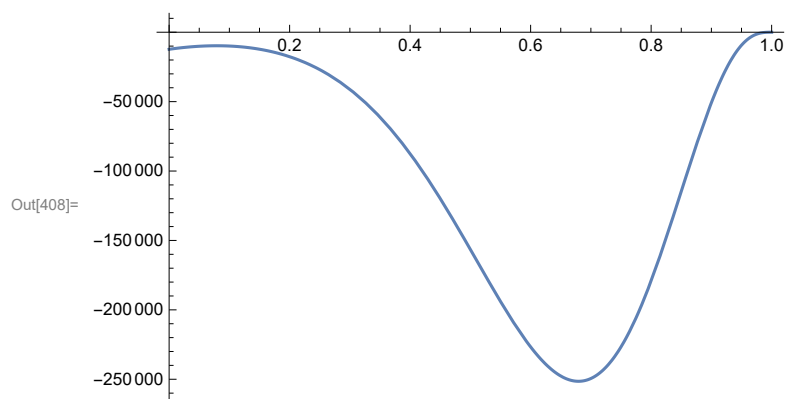

In[409]:= **Plot[Cf[12, 10, 1], {x, 0, 1}]**

[绘图](#)

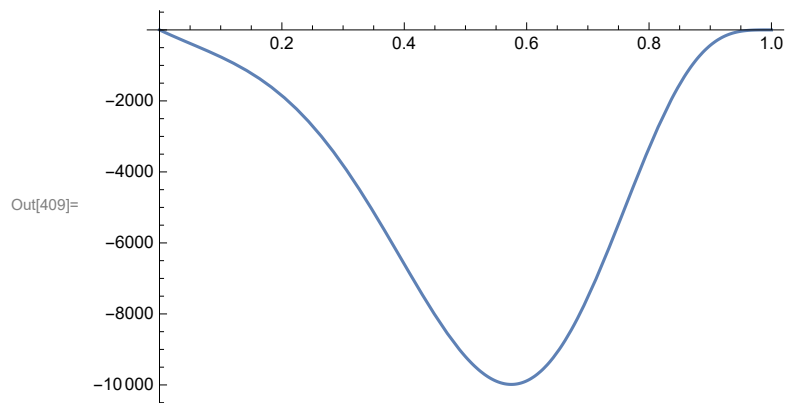

In[410]:= **Plot[Cf[12, 10, 0], {x, 0, 1}]**

[绘图](#)

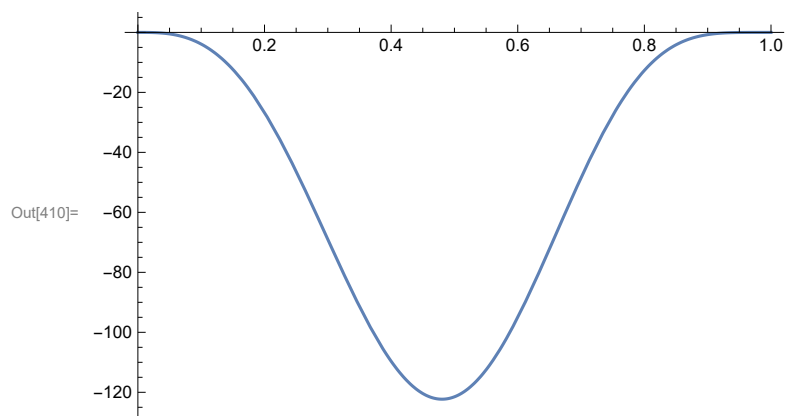

**(\*36th group coefficients r2^12r3^9\*)**

In[411]:= **Plot[Cf[12, 9, 14], {x, 0, 1}]**

[绘图](#)

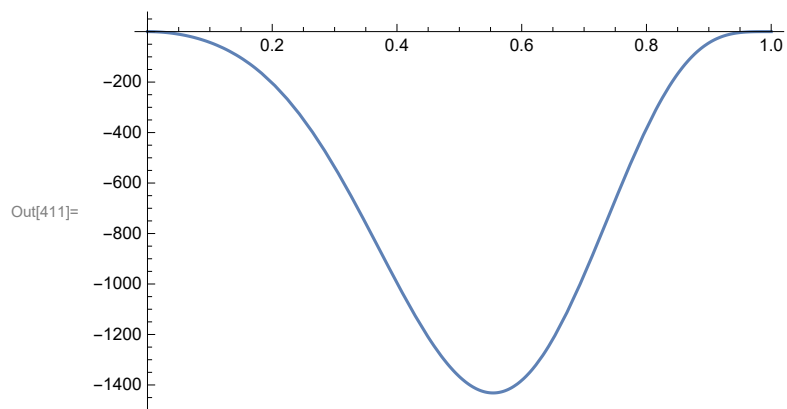



In[412]:= **Plot[Cf[12, 9, 13], {x, 0, 1}]**

[绘图](#)

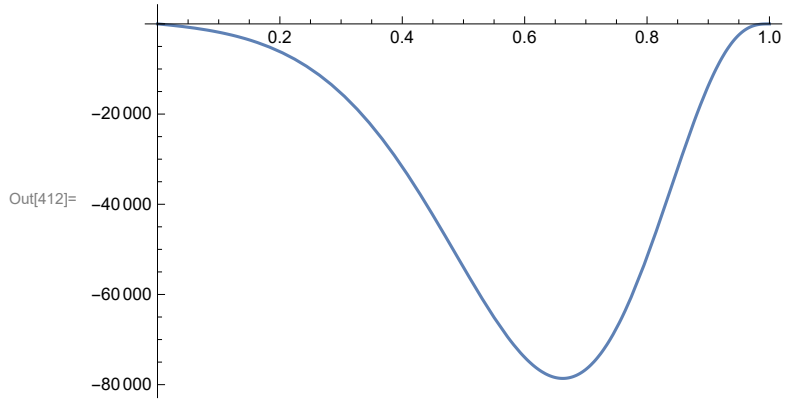

In[413]:= **Plot[Cf[12, 9, 12], {x, 0, 1}]**

[绘图](#)

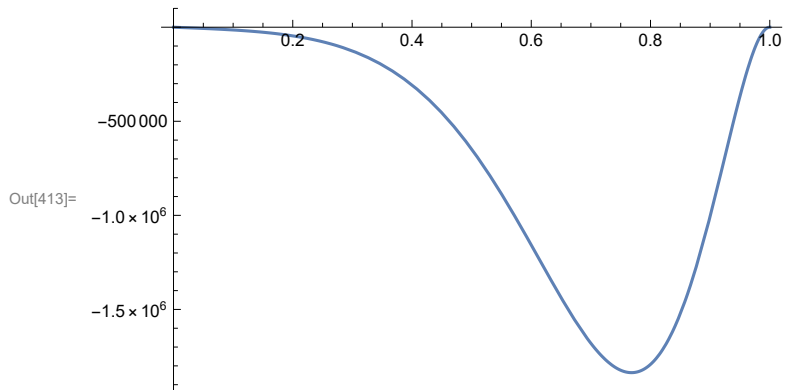

In[414]:= **Plot[Cf[12, 9, 11], {x, 0, 1}]**

[绘图](#)

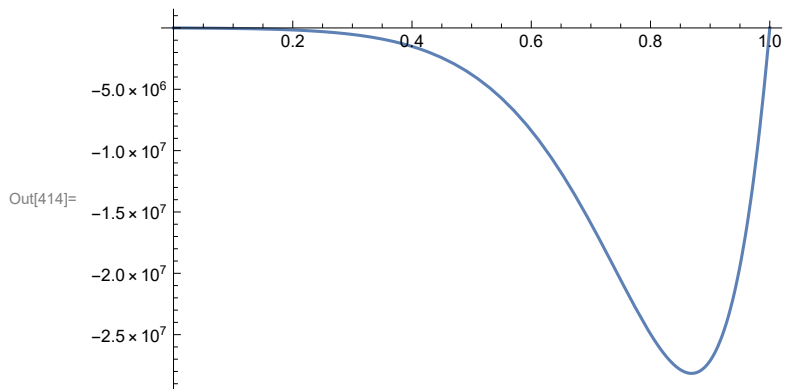

In[415]:= **Plot[Cf[12, 9, 10], {x, 0, 1}]**

[绘图](#)

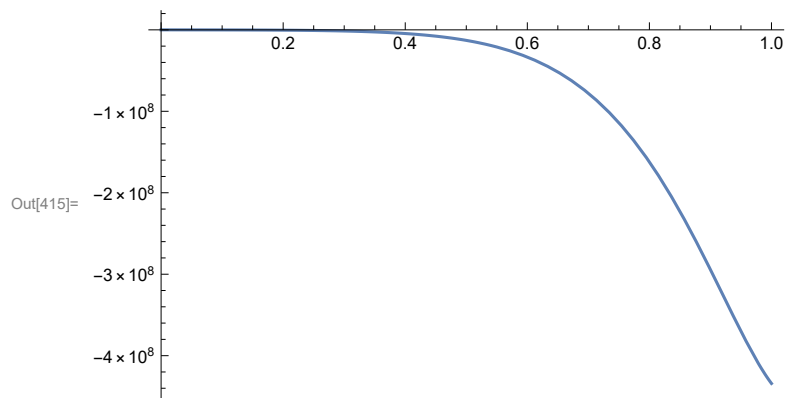

In[416]:= **Plot[Cf[12, 9, 9], {x, 0, 1}]**

[绘图](#)

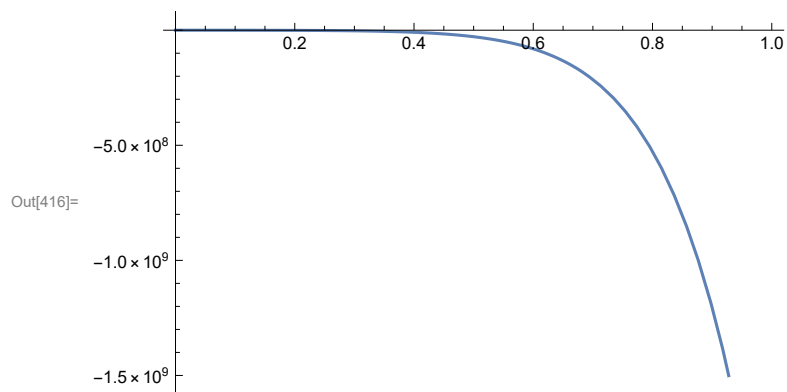

In[417]:= **Plot[Cf[12, 9, 8], {x, 0, 1}]**

[绘图](#)

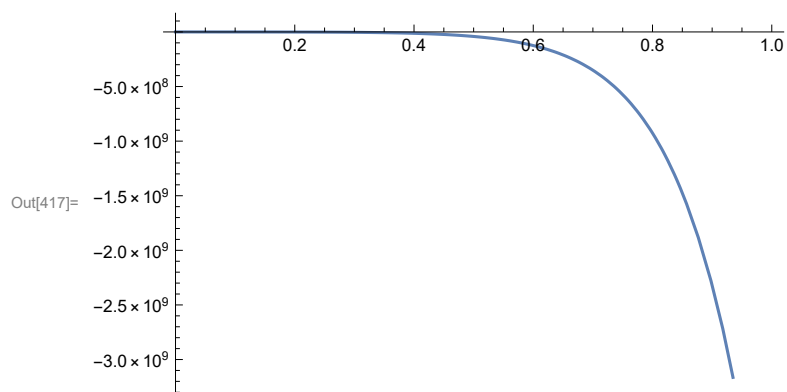

In[418]:= **Plot[Cf[12, 9, 7], {x, 0, 1}]**

[绘图](#)

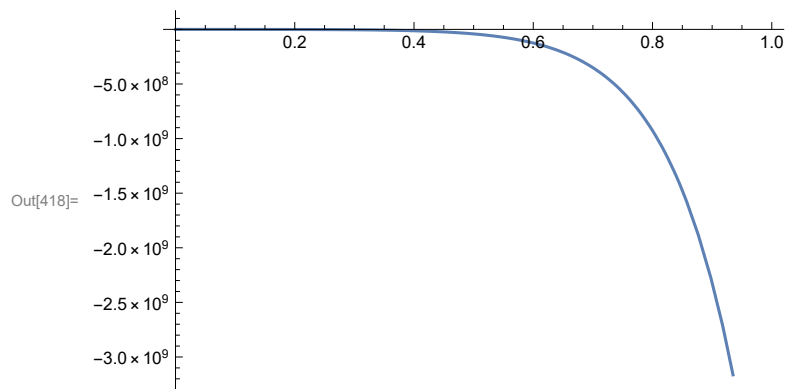

In[419]:= **Plot[Cf[12, 9, 6], {x, 0, 1}]**

[绘图](#)

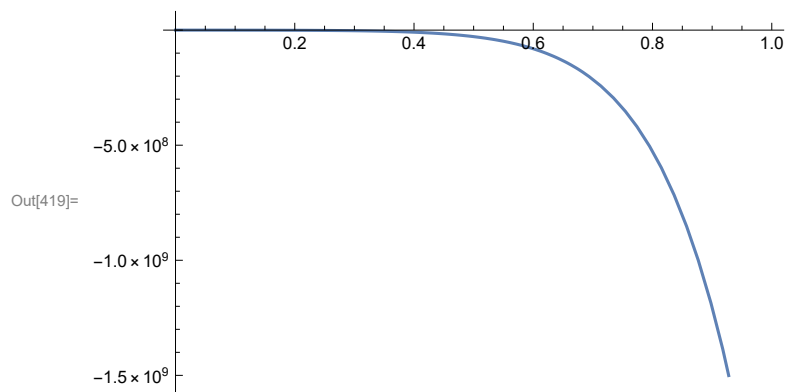

In[420]:= **Plot[Cf[12, 9, 5], {x, 0, 1}]**

[绘图](#)

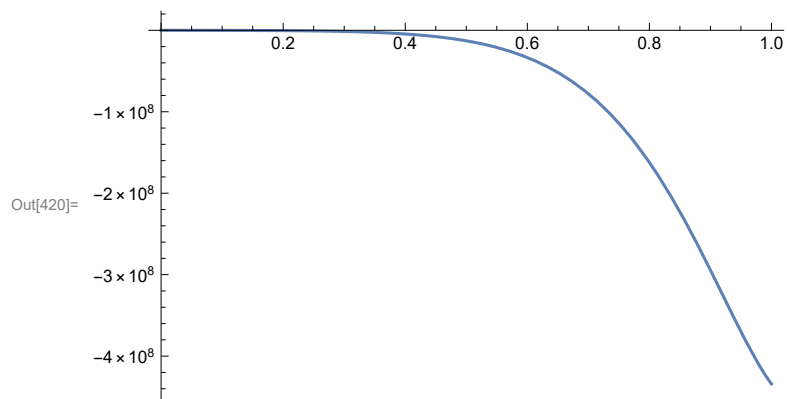

In[421]:= **Plot**[**Cf**[12, 9, 4], {x, 0, 1}]

[绘图](#)

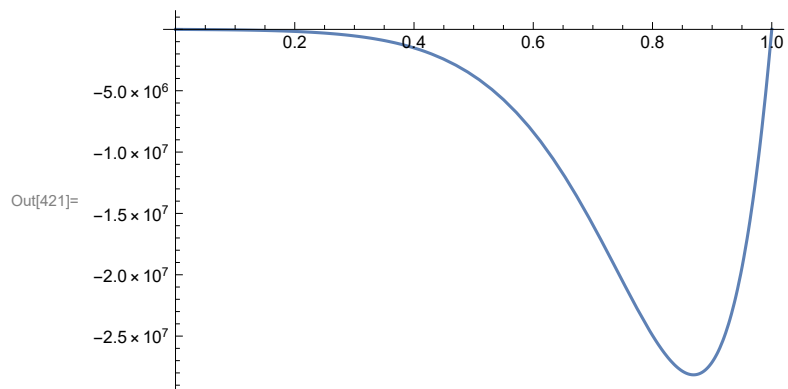

In[422]:= **Plot**[**Cf**[12, 9, 3], {x, 0, 1}]

[绘图](#)

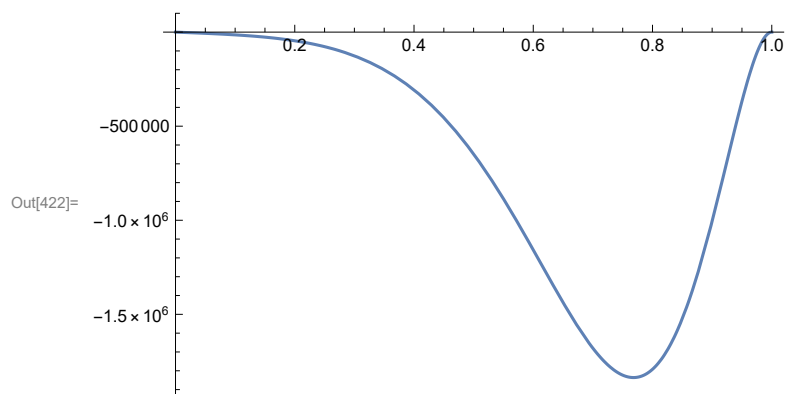

In[423]:= **Plot**[**Cf**[12, 9, 2], {x, 0, 1}]

[绘图](#)

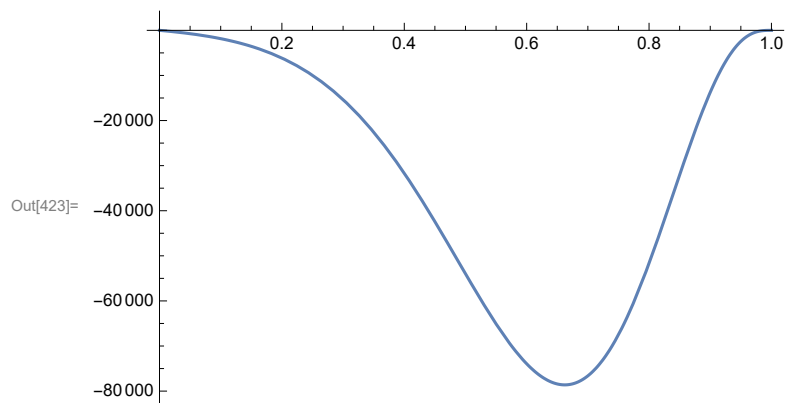

In[424]:= **Plot[Cf[12, 9, 1], {x, 0, 1}]**

[绘图](#)

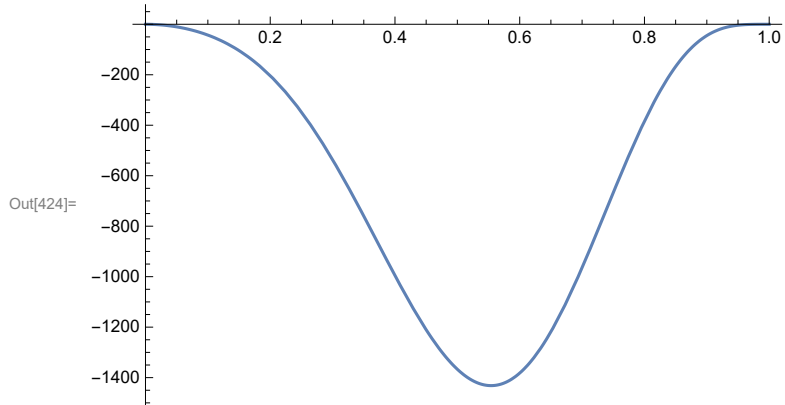

**Plot[Cf[12, 9, 0], {x, 0, 1}]**

[绘图](#)

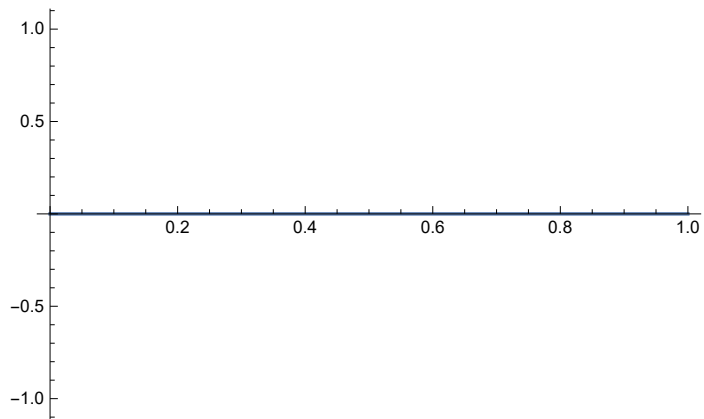

(\*37th group coefficients r2^12r3^8\*)

In[425]:= **Plot[Cf[12, 8, 14], {x, 0, 1}]**

[绘图](#)

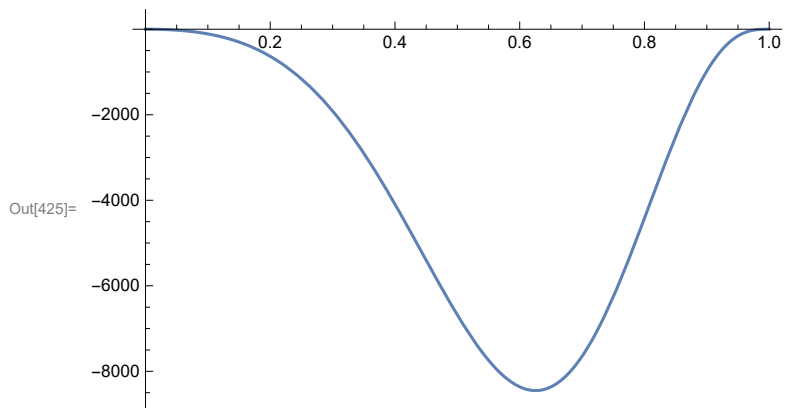

In[426]:= **Plot[Cf[12, 8, 13], {x, 0, 1}]**

[绘图](#)

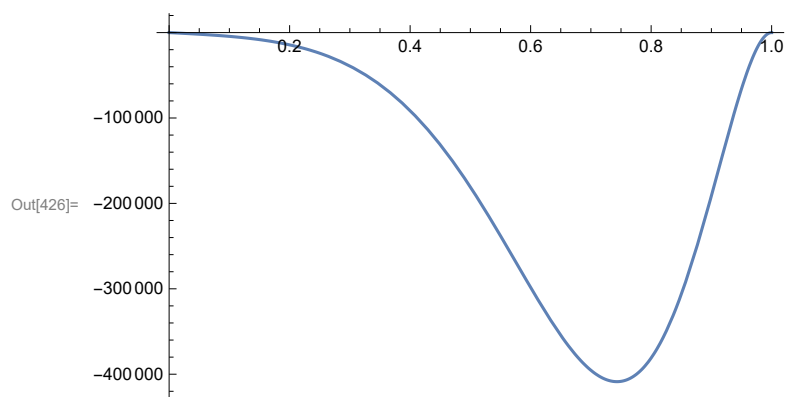

In[427]:= **Plot[Cf[12, 8, 12], {x, 0, 1}]**

[绘图](#)

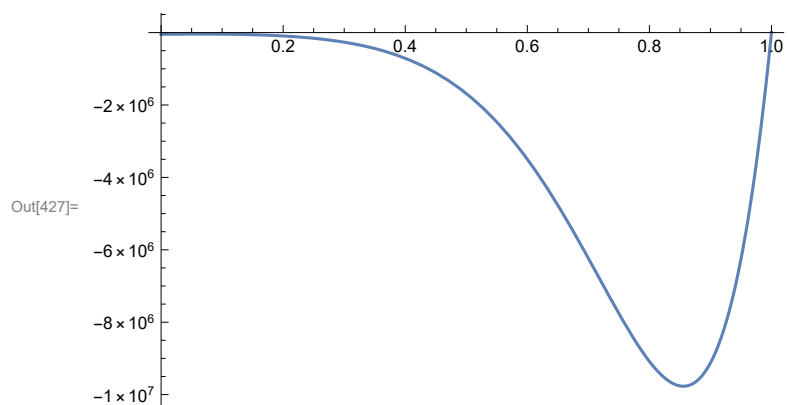

In[428]:= **Plot[Cf[12, 8, 11], {x, 0, 1}]**

[绘图](#)

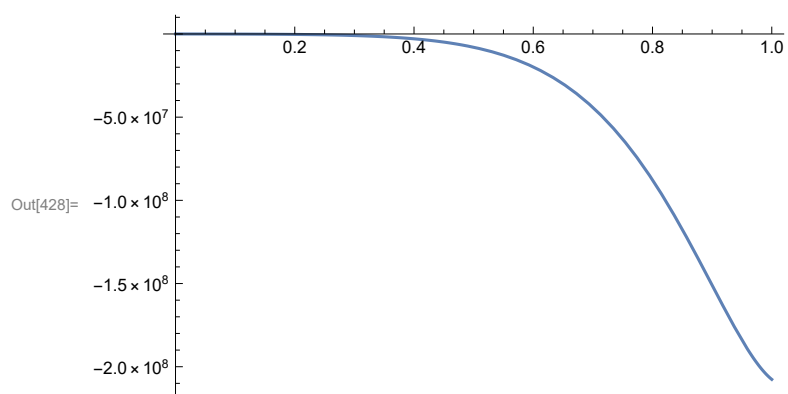

In[429]:= **Plot[Cf[12, 8, 10], {x, 0, 1}]**

[绘图](#)

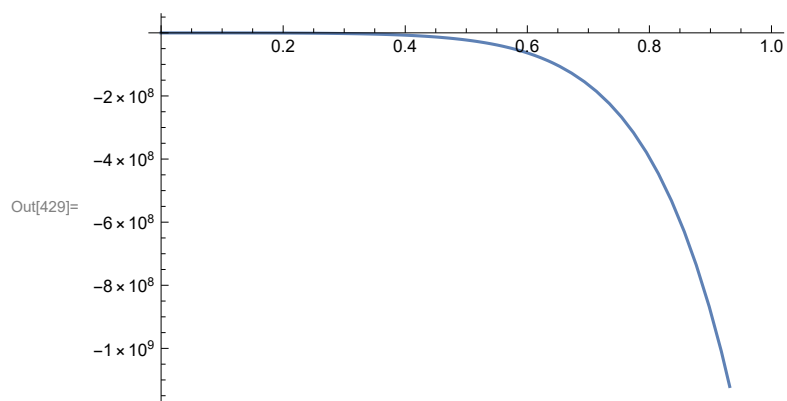

In[430]:= **Plot[Cf[12, 8, 9], {x, 0, 1}]**

[绘图](#)

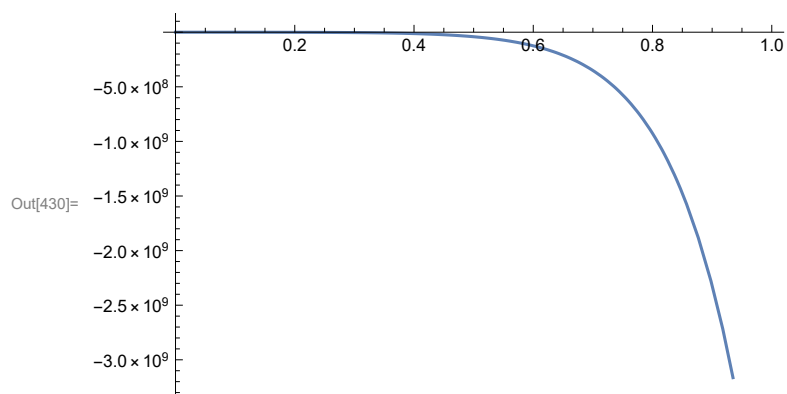

In[431]:= **Plot[Cf[12, 8, 8], {x, 0, 1}]**

[绘图](#)

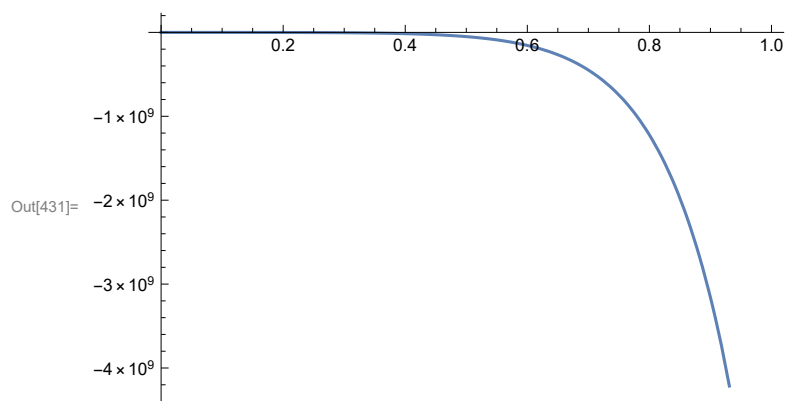

In[432]:= **Plot[Cf[12, 8, 7], {x, 0, 1}]**

[绘图](#)

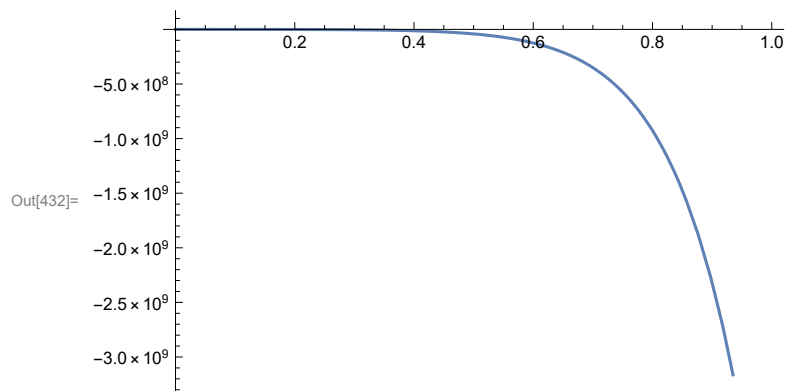

In[433]:= **Plot[Cf[12, 8, 6], {x, 0, 1}]**

[绘图](#)

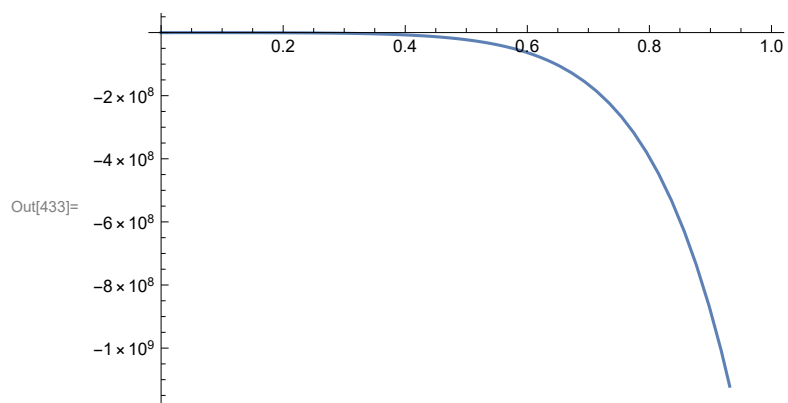

In[434]:= **Plot[Cf[12, 8, 5], {x, 0, 1}]**

[绘图](#)

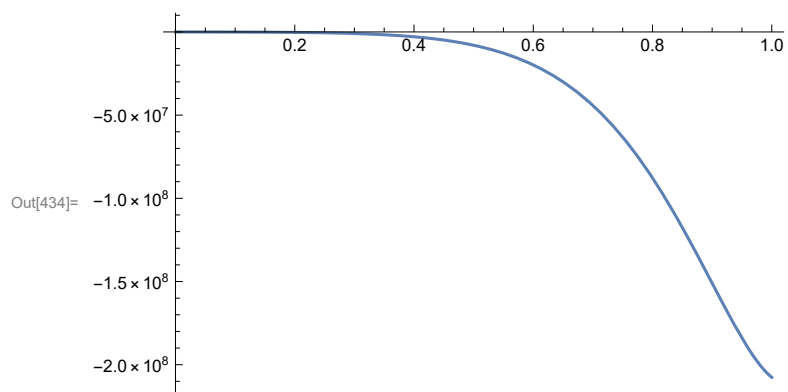



In[435]:= **Plot[Cf[12, 8, 4], {x, 0, 1}]**

[绘图](#)

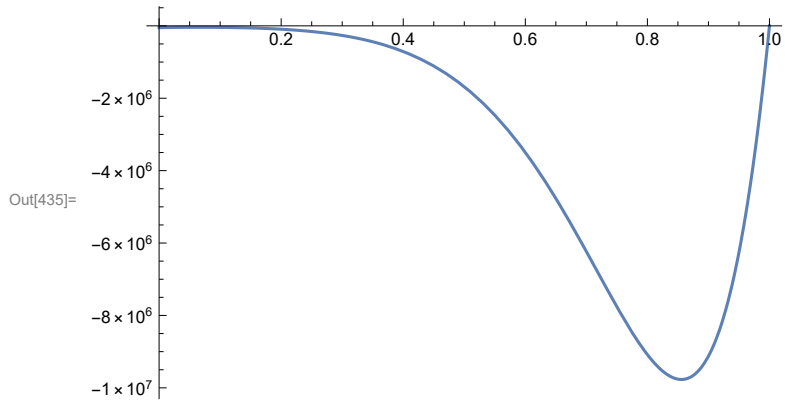

In[436]:= **Plot[Cf[12, 8, 3], {x, 0, 1}]**

[绘图](#)

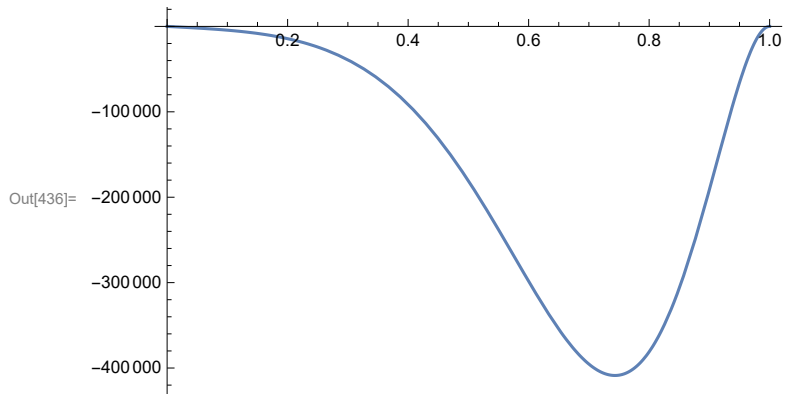

In[437]:= **Plot[Cf[12, 8, 2], {x, 0, 1}]**

[绘图](#)

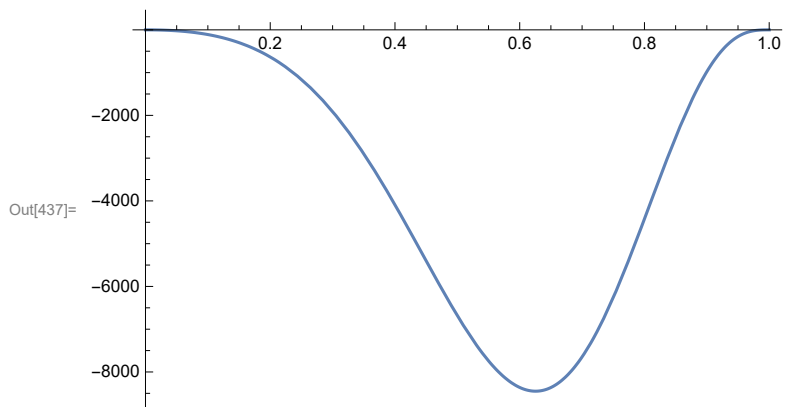

**Plot[Cf[12, 8, 1], {x, 0, 1}]**

[绘图](#)

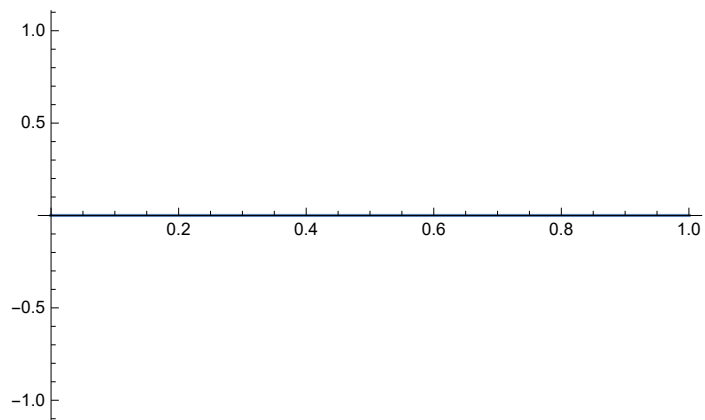

**Plot[Cf[12, 8, 0], {x, 0, 1}]**

[绘图](#)

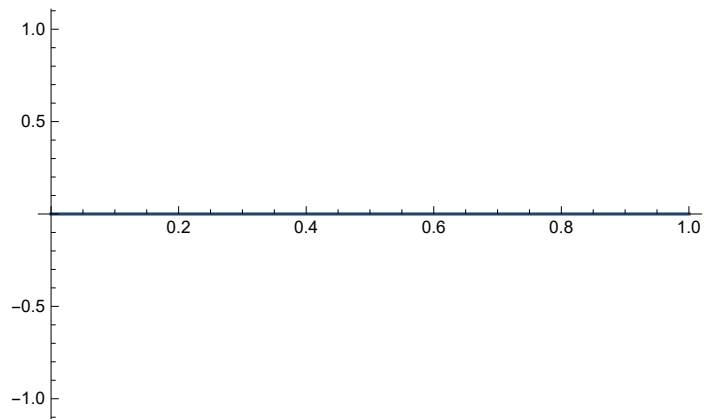

**(\*38th group coefficients r2^12r3^7\*)**

In[438]:= **Plot[Cf[12, 7, 14], {x, 0, 1}]**

[绘图](#)

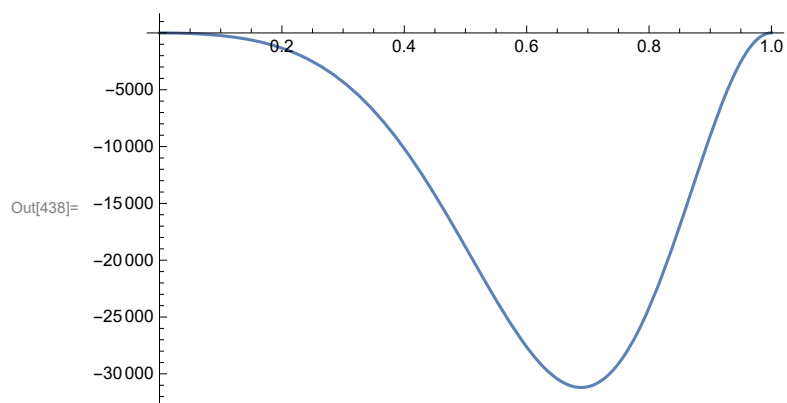

In[439]:= **Plot[Cf[12, 7, 13], {x, 0, 1}]**

[绘图](#)

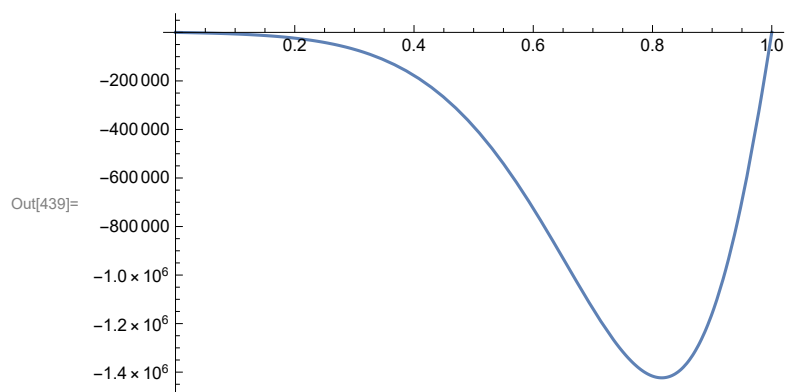

In[440]:= **Plot[Cf[12, 7, 12], {x, 0, 1}]**

[绘图](#)

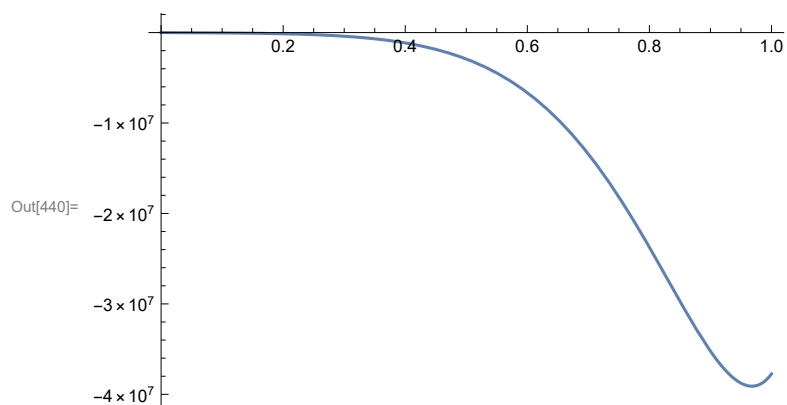

In[441]:= **Plot[Cf[12, 7, 11], {x, 0, 1}]**

[绘图](#)

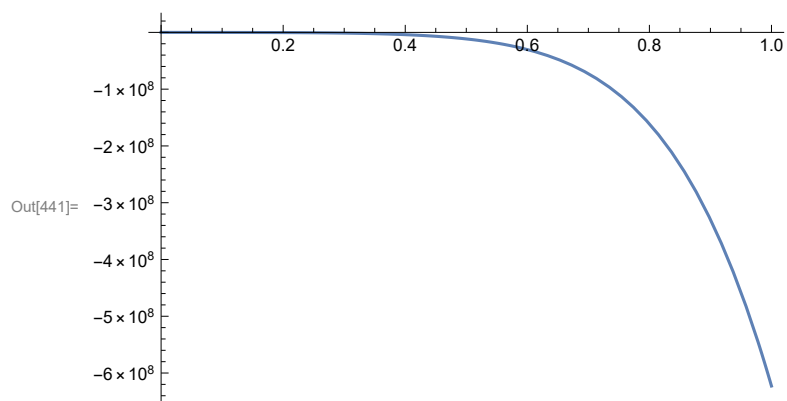

In[442]:= **Plot[Cf[12, 7, 10], {x, 0, 1}]**

[绘图](#)

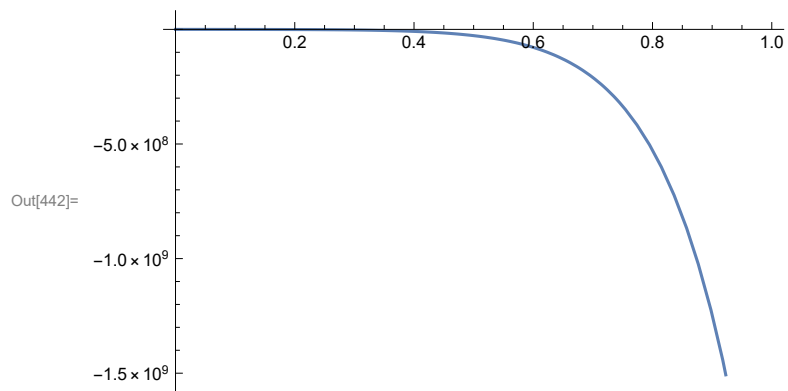

In[443]:= **Plot[Cf[12, 7, 9], {x, 0, 1}]**

[绘图](#)

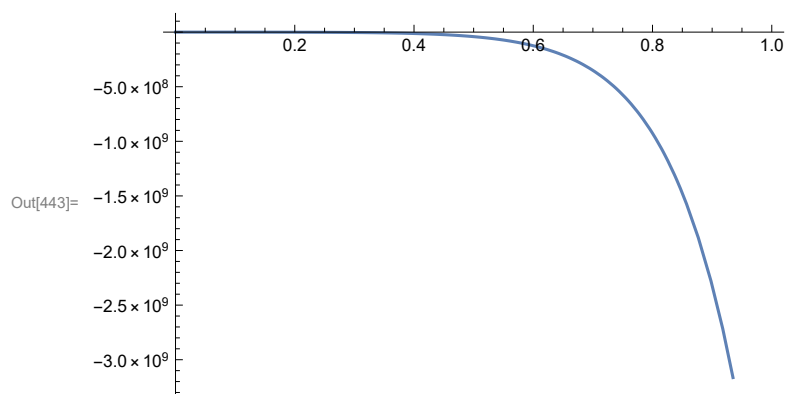

In[444]:= **Plot[Cf[12, 7, 8], {x, 0, 1}]**

[绘图](#)

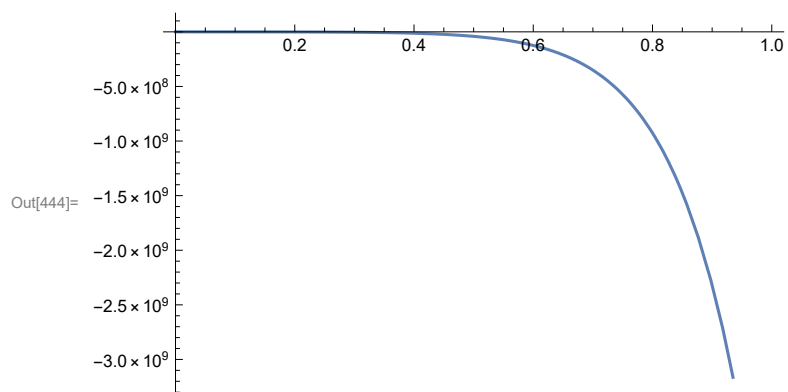

In[445]:= **Plot[Cf[12, 7, 7], {x, 0, 1}]**

[绘图](#)

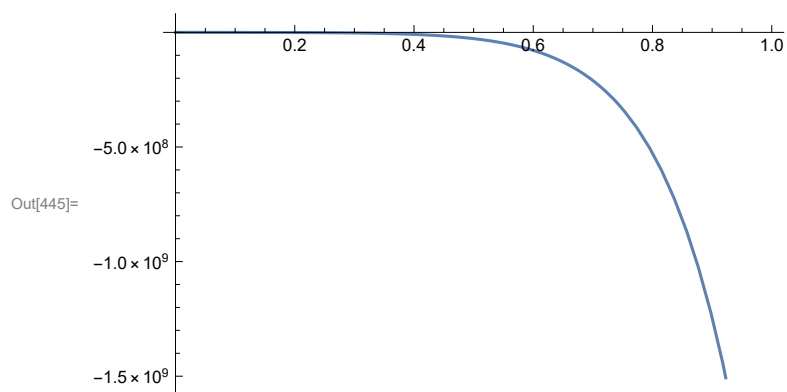

In[446]:= **Plot[Cf[12, 7, 6], {x, 0, 1}]**

[绘图](#)

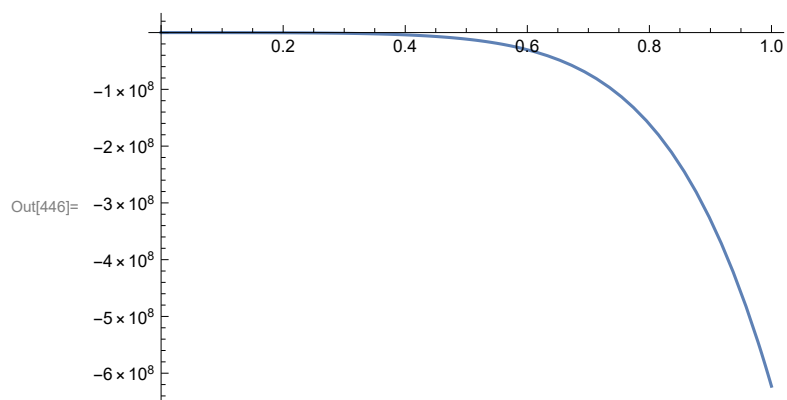

In[447]:= **Plot[Cf[12, 7, 5], {x, 0, 1}]**

[绘图](#)

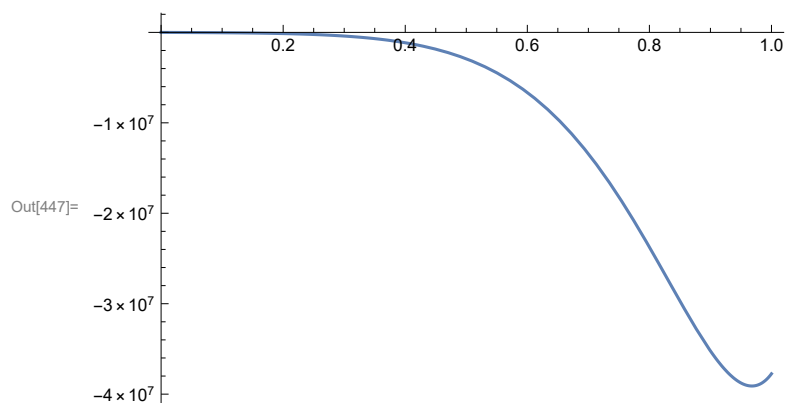

In[448]:= **Plot[Cf[12, 7, 4], {x, 0, 1}]**

[绘图](#)

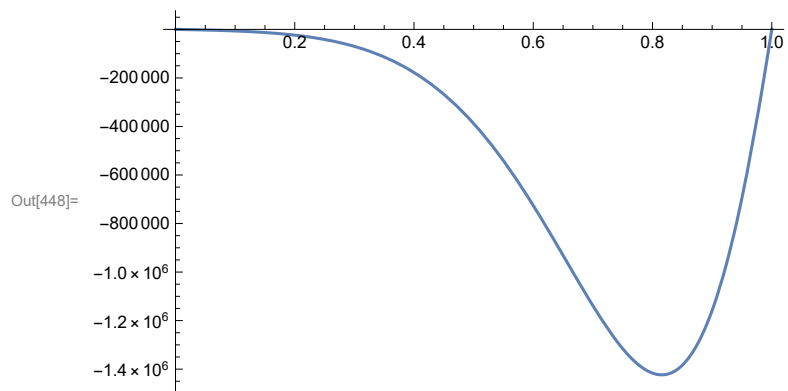

In[449]:= **Plot[Cf[12, 7, 3], {x, 0, 1}]**

[绘图](#)

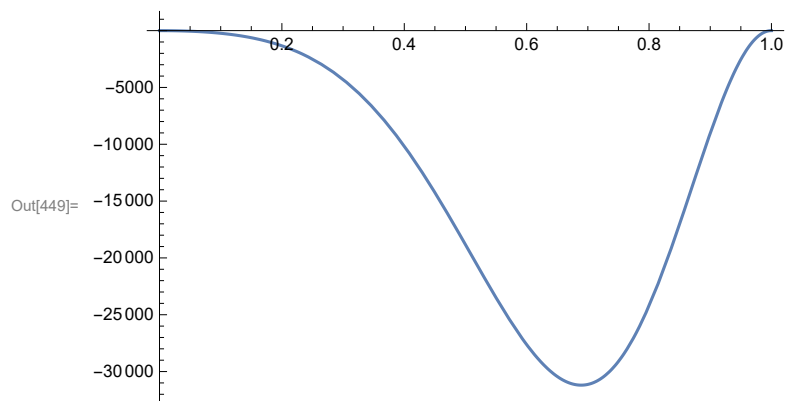

In[450]:= **Plot[Cf[12, 7, 2], {x, 0, 1}]**

[绘图](#)

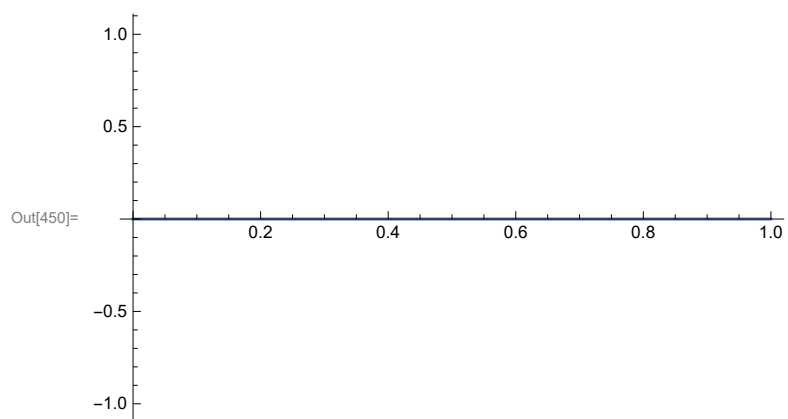

**Plot[Cf[12, 7, 1], {x, 0, 1}]**

[绘图](#)

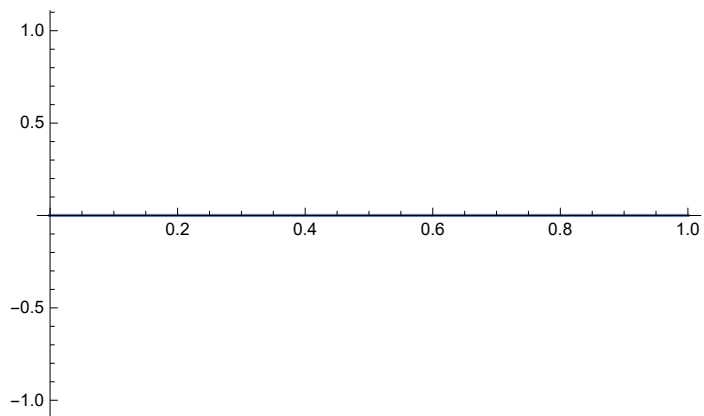

**Plot[Cf[12, 7, 0], {x, 0, 1}]**

[绘图](#)

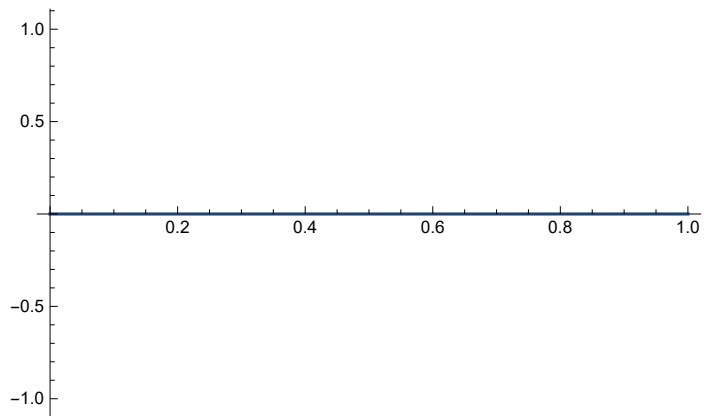

**(\*39th group coefficients r2^12r3^6\*)**

In[451]:= **Plot[Cf[12, 6, 14], {x, 0, 1}]**

[绘图](#)

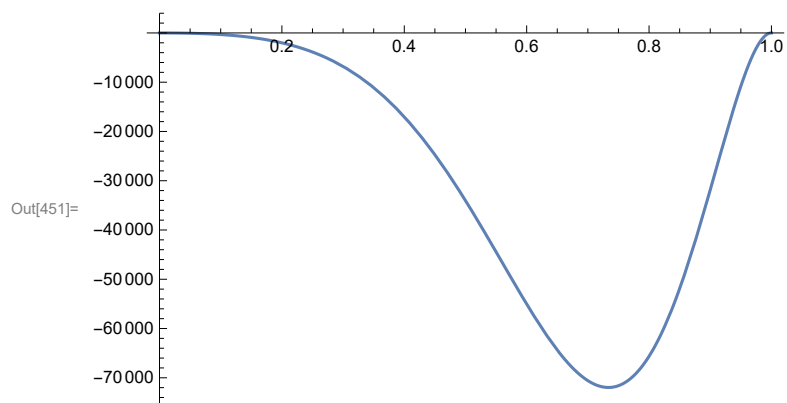

In[452]:= **Plot[Cf[12, 6, 13], {x, 0, 1}]**

[绘图](#)

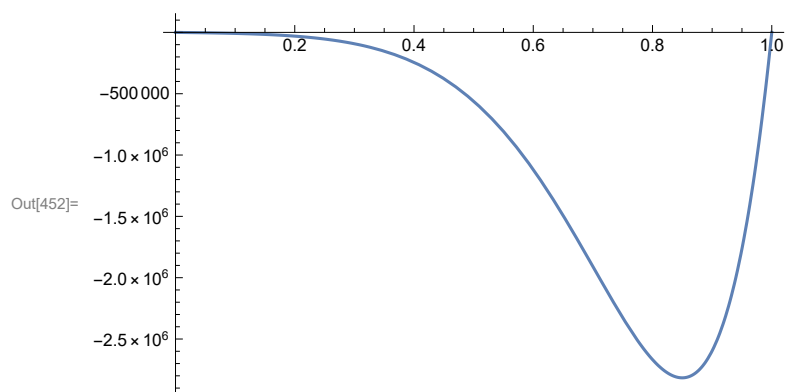

In[453]:= **Plot[Cf[12, 6, 12], {x, 0, 1}]**

[绘图](#)

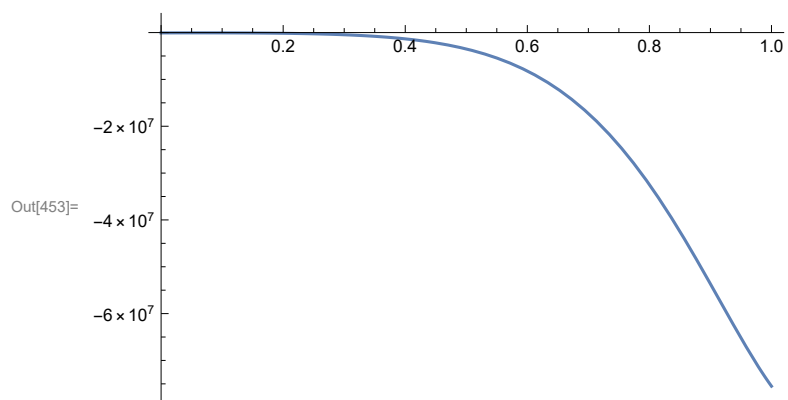

In[454]:= **Plot[Cf[12, 6, 11], {x, 0, 1}]**

[绘图](#)

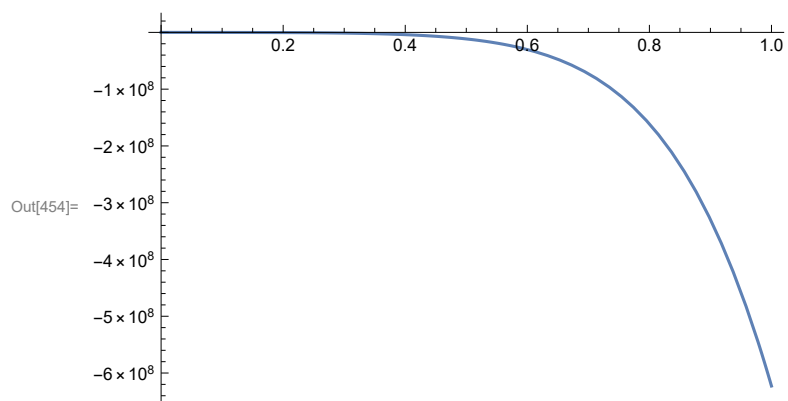



In[455]:= **Plot[Cf[12, 6, 10], {x, 0, 1}]**

[绘图](#)

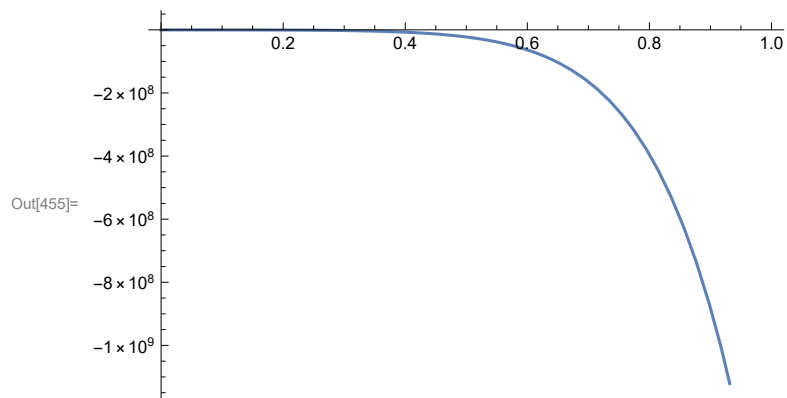

In[456]:= **Plot[Cf[12, 6, 9], {x, 0, 1}]**

[绘图](#)

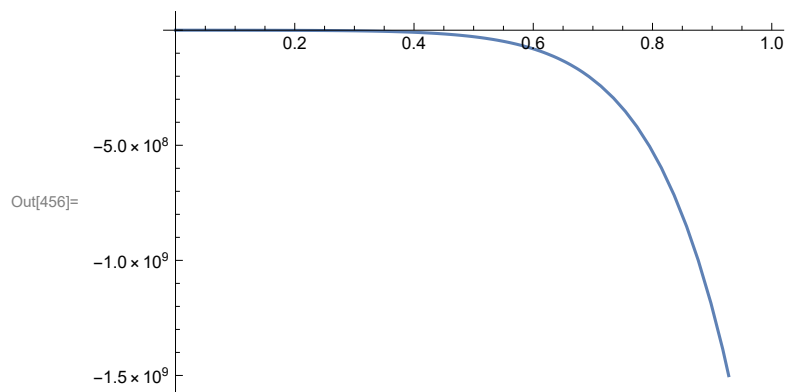

In[457]:= **Plot[Cf[12, 6, 8], {x, 0, 1}]**

[绘图](#)

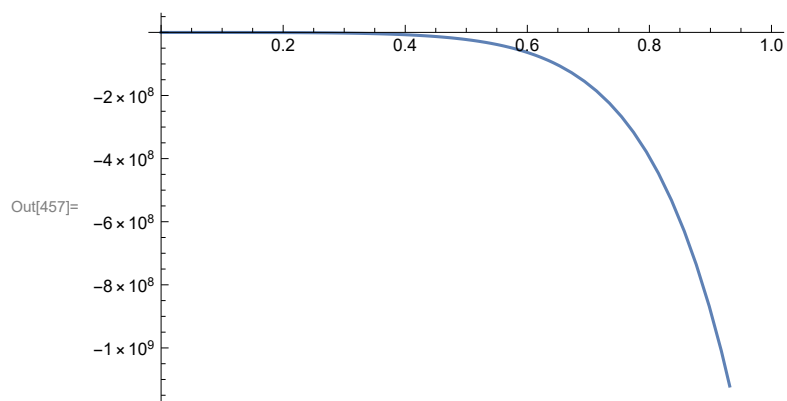

In[458]:= **Plot[Cf[12, 6, 7], {x, 0, 1}]**

[绘图](#)

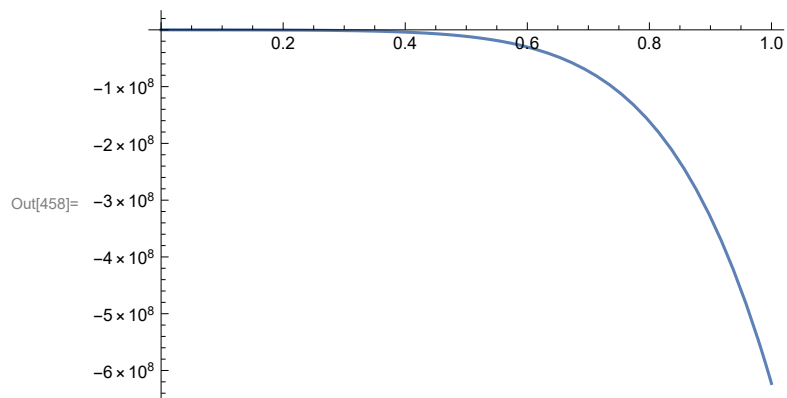

In[459]:= **Plot[Cf[12, 6, 6], {x, 0, 1}]**

[绘图](#)

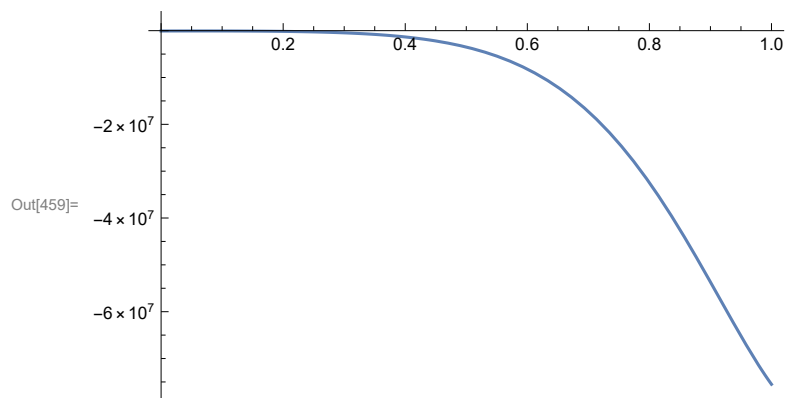

In[460]:= **Plot[Cf[12, 6, 5], {x, 0, 1}]**

[绘图](#)

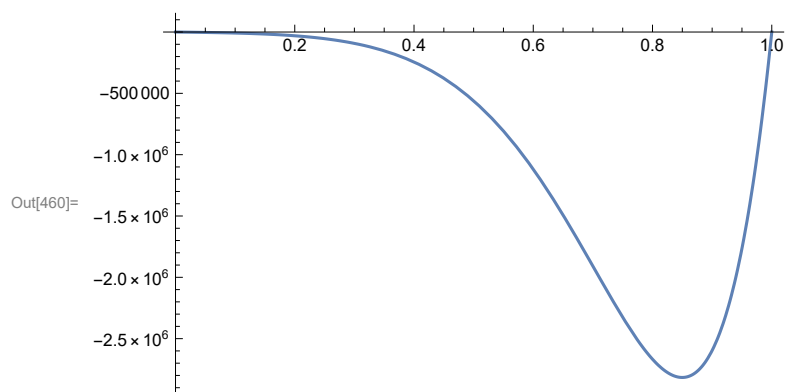

In[461]:= **Plot[Cf[12, 6, 4], {x, 0, 1}]**

[绘图](#)

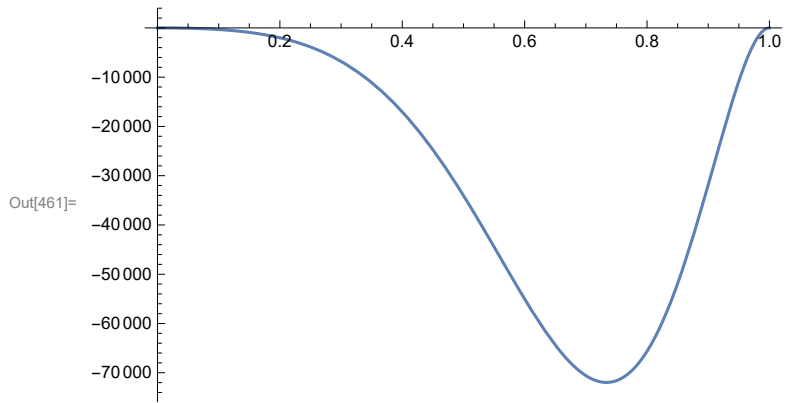

**Plot[Cf[12, 6, 3], {x, 0, 1}]**

[绘图](#)

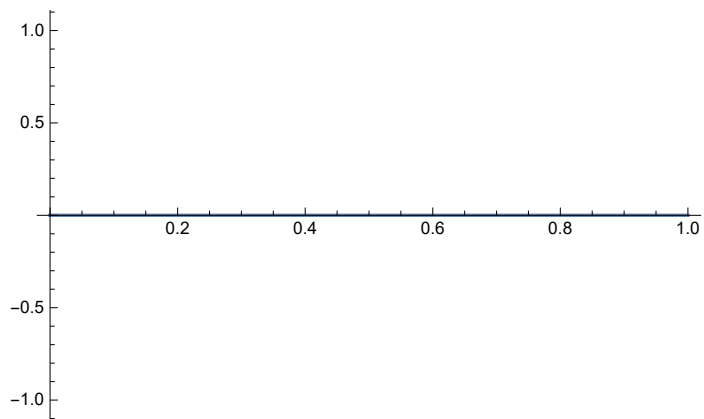

**Plot[Cf[12, 6, 2], {x, 0, 1}]**

[绘图](#)

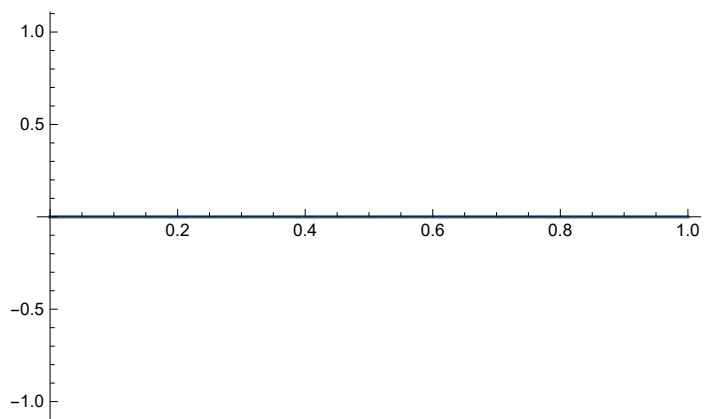

**Plot[Cf[12, 6, 1], {x, 0, 1}]**

[绘图](#)

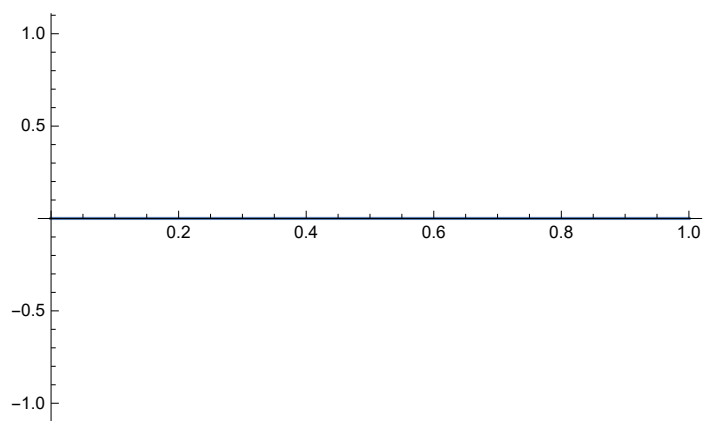

**Plot[Cf[12, 6, 0], {x, 0, 1}]**

[绘图](#)

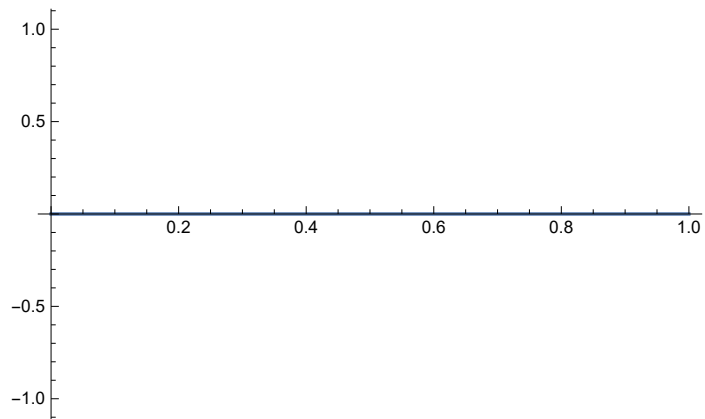

**(\*40th group coefficients r2^12r3^5\*)**

In[462]:= **Plot[Cf[12, 5, 14], {x, 0, 1}]**

[绘图](#)

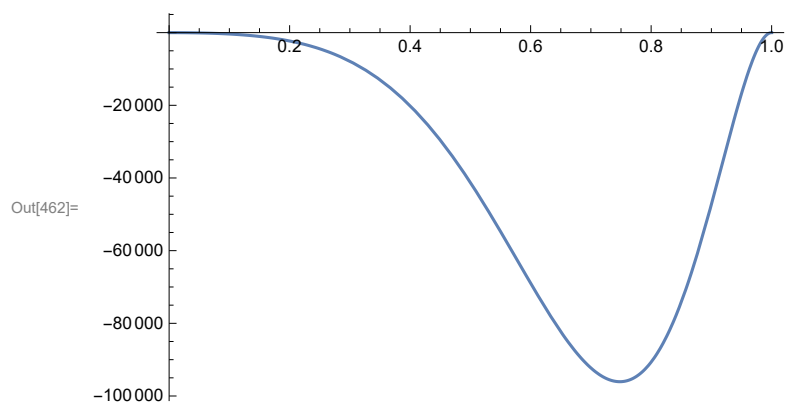

In[463]:= **Plot[Cf[12, 5, 13], {x, 0, 1}]**

[绘图](#)

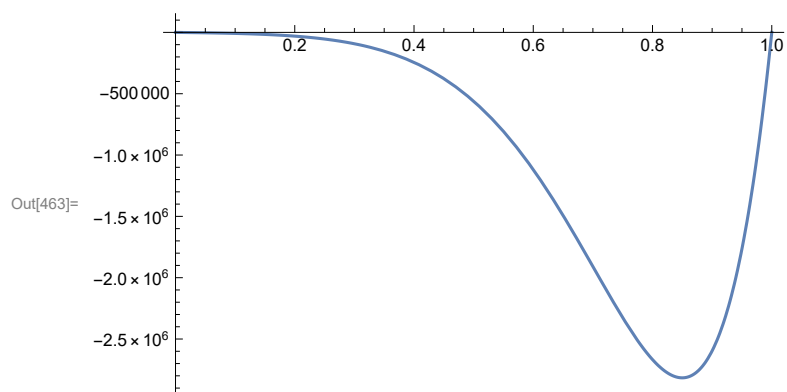

In[464]:= **Plot[Cf[12, 5, 12], {x, 0, 1}]**

[绘图](#)

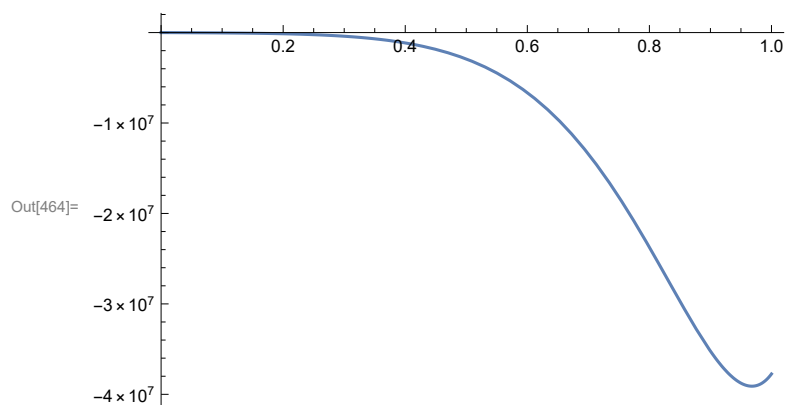

In[465]:= **Plot[Cf[12, 5, 11], {x, 0, 1}]**

[绘图](#)

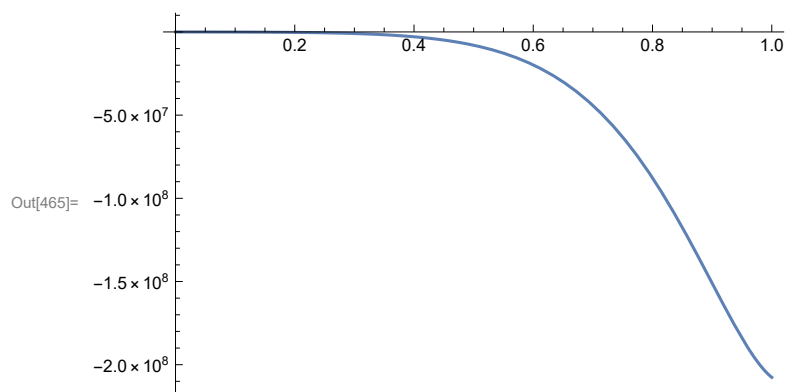

In[466]:= **Plot[Cf[12, 5, 10], {x, 0, 1}]**

[绘图](#)

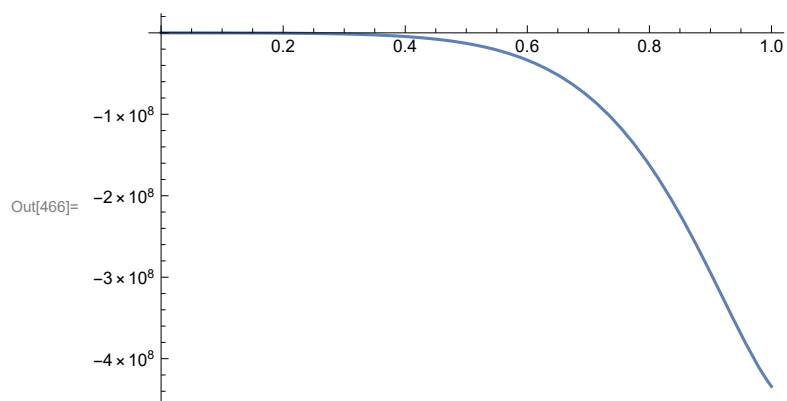

In[467]:= **Plot[Cf[12, 5, 9], {x, 0, 1}]**

[绘图](#)

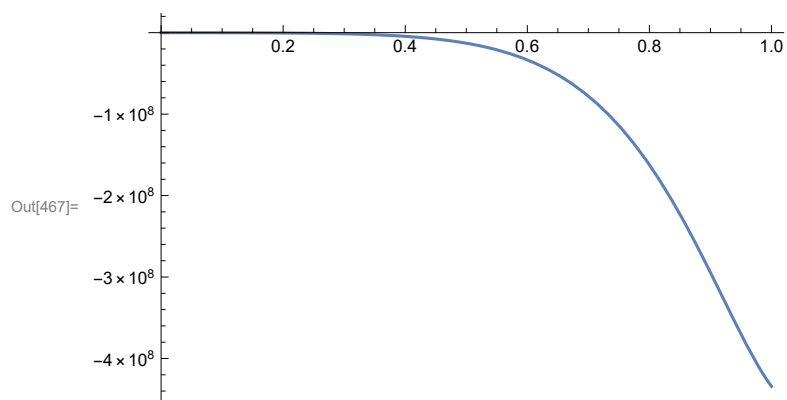

In[468]:= **Plot[Cf[12, 5, 8], {x, 0, 1}]**

[绘图](#)

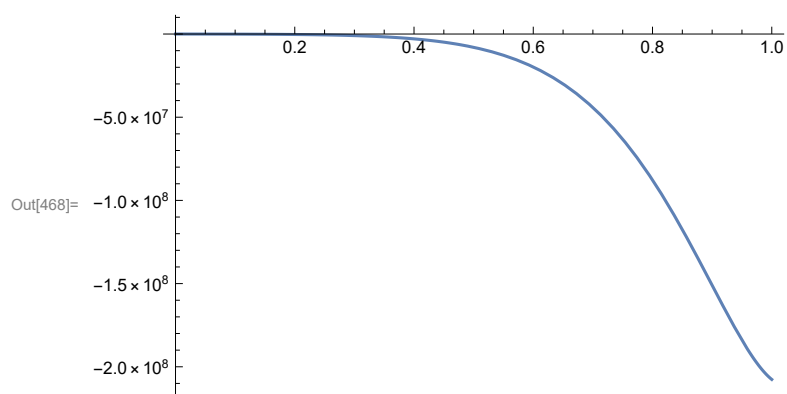

In[469]:= **Plot[Cf[12, 5, 7], {x, 0, 1}]**

[绘图](#)

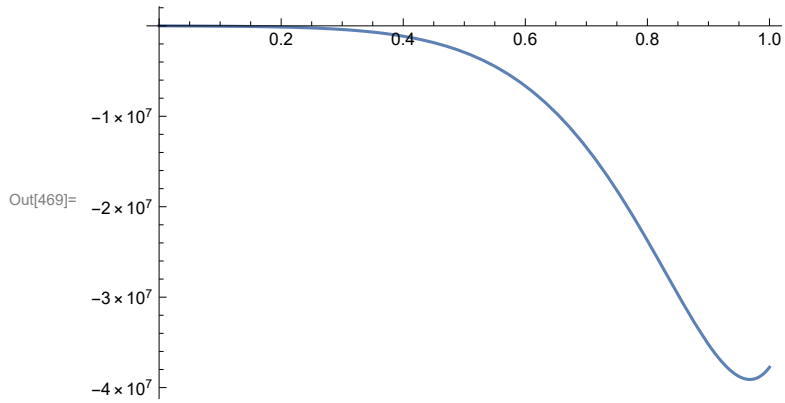

In[470]:= **Plot[Cf[12, 5, 6], {x, 0, 1}]**

[绘图](#)

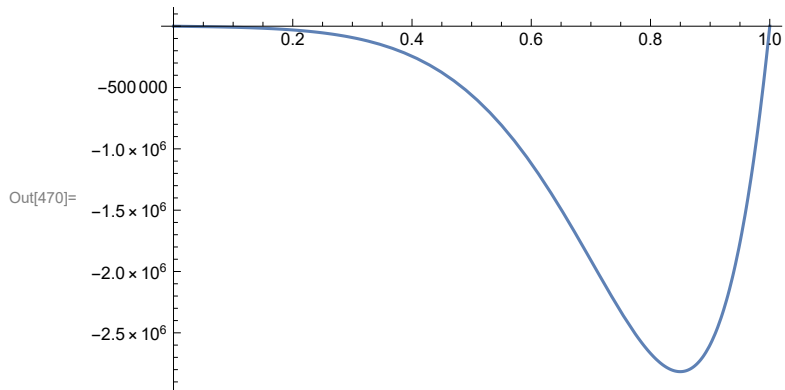

In[471]:= **Plot[Cf[12, 5, 5], {x, 0, 1}]**

[绘图](#)

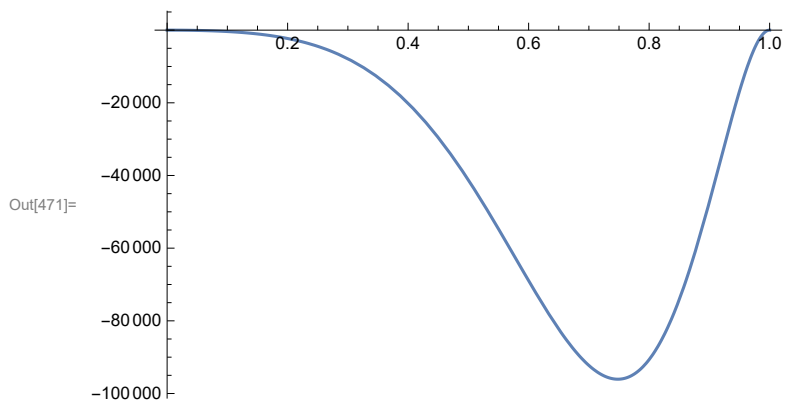

```
Plot[Cf[12, 5, 4], {x, 0, 1}]
```

[绘图](#)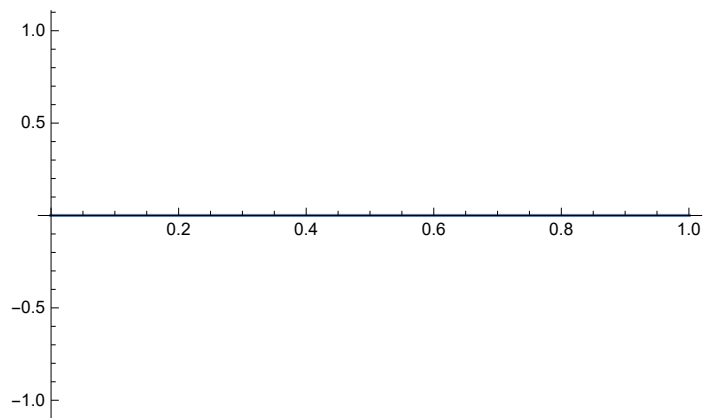

```
Plot[Cf[12, 5, 3], {x, 0, 1}]
```

[绘图](#)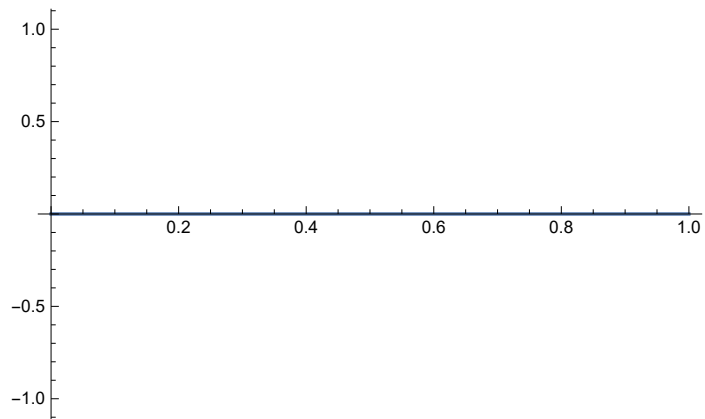

```
Plot[Cf[12, 5, 2], {x, 0, 1}]
```

[绘图](#)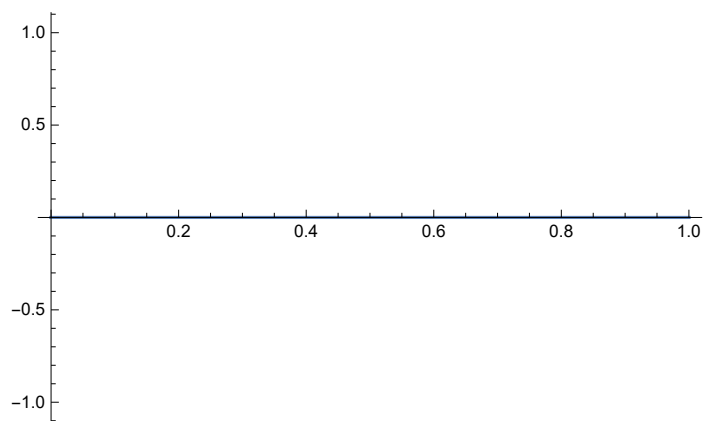



**Plot[Cf[12, 5, 1], {x, 0, 1}]**

[绘图](#)

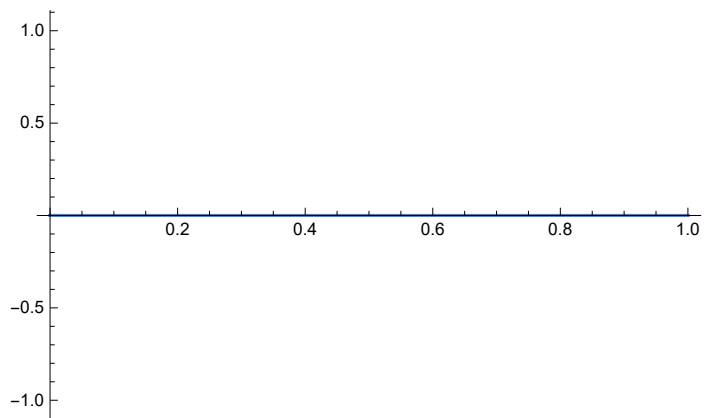

**Plot[Cf[12, 5, 0], {x, 0, 1}]**

[绘图](#)

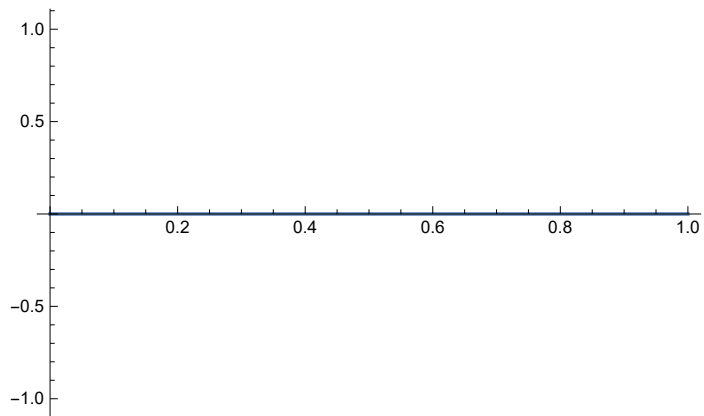

**(\*41th group coefficients r2^12r3^4\*)**

In[472]:= **Plot[Cf[12, 4, 14], {x, 0, 1}]**

[绘图](#)

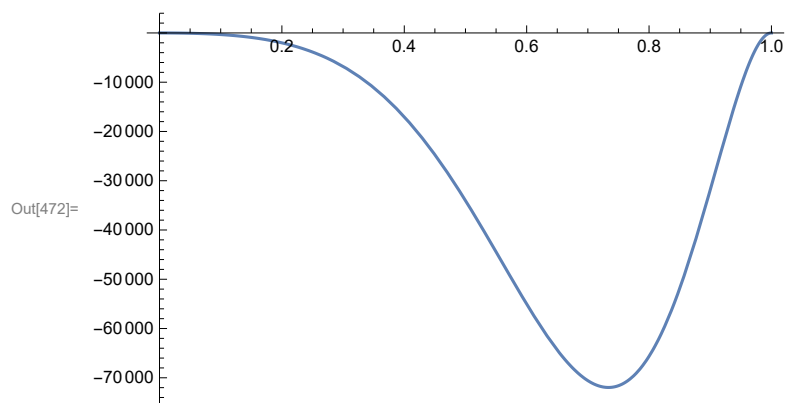

In[473]:= **Plot[Cf[12, 4, 13], {x, 0, 1}]**

[绘图](#)

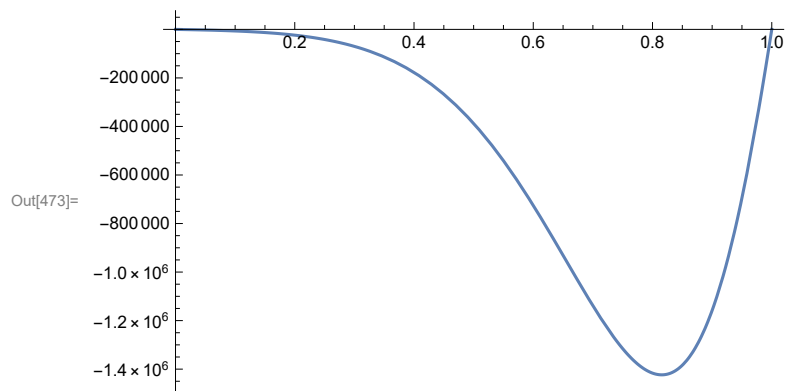

In[474]:= **Plot[Cf[12, 4, 12], {x, 0, 1}]**

[绘图](#)

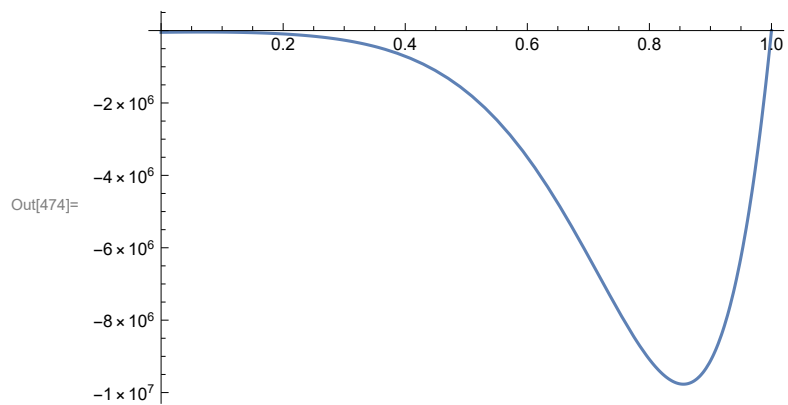

In[475]:= **Plot[Cf[12, 4, 11], {x, 0, 1}]**

[绘图](#)

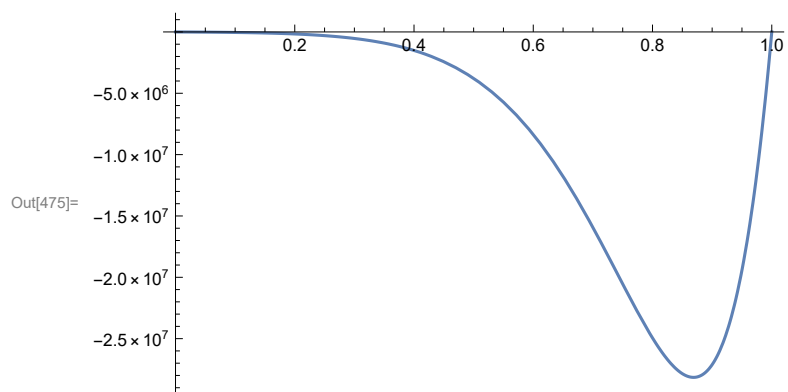

In[476]:= **Plot**[**Cf**[12, 4, 10], {x, 0, 1}]

[绘图](#)

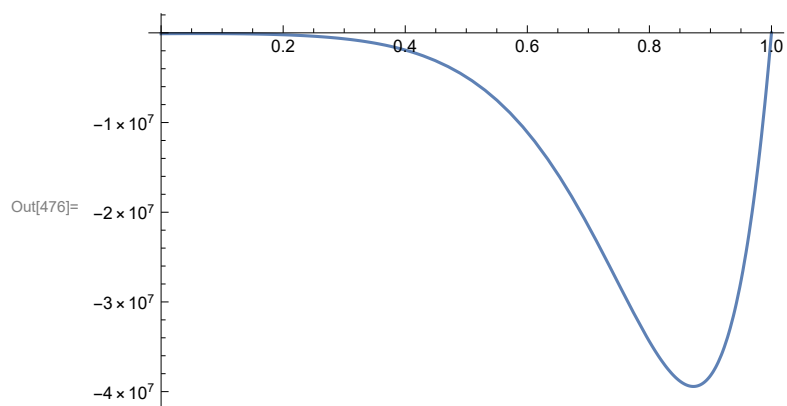

In[477]:= **Plot**[**Cf**[12, 4, 9], {x, 0, 1}]

[绘图](#)

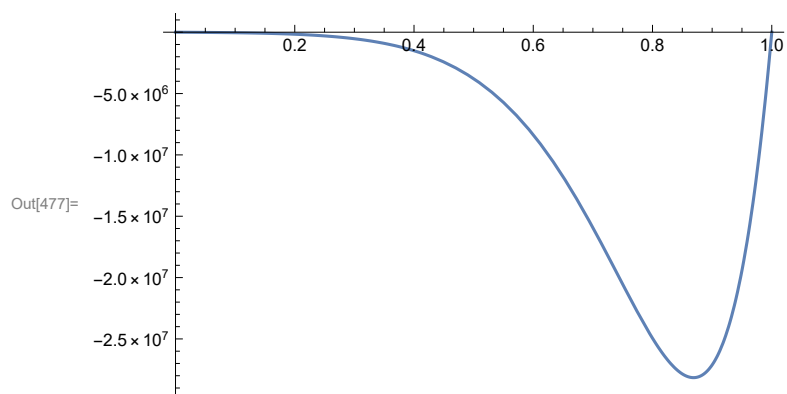

In[478]:= **Plot**[**Cf**[12, 4, 8], {x, 0, 1}]

[绘图](#)

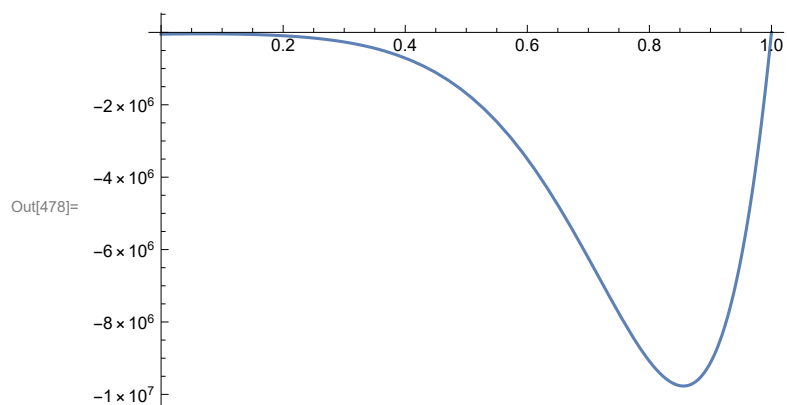

In[479]:= **Plot[Cf[12, 4, 7], {x, 0, 1}]**

[绘图](#)

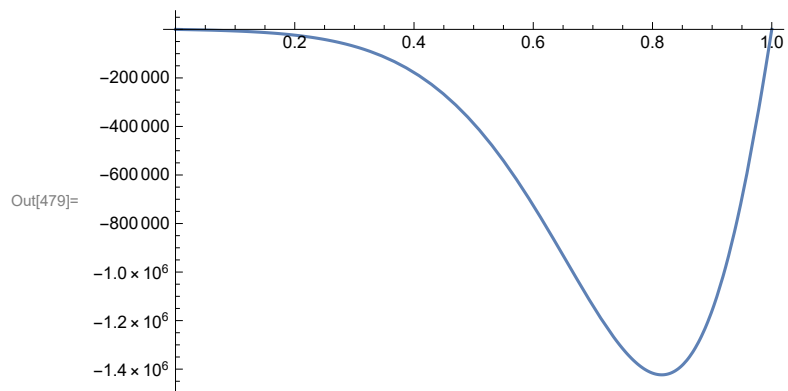

In[480]:= **Plot[Cf[12, 4, 6], {x, 0, 1}]**

[绘图](#)

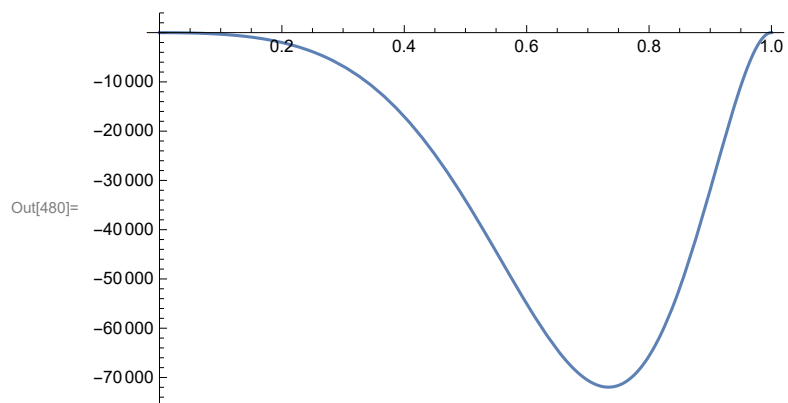

**Plot[Cf[12, 4, 5], {x, 0, 1}]**

[绘图](#)

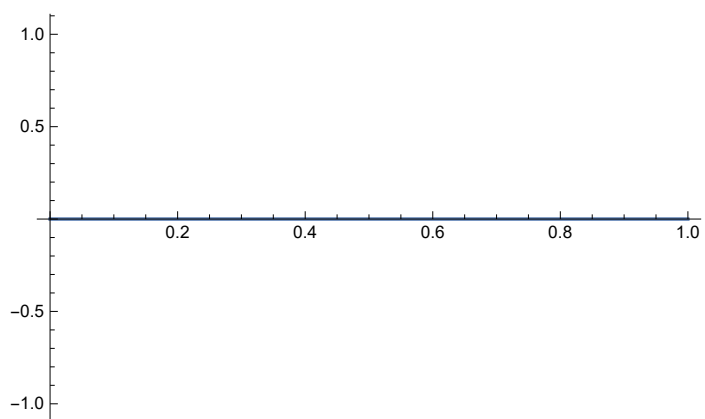

**Plot[Cf[12, 4, 4], {x, 0, 1}]**

[绘图](#)

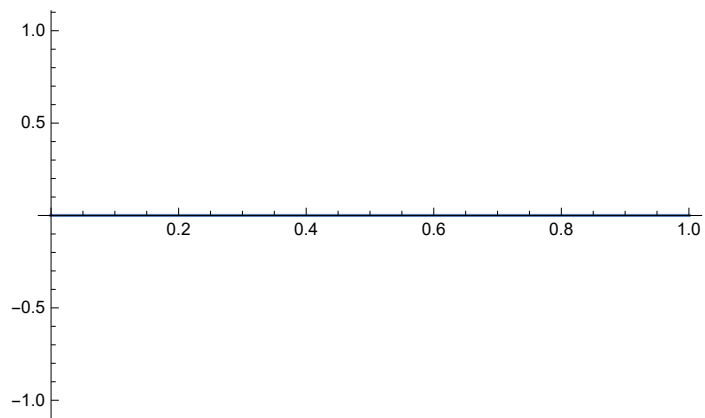

**Plot[Cf[12, 4, 3], {x, 0, 1}]**

[绘图](#)

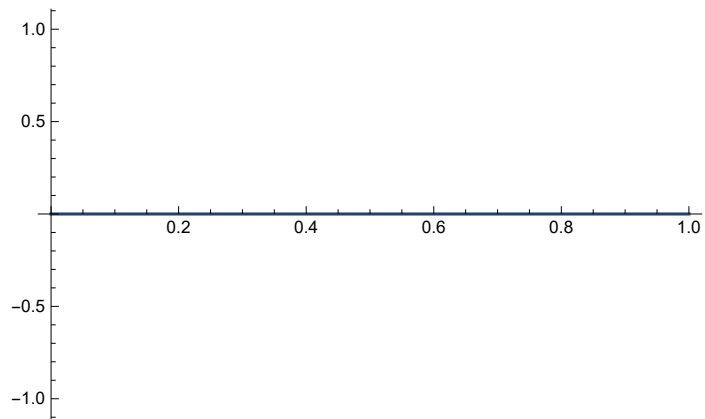

**Plot[Cf[12, 4, 2], {x, 0, 1}]**

[绘图](#)

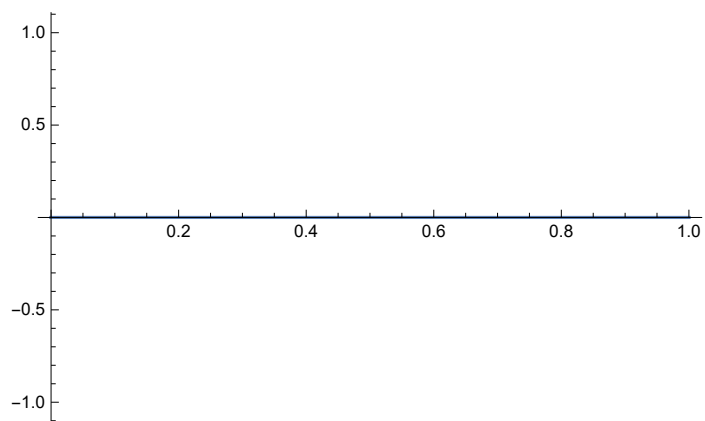

**Plot[Cf[12, 4, 1], {x, 0, 1}]**

[绘图](#)

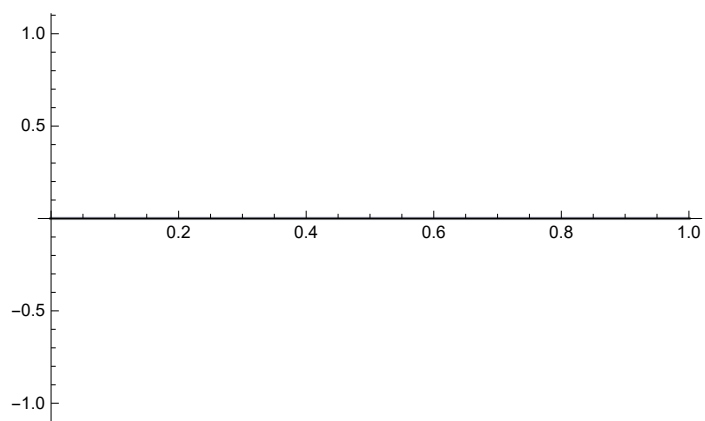

**Plot[Cf[12, 4, 0], {x, 0, 1}]**

[绘图](#)

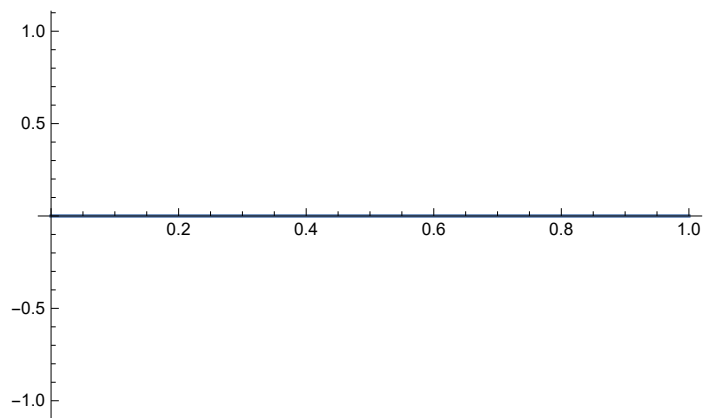

**(\*42th group coefficients r2^12r3^3\*)**

In[481]:= **Plot[Cf[12, 3, 14], {x, 0, 1}]**

[绘图](#)

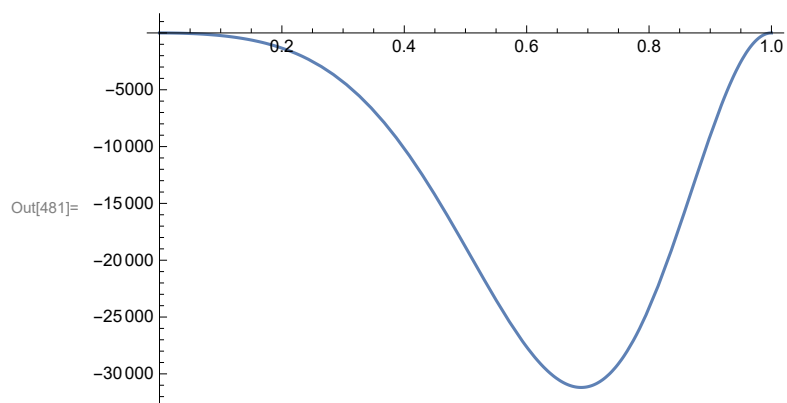

In[482]:= **Plot**[**Cf**[12, 3, 13], {x, 0, 1}]

[绘图](#)

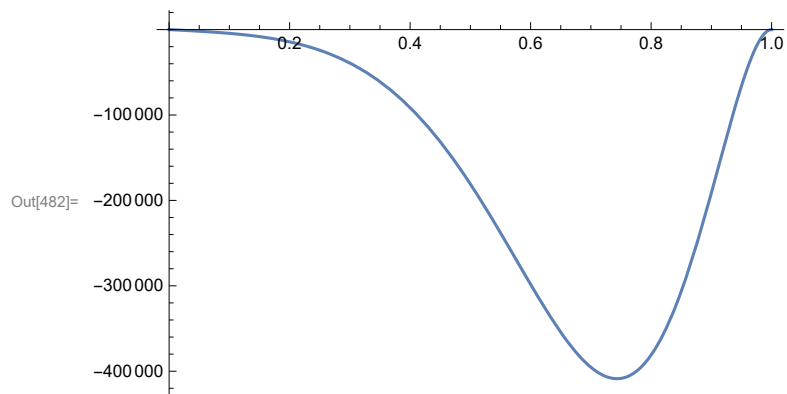

In[483]:= **Plot**[**Cf**[12, 3, 12], {x, 0, 1}]

[绘图](#)

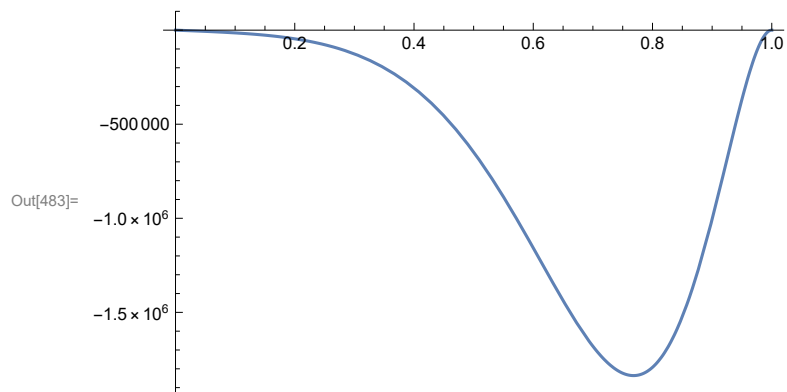

In[484]:= **Plot**[**Cf**[12, 3, 11], {x, 0, 1}]

[绘图](#)

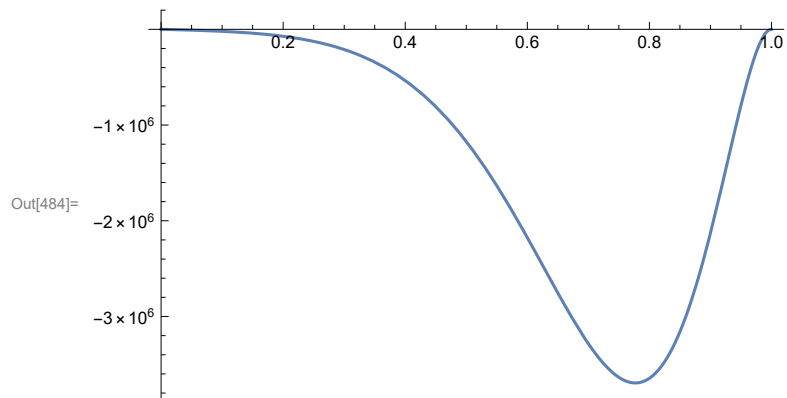

In[485]:= **Plot[Cf[12, 3, 10], {x, 0, 1}]**

[绘图](#)

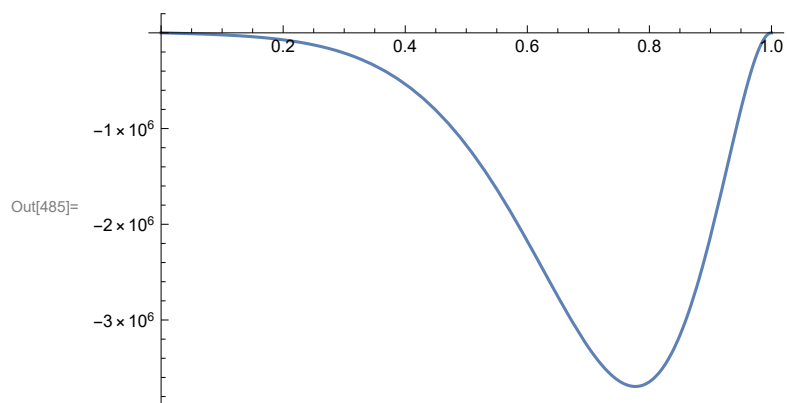

In[486]:= **Plot[Cf[12, 3, 9], {x, 0, 1}]**

[绘图](#)

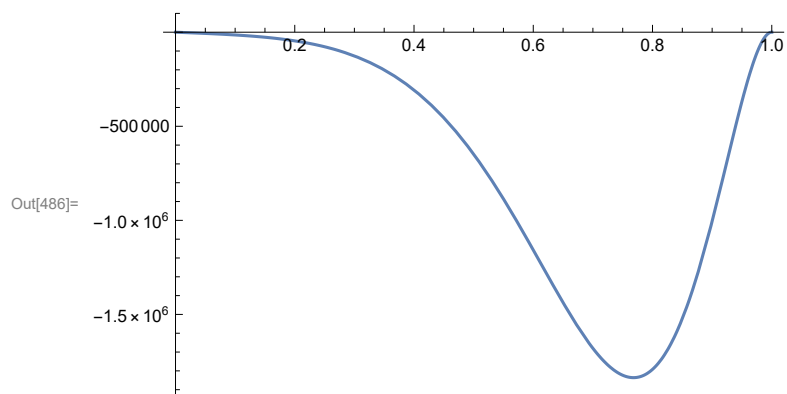

In[487]:= **Plot[Cf[12, 3, 8], {x, 0, 1}]**

[绘图](#)

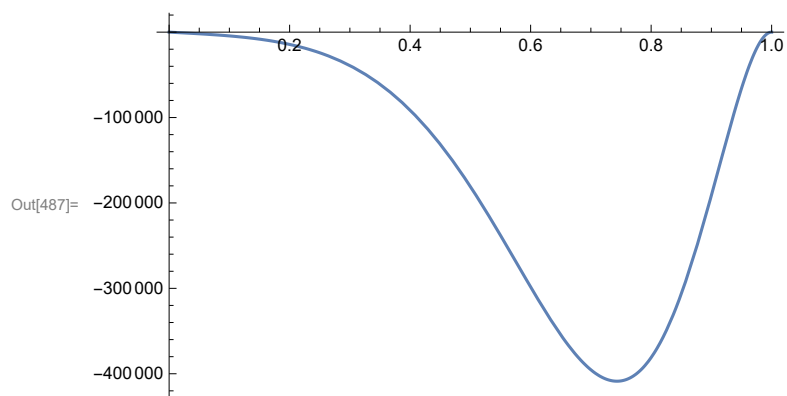



In[488]:= **Plot[Cf[12, 3, 7], {x, 0, 1}]**

[绘图](#)

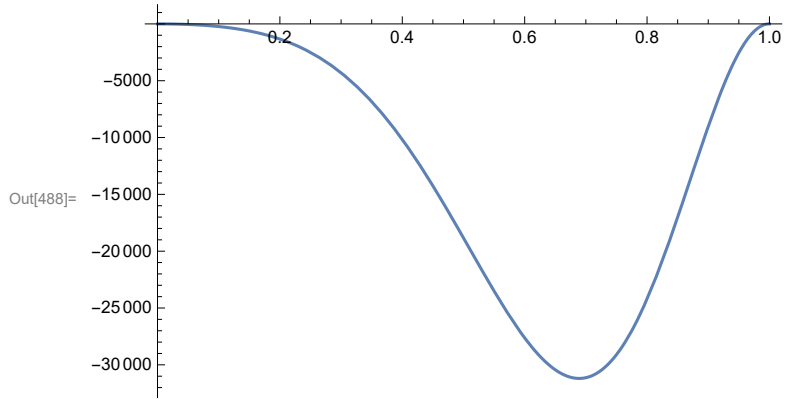

**Plot[Cf[12, 3, 6], {x, 0, 1}]**

[绘图](#)

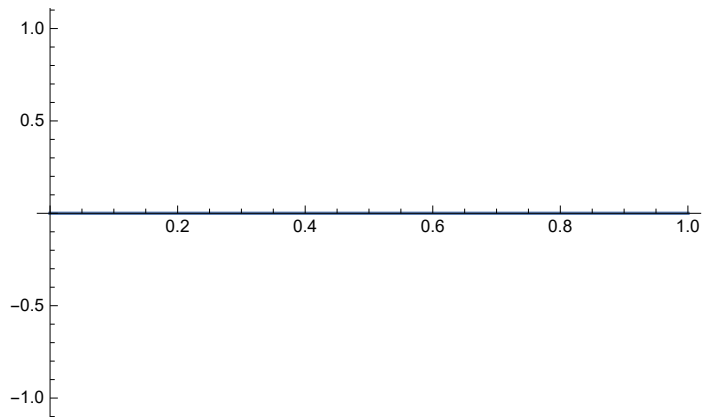

**Plot[Cf[12, 3, 5], {x, 0, 1}]**

[绘图](#)

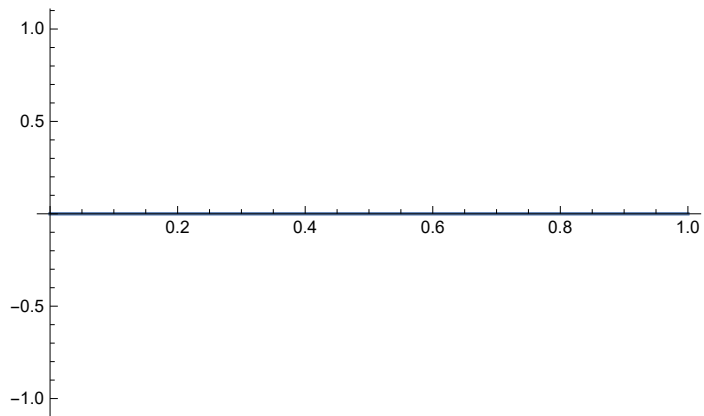

```
Plot[Cf[12, 3, 4], {x, 0, 1}]
```

[绘图](#)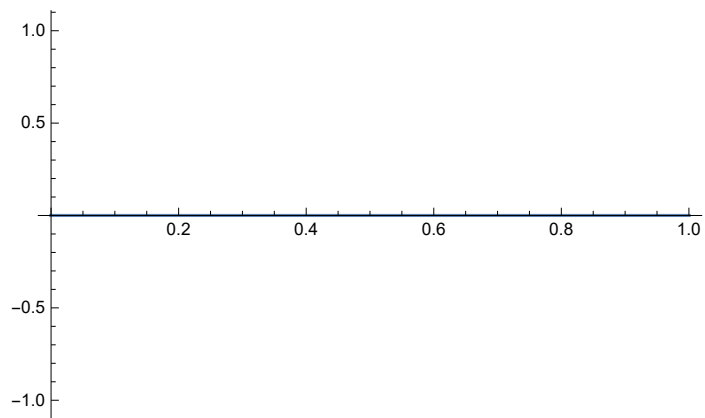

```
Plot[Cf[12, 3, 3], {x, 0, 1}]
```

[绘图](#)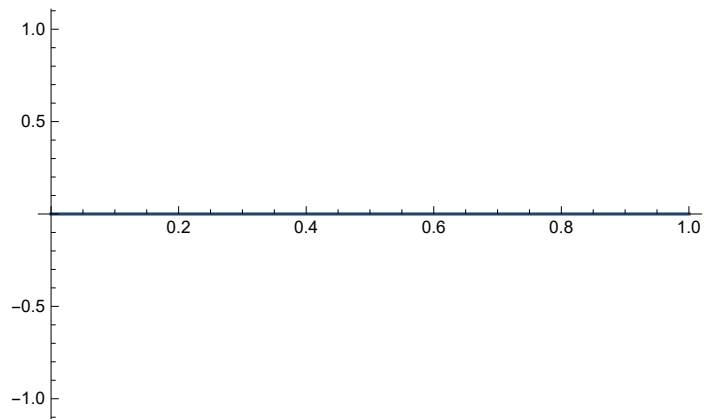

```
Plot[Cf[12, 3, 2], {x, 0, 1}]
```

[绘图](#)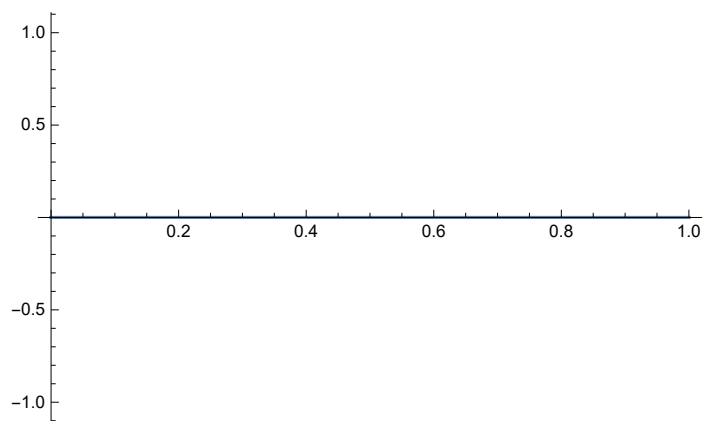

**Plot[Cf[12, 3, 1], {x, 0, 1}]**

[绘图](#)

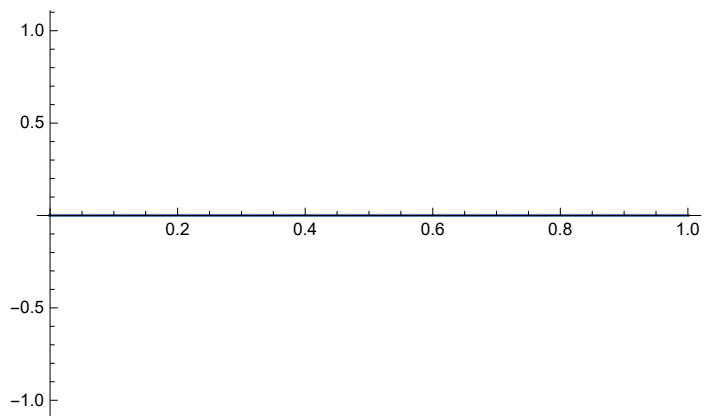

**Plot[Cf[12, 3, 0], {x, 0, 1}]**

[绘图](#)

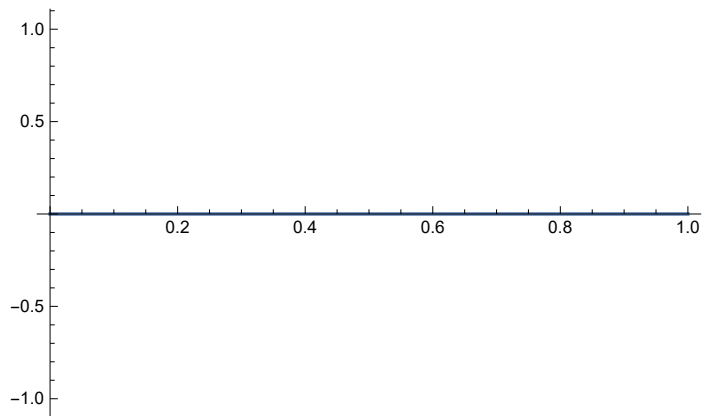

**(\*43th group coefficients r2^12r3^2\*)**

In[489]:= **Plot[Cf[12, 2, 14], {x, 0, 1}]**

[绘图](#)

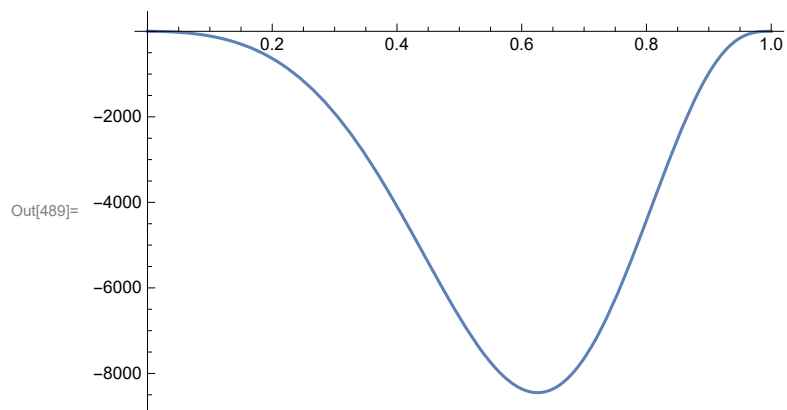

In[490]:= **Plot[Cf[12, 2, 13], {x, 0, 1}]**

[绘图](#)

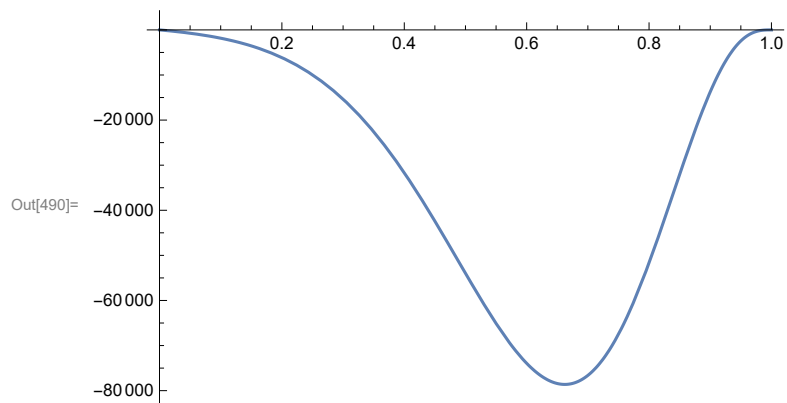

In[491]:= **Plot[Cf[12, 2, 12], {x, 0, 1}]**

[绘图](#)

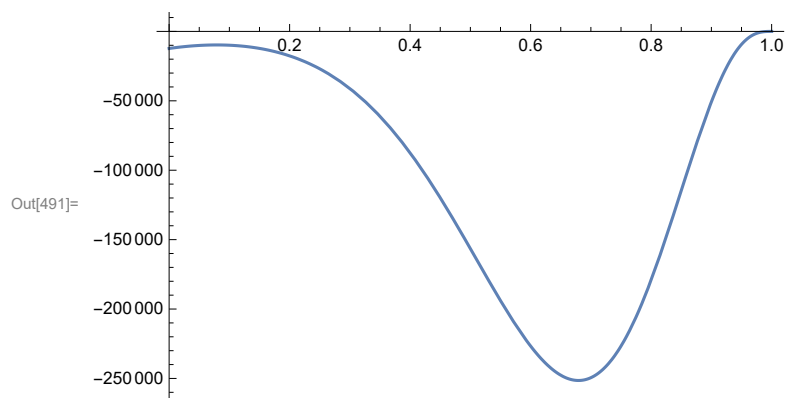

In[492]:= **Plot[Cf[12, 2, 11], {x, 0, 1}]**

[绘图](#)

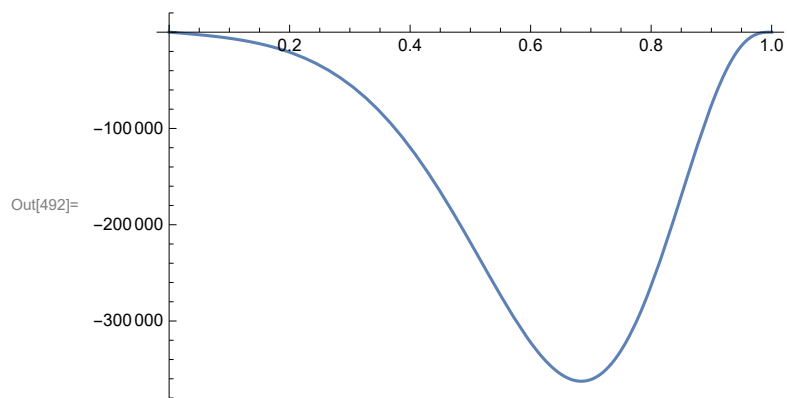

In[493]:= **Plot[Cf[12, 2, 10], {x, 0, 1}]**

[绘图](#)

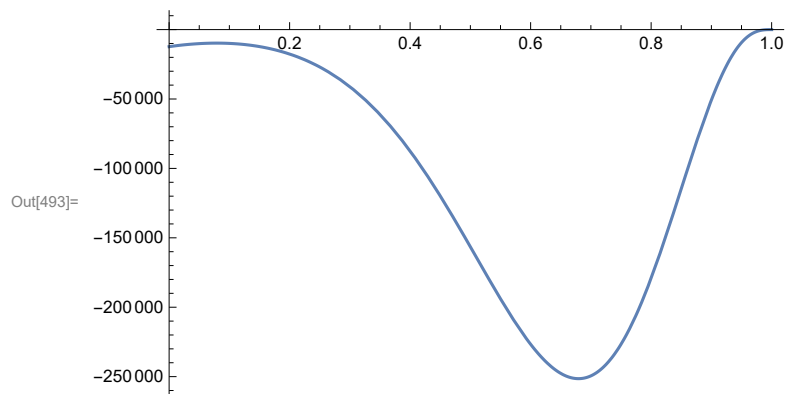

In[494]:= **Plot[Cf[12, 2, 9], {x, 0, 1}]**

[绘图](#)

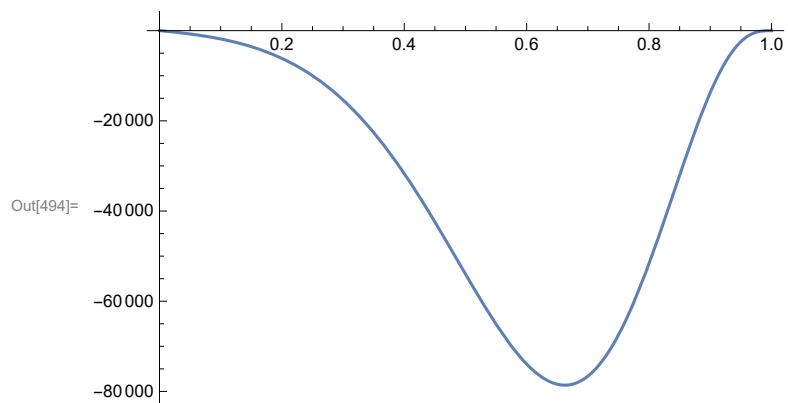

In[495]:= **Plot[Cf[12, 2, 8], {x, 0, 1}]**

[绘图](#)

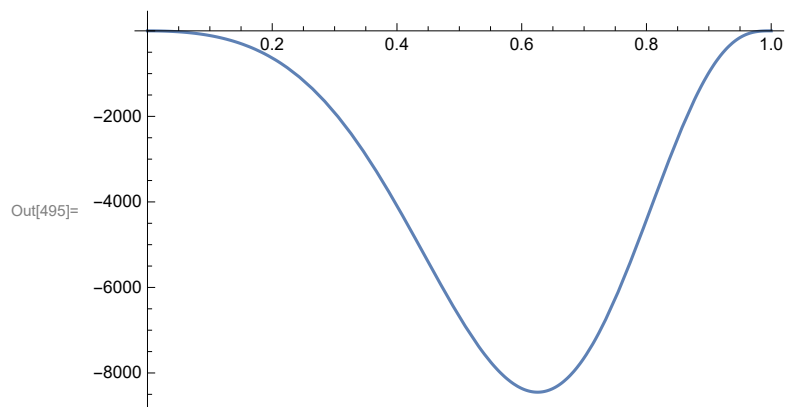

```
Plot[Cf[12, 2, 7], {x, 0, 1}]
```

[绘图](#)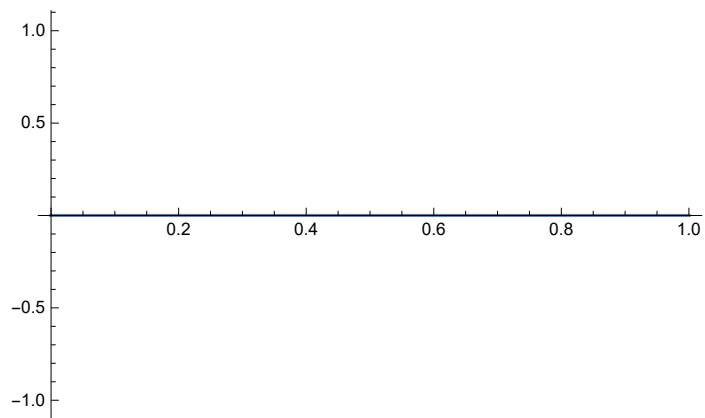

```
Plot[Cf[12, 2, 6], {x, 0, 1}]
```

[绘图](#)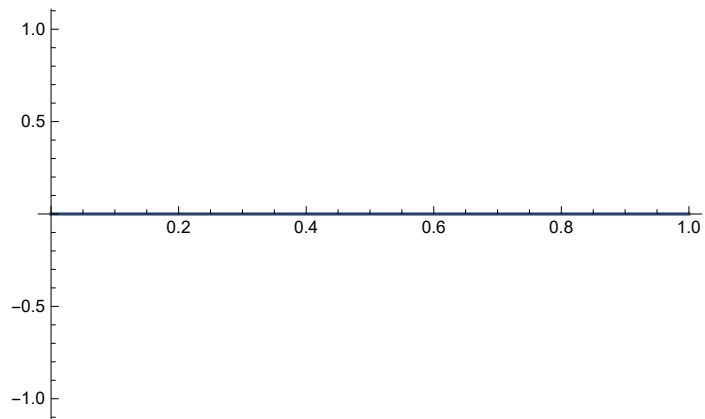

```
Plot[Cf[12, 2, 5], {x, 0, 1}]
```

[绘图](#)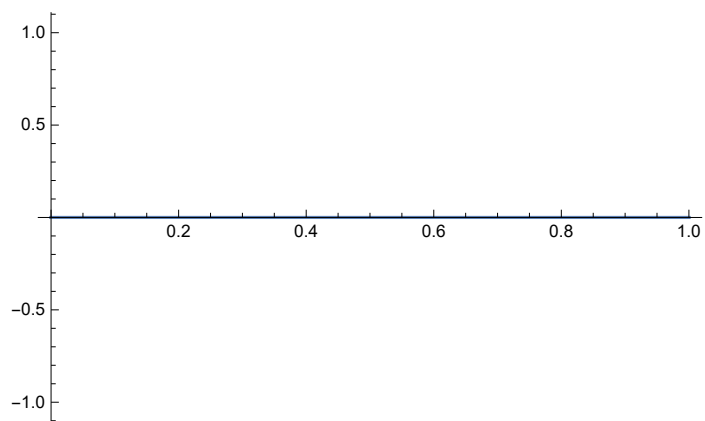

**Plot[Cf[12, 2, 4], {x, 0, 1}]**

[绘图](#)

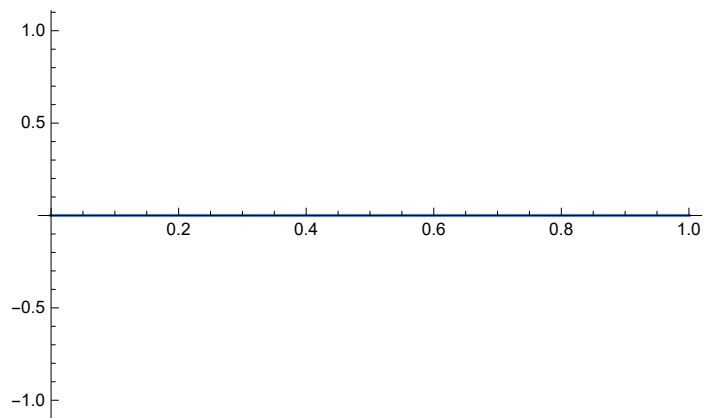

**Plot[Cf[12, 2, 3], {x, 0, 1}]**

[绘图](#)

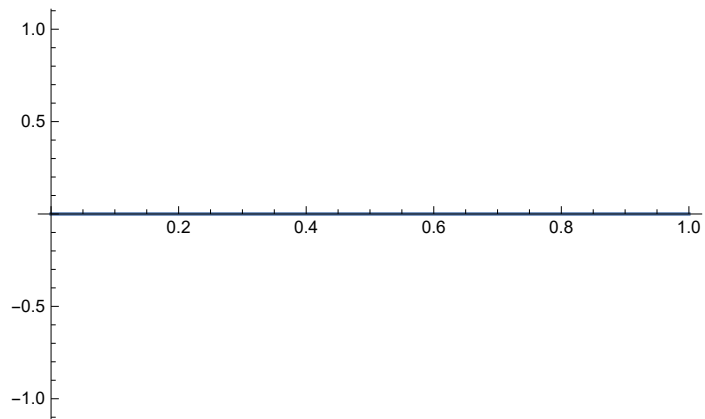

**Plot[Cf[12, 2, 2], {x, 0, 1}]**

[绘图](#)

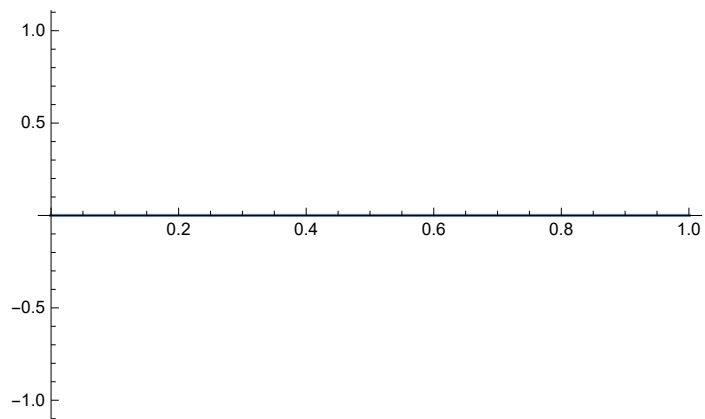

**Plot[Cf[12, 2, 1], {x, 0, 1}]**

[绘图](#)

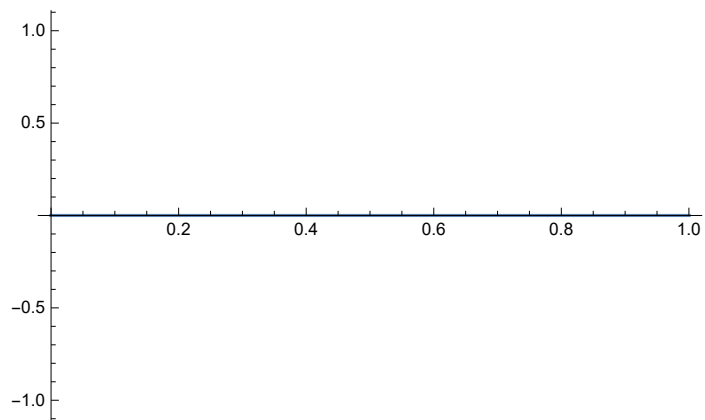

**Plot[Cf[12, 2, 0], {x, 0, 1}]**

[绘图](#)

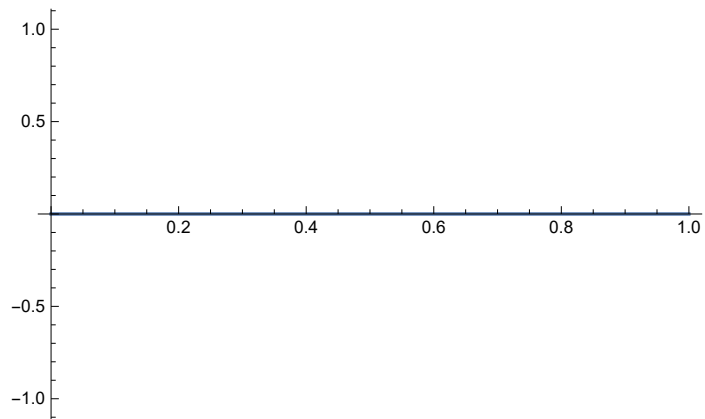

**(\*44th group coefficients r2^12r3^1\*)**

In[496]:= **Plot[Cf[12, 1, 14], {x, 0, 1}]**

[绘图](#)

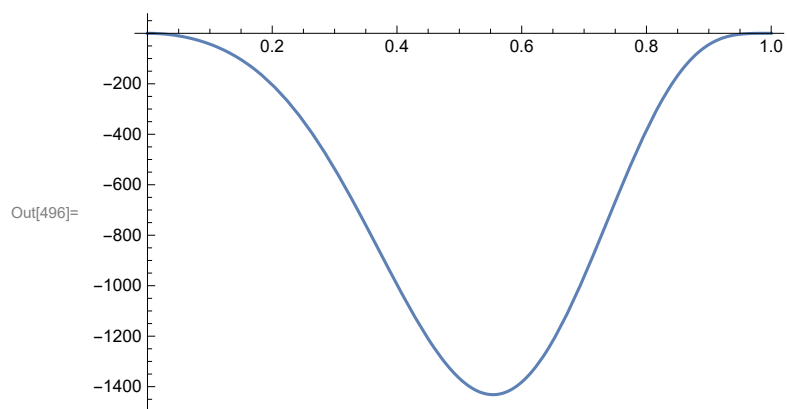



In[497]:= **Plot[Cf[12, 1, 13], {x, 0, 1}]**

[绘图](#)

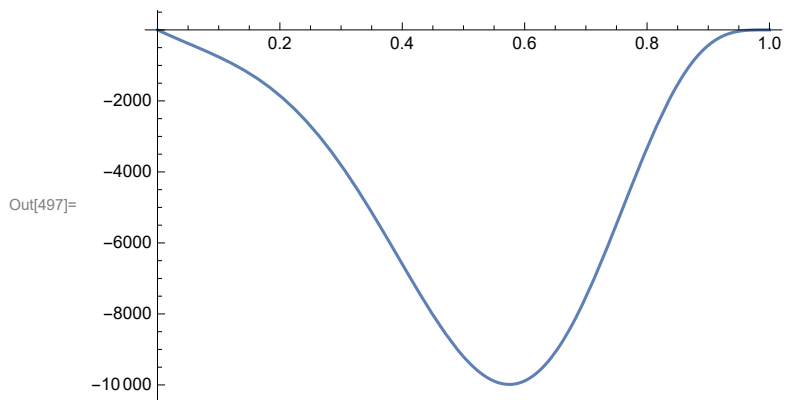

In[498]:= **Plot[Cf[12, 1, 12], {x, 0, 1}]**

[绘图](#)

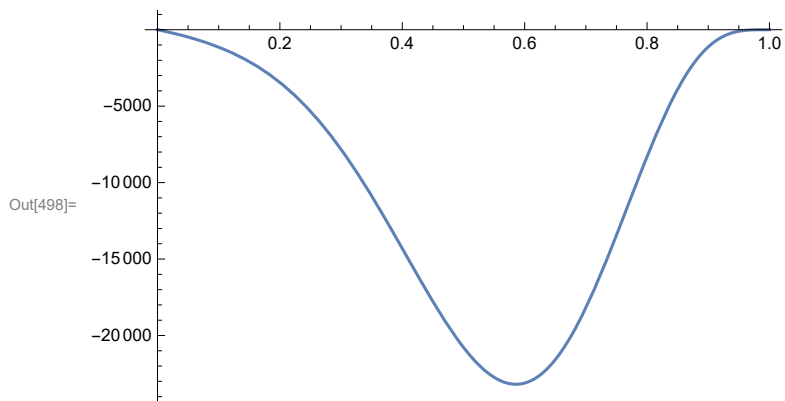

In[499]:= **Plot[Cf[12, 1, 11], {x, 0, 1}]**

[绘图](#)

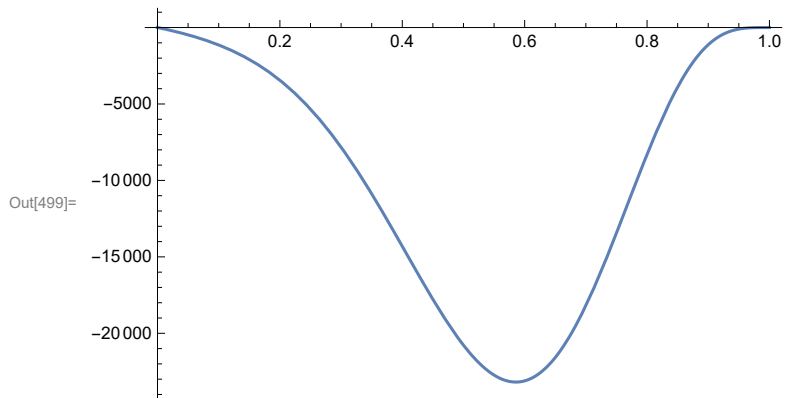

In[500]:= **Plot[Cf[12, 1, 10], {x, 0, 1}]**

[绘图](#)

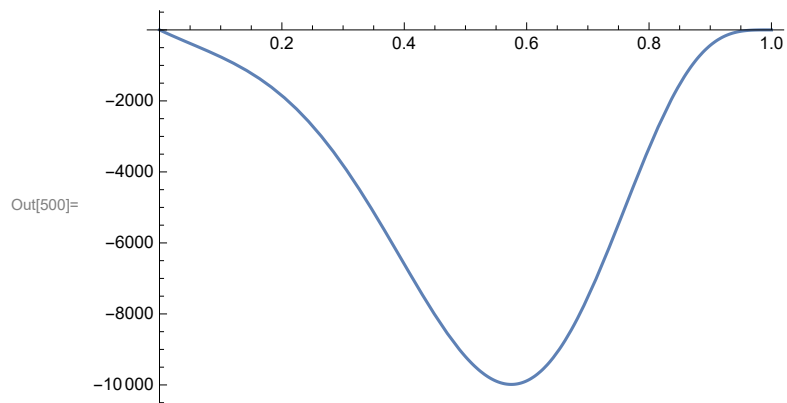

In[501]:= **Plot[Cf[12, 1, 9], {x, 0, 1}]**

[绘图](#)

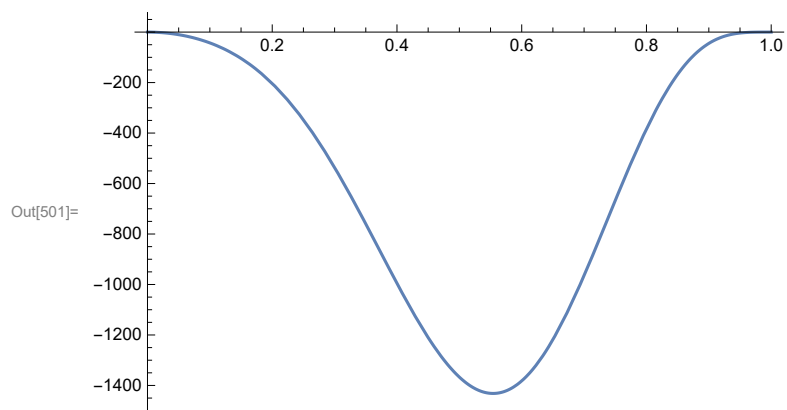

**Plot[Cf[12, 1, 8], {x, 0, 1}]**

[绘图](#)

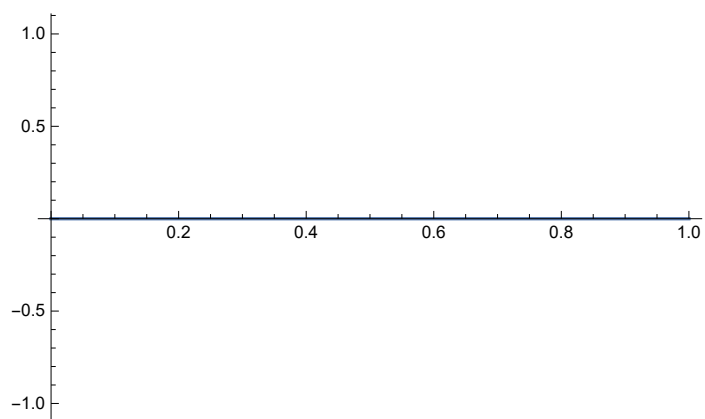

**Plot[Cf[12, 1, 7], {x, 0, 1}]**

[绘图](#)

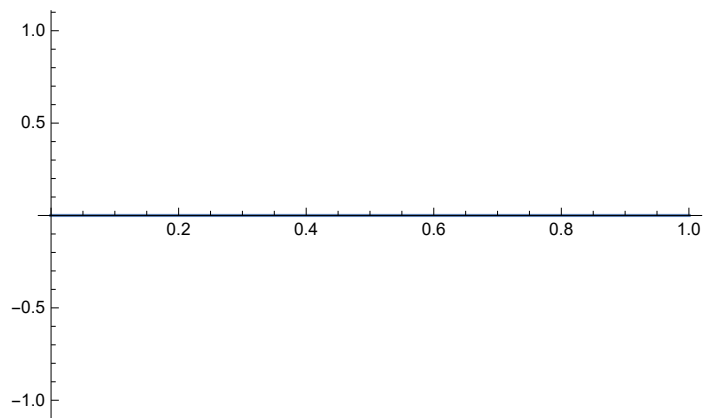

**Plot[Cf[12, 1, 6], {x, 0, 1}]**

[绘图](#)

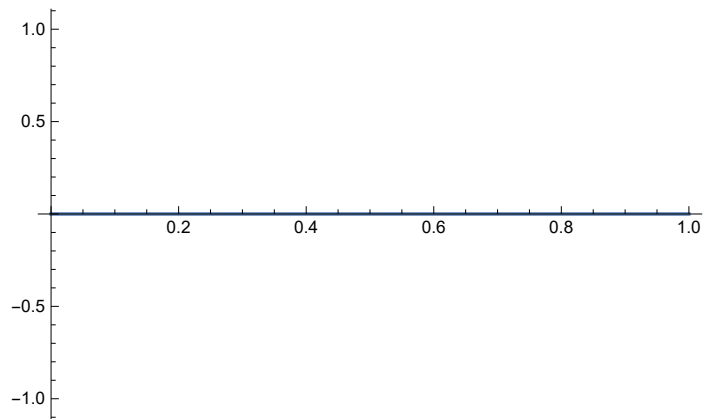

**Plot[Cf[12, 1, 5], {x, 0, 1}]**

[绘图](#)

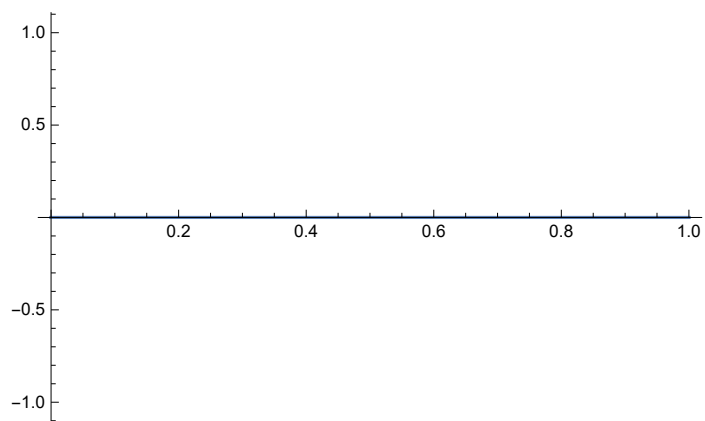

```
Plot[Cf[12, 1, 4], {x, 0, 1}]
```

[绘图](#)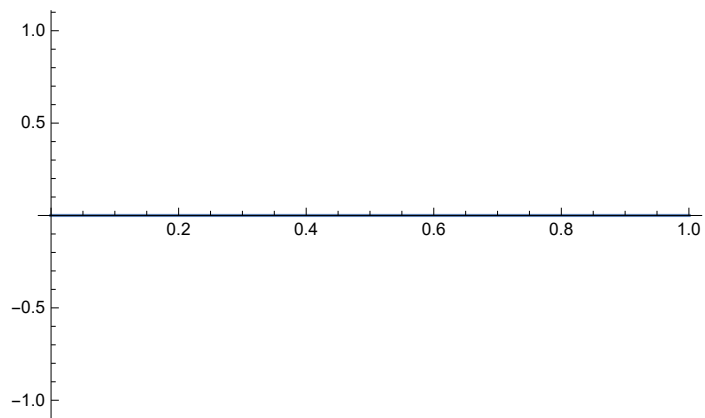

```
Plot[Cf[12, 1, 3], {x, 0, 1}]
```

[绘图](#)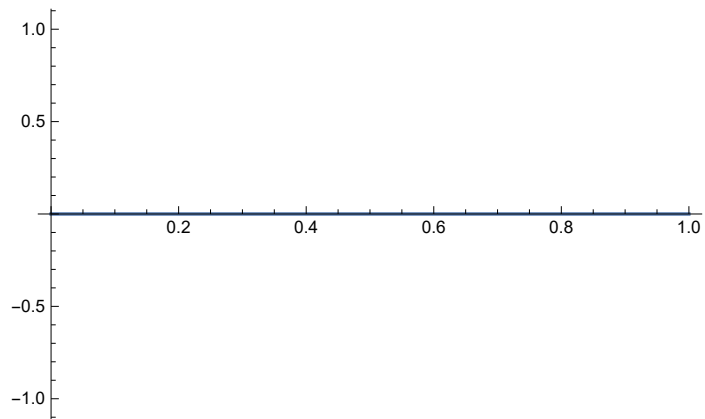

```
Plot[Cf[12, 1, 2], {x, 0, 1}]
```

[绘图](#)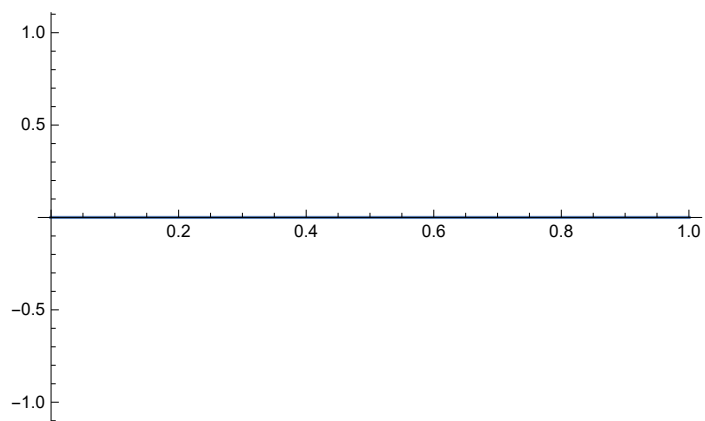

**Plot[Cf[12, 1, 1], {x, 0, 1}]**

[绘图](#)

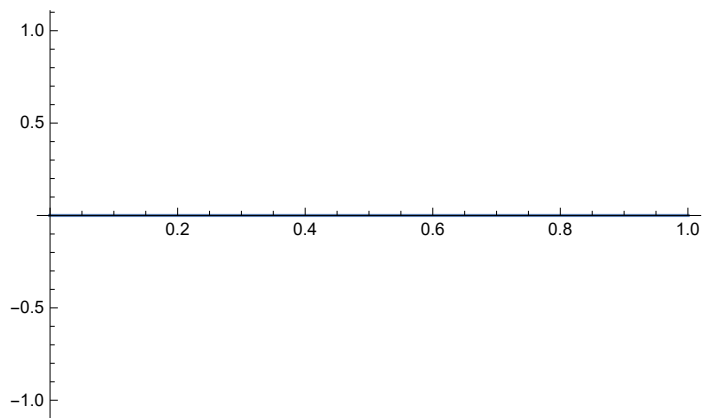

**Plot[Cf[12, 1, 0], {x, 0, 1}]**

[绘图](#)

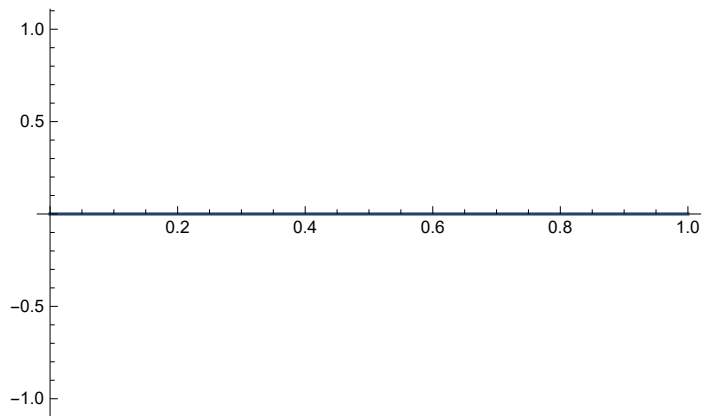

**(\*45th group coefficients r2^12r3^0\*)**

In[503]:= **Plot[Cf[12, 0, 14], {x, 0, 1}]**

[绘图](#)

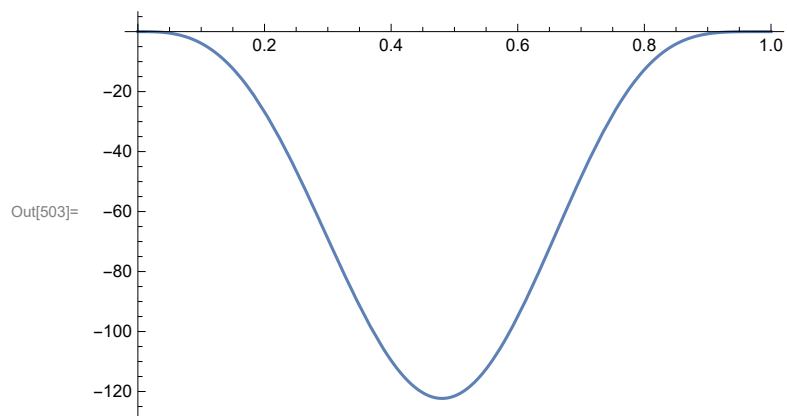

**(\*46th group coefficients r2^11r3^14\*)**

**Plot[Cf[11, 14, 14], {x, 0, 1}]**

[绘图](#)

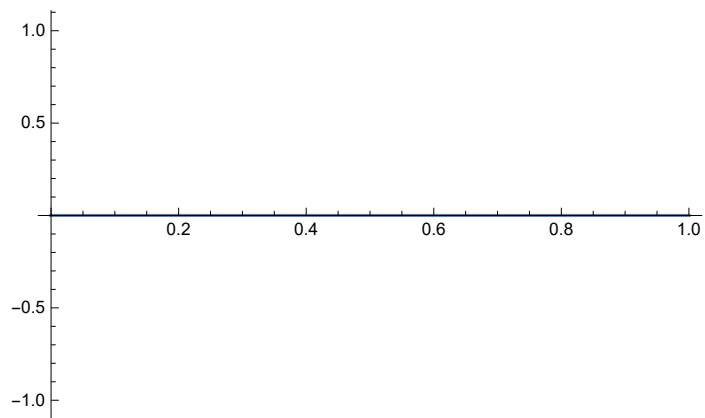

**Plot[Cf[11, 14, 13], {x, 0, 1}]**

[绘图](#)

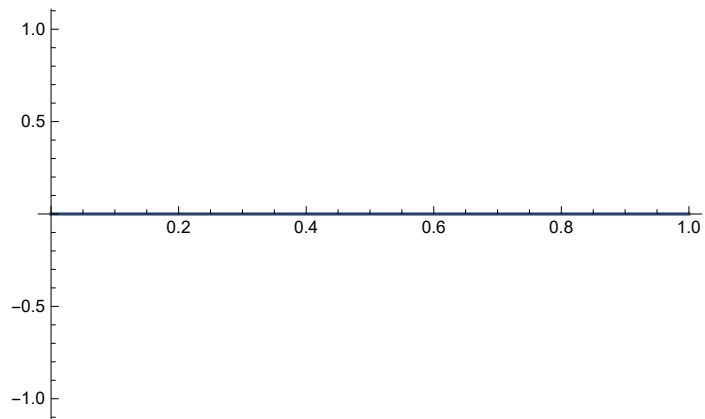

**Plot[Cf[11, 14, 12], {x, 0, 1}]**

[绘图](#)

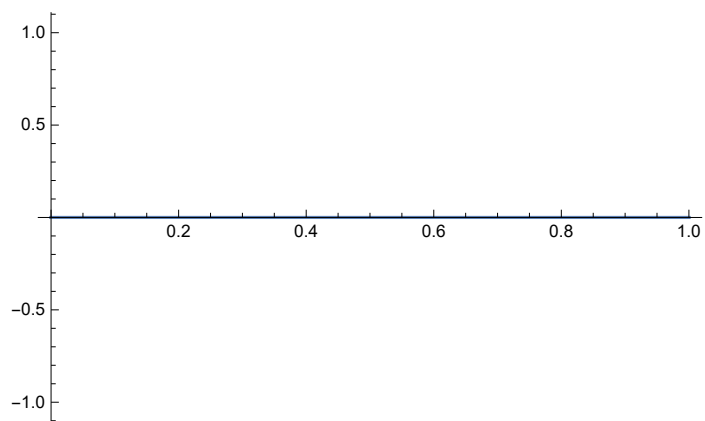

In[504]:= **Plot[Cf[11, 14, 11], {x, 0, 1}]**

[绘图](#)

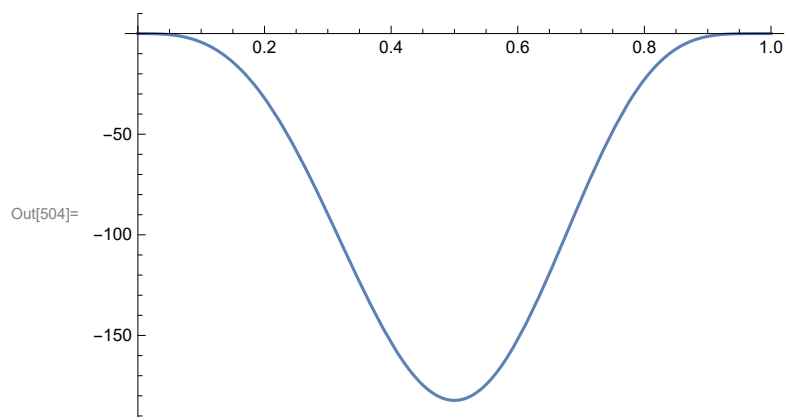

In[505]:= **Plot[Cf[11, 14, 10], {x, 0, 1}]**

[绘图](#)

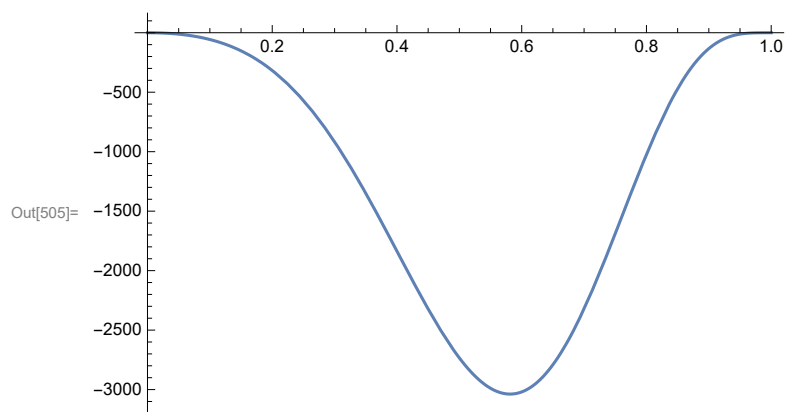

In[506]:= **Plot[Cf[11, 14, 9], {x, 0, 1}]**

[绘图](#)

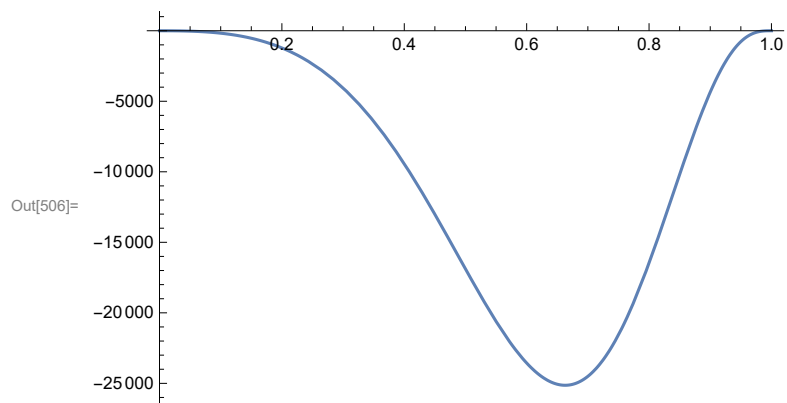

In[507]:= **Plot[Cf[11, 14, 8], {x, 0, 1}]**

[绘图](#)

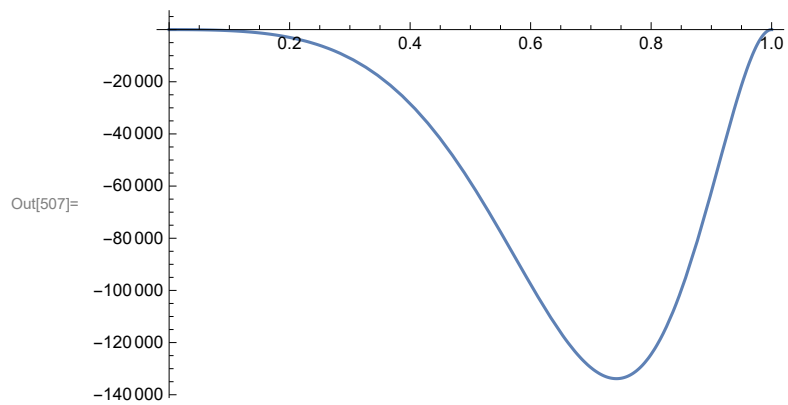

In[508]:= **Plot[Cf[11, 14, 7], {x, 0, 1}]**

[绘图](#)

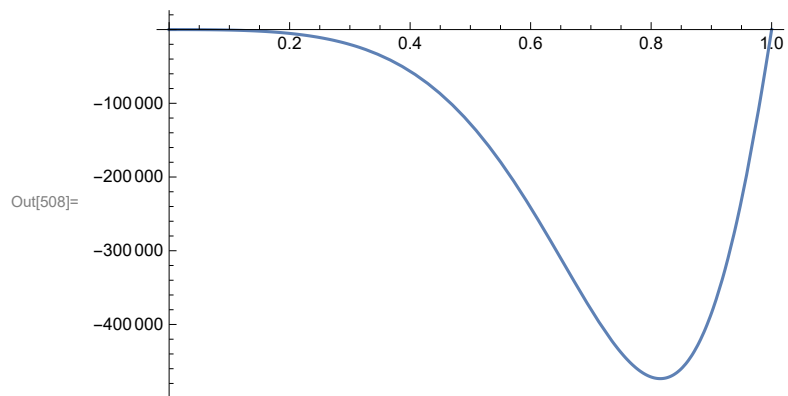

In[509]:= **Plot[Cf[11, 14, 6], {x, 0, 1}]**

[绘图](#)

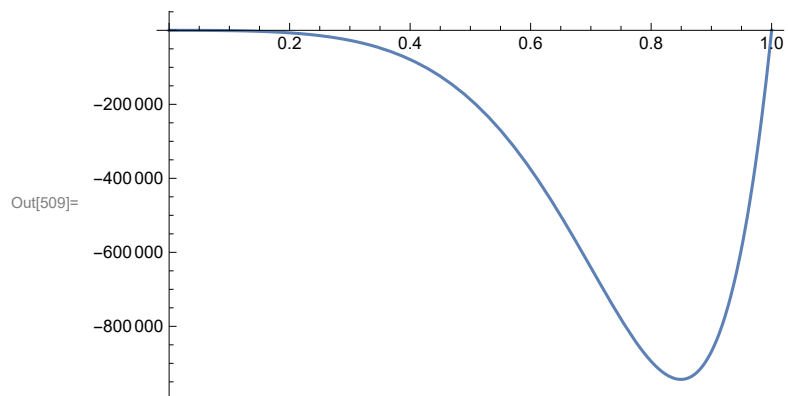



In[510]:= **Plot[Cf[11, 14, 5], {x, 0, 1}]**

[绘图](#)

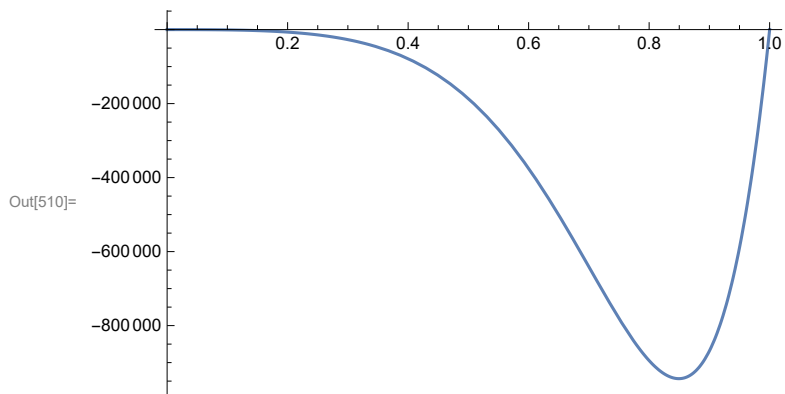

In[511]:= **Plot[Cf[11, 14, 4], {x, 0, 1}]**

[绘图](#)

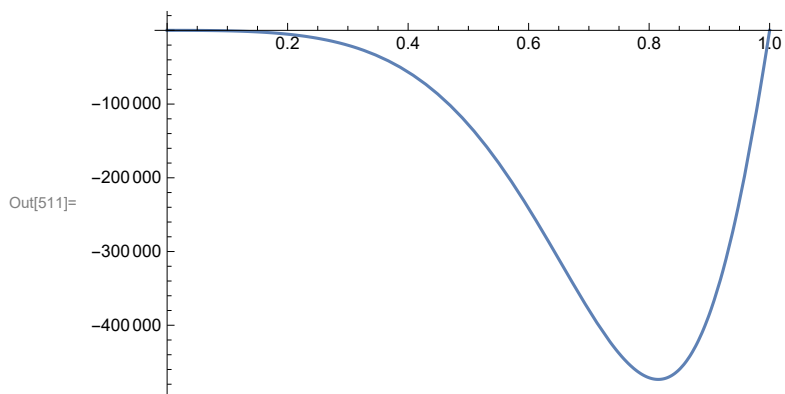

In[512]:= **Plot[Cf[11, 14, 3], {x, 0, 1}]**

[绘图](#)

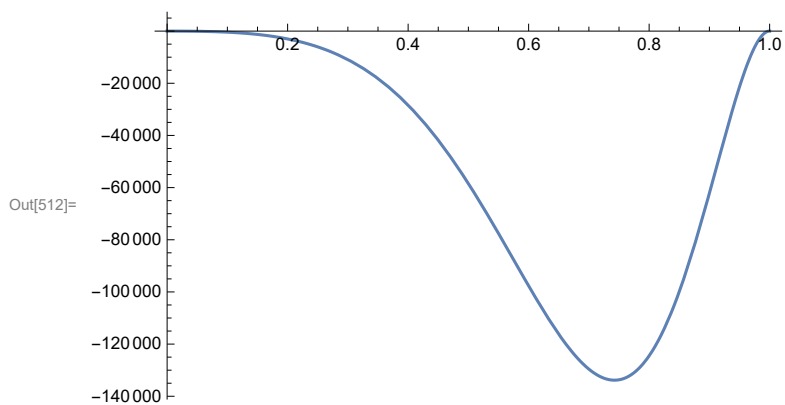

In[513]:= **Plot[Cf[11, 14, 2], {x, 0, 1}]**

[绘图](#)

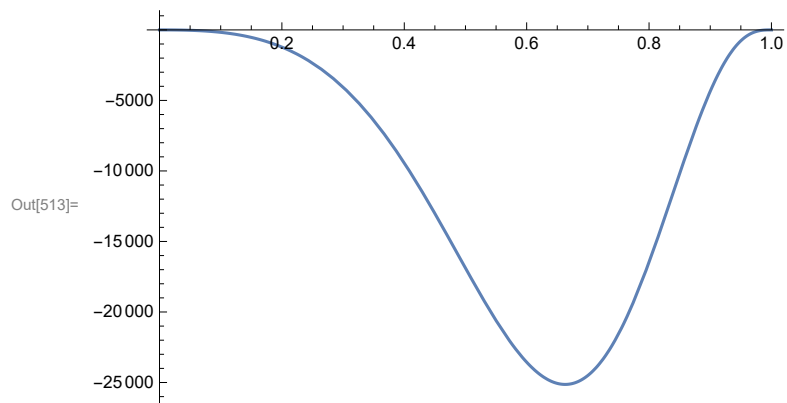

In[514]:= **Plot[Cf[11, 14, 1], {x, 0, 1}]**

[绘图](#)

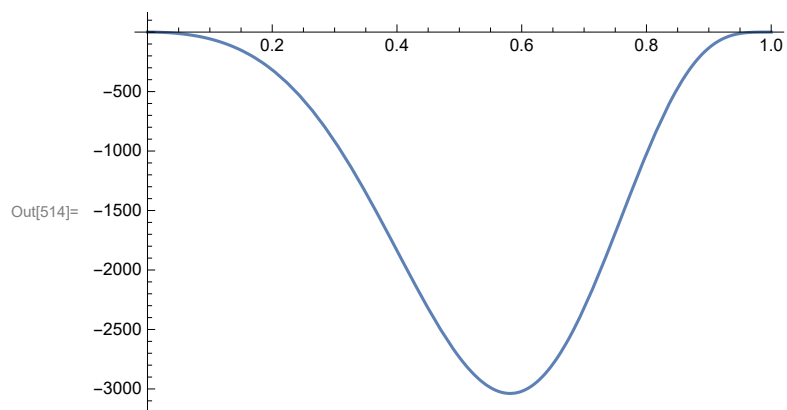

In[515]:= **Plot[Cf[11, 14, 0], {x, 0, 1}]**

[绘图](#)

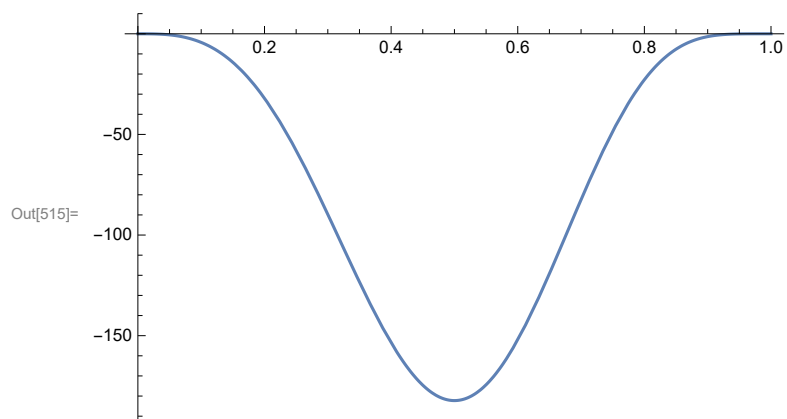

(\*47th group coefficients r2^11r3^13\*)

**Plot[Cf[11, 13, 14], {x, 0, 1}]**

[绘图](#)

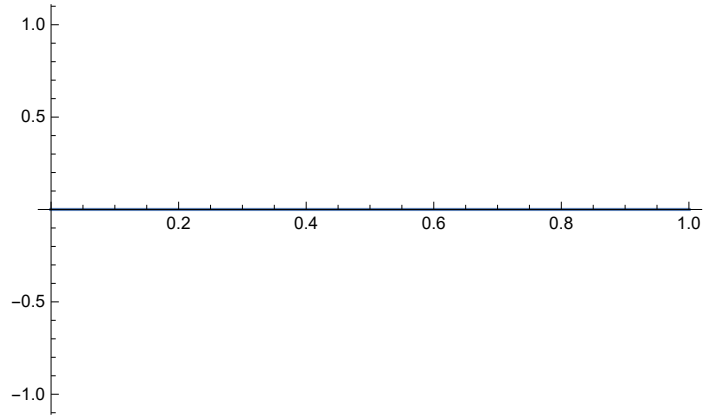

**Plot[Cf[11, 13, 13], {x, 0, 1}]**

[绘图](#)

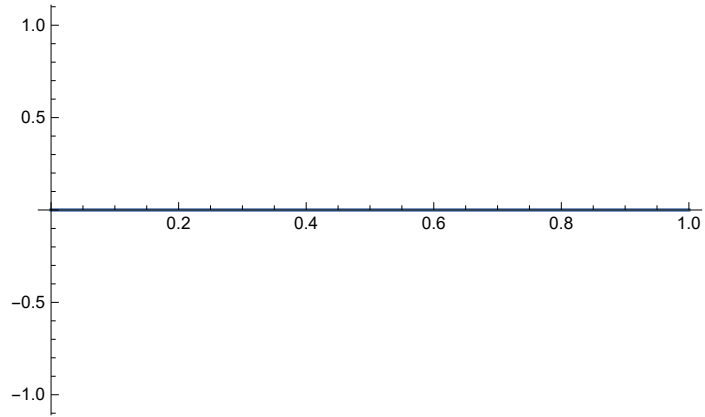

In[516]:= **Plot[Cf[11, 13, 12], {x, 0, 1}]**

[绘图](#)

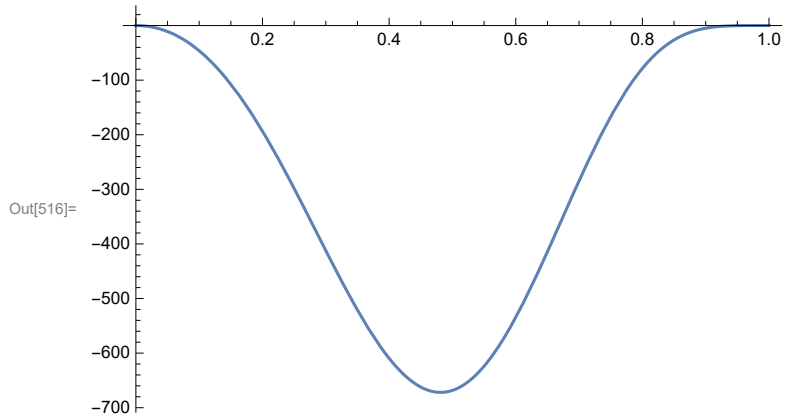

In[517]:= **Plot[Cf[11, 13, 11], {x, 0, 1}]**

[绘图](#)

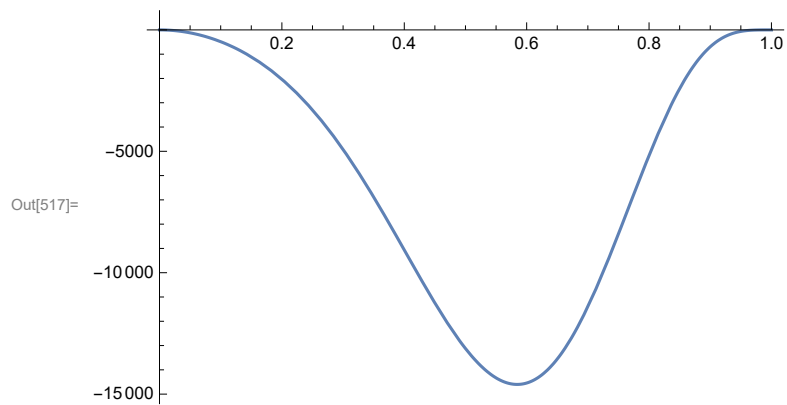

In[518]:= **Plot[Cf[11, 13, 10], {x, 0, 1}]**

[绘图](#)

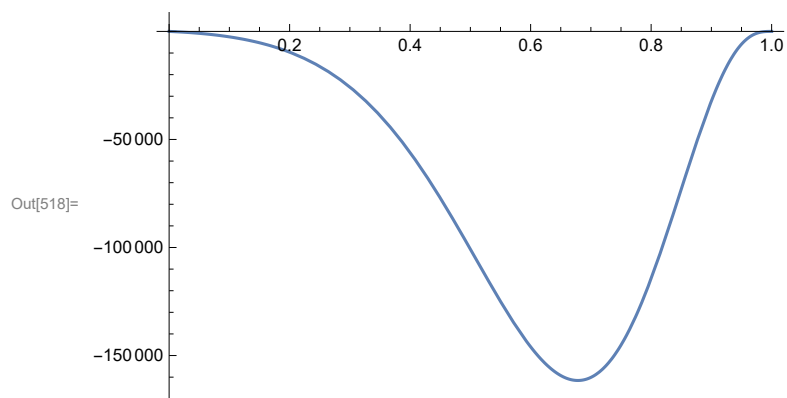

In[519]:= **Plot[Cf[11, 13, 9], {x, 0, 1}]**

[绘图](#)

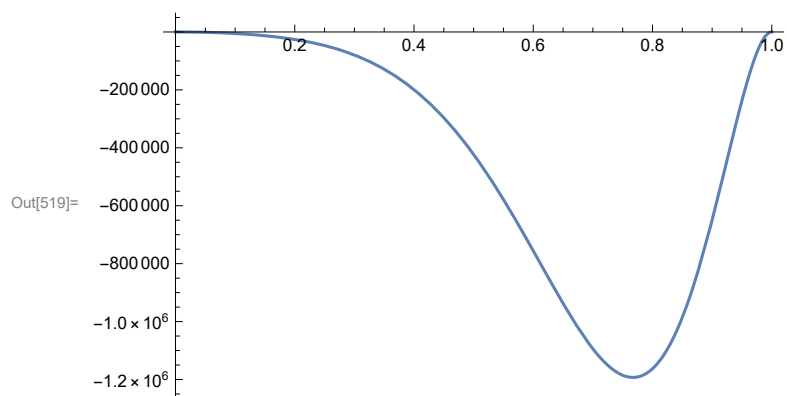

In[520]:= **Plot[Cf[11, 13, 8], {x, 0, 1}]**

[绘图](#)

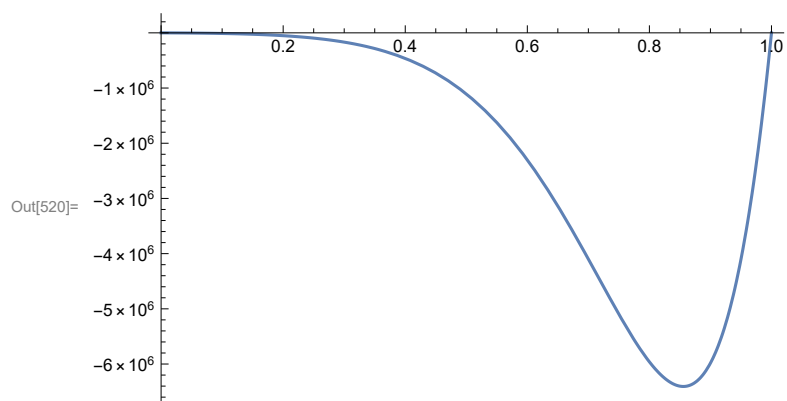

In[521]:= **Plot[Cf[11, 13, 7], {x, 0, 1}]**

[绘图](#)

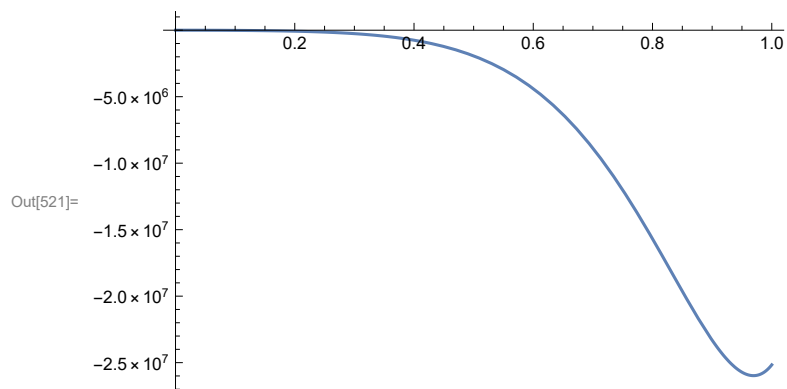

In[522]:= **Plot[Cf[11, 13, 6], {x, 0, 1}]**

[绘图](#)

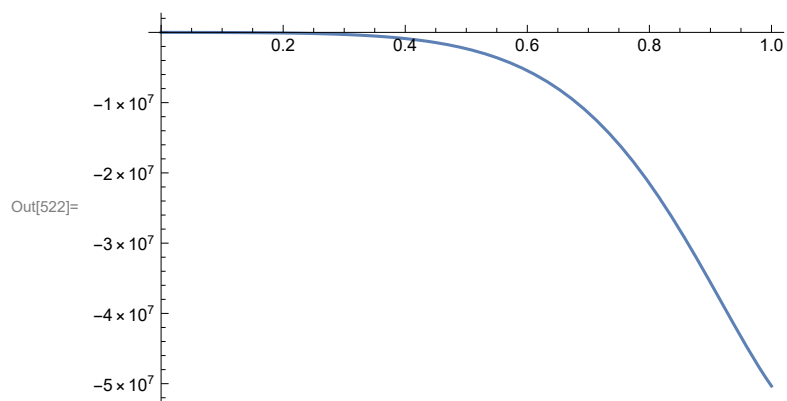

In[523]:= **Plot[Cf[11, 13, 5], {x, 0, 1}]**

[绘图](#)

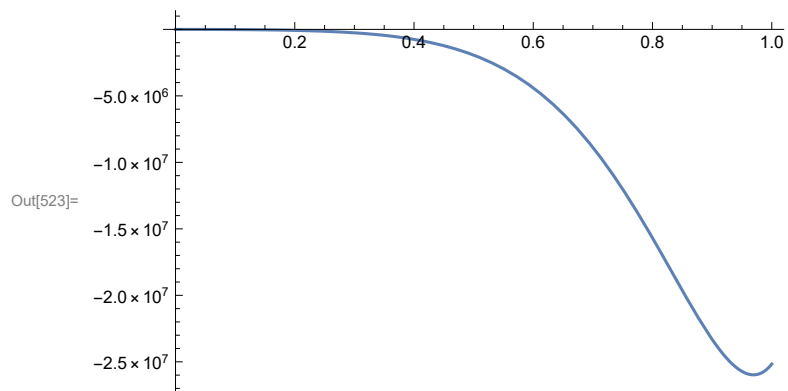

In[524]:= **Plot[Cf[11, 13, 4], {x, 0, 1}]**

[绘图](#)

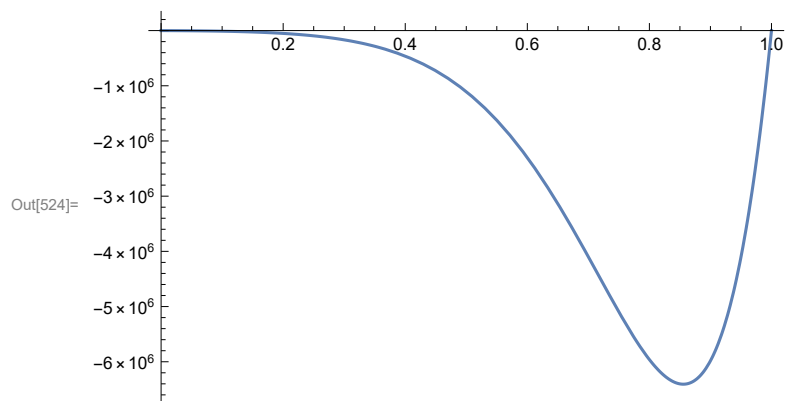

In[525]:= **Plot[Cf[11, 13, 3], {x, 0, 1}]**

[绘图](#)

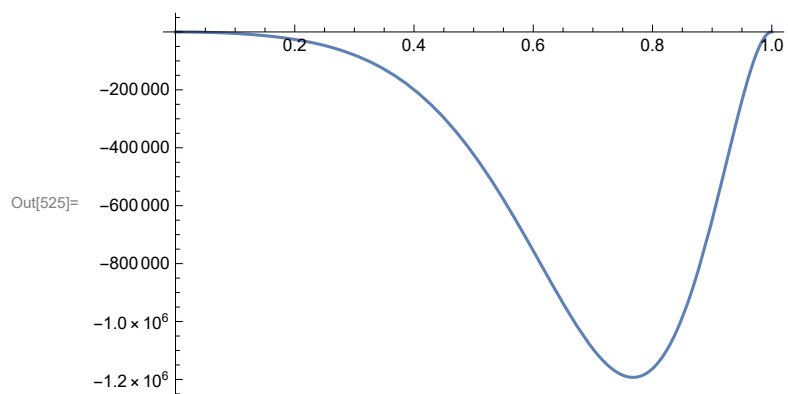

In[526]:= **Plot[Cf[11, 13, 2], {x, 0, 1}]**

[绘图](#)

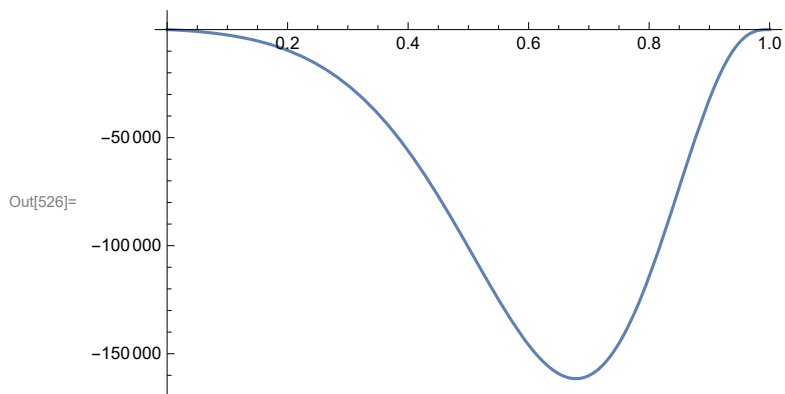

In[527]:= **Plot[Cf[11, 13, 1], {x, 0, 1}]**

[绘图](#)

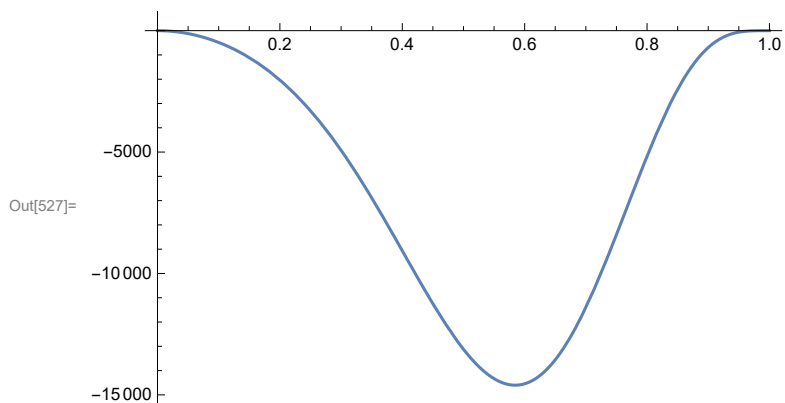

In[528]:= **Plot[Cf[11, 13, 0], {x, 0, 1}]**

[绘图](#)

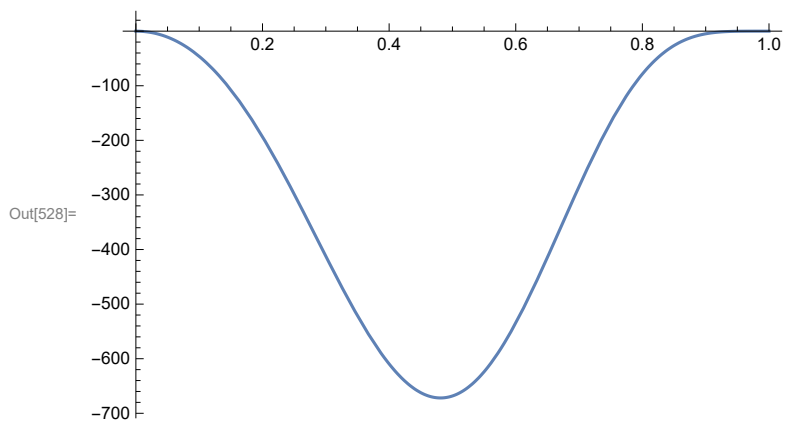

(\*48th group coefficients r2^11r3^12\*)

**Plot[Cf[11, 12, 14], {x, 0, 1}]**

[绘图](#)

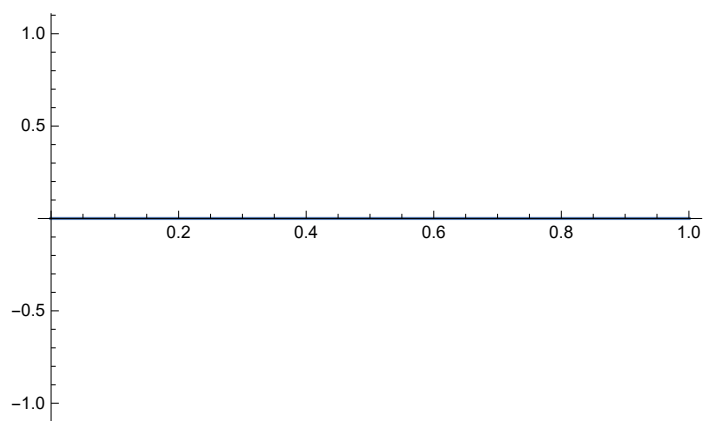

In[529]:= **Plot[Cf[11, 12, 13], {x, 0, 1}]**

[绘图](#)

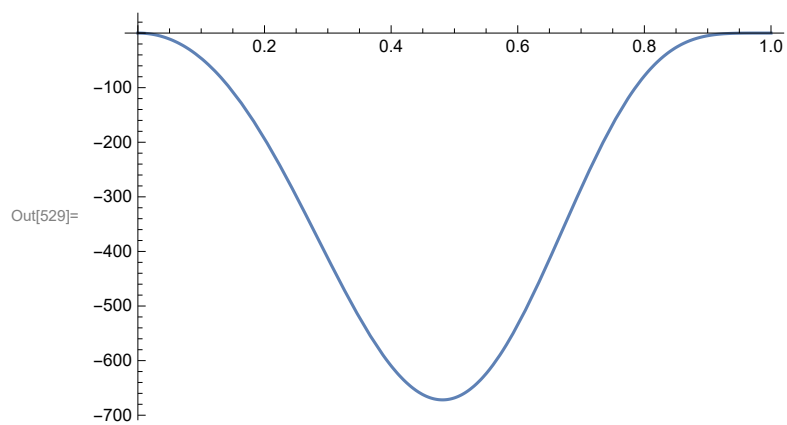

In[530]:= **Plot[Cf[11, 12, 12], {x, 0, 1}]**

[绘图](#)

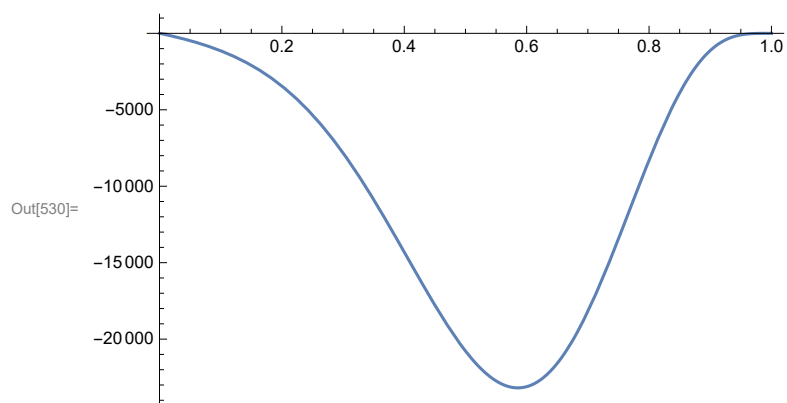



In[531]:= **Plot[Cf[11, 12, 11], {x, 0, 1}]**

[绘图](#)

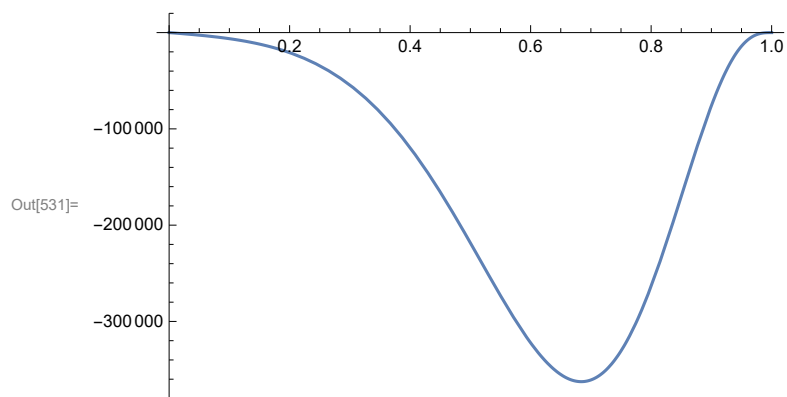

In[532]:= **Plot[Cf[11, 12, 10], {x, 0, 1}]**

[绘图](#)

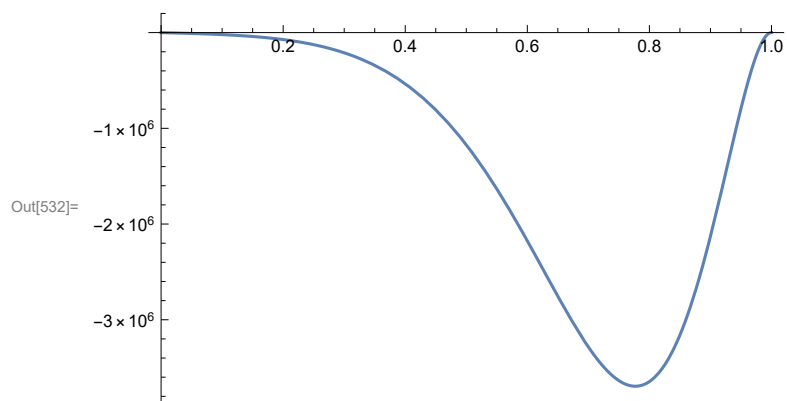

In[533]:= **Plot[Cf[11, 12, 9], {x, 0, 1}]**

[绘图](#)

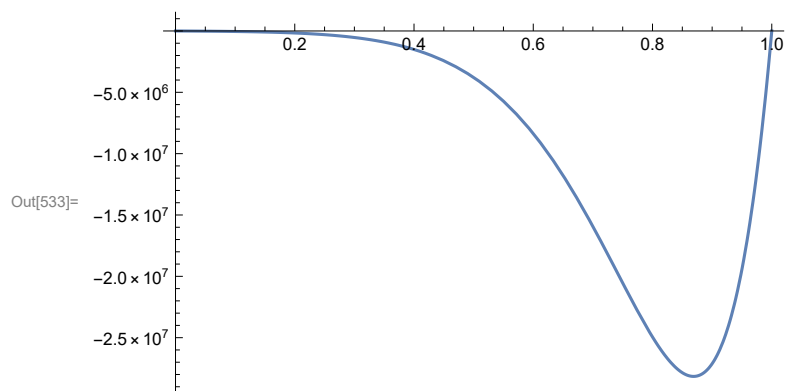

In[534]:= **Plot[Cf[11, 12, 8], {x, 0, 1}]**

[绘图](#)

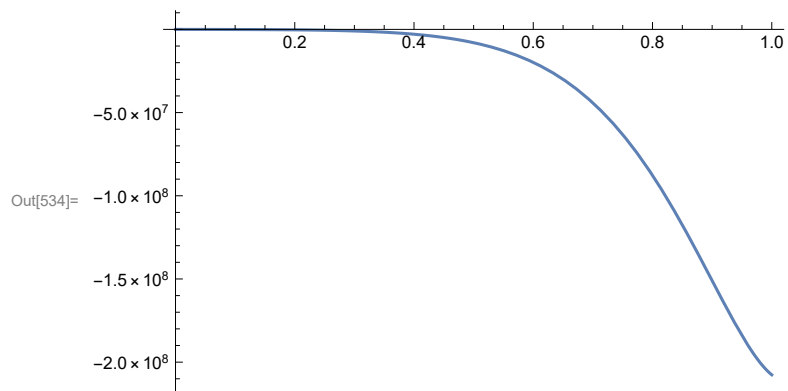

In[535]:= **Plot[Cf[11, 12, 7], {x, 0, 1}]**

[绘图](#)

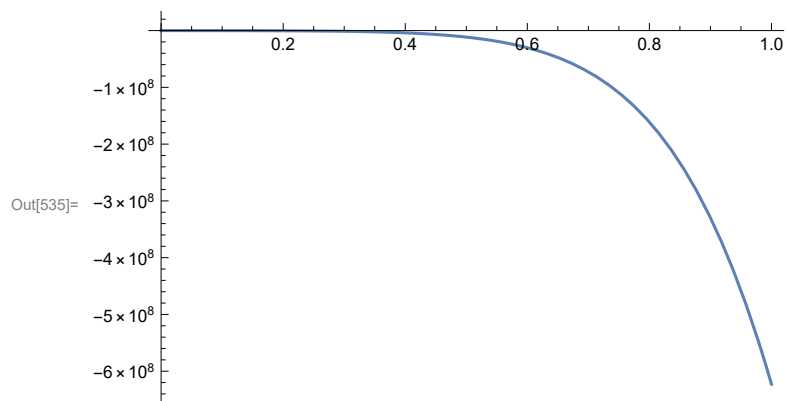

In[536]:= **Plot[Cf[11, 12, 6], {x, 0, 1}]**

[绘图](#)

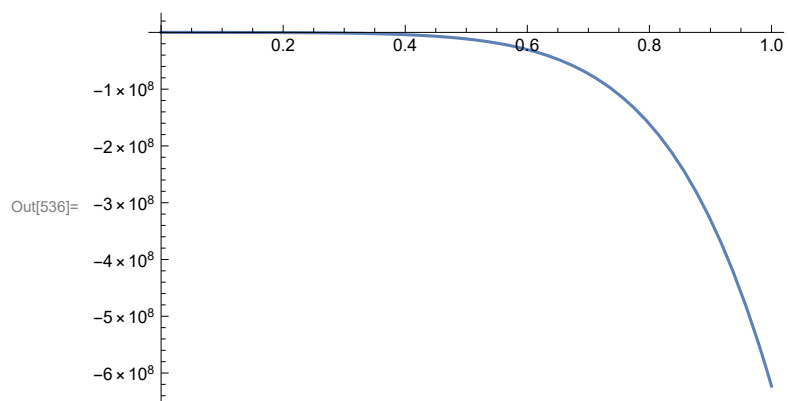

In[537]:= **Plot[Cf[11, 12, 5], {x, 0, 1}]**

[绘图](#)

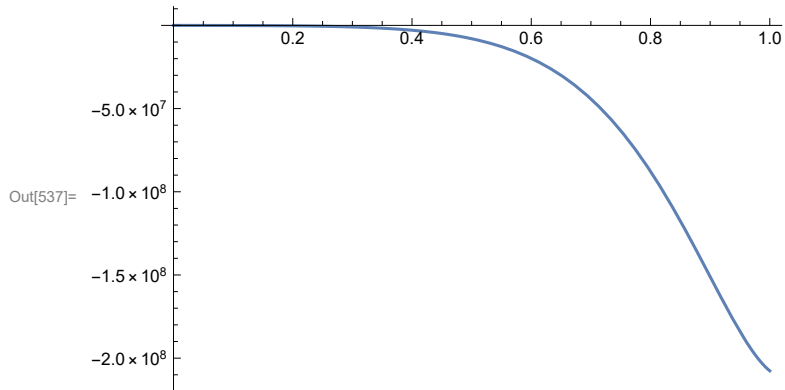

In[538]:= **Plot[Cf[11, 12, 4], {x, 0, 1}]**

[绘图](#)

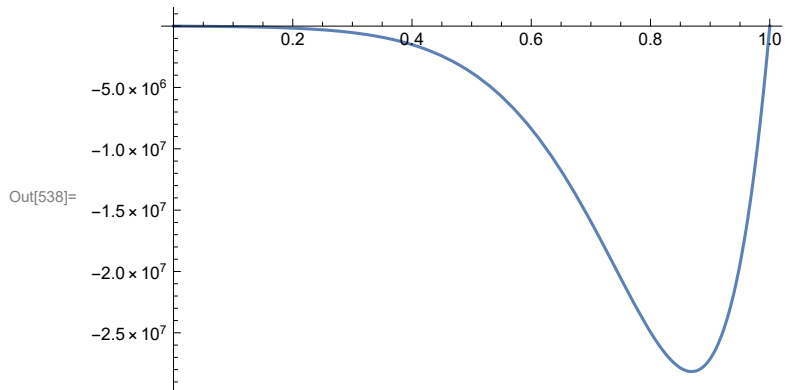

In[539]:= **Plot[Cf[11, 12, 3], {x, 0, 1}]**

[绘图](#)

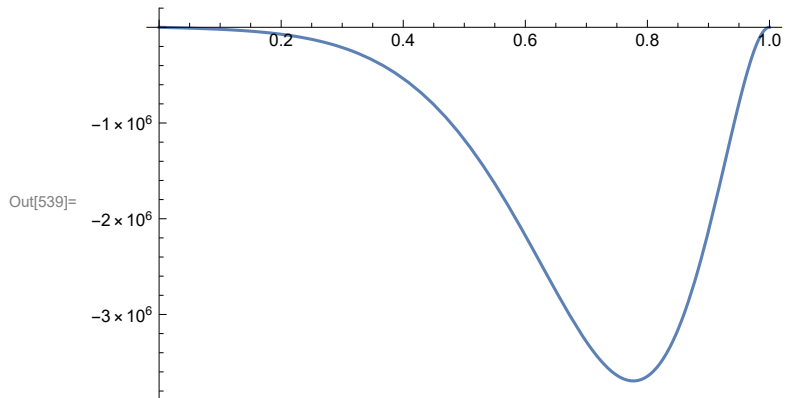

In[540]:= **Plot[Cf[11, 12, 2], {x, 0, 1}]**

[绘图](#)

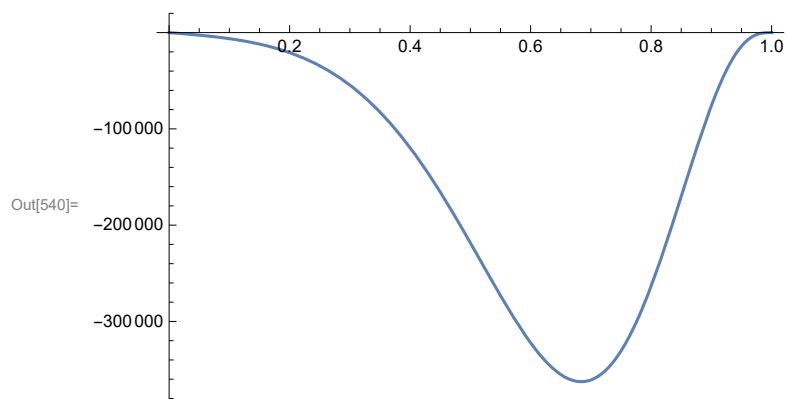

In[541]:= **Plot[Cf[11, 12, 1], {x, 0, 1}]**

[绘图](#)

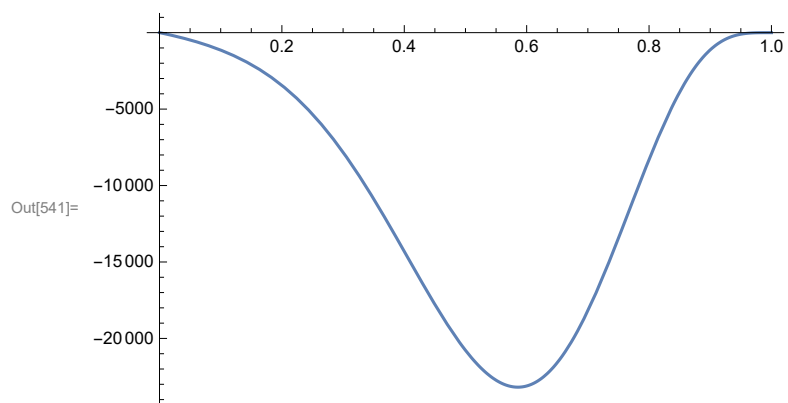

In[542]:= **Plot[Cf[11, 12, 0], {x, 0, 1}]**

[绘图](#)

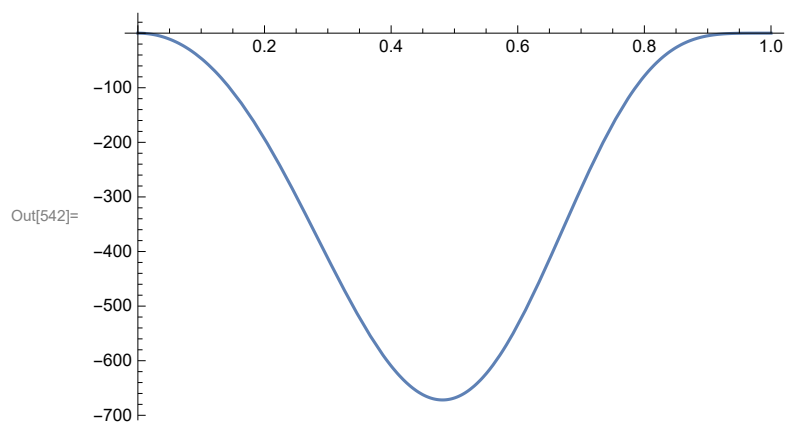

(\*49th group coefficients r2^11r3^11\*)

In[543]:= **Plot[Cf[11, 11, 14], {x, 0, 1}]**

[绘图](#)

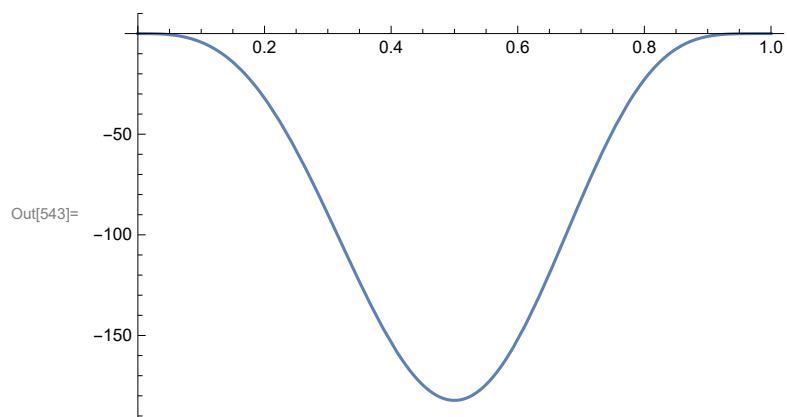

In[544]:= **Plot[Cf[11, 11, 13], {x, 0, 1}]**

[绘图](#)

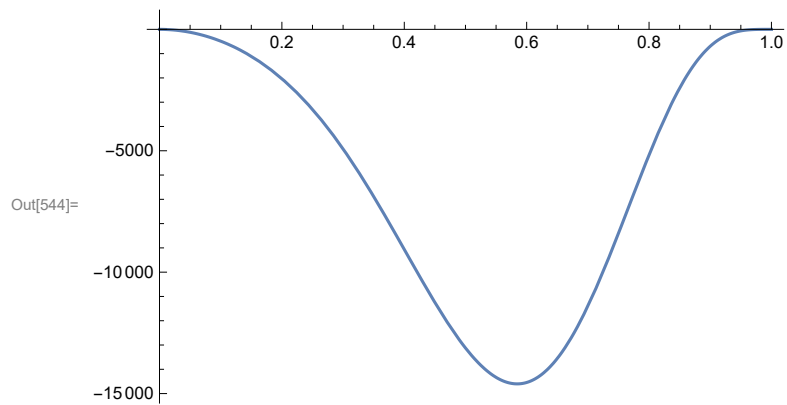

In[545]:= **Plot[Cf[11, 11, 12], {x, 0, 1}]**

[绘图](#)

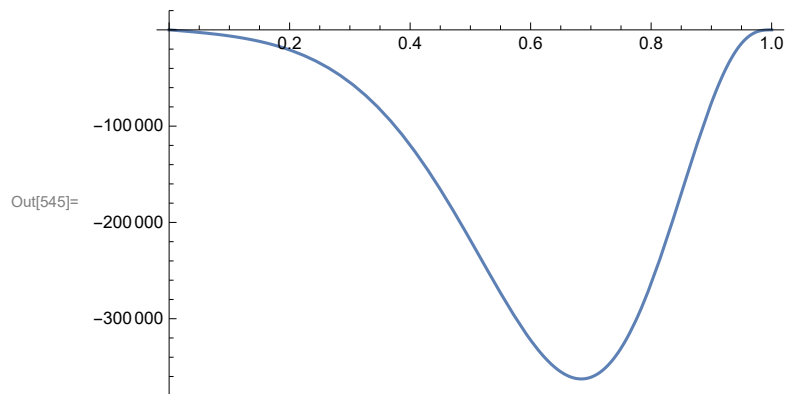

In[546]:= **Plot[Cf[11, 11, 11], {x, 0, 1}]**

[绘图](#)

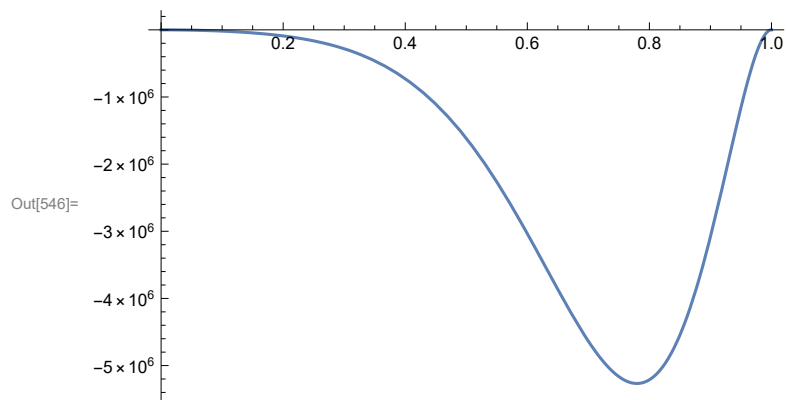

In[547]:= **Plot[Cf[11, 11, 10], {x, 0, 1}]**

[绘图](#)

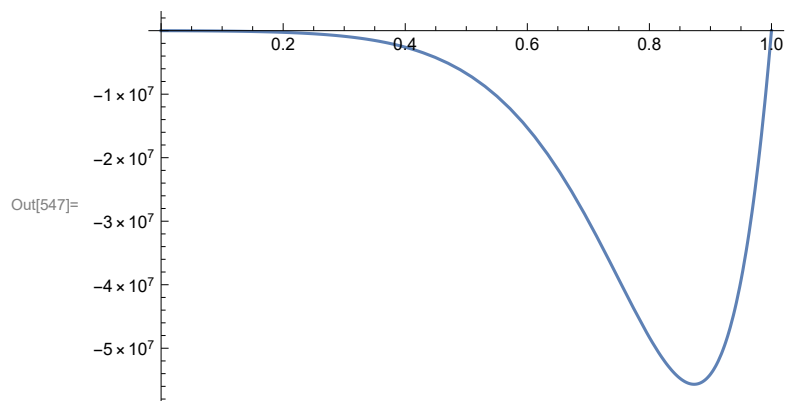

In[548]:= **Plot[Cf[11, 11, 9], {x, 0, 1}]**

[绘图](#)

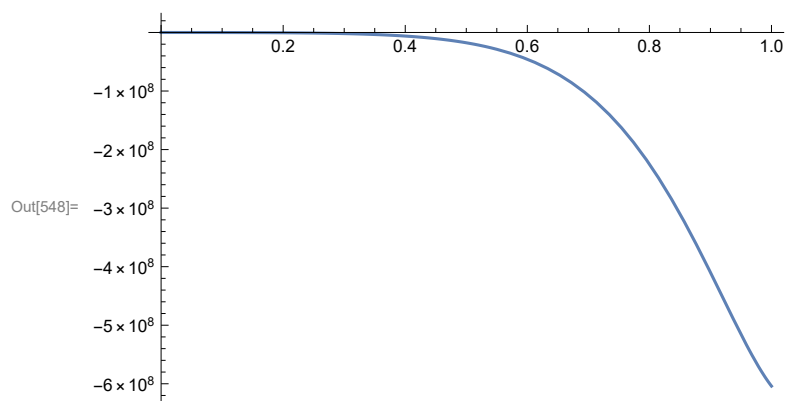

In[549]:= **Plot[Cf[11, 11, 8], {x, 0, 1}]**

[绘图](#)

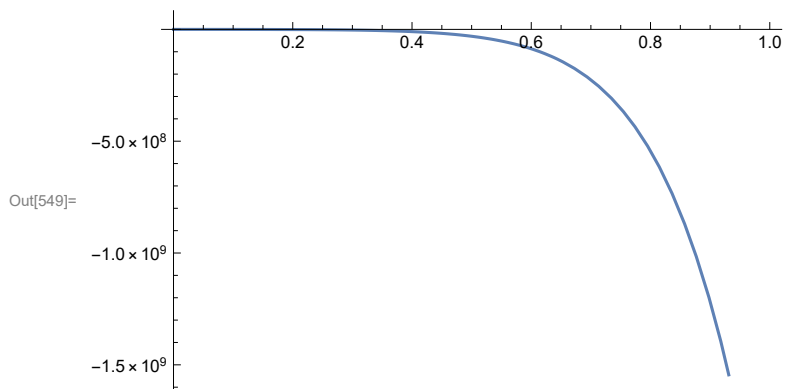

In[550]:= **Plot[Cf[11, 11, 7], {x, 0, 1}]**

[绘图](#)

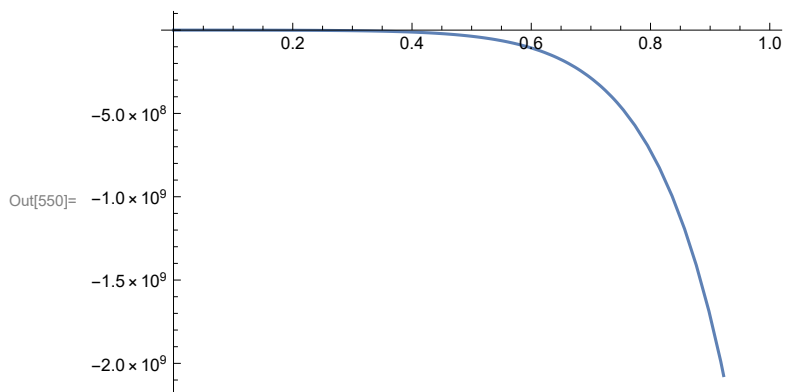

In[551]:= **Plot[Cf[11, 11, 6], {x, 0, 1}]**

[绘图](#)

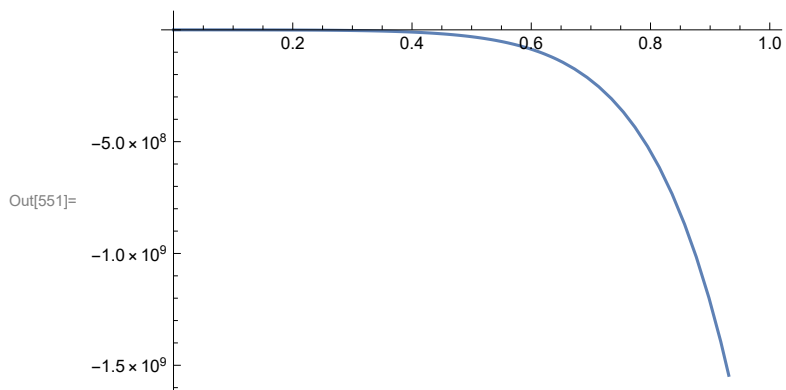

In[552]:= **Plot**[**Cf**[11, 11, 5], {x, 0, 1}]

[绘图](#)

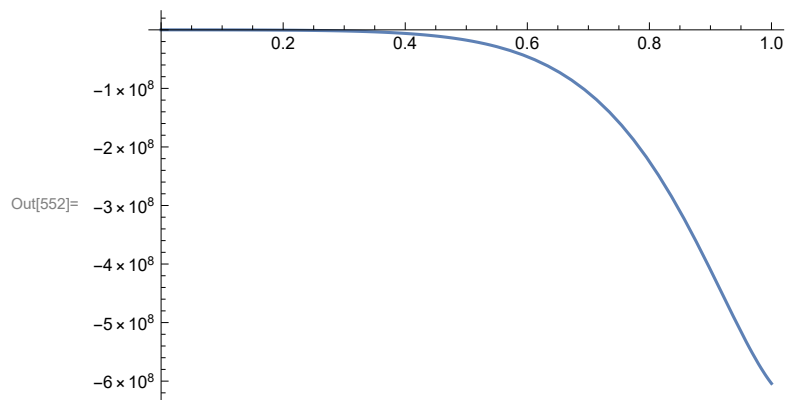

In[553]:= **Plot**[**Cf**[11, 11, 4], {x, 0, 1}]

[绘图](#)

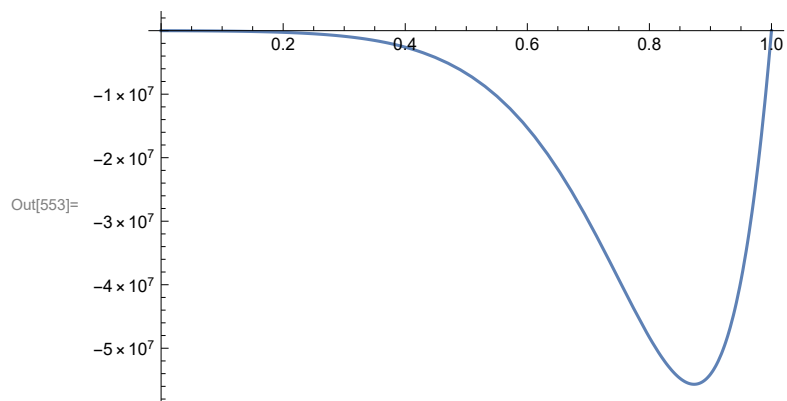

In[554]:= **Plot**[**Cf**[11, 11, 3], {x, 0, 1}]

[绘图](#)

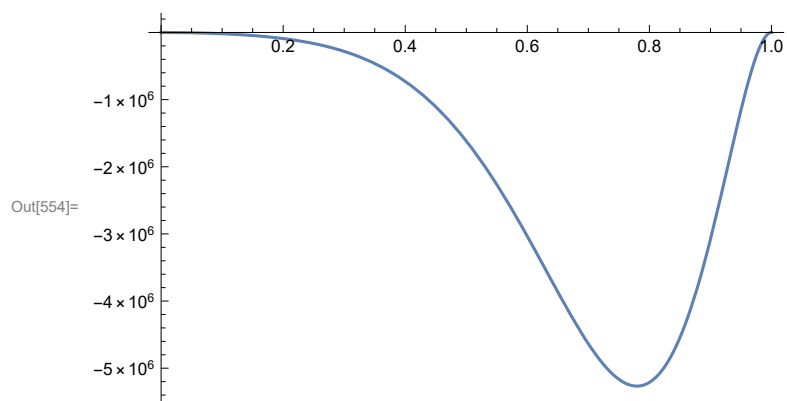



In[555]:= **Plot[Cf[11, 11, 2], {x, 0, 1}]**

[绘图](#)

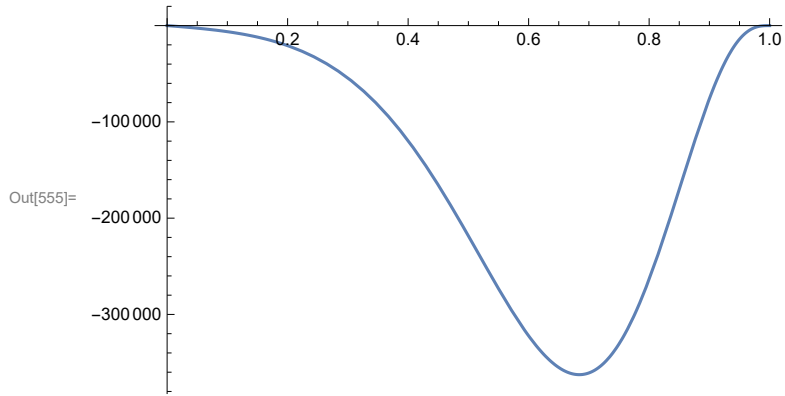

In[556]:= **Plot[Cf[11, 11, 1], {x, 0, 1}]**

[绘图](#)

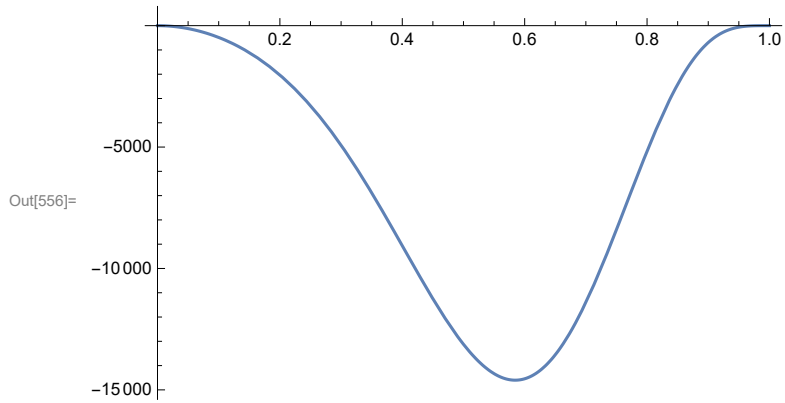

In[557]:= **Plot[Cf[11, 11, 0], {x, 0, 1}]**

[绘图](#)

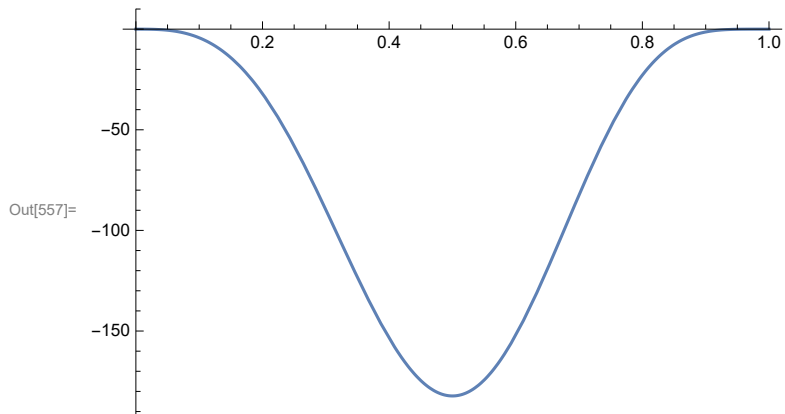

(\*50th group coefficients r2^11r3^10\*)

In[558]:= **Plot[Cf[11, 10, 14], {x, 0, 1}]**

[绘图](#)

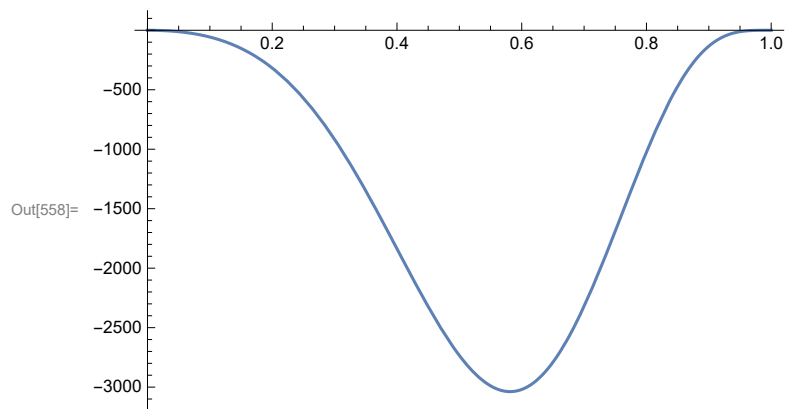

In[559]:= **Plot[Cf[11, 10, 13], {x, 0, 1}]**

[绘图](#)

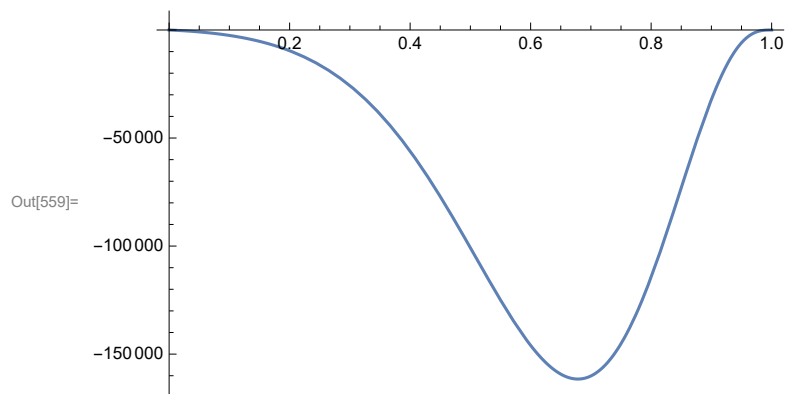

In[560]:= **Plot[Cf[11, 10, 12], {x, 0, 1}]**

[绘图](#)

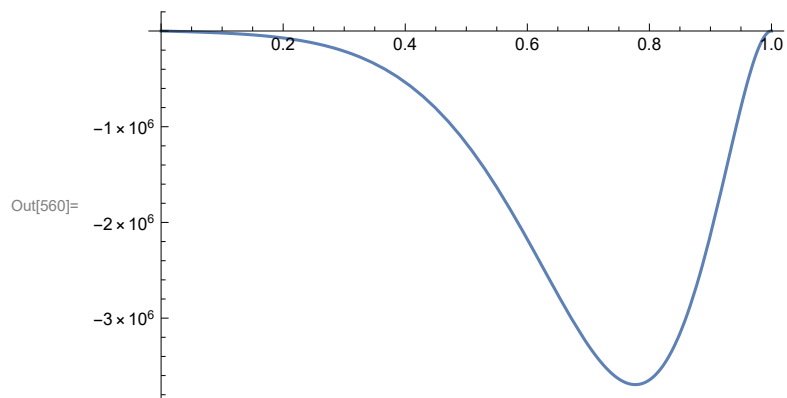

In[561]:= **Plot[Cf[11, 10, 11], {x, 0, 1}]**

[绘图](#)

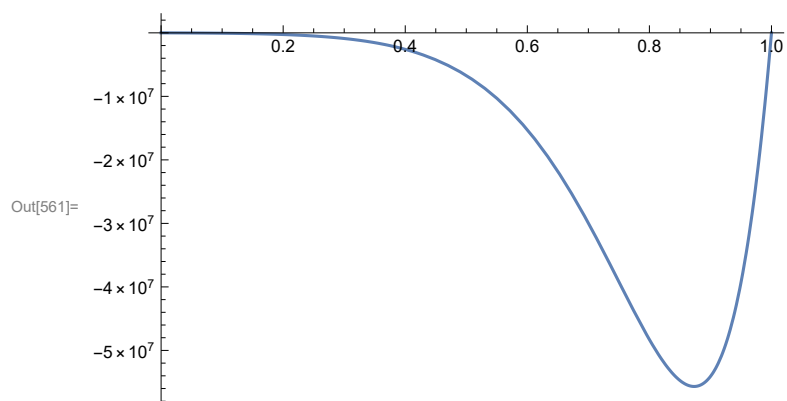

In[562]:= **Plot[Cf[11, 10, 10], {x, 0, 1}]**

[绘图](#)

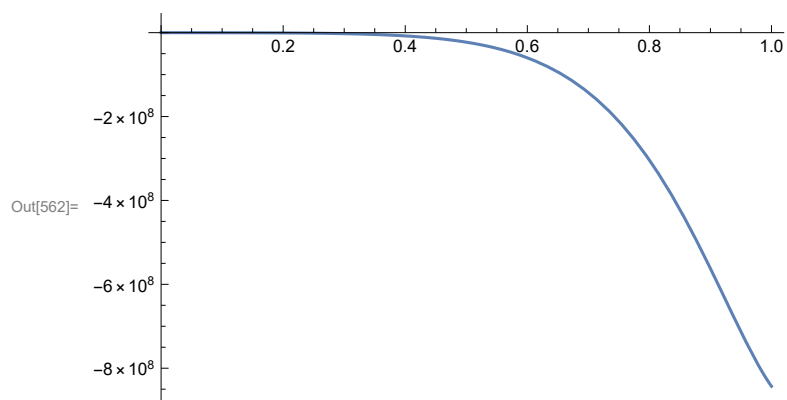

In[563]:= **Plot[Cf[11, 10, 9], {x, 0, 1}]**

[绘图](#)

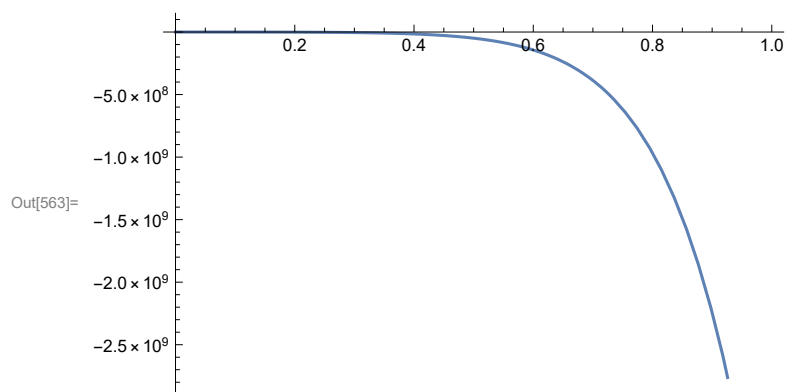

In[564]:= **Plot[Cf[11, 10, 8], {x, 0, 1}]**

[绘图](#)

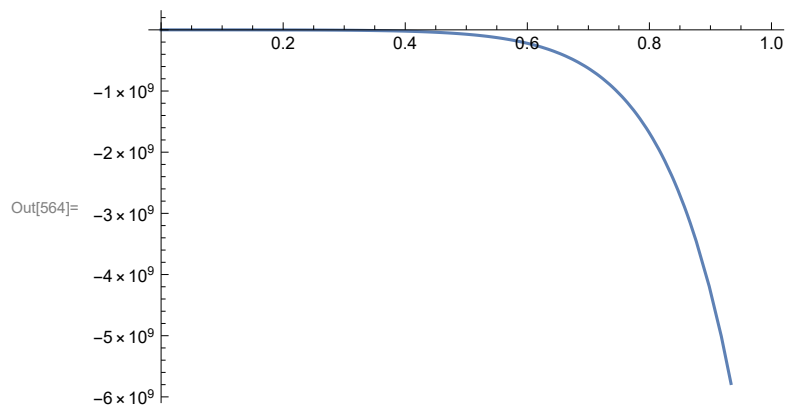

In[565]:= **Plot[Cf[11, 10, 7], {x, 0, 1}]**

[绘图](#)

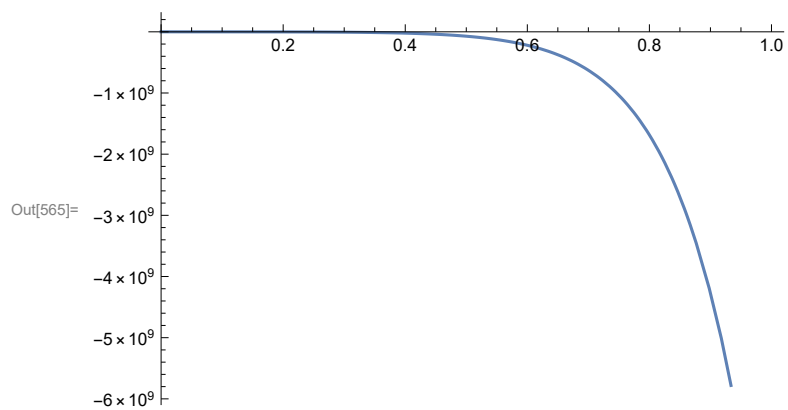

In[566]:= **Plot[Cf[11, 10, 6], {x, 0, 1}]**

[绘图](#)

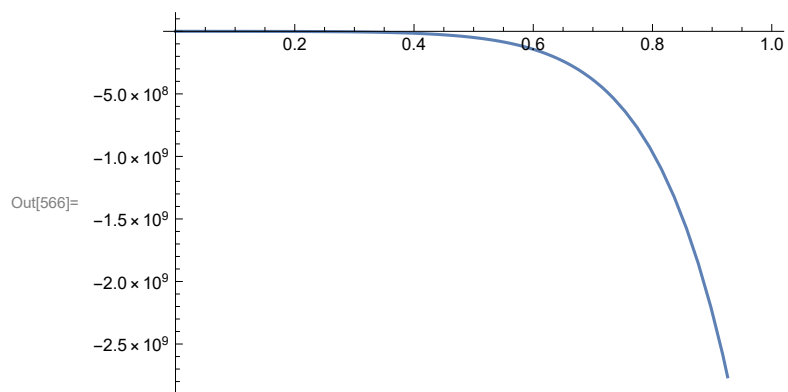

In[567]:= **Plot[Cf[11, 10, 5], {x, 0, 1}]**

[绘图](#)

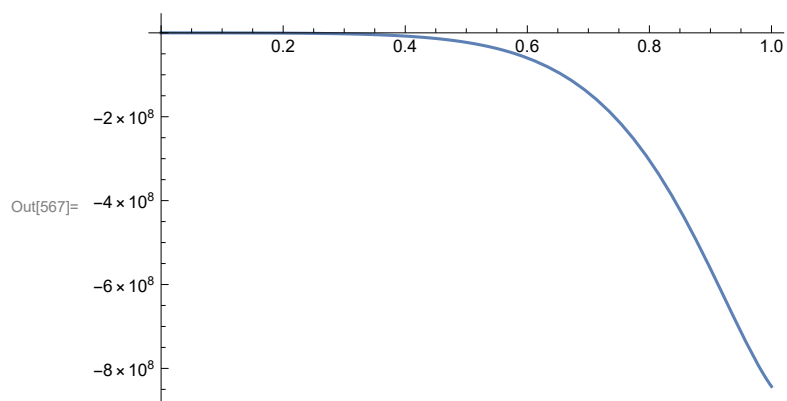

In[568]:= **Plot[Cf[11, 10, 4], {x, 0, 1}]**

[绘图](#)

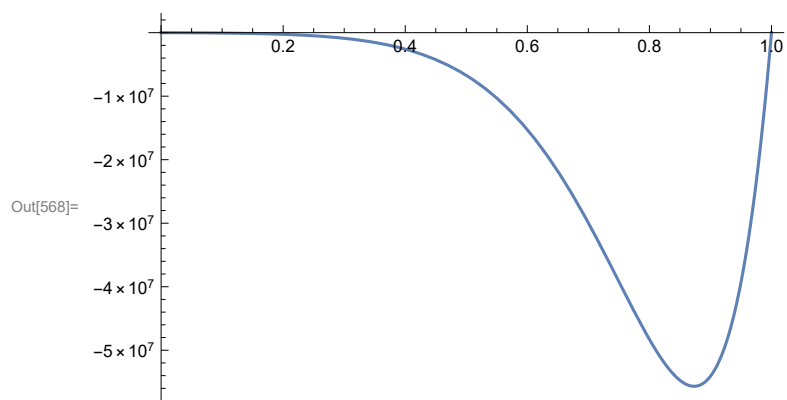

In[569]:= **Plot[Cf[11, 10, 3], {x, 0, 1}]**

[绘图](#)

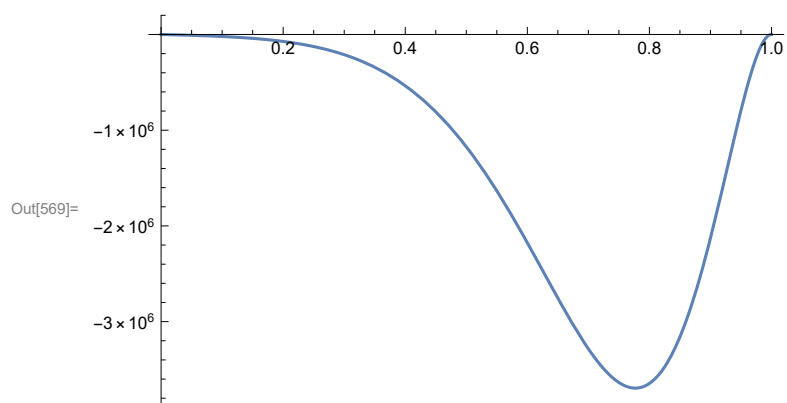

In[570]:= **Plot[Cf[11, 10, 2], {x, 0, 1}]**

[绘图](#)

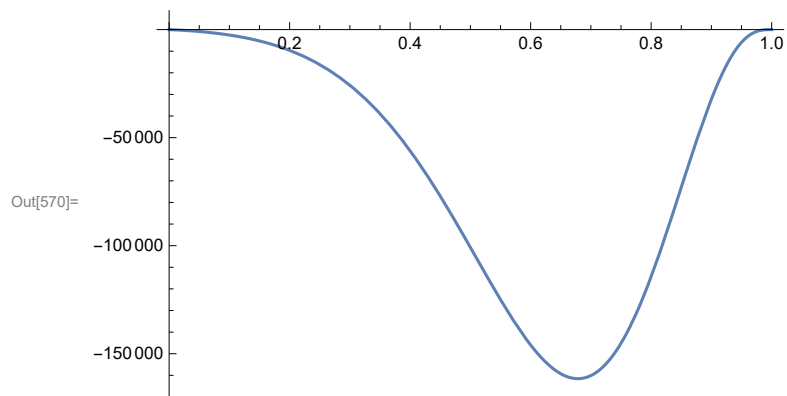

In[571]:= **Plot[Cf[11, 10, 1], {x, 0, 1}]**

[绘图](#)

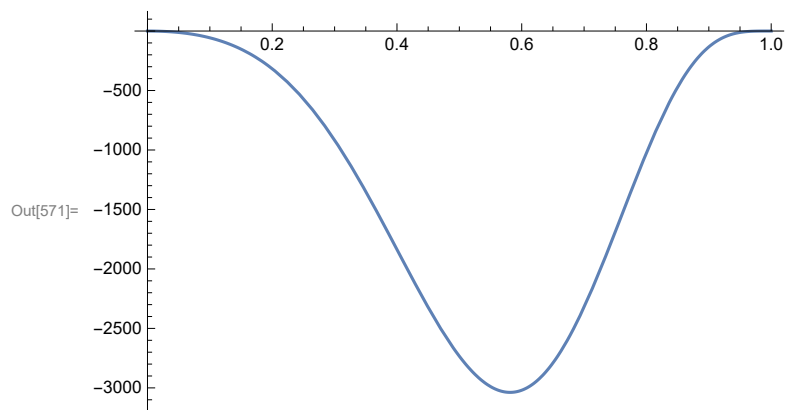

**Plot[Cf[11, 10, 0], {x, 0, 1}]**

[绘图](#)

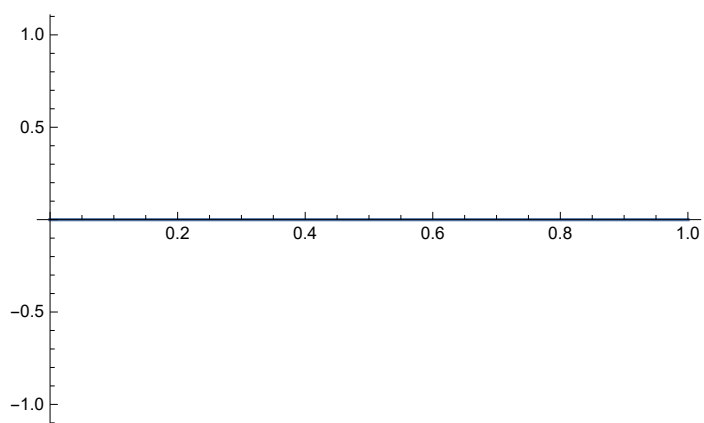

(\*51th group coefficients r2^11r3^9\*)

In[572]:= **Plot[Cf[11, 9, 14], {x, 0, 1}]**

[绘图](#)

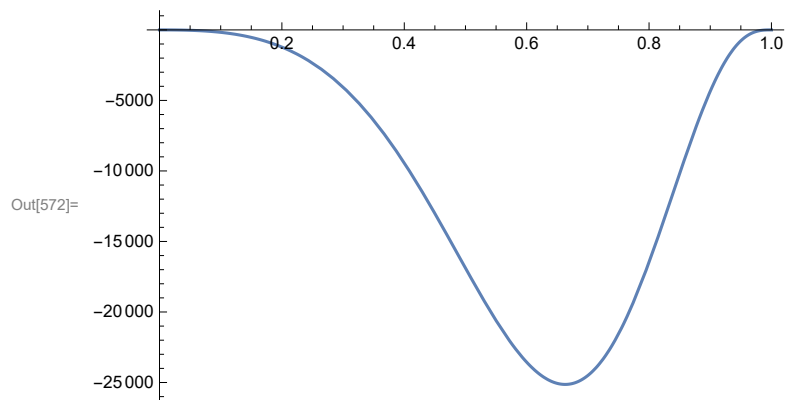

In[573]:= **Plot[Cf[11, 9, 13], {x, 0, 1}]**

[绘图](#)

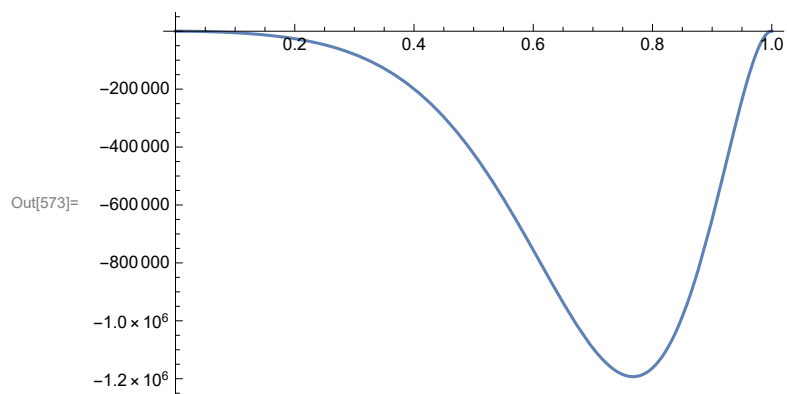

In[574]:= **Plot[Cf[11, 9, 13], {x, 0, 1}]**

[绘图](#)

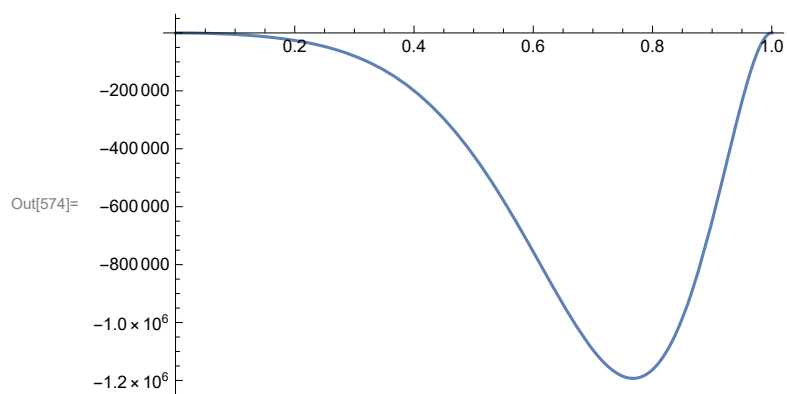

In[575]:= **Plot[Cf[11, 9, 12], {x, 0, 1}]**

[绘图](#)

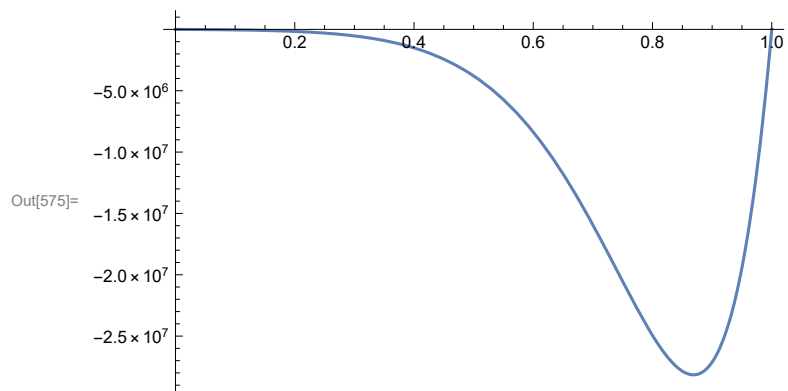

In[576]:= **Plot[Cf[11, 9, 11], {x, 0, 1}]**

[绘图](#)

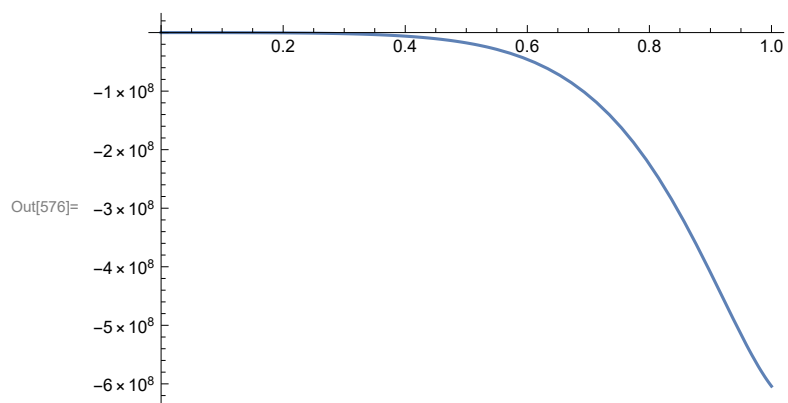

In[577]:= **Plot[Cf[11, 9, 11], {x, 0, 1}]**

[绘图](#)

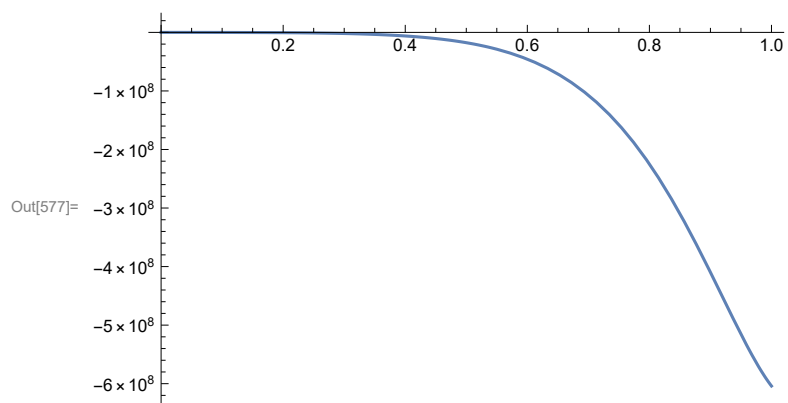



In[578]:= **Plot[Cf[11, 9, 10], {x, 0, 1}]**

[绘图](#)

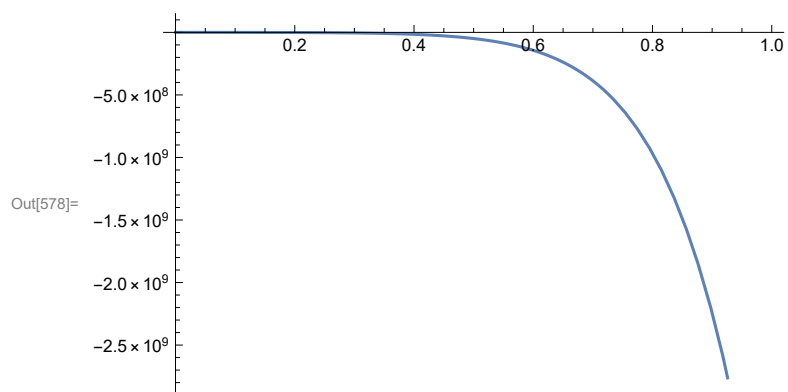

In[579]:= **Plot[Cf[11, 9, 9], {x, 0, 1}]**

[绘图](#)

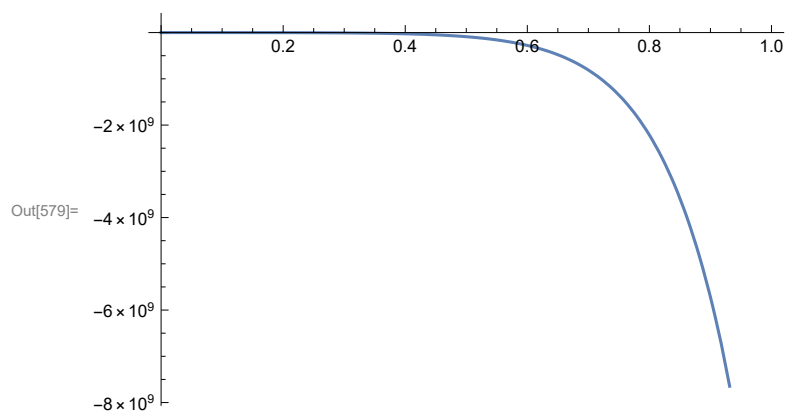

In[580]:= **Plot[Cf[11, 9, 8], {x, 0, 1}]**

[绘图](#)

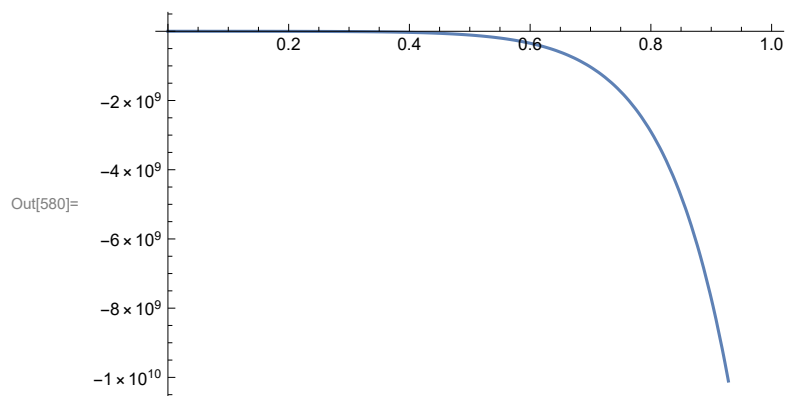

In[581]:= **Plot[Cf[11, 9, 7], {x, 0, 1}]**

[绘图](#)

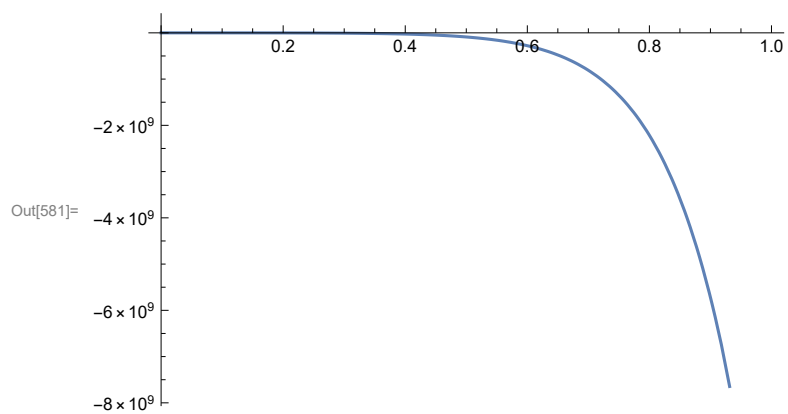

In[582]:= **Plot[Cf[11, 9, 6], {x, 0, 1}]**

[绘图](#)

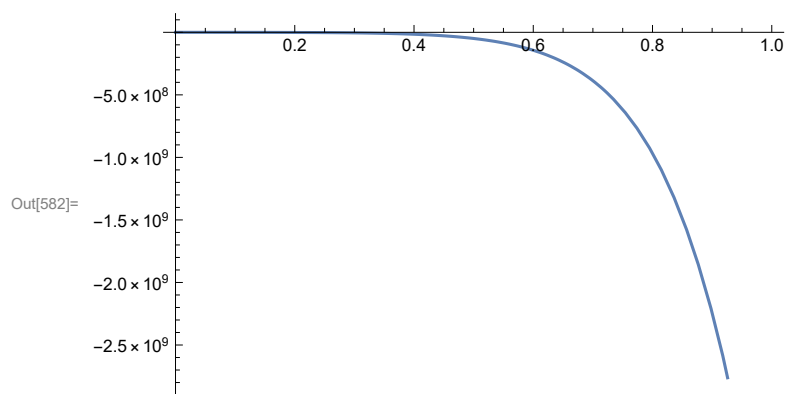

In[583]:= **Plot[Cf[11, 9, 5], {x, 0, 1}]**

[绘图](#)

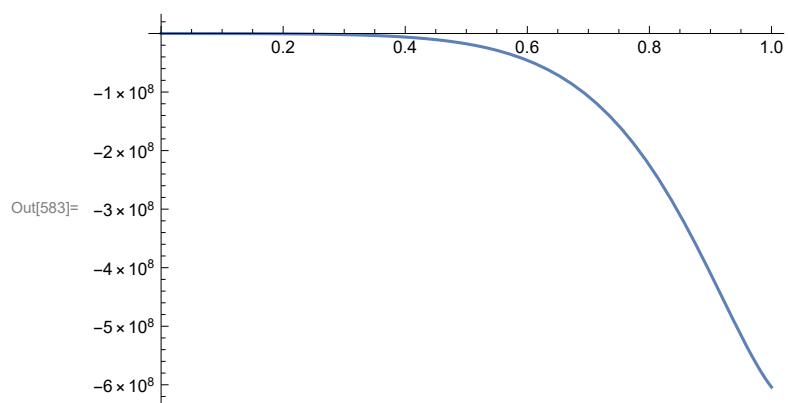

In[584]:= **Plot[Cf[11, 9, 4], {x, 0, 1}]**

[绘图](#)

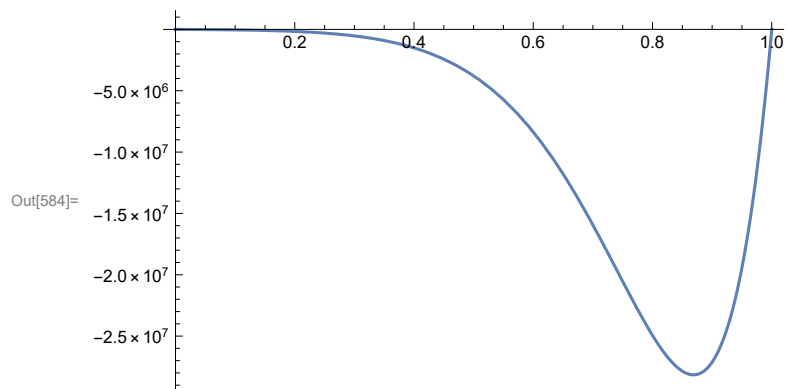

In[585]:= **Plot[Cf[11, 9, 3], {x, 0, 1}]**

[绘图](#)

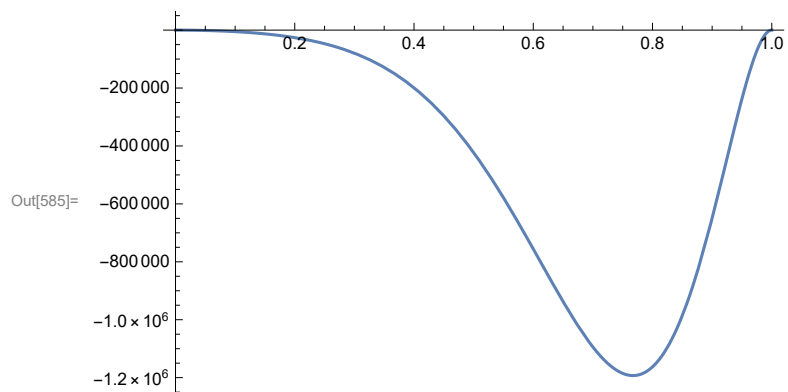

In[586]:= **Plot[Cf[11, 9, 2], {x, 0, 1}]**

[绘图](#)

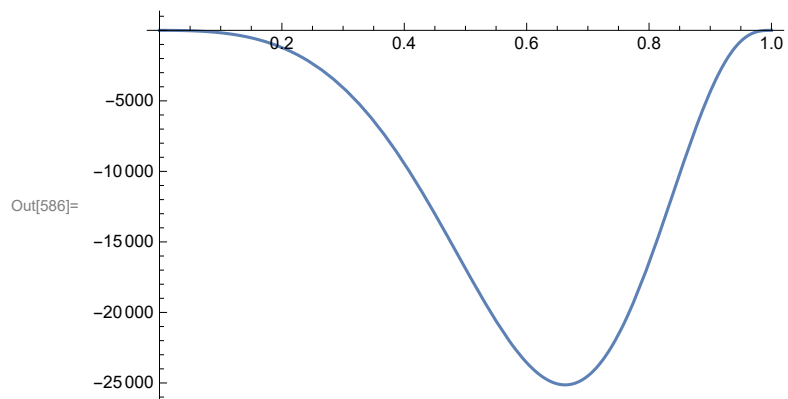

**Plot[Cf[11, 9, 1], {x, 0, 1}]**

[绘图](#)

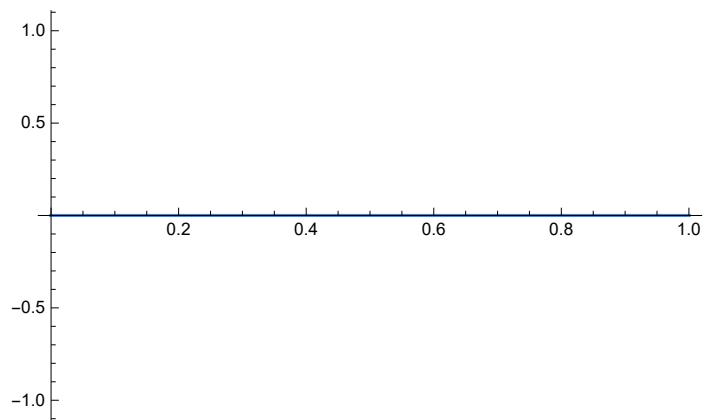

**Plot[Cf[11, 9, 0], {x, 0, 1}]**

[绘图](#)

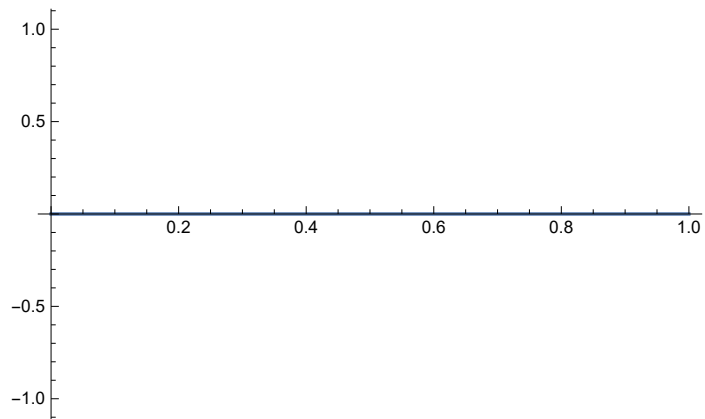

**(\*52th group coefficients r2^11r3^8\*)**

In[587]:= **Plot[Cf[11, 8, 14], {x, 0, 1}]**

[绘图](#)

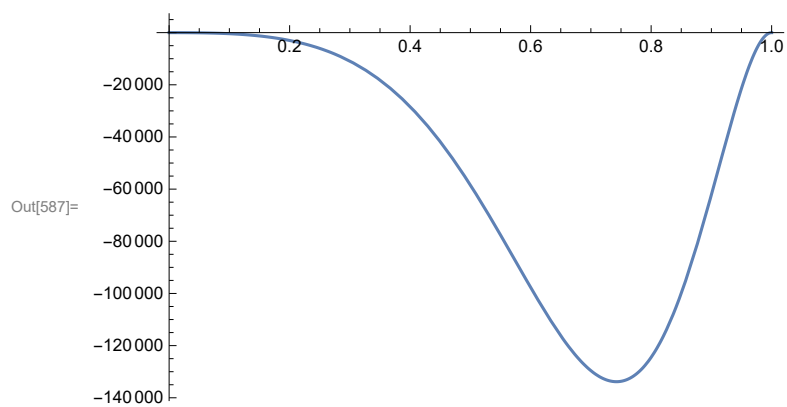

In[588]:= **Plot[Cf[11, 8, 13], {x, 0, 1}]**

[绘图](#)

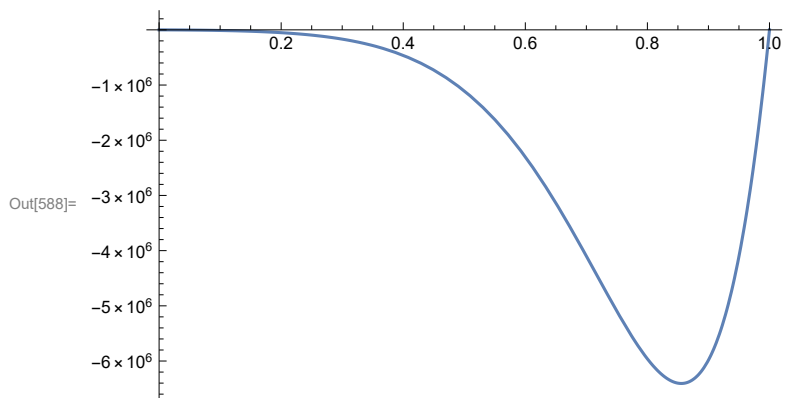

In[589]:= **Plot[Cf[11, 8, 12], {x, 0, 1}]**

[绘图](#)

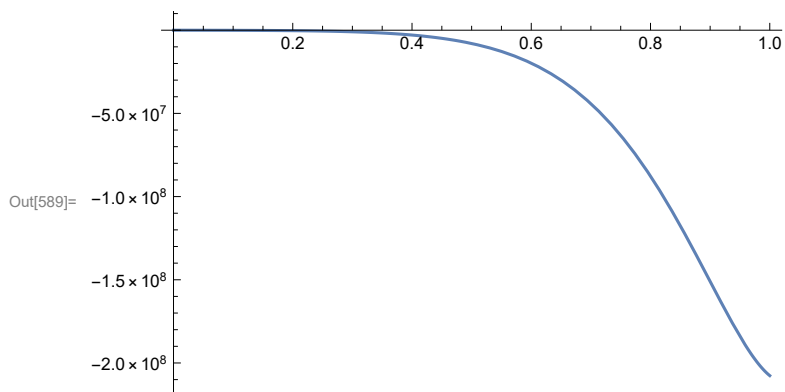

In[590]:= **Plot[Cf[11, 8, 11], {x, 0, 1}]**

[绘图](#)

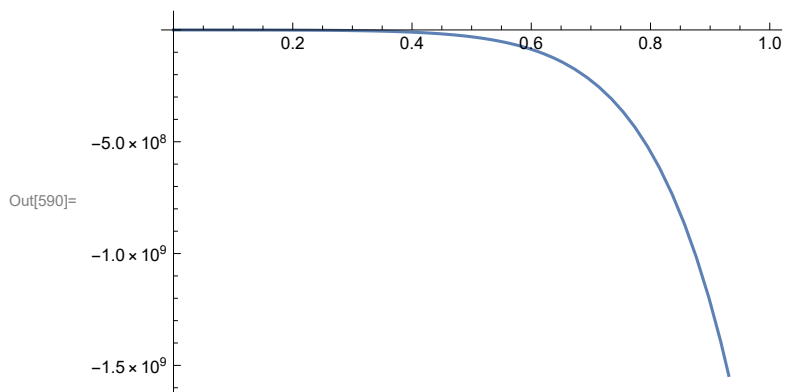

In[591]:= **Plot[Cf[11, 8, 10], {x, 0, 1}]**

[绘图](#)

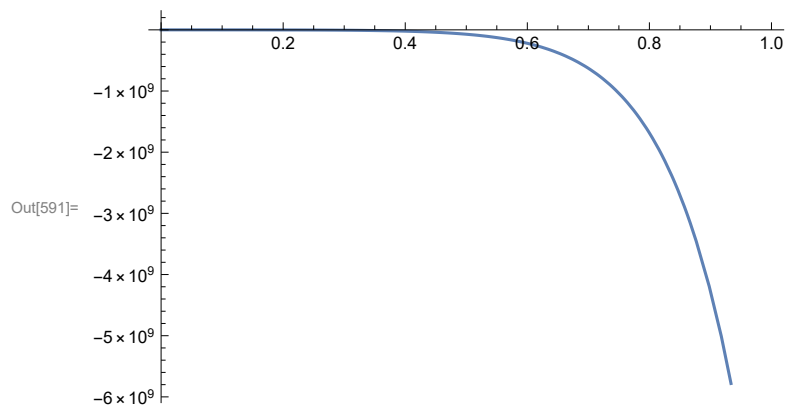

In[592]:= **Plot[Cf[11, 8, 9], {x, 0, 1}]**

[绘图](#)

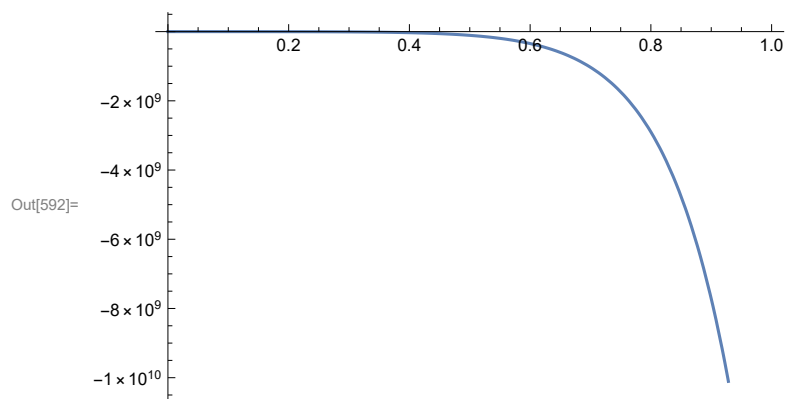

In[593]:= **Plot[Cf[11, 8, 8], {x, 0, 1}]**

[绘图](#)

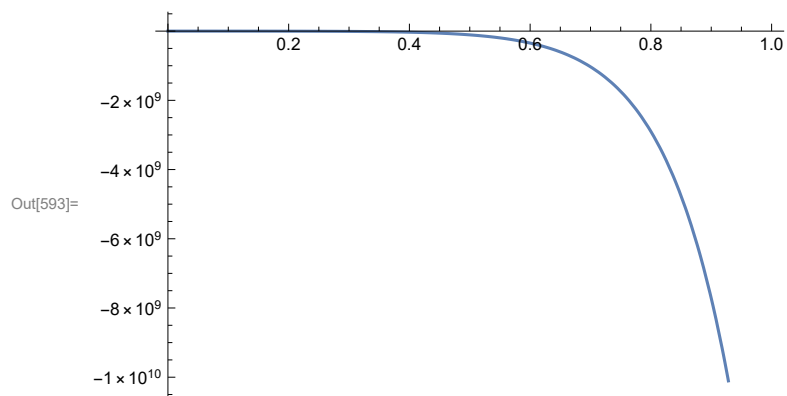

In[594]:= **Plot[Cf[11, 8, 7], {x, 0, 1}]**

[绘图](#)

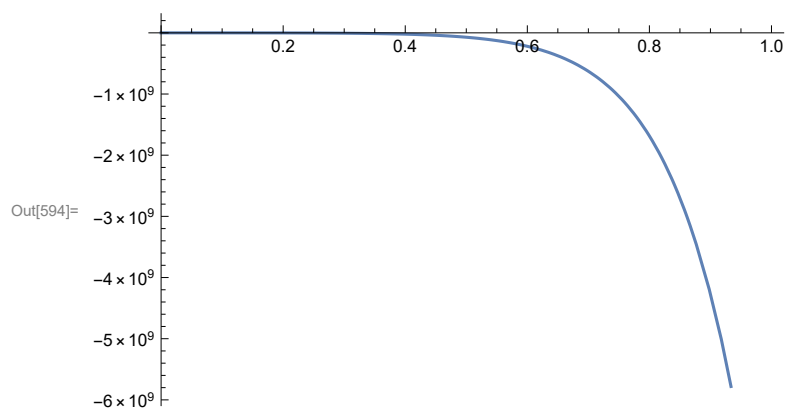

In[595]:= **Plot[Cf[11, 8, 6], {x, 0, 1}]**

[绘图](#)

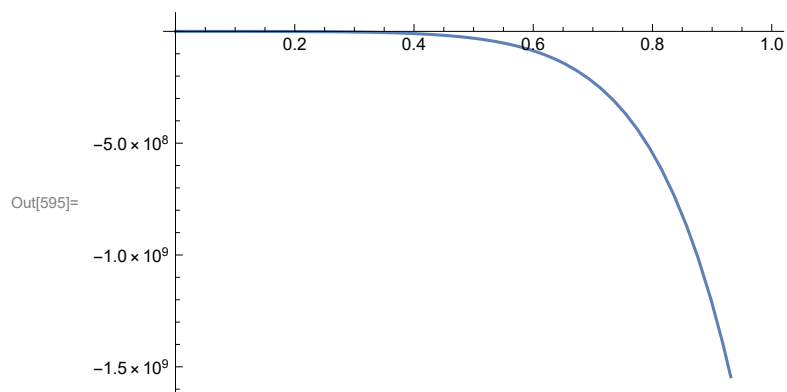

In[596]:= **Plot[Cf[11, 8, 5], {x, 0, 1}]**

[绘图](#)

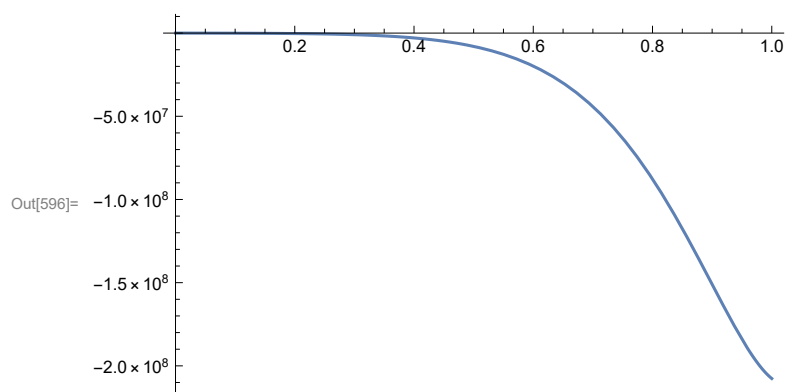

In[597]:= **Plot[Cf[11, 8, 4], {x, 0, 1}]**

[绘图](#)

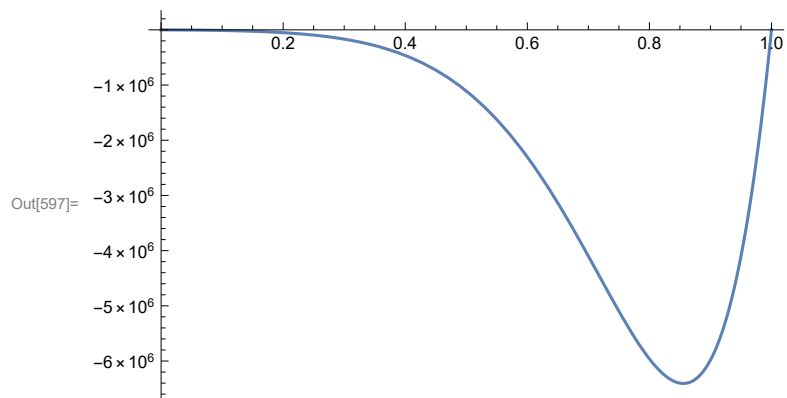

In[598]:= **Plot[Cf[11, 8, 3], {x, 0, 1}]**

[绘图](#)

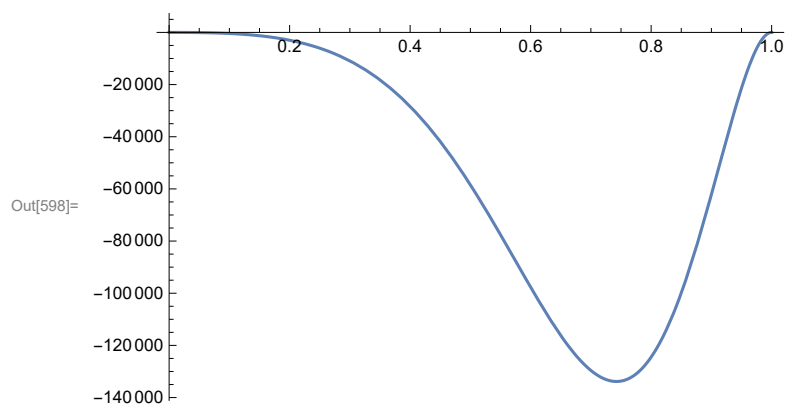

**Plot[Cf[11, 8, 2], {x, 0, 1}]**

[绘图](#)

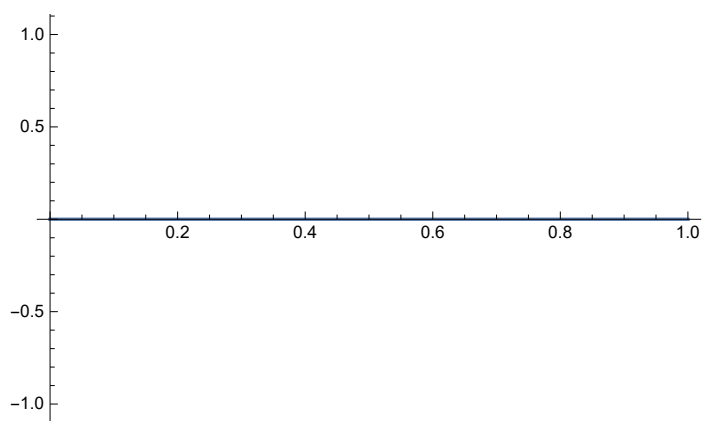



**Plot[Cf[11, 8, 1], {x, 0, 1}]**

[绘图](#)

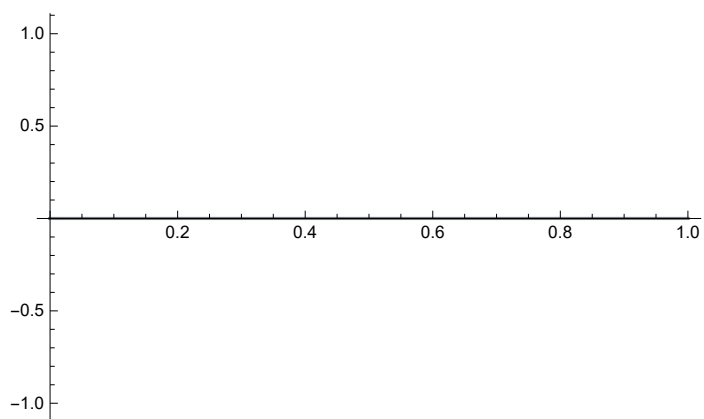

**Plot[Cf[11, 8, 0], {x, 0, 1}]**

[绘图](#)

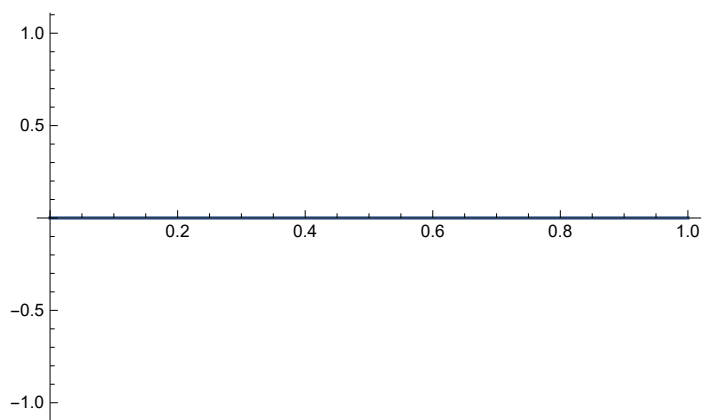

(\*53th group coefficients r2^11r3^7\*)

**Plot[Cf[11, 7, 14], {x, 0, 1}]**

[绘图](#)

In[599]:= **Plot[Cf[11, 7, 13], {x, 0, 1}]**

[绘图](#)

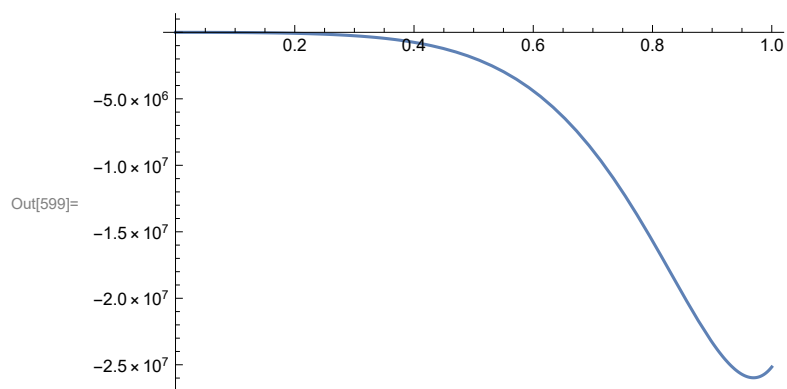

In[600]:= **Plot[Cf[11, 7, 12], {x, 0, 1}]**

[绘图](#)

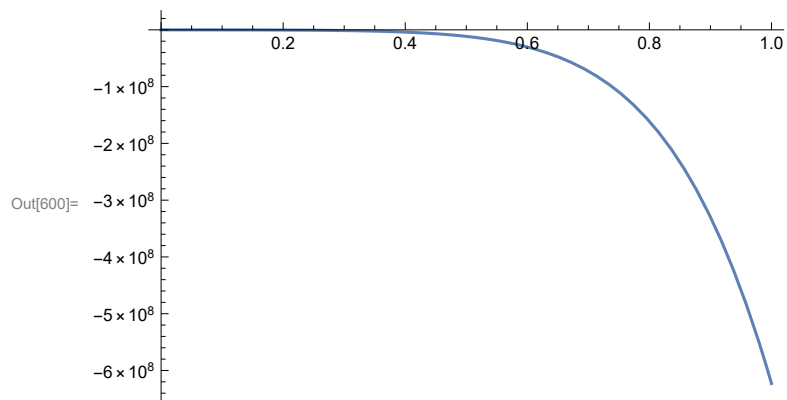

In[601]:= **Plot[Cf[11, 7, 11], {x, 0, 1}]**

[绘图](#)

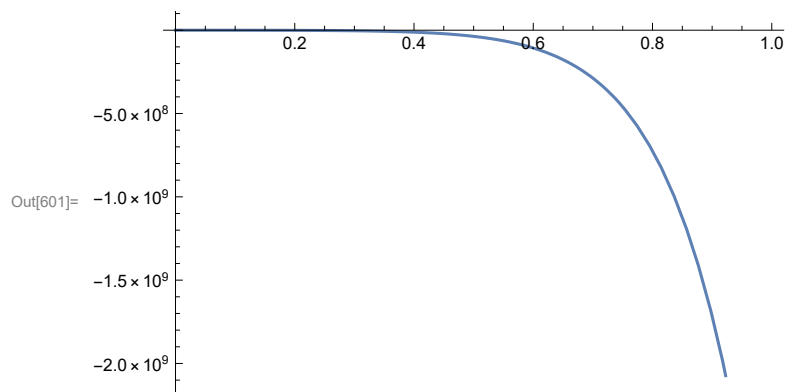

In[602]:= **Plot[Cf[11, 7, 10], {x, 0, 1}]**

[绘图](#)

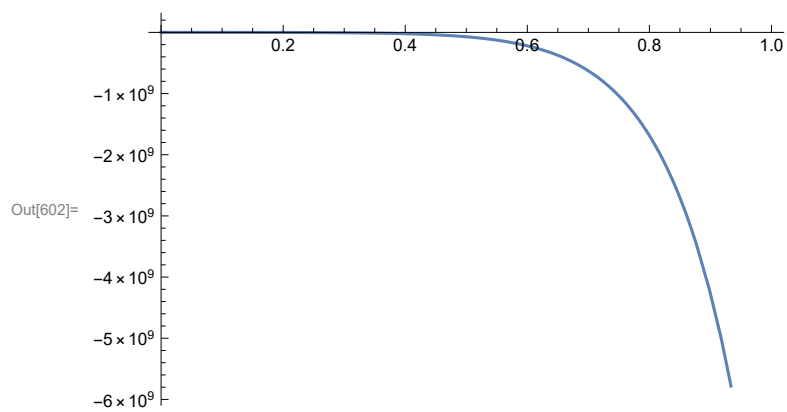

In[603]:= **Plot**[**Cf**[11, 7, 9], {x, 0, 1}]

[绘图](#)

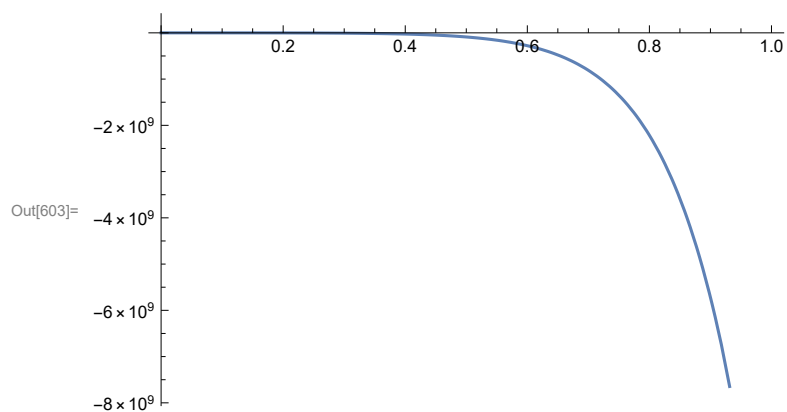

In[604]:= **Plot**[**Cf**[11, 7, 8], {x, 0, 1}]

[绘图](#)

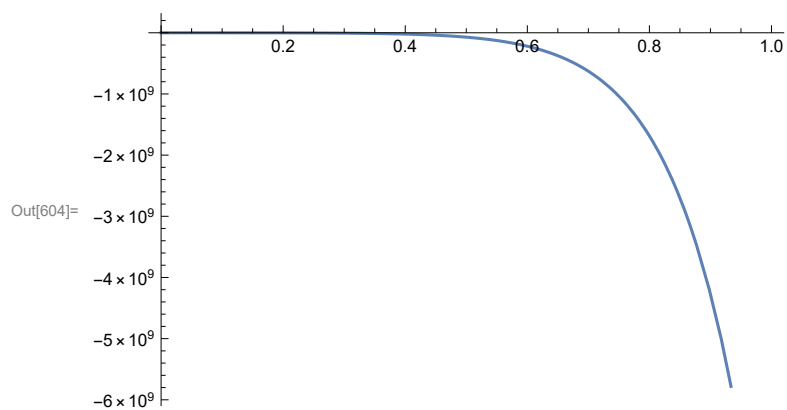

In[605]:= **Plot**[**Cf**[11, 7, 7], {x, 0, 1}]

[绘图](#)

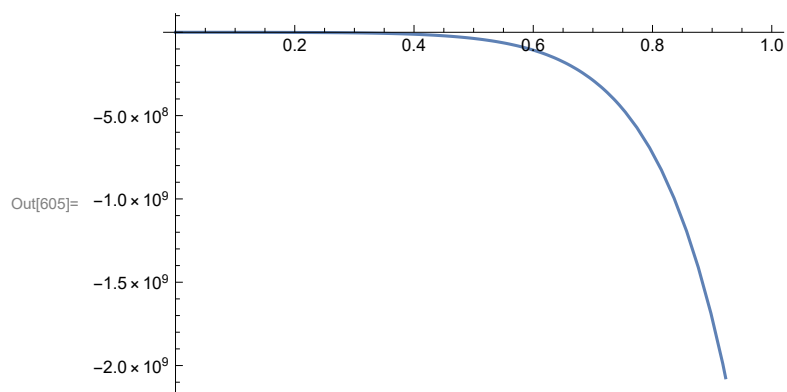

In[606]:= **Plot[Cf[11, 7, 6], {x, 0, 1}]**

[绘图](#)

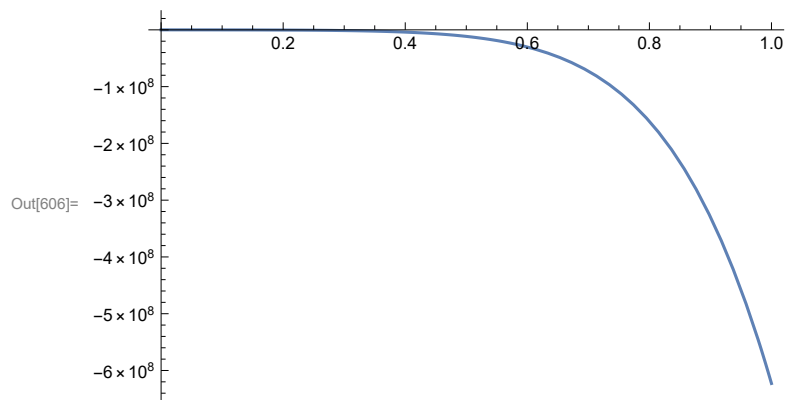

In[607]:= **Plot[Cf[11, 7, 5], {x, 0, 1}]**

[绘图](#)

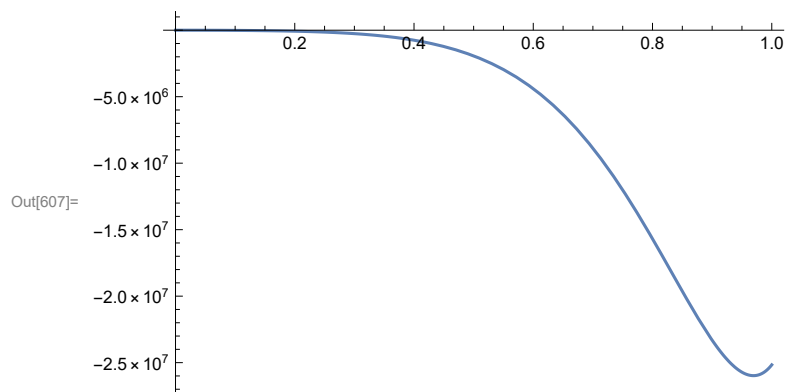

In[608]:= **Plot[Cf[11, 7, 4], {x, 0, 1}]**

[绘图](#)

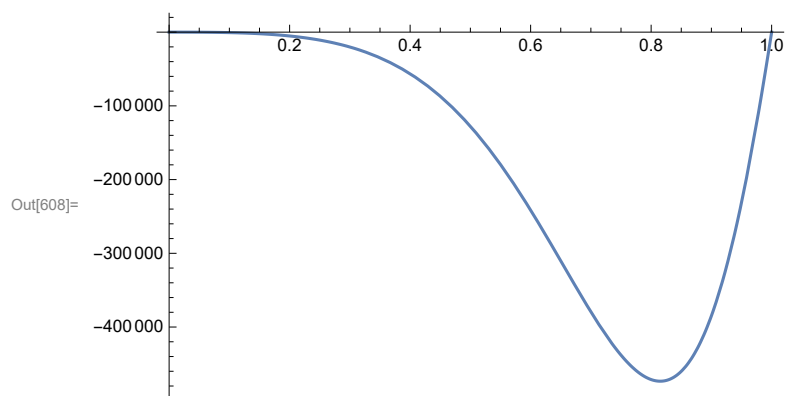

**Plot[Cf[11, 7, 3], {x, 0, 1}]**

[绘图](#)

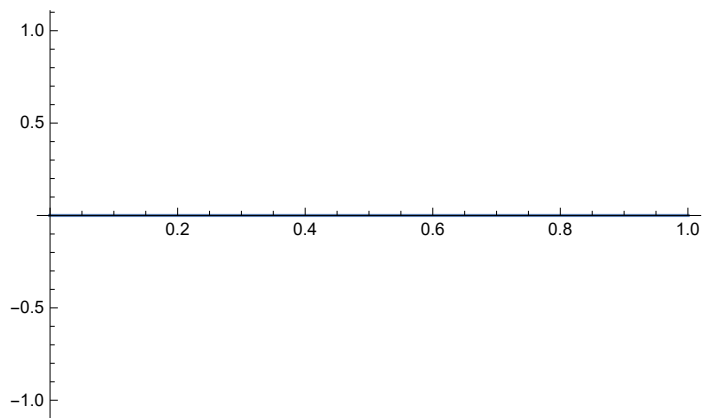

**Plot[Cf[11, 7, 2], {x, 0, 1}]**

[绘图](#)

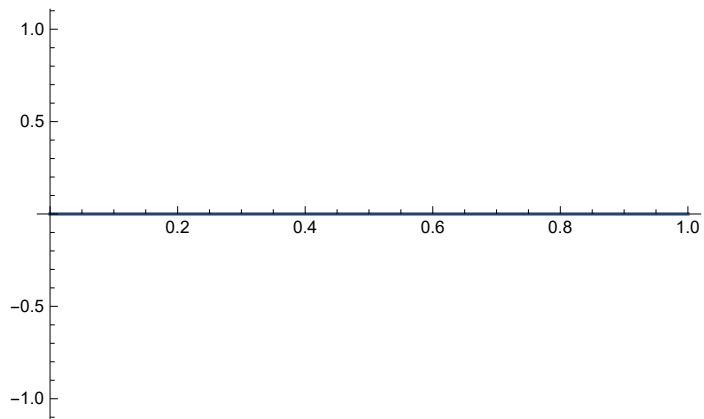

**Plot[Cf[11, 7, 1], {x, 0, 1}]**

[绘图](#)

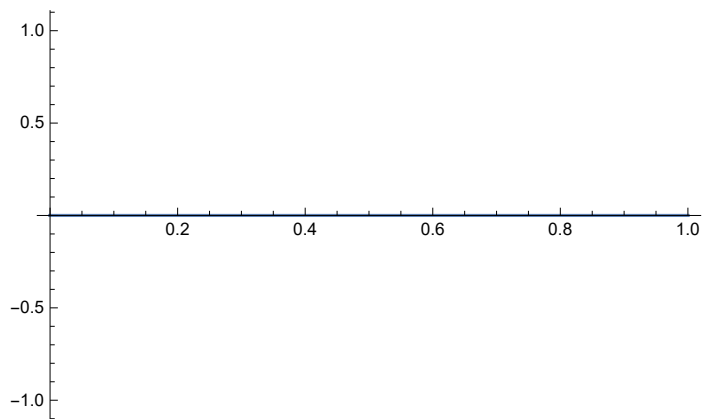

**Plot[Cf[11, 7, 0], {x, 0, 1}]**

[绘图](#)

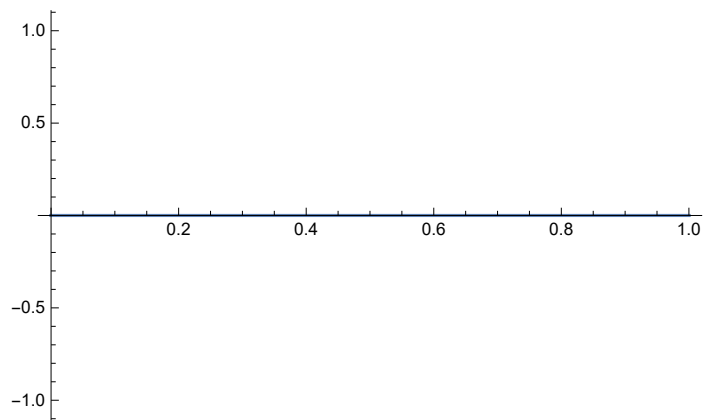

**(\*54th group coefficients r2^11r3^6\*)**

In[609]:= **Plot[Cf[11, 6, 14], {x, 0, 1}]**

[绘图](#)

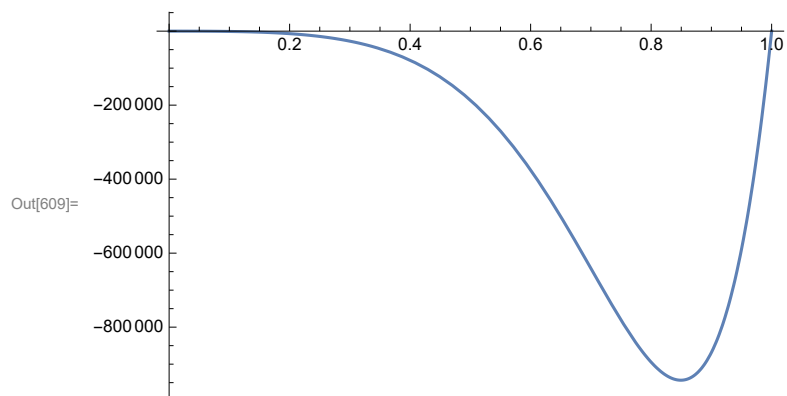

In[610]:= **Plot[Cf[11, 6, 13], {x, 0, 1}]**

[绘图](#)

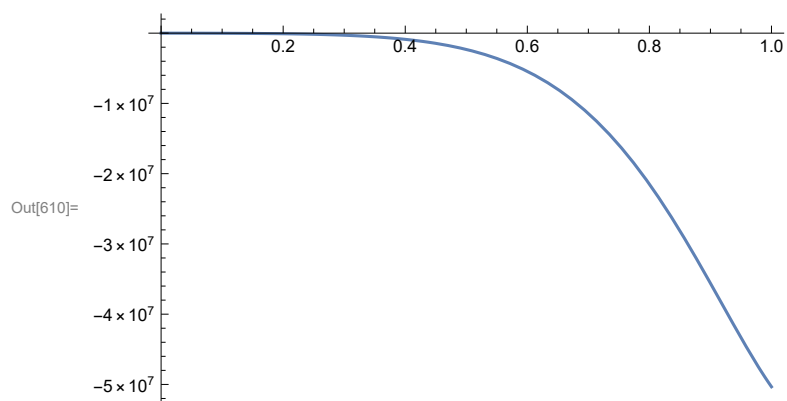

In[611]:= **Plot[Cf[11, 6, 12], {x, 0, 1}]**

[绘图](#)

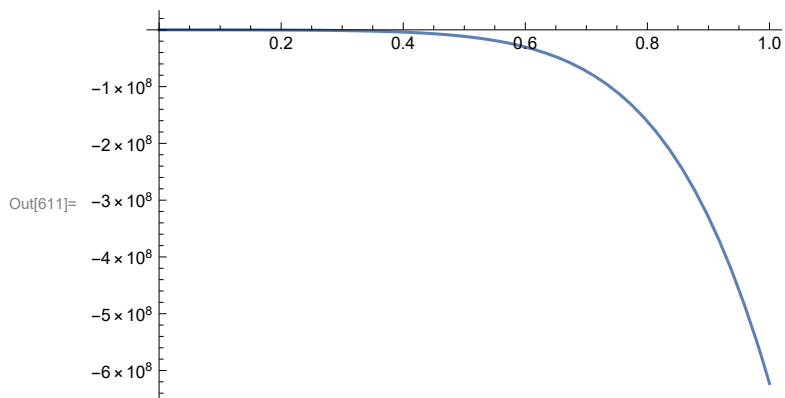

In[612]:= **Plot[Cf[11, 6, 11], {x, 0, 1}]**

[绘图](#)

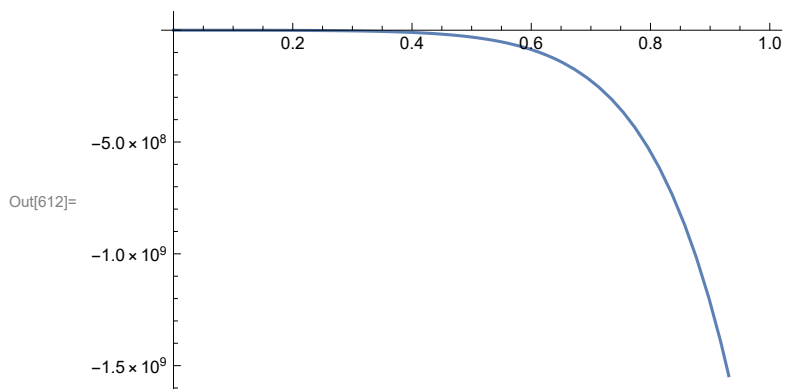

In[613]:= **Plot[Cf[11, 6, 10], {x, 0, 1}]**

[绘图](#)

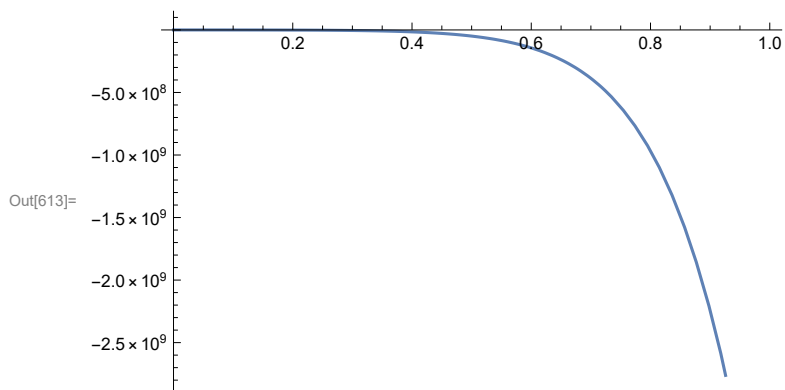

In[614]:= **Plot[Cf[11, 6, 9], {x, 0, 1}]**

[绘图](#)

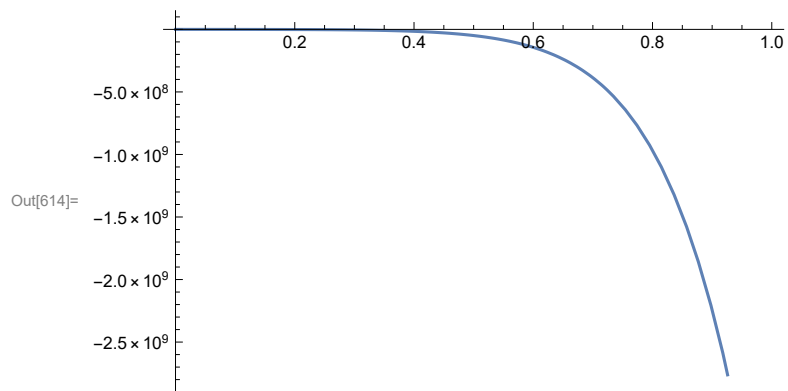

In[615]:= **Plot[Cf[11, 6, 8], {x, 0, 1}]**

[绘图](#)

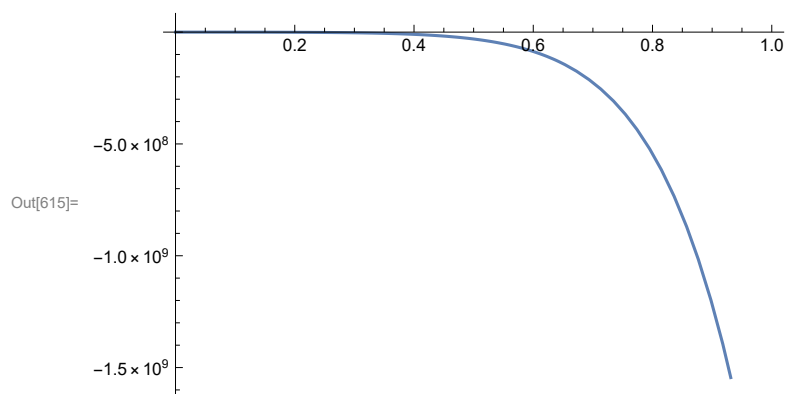

In[616]:= **Plot[Cf[11, 6, 7], {x, 0, 1}]**

[绘图](#)

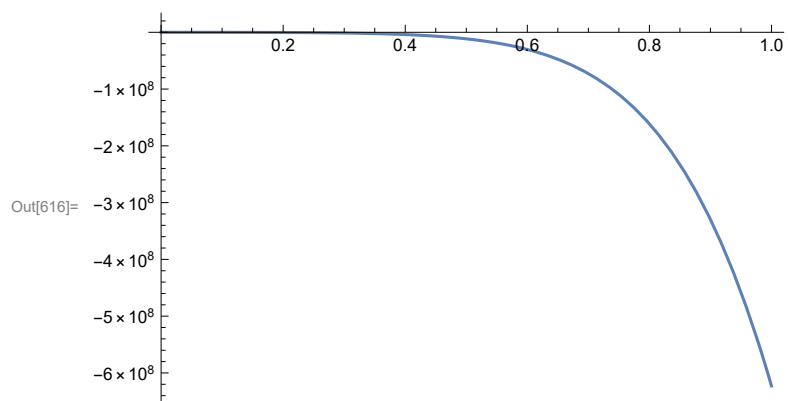



In[617]:= **Plot[Cf[11, 6, 6], {x, 0, 1}]**

[绘图](#)

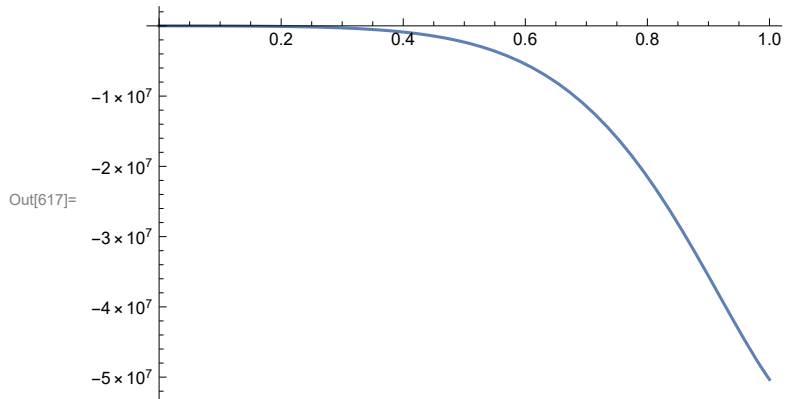

In[618]:= **Plot[Cf[11, 6, 5], {x, 0, 1}]**

[绘图](#)

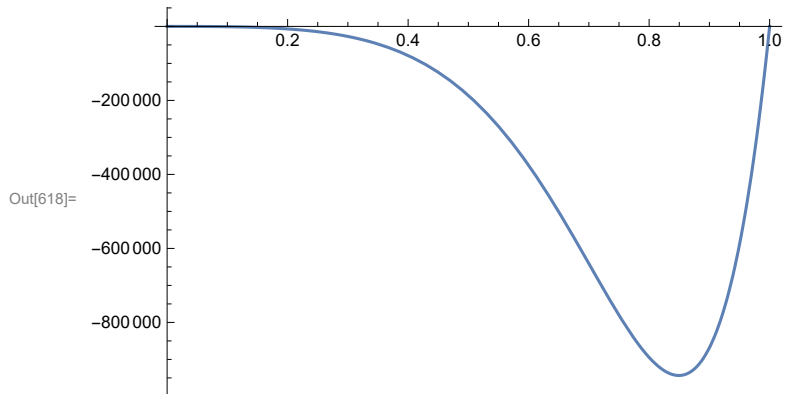

**Plot[Cf[11, 6, 4], {x, 0, 1}]**

[绘图](#)

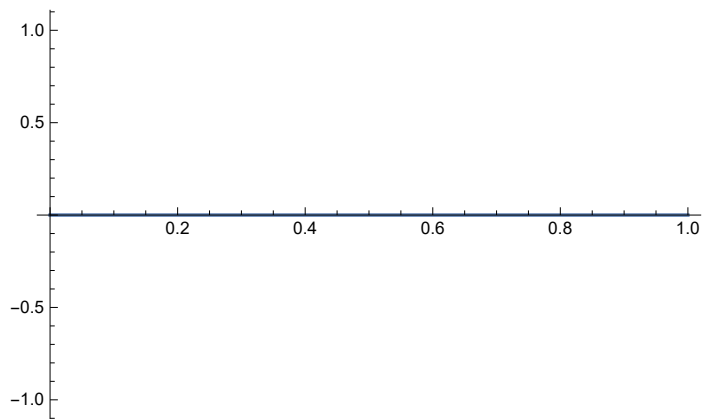

```
Plot[Cf[11, 6, 3], {x, 0, 1}]
```

[绘图](#)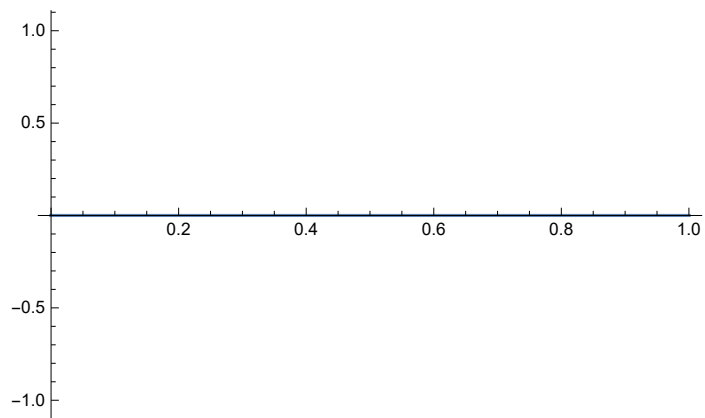

```
Plot[Cf[11, 6, 2], {x, 0, 1}]
```

[绘图](#)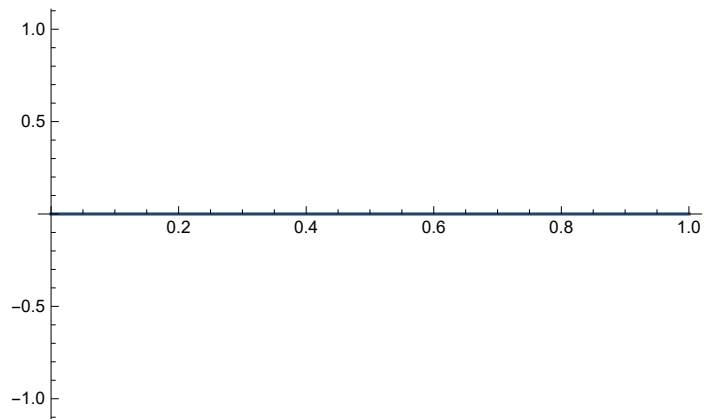

```
Plot[Cf[11, 6, 1], {x, 0, 1}]
```

[绘图](#)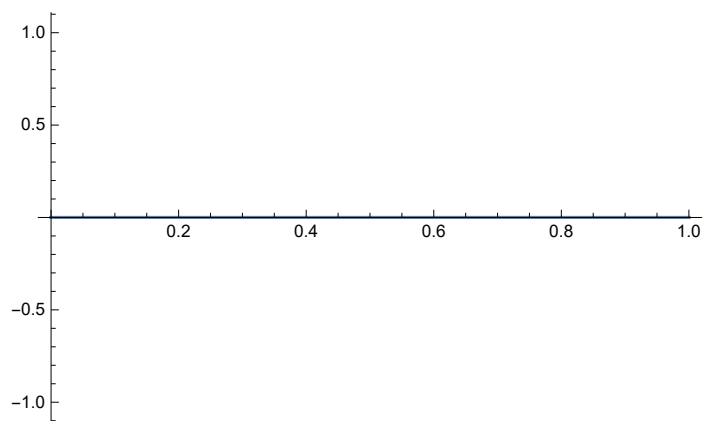

**Plot[Cf[11, 6, 0], {x, 0, 1}]**

[绘图](#)

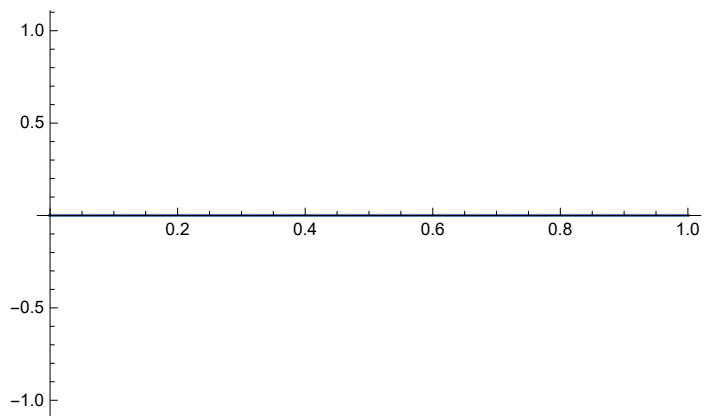

(\*55th group coefficients r2^11r3^5\*)

In[619]:= **Plot[Cf[11, 5, 14], {x, 0, 1}]**

[绘图](#)

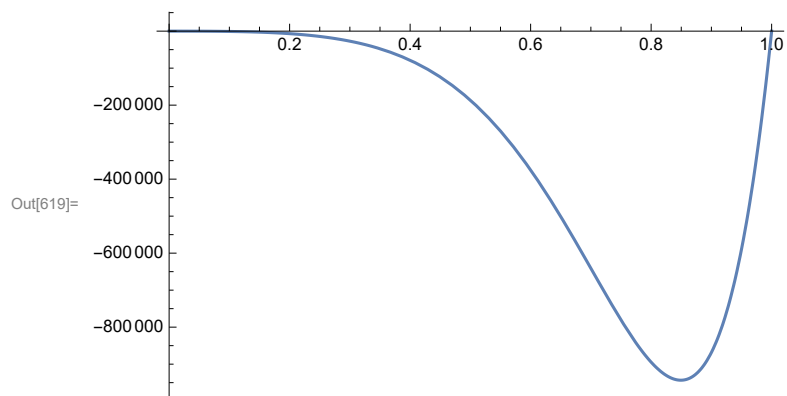

In[620]:= **Plot[Cf[11, 5, 13], {x, 0, 1}]**

[绘图](#)

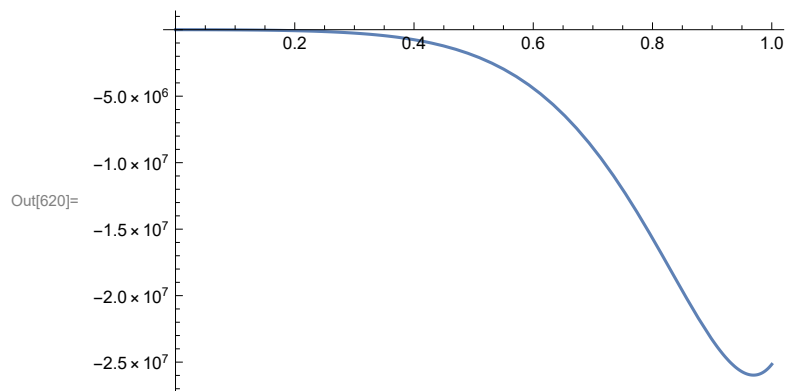

In[621]:= **Plot[Cf[11, 5, 12], {x, 0, 1}]**

[绘图](#)

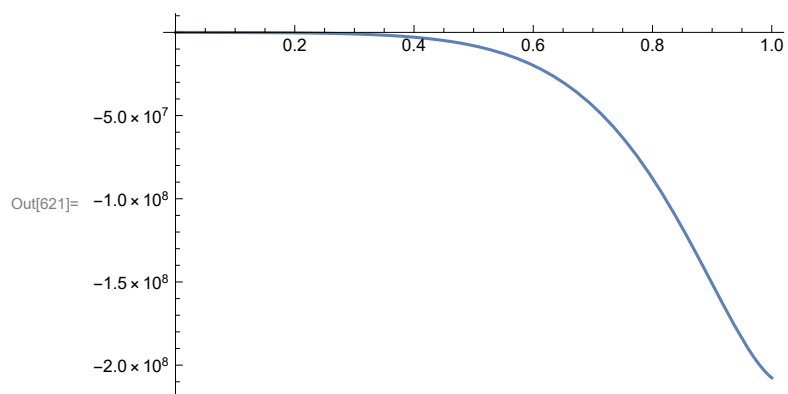

In[622]:= **Plot[Cf[11, 5, 11], {x, 0, 1}]**

[绘图](#)

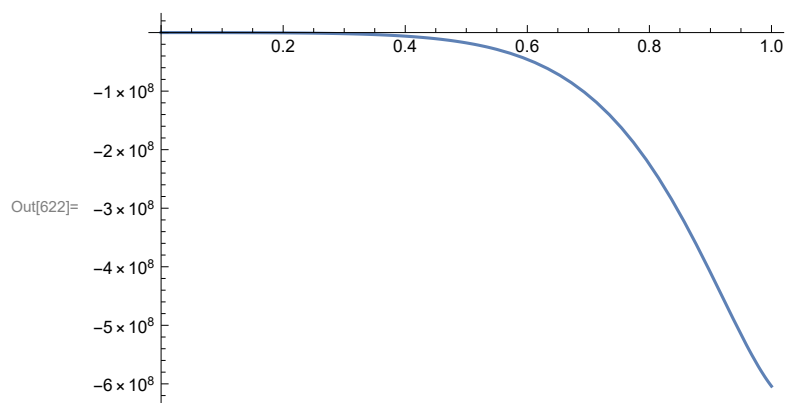

In[623]:= **Plot[Cf[11, 5, 10], {x, 0, 1}]**

[绘图](#)

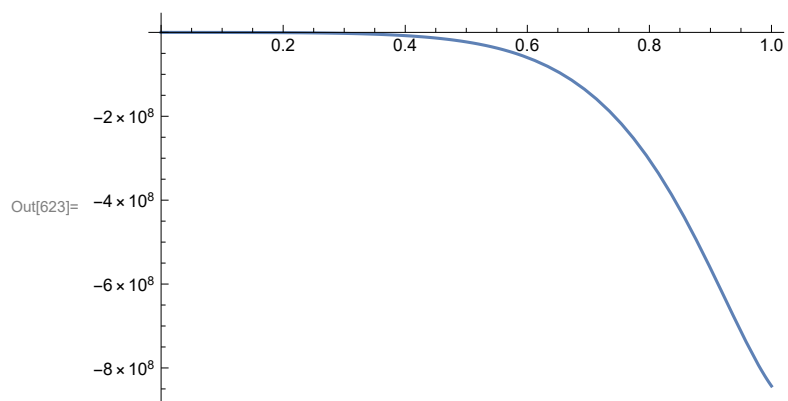

In[624]:= **Plot[Cf[11, 5, 9], {x, 0, 1}]**

[绘图](#)

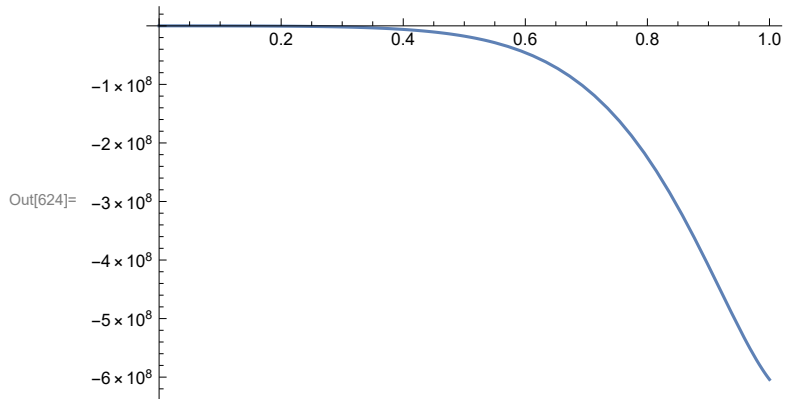

In[625]:= **Plot[Cf[11, 5, 8], {x, 0, 1}]**

[绘图](#)

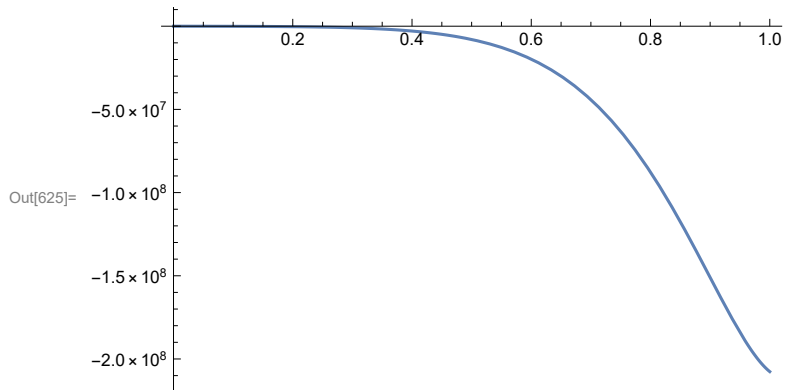

In[626]:= **Plot[Cf[11, 5, 7], {x, 0, 1}]**

[绘图](#)

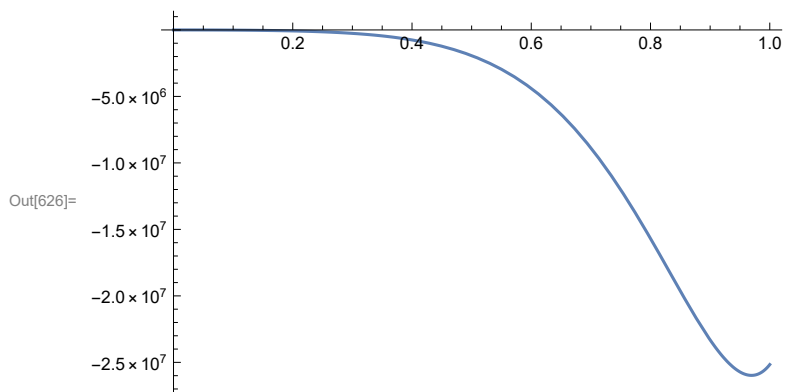

In[627]:= **Plot[Cf[11, 5, 6], {x, 0, 1}]**

[绘图](#)

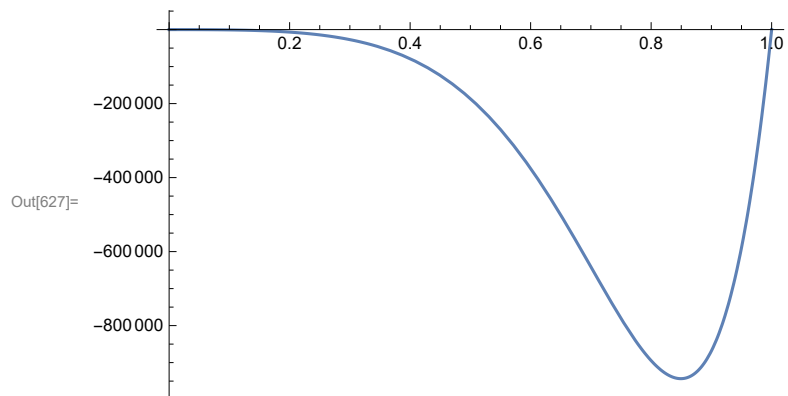

**Plot[Cf[11, 5, 5], {x, 0, 1}]**

[绘图](#)

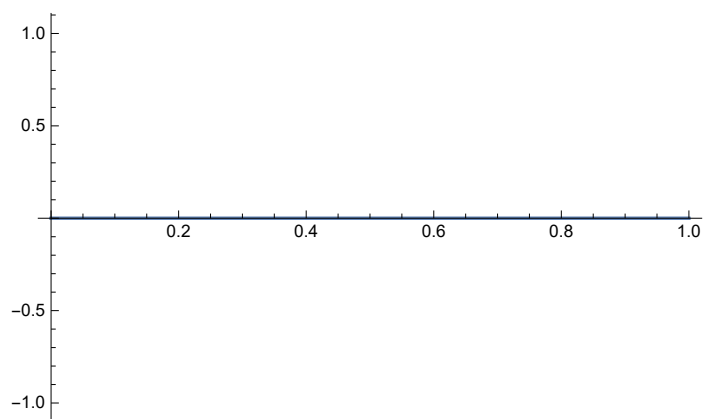

**Plot[Cf[11, 5, 4], {x, 0, 1}]**

[绘图](#)

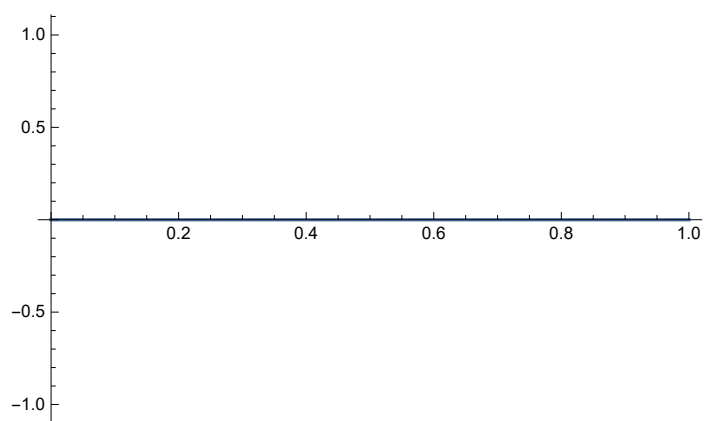

**Plot[Cf[11, 5, 3], {x, 0, 1}]**

[绘图](#)

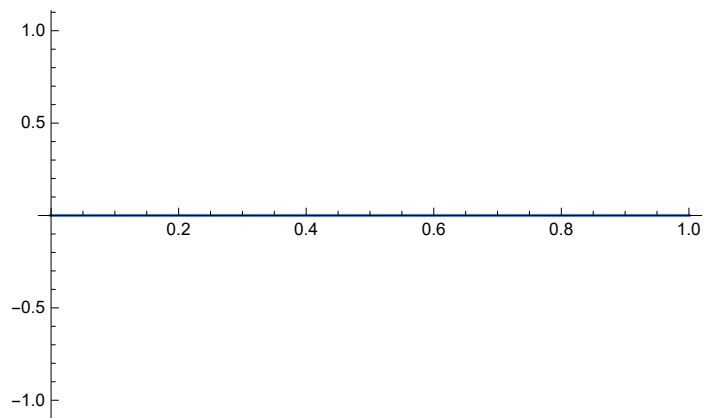

**Plot[Cf[11, 5, 2], {x, 0, 1}]**

[绘图](#)

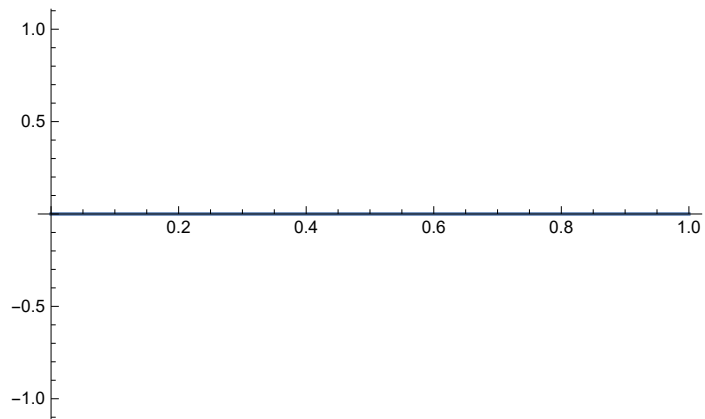

**Plot[Cf[11, 5, 1], {x, 0, 1}]**

[绘图](#)

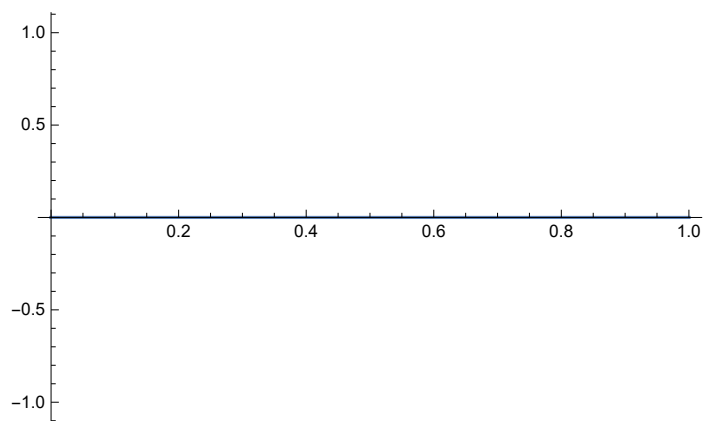

**Plot[Cf[11, 5, 0], {x, 0, 1}]**

[绘图](#)

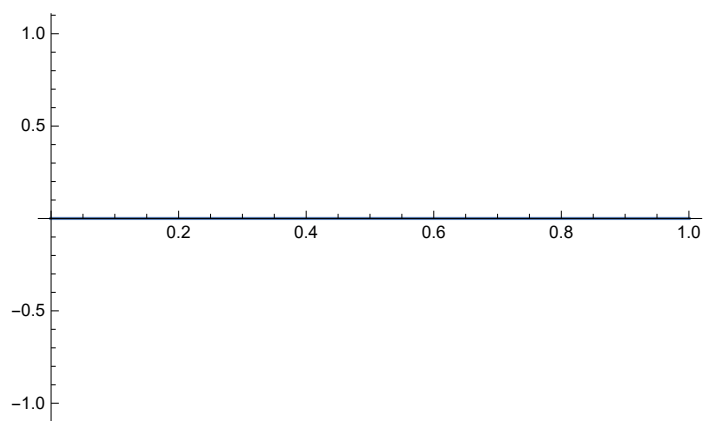

**(\*56th group coefficients r2^11r3^4\*)**

In[628]:= **Plot[Cf[11, 4, 14], {x, 0, 1}]**

[绘图](#)

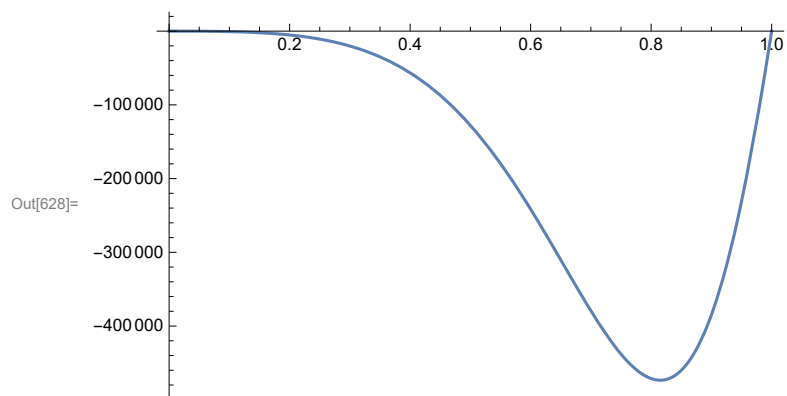

In[629]:= **Plot[Cf[11, 4, 13], {x, 0, 1}]**

[绘图](#)

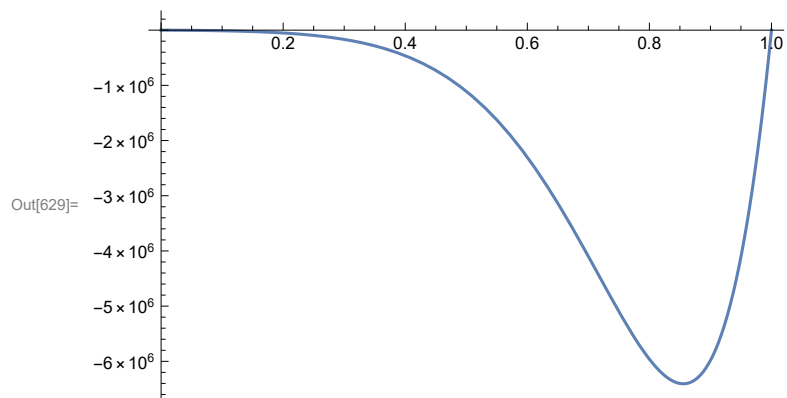



In[630]:= **Plot[Cf[11, 4, 12], {x, 0, 1}]**

[绘图](#)

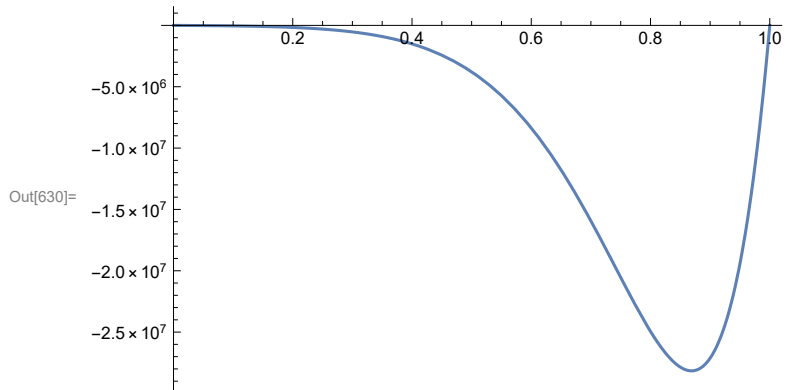

In[631]:= **Plot[Cf[11, 4, 11], {x, 0, 1}]**

[绘图](#)

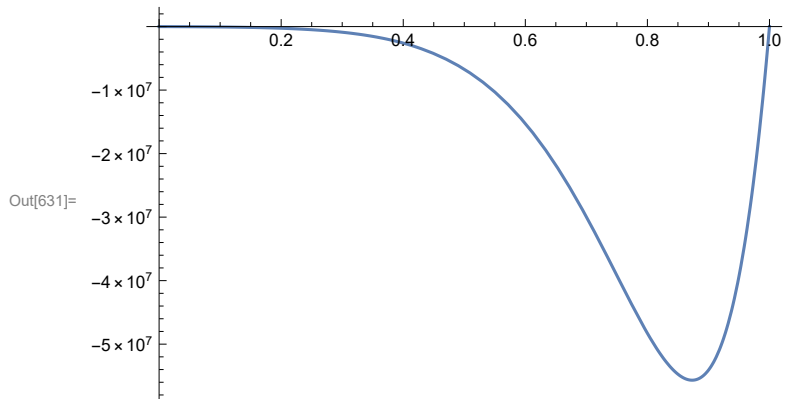

In[632]:= **Plot[Cf[11, 4, 10], {x, 0, 1}]**

[绘图](#)

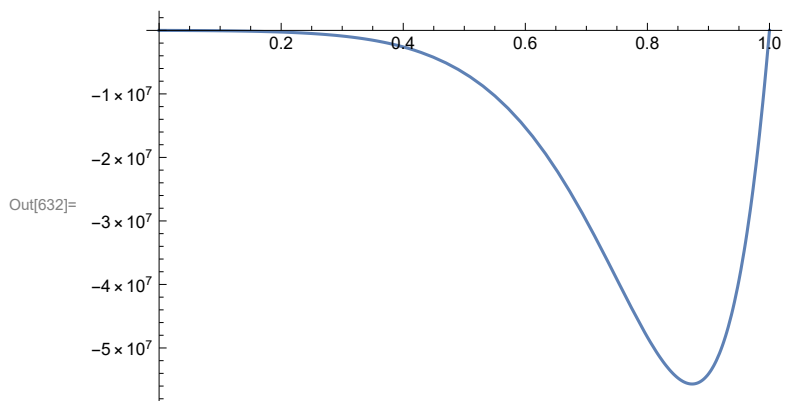

In[633]:= **Plot[Cf[11, 4, 9], {x, 0, 1}]**

[绘图](#)

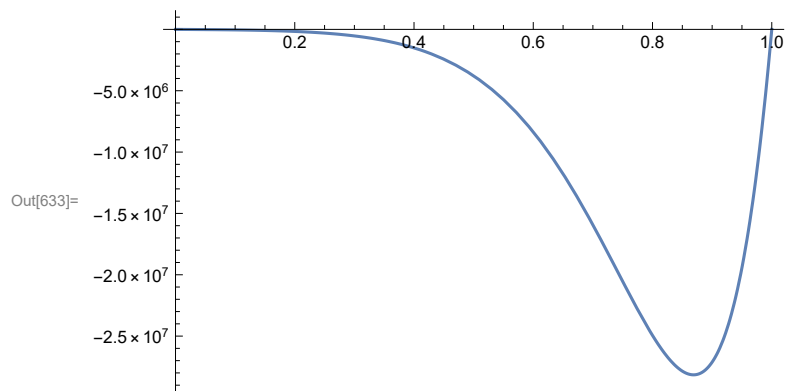

In[634]:= **Plot[Cf[11, 4, 8], {x, 0, 1}]**

[绘图](#)

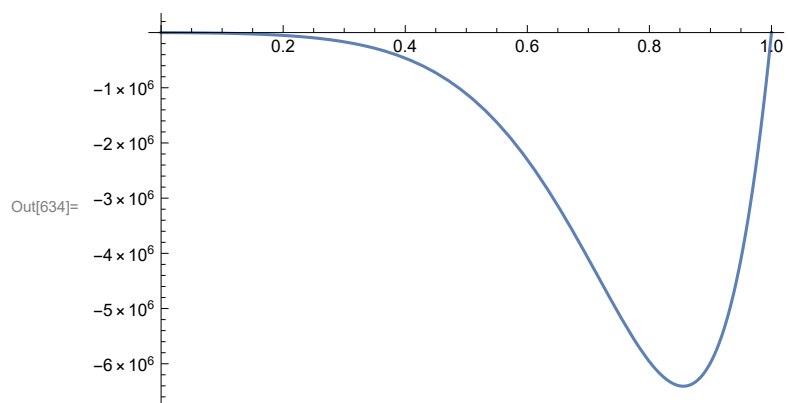

In[635]:= **Plot[Cf[11, 4, 7], {x, 0, 1}]**

[绘图](#)

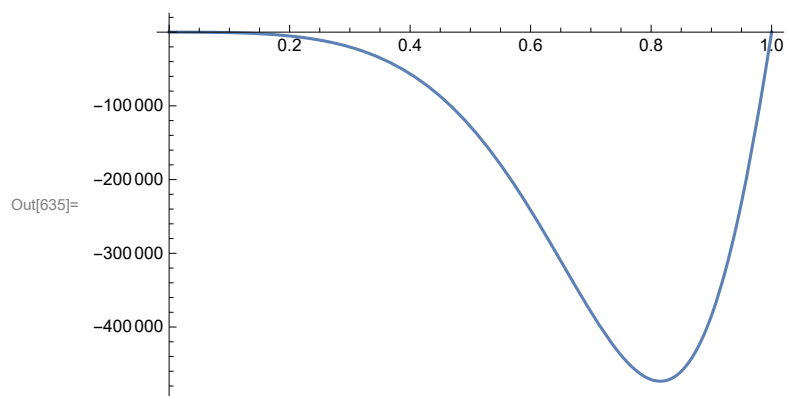

```
Plot[Cf[11, 4, 6], {x, 0, 1}]
```

[绘图](#)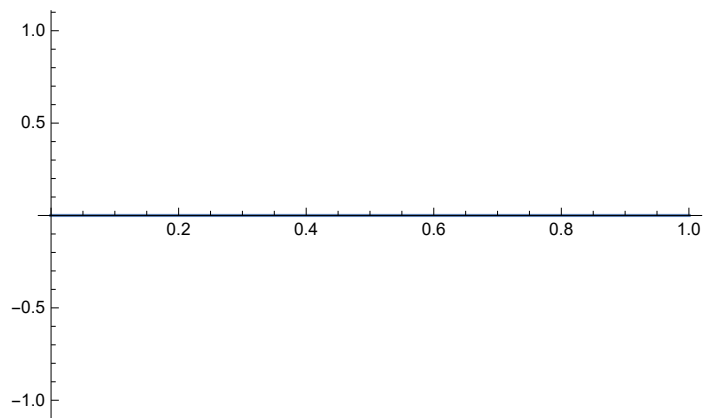

```
Plot[Cf[11, 4, 5], {x, 0, 1}]
```

[绘图](#)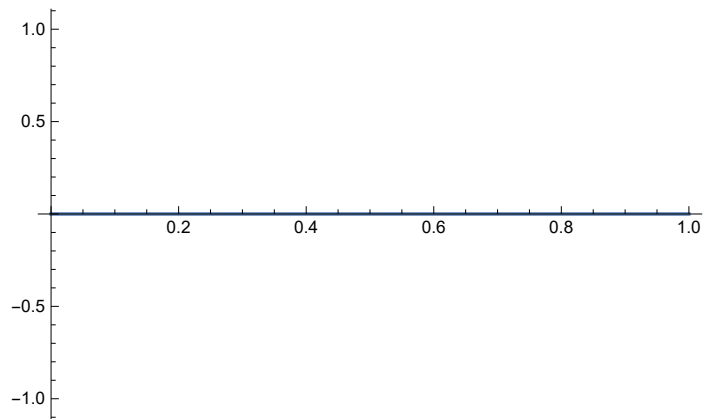

```
Plot[Cf[11, 4, 4], {x, 0, 1}]
```

[绘图](#)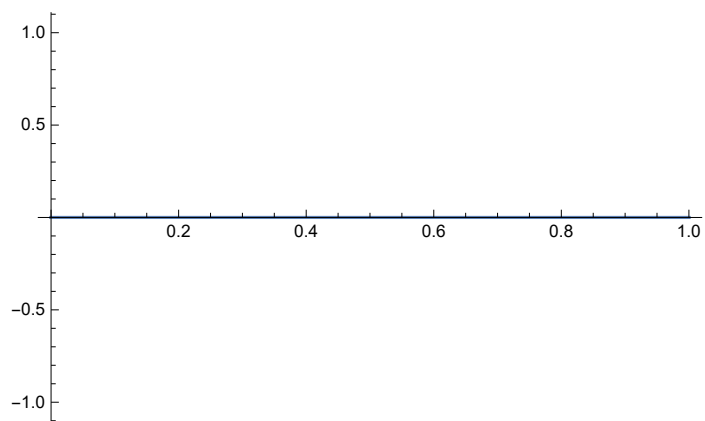

```
Plot[Cf[11, 4, 3], {x, 0, 1}]
```

[绘图](#)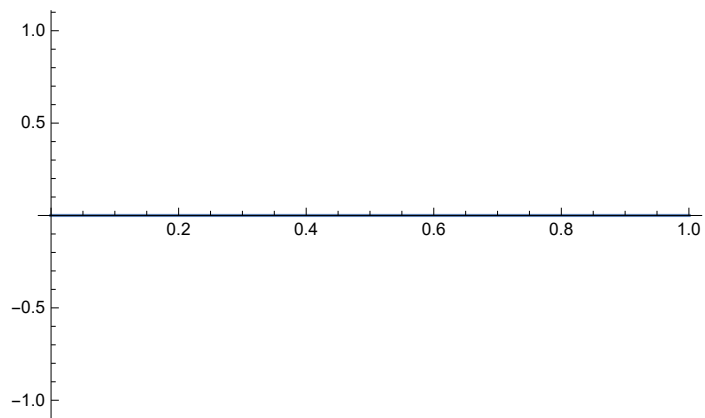

```
Plot[Cf[11, 4, 2], {x, 0, 1}]
```

[绘图](#)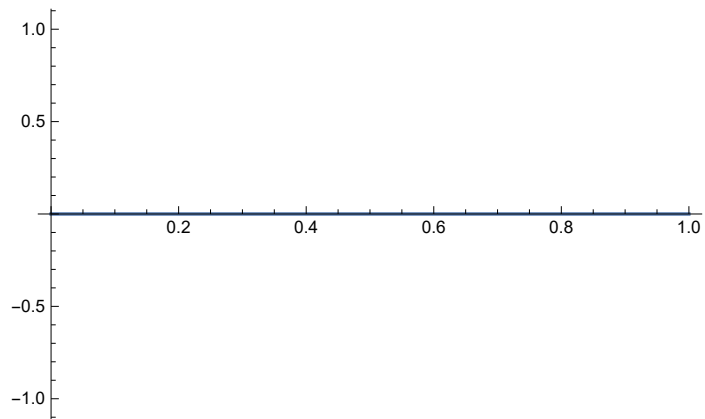

```
Plot[Cf[11, 4, 1], {x, 0, 1}]
```

[绘图](#)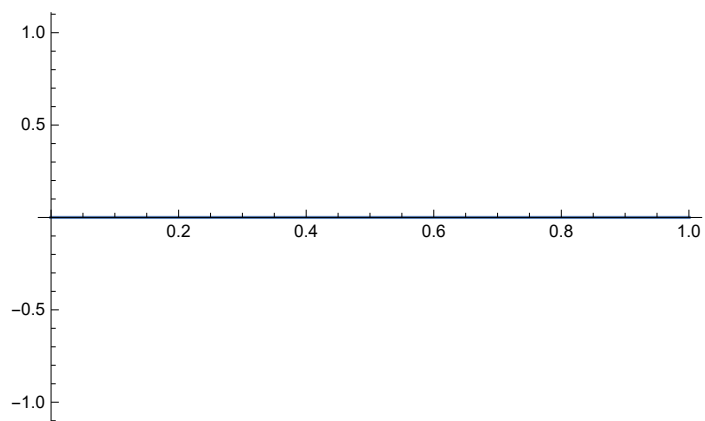

**Plot[Cf[11, 4, 0], {x, 0, 1}]**

[绘图](#)

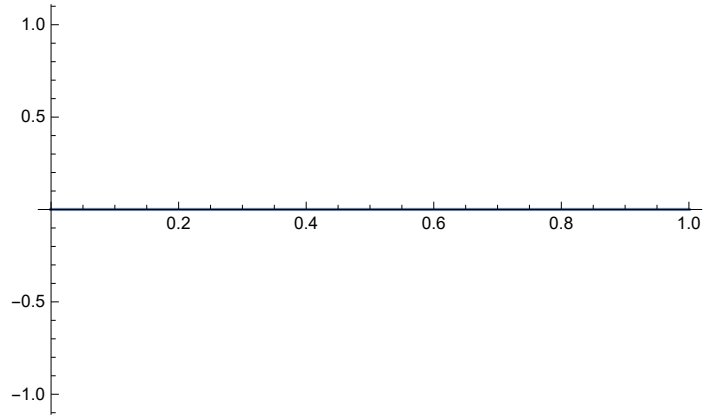

**(\*57th group coefficients r2^11r3^3\*)**

In[636]:= **Plot[Cf[11, 3, 14], {x, 0, 1}]**

[绘图](#)

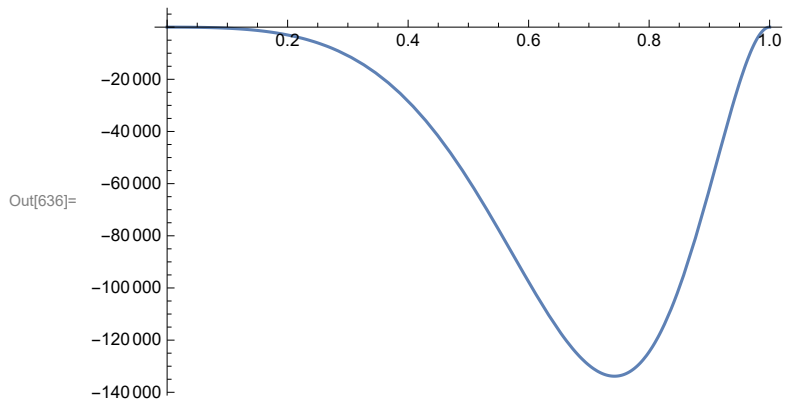

In[637]:= **Plot[Cf[11, 3, 13], {x, 0, 1}]**

[绘图](#)

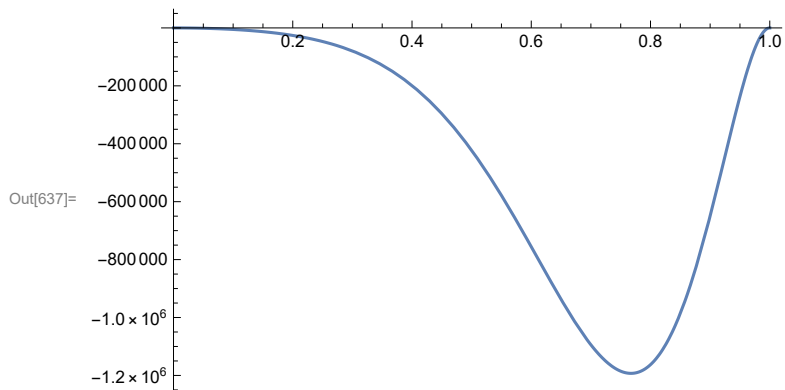

In[638]:= **Plot[Cf[11, 3, 12], {x, 0, 1}]**

[绘图](#)

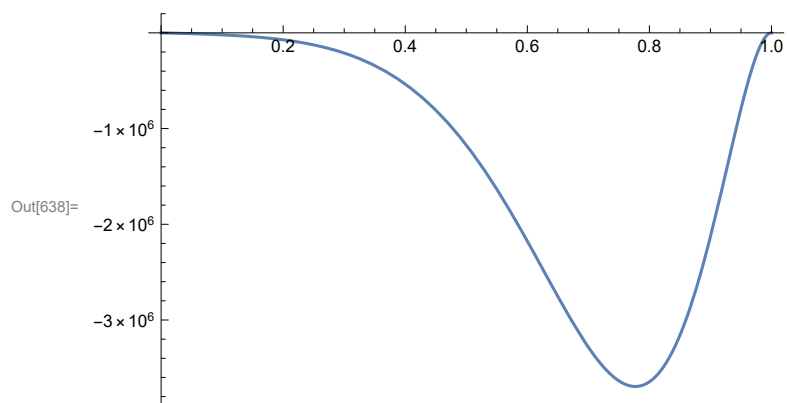

In[639]:= **Plot[Cf[11, 3, 11], {x, 0, 1}]**

[绘图](#)

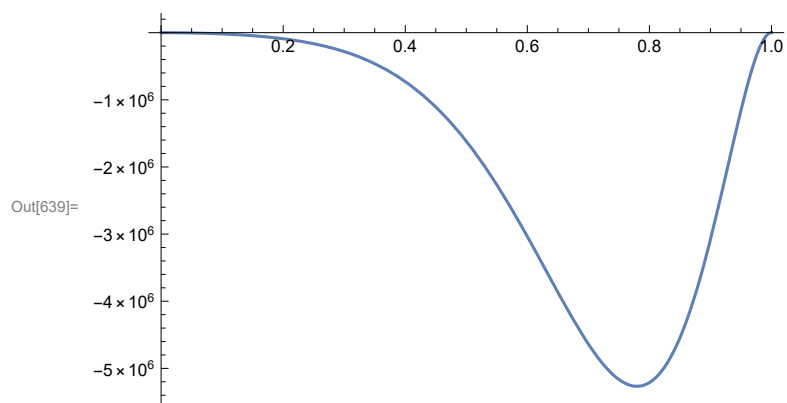

In[640]:= **Plot[Cf[11, 3, 10], {x, 0, 1}]**

[绘图](#)

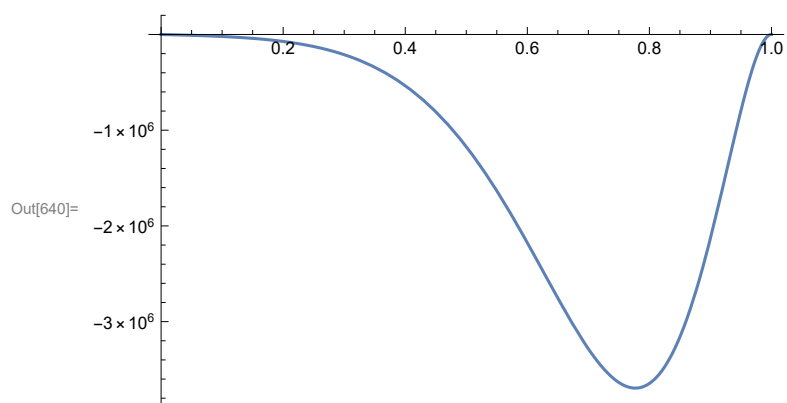

In[641]:= **Plot[Cf[11, 3, 9], {x, 0, 1}]**

[绘图](#)

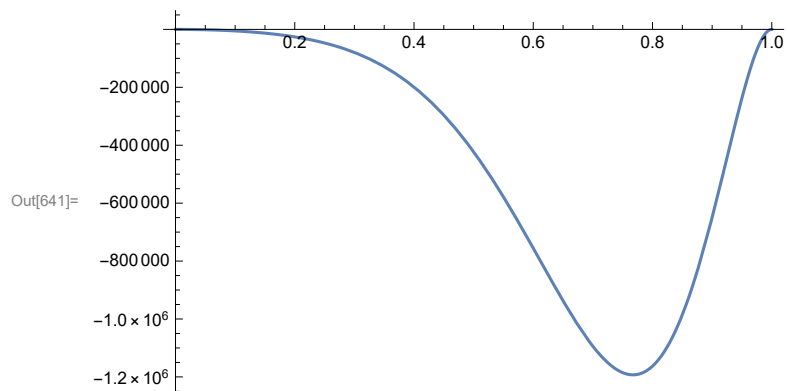

In[642]:= **Plot[Cf[11, 3, 8], {x, 0, 1}]**

[绘图](#)

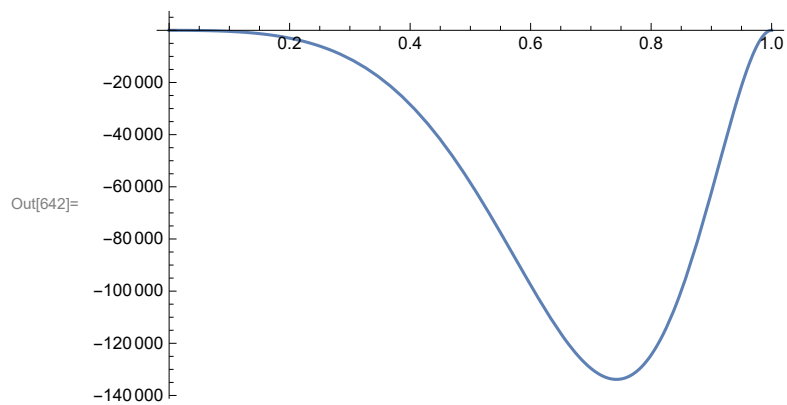

**Plot[Cf[11, 3, 7], {x, 0, 1}]**

[绘图](#)

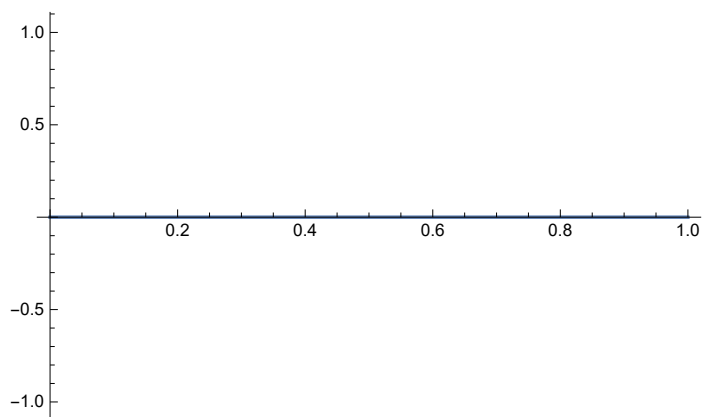

```
Plot[Cf[11, 3, 6], {x, 0, 1}]
```

[绘图](#)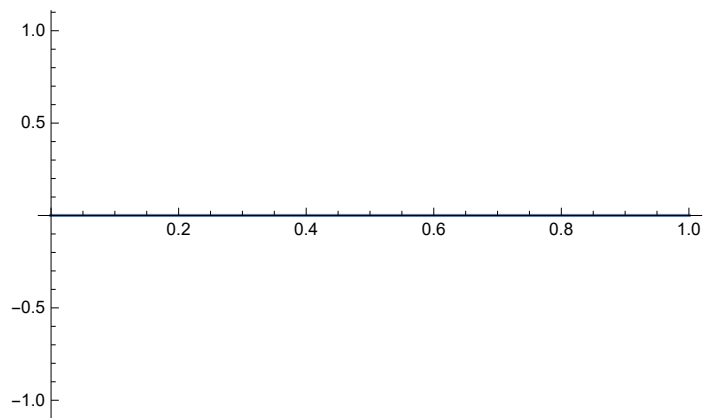

```
Plot[Cf[11, 3, 5], {x, 0, 1}]
```

[绘图](#)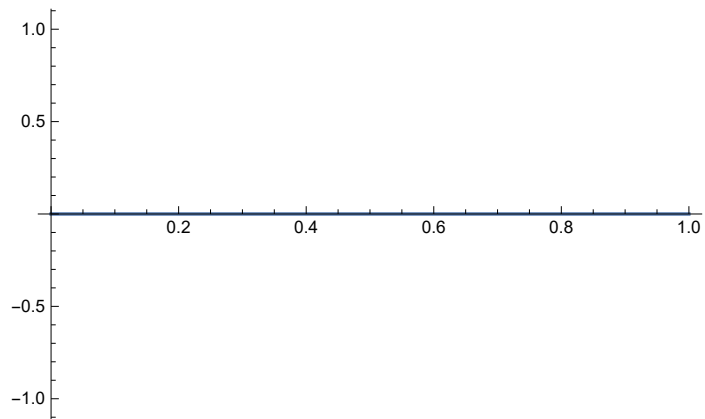

```
Plot[Cf[11, 3, 4], {x, 0, 1}]
```

[绘图](#)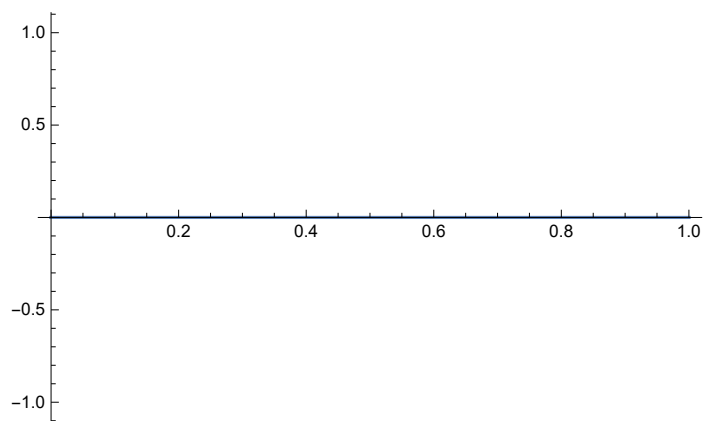



```
Plot[Cf[11, 3, 3], {x, 0, 1}]
```

[绘图](#)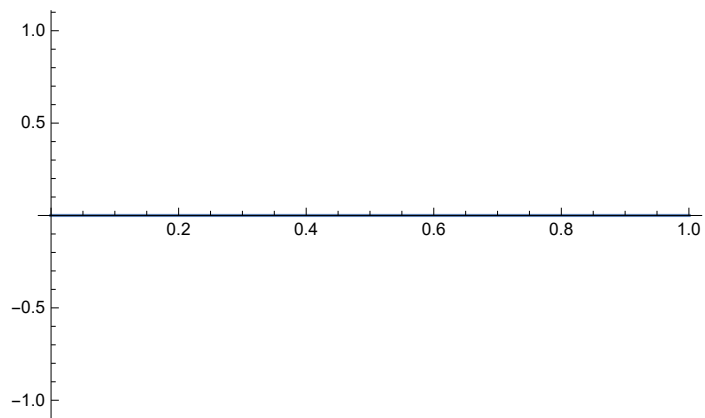

```
Plot[Cf[11, 3, 4], {x, 0, 1}]
```

[绘图](#)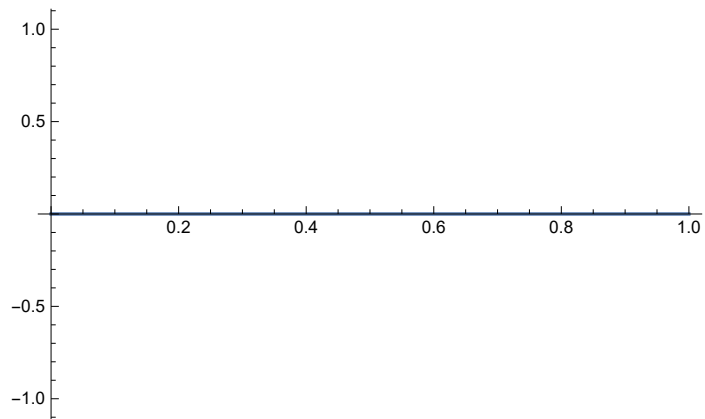

```
Plot[Cf[11, 3, 3], {x, 0, 1}]
```

[绘图](#)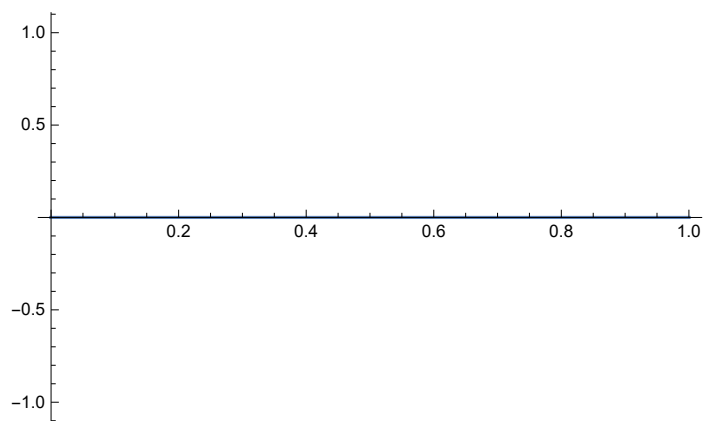

**Plot[Cf[11, 3, 2], {x, 0, 1}]**

[绘图](#)

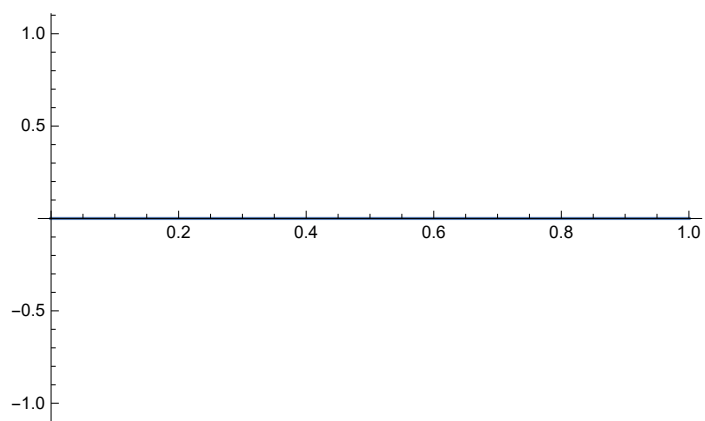

**Plot[Cf[11, 3, 1], {x, 0, 1}]**

[绘图](#)

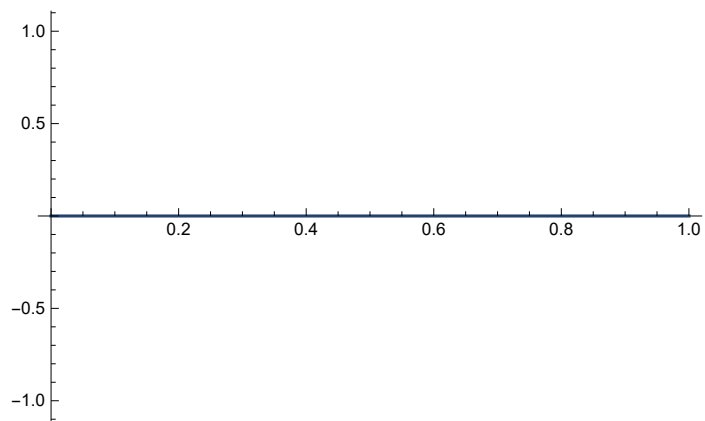

**Plot[Cf[11, 3, 0], {x, 0, 1}]**

[绘图](#)

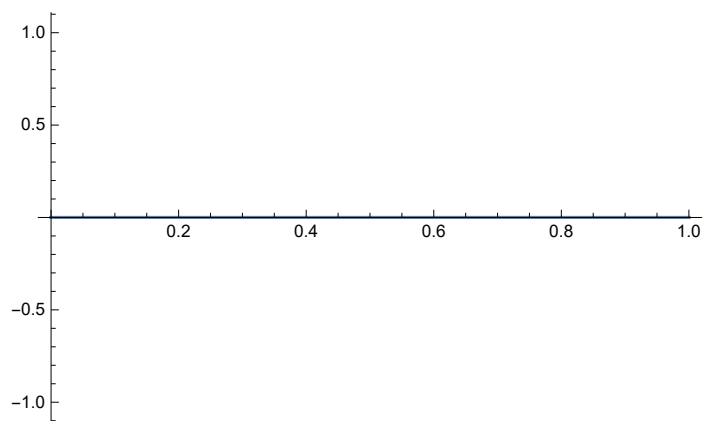

**(\*58th group coefficients r2^11r3^2\*)**

In[643]:= **Plot[Cf[11, 2, 14], {x, 0, 1}]**

[绘图](#)

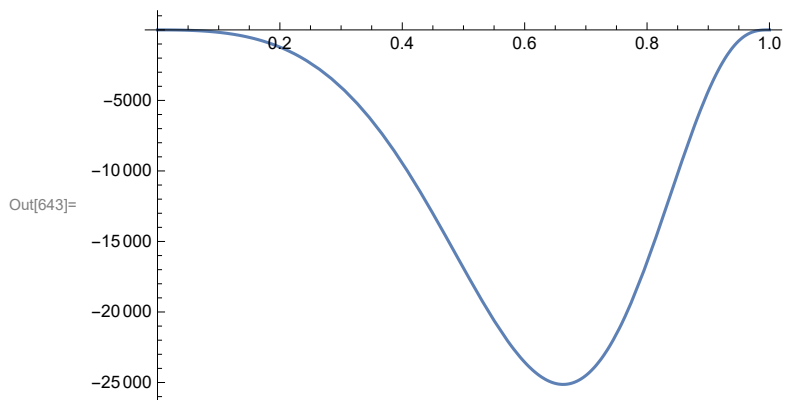

In[644]:= **Plot[Cf[11, 2, 13], {x, 0, 1}]**

[绘图](#)

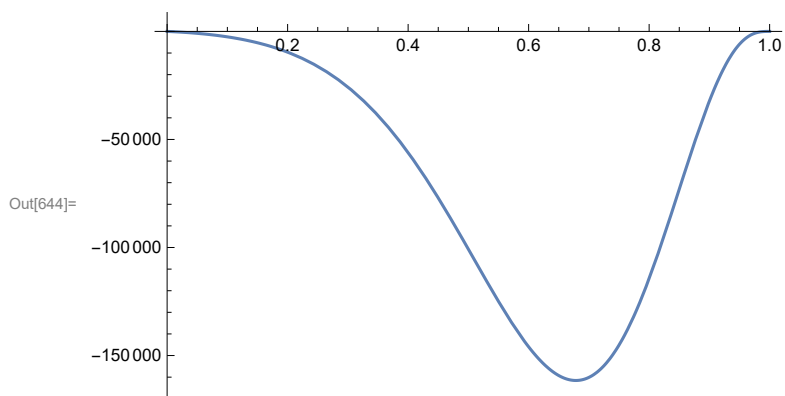

In[645]:= **Plot[Cf[11, 2, 12], {x, 0, 1}]**

[绘图](#)

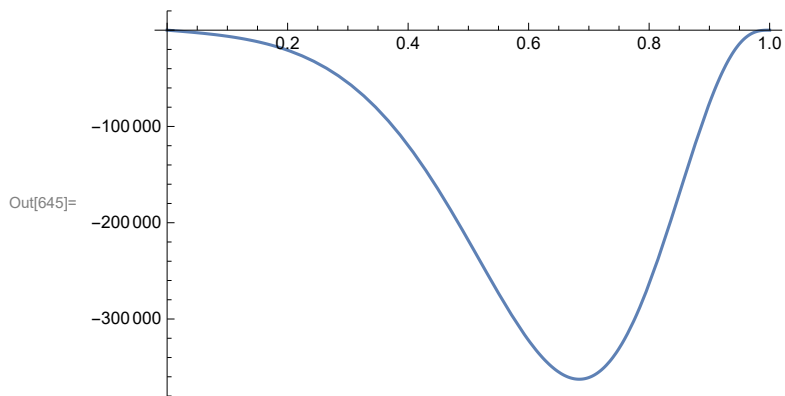

In[646]:= **Plot[Cf[11, 2, 11], {x, 0, 1}]**

[绘图](#)

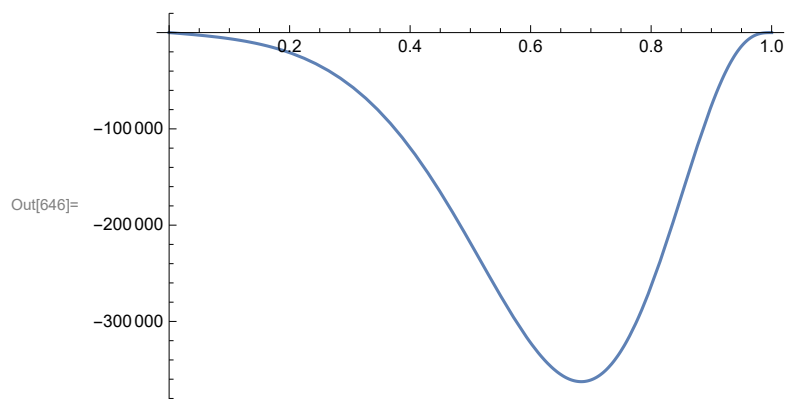

In[647]:= **Plot[Cf[11, 2, 10], {x, 0, 1}]**

[绘图](#)

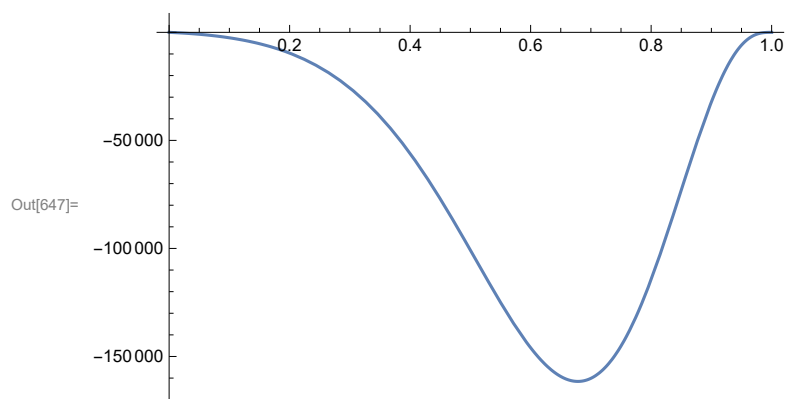

In[648]:= **Plot[Cf[11, 2, 9], {x, 0, 1}]**

[绘图](#)

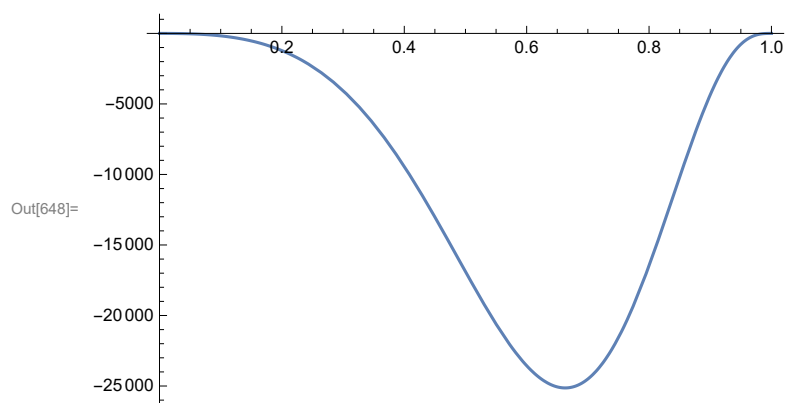

**Plot[Cf[11, 2, 8], {x, 0, 1}]**

[绘图](#)

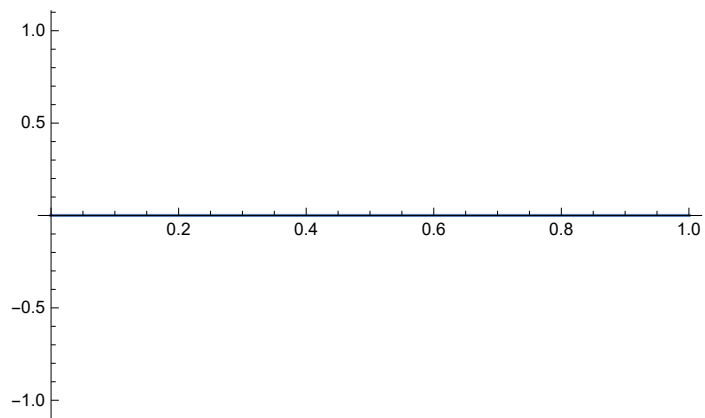

**Plot[Cf[11, 2, 7], {x, 0, 1}]**

[绘图](#)

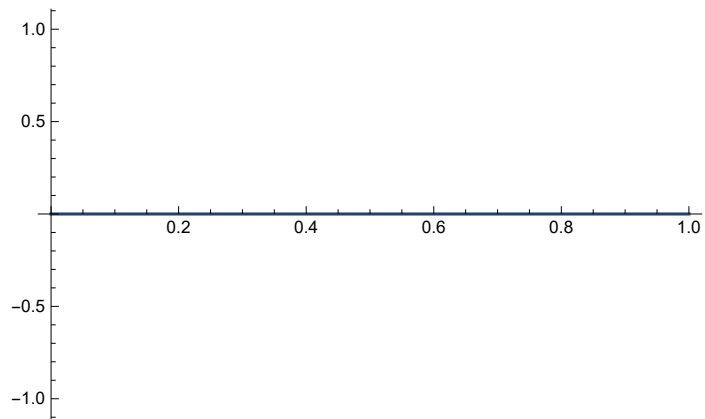

**Plot[Cf[11, 2, 6], {x, 0, 1}]**

[绘图](#)

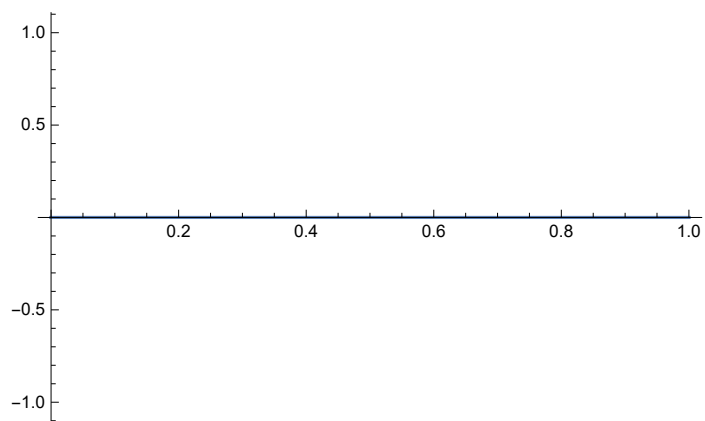

**Plot[Cf[11, 2, 5], {x, 0, 1}]**

[绘图](#)

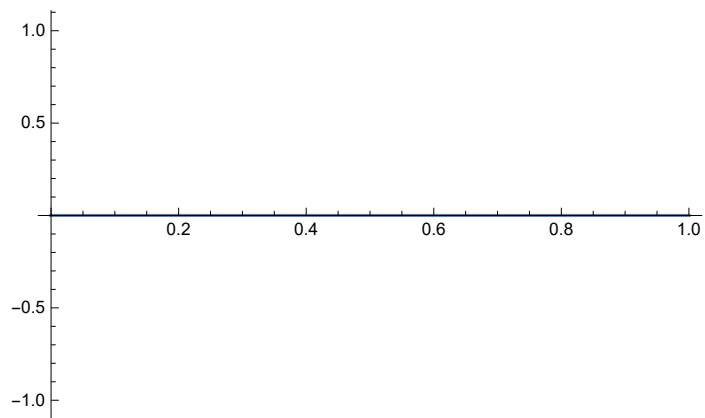

**Plot[Cf[11, 2, 4], {x, 0, 1}]**

[绘图](#)

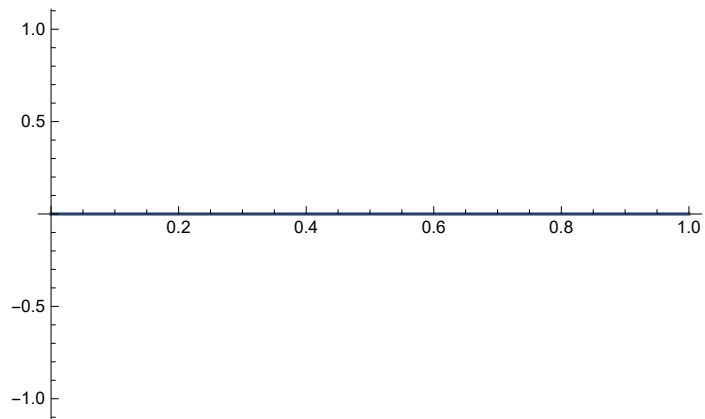

**Plot[Cf[11, 2, 3], {x, 0, 1}]**

[绘图](#)

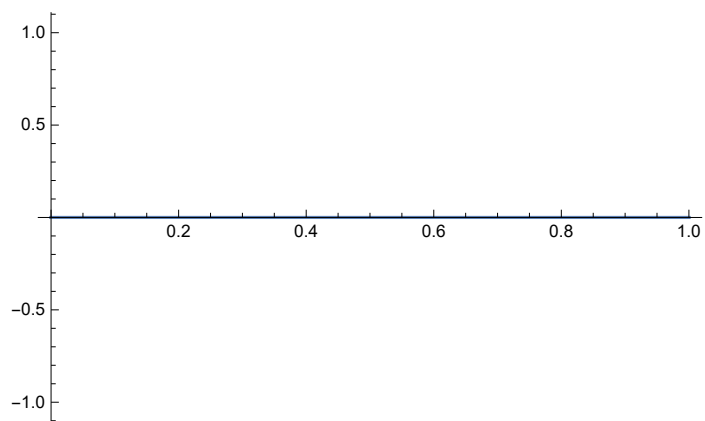

**Plot[Cf[11, 2, 2], {x, 0, 1}]**

[绘图](#)

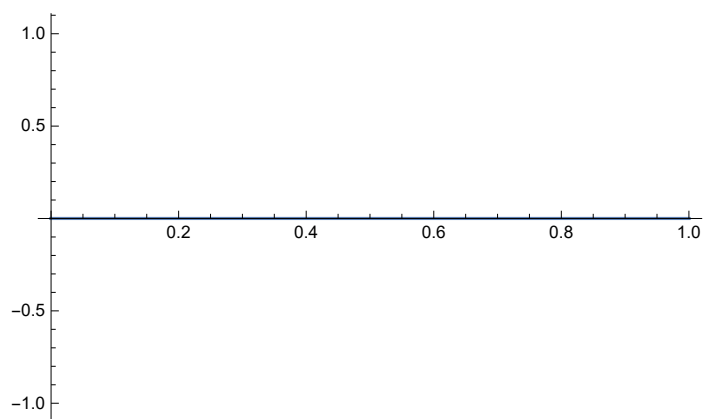

**Plot[Cf[11, 2, 1], {x, 0, 1}]**

[绘图](#)

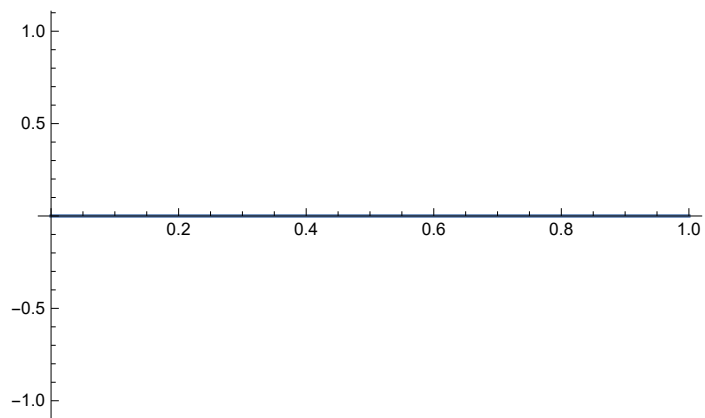

**Plot[Cf[11, 2, 0], {x, 0, 1}]**

[绘图](#)

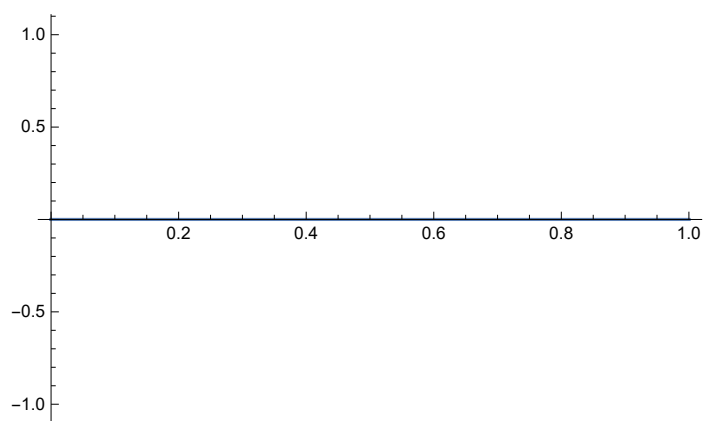

**(\*59th group coefficients r2^11r3^1\*)**

In[649]:= **Plot[Cf[11, 1, 14], {x, 0, 1}]**

[绘图](#)

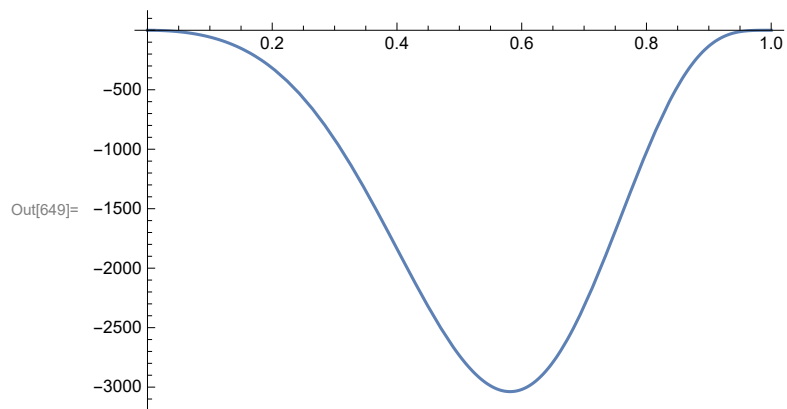

In[650]:= **Plot[Cf[11, 1, 13], {x, 0, 1}]**

[绘图](#)

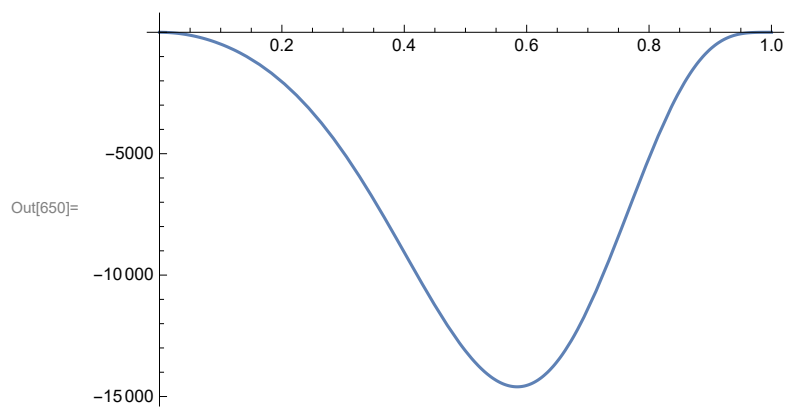

In[651]:= **Plot[Cf[11, 1, 12], {x, 0, 1}]**

[绘图](#)

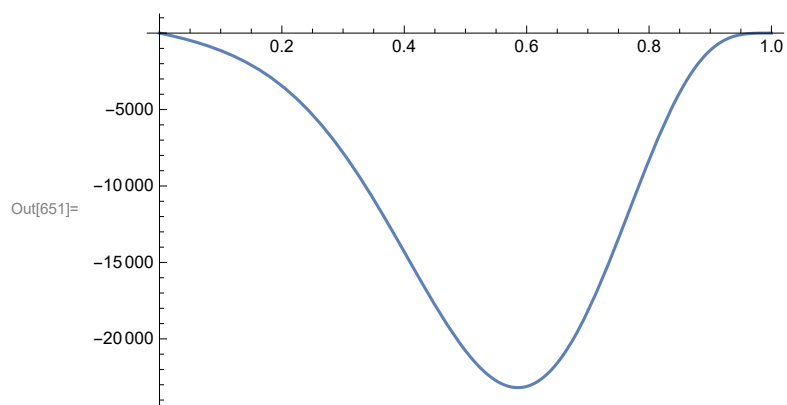



In[652]:= **Plot[Cf[11, 1, 11], {x, 0, 1}]**

[绘图](#)

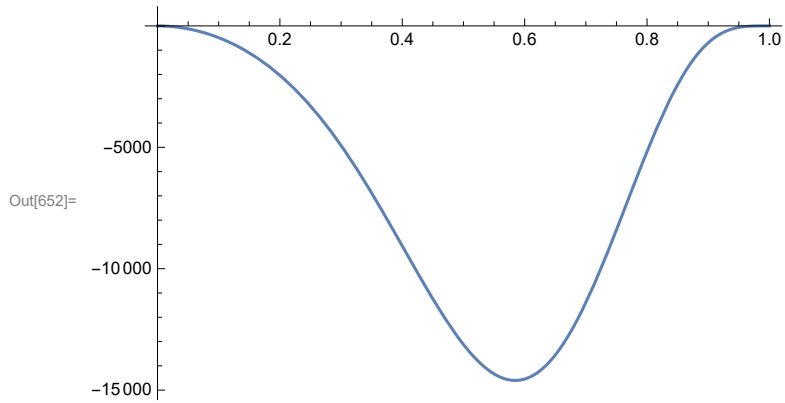

In[653]:= **Plot[Cf[11, 1, 10], {x, 0, 1}]**

[绘图](#)

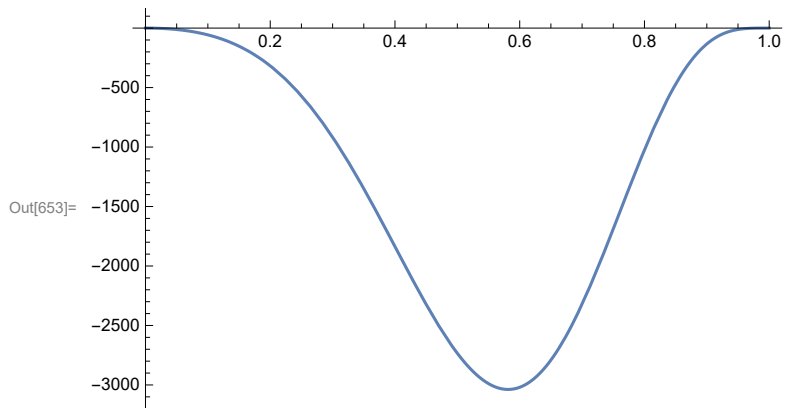

**Plot[Cf[11, 1, 9], {x, 0, 1}]**

[绘图](#)

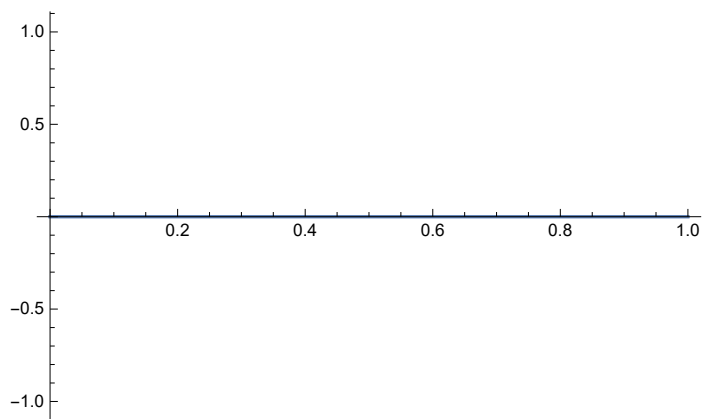

```
Plot[Cf[11, 1, 8], {x, 0, 1}]
```

[绘图](#)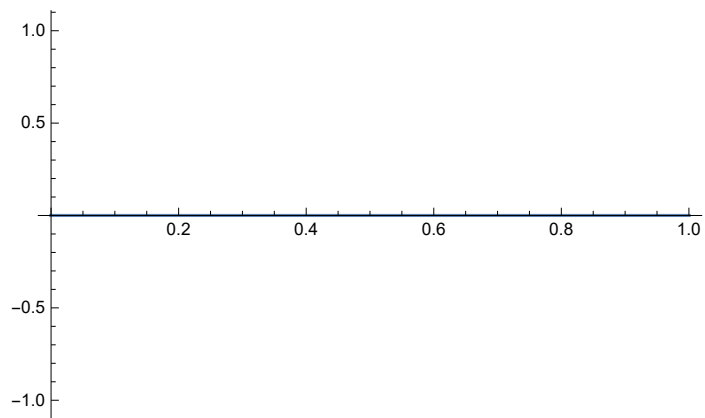

```
Plot[Cf[11, 1, 7], {x, 0, 1}]
```

[绘图](#)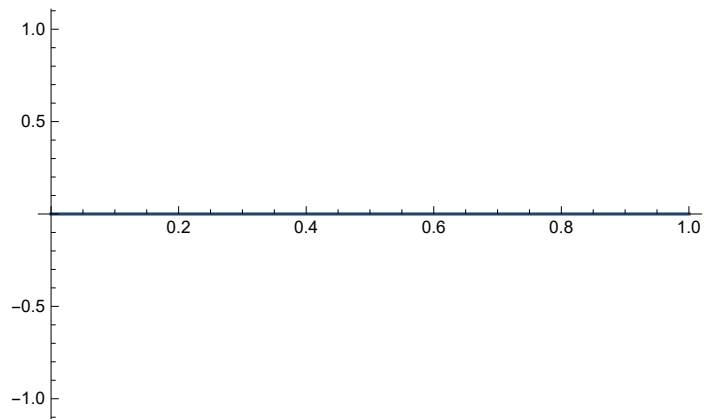

```
Plot[Cf[11, 1, 6], {x, 0, 1}]
```

[绘图](#)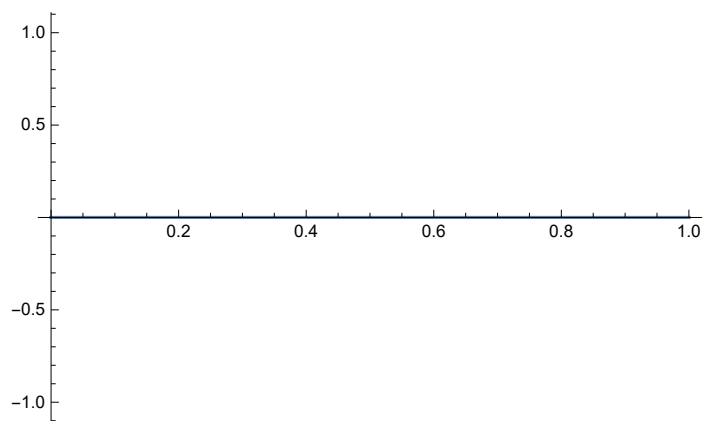

```
Plot[Cf[11, 1, 5], {x, 0, 1}]
```

[绘图](#)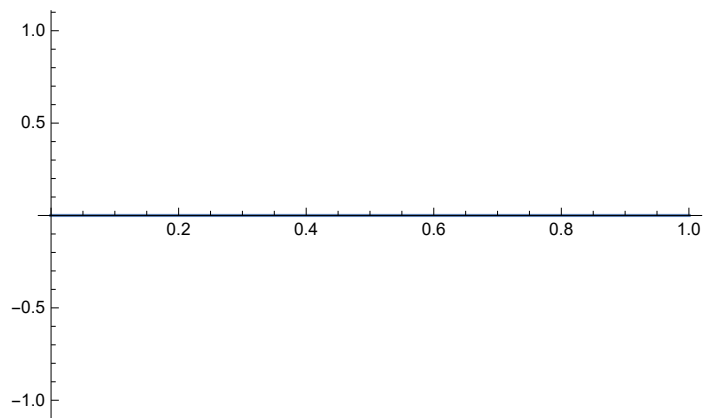

```
Plot[Cf[11, 1, 4], {x, 0, 1}]
```

[绘图](#)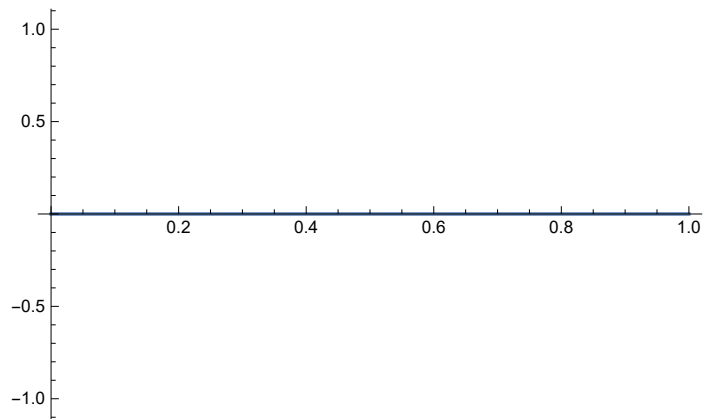

```
Plot[Cf[11, 1, 3], {x, 0, 1}]
```

[绘图](#)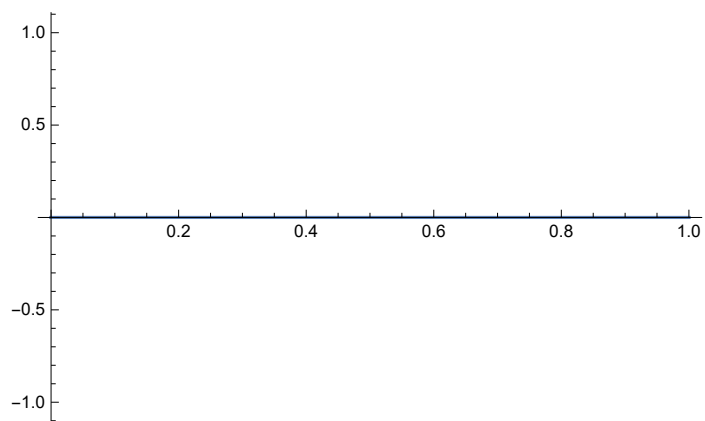

**Plot[Cf[11, 1, 2], {x, 0, 1}]**

[绘图](#)

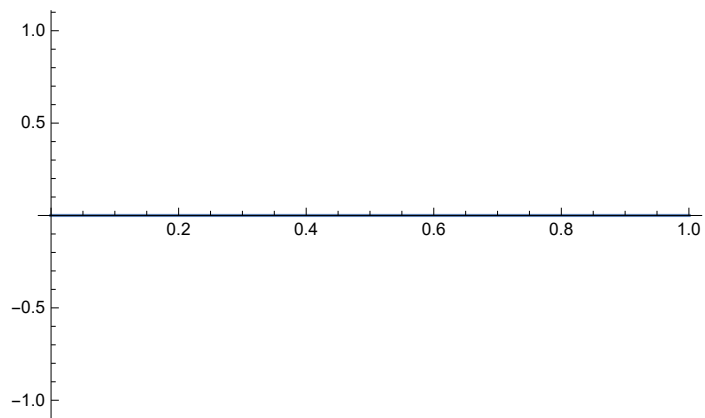

**Plot[Cf[11, 1, 1], {x, 0, 1}]**

[绘图](#)

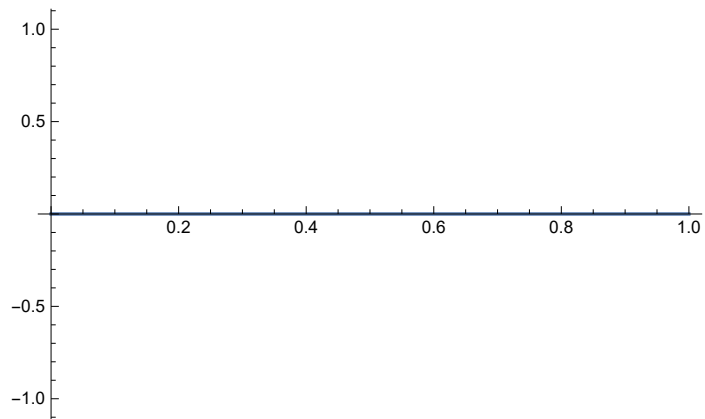

**Plot[Cf[11, 1, 0], {x, 0, 1}]**

[绘图](#)

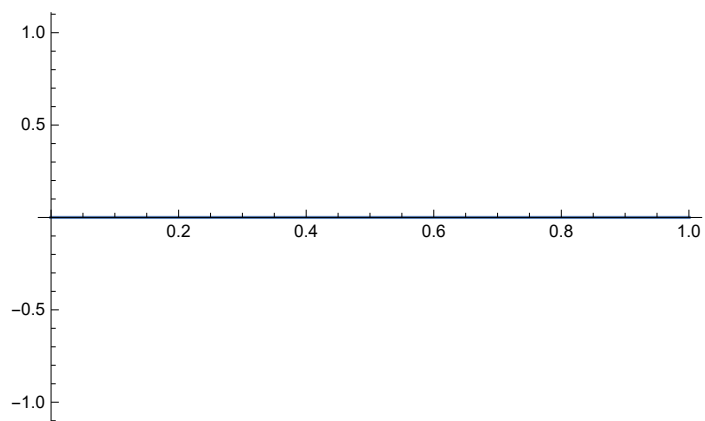

**(\*60th group coefficients r2^11r3^0\*)**

In[654]:= **Plot**[**Cf**[11, 0, 14], {x, 0, 1}]

[绘图](#)

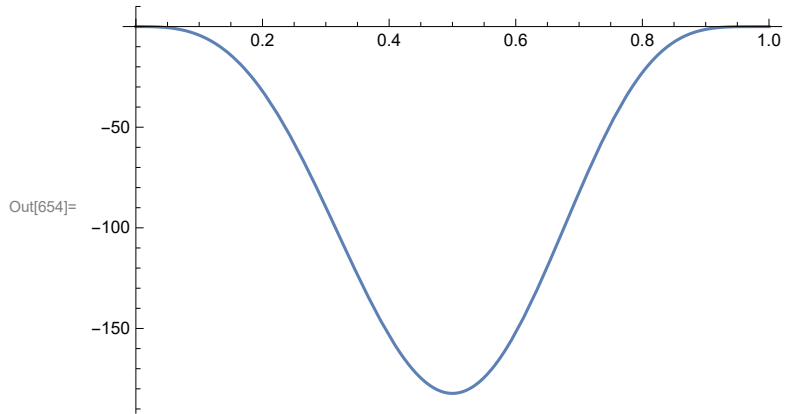

In[655]:= **Plot**[**Cf**[11, 0, 13], {x, 0, 1}]

[绘图](#)

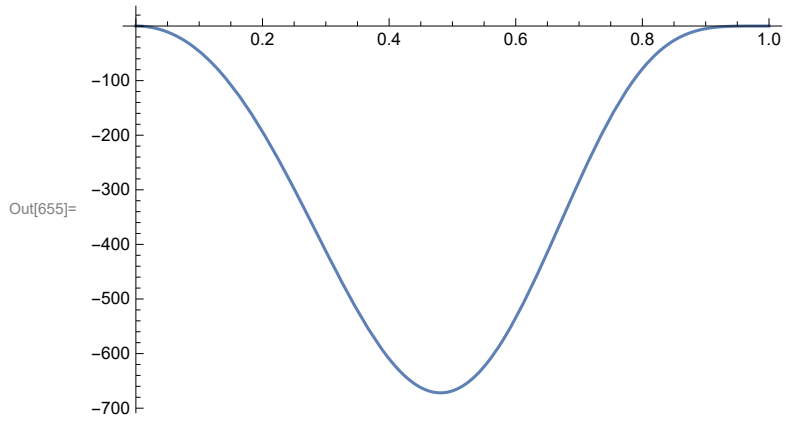

In[656]:= **Plot**[**Cf**[11, 0, 12], {x, 0, 1}]

[绘图](#)

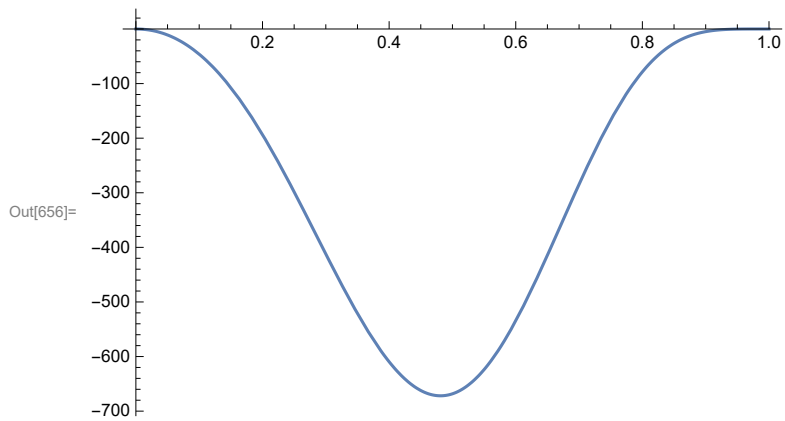

In[657]:= **Plot**[**Cf**[11, 0, 11], {x, 0, 1}]

[绘图](#)

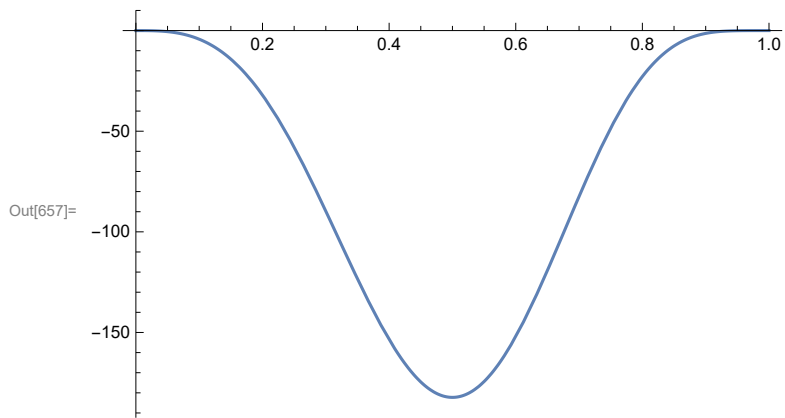

**Plot**[**Cf**[11, 0, 10], {x, 0, 1}]

[绘图](#)

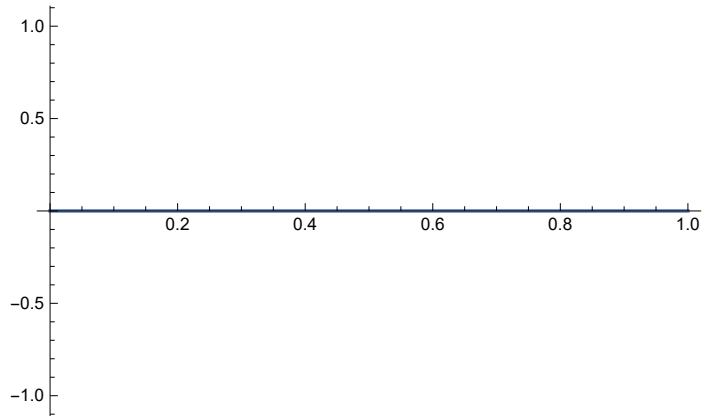

**Plot**[**Cf**[11, 0, 9], {x, 0, 1}]

[绘图](#)

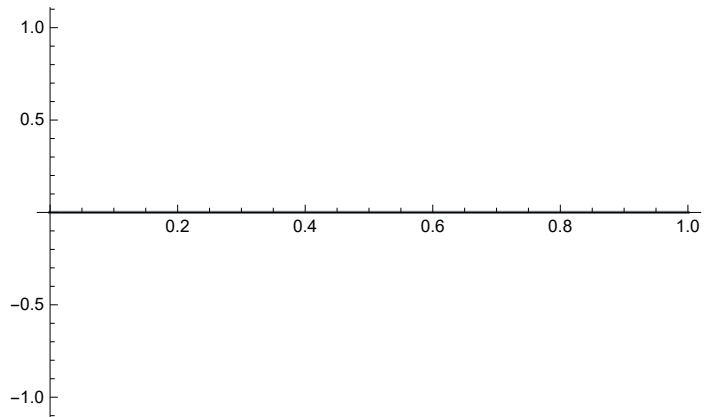

**Plot[Cf[11, 0, 8], {x, 0, 1}]**

[绘图](#)

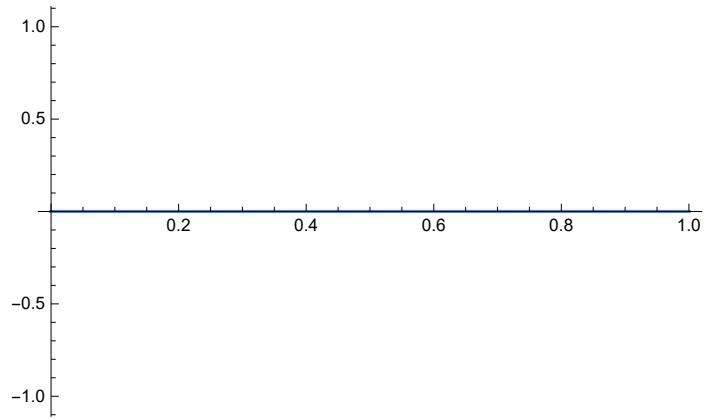

**Plot[Cf[11, 0, 7], {x, 0, 1}]**

[绘图](#)

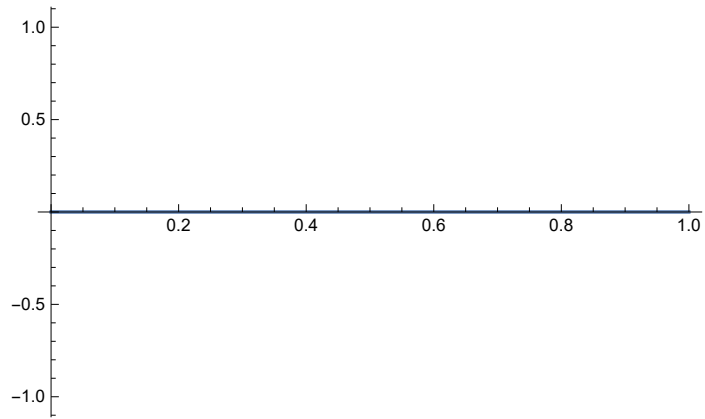

**Plot[Cf[11, 0, 6], {x, 0, 1}]**

[绘图](#)

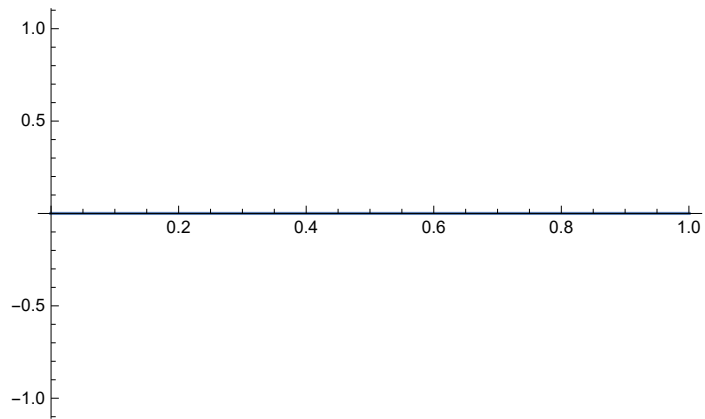

```
Plot[Cf[11, 0, 5], {x, 0, 1}]
```

[绘图](#)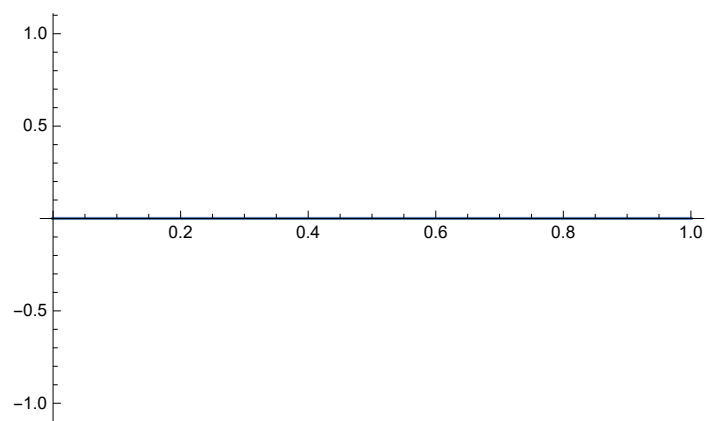

```
Plot[Cf[11, 0, 4], {x, 0, 1}]
```

[绘图](#)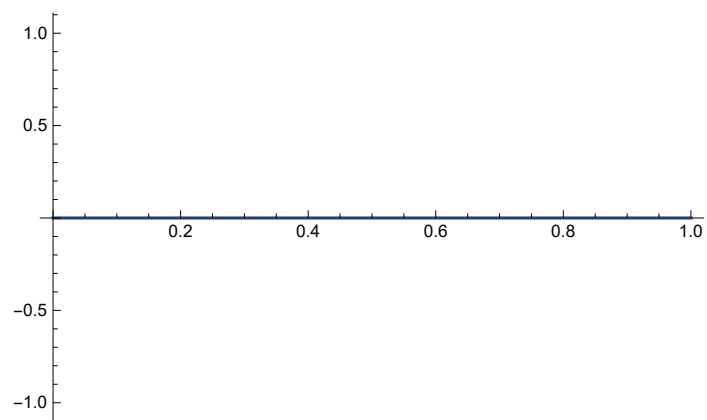



```
Plot[Cf[11, 0, 3], {x, 0, 1}]
```

[绘图](#)

```
Plot[Cf[11, 0, 2], {x, 0, 1}]
```

[绘图](#)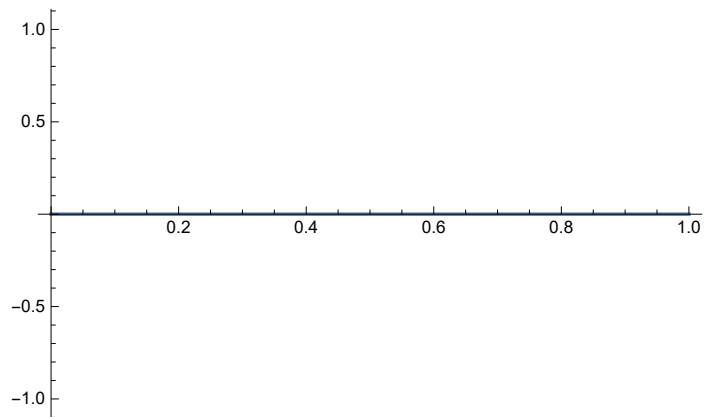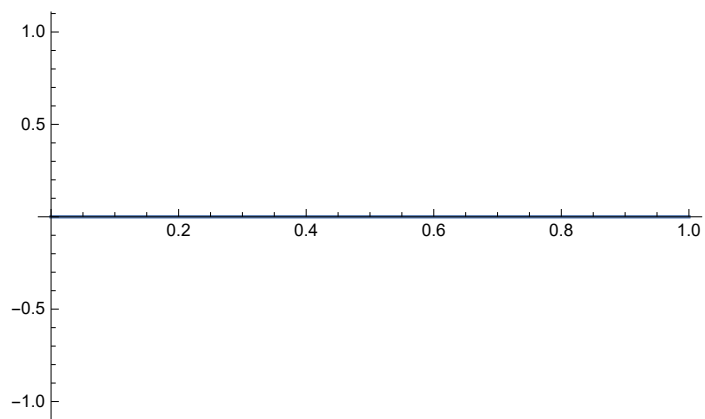

```
Plot[Cf[11, 0, 1], {x, 0, 1}]
```

[绘图](#)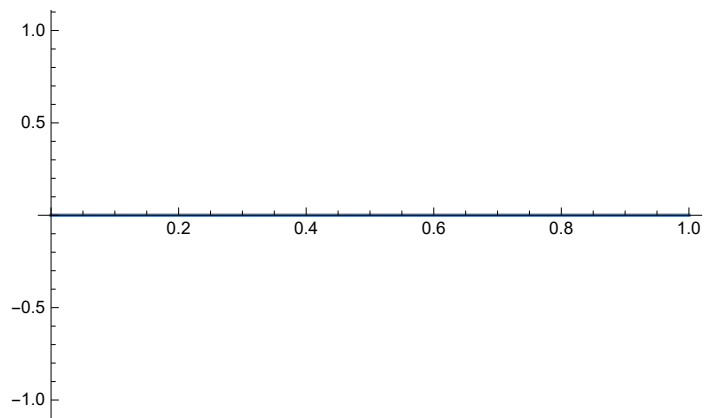

```
Plot[Cf[11, 0, 0], {x, 0, 1}]
```

[绘图](#)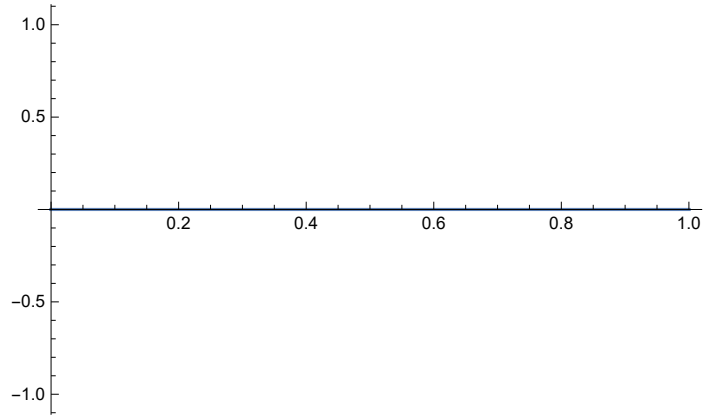

(\*61th group coefficients r2^10r3^14\*)

```
Plot[Cf[10, 14, 14], {x, 0, 1}]
```

[绘图](#)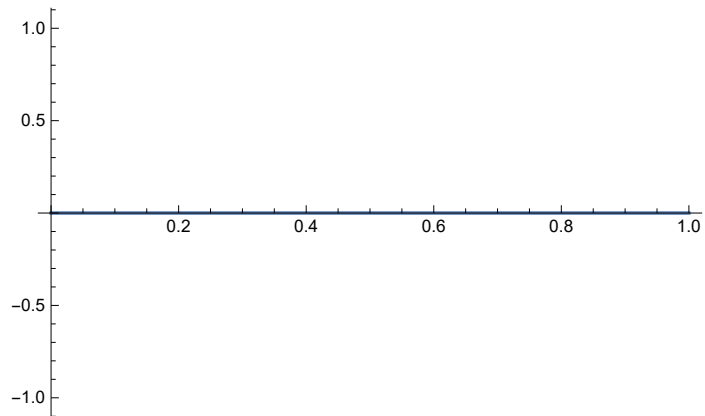

```
Plot[Cf[10, 14, 13], {x, 0, 1}]
```

[绘图](#)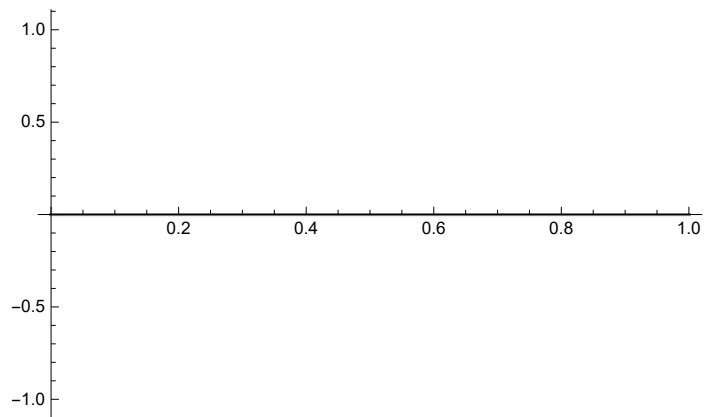

In[658]:= **Plot**[**Cf**[10, 14, 12], {x, 0, 1}]

[绘图](#)

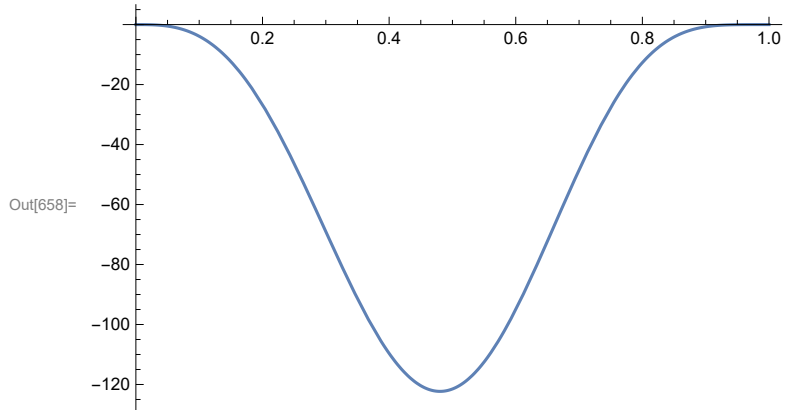

In[659]:= **Plot**[**Cf**[10, 14, 11], {x, 0, 1}]

[绘图](#)

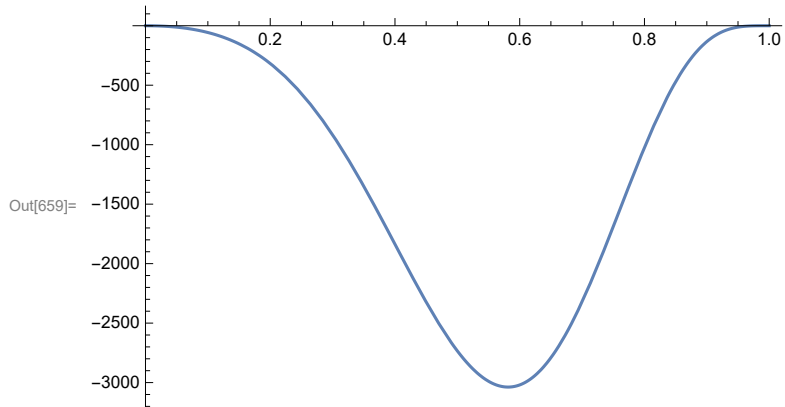

In[660]:= **Plot**[**Cf**[10, 14, 10], {x, 0, 1}]

[绘图](#)

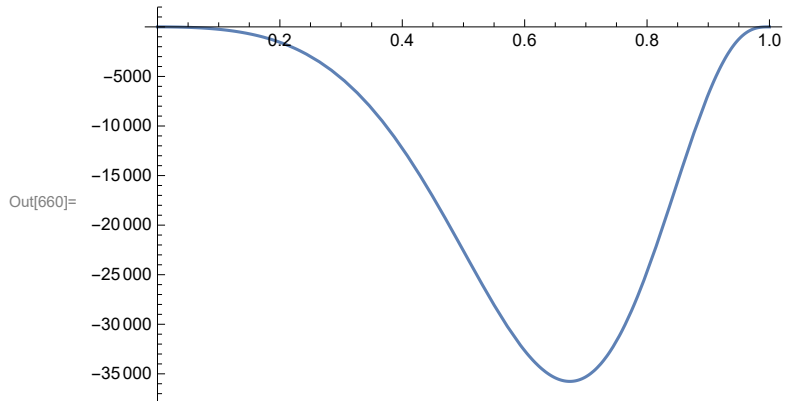

In[661]:= **Plot[Cf[10, 14, 9], {x, 0, 1}]**

[绘图](#)

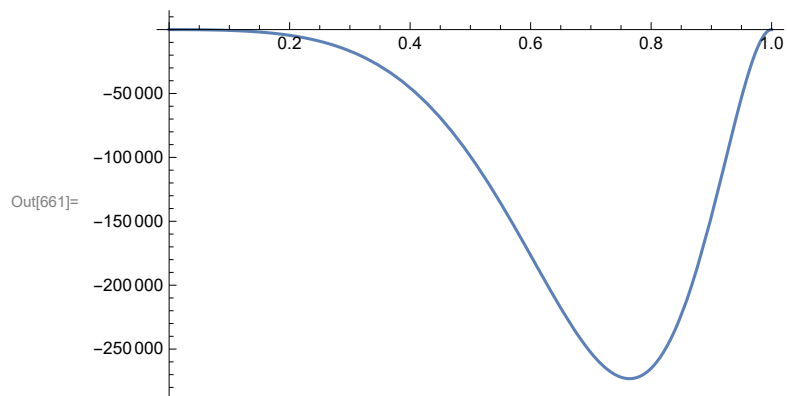

In[662]:= **Plot[Cf[10, 14, 8], {x, 0, 1}]**

[绘图](#)

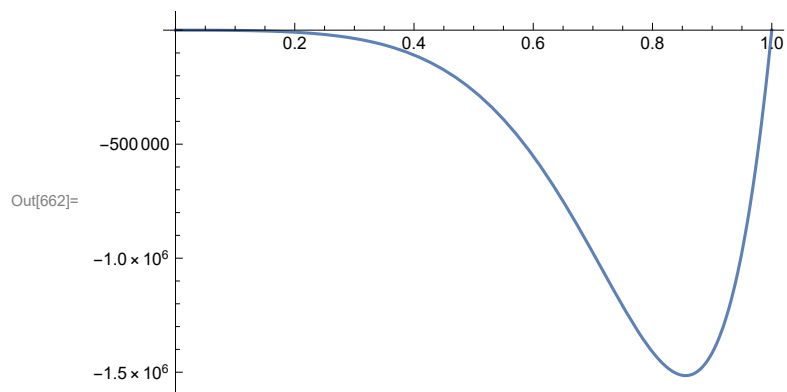

In[663]:= **Plot[Cf[10, 14, 7], {x, 0, 1}]**

[绘图](#)

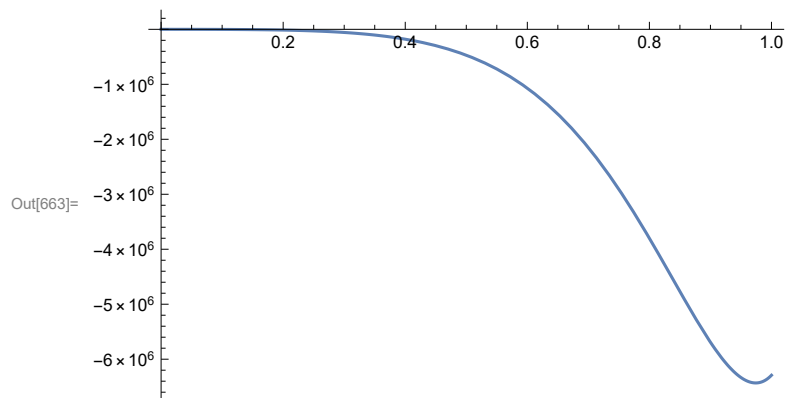

In[664]:= **Plot[Cf[10, 14, 6], {x, 0, 1}]**

[绘图](#)

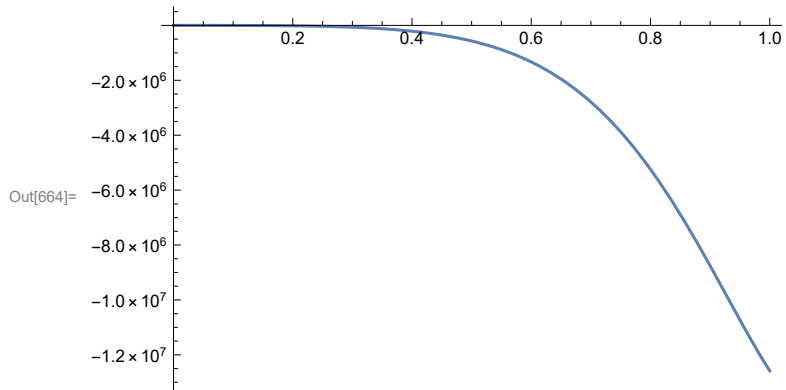

In[665]:= **Plot[Cf[10, 14, 5], {x, 0, 1}]**

[绘图](#)

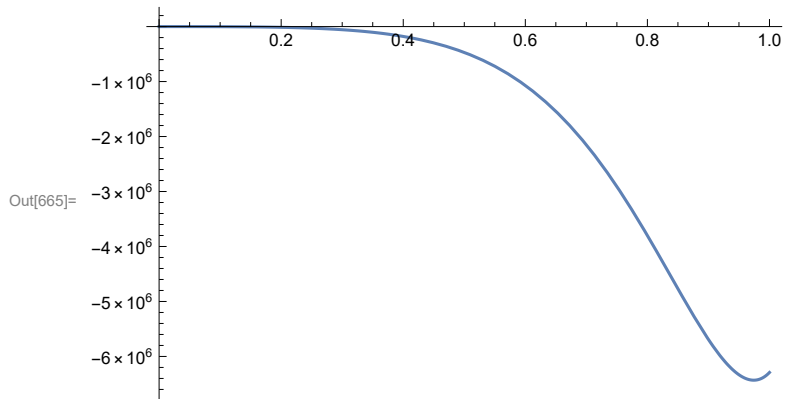

In[666]:= **Plot[Cf[10, 14, 4], {x, 0, 1}]**

[绘图](#)

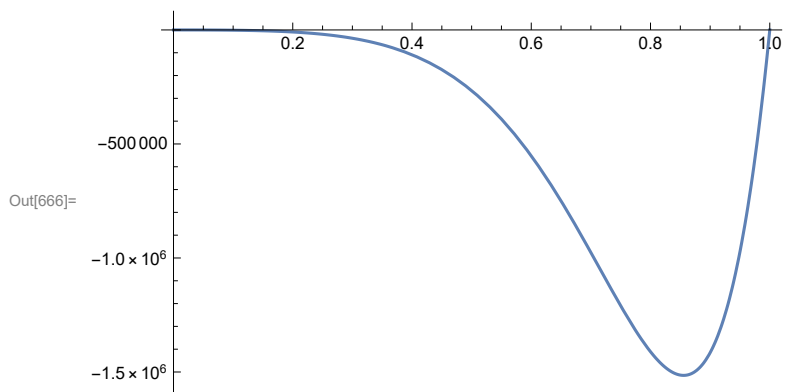

In[667]:= **Plot[Cf[10, 14, 3], {x, 0, 1}]**

[绘图](#)

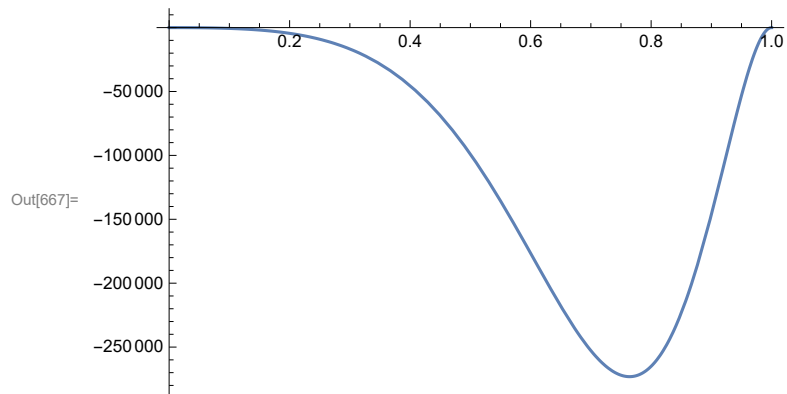

In[669]:= **Plot[Cf[10, 14, 2], {x, 0, 1}]**

[绘图](#)

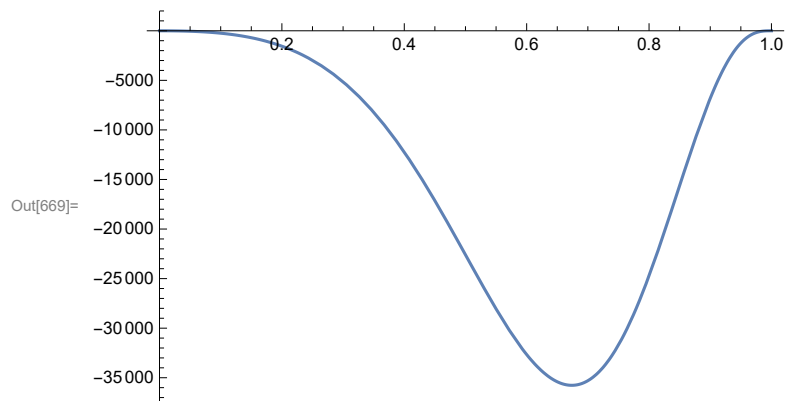

In[670]:= **Plot[Cf[10, 14, 1], {x, 0, 1}]**

[绘图](#)

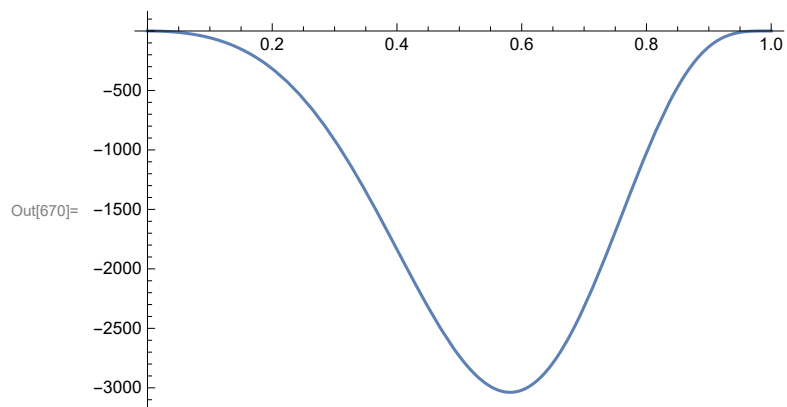

In[671]:= **Plot[Cf[10, 14, 0], {x, 0, 1}]**

[绘图](#)

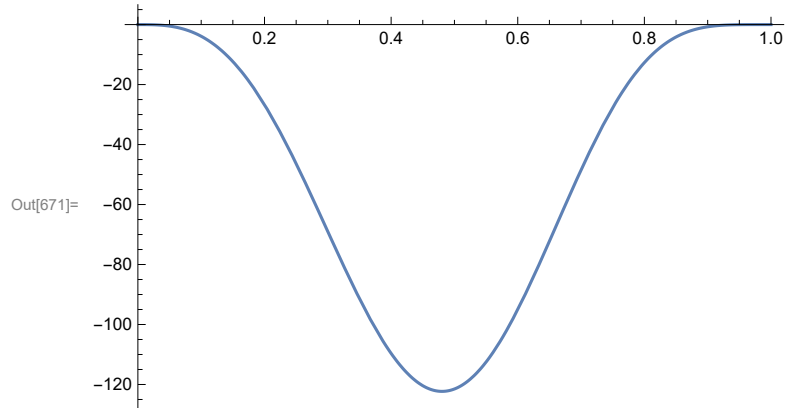

(\*62th group coefficients  $r^2^{10}r^3^{13}$ \*)

**Plot[Cf[10, 13, 14], {x, 0, 1}]**

[绘图](#)

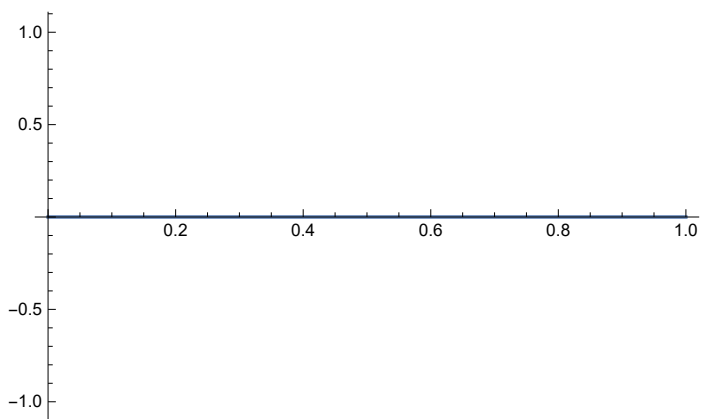

In[672]:= **Plot[Cf[10, 13, 13], {x, 0, 1}]**

[绘图](#)

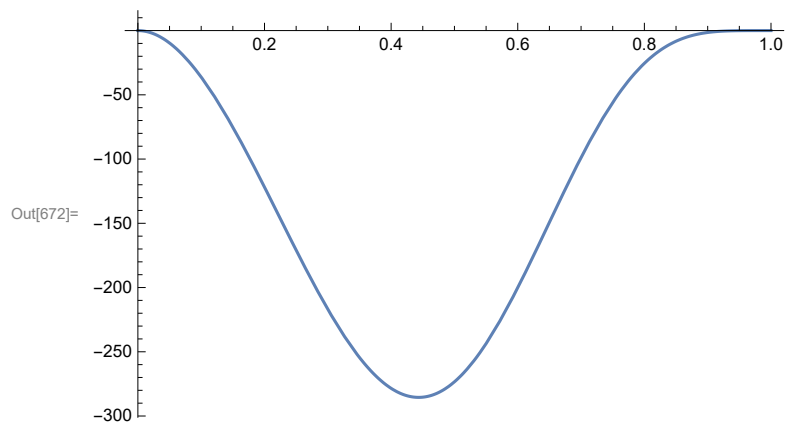

In[673]:= **Plot[Cf[10, 13, 12], {x, 0, 1}]**

[绘图](#)

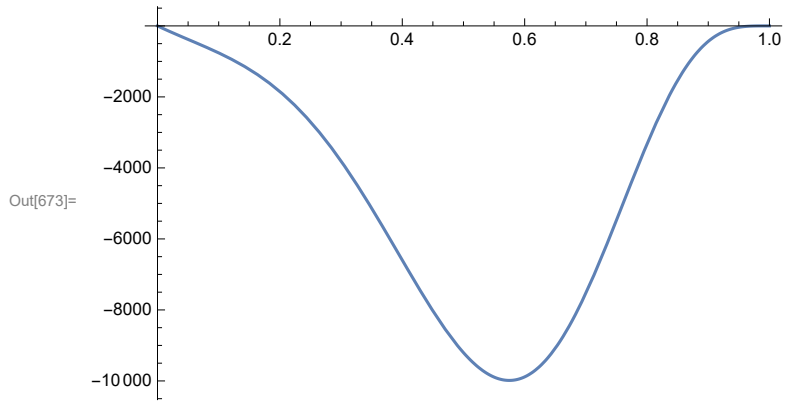

In[674]:= **Plot[Cf[10, 13, 11], {x, 0, 1}]**

[绘图](#)

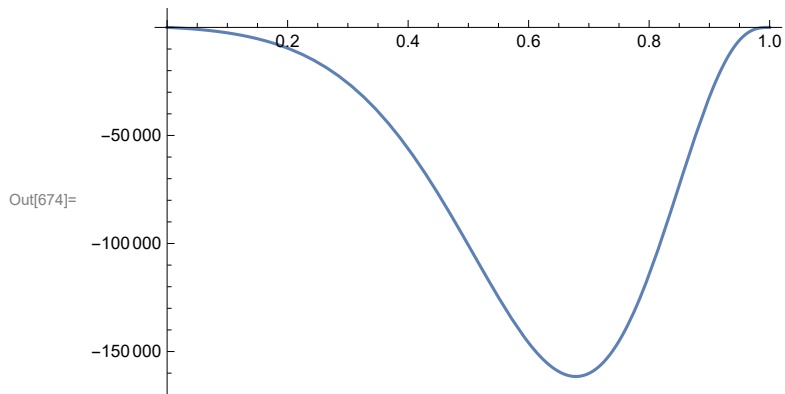

In[675]:= **Plot[Cf[10, 13, 10], {x, 0, 1}]**

[绘图](#)

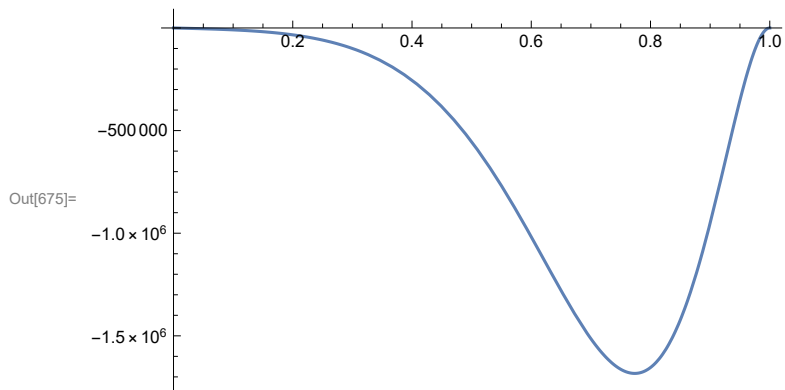



In[676]:= **Plot[Cf[10, 13, 9], {x, 0, 1}]**

[绘图](#)

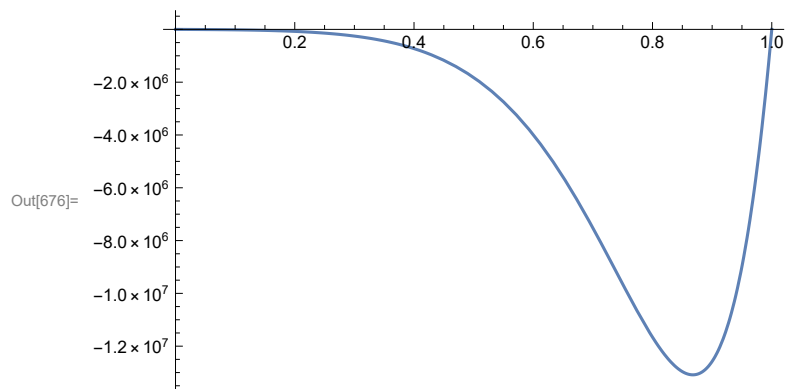

In[677]:= **Plot[Cf[10, 13, 8], {x, 0, 1}]**

[绘图](#)

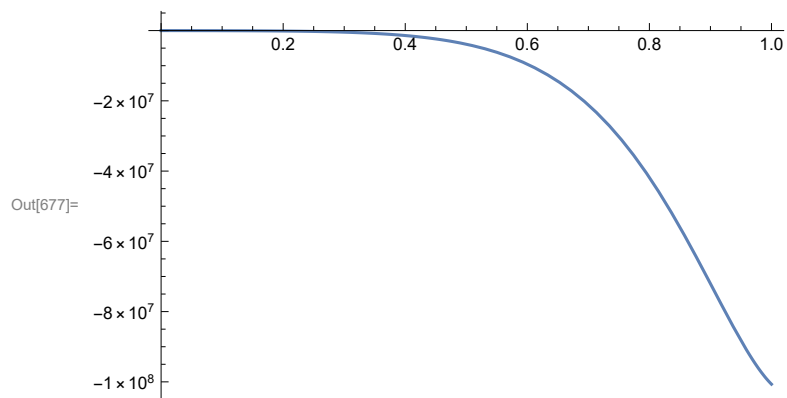

In[678]:= **Plot[Cf[10, 13, 7], {x, 0, 1}]**

[绘图](#)

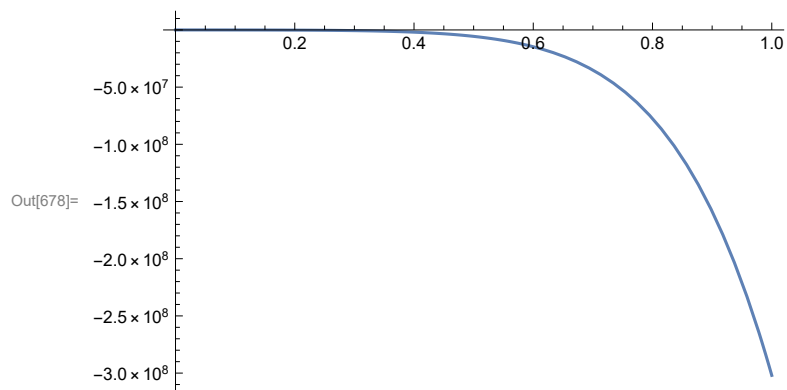

In[679]:= **Plot[Cf[10, 13, 6], {x, 0, 1}]**

[绘图](#)

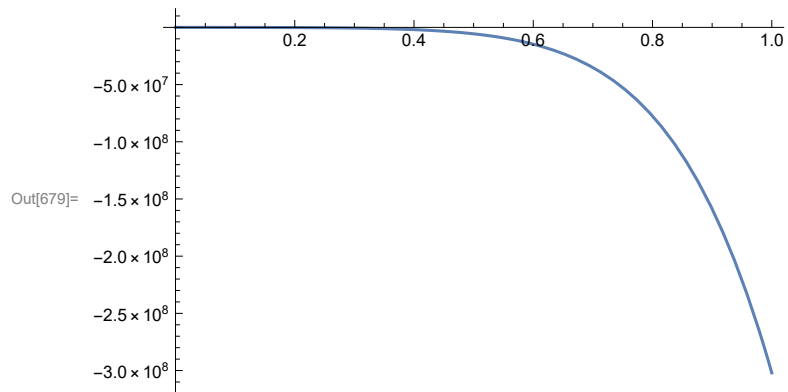

In[680]:= **Plot[Cf[10, 13, 5], {x, 0, 1}]**

[绘图](#)

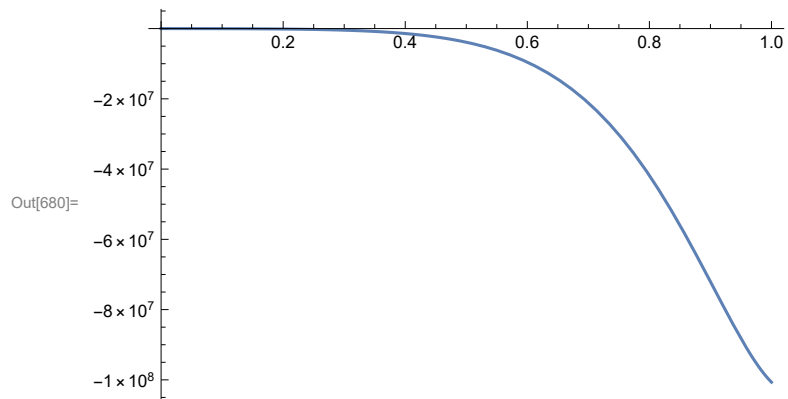

In[681]:= **Plot[Cf[10, 13, 4], {x, 0, 1}]**

[绘图](#)

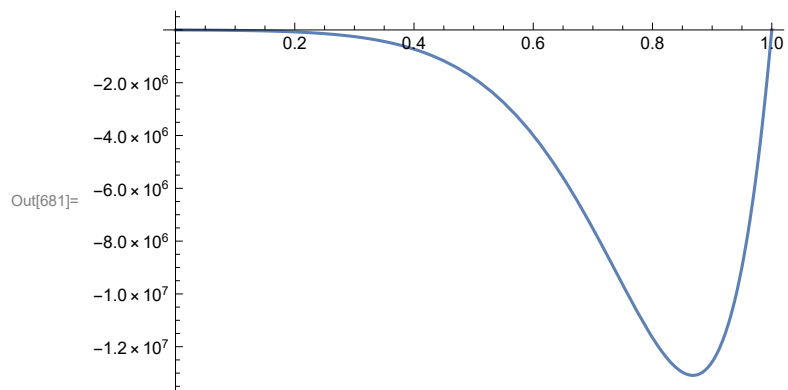

In[682]:= **Plot[Cf[10, 13, 3], {x, 0, 1}]**

[绘图](#)

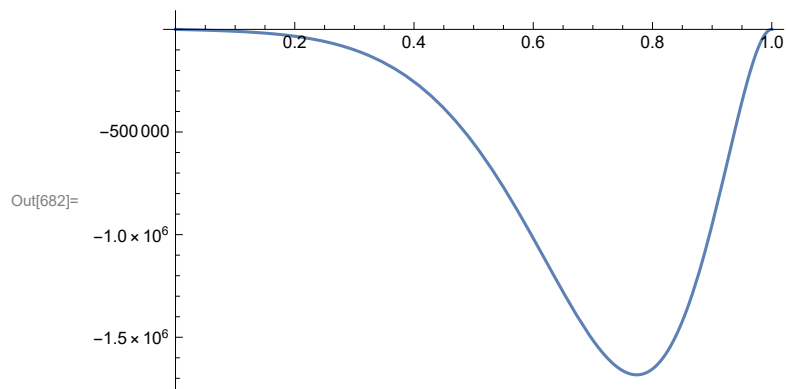

In[683]:= **Plot[Cf[10, 13, 2], {x, 0, 1}]**

[绘图](#)

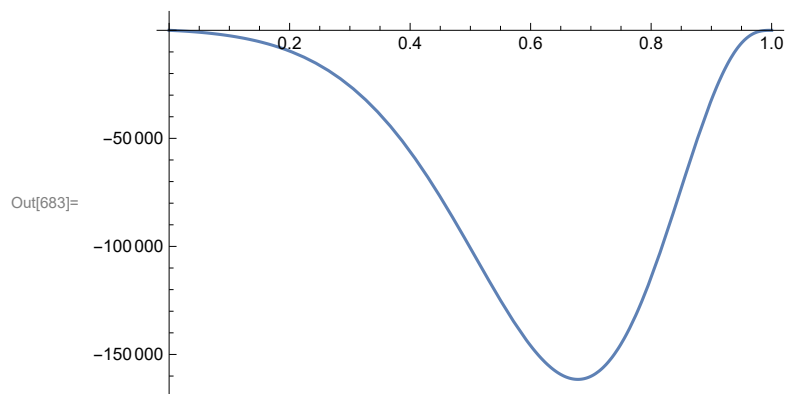

In[684]:= **Plot[Cf[10, 13, 1], {x, 0, 1}]**

[绘图](#)

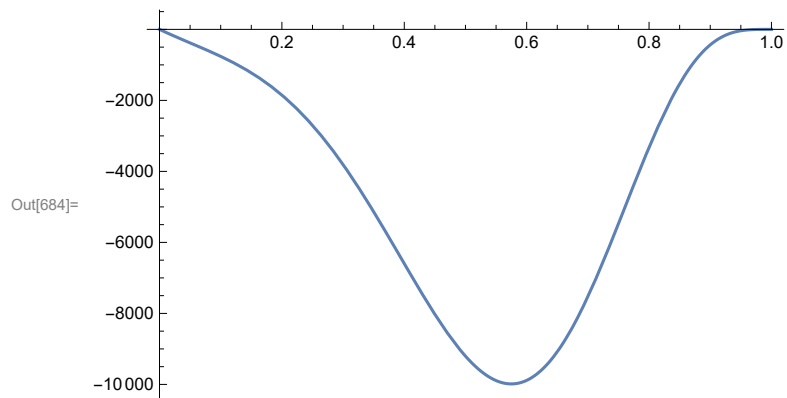

In[685]:= **Plot[Cf[10, 13, 0], {x, 0, 1}]**

[绘图](#)

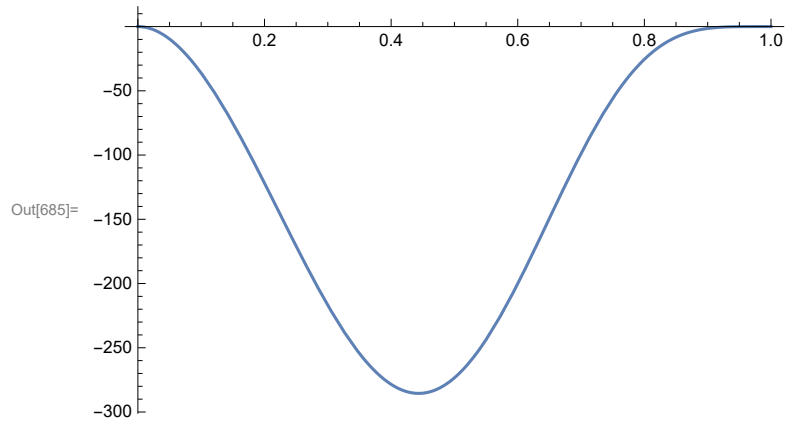

(\*63th group coefficients  $r^2^{10}r^3^{12}$ \*)

In[686]:= **Plot[Cf[10, 12, 14], {x, 0, 1}]**

[绘图](#)

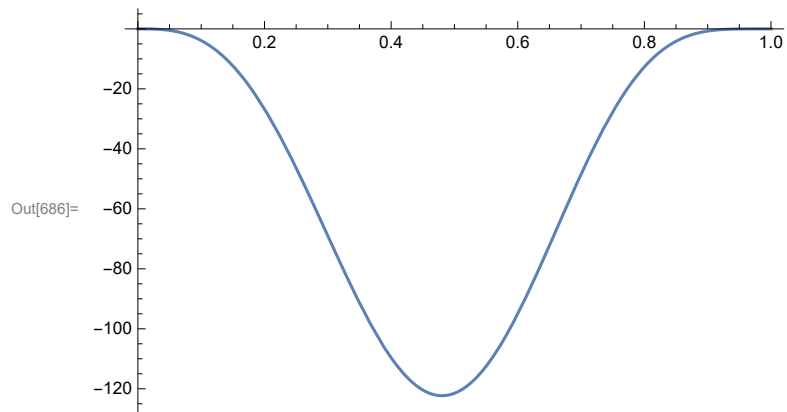

In[687]:= **Plot[Cf[10, 12, 13], {x, 0, 1}]**

[绘图](#)

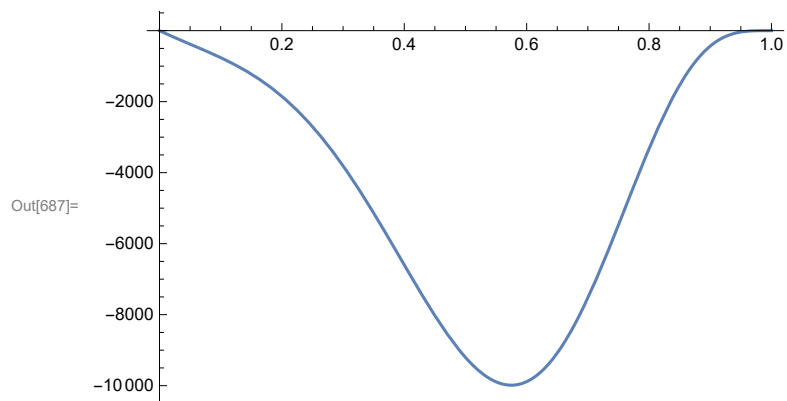

In[688]:= **Plot**[**Cf**[10, 12, 12], {x, 0, 1}]

[绘图](#)

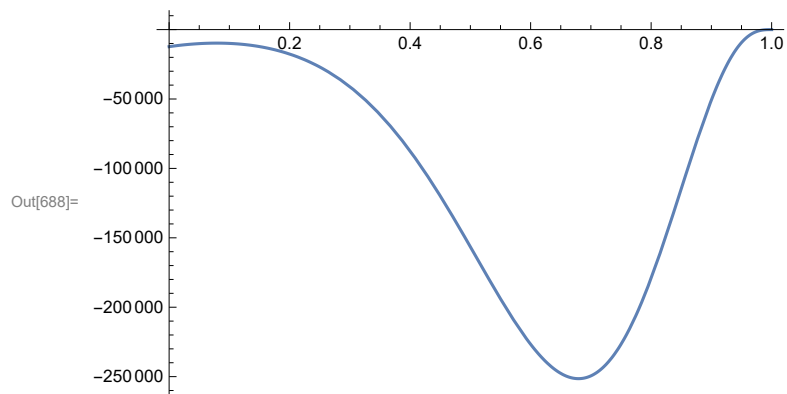

In[689]:= **Plot**[**Cf**[10, 12, 11], {x, 0, 1}]

[绘图](#)

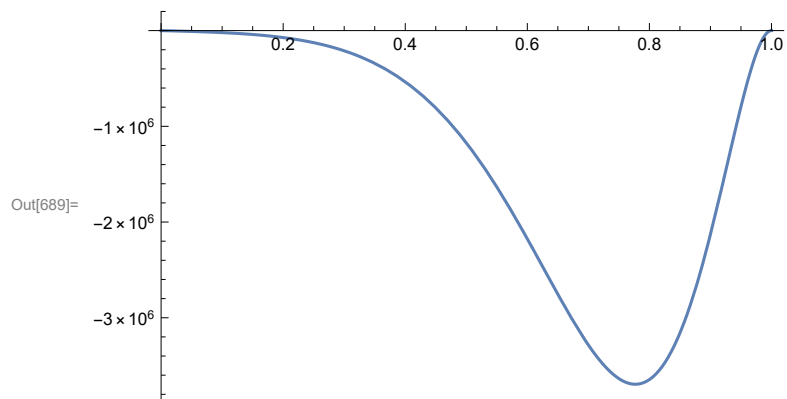

In[690]:= **Plot**[**Cf**[10, 12, 10], {x, 0, 1}]

[绘图](#)

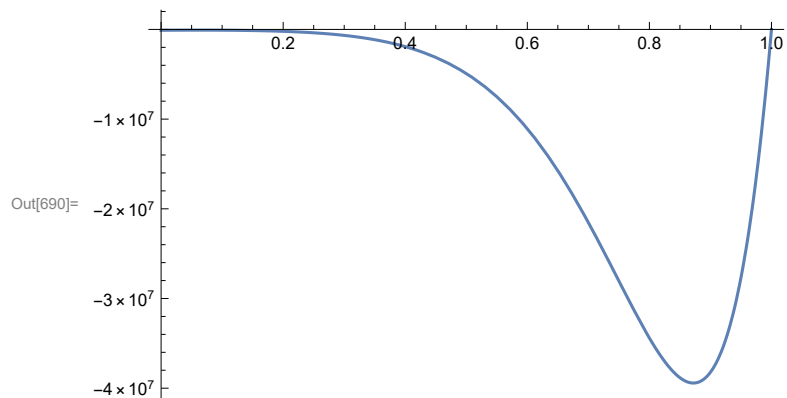

In[691]:= **Plot[Cf[10, 12, 9], {x, 0, 1}]**

[绘图](#)

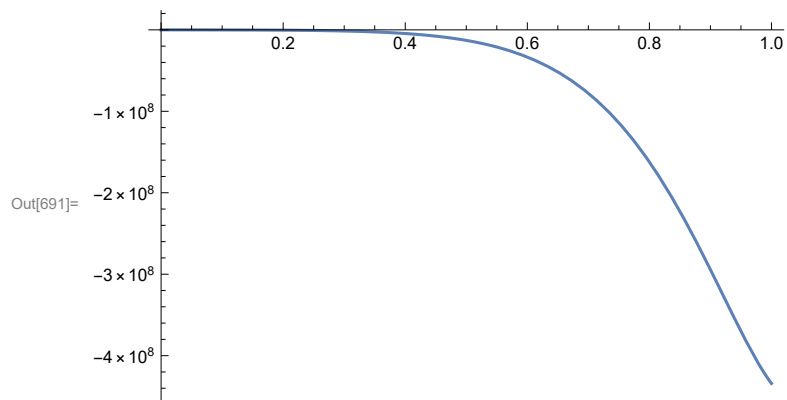

In[692]:= **Plot[Cf[10, 12, 8], {x, 0, 1}]**

[绘图](#)

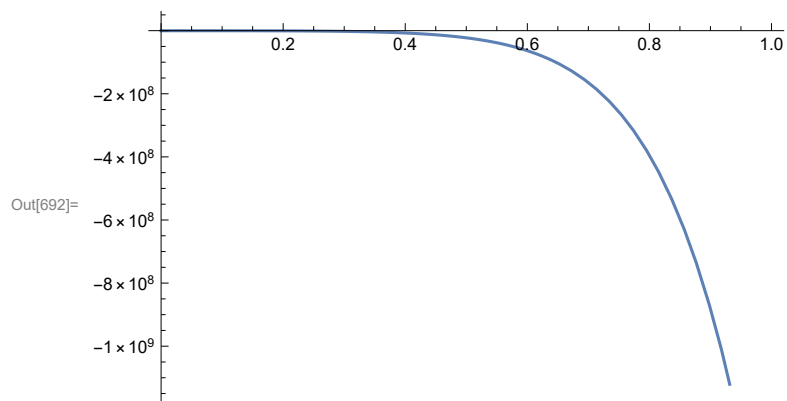

In[693]:= **Plot[Cf[10, 12, 7], {x, 0, 1}]**

[绘图](#)

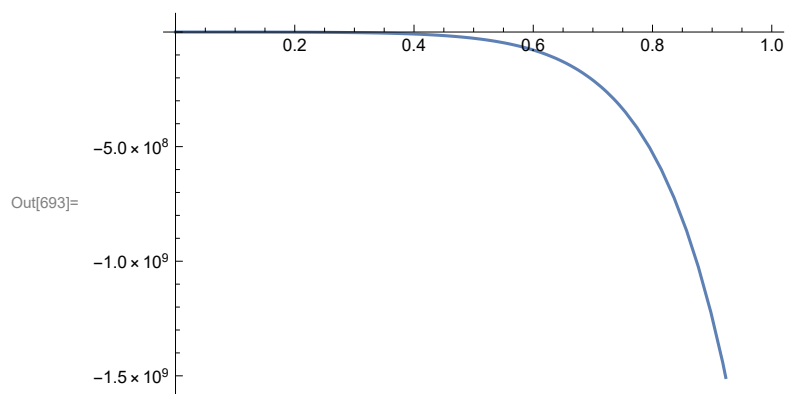

In[694]:= **Plot[Cf[10, 12, 6], {x, 0, 1}]**

[绘图](#)

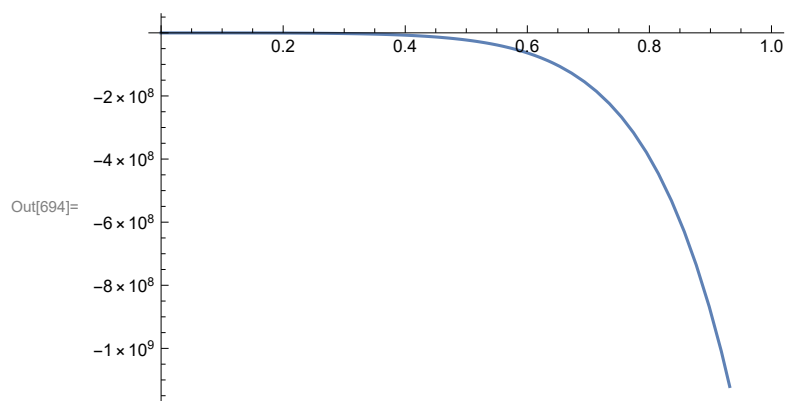

In[695]:= **Plot[Cf[10, 12, 5], {x, 0, 1}]**

[绘图](#)

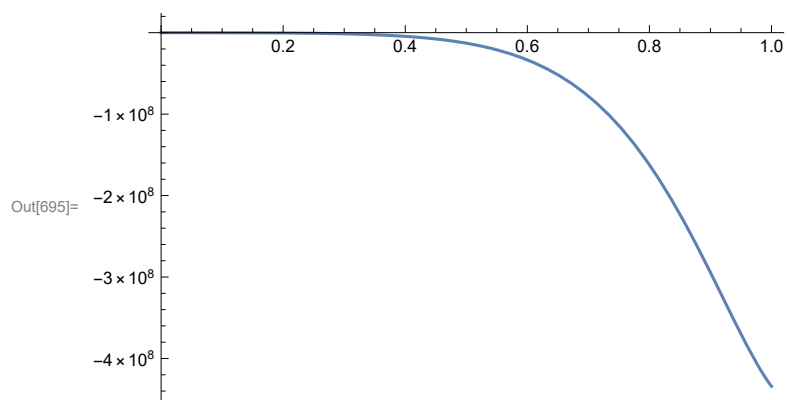

In[696]:= **Plot[Cf[10, 12, 4], {x, 0, 1}]**

[绘图](#)

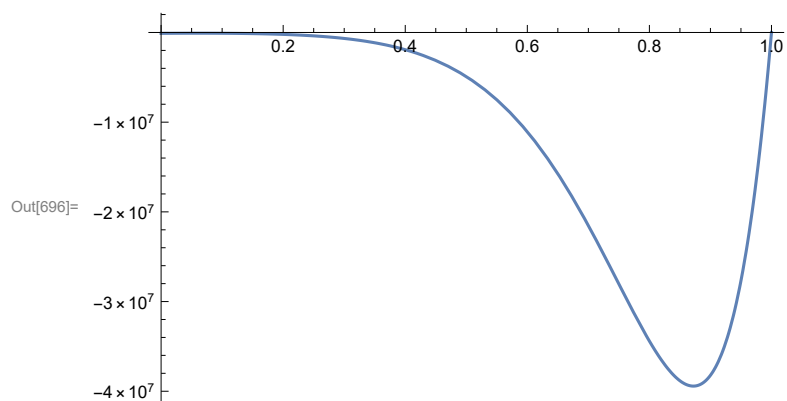

In[697]:= **Plot[Cf[10, 12, 3], {x, 0, 1}]**

[绘图](#)

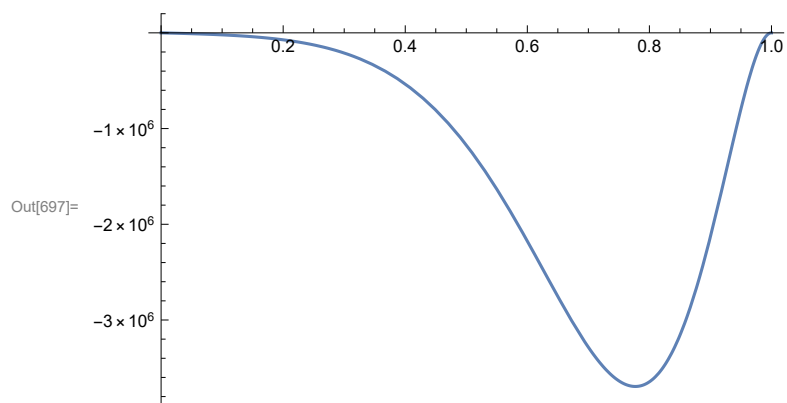

In[698]:= **Plot[Cf[10, 12, 2], {x, 0, 1}]**

[绘图](#)

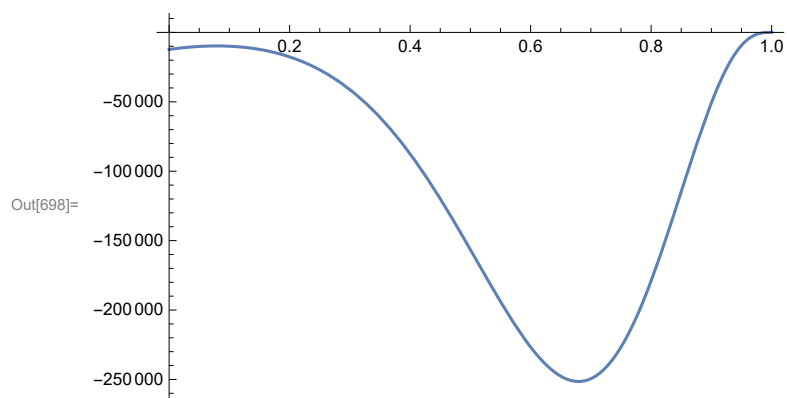

In[699]:= **Plot[Cf[10, 12, 1], {x, 0, 1}]**

[绘图](#)

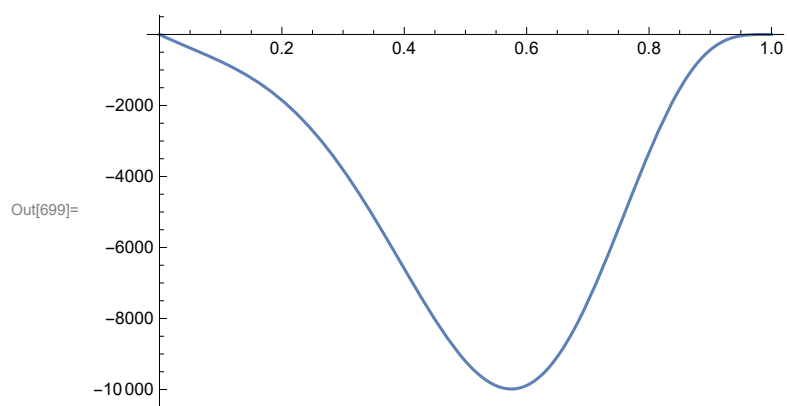



In[700]:= **Plot[Cf[10, 12, 0], {x, 0, 1}]**

[绘图](#)

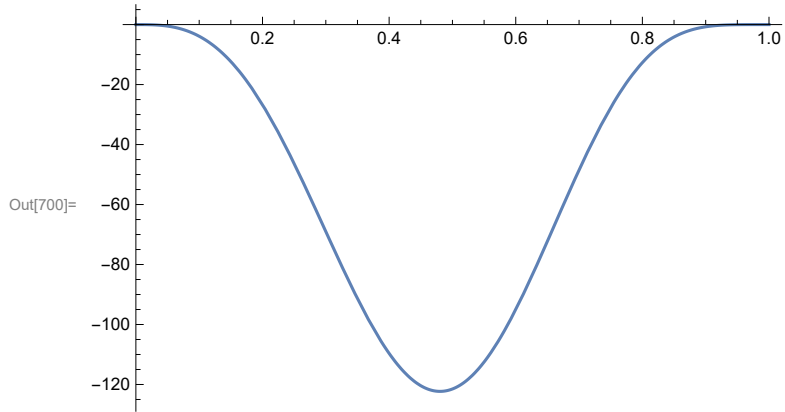

(\*64th group coefficients r2^10r3^11\*)

In[701]:= **Plot[Cf[10, 11, 14], {x, 0, 1}]**

[绘图](#)

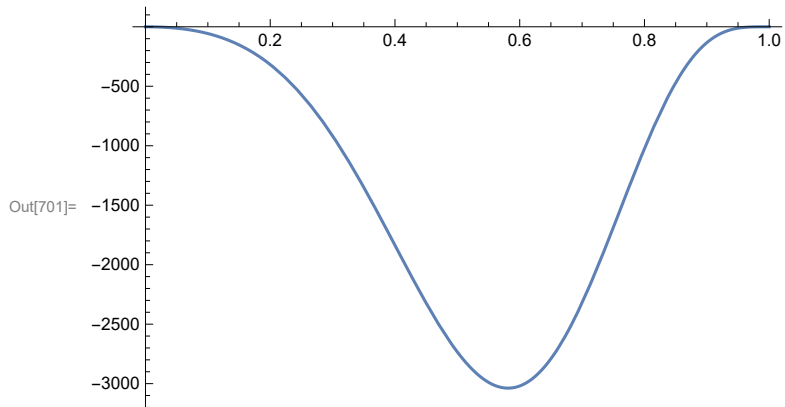

In[702]:= **Plot[Cf[10, 11, 13], {x, 0, 1}]**

[绘图](#)

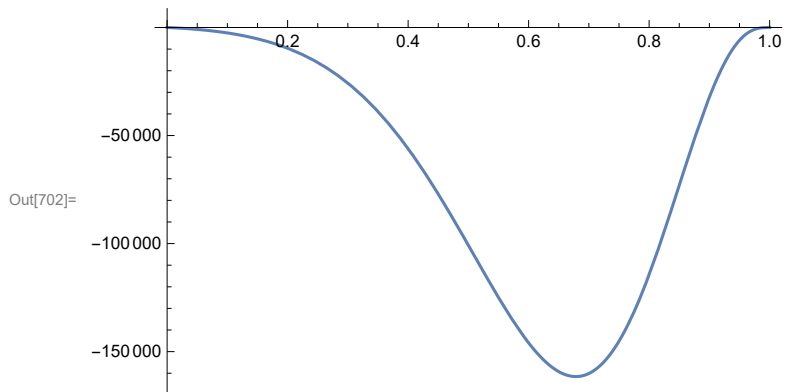

In[703]:= **Plot[Cf[10, 11, 12], {x, 0, 1}]**

[绘图](#)

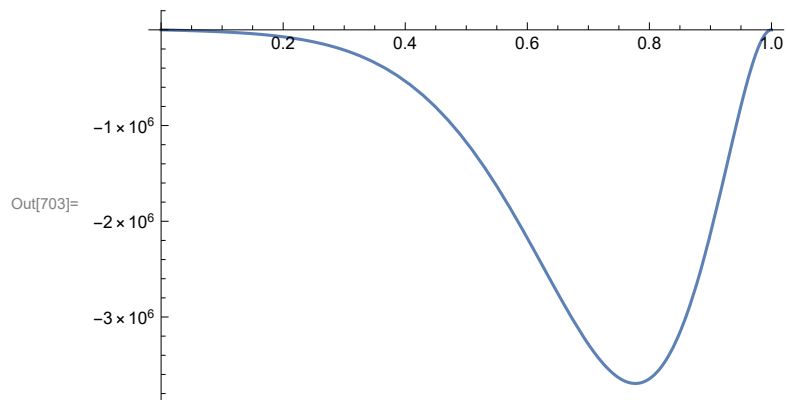

In[704]:= **Plot[Cf[10, 11, 11], {x, 0, 1}]**

[绘图](#)

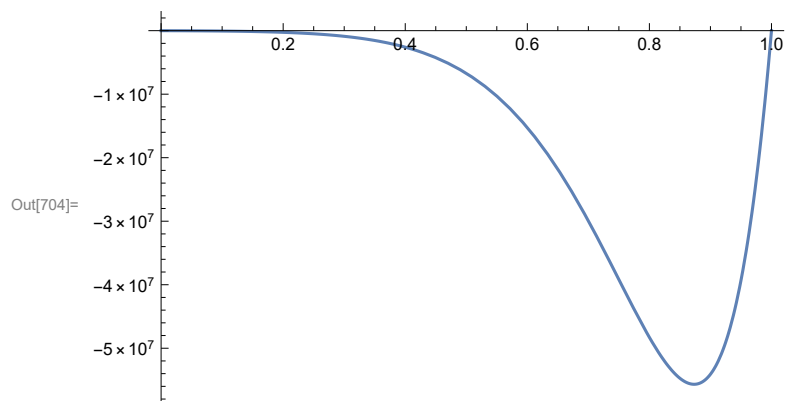

In[705]:= **Plot[Cf[10, 11, 10], {x, 0, 1}]**

[绘图](#)

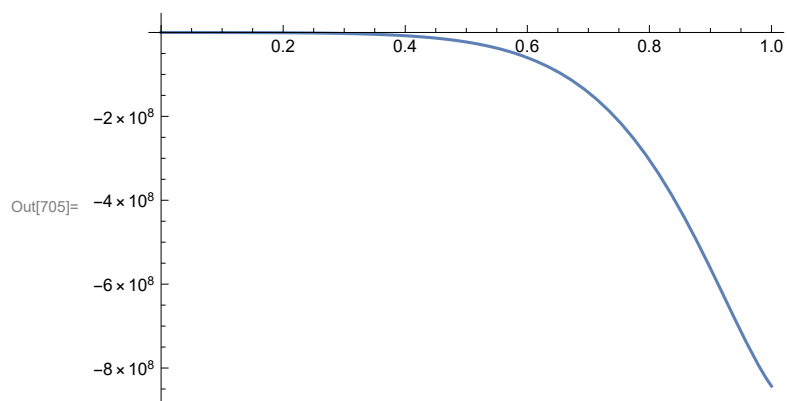

In[706]:= **Plot[Cf[10, 11, 9], {x, 0, 1}]**

[绘图](#)

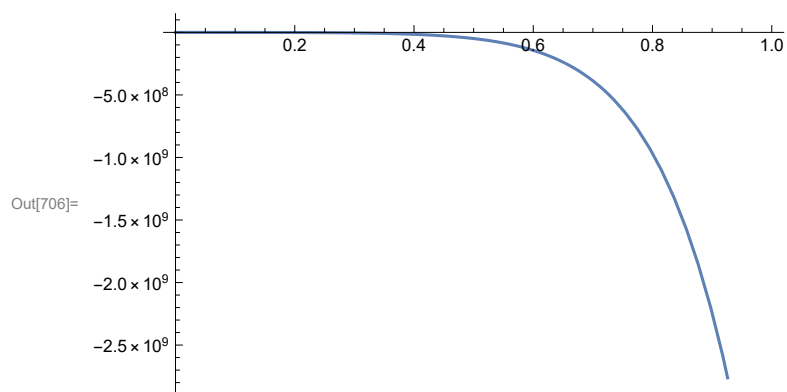

In[707]:= **Plot[Cf[10, 11, 8], {x, 0, 1}]**

[绘图](#)

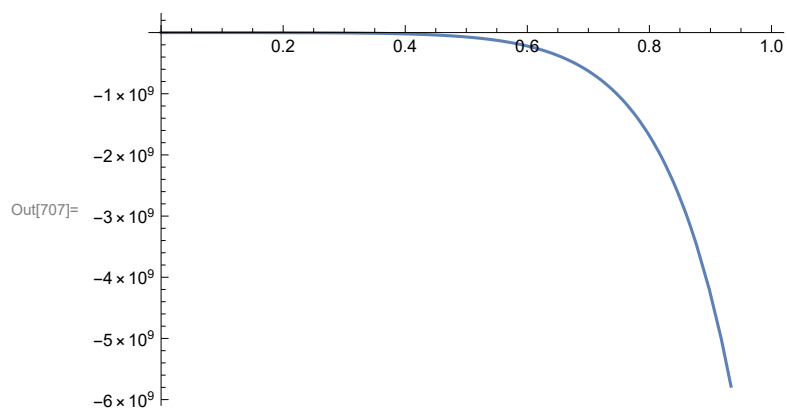

In[708]:= **Plot[Cf[10, 11, 7], {x, 0, 1}]**

[绘图](#)

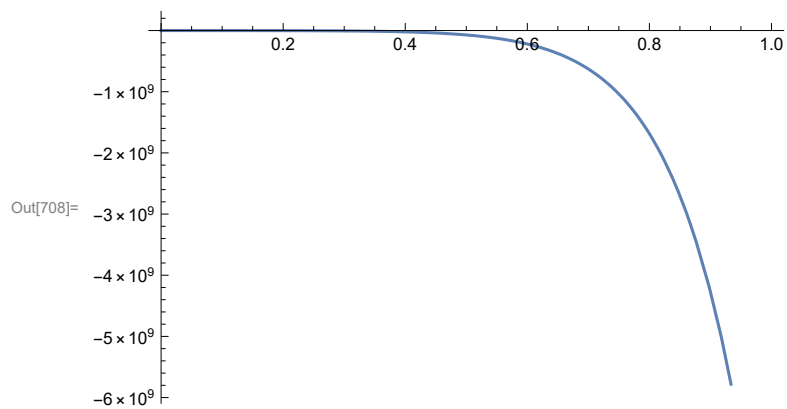

In[709]:= **Plot[Cf[10, 11, 8], {x, 0, 1}]**

[绘图](#)

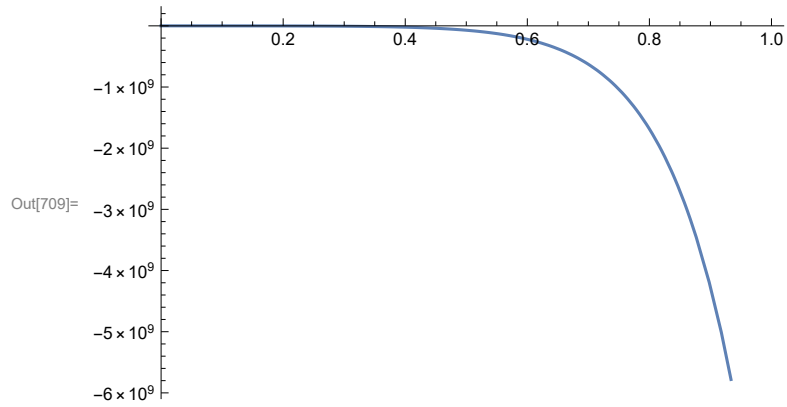

In[710]:= **Plot[Cf[10, 11, 7], {x, 0, 1}]**

[绘图](#)

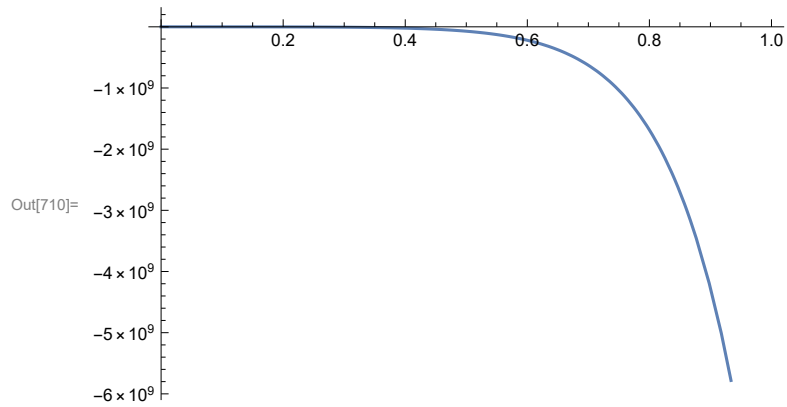

In[711]:= **Plot[Cf[10, 11, 6], {x, 0, 1}]**

[绘图](#)

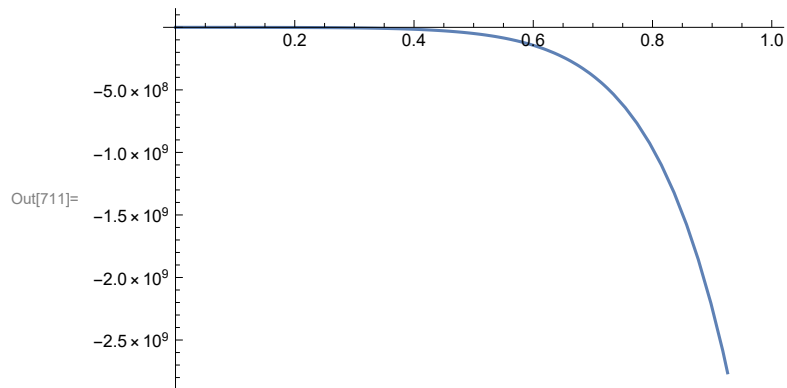

In[712]:= **Plot**[**Cf**[10, 11, 5], {x, 0, 1}]

[绘图](#)

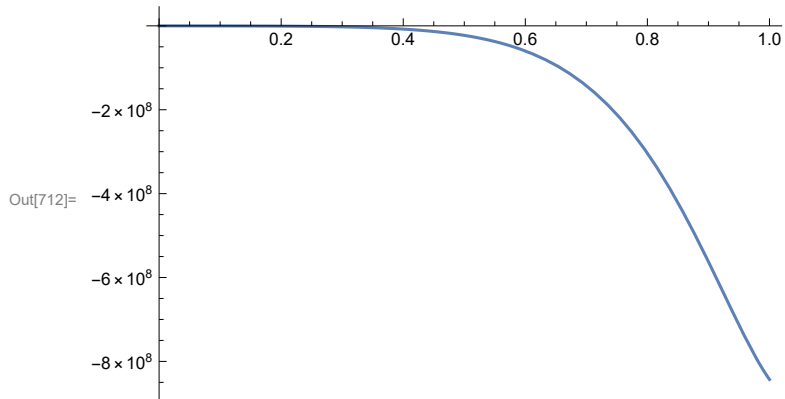

In[713]:= **Plot**[**Cf**[10, 11, 4], {x, 0, 1}]

[绘图](#)

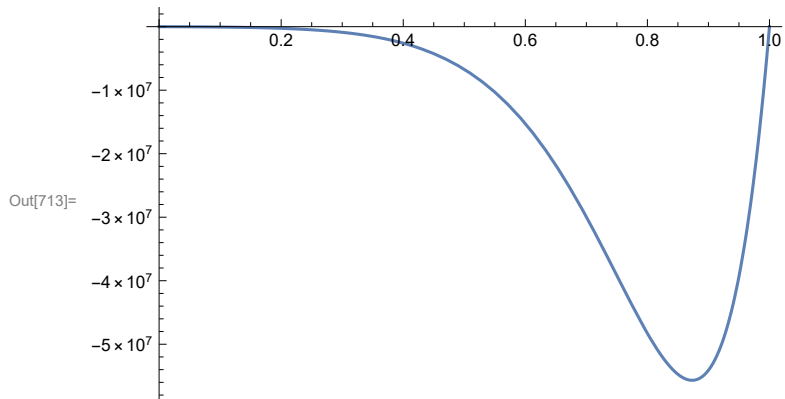

In[714]:= **Plot**[**Cf**[10, 11, 3], {x, 0, 1}]

[绘图](#)

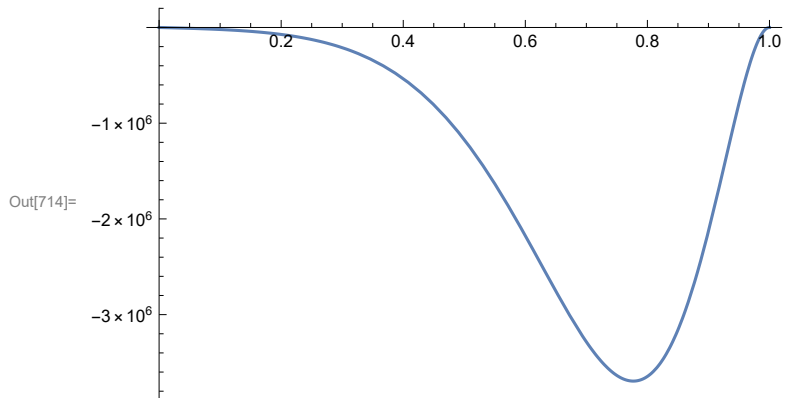

In[715]:= **Plot[Cf[10, 11, 2], {x, 0, 1}]**

[绘图](#)

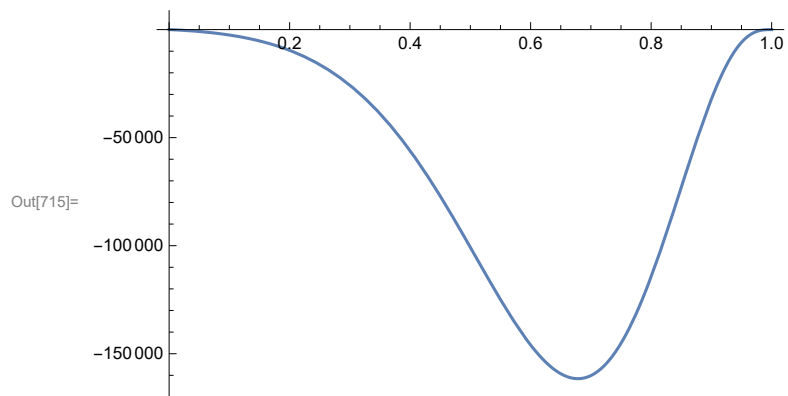

In[716]:= **Plot[Cf[10, 11, 1], {x, 0, 1}]**

[绘图](#)

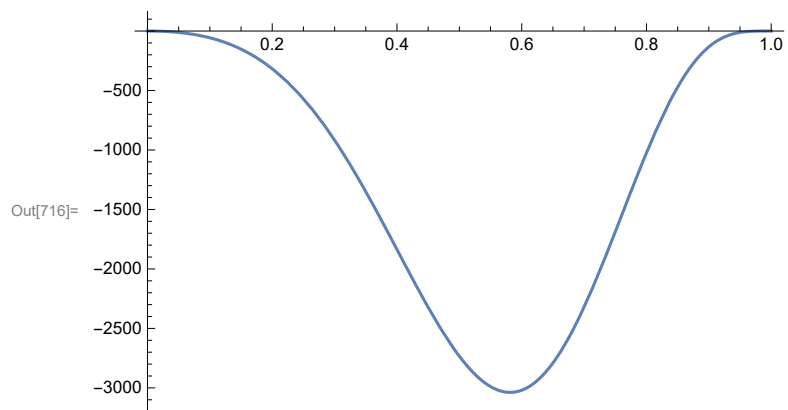

**Plot[Cf[10, 11, 0], {x, 0, 1}]**

[绘图](#)

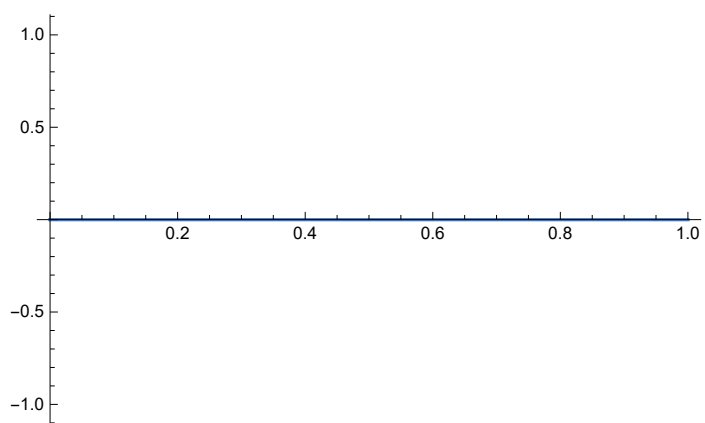

(\*65th group coefficients r2^10r3^10\*)

In[717]:= **Plot**[**Cf**[10, 10, 14], {x, 0, 1}]

[绘图](#)

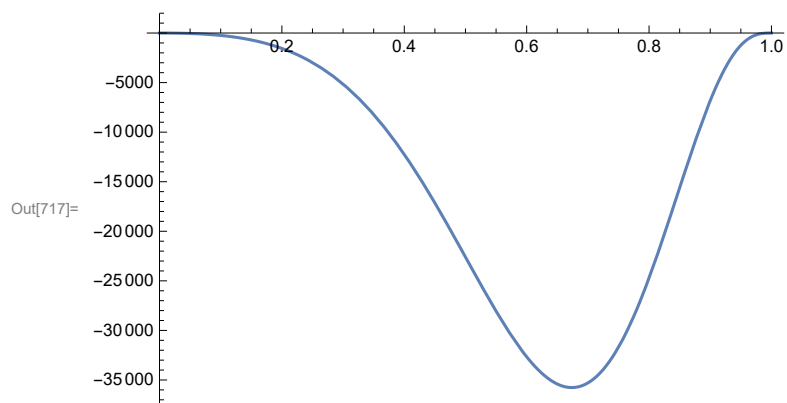

In[718]:= **Plot**[**Cf**[10, 10, 13], {x, 0, 1}]

[绘图](#)

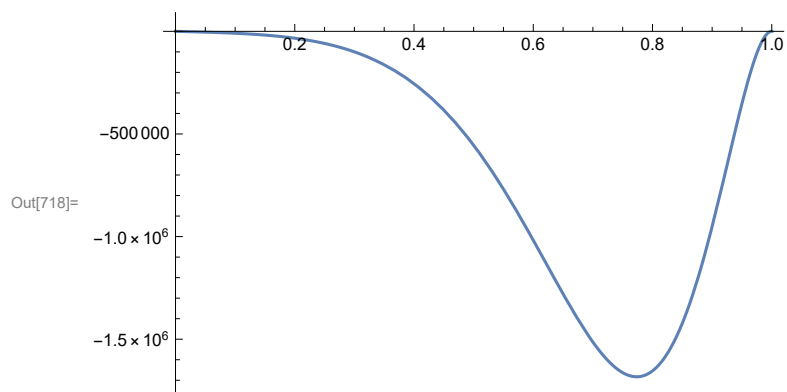

In[719]:= **Plot**[**Cf**[10, 10, 12], {x, 0, 1}]

[绘图](#)

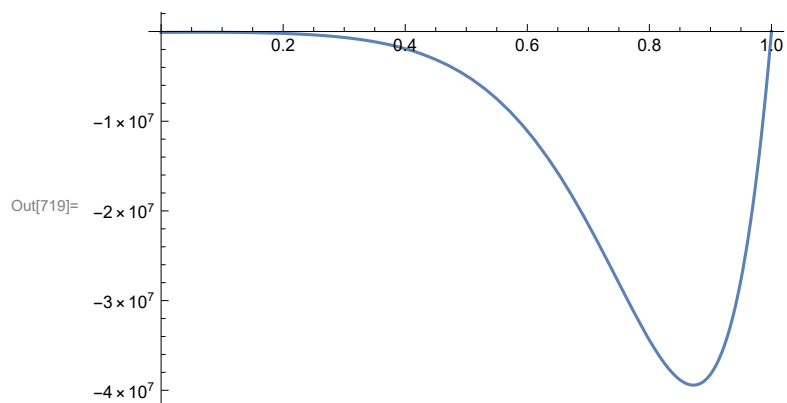

In[720]:= **Plot[Cf[10, 10, 11], {x, 0, 1}]**

[绘图](#)

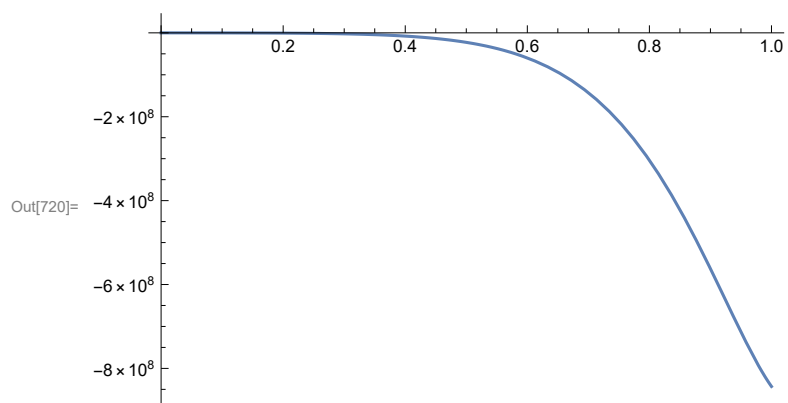

In[721]:= **Plot[Cf[10, 10, 10], {x, 0, 1}]**

[绘图](#)

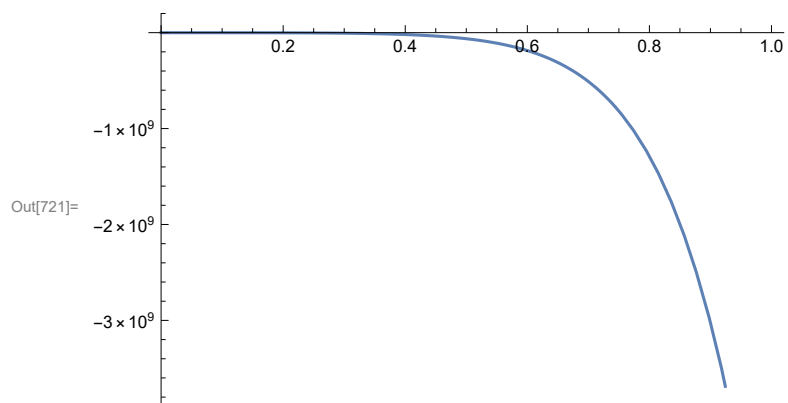

In[722]:= **Plot[Cf[10, 10, 9], {x, 0, 1}]**

[绘图](#)

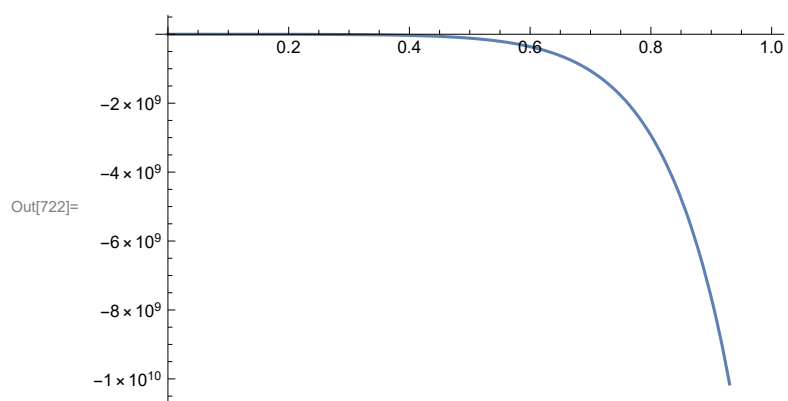



In[723]:= **Plot[Cf[10, 10, 8], {x, 0, 1}]**

[绘图](#)

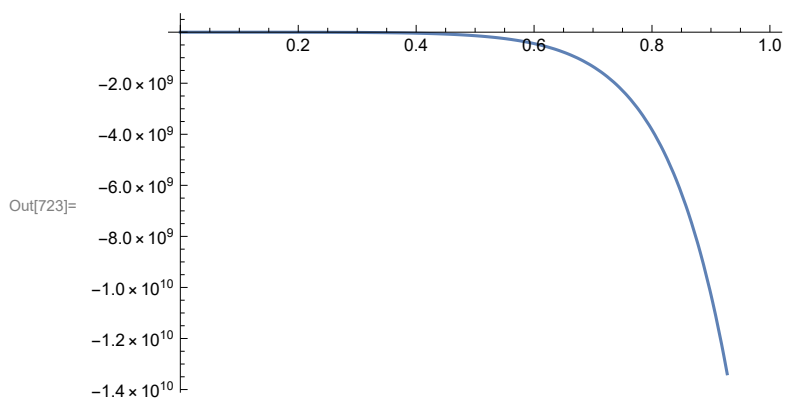

In[724]:= **Plot[Cf[10, 10, 7], {x, 0, 1}]**

[绘图](#)

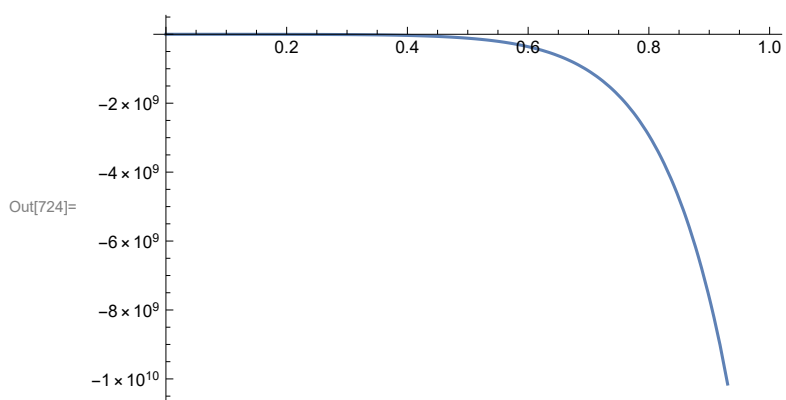

In[725]:= **Plot[Cf[10, 10, 6], {x, 0, 1}]**

[绘图](#)

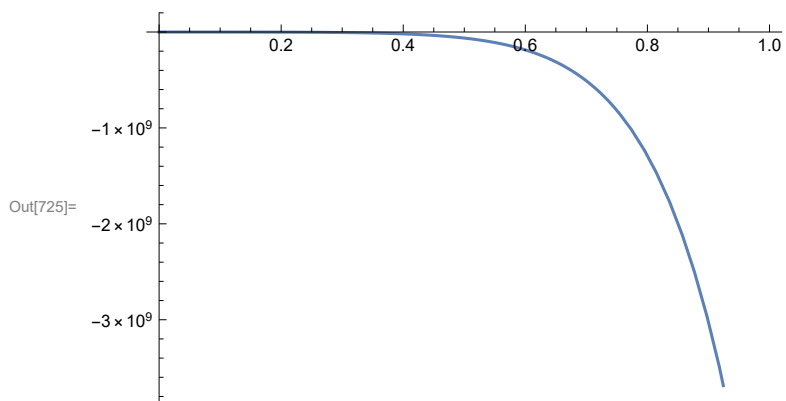

In[726]:= **Plot[Cf[10, 10, 5], {x, 0, 1}]**

[绘图](#)

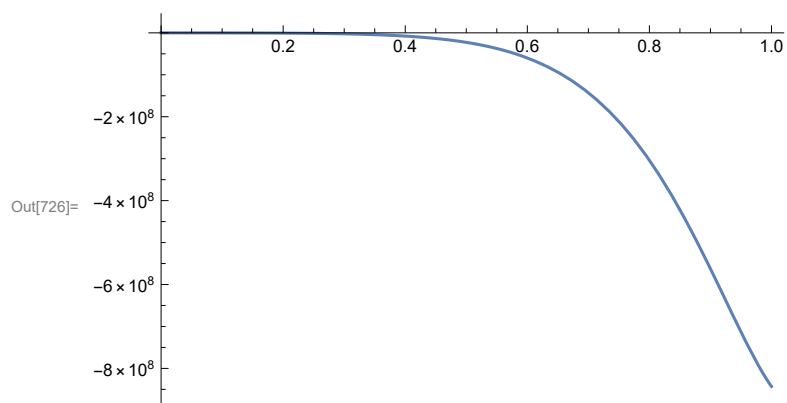

In[727]:= **Plot[Cf[10, 10, 4], {x, 0, 1}]**

[绘图](#)

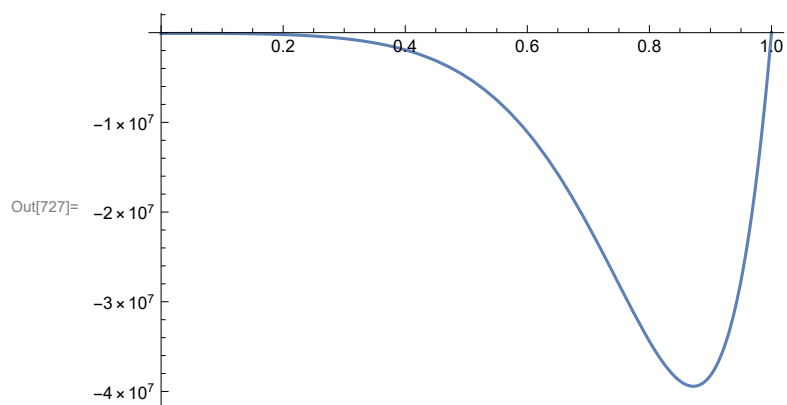

In[728]:= **Plot[Cf[10, 10, 3], {x, 0, 1}]**

[绘图](#)

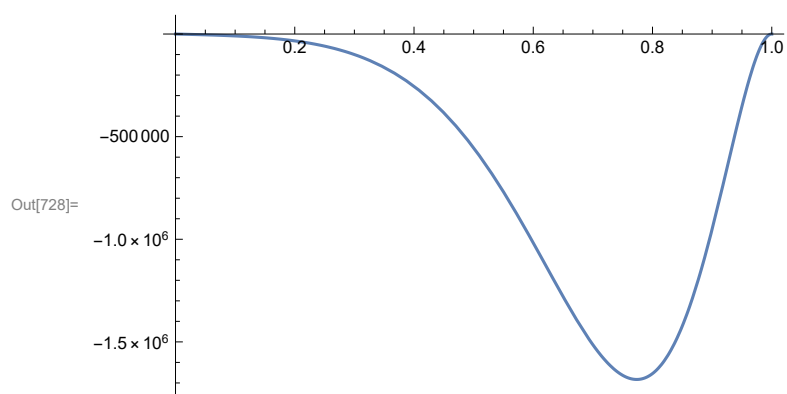

In[729]:= **Plot[Cf[10, 10, 2], {x, 0, 1}]**

[绘图](#)

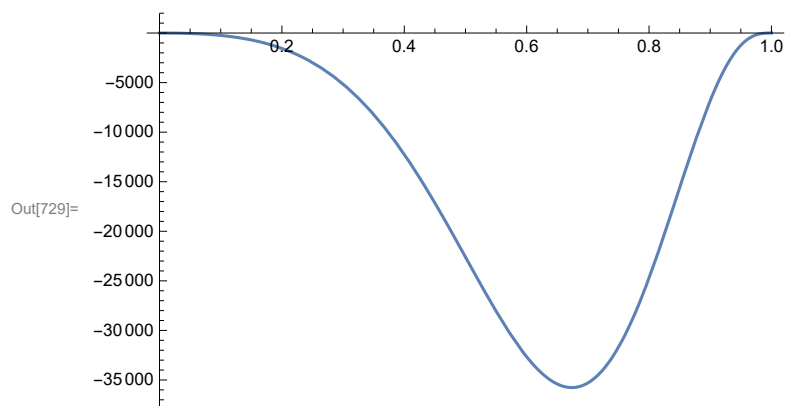

**Plot[Cf[10, 10, 1], {x, 0, 1}]**

[绘图](#)

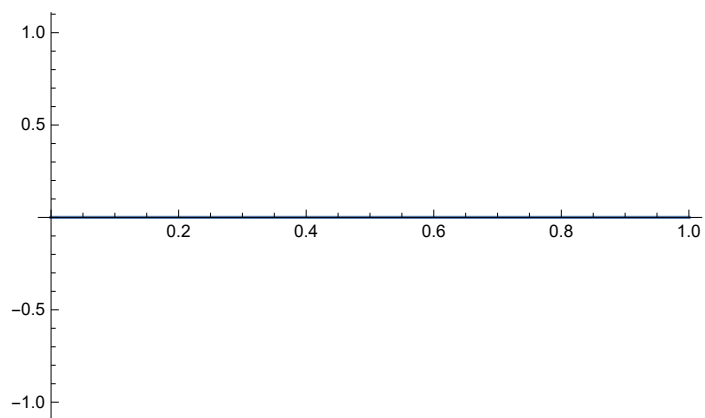

**Plot[Cf[10, 10, 0], {x, 0, 1}]**

[绘图](#)

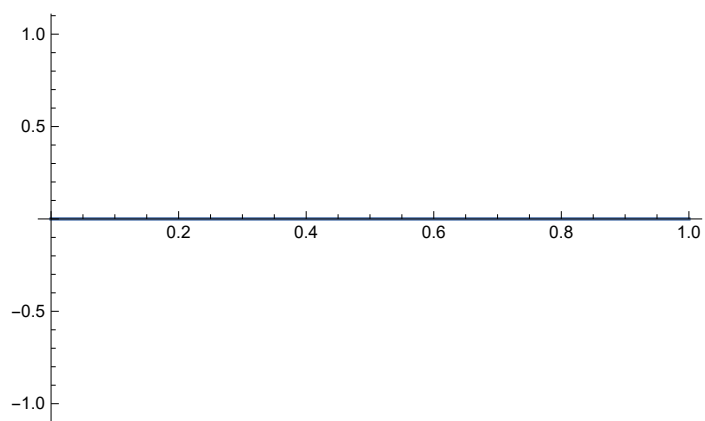

(\*66th group coefficients r2^10r3^9\*)

In[730]:= **Plot[Cf[10, 9, 14], {x, 0, 1}]**

[绘图](#)

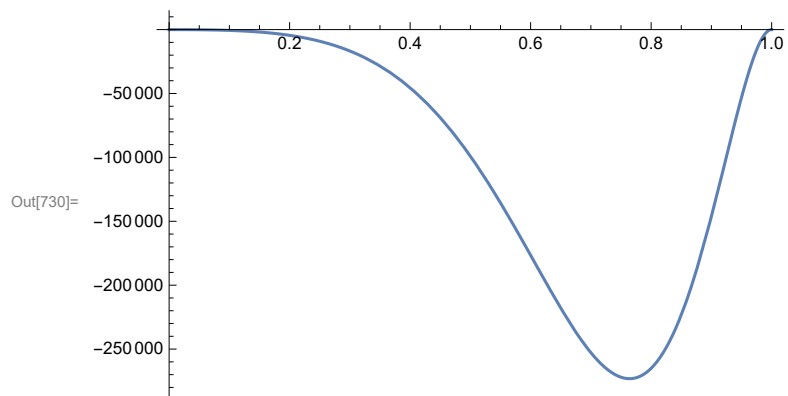

In[731]:= **Plot[Cf[10, 9, 13], {x, 0, 1}]**

[绘图](#)

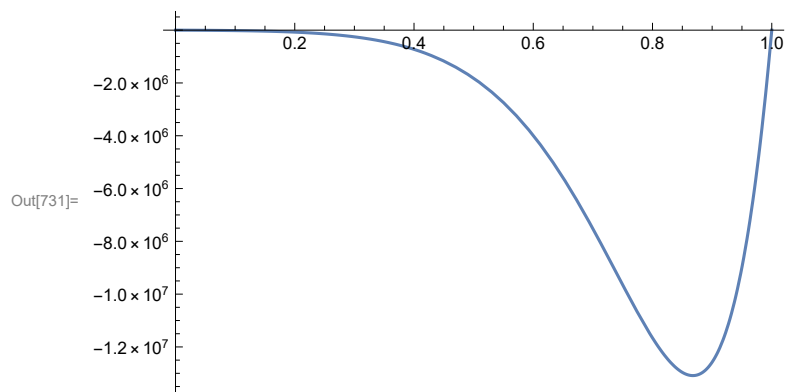

In[732]:= **Plot[Cf[10, 9, 12], {x, 0, 1}]**

[绘图](#)

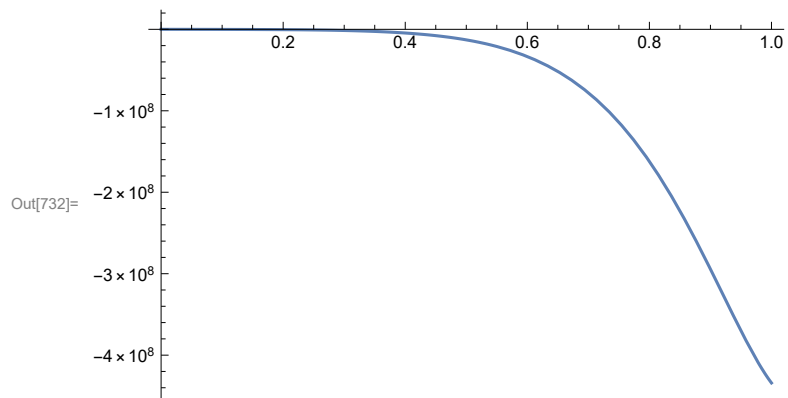

In[733]:= **Plot[Cf[10, 9, 11], {x, 0, 1}]**

[绘图](#)

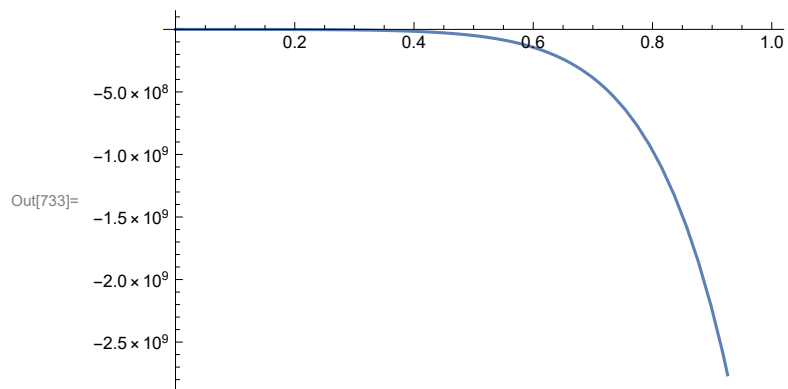

In[734]:= **Plot[Cf[10, 9, 10], {x, 0, 1}]**

[绘图](#)

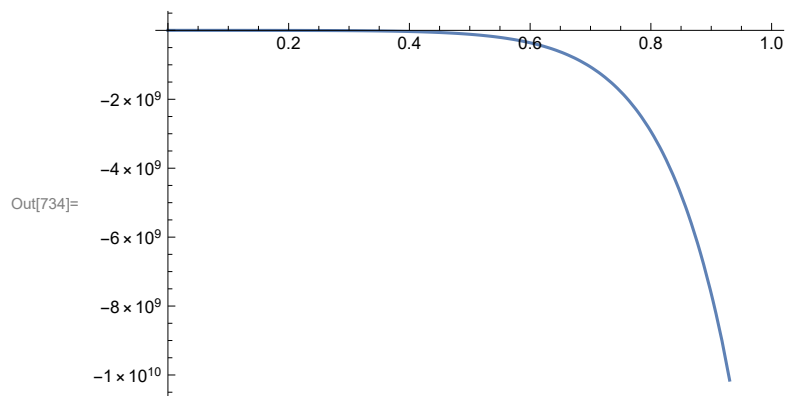

In[735]:= **Plot[Cf[10, 9, 9], {x, 0, 1}]**

[绘图](#)

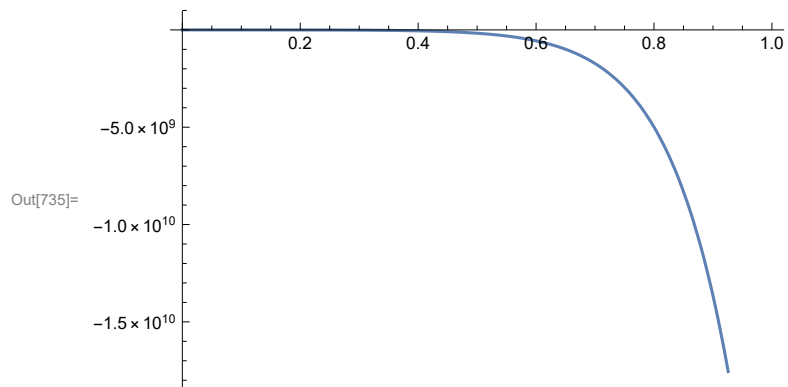

In[736]:= **Plot[Cf[10, 9, 8], {x, 0, 1}]**

[绘图](#)

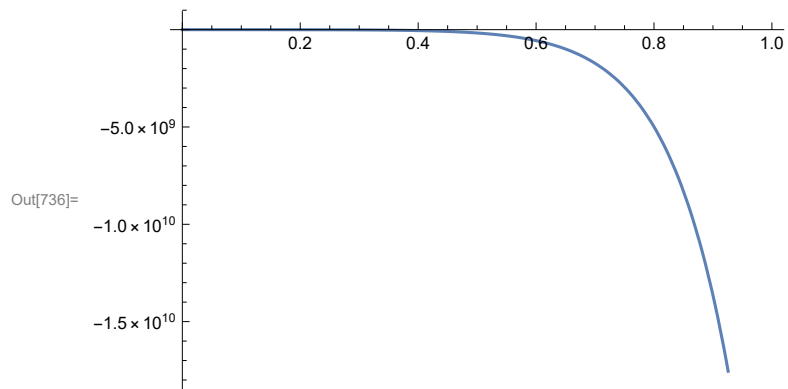

In[737]:= **Plot[Cf[10, 9, 7], {x, 0, 1}]**

[绘图](#)

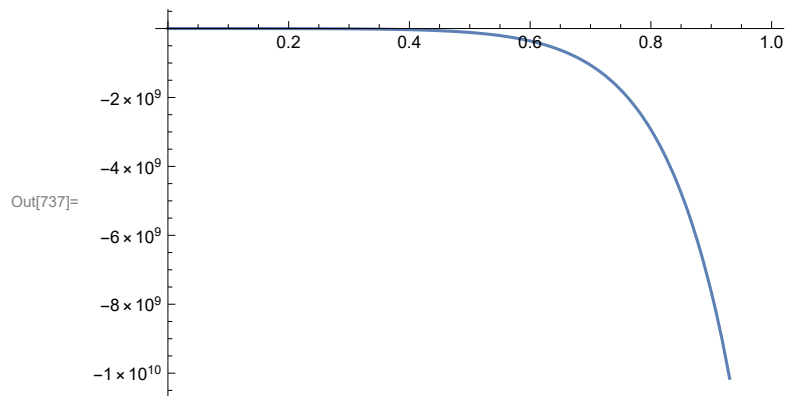

In[738]:= **Plot[Cf[10, 9, 6], {x, 0, 1}]**

[绘图](#)

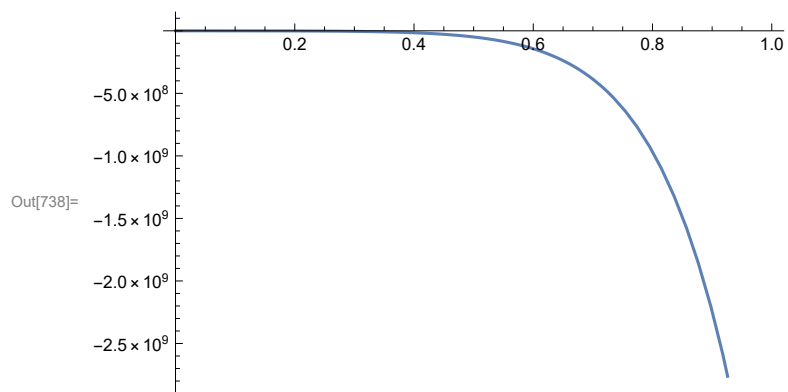

In[739]:= **Plot[Cf[10, 9, 5], {x, 0, 1}]**

[绘图](#)

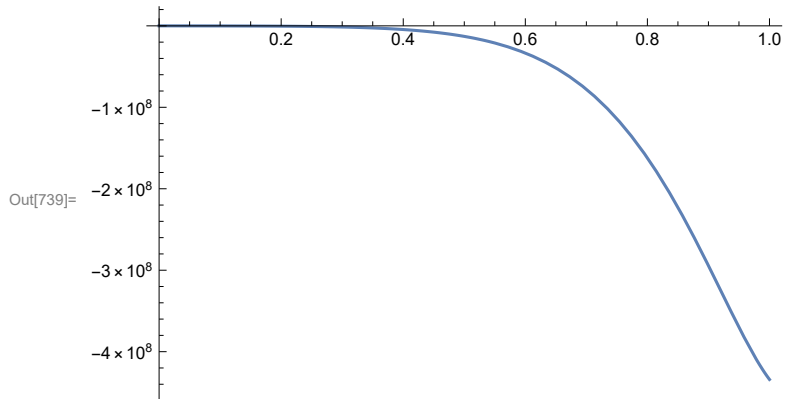

In[740]:= **Plot[Cf[10, 9, 4], {x, 0, 1}]**

[绘图](#)

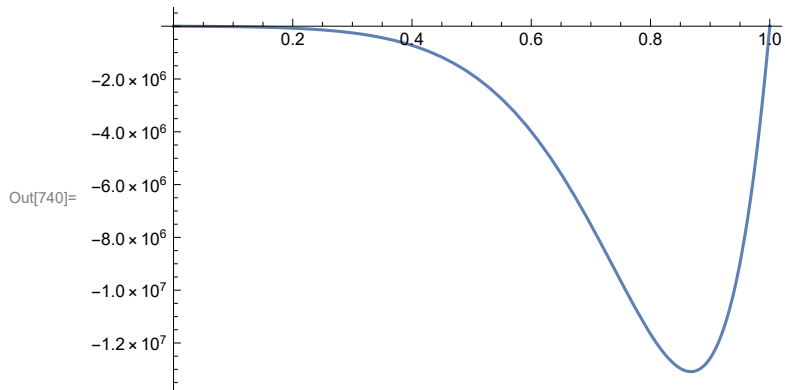

In[741]:= **Plot[Cf[10, 9, 3], {x, 0, 1}]**

[绘图](#)

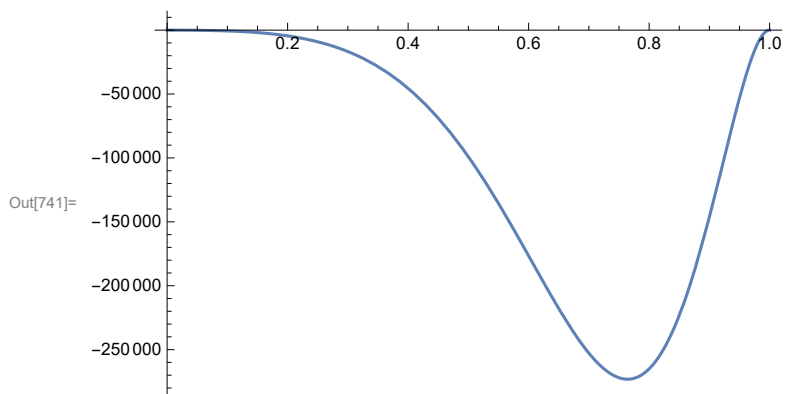

`Plot[Cf[10, 9, 2], {x, 0, 1}]`

[绘图](#)

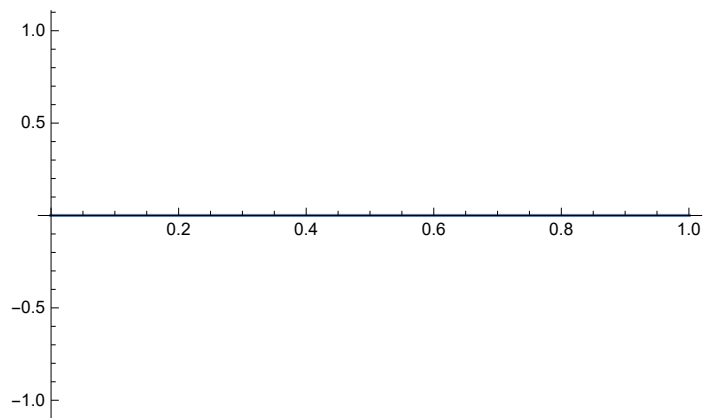

`Plot[Cf[10, 9, 1], {x, 0, 1}]`

[绘图](#)

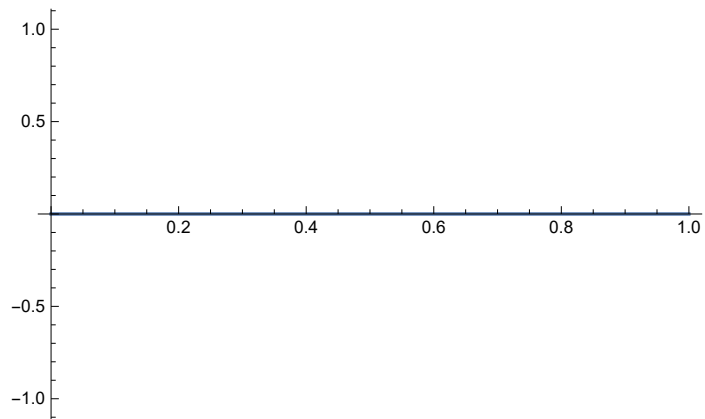

`Plot[Cf[10, 9, 0], {x, 0, 1}]`

[绘图](#)

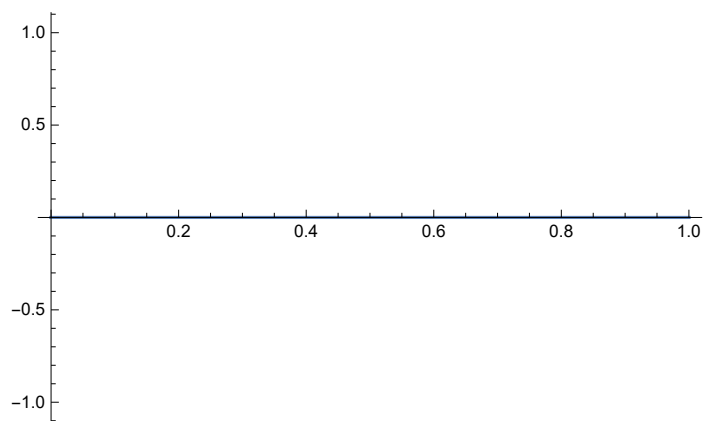

`(*67th group coefficients r2^10r3^8*)`



In[742]:= **Plot[Cf[10, 8, 14], {x, 0, 1}]**

[绘图](#)

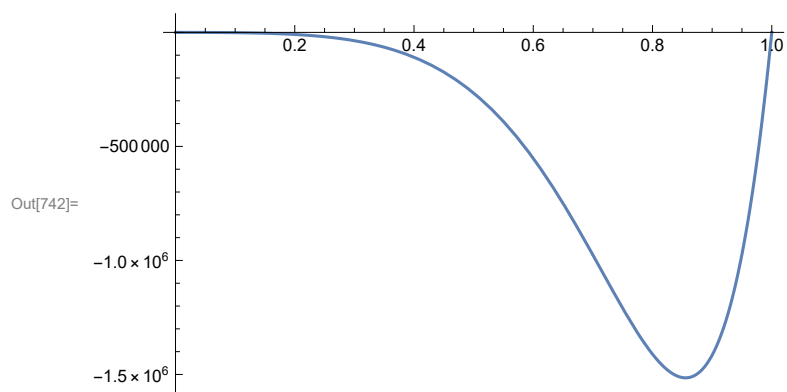

In[743]:= **Plot[Cf[10, 8, 13], {x, 0, 1}]**

[绘图](#)

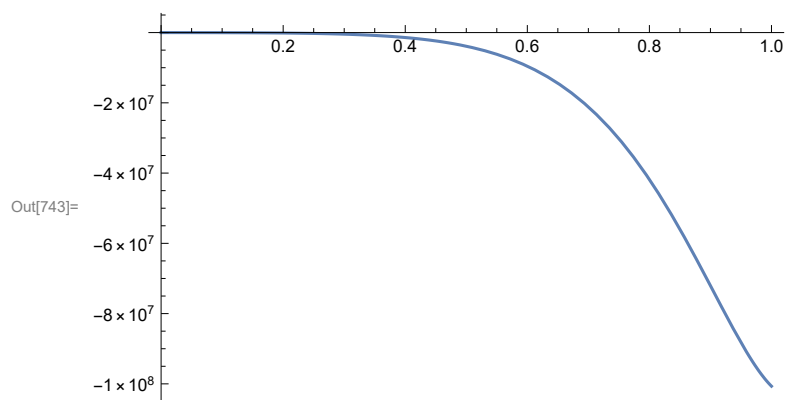

In[744]:= **Plot[Cf[10, 8, 12], {x, 0, 1}]**

[绘图](#)

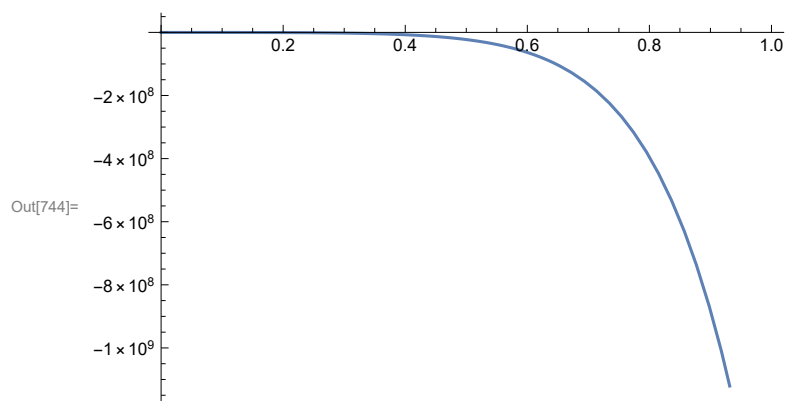

In[745]:= **Plot[Cf[10, 8, 11], {x, 0, 1}]**

[绘图](#)

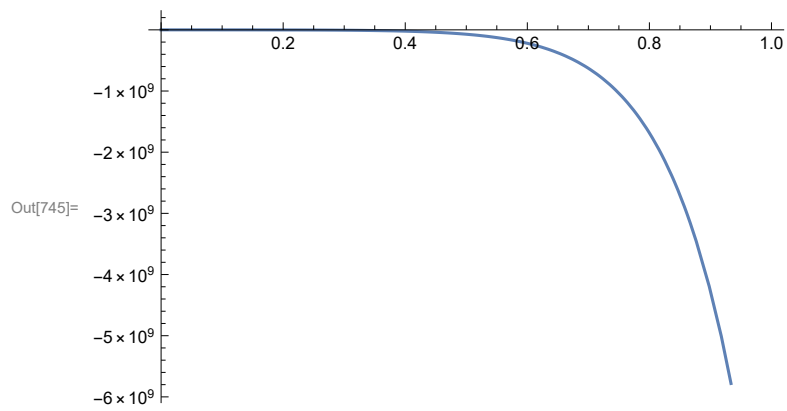

In[746]:= **Plot[Cf[10, 8, 10], {x, 0, 1}]**

[绘图](#)

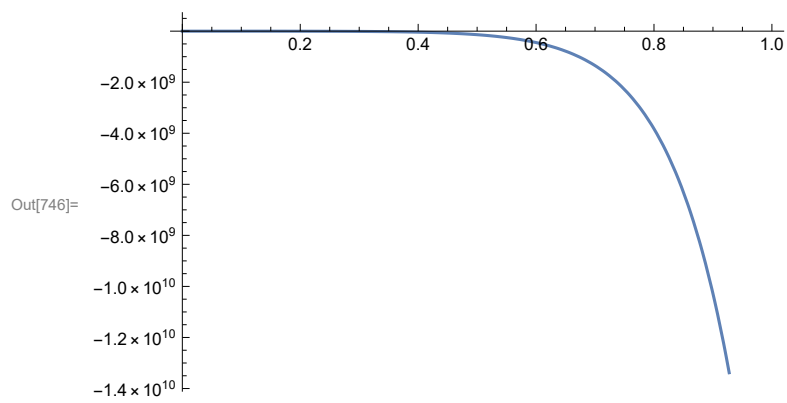

In[747]:= **Plot[Cf[10, 8, 9], {x, 0, 1}]**

[绘图](#)

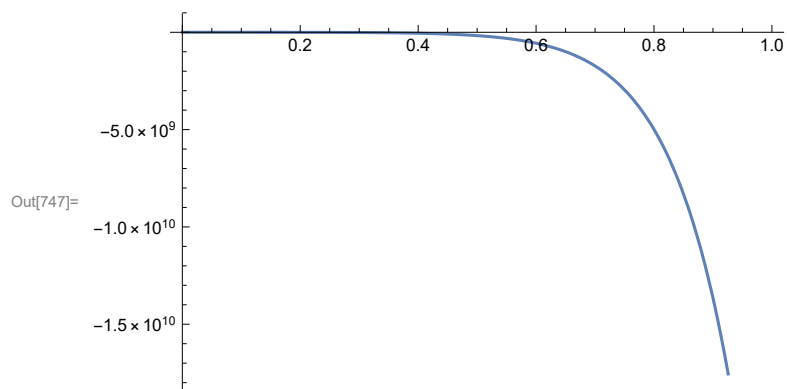

In[748]:= **Plot[Cf[10, 8, 8], {x, 0, 1}]**

[绘图](#)

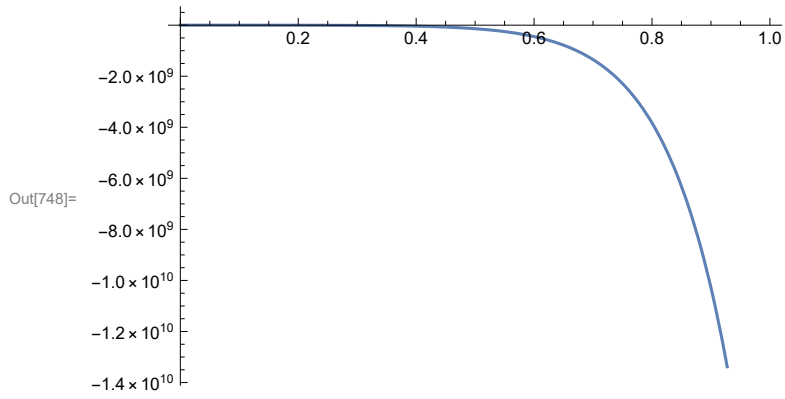

In[749]:= **Plot[Cf[10, 8, 7], {x, 0, 1}]**

[绘图](#)

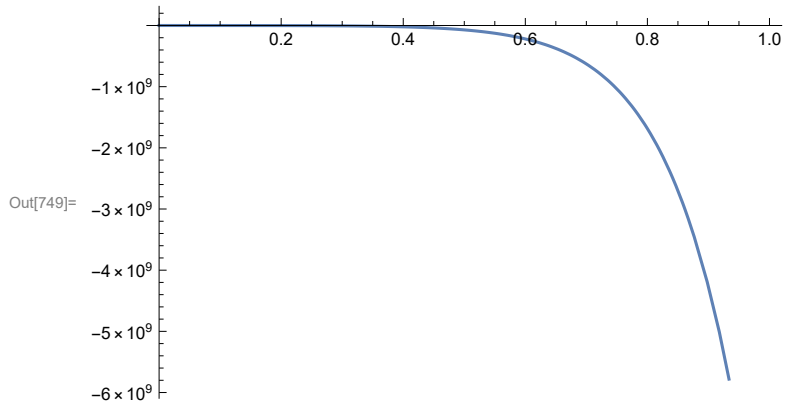

In[750]:= **Plot[Cf[10, 8, 6], {x, 0, 1}]**

[绘图](#)

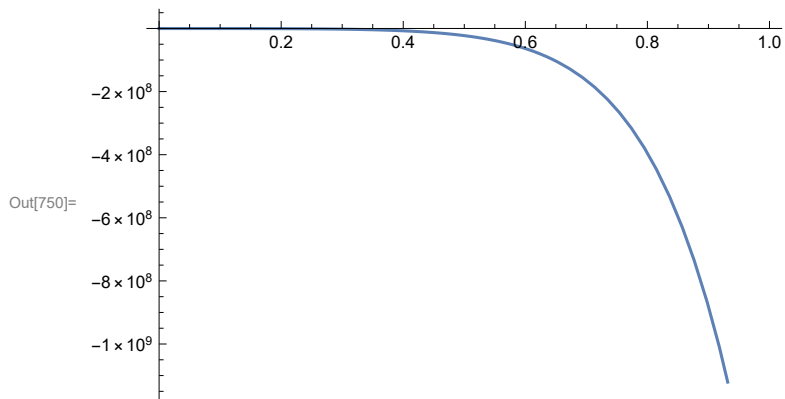

In[751]:= **Plot[Cf[10, 8, 5], {x, 0, 1}]**

[绘图](#)

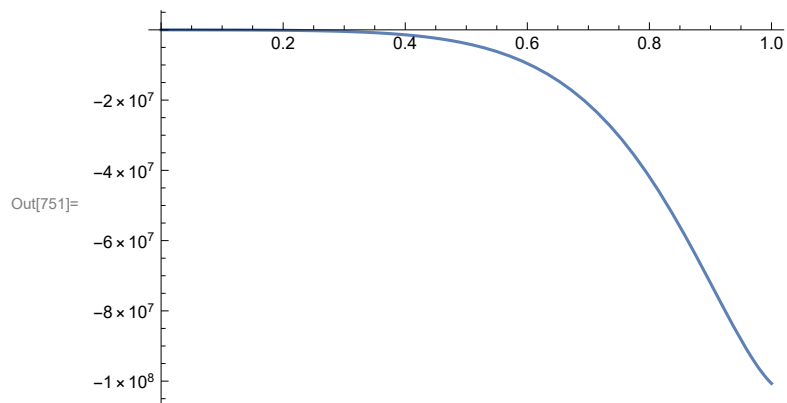

In[752]:= **Plot[Cf[10, 8, 4], {x, 0, 1}]**

[绘图](#)

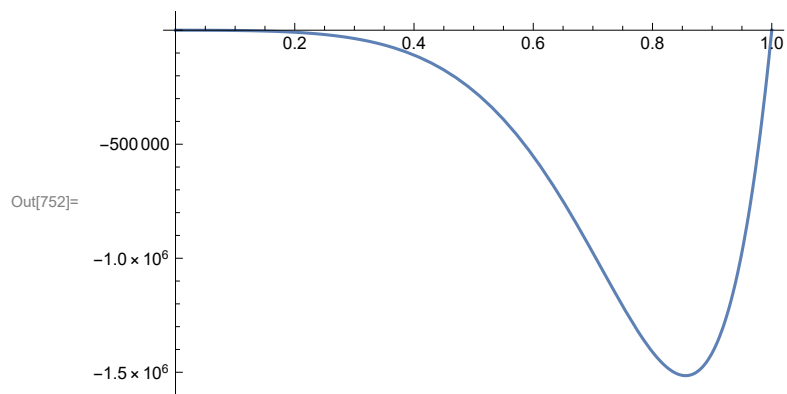

**Plot[Cf[10, 8, 3], {x, 0, 1}]**

[绘图](#)

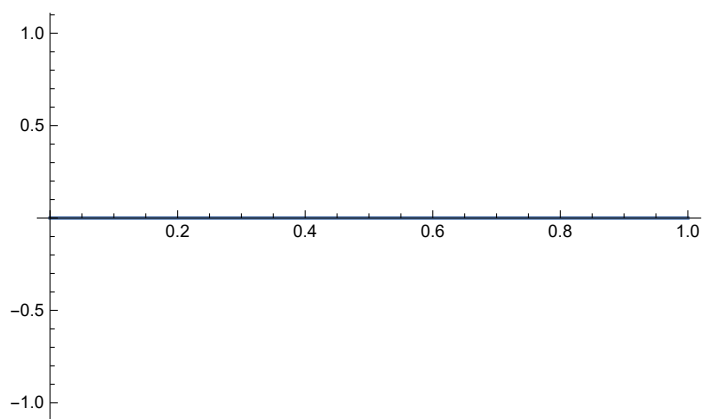

**Plot[Cf[10, 8, 2], {x, 0, 1}]**

[绘图](#)

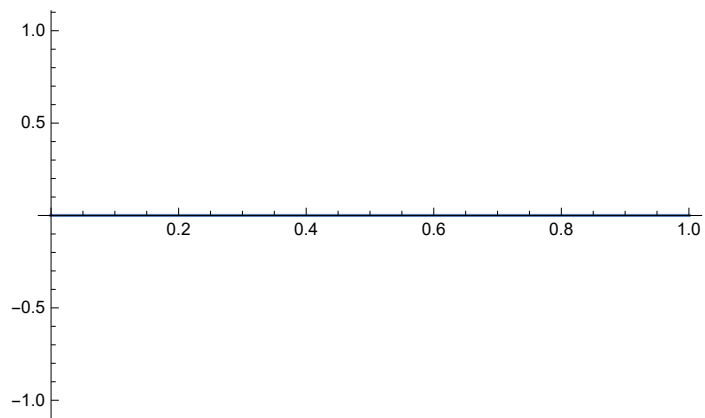

**Plot[Cf[10, 8, 1], {x, 0, 1}]**

[绘图](#)

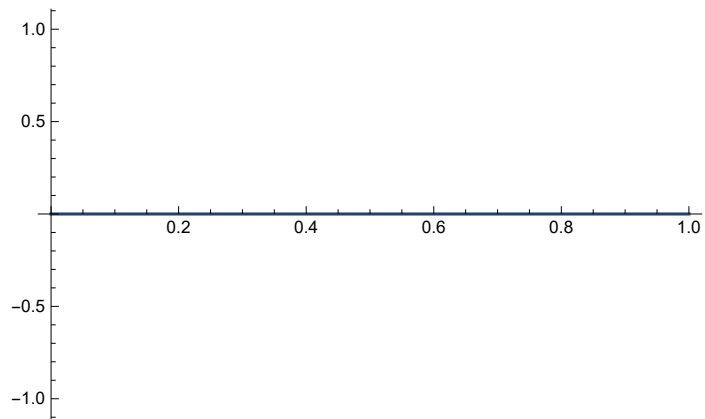

**Plot[Cf[10, 8, 0], {x, 0, 1}]**

[绘图](#)

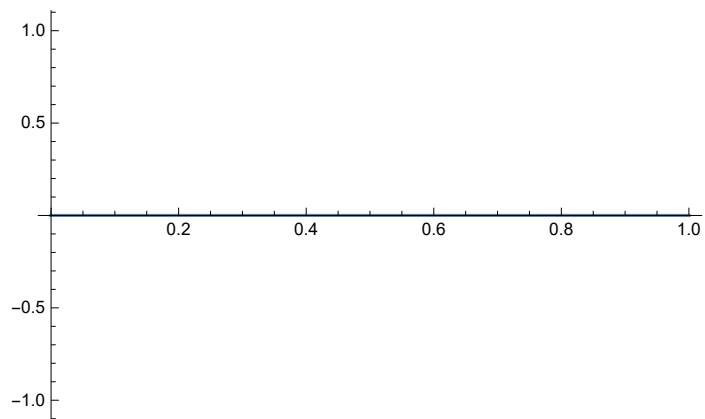

**(\*68th group coefficients r2^10r3^7\*)**

In[753]:= **Plot[Cf[10, 7, 14], {x, 0, 1}]**

[绘图](#)

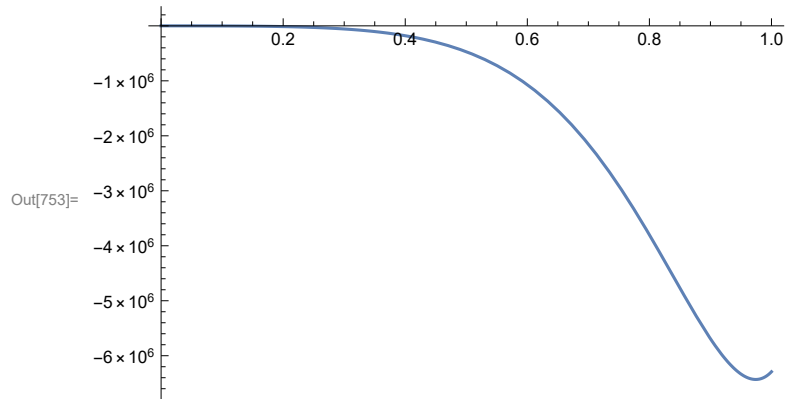

In[754]:= **Plot[Cf[10, 7, 13], {x, 0, 1}]**

[绘图](#)

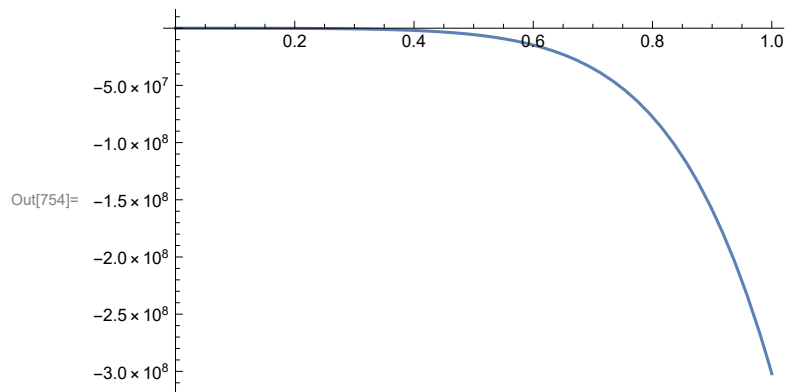

In[755]:= **Plot[Cf[10, 7, 12], {x, 0, 1}]**

[绘图](#)

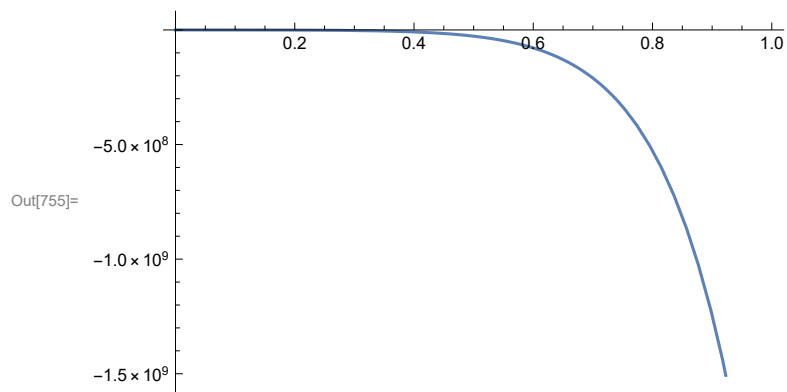

In[756]:= **Plot[Cf[10, 7, 11], {x, 0, 1}]**

[绘图](#)

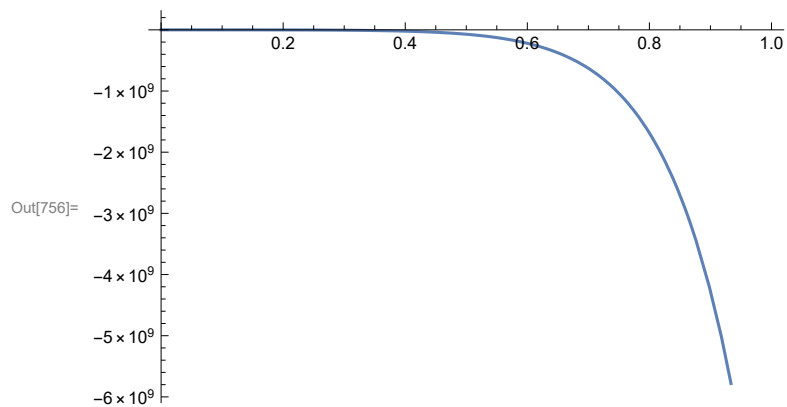

In[757]:= **Plot[Cf[10, 7, 10], {x, 0, 1}]**

[绘图](#)

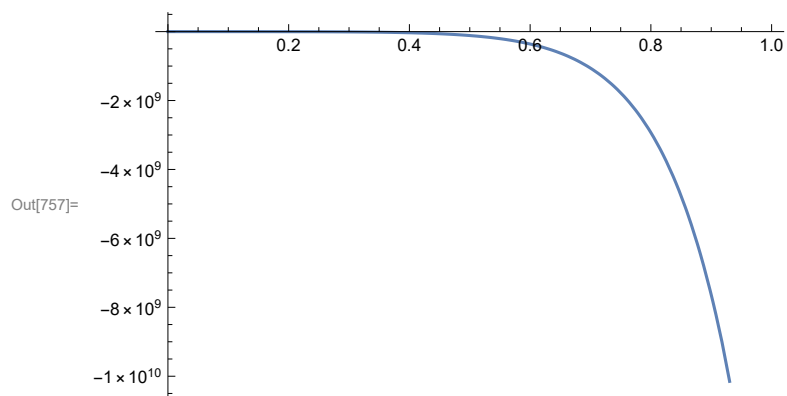

In[758]:= **Plot[Cf[10, 7, 9], {x, 0, 1}]**

[绘图](#)

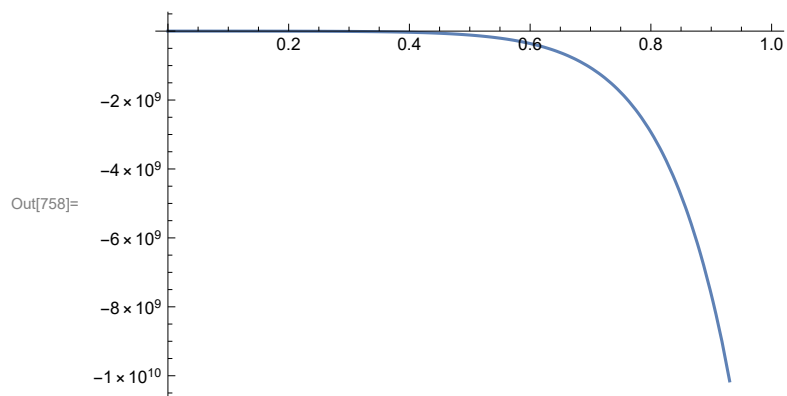

In[759]:= **Plot[Cf[10, 7, 8], {x, 0, 1}]**

[绘图](#)

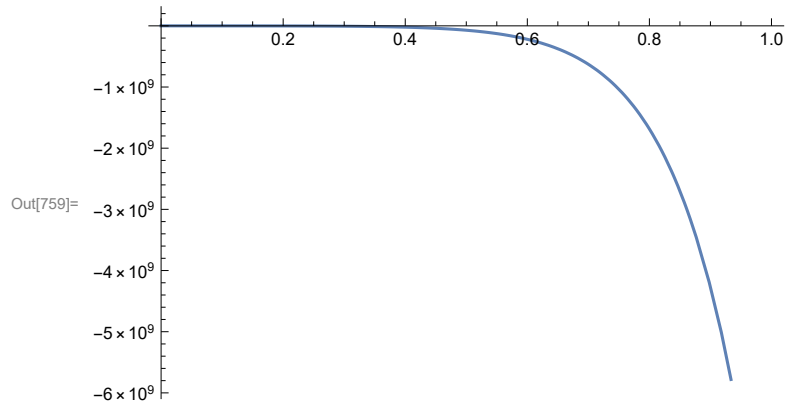

In[760]:= **Plot[Cf[10, 7, 7], {x, 0, 1}]**

[绘图](#)

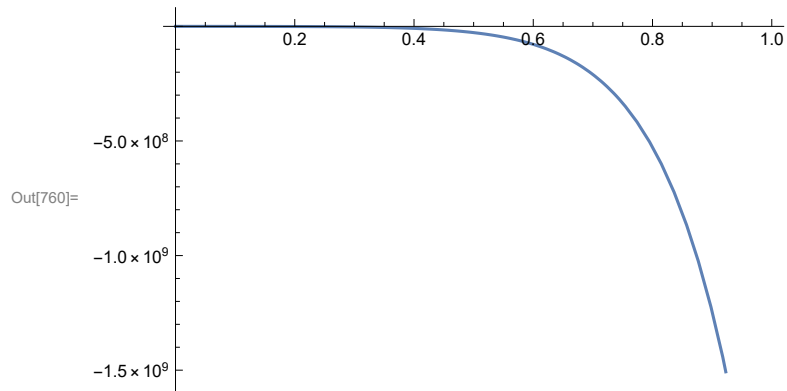

In[761]:= **Plot[Cf[10, 7, 6], {x, 0, 1}]**

[绘图](#)

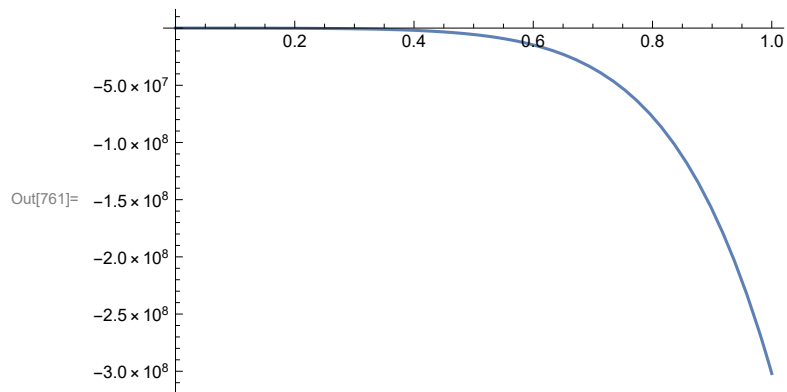



In[763]:= **Plot[Cf[10, 7, 5], {x, 0, 1}]**

[绘图](#)

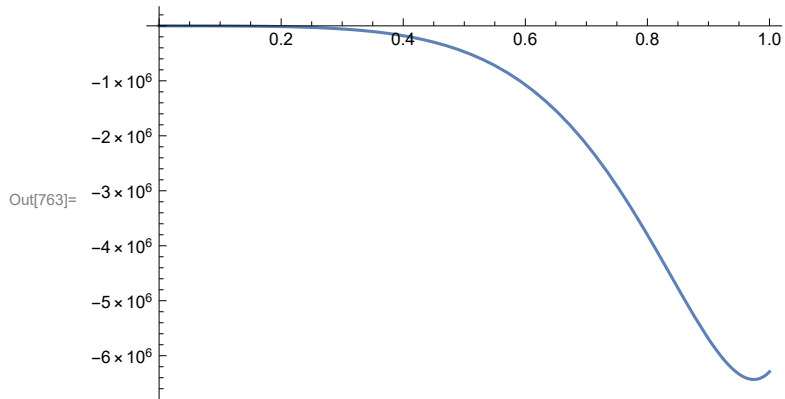

**Plot[Cf[10, 7, 4], {x, 0, 1}]**

[绘图](#)

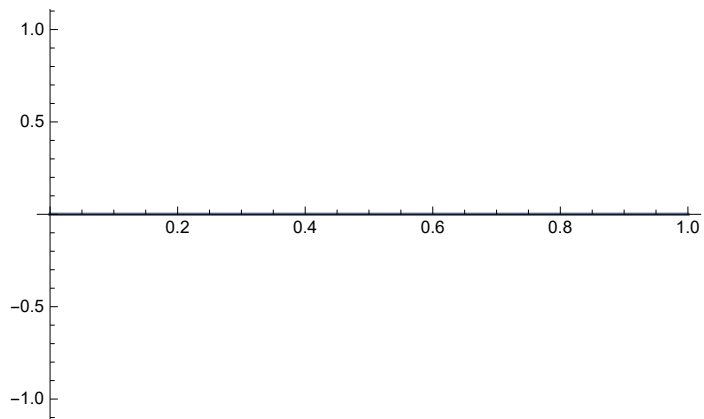

**Plot[Cf[10, 7, 3], {x, 0, 1}]**

[绘图](#)

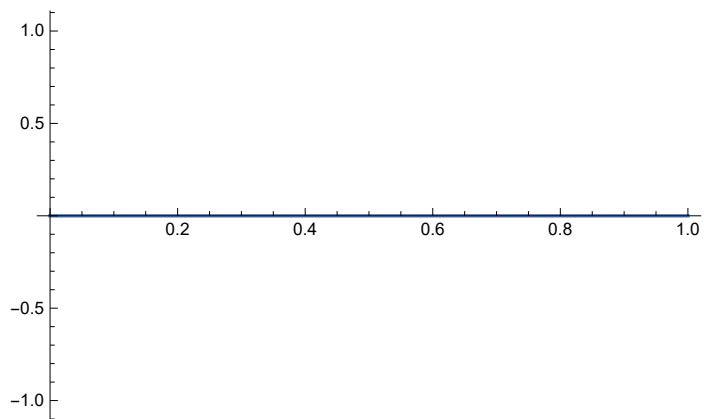

**Plot[Cf[10, 7, 2], {x, 0, 1}]**

[绘图](#)

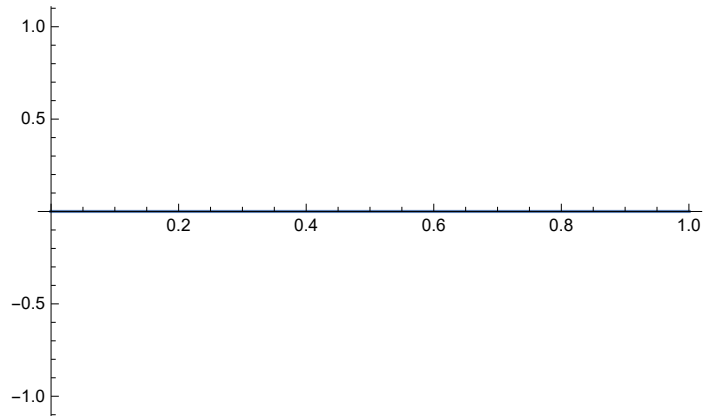

**Plot[Cf[10, 7, 1], {x, 0, 1}]**

[绘图](#)

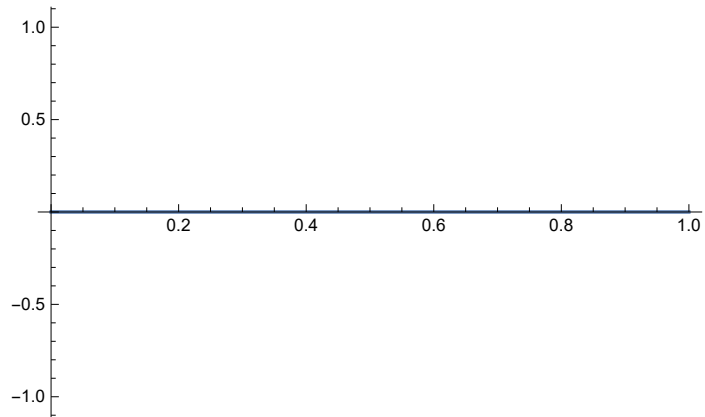

**Plot[Cf[10, 7, 0], {x, 0, 1}]**

[绘图](#)

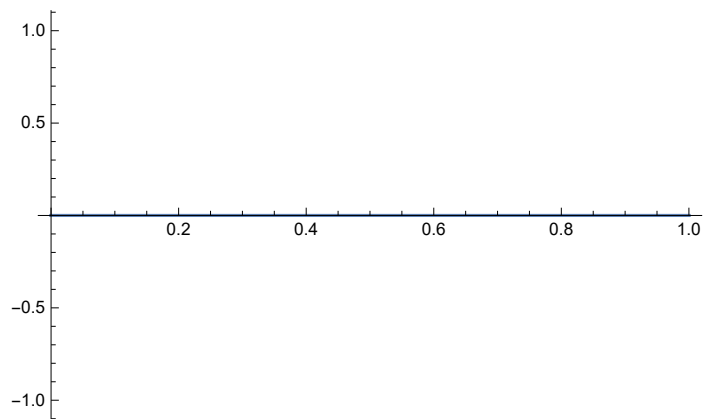

**(\*69th group coefficients r2^10r3^6\*)**

In[764]:= **Plot[Cf[10, 6, 14], {x, 0, 1}]**

[绘图](#)

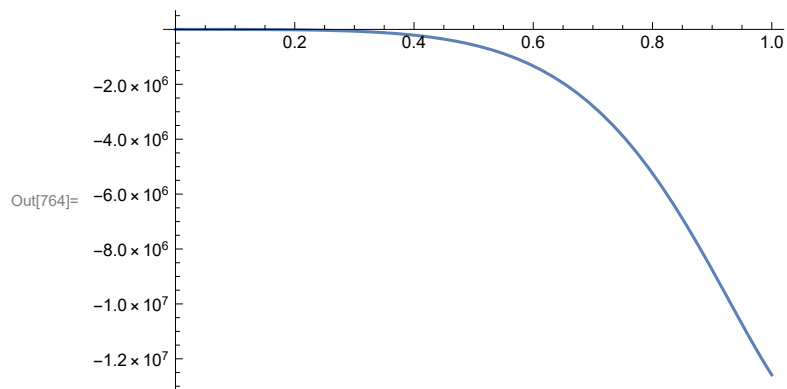

In[765]:= **Plot[Cf[10, 6, 13], {x, 0, 1}]**

[绘图](#)

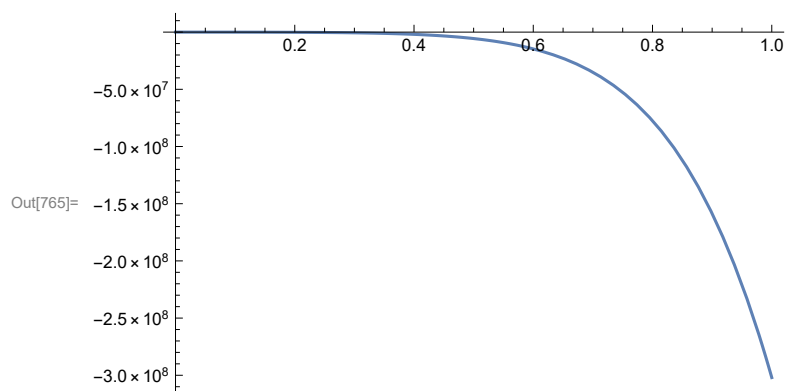

In[766]:= **Plot[Cf[10, 6, 12], {x, 0, 1}]**

[绘图](#)

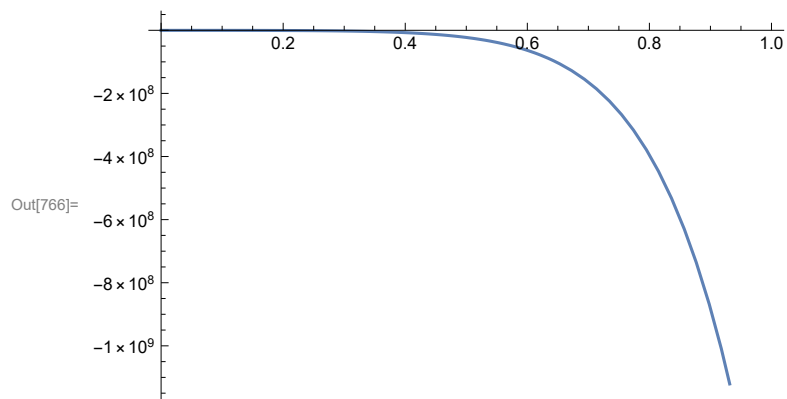

In[767]:= **Plot[Cf[10, 6, 11], {x, 0, 1}]**

[绘图](#)

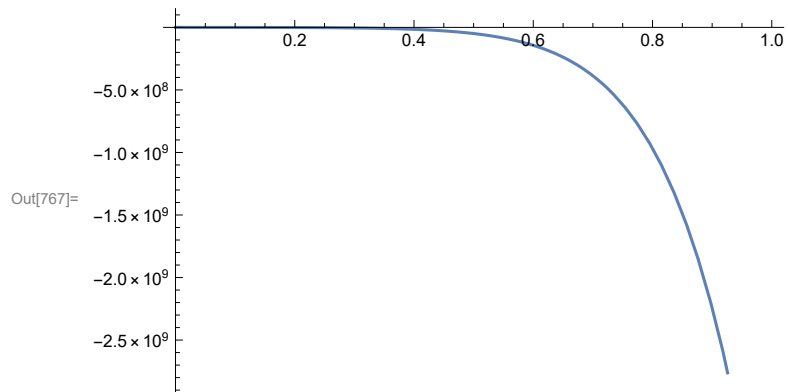

In[768]:= **Plot[Cf[10, 6, 10], {x, 0, 1}]**

[绘图](#)

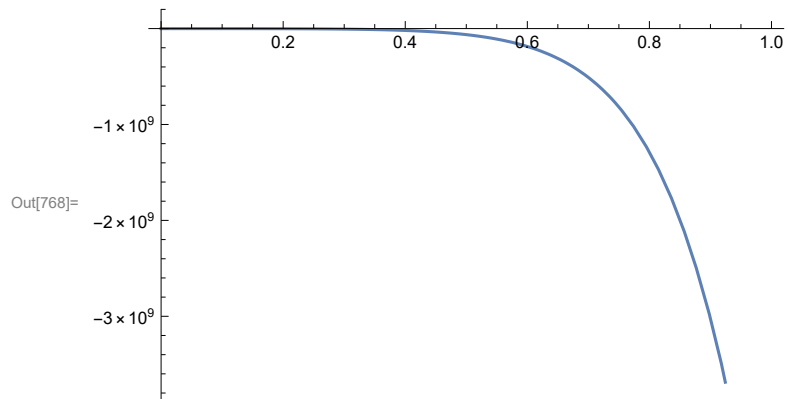

In[769]:= **Plot[Cf[10, 6, 9], {x, 0, 1}]**

[绘图](#)

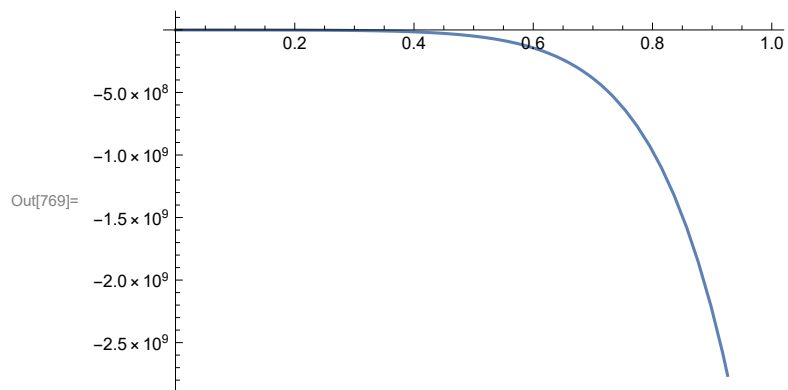

In[770]:= **Plot[Cf[10, 6, 8], {x, 0, 1}]**

[绘图](#)

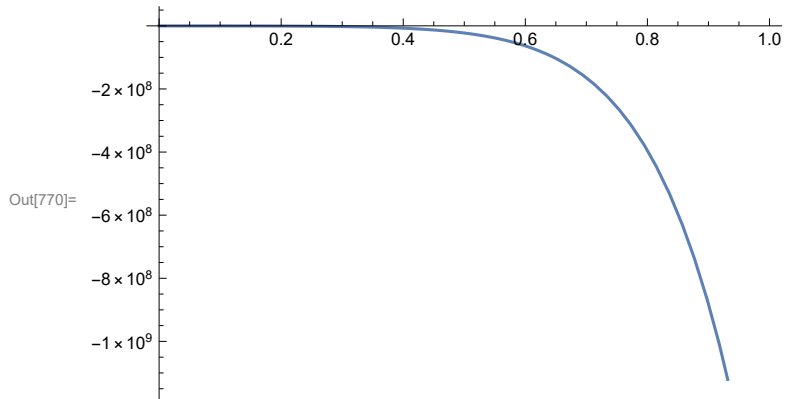

In[771]:= **Plot[Cf[10, 6, 7], {x, 0, 1}]**

[绘图](#)

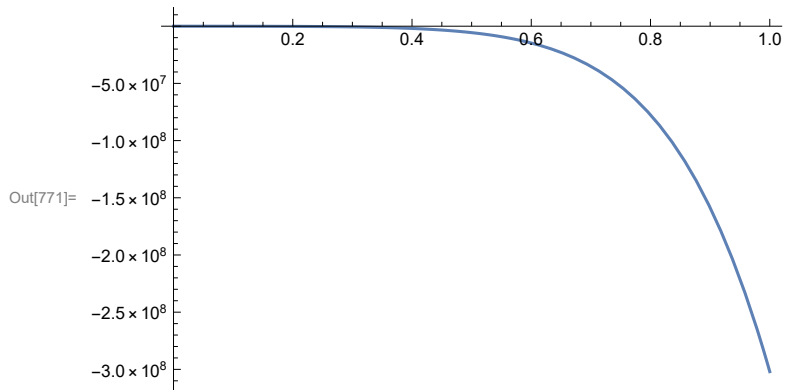

In[772]:= **Plot[Cf[10, 6, 6], {x, 0, 1}]**

[绘图](#)

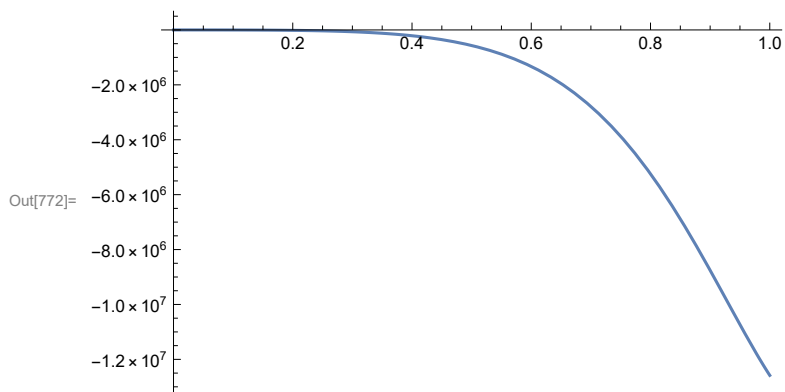

```
Plot[Cf[10, 6, 5], {x, 0, 1}]
```

[绘图](#)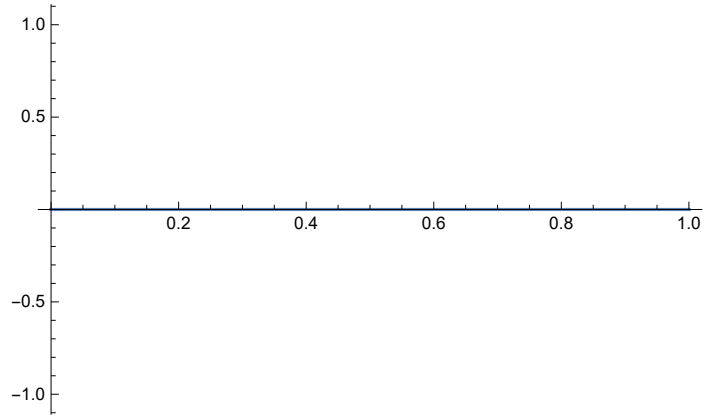

```
Plot[Cf[10, 6, 4], {x, 0, 1}]
```

[绘图](#)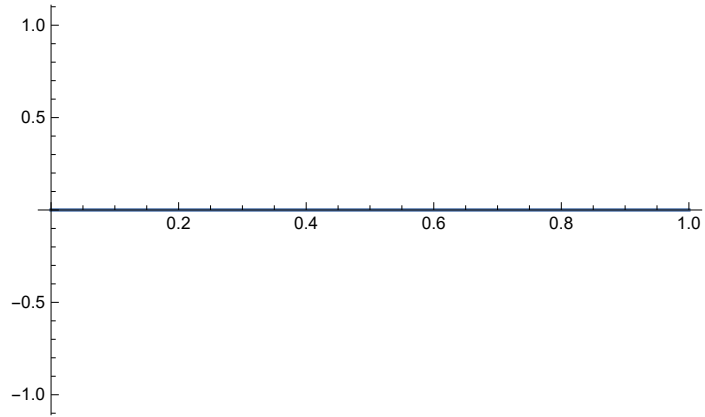

```
Plot[Cf[10, 6, 3], {x, 0, 1}]
```

[绘图](#)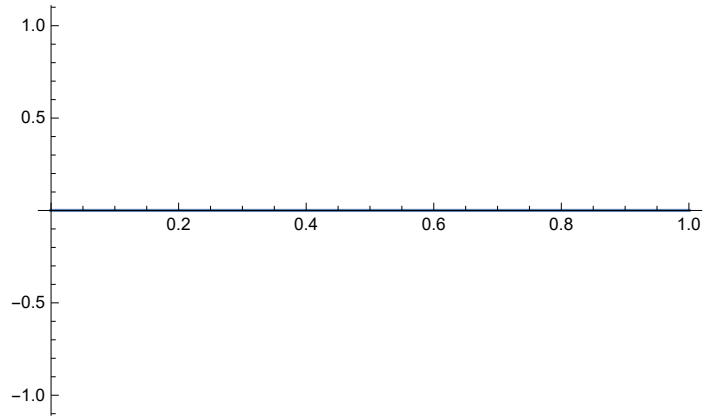

**Plot[Cf[10, 6, 2], {x, 0, 1}]**

[绘图](#)

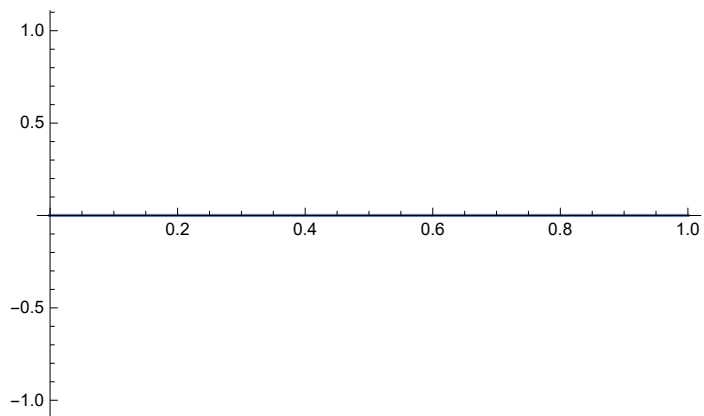

**Plot[Cf[10, 6, 1], {x, 0, 1}]**

[绘图](#)

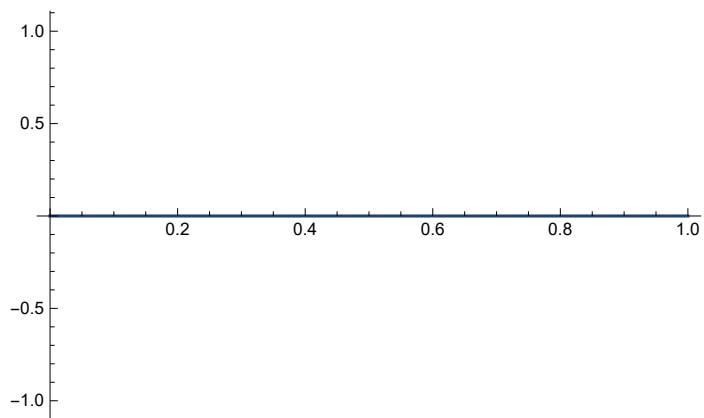

**Plot[Cf[10, 6, 0], {x, 0, 1}]**

[绘图](#)

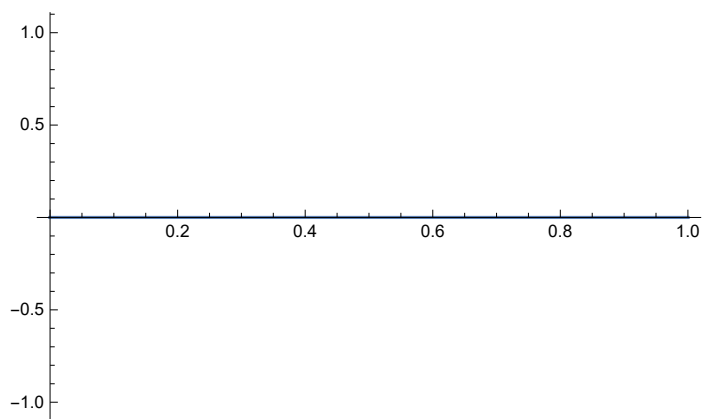

**(\*70th group coefficients r2^10r3^5\*)**

In[773]:= **Plot[Cf[10, 5, 14], {x, 0, 1}]**

[绘图](#)

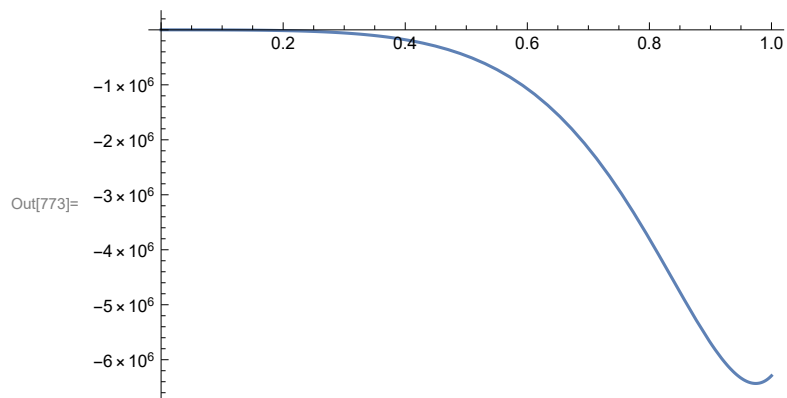

In[774]:= **Plot[Cf[10, 5, 13], {x, 0, 1}]**

[绘图](#)

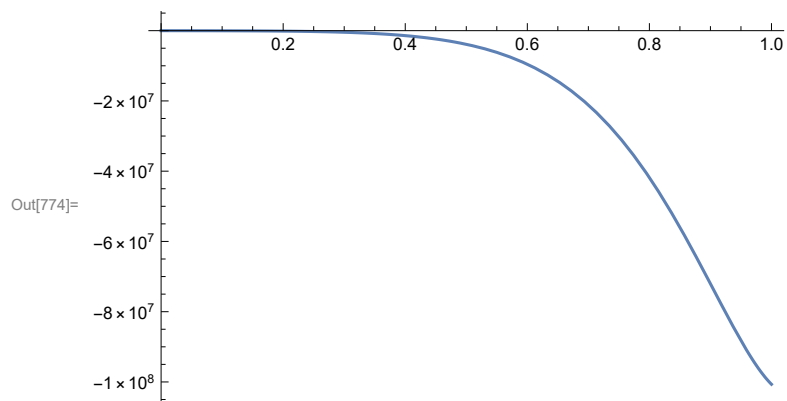

In[775]:= **Plot[Cf[10, 5, 12], {x, 0, 1}]**

[绘图](#)

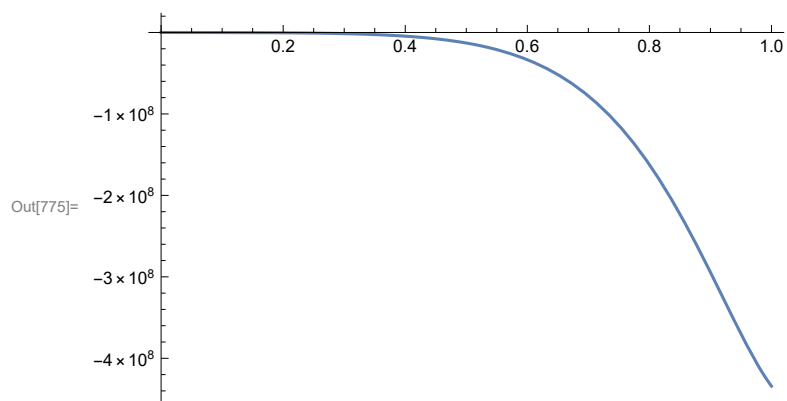



In[776]:= **Plot[Cf[10, 5, 11], {x, 0, 1}]**

[绘图](#)

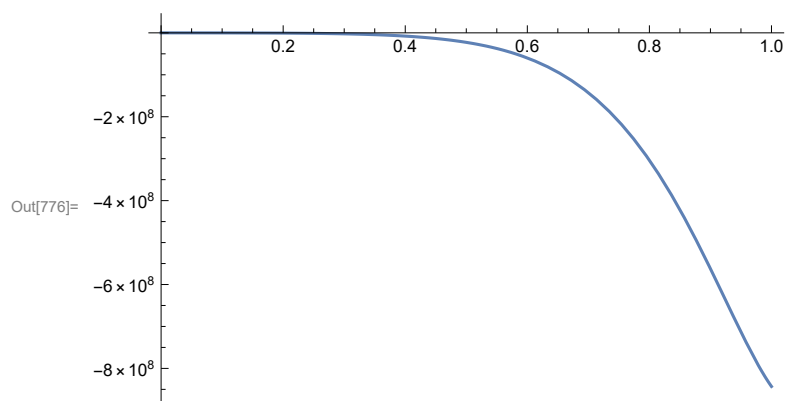

In[777]:= **Plot[Cf[10, 5, 10], {x, 0, 1}]**

[绘图](#)

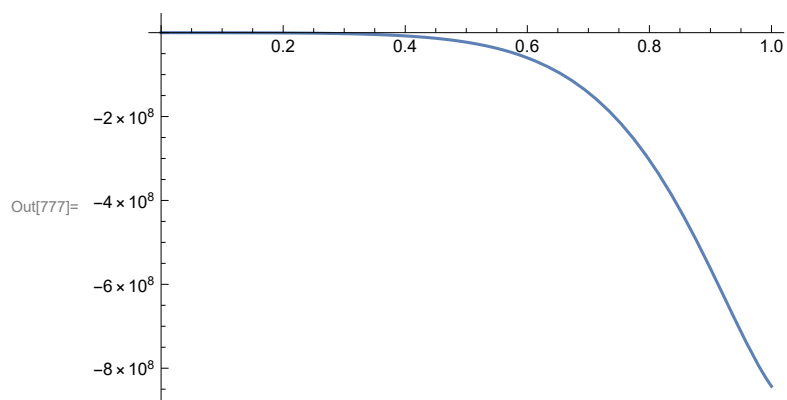

In[778]:= **Plot[Cf[10, 5, 9], {x, 0, 1}]**

[绘图](#)

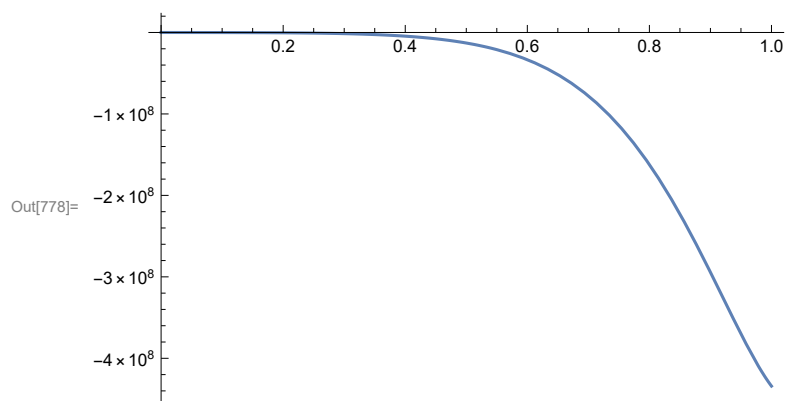

In[779]:= **Plot[Cf[10, 5, 8], {x, 0, 1}]**

[绘图](#)

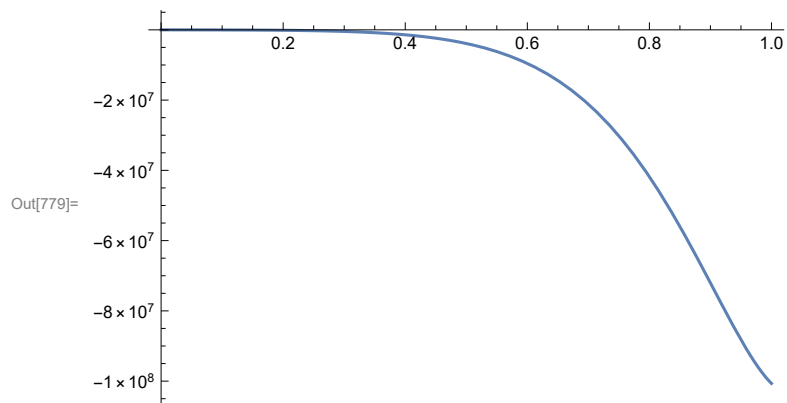

In[780]:= **Plot[Cf[10, 5, 7], {x, 0, 1}]**

[绘图](#)

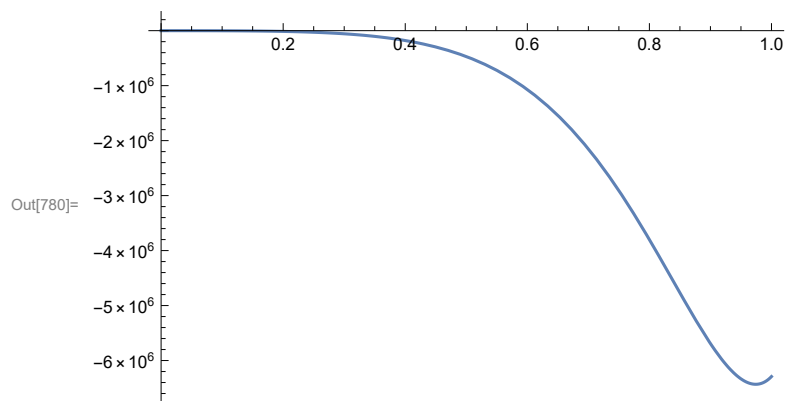

**Plot[Cf[10, 5, 6], {x, 0, 1}]**

[绘图](#)

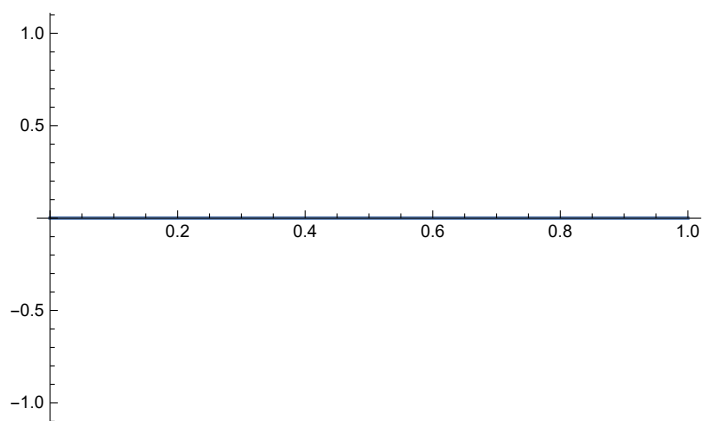

**Plot[Cf[10, 5, 5], {x, 0, 1}]**

[绘图](#)

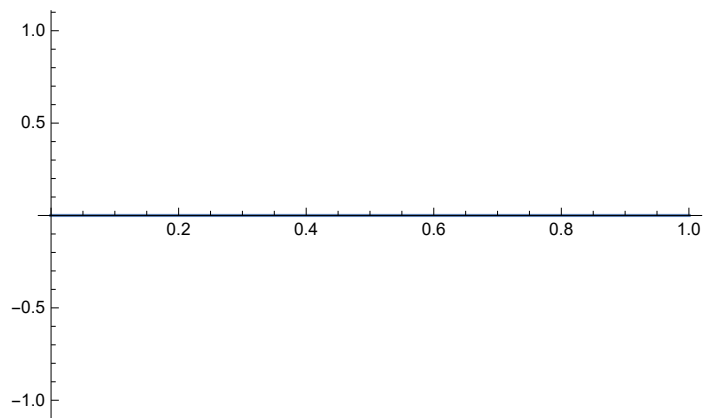

**Plot[Cf[10, 5, 4], {x, 0, 1}]**

[绘图](#)

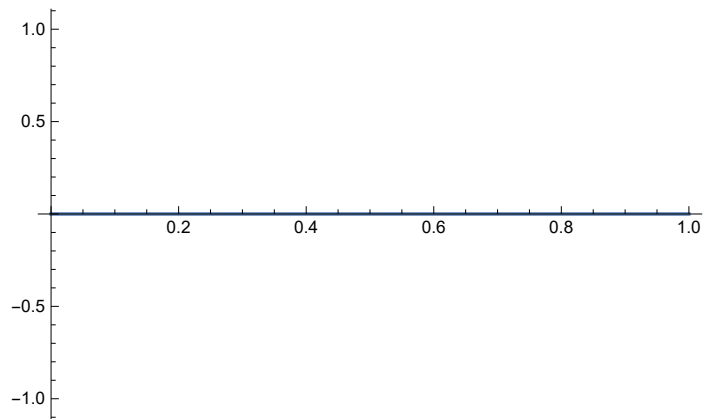

**Plot[Cf[10, 5, 3], {x, 0, 1}]**

[绘图](#)

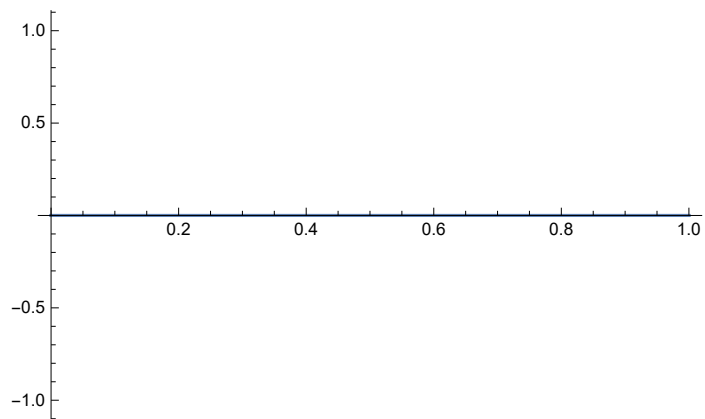

**Plot[Cf[10, 5, 2], {x, 0, 1}]**

[绘图](#)

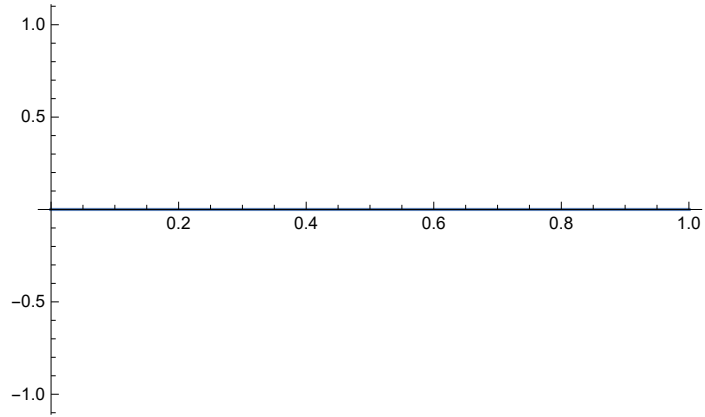

**Plot[Cf[10, 5, 1], {x, 0, 1}]**

[绘图](#)

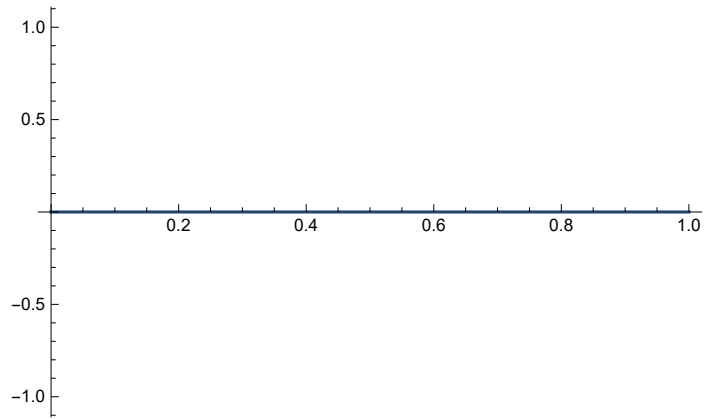

**Plot[Cf[10, 5, 0], {x, 0, 1}]**

[绘图](#)

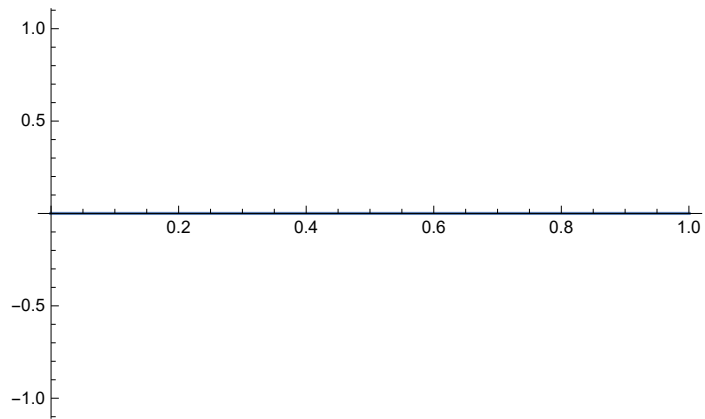

**(\*71th group coefficients r2^10r3^4\*)**

In[781]:= **Plot[Cf[10, 4, 14], {x, 0, 1}]**

[绘图](#)

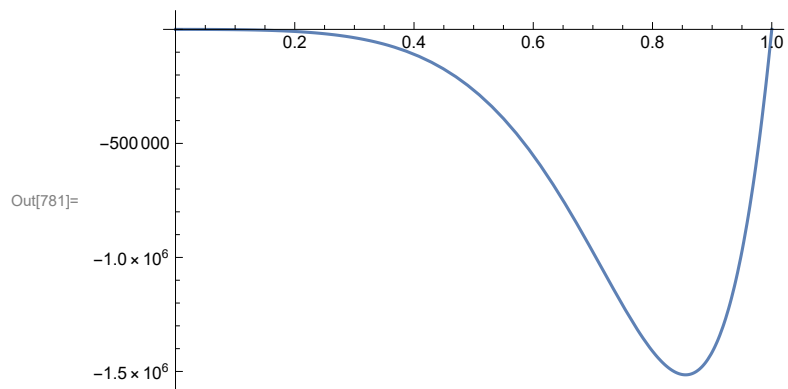

In[782]:= **Plot[Cf[10, 4, 13], {x, 0, 1}]**

[绘图](#)

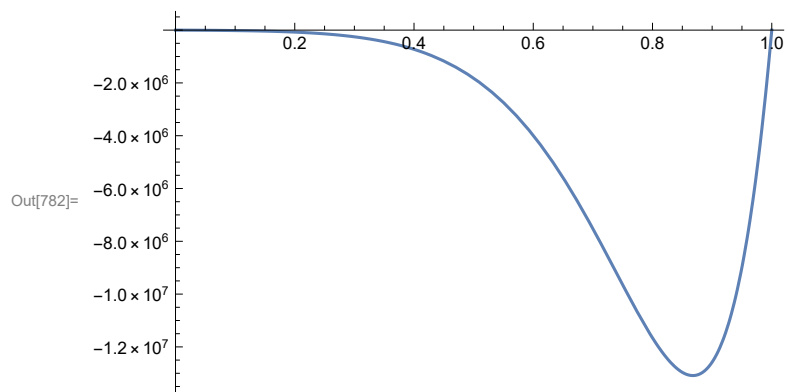

In[783]:= **Plot[Cf[10, 4, 12], {x, 0, 1}]**

[绘图](#)

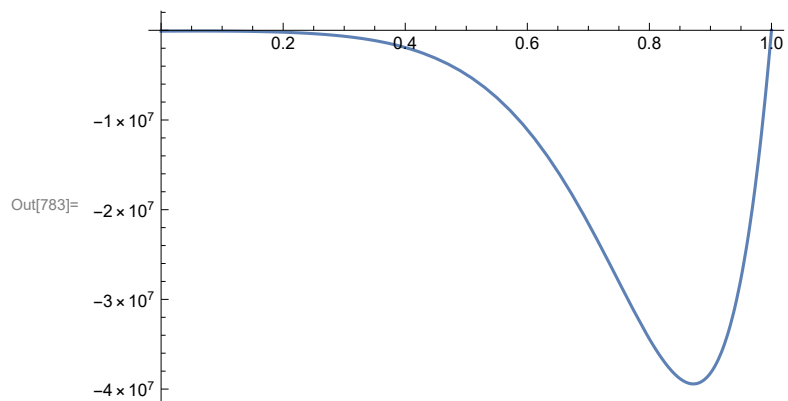

In[784]:= **Plot[Cf[10, 4, 11], {x, 0, 1}]**

[绘图](#)

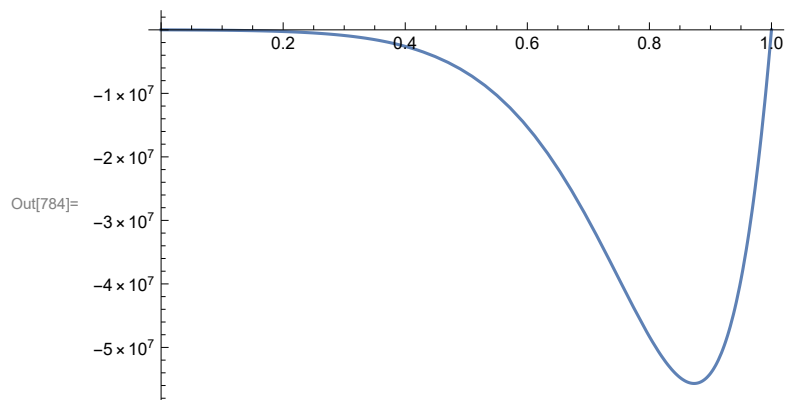

In[785]:= **Plot[Cf[10, 4, 10], {x, 0, 1}]**

[绘图](#)

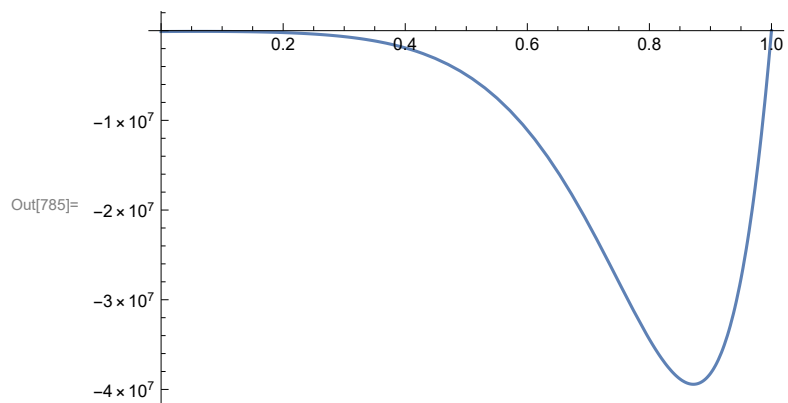

In[786]:= **Plot[Cf[10, 4, 9], {x, 0, 1}]**

[绘图](#)

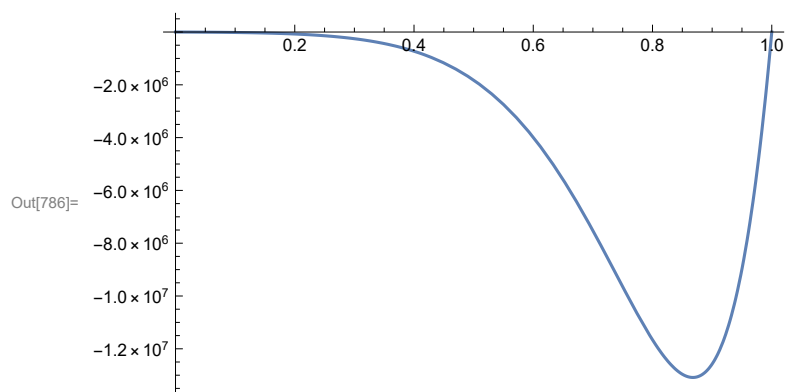

In[787]:= **Plot[Cf[10, 4, 8], {x, 0, 1}]**

[绘图](#)

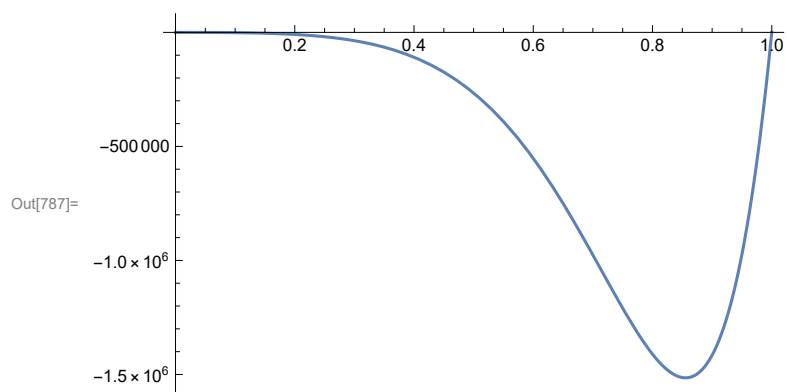

**Plot[Cf[10, 4, 7], {x, 0, 1}]**

[绘图](#)

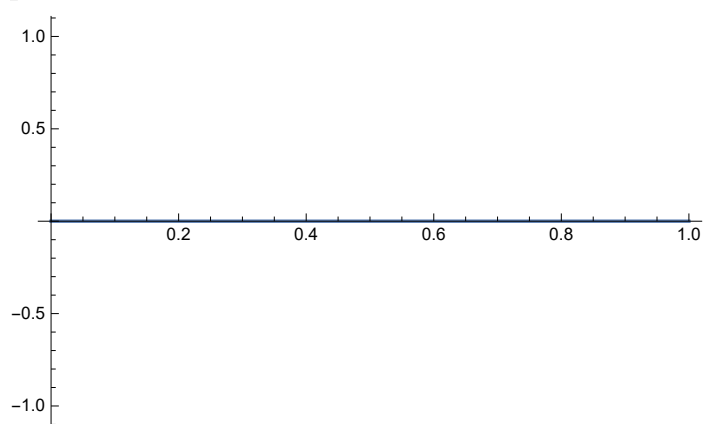

**Plot[Cf[10, 4, 6], {x, 0, 1}]**

[绘图](#)

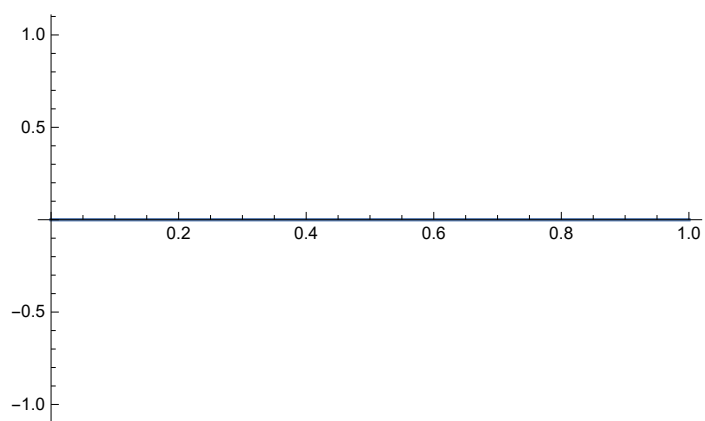

```
Plot[Cf[10, 4, 5], {x, 0, 1}]
```

[绘图](#)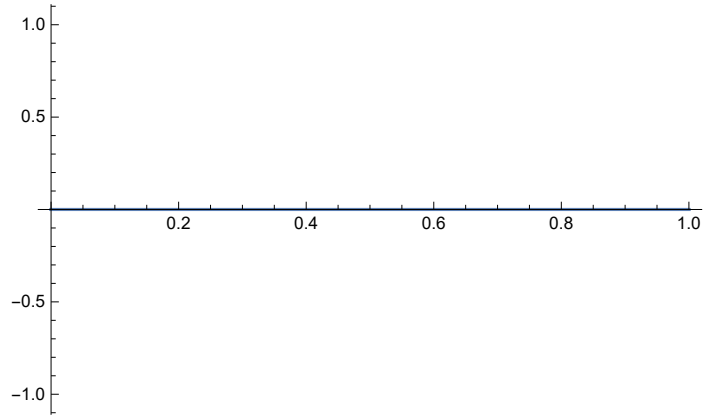

```
Plot[Cf[10, 4, 4], {x, 0, 1}]
```

[绘图](#)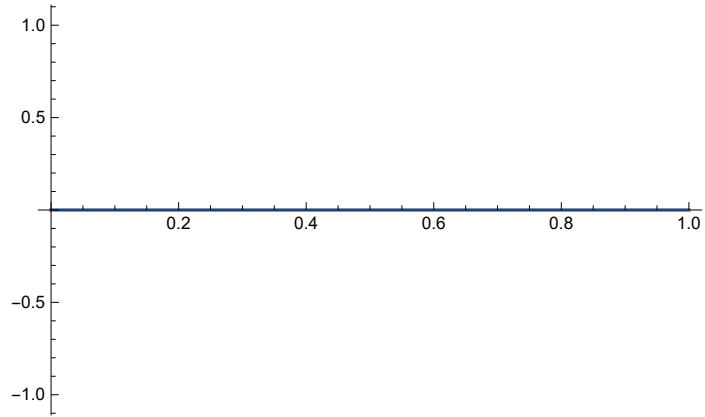

```
Plot[Cf[10, 4, 3], {x, 0, 1}]
```

[绘图](#)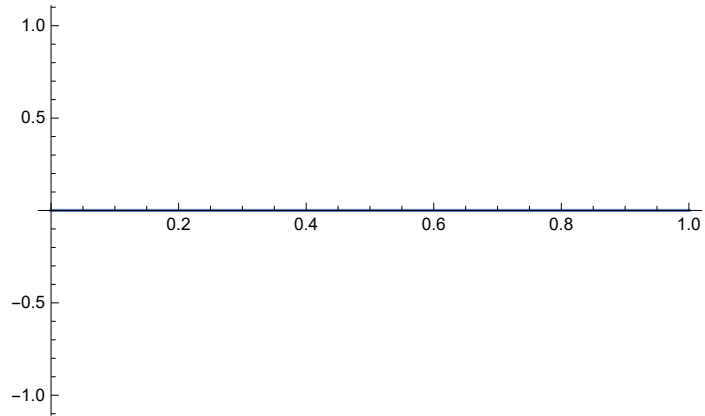



**Plot[Cf[10, 4, 2], {x, 0, 1}]**

[绘图](#)

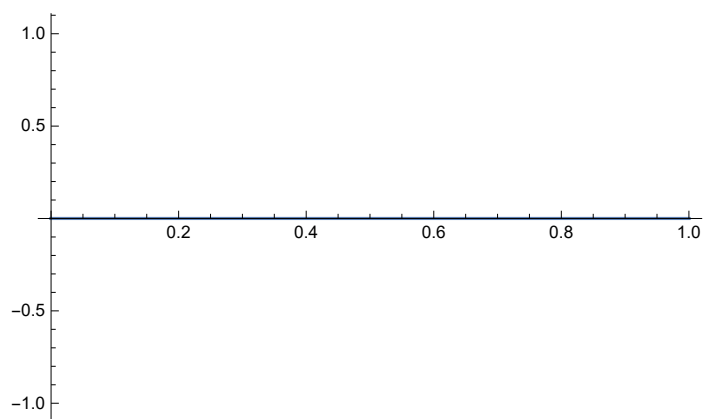

**Plot[Cf[10, 4, 1], {x, 0, 1}]**

[绘图](#)

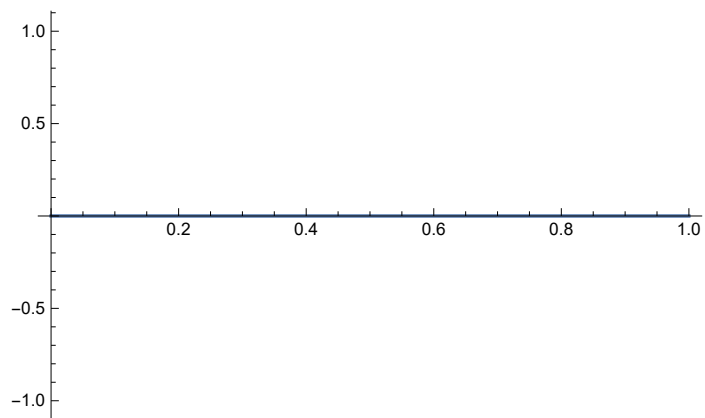

**Plot[Cf[10, 4, 0], {x, 0, 1}]**

[绘图](#)

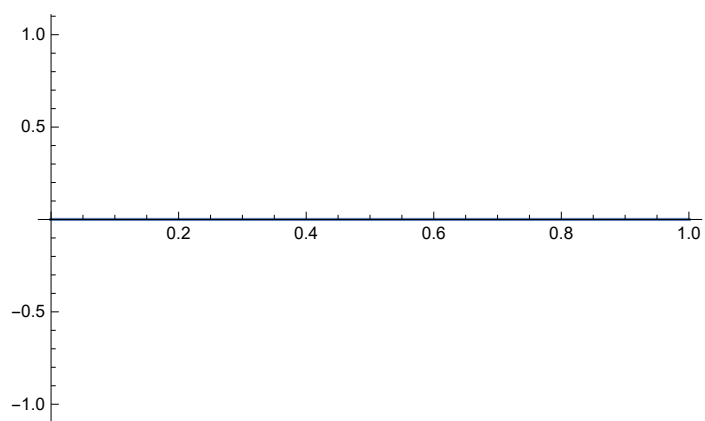

**(\*72th group coefficients r2^10r3^3\*)**

In[788]:= **Plot[Cf[10, 3, 14], {x, 0, 1}]**

[绘图](#)

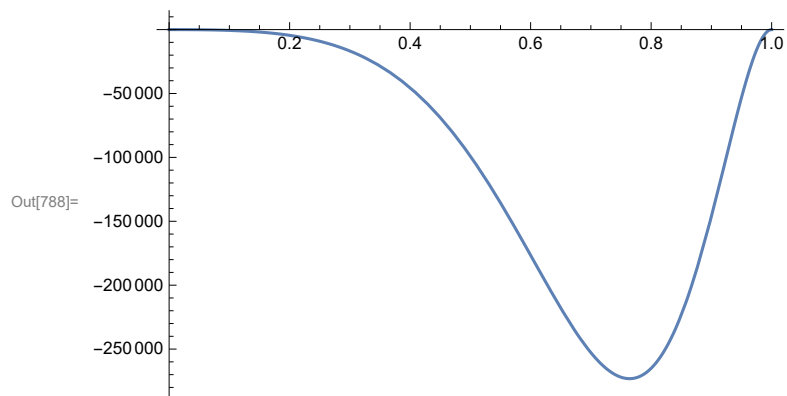

In[789]:= **Plot[Cf[10, 3, 13], {x, 0, 1}]**

[绘图](#)

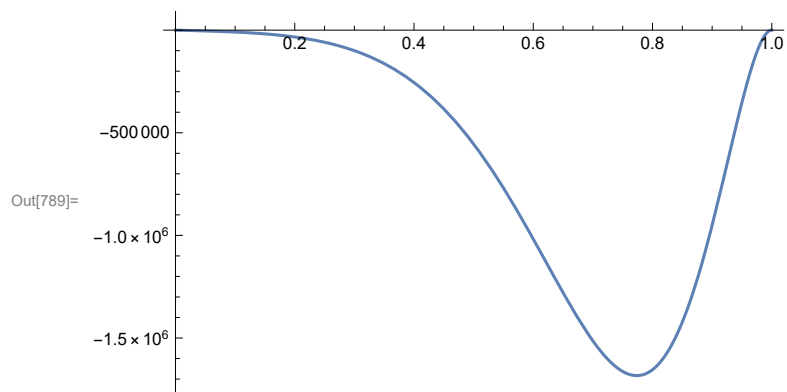

In[790]:= **Plot[Cf[10, 3, 12], {x, 0, 1}]**

[绘图](#)

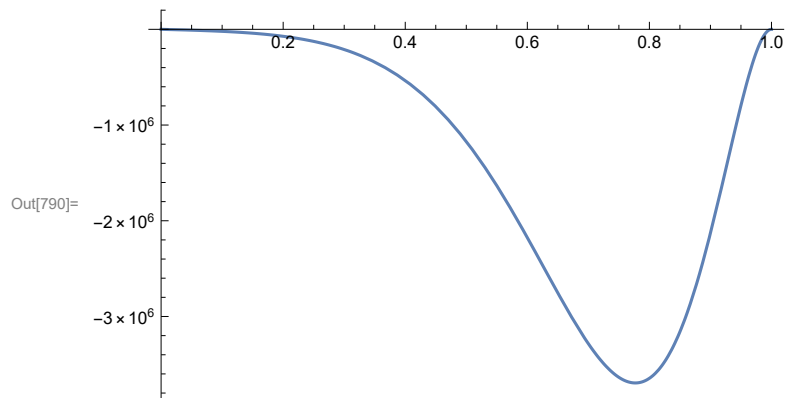

In[791]:= **Plot[Cf[10, 3, 11], {x, 0, 1}]**

[绘图](#)

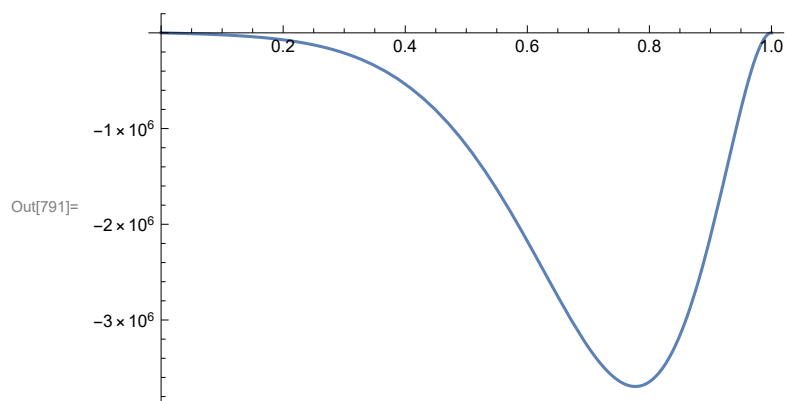

In[792]:= **Plot[Cf[10, 3, 10], {x, 0, 1}]**

[绘图](#)

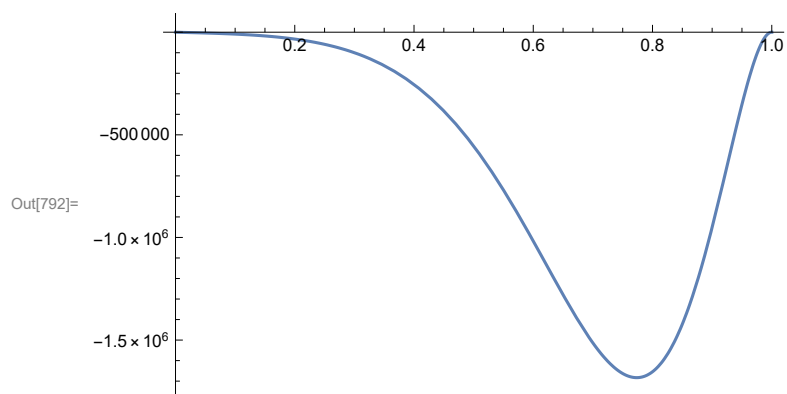

In[793]:= **Plot[Cf[10, 3, 9], {x, 0, 1}]**

[绘图](#)

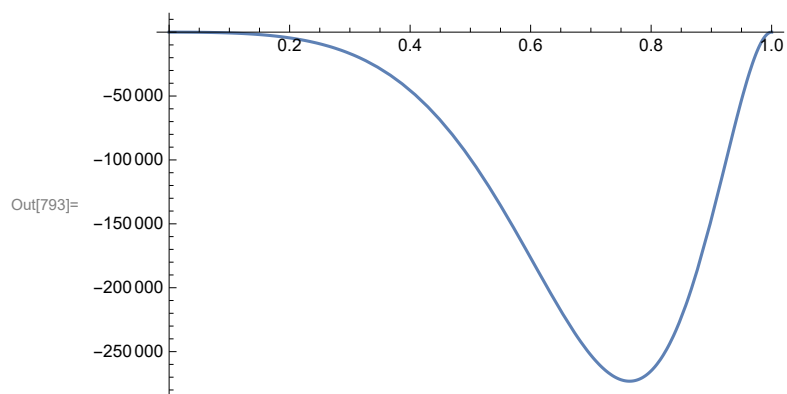

```
Plot[Cf[10, 3, 8], {x, 0, 1}]
```

[绘图](#)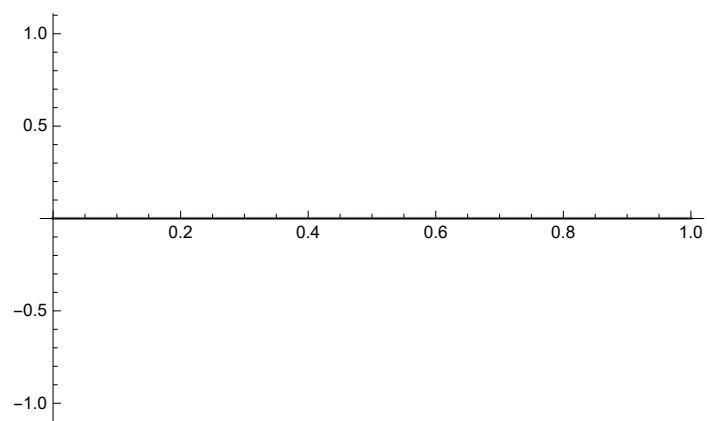

```
Plot[Cf[10, 3, 7], {x, 0, 1}]
```

[绘图](#)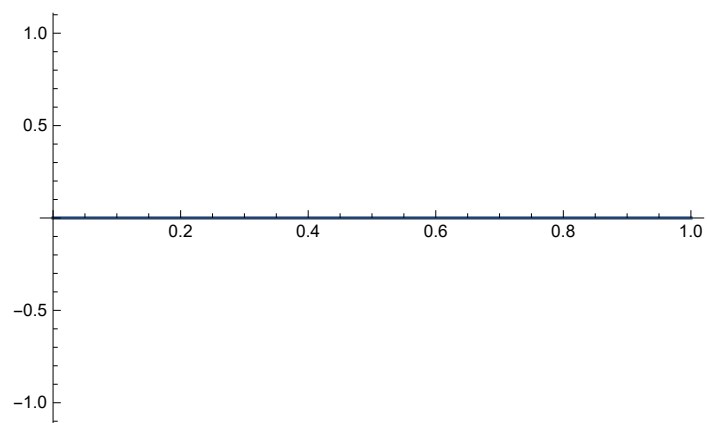

```
Plot[Cf[10, 3, 6], {x, 0, 1}]
```

[绘图](#)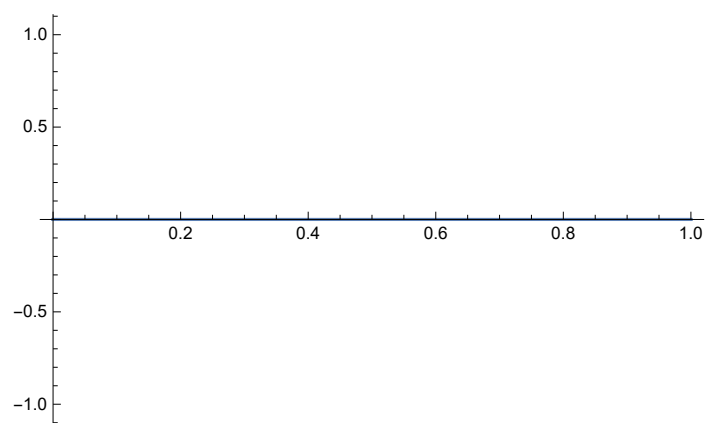

```
Plot[Cf[10, 3, 5], {x, 0, 1}]
```

[绘图](#)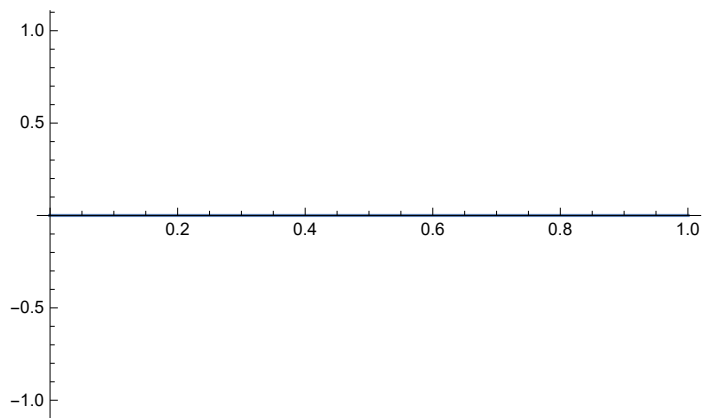

```
Plot[Cf[10, 3, 4], {x, 0, 1}]
```

[绘图](#)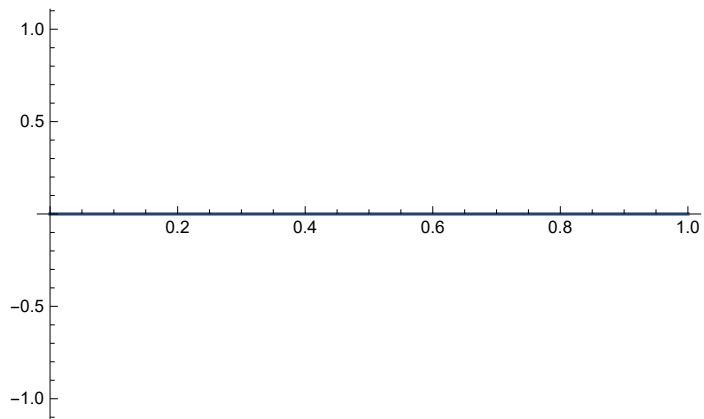

```
Plot[Cf[10, 3, 3], {x, 0, 1}]
```

[绘图](#)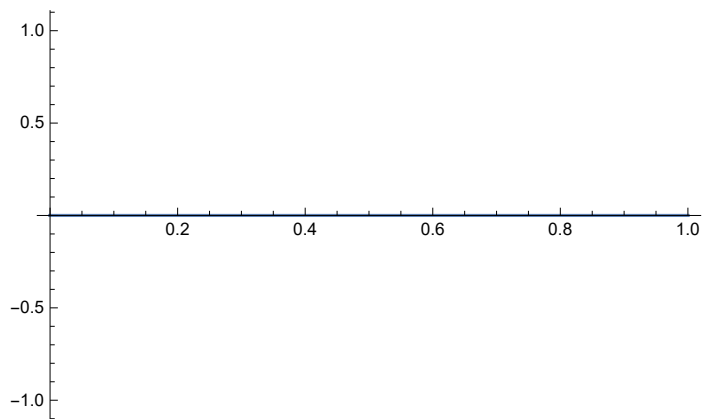

**Plot[Cf[10, 3, 2], {x, 0, 1}]**

[绘图](#)

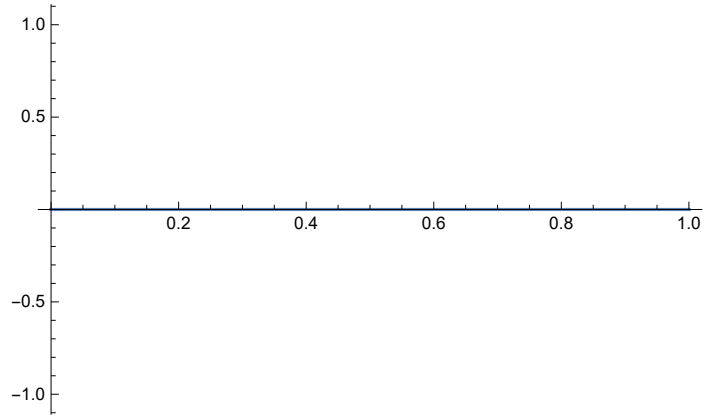

**Plot[Cf[10, 3, 1], {x, 0, 1}]**

[绘图](#)

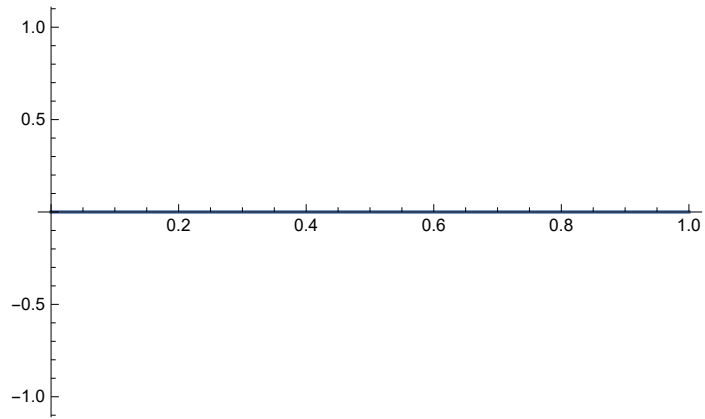

**Plot[Cf[10, 3, 0], {x, 0, 1}]**

[绘图](#)

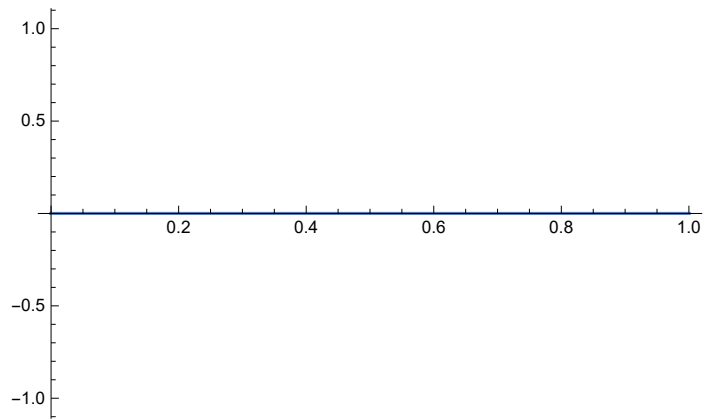

**(\*73th group coefficients r2^10r3^2\*)**

In[794]:= **Plot[Cf[10, 2, 14], {x, 0, 1}]**

[绘图](#)

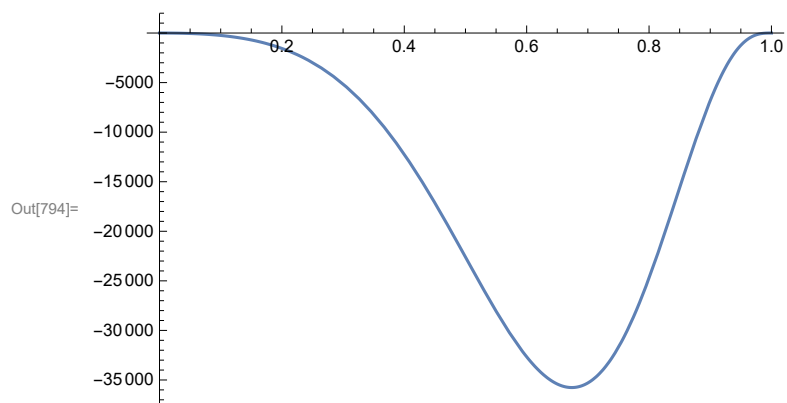

In[795]:= **Plot[Cf[10, 2, 13], {x, 0, 1}]**

[绘图](#)

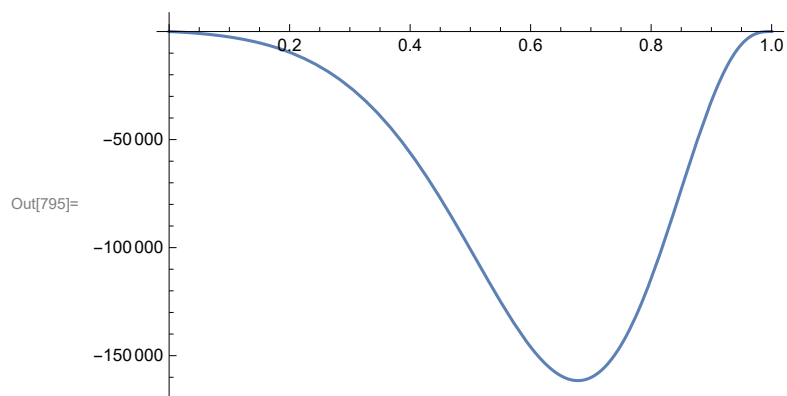

In[796]:= **Plot[Cf[10, 2, 12], {x, 0, 1}]**

[绘图](#)

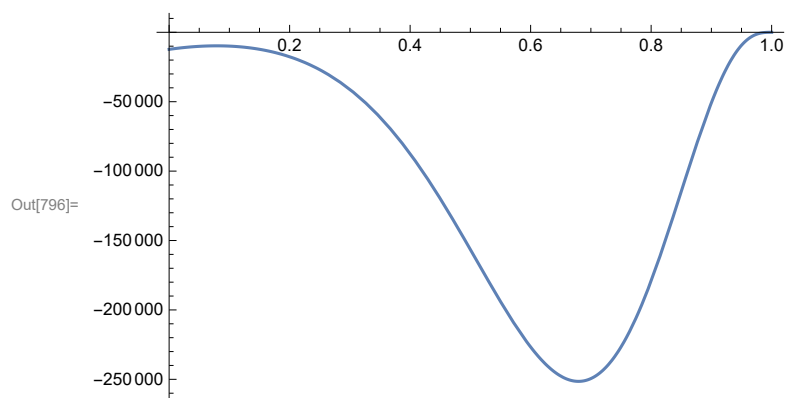

In[797]:= **Plot**[**Cf**[10, 2, 11], {x, 0, 1}]

[绘图](#)

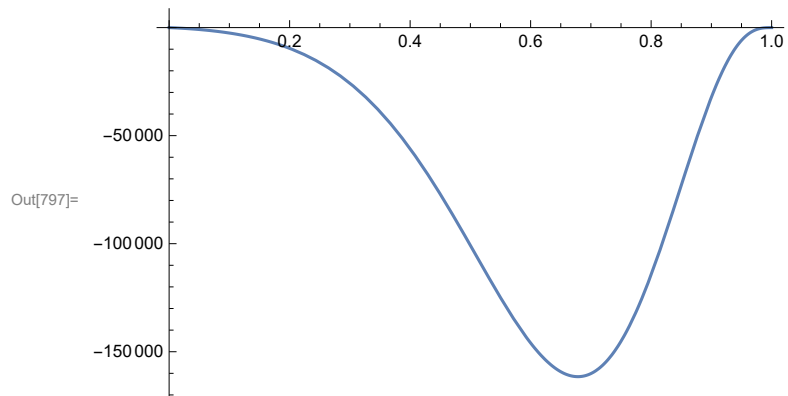

In[798]:= **Plot**[**Cf**[10, 2, 12], {x, 0, 1}]

[绘图](#)

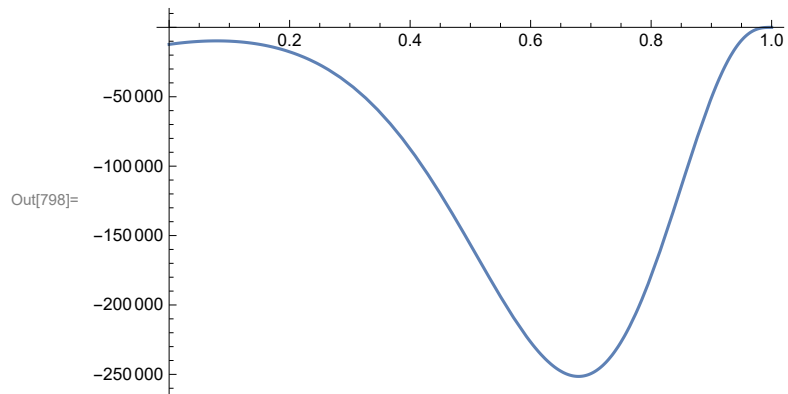

In[799]:= **Plot**[**Cf**[10, 2, 13], {x, 0, 1}]

[绘图](#)

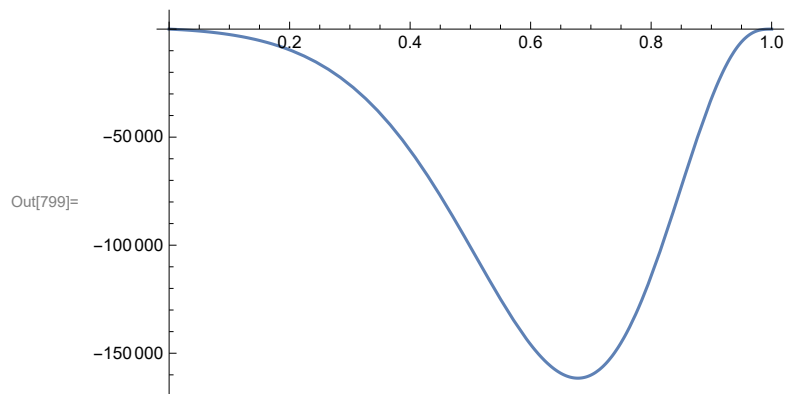



In[800]:= **Plot[Cf[10, 2, 12], {x, 0, 1}]**

[绘图](#)

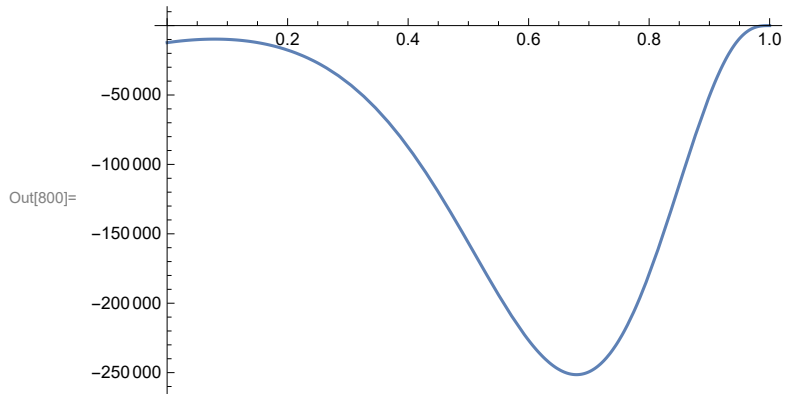

In[801]:= **Plot[Cf[10, 2, 11], {x, 0, 1}]**

[绘图](#)

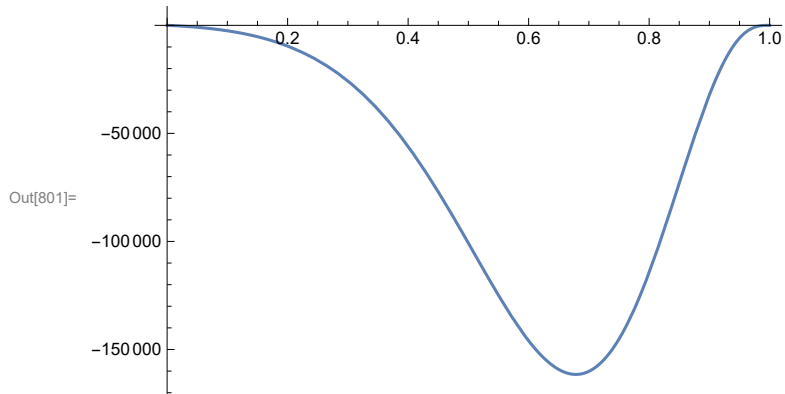

In[802]:= **Plot[Cf[10, 2, 10], {x, 0, 1}]**

[绘图](#)

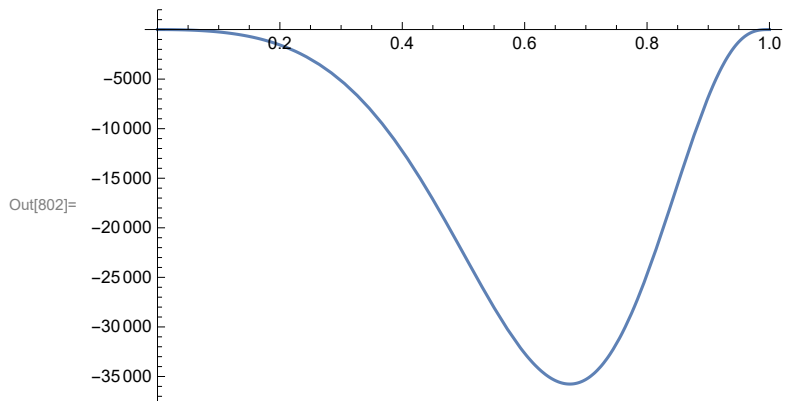

**Plot[Cf[10, 2, 9], {x, 0, 1}]**

[绘图](#)

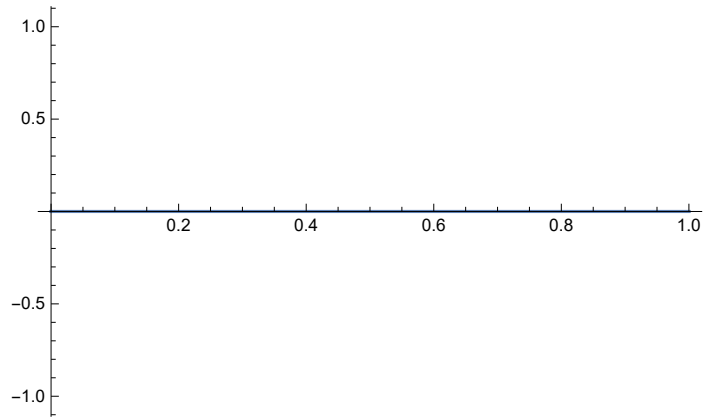

**Plot[Cf[10, 2, 8], {x, 0, 1}]**

[绘图](#)

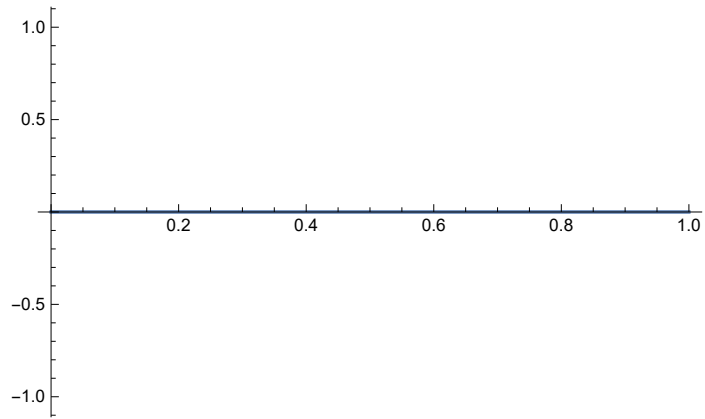

**Plot[Cf[10, 2, 7], {x, 0, 1}]**

[绘图](#)

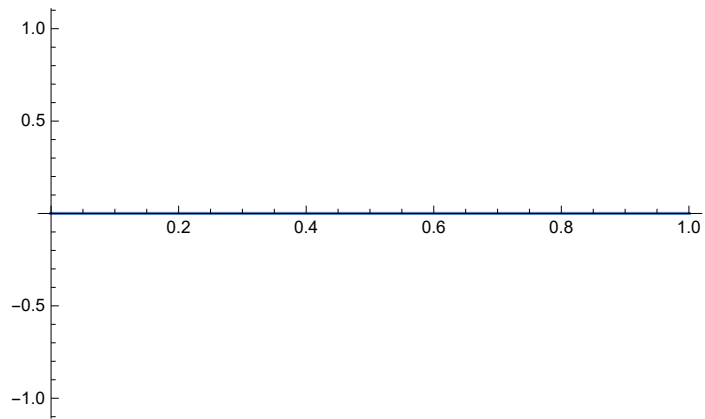

**Plot[Cf[10, 2, 6], {x, 0, 1}]**

[绘图](#)

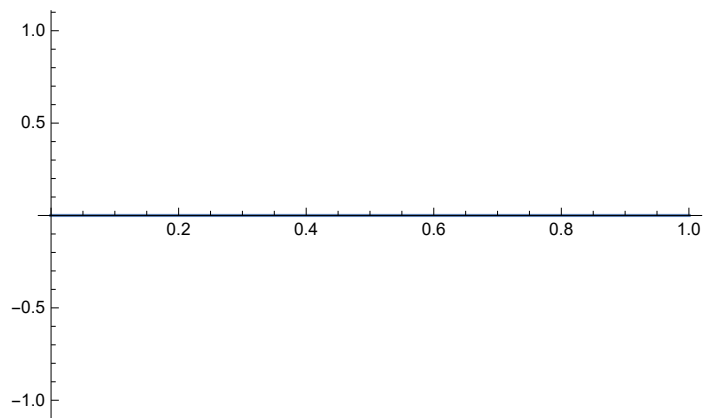

**Plot[Cf[10, 2, 5], {x, 0, 1}]**

[绘图](#)

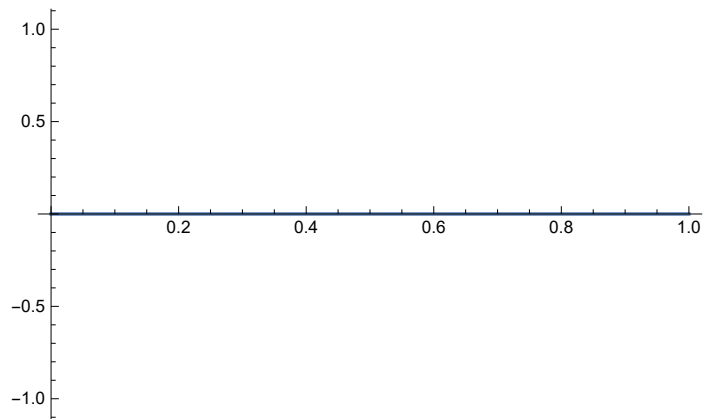

**Plot[Cf[10, 2, 4], {x, 0, 1}]**

[绘图](#)

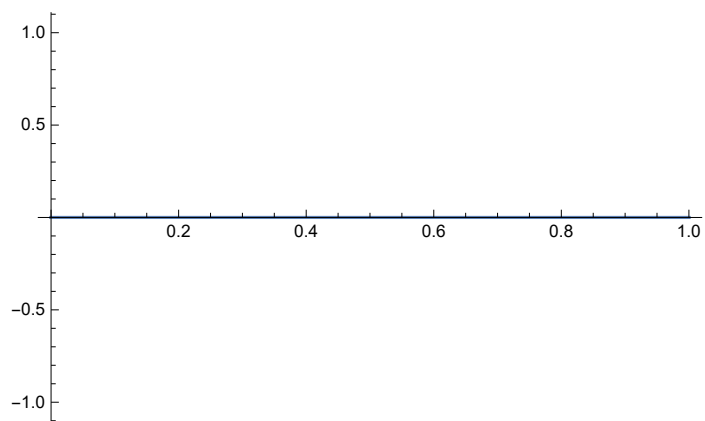

```
Plot[Cf[10, 2, 3], {x, 0, 1}]
```

[绘图](#)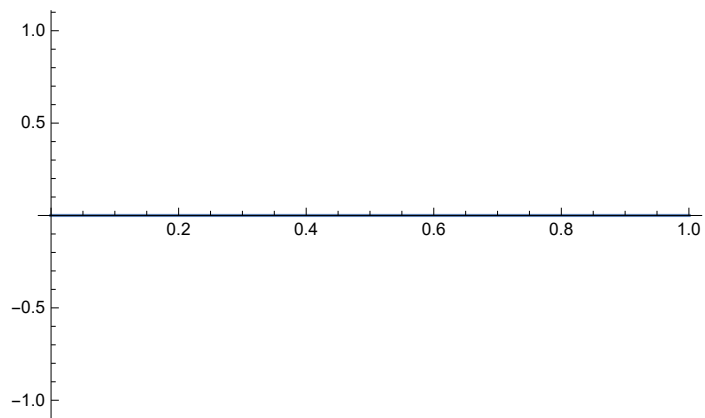

```
Plot[Cf[10, 2, 2], {x, 0, 1}]
```

[绘图](#)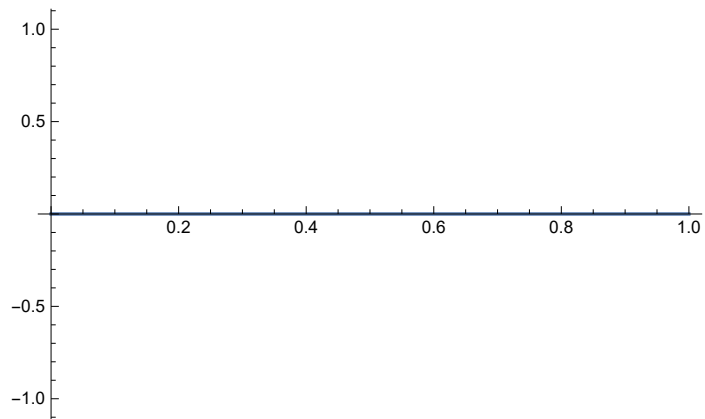

```
Plot[Cf[10, 2, 1], {x, 0, 1}]
```

[绘图](#)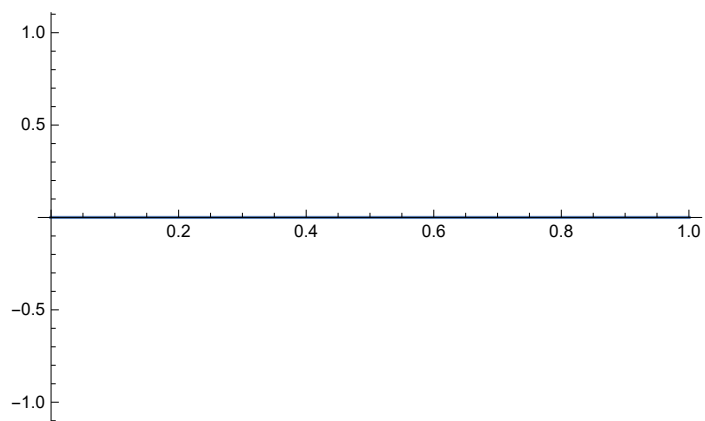

**Plot[Cf[10, 2, 0], {x, 0, 1}]**

[绘图](#)

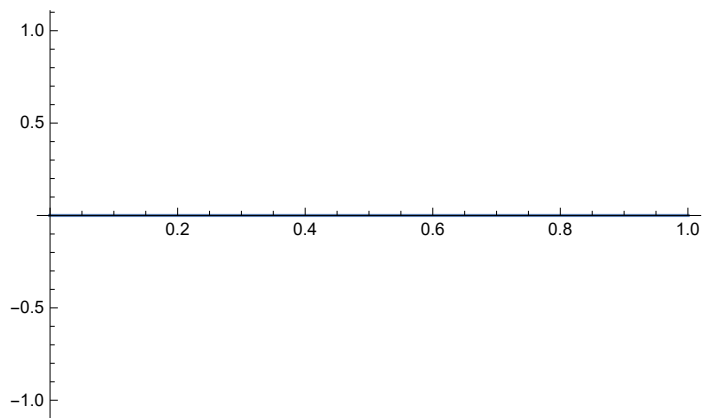

(\*74th group coefficients r2^10r3^1\*)

In[803]:= **Plot[Cf[10, 1, 14], {x, 0, 1}]**

[绘图](#)

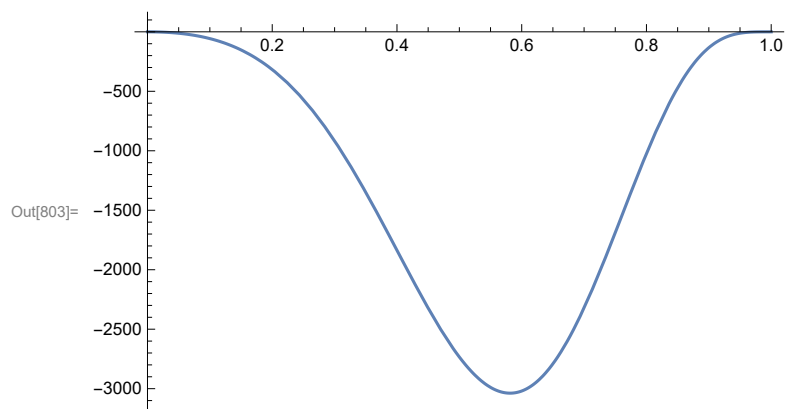

In[804]:= **Plot[Cf[10, 1, 13], {x, 0, 1}]**

[绘图](#)

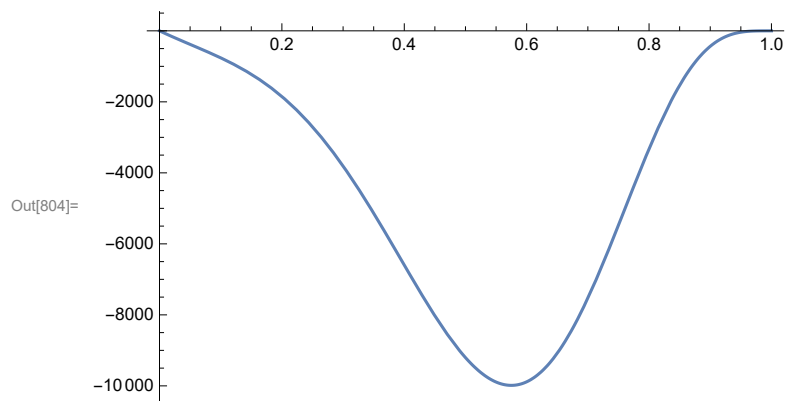

In[805]:= **Plot[Cf[10, 1, 12], {x, 0, 1}]**

[绘图](#)

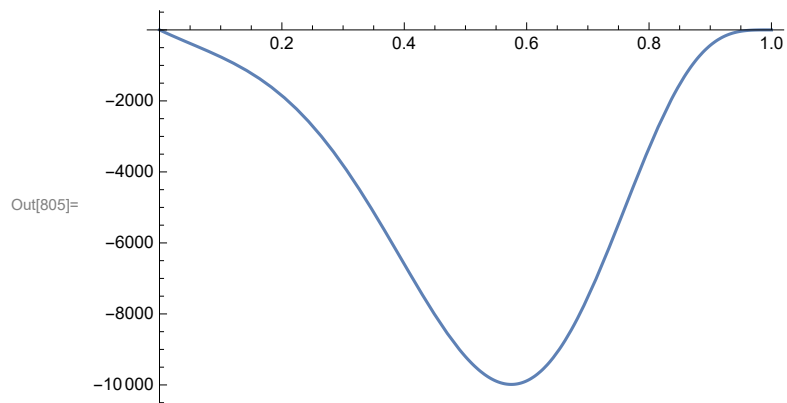

In[806]:= **Plot[Cf[10, 1, 11], {x, 0, 1}]**

[绘图](#)

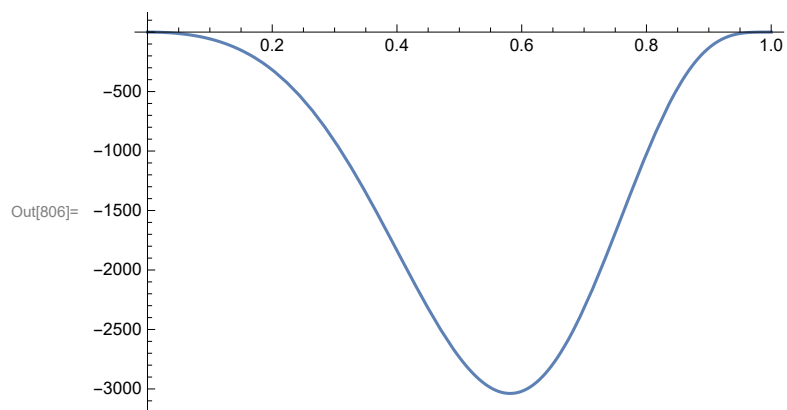

**Plot[Cf[10, 1, 10], {x, 0, 1}]**

[绘图](#)

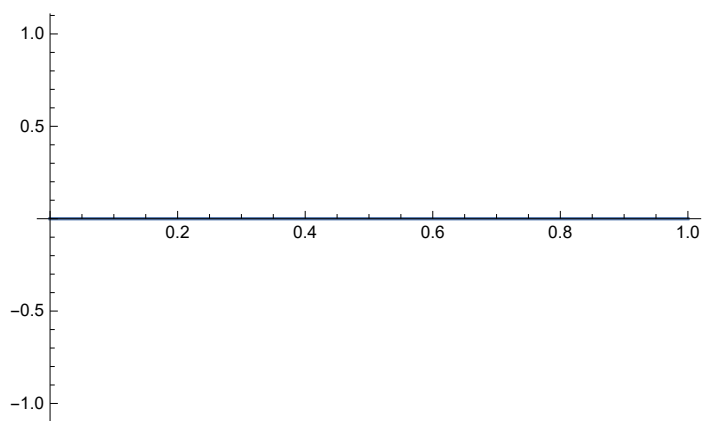

```
Plot[Cf[10, 1, 9], {x, 0, 1}]
```

[绘图](#)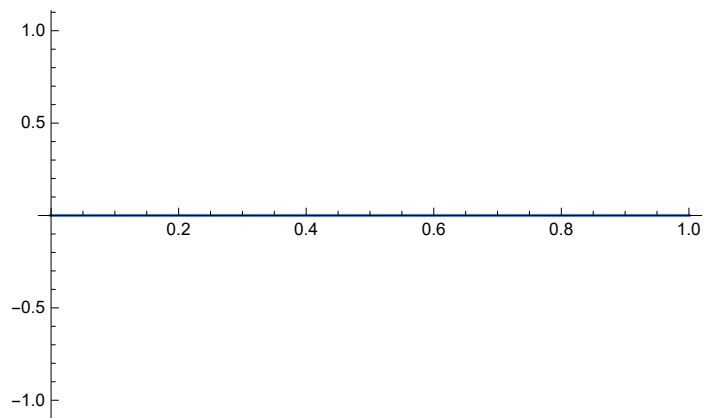

```
Plot[Cf[10, 1, 8], {x, 0, 1}]
```

[绘图](#)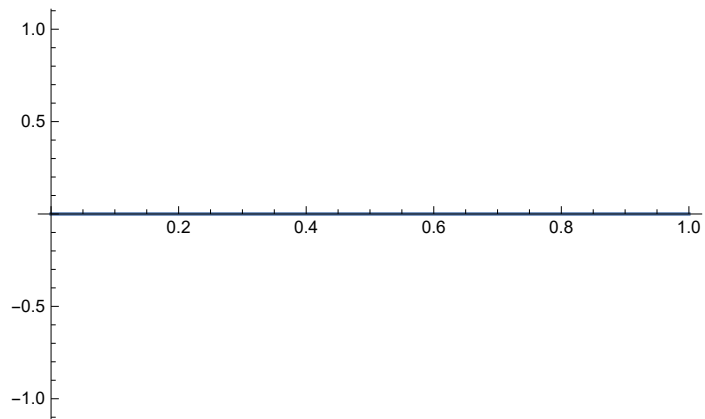

```
Plot[Cf[10, 1, 7], {x, 0, 1}]
```

[绘图](#)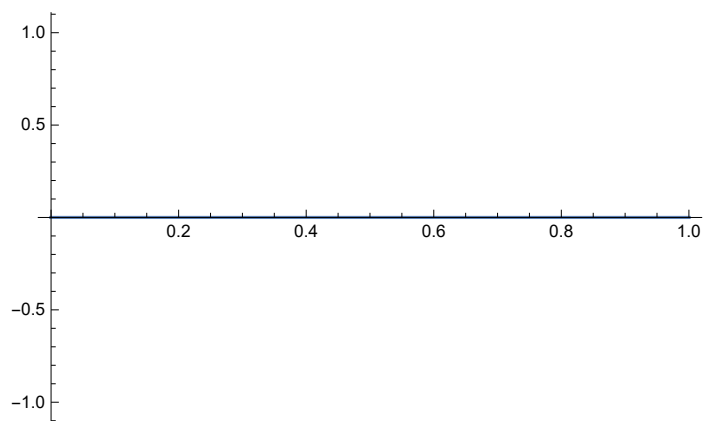

```
Plot[Cf[10, 1, 6], {x, 0, 1}]
```

[绘图](#)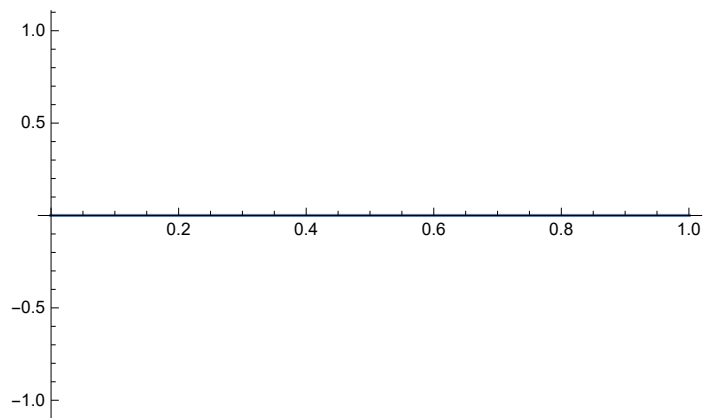

```
Plot[Cf[10, 1, 5], {x, 0, 1}]
```

[绘图](#)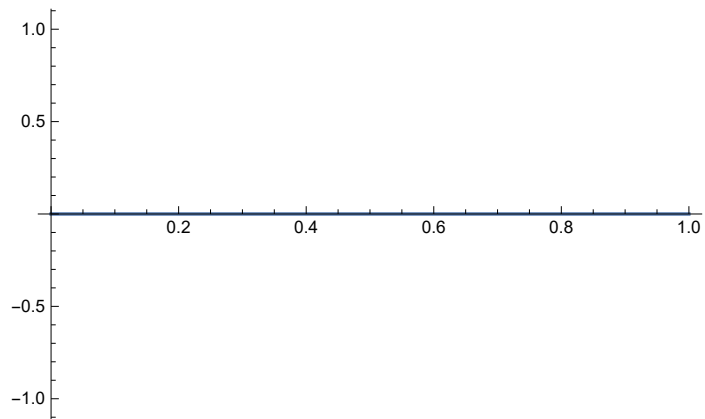

```
Plot[Cf[10, 1, 4], {x, 0, 1}]
```

[绘图](#)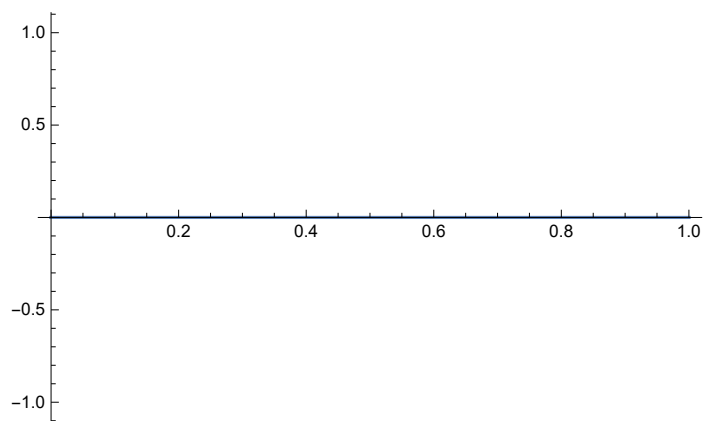



```
Plot[Cf[10, 1, 3], {x, 0, 1}]
```

[绘图](#)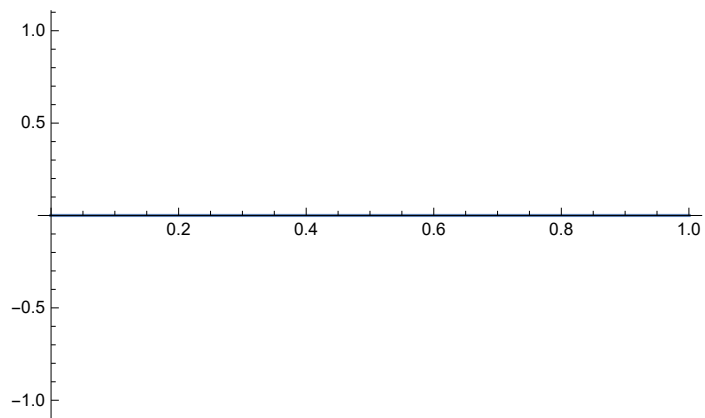

```
Plot[Cf[10, 1, 2], {x, 0, 1}]
```

[绘图](#)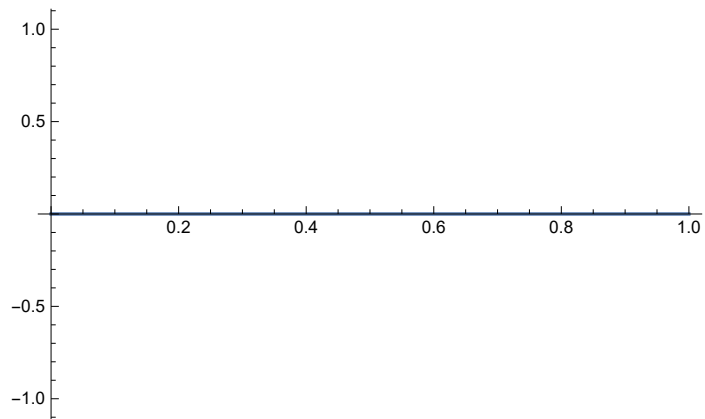

```
Plot[Cf[10, 1, 1], {x, 0, 1}]
```

[绘图](#)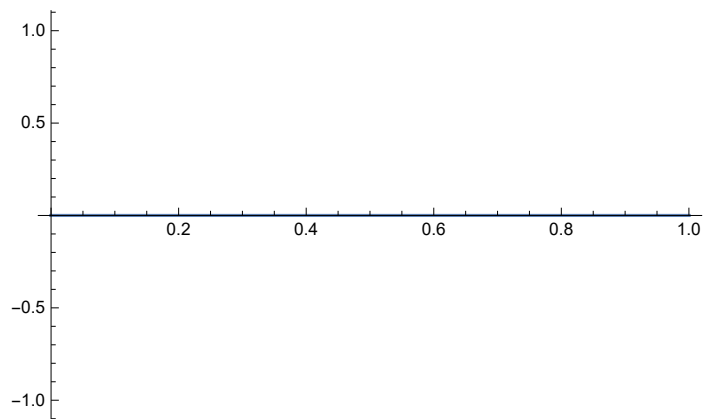

**Plot[Cf[10, 1, 0], {x, 0, 1}]**

[绘图](#)

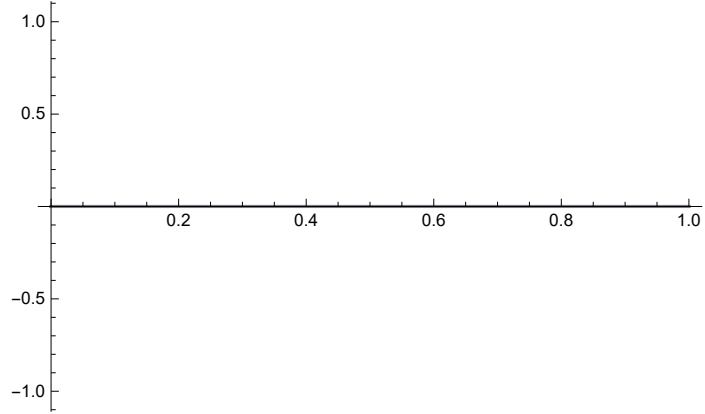

**(\*75th group coefficients r2^10r3^0\*)**

In[807]:= **Plot[Cf[10, 0, 14], {x, 0, 1}]**

[绘图](#)

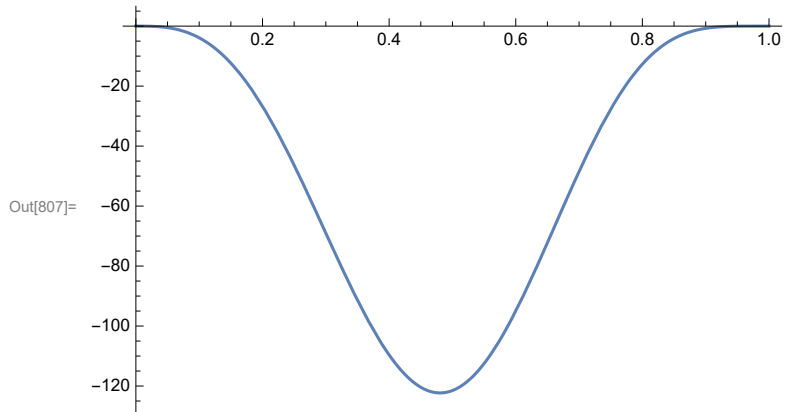

In[808]:= **Plot[Cf[10, 0, 13], {x, 0, 1}]**

[绘图](#)

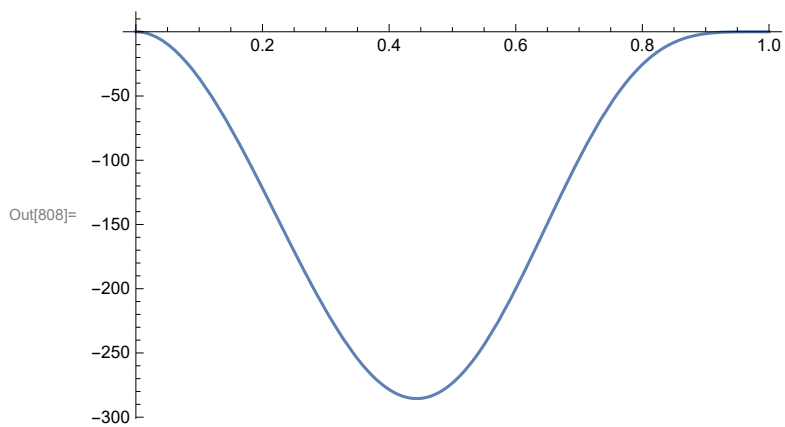

In[809]:= **Plot[Cf[10, 0, 12], {x, 0, 1}]**

[绘图](#)

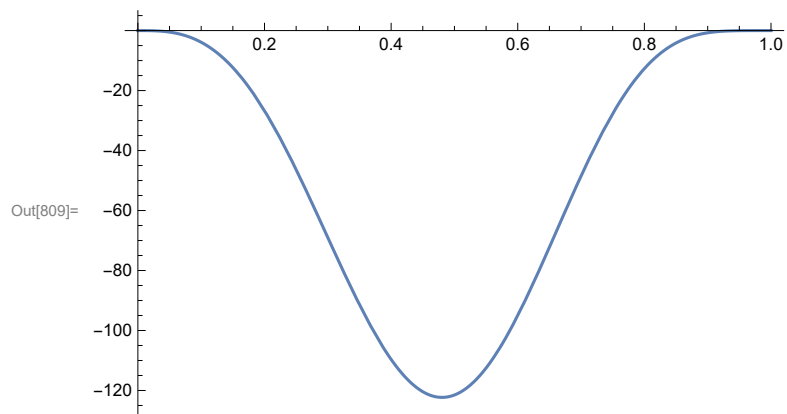

**Plot[Cf[10, 0, 11], {x, 0, 1}]**

[绘图](#)

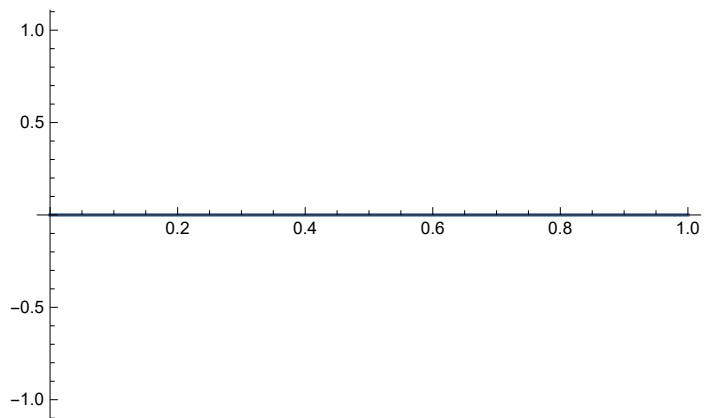

**Plot[Cf[10, 0, 10], {x, 0, 1}]**

[绘图](#)

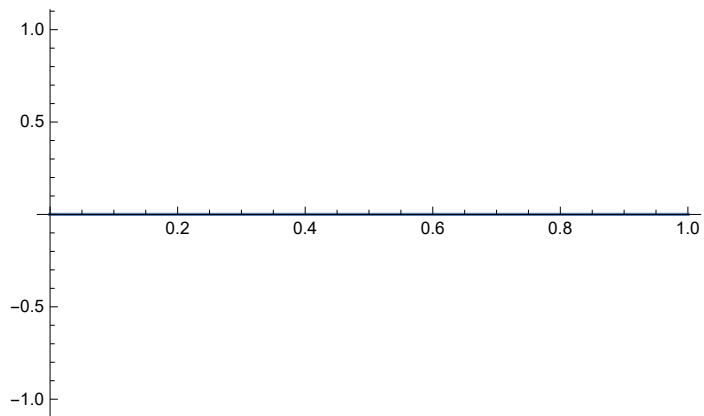

```
Plot[Cf[10, 0, 9], {x, 0, 1}]
```

[绘图](#)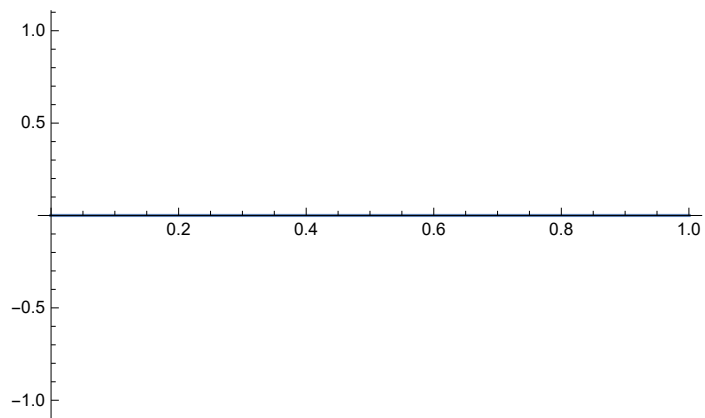

```
Plot[Cf[10, 0, 8], {x, 0, 1}]
```

[绘图](#)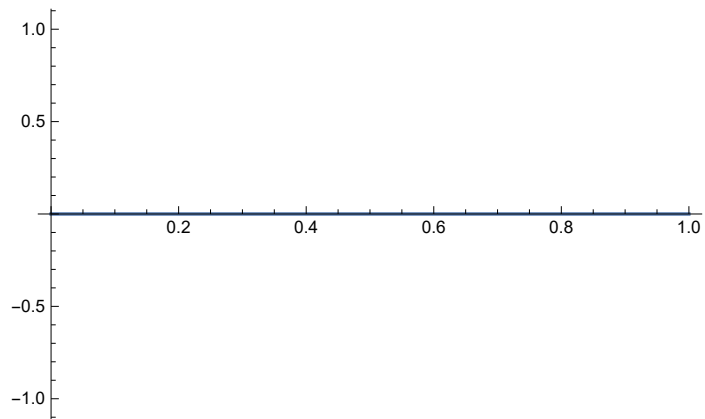

```
Plot[Cf[10, 0, 7], {x, 0, 1}]
```

[绘图](#)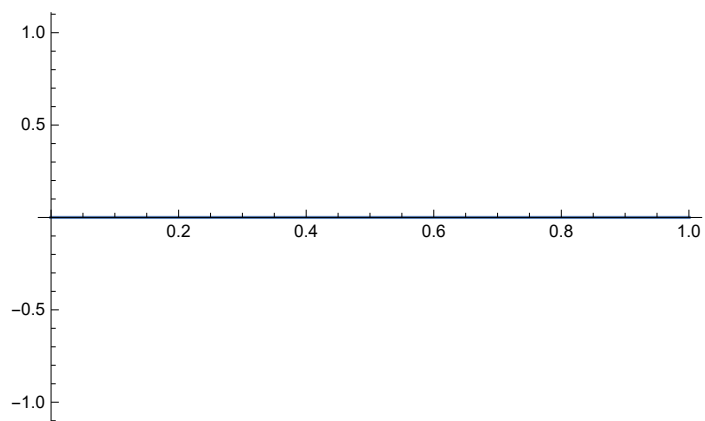

```
Plot[Cf[10, 0, 6], {x, 0, 1}]
```

[绘图](#)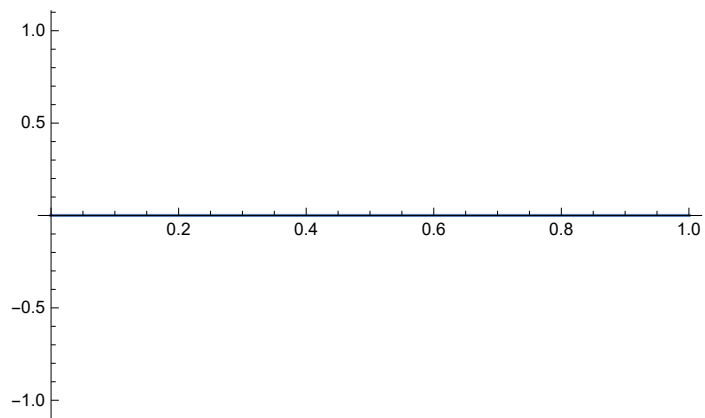

```
Plot[Cf[10, 0, 5], {x, 0, 1}]
```

[绘图](#)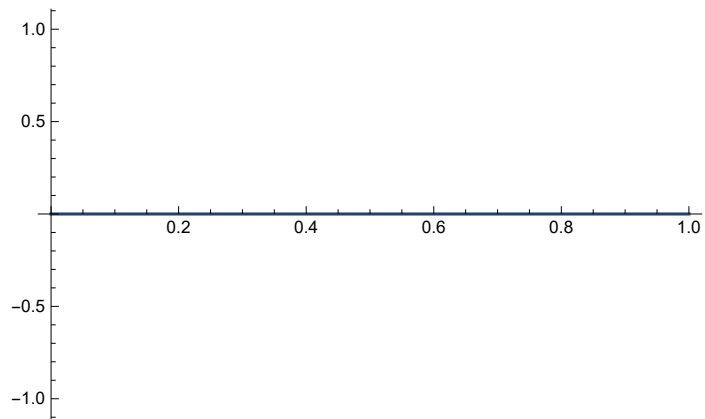

```
Plot[Cf[10, 0, 4], {x, 0, 1}]
```

[绘图](#)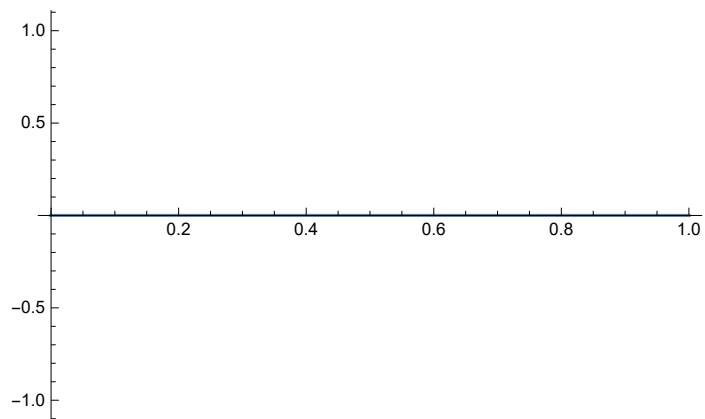

```
Plot[Cf[10, 0, 3], {x, 0, 1}]
```

[绘图](#)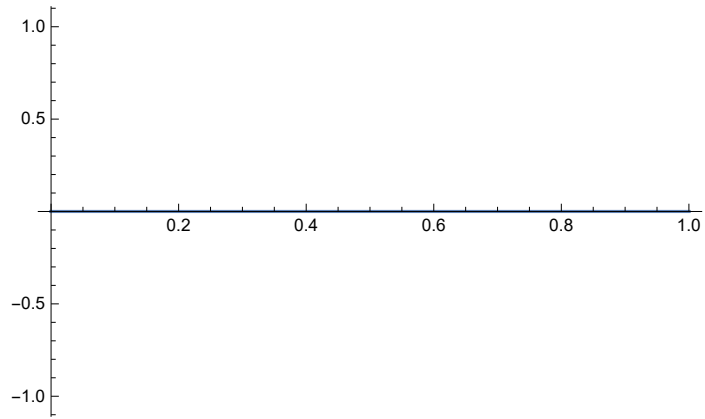

```
Plot[Cf[10, 0, 2], {x, 0, 1}]
```

[绘图](#)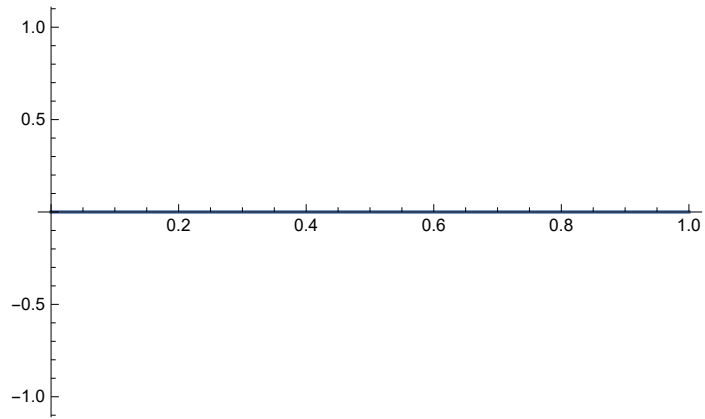

```
Plot[Cf[10, 0, 1], {x, 0, 1}]
```

[绘图](#)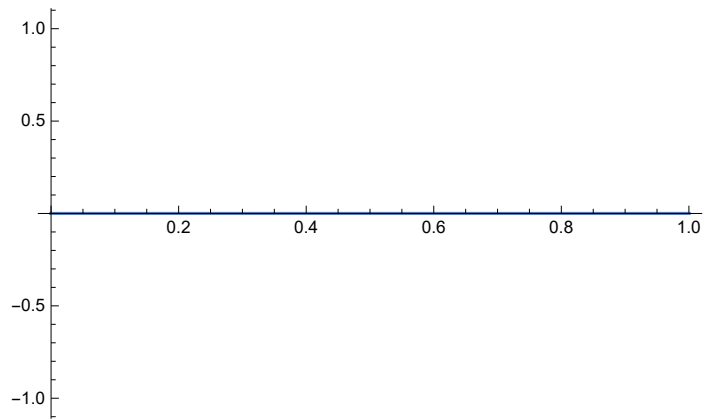

**Plot[Cf[10, 0, 0], {x, 0, 1}]**

[绘图](#)

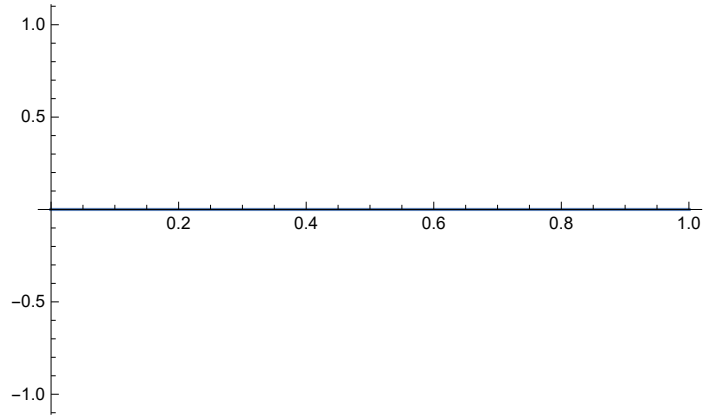

**(\*76th group coefficients r2^9r3^14\*)**

**Plot[Cf[9, 14, 14], {x, 0, 1}]**

[绘图](#)

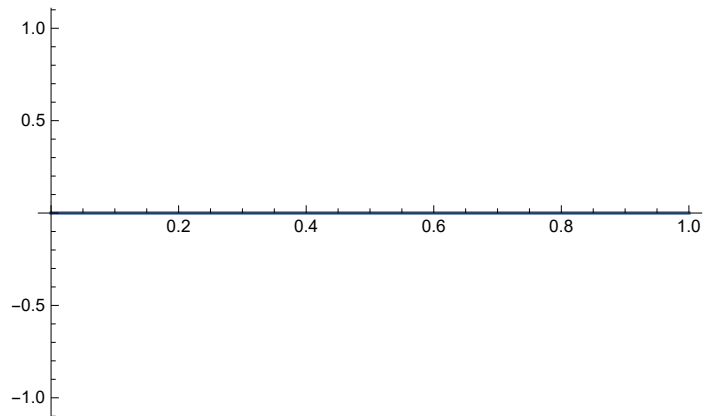

In[810]:= **Plot[Cf[9, 14, 13], {x, 0, 1}]**

[绘图](#)

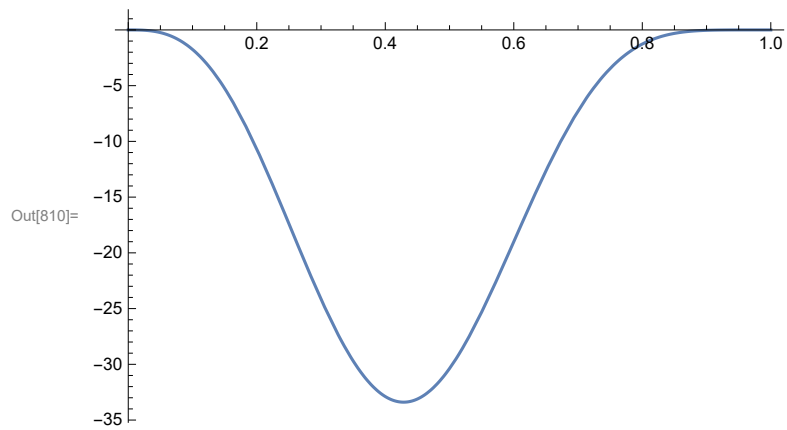

In[811]:= **Plot[Cf[9, 14, 12], {x, 0, 1}]**

[绘图](#)

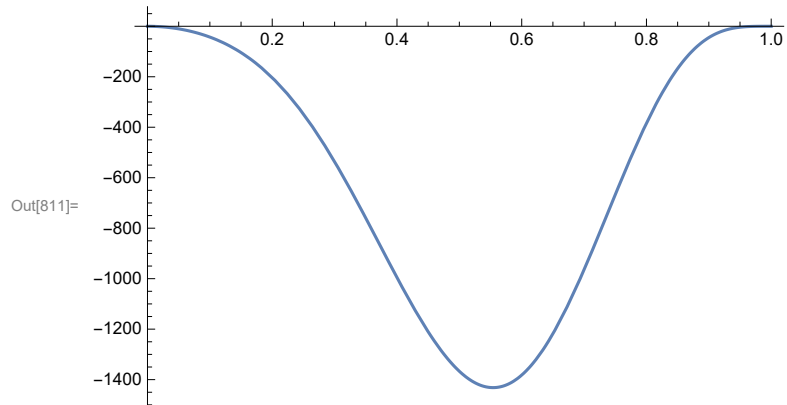

In[812]:= **Plot[Cf[9, 14, 11], {x, 0, 1}]**

[绘图](#)

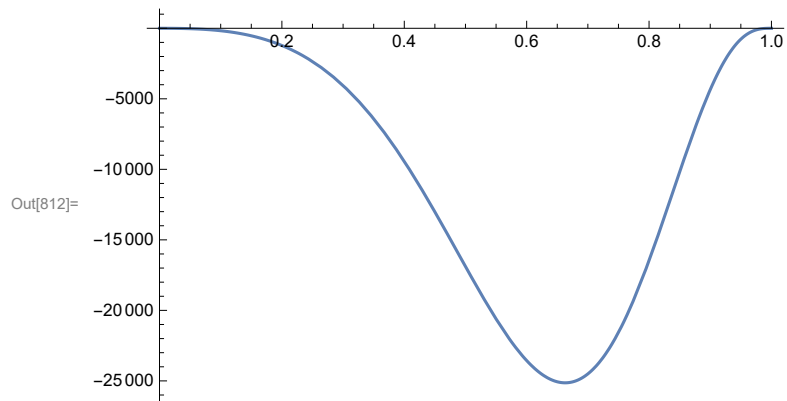

In[813]:= **Plot[Cf[9, 14, 10], {x, 0, 1}]**

[绘图](#)

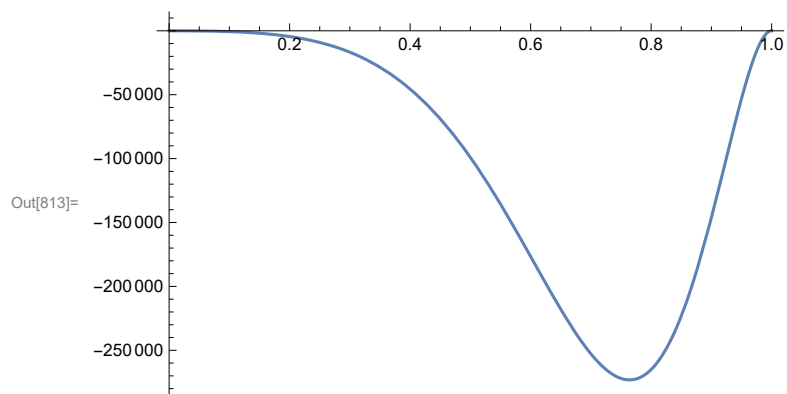



In[814]:= **Plot[Cf[9, 14, 9], {x, 0, 1}]**

[绘图](#)

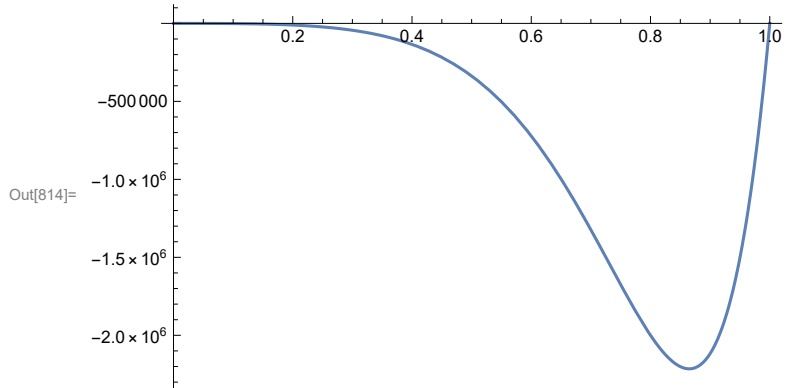

In[815]:= **Plot[Cf[9, 14, 8], {x, 0, 1}]**

[绘图](#)

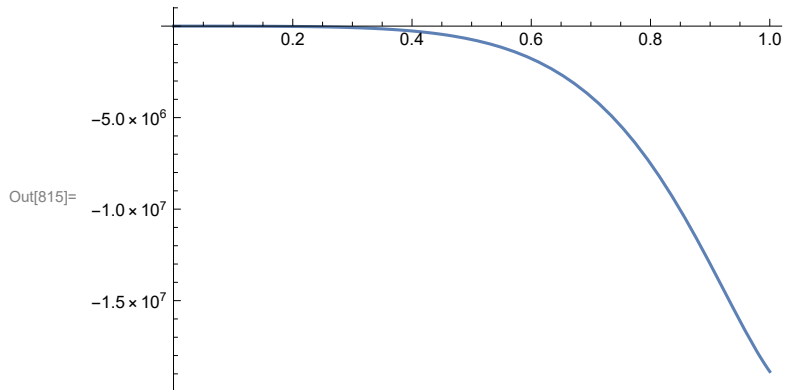

In[816]:= **Plot[Cf[9, 14, 7], {x, 0, 1}]**

[绘图](#)

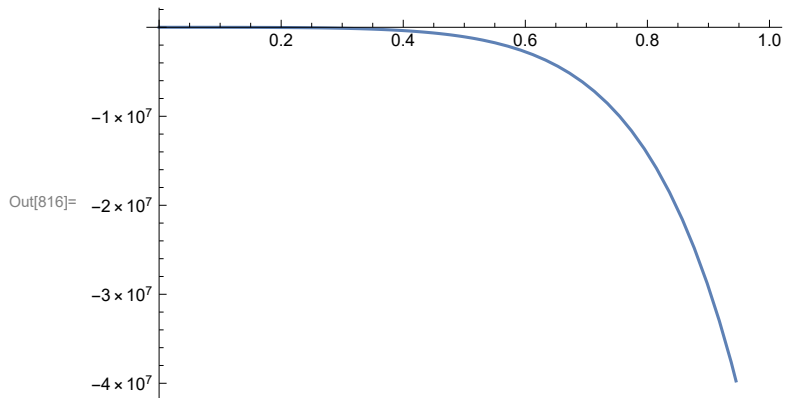

In[817]:= **Plot[Cf[9, 14, 6], {x, 0, 1}]**

[绘图](#)

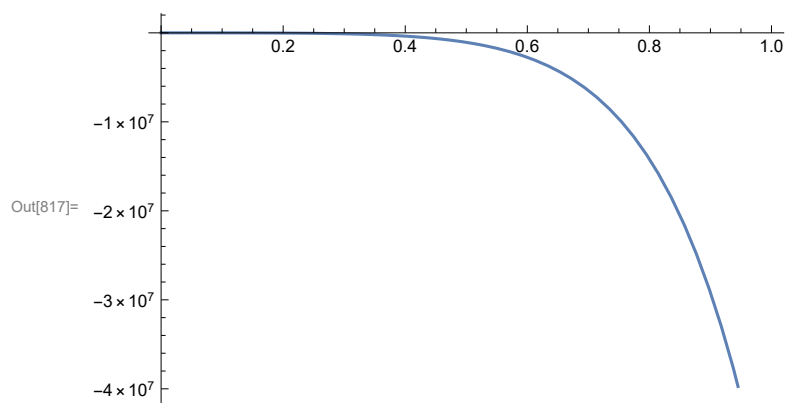

In[818]:= **Plot[Cf[9, 14, 5], {x, 0, 1}]**

[绘图](#)

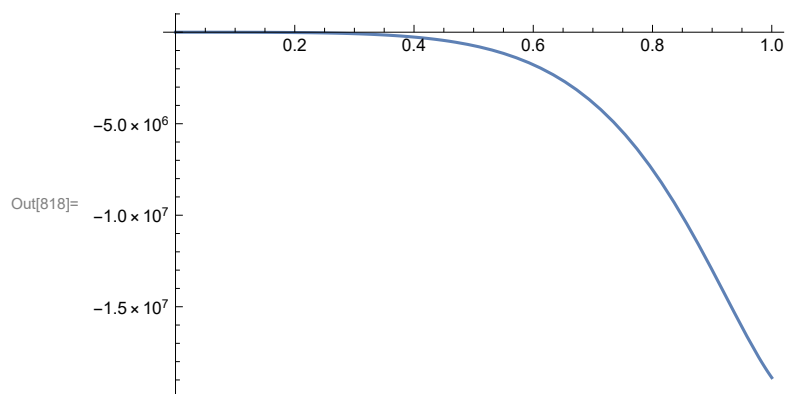

In[819]:= **Plot[Cf[9, 14, 4], {x, 0, 1}]**

[绘图](#)

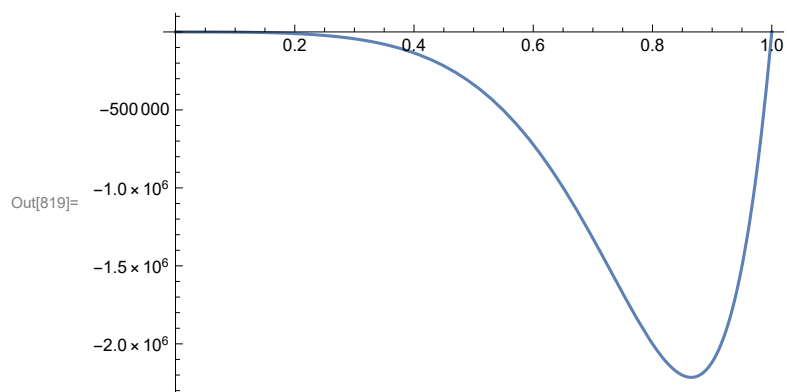

In[820]:= **Plot[Cf[9, 14, 3], {x, 0, 1}]**

[绘图](#)

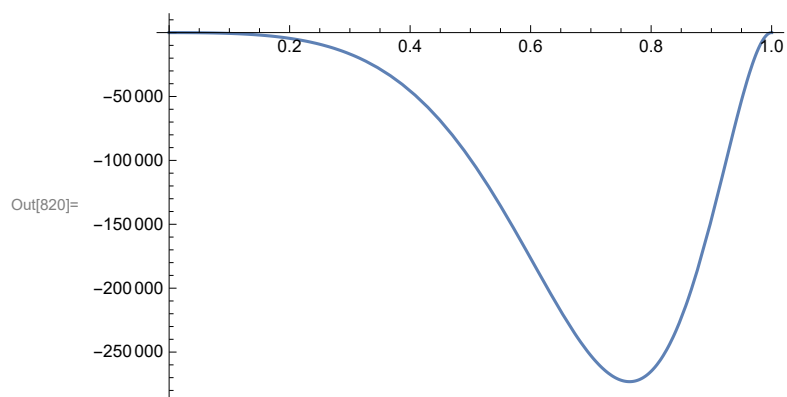

In[821]:= **Plot[Cf[9, 14, 2], {x, 0, 1}]**

[绘图](#)

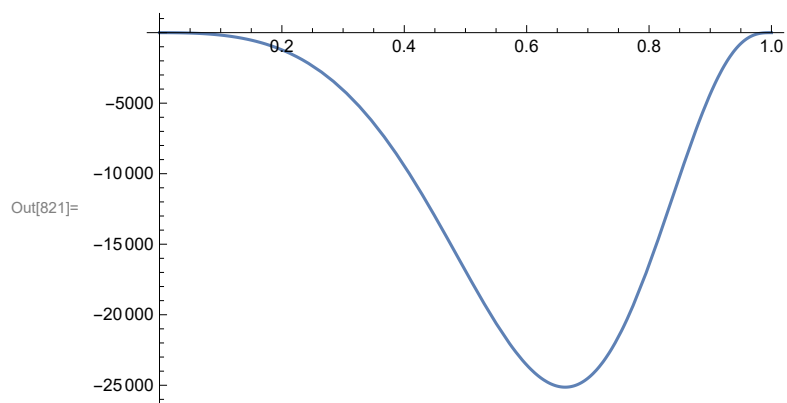

In[822]:= **Plot[Cf[9, 14, 1], {x, 0, 1}]**

[绘图](#)

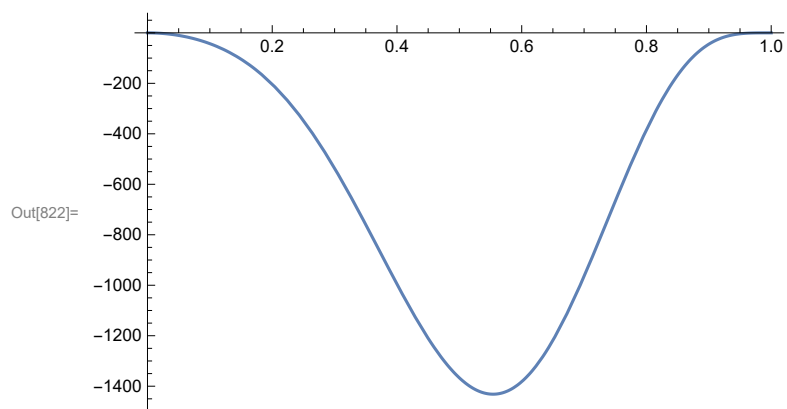

In[823]:= **Plot[Cf[9, 14, 0], {x, 0, 1}]**

[绘图](#)

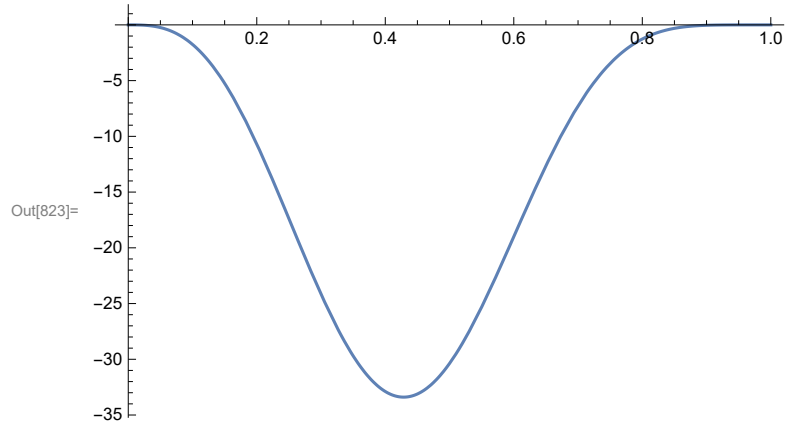

(\*77th group coefficients r2^9r3^13\*)

In[824]:= **Plot[Cf[9, 13, 14], {x, 0, 1}]**

[绘图](#)

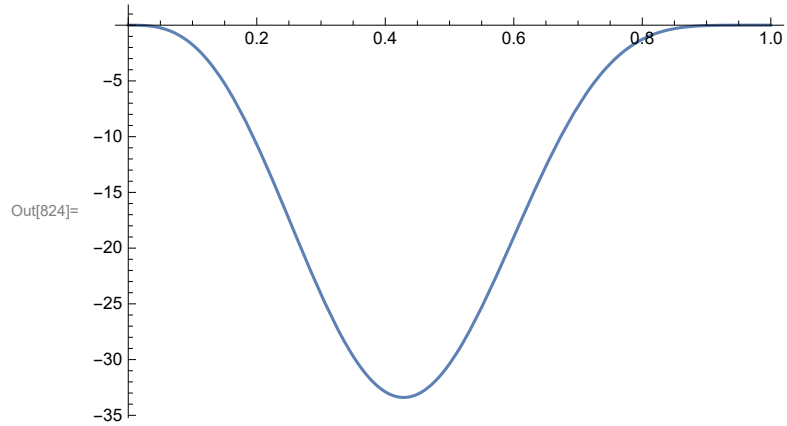

In[825]:= **Plot[Cf[9, 13, 13], {x, 0, 1}]**

[绘图](#)

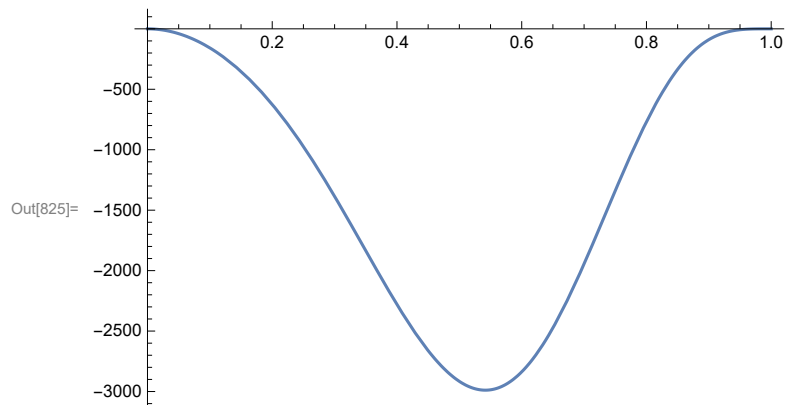

In[826]:= **Plot[Cf[9, 13, 12], {x, 0, 1}]**

[绘图](#)

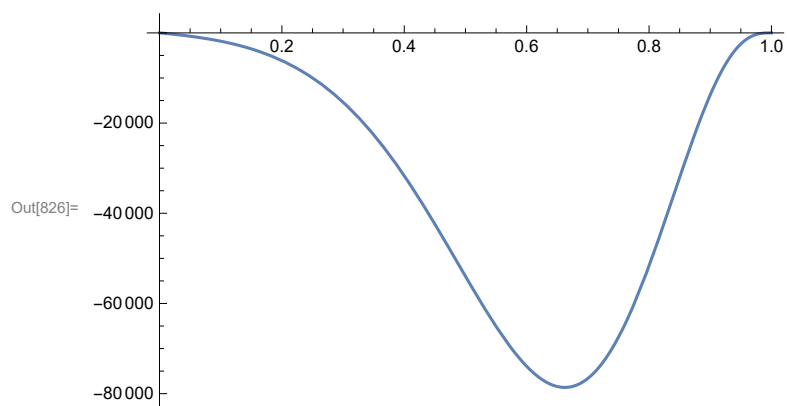

In[827]:= **Plot[Cf[9, 13, 11], {x, 0, 1}]**

[绘图](#)

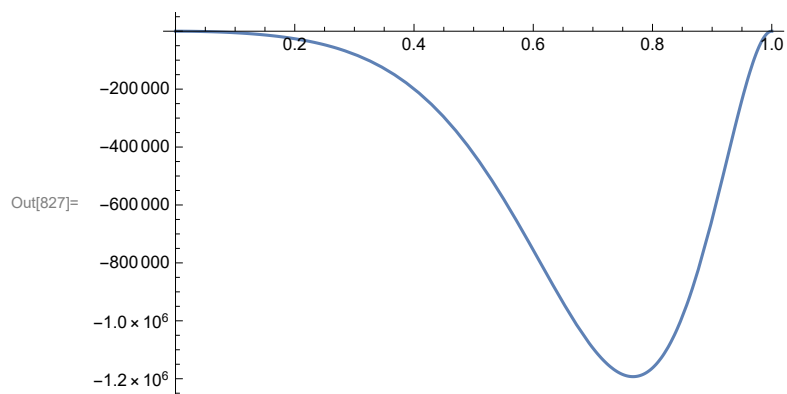

In[828]:= **Plot[Cf[9, 13, 10], {x, 0, 1}]**

[绘图](#)

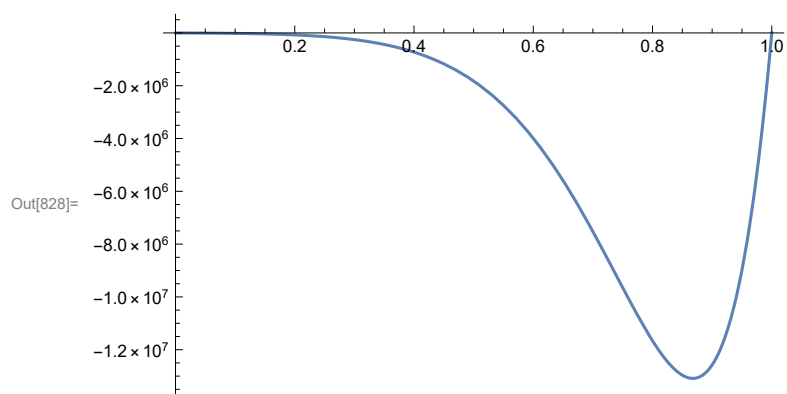

In[829]:= **Plot[Cf[9, 13, 9], {x, 0, 1}]**

[绘图](#)

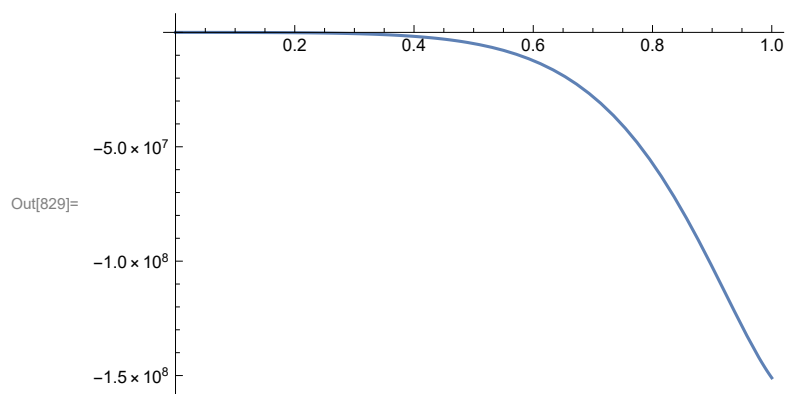

In[830]:= **Plot[Cf[9, 13, 8], {x, 0, 1}]**

[绘图](#)

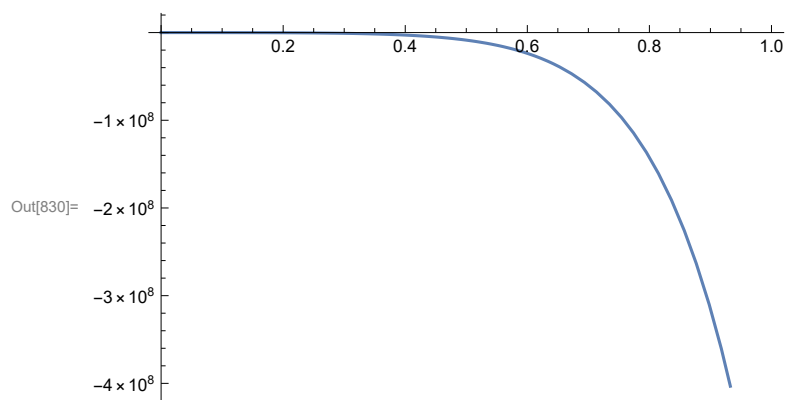

In[831]:= **Plot[Cf[9, 13, 7], {x, 0, 1}]**

[绘图](#)

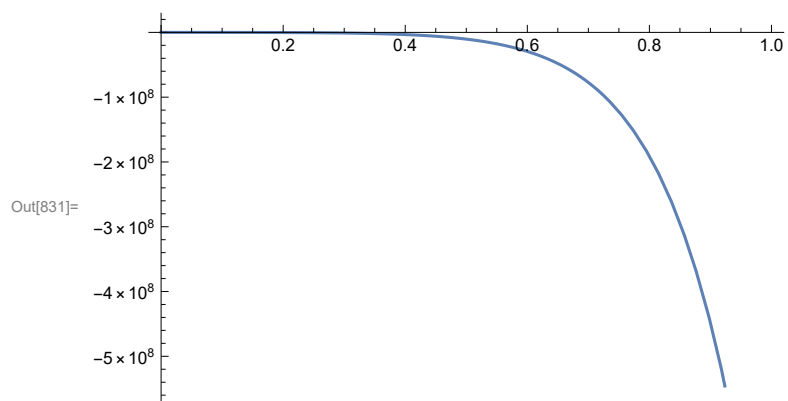

In[832]:= **Plot[Cf[9, 13, 6], {x, 0, 1}]**

[绘图](#)

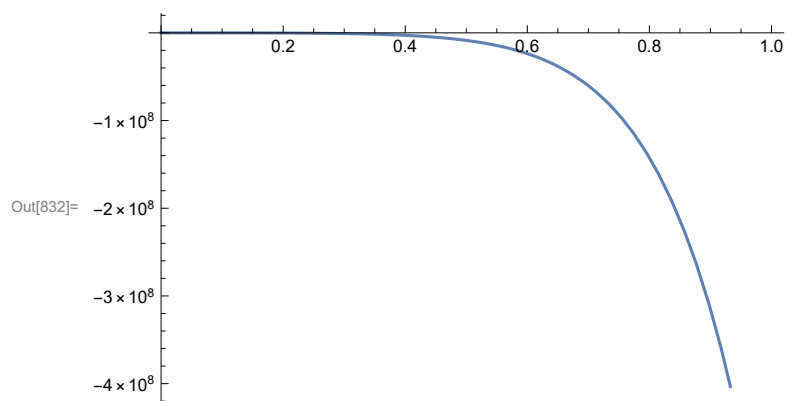

In[833]:= **Plot[Cf[9, 13, 5], {x, 0, 1}]**

[绘图](#)

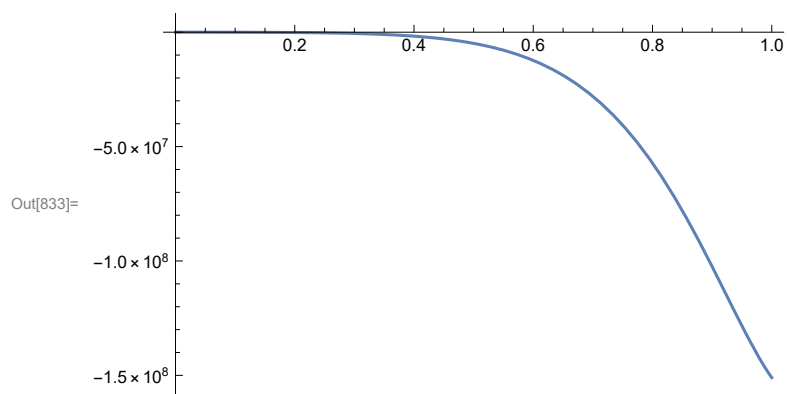

In[834]:= **Plot[Cf[9, 13, 4], {x, 0, 1}]**

[绘图](#)

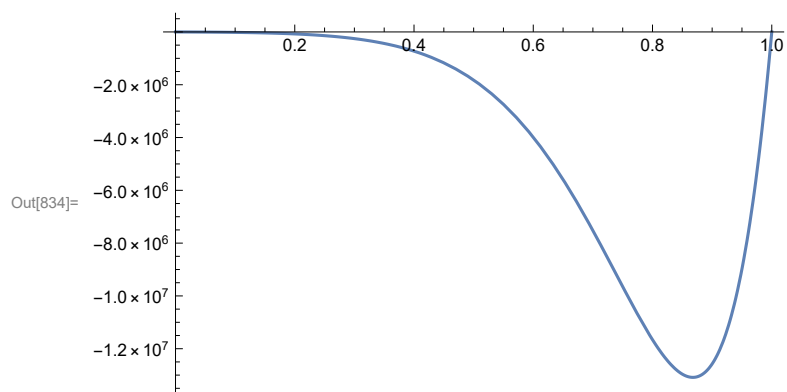

In[835]:= **Plot[Cf[9, 13, 3], {x, 0, 1}]**

[绘图](#)

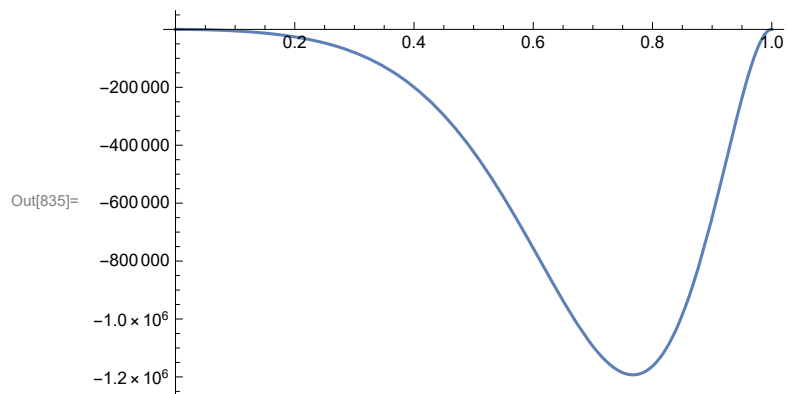

In[836]:= **Plot[Cf[9, 13, 2], {x, 0, 1}]**

[绘图](#)

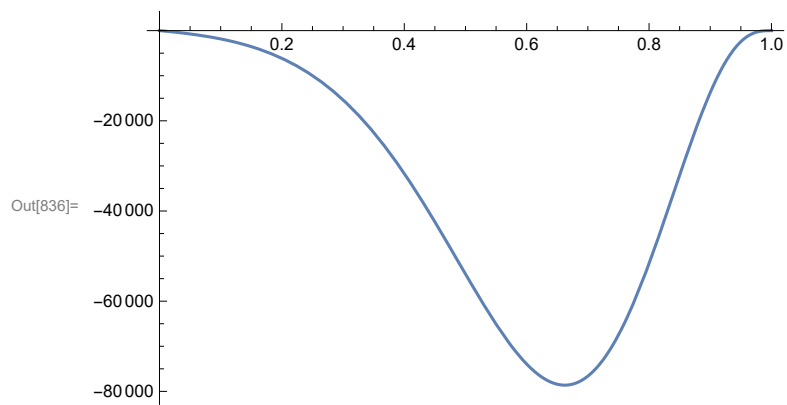

In[837]:= **Plot[Cf[9, 13, 1], {x, 0, 1}]**

[绘图](#)

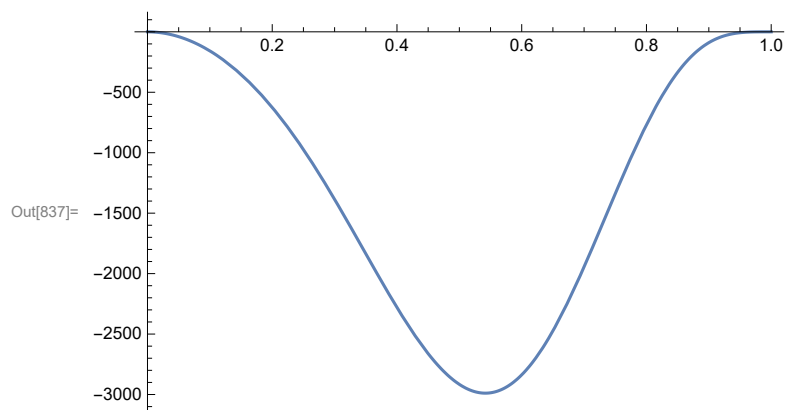



In[838]:= **Plot[Cf[9, 13, 0], {x, 0, 1}]**

[绘图](#)

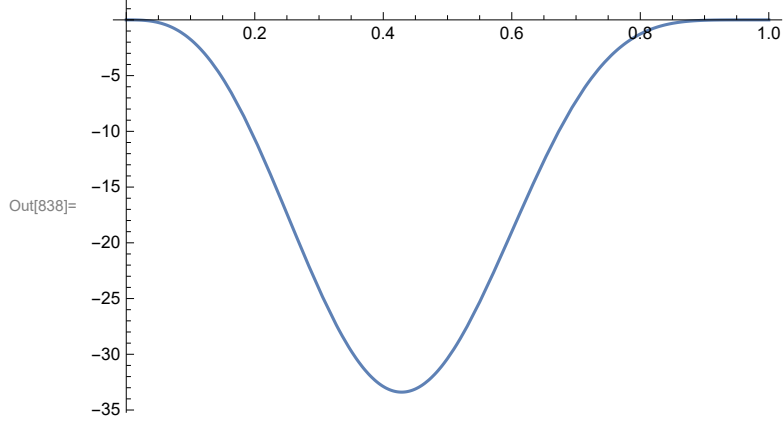

(\*78th group coefficients  $r^2 r^3^{12}$ \*)

In[839]:= **Plot[Cf[9, 12, 14], {x, 0, 1}]**

[绘图](#)

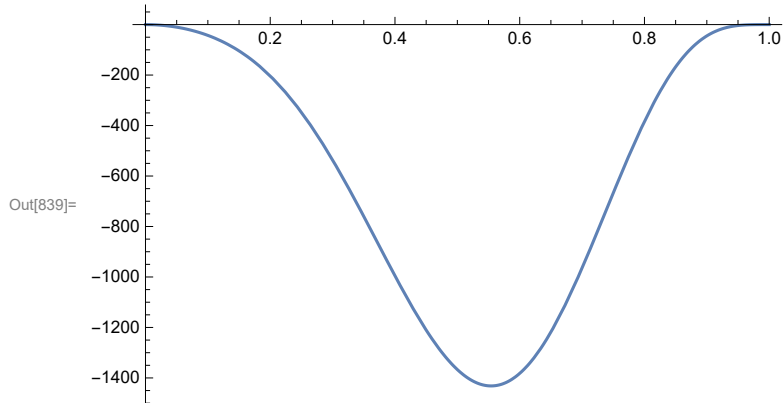

In[840]:= **Plot[Cf[9, 12, 13], {x, 0, 1}]**

[绘图](#)

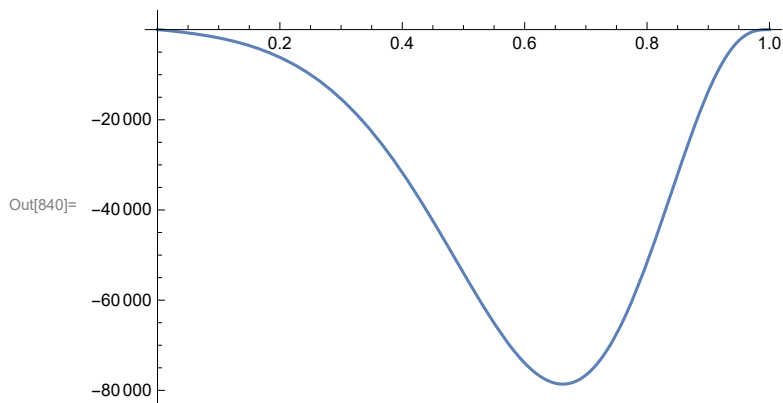

In[841]:= **Plot[Cf[9, 12, 12], {x, 0, 1}]**

[绘图](#)

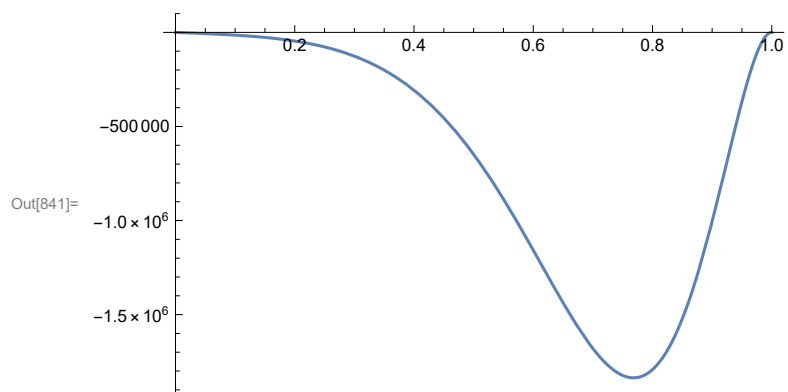

In[842]:= **Plot[Cf[9, 12, 11], {x, 0, 1}]**

[绘图](#)

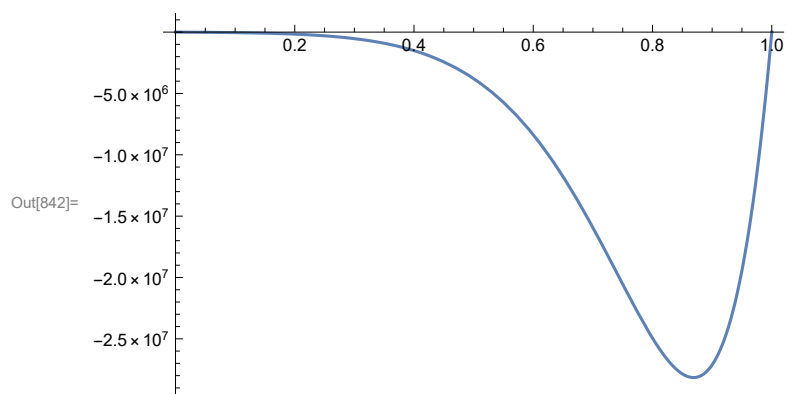

In[843]:= **Plot[Cf[9, 12, 10], {x, 0, 1}]**

[绘图](#)

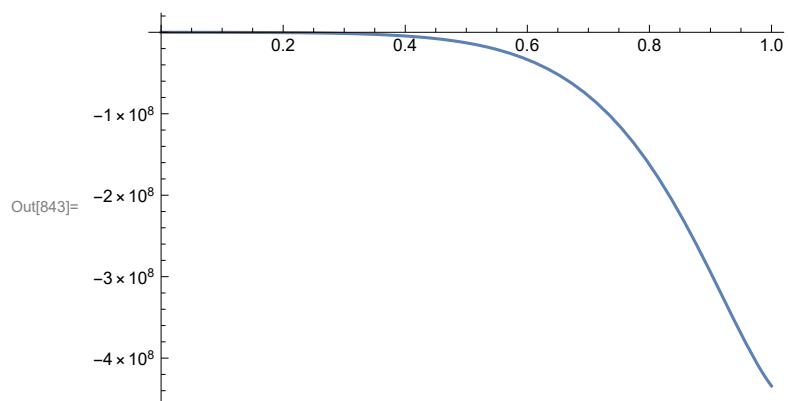

In[845]:= **Plot[Cf[9, 12, 9], {x, 0, 1}]**

[绘图](#)

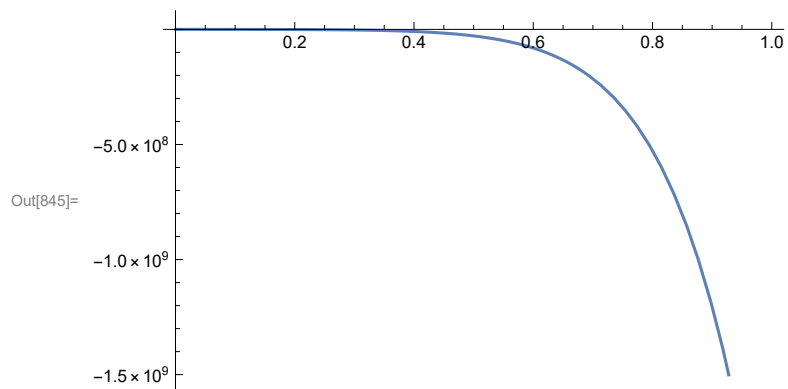

In[844]:= **Plot[Cf[9, 12, 8], {x, 0, 1}]**

[绘图](#)

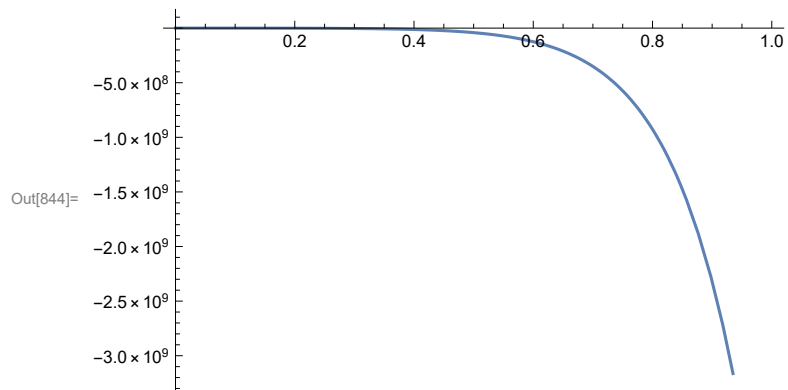

In[846]:= **Plot[Cf[9, 12, 7], {x, 0, 1}]**

[绘图](#)

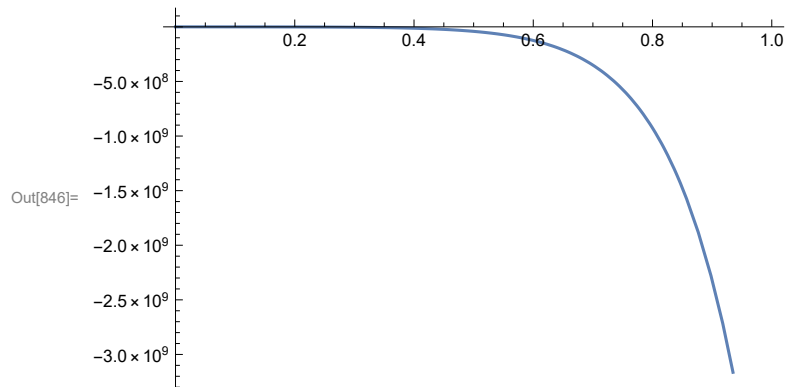

In[847]:= **Plot[Cf[9, 12, 6], {x, 0, 1}]**

[绘图](#)

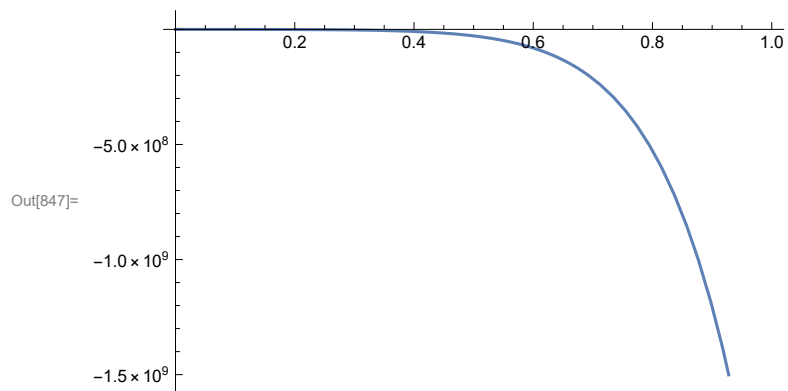

In[848]:= **Plot[Cf[9, 12, 5], {x, 0, 1}]**

[绘图](#)

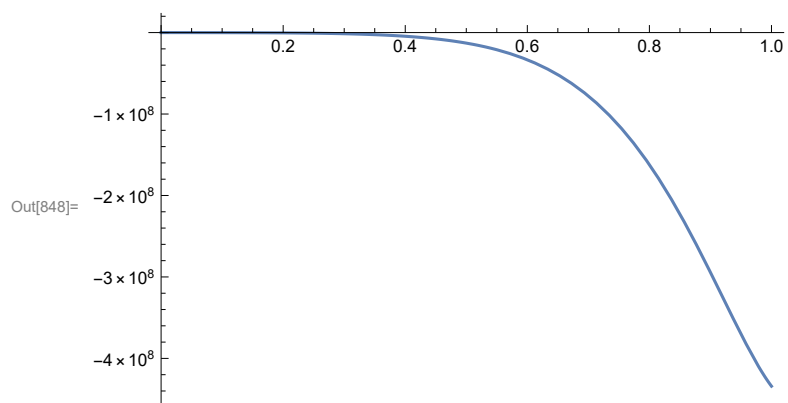

In[849]:= **Plot[Cf[9, 12, 4], {x, 0, 1}]**

[绘图](#)

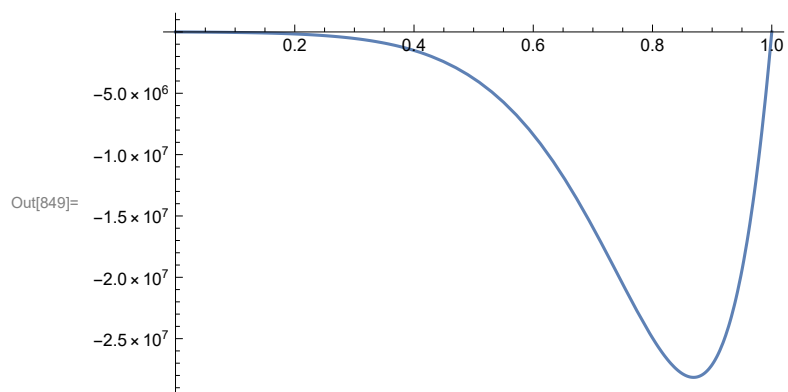

In[850]:= **Plot[Cf[9, 12, 3], {x, 0, 1}]**

[绘图](#)

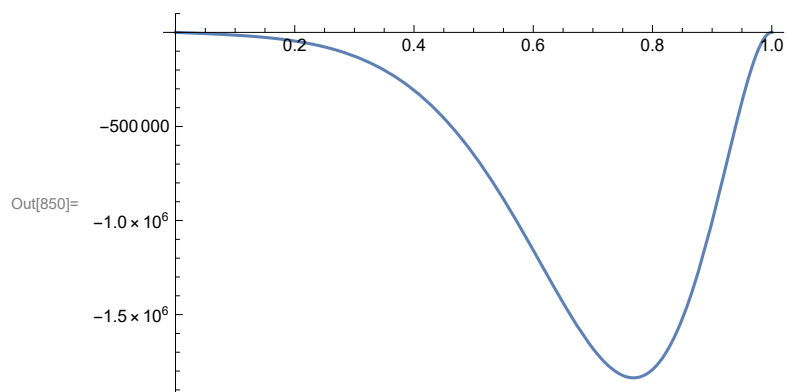

In[851]:= **Plot[Cf[9, 12, 2], {x, 0, 1}]**

[绘图](#)

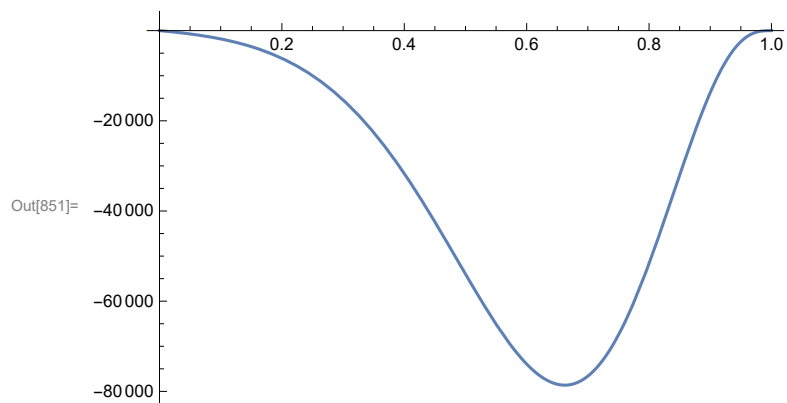

In[852]:= **Plot[Cf[9, 12, 1], {x, 0, 1}]**

[绘图](#)

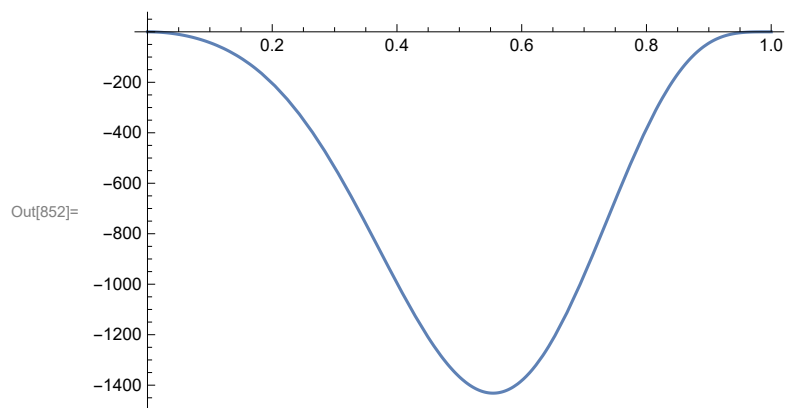

**Plot[Cf[9, 12, 0], {x, 0, 1}]**

[绘图](#)

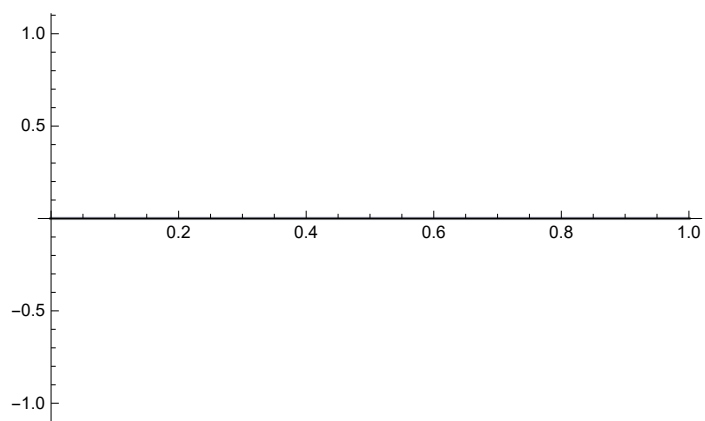

**(\*79th group coefficients r2^9r3^11\*)**

In[853]:= **Plot[Cf[9, 11, 14], {x, 0, 1}]**

[绘图](#)

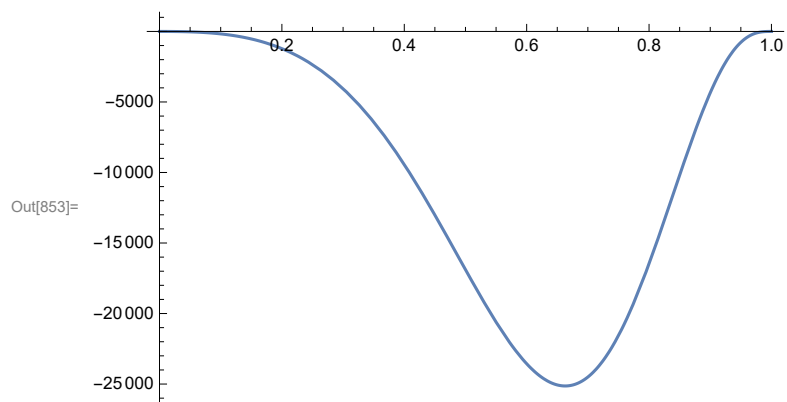

In[854]:= **Plot[Cf[9, 11, 13], {x, 0, 1}]**

[绘图](#)

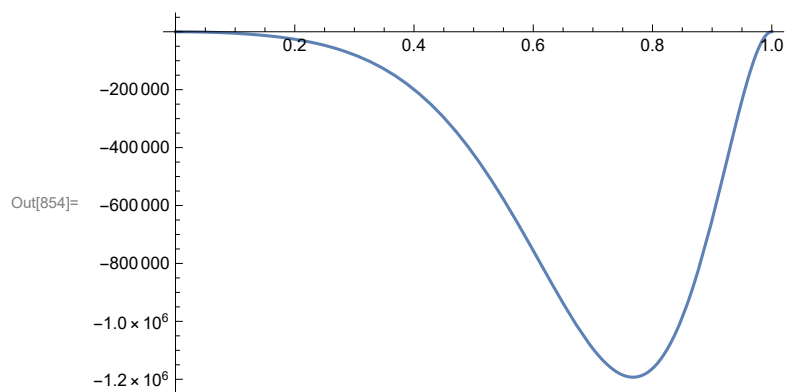

In[855]:= **Plot[Cf[9, 11, 12], {x, 0, 1}]**

[绘图](#)

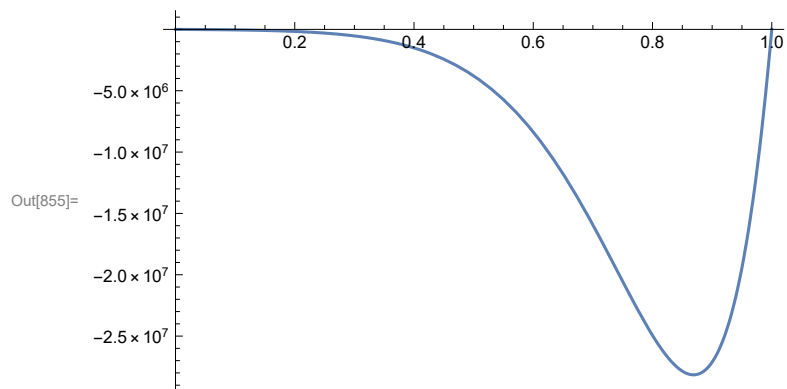

In[856]:= **Plot[Cf[9, 11, 11], {x, 0, 1}]**

[绘图](#)

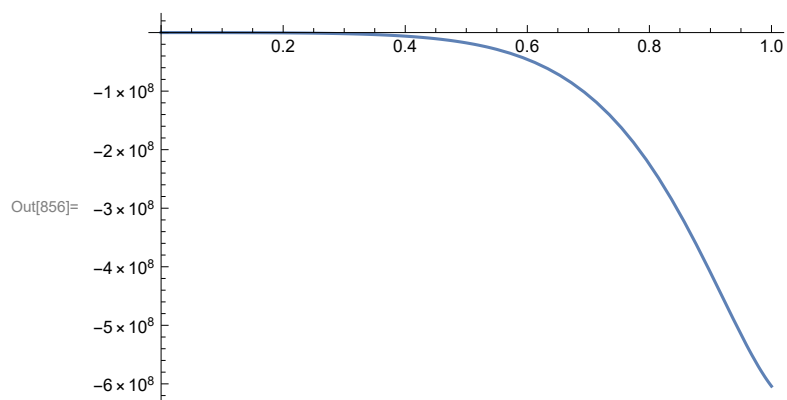

In[857]:= **Plot[Cf[9, 11, 10], {x, 0, 1}]**

[绘图](#)

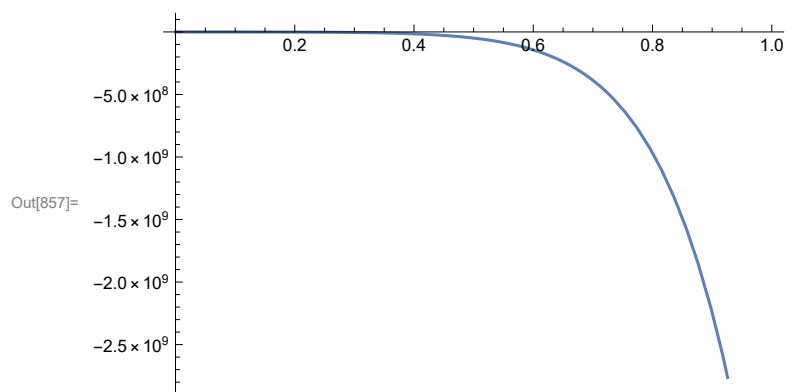

In[858]:= **Plot[Cf[9, 11, 9], {x, 0, 1}]**

[绘图](#)

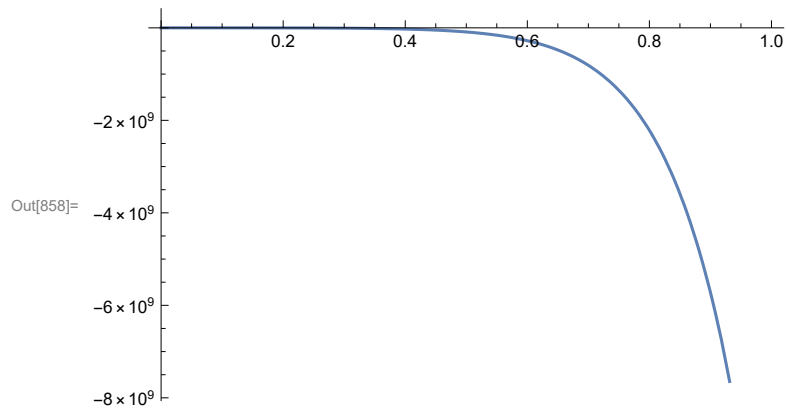

In[859]:= **Plot[Cf[9, 11, 8], {x, 0, 1}]**

[绘图](#)

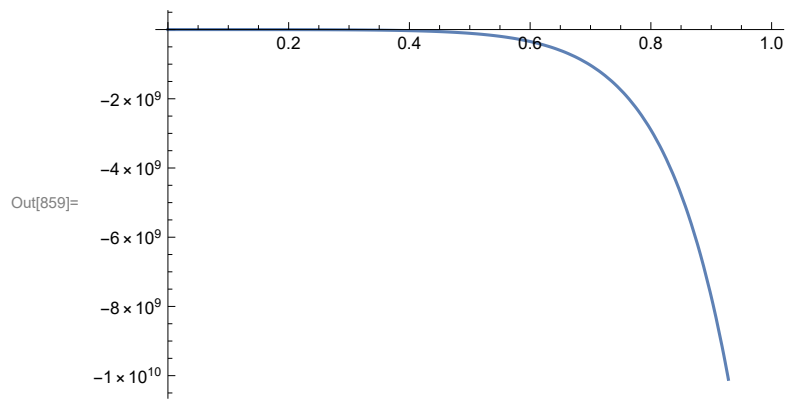

In[860]:= **Plot[Cf[9, 11, 7], {x, 0, 1}]**

[绘图](#)

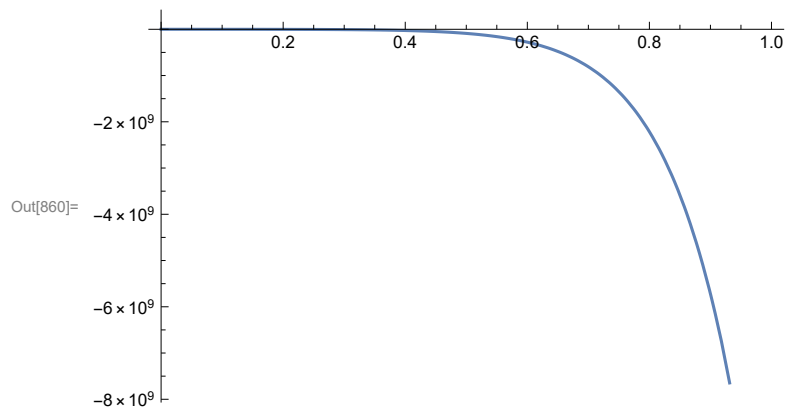



In[861]:= **Plot[Cf[9, 11, 6], {x, 0, 1}]**

[绘图](#)

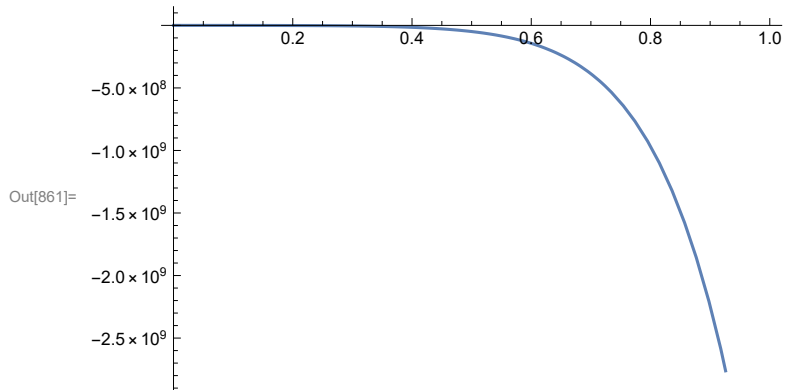

In[862]:= **Plot[Cf[9, 11, 5], {x, 0, 1}]**

[绘图](#)

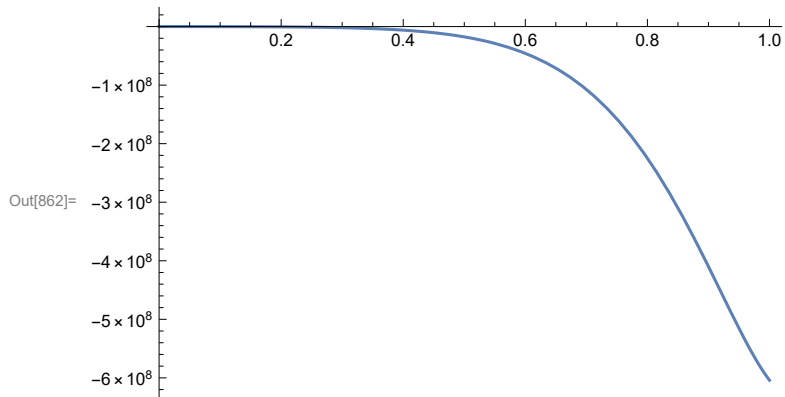

In[863]:= **Plot[Cf[9, 11, 4], {x, 0, 1}]**

[绘图](#)

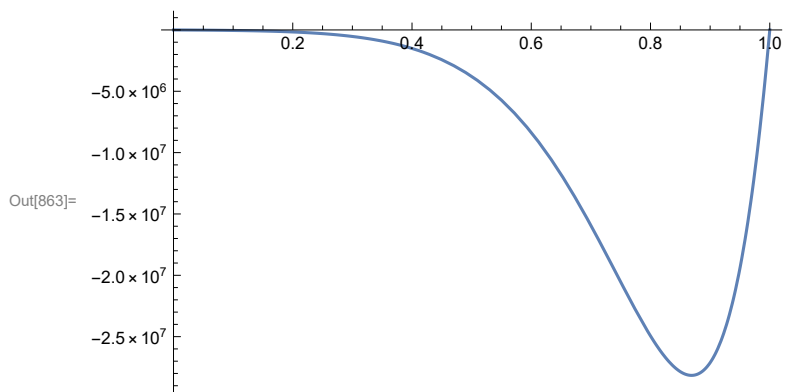

In[864]:= **Plot[Cf[9, 11, 3], {x, 0, 1}]**

[绘图](#)

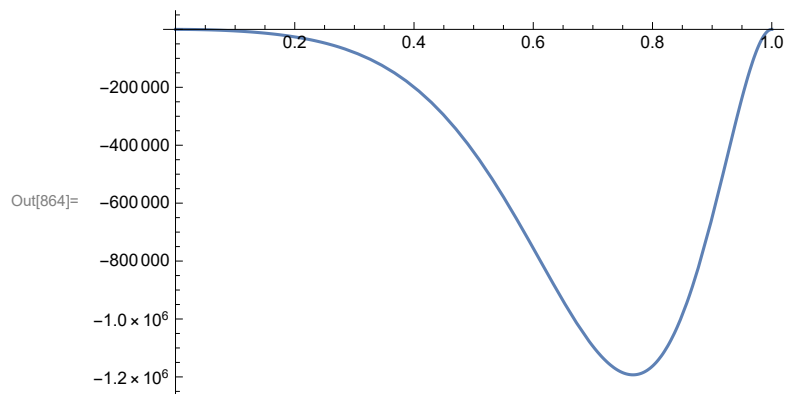

In[865]:= **Plot[Cf[9, 11, 2], {x, 0, 1}]**

[绘图](#)

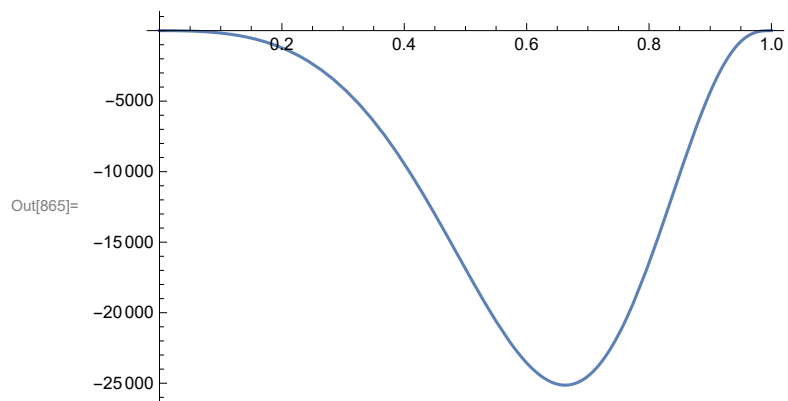

**Plot[Cf[9, 11, 1], {x, 0, 1}]**

[绘图](#)

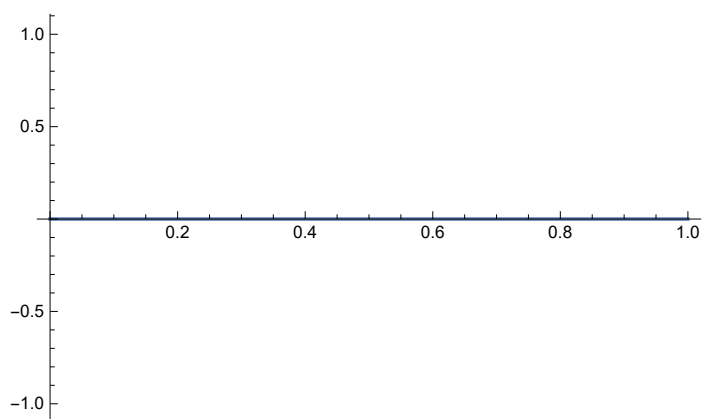

**Plot[Cf[9, 11, 0], {x, 0, 1}]**

[绘图](#)

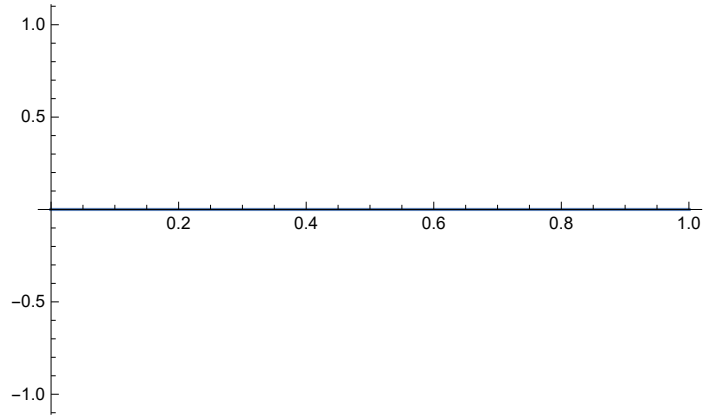

**(\*80th group coefficients r2^9r3^10\*)**

In[866]:= **Plot[Cf[9, 10, 14], {x, 0, 1}]**

[绘图](#)

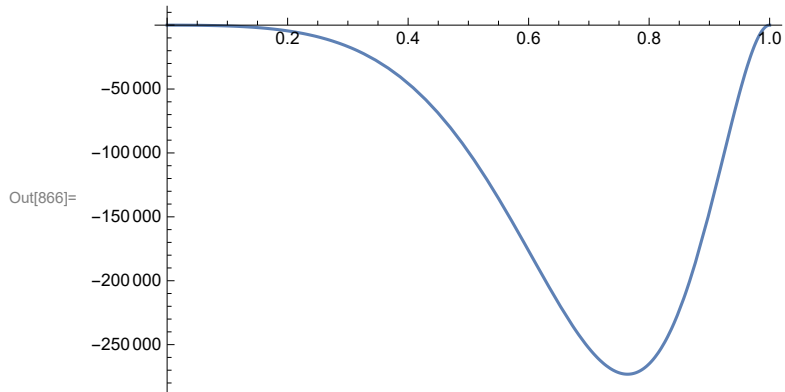

In[867]:= **Plot[Cf[9, 10, 13], {x, 0, 1}]**

[绘图](#)

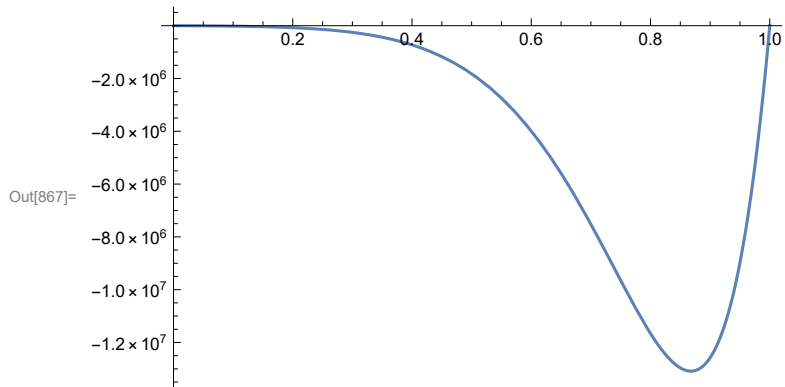

In[868]:= **Plot[Cf[9, 10, 12], {x, 0, 1}]**

[绘图](#)

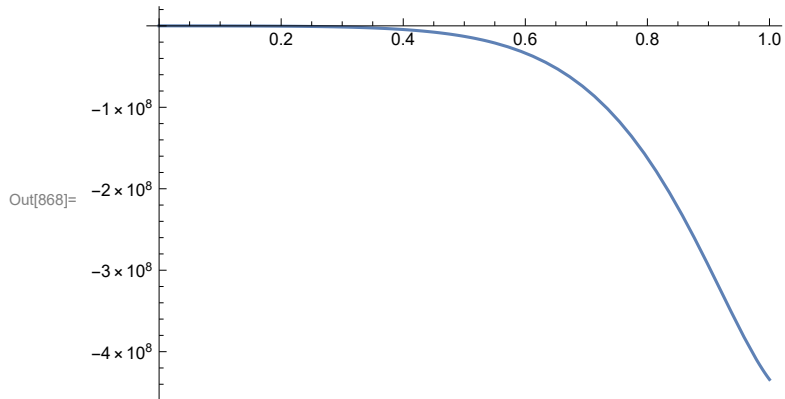

In[869]:= **Plot[Cf[9, 10, 11], {x, 0, 1}]**

[绘图](#)

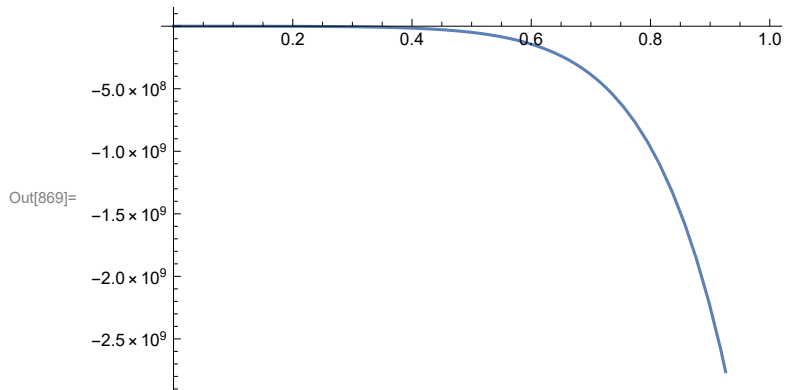

In[870]:= **Plot[Cf[9, 10, 10], {x, 0, 1}]**

[绘图](#)

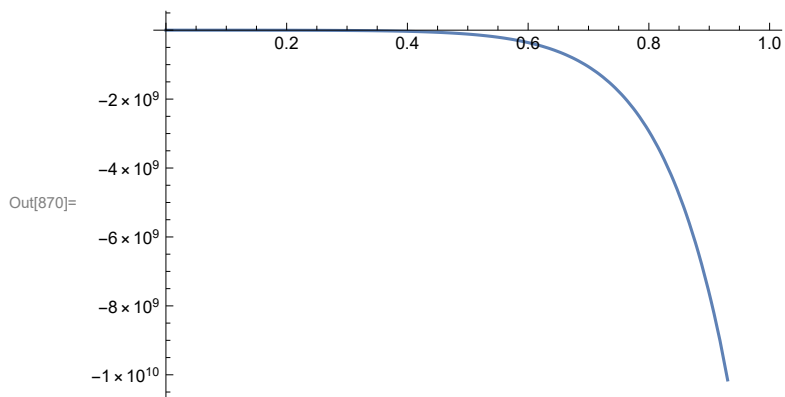

In[871]:= **Plot[Cf[9, 10, 9], {x, 0, 1}]**

[绘图](#)

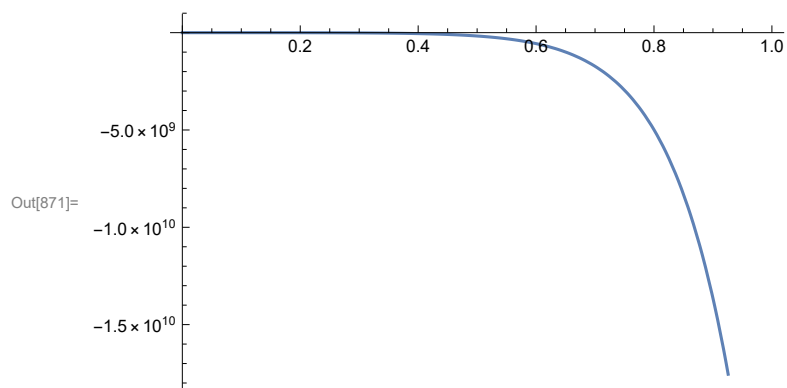

In[872]:= **Plot[Cf[9, 10, 8], {x, 0, 1}]**

[绘图](#)

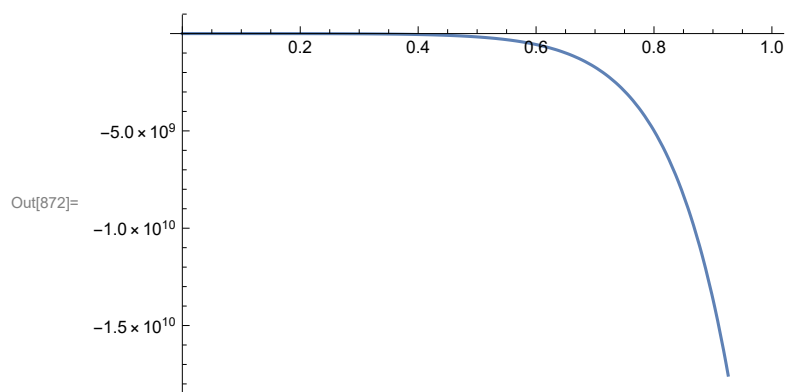

In[873]:= **Plot[Cf[9, 10, 7], {x, 0, 1}]**

[绘图](#)

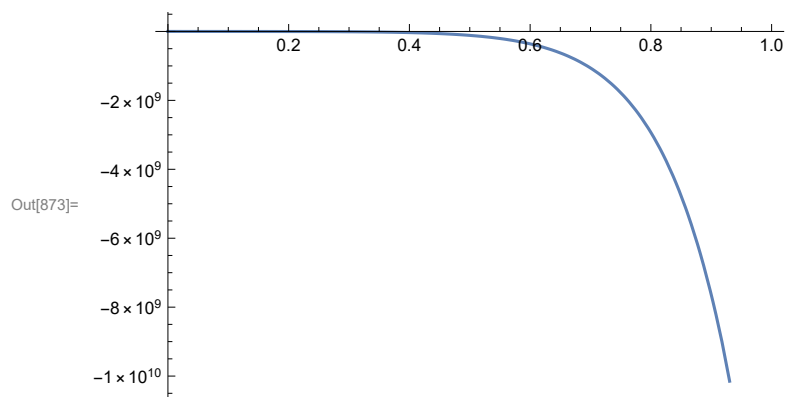

In[874]:= **Plot[Cf[9, 10, 6], {x, 0, 1}]**

[绘图](#)

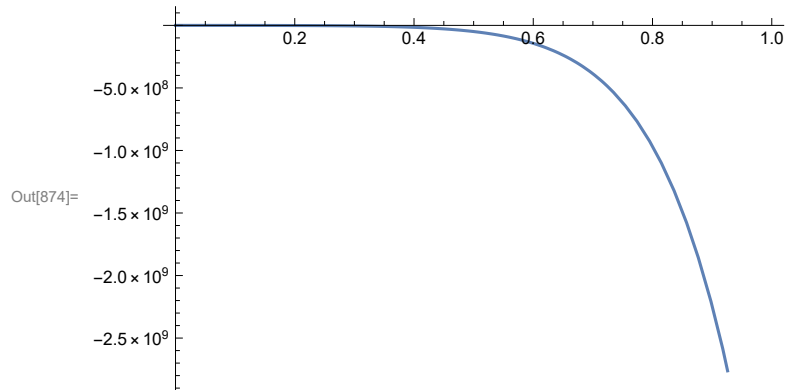

In[875]:= **Plot[Cf[9, 10, 5], {x, 0, 1}]**

[绘图](#)

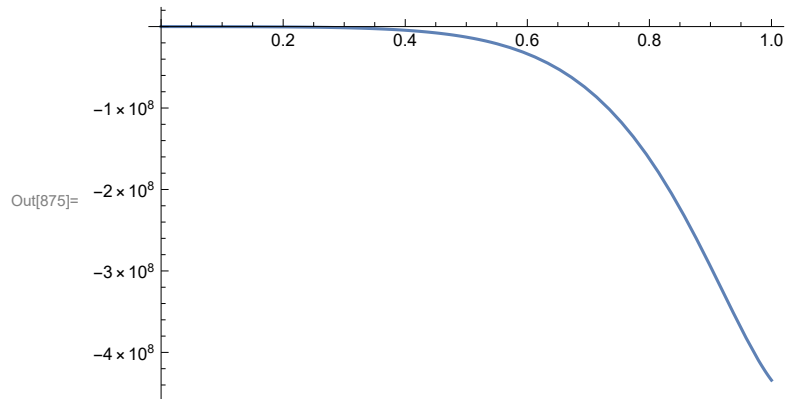

In[876]:= **Plot[Cf[9, 10, 4], {x, 0, 1}]**

[绘图](#)

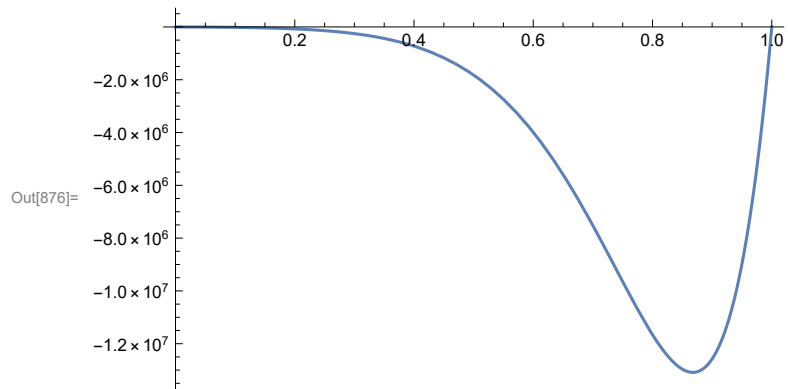

In[877]:= **Plot[Cf[9, 10, 3], {x, 0, 1}]**

[绘图](#)

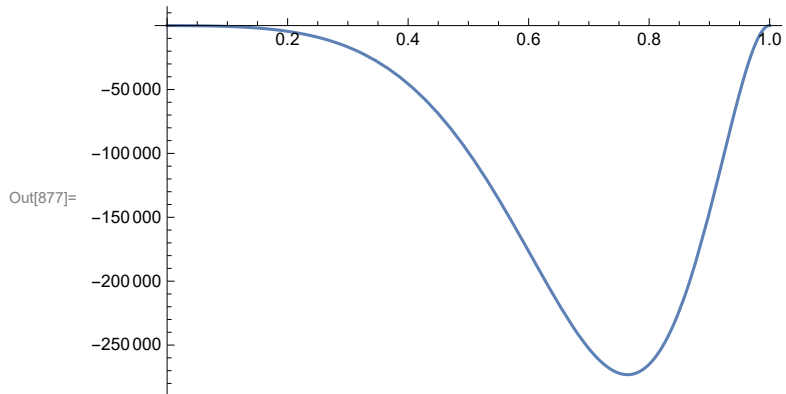

**Plot[Cf[9, 10, 2], {x, 0, 1}]**

[绘图](#)

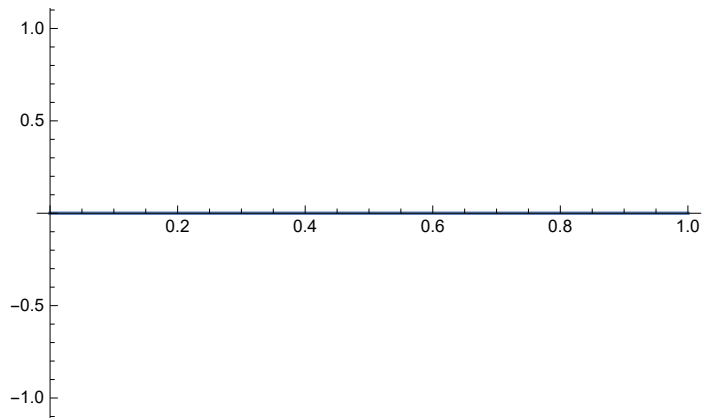

**Plot[Cf[9, 10, 1], {x, 0, 1}]**

[绘图](#)

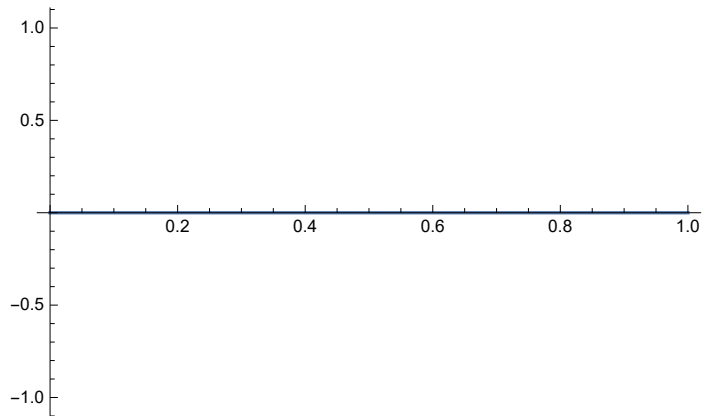

**Plot[Cf[9, 10, 0], {x, 0, 1}]**

[绘图](#)

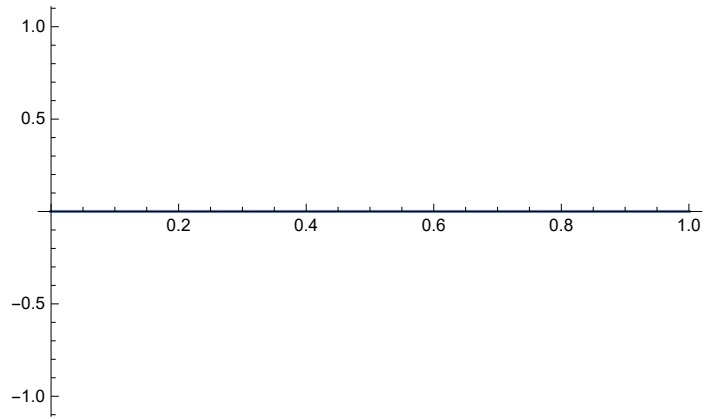

**(\*81th group coefficients r2^9r3^9\*)**

In[878]:= **Plot[Cf[9, 9, 14], {x, 0, 1}]**

[绘图](#)

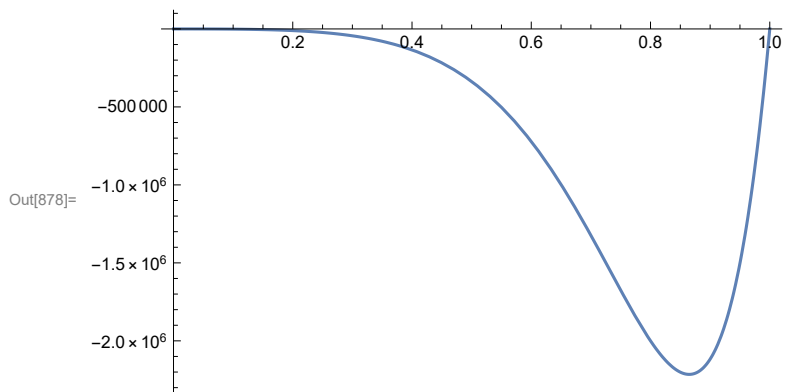

In[879]:= **Plot[Cf[9, 9, 13], {x, 0, 1}]**

[绘图](#)

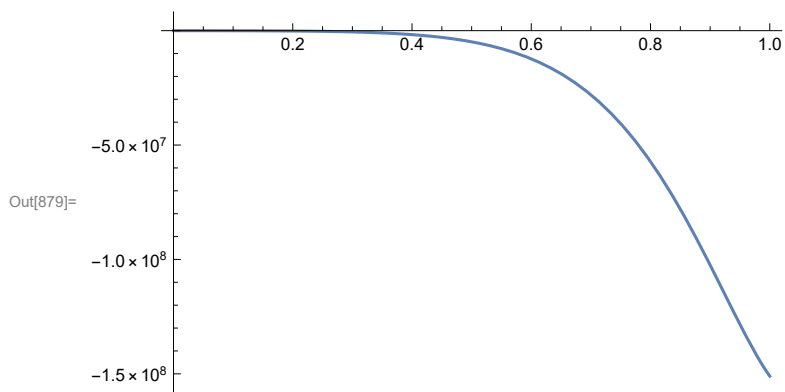



In[880]:= **Plot[Cf[9, 9, 12], {x, 0, 1}]**

[绘图](#)

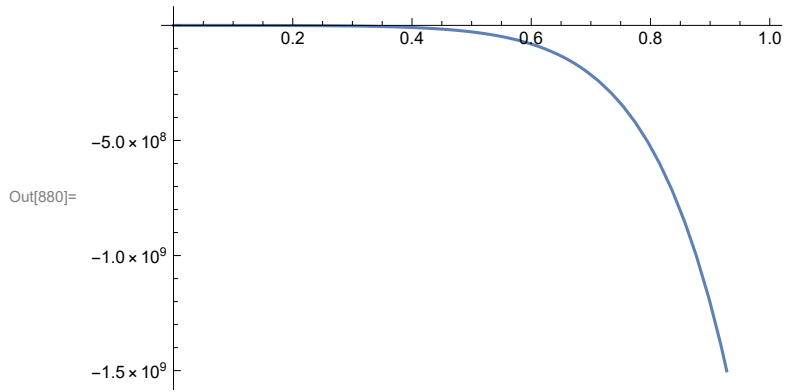

In[881]:= **Plot[Cf[9, 9, 11], {x, 0, 1}]**

[绘图](#)

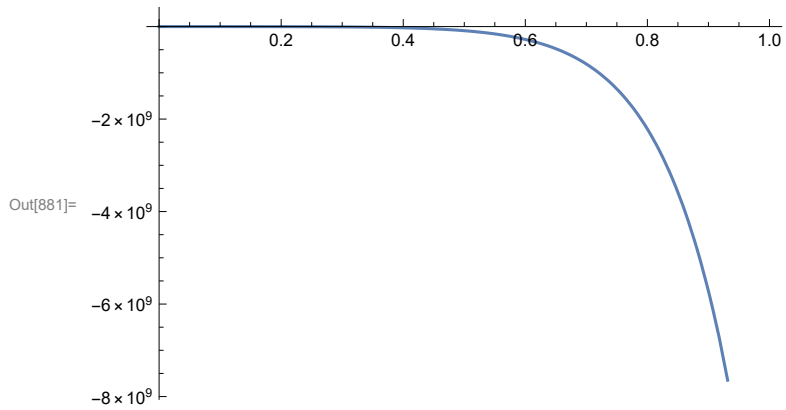

In[882]:= **Plot[Cf[9, 9, 10], {x, 0, 1}]**

[绘图](#)

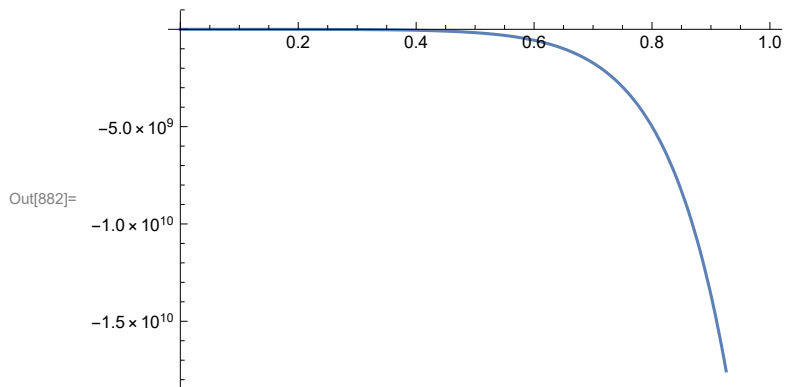

In[883]:= **Plot[Cf[9, 9, 9], {x, 0, 1}]**

[绘图](#)

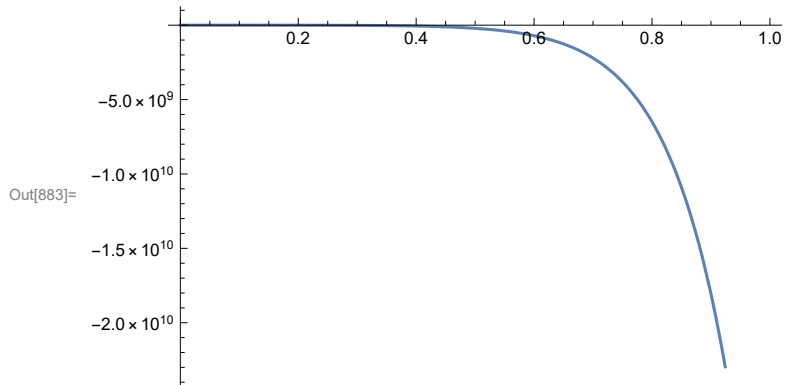

In[884]:= **Plot[Cf[9, 9, 8], {x, 0, 1}]**

[绘图](#)

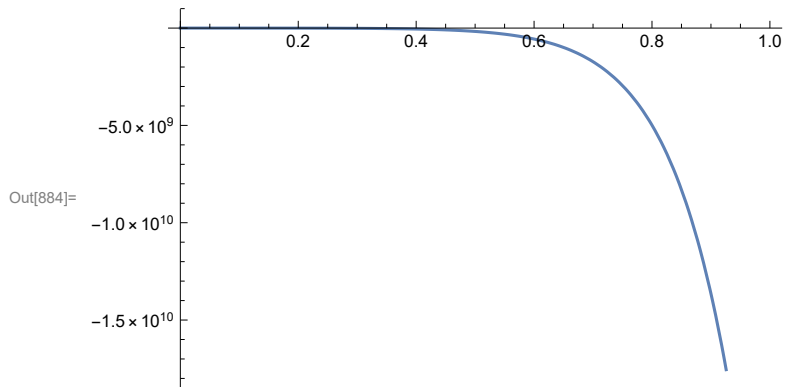

In[885]:= **Plot[Cf[9, 9, 7], {x, 0, 1}]**

[绘图](#)

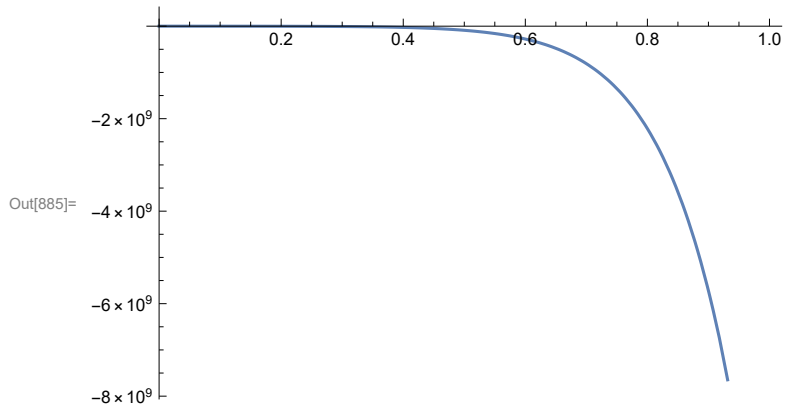

In[886]:= **Plot[Cf[9, 9, 6], {x, 0, 1}]**

[绘图](#)

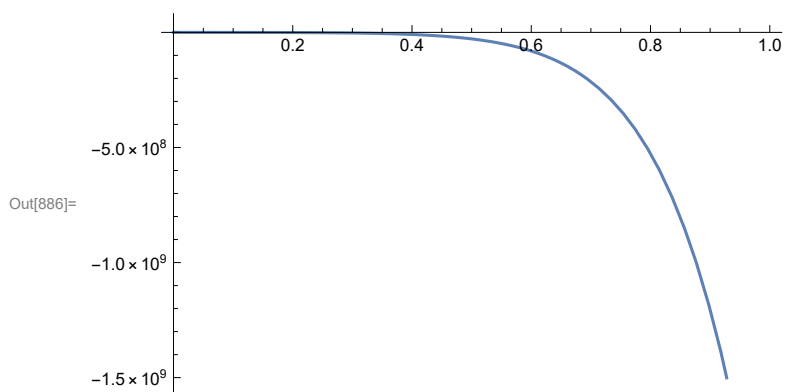

In[887]:= **Plot[Cf[9, 9, 5], {x, 0, 1}]**

[绘图](#)

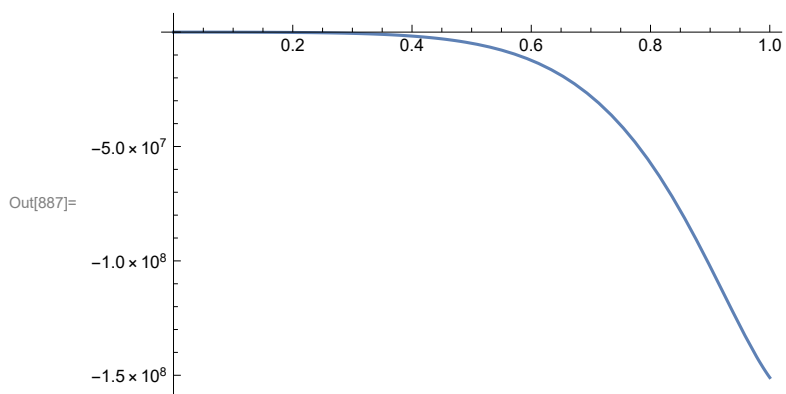

In[888]:= **Plot[Cf[9, 9, 4], {x, 0, 1}]**

[绘图](#)

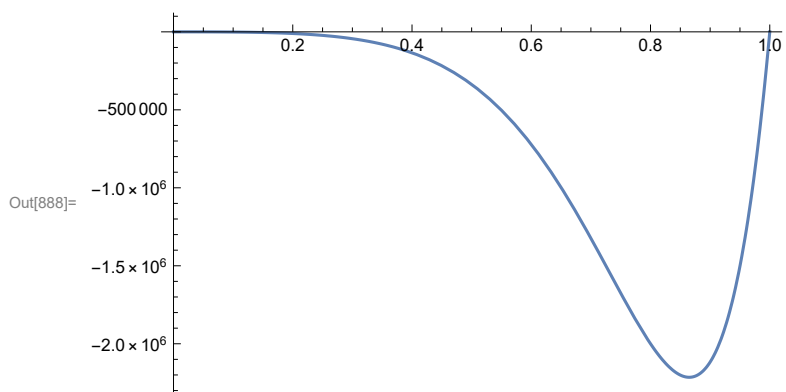

**Plot[Cf[9, 9, 3], {x, 0, 1}]**

[绘图](#)

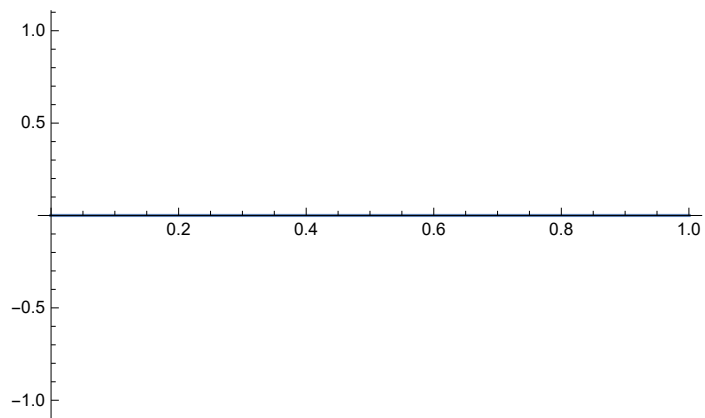

**Plot[Cf[9, 9, 2], {x, 0, 1}]**

[绘图](#)

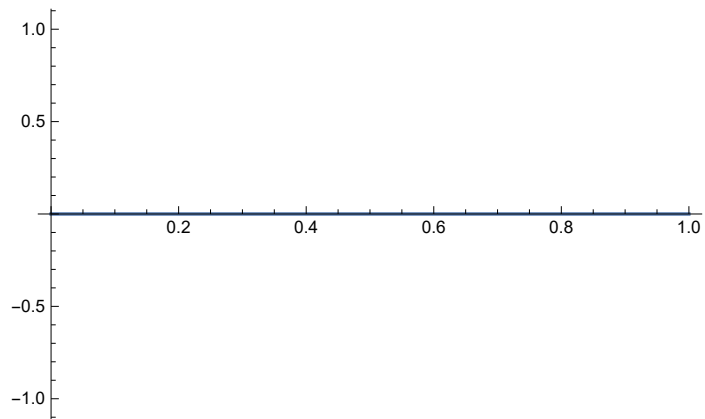

**Plot[Cf[9, 9, 1], {x, 0, 1}]**

[绘图](#)

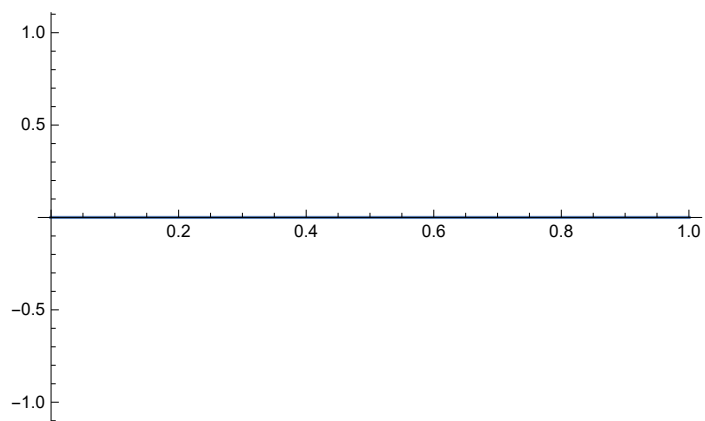

**Plot[Cf[9, 9, 0], {x, 0, 1}]**

[绘图](#)

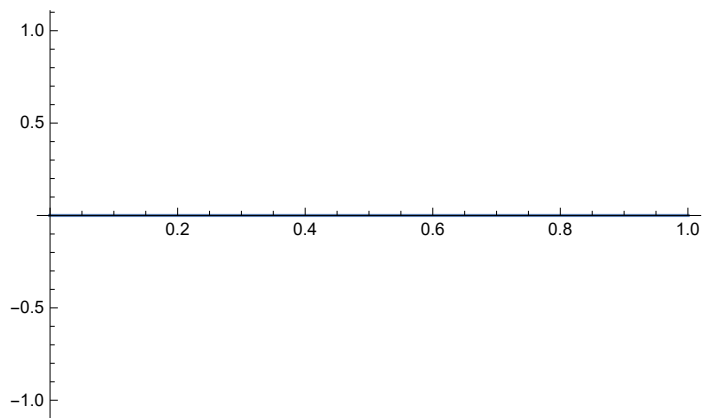

(\*82th group coefficients r2^9r3^8\*)

In[889]:= **Plot[Cf[9, 8, 14], {x, 0, 1}]**

[绘图](#)

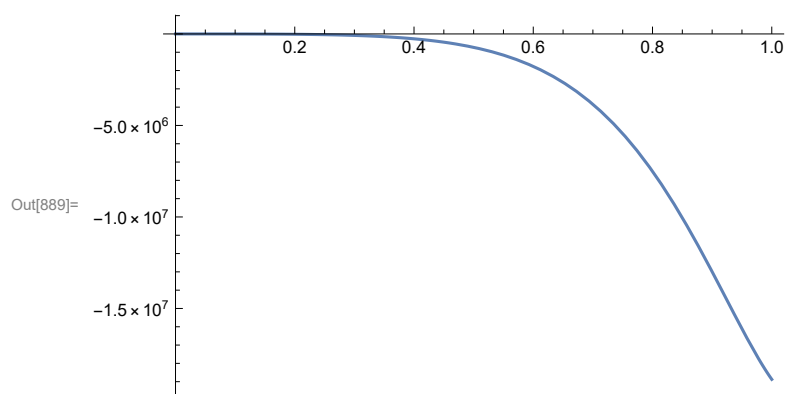

In[890]:= **Plot[Cf[9, 8, 13], {x, 0, 1}]**

[绘图](#)

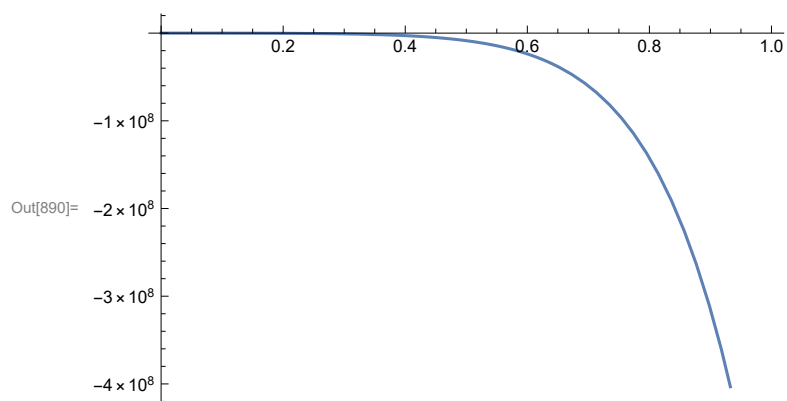

In[891]:= **Plot[Cf[9, 8, 12], {x, 0, 1}]**

[绘图](#)

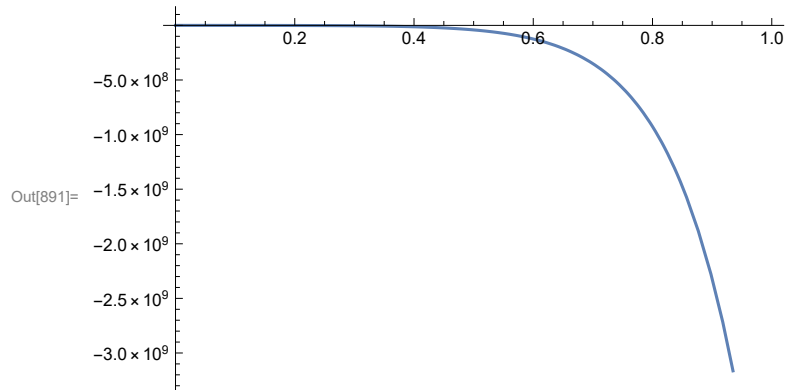

In[892]:= **Plot[Cf[9, 8, 11], {x, 0, 1}]**

[绘图](#)

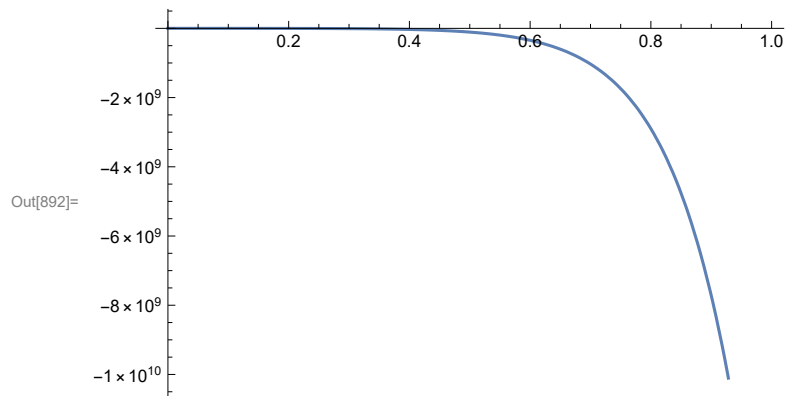

In[893]:= **Plot[Cf[9, 8, 10], {x, 0, 1}]**

[绘图](#)

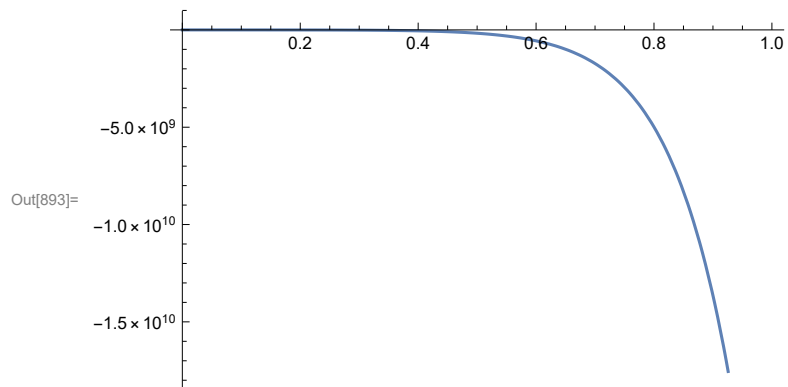

In[894]:= **Plot[Cf[9, 8, 9], {x, 0, 1}]**

[绘图](#)

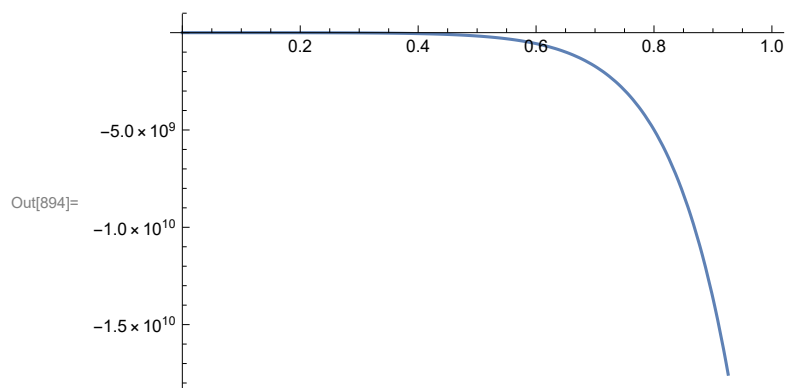

In[895]:= **Plot[Cf[9, 8, 8], {x, 0, 1}]**

[绘图](#)

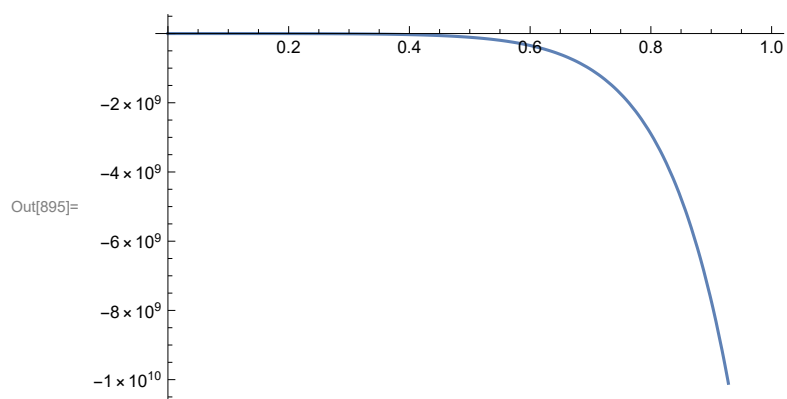

In[896]:= **Plot[Cf[9, 8, 7], {x, 0, 1}]**

[绘图](#)

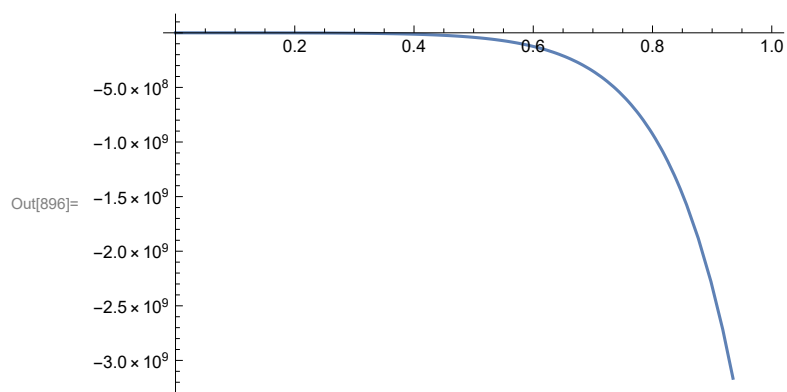

In[897]:= **Plot[Cf[9, 8, 6], {x, 0, 1}]**

[绘图](#)

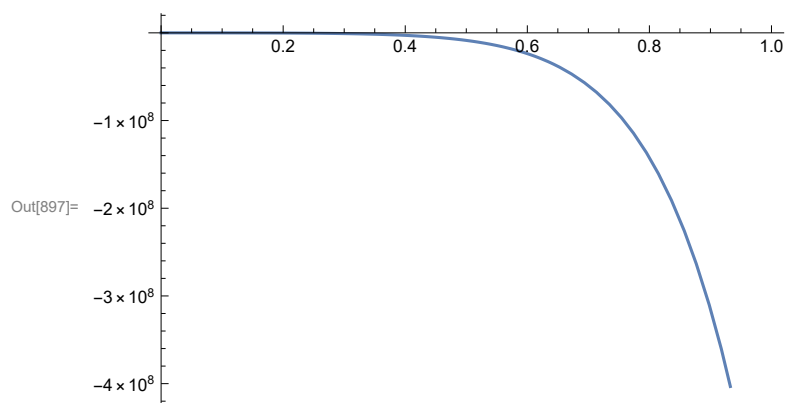

In[898]:= **Plot[Cf[9, 8, 5], {x, 0, 1}]**

[绘图](#)

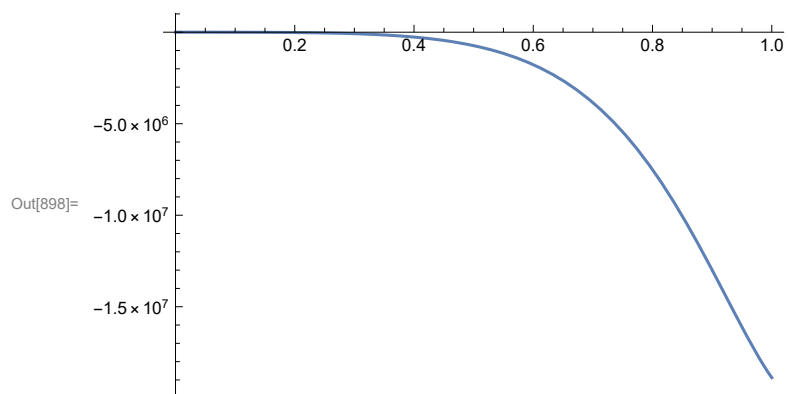

**Plot[Cf[9, 8, 4], {x, 0, 1}]**

[绘图](#)

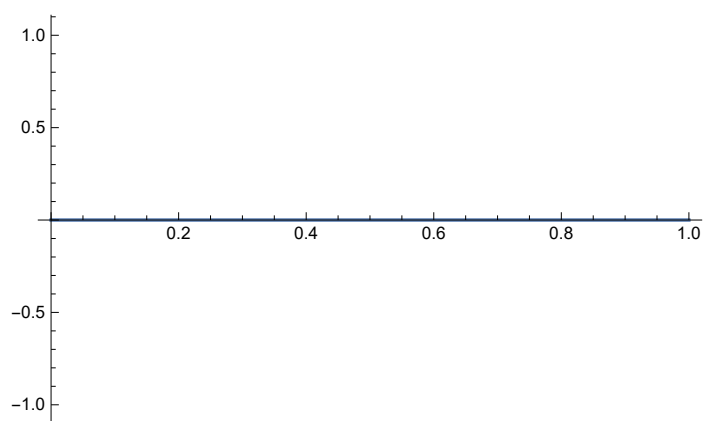



**Plot[Cf[9, 8, 3], {x, 0, 1}]**

[绘图](#)

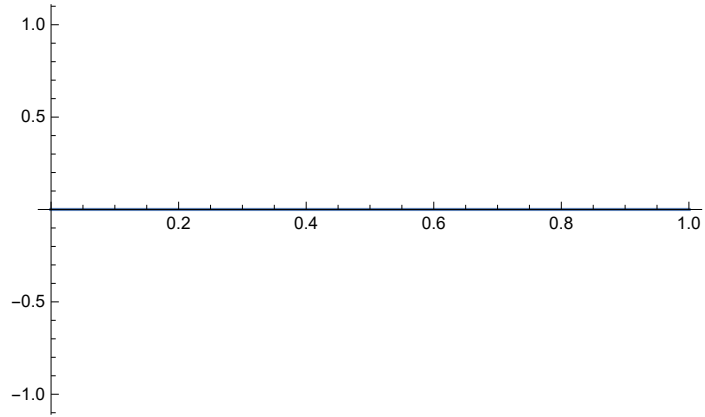

**Plot[Cf[9, 8, 2], {x, 0, 1}]**

[绘图](#)

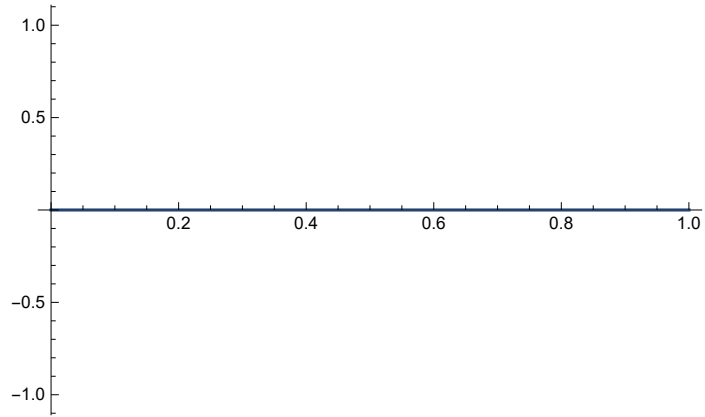

**Plot[Cf[9, 8, 1], {x, 0, 1}]**

[绘图](#)

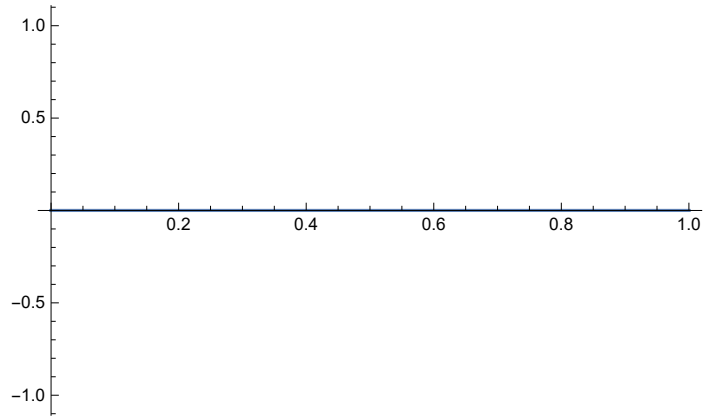

**Plot[Cf[9, 8, 0], {x, 0, 1}]**

[绘图](#)

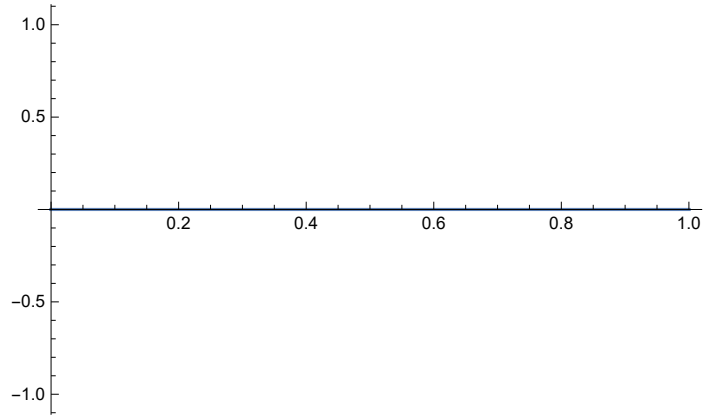

**(\*83th group coefficients r2^9r3^7\*)**

In[899]:= **Plot[Cf[9, 7, 14], {x, 0, 1}]**

[绘图](#)

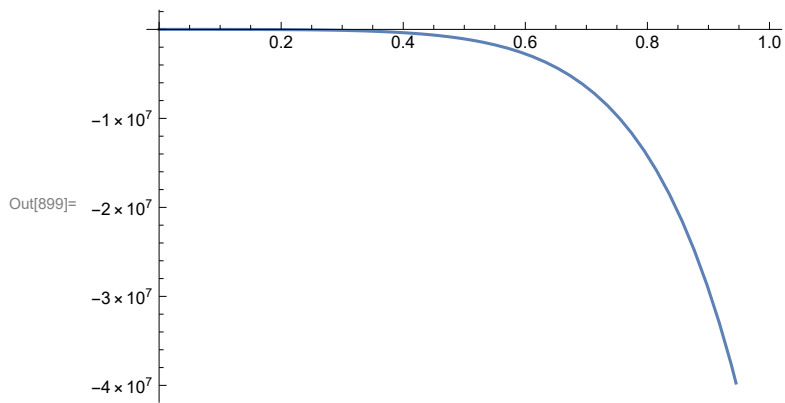

In[900]:= **Plot[Cf[9, 7, 13], {x, 0, 1}]**

[绘图](#)

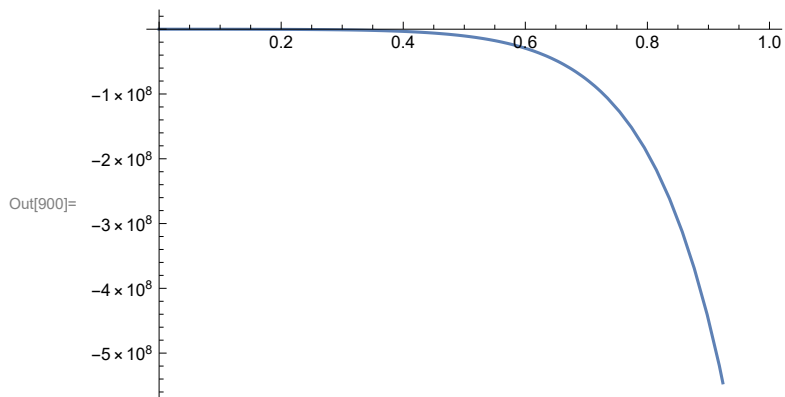

In[901]:= **Plot[Cf[9, 7, 12], {x, 0, 1}]**

[绘图](#)

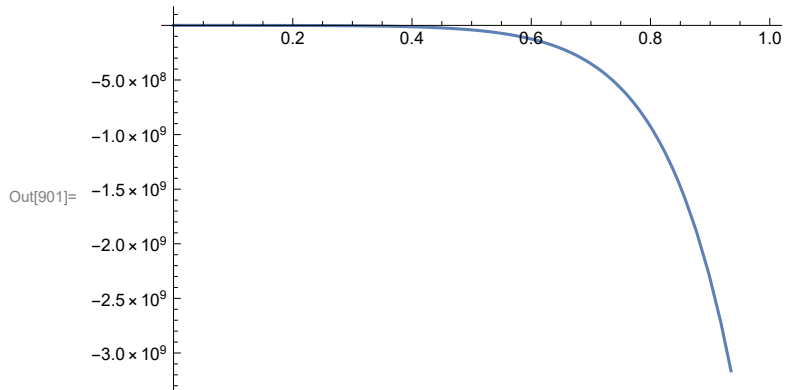

In[902]:= **Plot[Cf[9, 7, 11], {x, 0, 1}]**

[绘图](#)

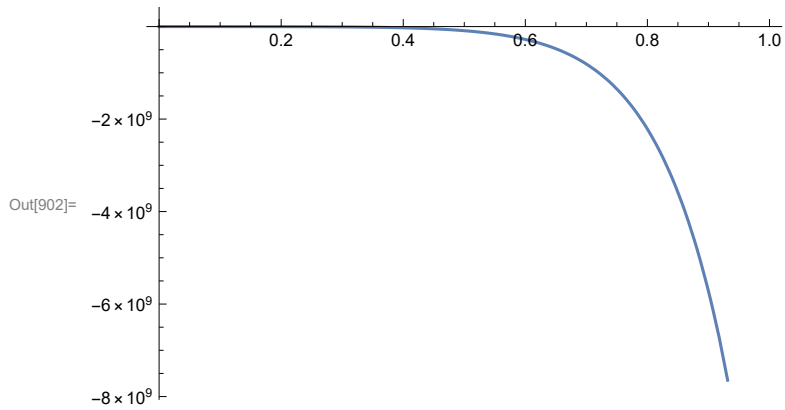

In[903]:= **Plot[Cf[9, 7, 10], {x, 0, 1}]**

[绘图](#)

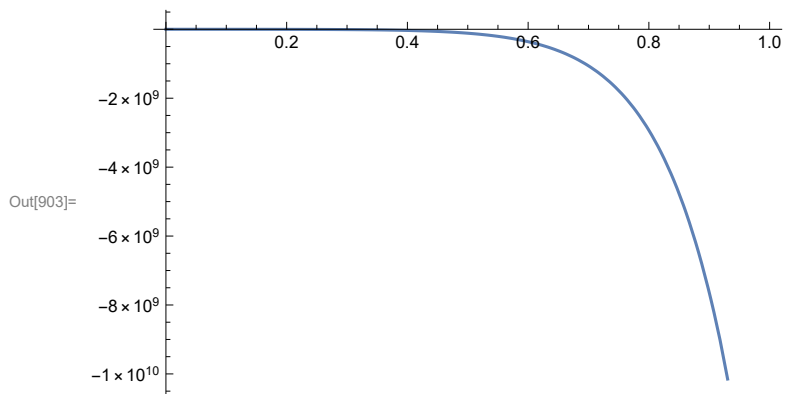

In[904]:= **Plot[Cf[9, 7, 9], {x, 0, 1}]**

[绘图](#)

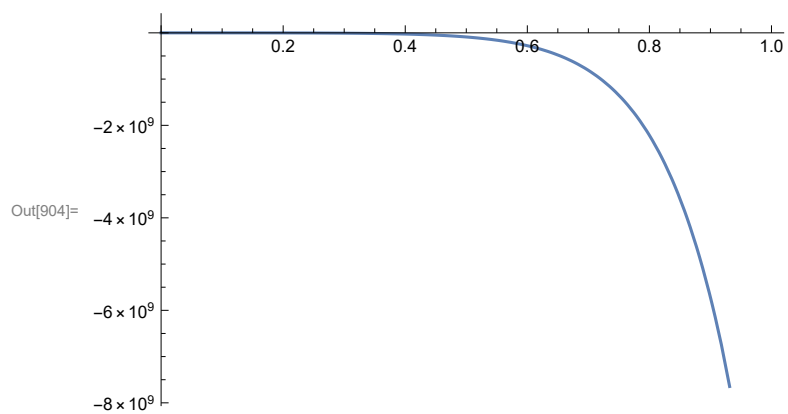

In[905]:= **Plot[Cf[9, 7, 8], {x, 0, 1}]**

[绘图](#)

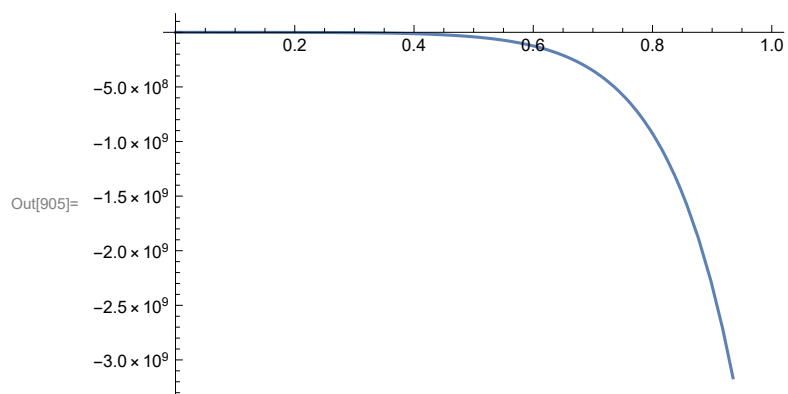

In[906]:= **Plot[Cf[9, 7, 7], {x, 0, 1}]**

[绘图](#)

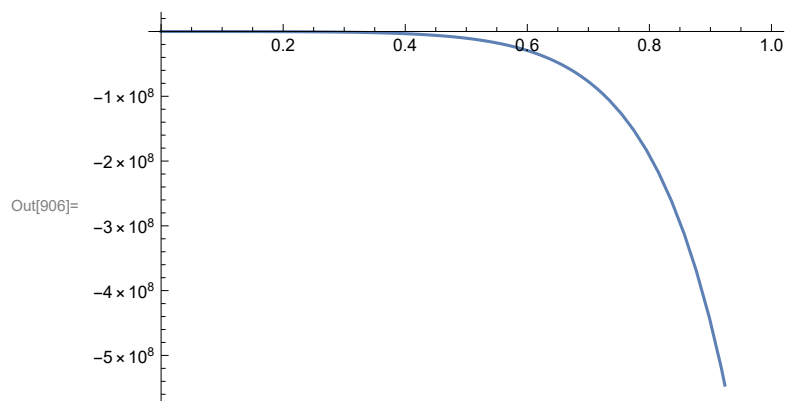

In[907]:= **Plot[Cf[9, 7, 6], {x, 0, 1}]**

[绘图](#)

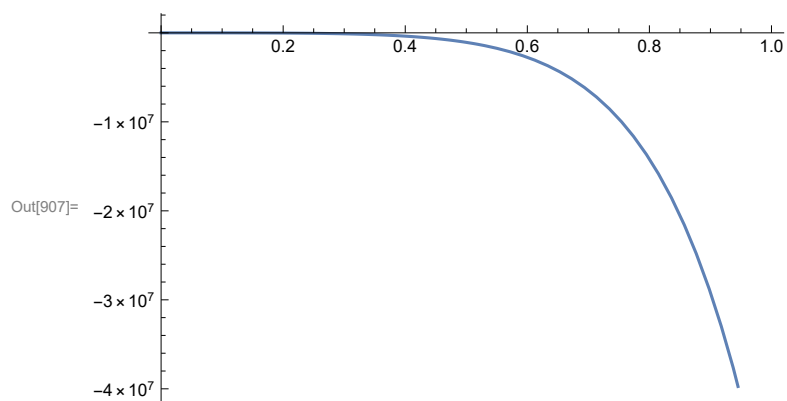

**Plot[Cf[9, 7, 5], {x, 0, 1}]**

[绘图](#)

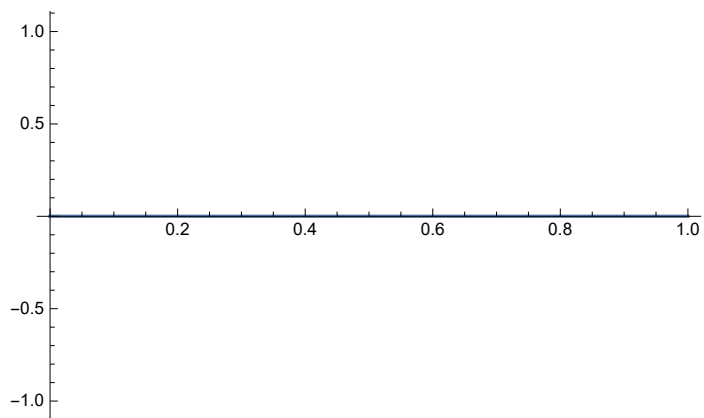

**Plot[Cf[9, 7, 4], {x, 0, 1}]**

[绘图](#)

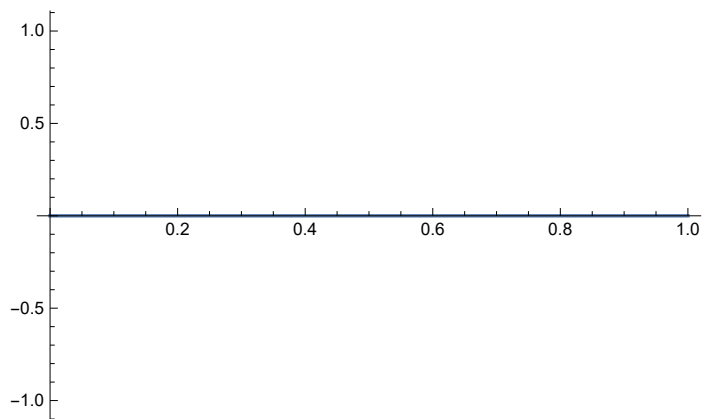

```
Plot[Cf[9, 7, 3], {x, 0, 1}]
```

[绘图](#)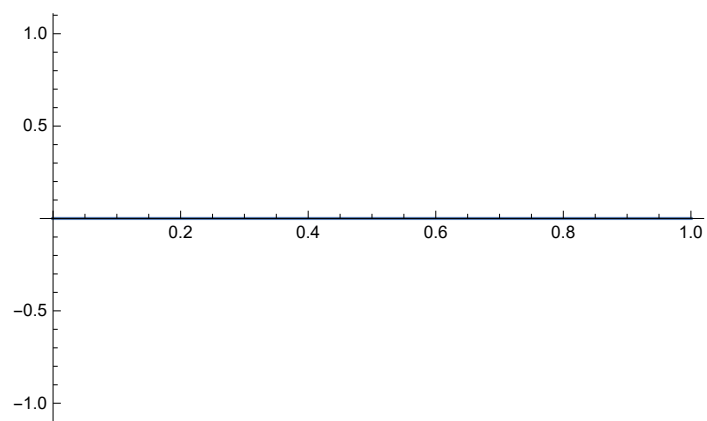

```
Plot[Cf[9, 7, 2], {x, 0, 1}]
```

[绘图](#)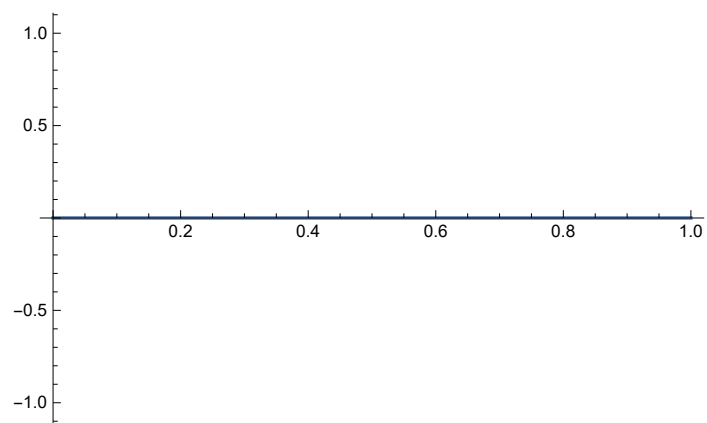

```
Plot[Cf[9, 7, 1], {x, 0, 1}]
```

[绘图](#)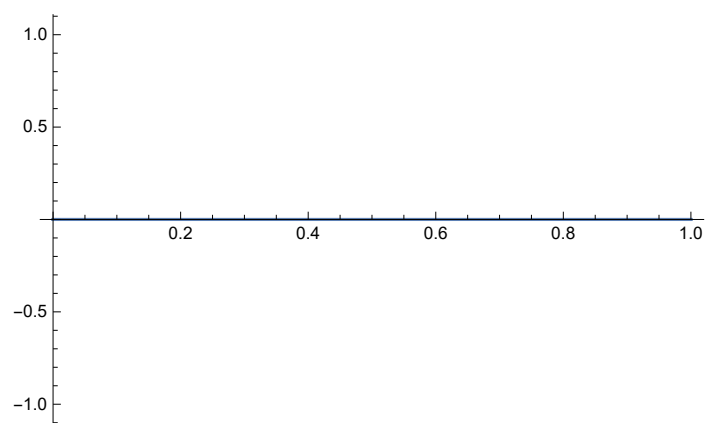

**Plot[Cf[9, 7, 0], {x, 0, 1}]**

[绘图](#)

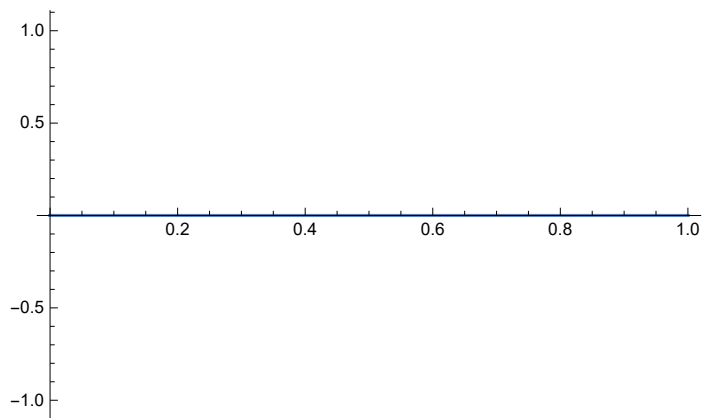

**(\*84th group coefficients r2^9r3^6\*)**

In[908]:= **Plot[Cf[9, 6, 14], {x, 0, 1}]**

[绘图](#)

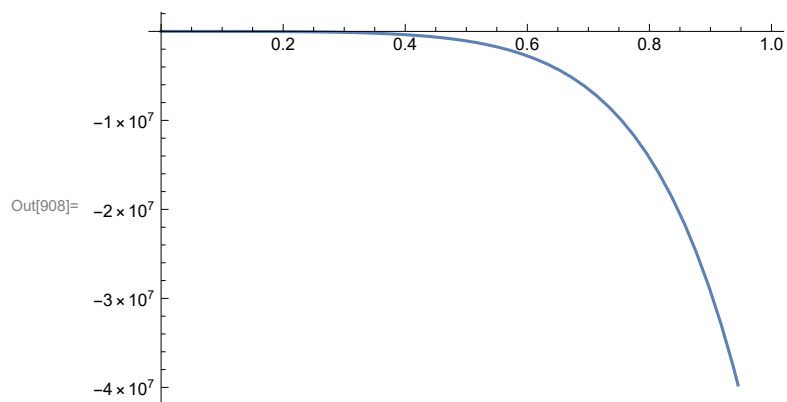

In[909]:= **Plot[Cf[9, 6, 13], {x, 0, 1}]**

[绘图](#)

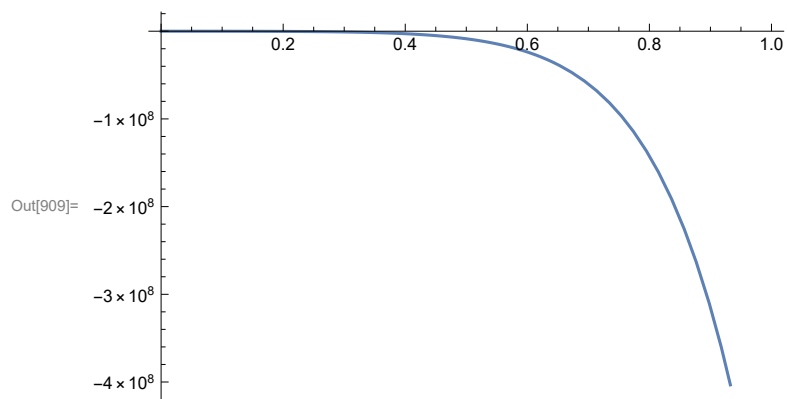

In[910]:= **Plot[Cf[9, 6, 12], {x, 0, 1}]**

[绘图](#)

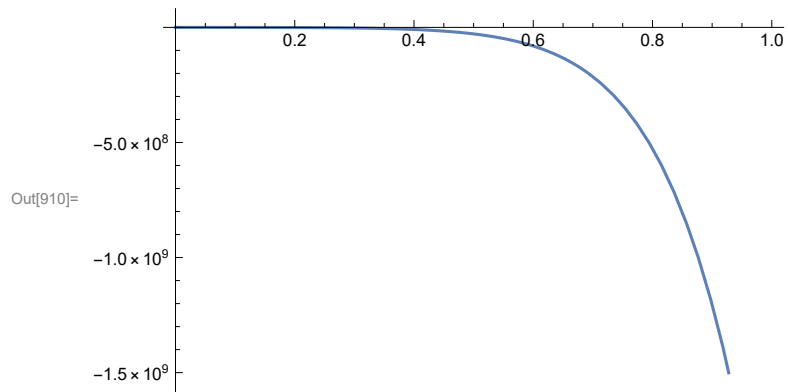

In[911]:= **Plot[Cf[9, 6, 11], {x, 0, 1}]**

[绘图](#)

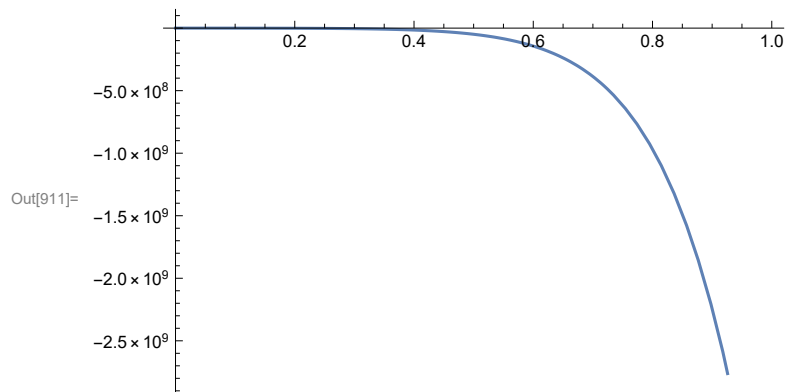

In[912]:= **Plot[Cf[9, 6, 10], {x, 0, 1}]**

[绘图](#)

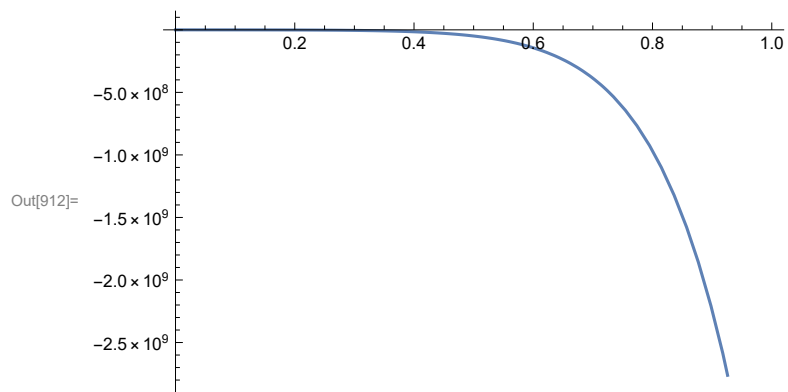



In[913]:= **Plot[Cf[9, 6, 9], {x, 0, 1}]**

[绘图](#)

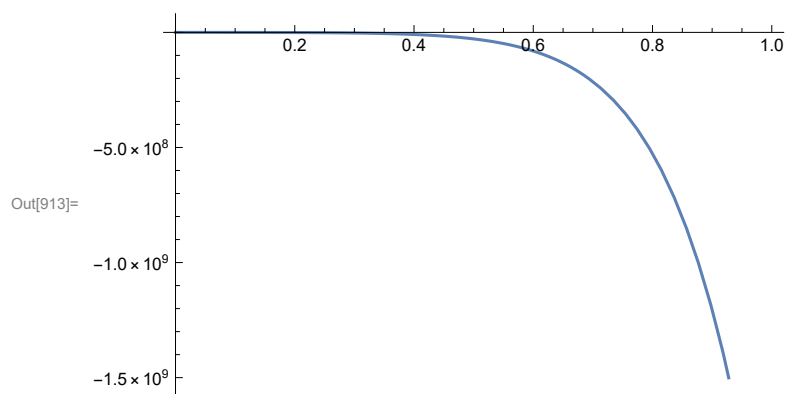

In[914]:= **Plot[Cf[9, 6, 8], {x, 0, 1}]**

[绘图](#)

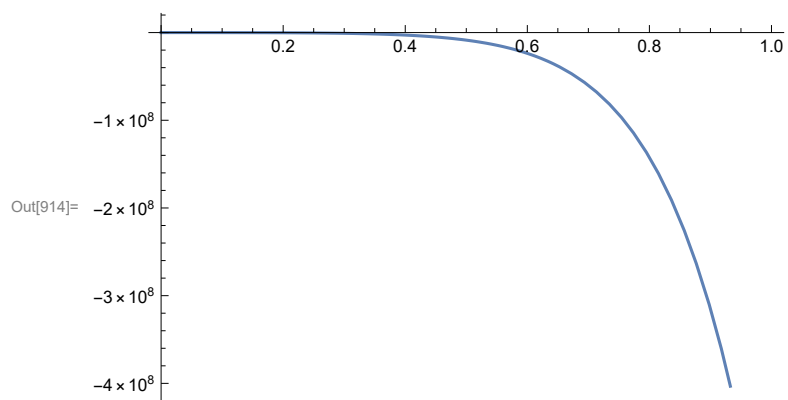

In[915]:= **Plot[Cf[9, 6, 7], {x, 0, 1}]**

[绘图](#)

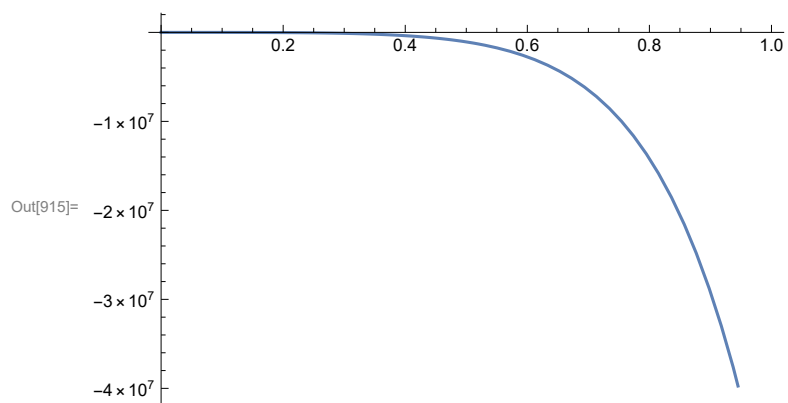

**Plot[Cf[9, 6, 6], {x, 0, 1}]**

[绘图](#)

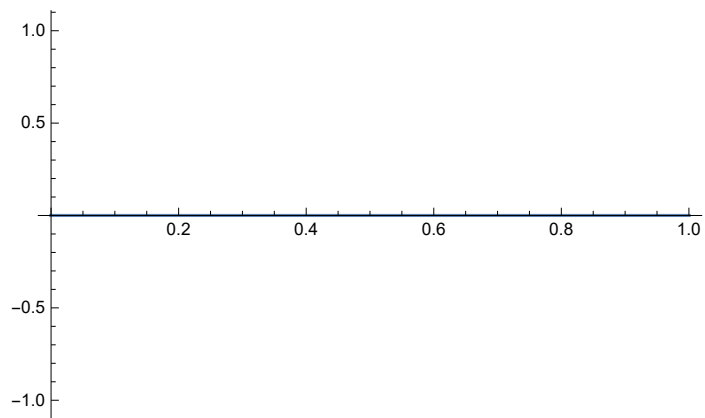

**Plot[Cf[9, 6, 5], {x, 0, 1}]**

[绘图](#)

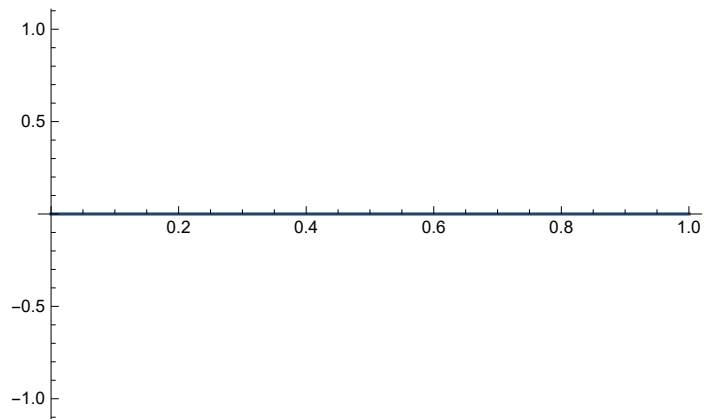

**Plot[Cf[9, 6, 4], {x, 0, 1}]**

[绘图](#)

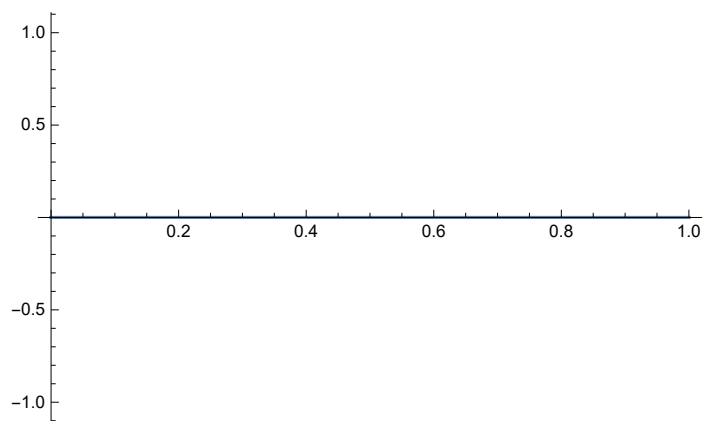

**Plot[Cf[9, 6, 3], {x, 0, 1}]**

[绘图](#)

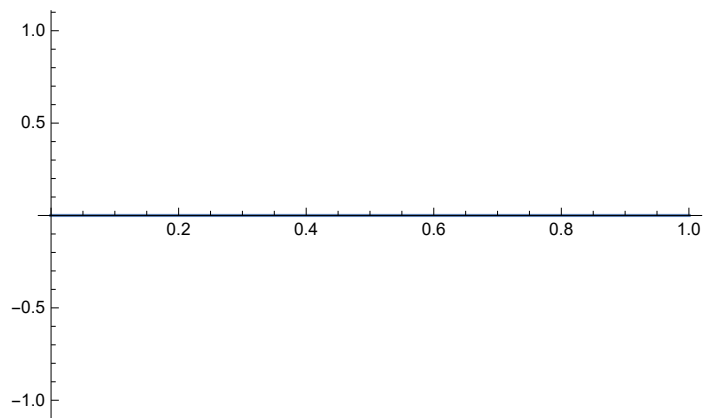

**Plot[Cf[9, 6, 2], {x, 0, 1}]**

[绘图](#)

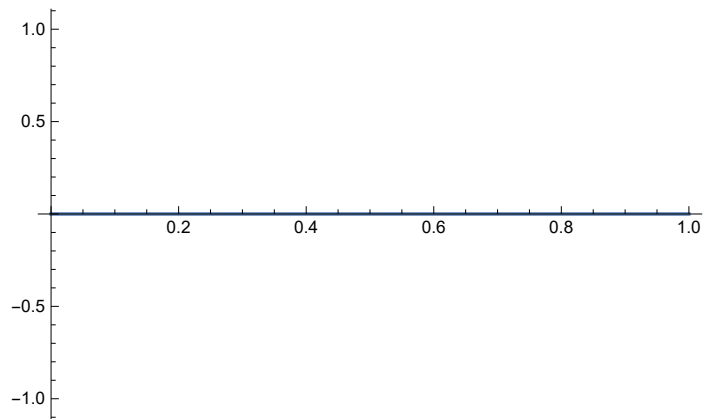

**Plot[Cf[9, 6, 1], {x, 0, 1}]**

[绘图](#)

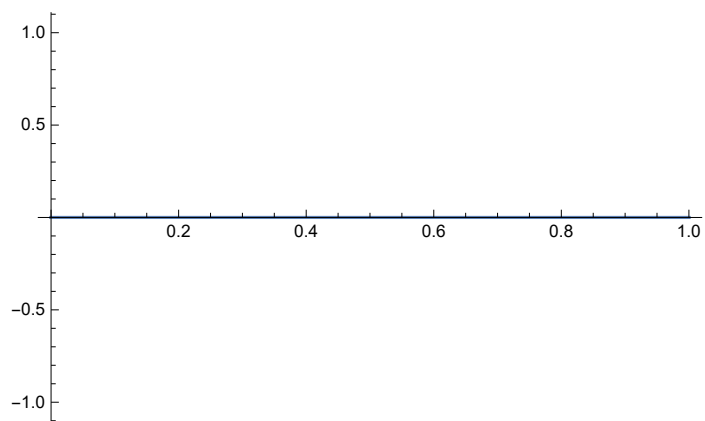

**Plot[Cf[9, 6, 0], {x, 0, 1}]**

[绘图](#)

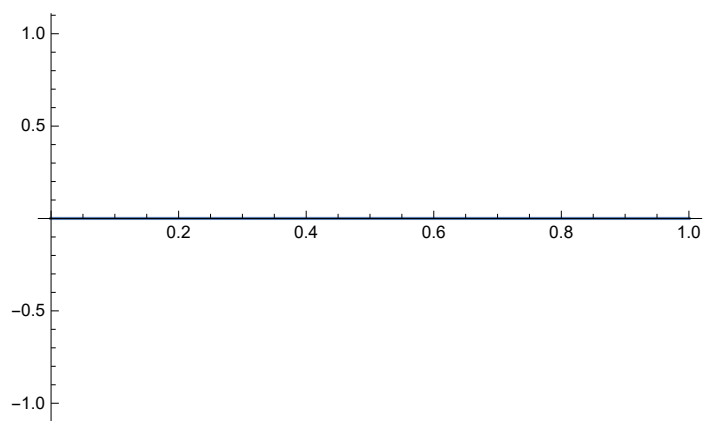

**(\*85th group coefficients r2^9r3^5\*)**

In[917]:= **Plot[Cf[9, 5, 14], {x, 0, 1}]**

[绘图](#)

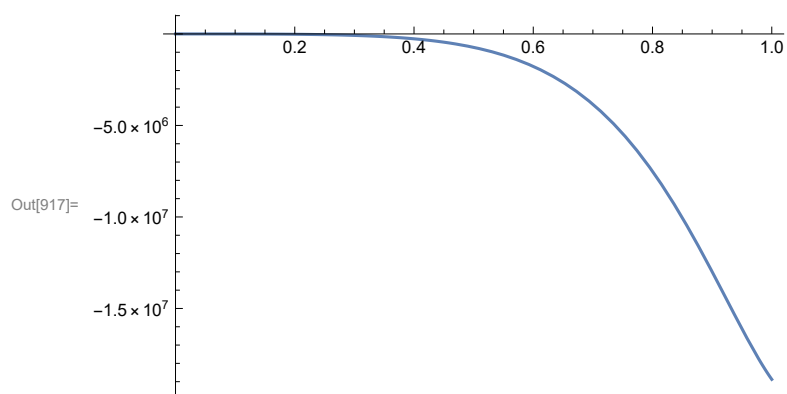

In[916]:= **Plot[Cf[9, 5, 13], {x, 0, 1}]**

[绘图](#)

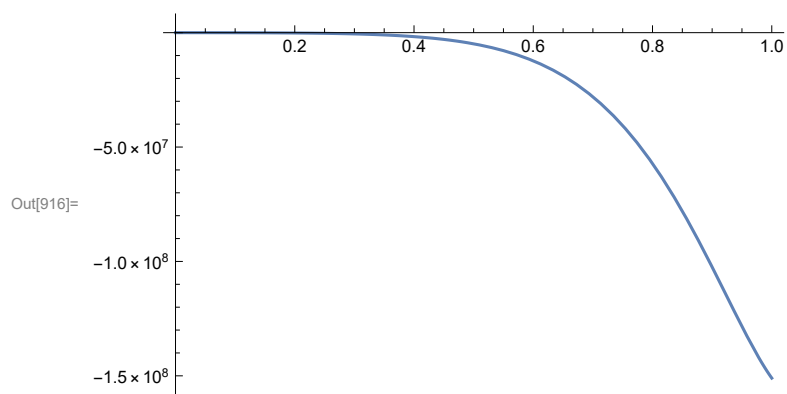

In[918]:= **Plot[Cf[9, 5, 12], {x, 0, 1}]**

[绘图](#)

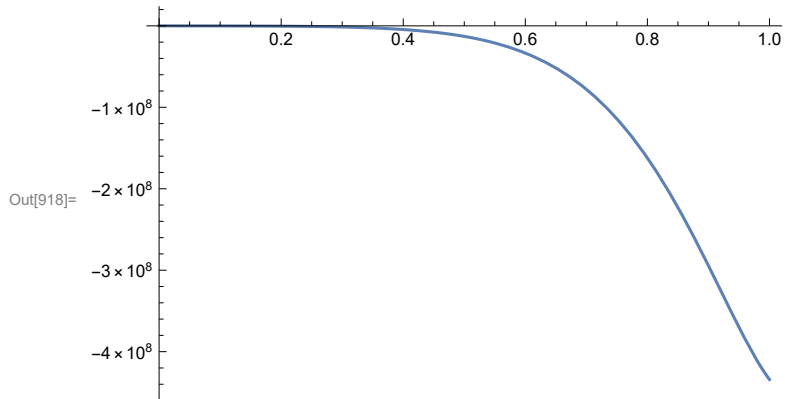

In[919]:= **Plot[Cf[9, 5, 11], {x, 0, 1}]**

[绘图](#)

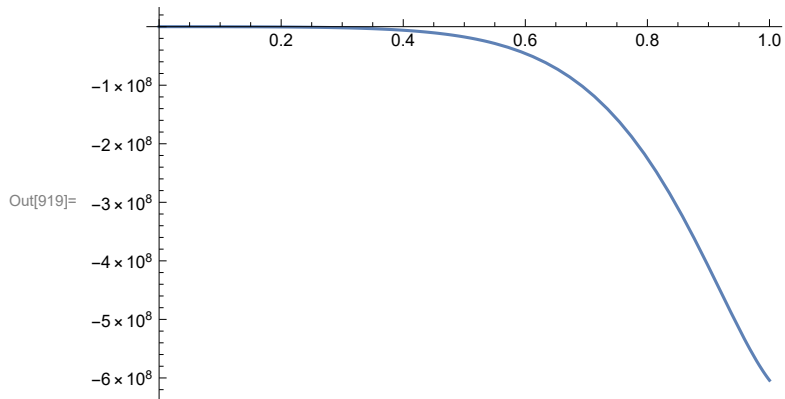

In[920]:= **Plot[Cf[9, 5, 10], {x, 0, 1}]**

[绘图](#)

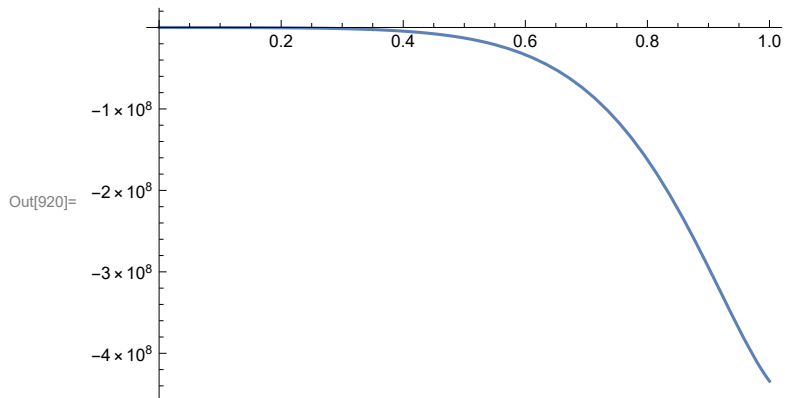

In[921]:= **Plot[Cf[9, 5, 9], {x, 0, 1}]**

[绘图](#)

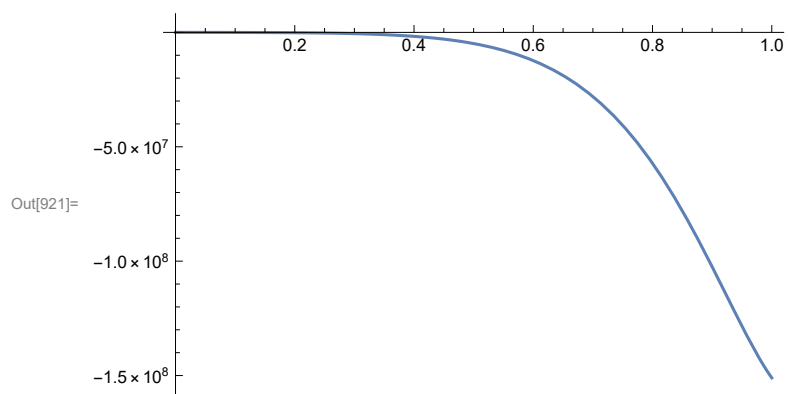

In[922]:= **Plot[Cf[9, 5, 8], {x, 0, 1}]**

[绘图](#)

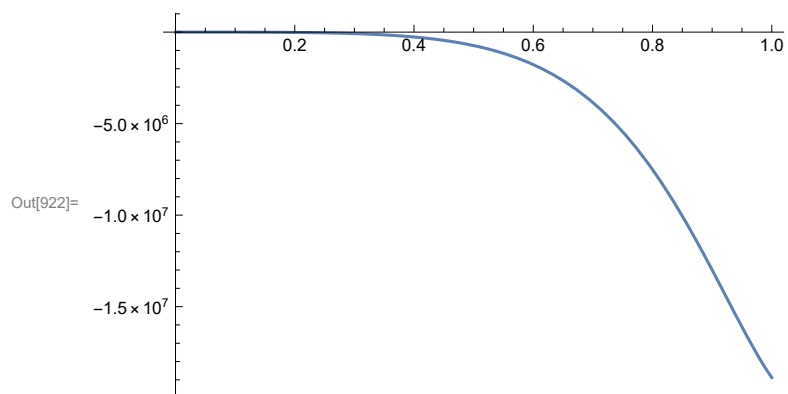

**Plot[Cf[9, 5, 7], {x, 0, 1}]**

[绘图](#)

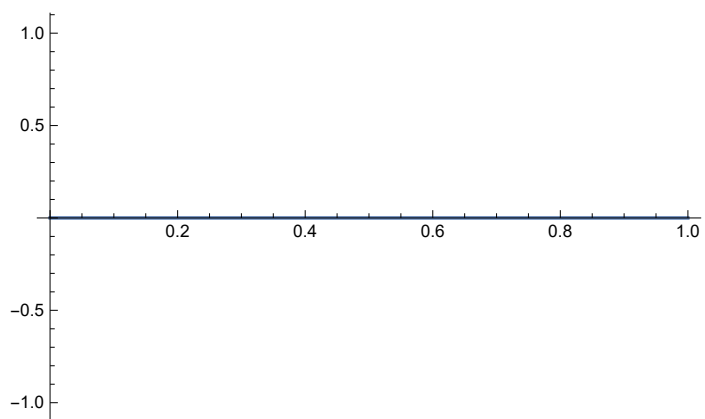

**Plot[Cf[9, 5, 6], {x, 0, 1}]**

[绘图](#)

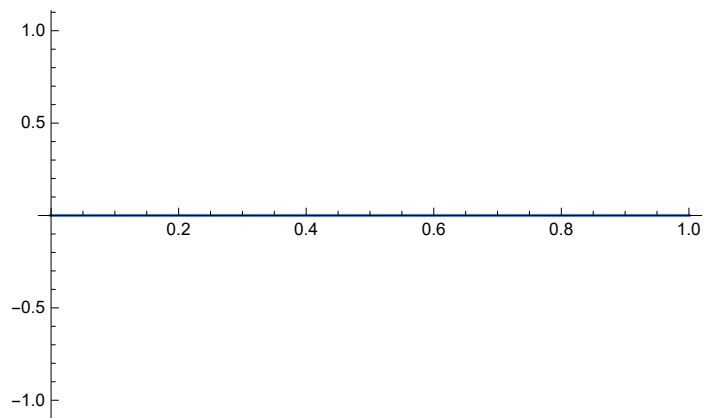

**Plot[Cf[9, 5, 5], {x, 0, 1}]**

[绘图](#)

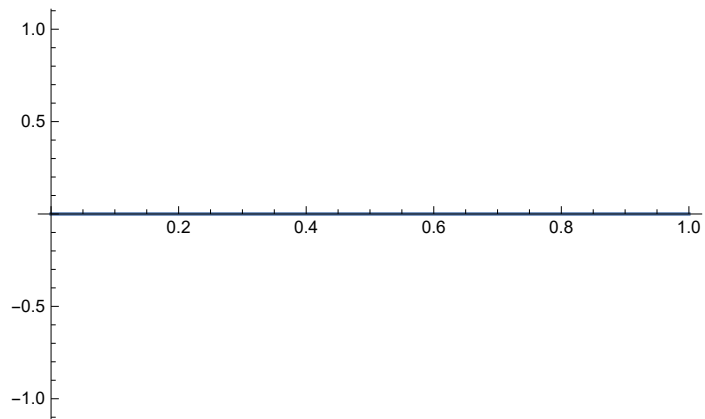

**Plot[Cf[9, 5, 4], {x, 0, 1}]**

[绘图](#)

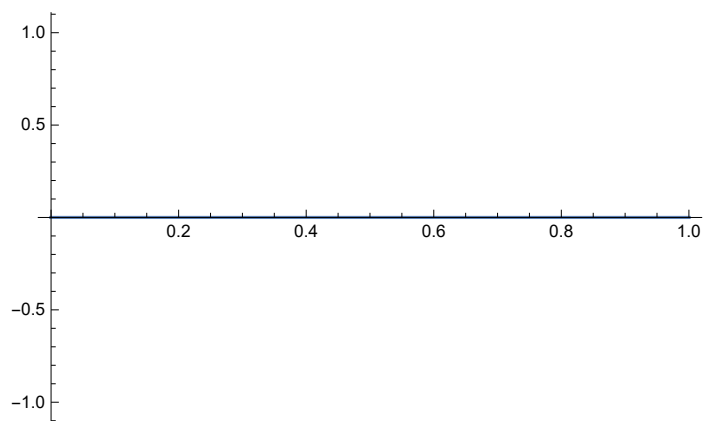

```
Plot[Cf[9, 5, 3], {x, 0, 1}]
```

[绘图](#)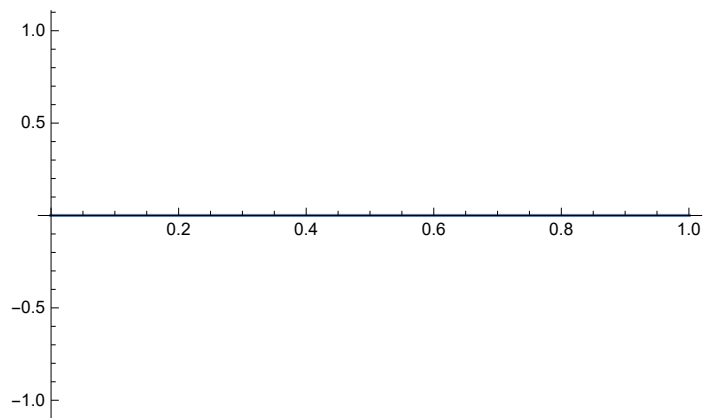

```
Plot[Cf[9, 5, 2], {x, 0, 1}]
```

[绘图](#)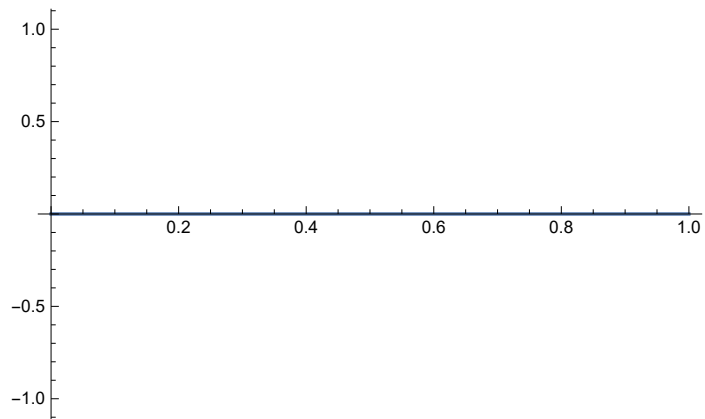

```
Plot[Cf[9, 5, 1], {x, 0, 1}]
```

[绘图](#)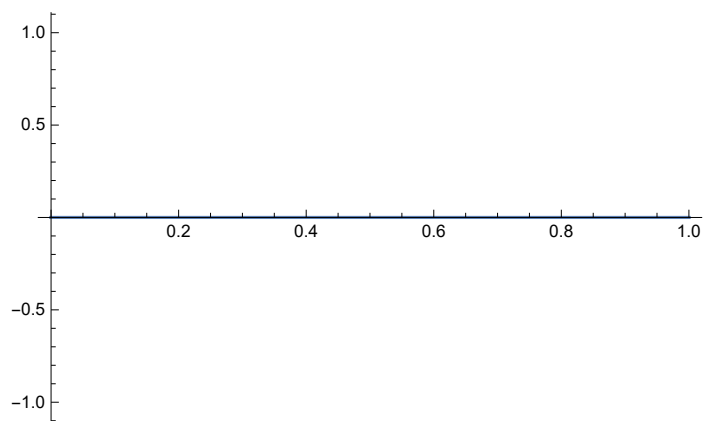



**Plot[Cf[9, 5, 0], {x, 0, 1}]**

[绘图](#)

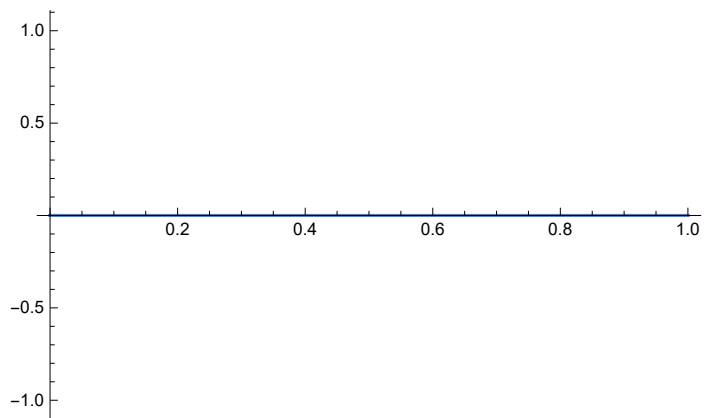

(\*86th group coefficients r2^9r3^4\*)

In[923]:= **Plot[Cf[9, 4, 14], {x, 0, 1}]**

[绘图](#)

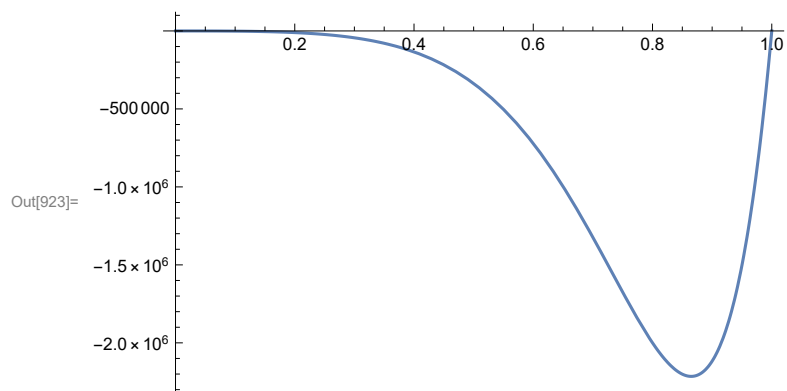

In[924]:= **Plot[Cf[9, 4, 13], {x, 0, 1}]**

[绘图](#)

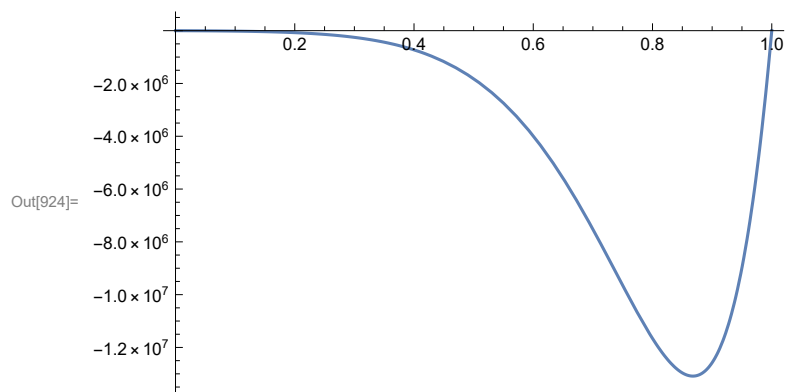

In[925]:= **Plot[Cf[9, 4, 12], {x, 0, 1}]**

[绘图](#)

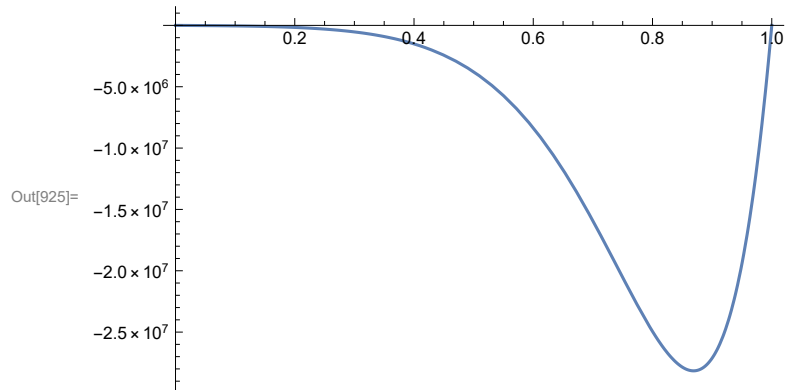

In[926]:= **Plot[Cf[9, 4, 11], {x, 0, 1}]**

[绘图](#)

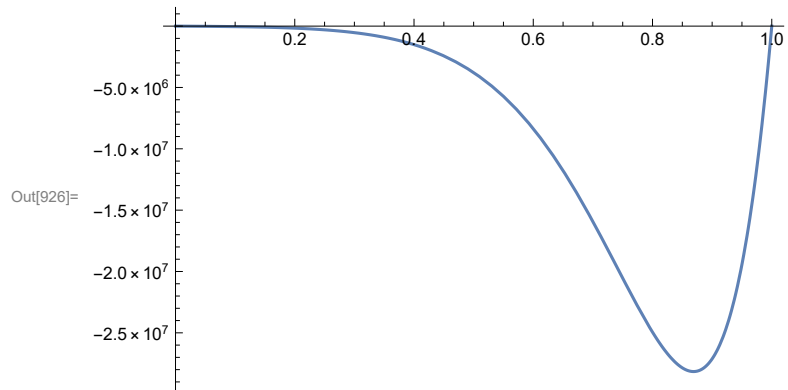

In[927]:= **Plot[Cf[9, 4, 10], {x, 0, 1}]**

[绘图](#)

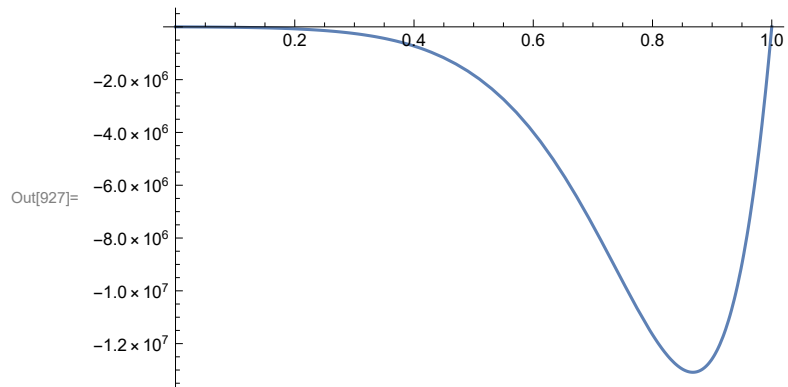

In[928]:= **Plot[Cf[9, 4, 9], {x, 0, 1}]**

[绘图](#)

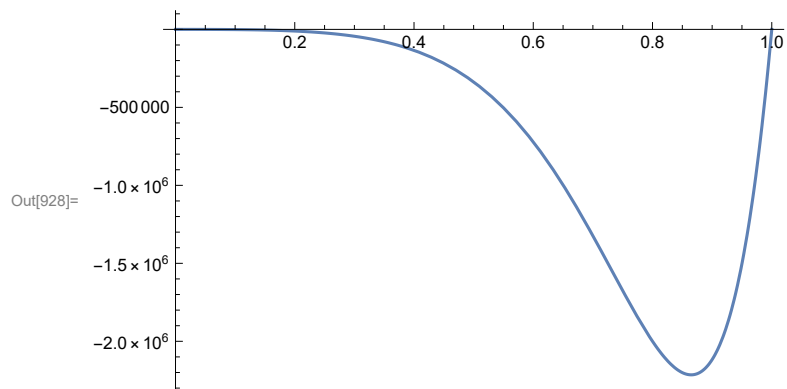

**Plot[Cf[9, 4, 8], {x, 0, 1}]**

[绘图](#)

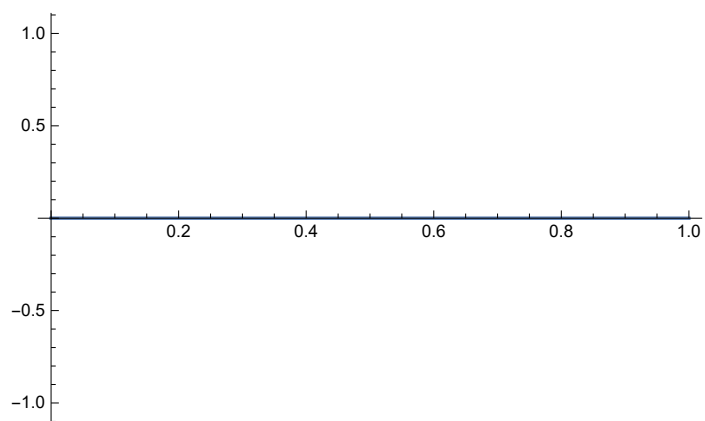

**Plot[Cf[9, 4, 7], {x, 0, 1}]**

[绘图](#)

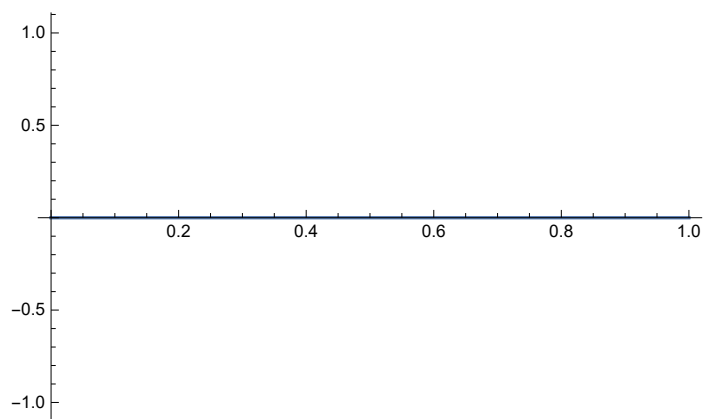

**Plot[Cf[9, 4, 6], {x, 0, 1}]**

[绘图](#)

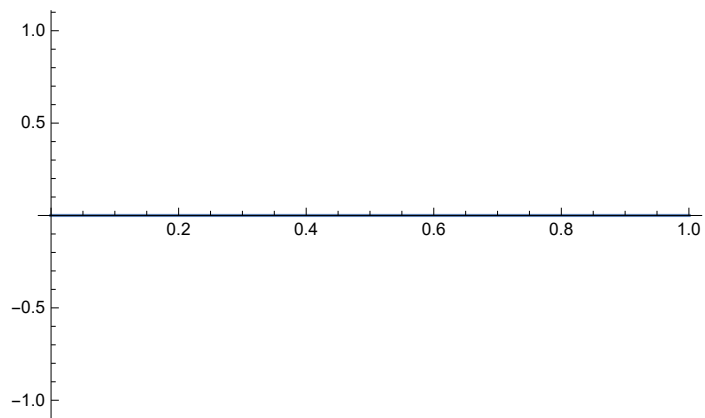

**Plot[Cf[9, 4, 5], {x, 0, 1}]**

[绘图](#)

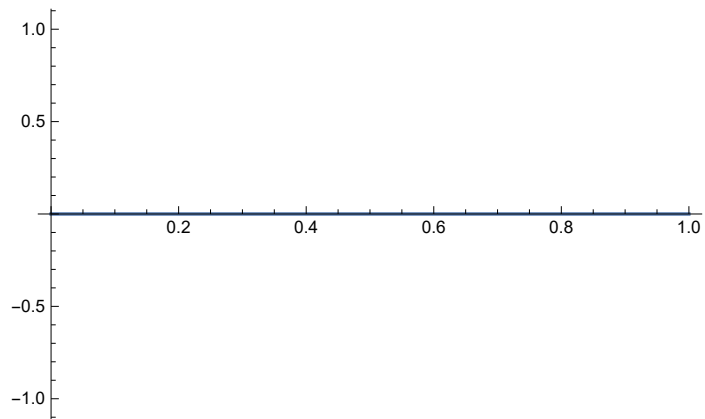

**Plot[Cf[9, 4, 4], {x, 0, 1}]**

[绘图](#)

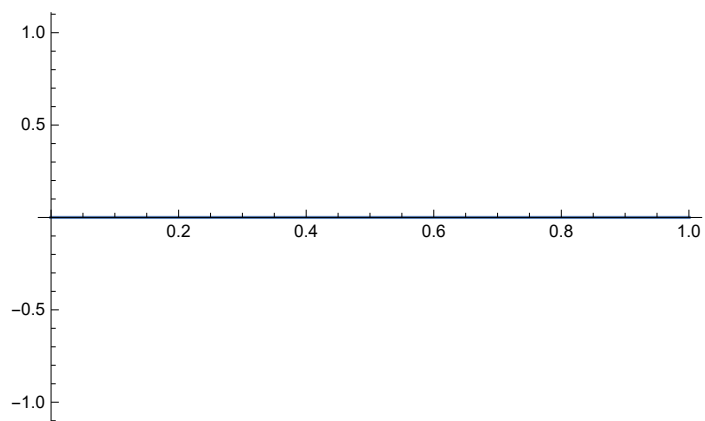

**Plot[Cf[9, 4, 3], {x, 0, 1}]**

[绘图](#)

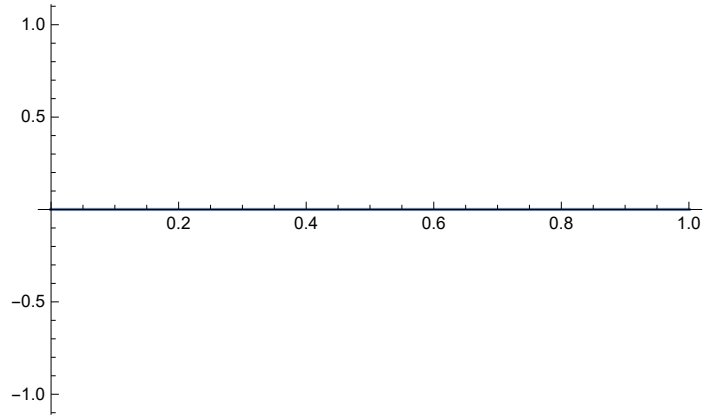

**Plot[Cf[9, 4, 2], {x, 0, 1}]**

[绘图](#)

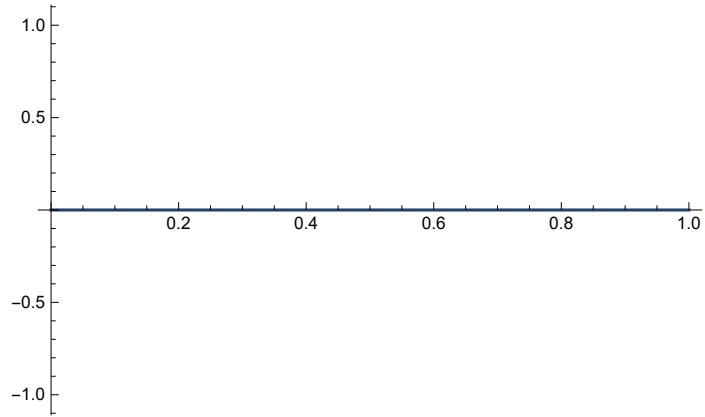

**Plot[Cf[9, 4, 1], {x, 0, 1}]**

[绘图](#)

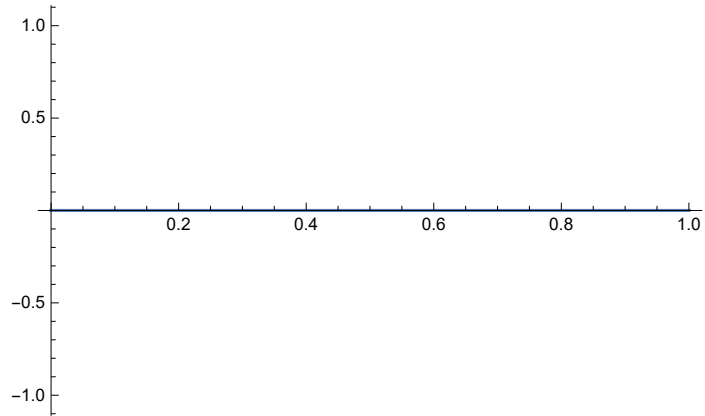

**Plot[Cf[9, 4, 0], {x, 0, 1}]**

[绘图](#)

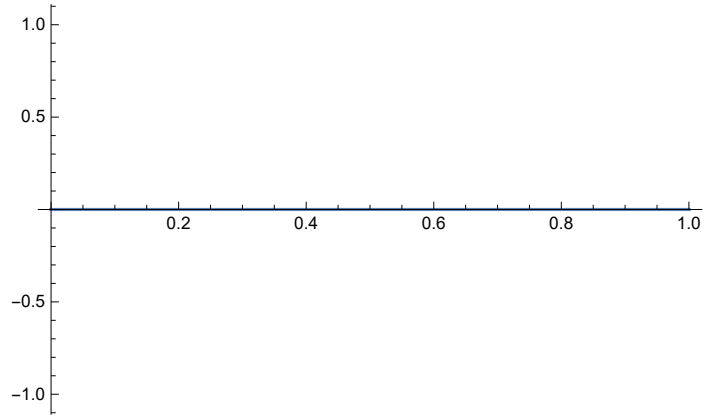

**(\*87th group coefficients r2^9r3^3\*)**

In[929]:= **Plot[Cf[9, 3, 14], {x, 0, 1}]**

[绘图](#)

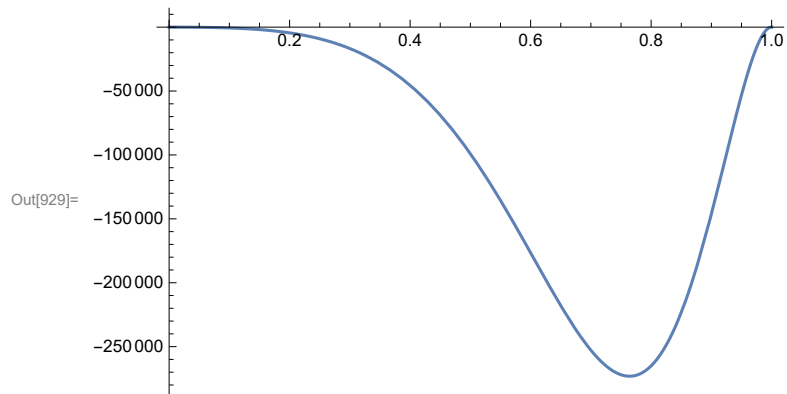

In[930]:= **Plot[Cf[9, 3, 13], {x, 0, 1}]**

[绘图](#)

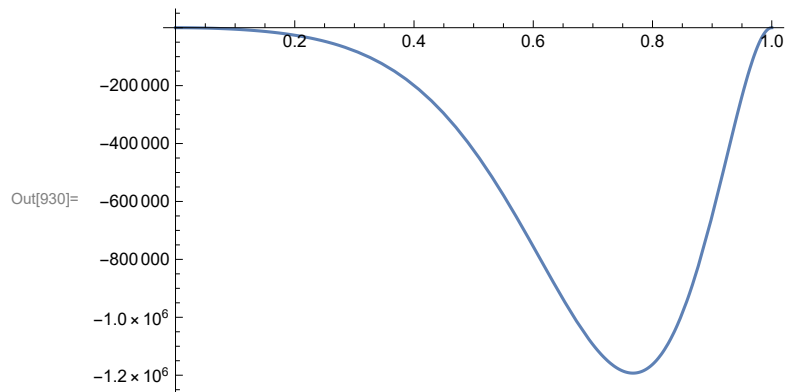

In[931]:= **Plot[Cf[9, 3, 12], {x, 0, 1}]**

[绘图](#)

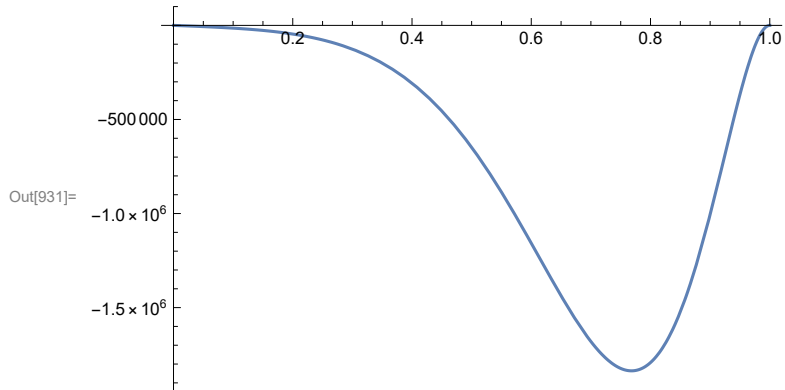

In[932]:= **Plot[Cf[9, 3, 11], {x, 0, 1}]**

[绘图](#)

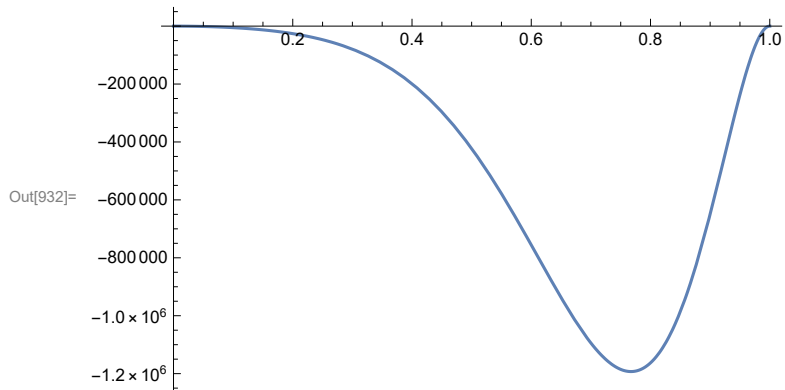

In[933]:= **Plot[Cf[9, 3, 10], {x, 0, 1}]**

[绘图](#)

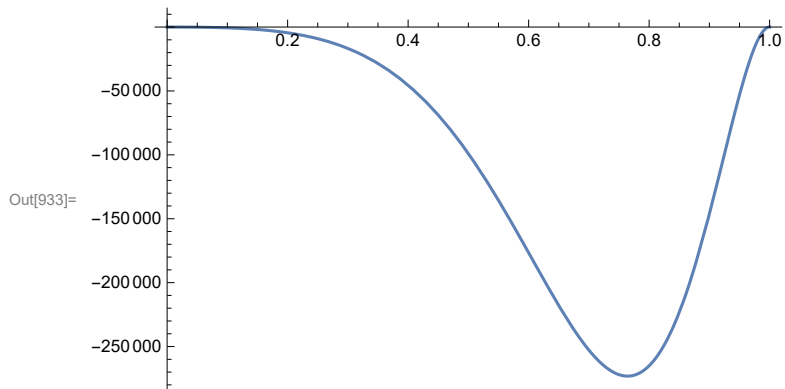

**Plot[Cf[9, 3, 9], {x, 0, 1}]**

[绘图](#)

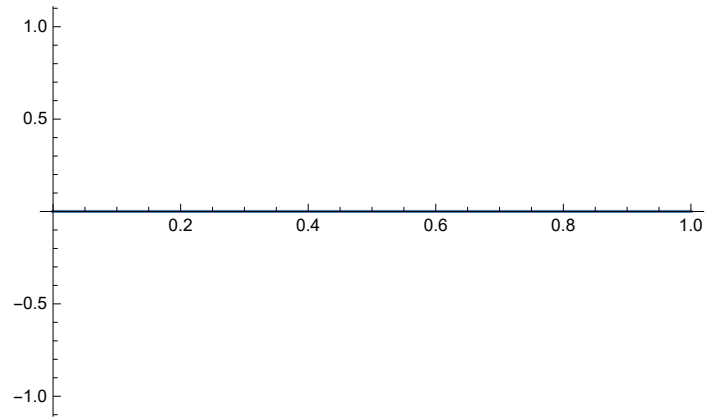

**Plot[Cf[9, 3, 8], {x, 0, 1}]**

[绘图](#)

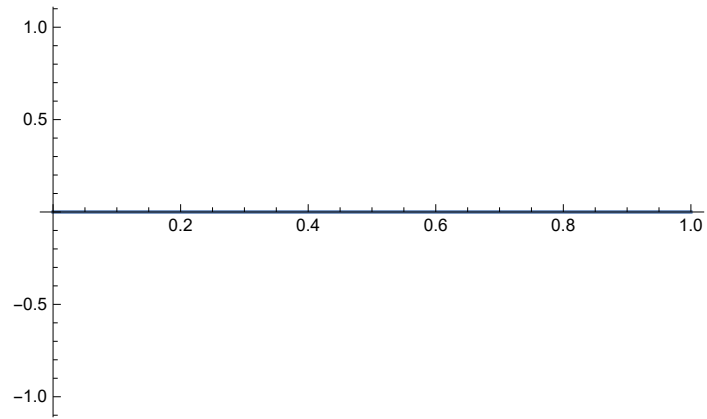

**Plot[Cf[9, 3, 7], {x, 0, 1}]**

[绘图](#)

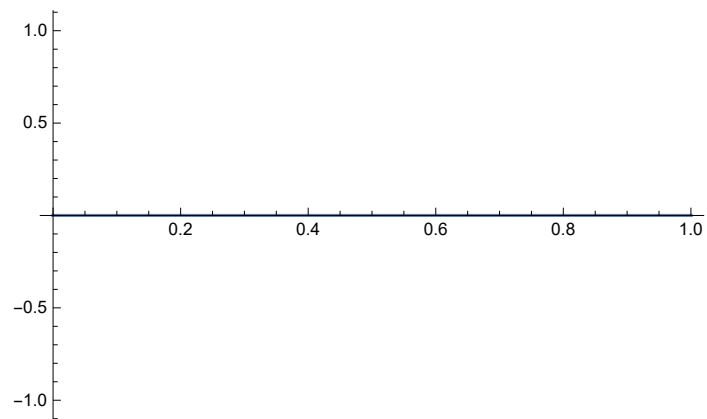



**Plot[Cf[9, 3, 6], {x, 0, 1}]**

[绘图](#)

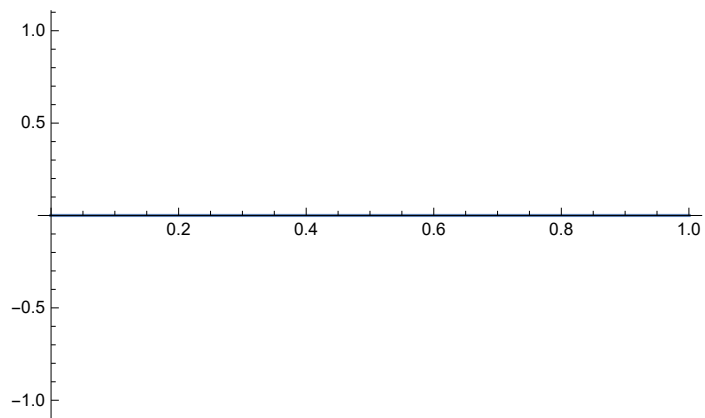

**Plot[Cf[9, 3, 5], {x, 0, 1}]**

[绘图](#)

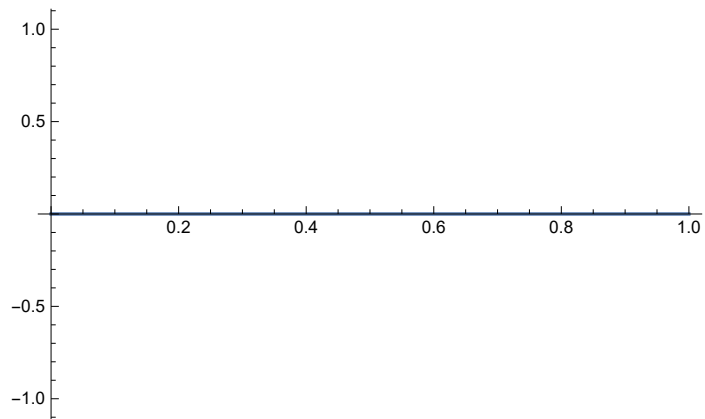

**Plot[Cf[9, 3, 4], {x, 0, 1}]**

[绘图](#)

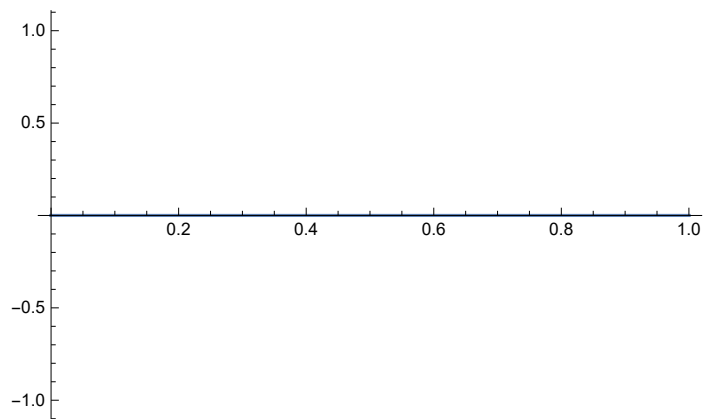

**Plot[Cf[9, 3, 3], {x, 0, 1}]**

[绘图](#)

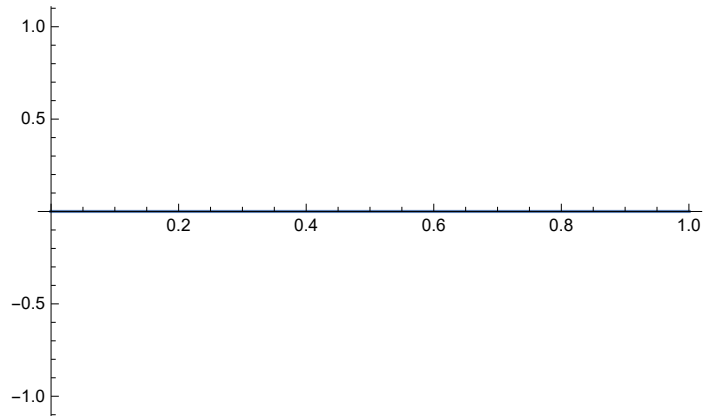

**Plot[Cf[9, 3, 2], {x, 0, 1}]**

[绘图](#)

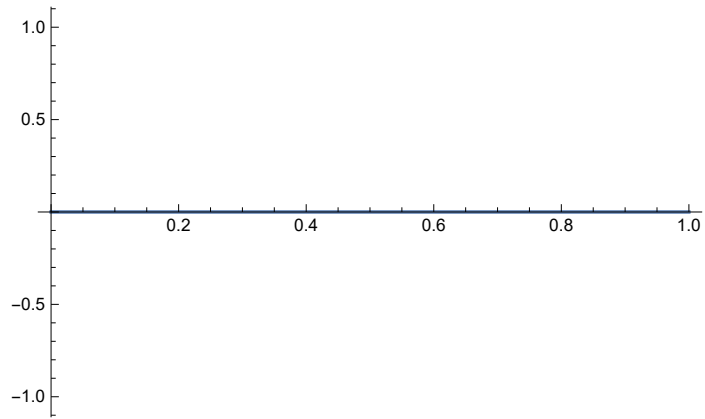

**Plot[Cf[9, 3, 1], {x, 0, 1}]**

[绘图](#)

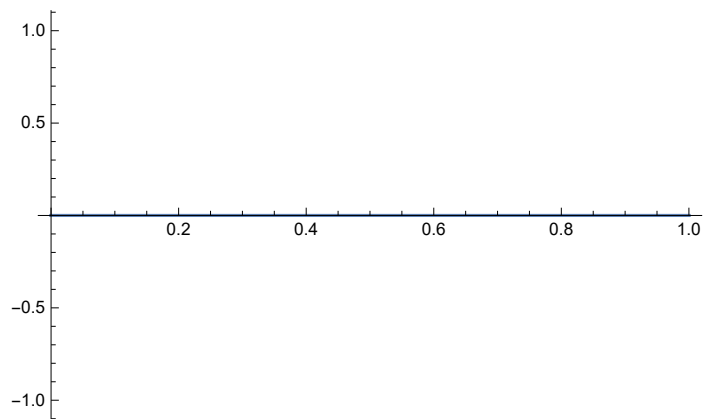

**Plot[Cf[9, 3, 0], {x, 0, 1}]**

[绘图](#)

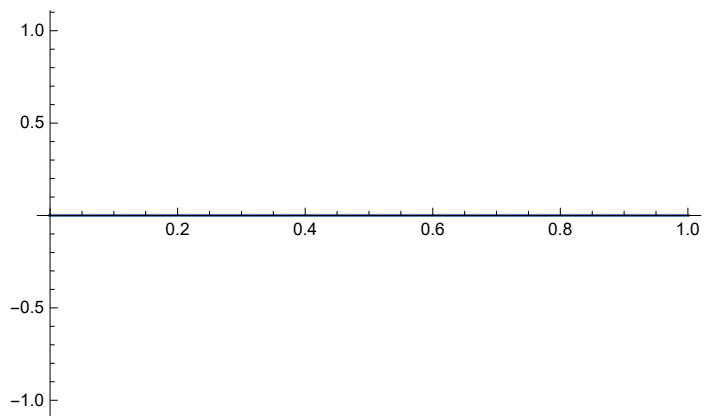

(\*88th group coefficients r2^9r3^2\*)

In[934]:= **Plot[Cf[9, 2, 14], {x, 0, 1}]**

[绘图](#)

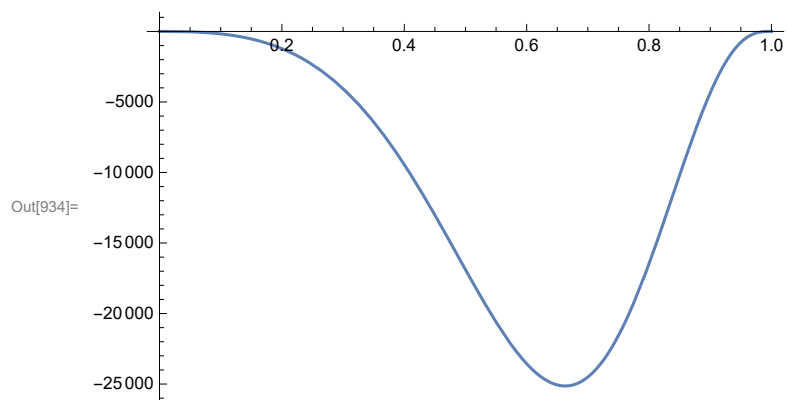

In[935]:= **Plot[Cf[9, 2, 13], {x, 0, 1}]**

[绘图](#)

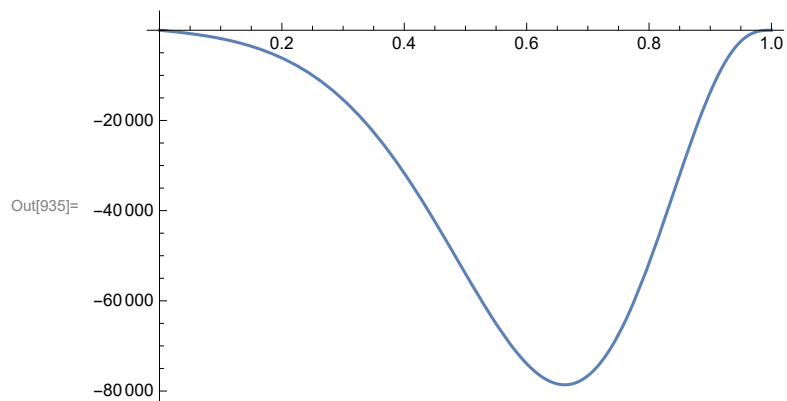

In[936]:= **Plot[Cf[9, 2, 12], {x, 0, 1}]**

[绘图](#)

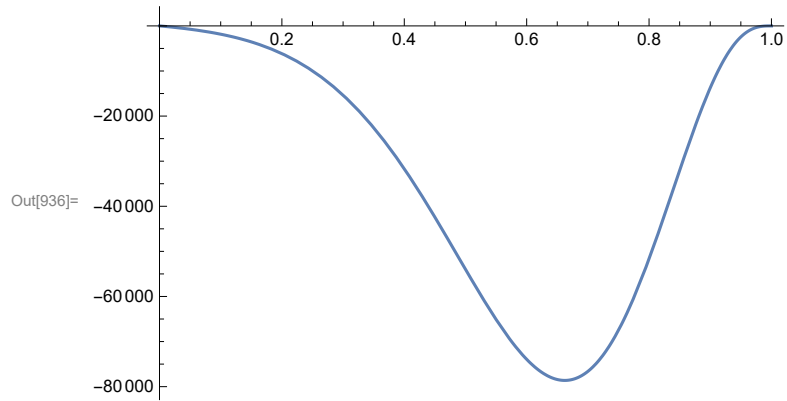

In[937]:= **Plot[Cf[9, 2, 11], {x, 0, 1}]**

[绘图](#)

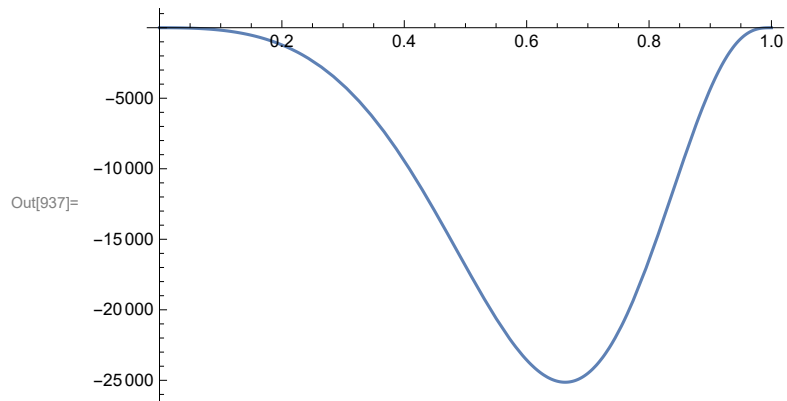

**Plot[Cf[9, 2, 10], {x, 0, 1}]**

[绘图](#)

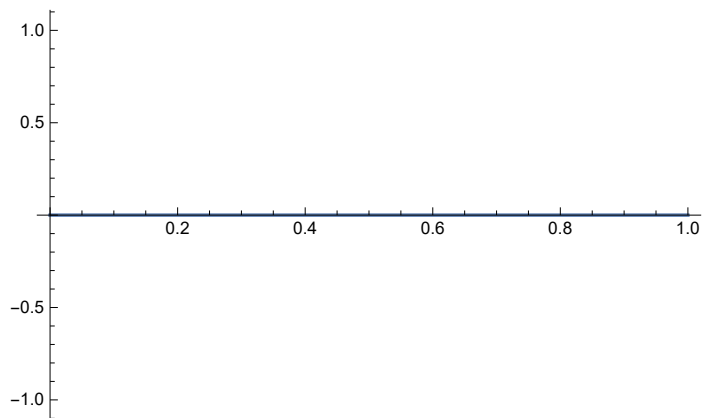

**Plot[Cf[9, 2, 9], {x, 0, 1}]**

[绘图](#)

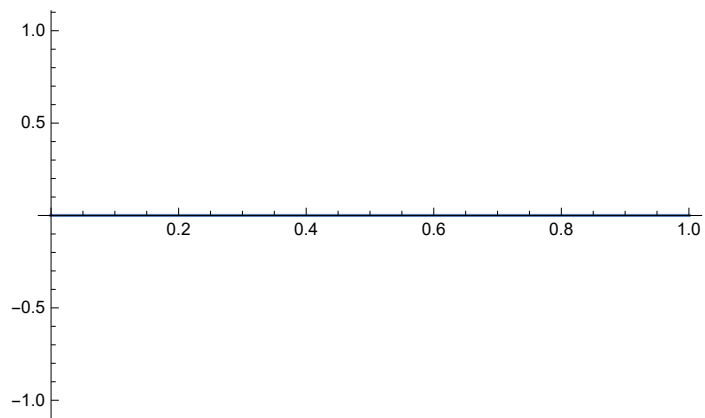

**Plot[Cf[9, 2, 8], {x, 0, 1}]**

[绘图](#)

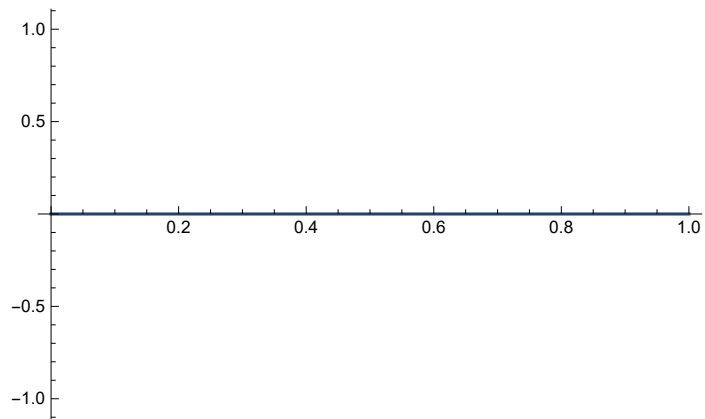

**Plot[Cf[9, 2, 7], {x, 0, 1}]**

[绘图](#)

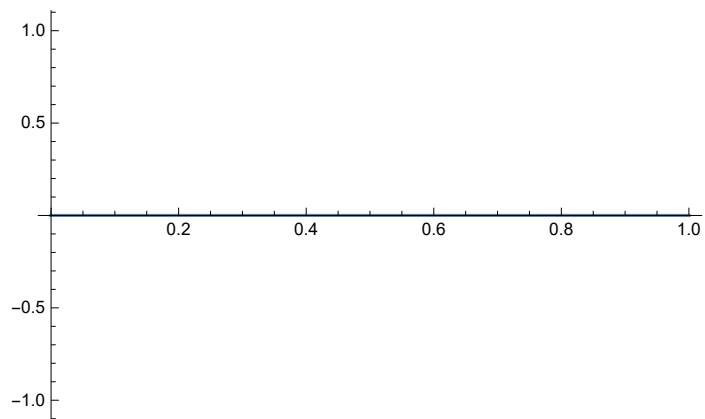

**Plot[Cf[9, 2, 6], {x, 0, 1}]**

[绘图](#)

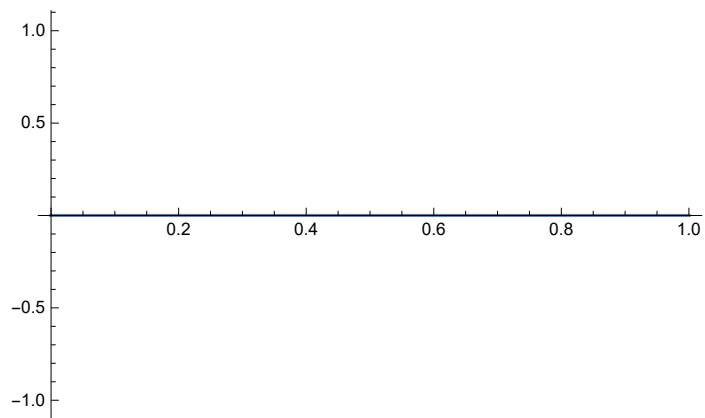

**Plot[Cf[9, 2, 5], {x, 0, 1}]**

[绘图](#)

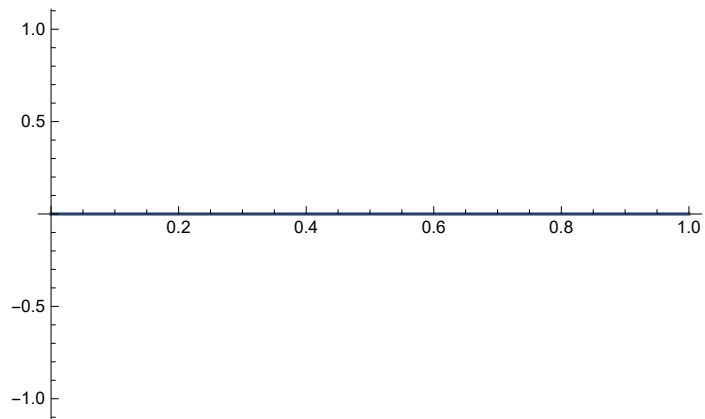

**Plot[Cf[9, 2, 4], {x, 0, 1}]**

[绘图](#)

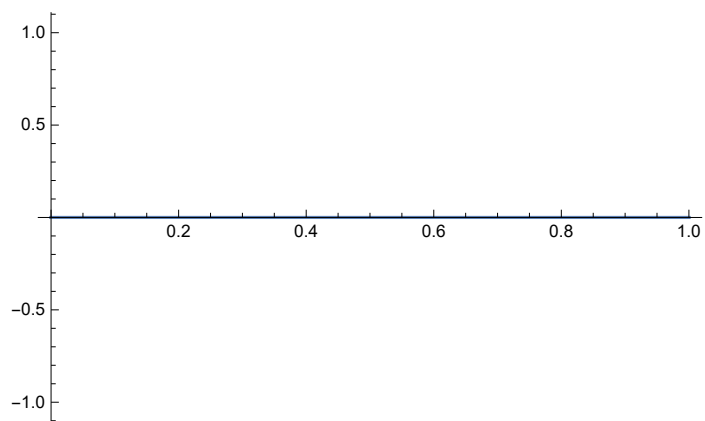

**Plot[Cf[9, 2, 3], {x, 0, 1}]**

[绘图](#)

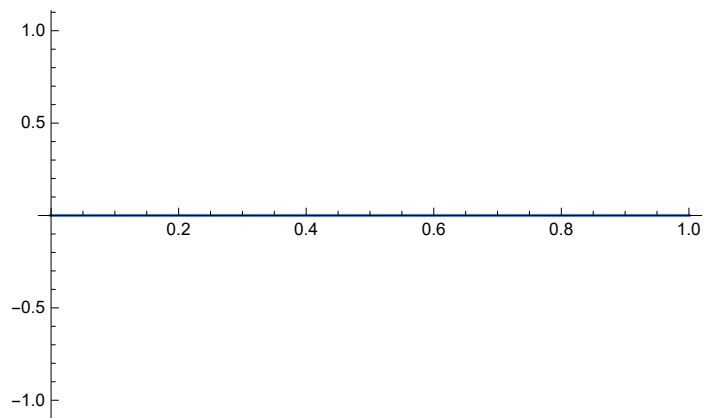

**Plot[Cf[9, 2, 2], {x, 0, 1}]**

[绘图](#)

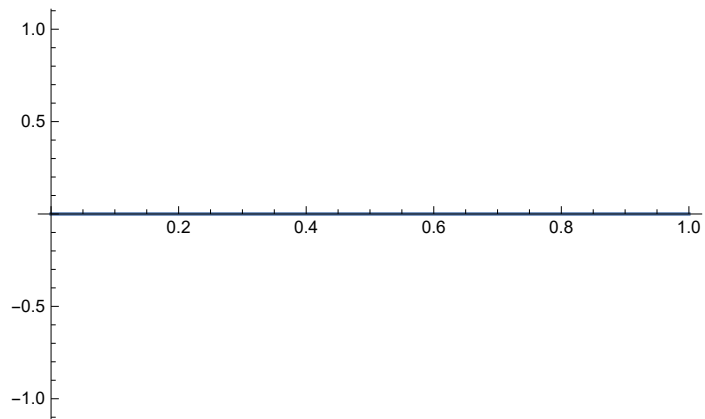

**Plot[Cf[9, 2, 1], {x, 0, 1}]**

[绘图](#)

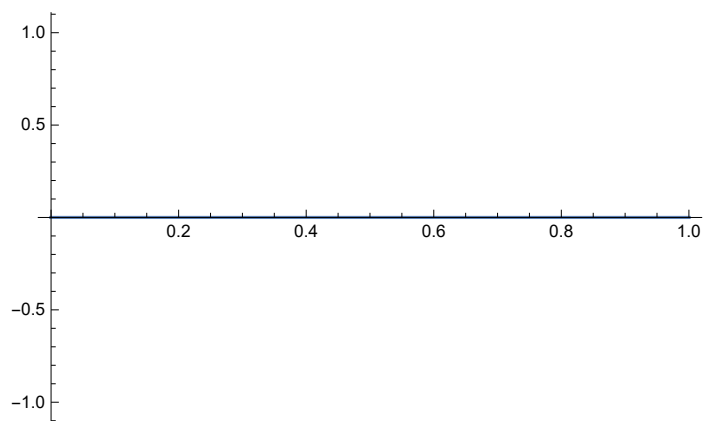

**Plot[Cf[9, 2, 0], {x, 0, 1}]**

[绘图](#)

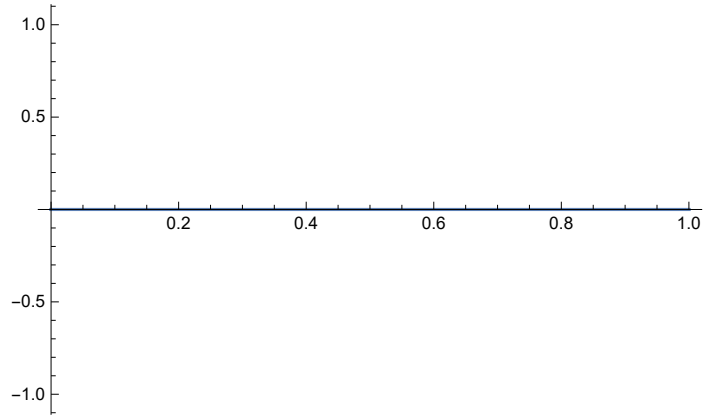

**(\*89th group coefficients r2^9r3^1\*)**

In[938]:= **Plot[Cf[9, 1, 14], {x, 0, 1}]**

[绘图](#)

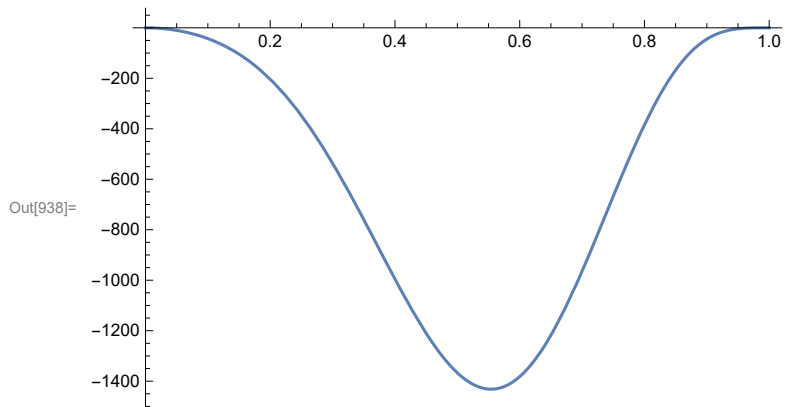

In[939]:= **Plot[Cf[9, 1, 13], {x, 0, 1}]**

[绘图](#)

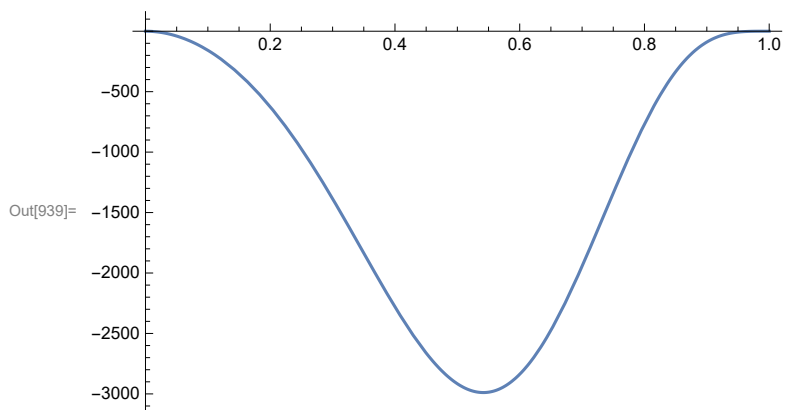



In[940]:= **Plot[Cf[9, 1, 12], {x, 0, 1}]**

[绘图](#)

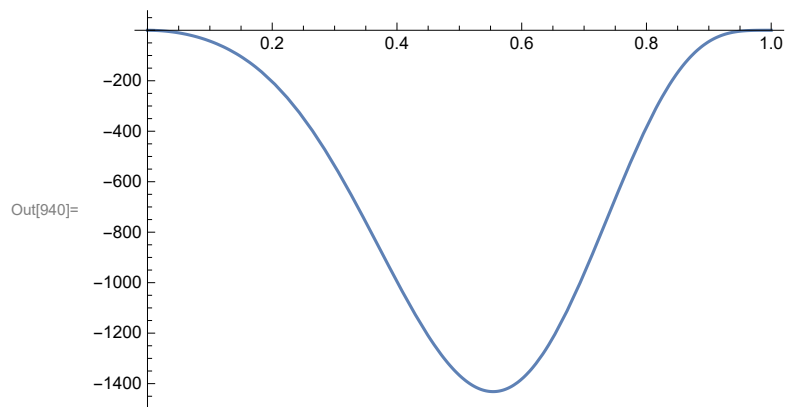

**Plot[Cf[9, 1, 11], {x, 0, 1}]**

[绘图](#)

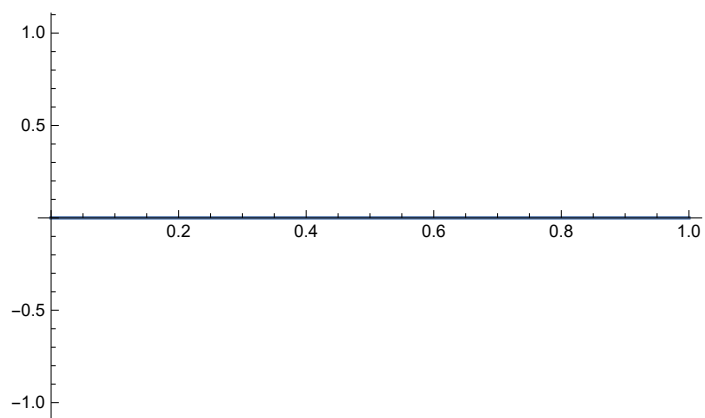

**Plot[Cf[9, 1, 10], {x, 0, 1}]**

[绘图](#)

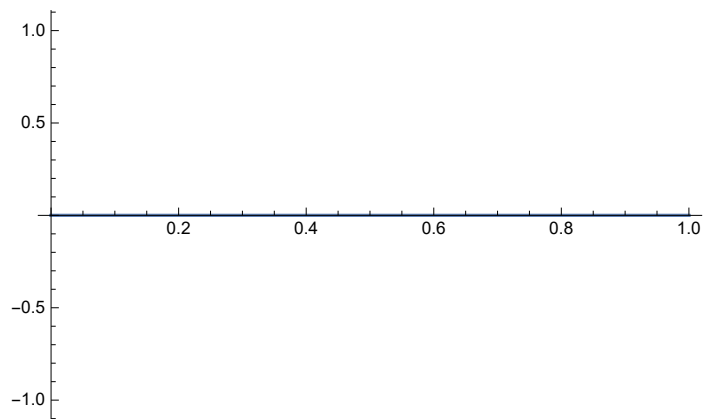

```
Plot[Cf[9, 1, 9], {x, 0, 1}]
```

[绘图](#)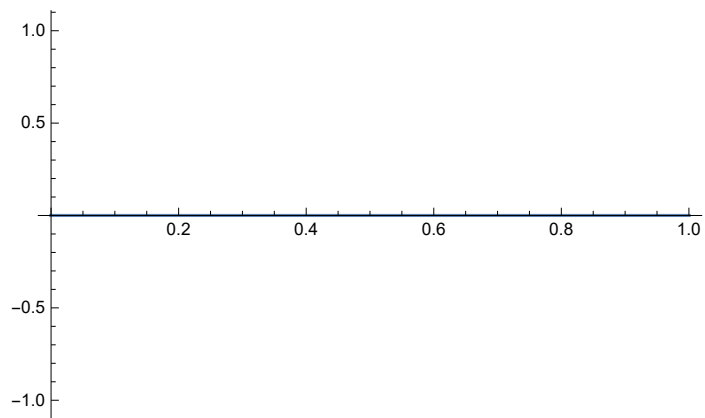

```
Plot[Cf[9, 1, 8], {x, 0, 1}]
```

[绘图](#)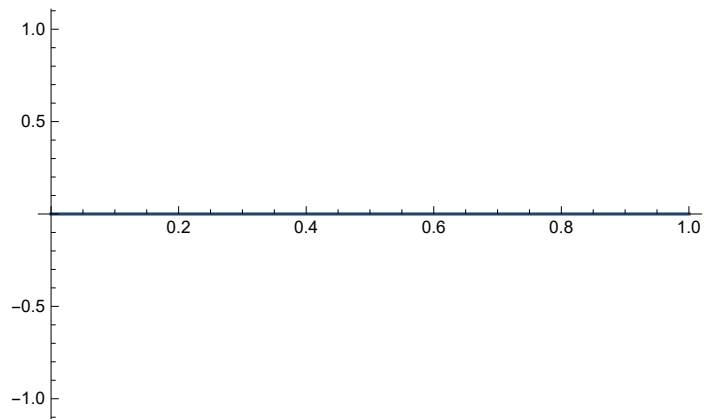

```
Plot[Cf[9, 1, 7], {x, 0, 1}]
```

[绘图](#)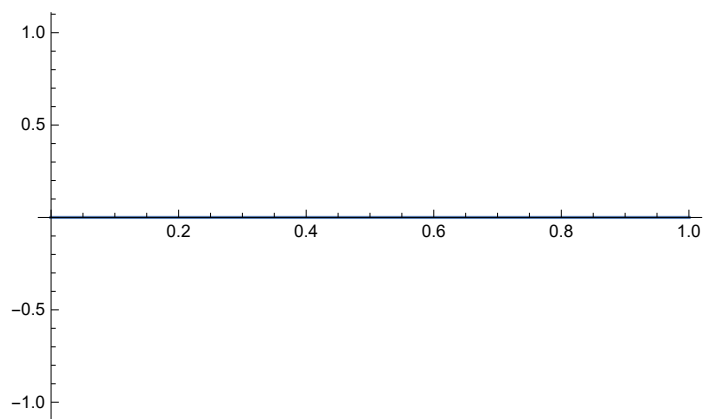

**Plot[Cf[9, 1, 6], {x, 0, 1}]**

[绘图](#)

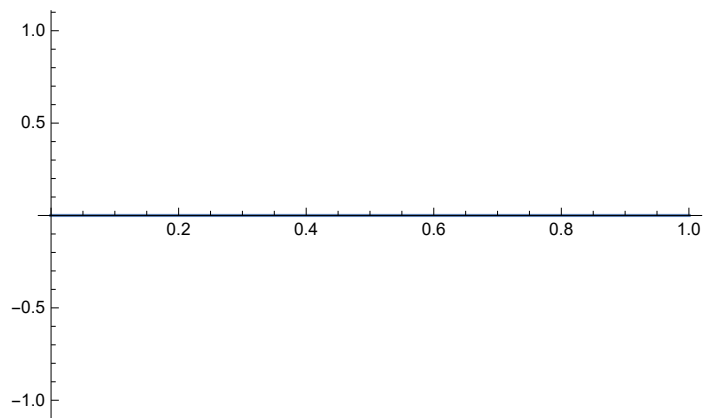

**Plot[Cf[9, 1, 5], {x, 0, 1}]**

[绘图](#)

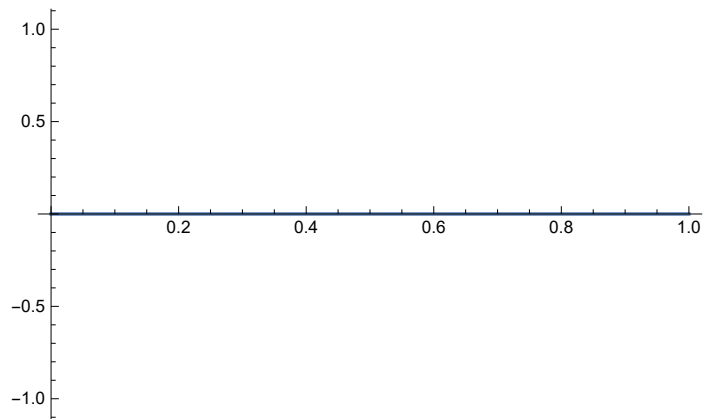

**Plot[Cf[9, 1, 4], {x, 0, 1}]**

[绘图](#)

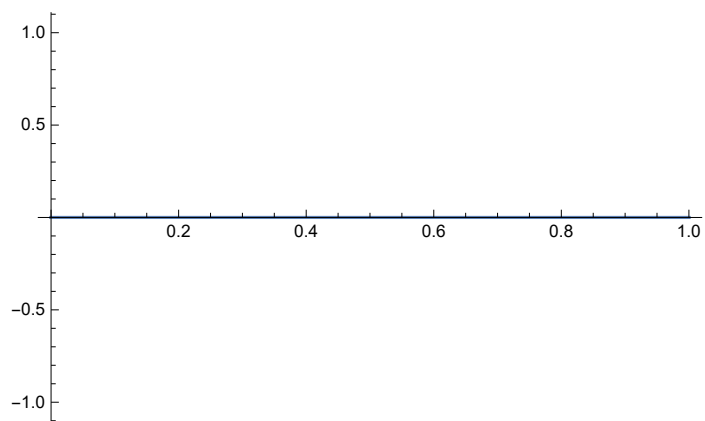

**Plot[Cf[9, 1, 3], {x, 0, 1}]**

[绘图](#)

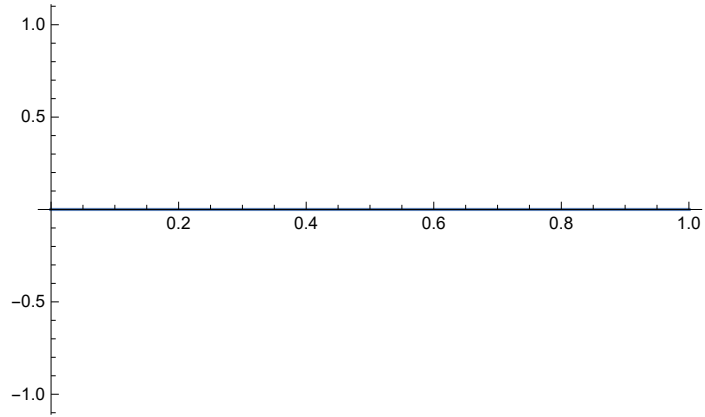

**Plot[Cf[9, 1, 2], {x, 0, 1}]**

[绘图](#)

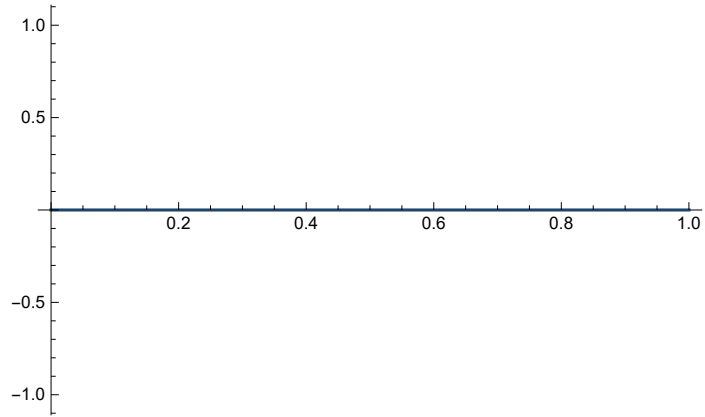

**Plot[Cf[9, 1, 1], {x, 0, 1}]**

[绘图](#)

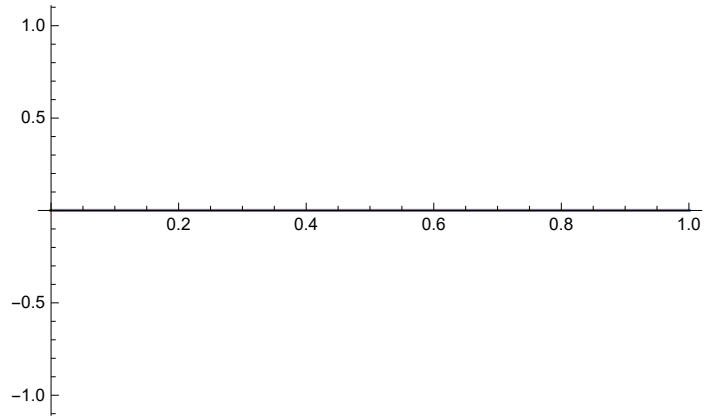

**Plot[Cf[9, 1, 0], {x, 0, 1}]**

[绘图](#)

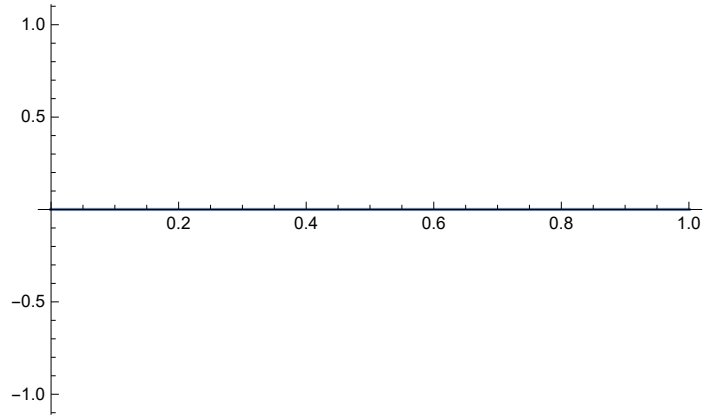

**(\*90th group coefficients r2^9r3^0\*)**

In[941]:= **Plot[Cf[9, 0, 14], {x, 0, 1}]**

[绘图](#)

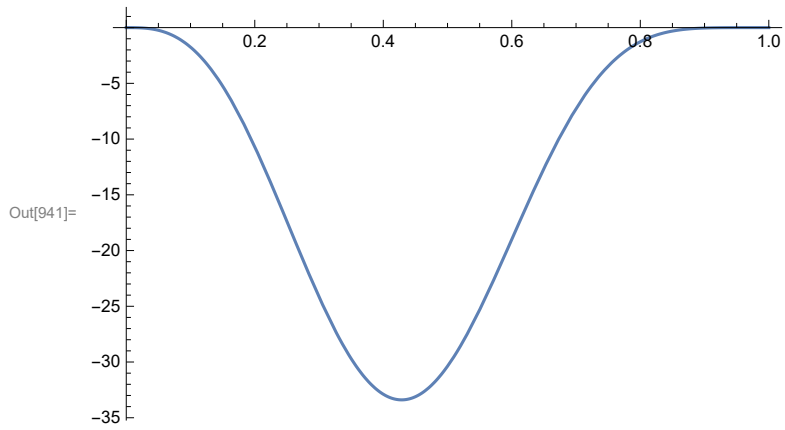

In[942]:= **Plot[Cf[9, 0, 13], {x, 0, 1}]**

[绘图](#)

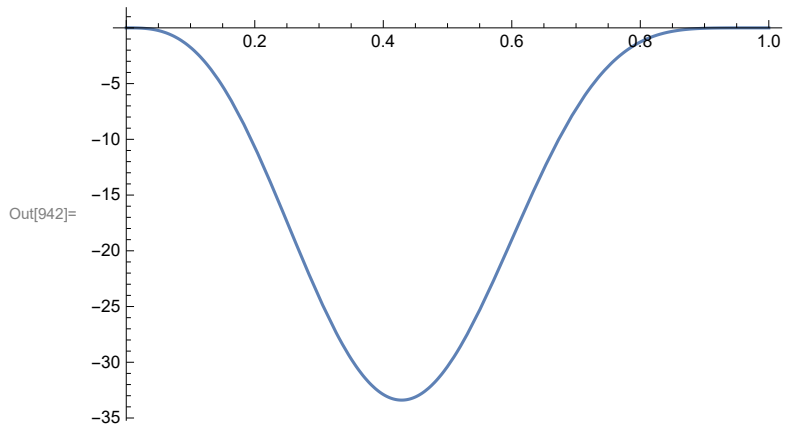

```
Plot[Cf[9, 0, 12], {x, 0, 1}]
```

[绘图](#)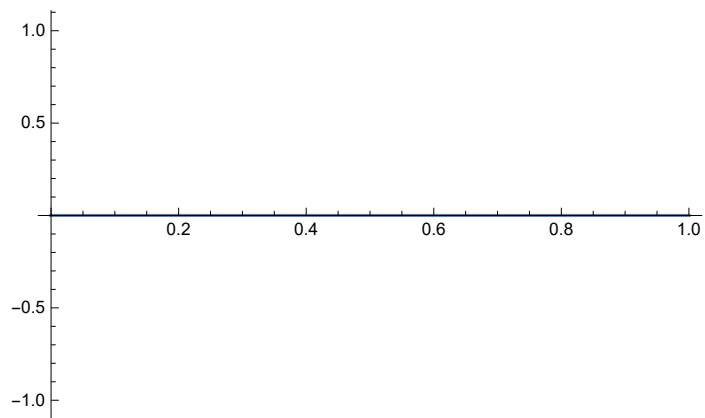

```
Plot[Cf[9, 0, 11], {x, 0, 1}]
```

[绘图](#)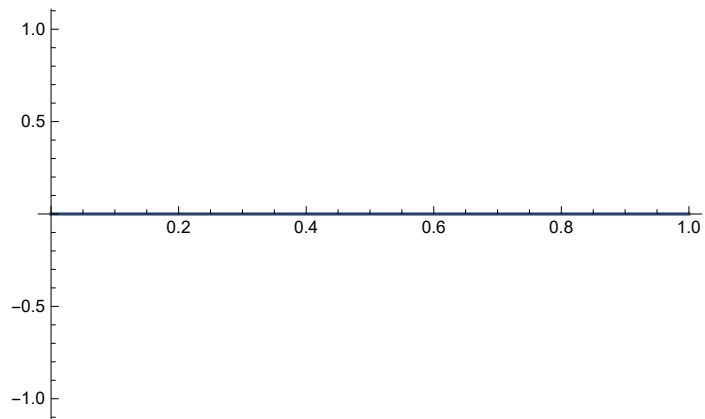

```
Plot[Cf[9, 0, 10], {x, 0, 1}]
```

[绘图](#)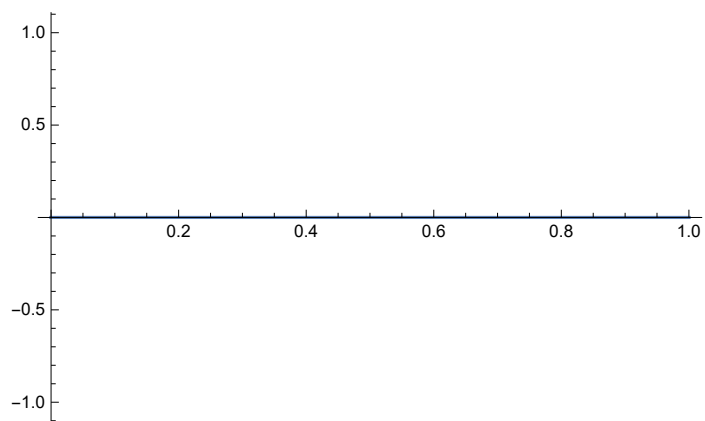

**Plot[Cf[9, 0, 9], {x, 0, 1}]**

[绘图](#)

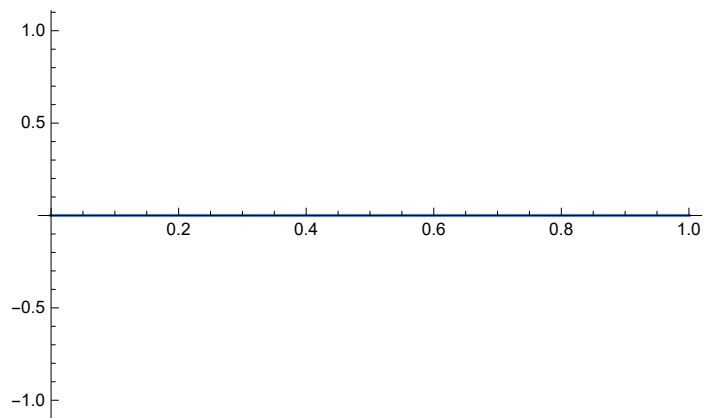

**Plot[Cf[9, 0, 8], {x, 0, 1}]**

[绘图](#)

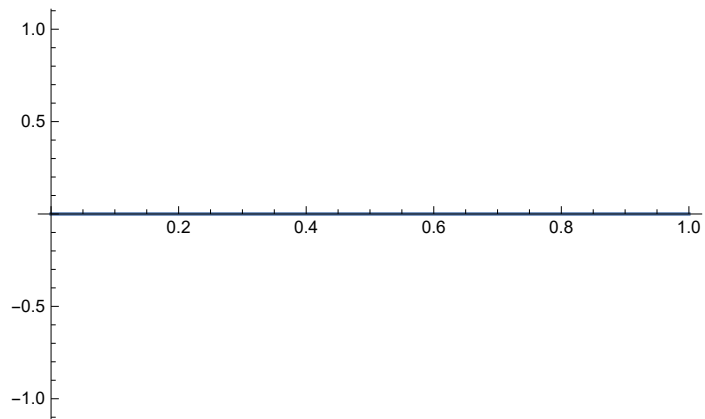

**Plot[Cf[9, 0, 7], {x, 0, 1}]**

[绘图](#)

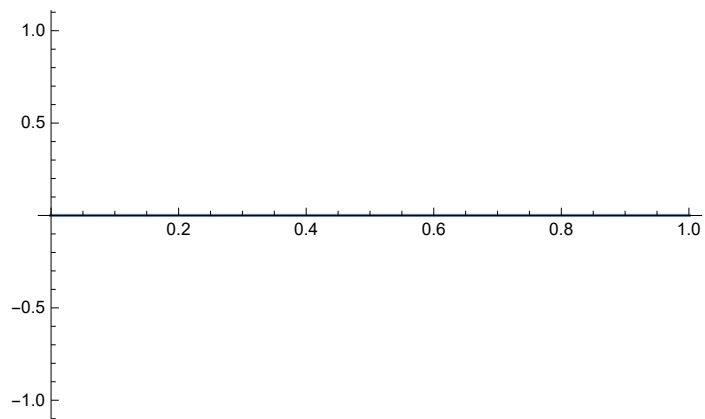

**Plot[Cf[9, 0, 6], {x, 0, 1}]**

[绘图](#)

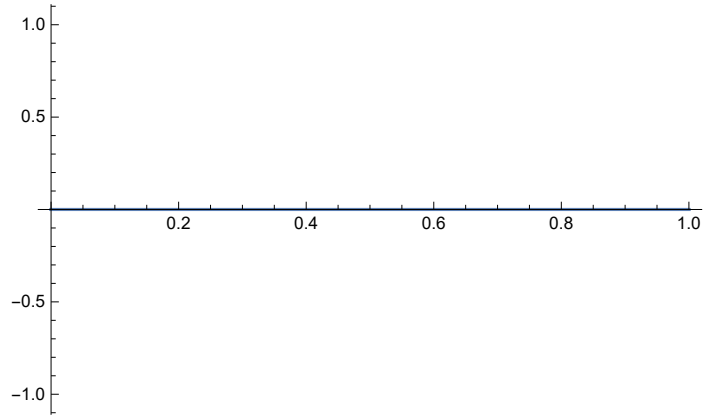

**Plot[Cf[9, 0, 5], {x, 0, 1}]**

[绘图](#)

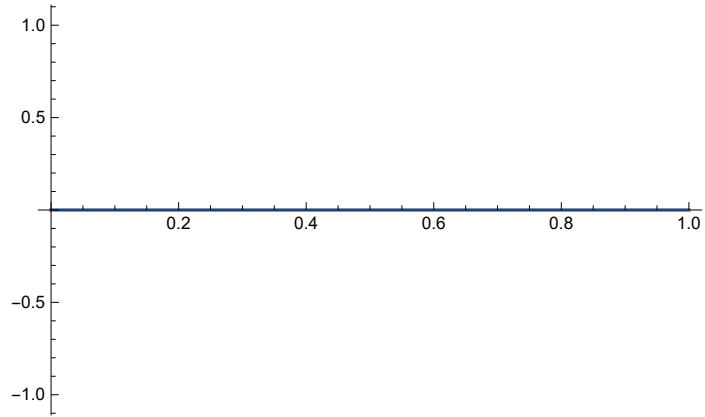

**Plot[Cf[9, 0, 4], {x, 0, 1}]**

[绘图](#)

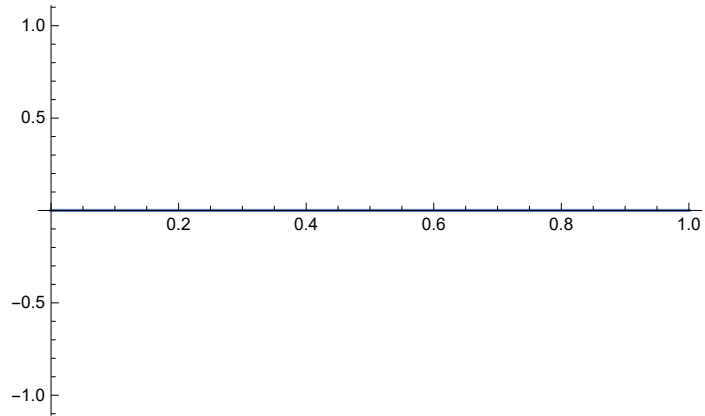



**Plot[Cf[9, 0, 3], {x, 0, 1}]**

[绘图](#)

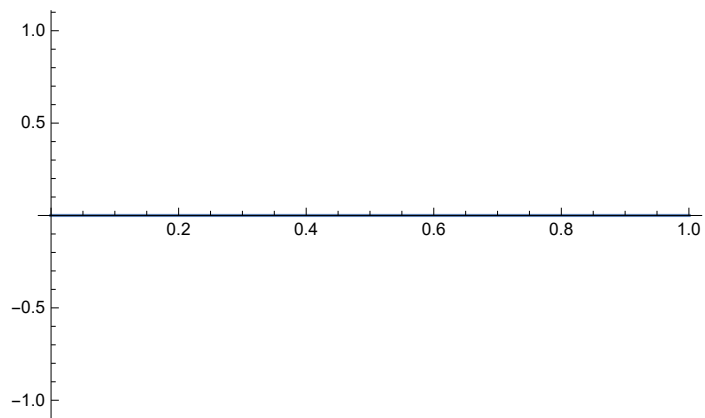

**Plot[Cf[9, 0, 2], {x, 0, 1}]**

[绘图](#)

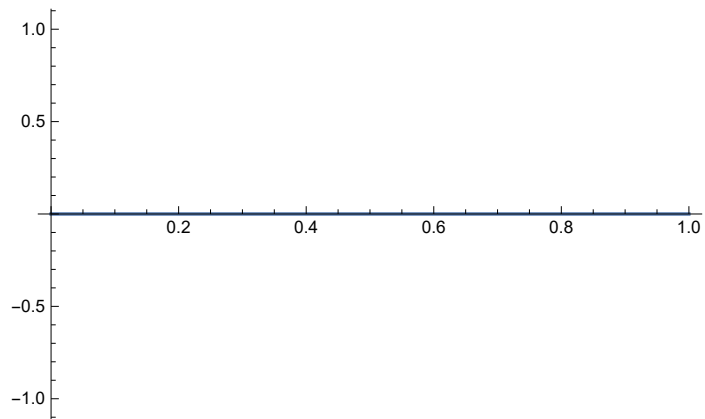

**Plot[Cf[9, 0, 1], {x, 0, 1}]**

[绘图](#)

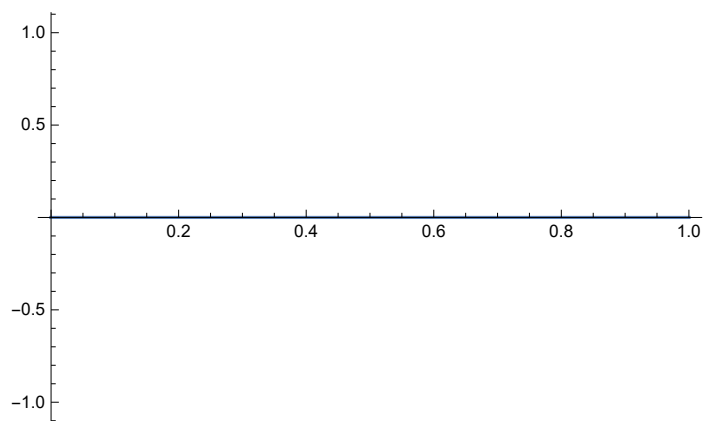

**Plot[Cf[9, 0, 0], {x, 0, 1}]**

[绘图](#)

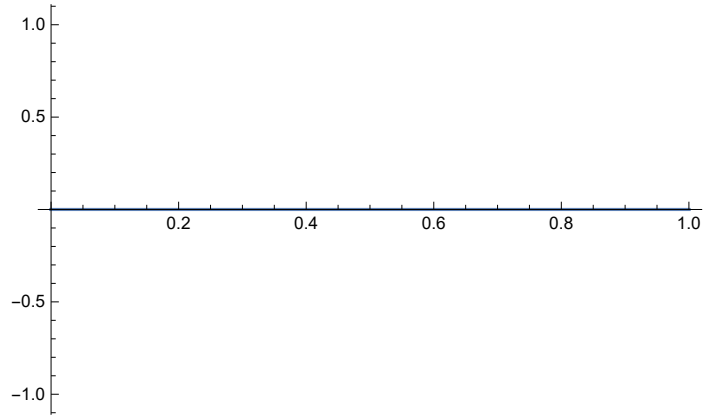

**(\*91th group coefficients r2^8r3^14\*)**

**Plot[Cf[8, 14, 14], {x, 0, 1}]**

[绘图](#)

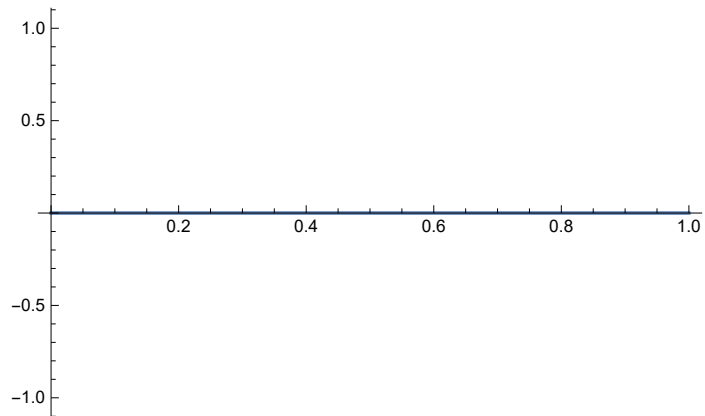

In[943]:= **Plot[Cf[8, 14, 13], {x, 0, 1}]**

[绘图](#)

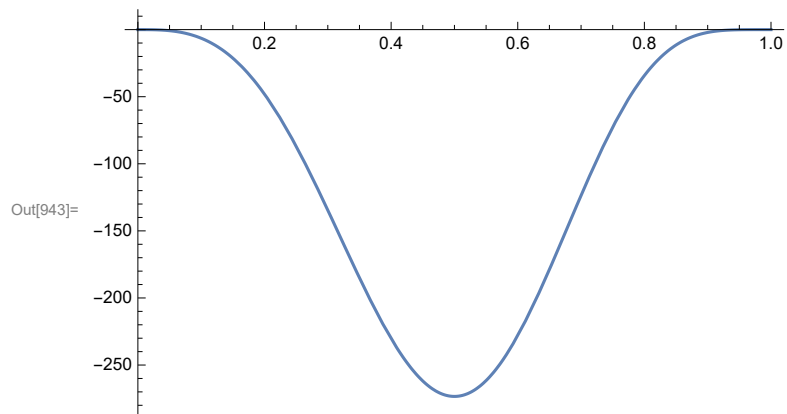

Out[943]=

In[944]:= **Plot[Cf[8, 14, 12], {x, 0, 1}]**

[绘图](#)

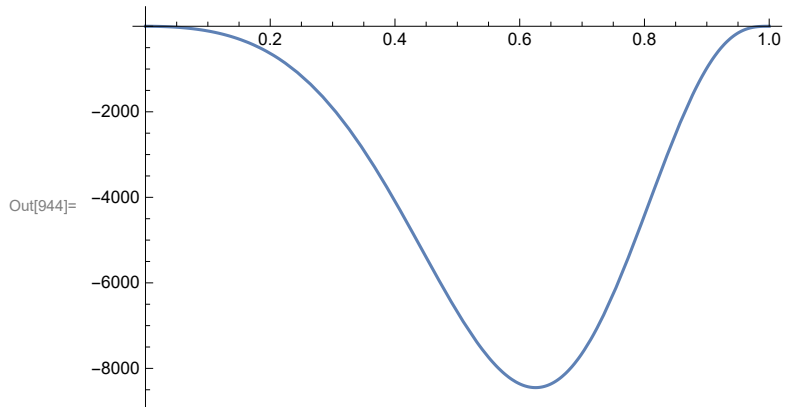

In[946]:= **Plot[Cf[8, 14, 11], {x, 0, 1}]**

[绘图](#)

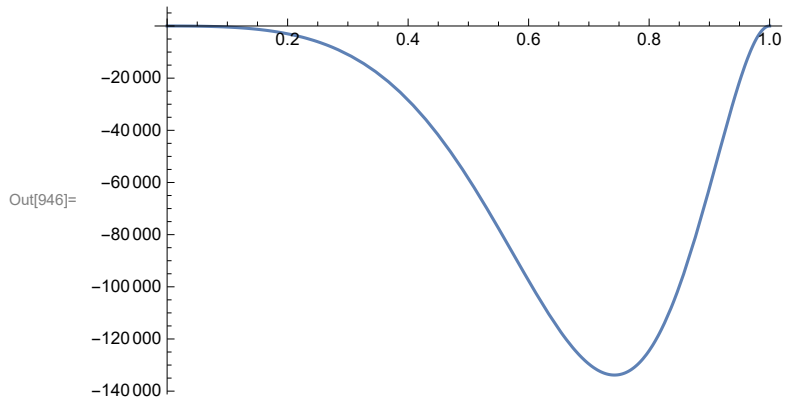

In[947]:= **Plot[Cf[8, 14, 10], {x, 0, 1}]**

[绘图](#)

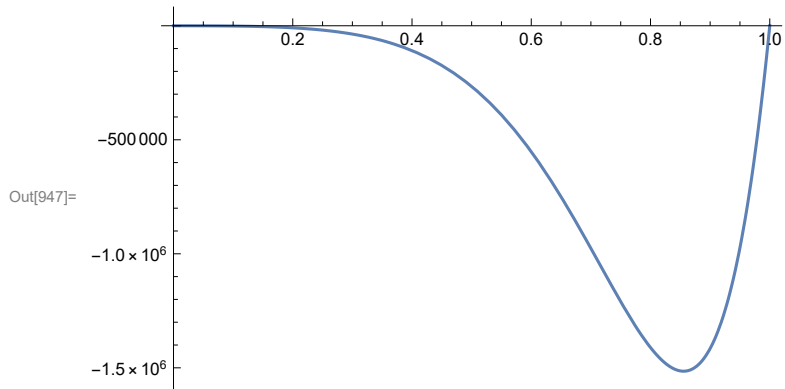

In[948]:= **Plot[Cf[8, 14, 9], {x, 0, 1}]**

[绘图](#)

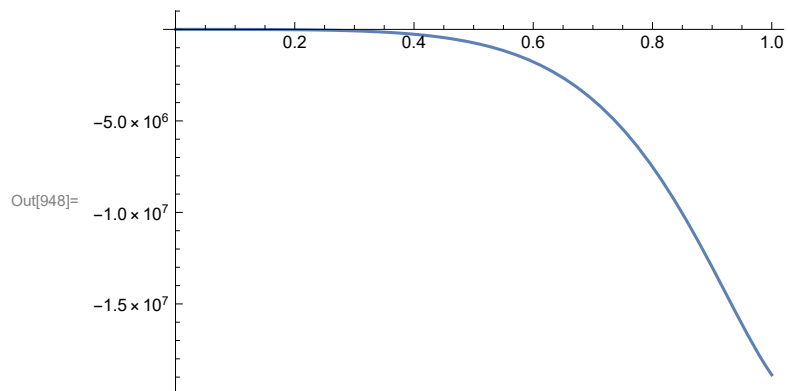

In[949]:= **Plot[Cf[8, 14, 8], {x, 0, 1}]**

[绘图](#)

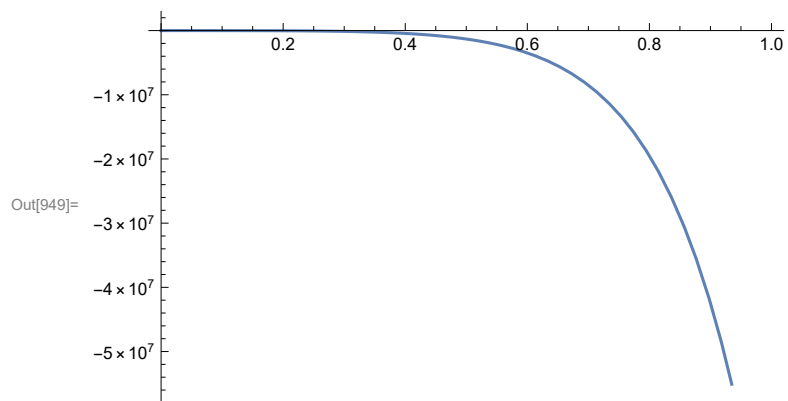

In[950]:= **Plot[Cf[8, 14, 7], {x, 0, 1}]**

[绘图](#)

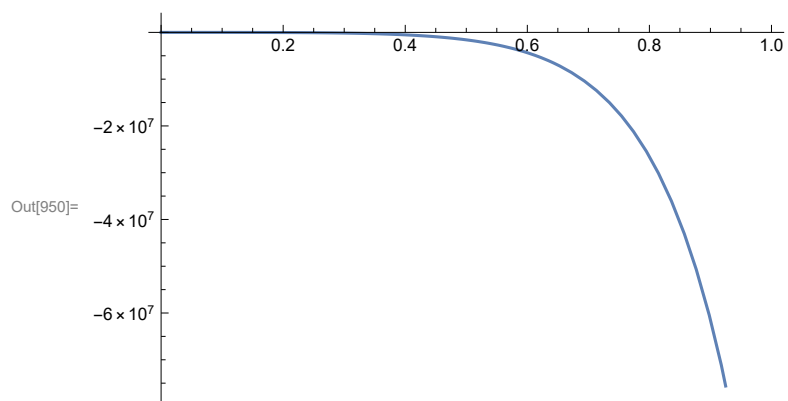

In[951]:= **Plot[Cf[8, 14, 6], {x, 0, 1}]**

[绘图](#)

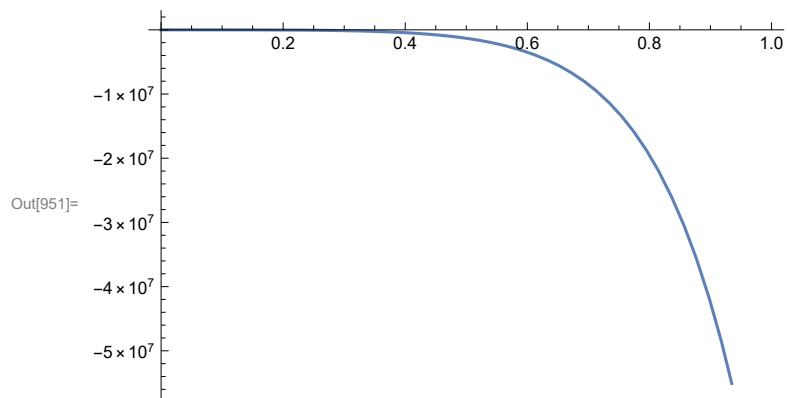

In[952]:= **Plot[Cf[8, 14, 5], {x, 0, 1}]**

[绘图](#)

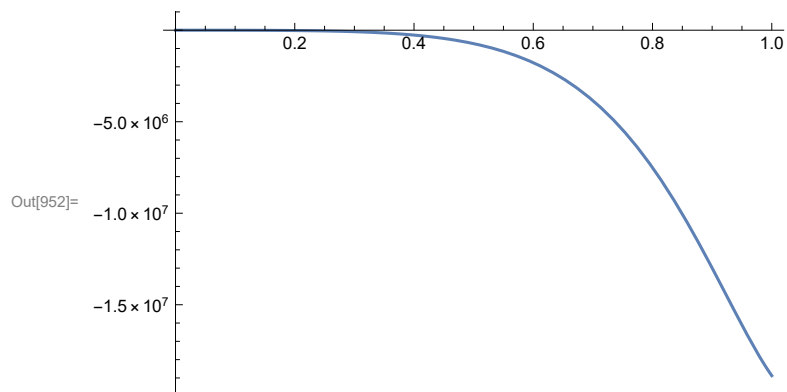

In[953]:= **Plot[Cf[8, 14, 4], {x, 0, 1}]**

[绘图](#)

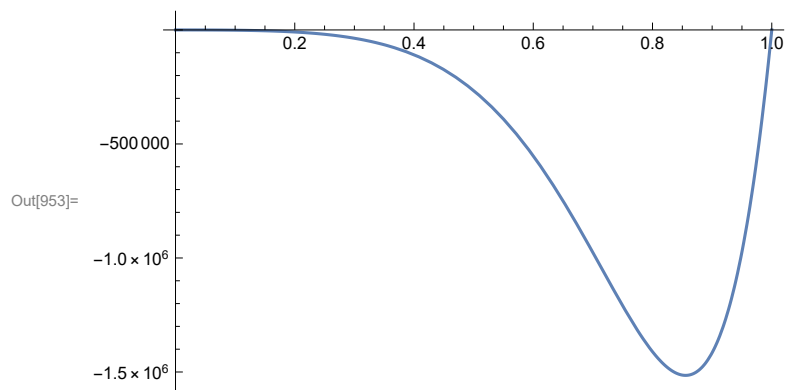

In[954]:= **Plot[Cf[8, 14, 3], {x, 0, 1}]**

[绘图](#)

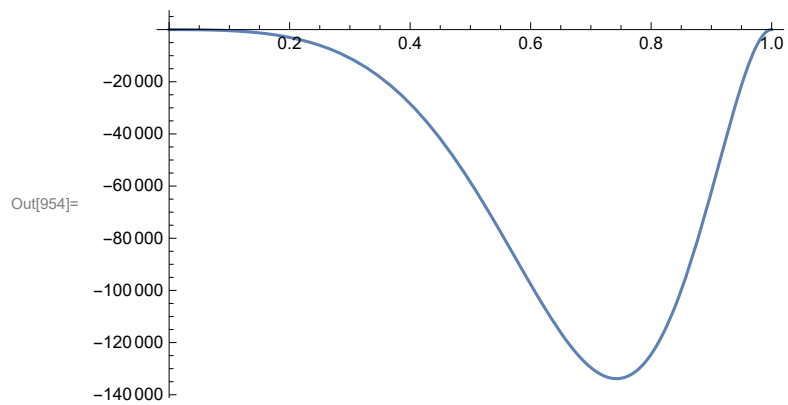

In[955]:= **Plot[Cf[8, 14, 2], {x, 0, 1}]**

[绘图](#)

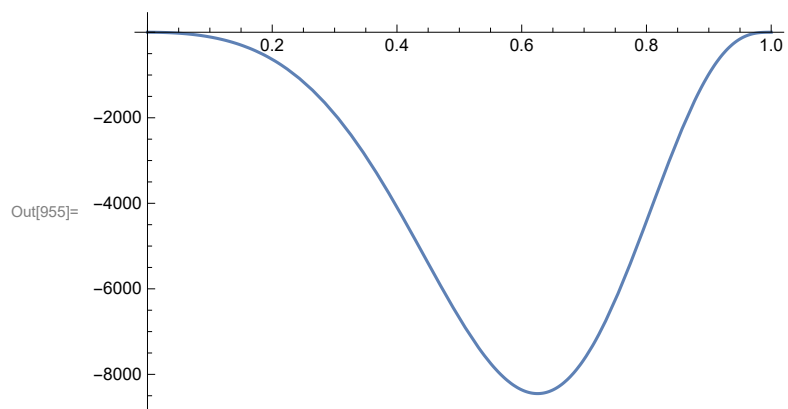

In[956]:= **Plot[Cf[8, 14, 1], {x, 0, 1}]**

[绘图](#)

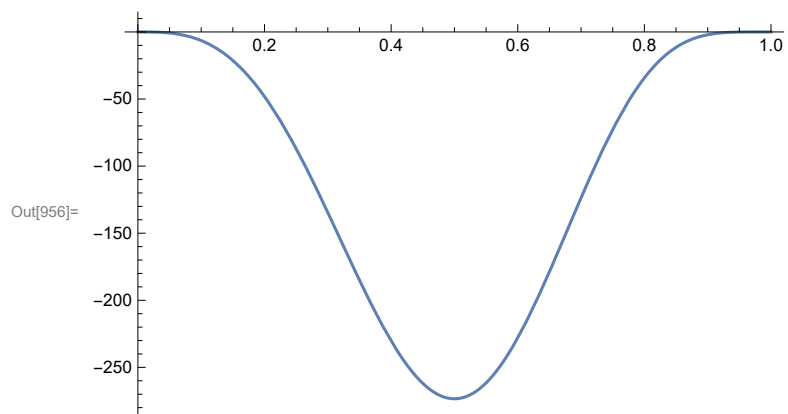

**Plot[Cf[8, 14, 0], {x, 0, 1}]**

[绘图](#)

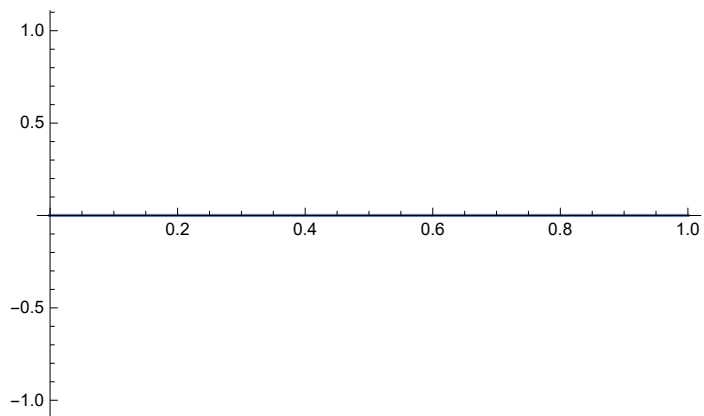

**(\*92th group coefficients r2^8r3^13\*)**

In[957]:= **Plot[Cf[8, 13, 14], {x, 0, 1}]**

[绘图](#)

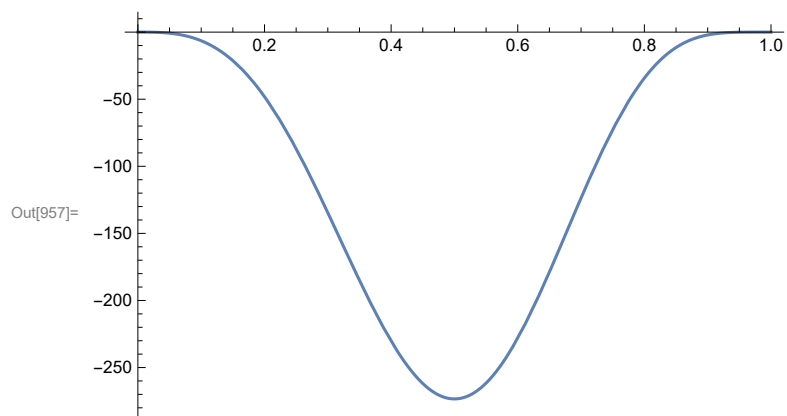

In[958]:= **Plot[Cf[8, 13, 13], {x, 0, 1}]**

[绘图](#)

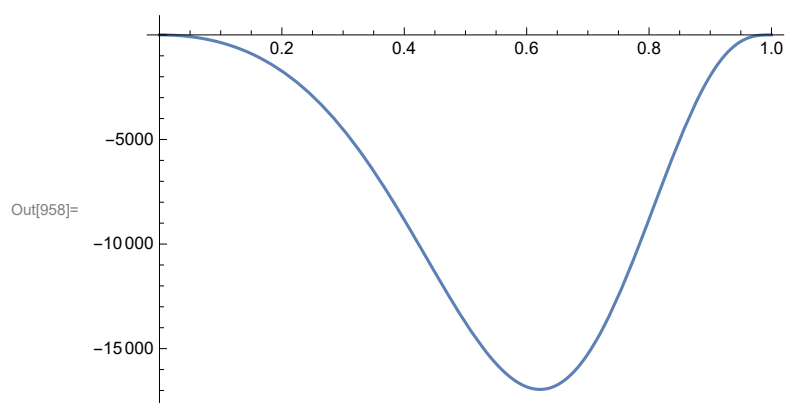

In[959]:= **Plot[Cf[8, 13, 12], {x, 0, 1}]**

[绘图](#)

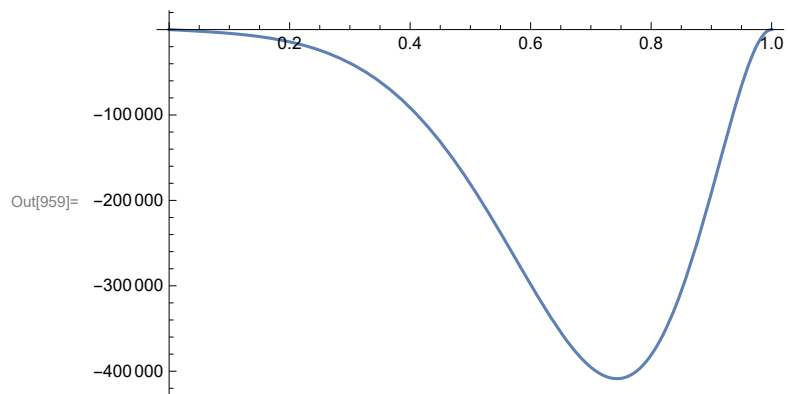

In[960]:= **Plot[Cf[8, 13, 11], {x, 0, 1}]**

[绘图](#)

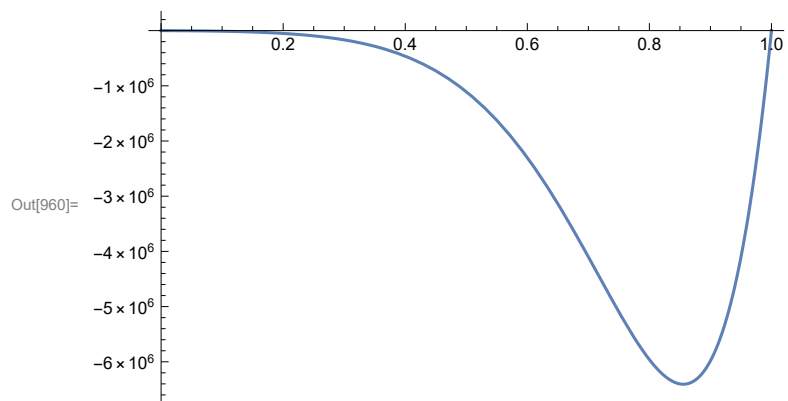

In[961]:= **Plot[Cf[8, 13, 10], {x, 0, 1}]**

[绘图](#)

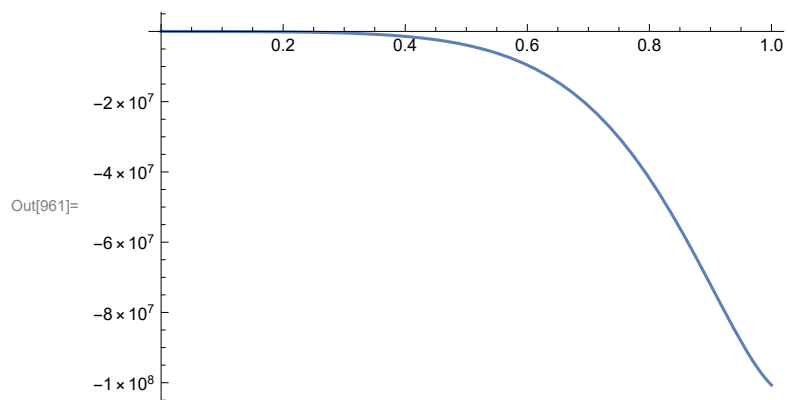



In[962]:= **Plot[Cf[8, 13, 9], {x, 0, 1}]**

[绘图](#)

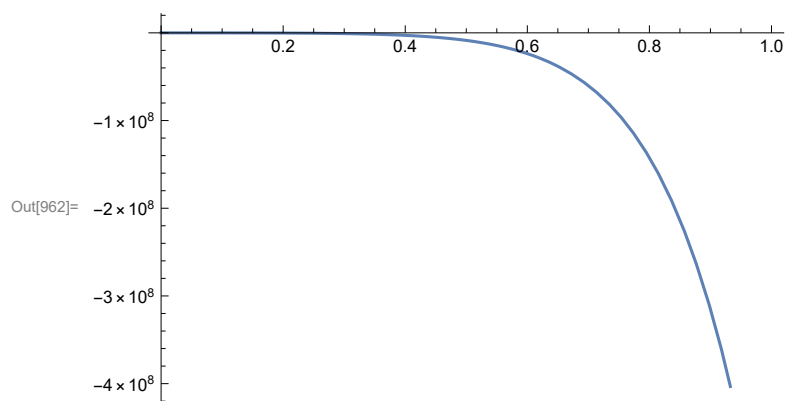

In[963]:= **Plot[Cf[8, 13, 8], {x, 0, 1}]**

[绘图](#)

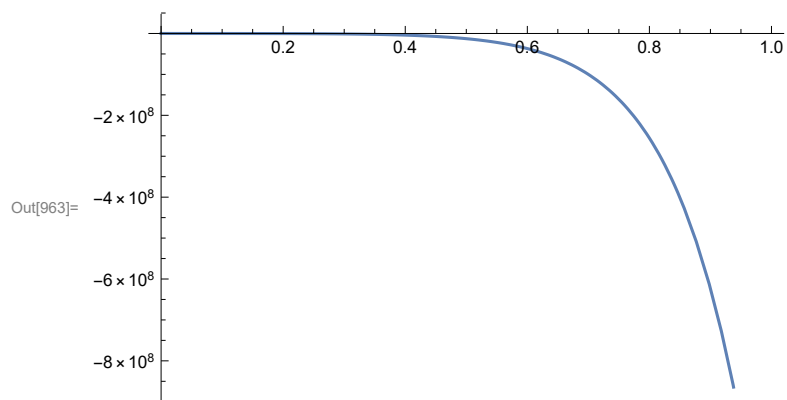

In[964]:= **Plot[Cf[8, 13, 7], {x, 0, 1}]**

[绘图](#)

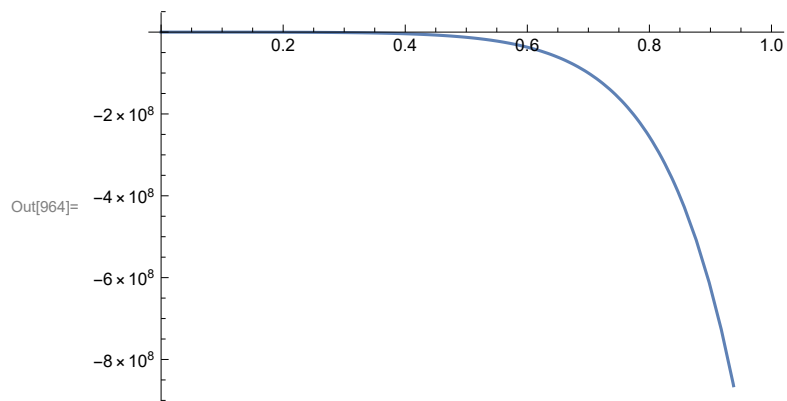

In[965]:= **Plot[Cf[8, 13, 6], {x, 0, 1}]**

[绘图](#)

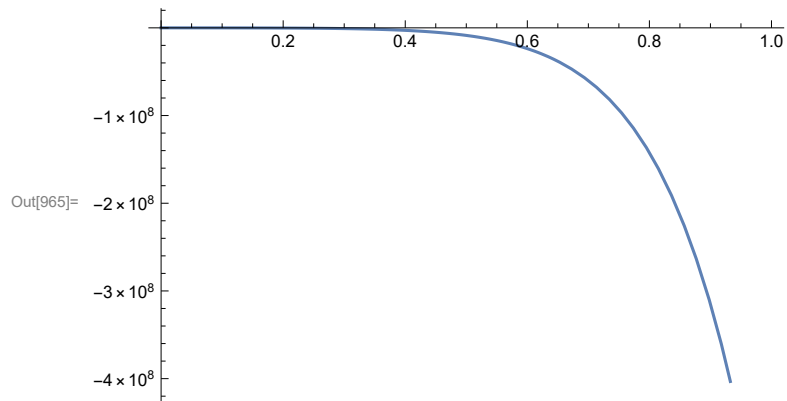

In[966]:= **Plot[Cf[8, 13, 5], {x, 0, 1}]**

[绘图](#)

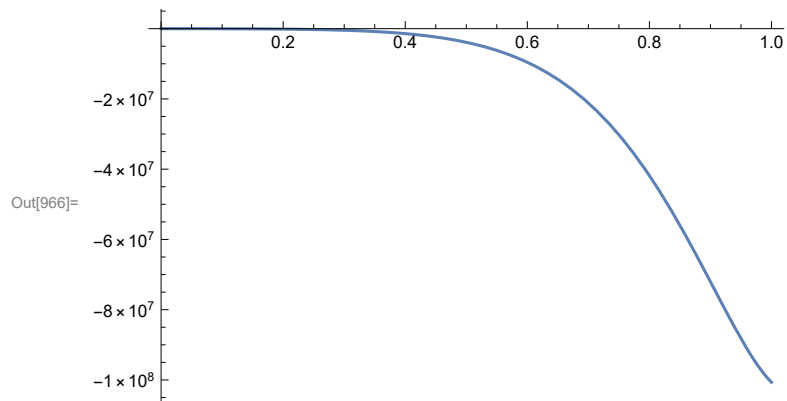

In[967]:= **Plot[Cf[8, 13, 4], {x, 0, 1}]**

[绘图](#)

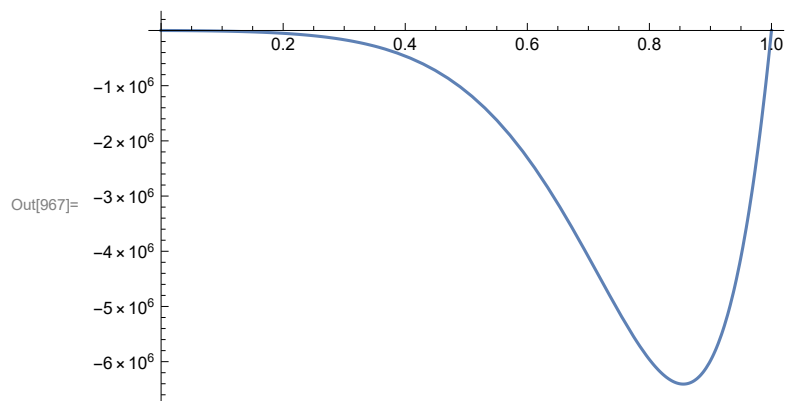

In[968]:= **Plot[Cf[8, 13, 3], {x, 0, 1}]**

[绘图](#)

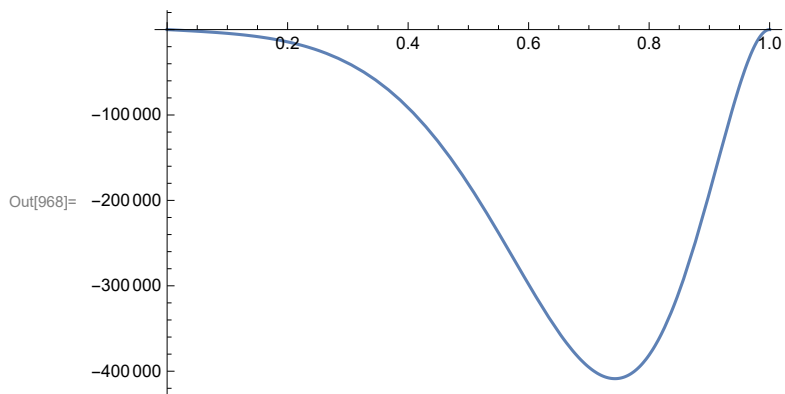

In[969]:= **Plot[Cf[8, 13, 2], {x, 0, 1}]**

[绘图](#)

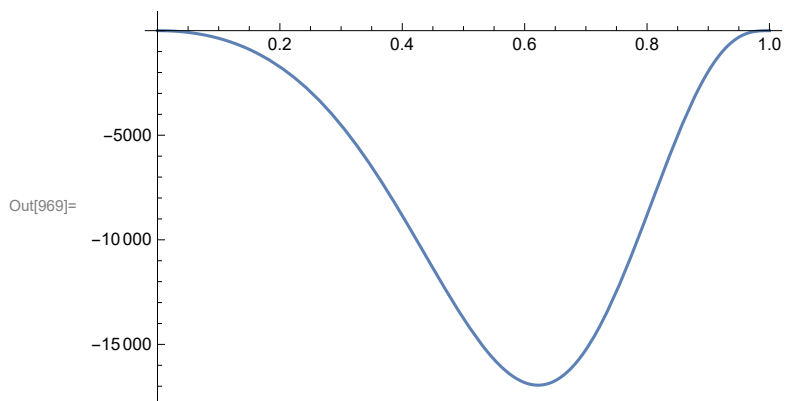

In[970]:= **Plot[Cf[8, 13, 1], {x, 0, 1}]**

[绘图](#)

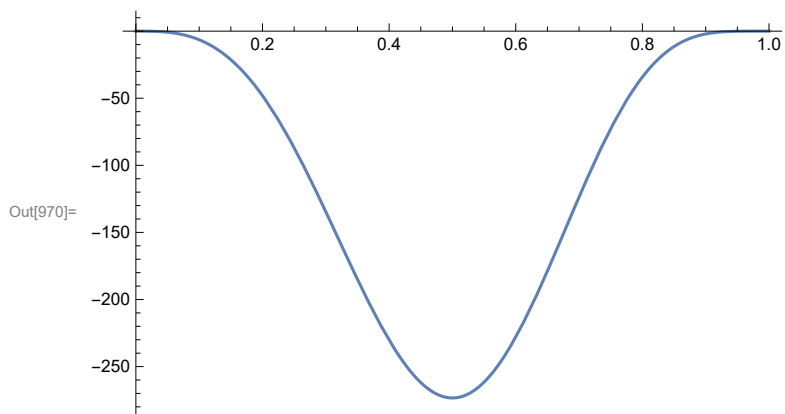

**Plot[Cf[8, 13, 0], {x, 0, 1}]**

[绘图](#)

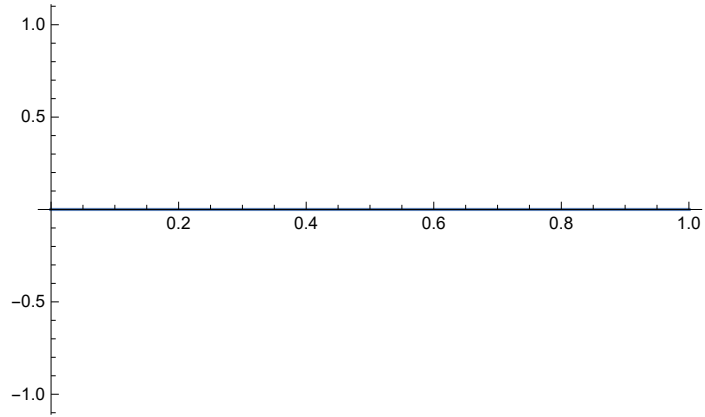

**(\*93th group coefficients r2^8r3^12\*)**

In[971]:= **Plot[Cf[8, 12, 14], {x, 0, 1}]**

[绘图](#)

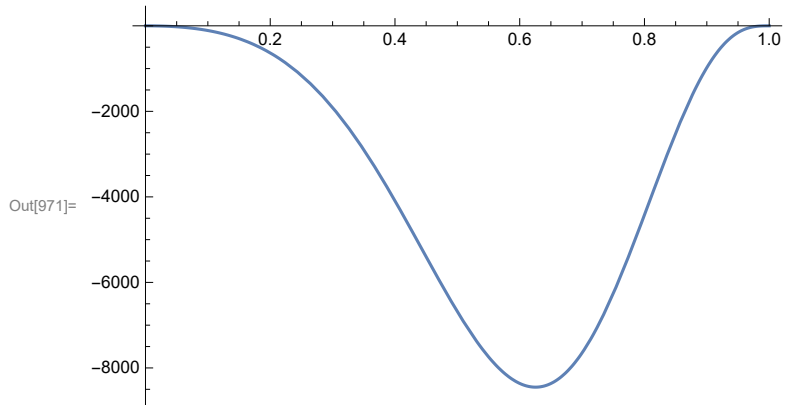

In[972]:= **Plot[Cf[8, 12, 13], {x, 0, 1}]**

[绘图](#)

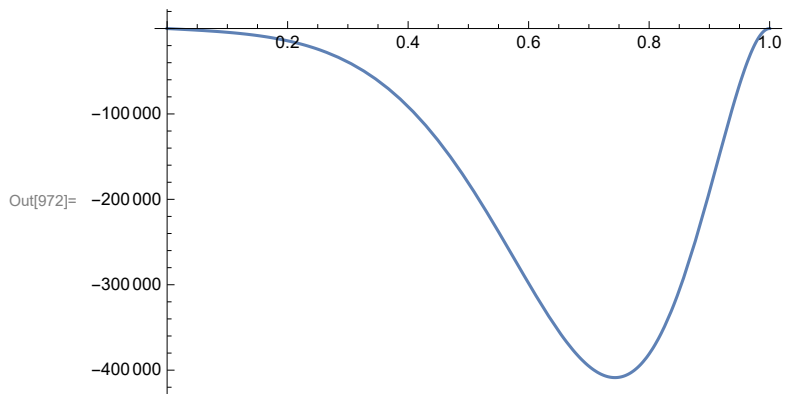

In[973]:= **Plot[Cf[8, 12, 12], {x, 0, 1}]**

[绘图](#)

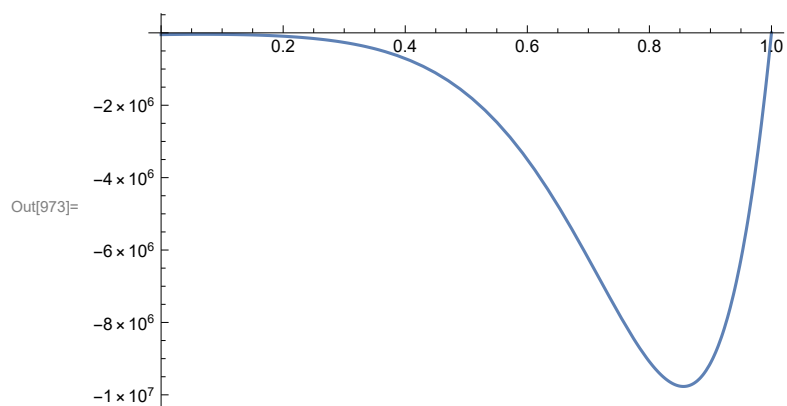

In[974]:= **Plot[Cf[8, 12, 11], {x, 0, 1}]**

[绘图](#)

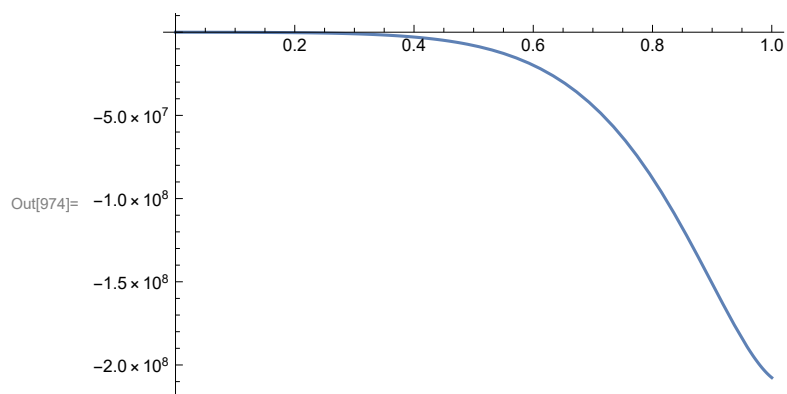

In[975]:= **Plot[Cf[8, 12, 10], {x, 0, 1}]**

[绘图](#)

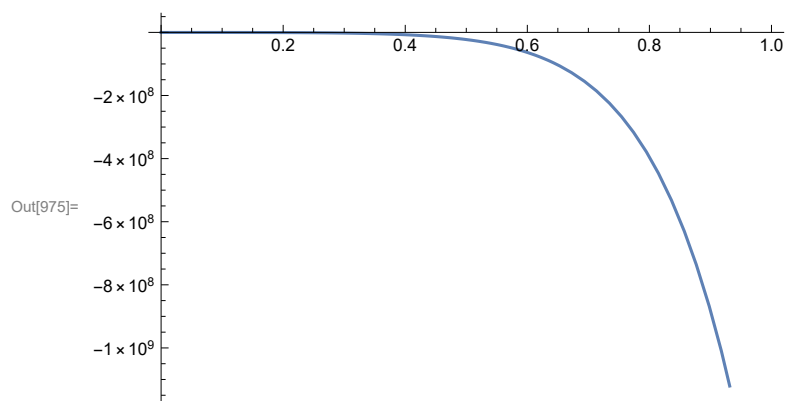

In[976]:= **Plot[Cf[8, 12, 9], {x, 0, 1}]**

[绘图](#)

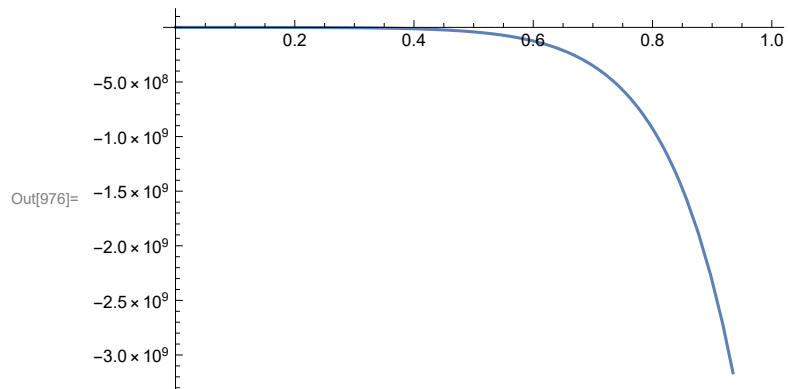

In[977]:= **Plot[Cf[8, 12, 8], {x, 0, 1}]**

[绘图](#)

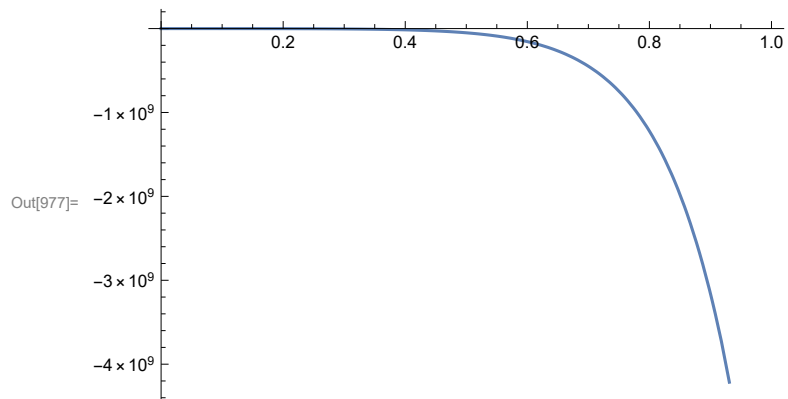

In[978]:= **Plot[Cf[8, 12, 7], {x, 0, 1}]**

[绘图](#)

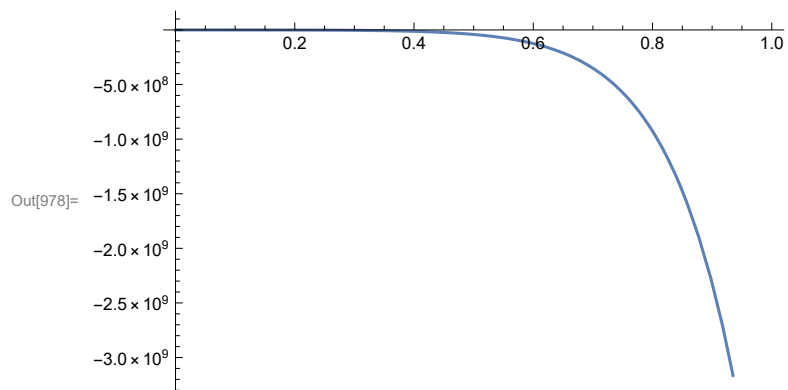

In[979]:= **Plot[Cf[8, 12, 6], {x, 0, 1}]**

[绘图](#)

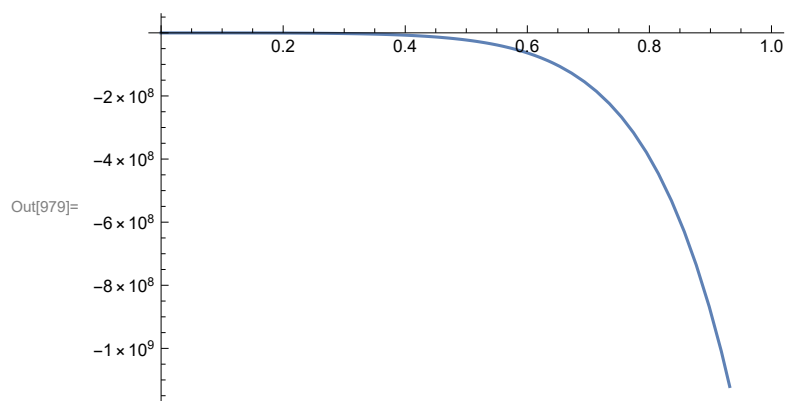

In[980]:= **Plot[Cf[8, 12, 5], {x, 0, 1}]**

[绘图](#)

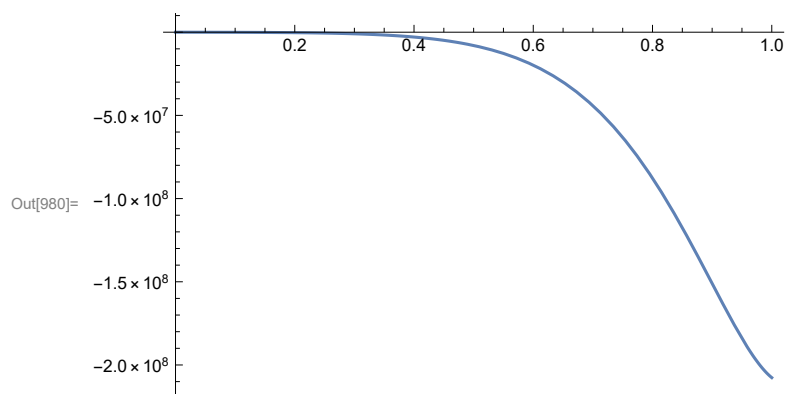

In[981]:= **Plot[Cf[8, 12, 4], {x, 0, 1}]**

[绘图](#)

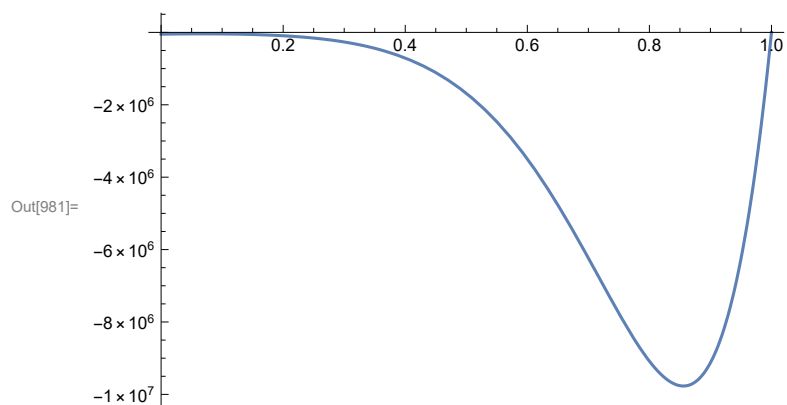

In[982]:= **Plot[Cf[8, 12, 3], {x, 0, 1}]**

[绘图](#)

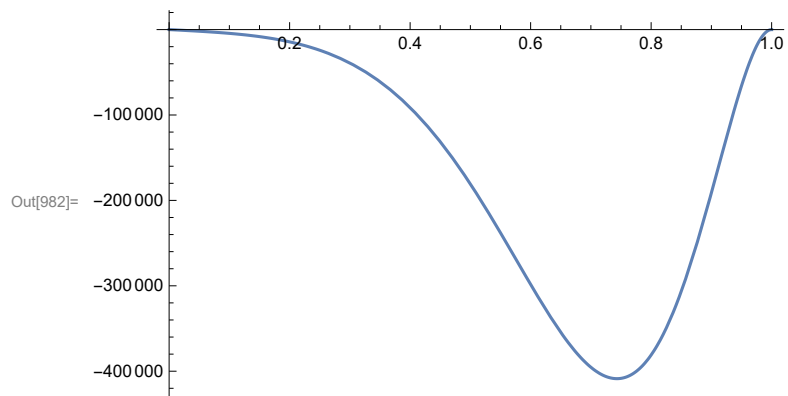

In[983]:= **Plot[Cf[8, 12, 2], {x, 0, 1}]**

[绘图](#)

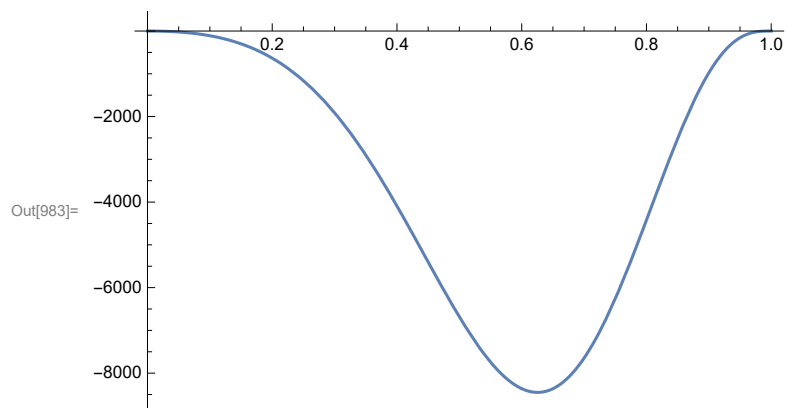

**Plot[Cf[8, 12, 1], {x, 0, 1}]**

[绘图](#)

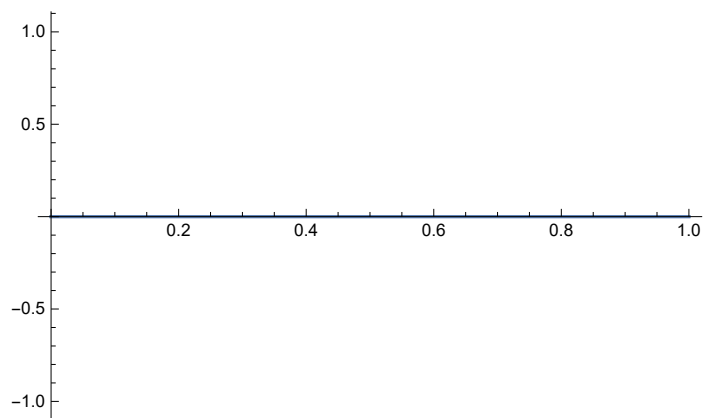



**Plot[Cf[8, 12, 0], {x, 0, 1}]**

[绘图](#)

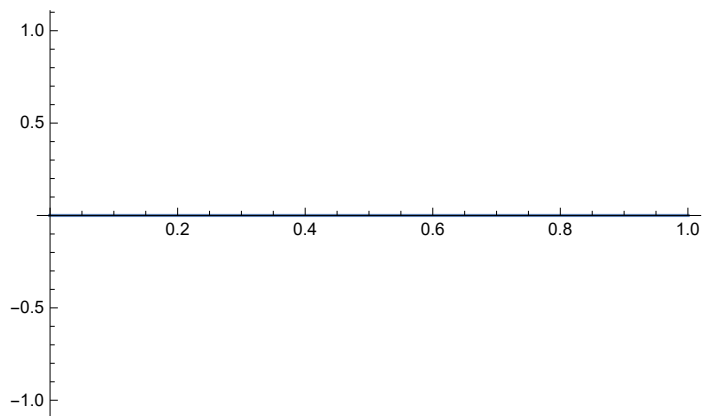

**(\*94th group coefficients r2^8r3^11\*)**

In[984]:= **Plot[Cf[8, 11, 14], {x, 0, 1}]**

[绘图](#)

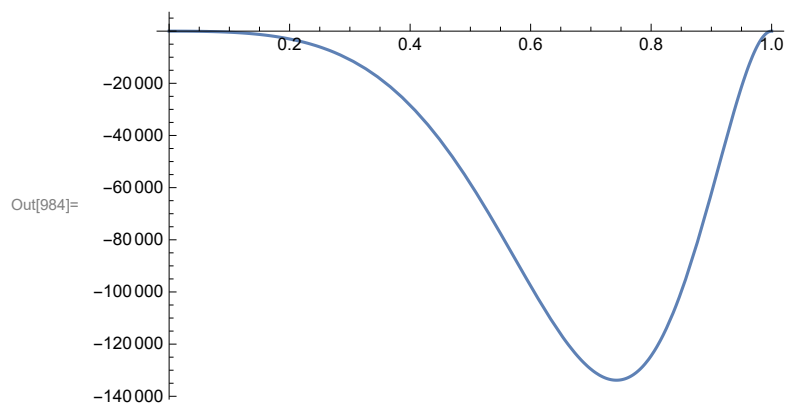

In[985]:= **Plot[Cf[8, 11, 13], {x, 0, 1}]**

[绘图](#)

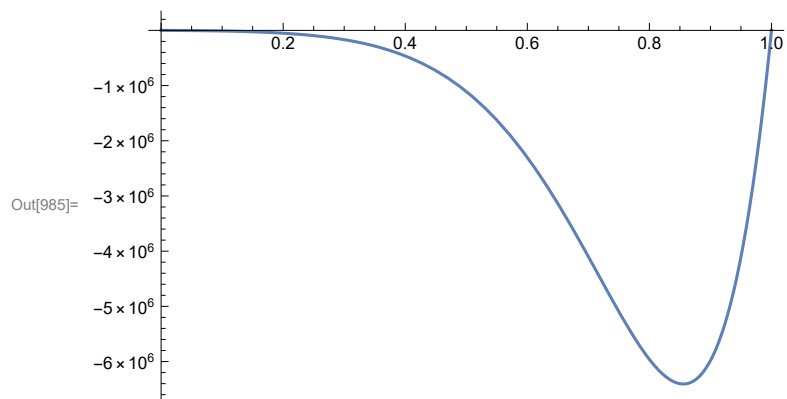

In[986]:= **Plot[Cf[8, 11, 12], {x, 0, 1}]**

[绘图](#)

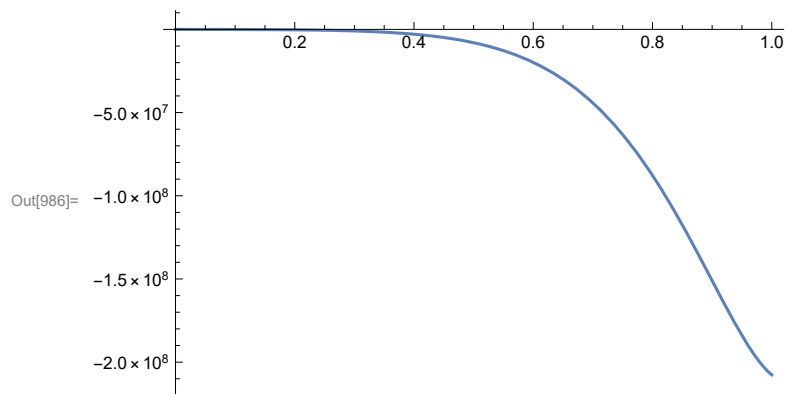

In[987]:= **Plot[Cf[8, 11, 11], {x, 0, 1}]**

[绘图](#)

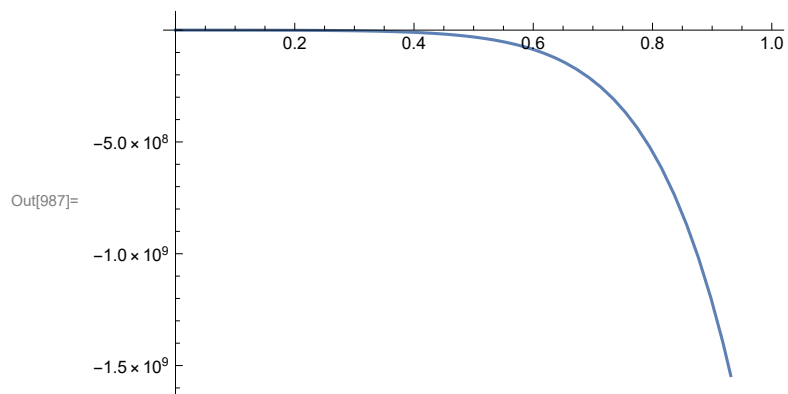

In[988]:= **Plot[Cf[8, 11, 10], {x, 0, 1}]**

[绘图](#)

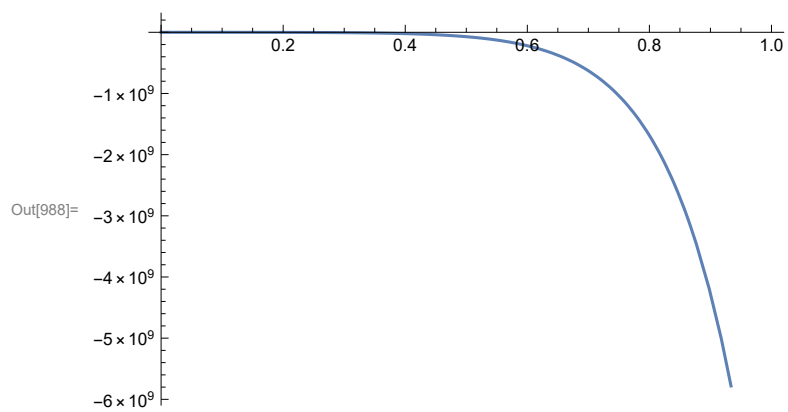

In[989]:= **Plot[Cf[8, 11, 9], {x, 0, 1}]**

[绘图](#)

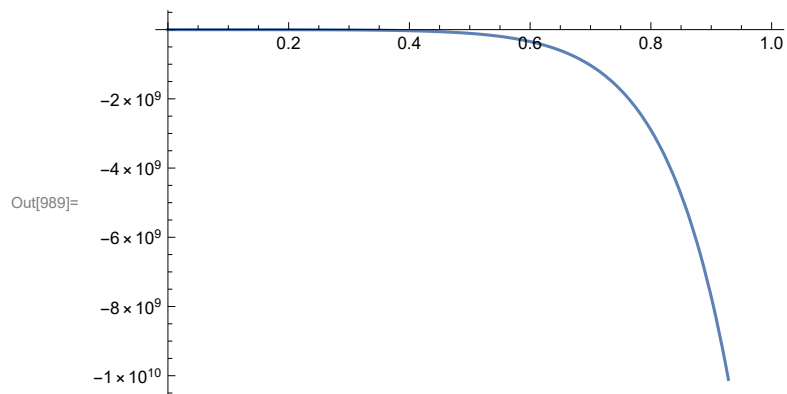

In[990]:= **Plot[Cf[8, 11, 8], {x, 0, 1}]**

[绘图](#)

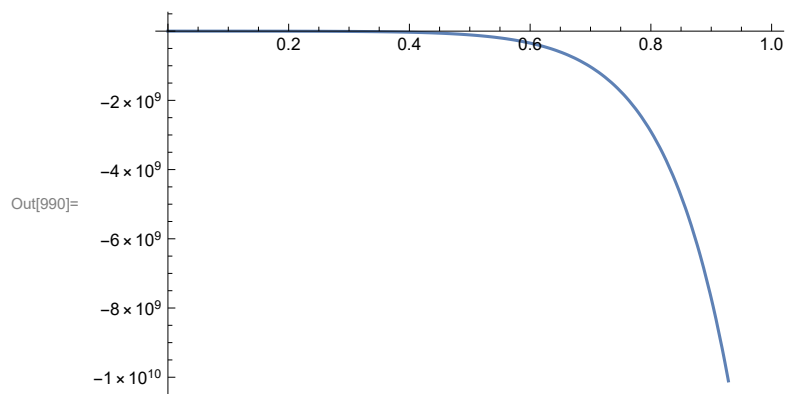

In[991]:= **Plot[Cf[8, 11, 7], {x, 0, 1}]**

[绘图](#)

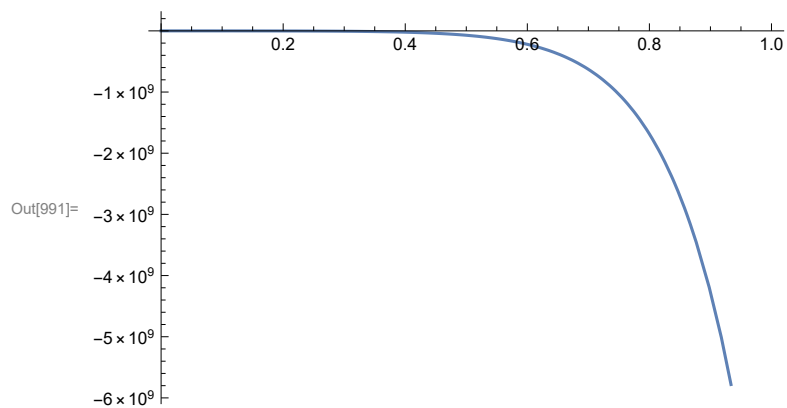

In[992]:= **Plot[Cf[8, 11, 6], {x, 0, 1}]**

[绘图](#)

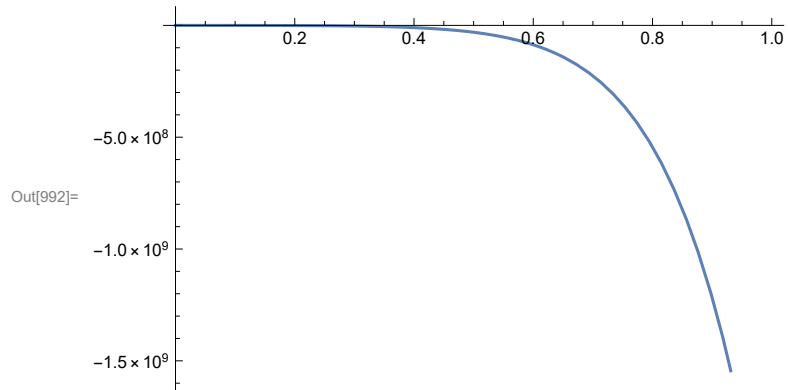

In[993]:= **Plot[Cf[8, 11, 5], {x, 0, 1}]**

[绘图](#)

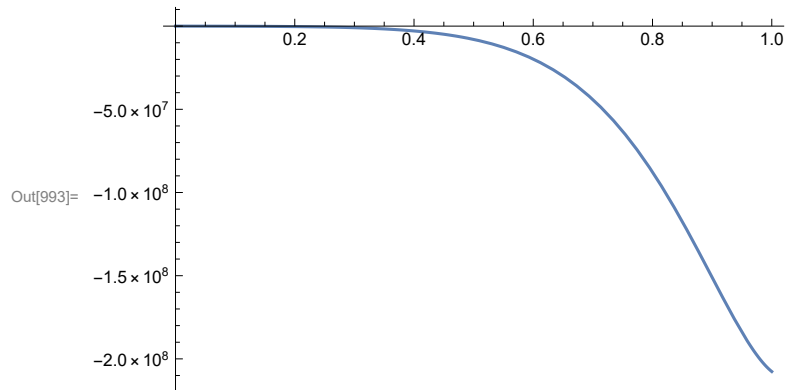

In[994]:= **Plot[Cf[8, 11, 4], {x, 0, 1}]**

[绘图](#)

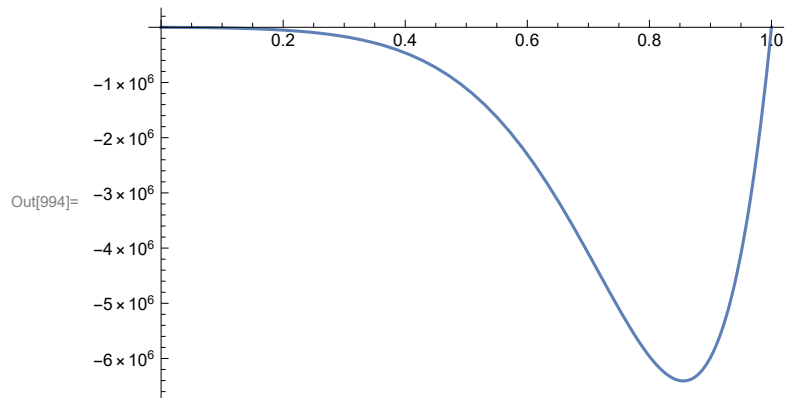

In[995]:= **Plot[Cf[8, 11, 3], {x, 0, 1}]**

[绘图](#)

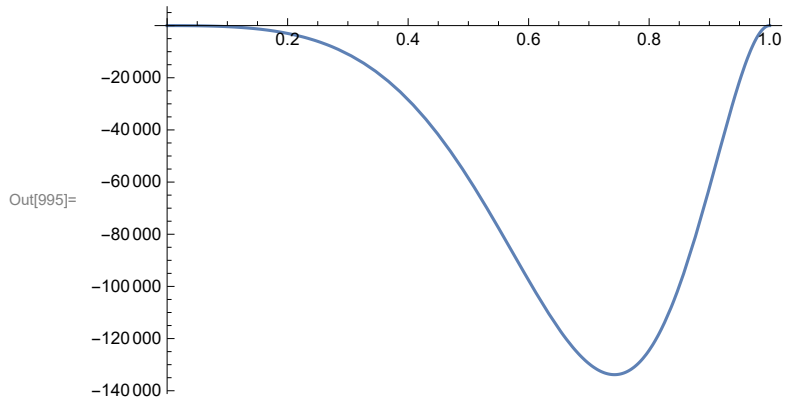

**Plot[Cf[8, 11, 2], {x, 0, 1}]**

[绘图](#)

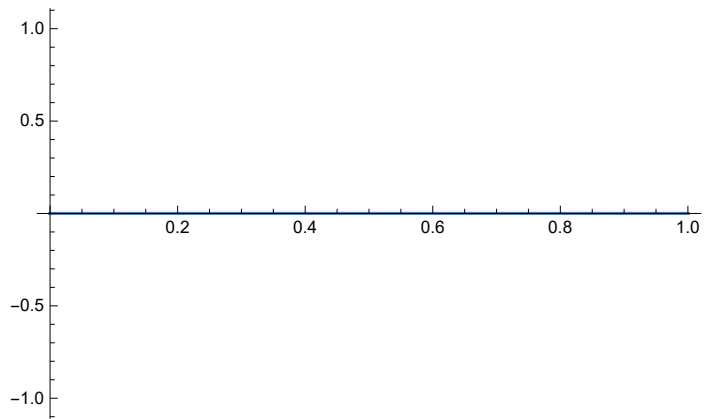

**Plot[Cf[8, 11, 1], {x, 0, 1}]**

[绘图](#)

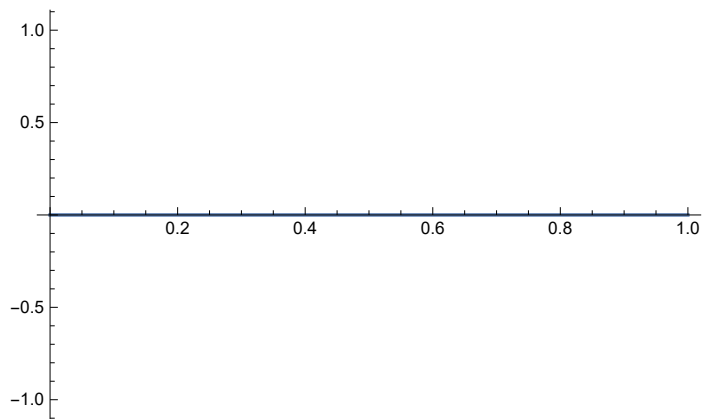

**Plot[Cf[8, 11, 0], {x, 0, 1}]**

[绘图](#)

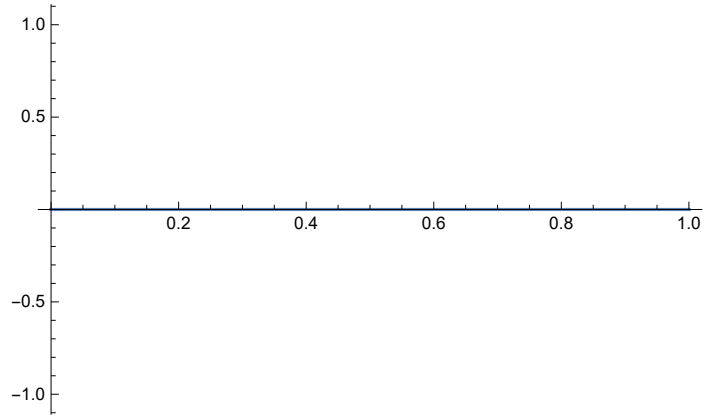

**(\*95th group coefficients r2^8r3^10\*)**

In[996]:= **Plot[Cf[8, 10, 14], {x, 0, 1}]**

[绘图](#)

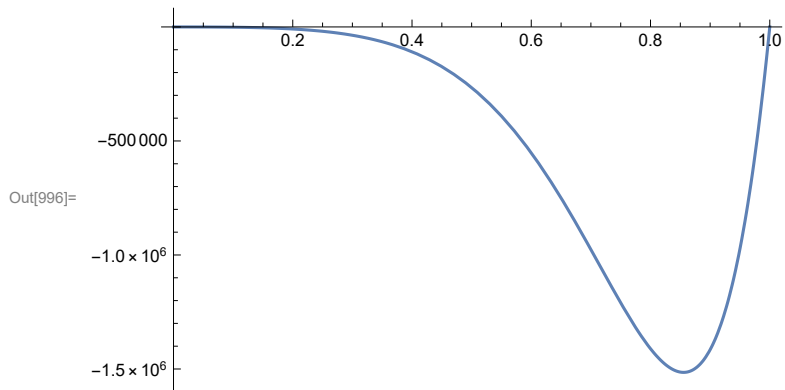

In[997]:= **Plot[Cf[8, 10, 13], {x, 0, 1}]**

[绘图](#)

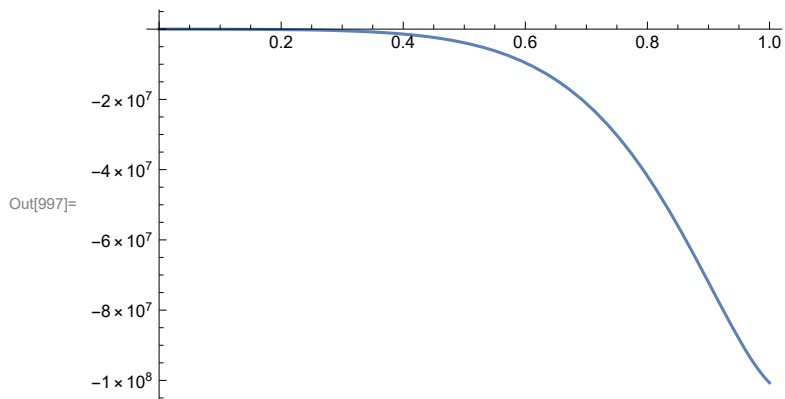

In[998]:= **Plot[Cf[8, 10, 12], {x, 0, 1}]**

[绘图](#)

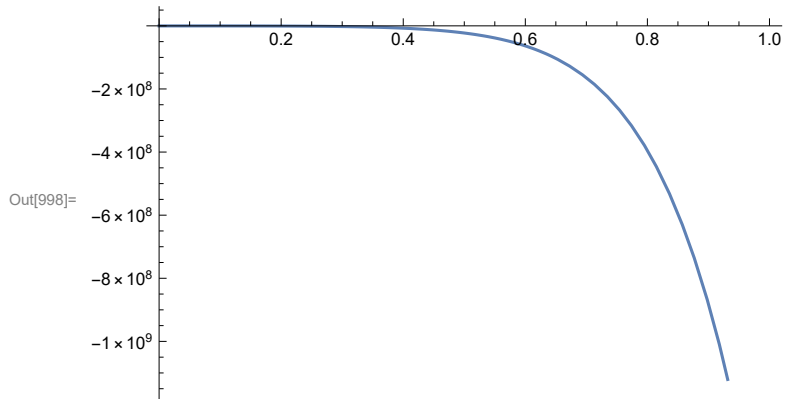

In[999]:= **Plot[Cf[8, 10, 11], {x, 0, 1}]**

[绘图](#)

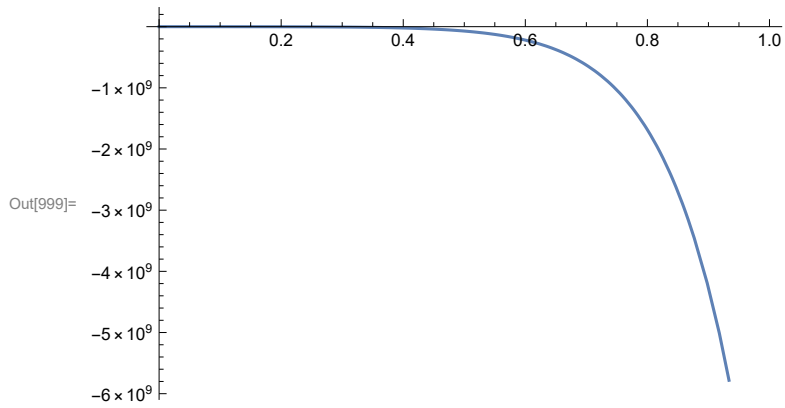

In[1000]:= **Plot[Cf[8, 10, 10], {x, 0, 1}]**

[绘图](#)

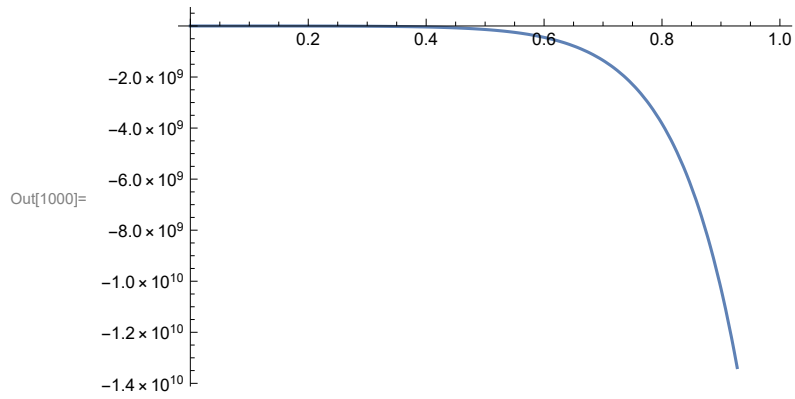

In[1001]:= **Plot[Cf[8, 10, 9], {x, 0, 1}]**

[绘图](#)

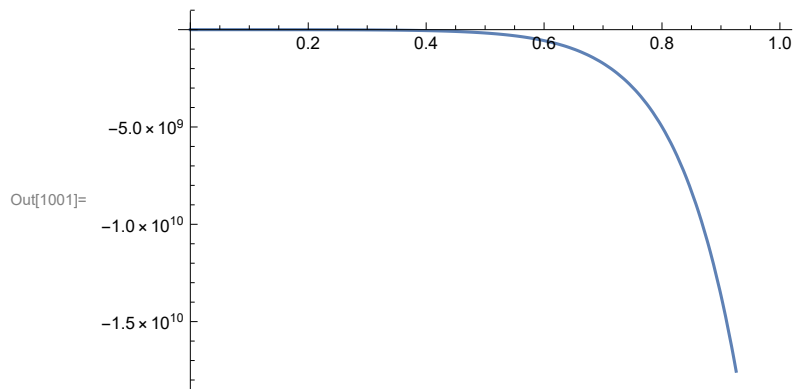

In[1002]:= **Plot[Cf[8, 10, 8], {x, 0, 1}]**

[绘图](#)

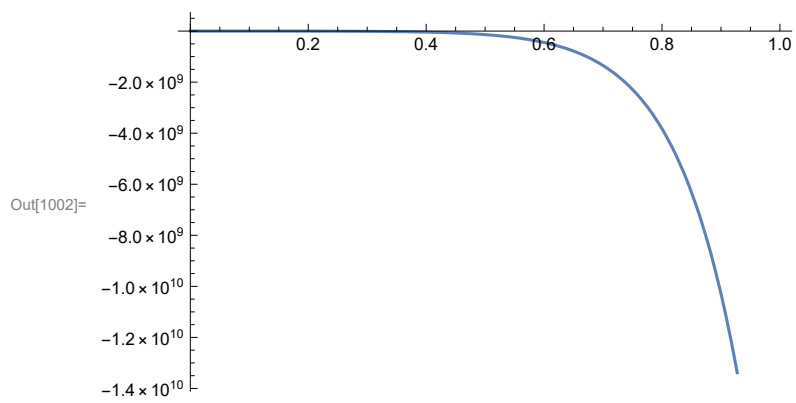

In[1003]:= **Plot[Cf[8, 10, 7], {x, 0, 1}]**

[绘图](#)

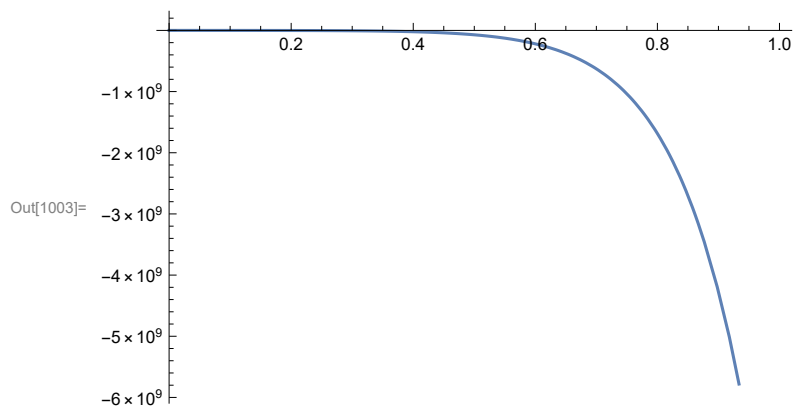



In[1004]:= **Plot[Cf[8, 10, 6], {x, 0, 1}]**

[绘图](#)

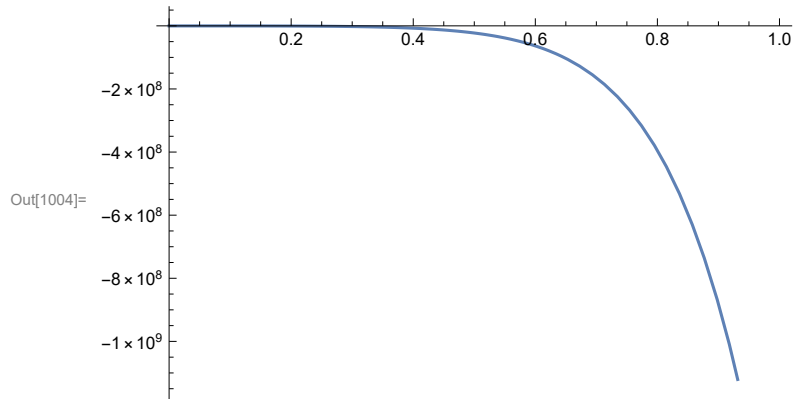

In[1005]:= **Plot[Cf[8, 10, 5], {x, 0, 1}]**

[绘图](#)

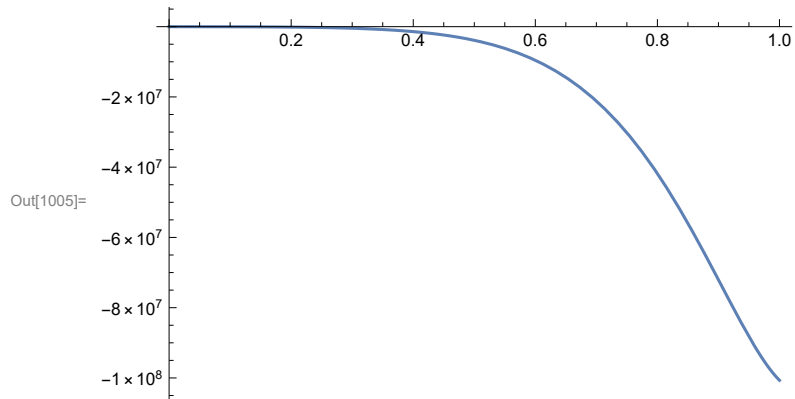

In[1006]:= **Plot[Cf[8, 10, 4], {x, 0, 1}]**

[绘图](#)

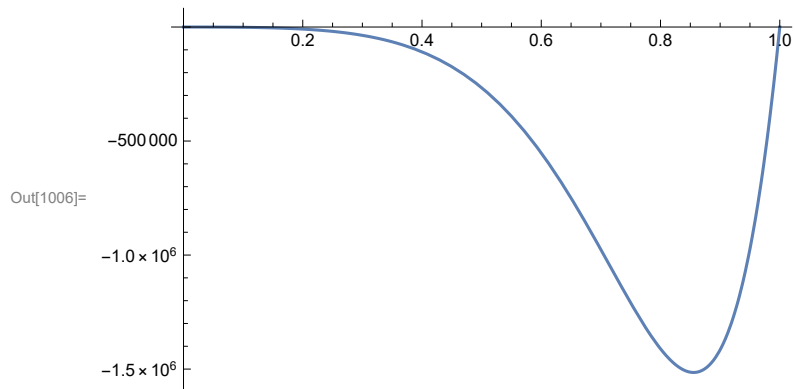

```
Plot[Cf[8, 10, 3], {x, 0, 1}]
```

[绘图](#)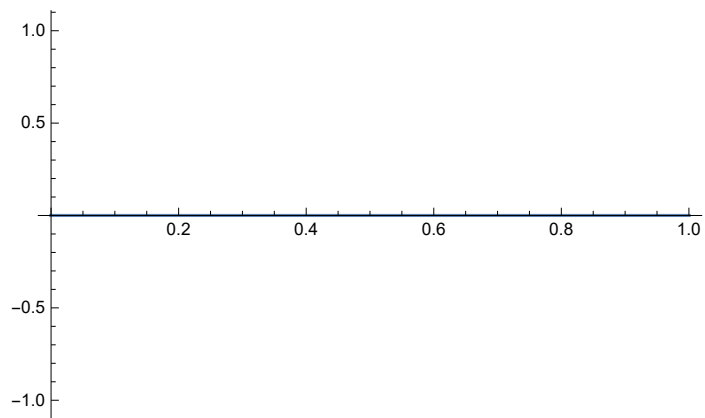

```
Plot[Cf[8, 10, 2], {x, 0, 1}]
```

[绘图](#)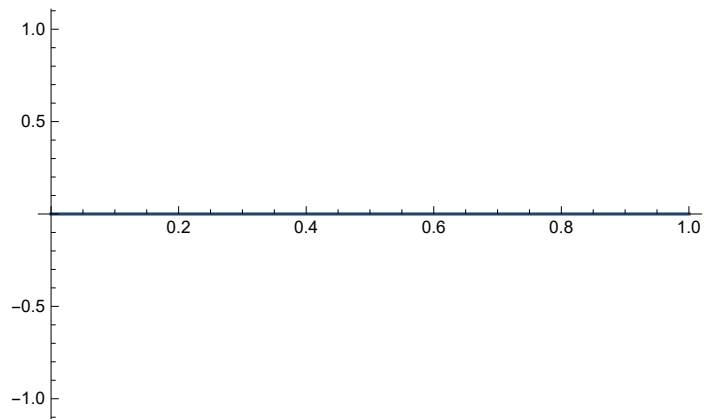

```
Plot[Cf[8, 10, 1], {x, 0, 1}]
```

[绘图](#)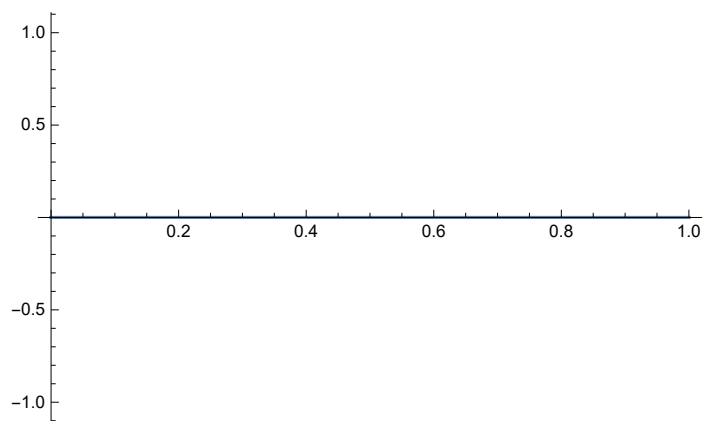

**Plot[Cf[8, 10, 0], {x, 0, 1}]**

[绘图](#)

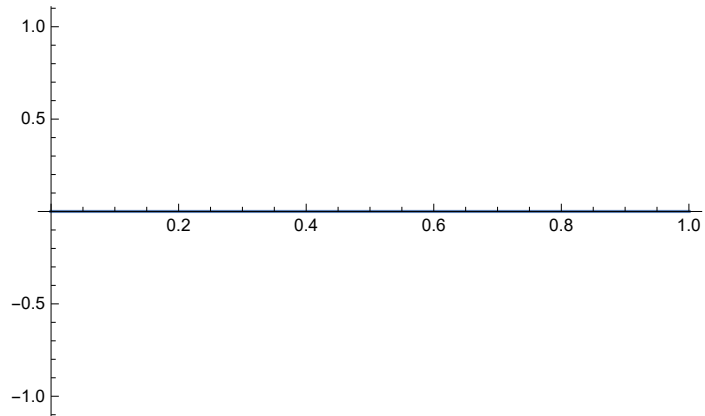

**(\*96th group coefficients r2^8r3^9\*)**

In[1007]:= **Plot[Cf[8, 9, 14], {x, 0, 1}]**

[绘图](#)

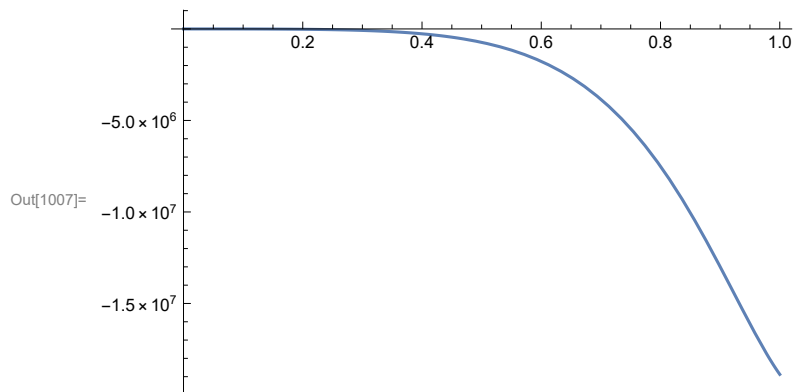

In[1008]:= **Plot[Cf[8, 9, 13], {x, 0, 1}]**

[绘图](#)

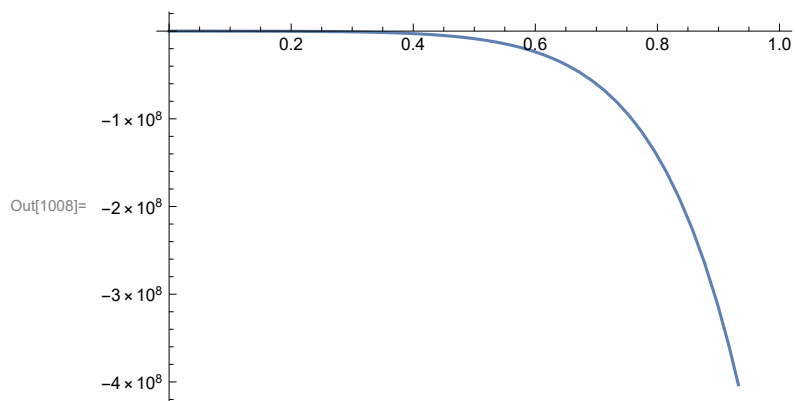

In[1009]:= **Plot[Cf[8, 9, 12], {x, 0, 1}]**

[绘图](#)

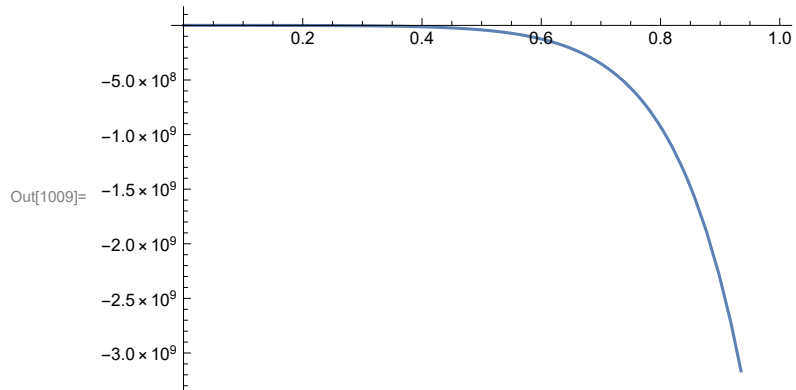

In[1010]:= **Plot[Cf[8, 9, 11], {x, 0, 1}]**

[绘图](#)

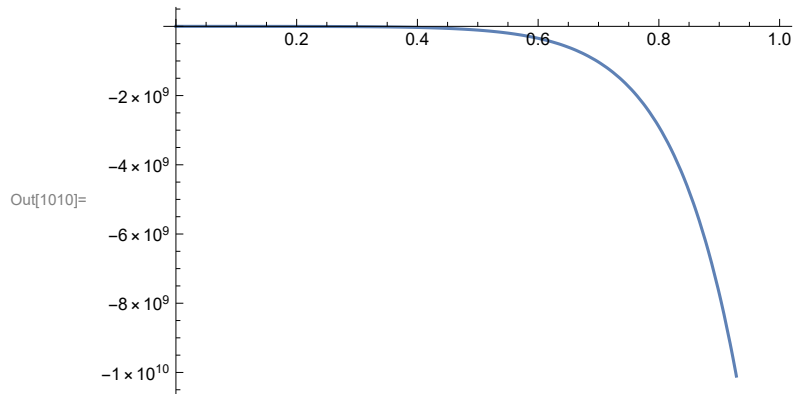

In[1011]:= **Plot[Cf[8, 9, 10], {x, 0, 1}]**

[绘图](#)

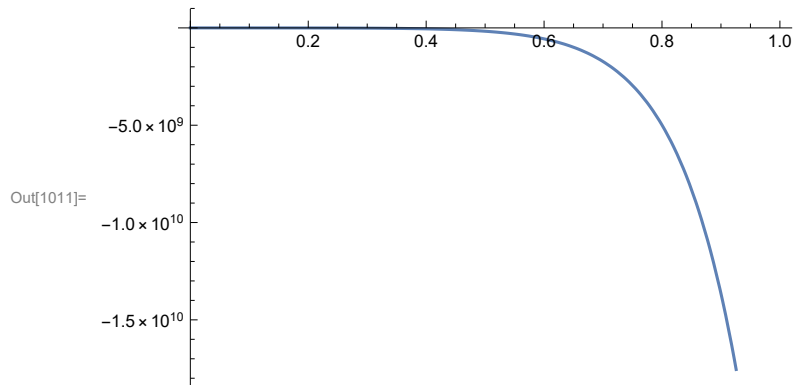

In[1012]:= **Plot[Cf[8, 9, 9], {x, 0, 1}]**

[绘图](#)

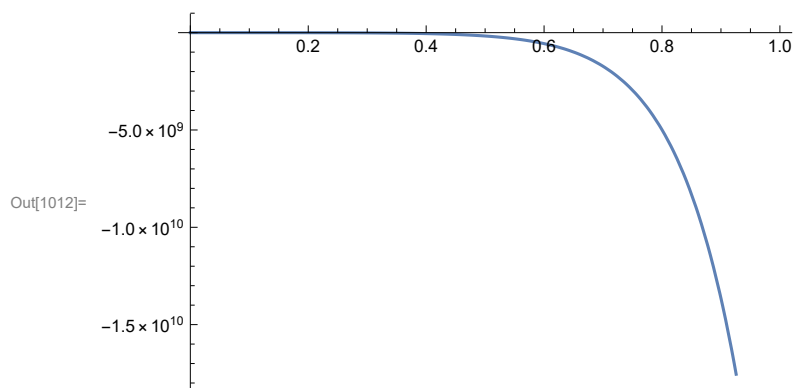

In[1013]:= **Plot[Cf[8, 9, 8], {x, 0, 1}]**

[绘图](#)

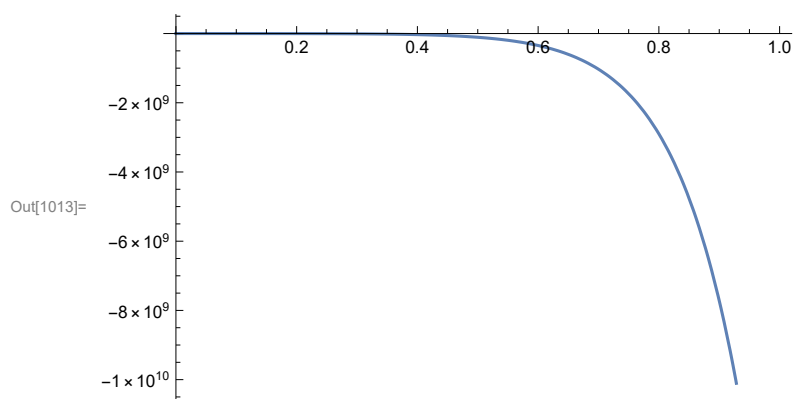

In[1014]:= **Plot[Cf[8, 9, 7], {x, 0, 1}]**

[绘图](#)

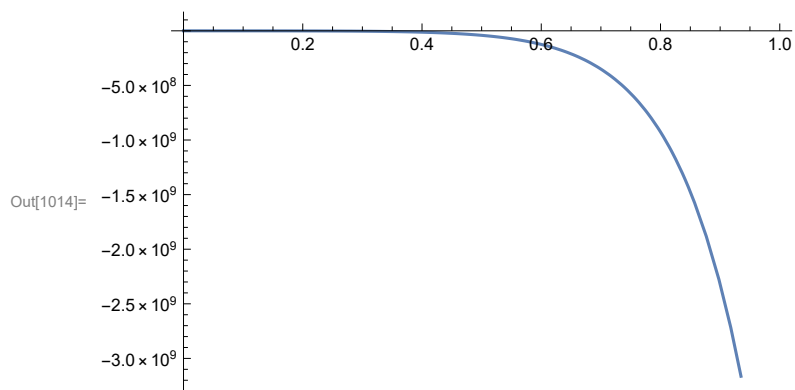

In[1015]:= **Plot[Cf[8, 9, 6], {x, 0, 1}]**

[绘图](#)

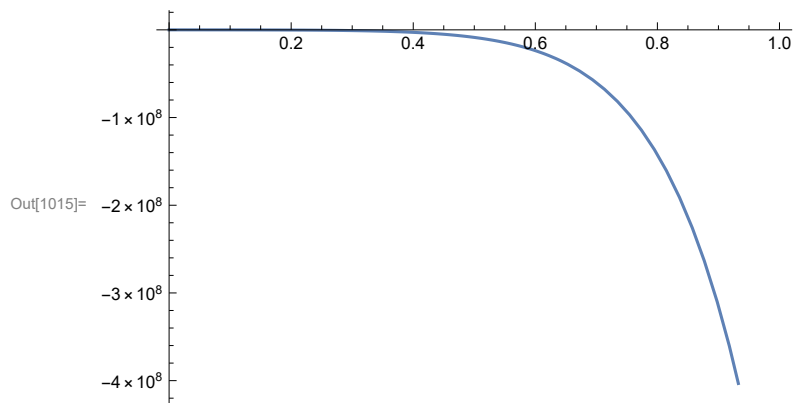

In[1016]:= **Plot[Cf[8, 9, 5], {x, 0, 1}]**

[绘图](#)

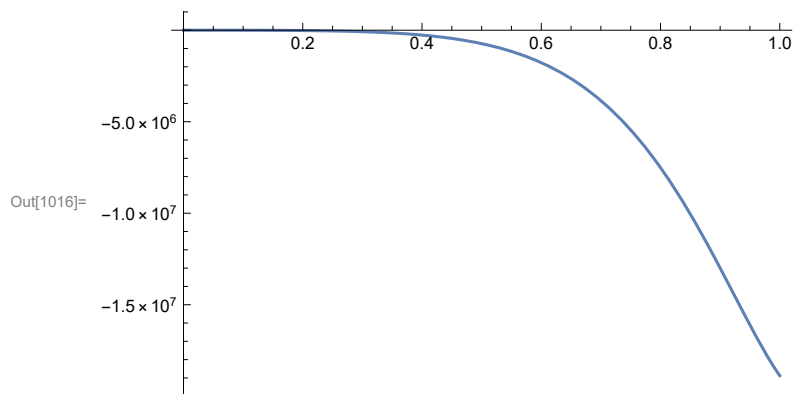

**Plot[Cf[8, 9, 4], {x, 0, 1}]**

[绘图](#)

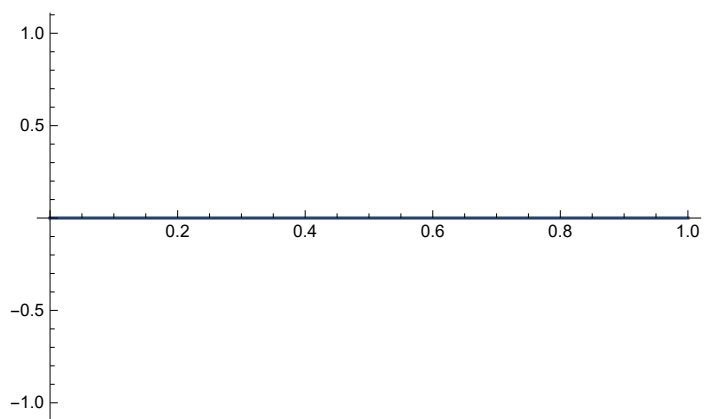

**Plot[Cf[8, 9, 3], {x, 0, 1}]**

[绘图](#)

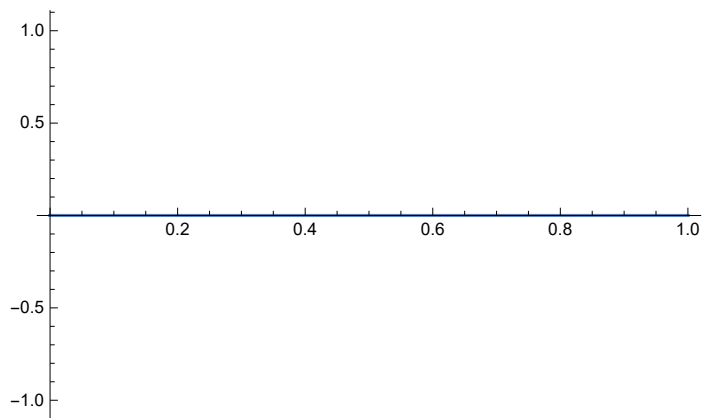

(\*97th group coefficients r2^8r3^8\*)

In[1017]:= **Plot[Cf[8, 8, 14], {x, 0, 1}]**

[绘图](#)

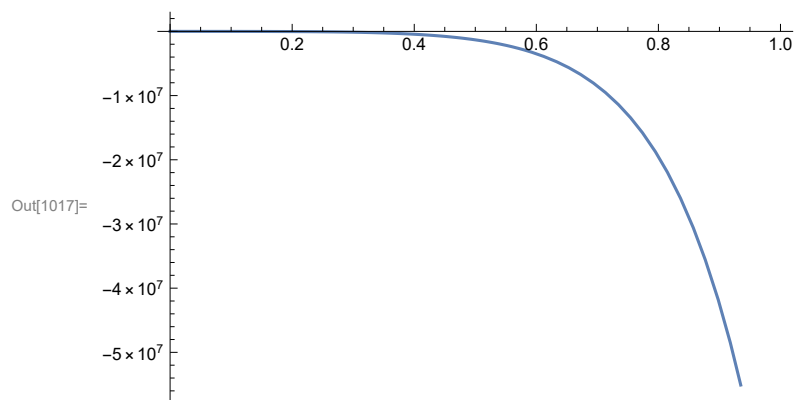

In[1019]:= **Plot[Cf[8, 8, 13], {x, 0, 1}]**

[绘图](#)

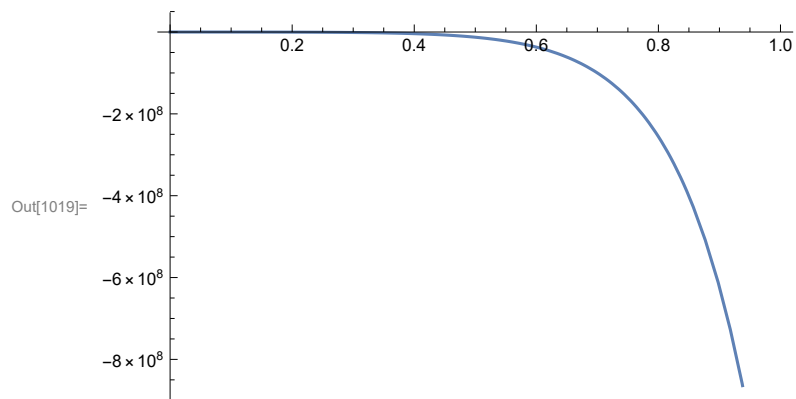

In[1020]:= **Plot[Cf[8, 8, 12], {x, 0, 1}]**

[绘图](#)

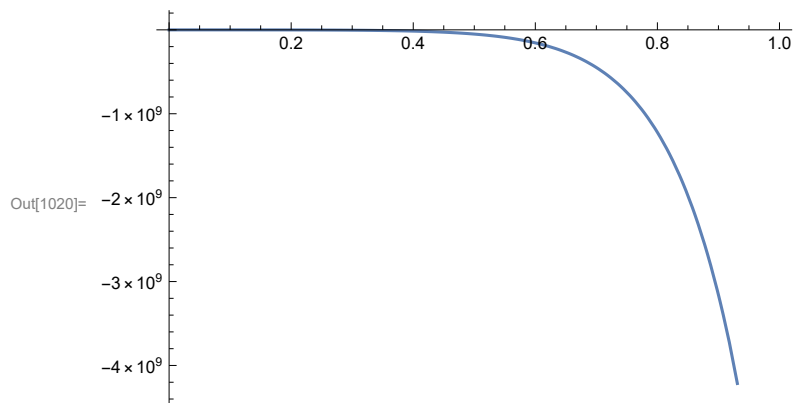

In[1021]:= **Plot[Cf[8, 8, 11], {x, 0, 1}]**

[绘图](#)

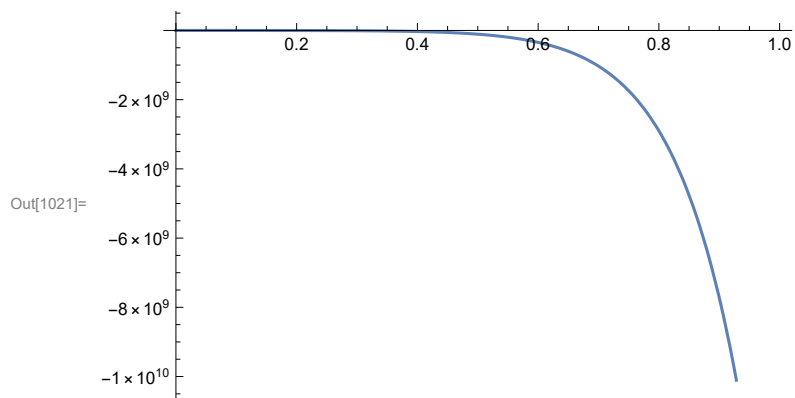

In[1022]:= **Plot[Cf[8, 8, 10], {x, 0, 1}]**

[绘图](#)

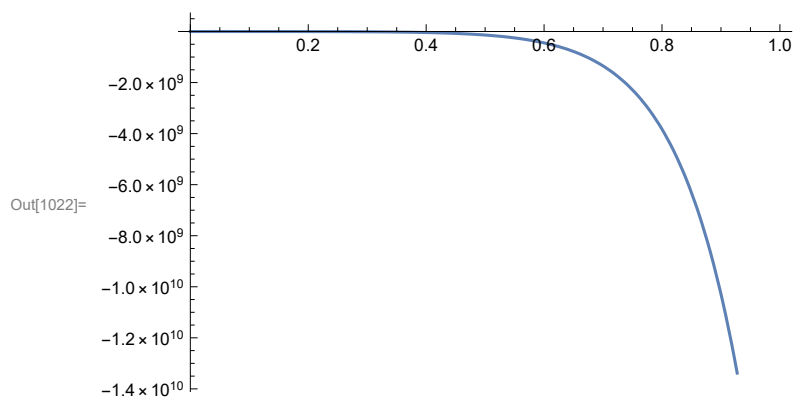



In[1023]:= **Plot[Cf[8, 8, 9], {x, 0, 1}]**

[绘图](#)

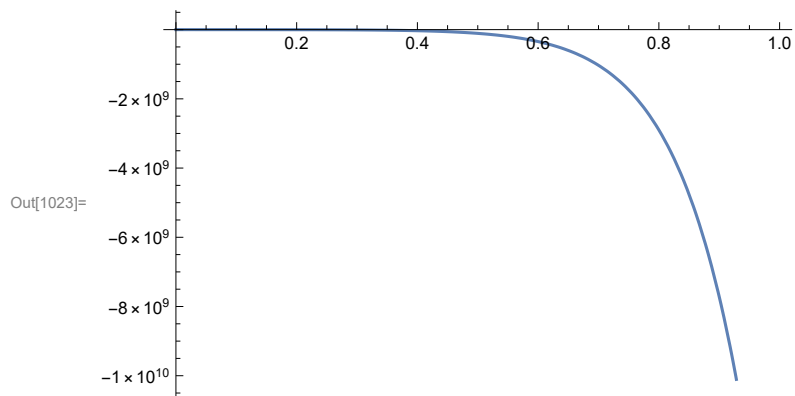

In[1024]:= **Plot[Cf[8, 8, 8], {x, 0, 1}]**

[绘图](#)

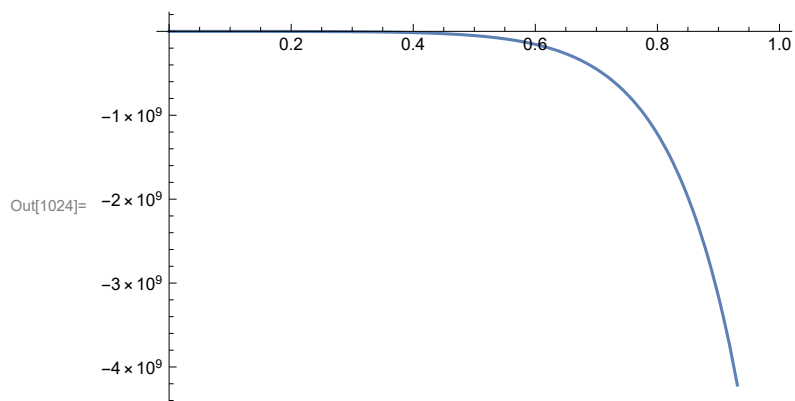

In[1025]:= **Plot[Cf[8, 8, 7], {x, 0, 1}]**

[绘图](#)

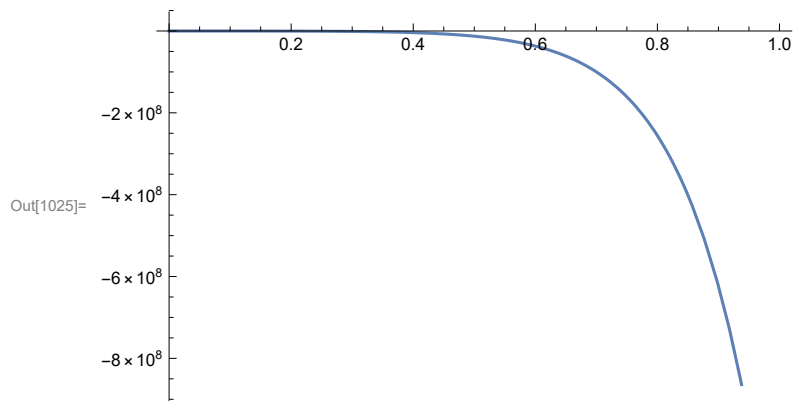

In[1026]:= **Plot[Cf[8, 8, 6], {x, 0, 1}]**

[绘图](#)

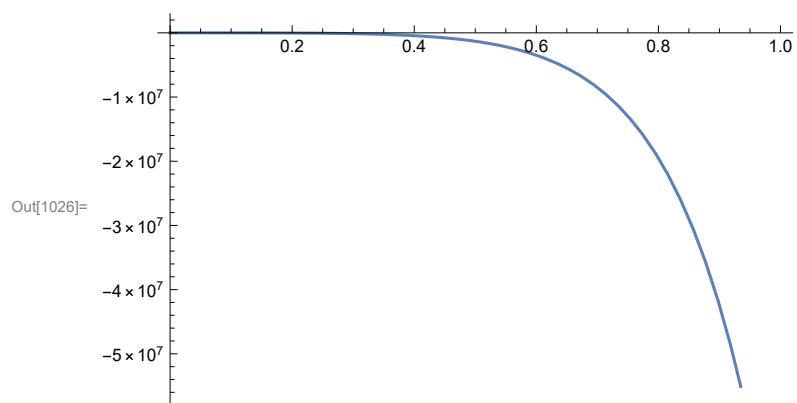

**Plot[Cf[8, 8, 5], {x, 0, 1}]**

[绘图](#)

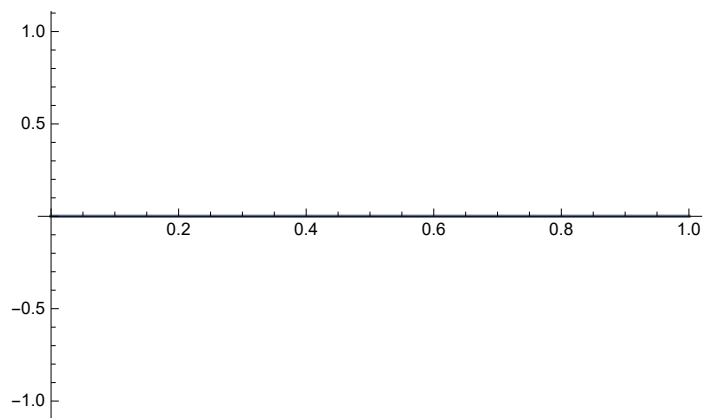

**Plot[Cf[8, 8, 4], {x, 0, 1}]**

[绘图](#)

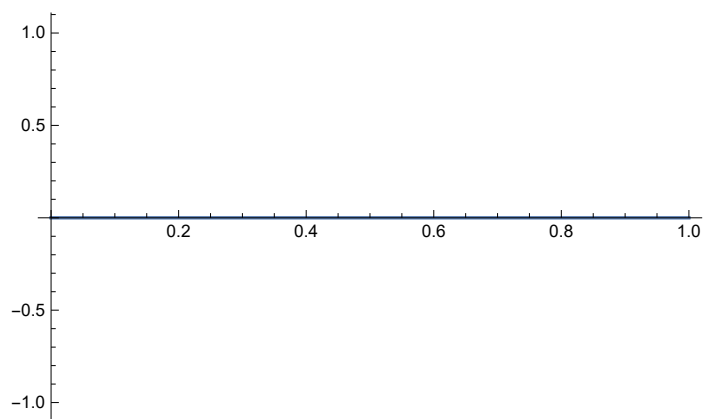

**Plot[Cf[8, 8, 3], {x, 0, 1}]**

[绘图](#)

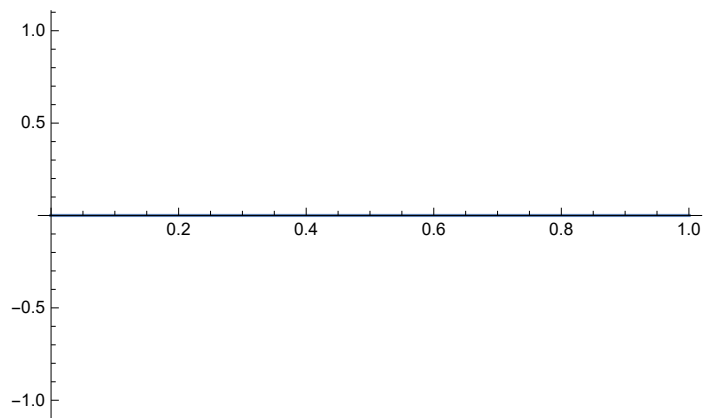

**Plot[Cf[8, 8, 2], {x, 0, 1}]**

[绘图](#)

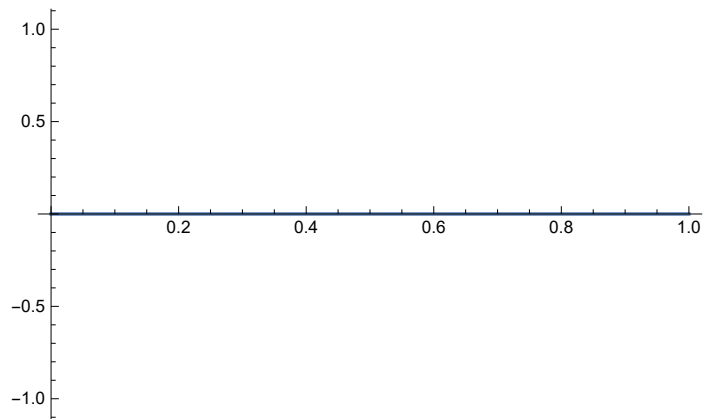

**Plot[Cf[8, 8, 1], {x, 0, 1}]**

[绘图](#)

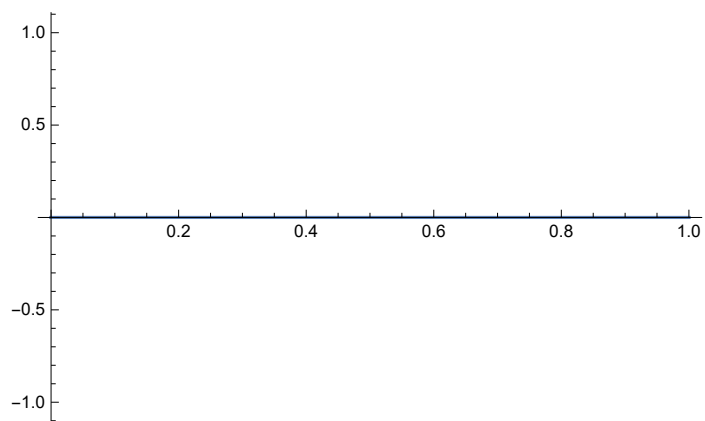

**Plot[Cf[8, 8, 0], {x, 0, 1}]**

[绘图](#)

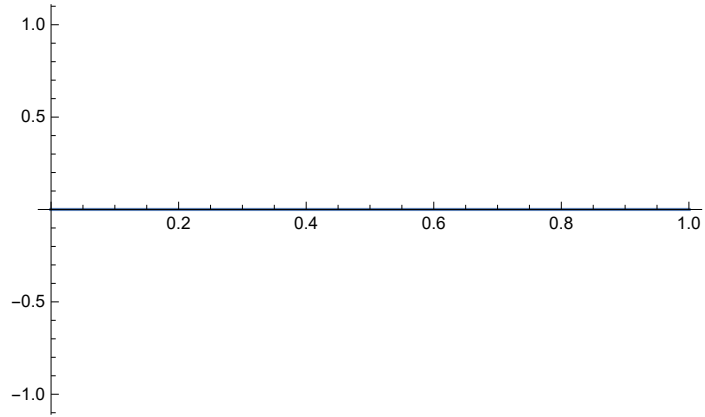

**(\*98th group coefficients r2^8r3^7\*)**

In[1027]:= **Plot[Cf[8, 7, 14], {x, 0, 1}]**

[绘图](#)

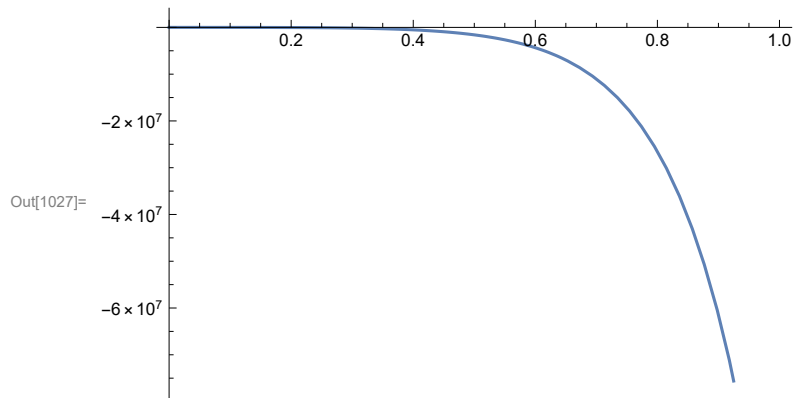

In[1028]:= **Plot[Cf[8, 7, 13], {x, 0, 1}]**

[绘图](#)

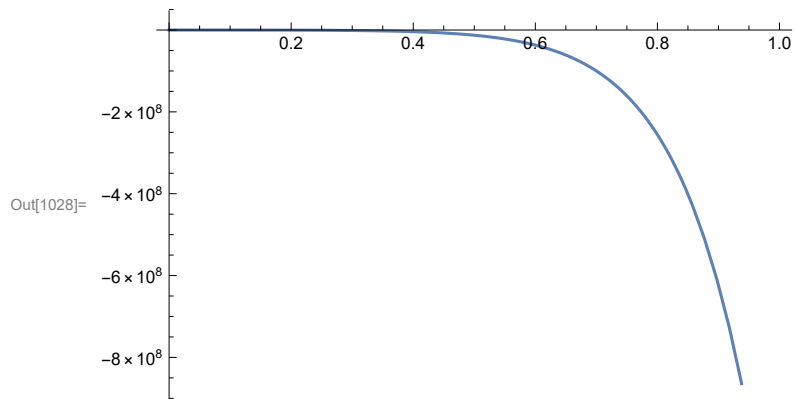

In[1029]:= **Plot**[**Cf**[8, 7, 12], {x, 0, 1}]

[绘图](#)

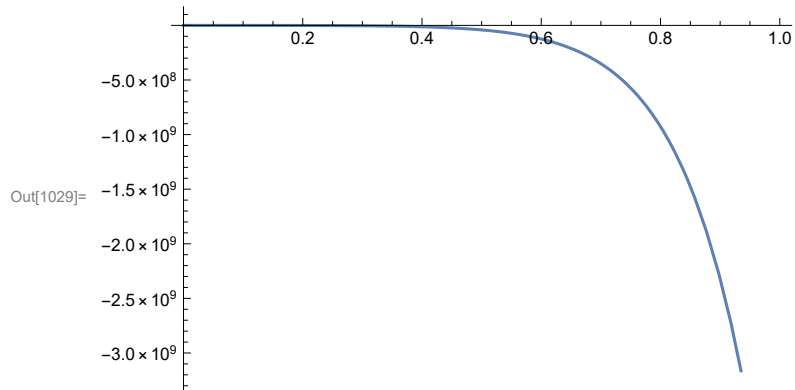

In[1030]:= **Plot**[**Cf**[8, 7, 11], {x, 0, 1}]

[绘图](#)

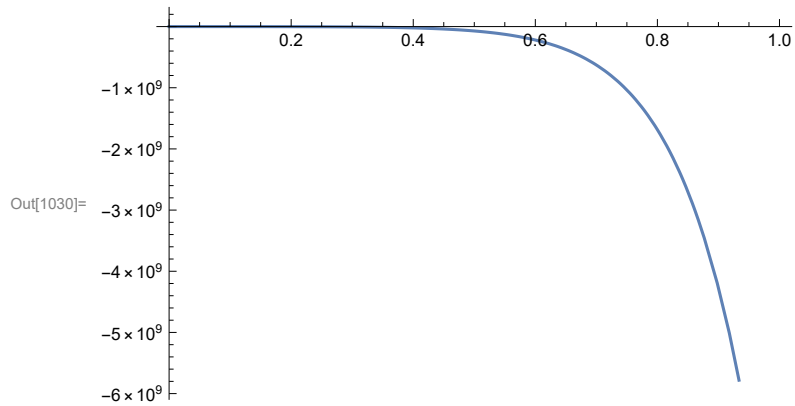

In[1031]:= **Plot**[**Cf**[8, 7, 10], {x, 0, 1}]

[绘图](#)

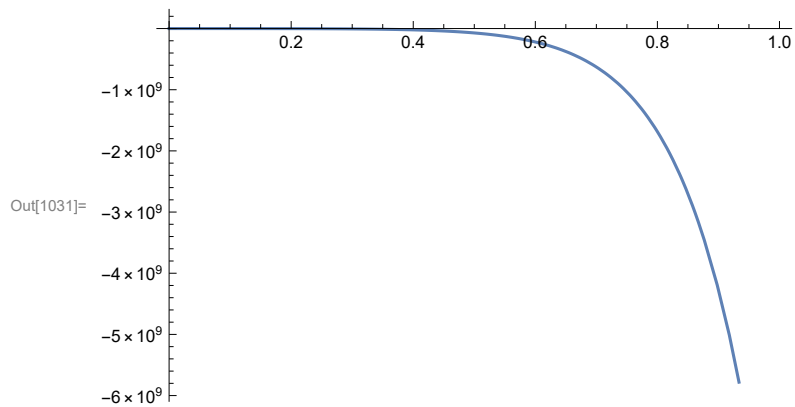

In[1032]:= **Plot**[**Cf**[8, 7, 9], {x, 0, 1}]

[绘图](#)

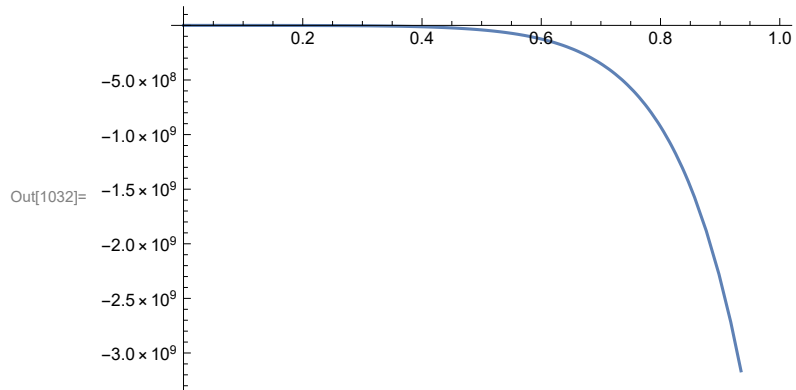

In[1033]:= **Plot**[**Cf**[8, 7, 8], {x, 0, 1}]

[绘图](#)

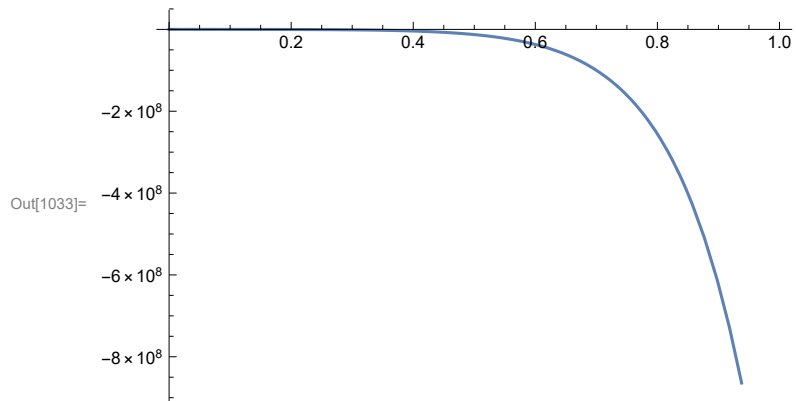

In[1034]:= **Plot**[**Cf**[8, 7, 7], {x, 0, 1}]

[绘图](#)

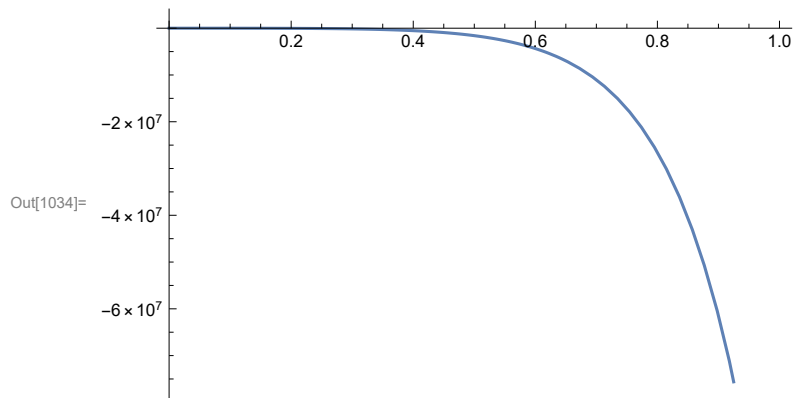

**Plot[Cf[8, 7, 6], {x, 0, 1}]**

[绘图](#)

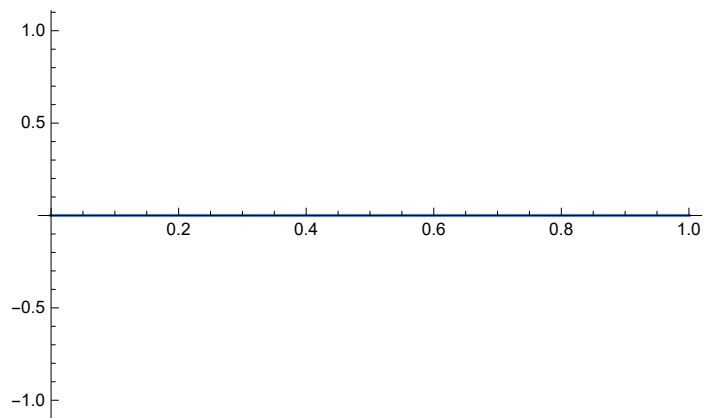

**Plot[Cf[8, 7, 5], {x, 0, 1}]**

[绘图](#)

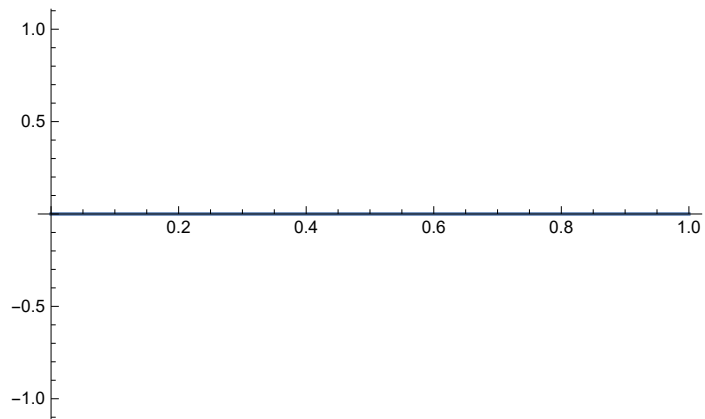

**Plot[Cf[8, 7, 4], {x, 0, 1}]**

[绘图](#)

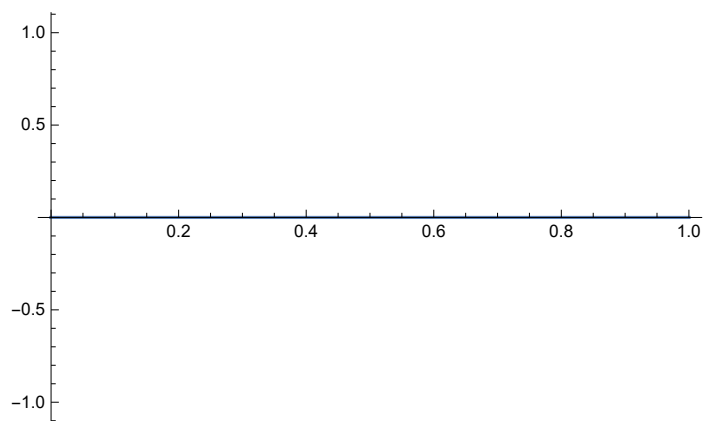

```
Plot[Cf[8, 7, 3], {x, 0, 1}]
```

[绘图](#)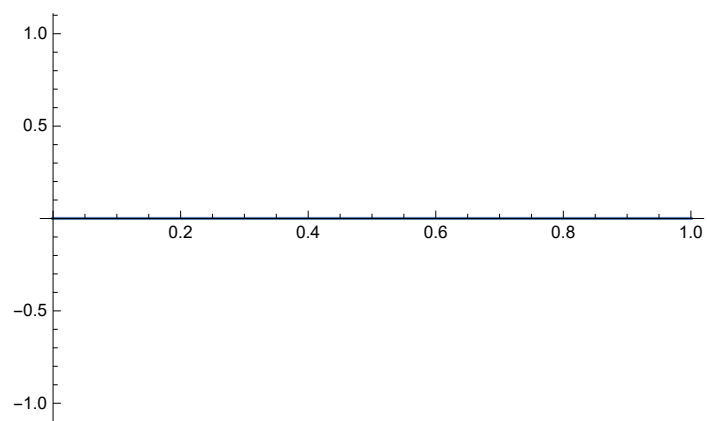

```
Plot[Cf[8, 7, 2], {x, 0, 1}]
```

[绘图](#)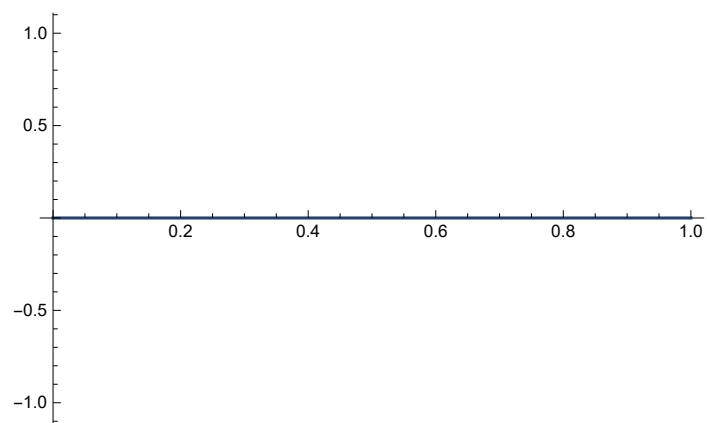

```
Plot[Cf[8, 7, 1], {x, 0, 1}]
```

[绘图](#)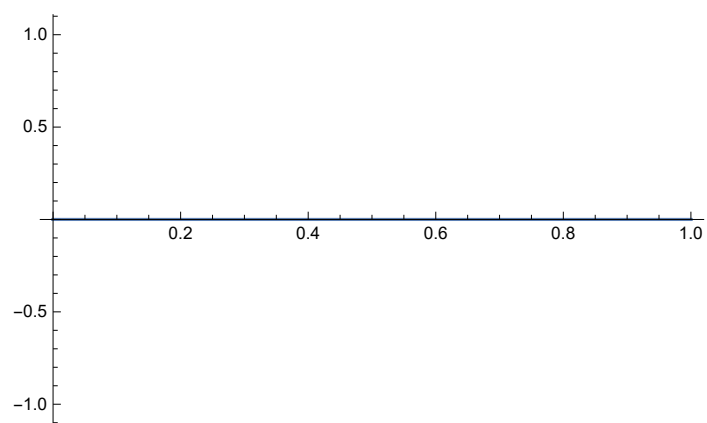



**Plot[Cf[8, 7, 0], {x, 0, 1}]**

[绘图](#)

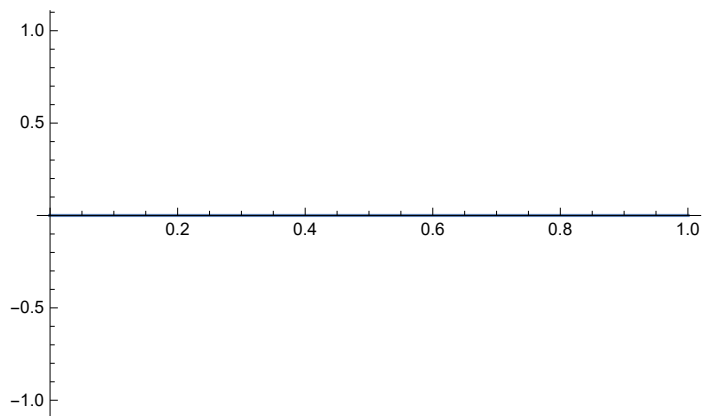

(\*99th group coefficients r2^8r3^6\*)

In[1035]:= **Plot[Cf[8, 6, 14], {x, 0, 1}]**

[绘图](#)

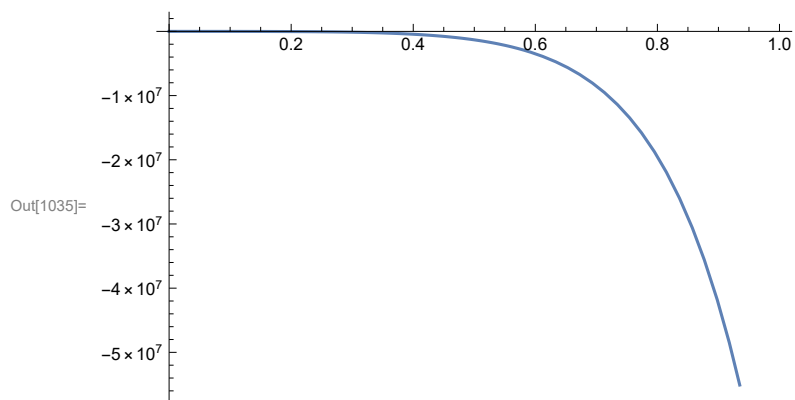

In[1036]:= **Plot[Cf[8, 6, 13], {x, 0, 1}]**

[绘图](#)

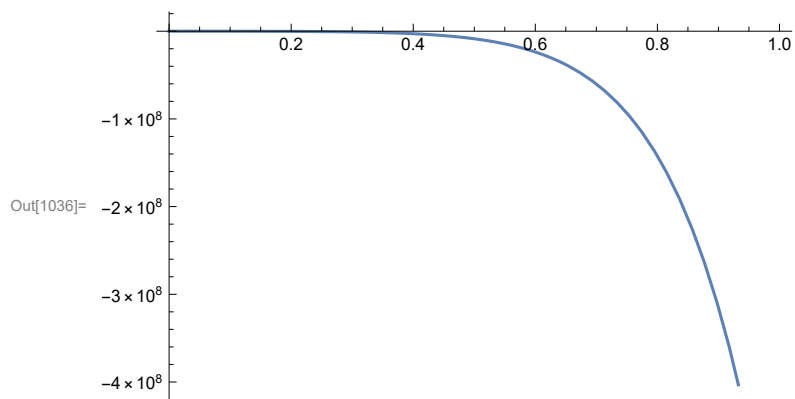

In[1037]:= **Plot[Cf[8, 6, 12], {x, 0, 1}]**

[绘图](#)

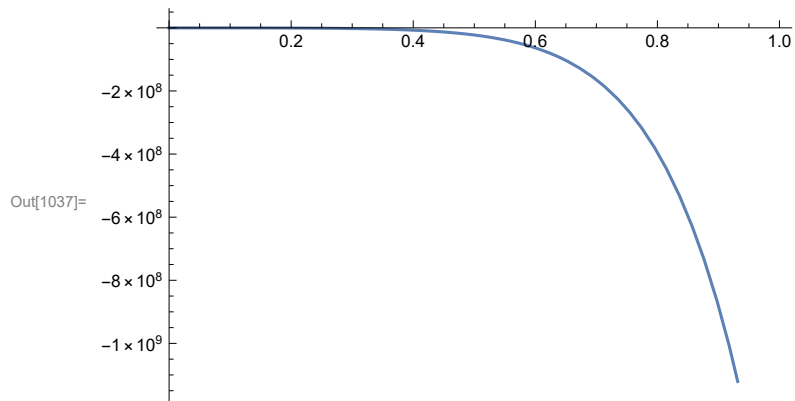

In[1038]:= **Plot[Cf[8, 6, 11], {x, 0, 1}]**

[绘图](#)

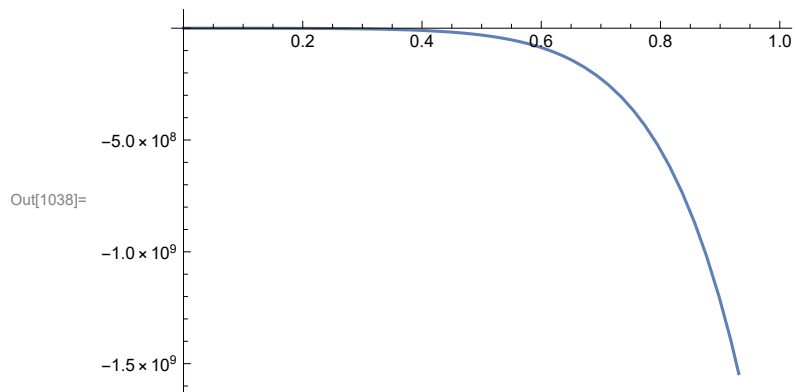

In[1039]:= **Plot[Cf[8, 6, 10], {x, 0, 1}]**

[绘图](#)

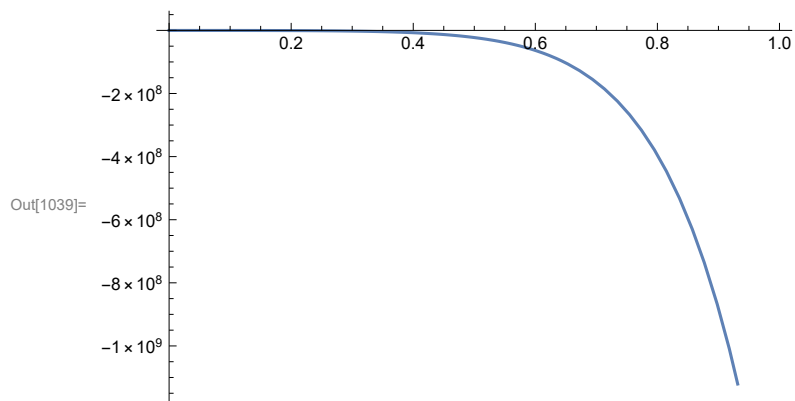

In[1040]:= **Plot[Cf[8, 6, 9], {x, 0, 1}]**

[绘图](#)

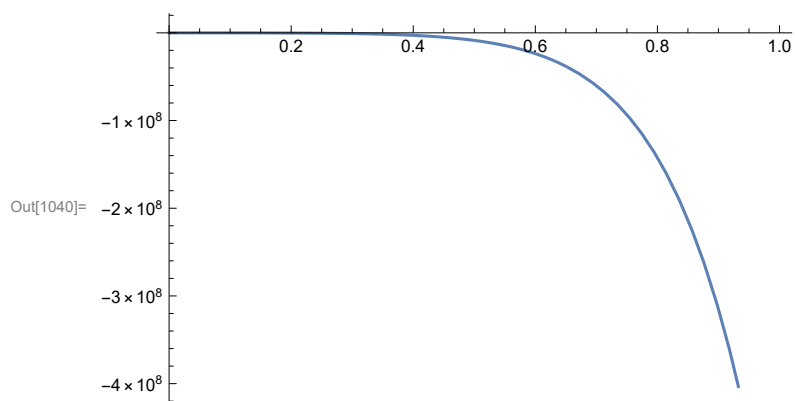

In[1041]:= **Plot[Cf[8, 6, 8], {x, 0, 1}]**

[绘图](#)

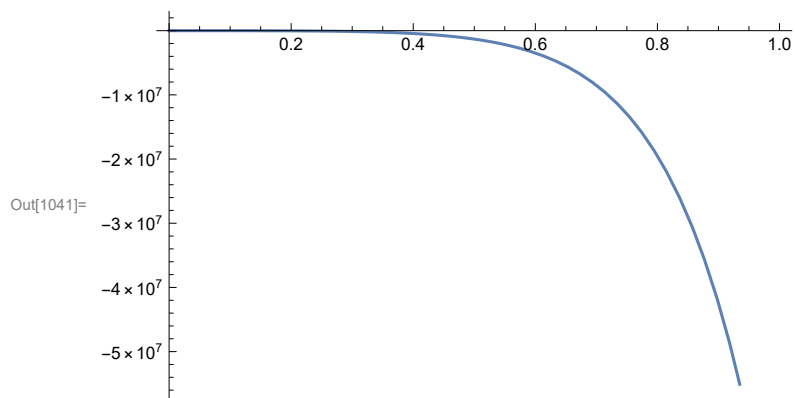

**Plot[Cf[8, 6, 7], {x, 0, 1}]**

[绘图](#)

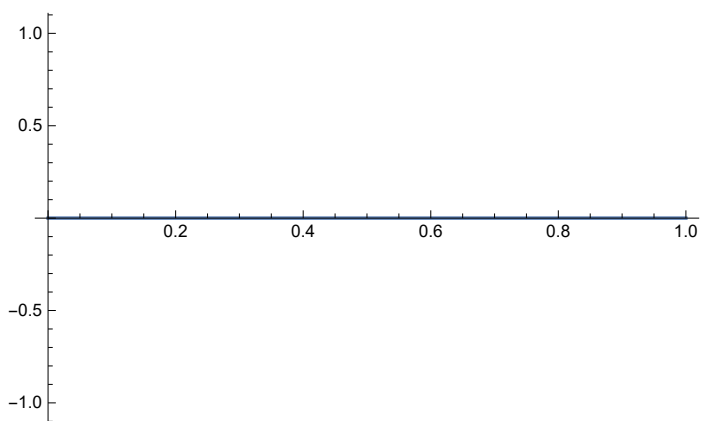

**Plot[Cf[8, 6, 6], {x, 0, 1}]**

[绘图](#)

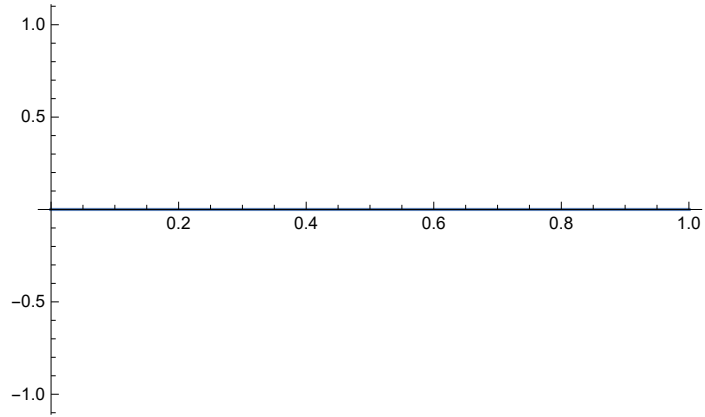

**Plot[Cf[8, 6, 5], {x, 0, 1}]**

[绘图](#)

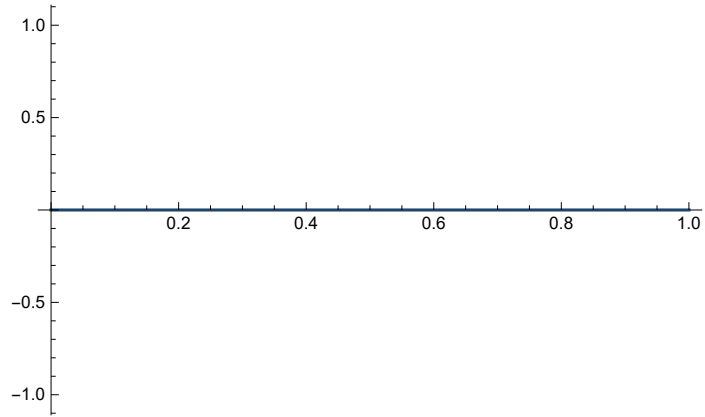

**Plot[Cf[8, 6, 4], {x, 0, 1}]**

[绘图](#)

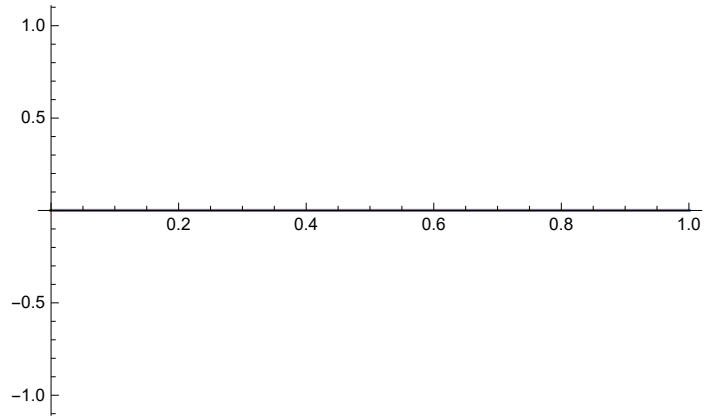

**Plot[Cf[8, 6, 3], {x, 0, 1}]**

[绘图](#)

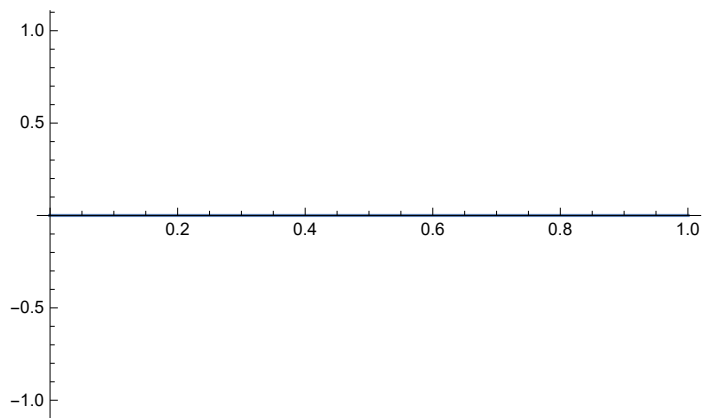

**Plot[Cf[8, 6, 2], {x, 0, 1}]**

[绘图](#)

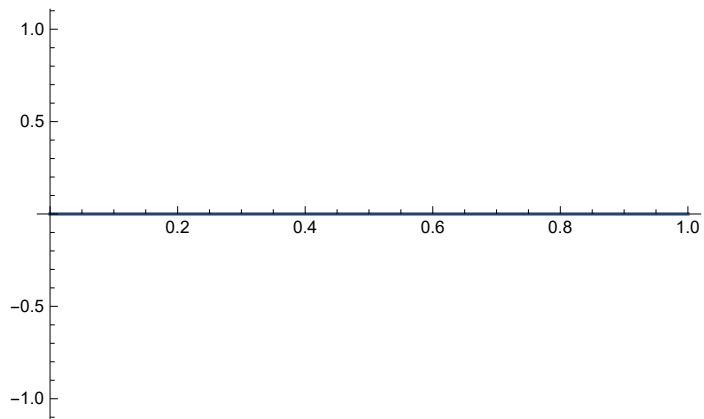

**Plot[Cf[8, 6, 1], {x, 0, 1}]**

[绘图](#)

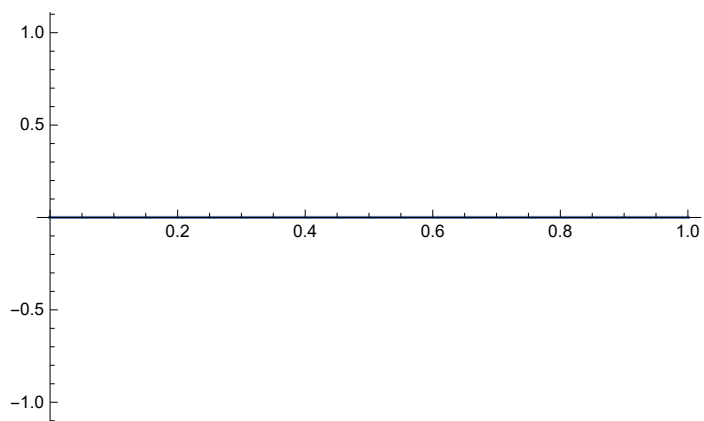

**Plot[Cf[8, 6, 0], {x, 0, 1}]**

[绘图](#)

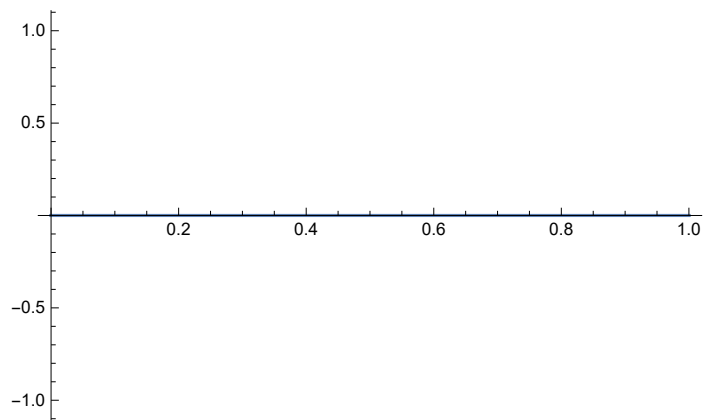

**(\*100th group coefficients r2^8r3^5\*)**

In[1042]:= **Plot[Cf[8, 5, 14], {x, 0, 1}]**

[绘图](#)

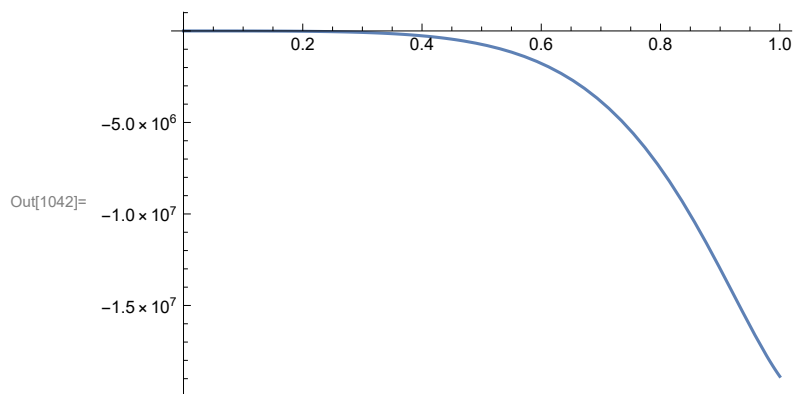

In[1043]:= **Plot[Cf[8, 5, 13], {x, 0, 1}]**

[绘图](#)

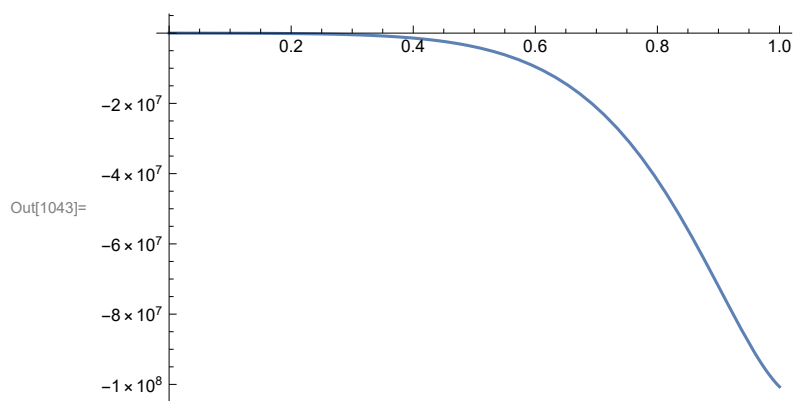

In[1044]:= **Plot[Cf[8, 5, 12], {x, 0, 1}]**

[绘图](#)

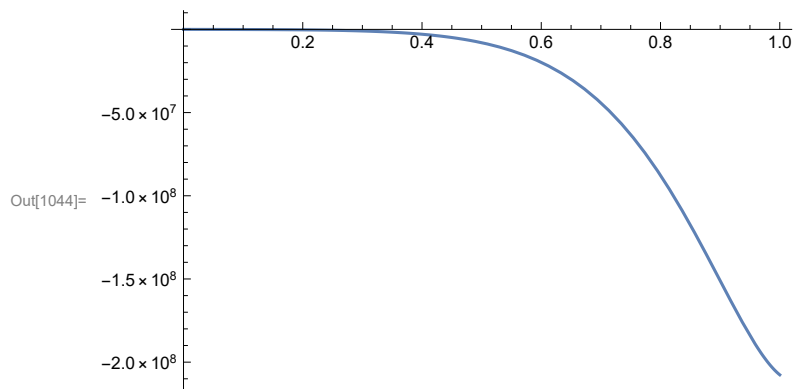

In[1045]:= **Plot[Cf[8, 5, 11], {x, 0, 1}]**

[绘图](#)

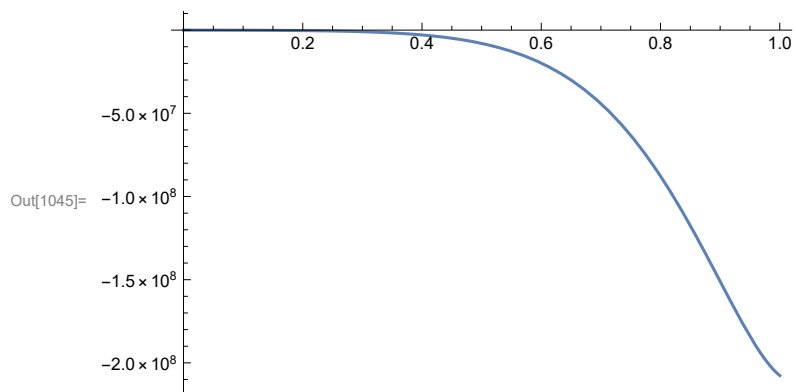

In[1046]:= **Plot[Cf[8, 5, 10], {x, 0, 1}]**

[绘图](#)

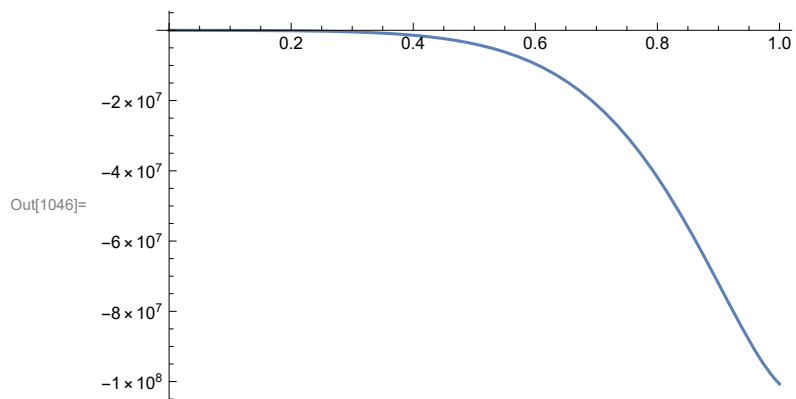

In[1047]:= **Plot[Cf[8, 5, 9], {x, 0, 1}]**

[绘图](#)

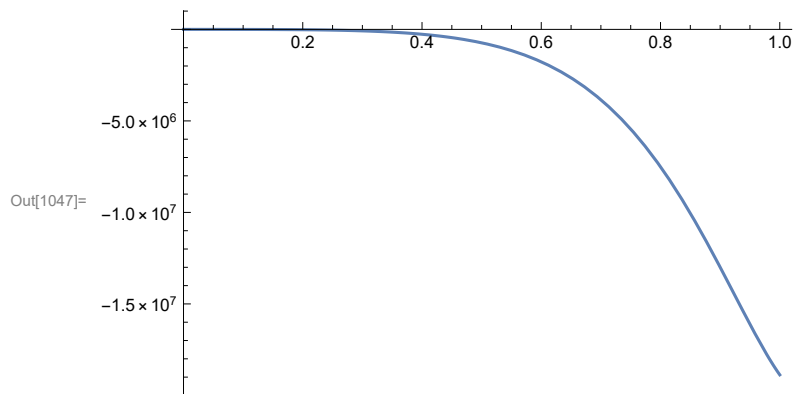

**Plot[Cf[8, 5, 8], {x, 0, 1}]**

[绘图](#)

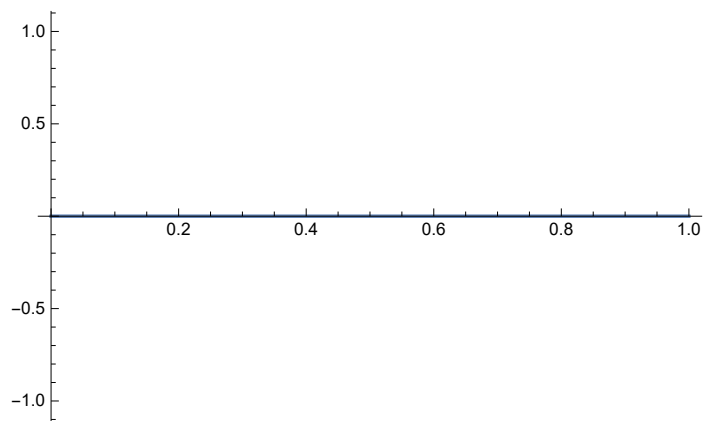

**Plot[Cf[8, 5, 7], {x, 0, 1}]**

[绘图](#)

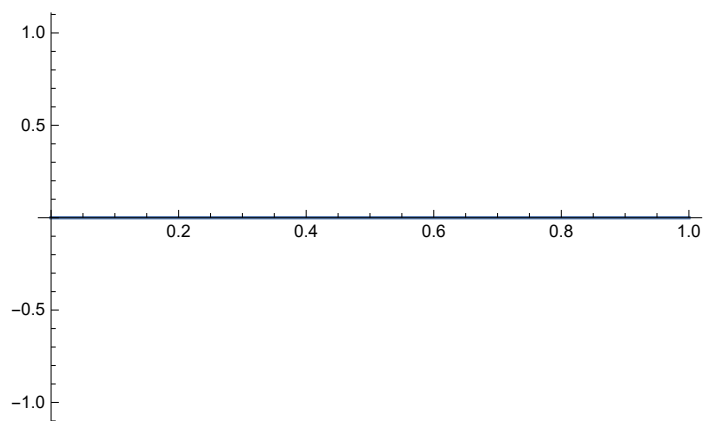



**Plot[Cf[8, 5, 6], {x, 0, 1}]**

[绘图](#)

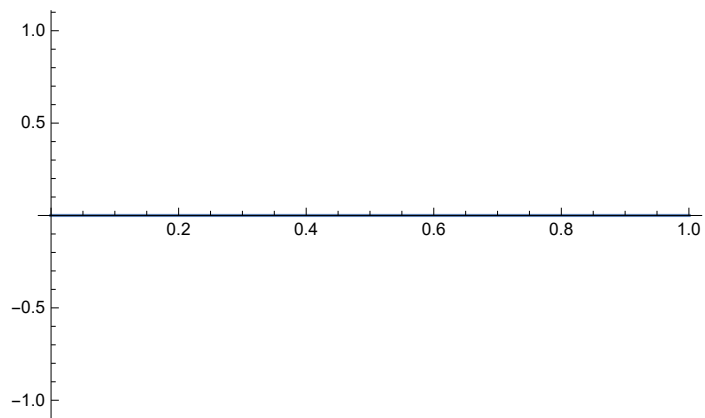

**Plot[Cf[8, 5, 5], {x, 0, 1}]**

[绘图](#)

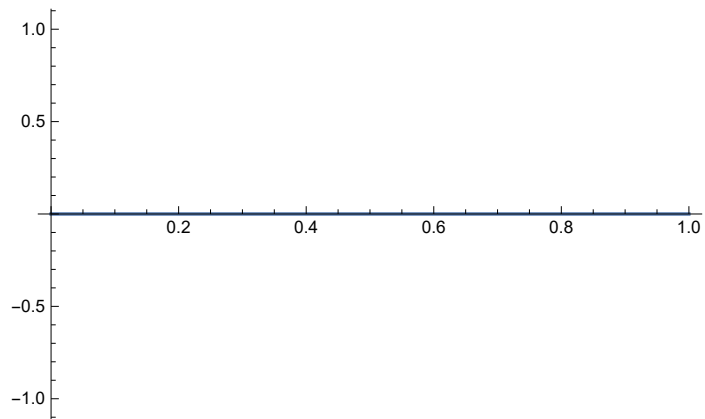

**Plot[Cf[8, 5, 4], {x, 0, 1}]**

[绘图](#)

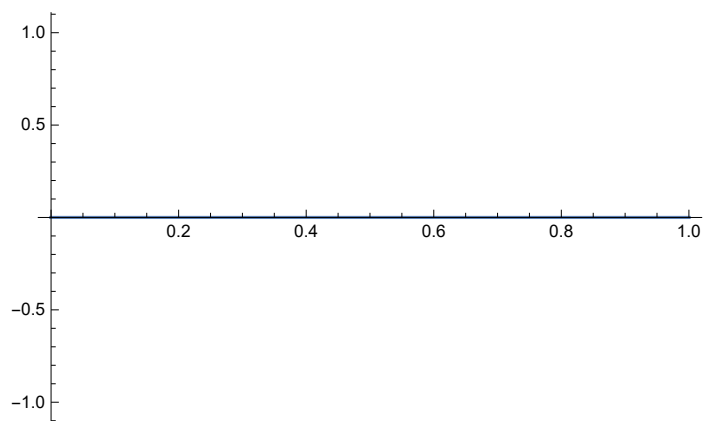

**Plot[Cf[8, 5, 3], {x, 0, 1}]**

[绘图](#)

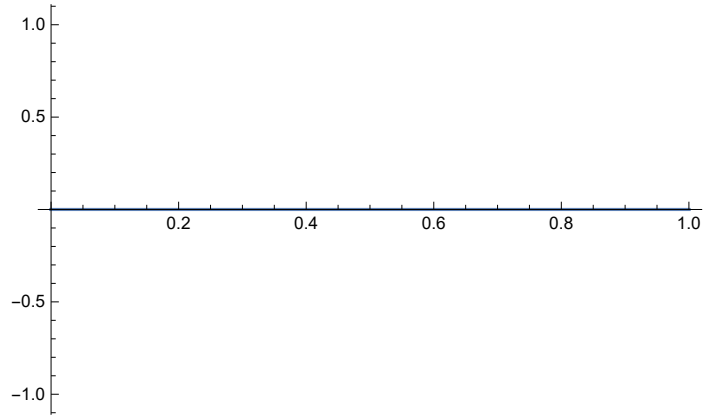

**Plot[Cf[8, 5, 2], {x, 0, 1}]**

[绘图](#)

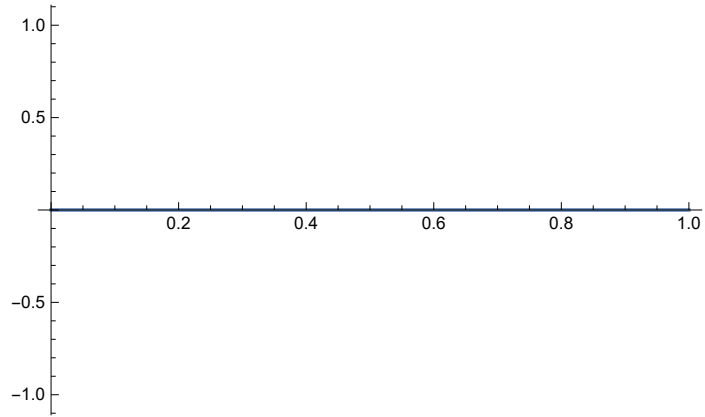

**Plot[Cf[8, 5, 1], {x, 0, 1}]**

[绘图](#)

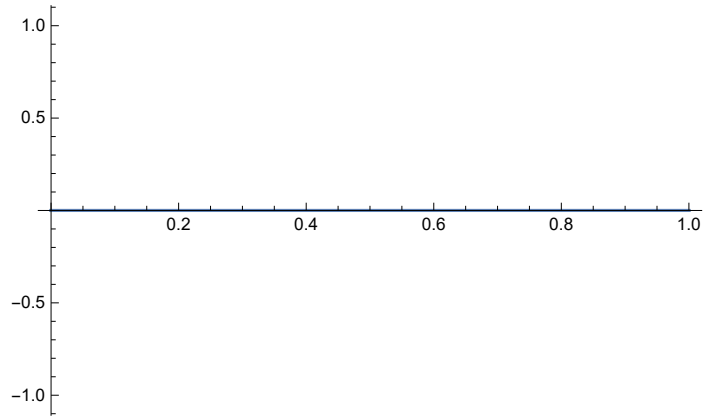

**Plot[Cf[8, 5, 0], {x, 0, 1}]**

[绘图](#)

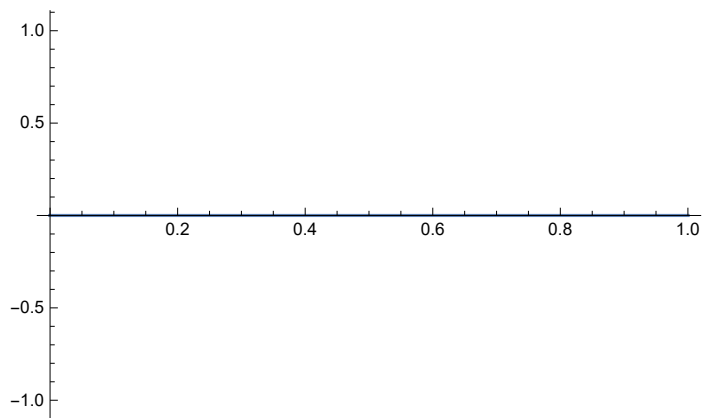

**(\*101th group coefficients r2^8r3^4\*)**

In[1048]:= **Plot[Cf[8, 4, 14], {x, 0, 1}]**

[绘图](#)

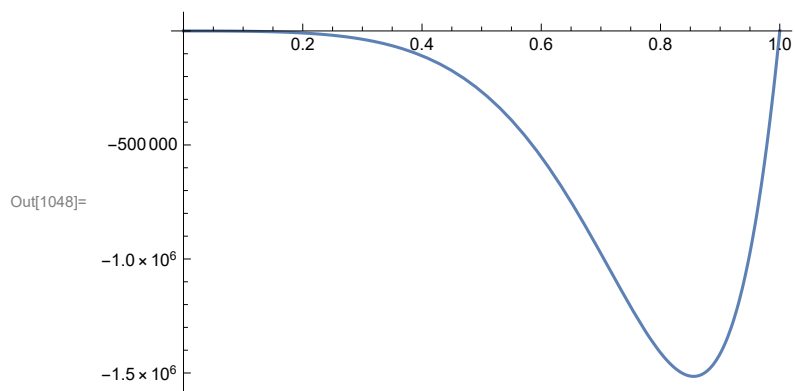

In[1049]:= **Plot[Cf[8, 4, 13], {x, 0, 1}]**

[绘图](#)

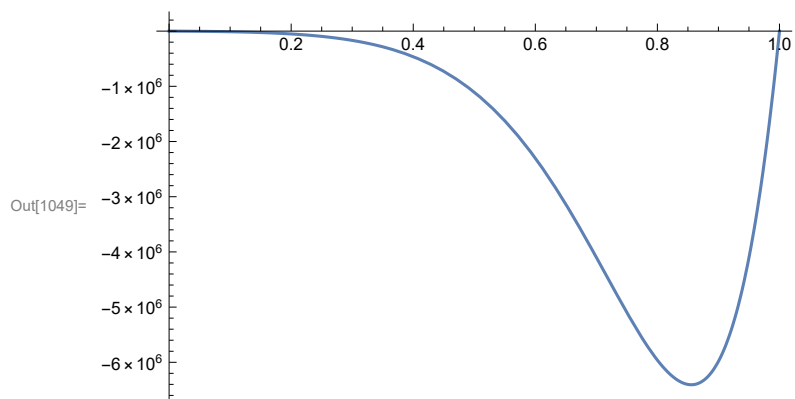

In[1050]:= **Plot[Cf[8, 4, 12], {x, 0, 1}]**

[绘图](#)

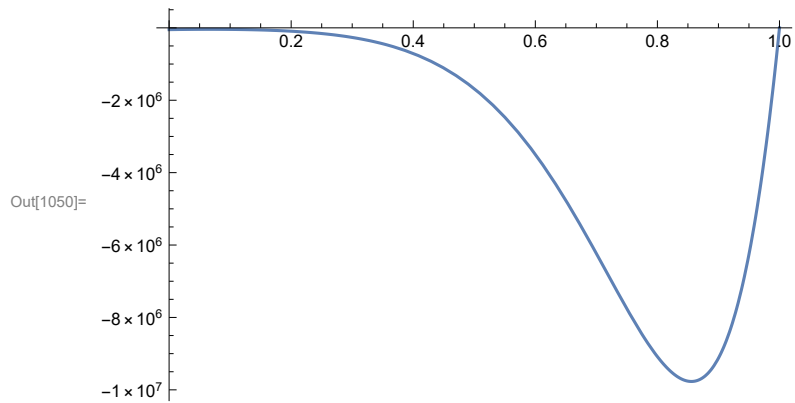

In[1051]:= **Plot[Cf[8, 4, 11], {x, 0, 1}]**

[绘图](#)

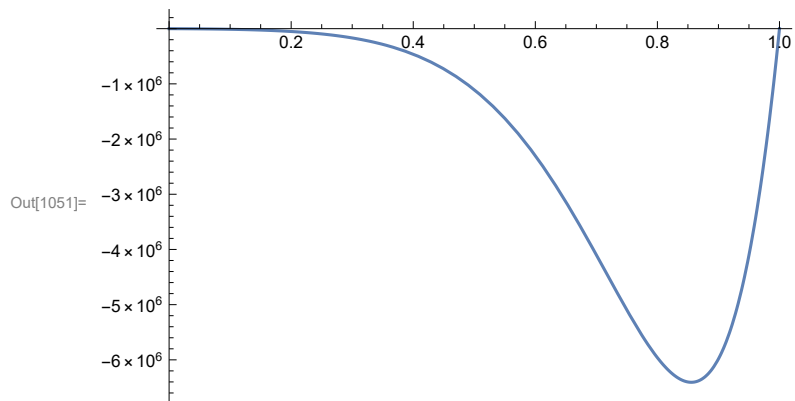

In[1052]:= **Plot[Cf[8, 4, 10], {x, 0, 1}]**

[绘图](#)

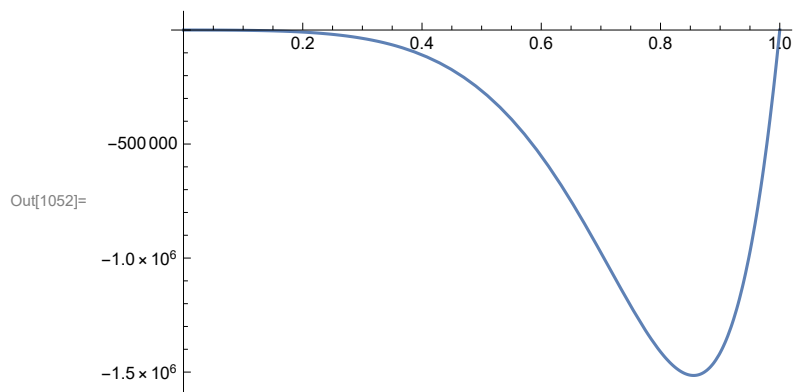

**Plot[Cf[8, 4, 9], {x, 0, 1}]**

[绘图](#)

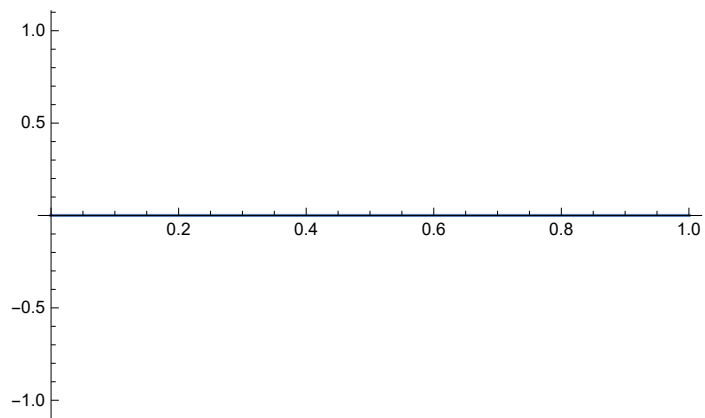

**Plot[Cf[8, 4, 8], {x, 0, 1}]**

[绘图](#)

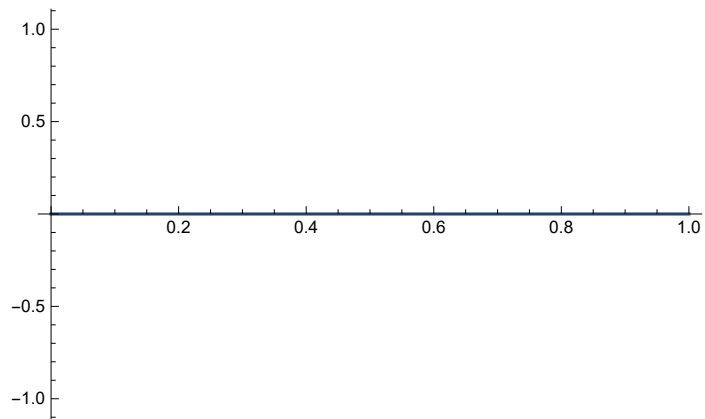

**Plot[Cf[8, 4, 7], {x, 0, 1}]**

[绘图](#)

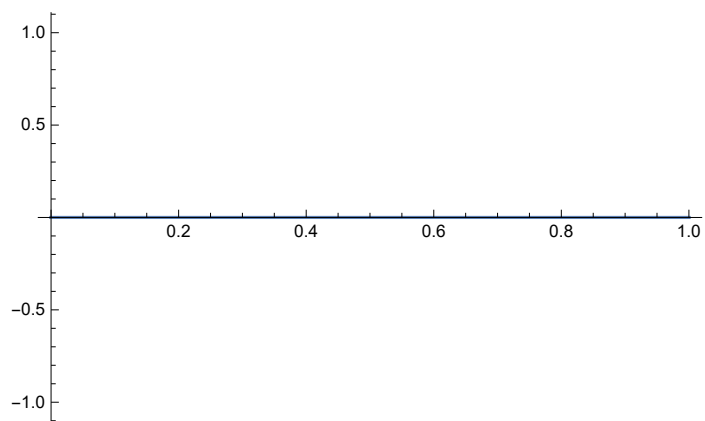

**Plot[Cf[8, 4, 6], {x, 0, 1}]**

[绘图](#)

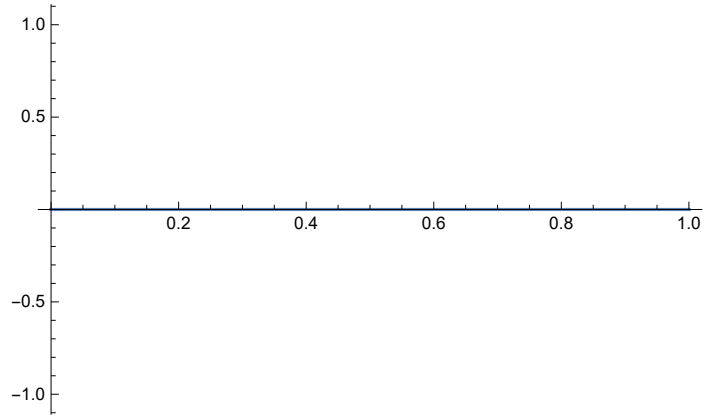

**Plot[Cf[8, 4, 5], {x, 0, 1}]**

[绘图](#)

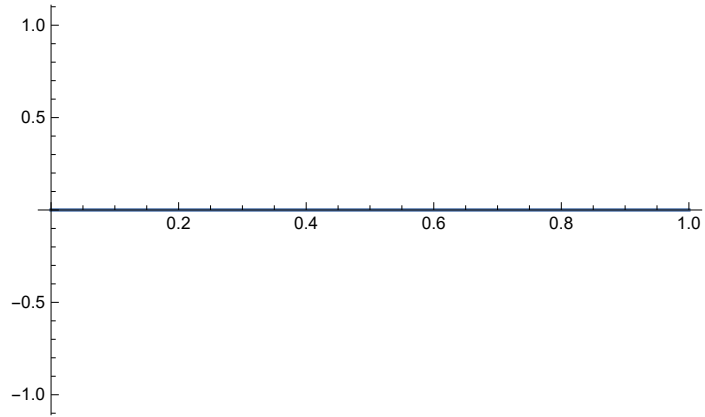

**Plot[Cf[8, 4, 4], {x, 0, 1}]**

[绘图](#)

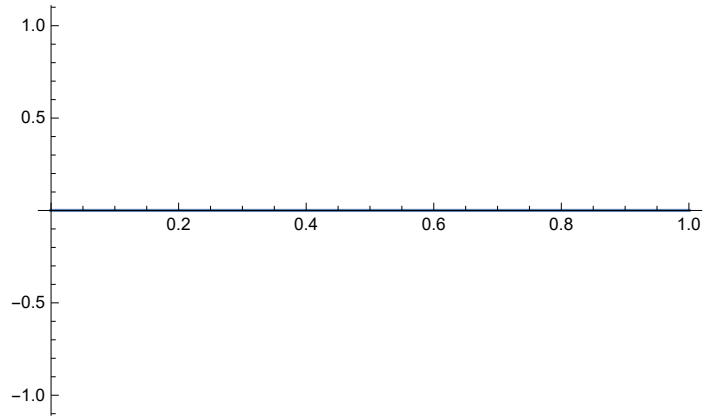

**Plot[Cf[8, 4, 3], {x, 0, 1}]**

[绘图](#)

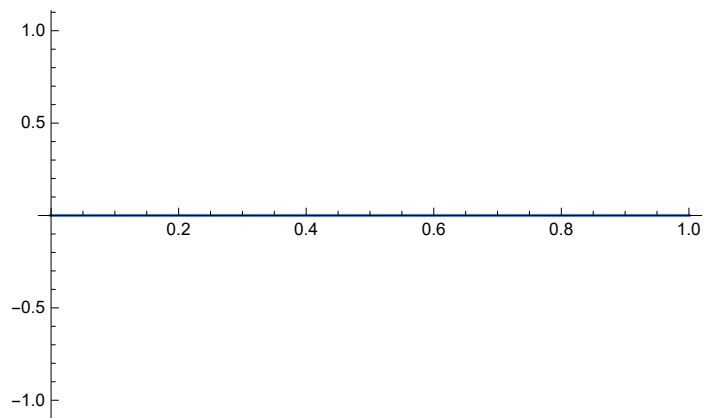

**Plot[Cf[8, 4, 2], {x, 0, 1}]**

[绘图](#)

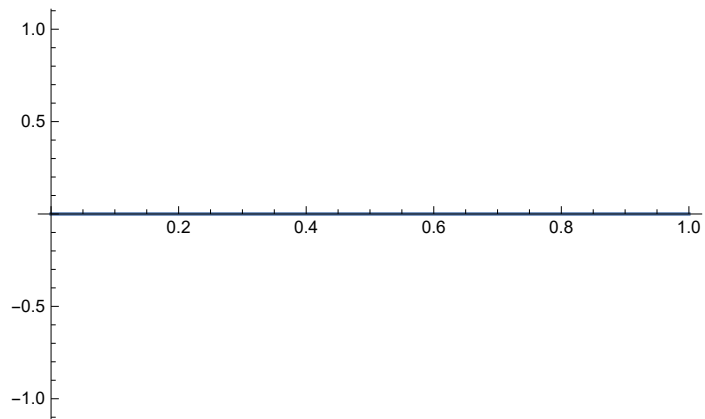

**Plot[Cf[8, 4, 1], {x, 0, 1}]**

[绘图](#)

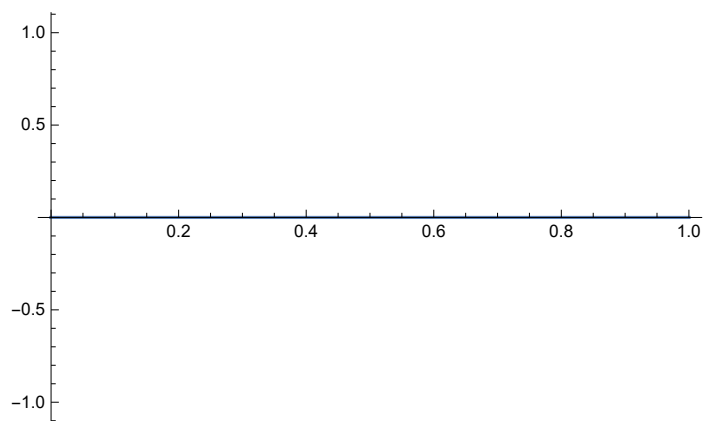

**Plot[Cf[8, 4, 0], {x, 0, 1}]**

[绘图](#)

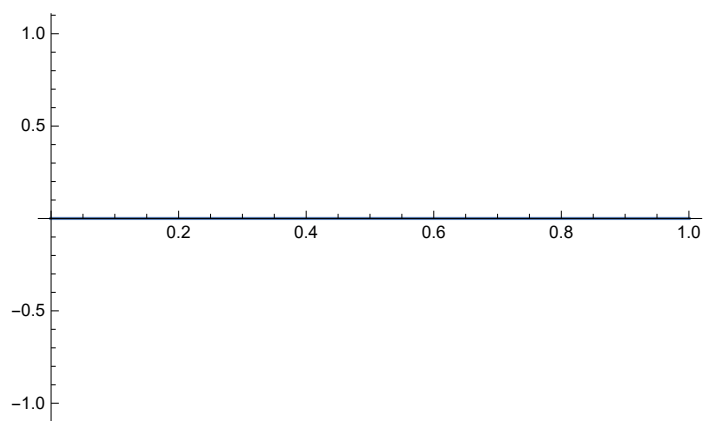

**(\*102th group coefficients r2^8r3^3\*)**

In[1053]:= **Plot[Cf[8, 3, 14], {x, 0, 1}]**

[绘图](#)

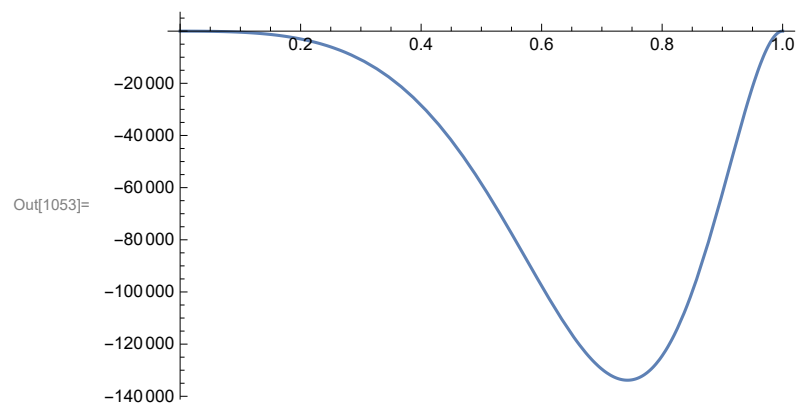

In[1054]:= **Plot[Cf[8, 3, 13], {x, 0, 1}]**

[绘图](#)

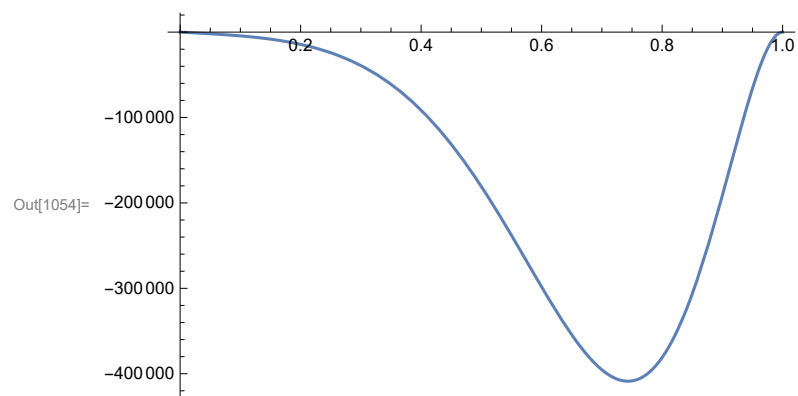



In[1055]:= **Plot**[**Cf**[8, 3, 12], {x, 0, 1}]

[绘图](#)

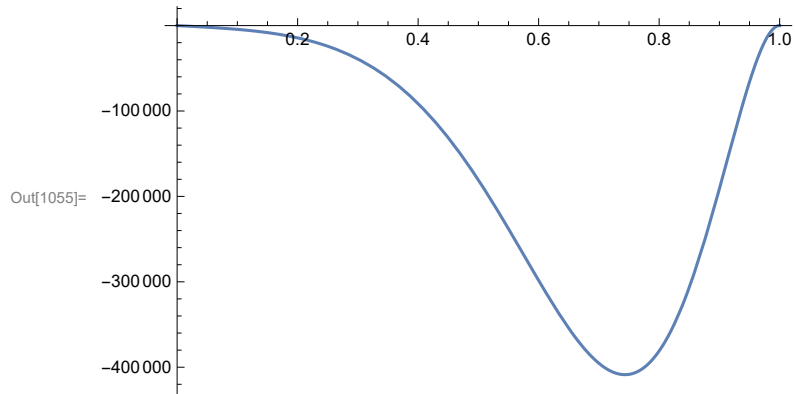

In[1056]:= **Plot**[**Cf**[8, 3, 11], {x, 0, 1}]

[绘图](#)

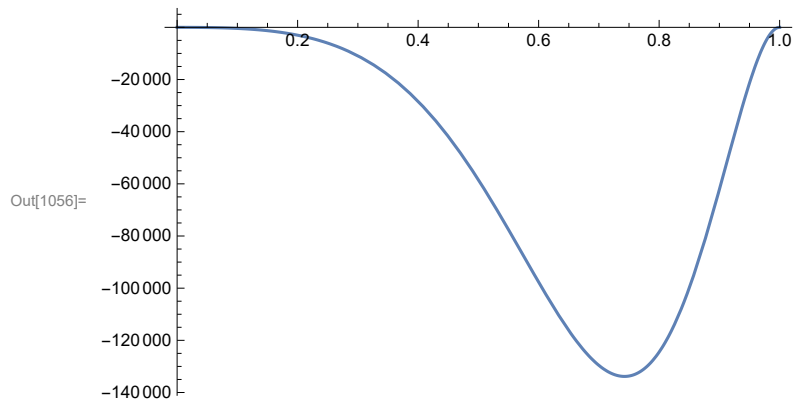

**Plot**[**Cf**[8, 3, 10], {x, 0, 1}]

[绘图](#)

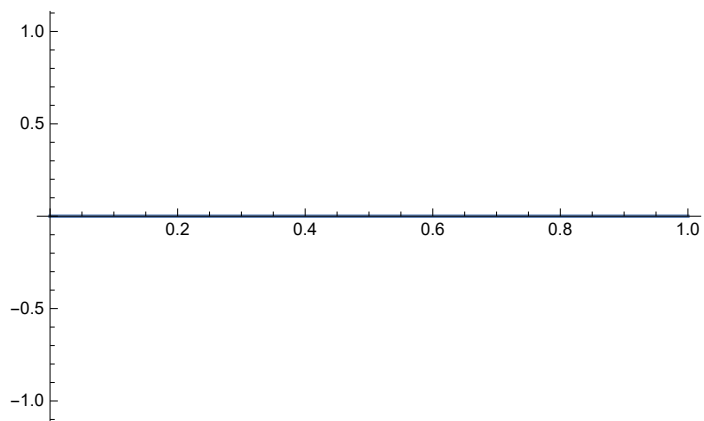

```
Plot[Cf[8, 3, 9], {x, 0, 1}]
```

[绘图](#)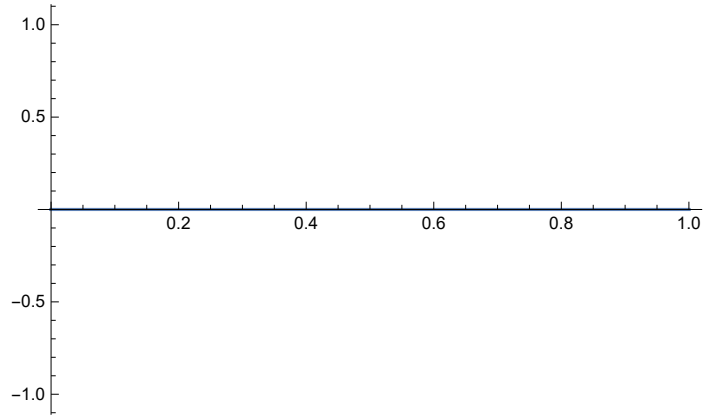

```
Plot[Cf[8, 3, 8], {x, 0, 1}]
```

[绘图](#)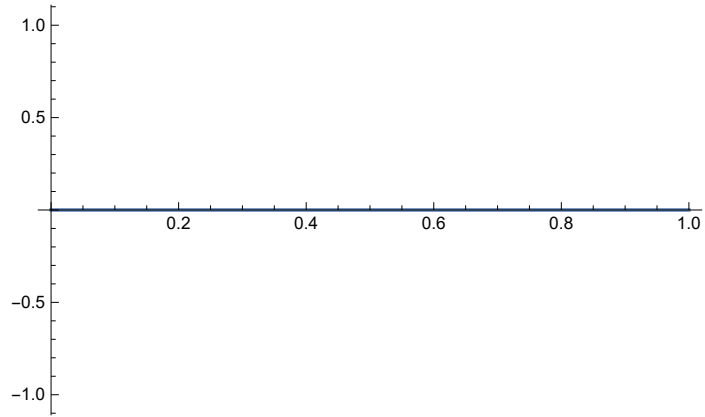

```
Plot[Cf[8, 3, 7], {x, 0, 1}]
```

[绘图](#)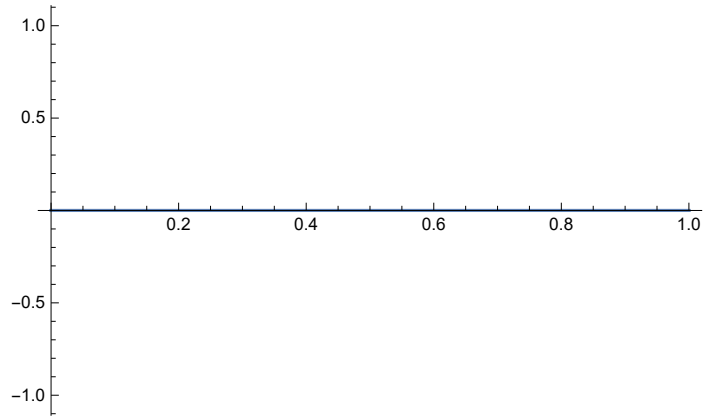

**Plot[Cf[8, 3, 6], {x, 0, 1}]**

[绘图](#)

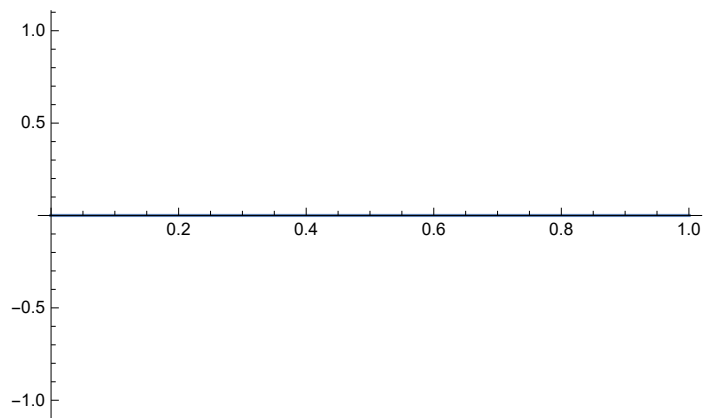

**Plot[Cf[8, 3, 5], {x, 0, 1}]**

[绘图](#)

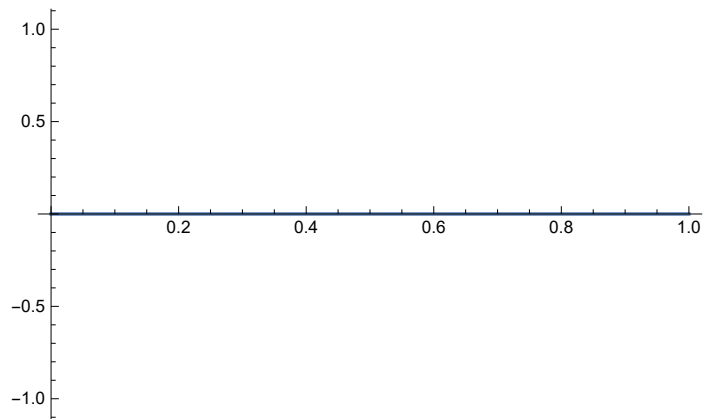

**Plot[Cf[8, 3, 4], {x, 0, 1}]**

[绘图](#)

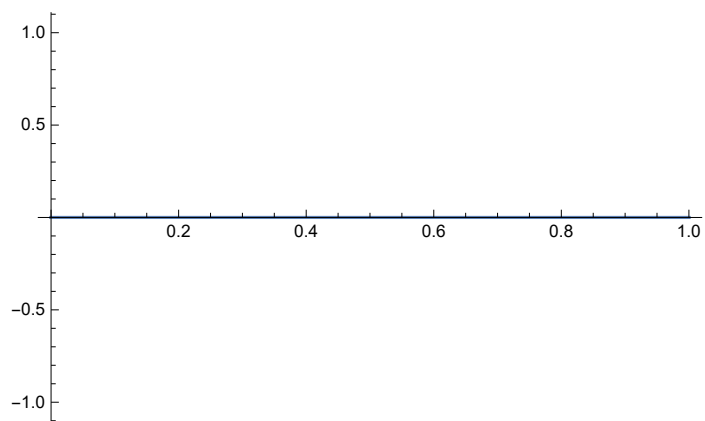

**Plot[Cf[8, 3, 3], {x, 0, 1}]**

[绘图](#)

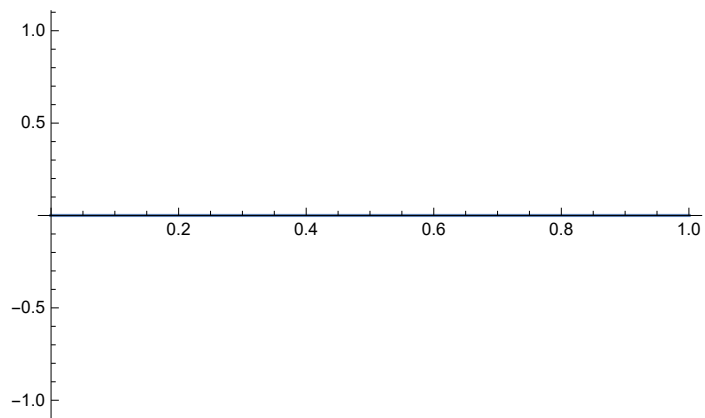

**Plot[Cf[8, 3, 2], {x, 0, 1}]**

[绘图](#)

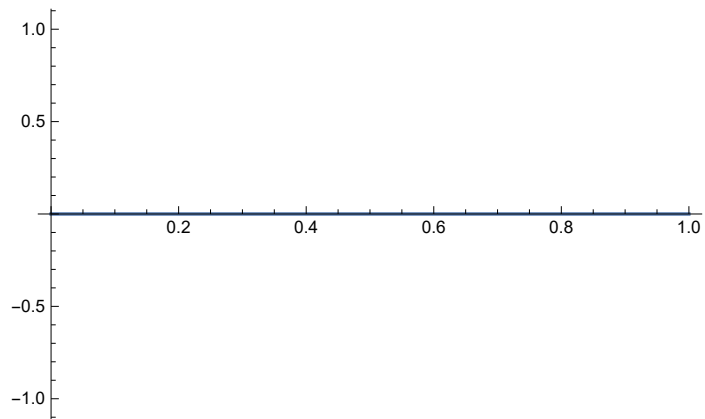

**Plot[Cf[8, 3, 1], {x, 0, 1}]**

[绘图](#)

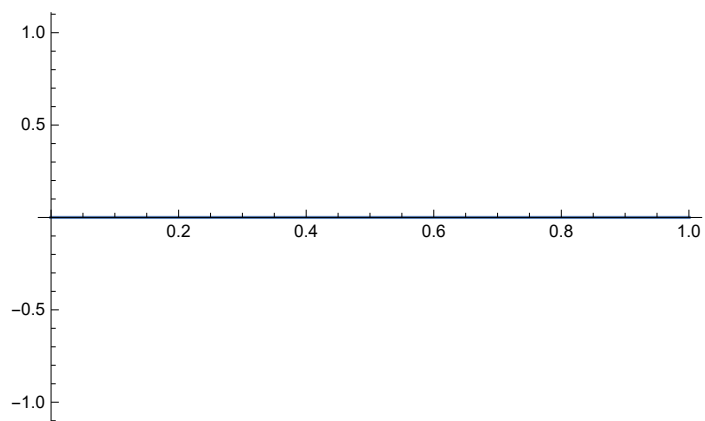

`Plot[Cf[8, 3, 0], {x, 0, 1}]`

[绘图](#)

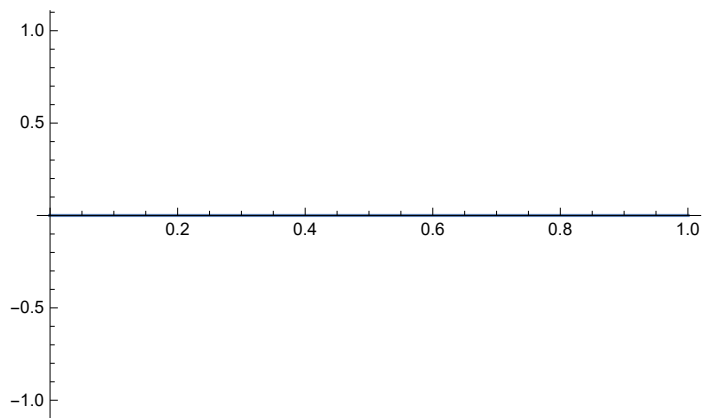

(\*103th group coefficients r2^8r3^2\*)

`In[1057]:= Plot[Cf[8, 2, 14], {x, 0, 1}]`

[绘图](#)

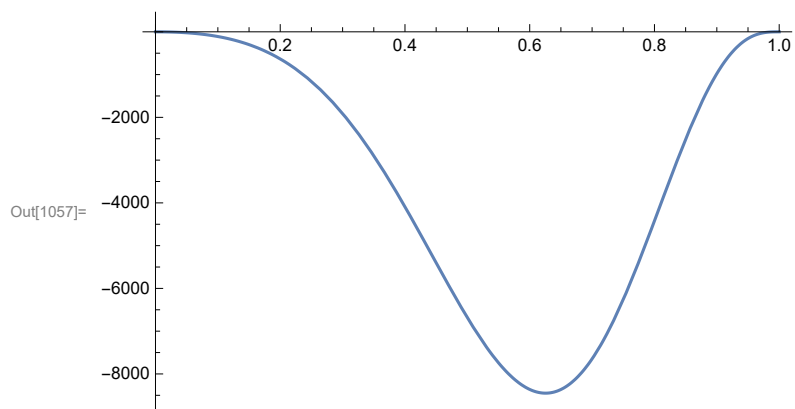

`In[1059]:= Plot[Cf[8, 2, 13], {x, 0, 1}]`

[绘图](#)

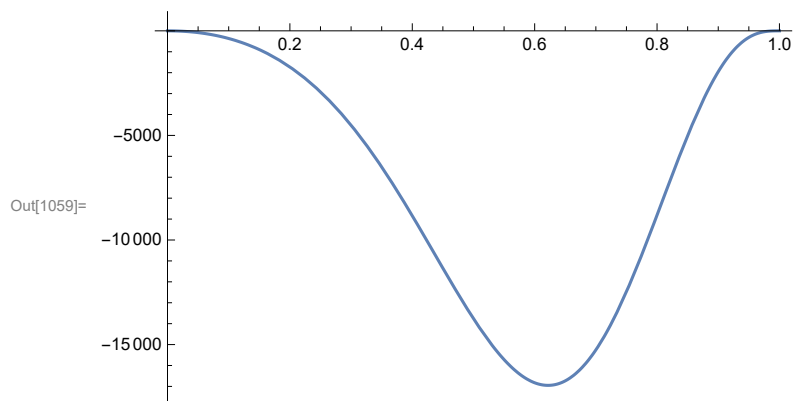

In[1060]:= **Plot[Cf[8, 2, 12], {x, 0, 1}]**

[绘图](#)

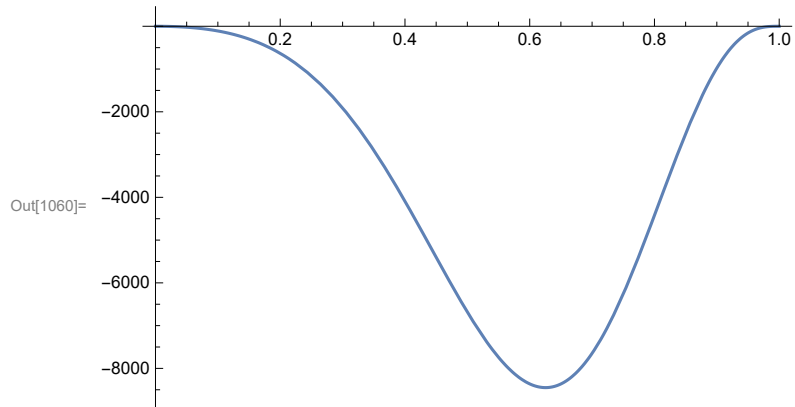

**Plot[Cf[8, 2, 11], {x, 0, 1}]**

[绘图](#)

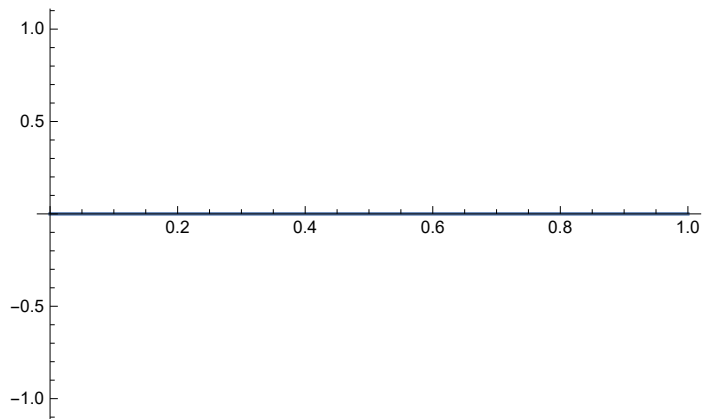

**Plot[Cf[8, 2, 10], {x, 0, 1}]**

[绘图](#)

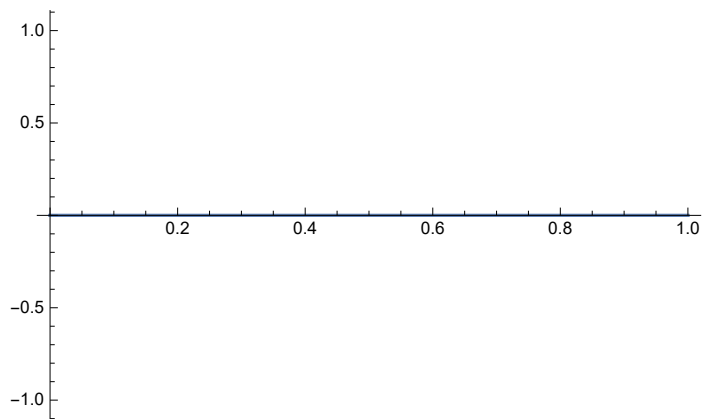

**Plot[Cf[8, 2, 9], {x, 0, 1}]**

[绘图](#)

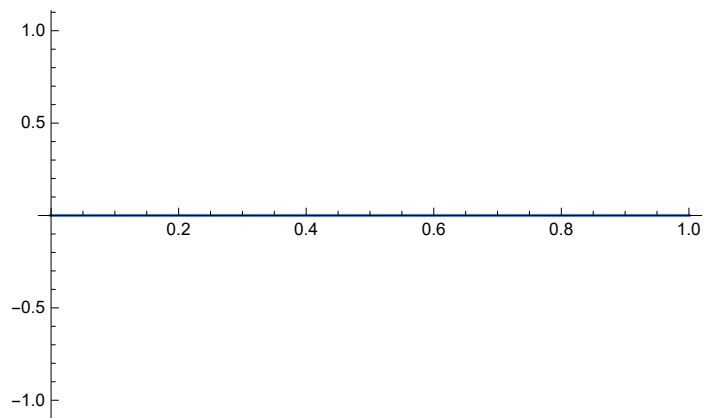

**Plot[Cf[8, 2, 8], {x, 0, 1}]**

[绘图](#)

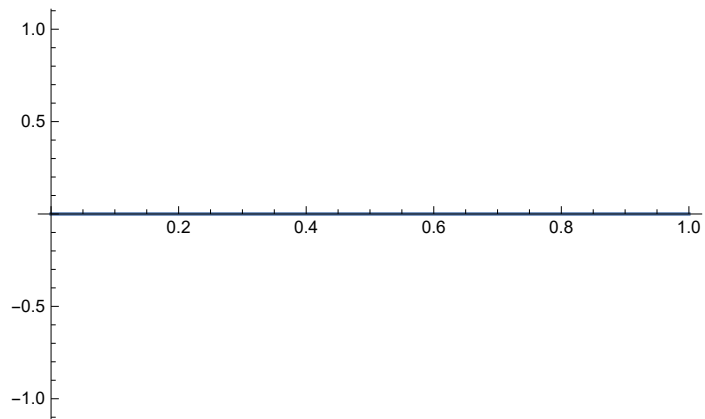

**Plot[Cf[8, 2, 7], {x, 0, 1}]**

[绘图](#)

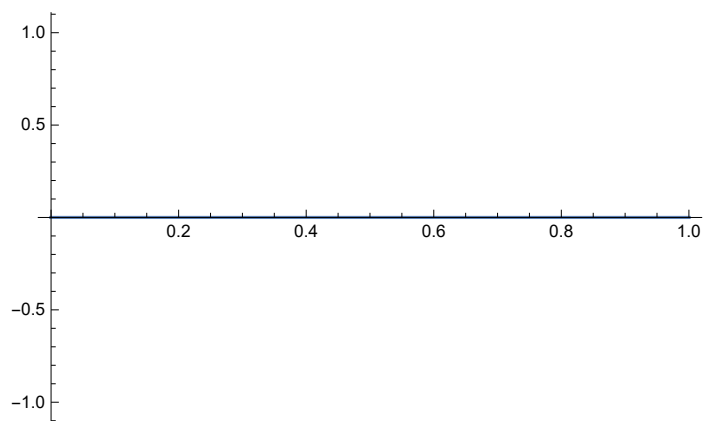

**Plot[Cf[8, 2, 6], {x, 0, 1}]**

[绘图](#)

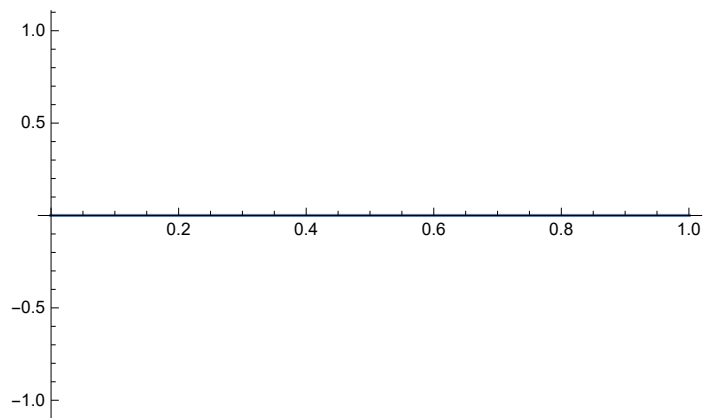

**Plot[Cf[8, 2, 5], {x, 0, 1}]**

[绘图](#)

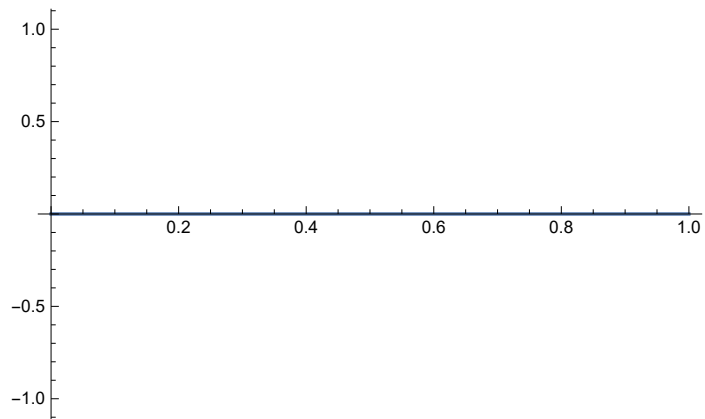

**Plot[Cf[8, 2, 4], {x, 0, 1}]**

[绘图](#)

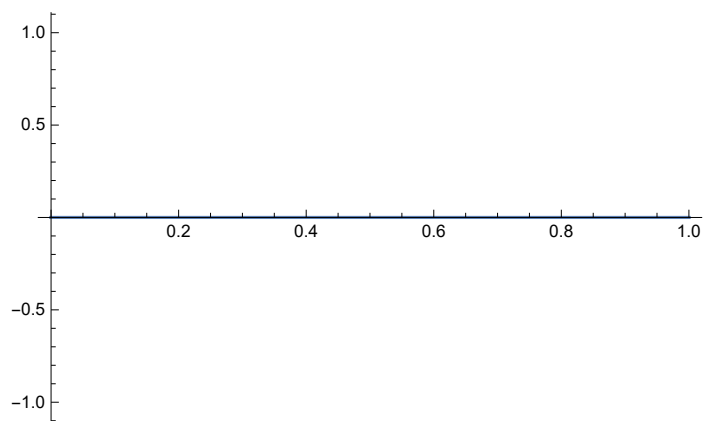



**Plot[Cf[8, 2, 3], {x, 0, 1}]**

[绘图](#)

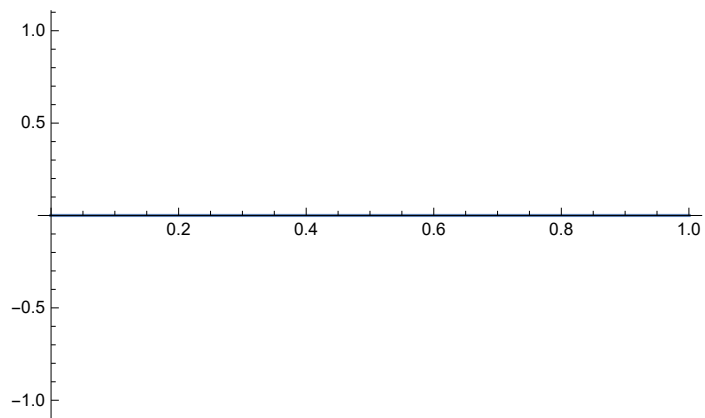

**Plot[Cf[8, 2, 2], {x, 0, 1}]**

[绘图](#)

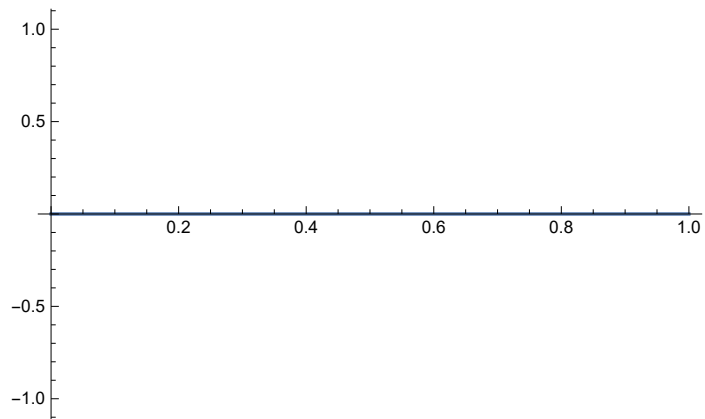

**Plot[Cf[8, 2, 1], {x, 0, 1}]**

[绘图](#)

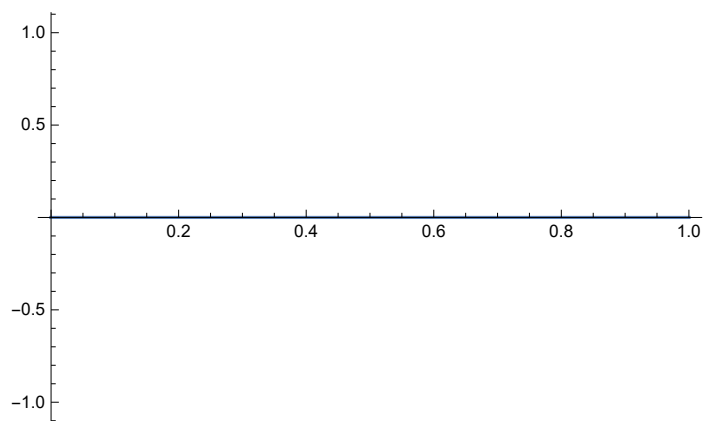

**Plot[Cf[8, 2, 0], {x, 0, 1}]**

[绘图](#)

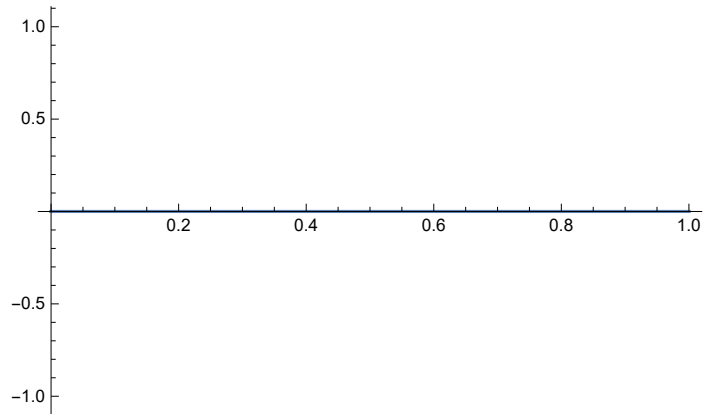

**(\*104th group coefficients r2^8r3^1\*)**

In[1061]:= **Plot[Cf[8, 1, 14], {x, 0, 1}]**

[绘图](#)

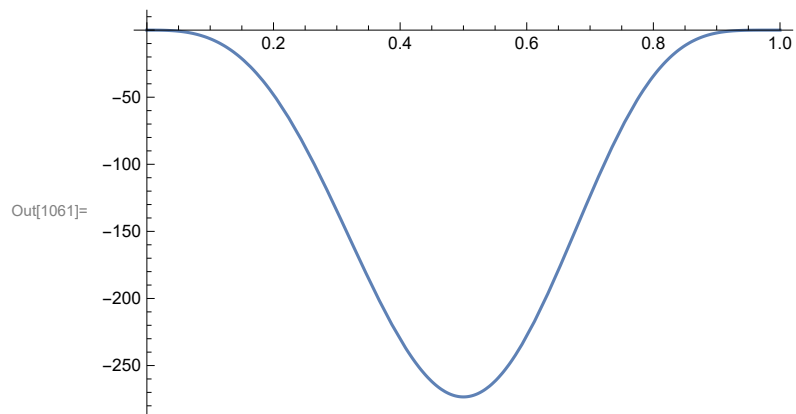

In[1062]:= **Plot[Cf[8, 1, 13], {x, 0, 1}]**

[绘图](#)

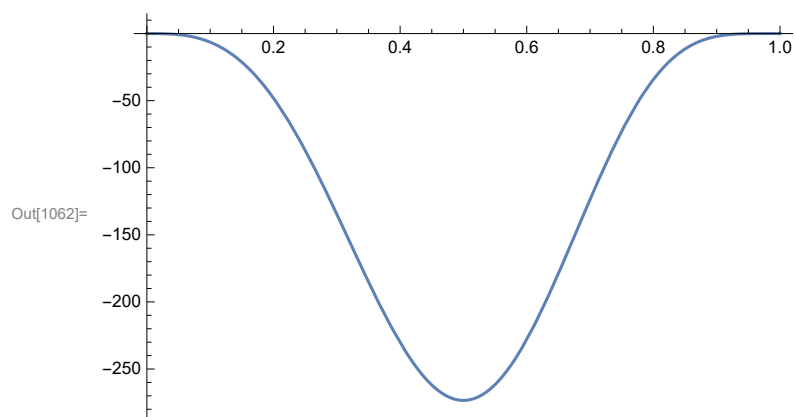

**Plot[Cf[8, 1, 12], {x, 0, 1}]**

[绘图](#)

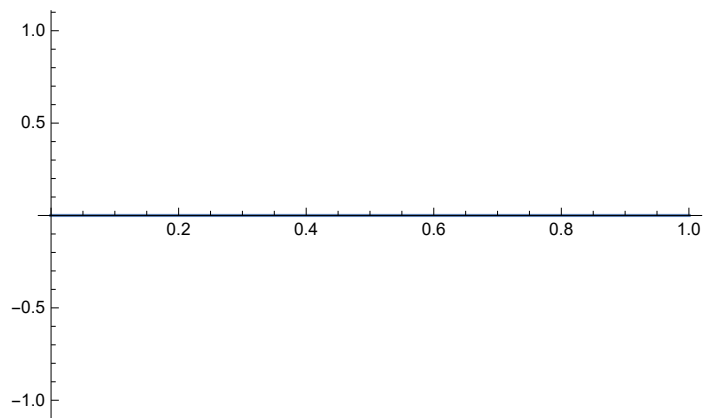

**Plot[Cf[8, 1, 11], {x, 0, 1}]**

[绘图](#)

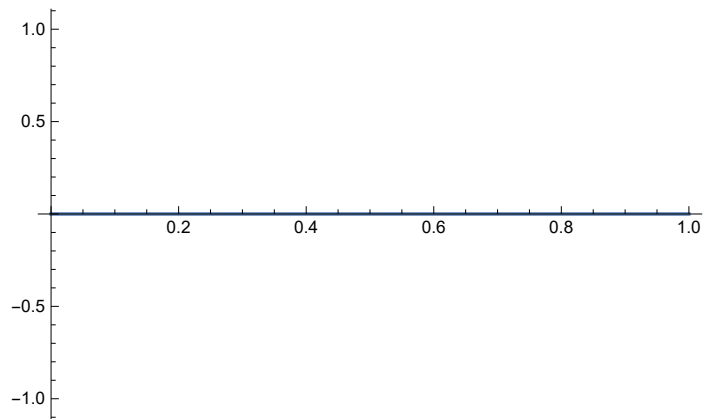

**Plot[Cf[8, 1, 10], {x, 0, 1}]**

[绘图](#)

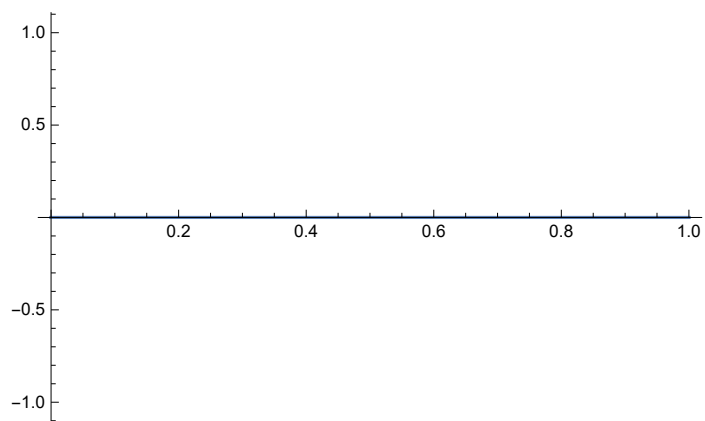

**Plot[Cf[8, 1, 9], {x, 0, 1}]**

[绘图](#)

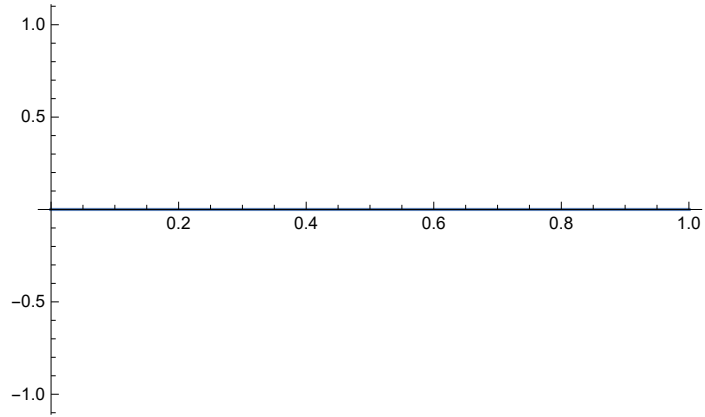

**Plot[Cf[8, 1, 8], {x, 0, 1}]**

[绘图](#)

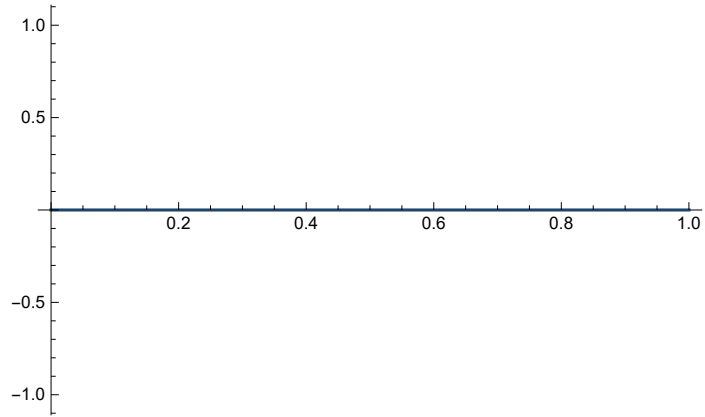

**Plot[Cf[8, 1, 7], {x, 0, 1}]**

[绘图](#)

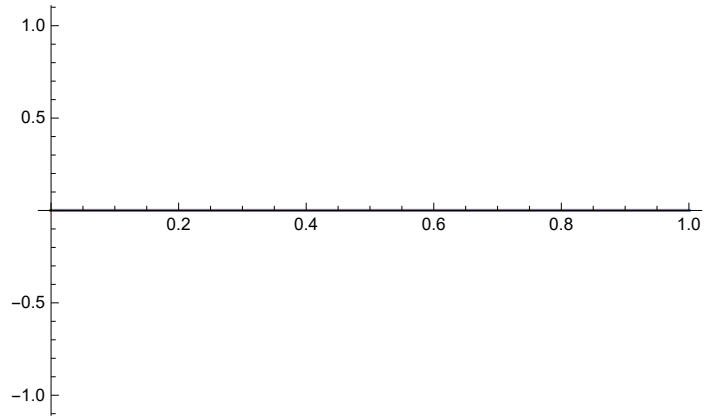

**Plot[Cf[8, 1, 6], {x, 0, 1}]**

[绘图](#)

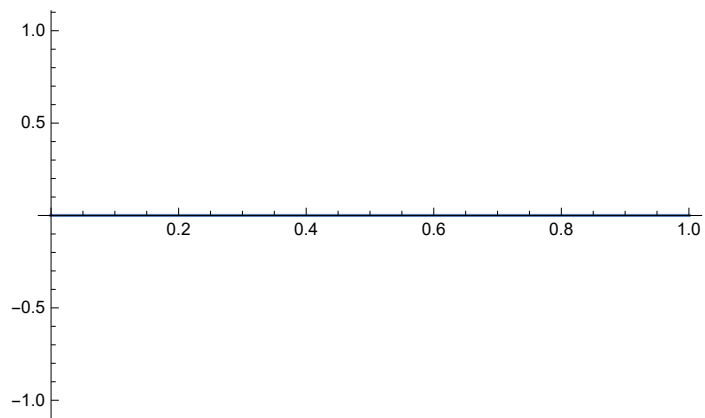

**Plot[Cf[8, 1, 5], {x, 0, 1}]**

[绘图](#)

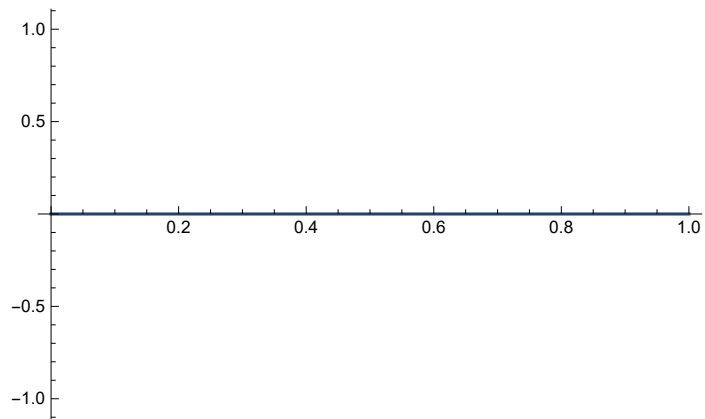

**Plot[Cf[8, 1, 4], {x, 0, 1}]**

[绘图](#)

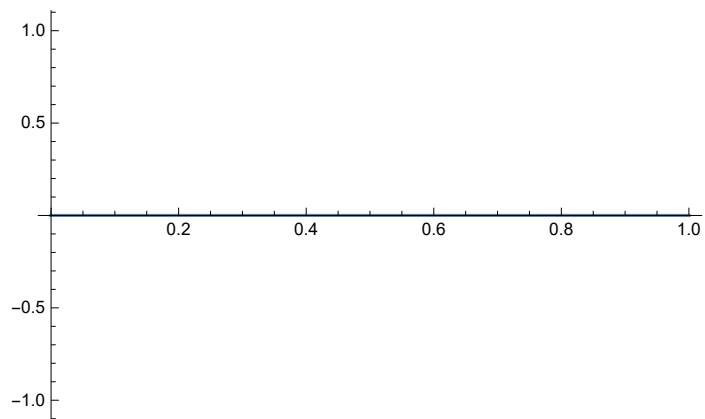

**Plot[Cf[8, 1, 3], {x, 0, 1}]**

[绘图](#)

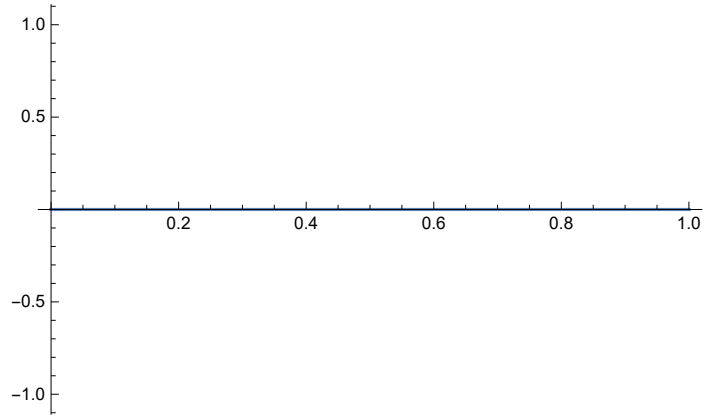

**Plot[Cf[8, 1, 2], {x, 0, 1}]**

[绘图](#)

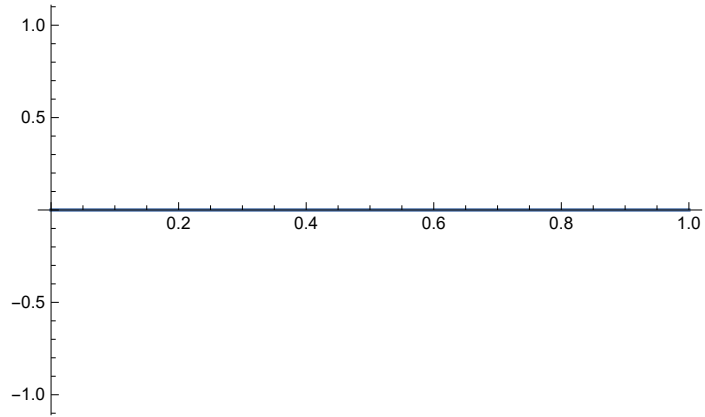

**Plot[Cf[8, 1, 1], {x, 0, 1}]**

[绘图](#)

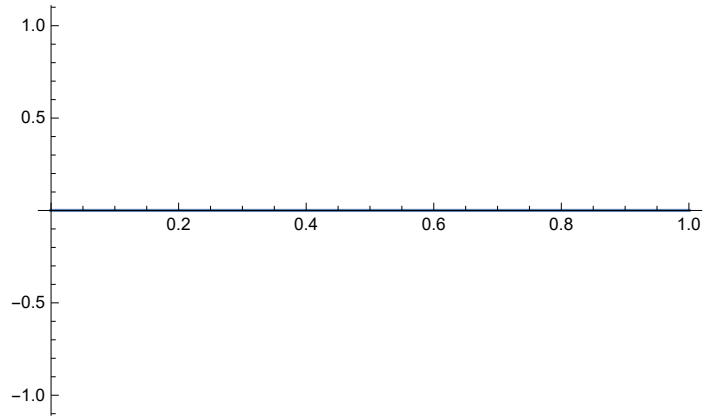

**Plot[Cf[8, 1, 0], {x, 0, 1}]**

[绘图](#)

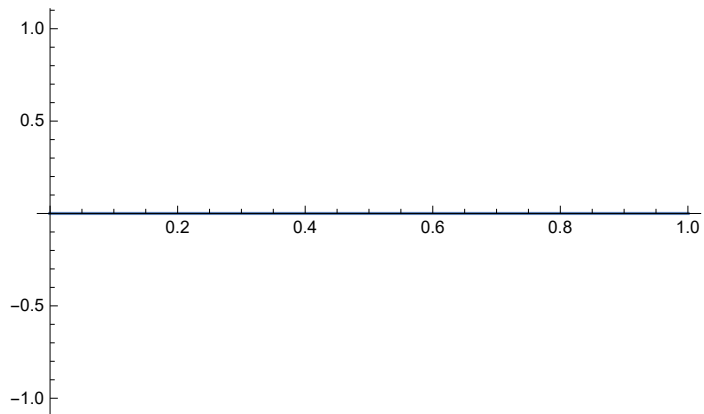

**(\*105th group coefficients r2^8r3^0\*)**

**Plot[Cf[8, 0, 14], {x, 0, 1}]**

[绘图](#)

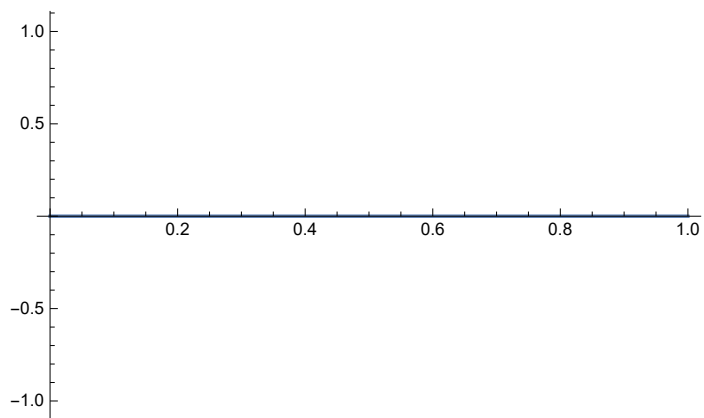

**Plot[Cf[8, 0, 13], {x, 0, 1}]**

[绘图](#)

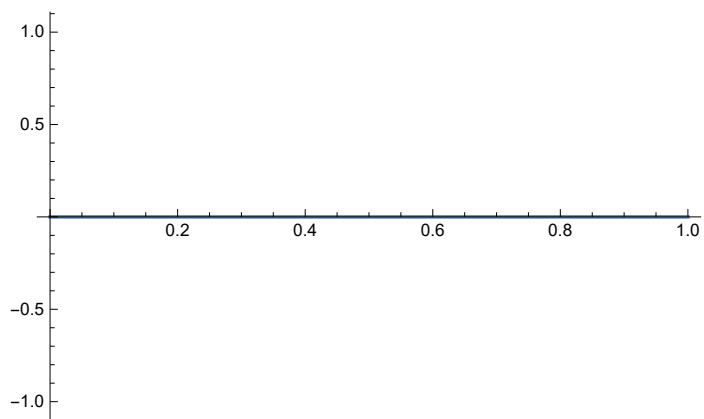

```
Plot[Cf[8, 0, 12], {x, 0, 1}]
```

[绘图](#)

```
Plot[Cf[8, 0, 11], {x, 0, 1}]
```

[绘图](#)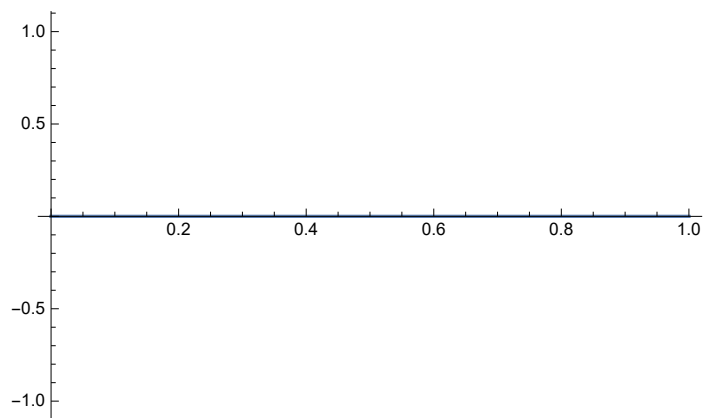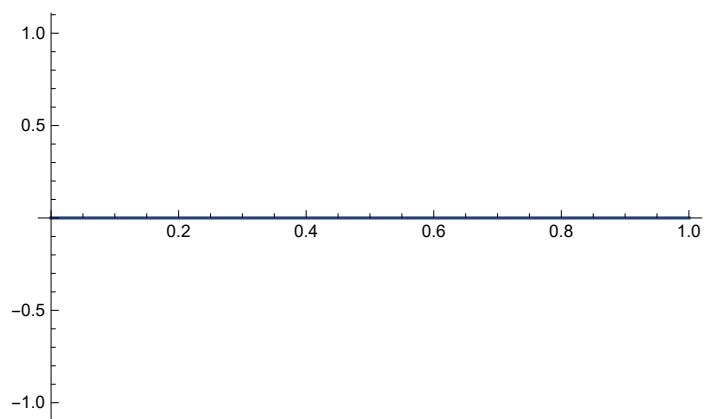

```
Plot[Cf[8, 0, 10], {x, 0, 1}]
```

[绘图](#)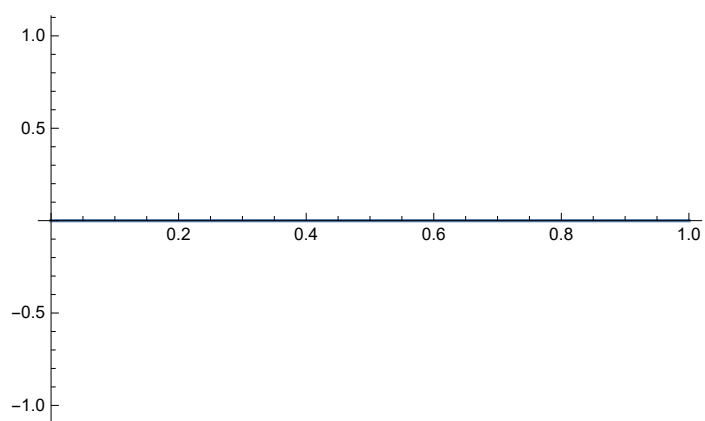



**Plot[Cf[8, 0, 9], {x, 0, 1}]**

[绘图](#)

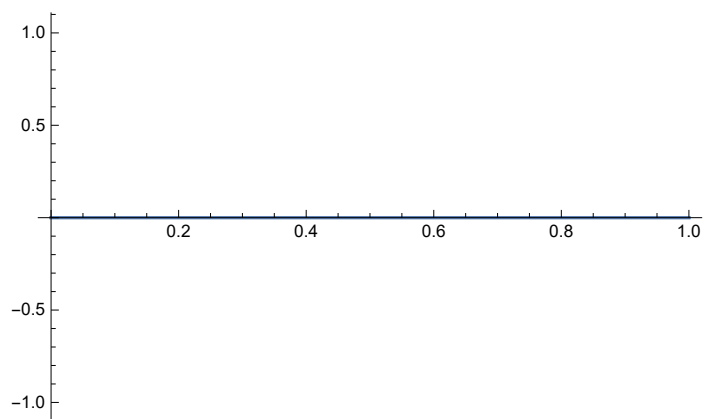

**Plot[Cf[8, 0, 8], {x, 0, 1}]**

[绘图](#)

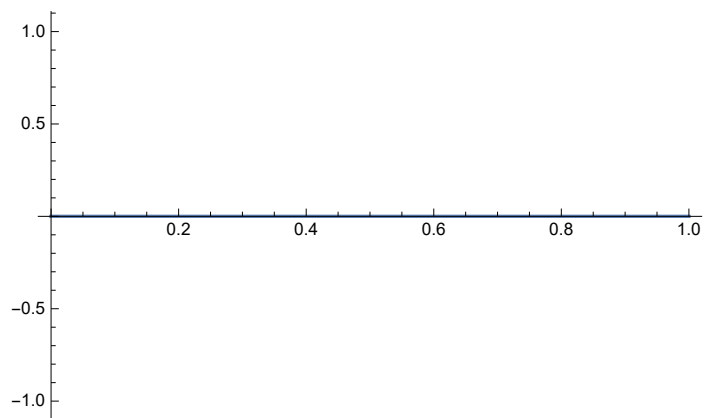

**Plot[Cf[8, 0, 7], {x, 0, 1}]**

[绘图](#)

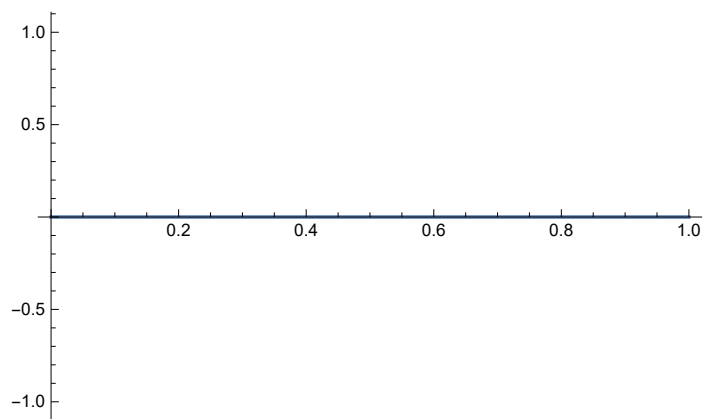

```
Plot[Cf[8, 0, 6], {x, 0, 1}]
```

[绘图](#)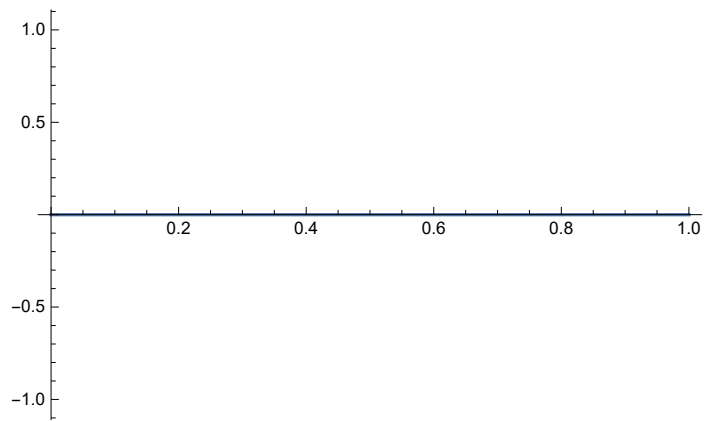

```
Plot[Cf[8, 0, 5], {x, 0, 1}]
```

[绘图](#)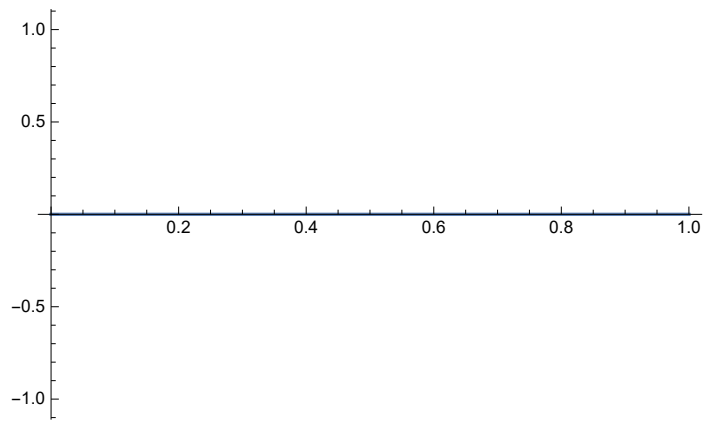

```
Plot[Cf[8, 0, 4], {x, 0, 1}]
```

[绘图](#)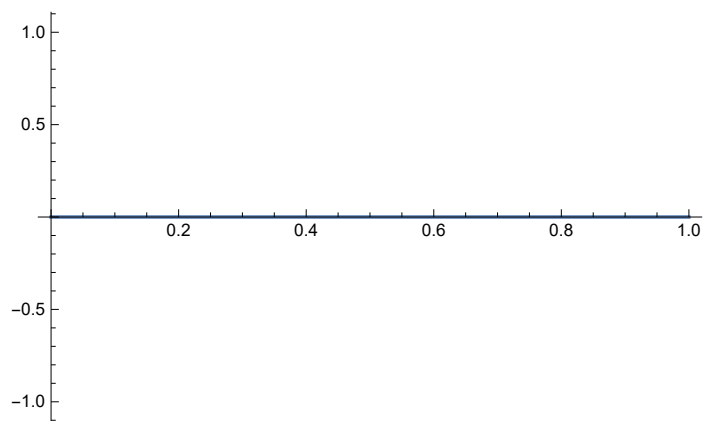

```
Plot[Cf[8, 0, 3], {x, 0, 1}]
```

[绘图](#)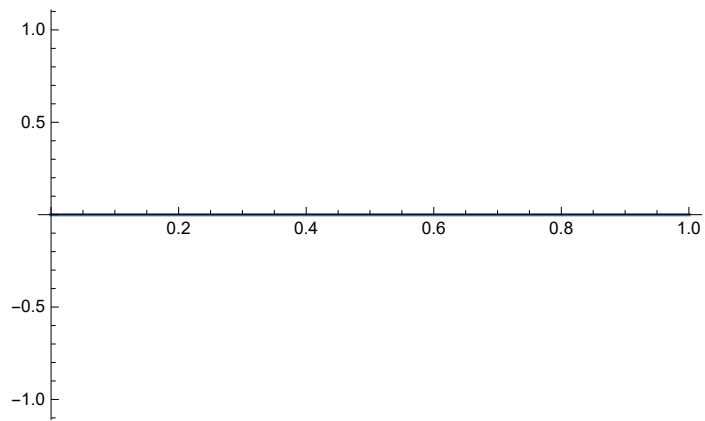

```
Plot[Cf[8, 0, 2], {x, 0, 1}]
```

[绘图](#)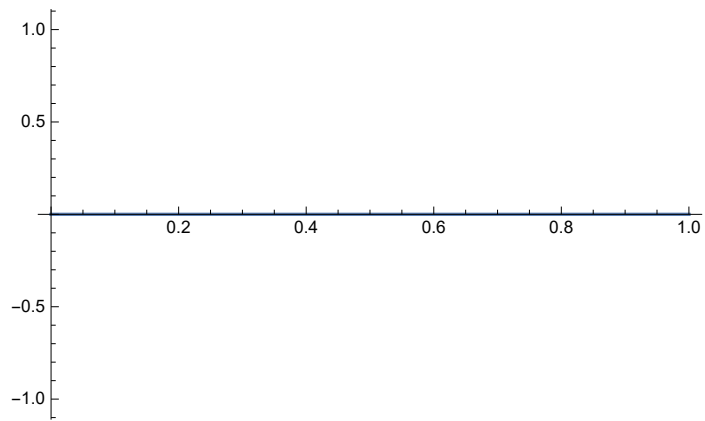

```
Plot[Cf[8, 0, 1], {x, 0, 1}]
```

[绘图](#)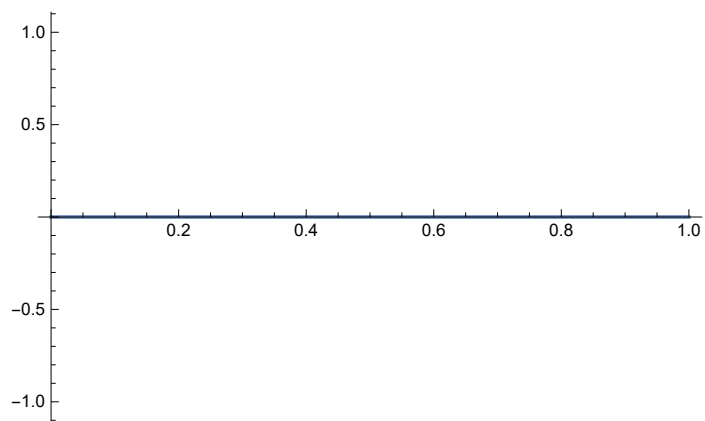

**Plot[Cf[8, 0, 0], {x, 0, 1}]**

[绘图](#)

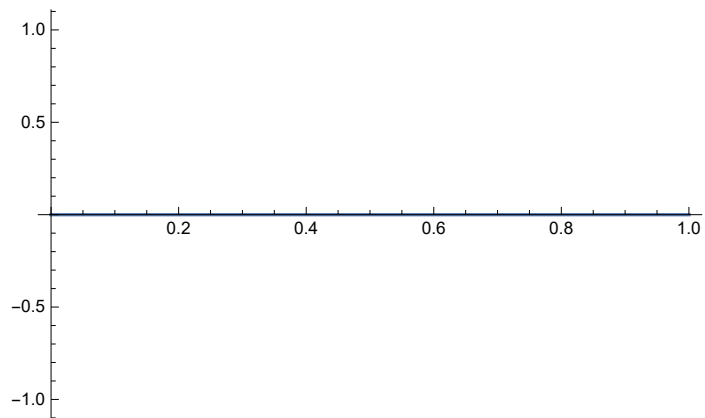

**(\*106th group coefficients r2^7r3^14\*)**

**Plot[Cf[7, 14, 14], {x, 0, 1}]**

[绘图](#)

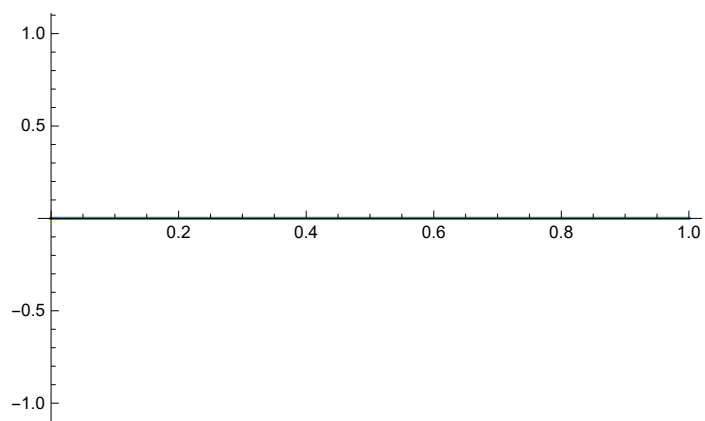

In[1063]:= **Plot[Cf[7, 14, 13], {x, 0, 1}]**

[绘图](#)

Out[1063]=

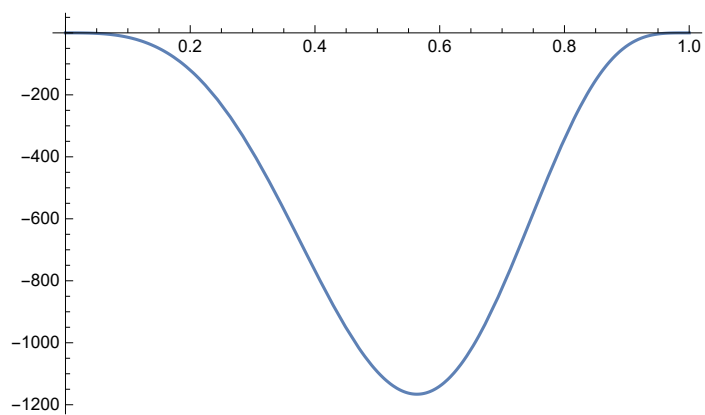

In[1064]:= **Plot[Cf[7, 14, 12], {x, 0, 1}]**

[绘图](#)

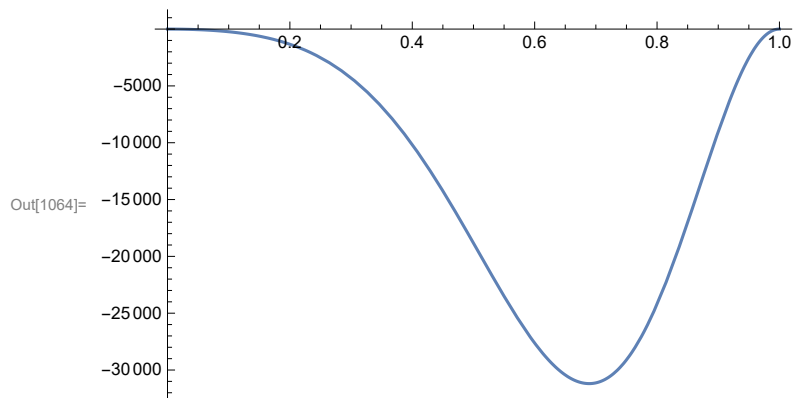

In[1065]:= **Plot[Cf[7, 14, 11], {x, 0, 1}]**

[绘图](#)

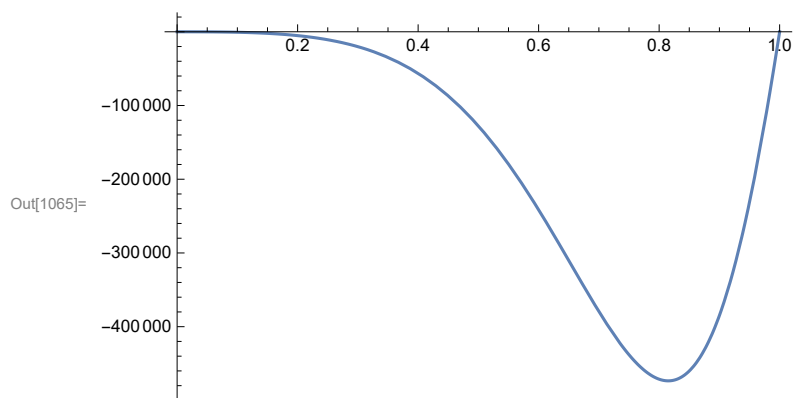

In[1066]:= **Plot[Cf[7, 14, 10], {x, 0, 1}]**

[绘图](#)

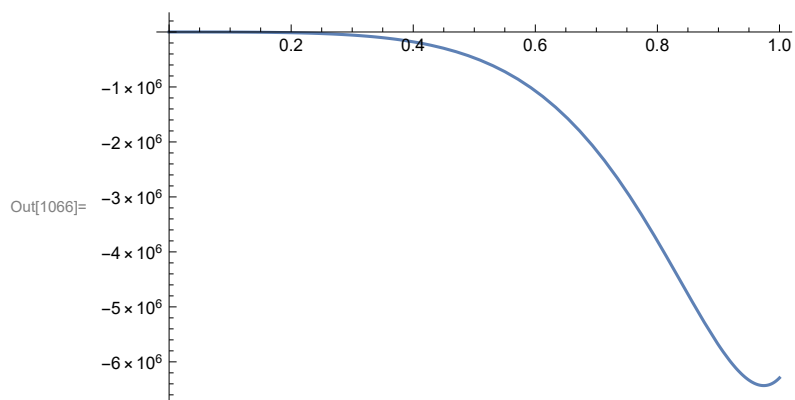

```
In[1067]:= Plot[Cf[7, 14, 9], {x, 0, 1}]
```

[绘图](#)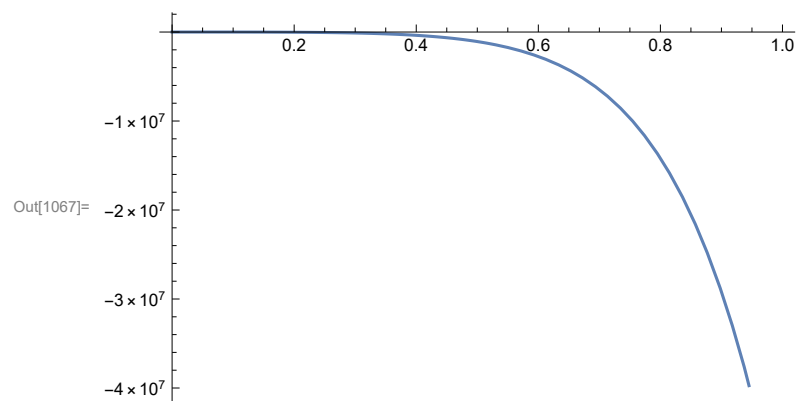

```
In[1068]:= Plot[Cf[7, 14, 8], {x, 0, 1}]
```

[绘图](#)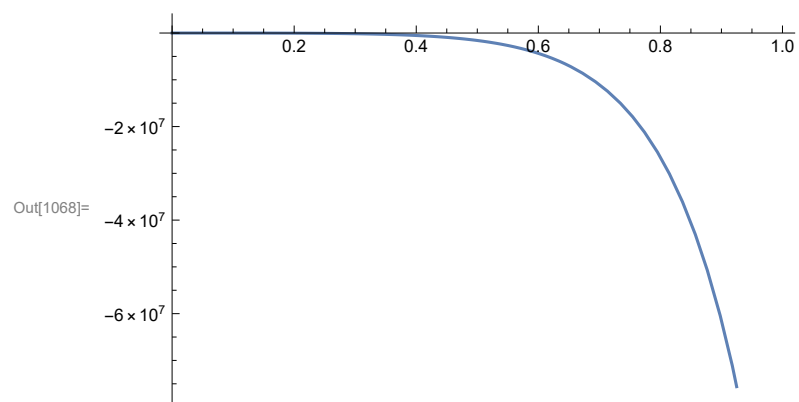

```
In[1069]:= Plot[Cf[7, 14, 7], {x, 0, 1}]
```

[绘图](#)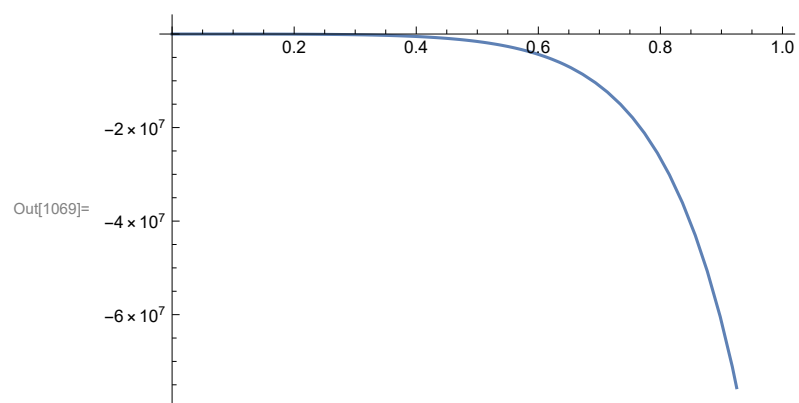

In[1070]:= **Plot[Cf[7, 14, 6], {x, 0, 1}]**

[绘图](#)

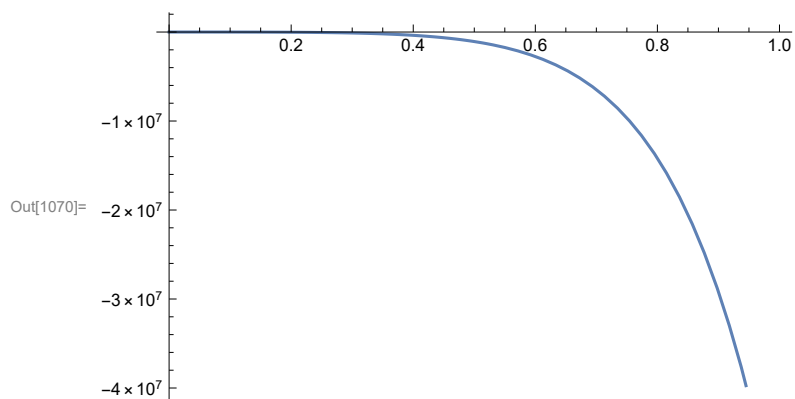

In[1071]:= **Plot[Cf[7, 14, 5], {x, 0, 1}]**

[绘图](#)

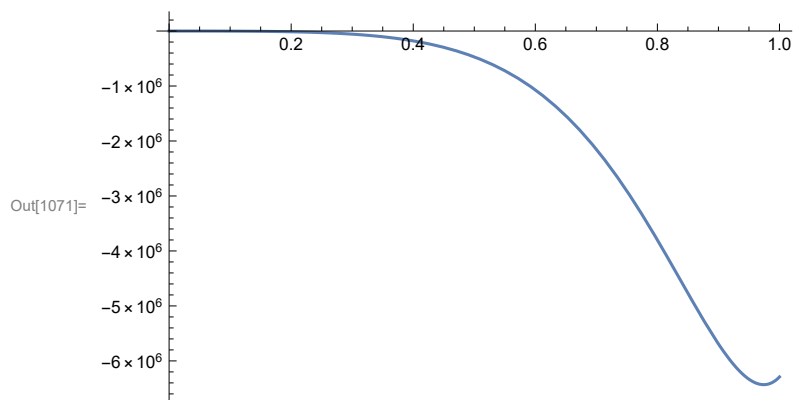

In[1072]:= **Plot[Cf[7, 14, 4], {x, 0, 1}]**

[绘图](#)

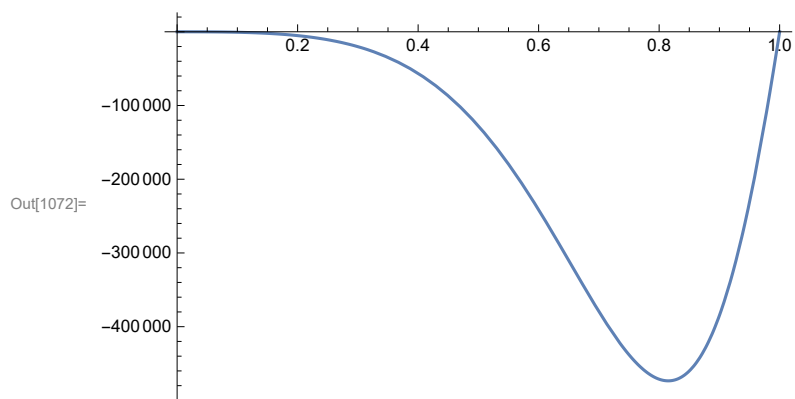

```
In[1073]:= Plot[Cf[7, 14, 3], {x, 0, 1}]
```

[绘图](#)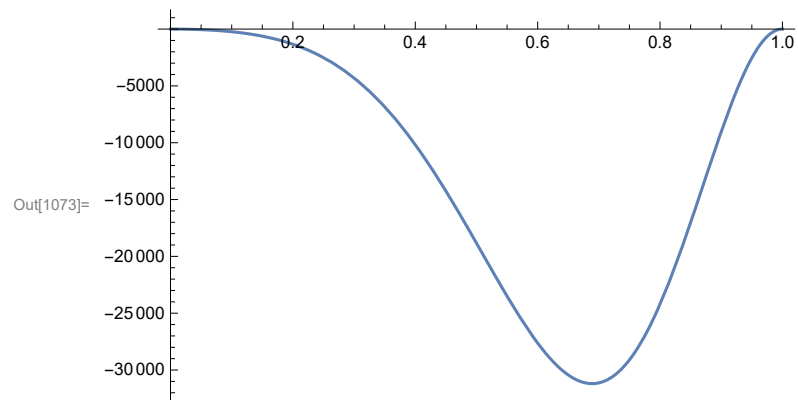

```
In[1074]:= Plot[Cf[7, 14, 2], {x, 0, 1}]
```

[绘图](#)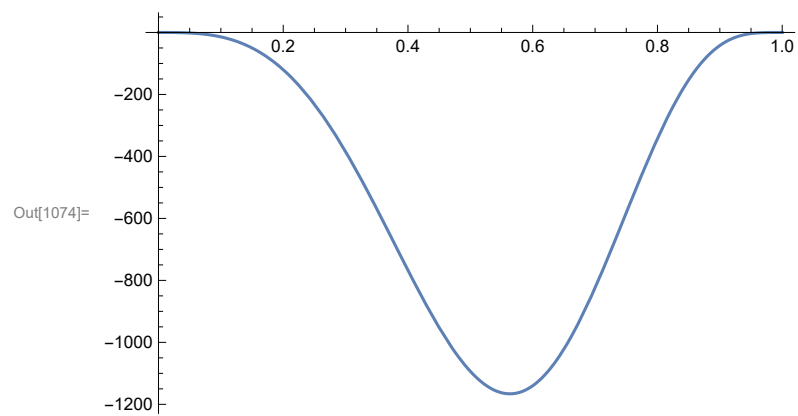

```
Plot[Cf[7, 14, 1], {x, 0, 1}]
```

[绘图](#)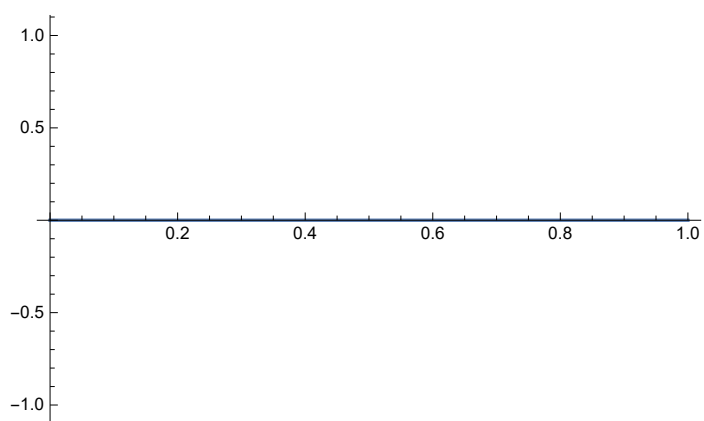



`Plot[Cf[7, 14, 0], {x, 0, 1}]`

[绘图](#)

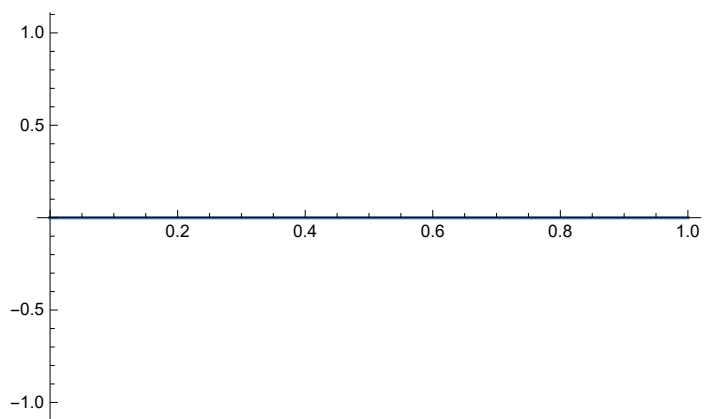

(\*107th group coefficients r2^7r3^13\*)

`Plot[Cf[7, 13, 14], {x, 0, 1}]`

[绘图](#)

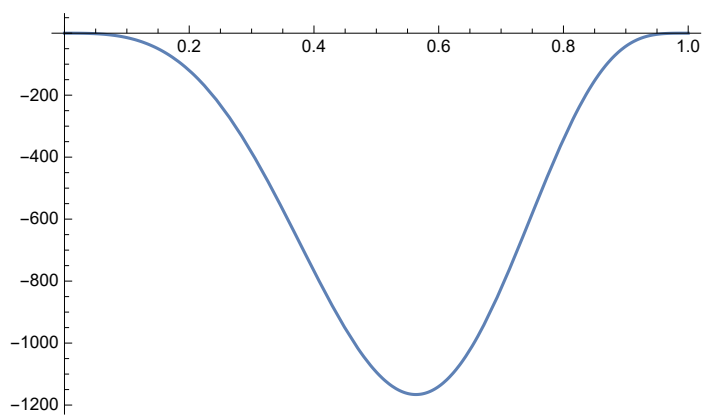

`Plot[Cf[7, 13, 13], {x, 0, 1}]`

[绘图](#)

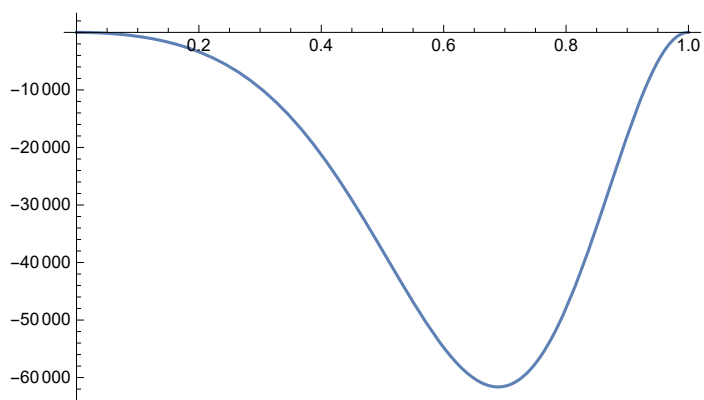

```
Plot[Cf[7, 13, 12], {x, 0, 1}]
```

[绘图](#)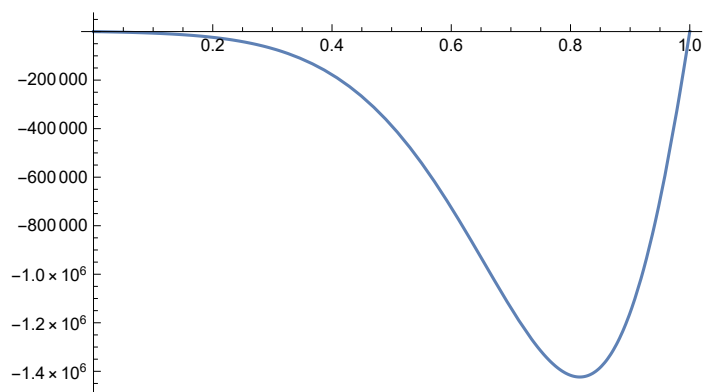

```
Plot[Cf[7, 13, 11], {x, 0, 1}]
```

[绘图](#)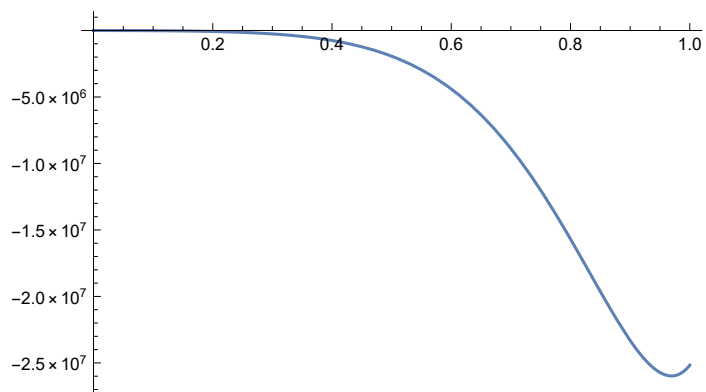

```
Plot[Cf[7, 13, 10], {x, 0, 1}]
```

[绘图](#)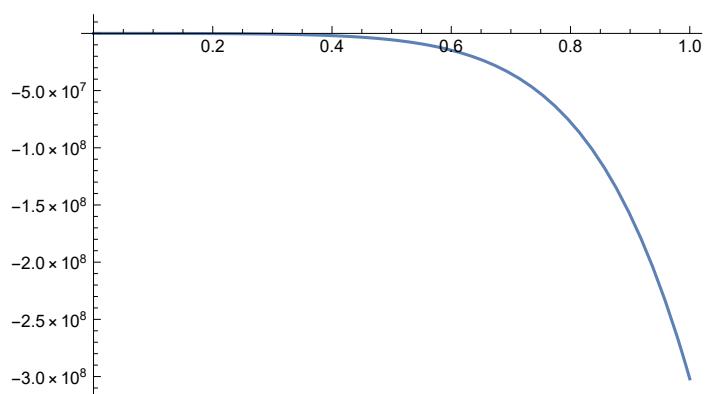

**Plot[Cf[7, 13, 9], {x, 0, 1}]**

[绘图](#)

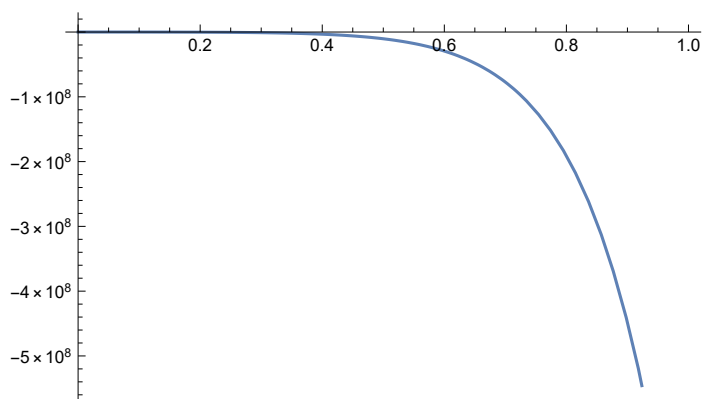

**Plot[Cf[7, 13, 8], {x, 0, 1}]**

[绘图](#)

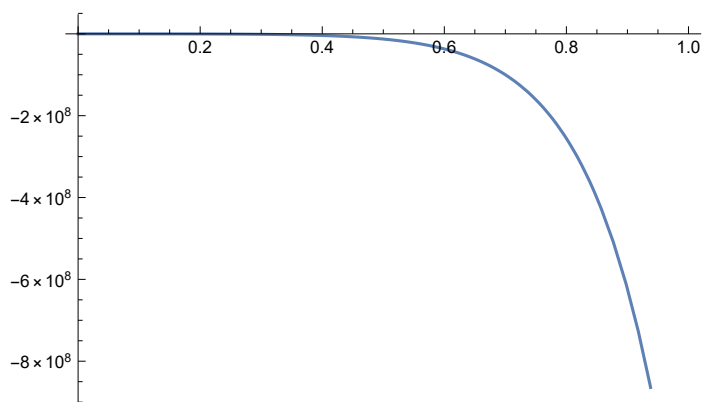

**Plot[Cf[7, 13, 7], {x, 0, 1}]**

[绘图](#)

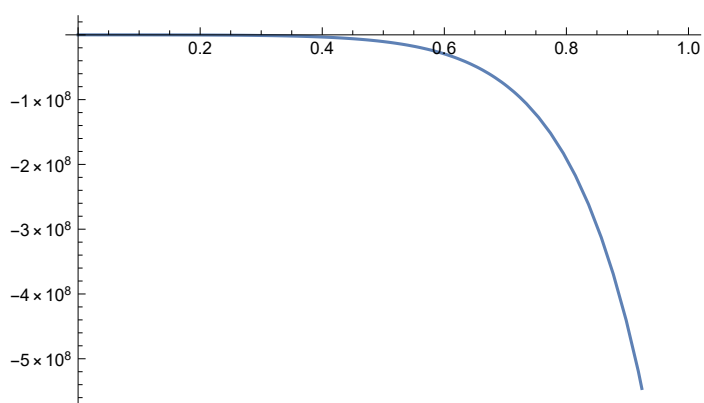

```
Plot[Cf[7, 13, 6], {x, 0, 1}]
```

[绘图](#)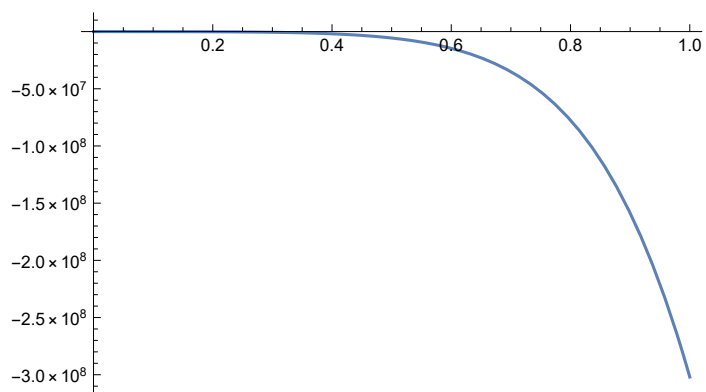

```
Plot[Cf[7, 13, 5], {x, 0, 1}]
```

[绘图](#)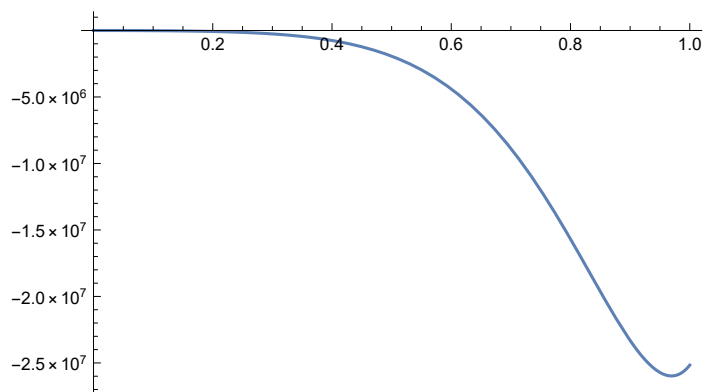

```
Plot[Cf[7, 13, 4], {x, 0, 1}]
```

[绘图](#)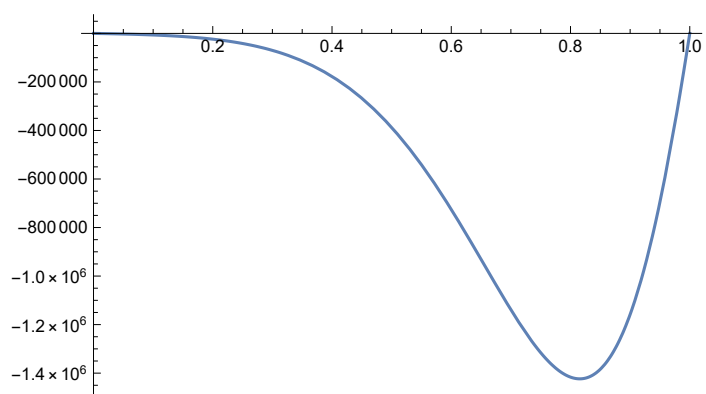

**Plot[Cf[7, 13, 3], {x, 0, 1}]**

[绘图](#)

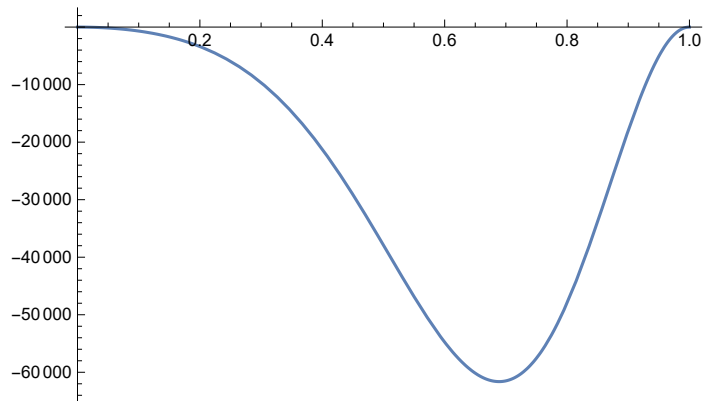

**Plot[Cf[7, 13, 2], {x, 0, 1}]**

[绘图](#)

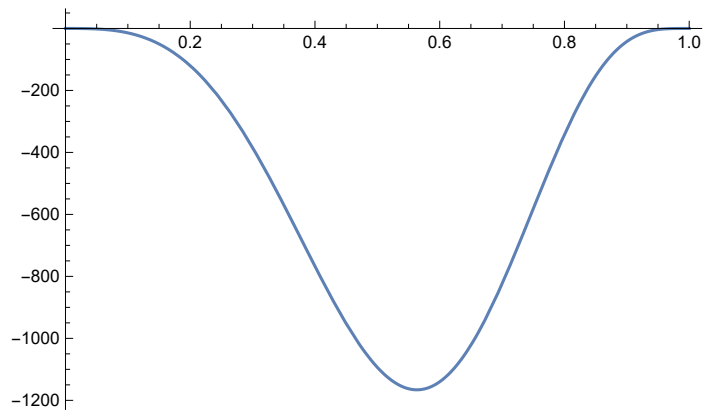

**Plot[Cf[7, 13, 1], {x, 0, 1}]**

[绘图](#)

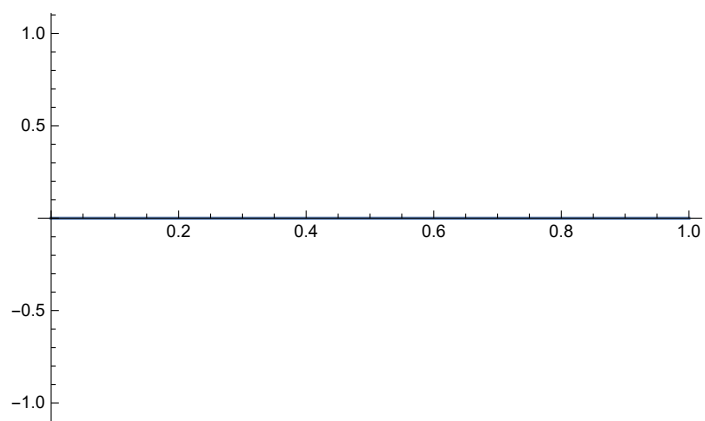

**Plot[Cf[7, 13, 0], {x, 0, 1}]**

[绘图](#)

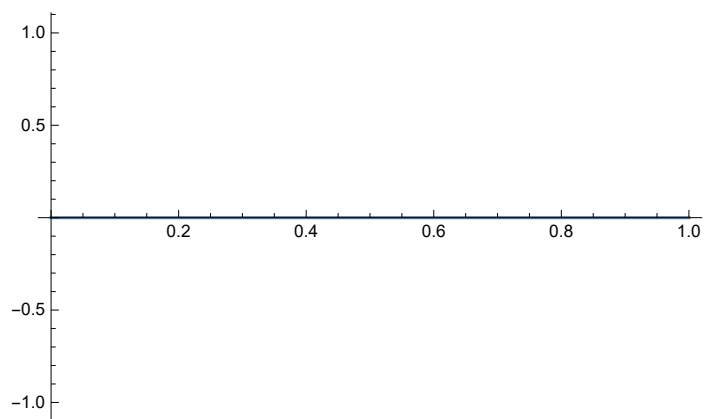

(\*108th group coefficients r2^7r3^12\*)

**Plot[Cf[7, 12, 14], {x, 0, 1}]**

[绘图](#)

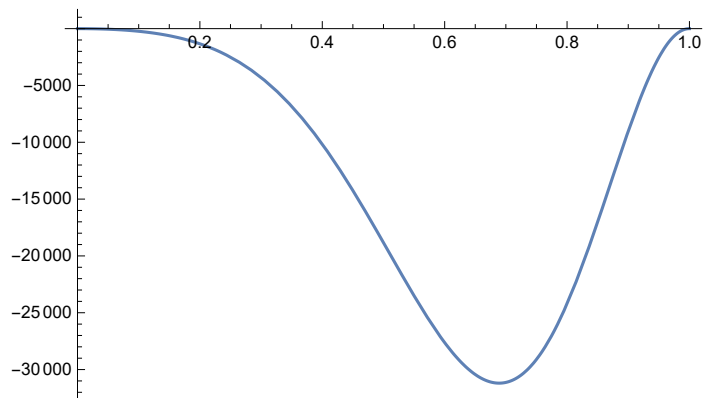

**Plot[Cf[7, 12, 13], {x, 0, 1}]**

[绘图](#)

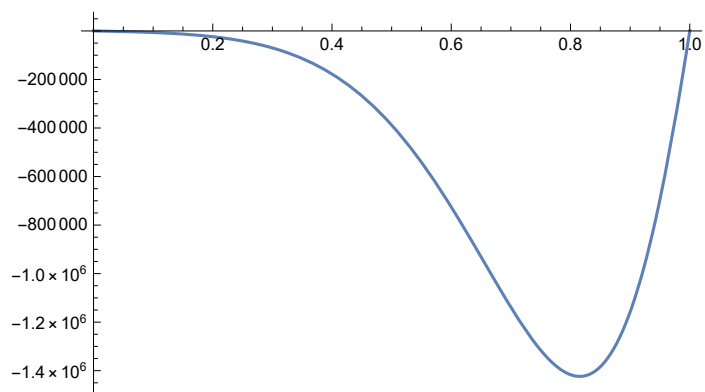

**Plot[Cf[7, 12, 12], {x, 0, 1}]**

[绘图](#)

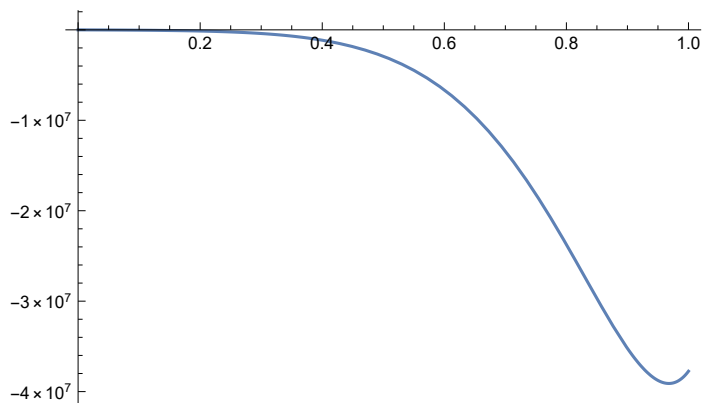

**Plot[Cf[7, 12, 11], {x, 0, 1}]**

[绘图](#)

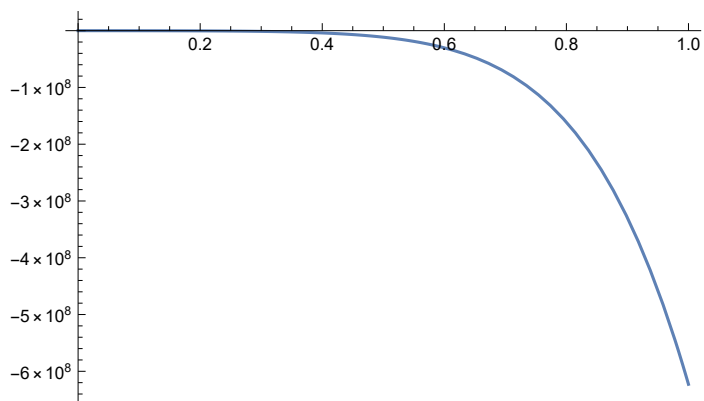

**Plot[Cf[7, 12, 10], {x, 0, 1}]**

[绘图](#)

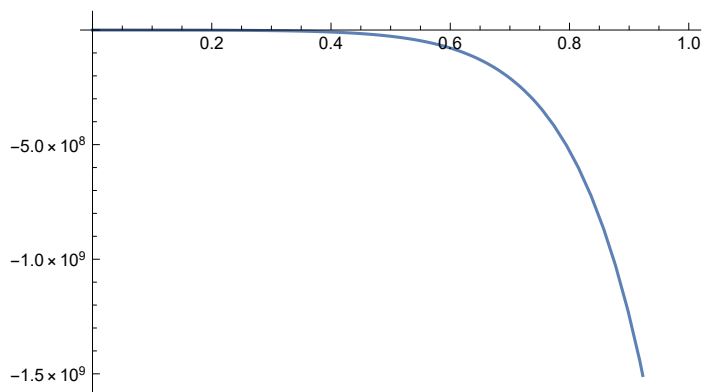

**Plot[Cf[7, 12, 9], {x, 0, 1}]**

[绘图](#)

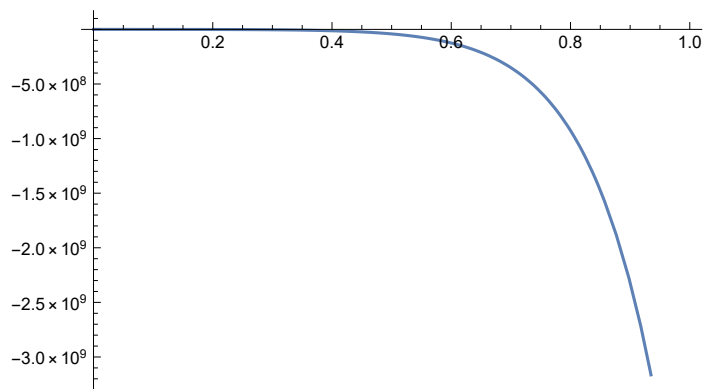

**Plot[Cf[7, 12, 8], {x, 0, 1}]**

[绘图](#)

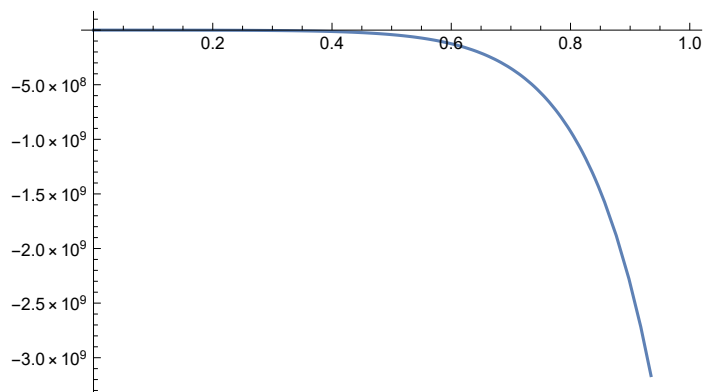

**Plot[Cf[7, 12, 7], {x, 0, 1}]**

[绘图](#)

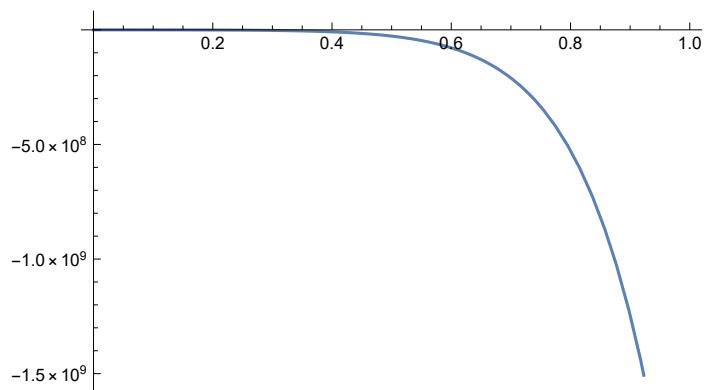



**Plot[Cf[7, 12, 6], {x, 0, 1}]**

[绘图](#)

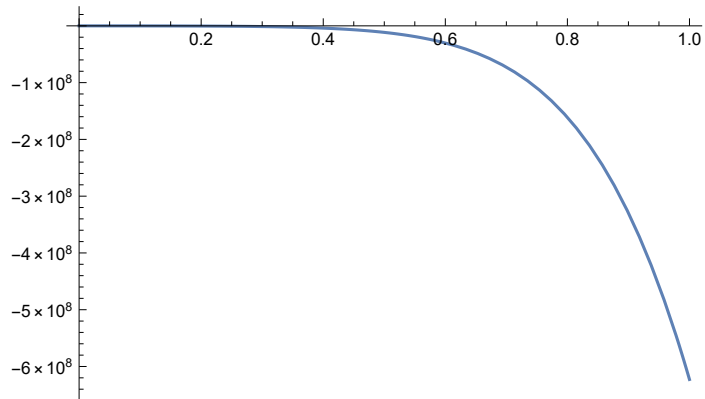

**Plot[Cf[7, 12, 5], {x, 0, 1}]**

[绘图](#)

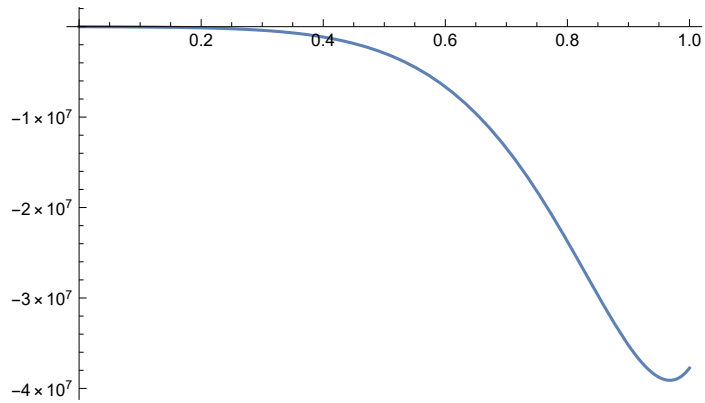

**Plot[Cf[7, 12, 4], {x, 0, 1}]**

[绘图](#)

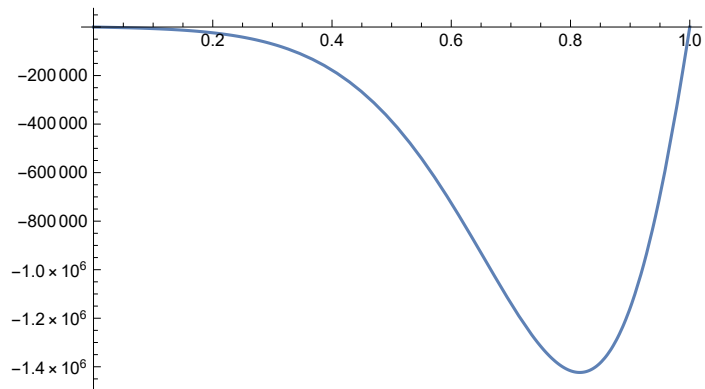

**Plot[Cf[7, 12, 3], {x, 0, 1}]**

[绘图](#)

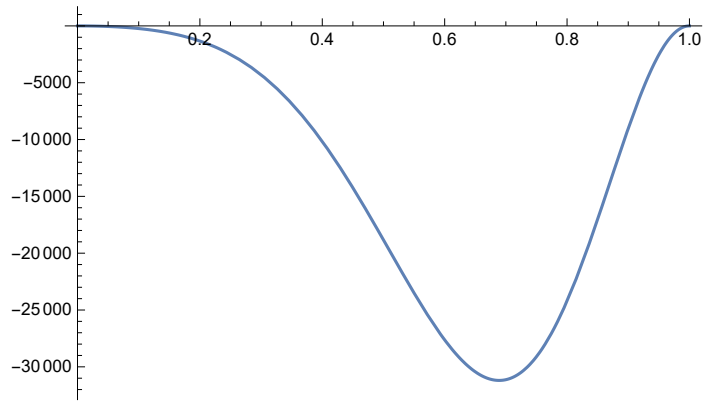

**Plot[Cf[7, 12, 2], {x, 0, 1}]**

[绘图](#)

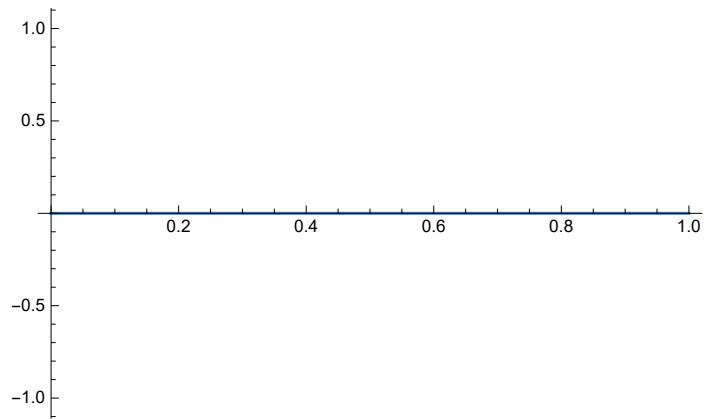

**Plot[Cf[7, 12, 1], {x, 0, 1}]**

[绘图](#)

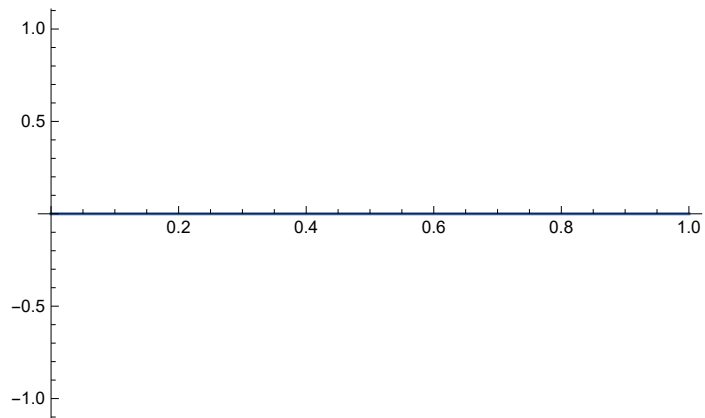

`Plot[Cf[7, 12, 0], {x, 0, 1}]`

[绘图](#)

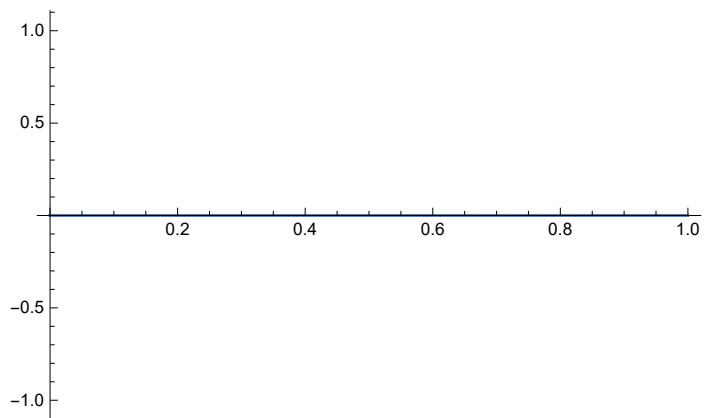

(\*109th group coefficients r2^7r3^11\*)

`Plot[Cf[7, 11, 14], {x, 0, 1}]`

[绘图](#)

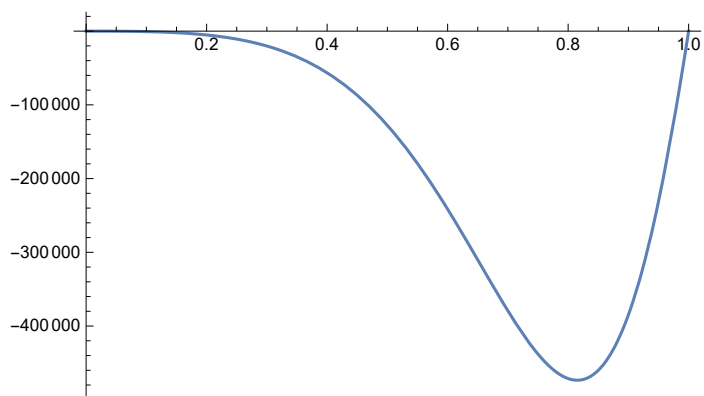

`Plot[Cf[7, 11, 13], {x, 0, 1}]`

[绘图](#)

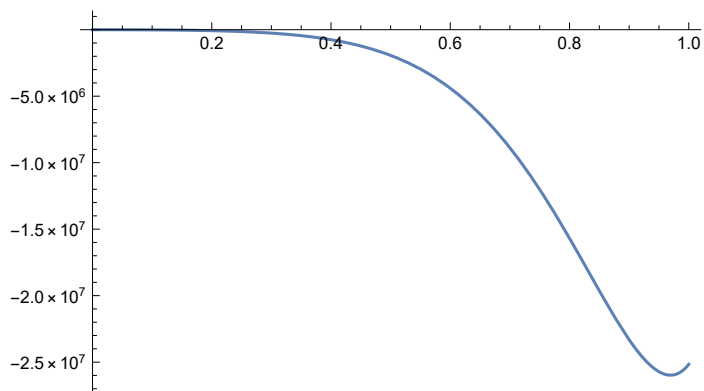

**Plot[Cf[7, 11, 12], {x, 0, 1}]**

[绘图](#)

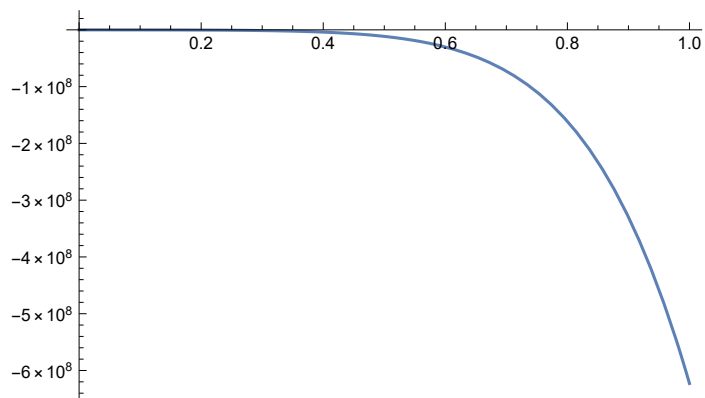

**Plot[Cf[7, 11, 11], {x, 0, 1}]**

[绘图](#)

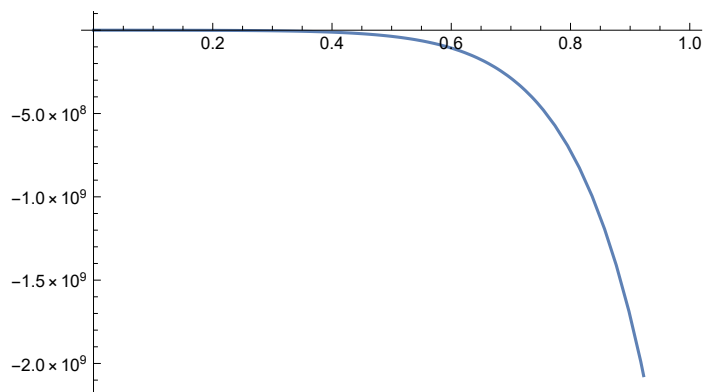

**Plot[Cf[7, 11, 10], {x, 0, 1}]**

[绘图](#)

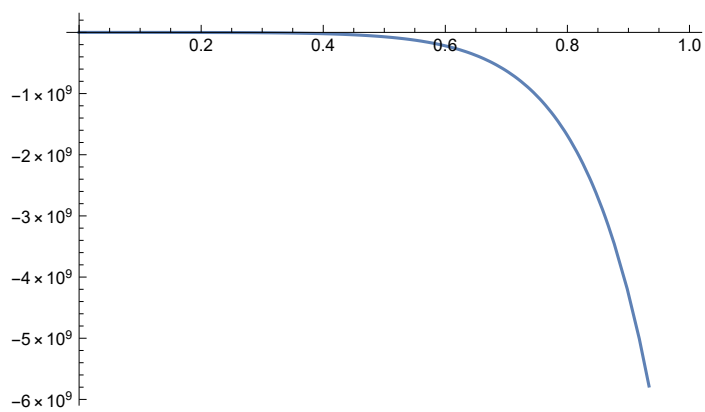

**Plot[Cf[7, 11, 9], {x, 0, 1}]**

[绘图](#)

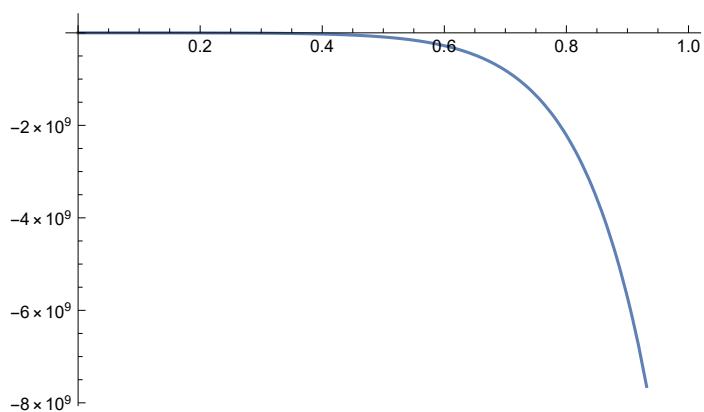

**Plot[Cf[7, 11, 8], {x, 0, 1}]**

[绘图](#)

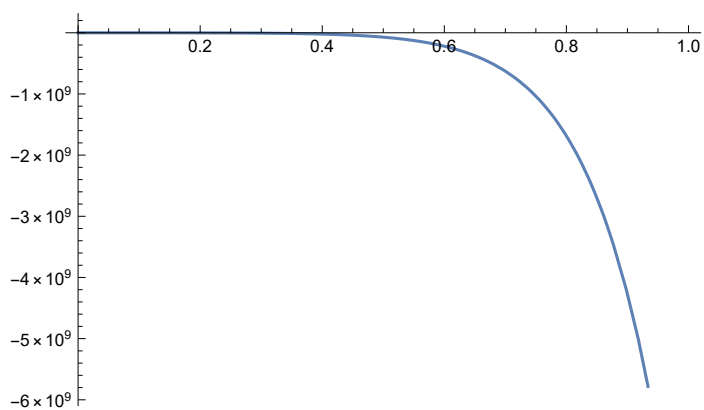

**Plot[Cf[7, 11, 7], {x, 0, 1}]**

[绘图](#)

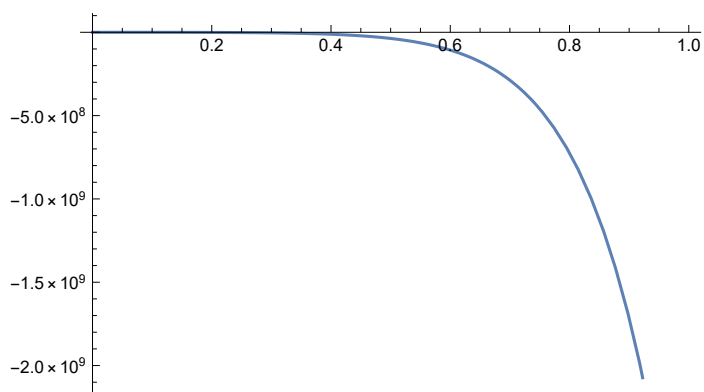

**Plot[Cf[7, 11, 6], {x, 0, 1}]**

[绘图](#)

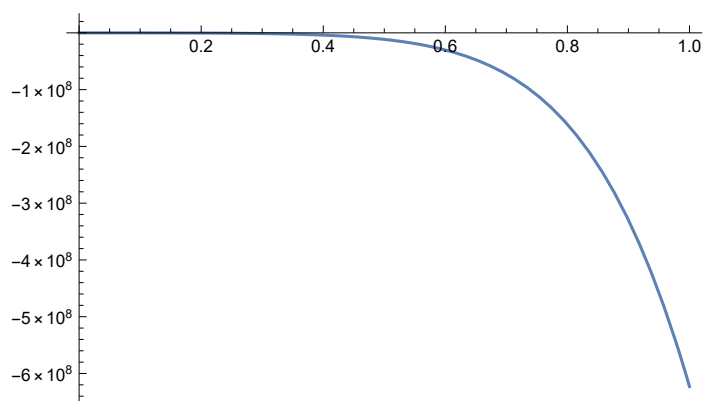

**Plot[Cf[7, 11, 5], {x, 0, 1}]**

[绘图](#)

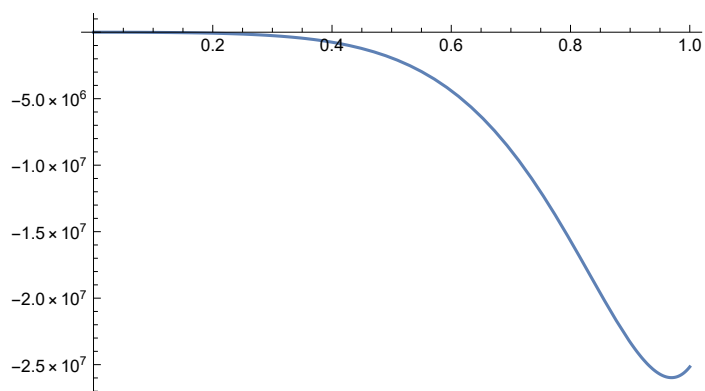

**Plot[Cf[7, 11, 4], {x, 0, 1}]**

[绘图](#)

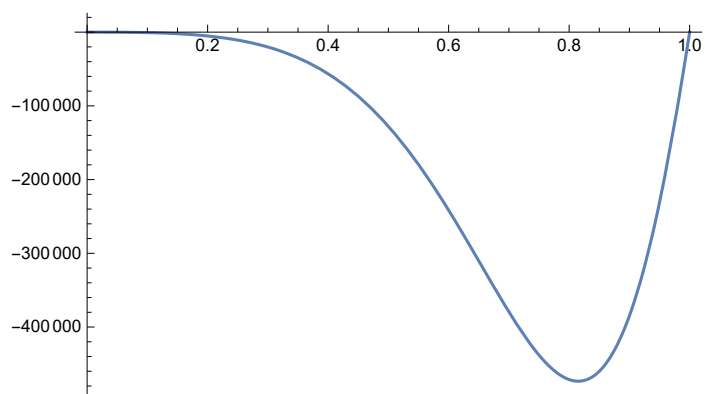

**Plot[Cf[7, 11, 3], {x, 0, 1}]**

[绘图](#)

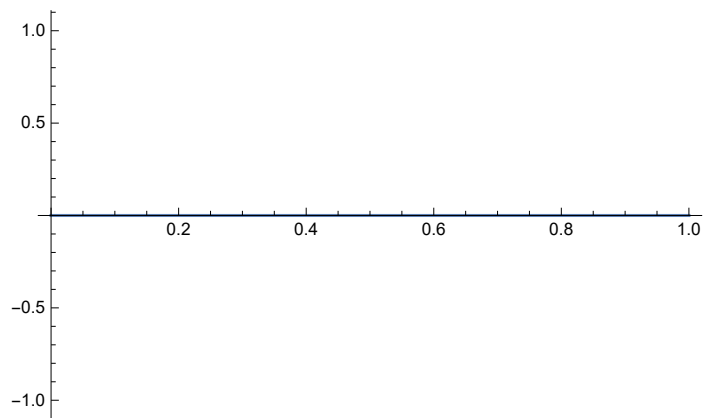

**Plot[Cf[7, 11, 2], {x, 0, 1}]**

[绘图](#)

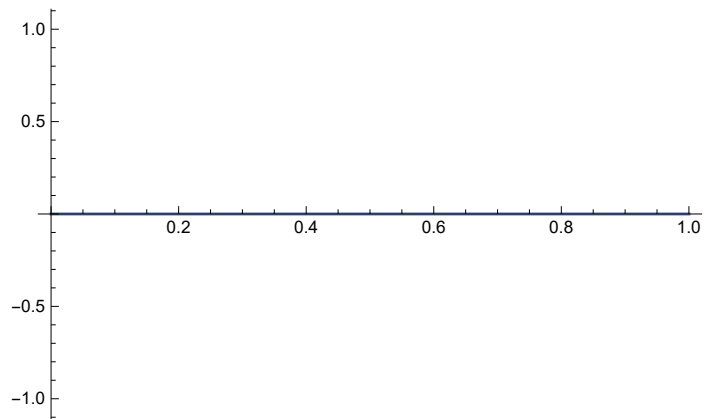

**Plot[Cf[7, 11, 1], {x, 0, 1}]**

[绘图](#)

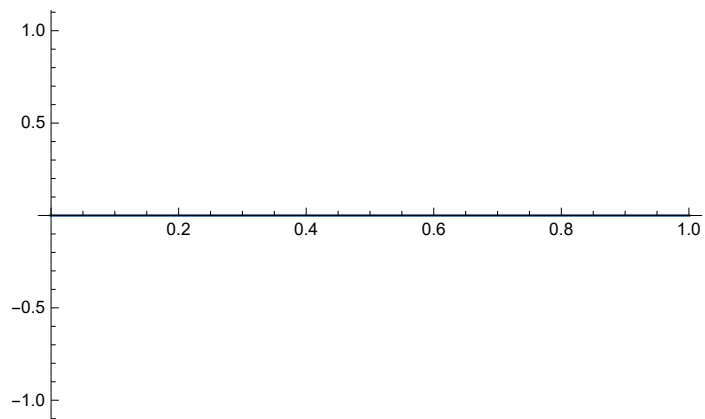

**Plot[Cf[7, 11, 0], {x, 0, 1}]**

[绘图](#)

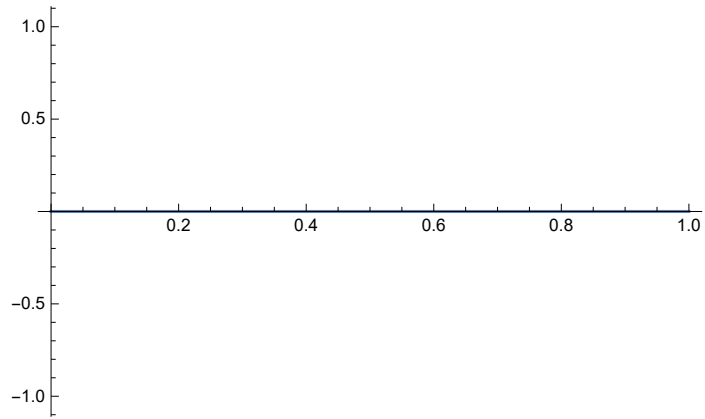

**(\*110th group coefficients r2^7r3^10\*)**

**Plot[Cf[7, 10, 14], {x, 0, 1}]**

[绘图](#)

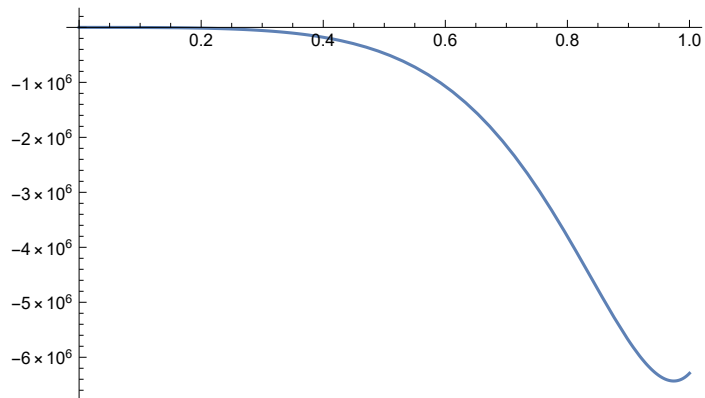

**Plot[Cf[7, 10, 13], {x, 0, 1}]**

[绘图](#)

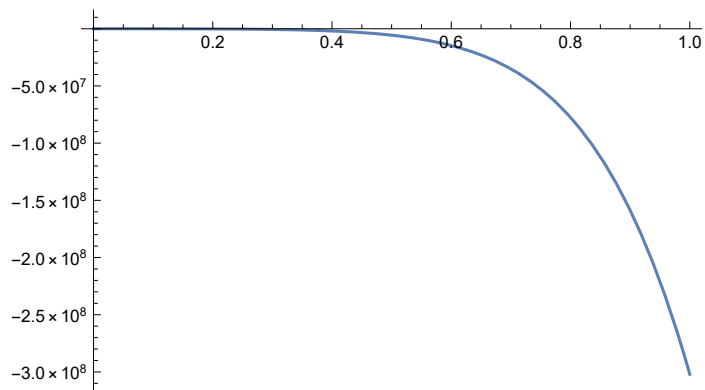



**Plot[Cf[7, 10, 12], {x, 0, 1}]**

[绘图](#)

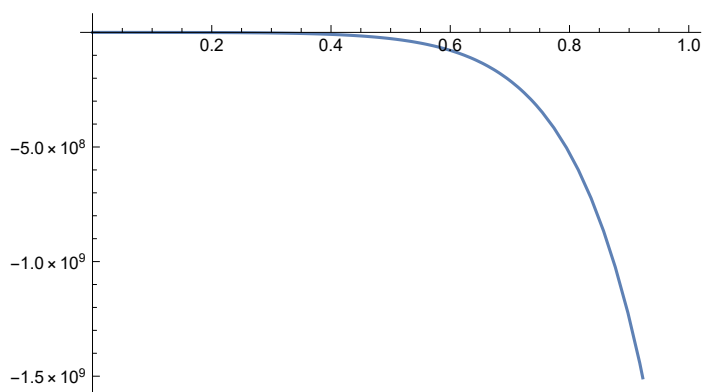

**Plot[Cf[7, 10, 11], {x, 0, 1}]**

[绘图](#)

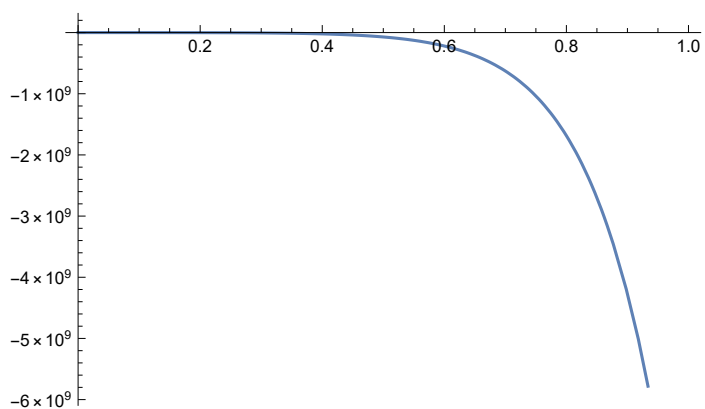

**Plot[Cf[7, 10, 10], {x, 0, 1}]**

[绘图](#)

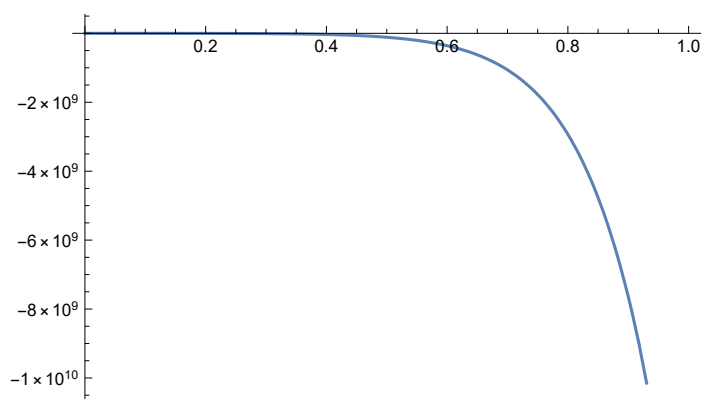

**Plot[Cf[7, 10, 9], {x, 0, 1}]**

[绘图](#)

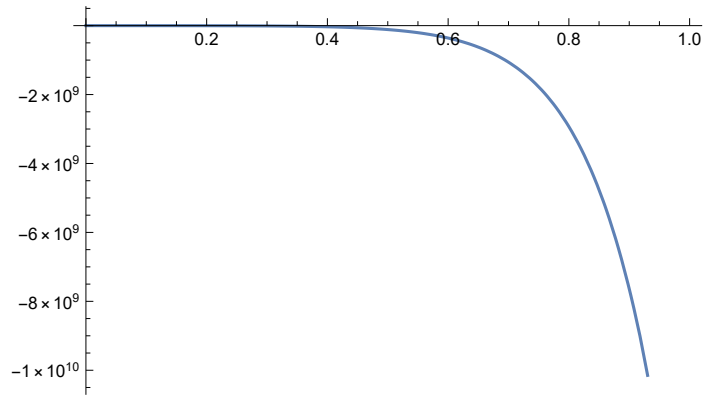

**Plot[Cf[7, 10, 8], {x, 0, 1}]**

[绘图](#)

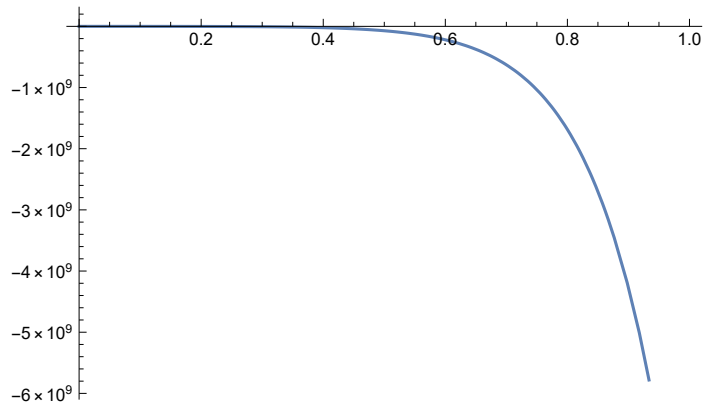

**Plot[Cf[7, 10, 7], {x, 0, 1}]**

[绘图](#)

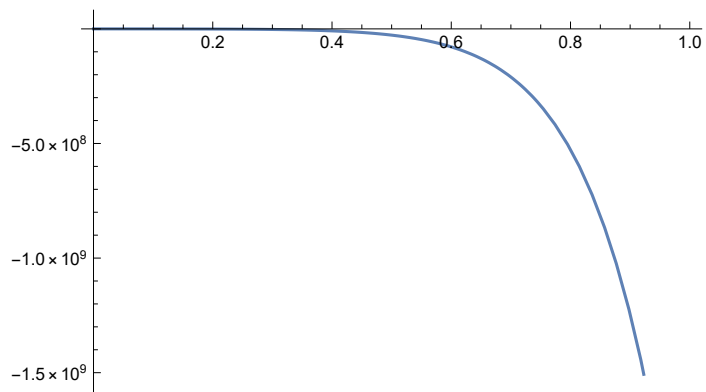

**Plot[Cf[7, 10, 6], {x, 0, 1}]**

[绘图](#)

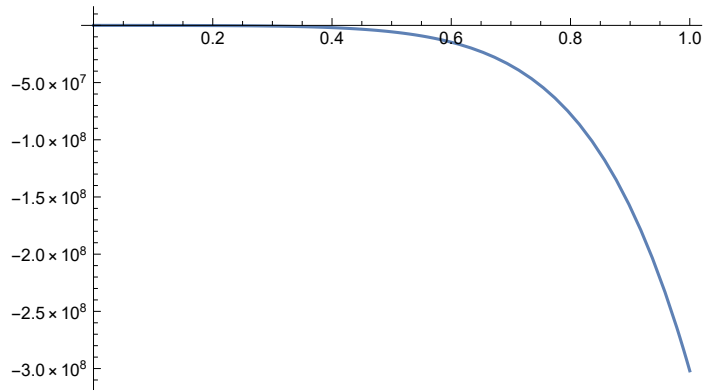

**Plot[Cf[7, 10, 5], {x, 0, 1}]**

[绘图](#)

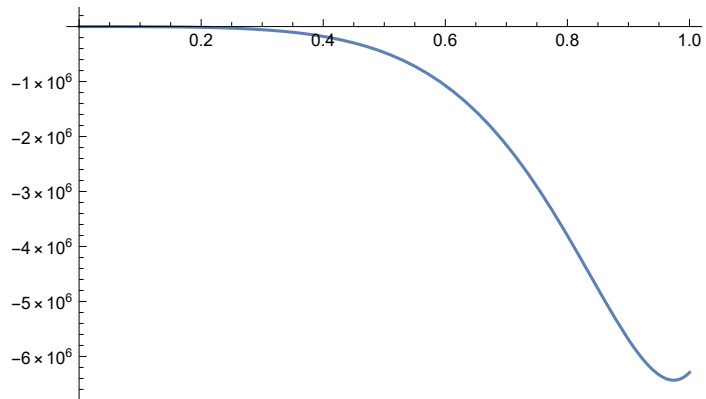

**Plot[Cf[7, 10, 4], {x, 0, 1}]**

[绘图](#)

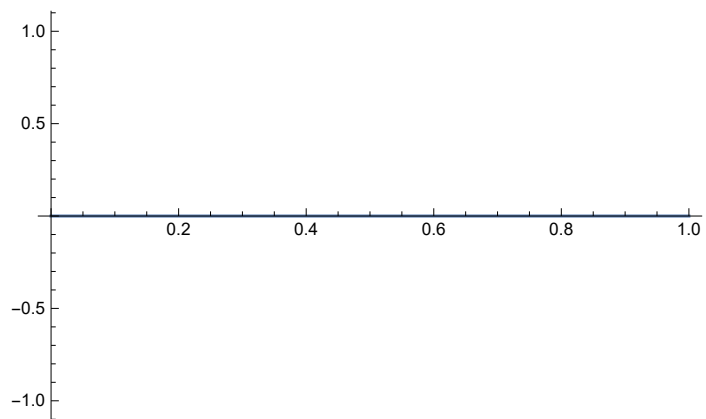

**Plot[Cf[7, 10, 3], {x, 0, 1}]**

[绘图](#)

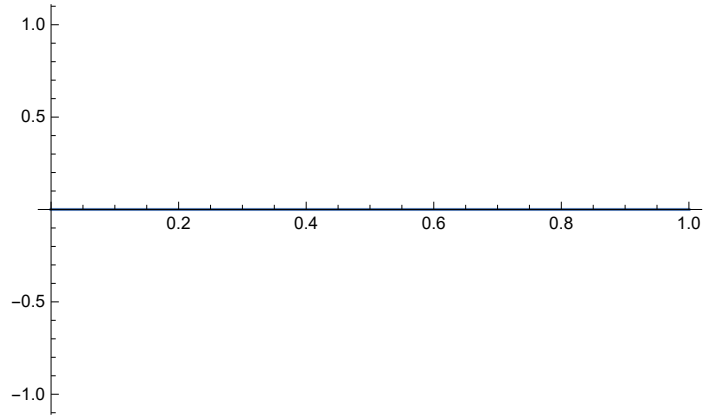

**Plot[Cf[7, 10, 2], {x, 0, 1}]**

[绘图](#)

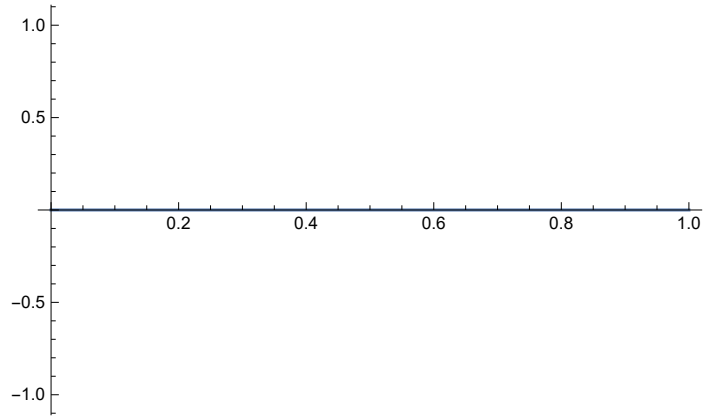

**Plot[Cf[7, 10, 1], {x, 0, 1}]**

[绘图](#)

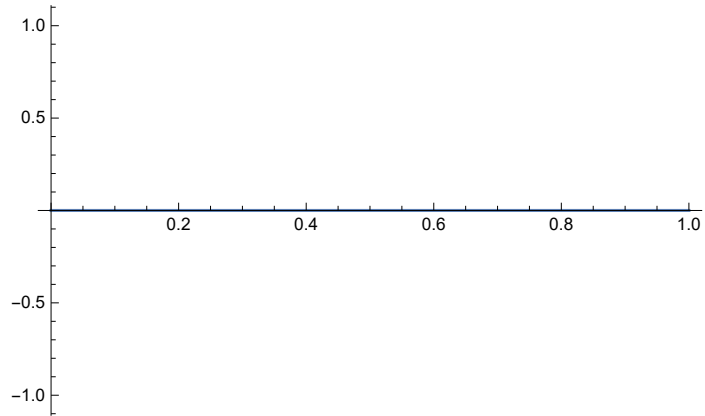

**Plot[Cf[7, 10, 0], {x, 0, 1}]**

[绘图](#)

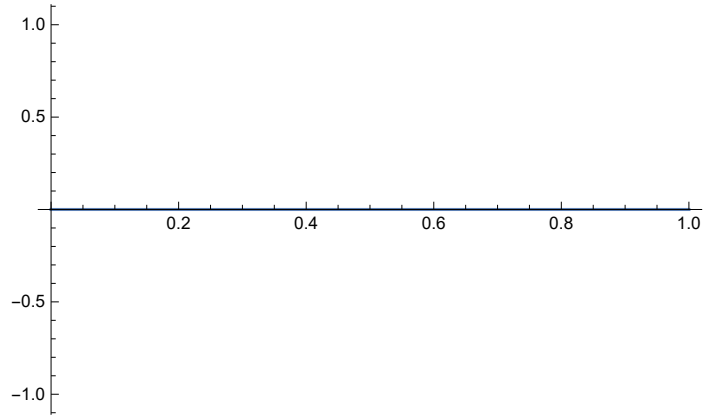

**(\*111th group coefficients r2^7r3^9\*)**

**Plot[Cf[7, 9, 14], {x, 0, 1}]**

[绘图](#)

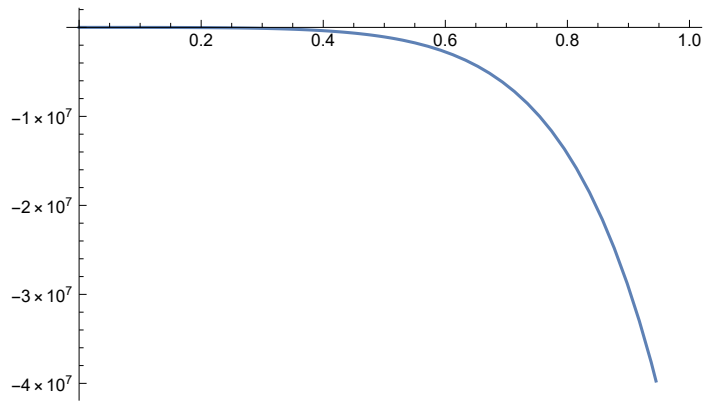

**Plot[Cf[7, 9, 13], {x, 0, 1}]**

[绘图](#)

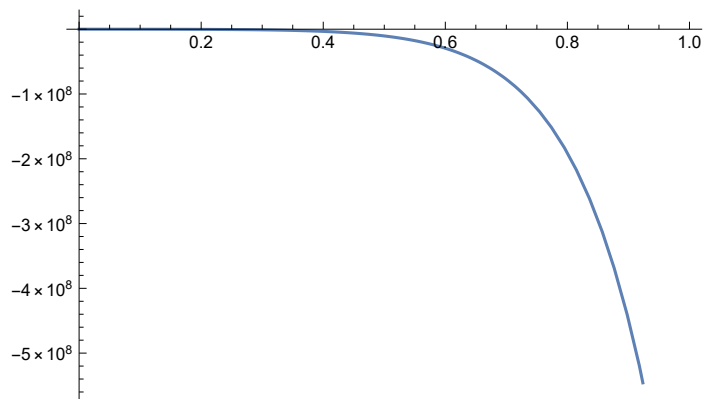

**Plot[Cf[7, 9, 12], {x, 0, 1}]**

[绘图](#)

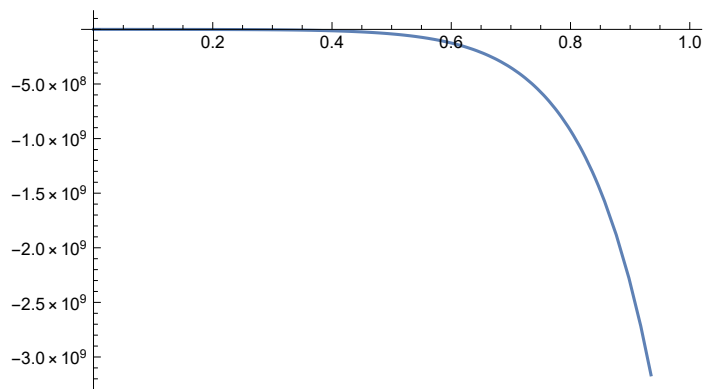

**Plot[Cf[7, 9, 11], {x, 0, 1}]**

[绘图](#)

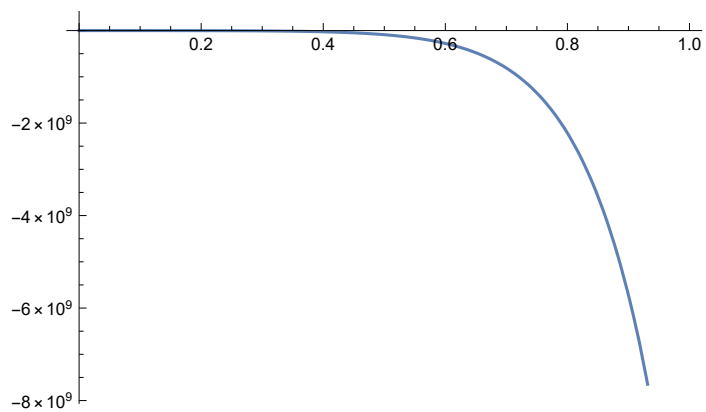

**Plot[Cf[7, 9, 10], {x, 0, 1}]**

[绘图](#)

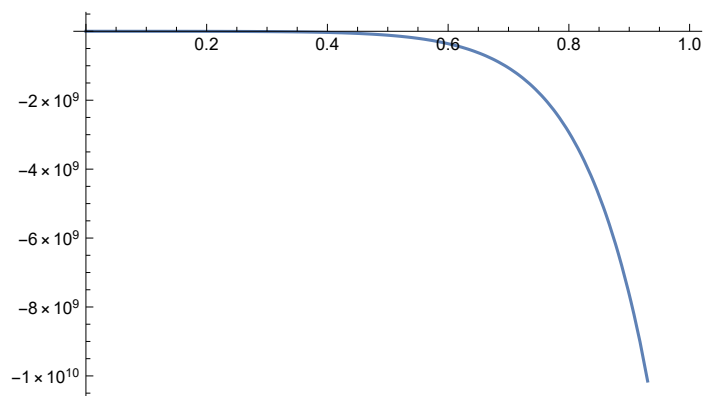

**Plot[Cf[7, 9, 9], {x, 0, 1}]**

[绘图](#)

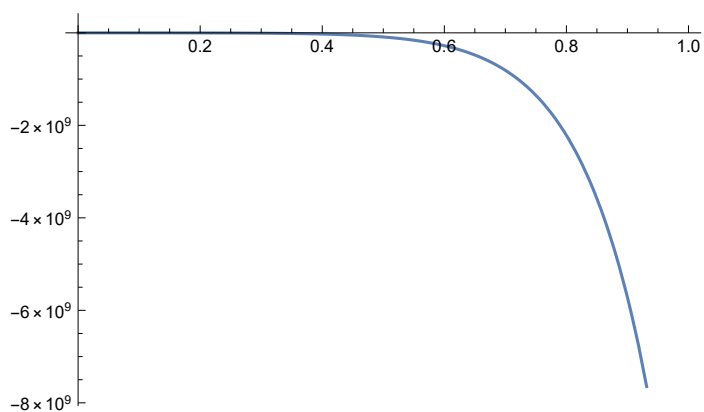

**Plot[Cf[7, 9, 8], {x, 0, 1}]**

[绘图](#)

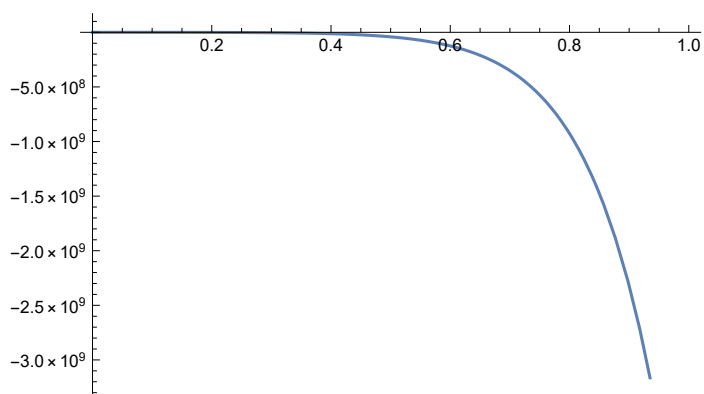

**Plot[Cf[7, 9, 7], {x, 0, 1}]**

[绘图](#)

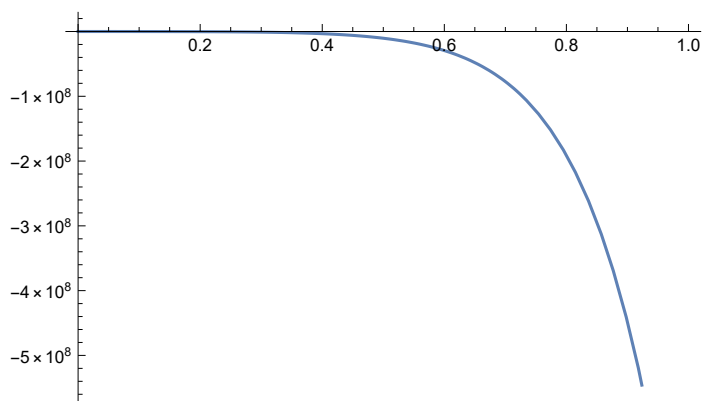

**Plot[Cf[7, 9, 6], {x, 0, 1}]**

[绘图](#)

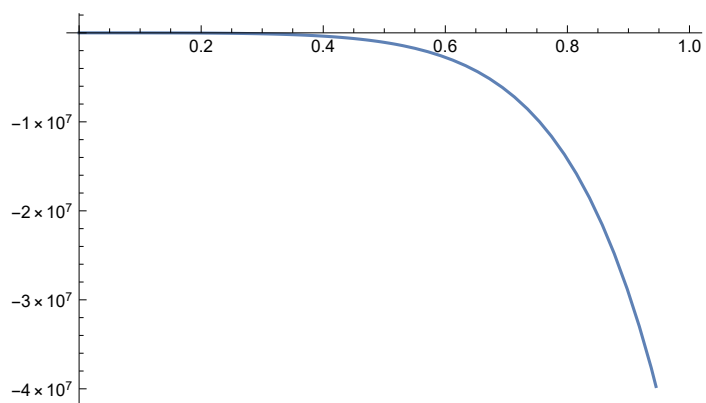

**Plot[Cf[7, 9, 5], {x, 0, 1}]**

[绘图](#)

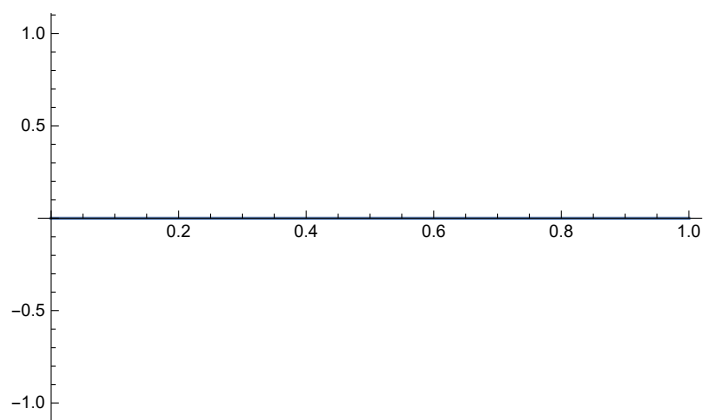

**Plot[Cf[7, 9, 4], {x, 0, 1}]**

[绘图](#)

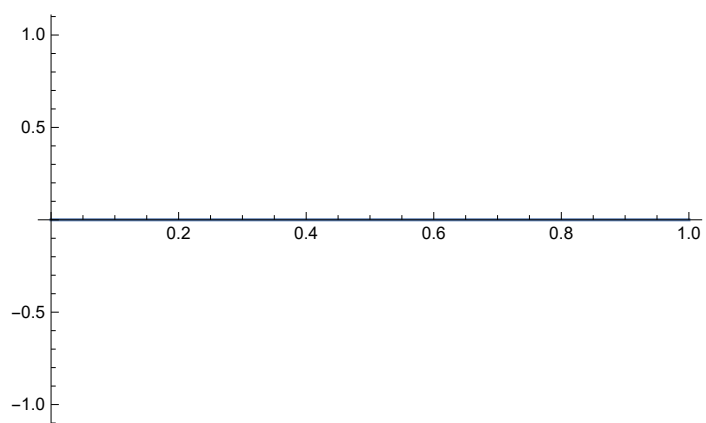



**Plot[Cf[7, 9, 3], {x, 0, 1}]**

[绘图](#)

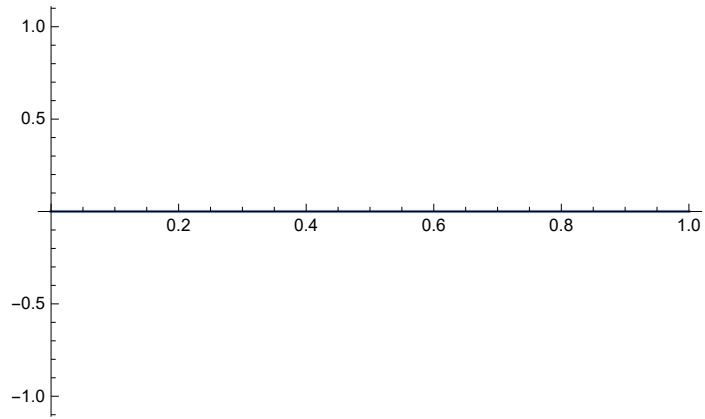

**Plot[Cf[7, 9, 2], {x, 0, 1}]**

[绘图](#)

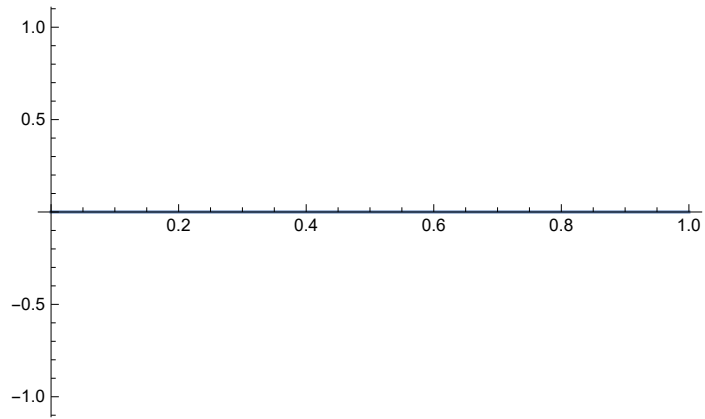

**Plot[Cf[7, 9, 1], {x, 0, 1}]**

[绘图](#)

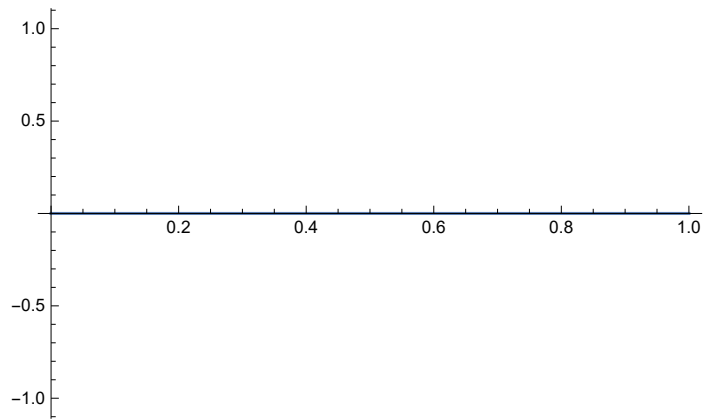

`Plot[Cf[7, 9, 0], {x, 0, 1}]`

[绘图](#)

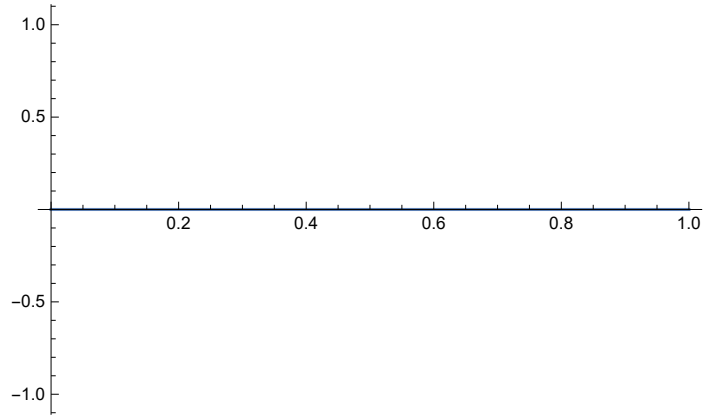

(\*112th group coefficients  $r_2^7 r_3^8$ \*)

`Plot[Cf[7, 8, 14], {x, 0, 1}]`

[绘图](#)

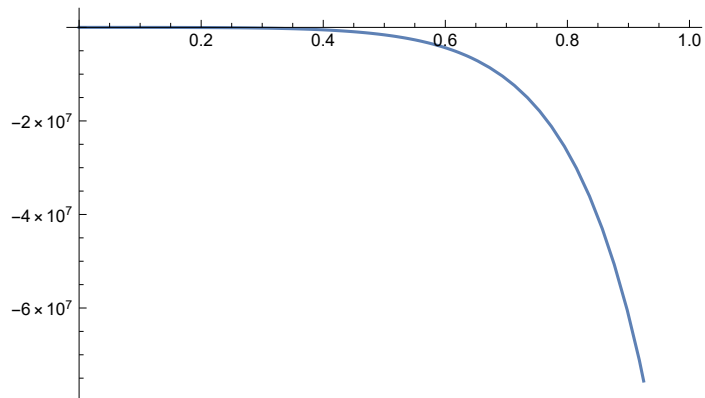

`Plot[Cf[7, 8, 13], {x, 0, 1}]`

[绘图](#)

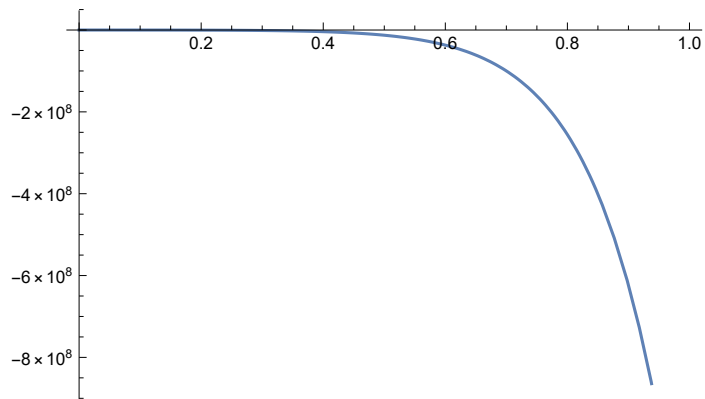

**Plot[Cf[7, 8, 12], {x, 0, 1}]**

[绘图](#)

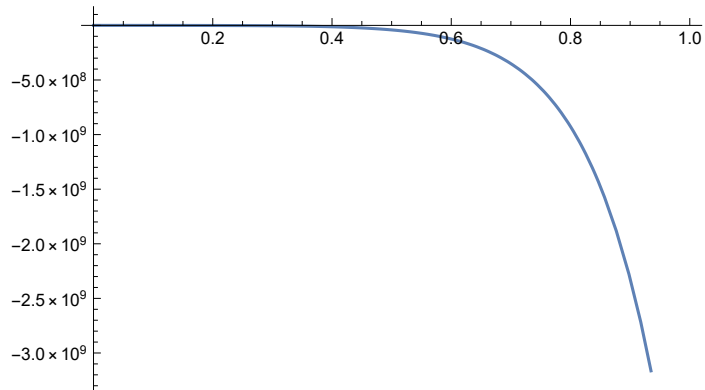

**Plot[Cf[7, 8, 11], {x, 0, 1}]**

[绘图](#)

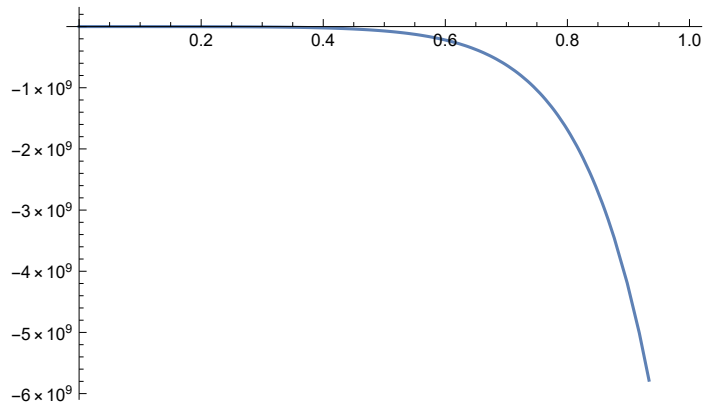

**Plot[Cf[7, 8, 10], {x, 0, 1}]**

[绘图](#)

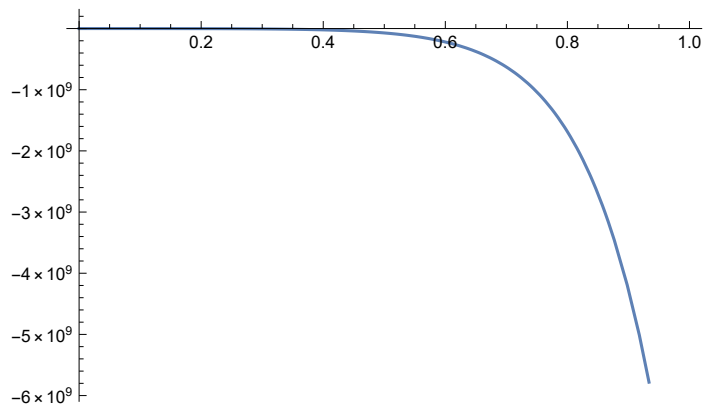

**Plot[Cf[7, 8, 9], {x, 0, 1}]**

[绘图](#)

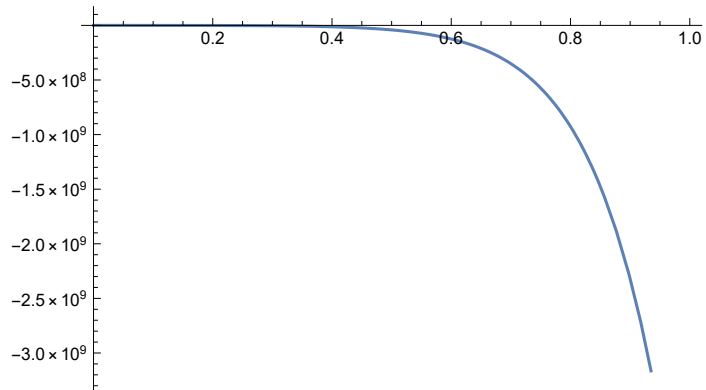

**Plot[Cf[7, 8, 8], {x, 0, 1}]**

[绘图](#)

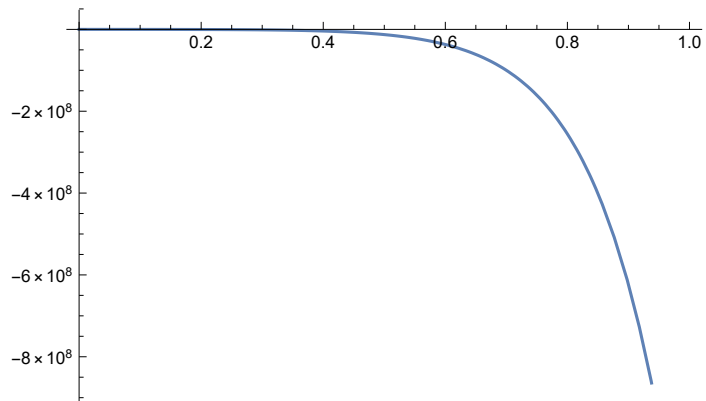

**Plot[Cf[7, 8, 7], {x, 0, 1}]**

[绘图](#)

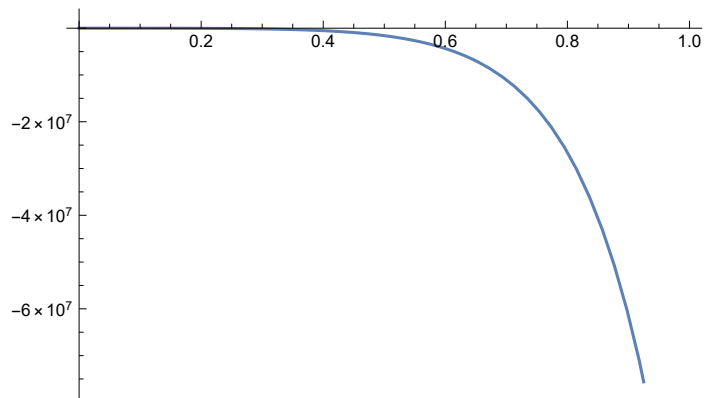

**Plot[Cf[7, 8, 6], {x, 0, 1}]**

[绘图](#)

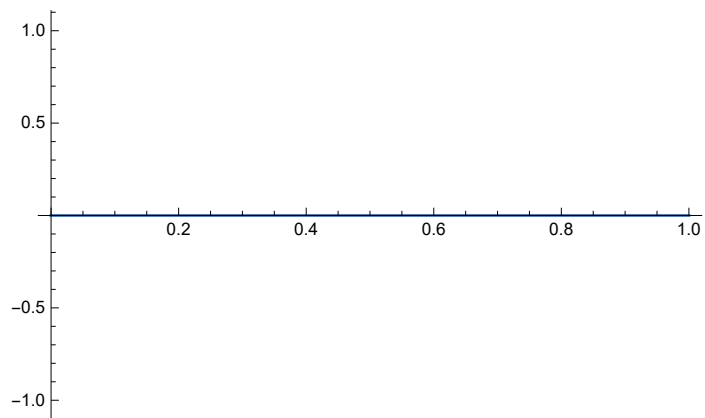

**Plot[Cf[7, 8, 5], {x, 0, 1}]**

[绘图](#)

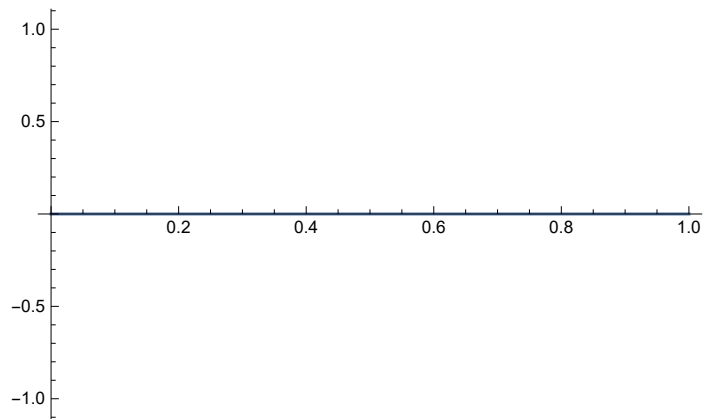

**Plot[Cf[7, 8, 4], {x, 0, 1}]**

[绘图](#)

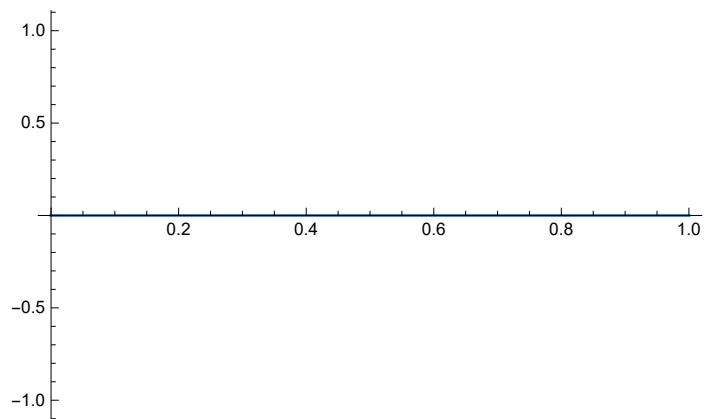

**Plot[Cf[7, 8, 3], {x, 0, 1}]**

[绘图](#)

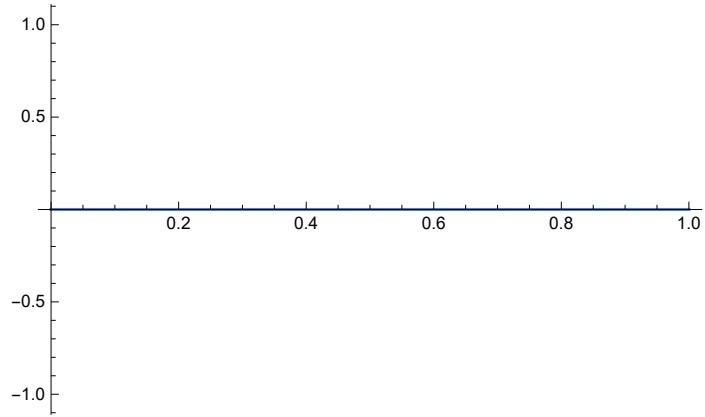

**Plot[Cf[7, 8, 2], {x, 0, 1}]**

[绘图](#)

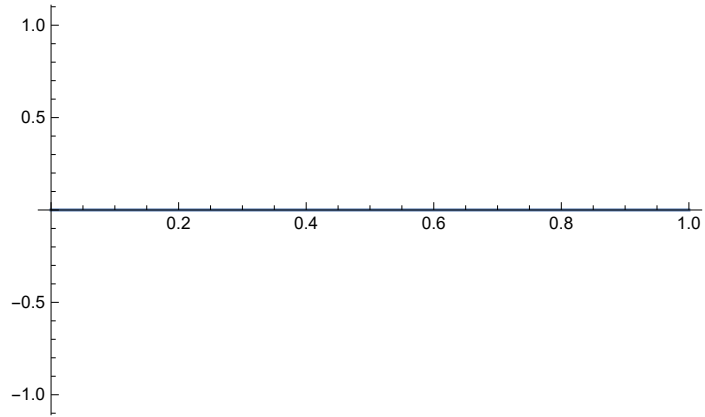

**Plot[Cf[7, 8, 1], {x, 0, 1}]**

[绘图](#)

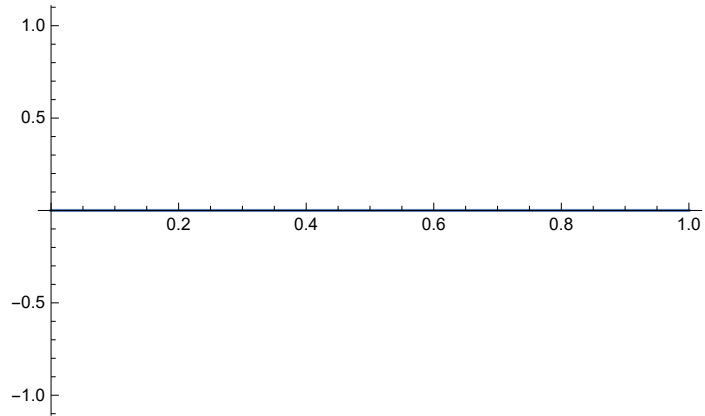

**Plot[Cf[7, 8, 0], {x, 0, 1}]**

[绘图](#)

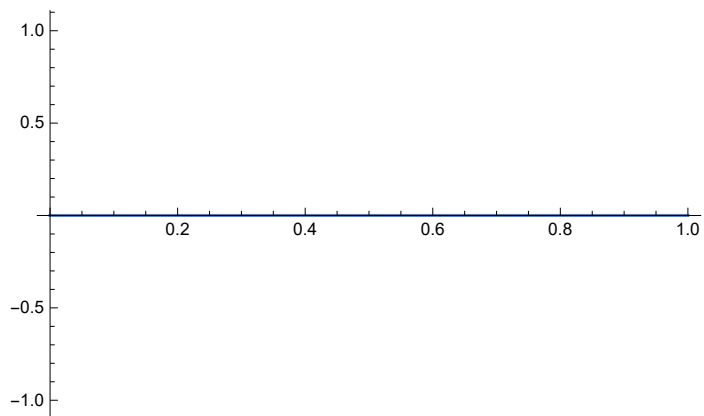

**(\*113th group coefficients r2^7r3^7\*)**

**Plot[Cf[7, 7, 14], {x, 0, 1}]**

[绘图](#)

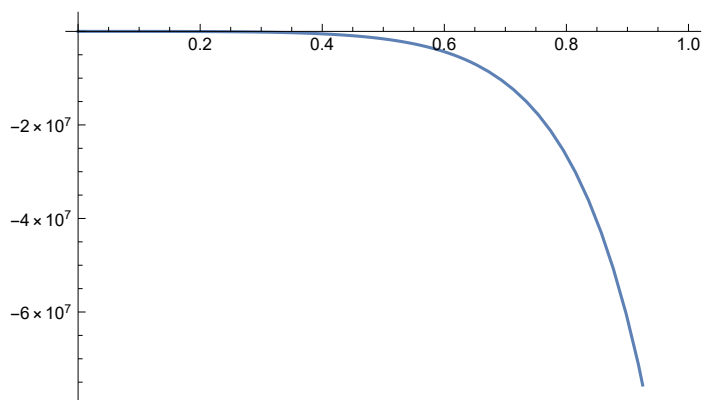

**Plot[Cf[7, 7, 13], {x, 0, 1}]**

[绘图](#)

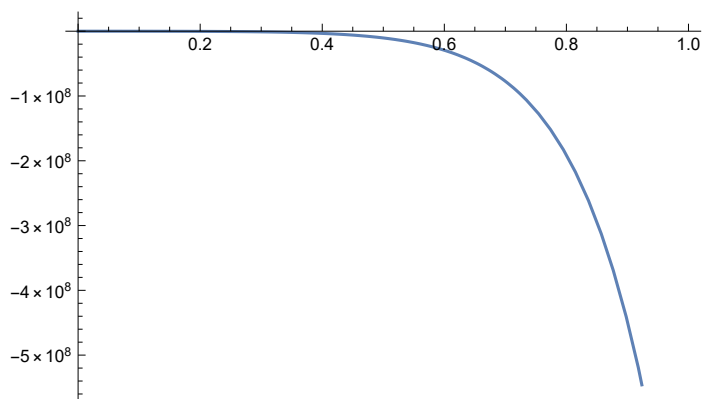

**Plot[Cf[7, 7, 12], {x, 0, 1}]**

[绘图](#)

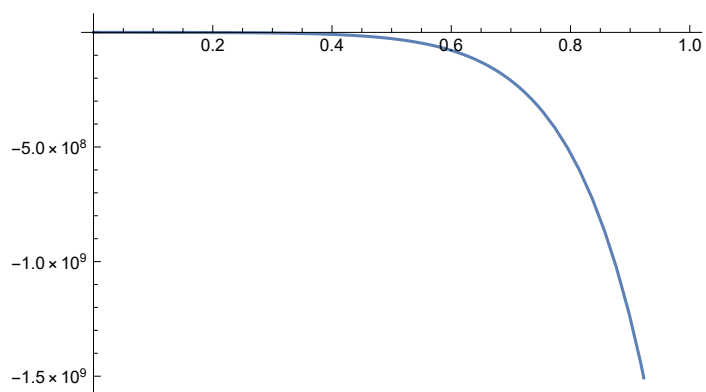

**Plot[Cf[7, 7, 11], {x, 0, 1}]**

[绘图](#)

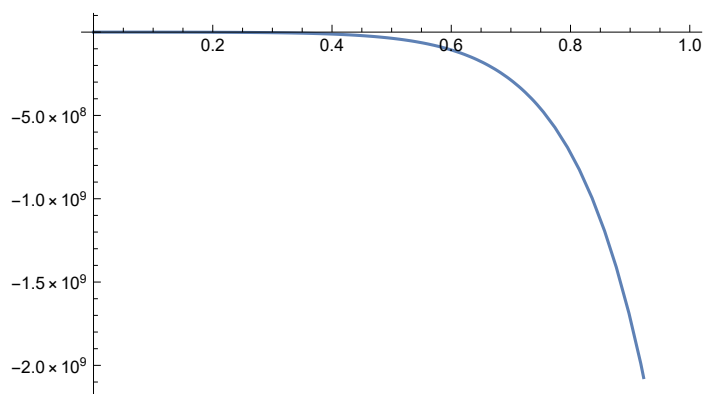

**Plot[Cf[7, 7, 10], {x, 0, 1}]**

[绘图](#)

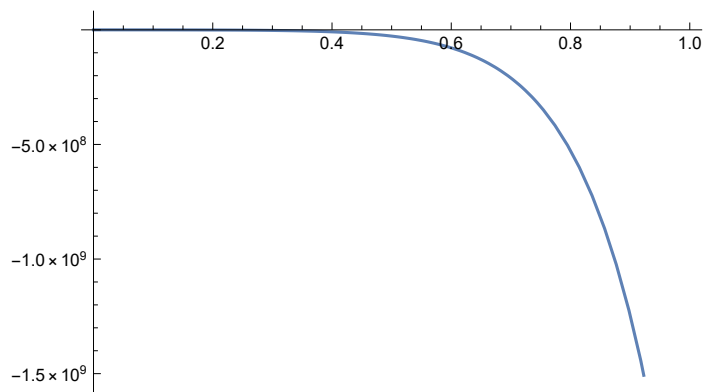



**Plot[Cf[7, 7, 9], {x, 0, 1}]**

[绘图](#)

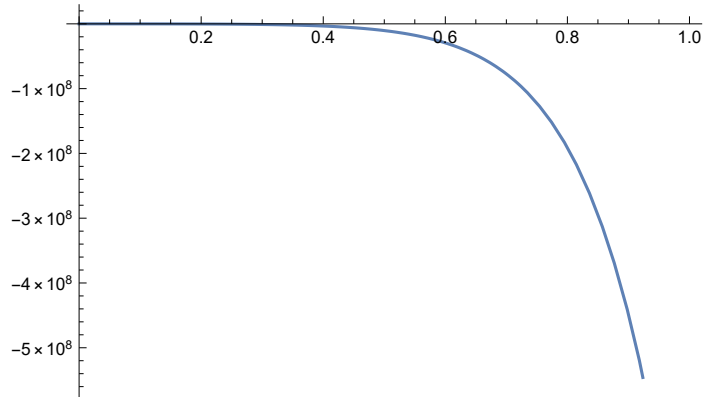

**Plot[Cf[7, 7, 8], {x, 0, 1}]**

[绘图](#)

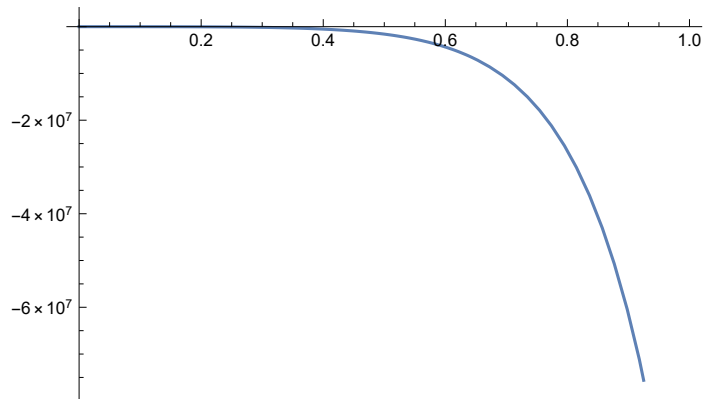

**Plot[Cf[7, 7, 7], {x, 0, 1}]**

[绘图](#)

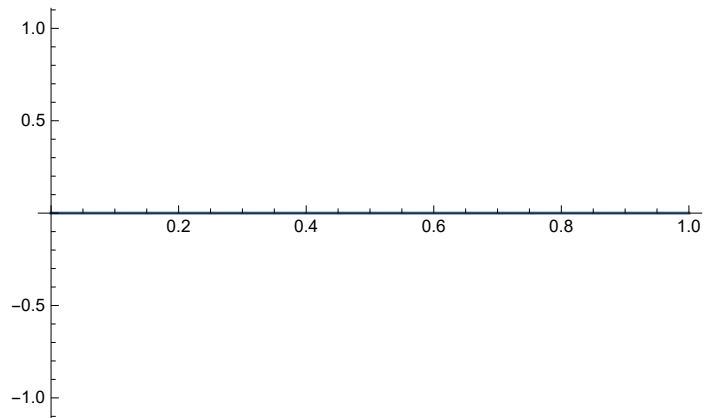

**Plot[Cf[7, 7, 6], {x, 0, 1}]**

[绘图](#)

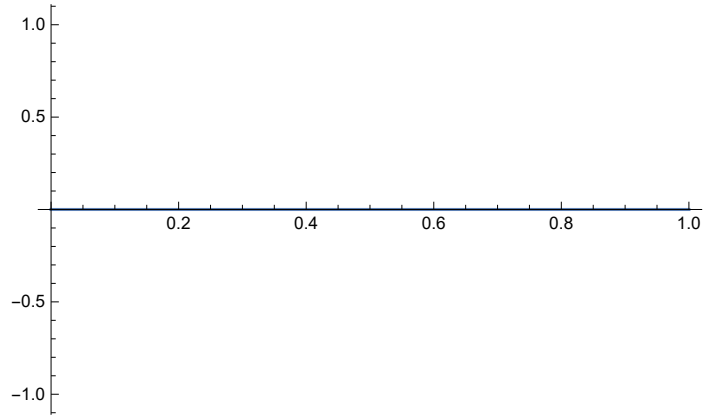

**Plot[Cf[7, 7, 5], {x, 0, 1}]**

[绘图](#)

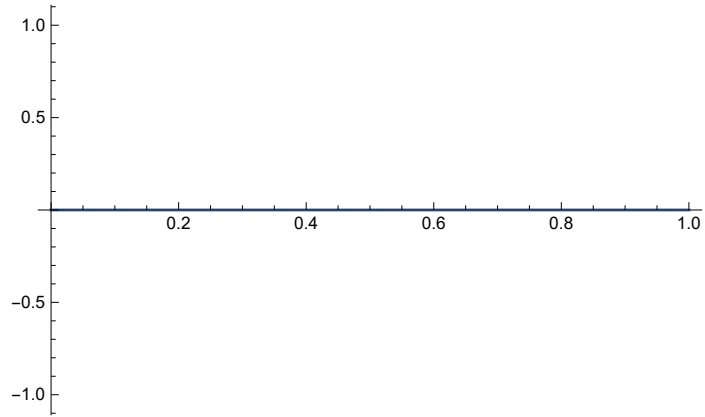

**Plot[Cf[7, 7, 4], {x, 0, 1}]**

[绘图](#)

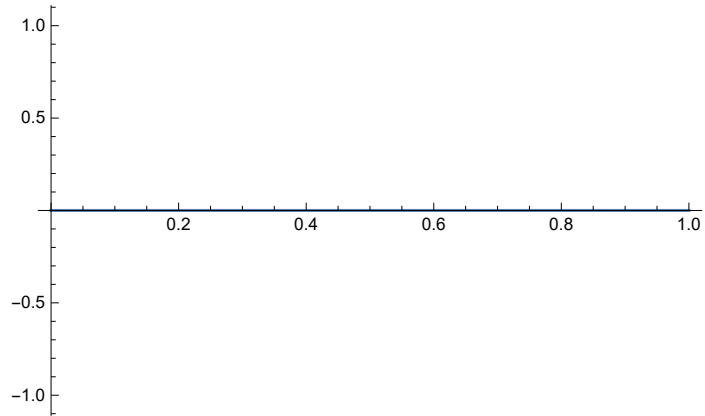

**Plot[Cf[7, 7, 3], {x, 0, 1}]**

[绘图](#)

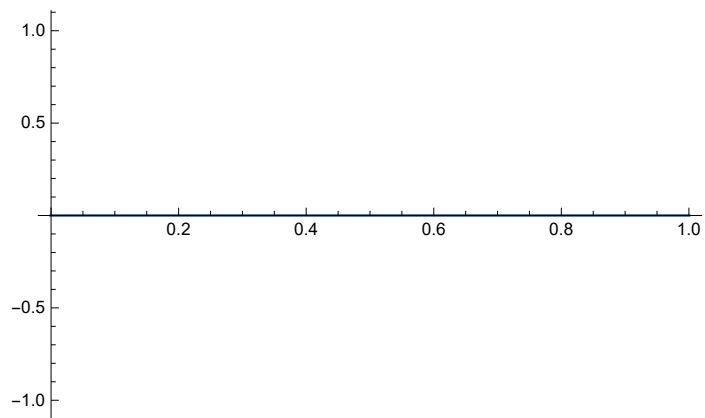

**Plot[Cf[7, 7, 2], {x, 0, 1}]**

[绘图](#)

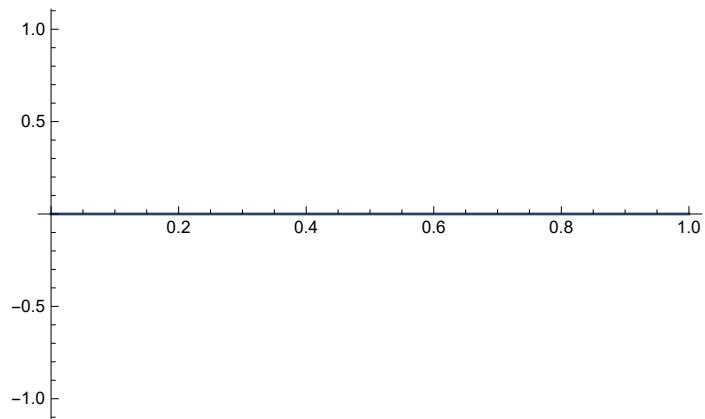

**Plot[Cf[7, 7, 1], {x, 0, 1}]**

[绘图](#)

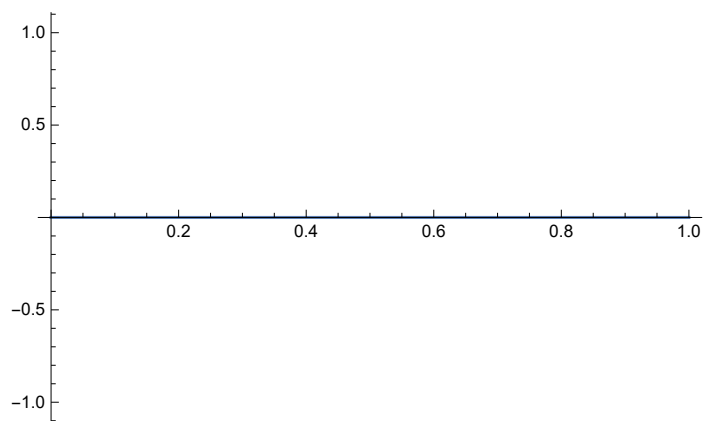

**Plot[Cf[7, 7, 0], {x, 0, 1}]**

[绘图](#)

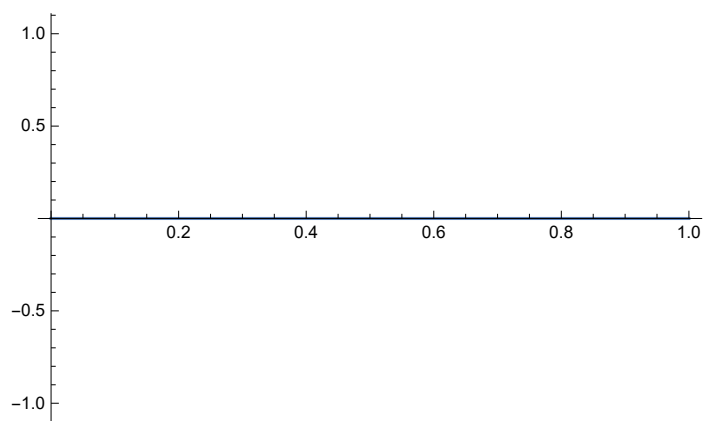

**(\*114th group coefficients r2^7r3^6\*)**

**Plot[Cf[7, 6, 14], {x, 0, 1}]**

[绘图](#)

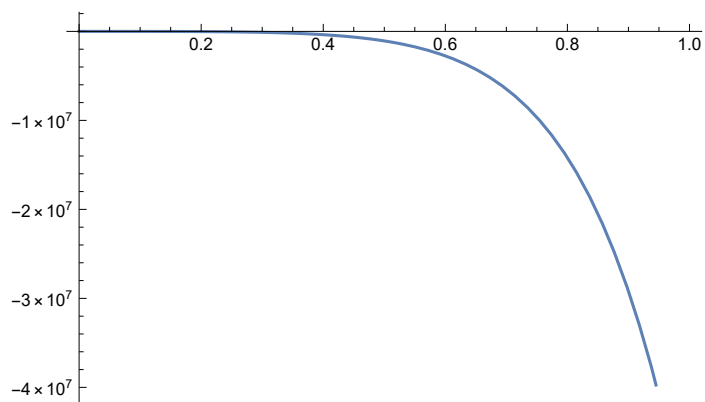

**Plot[Cf[7, 6, 13], {x, 0, 1}]**

[绘图](#)

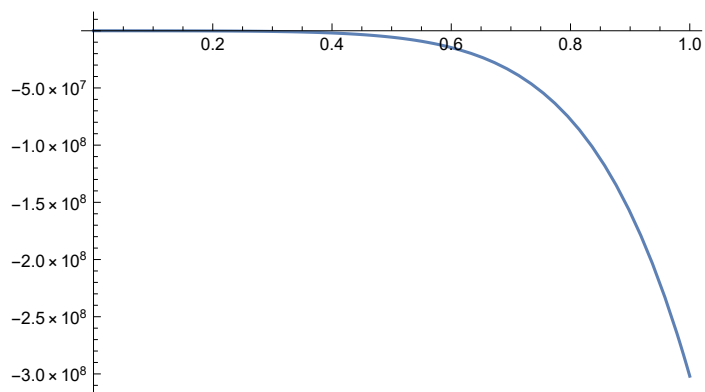

**Plot[Cf[7, 6, 12], {x, 0, 1}]**

[绘图](#)

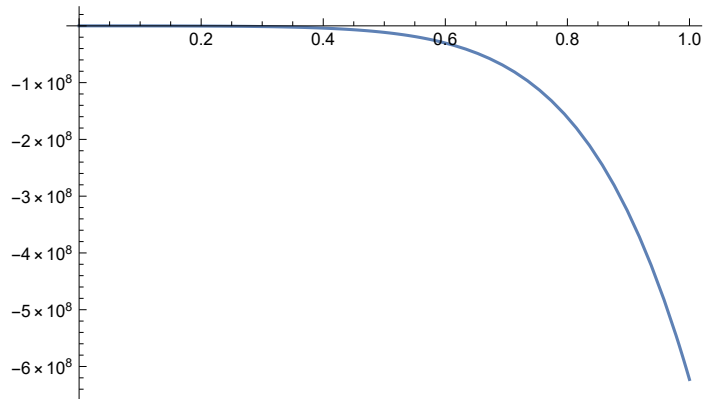

**Plot[Cf[7, 6, 11], {x, 0, 1}]**

[绘图](#)

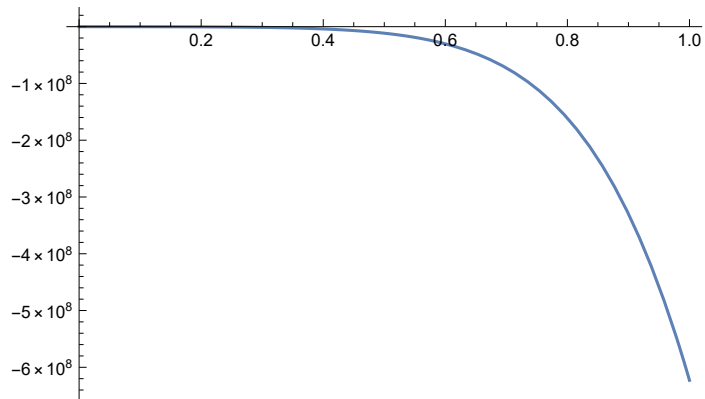

**Plot[Cf[7, 6, 10], {x, 0, 1}]**

[绘图](#)

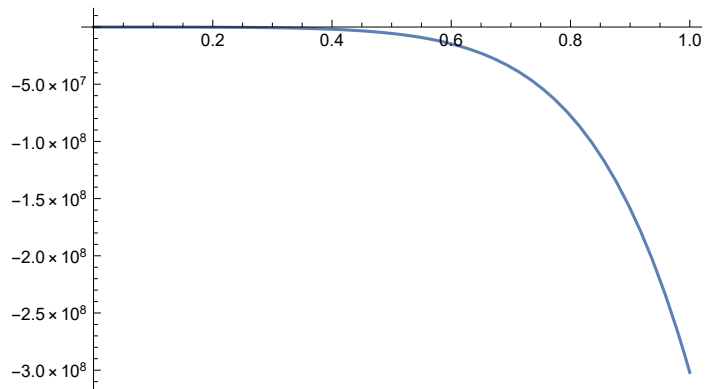

**Plot[Cf[7, 6, 9], {x, 0, 1}]**

[绘图](#)

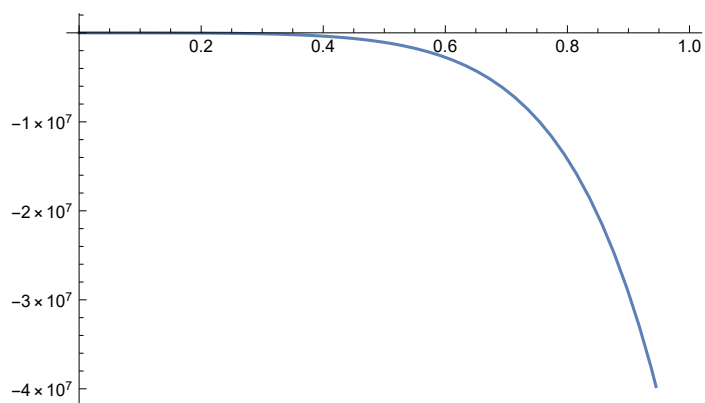

**Plot[Cf[7, 6, 8], {x, 0, 1}]**

[绘图](#)

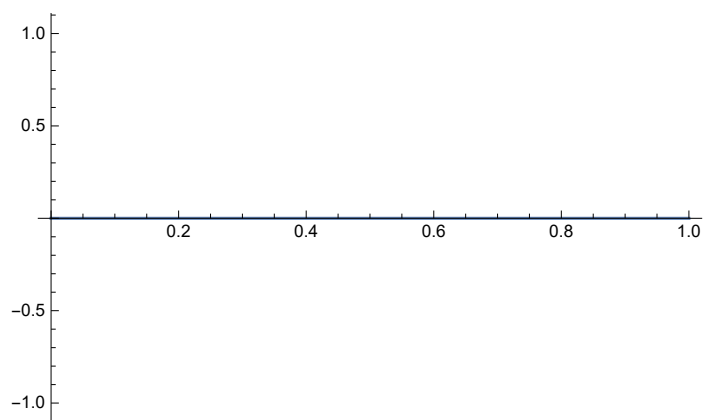

**Plot[Cf[7, 6, 7], {x, 0, 1}]**

[绘图](#)

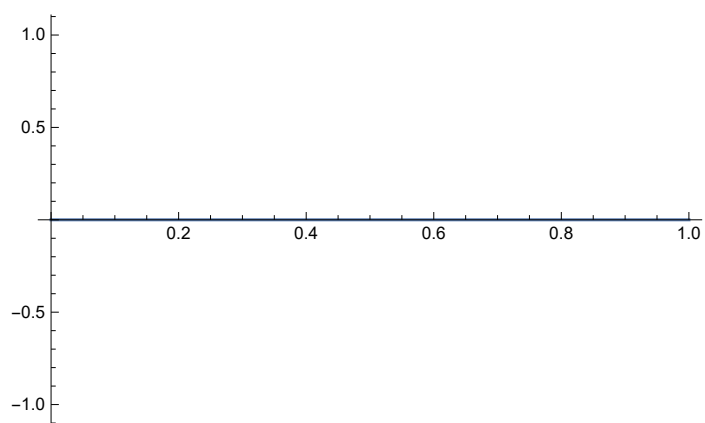

(\*115th group coefficients r2^7r3^5\*)

**Plot[Cf[7, 5, 14], {x, 0, 1}]**

[绘图](#)

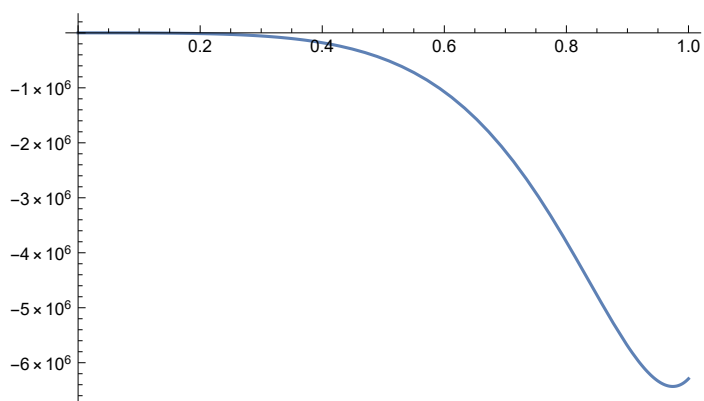

**Plot[Cf[7, 5, 13], {x, 0, 1}]**

[绘图](#)

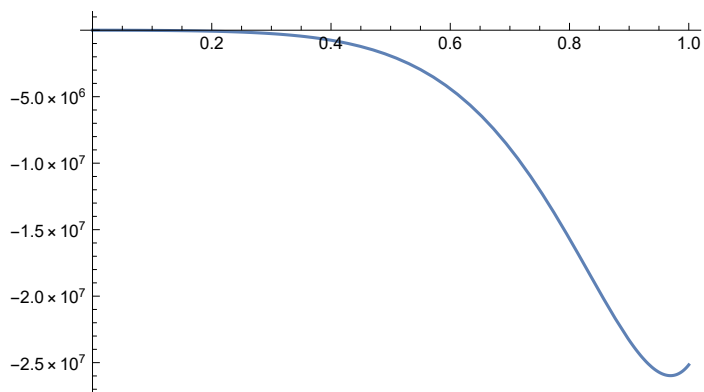

**Plot[Cf[7, 5, 12], {x, 0, 1}]**

[绘图](#)

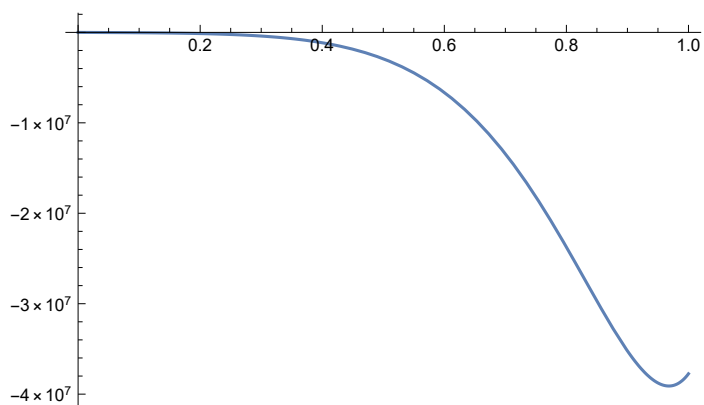

**Plot[Cf[7, 5, 11], {x, 0, 1}]**

[绘图](#)

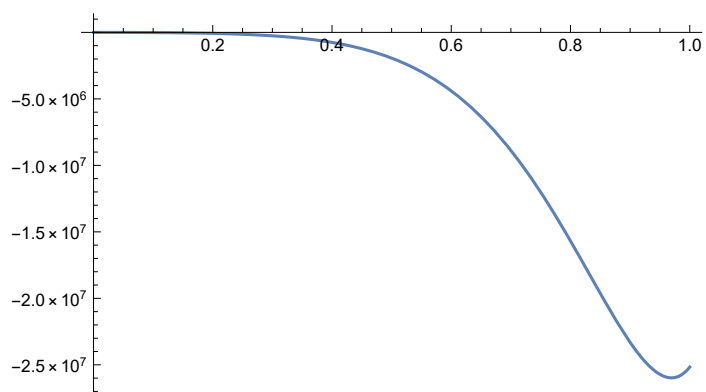

**Plot[Cf[7, 5, 10], {x, 0, 1}]**

[绘图](#)

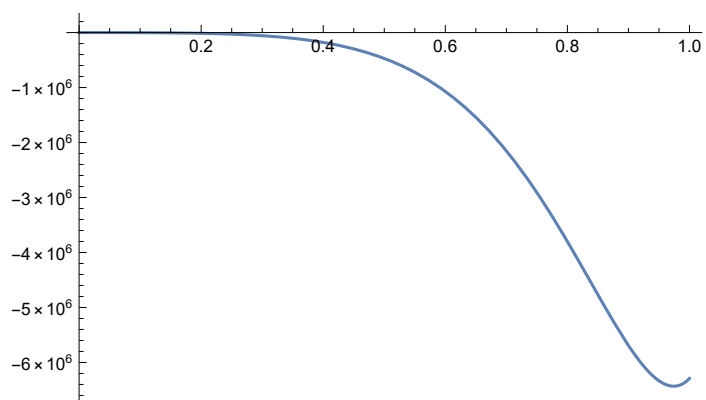

**Plot[Cf[7, 5, 9], {x, 0, 1}]**

[绘图](#)

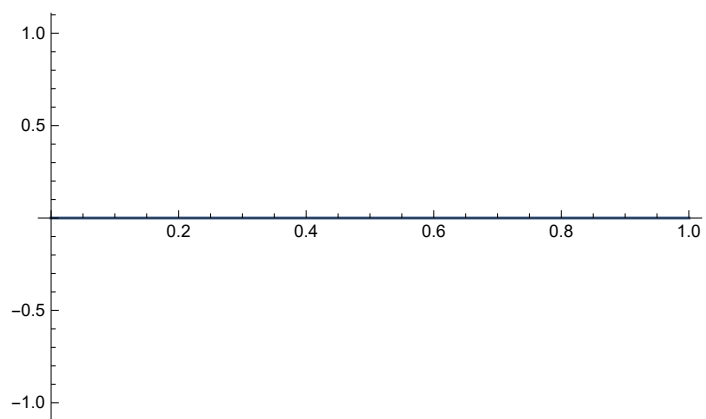

(\*116th group coefficients r2^7r3^4\*)



**Plot[Cf[7, 4, 14], {x, 0, 1}]**

[绘图](#)

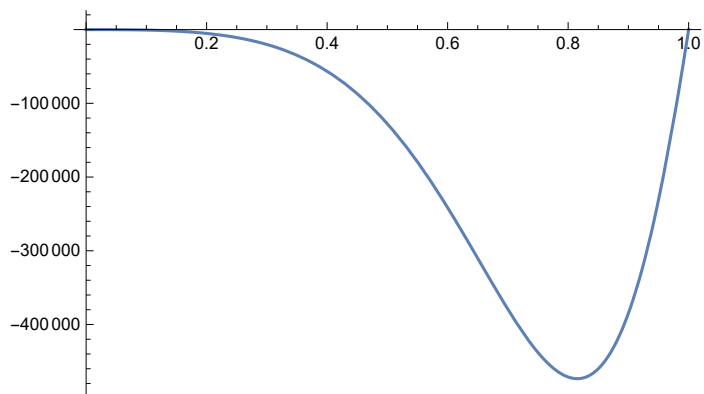

**Plot[Cf[7, 4, 13], {x, 0, 1}]**

[绘图](#)

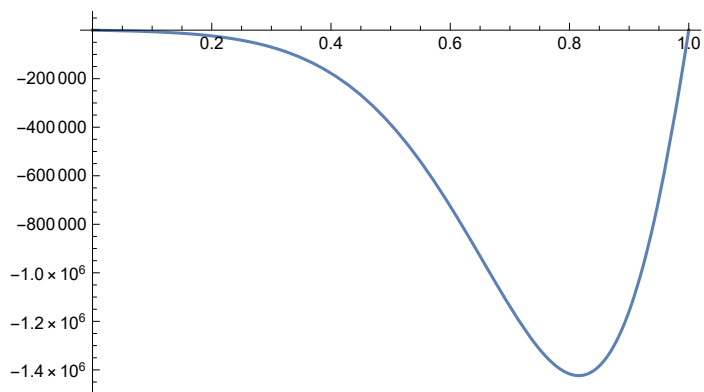

**Plot[Cf[7, 4, 12], {x, 0, 1}]**

[绘图](#)

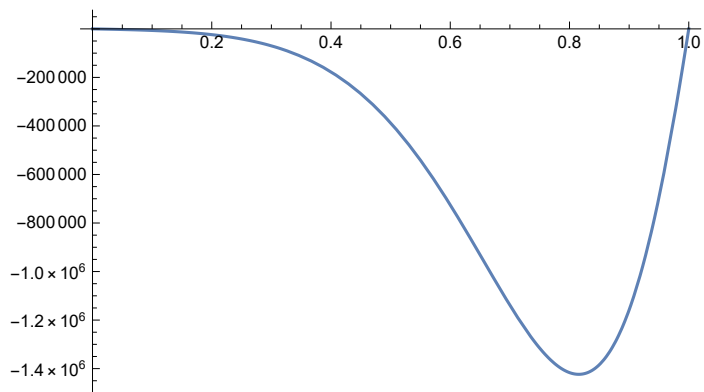

**Plot[Cf[7, 4, 11], {x, 0, 1}]**

[绘图](#)

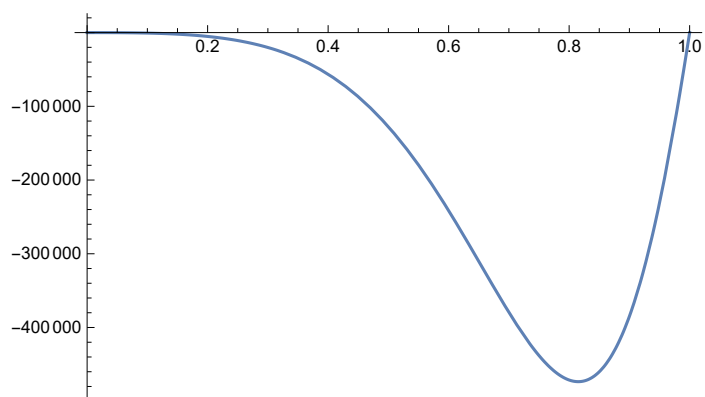

**Plot[Cf[7, 4, 10], {x, 0, 1}]**

[绘图](#)

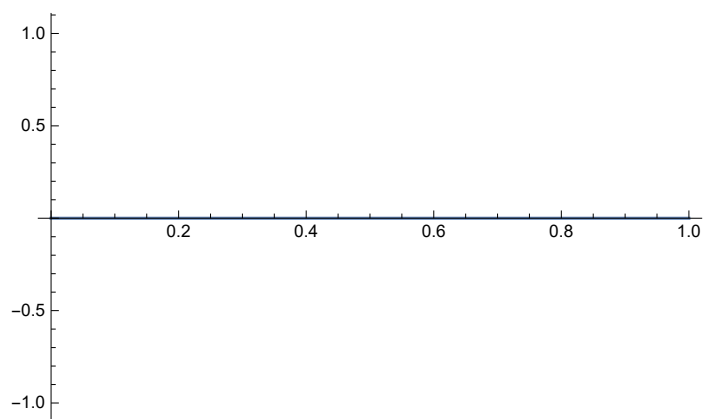

**(\*117th group coefficients r2^7r3^3\*)**

**Plot[Cf[7, 3, 14], {x, 0, 1}]**

[绘图](#)

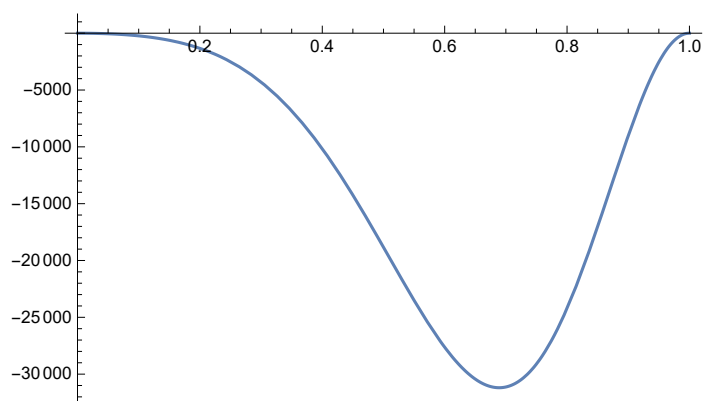

**Plot[Cf[7, 3, 13], {x, 0, 1}]**

[绘图](#)

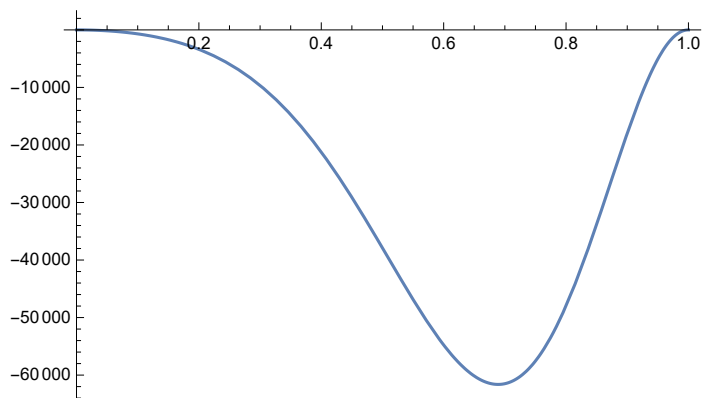

**Plot[Cf[7, 3, 12], {x, 0, 1}]**

[绘图](#)

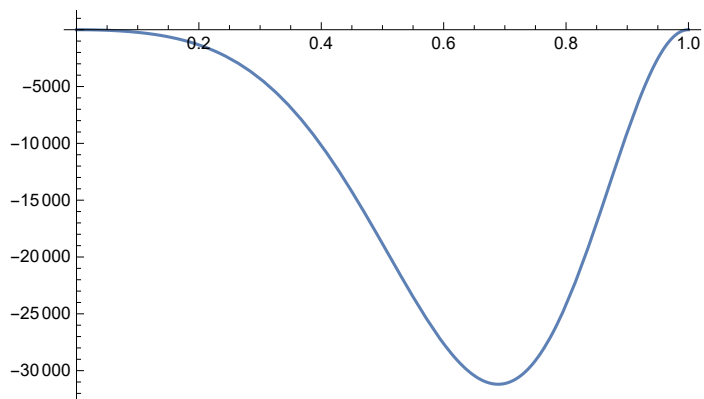

**Plot[Cf[7, 3, 11], {x, 0, 1}]**

[绘图](#)

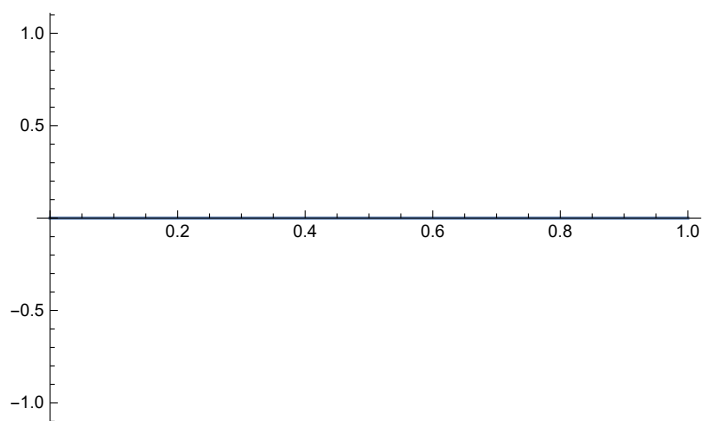

(\*118th group coefficients r2^7r3^2\*)

**Plot[Cf[7, 2, 14], {x, 0, 1}]**

[绘图](#)

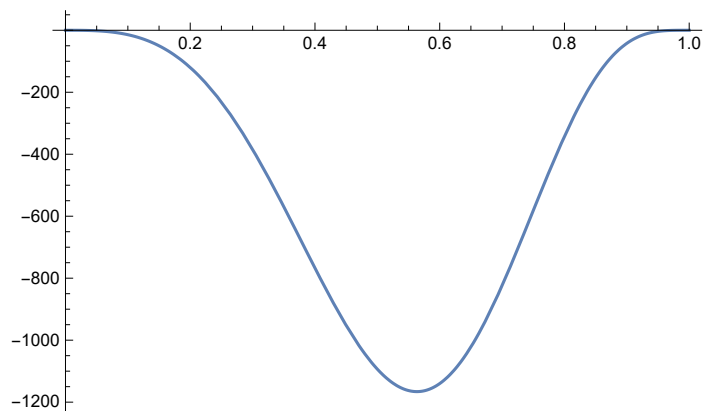

**Plot[Cf[7, 2, 13], {x, 0, 1}]**

[绘图](#)

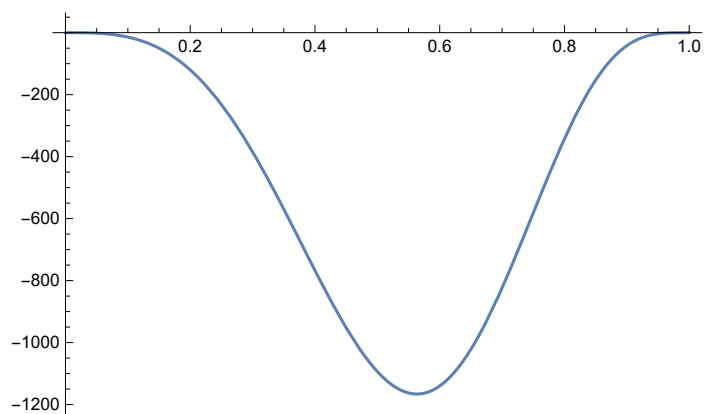

**Plot[Cf[7, 2, 12], {x, 0, 1}]**

[绘图](#)

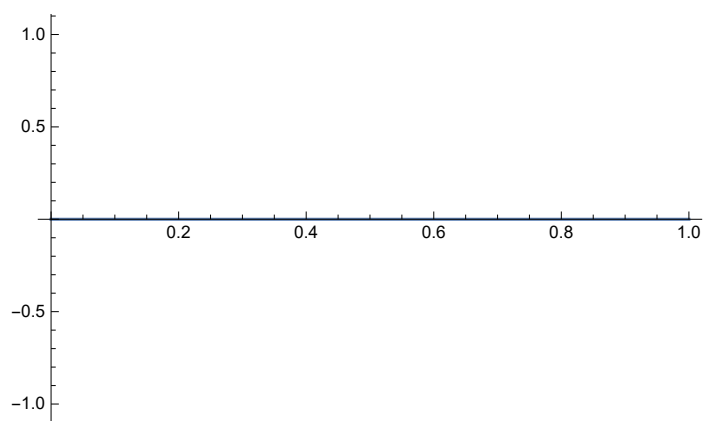

**(\*119th group coefficients r2^7r3^1\*)**

**Plot[Cf[7, 1, 14], {x, 0, 1}]**

[绘图](#)

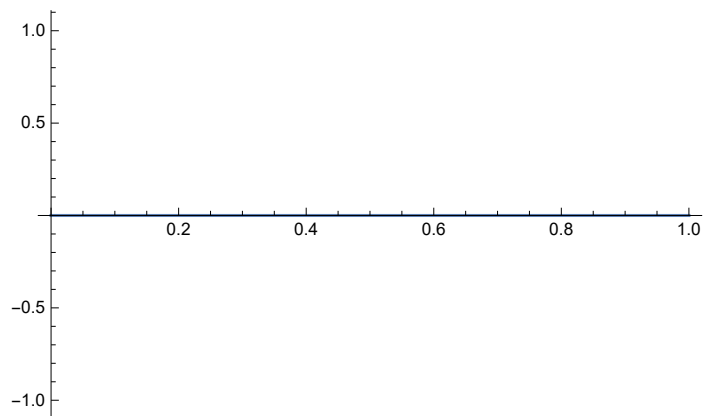

(\*120th group coefficients r2^7r3^0\*)

**Plot[Cf[7, 0, 14], {x, 0, 1}]**

[绘图](#)

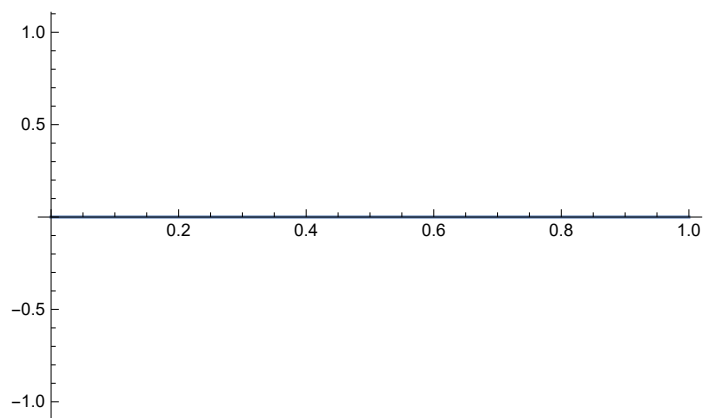

(\*121th group coefficients r2^6r3^14\*)

**Plot[Cf[6, 14, 14], {x, 0, 1}]**

[绘图](#)

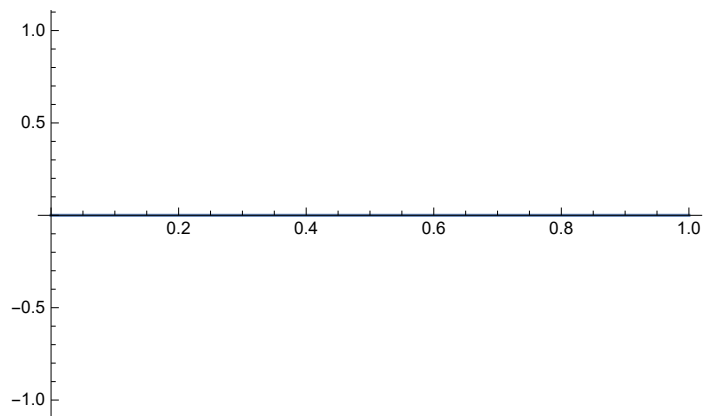

**Plot[Cf[6, 14, 13], {x, 0, 1}]**

[绘图](#)

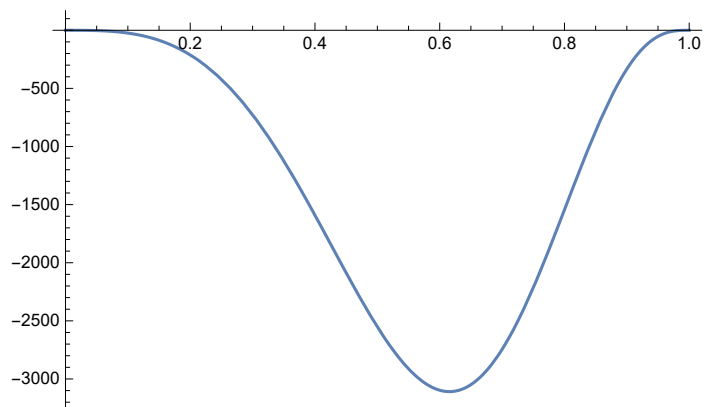

**Plot[Cf[6, 14, 12], {x, 0, 1}]**

[绘图](#)

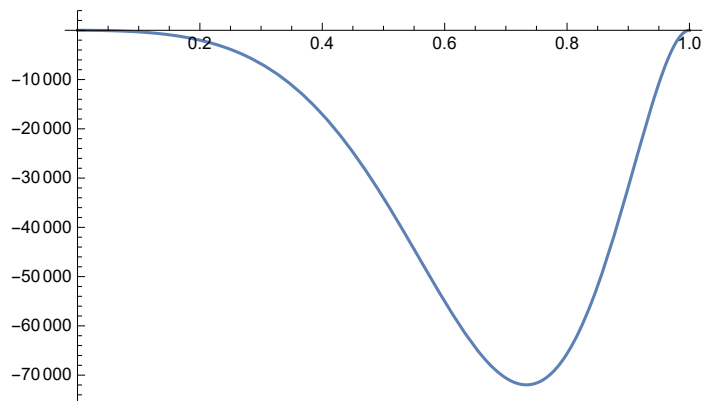

**Plot[Cf[6, 14, 11], {x, 0, 1}]**

[绘图](#)

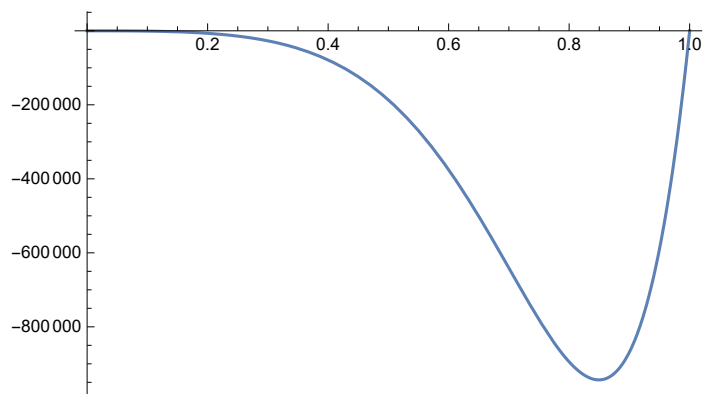

**Plot[Cf[6, 14, 10], {x, 0, 1}]**

[绘图](#)

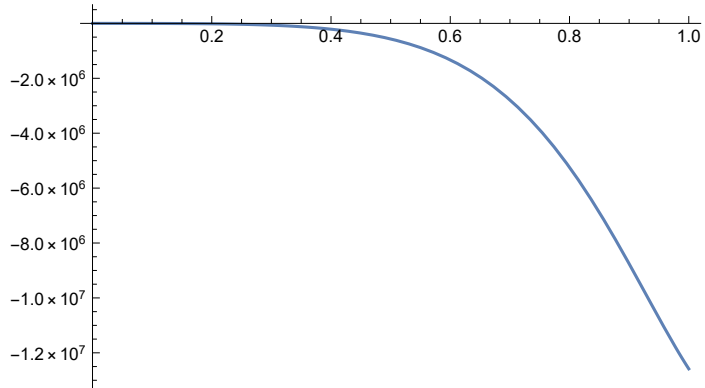

**Plot[Cf[6, 14, 9], {x, 0, 1}]**

[绘图](#)

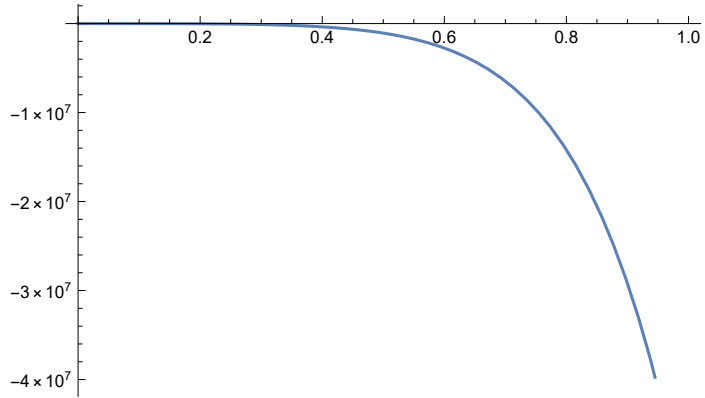

**Plot[Cf[6, 14, 8], {x, 0, 1}]**

[绘图](#)

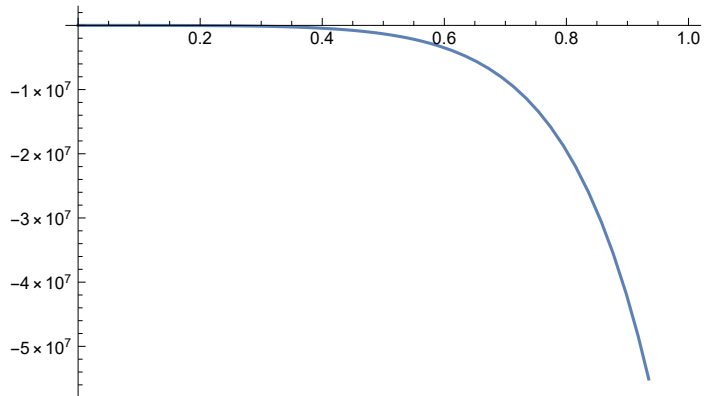

**Plot[Cf[6, 14, 7], {x, 0, 1}]**

[绘图](#)

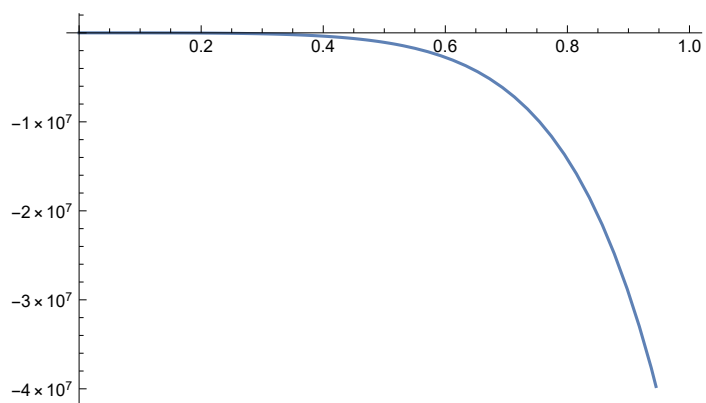

**Plot[Cf[6, 14, 6], {x, 0, 1}]**

[绘图](#)

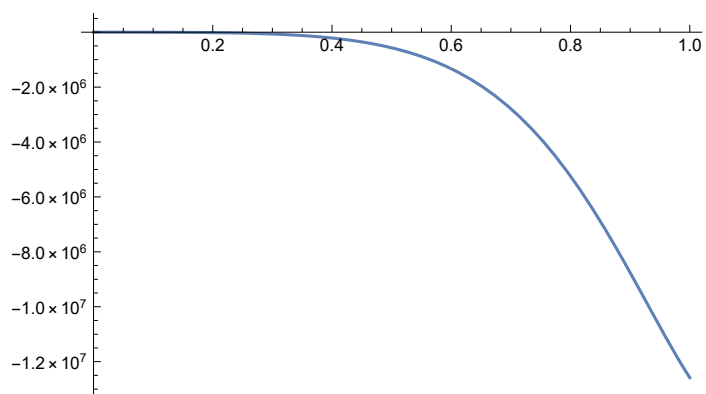

**Plot[Cf[6, 14, 5], {x, 0, 1}]**

[绘图](#)

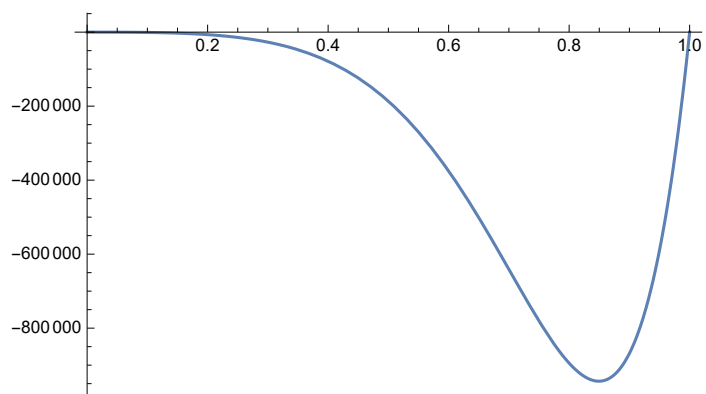



**Plot[Cf[6, 14, 4], {x, 0, 1}]**

[绘图](#)

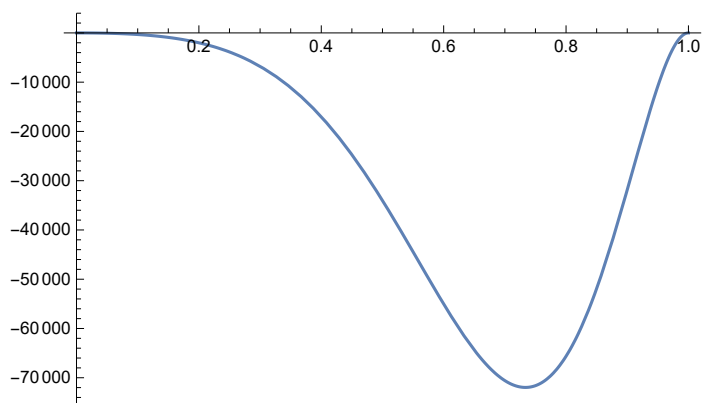

**Plot[Cf[6, 14, 3], {x, 0, 1}]**

[绘图](#)

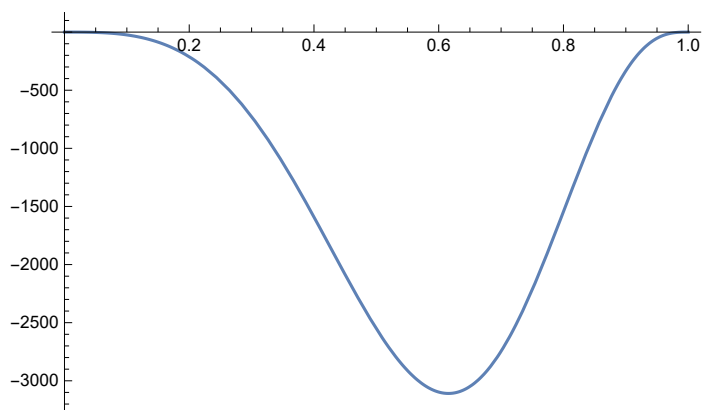

**Plot[Cf[6, 14, 2], {x, 0, 1}]**

[绘图](#)

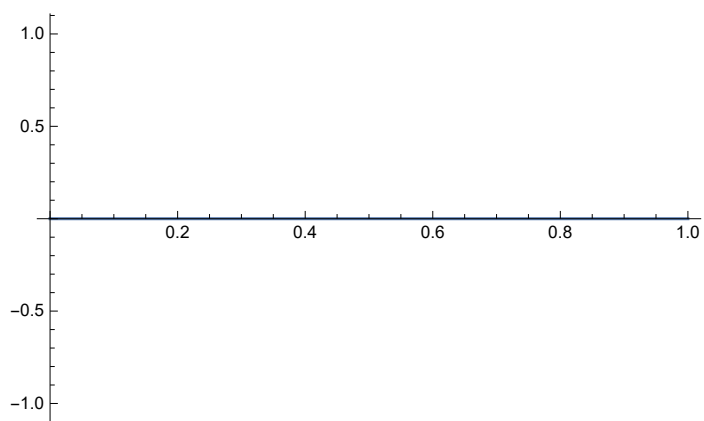

**Plot[Cf[6, 14, 1], {x, 0, 1}]**

[绘图](#)

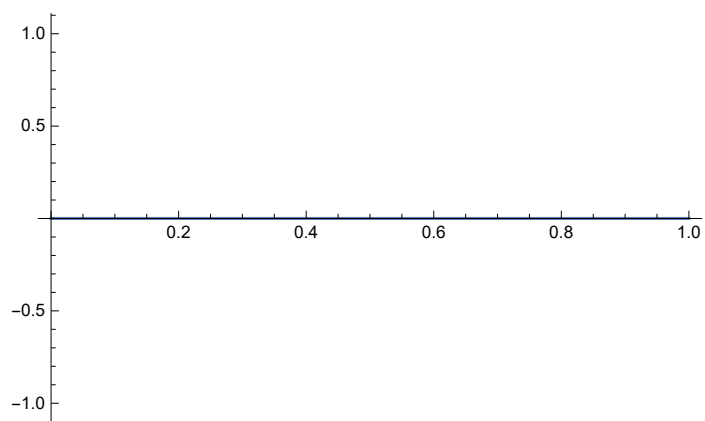

(\*122th group coefficients r2^6r3^13\*)

**Plot[Cf[6, 13, 14], {x, 0, 1}]**

[绘图](#)

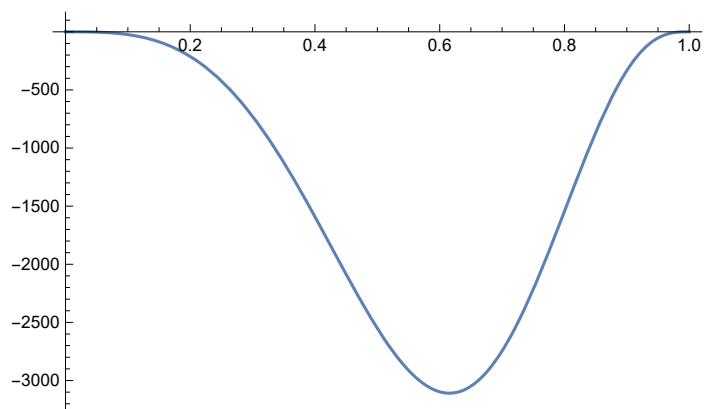

**Plot[Cf[6, 13, 13], {x, 0, 1}]**

[绘图](#)

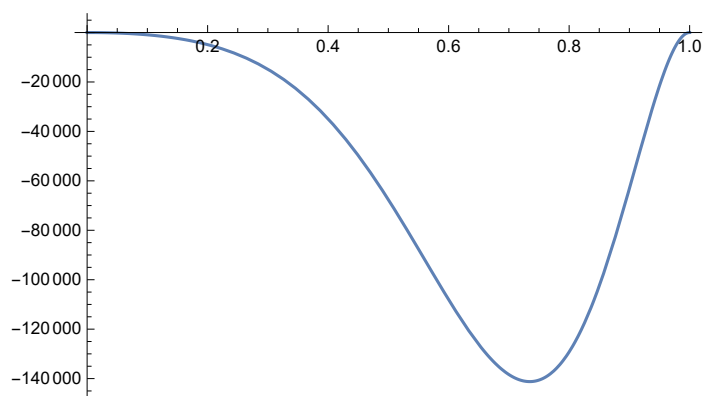

**Plot[Cf[6, 13, 12], {x, 0, 1}]**

[绘图](#)

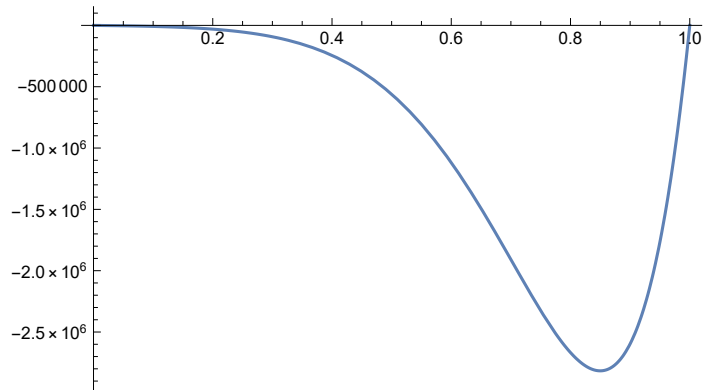

**Plot[Cf[6, 13, 11], {x, 0, 1}]**

[绘图](#)

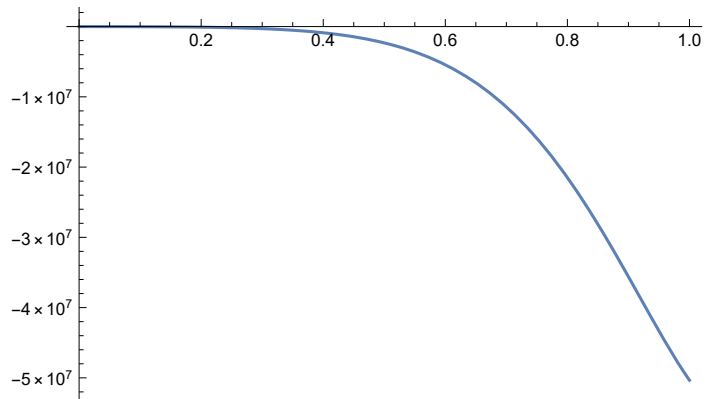

**Plot[Cf[6, 13, 10], {x, 0, 1}]**

[绘图](#)

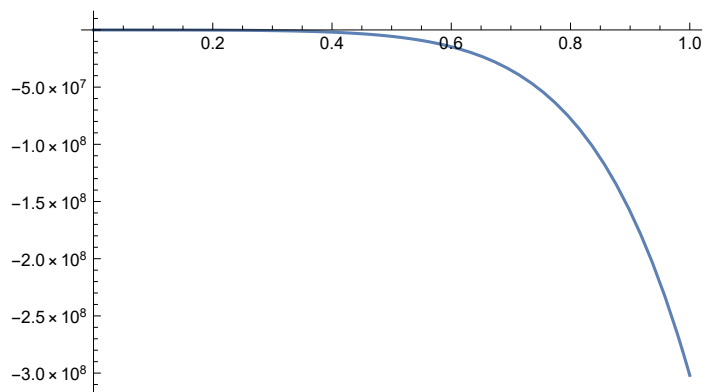

**Plot[Cf[6, 13, 9], {x, 0, 1}]**

[绘图](#)

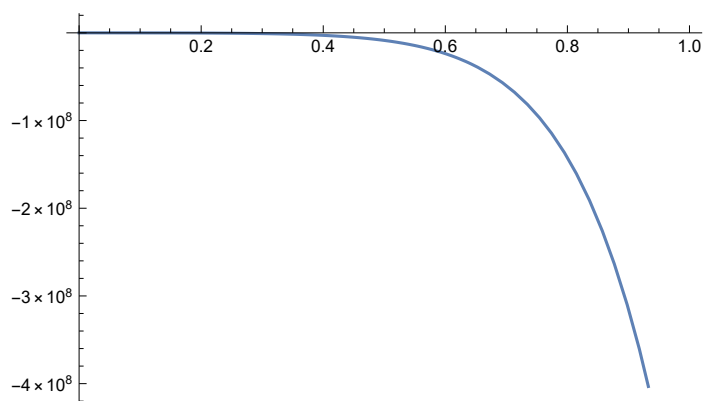

**Plot[Cf[6, 13, 8], {x, 0, 1}]**

[绘图](#)

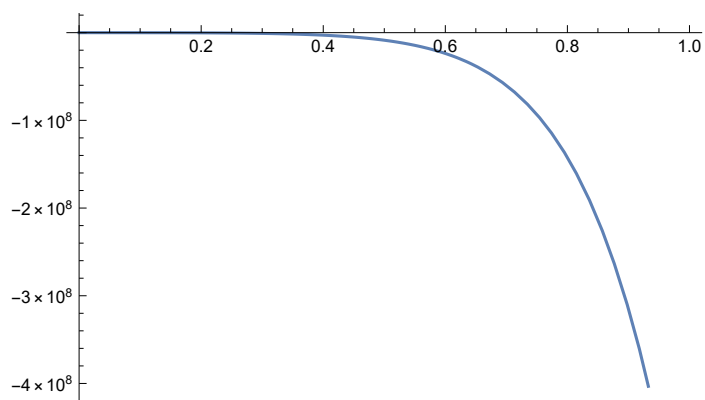

**Plot[Cf[6, 13, 7], {x, 0, 1}]**

[绘图](#)

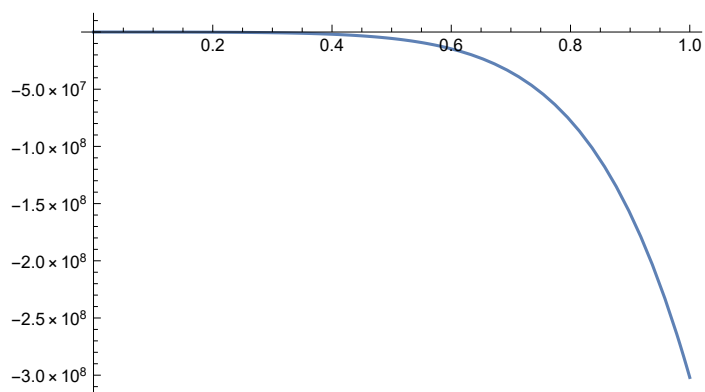

**Plot[Cf[6, 13, 6], {x, 0, 1}]**

[绘图](#)

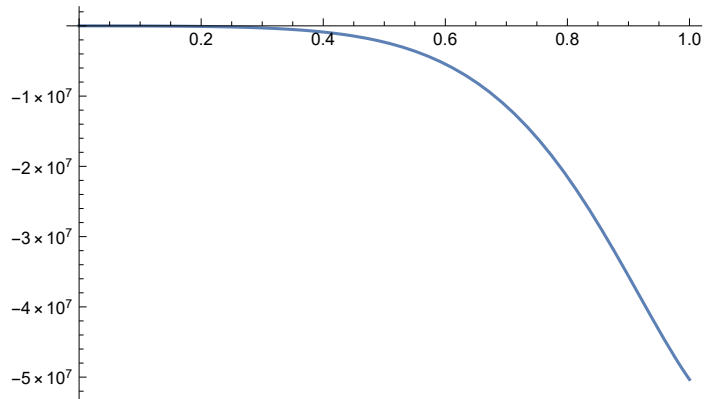

**Plot[Cf[6, 13, 5], {x, 0, 1}]**

[绘图](#)

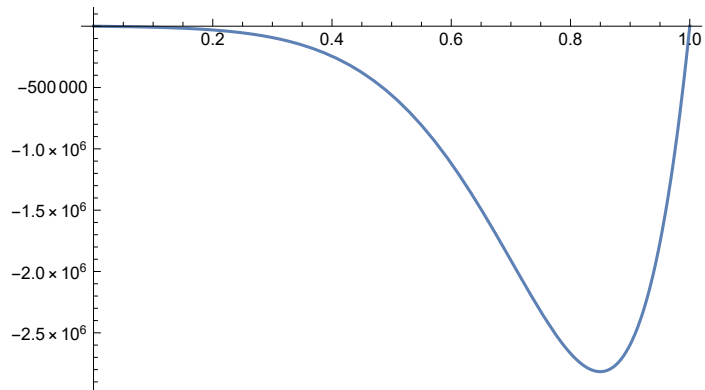

**Plot[Cf[6, 13, 4], {x, 0, 1}]**

[绘图](#)

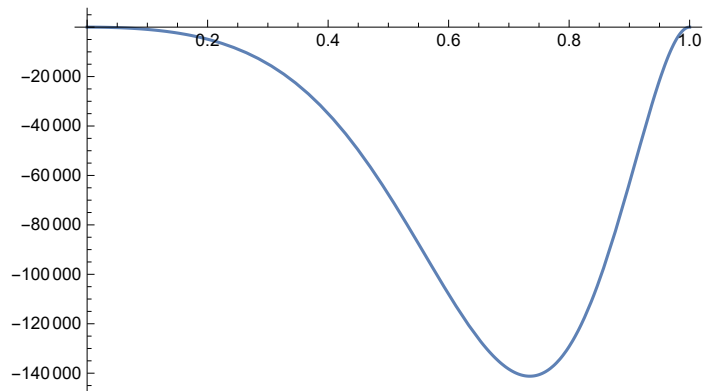

**Plot[Cf[6, 13, 3], {x, 0, 1}]**

[绘图](#)

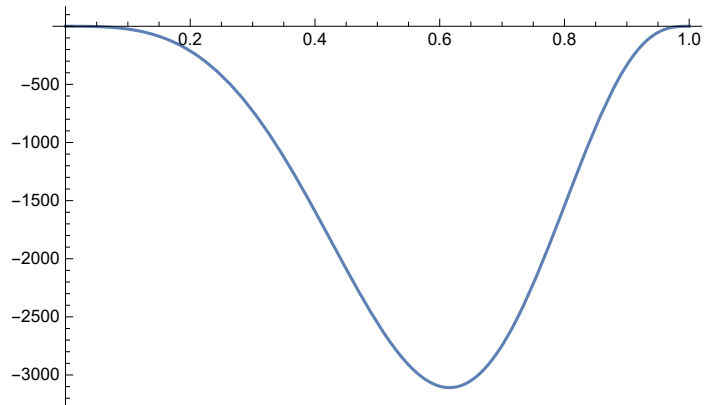

**Plot[Cf[6, 13, 2], {x, 0, 1}]**

[绘图](#)

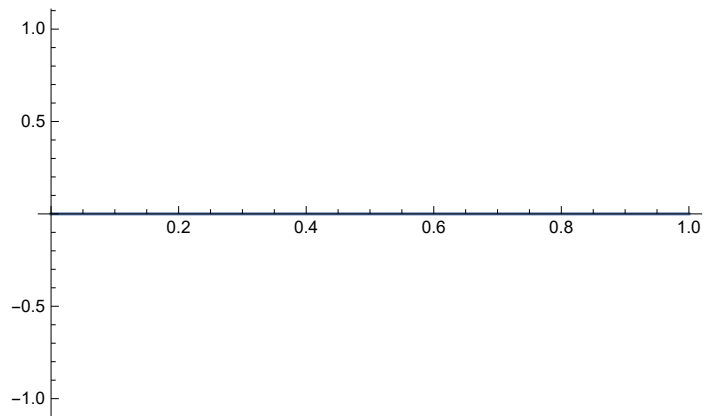

**(\*123th group coefficients r2^6r3^12\*)**

**Plot[Cf[6, 12, 14], {x, 0, 1}]**

[绘图](#)

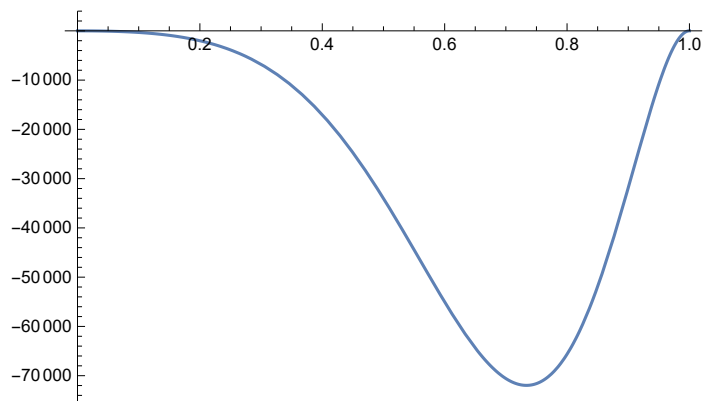

**Plot[Cf[6, 12, 13], {x, 0, 1}]**

[绘图](#)

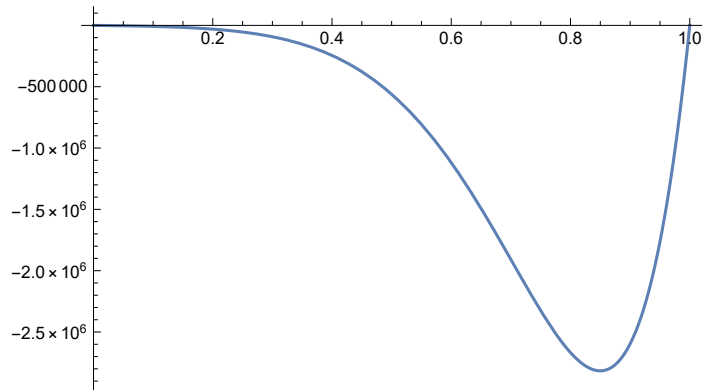

**Plot[Cf[6, 12, 12], {x, 0, 1}]**

[绘图](#)

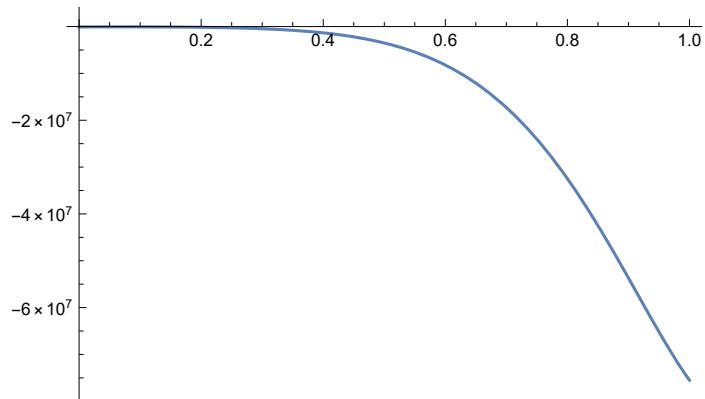

**Plot[Cf[6, 12, 11], {x, 0, 1}]**

[绘图](#)

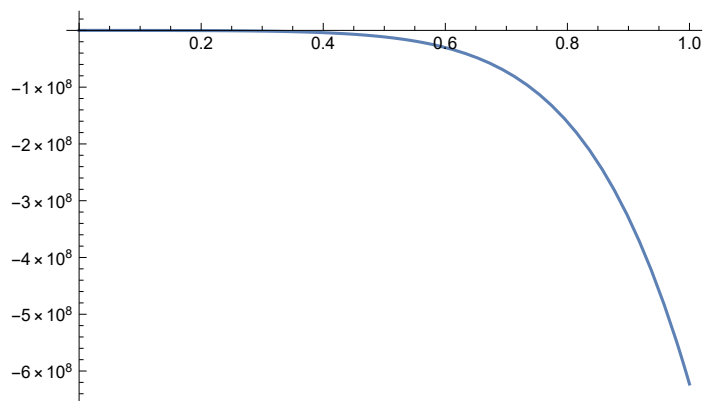

**Plot[Cf[6, 12, 10], {x, 0, 1}]**

[绘图](#)

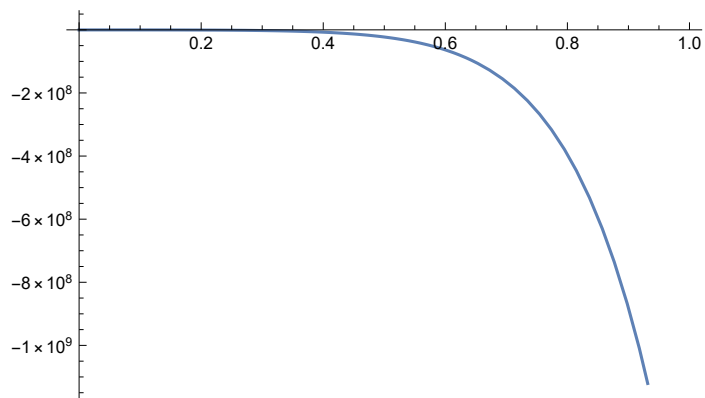

**Plot[Cf[6, 12, 9], {x, 0, 1}]**

[绘图](#)

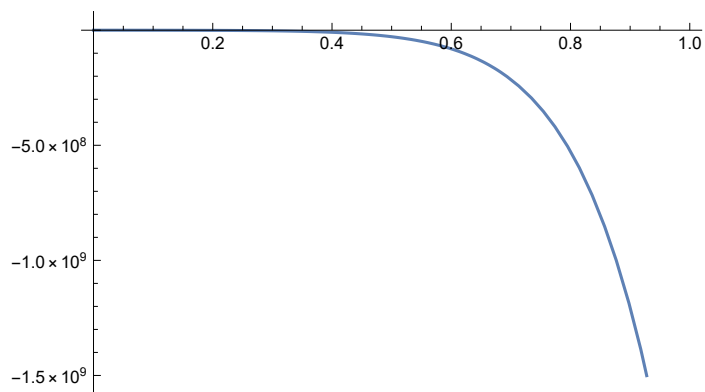

**Plot[Cf[6, 12, 8], {x, 0, 1}]**

[绘图](#)

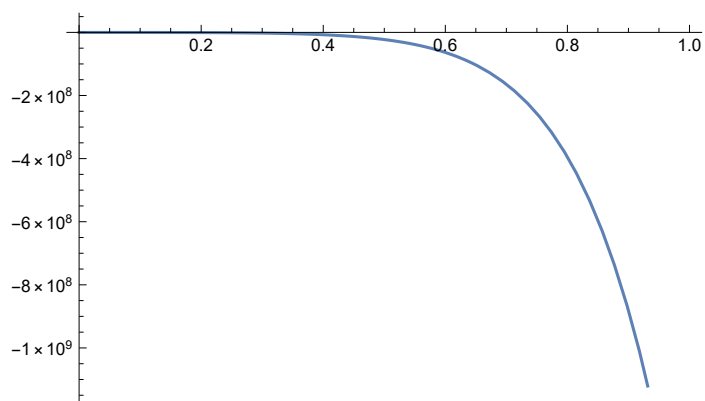



**Plot[Cf[6, 12, 7], {x, 0, 1}]**

[绘图](#)

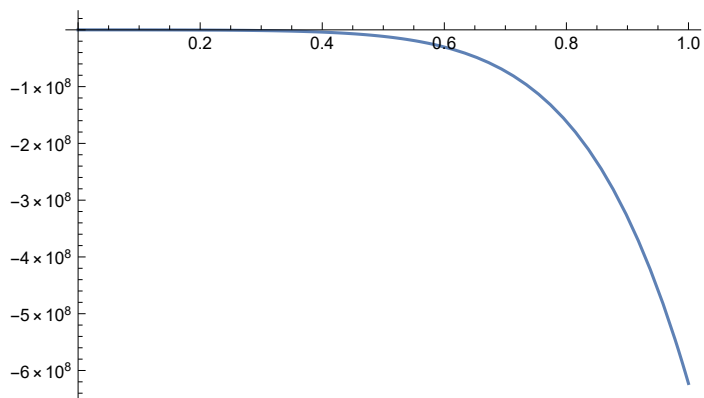

**Plot[Cf[6, 12, 6], {x, 0, 1}]**

[绘图](#)

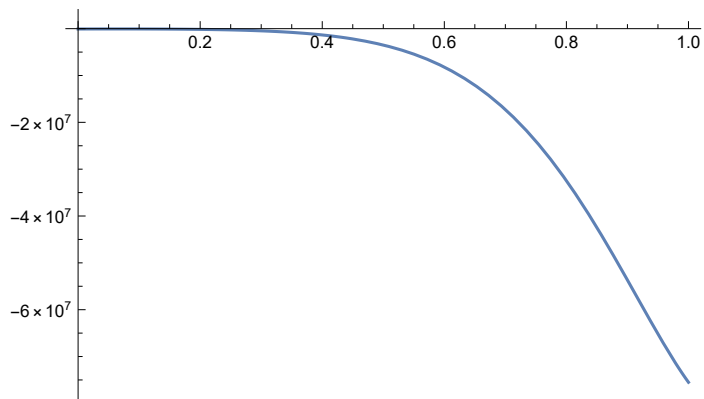

**Plot[Cf[6, 12, 5], {x, 0, 1}]**

[绘图](#)

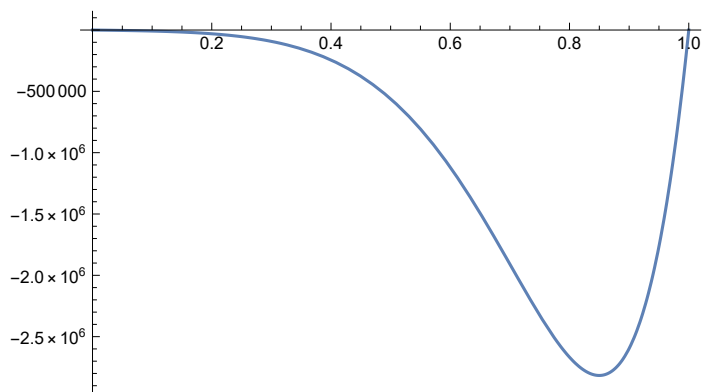

**Plot[Cf[6, 12, 4], {x, 0, 1}]**

[绘图](#)

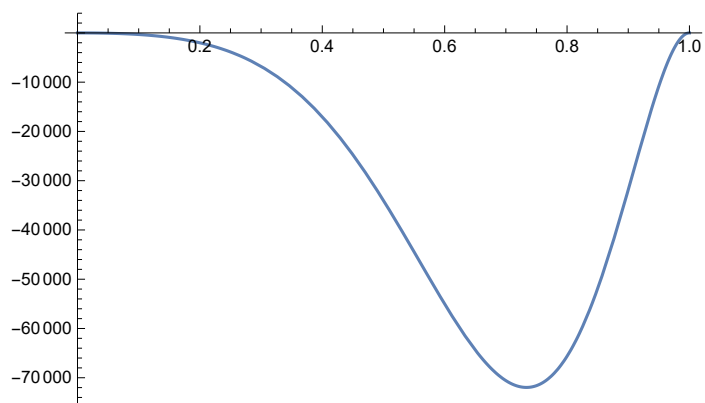

**Plot[Cf[6, 12, 3], {x, 0, 1}]**

[绘图](#)

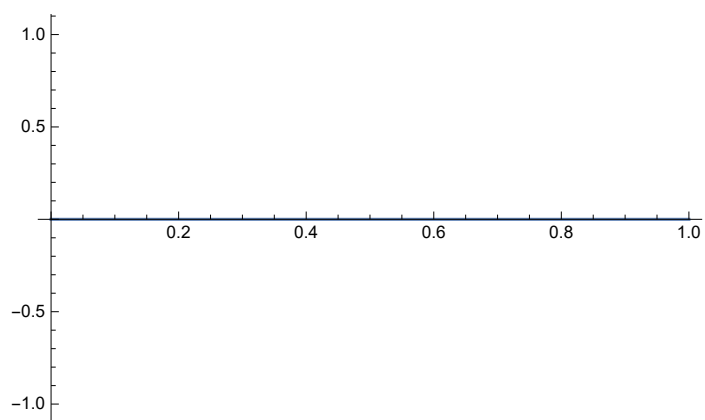

**(\*124th group coefficients r2^6r3^11\*)**

**Plot[Cf[6, 11, 14], {x, 0, 1}]**

[绘图](#)

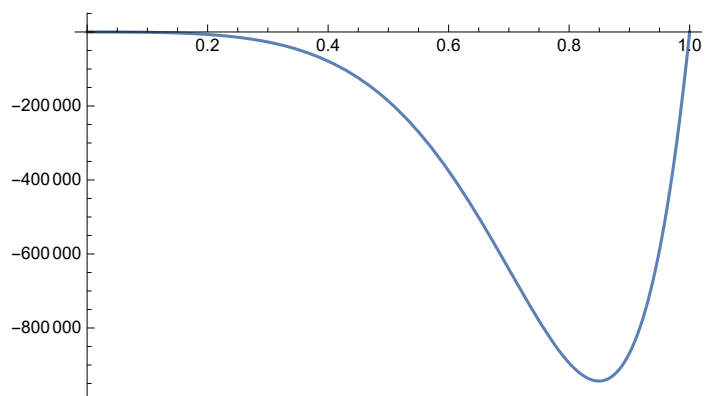

**Plot[Cf[6, 11, 13], {x, 0, 1}]**

[绘图](#)

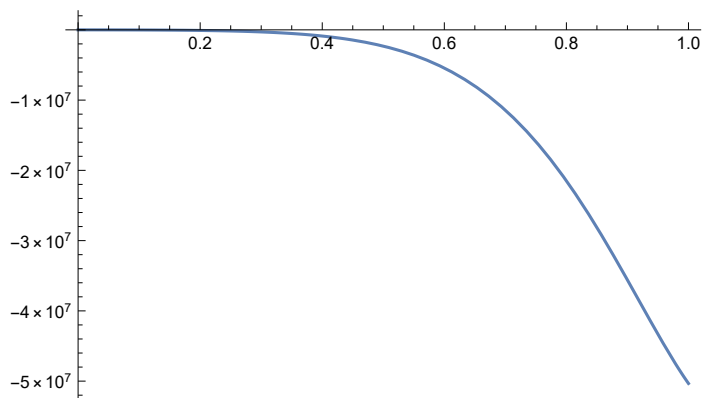

**Plot[Cf[6, 11, 12], {x, 0, 1}]**

[绘图](#)

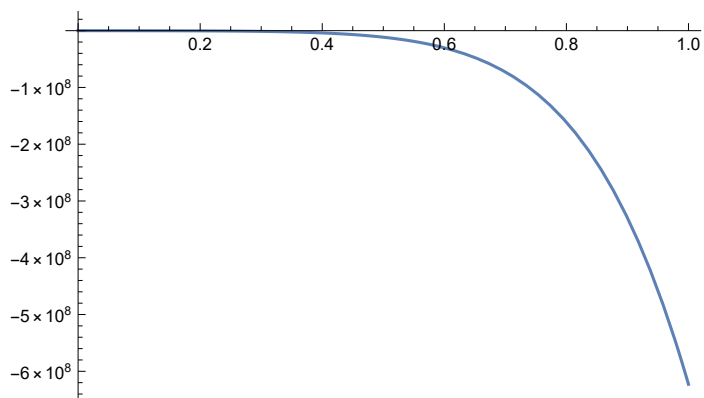

**Plot[Cf[6, 11, 11], {x, 0, 1}]**

[绘图](#)

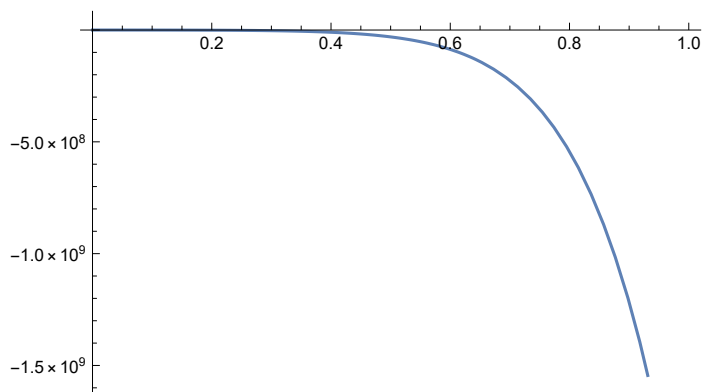

**Plot[Cf[6, 11, 10], {x, 0, 1}]**

[绘图](#)

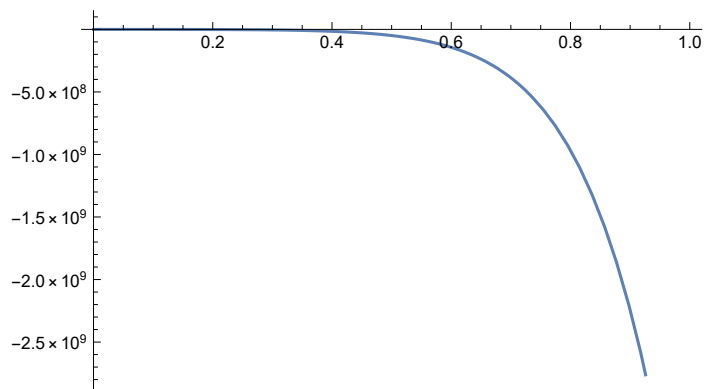

**Plot[Cf[6, 11, 9], {x, 0, 1}]**

[绘图](#)

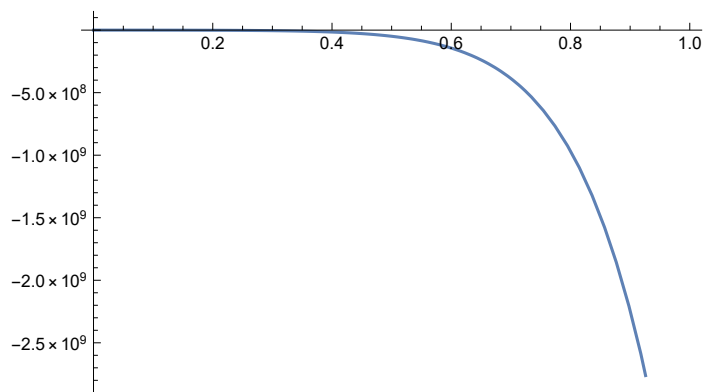

**Plot[Cf[6, 11, 8], {x, 0, 1}]**

[绘图](#)

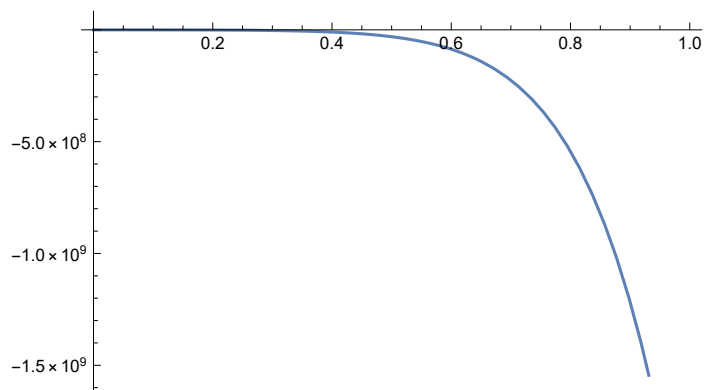

**Plot[Cf[6, 11, 7], {x, 0, 1}]**

[绘图](#)

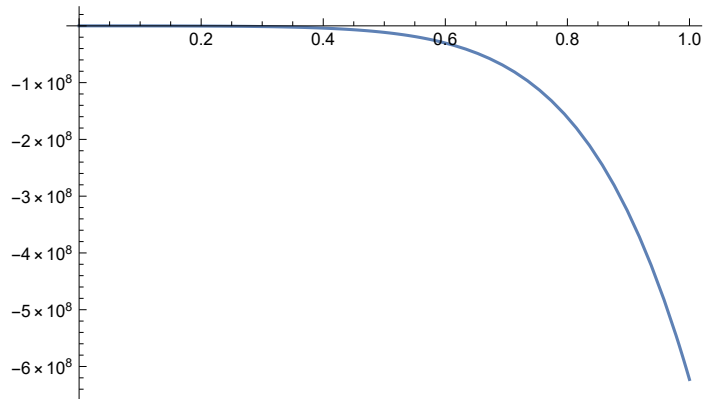

**Plot[Cf[6, 11, 6], {x, 0, 1}]**

[绘图](#)

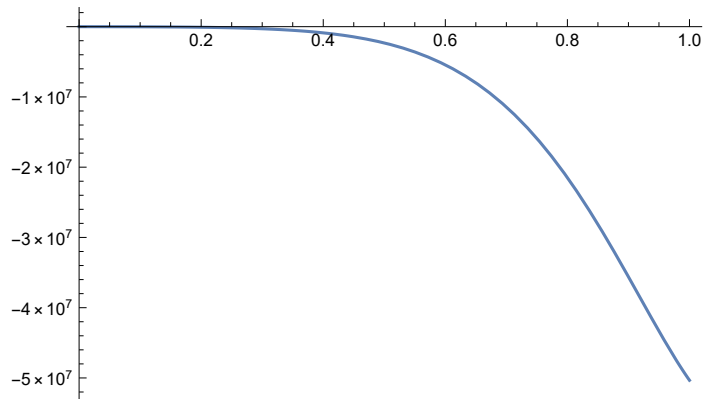

**Plot[Cf[6, 11, 5], {x, 0, 1}]**

[绘图](#)

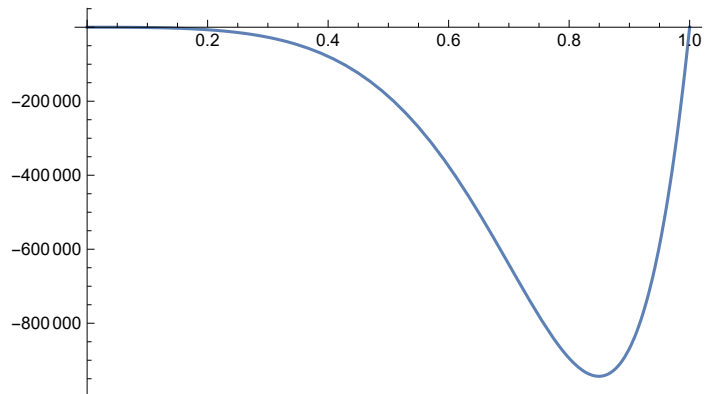

**Plot[Cf[6, 11, 4], {x, 0, 1}]**

[绘图](#)

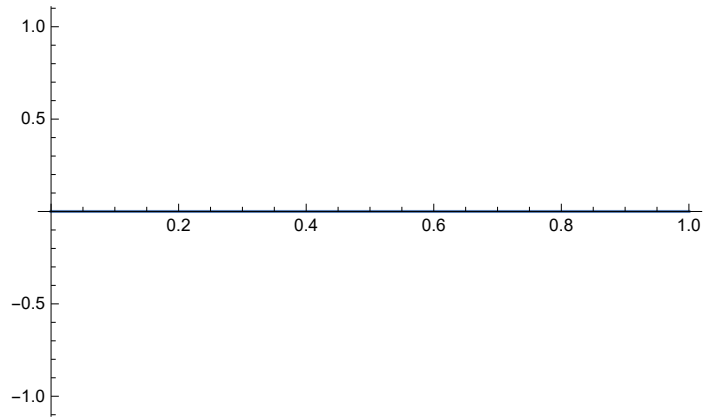

(\*125th group coefficients  $r2^6 r3^{10}$ \*)

**Plot[Cf[6, 10, 14], {x, 0, 1}]**

[绘图](#)

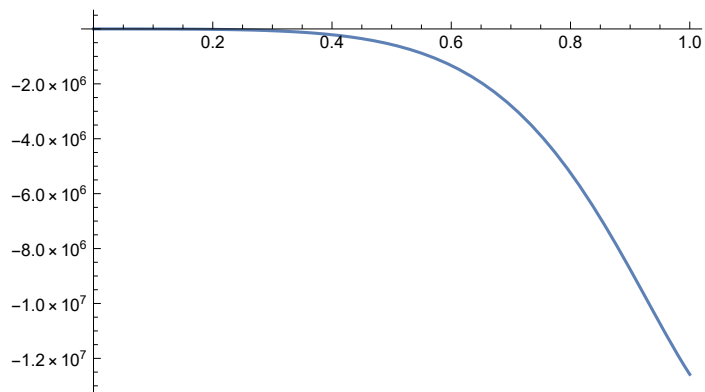

**Plot[Cf[6, 10, 13], {x, 0, 1}]**

[绘图](#)

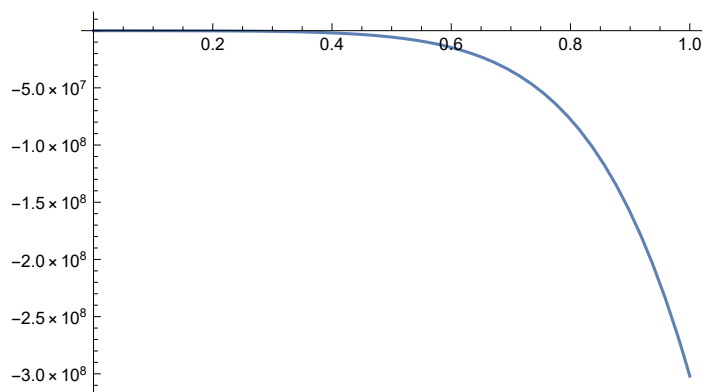

**Plot[Cf[6, 10, 12], {x, 0, 1}]**

[绘图](#)

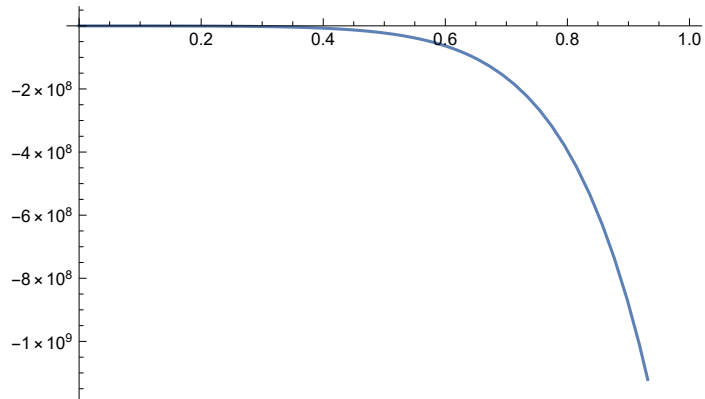

**Plot[Cf[6, 10, 11], {x, 0, 1}]**

[绘图](#)

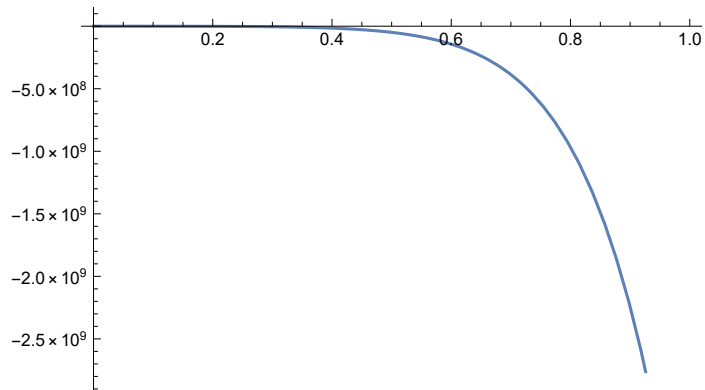

**Plot[Cf[6, 10, 10], {x, 0, 1}]**

[绘图](#)

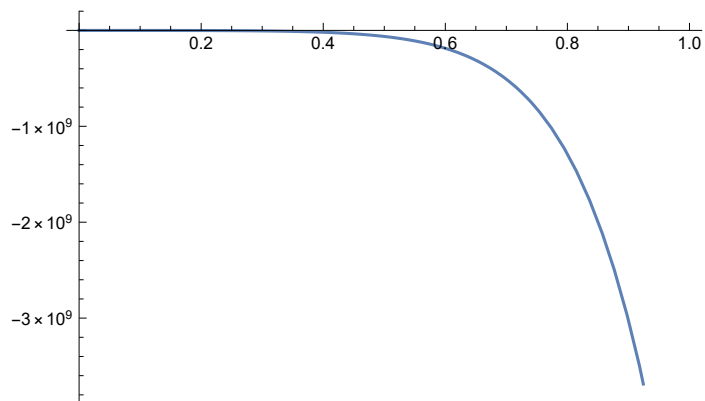

**Plot[Cf[6, 10, 9], {x, 0, 1}]**

[绘图](#)

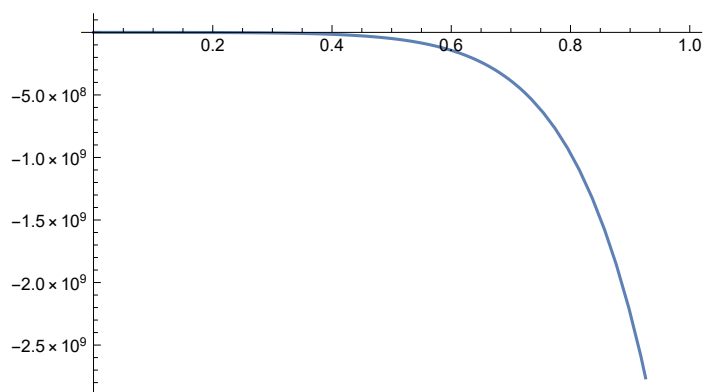

**Plot[Cf[6, 10, 8], {x, 0, 1}]**

[绘图](#)

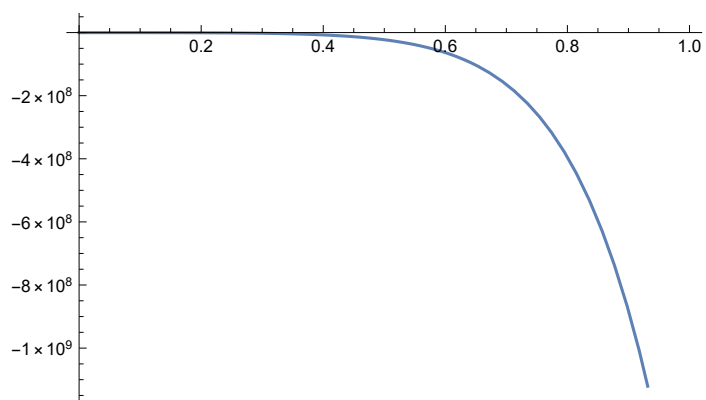

**Plot[Cf[6, 10, 7], {x, 0, 1}]**

[绘图](#)

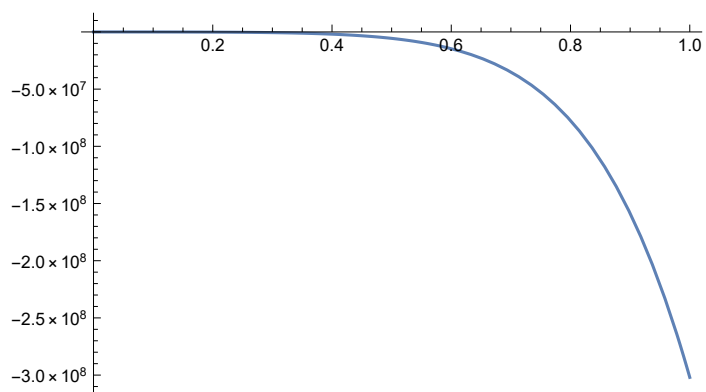



**Plot[Cf[6, 10, 6], {x, 0, 1}]**

[绘图](#)

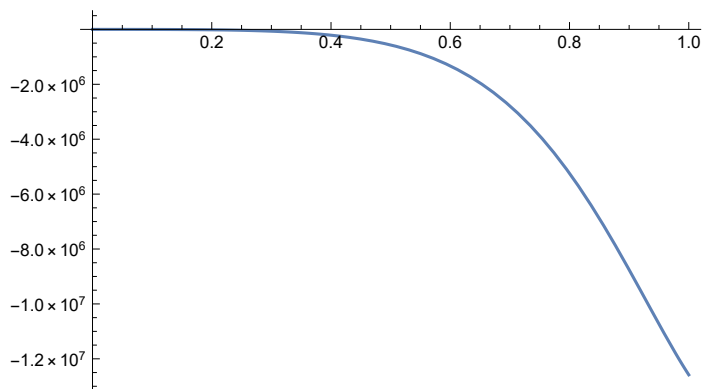

**Plot[Cf[6, 10, 5], {x, 0, 1}]**

[绘图](#)

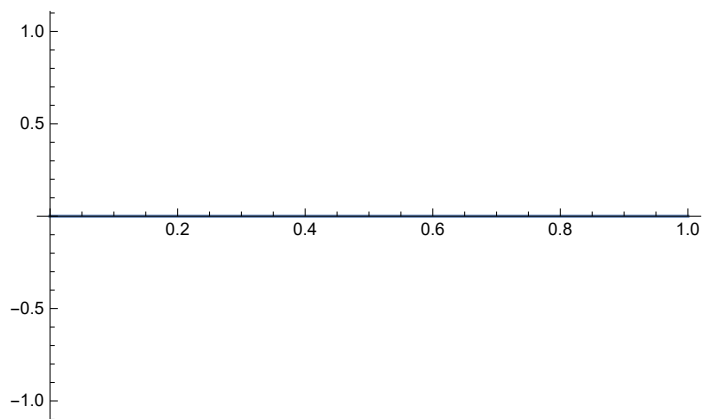

**(\*126th group coefficients r2^6r3^9\*)**

**Plot[Cf[6, 9, 14], {x, 0, 1}]**

[绘图](#)

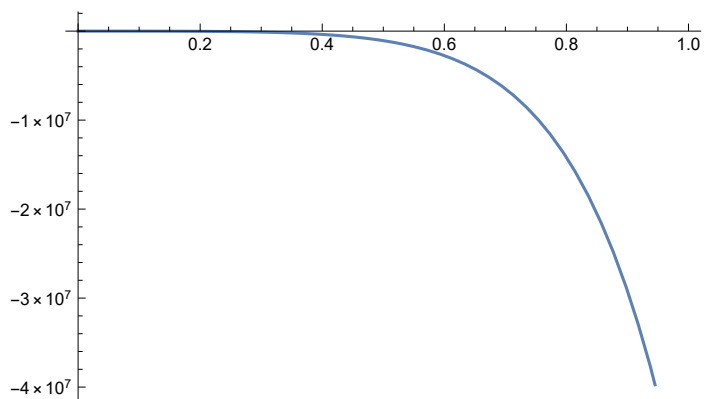

**Plot[Cf[6, 9, 13], {x, 0, 1}]**

[绘图](#)

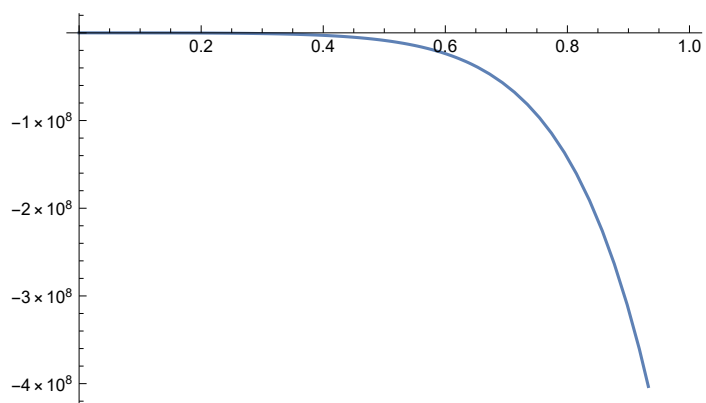

**Plot[Cf[6, 9, 12], {x, 0, 1}]**

[绘图](#)

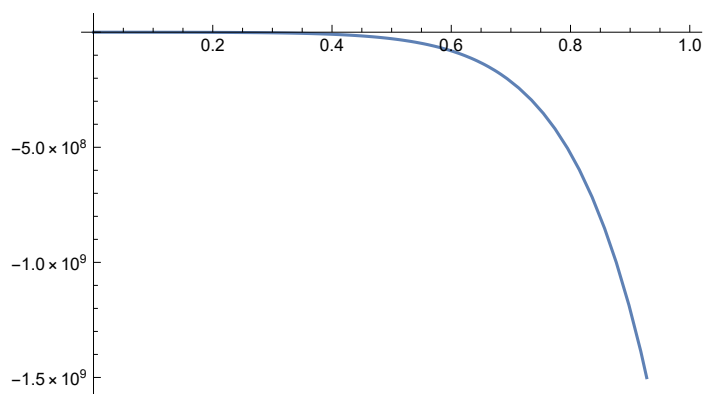

**Plot[Cf[6, 9, 11], {x, 0, 1}]**

[绘图](#)

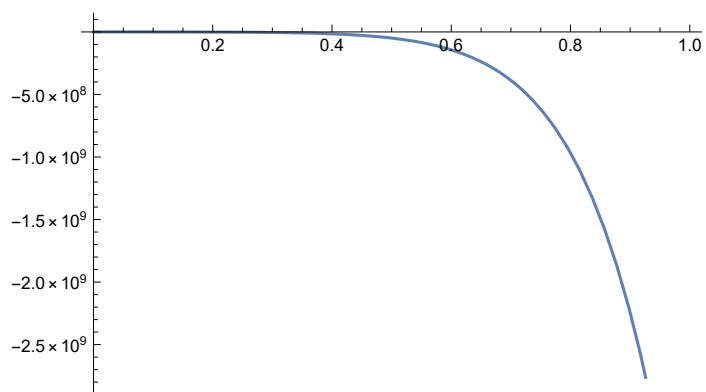

**Plot[Cf[6, 9, 10], {x, 0, 1}]**

[绘图](#)

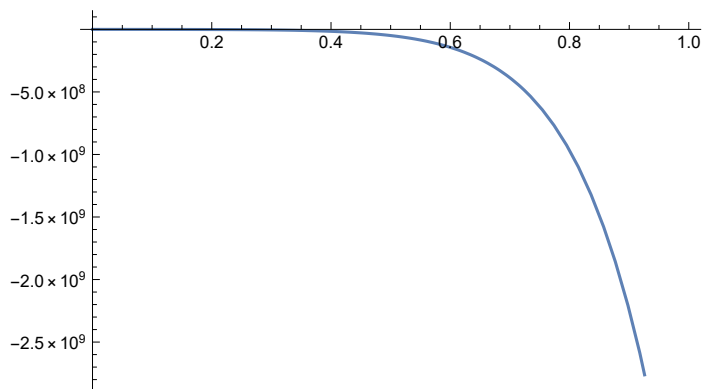

**Plot[Cf[6, 9, 9], {x, 0, 1}]**

[绘图](#)

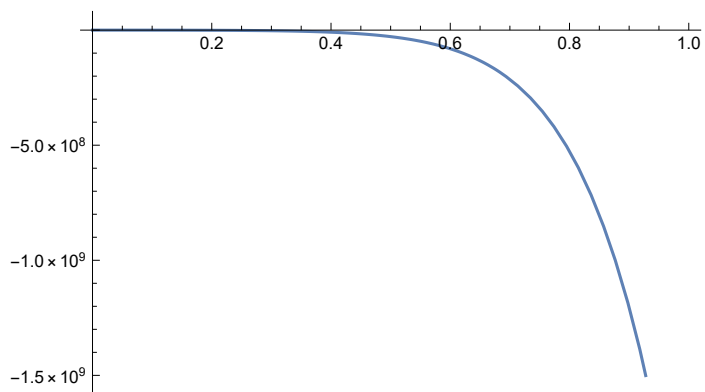

**Plot[Cf[6, 9, 8], {x, 0, 1}]**

[绘图](#)

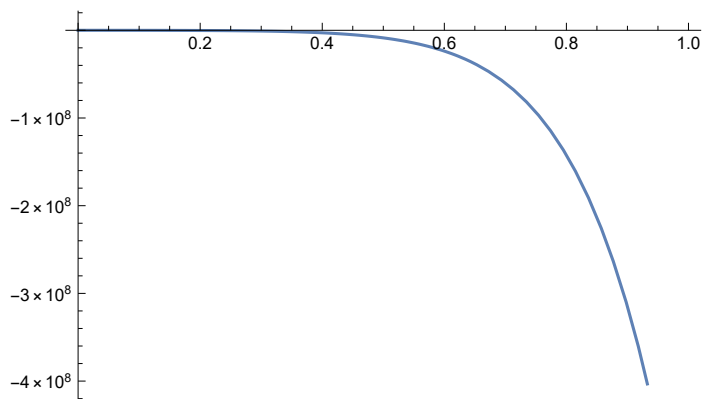

**Plot[Cf[6, 9, 7], {x, 0, 1}]**

[绘图](#)

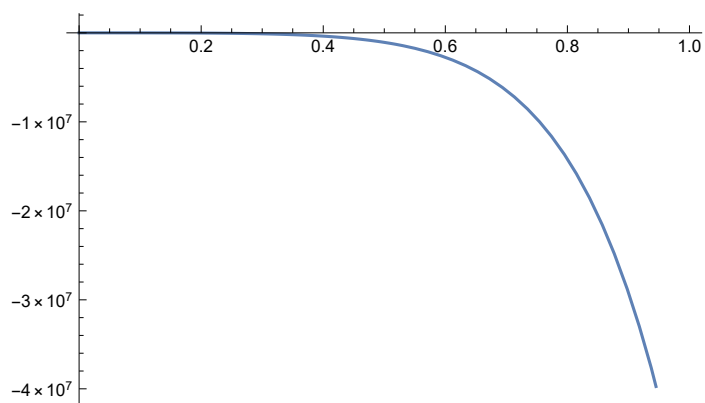

**Plot[Cf[6, 9, 6], {x, 0, 1}]**

[绘图](#)

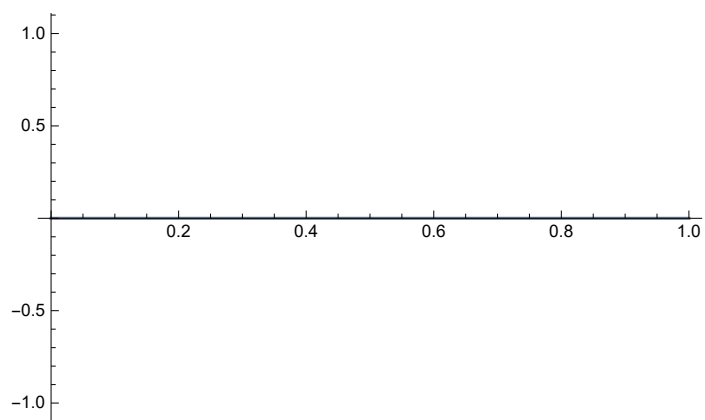

**(\*127th group coefficients r2^6r3^8\*)**

**Plot[Cf[6, 8, 14], {x, 0, 1}]**

[绘图](#)

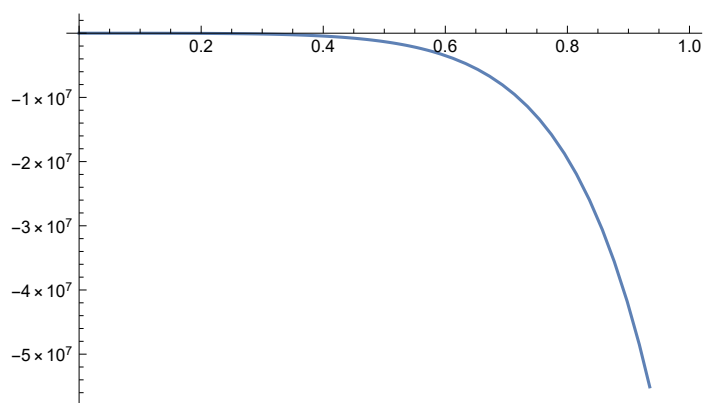

```
Plot[Cf[6, 8, 13], {x, 0, 1}]
```

[绘图](#)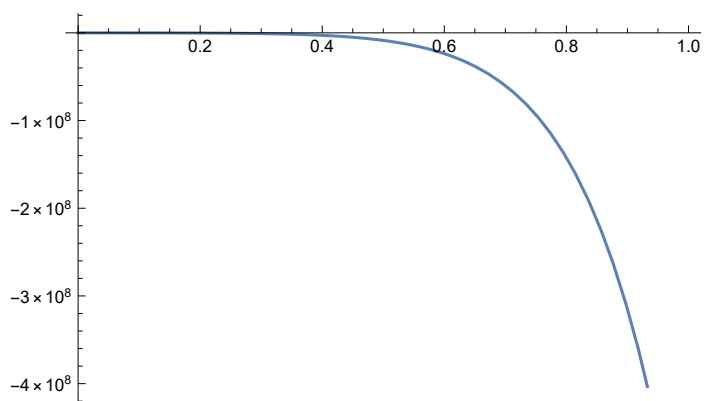

```
Plot[Cf[6, 8, 12], {x, 0, 1}]
```

[绘图](#)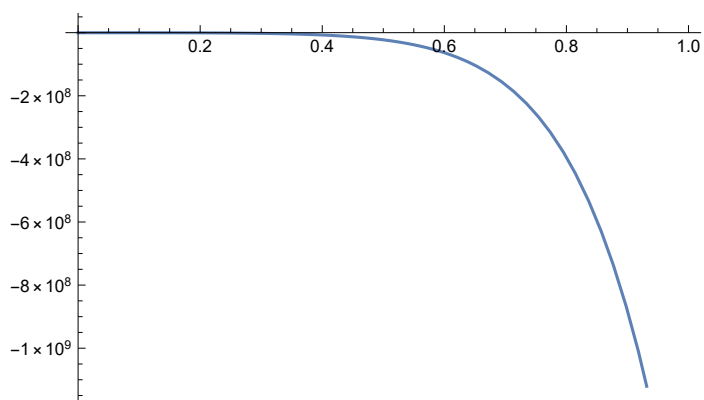

```
Plot[Cf[6, 8, 11], {x, 0, 1}]
```

[绘图](#)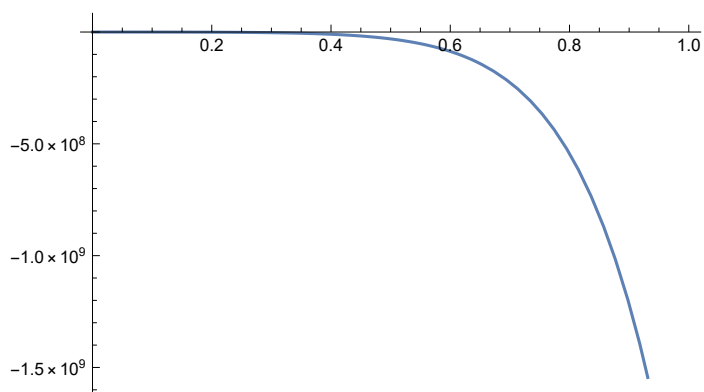

**Plot[Cf[6, 8, 10], {x, 0, 1}]**

[绘图](#)

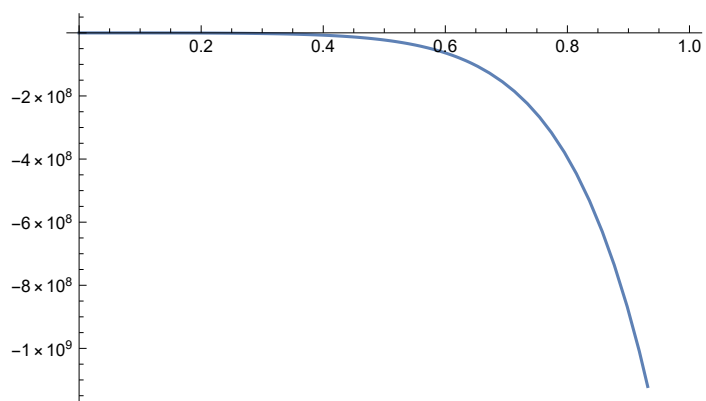

**Plot[Cf[6, 8, 9], {x, 0, 1}]**

[绘图](#)

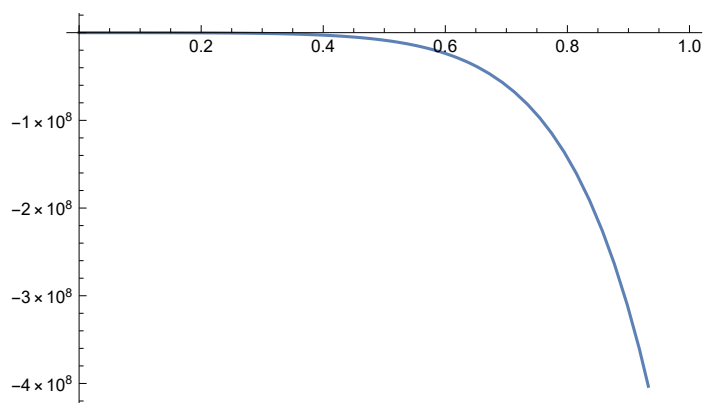

**Plot[Cf[6, 8, 8], {x, 0, 1}]**

[绘图](#)

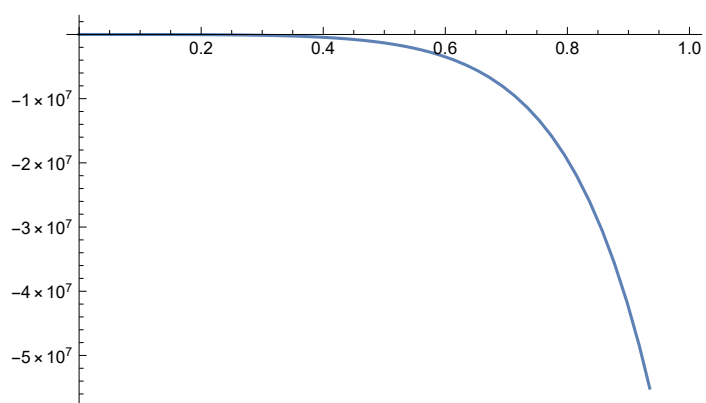

**Plot[Cf[6, 8, 7], {x, 0, 1}]**

[绘图](#)

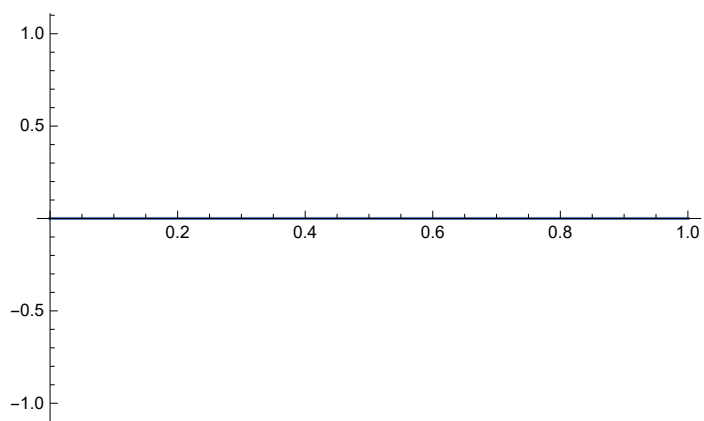

(\*128th group coefficients r2^6r3^7\*)

**Plot[Cf[6, 7, 14], {x, 0, 1}]**

[绘图](#)

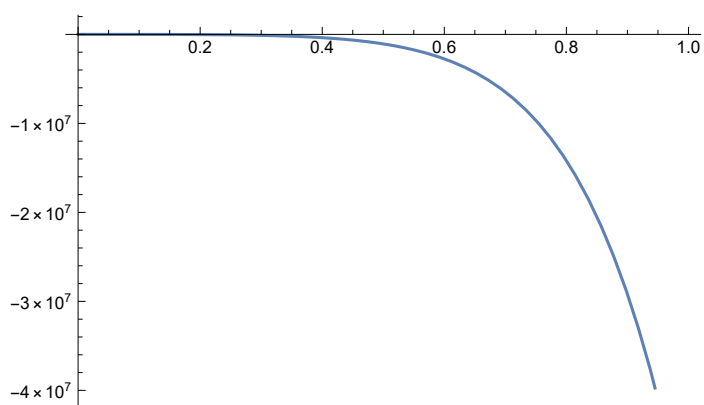

**Plot[Cf[6, 7, 13], {x, 0, 1}]**

[绘图](#)

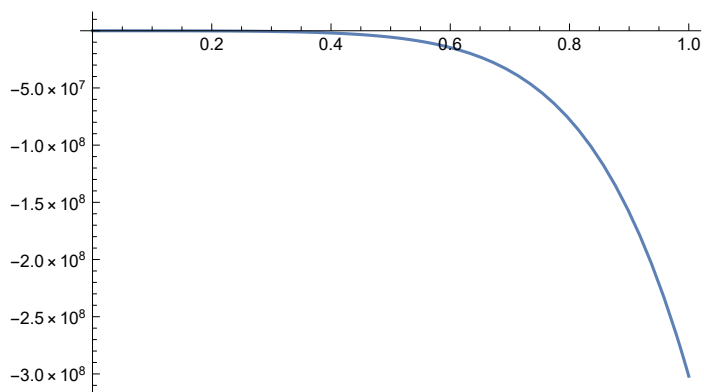

**Plot[Cf[6, 7, 12], {x, 0, 1}]**

[绘图](#)

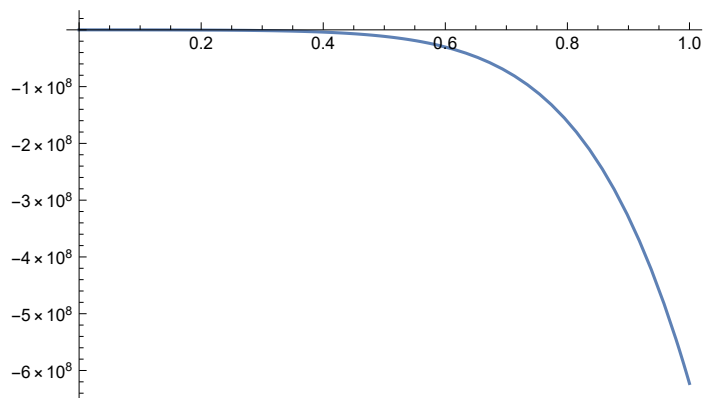

**Plot[Cf[6, 7, 11], {x, 0, 1}]**

[绘图](#)

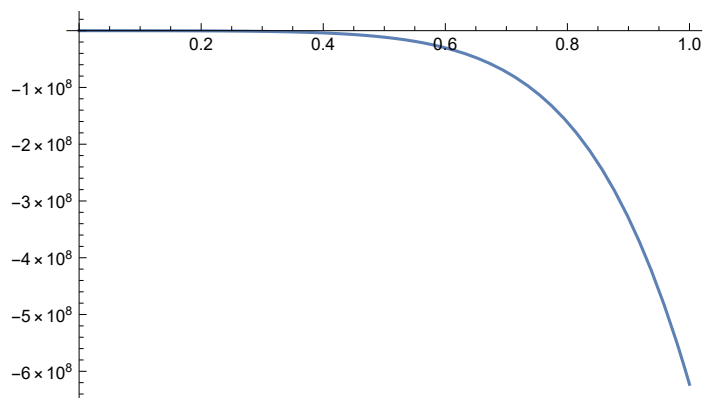

**Plot[Cf[6, 7, 10], {x, 0, 1}]**

[绘图](#)

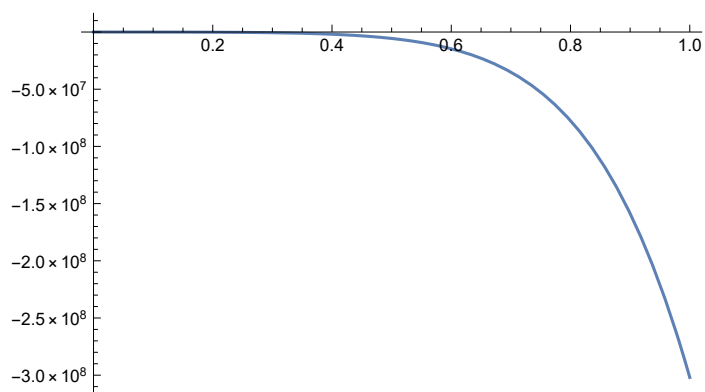



**Plot[Cf[6, 7, 9], {x, 0, 1}]**

[绘图](#)

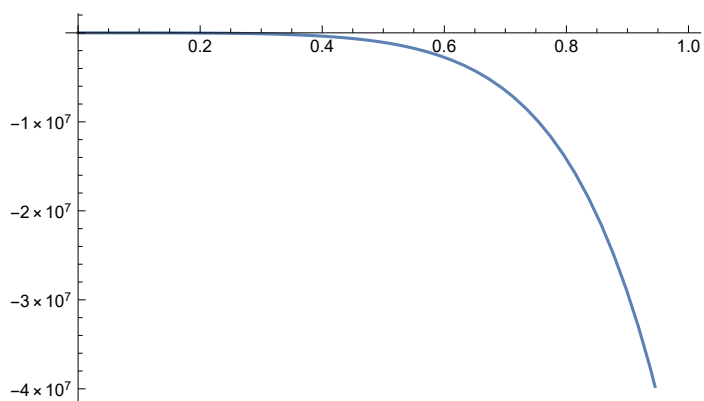

**Plot[Cf[6, 7, 8], {x, 0, 1}]**

[绘图](#)

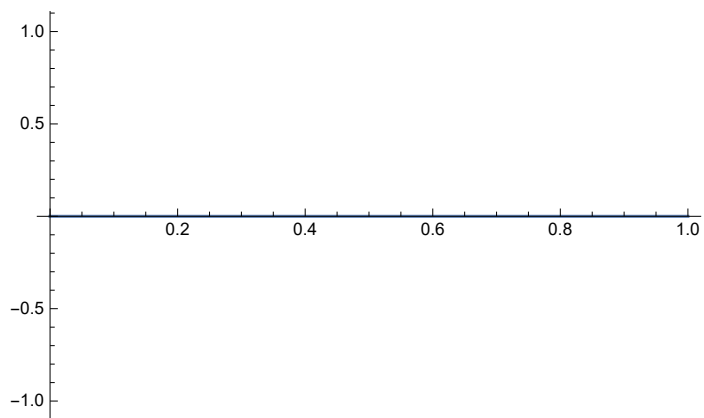

**(\*129th group coefficients r2^6r3^6\*)**

**Plot[Cf[6, 6, 14], {x, 0, 1}]**

[绘图](#)

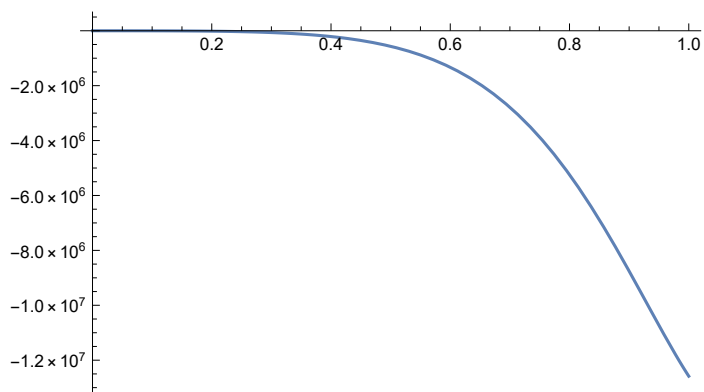

**Plot[Cf[6, 6, 13], {x, 0, 1}]**

[绘图](#)

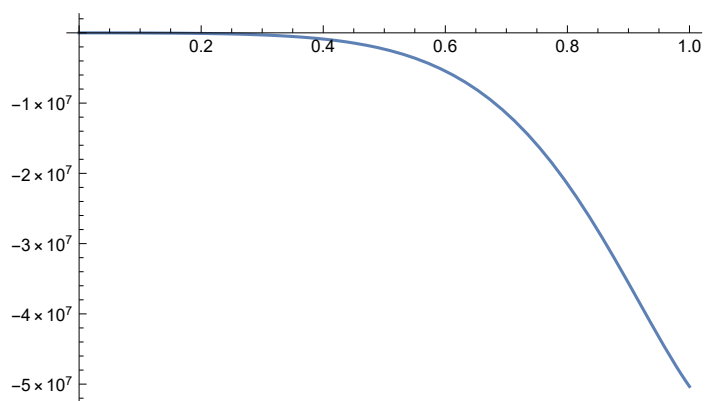

**Plot[Cf[6, 6, 12], {x, 0, 1}]**

[绘图](#)

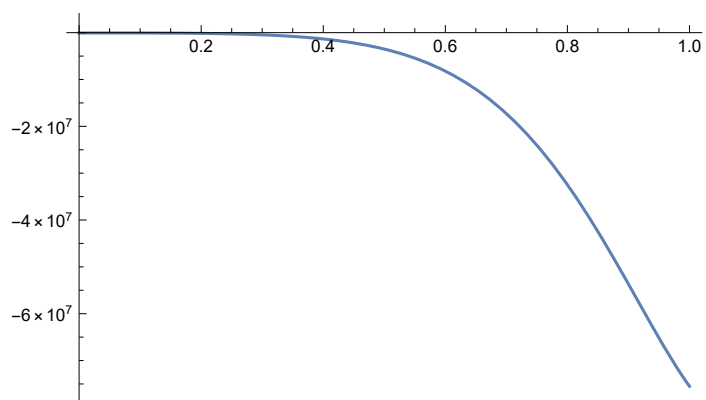

**Plot[Cf[6, 6, 11], {x, 0, 1}]**

[绘图](#)

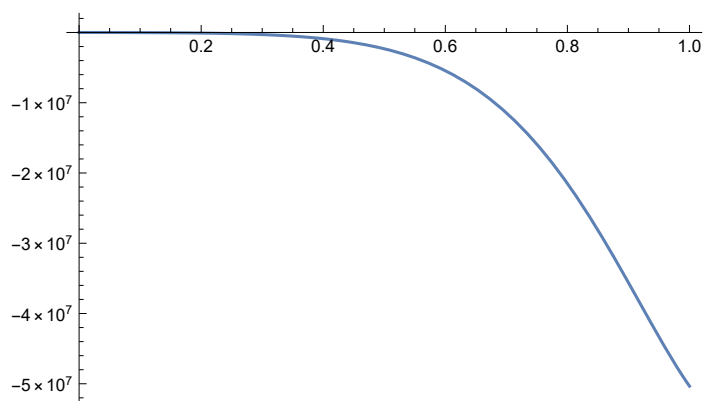

**Plot[Cf[6, 6, 10], {x, 0, 1}]**

[绘图](#)

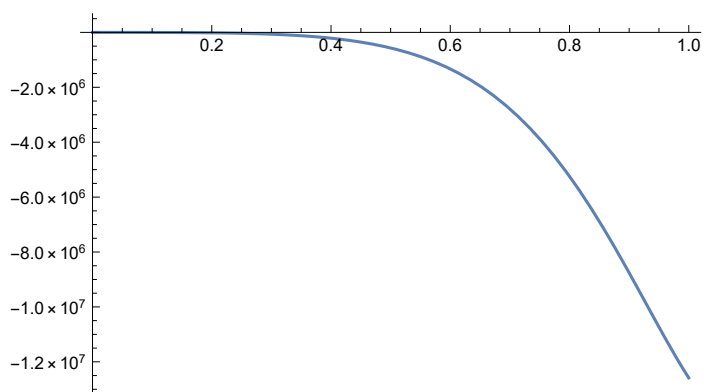

**Plot[Cf[6, 6, 9], {x, 0, 1}]**

[绘图](#)

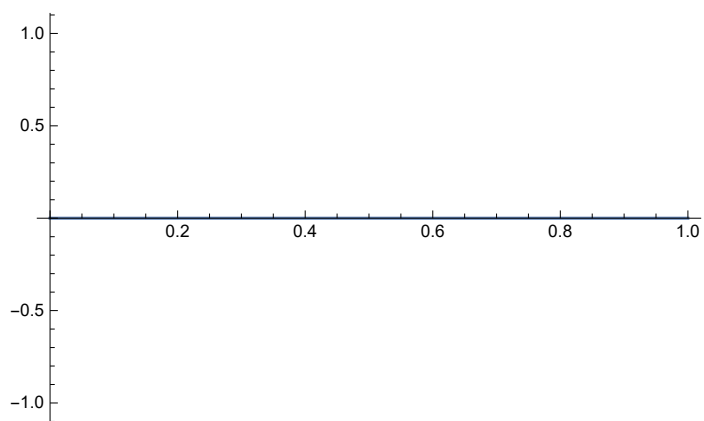

(\*130th group coefficients r2^6r3^5\*)

**Plot[Cf[6, 5, 14], {x, 0, 1}]**

[绘图](#)

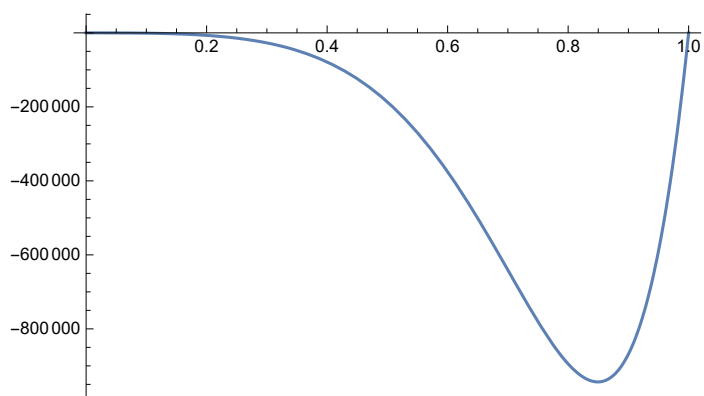

**Plot[Cf[6, 5, 13], {x, 0, 1}]**

[绘图](#)

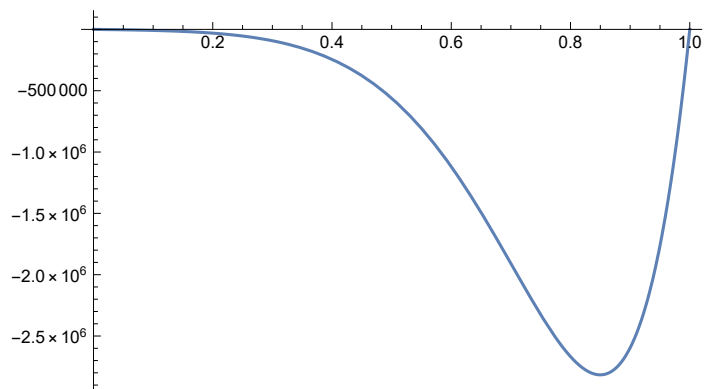

**Plot[Cf[6, 5, 12], {x, 0, 1}]**

[绘图](#)

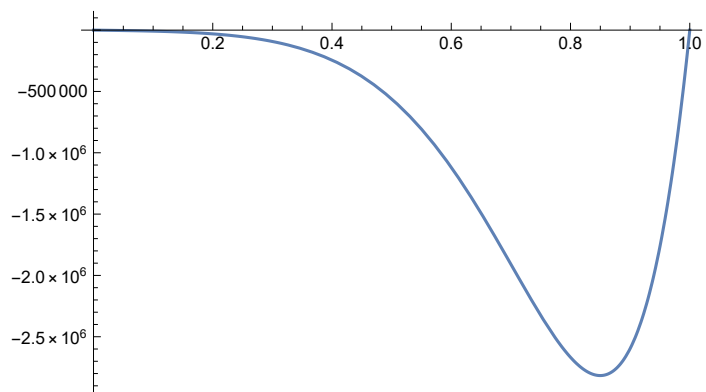

**Plot[Cf[6, 5, 11], {x, 0, 1}]**

[绘图](#)

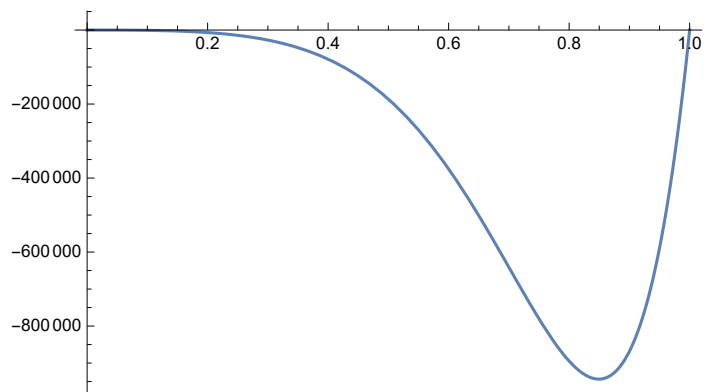

**Plot[Cf[6, 5, 10], {x, 0, 1}]**

[绘图](#)

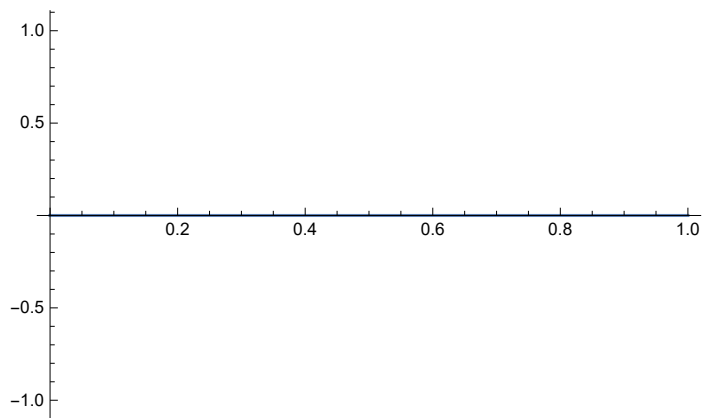

(\*131th group coefficients r2^6r3^4\*)

**Plot[Cf[6, 4, 14], {x, 0, 1}]**

[绘图](#)

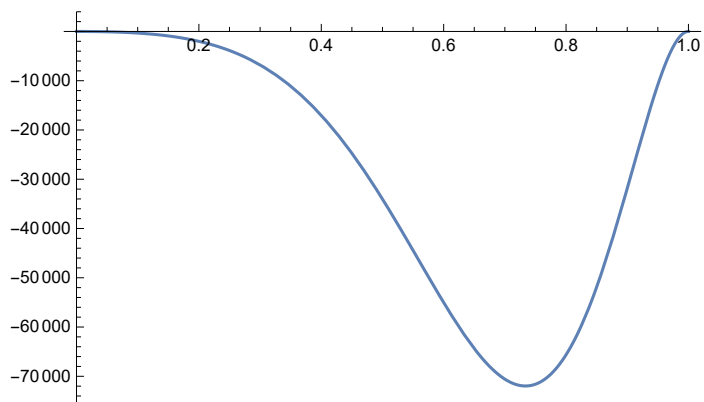

**Plot[Cf[6, 4, 13], {x, 0, 1}]**

[绘图](#)

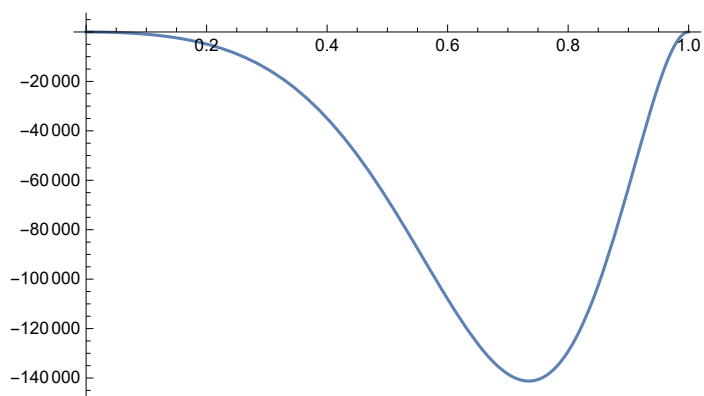

**Plot[Cf[6, 4, 12], {x, 0, 1}]**

[绘图](#)

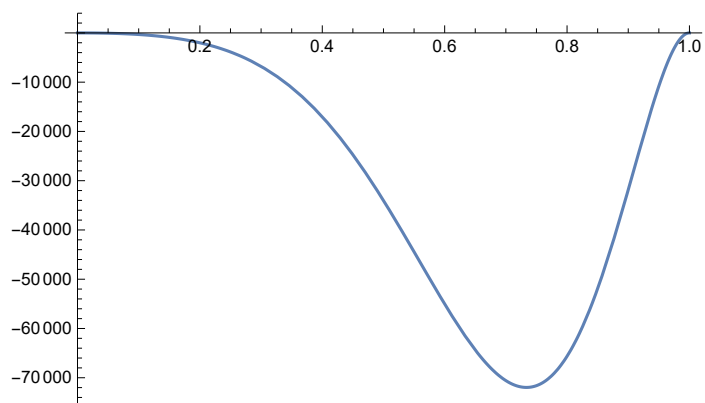

**Plot[Cf[6, 4, 11], {x, 0, 1}]**

[绘图](#)

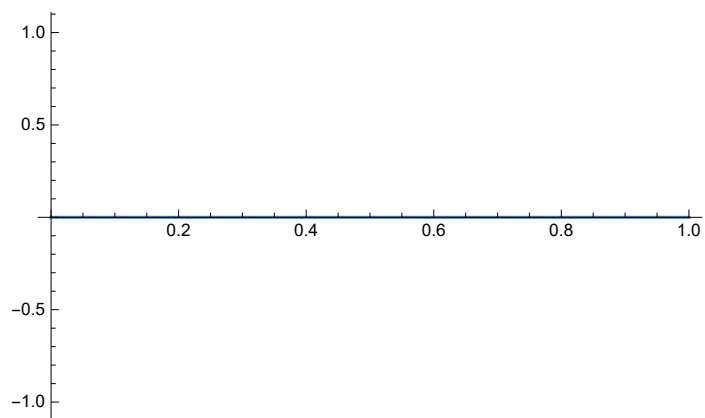

**(\*132th group coefficients r2^6r3^3\*)**

**Plot[Cf[6, 3, 14], {x, 0, 1}]**

[绘图](#)

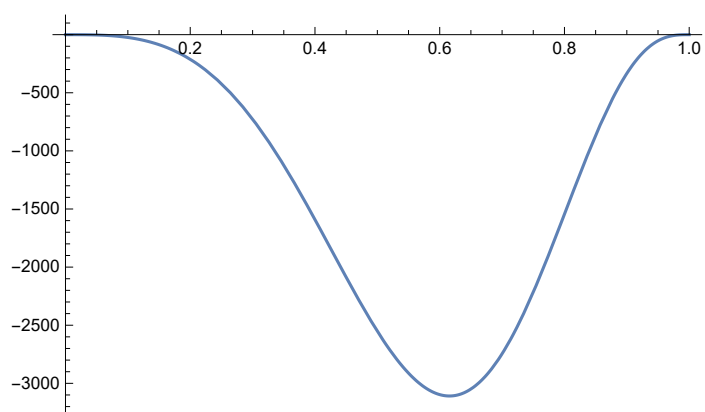

**Plot[Cf[6, 3, 13], {x, 0, 1}]**

[绘图](#)

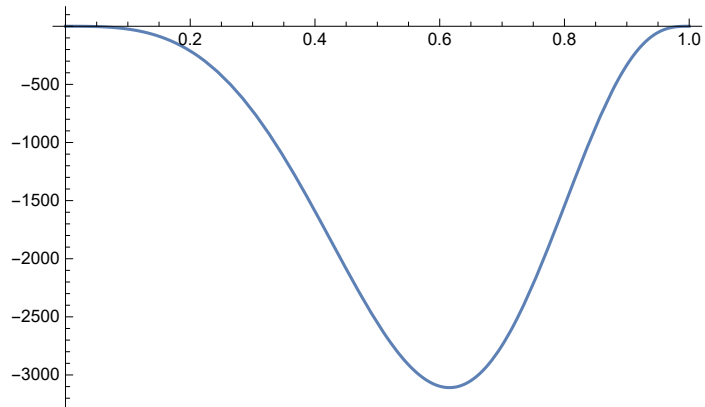

**Plot[Cf[6, 3, 12], {x, 0, 1}]**

[绘图](#)

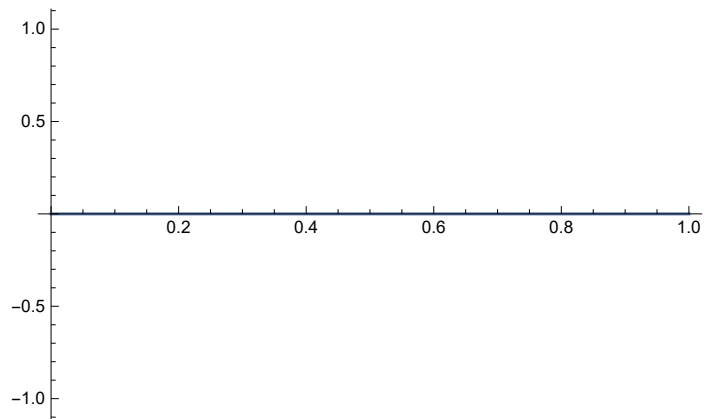

**(\*133th group coefficients r2^6r3^2\*)**

**Plot[Cf[6, 2, 14], {x, 0, 1}]**

[绘图](#)

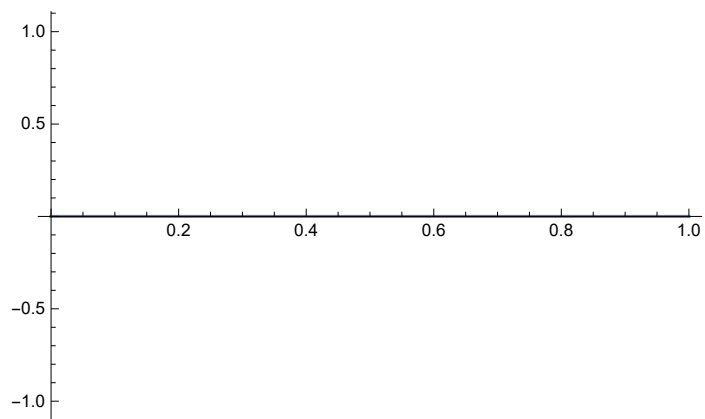

**Plot[Cf[6, 2, 13], {x, 0, 1}]**

[绘图](#)

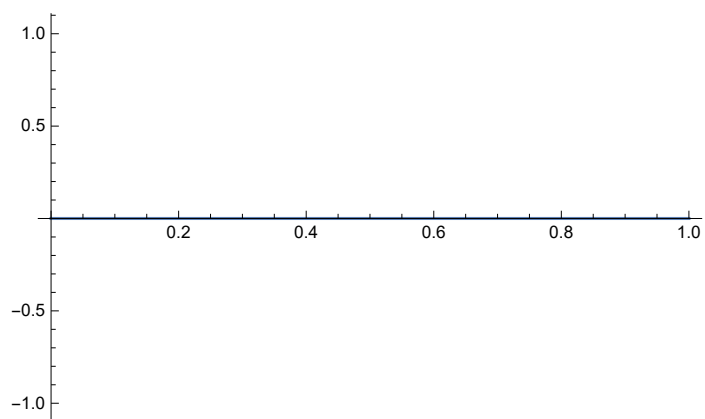

(\*134th group coefficients r2^6r3^1\*)

**Plot[Cf[6, 1, 14], {x, 0, 1}]**

[绘图](#)

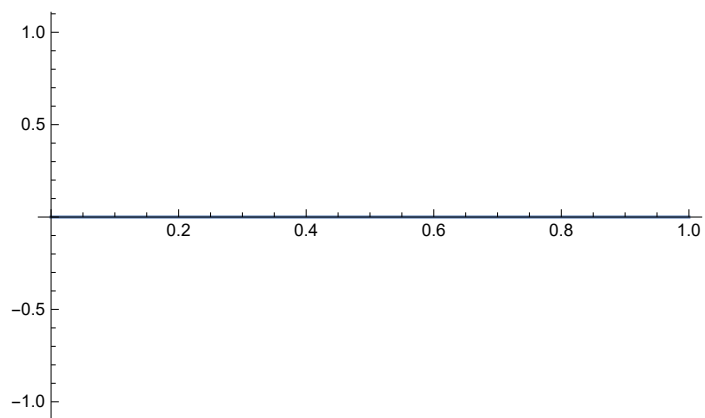

(\*135th group coefficients r2^6r3^0\*)

**Plot[Cf[6, 0, 14], {x, 0, 1}]**

[绘图](#)

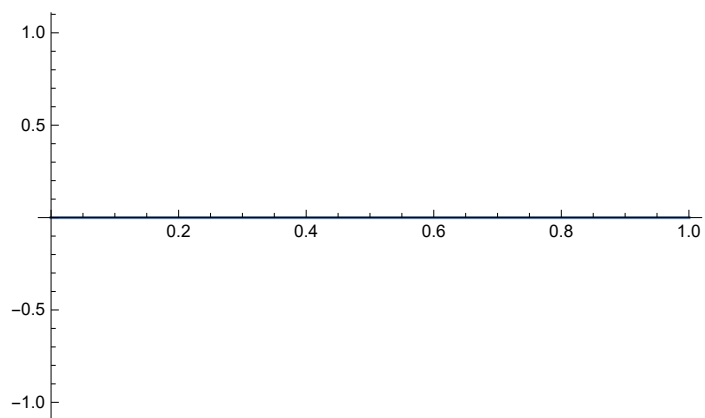

(\*136th group coefficients r2^5r3^14\*)



**Plot[Cf[5, 14, 14], {x, 0, 1}]**

[绘图](#)

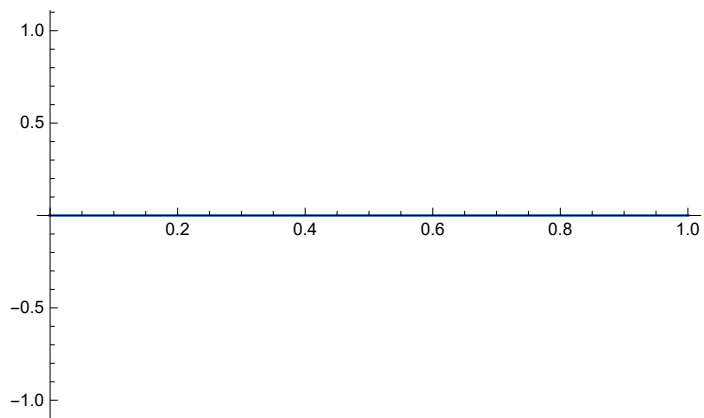

**Plot[Cf[5, 14, 13], {x, 0, 1}]**

[绘图](#)

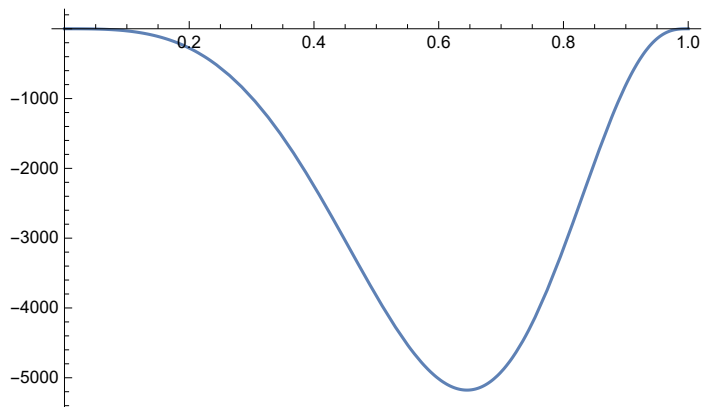

**Plot[Cf[5, 14, 12], {x, 0, 1}]**

[绘图](#)

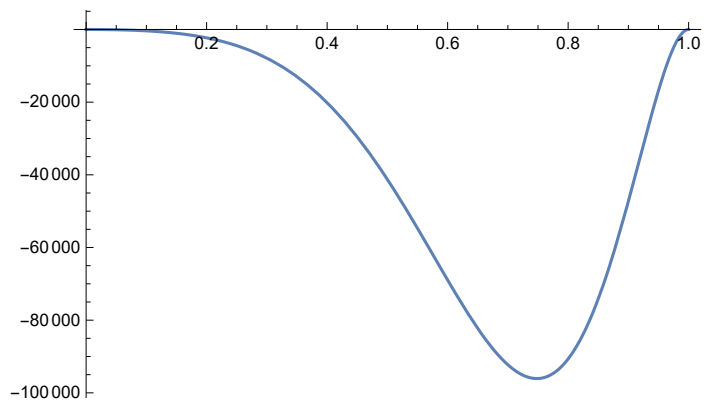

```
Plot[Cf[5, 14, 11], {x, 0, 1}]
```

[绘图](#)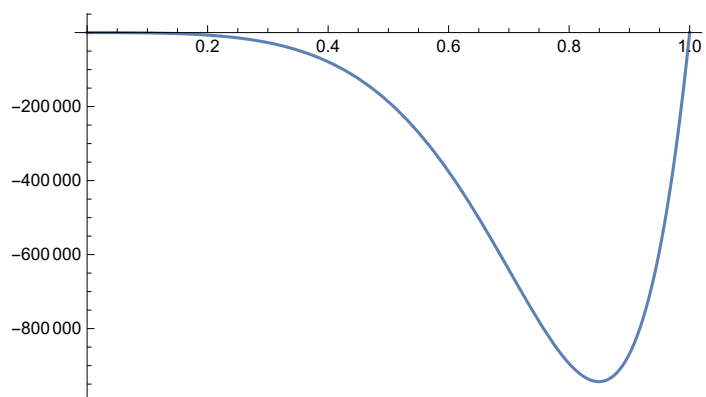

```
Plot[Cf[5, 14, 10], {x, 0, 1}]
```

[绘图](#)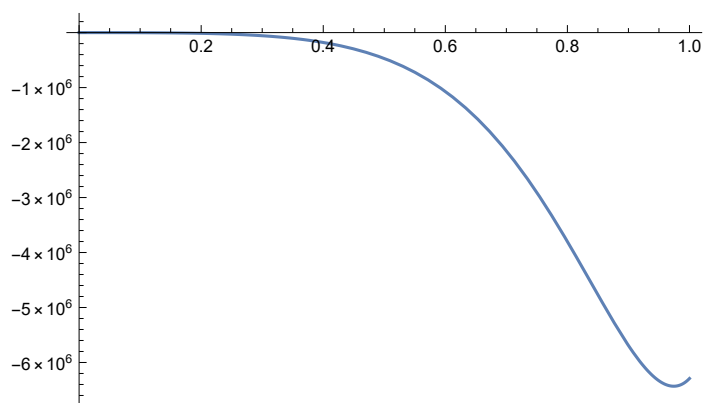

```
Plot[Cf[5, 14, 9], {x, 0, 1}]
```

[绘图](#)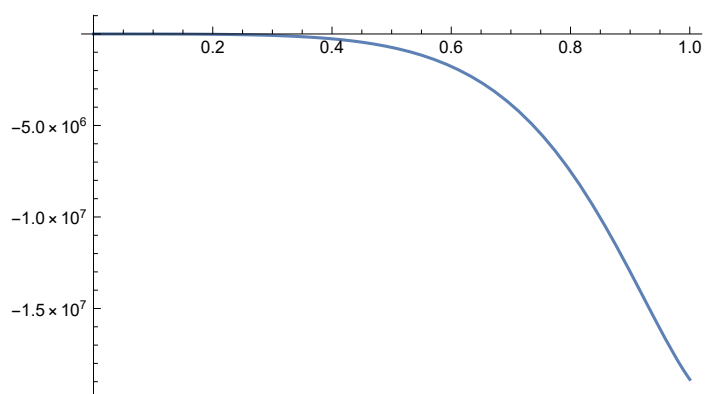

**Plot[Cf[5, 14, 8], {x, 0, 1}]**

[绘图](#)

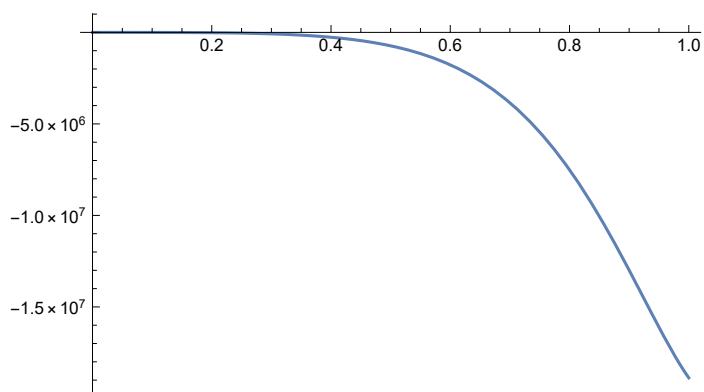

**Plot[Cf[5, 14, 7], {x, 0, 1}]**

[绘图](#)

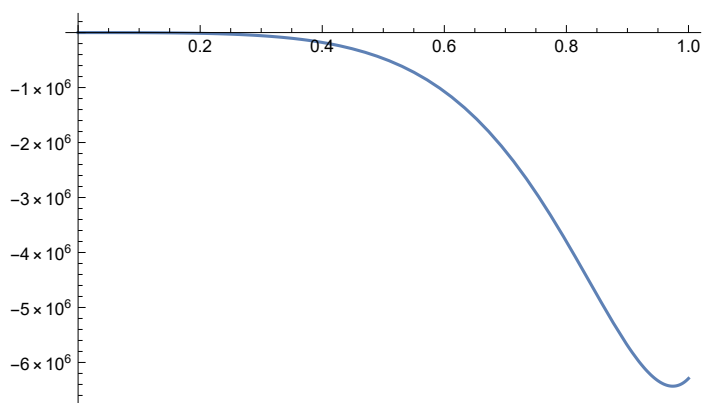

**Plot[Cf[5, 14, 6], {x, 0, 1}]**

[绘图](#)

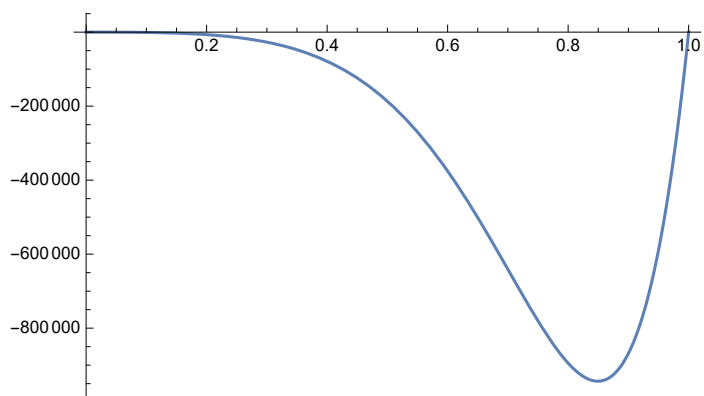

**Plot[Cf[5, 14, 5], {x, 0, 1}]**

[绘图](#)

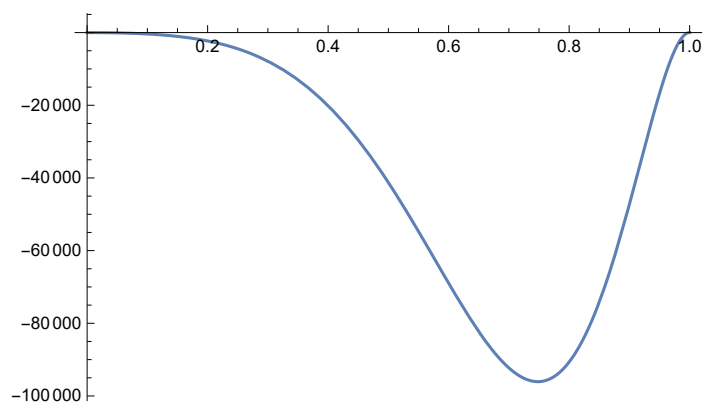

**Plot[Cf[5, 14, 4], {x, 0, 1}]**

[绘图](#)

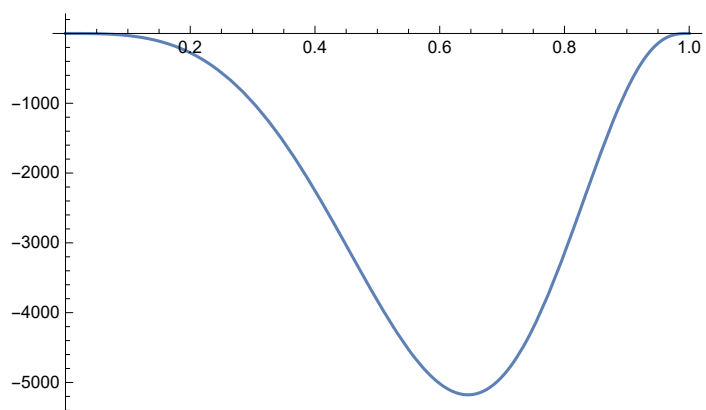

**Plot[Cf[5, 14, 3], {x, 0, 1}]**

[绘图](#)

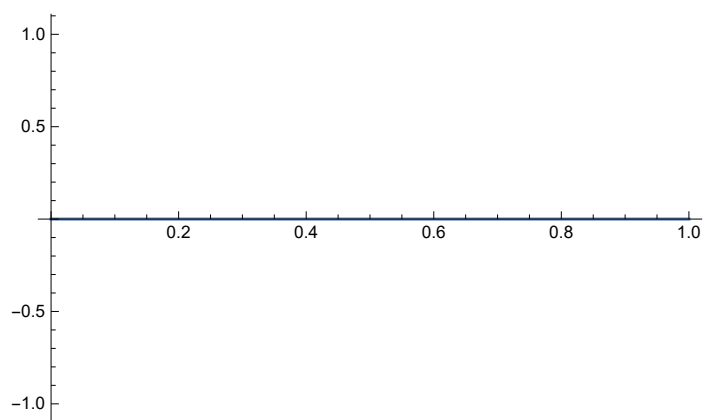

**(\*137th group coefficients r2^5r3^13\*)**

```
Plot[Cf[5, 13, 14], {x, 0, 1}]
```

[绘图](#)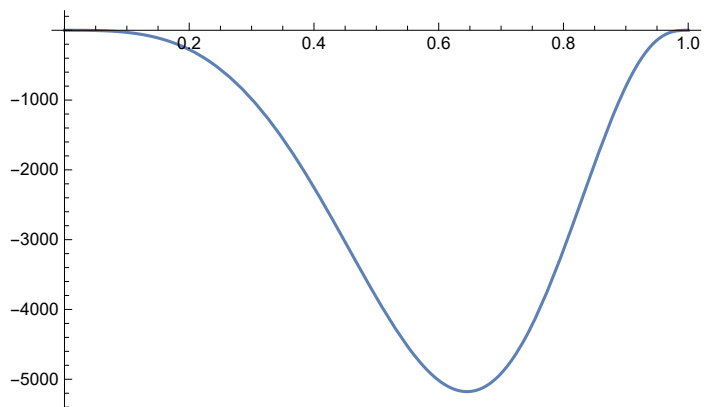

```
Plot[Cf[5, 13, 13], {x, 0, 1}]
```

[绘图](#)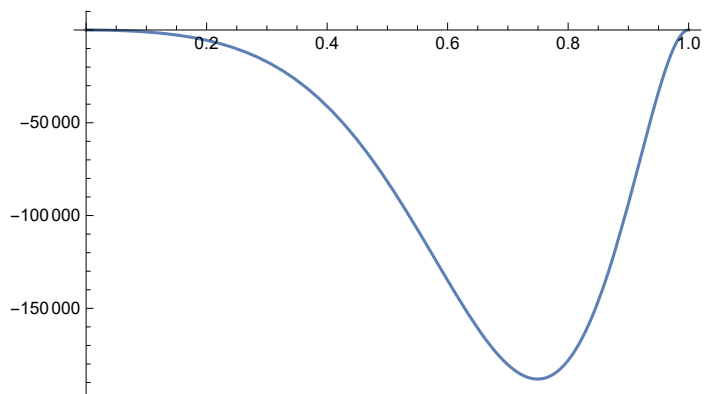

```
Plot[Cf[5, 13, 12], {x, 0, 1}]
```

[绘图](#)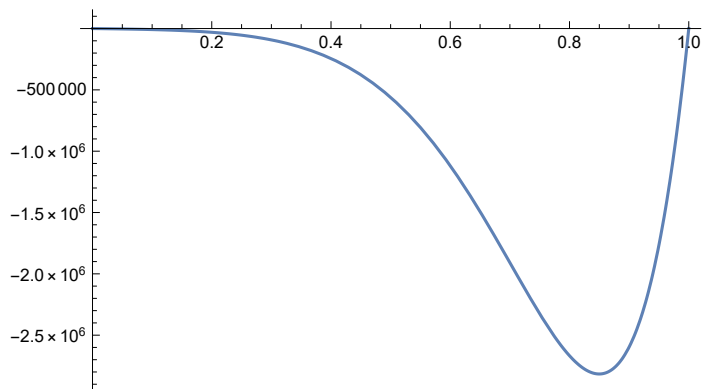

**Plot[Cf[5, 13, 11], {x, 0, 1}]**

[绘图](#)

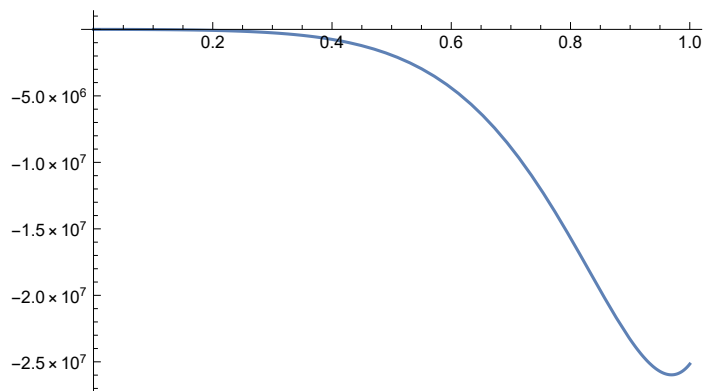

**Plot[Cf[5, 13, 10], {x, 0, 1}]**

[绘图](#)

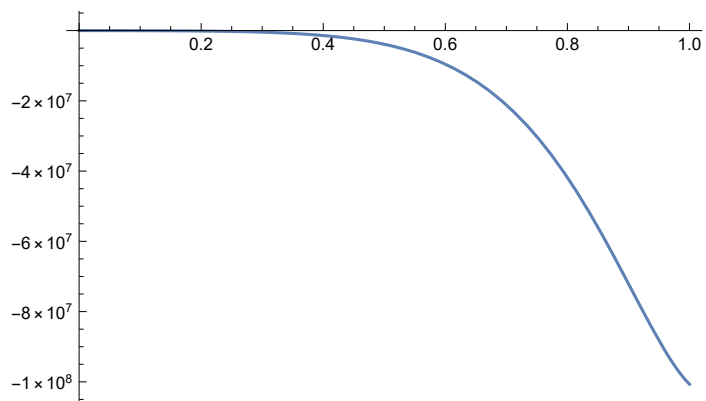

**Plot[Cf[5, 13, 9], {x, 0, 1}]**

[绘图](#)

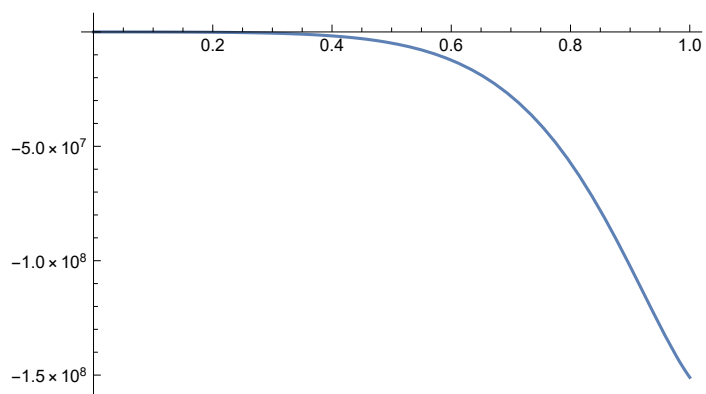

**Plot[Cf[5, 13, 8], {x, 0, 1}]**

[绘图](#)

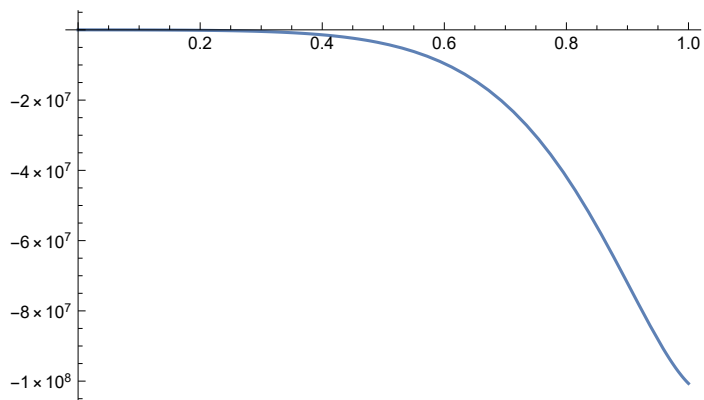

**Plot[Cf[5, 13, 7], {x, 0, 1}]**

[绘图](#)

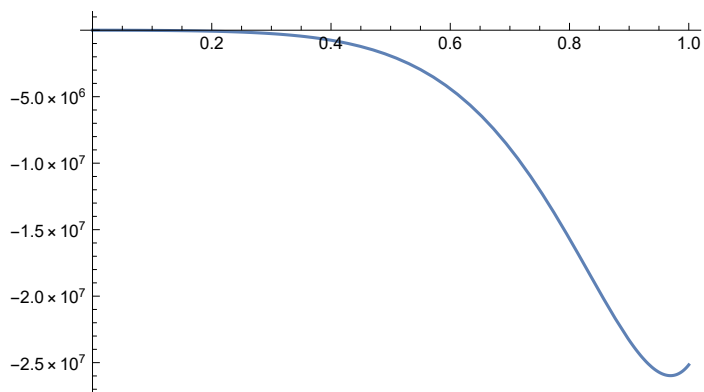

**Plot[Cf[5, 13, 6], {x, 0, 1}]**

[绘图](#)

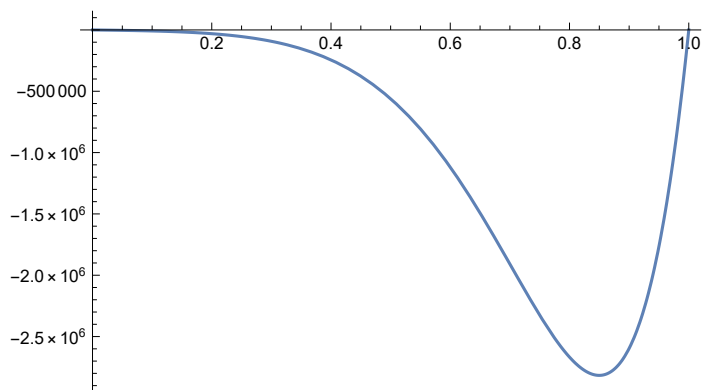

`Plot[Cf[5, 13, 5], {x, 0, 1}]`

[绘图](#)

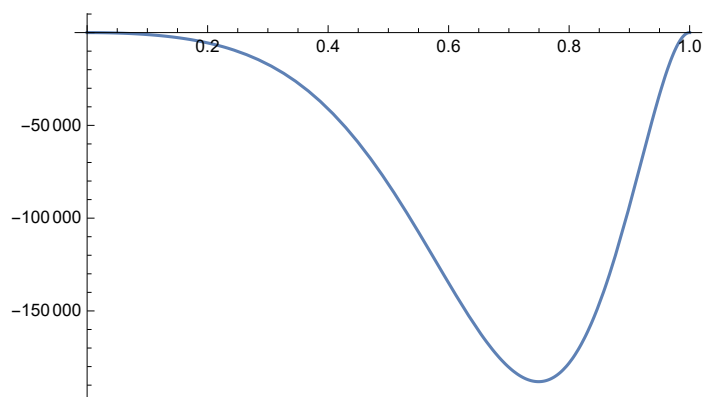

`Plot[Cf[5, 13, 4], {x, 0, 1}]`

[绘图](#)

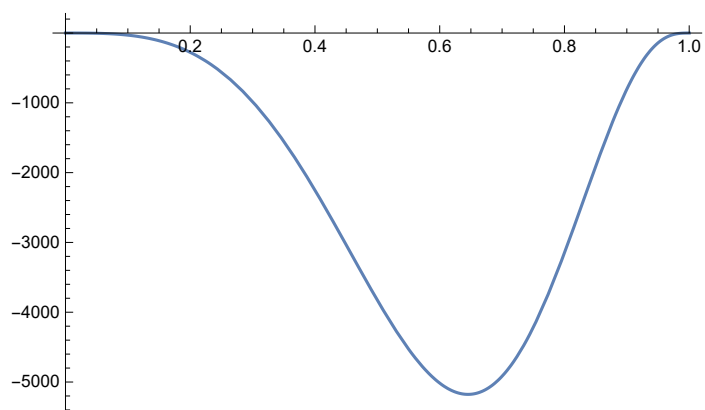

`Plot[Cf[5, 13, 3], {x, 0, 1}]`

[绘图](#)

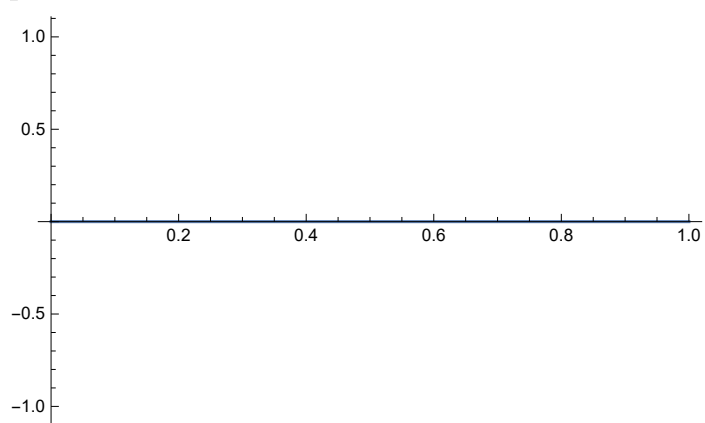

`(*138th group coefficients r2^5r3^12*)`



```
Plot[Cf[5, 12, 14], {x, 0, 1}]
```

[绘图](#)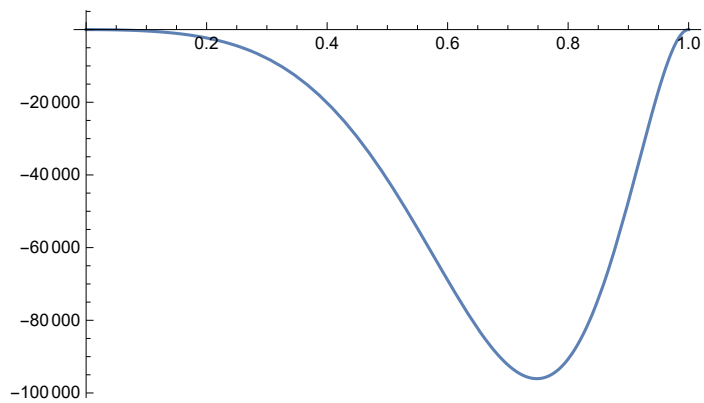

```
Plot[Cf[5, 12, 13], {x, 0, 1}]
```

[绘图](#)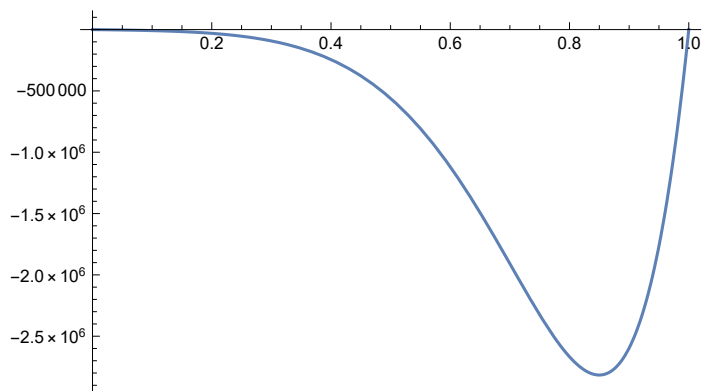

```
Plot[Cf[5, 12, 12], {x, 0, 1}]
```

[绘图](#)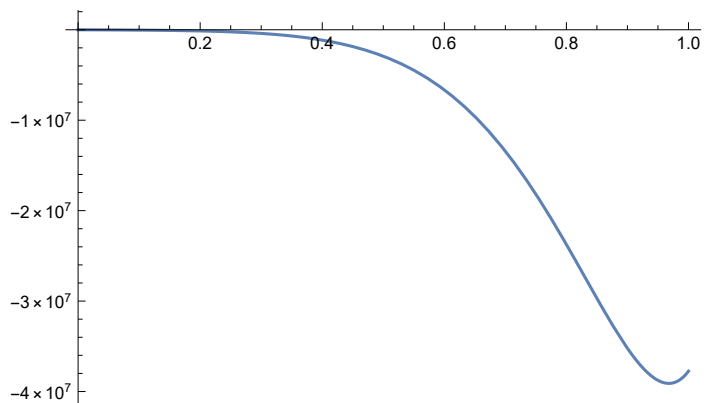

**Plot[Cf[5, 12, 11], {x, 0, 1}]**

[绘图](#)

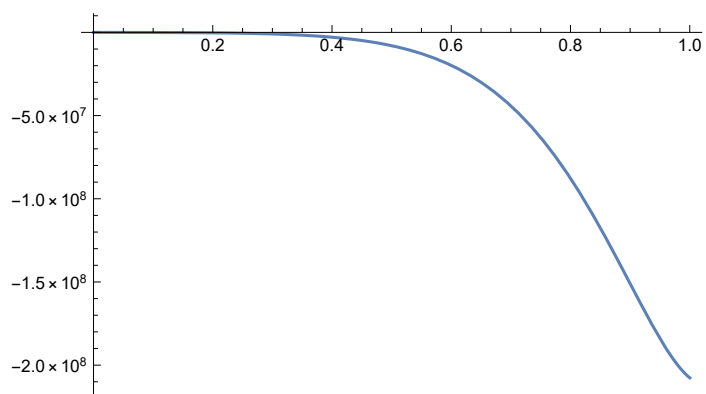

**Plot[Cf[5, 12, 10], {x, 0, 1}]**

[绘图](#)

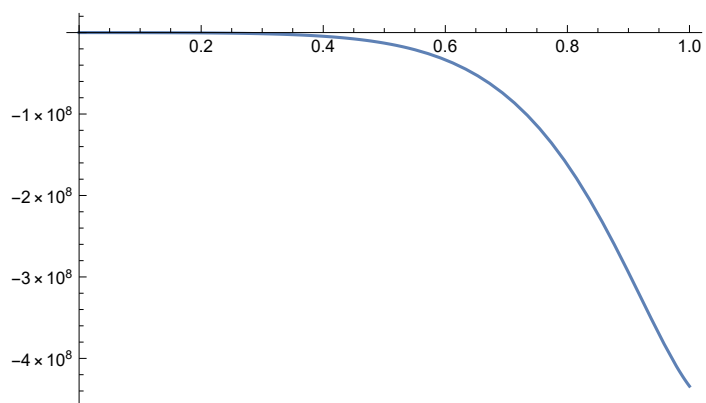

**Plot[Cf[5, 12, 9], {x, 0, 1}]**

[绘图](#)

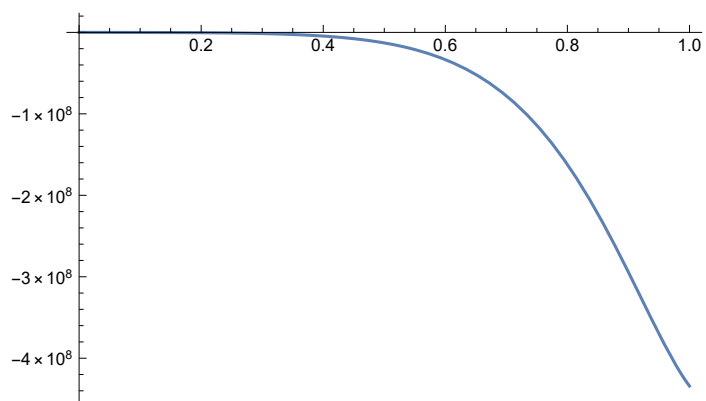

**Plot[Cf[5, 12, 8], {x, 0, 1}]**

[绘图](#)

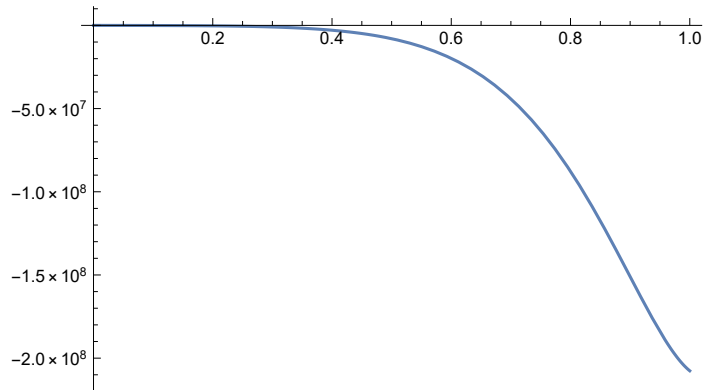

**Plot[Cf[5, 12, 7], {x, 0, 1}]**

[绘图](#)

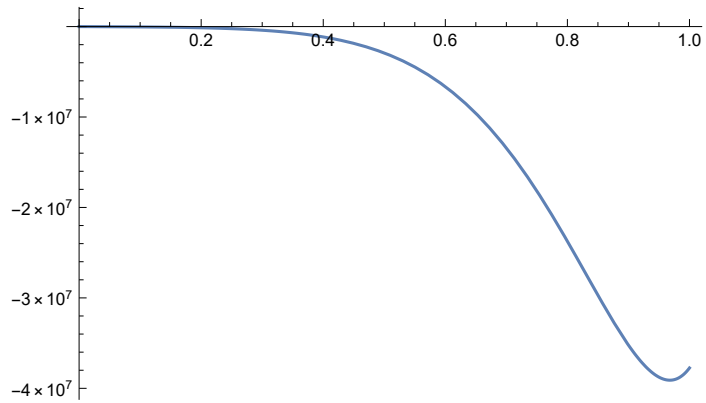

**Plot[Cf[5, 12, 6], {x, 0, 1}]**

[绘图](#)

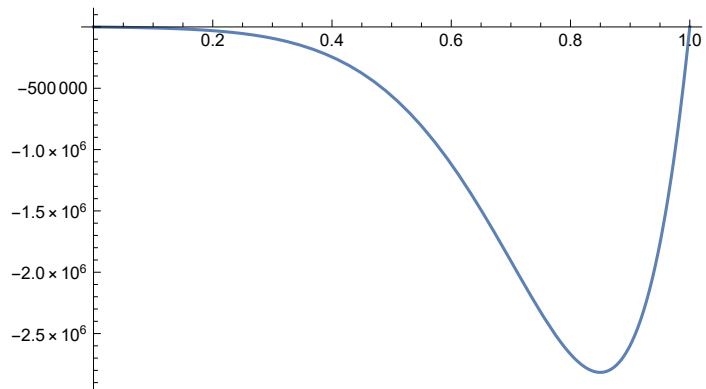

**Plot[Cf[5, 12, 5], {x, 0, 1}]**

[绘图](#)

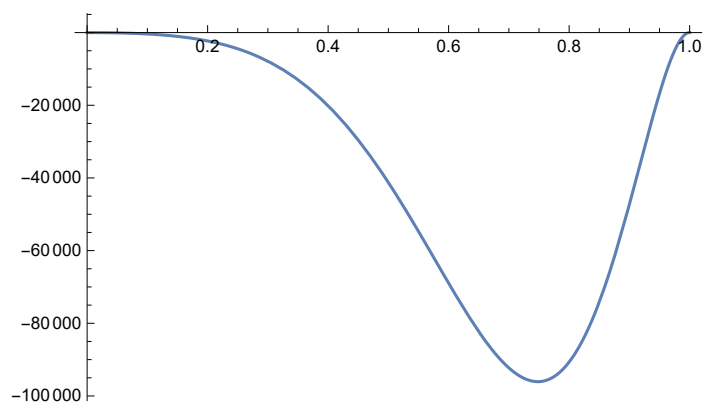

**Plot[Cf[5, 12, 4], {x, 0, 1}]**

[绘图](#)

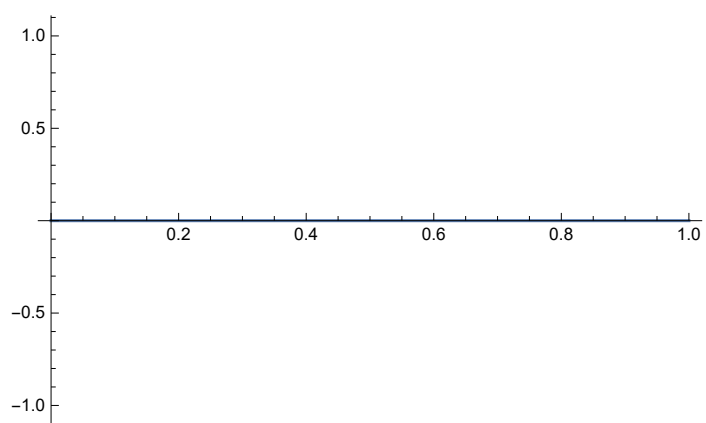

**(\*139th group coefficients r2^5r3^11\*)**

**Plot[Cf[5, 11, 14], {x, 0, 1}]**

[绘图](#)

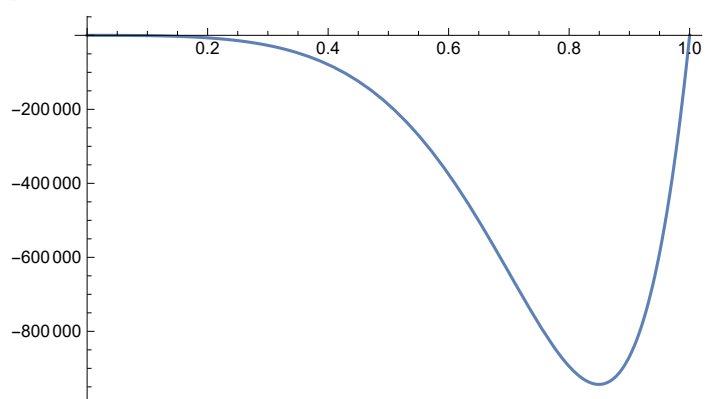

**Plot[Cf[5, 11, 13], {x, 0, 1}]**

[绘图](#)

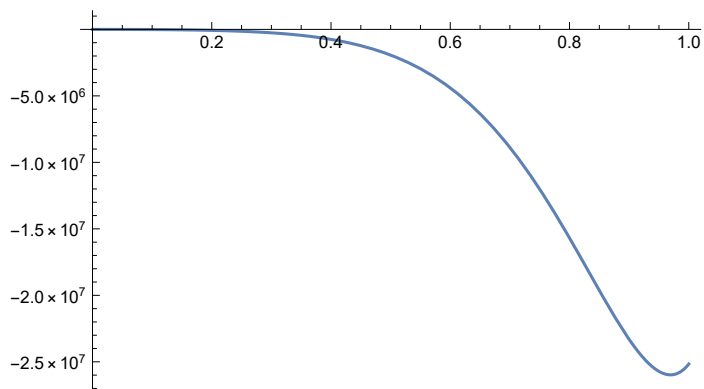

**Plot[Cf[5, 11, 12], {x, 0, 1}]**

[绘图](#)

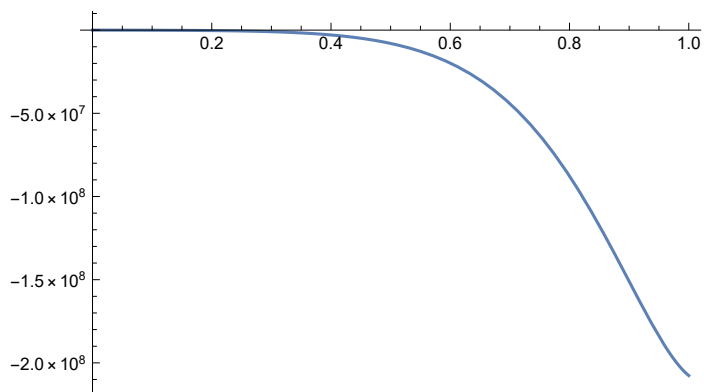

**Plot[Cf[5, 11, 11], {x, 0, 1}]**

[绘图](#)

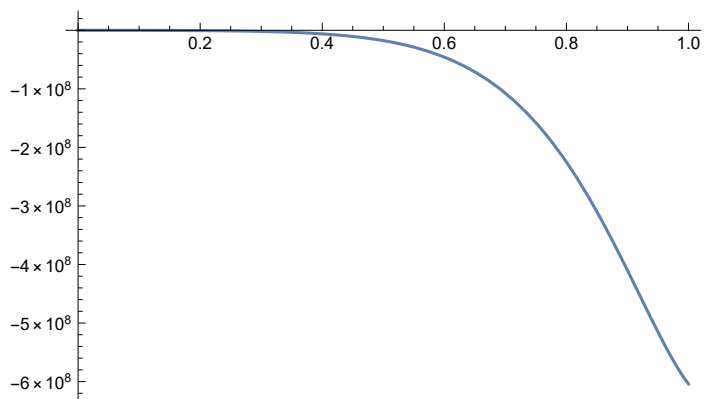

```
Plot[Cf[5, 11, 10], {x, 0, 1}]
```

[绘图](#)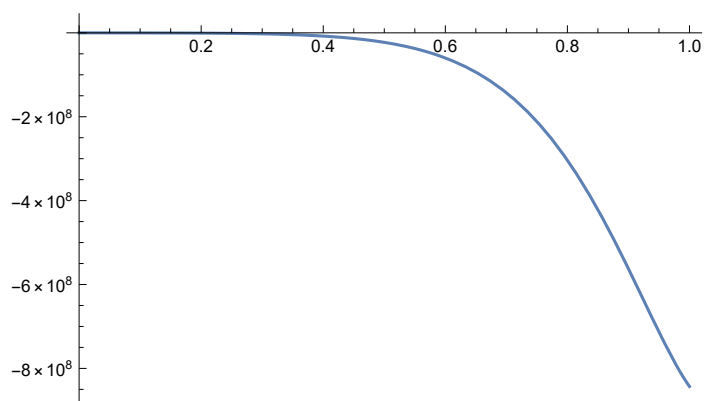

```
Plot[Cf[5, 11, 9], {x, 0, 1}]
```

[绘图](#)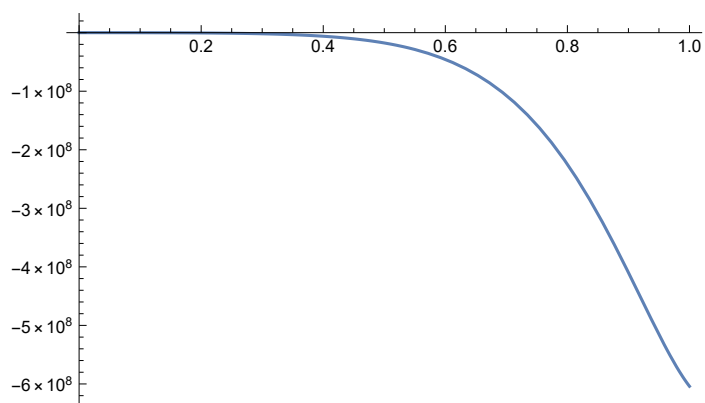

```
Plot[Cf[5, 11, 8], {x, 0, 1}]
```

[绘图](#)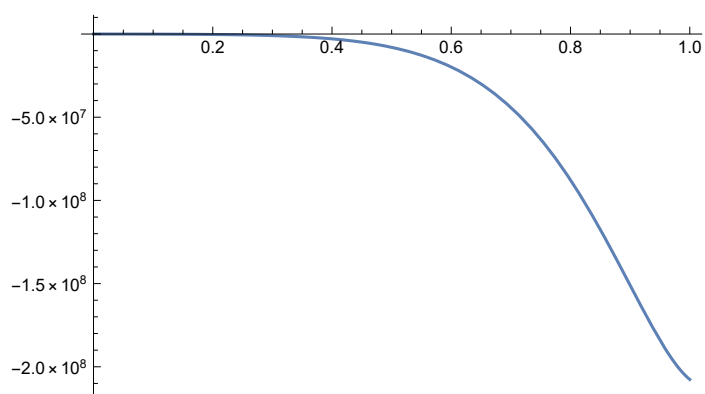

**Plot[Cf[5, 11, 7], {x, 0, 1}]**

[绘图](#)

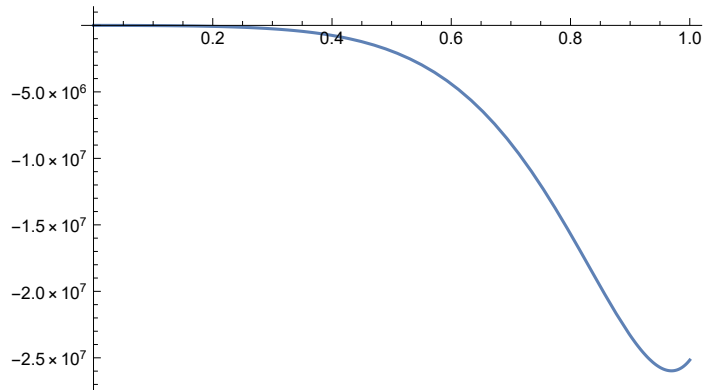

**Plot[Cf[5, 11, 6], {x, 0, 1}]**

[绘图](#)

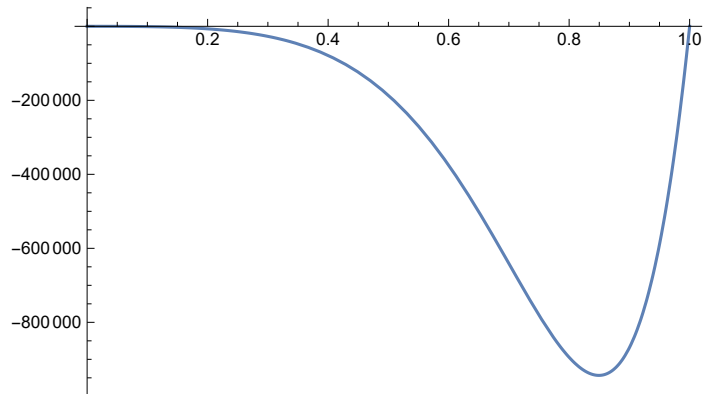

**Plot[Cf[5, 11, 5], {x, 0, 1}]**

[绘图](#)

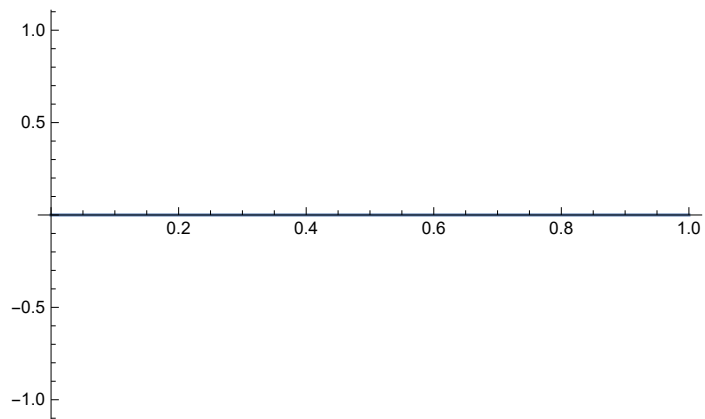

(\*140th group coefficients r2^5r3^10\*)

**Plot[Cf[5, 10, 14], {x, 0, 1}]**

[绘图](#)

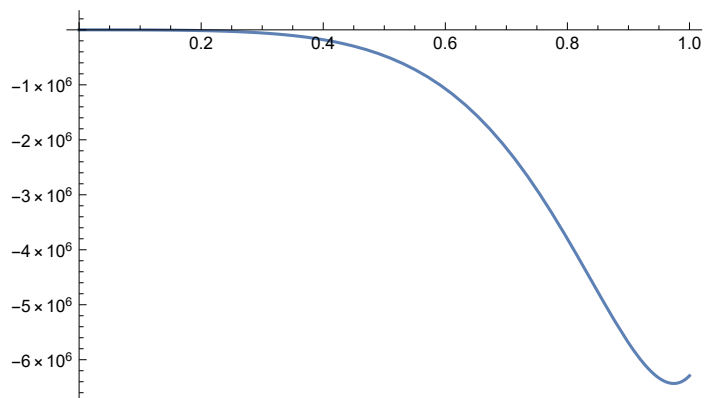

**Plot[Cf[5, 10, 13], {x, 0, 1}]**

[绘图](#)

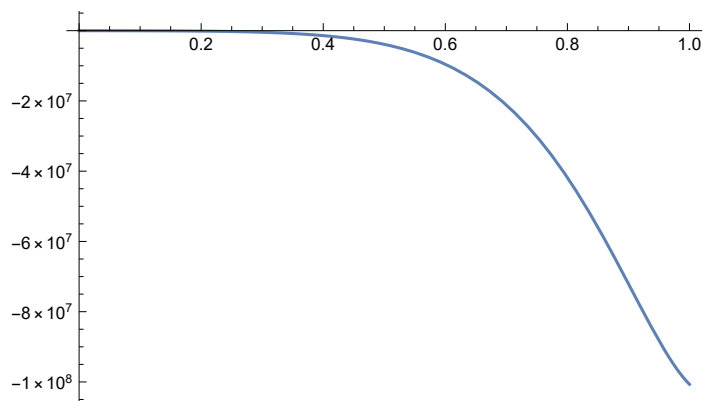

**Plot[Cf[5, 10, 12], {x, 0, 1}]**

[绘图](#)

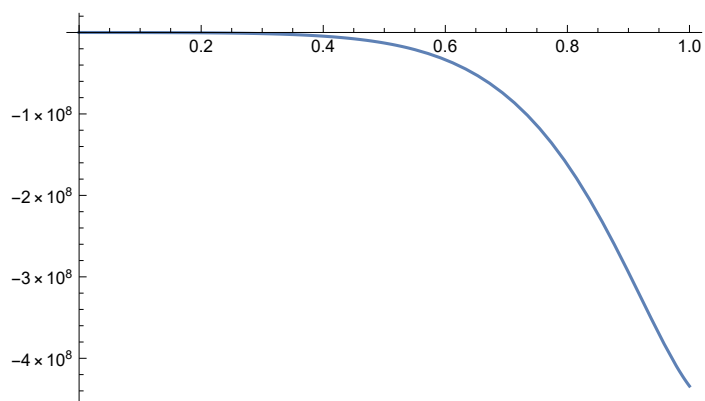



**Plot[Cf[5, 10, 11], {x, 0, 1}]**

[绘图](#)

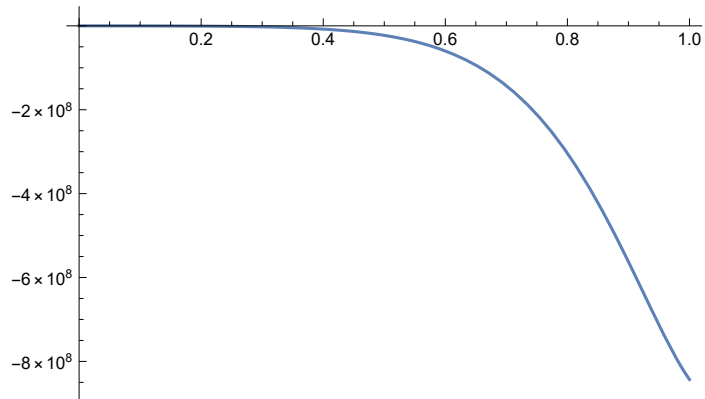

**Plot[Cf[5, 10, 10], {x, 0, 1}]**

[绘图](#)

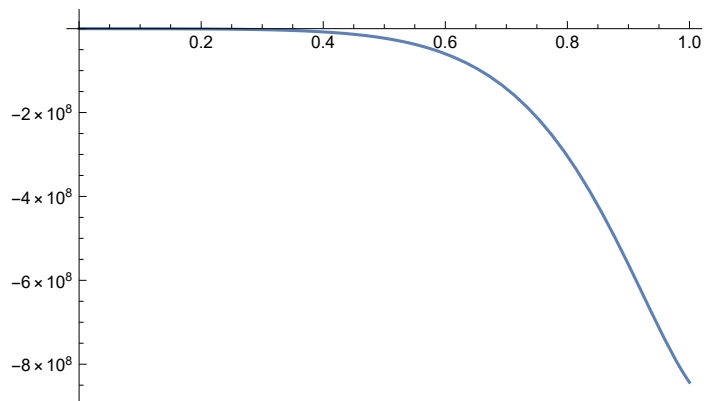

**Plot[Cf[5, 10, 9], {x, 0, 1}]**

[绘图](#)

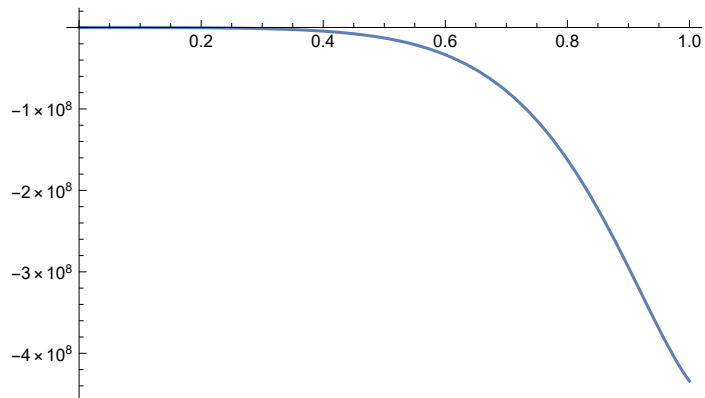

**Plot[Cf[5, 10, 8], {x, 0, 1}]**

[绘图](#)

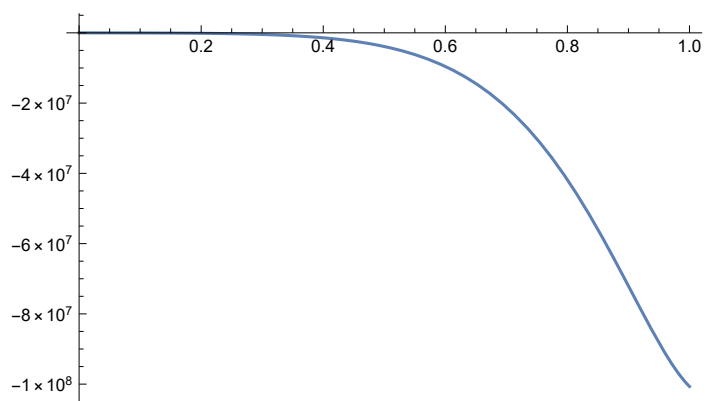

**Plot[Cf[5, 10, 7], {x, 0, 1}]**

[绘图](#)

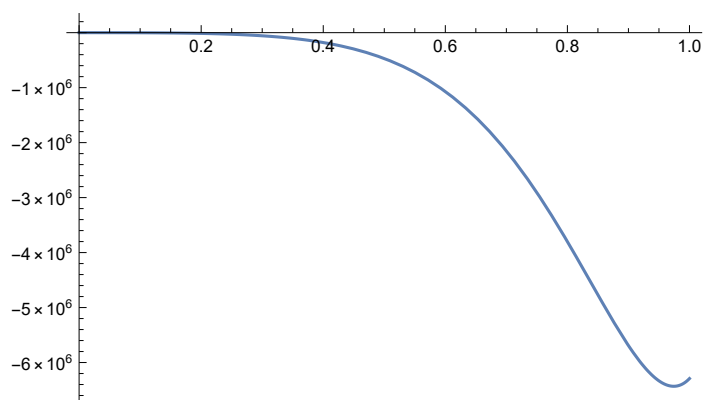

**Plot[Cf[5, 10, 6], {x, 0, 1}]**

[绘图](#)

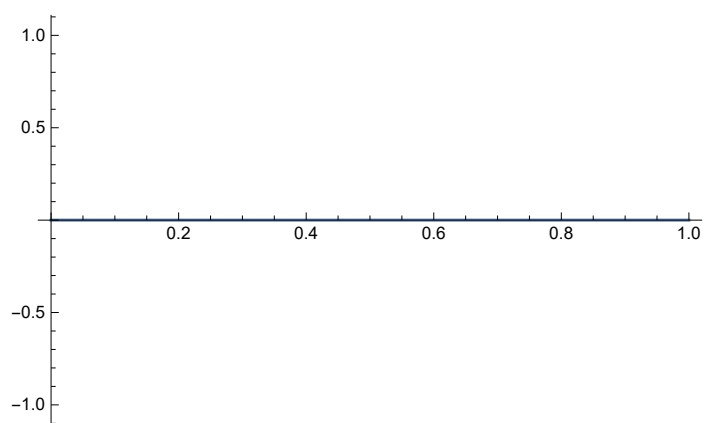

(\*141th group coefficients r2^5r3^9\*)

**Plot[Cf[5, 9, 14], {x, 0, 1}]**

[绘图](#)

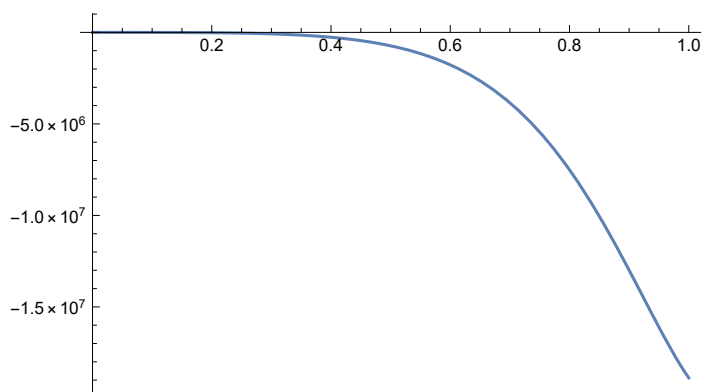

**Plot[Cf[5, 9, 13], {x, 0, 1}]**

[绘图](#)

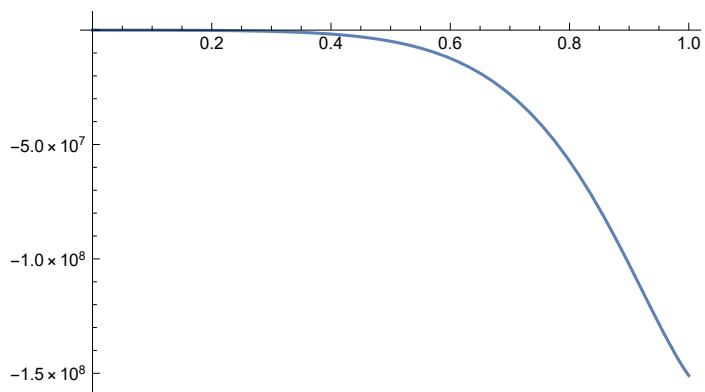

**Plot[Cf[5, 9, 12], {x, 0, 1}]**

[绘图](#)

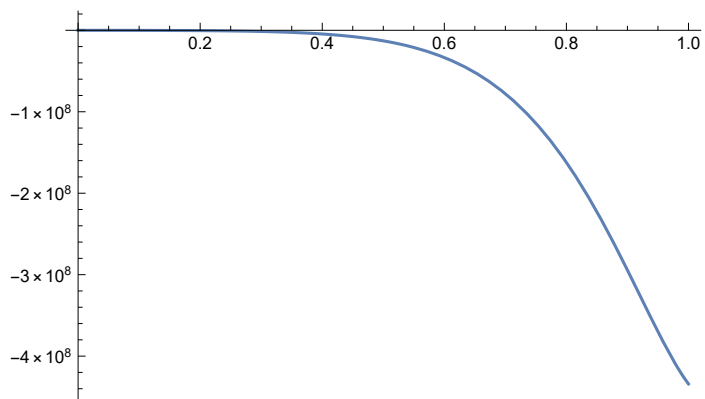

**Plot[Cf[5, 9, 11], {x, 0, 1}]**

[绘图](#)

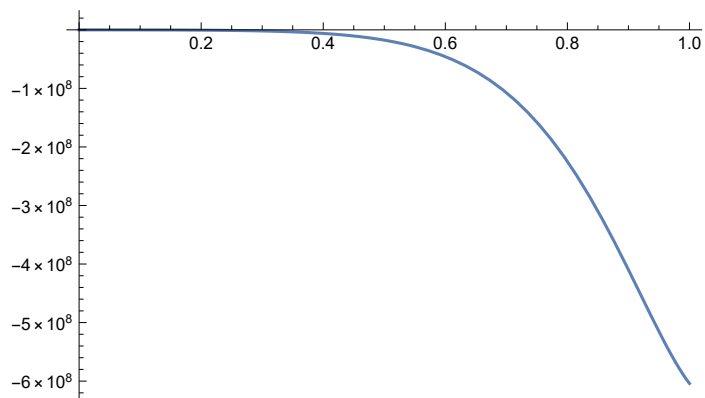

**Plot[Cf[5, 9, 10], {x, 0, 1}]**

[绘图](#)

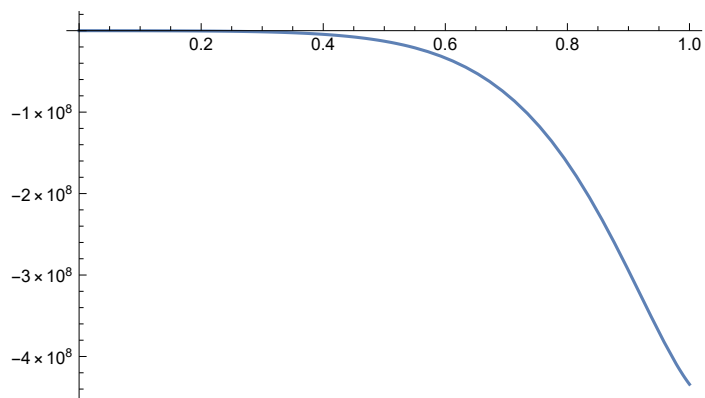

**Plot[Cf[5, 9, 9], {x, 0, 1}]**

[绘图](#)

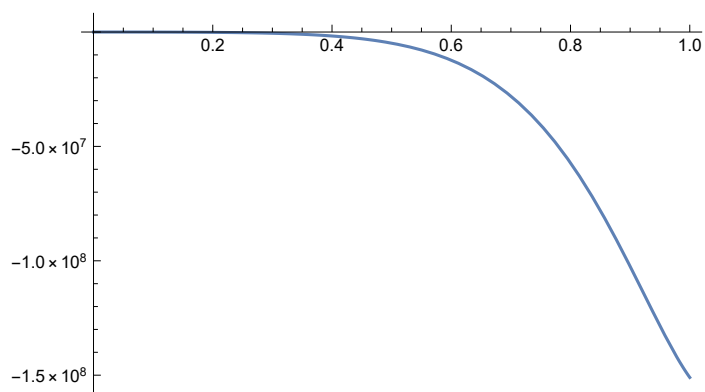

`Plot[Cf[5, 9, 8], {x, 0, 1}]`

[绘图](#)

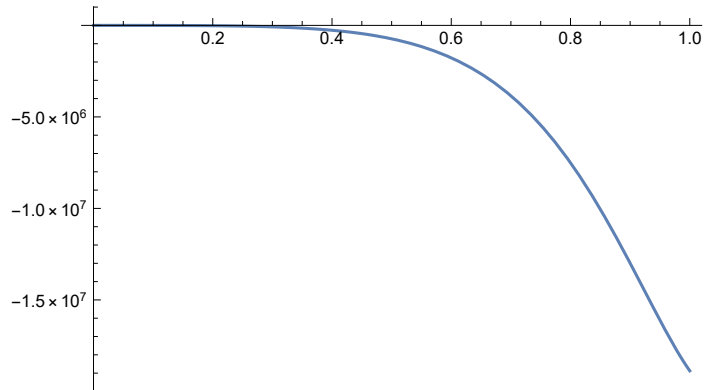

`Plot[Cf[5, 9, 7], {x, 0, 1}]`

[绘图](#)

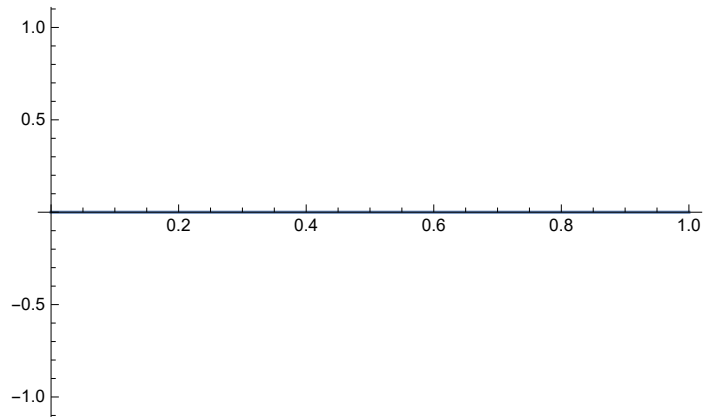

(\*142th group coefficients r2^5r3^8\*)

`Plot[Cf[5, 8, 14], {x, 0, 1}]`

[绘图](#)

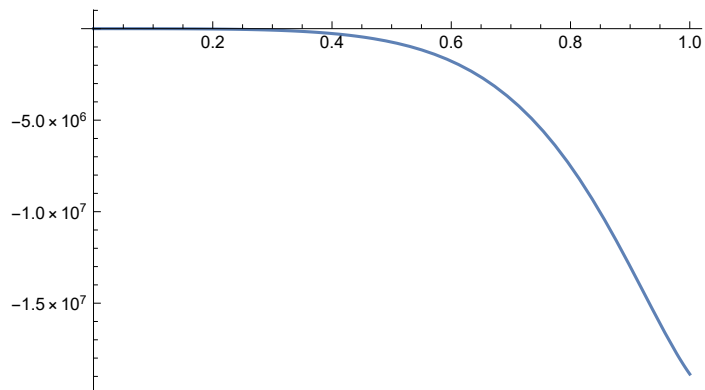

**Plot[Cf[5, 8, 13], {x, 0, 1}]**

[绘图](#)

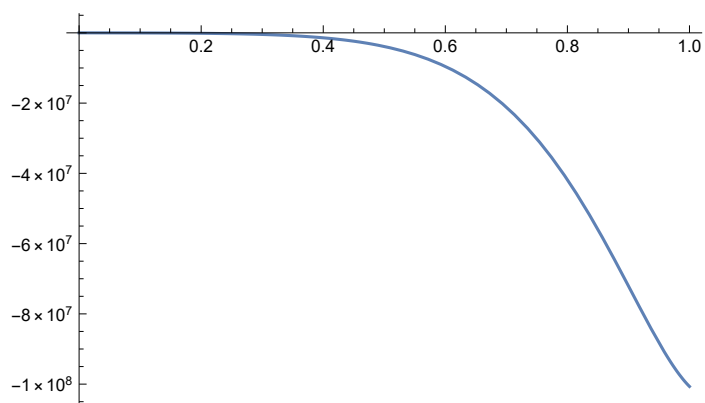

**Plot[Cf[5, 8, 12], {x, 0, 1}]**

[绘图](#)

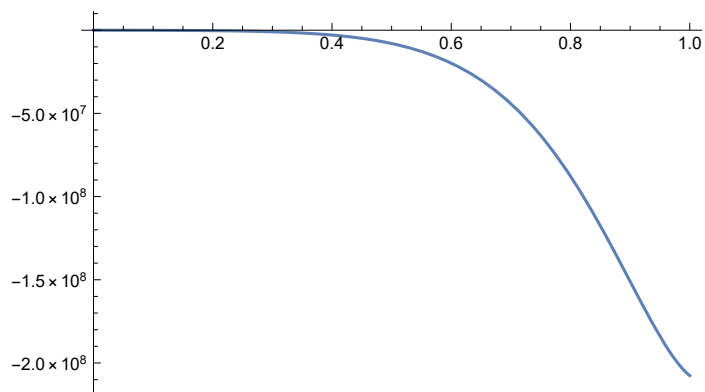

**Plot[Cf[5, 8, 11], {x, 0, 1}]**

[绘图](#)

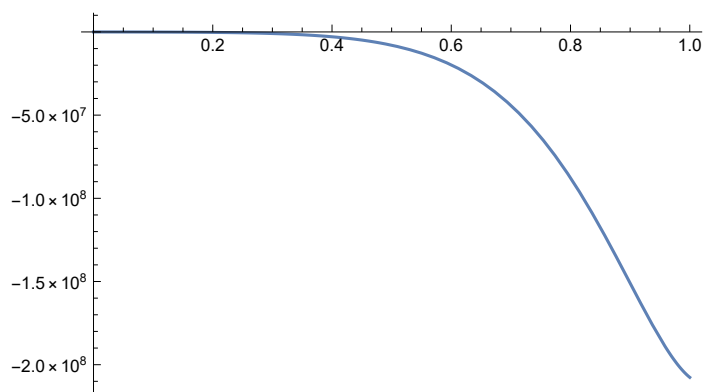

**Plot[Cf[5, 8, 10], {x, 0, 1}]**

[绘图](#)

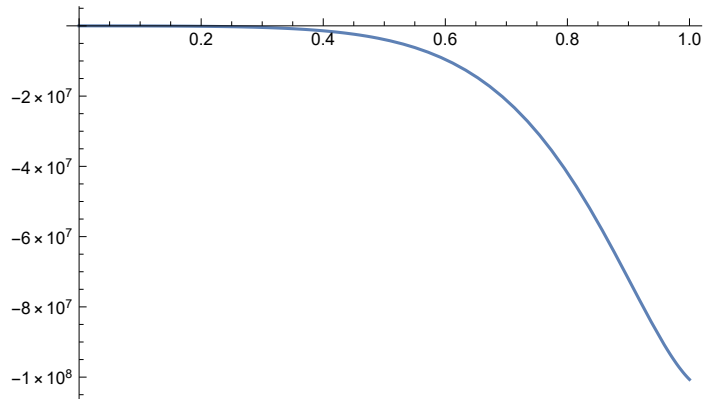

**Plot[Cf[5, 8, 9], {x, 0, 1}]**

[绘图](#)

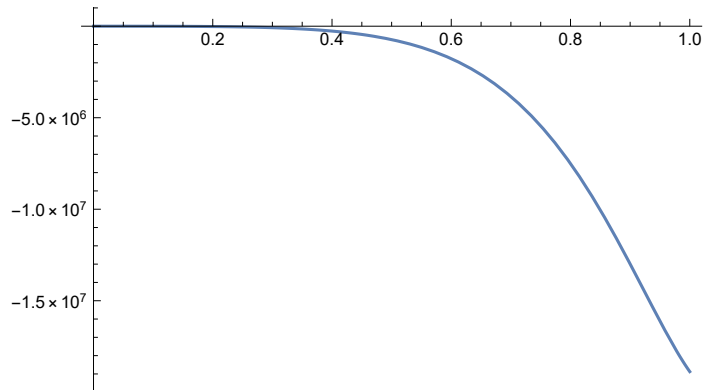

**Plot[Cf[5, 8, 8], {x, 0, 1}]**

[绘图](#)

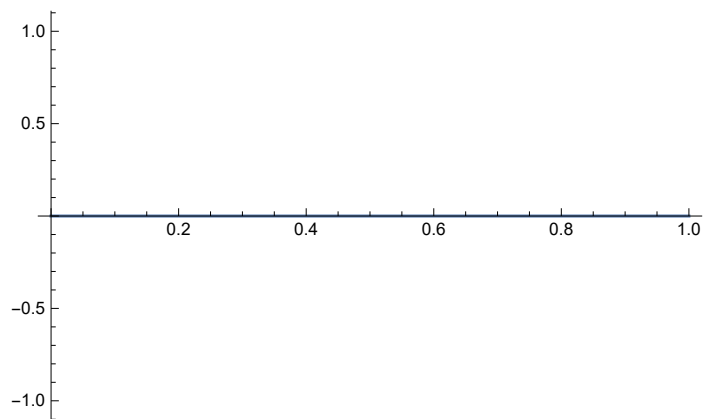

**(\*143th group coefficients r2^5r3^7\*)**

**Plot[Cf[5, 7, 14], {x, 0, 1}]**

[绘图](#)

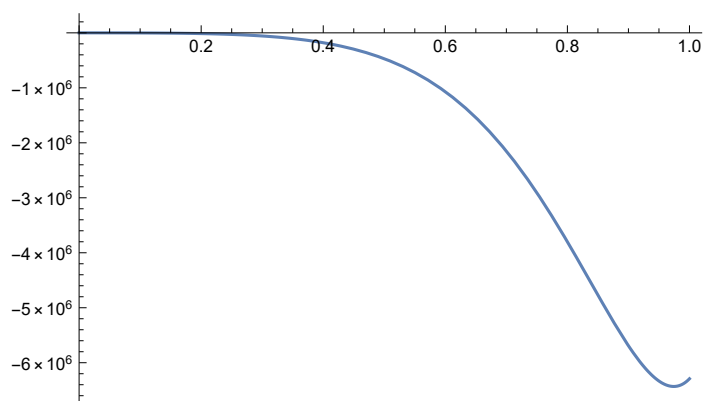

**Plot[Cf[5, 7, 13], {x, 0, 1}]**

[绘图](#)

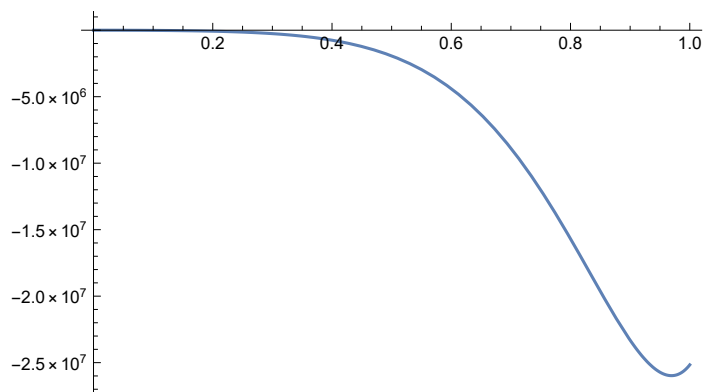

**Plot[Cf[5, 7, 12], {x, 0, 1}]**

[绘图](#)

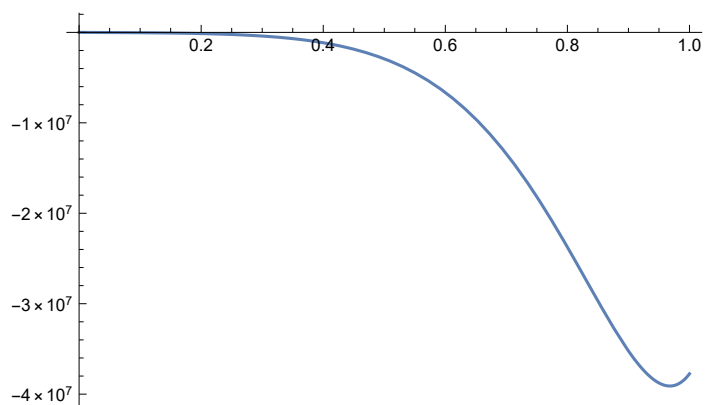



**Plot[Cf[5, 7, 11], {x, 0, 1}]**

[绘图](#)

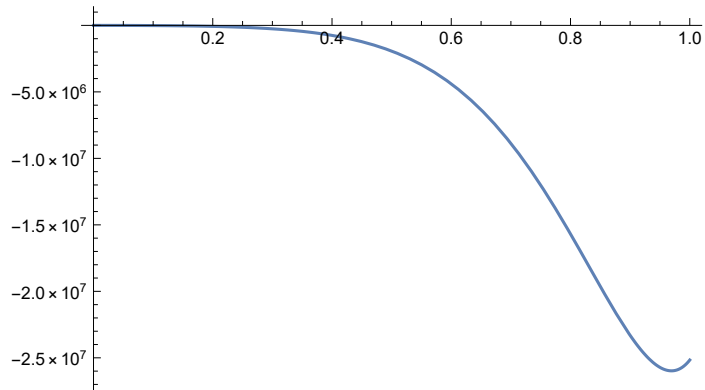

**Plot[Cf[5, 7, 10], {x, 0, 1}]**

[绘图](#)

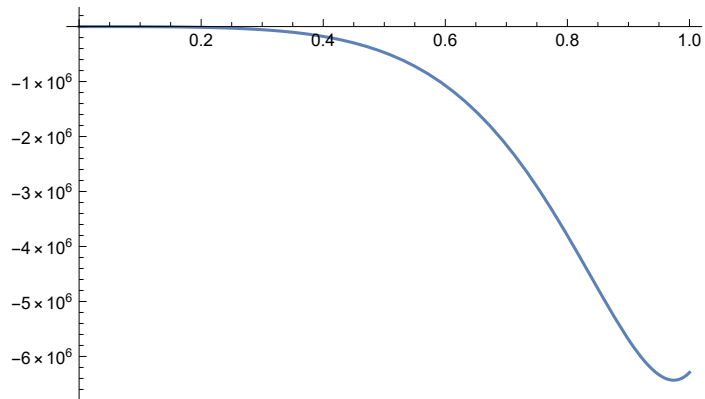

**Plot[Cf[5, 7, 9], {x, 0, 1}]**

[绘图](#)

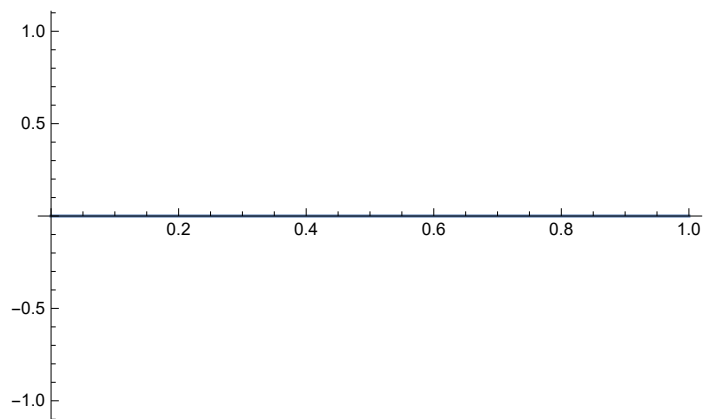

**(\*144th group coefficients r2^5r3^6\*)**

```
Plot[Cf[5, 6, 14], {x, 0, 1}]
```

[绘图](#)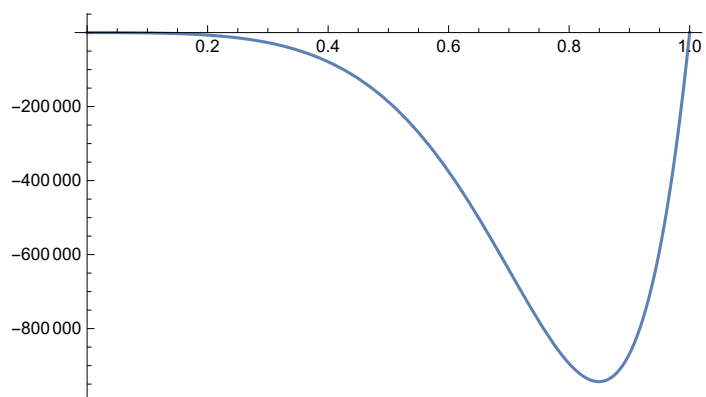

```
Plot[Cf[5, 6, 13], {x, 0, 1}]
```

[绘图](#)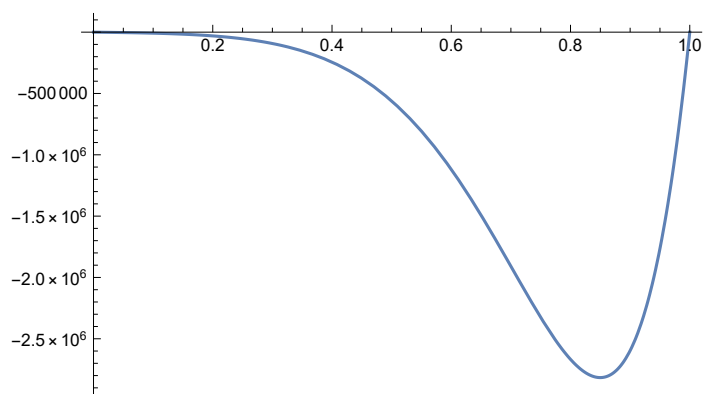

```
Plot[Cf[5, 6, 12], {x, 0, 1}]
```

[绘图](#)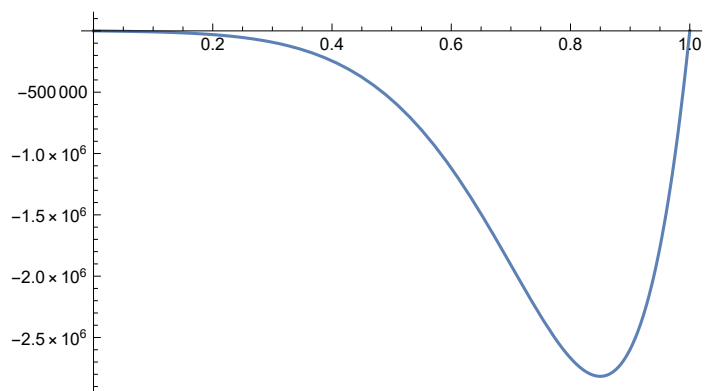

**Plot[Cf[5, 6, 11], {x, 0, 1}]**

[绘图](#)

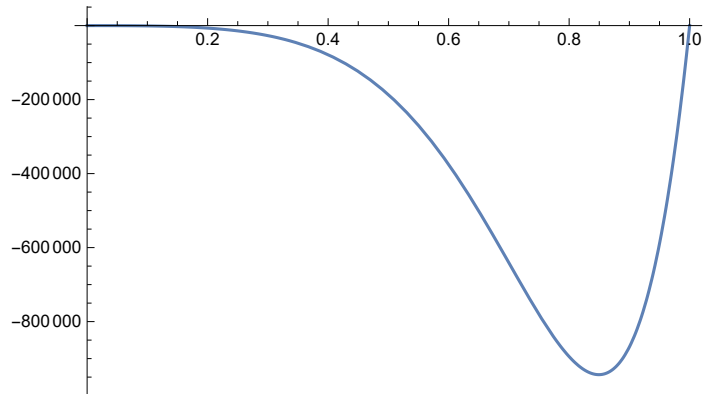

**Plot[Cf[5, 6, 10], {x, 0, 1}]**

[绘图](#)

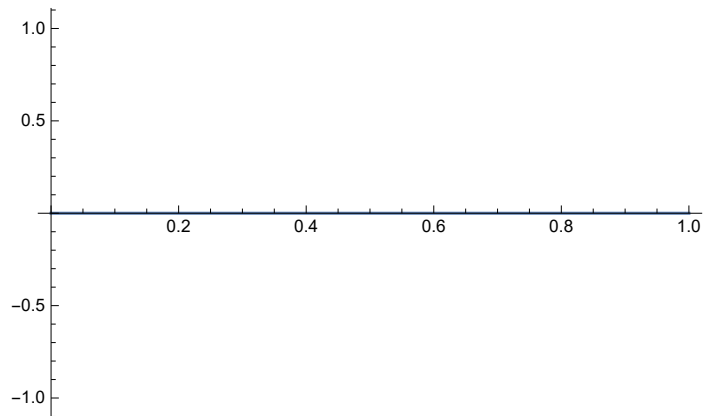

**(\*145th group coefficients r2^5r3^5\*)**

**Plot[Cf[5, 5, 14], {x, 0, 1}]**

[绘图](#)

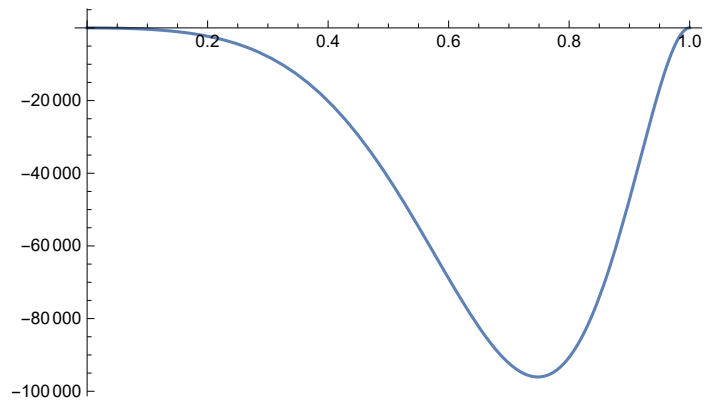

`Plot[Cf[5, 5, 13], {x, 0, 1}]`

[绘图](#)

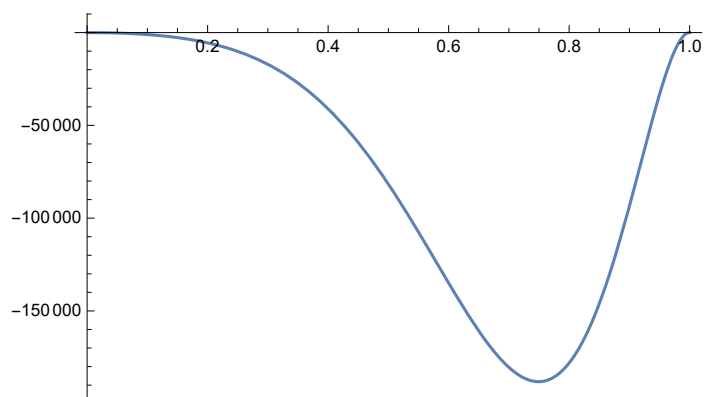

`Plot[Cf[5, 5, 12], {x, 0, 1}]`

[绘图](#)

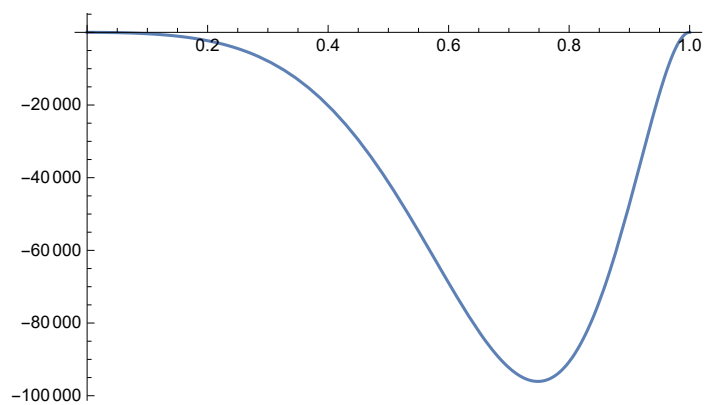

`Plot[Cf[5, 5, 11], {x, 0, 1}]`

[绘图](#)

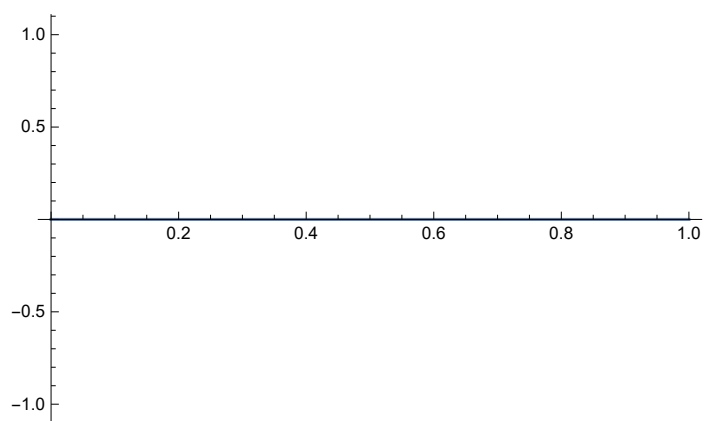

(\*146th group coefficients  $r^2{}^5r^3{}^4*$ )

**Plot[Cf[5, 4, 14], {x, 0, 1}]**

[绘图](#)

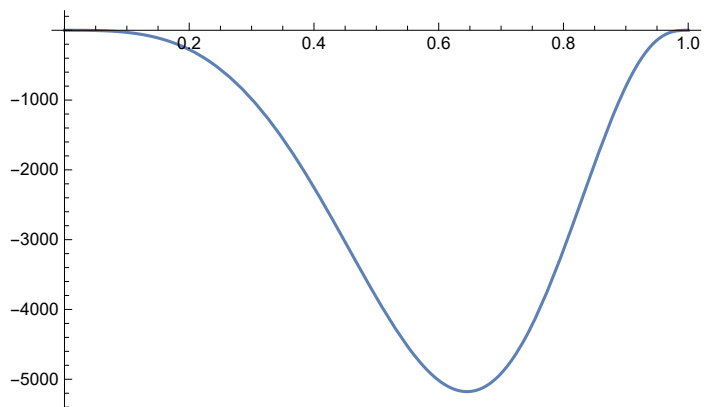

**Plot[Cf[5, 4, 13], {x, 0, 1}]**

[绘图](#)

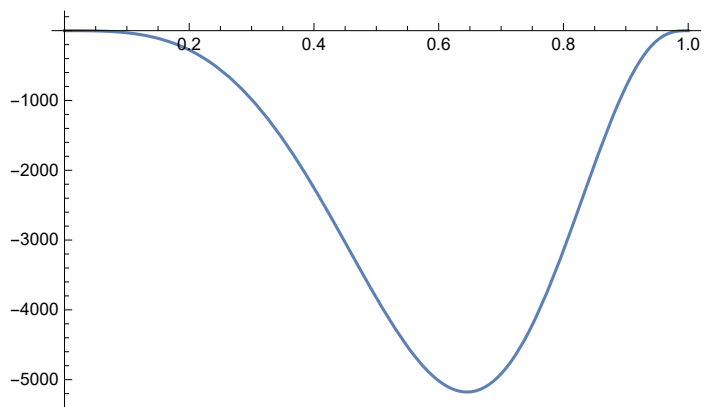

**Plot[Cf[5, 4, 12], {x, 0, 1}]**

[绘图](#)

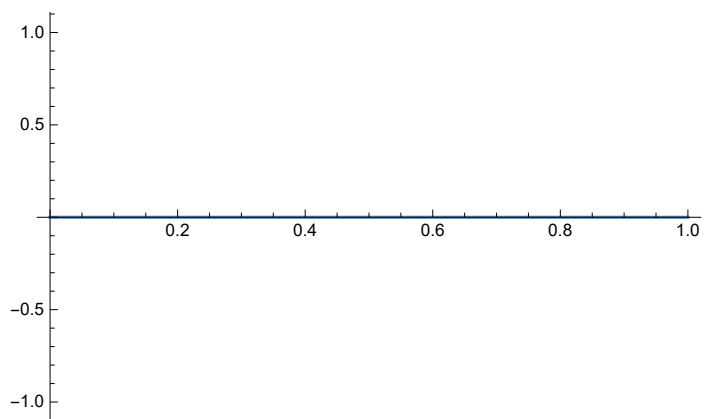

**Plot[Cf[5, 4, 11], {x, 0, 1}]**

[绘图](#)

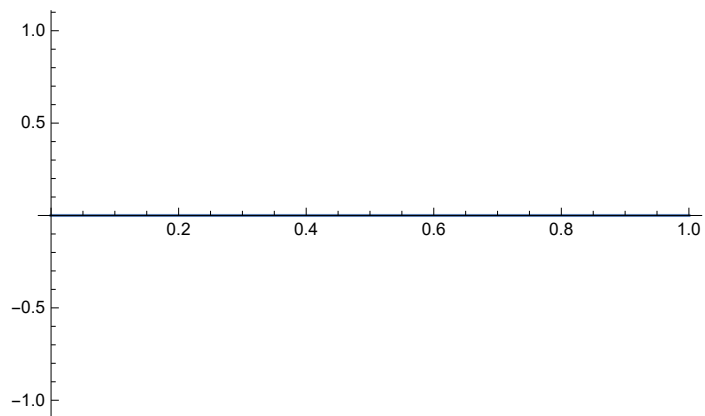

**(\*147th group coefficients r2^5r3^3\*)**

**Plot[Cf[5, 3, 14], {x, 0, 1}]**

[绘图](#)

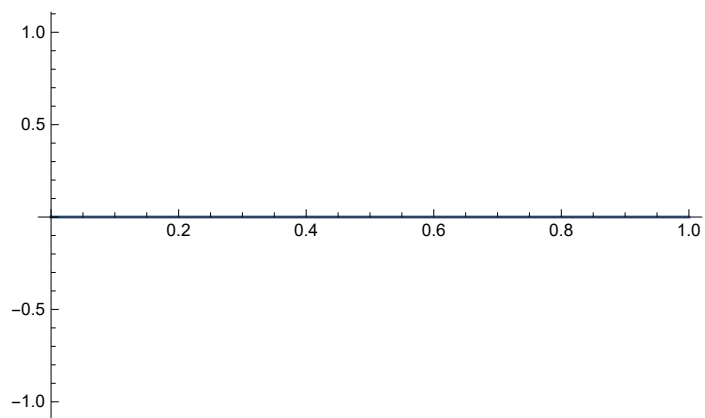

**(\*148th group coefficients r2^5r3^2\*)**

**Plot[Cf[5, 2, 14], {x, 0, 1}]**

[绘图](#)

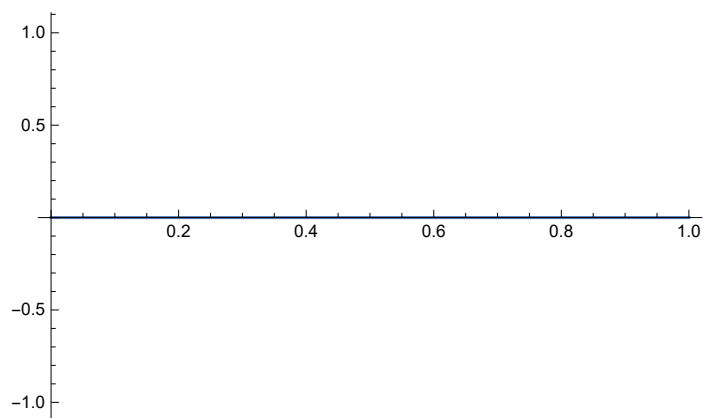

**(\*149th group coefficients r2^5r3^1\*)**

**Plot[Cf[5, 1, 14], {x, 0, 1}]**

[绘图](#)

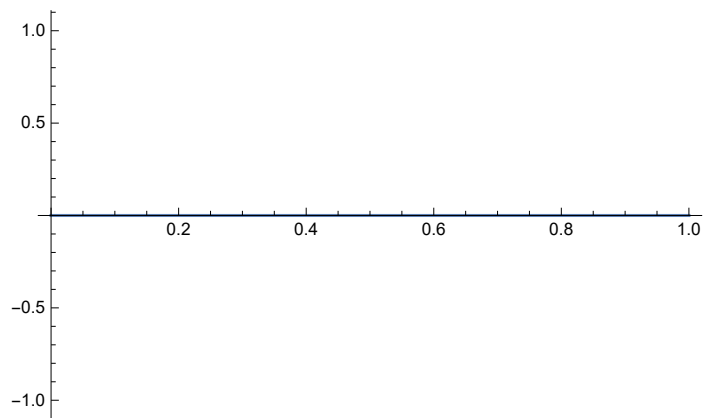

(\*150th group coefficients r2^5r3^0\*)

**Plot[Cf[5, 0, 14], {x, 0, 1}]**

[绘图](#)

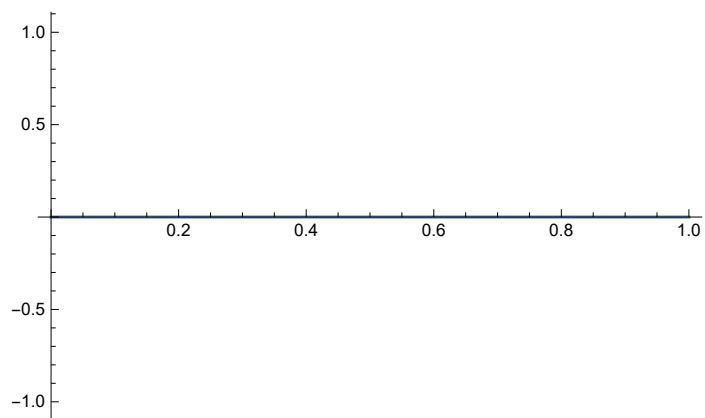

(\*151th group coefficients r2^4r3^14\*)

**Plot[Cf[4, 14, 14], {x, 0, 1}]**

[绘图](#)

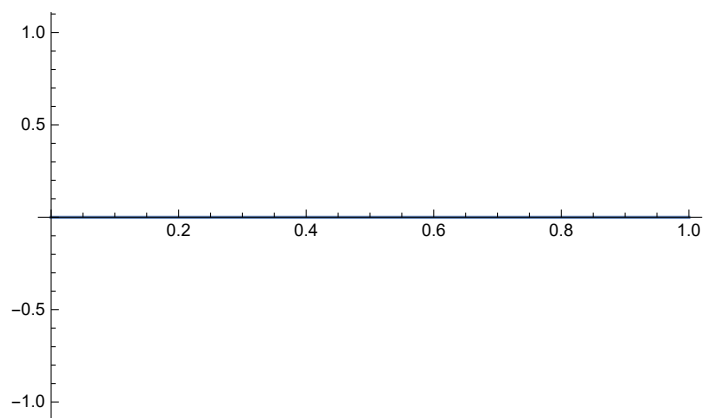

```
Plot[Cf[4, 14, 13], {x, 0, 1}]
```

[绘图](#)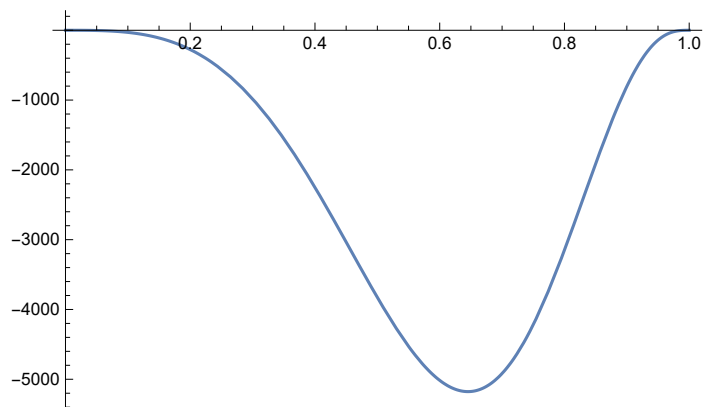

```
Plot[Cf[4, 14, 12], {x, 0, 1}]
```

[绘图](#)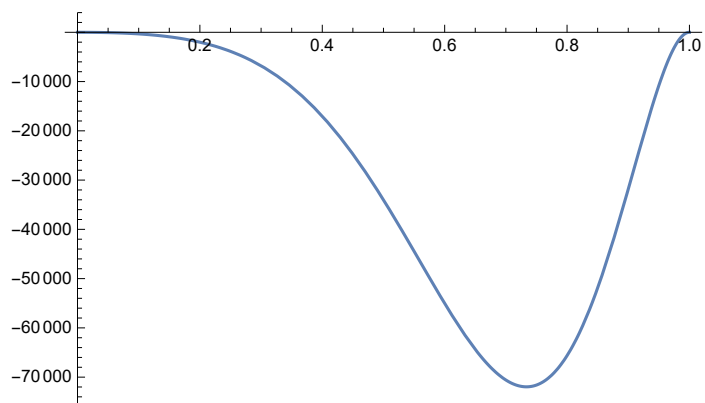

```
Plot[Cf[4, 14, 11], {x, 0, 1}]
```

[绘图](#)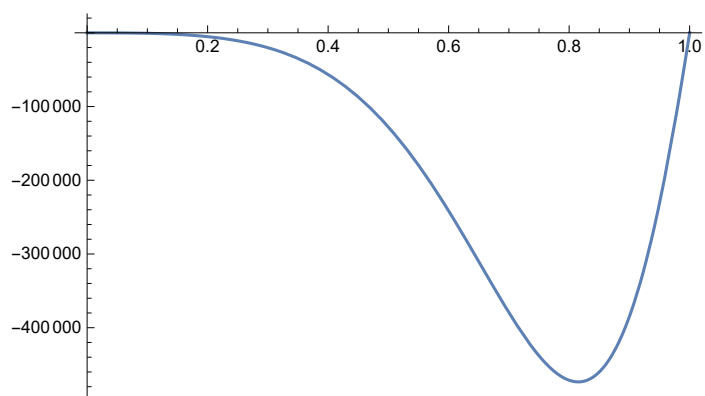



**Plot[Cf[4, 14, 10], {x, 0, 1}]**

[绘图](#)

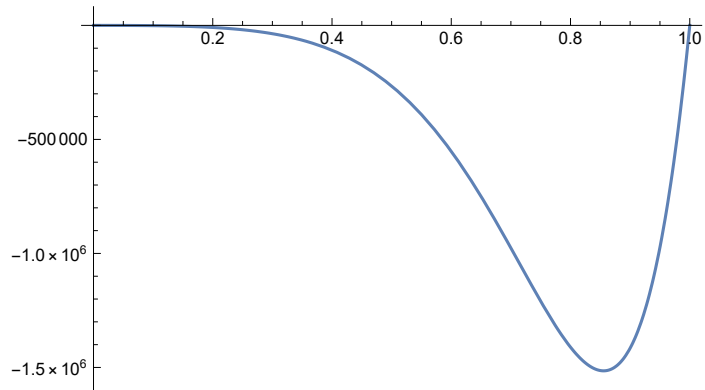

**Plot[Cf[4, 14, 9], {x, 0, 1}]**

[绘图](#)

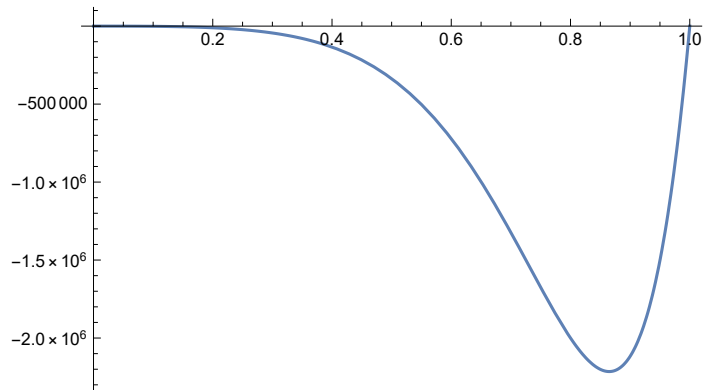

**Plot[Cf[4, 14, 8], {x, 0, 1}]**

[绘图](#)

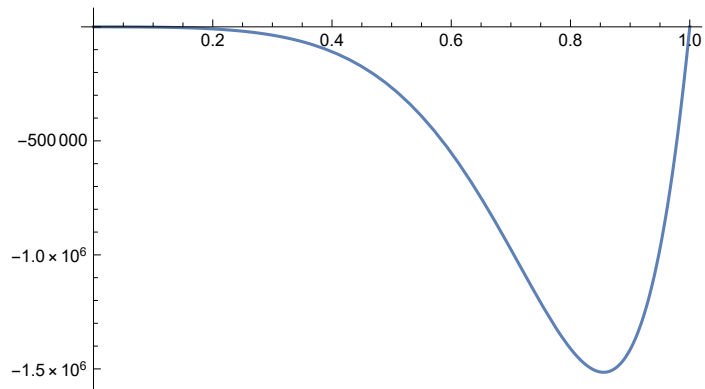

**Plot[Cf[4, 14, 7], {x, 0, 1}]**

[绘图](#)

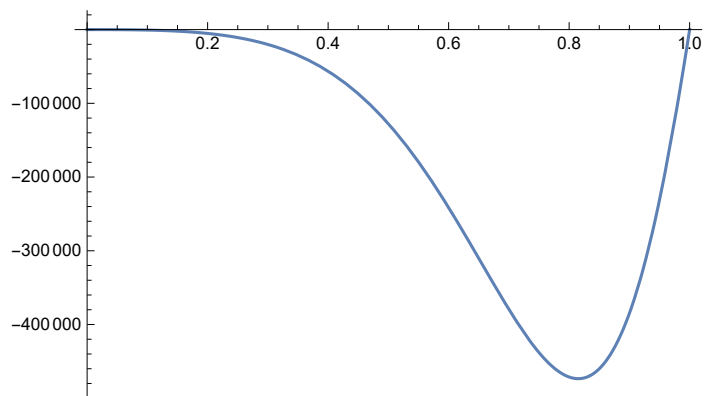

**Plot[Cf[4, 14, 6], {x, 0, 1}]**

[绘图](#)

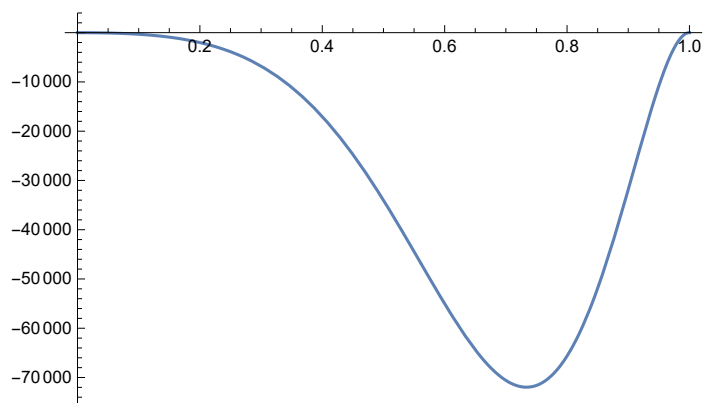

**Plot[Cf[4, 14, 5], {x, 0, 1}]**

[绘图](#)

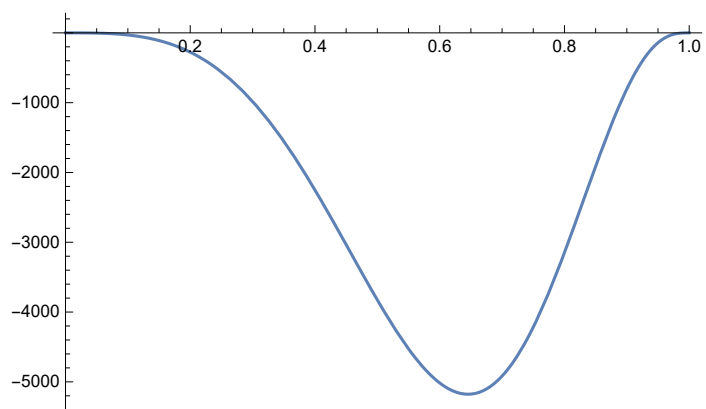

**Plot[Cf[4, 14, 4], {x, 0, 1}]**

[绘图](#)

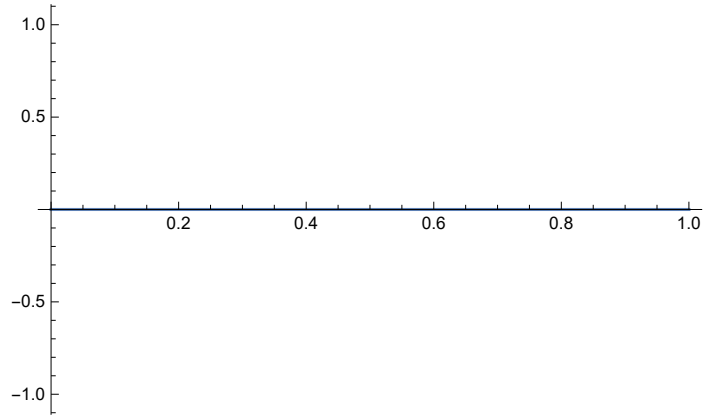

**(\*152th group coefficients r2^4r3^13\*)**

**Plot[Cf[4, 13, 14], {x, 0, 1}]**

[绘图](#)

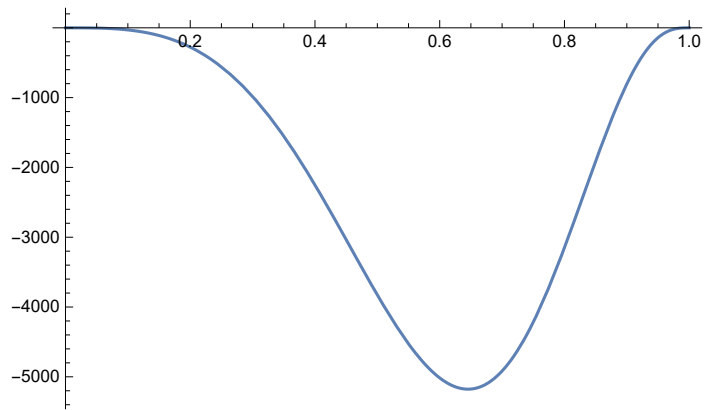

**Plot[Cf[4, 13, 13], {x, 0, 1}]**

[绘图](#)

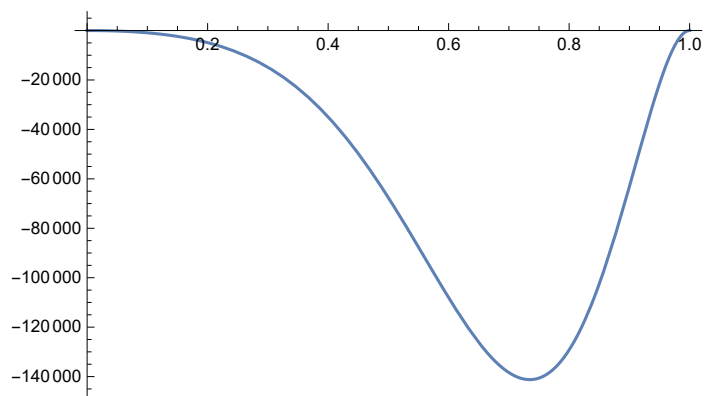

```
Plot[Cf[4, 13, 12], {x, 0, 1}]
```

[绘图](#)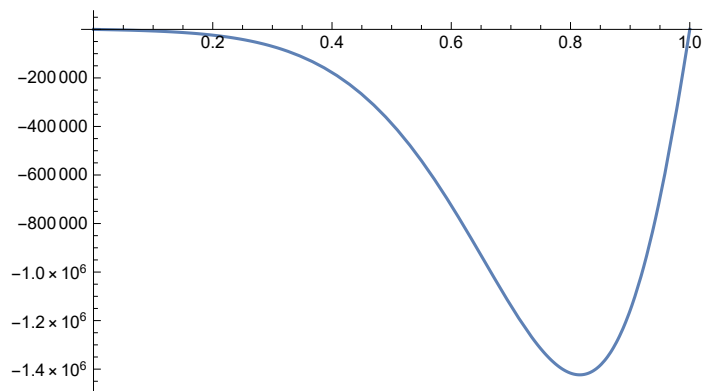

```
Plot[Cf[4, 13, 11], {x, 0, 1}]
```

[绘图](#)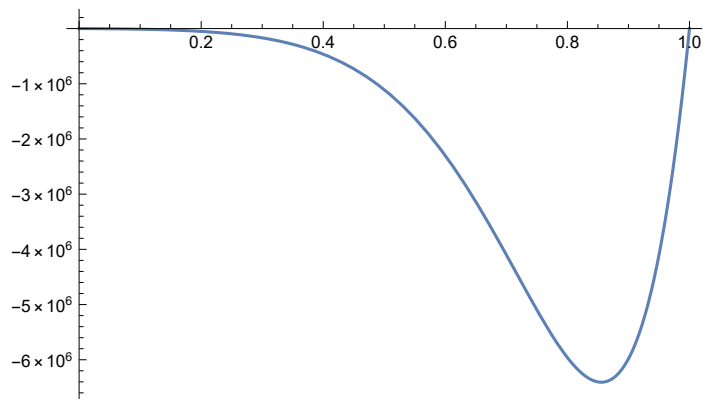

```
Plot[Cf[4, 13, 10], {x, 0, 1}]
```

[绘图](#)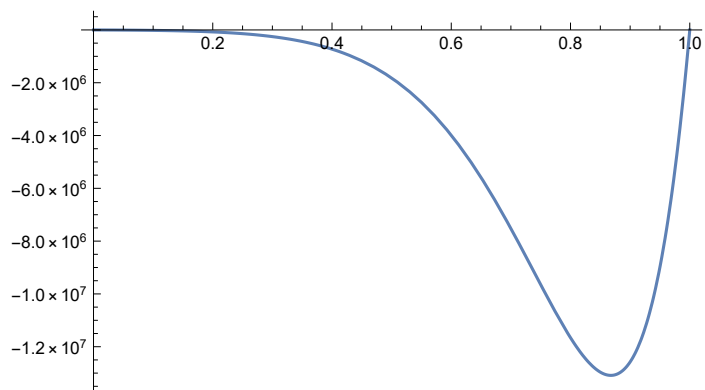

**Plot[Cf[4, 13, 9], {x, 0, 1}]**

[绘图](#)

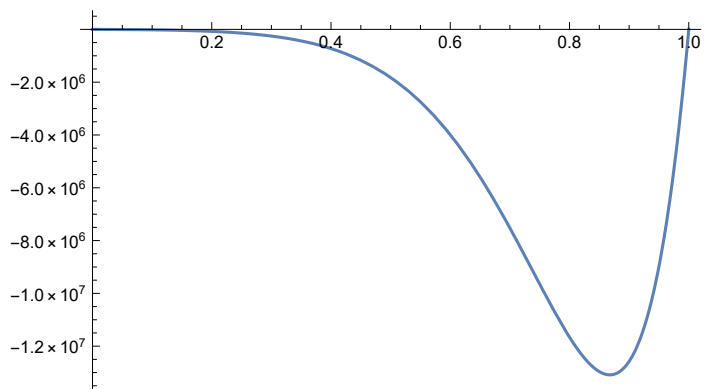

**Plot[Cf[4, 13, 8], {x, 0, 1}]**

[绘图](#)

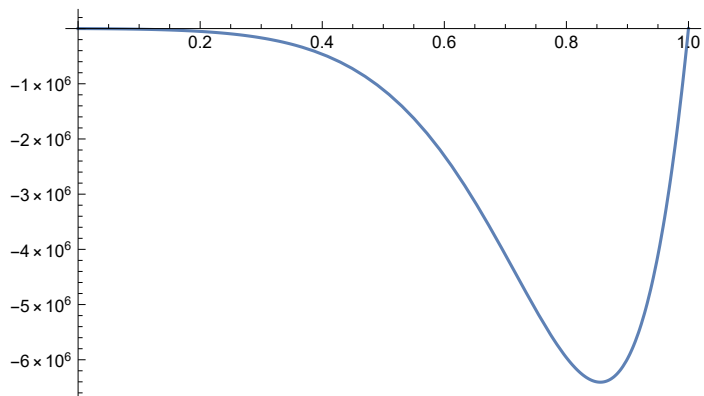

**Plot[Cf[4, 13, 7], {x, 0, 1}]**

[绘图](#)

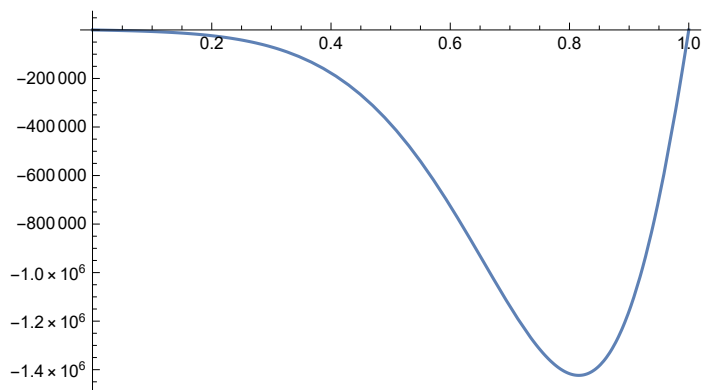

**Plot[Cf[4, 13, 6], {x, 0, 1}]**

[绘图](#)

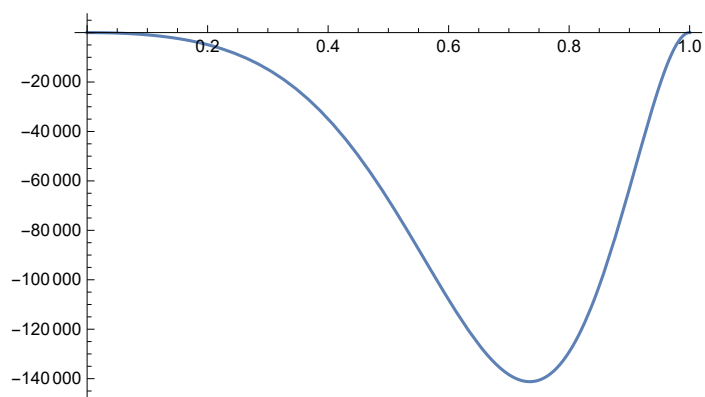

**Plot[Cf[4, 13, 5], {x, 0, 1}]**

[绘图](#)

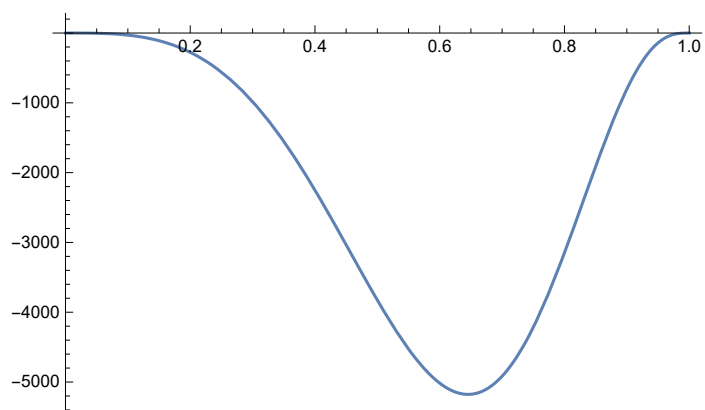

**Plot[Cf[4, 13, 4], {x, 0, 1}]**

[绘图](#)

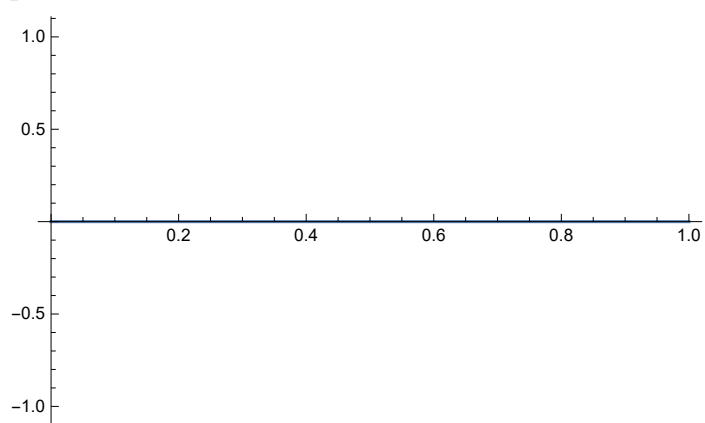

(\*153th group coefficients r2^4r3^12\*)

**Plot[Cf[4, 12, 14], {x, 0, 1}]**

[绘图](#)

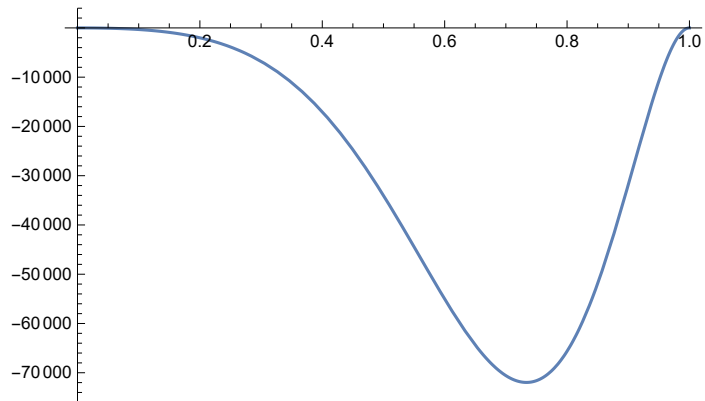

**Plot[Cf[4, 12, 13], {x, 0, 1}]**

[绘图](#)

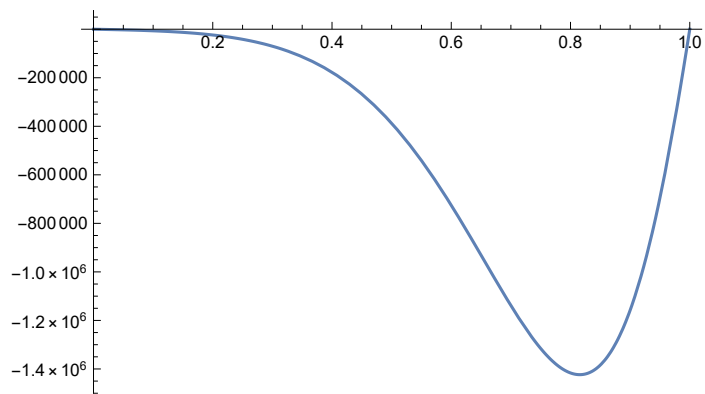

**Plot[Cf[4, 12, 12], {x, 0, 1}]**

[绘图](#)

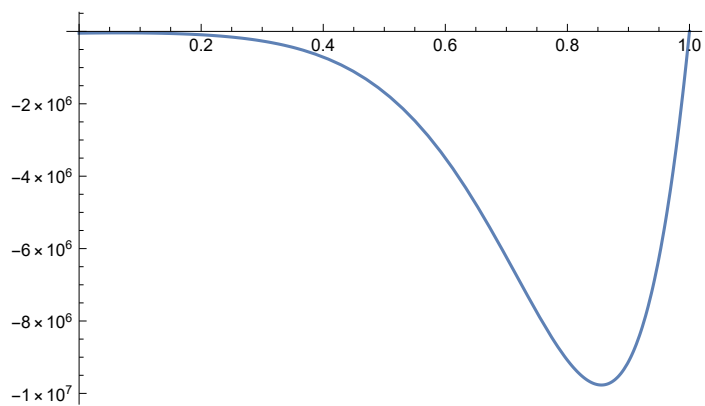

**Plot[Cf[4, 12, 11], {x, 0, 1}]**

[绘图](#)

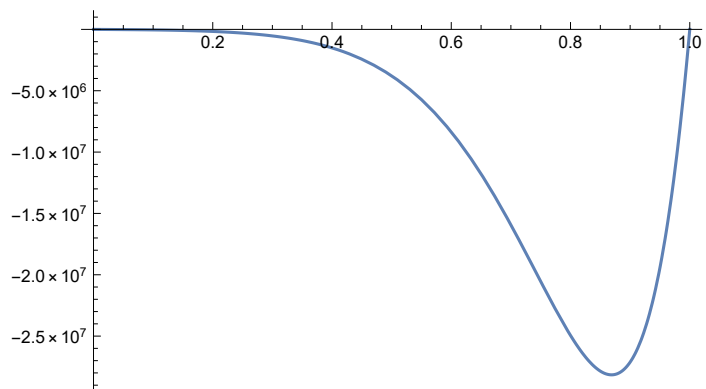

**Plot[Cf[4, 12, 10], {x, 0, 1}]**

[绘图](#)

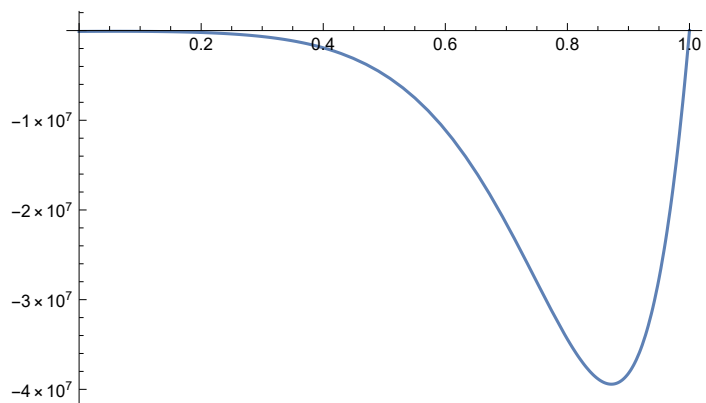

**Plot[Cf[4, 12, 9], {x, 0, 1}]**

[绘图](#)

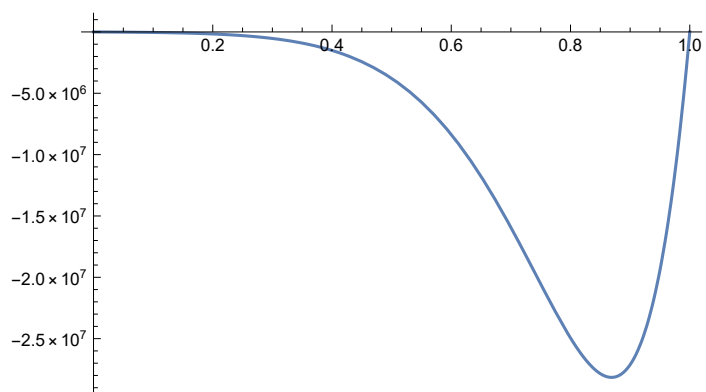



**Plot[Cf[4, 12, 8], {x, 0, 1}]**

[绘图](#)

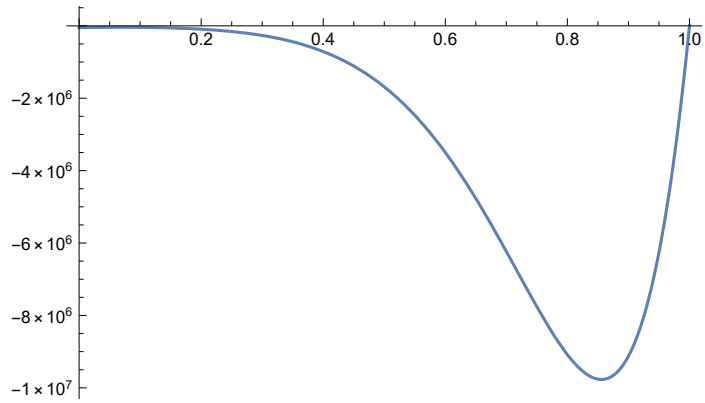

**Plot[Cf[4, 12, 7], {x, 0, 1}]**

[绘图](#)

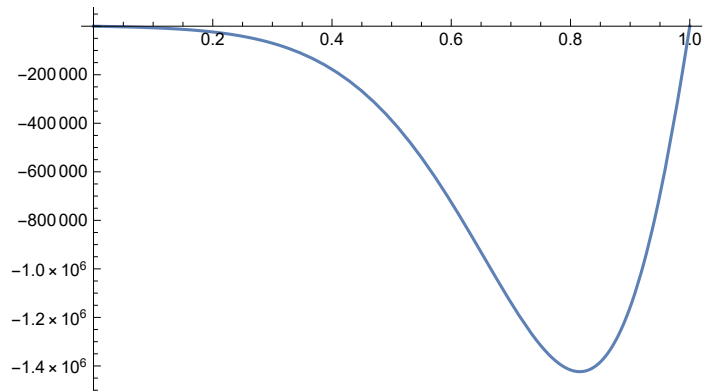

**Plot[Cf[4, 12, 6], {x, 0, 1}]**

[绘图](#)

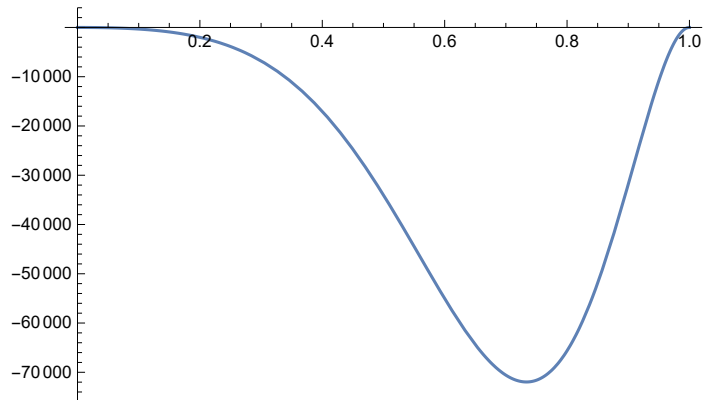

`Plot[Cf[4, 12, 5], {x, 0, 1}]`

[绘图](#)

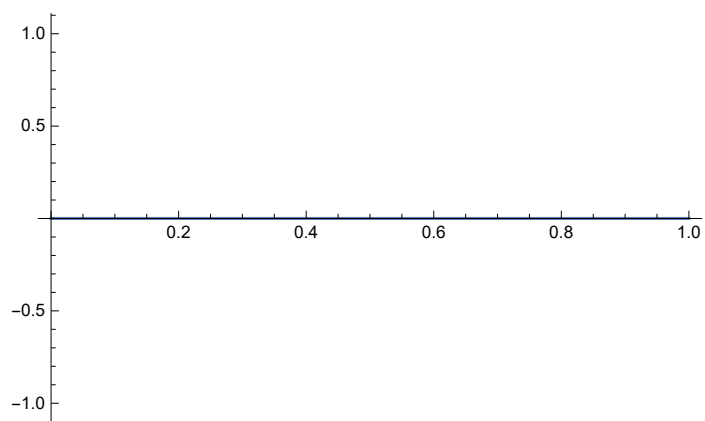

(\*154th group coefficients  $r^2 r^3$ \*)

`Plot[Cf[4, 11, 14], {x, 0, 1}]`

[绘图](#)

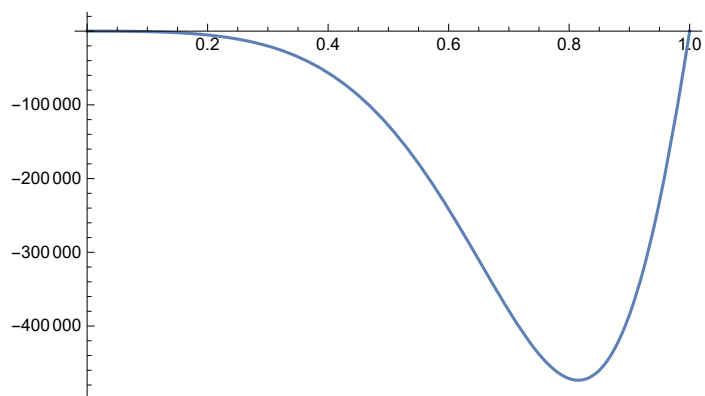

`Plot[Cf[4, 11, 13], {x, 0, 1}]`

[绘图](#)

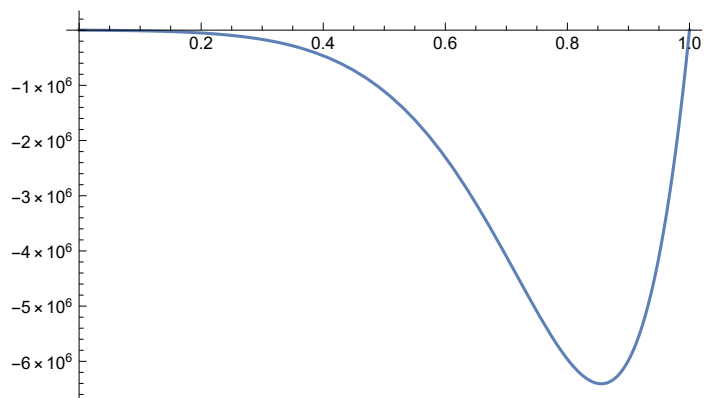

**Plot[Cf[4, 11, 12], {x, 0, 1}]**

[绘图](#)

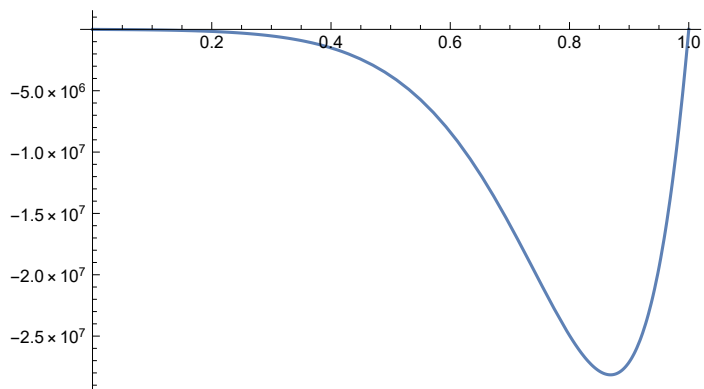

**Plot[Cf[4, 11, 11], {x, 0, 1}]**

[绘图](#)

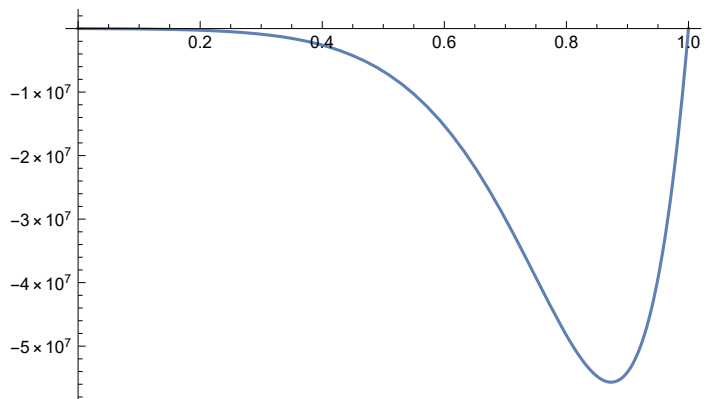

**Plot[Cf[4, 11, 10], {x, 0, 1}]**

[绘图](#)

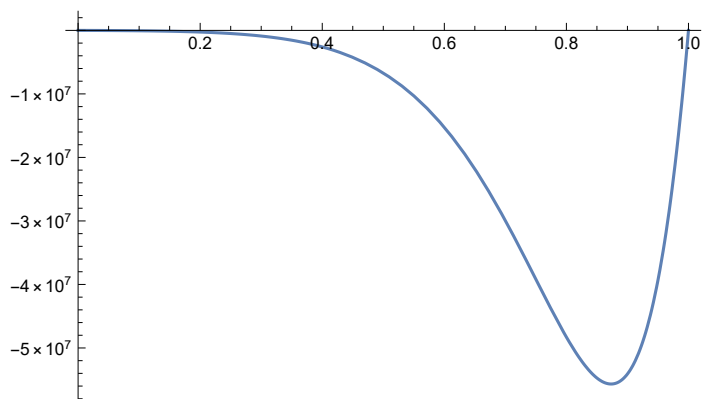

**Plot[Cf[4, 11, 9], {x, 0, 1}]**

[绘图](#)

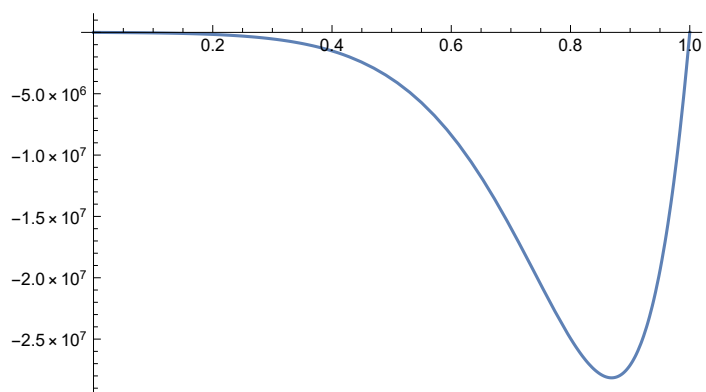

**Plot[Cf[4, 11, 8], {x, 0, 1}]**

[绘图](#)

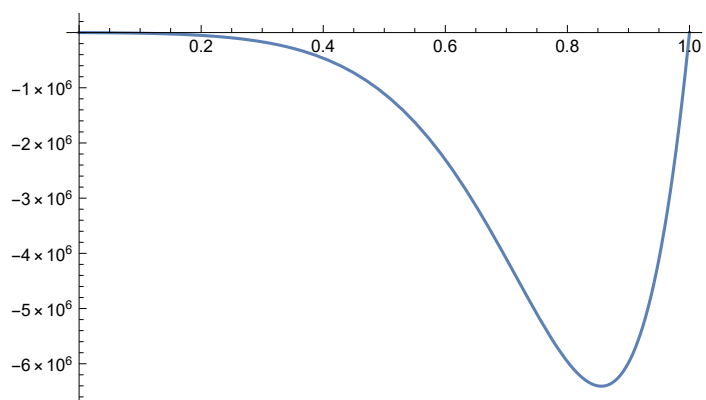

**Plot[Cf[4, 11, 7], {x, 0, 1}]**

[绘图](#)

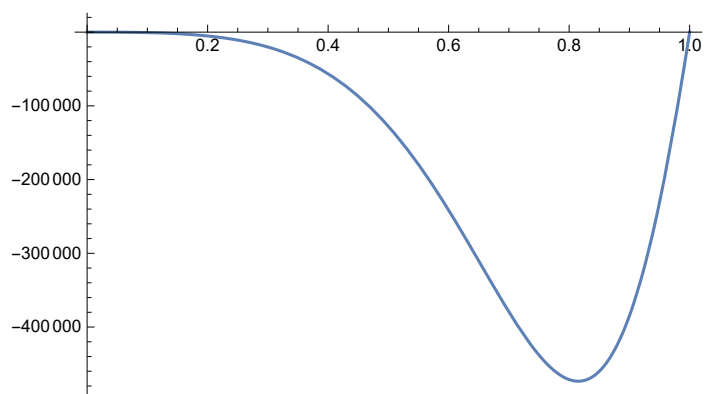

**Plot[Cf[4, 11, 6], {x, 0, 1}]**

[绘图](#)

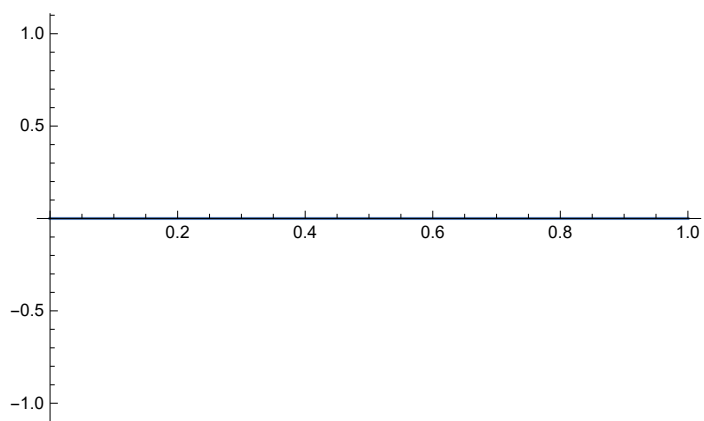

(\*155th group coefficients r2^4r3^10\*)

**Plot[Cf[4, 10, 14], {x, 0, 1}]**

[绘图](#)

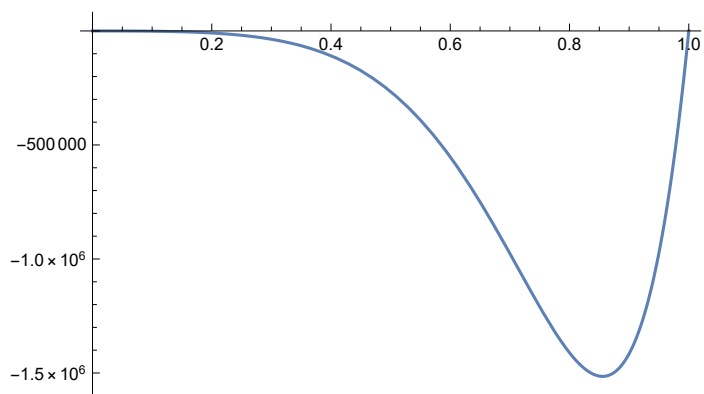

**Plot[Cf[4, 10, 13], {x, 0, 1}]**

[绘图](#)

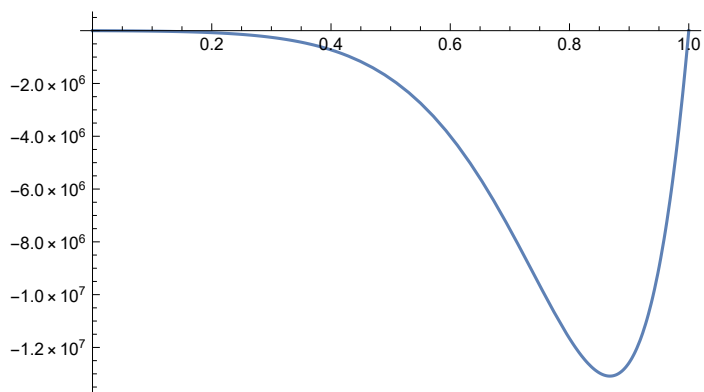

```
Plot[Cf[4, 10, 12], {x, 0, 1}]
```

[绘图](#)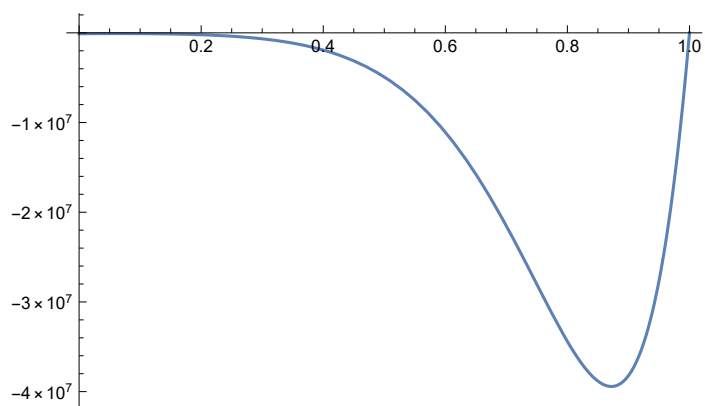

```
Plot[Cf[4, 10, 11], {x, 0, 1}]
```

[绘图](#)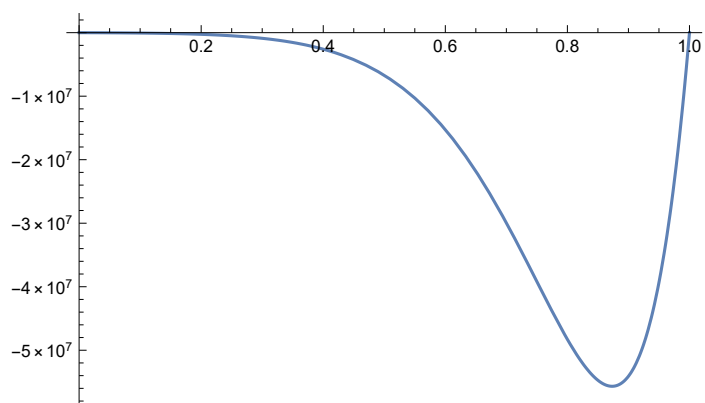

```
Plot[Cf[4, 10, 10], {x, 0, 1}]
```

[绘图](#)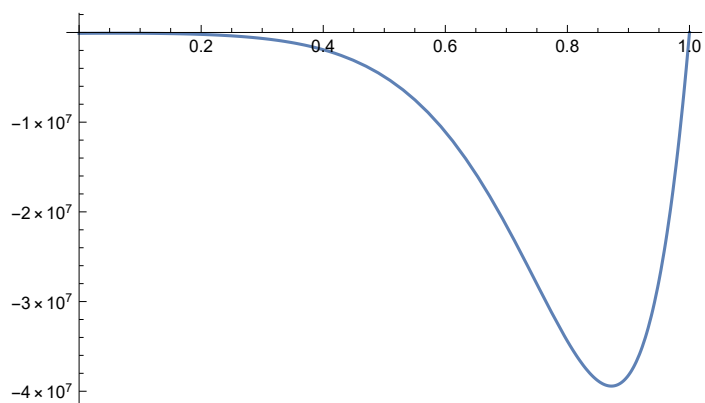

**Plot[Cf[4, 10, 9], {x, 0, 1}]**

[绘图](#)

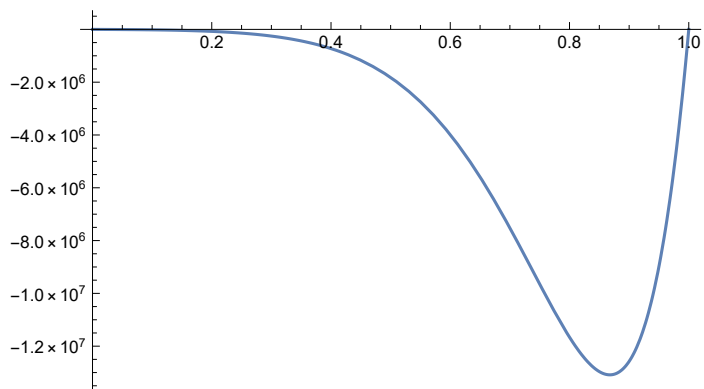

**Plot[Cf[4, 10, 8], {x, 0, 1}]**

[绘图](#)

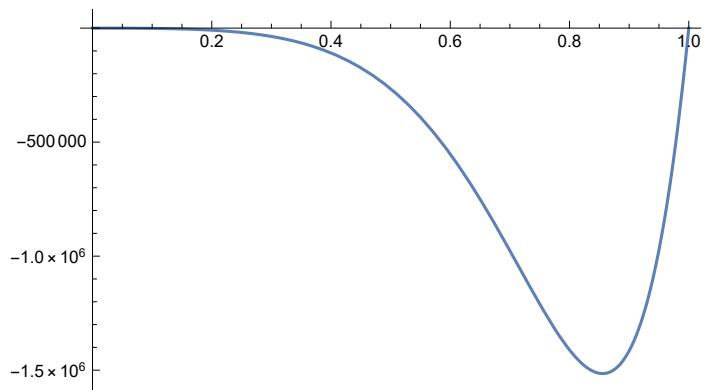

**Plot[Cf[4, 10, 7], {x, 0, 1}]**

[绘图](#)

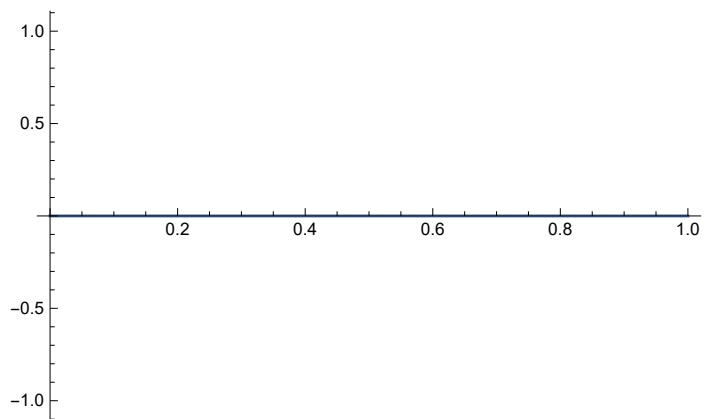

(\*156th group coefficients r2^4r3^9\*)

```
Plot[Cf[4, 9, 14], {x, 0, 1}]
```

[绘图](#)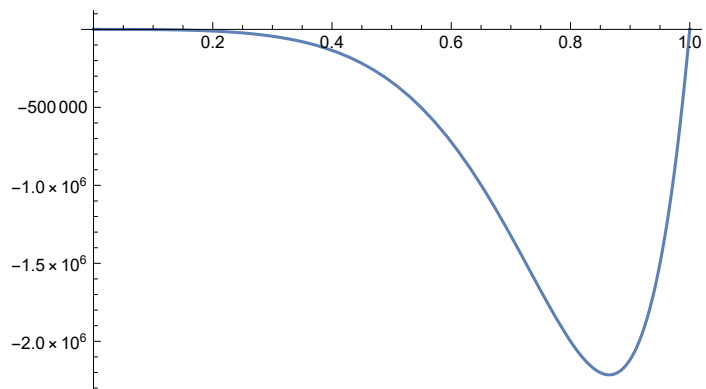

```
Plot[Cf[4, 9, 13], {x, 0, 1}]
```

[绘图](#)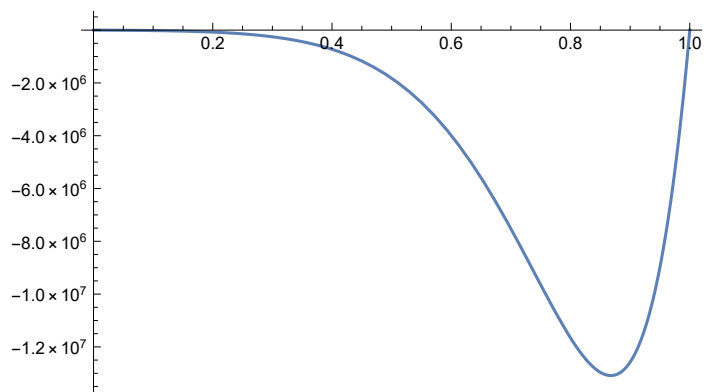

```
Plot[Cf[4, 9, 12], {x, 0, 1}]
```

[绘图](#)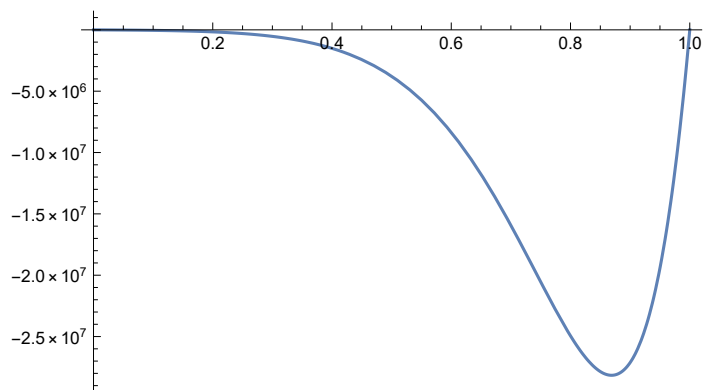



**Plot[Cf[4, 9, 11], {x, 0, 1}]**

[绘图](#)

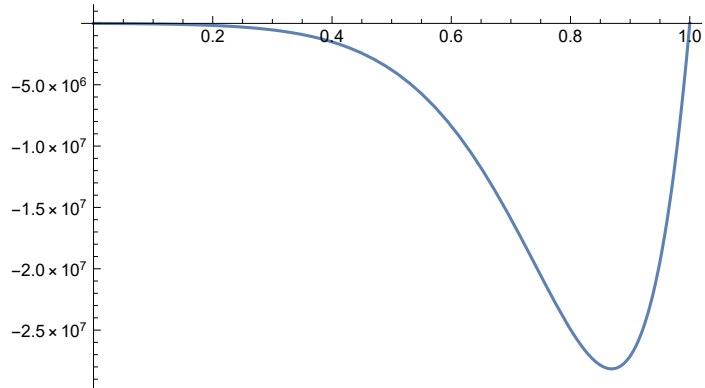

**Plot[Cf[4, 9, 10], {x, 0, 1}]**

[绘图](#)

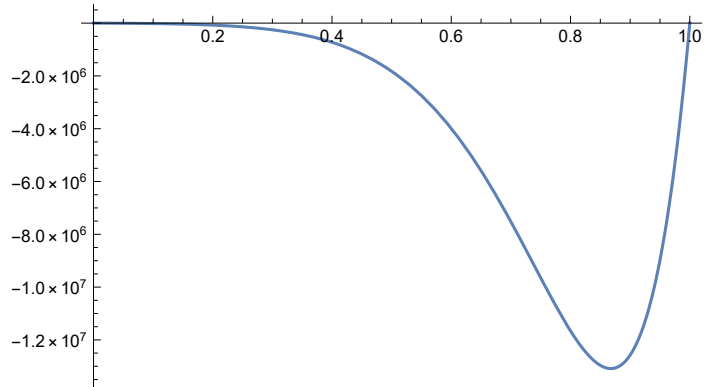

**Plot[Cf[4, 9, 9], {x, 0, 1}]**

[绘图](#)

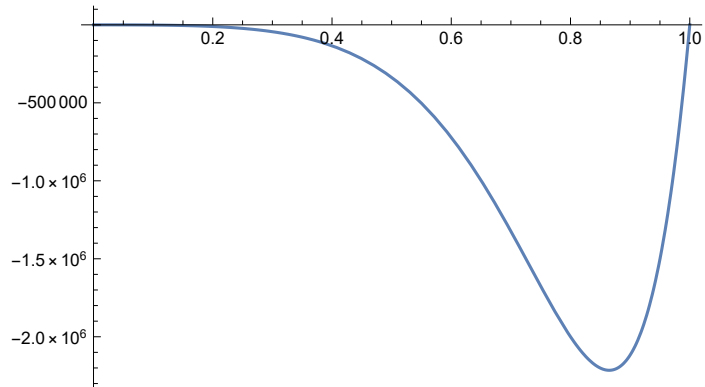

`Plot[Cf[4, 9, 8], {x, 0, 1}]`

[绘图](#)

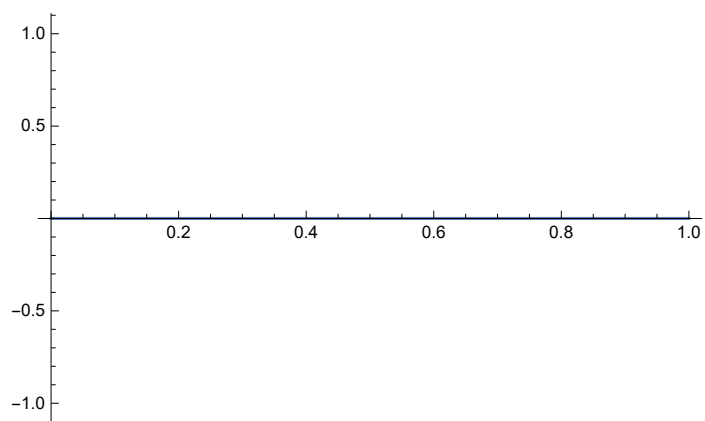

(\*157th group coefficients  $r^2 r^3 r^8$ \*)

`Plot[Cf[4, 8, 14], {x, 0, 1}]`

[绘图](#)

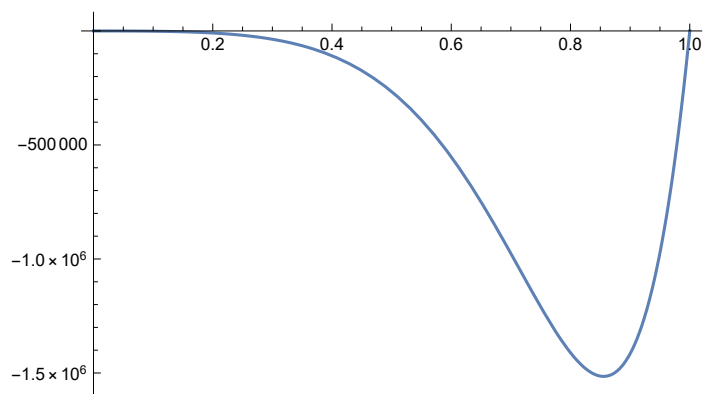

`Plot[Cf[4, 8, 13], {x, 0, 1}]`

[绘图](#)

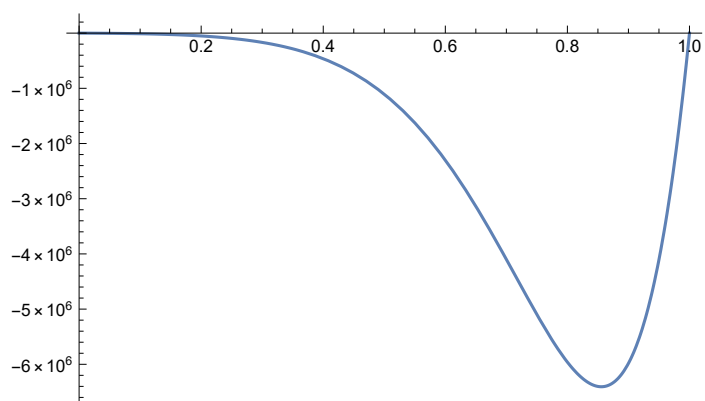

**Plot[Cf[4, 8, 12], {x, 0, 1}]**

[绘图](#)

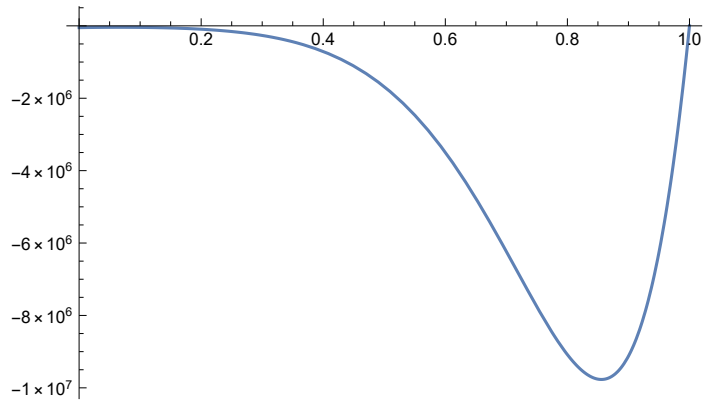

**Plot[Cf[4, 8, 11], {x, 0, 1}]**

[绘图](#)

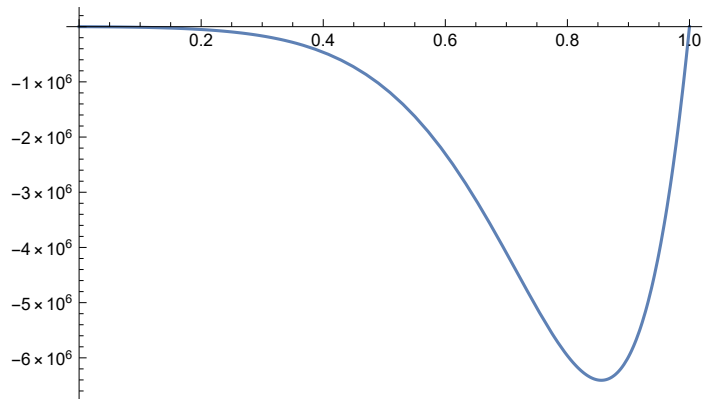

**Plot[Cf[4, 8, 10], {x, 0, 1}]**

[绘图](#)

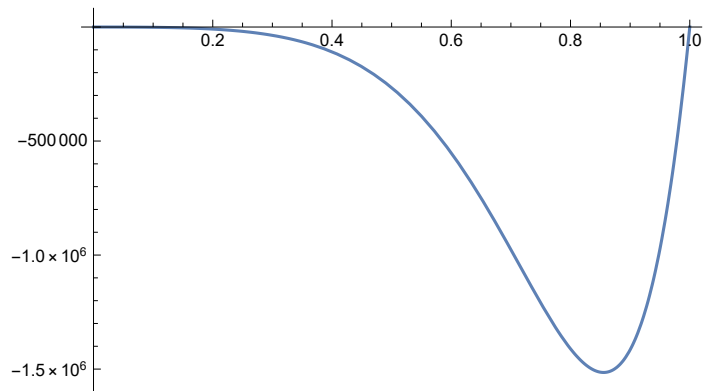

**Plot[Cf[4, 8, 9], {x, 0, 1}]**

[绘图](#)

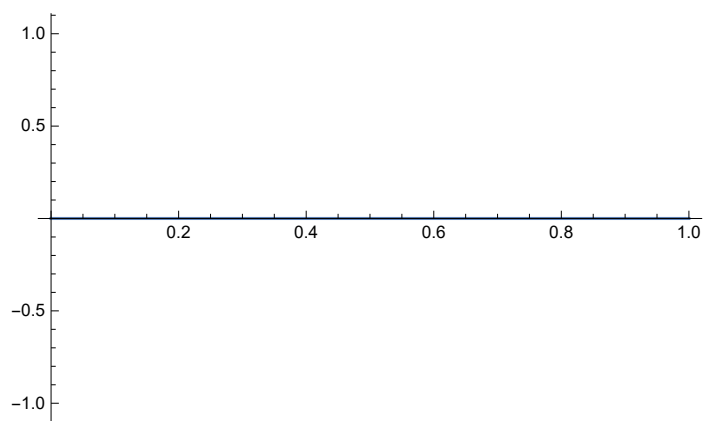

(\*158th group coefficients  $r_2^4 r_3^7$ \*)

**Plot[Cf[4, 7, 14], {x, 0, 1}]**

[绘图](#)

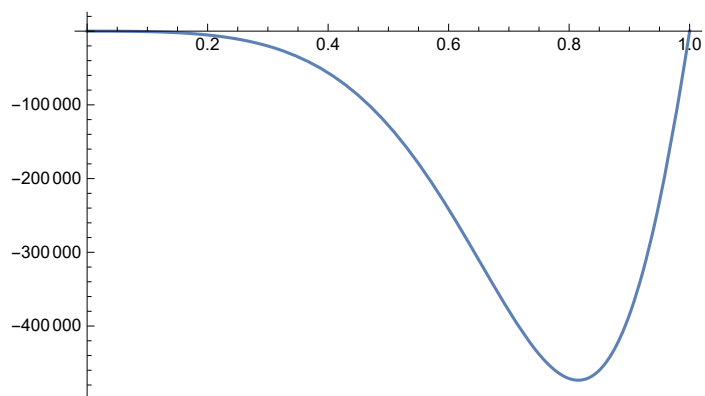

**Plot[Cf[4, 7, 13], {x, 0, 1}]**

[绘图](#)

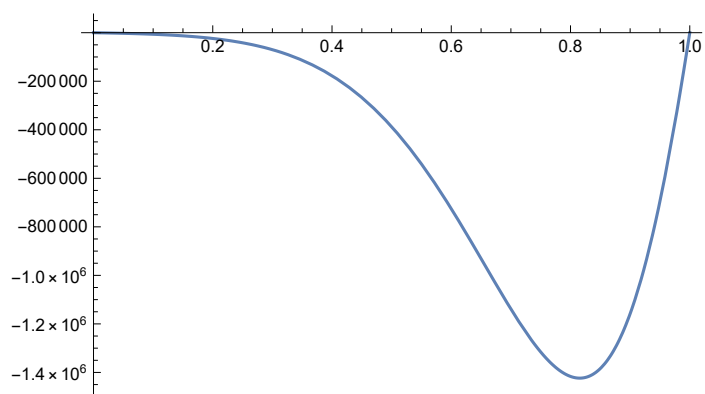

**Plot[Cf[4, 7, 12], {x, 0, 1}]**

[绘图](#)

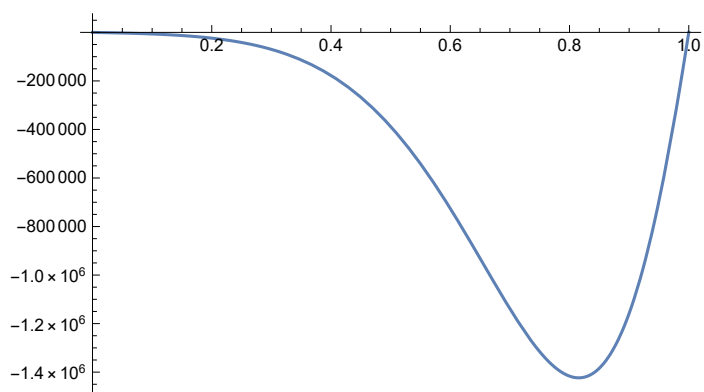

**Plot[Cf[4, 7, 11], {x, 0, 1}]**

[绘图](#)

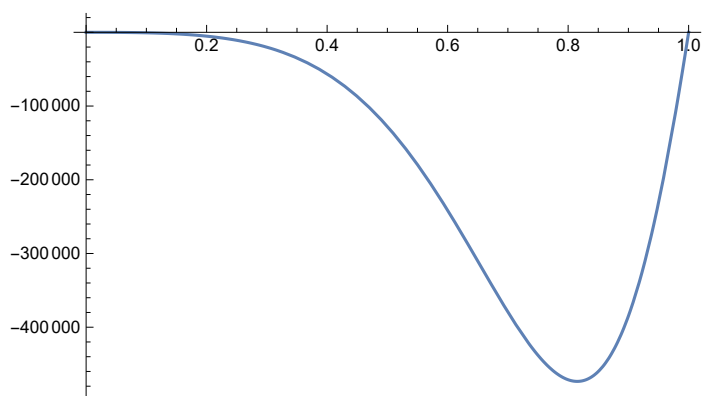

**Plot[Cf[4, 7, 10], {x, 0, 1}]**

[绘图](#)

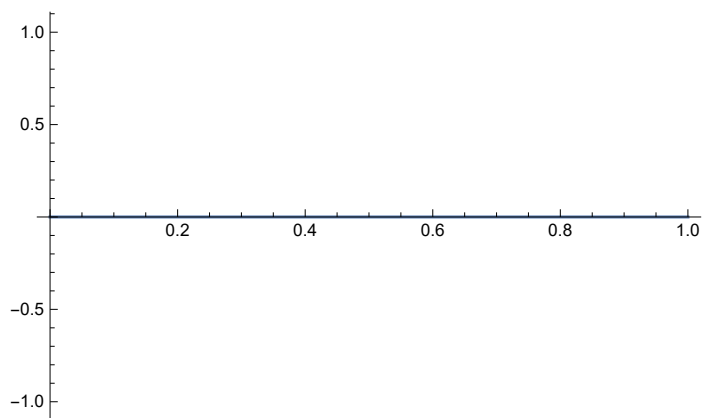

(\*159th group coefficients r2^4r3^6\*)

**Plot[Cf[4, 6, 14], {x, 0, 1}]**

[绘图](#)

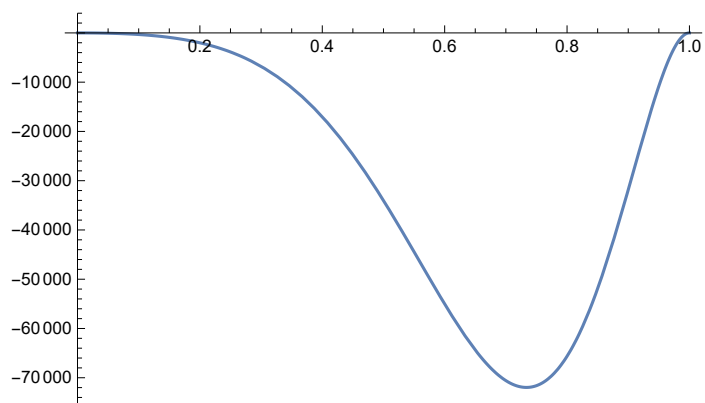

**Plot[Cf[4, 6, 13], {x, 0, 1}]**

[绘图](#)

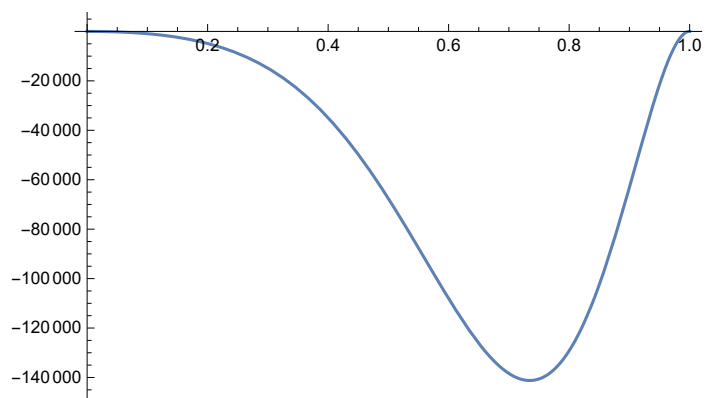

**Plot[Cf[4, 6, 12], {x, 0, 1}]**

[绘图](#)

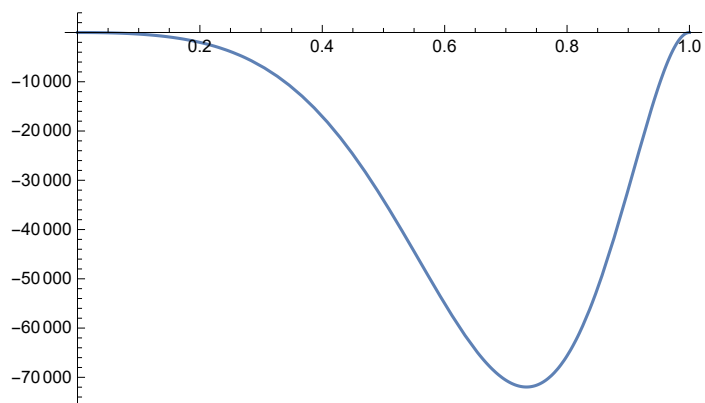

**Plot[Cf[4, 6, 11], {x, 0, 1}]**

[绘图](#)

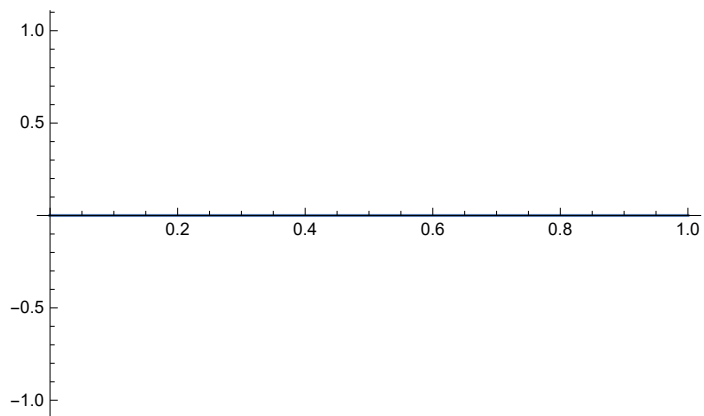

**(\*160th group coefficients r2^4r3^5\*)**

**Plot[Cf[4, 5, 14], {x, 0, 1}]**

[绘图](#)

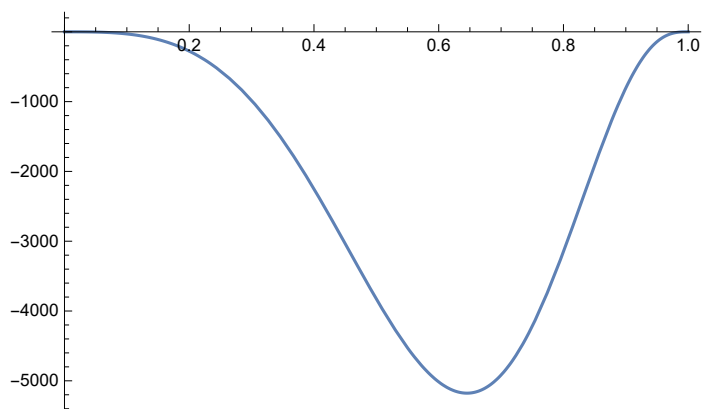

**Plot[Cf[4, 5, 13], {x, 0, 1}]**

[绘图](#)

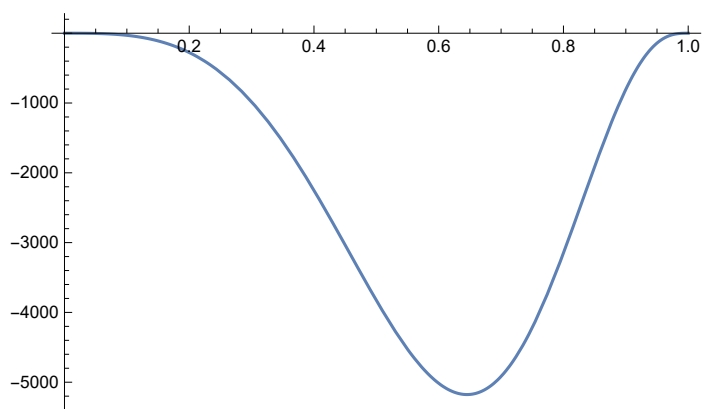

**Plot[Cf[4, 5, 12], {x, 0, 1}]**

[绘图](#)

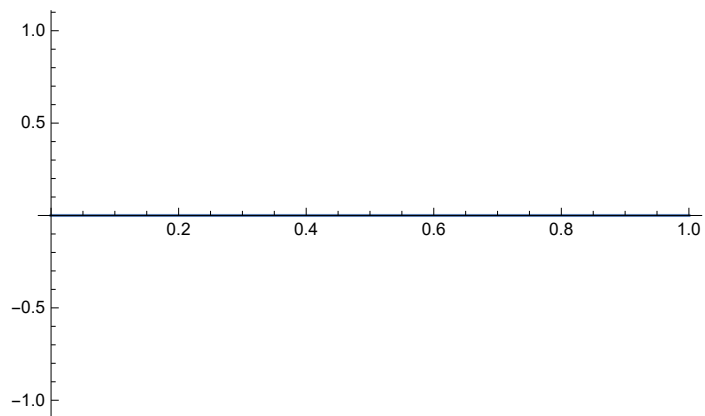

(\*161th group coefficients r2^4r3^4\*)

**Plot[Cf[4, 4, 14], {x, 0, 1}]**

[绘图](#)

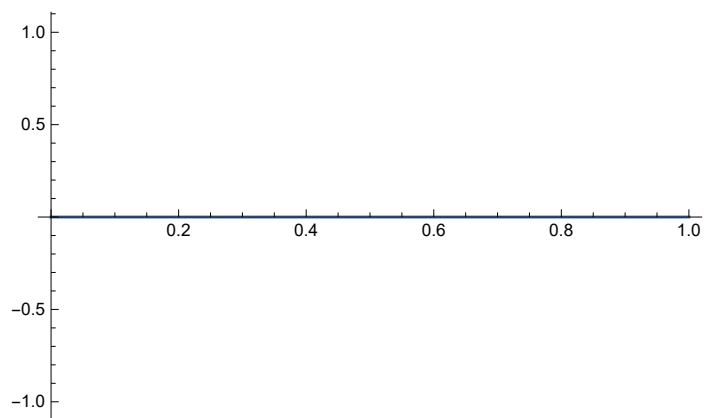

(\*162th group coefficients r2^4r3^3\*)

**Plot[Cf[4, 3, 14], {x, 0, 1}]**

[绘图](#)

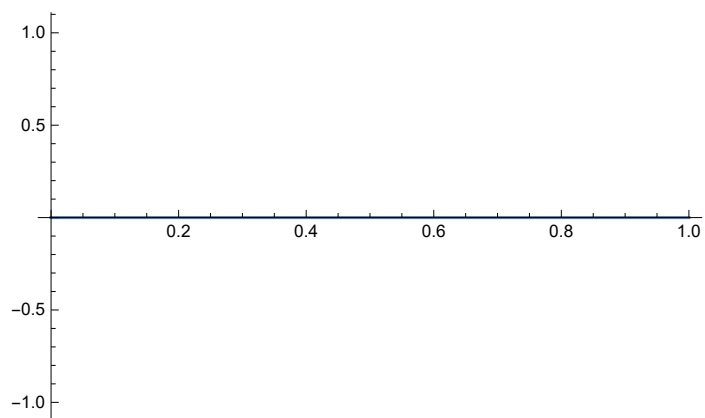

(\*163th group coefficients r2^4r3^2\*)



**Plot[Cf[4, 2, 14], {x, 0, 1}]**

[绘图](#)

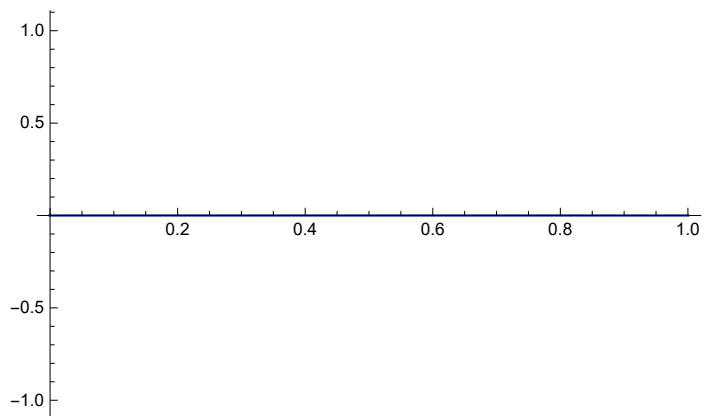

(\*164th group coefficients r2^4r3^1\*)

**Plot[Cf[4, 1, 14], {x, 0, 1}]**

[绘图](#)

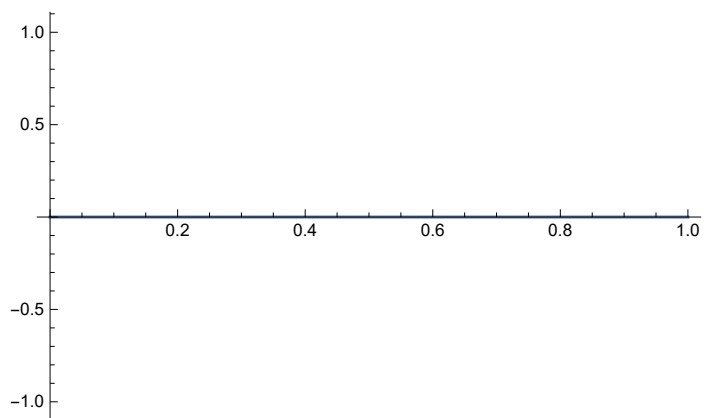

(\*165th group coefficients r2^4r3^0\*)

**Plot[Cf[4, 0, 14], {x, 0, 1}]**

[绘图](#)

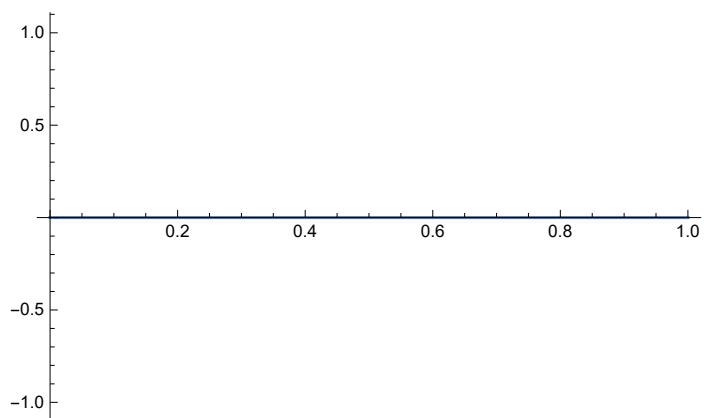

(\*166th group coefficients r2^3r3^14\*)

**Plot[Cf[3, 14, 14], {x, 0, 1}]**

[绘图](#)

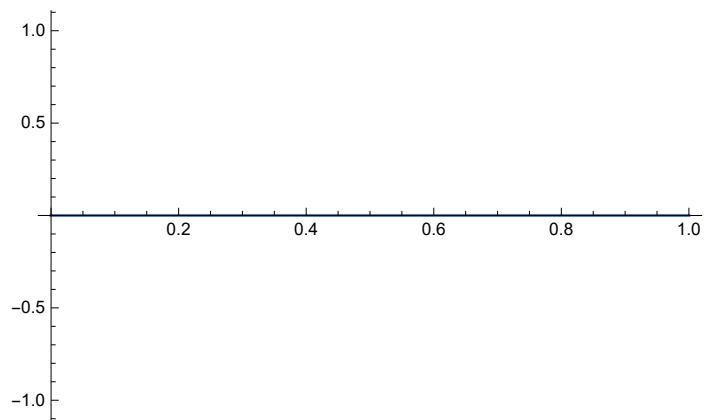

**Plot[Cf[3, 14, 13], {x, 0, 1}]**

[绘图](#)

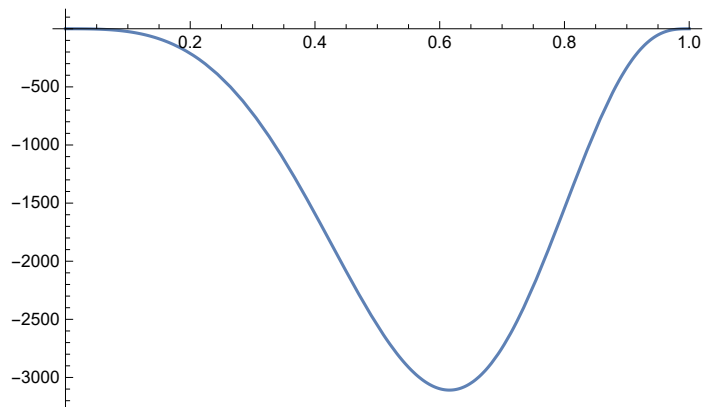

**Plot[Cf[3, 14, 12], {x, 0, 1}]**

[绘图](#)

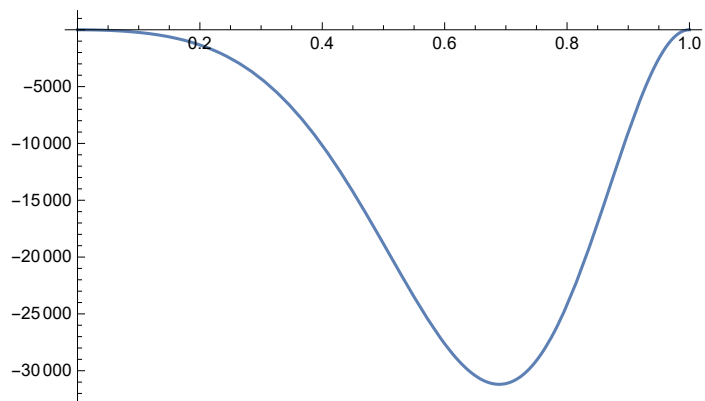

```
Plot[Cf[3, 14, 11], {x, 0, 1}]
```

[绘图](#)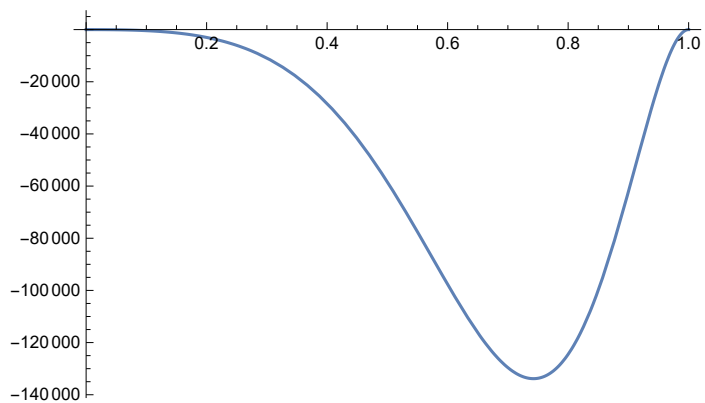

```
Plot[Cf[3, 14, 10], {x, 0, 1}]
```

[绘图](#)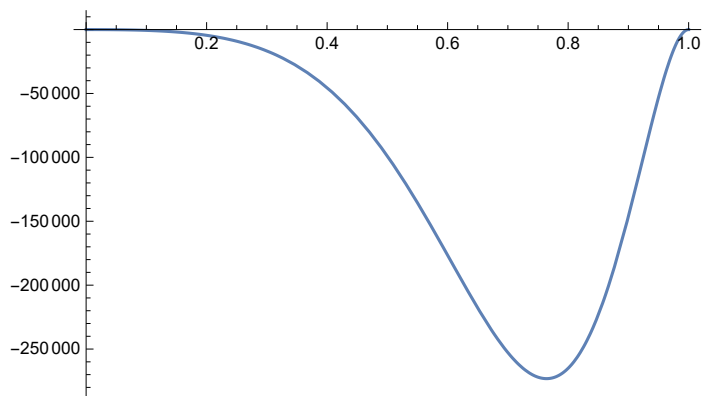

```
Plot[Cf[3, 14, 9], {x, 0, 1}]
```

[绘图](#)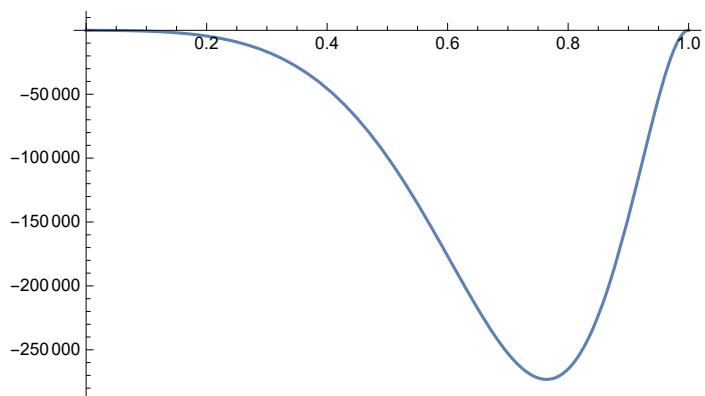

```
Plot[Cf[3, 14, 8], {x, 0, 1}]
```

[绘图](#)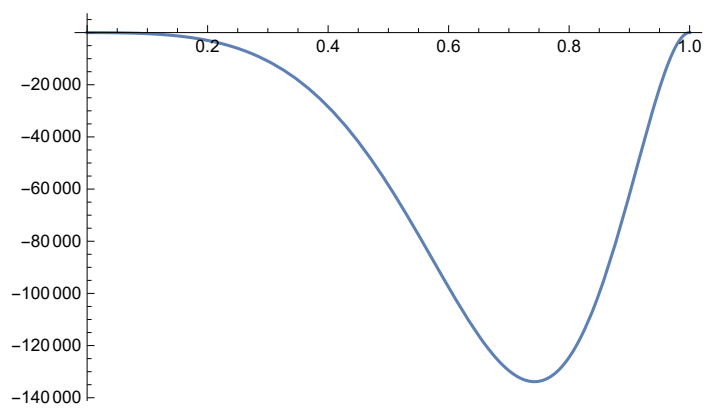

```
Plot[Cf[3, 14, 7], {x, 0, 1}]
```

[绘图](#)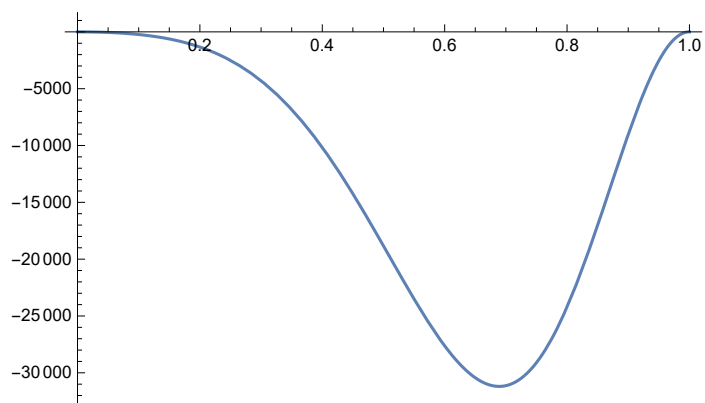

```
Plot[Cf[3, 14, 6], {x, 0, 1}]
```

[绘图](#)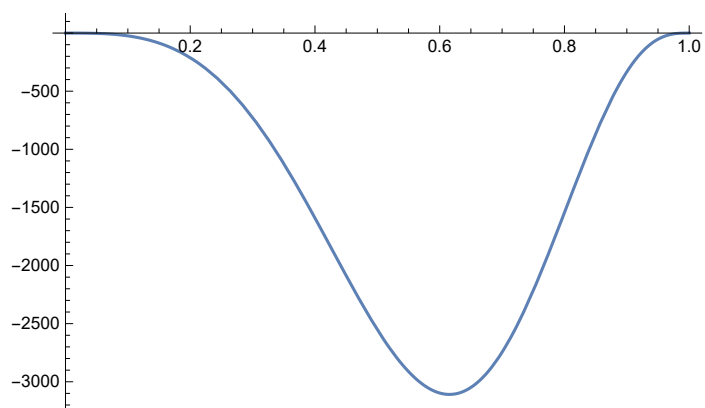

**Plot[Cf[3, 14, 5], {x, 0, 1}]**

[绘图](#)

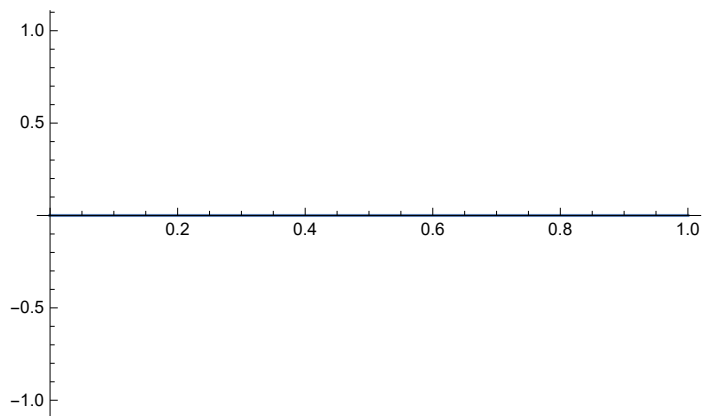

**(\*167th group coefficients r2^3r3^13\*)**

**Plot[Cf[3, 13, 14], {x, 0, 1}]**

[绘图](#)

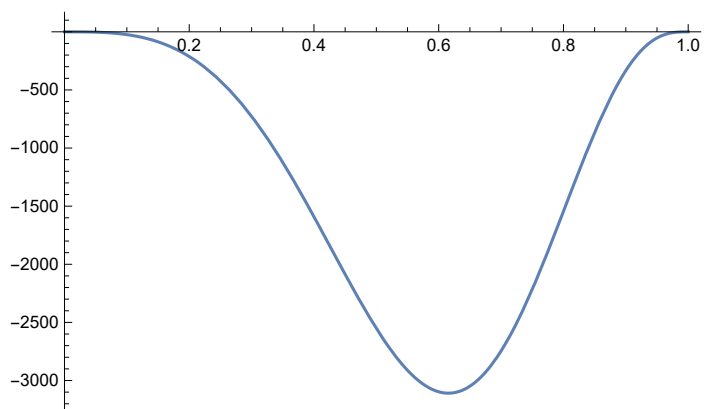

**Plot[Cf[3, 13, 13], {x, 0, 1}]**

[绘图](#)

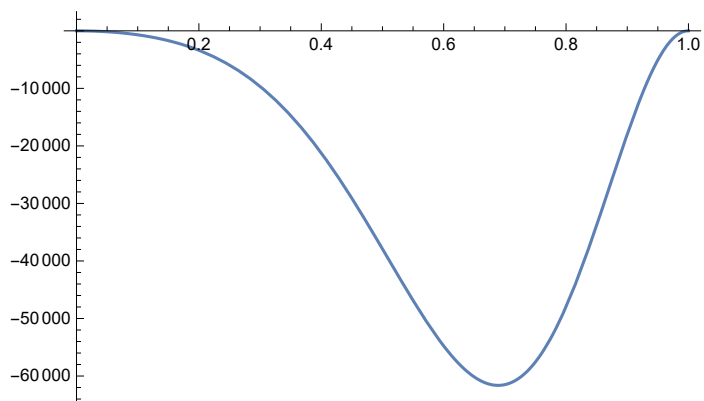

```
Plot[Cf[3, 13, 12], {x, 0, 1}]
```

[绘图](#)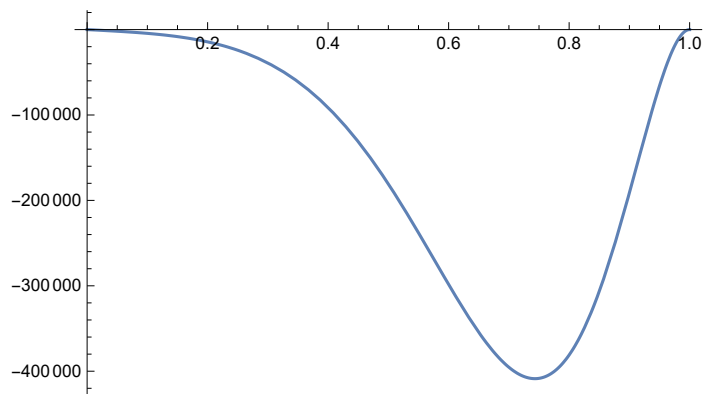

```
Plot[Cf[3, 13, 11], {x, 0, 1}]
```

[绘图](#)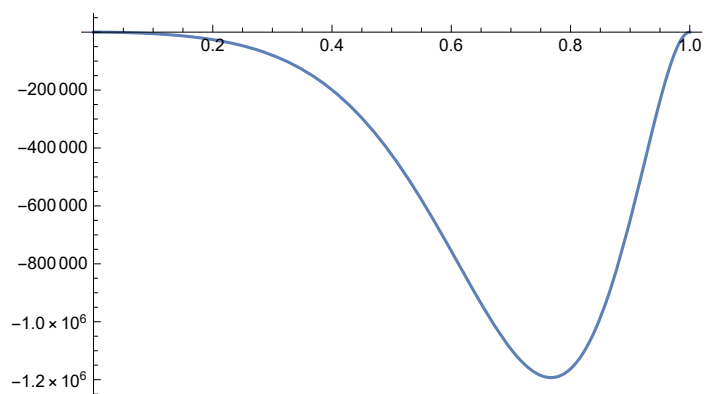

```
Plot[Cf[3, 13, 10], {x, 0, 1}]
```

[绘图](#)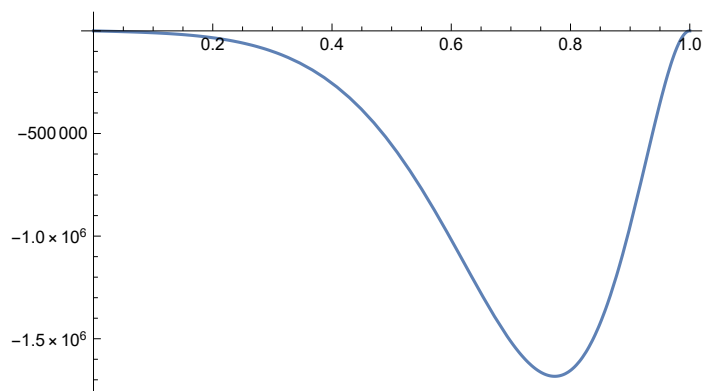

**Plot[Cf[3, 13, 9], {x, 0, 1}]**

[绘图](#)

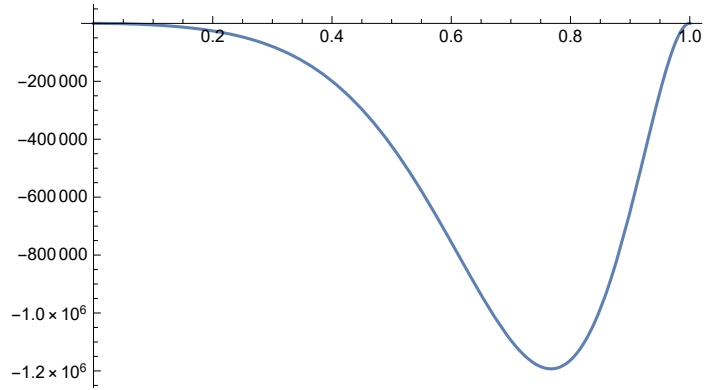

**Plot[Cf[3, 13, 8], {x, 0, 1}]**

[绘图](#)

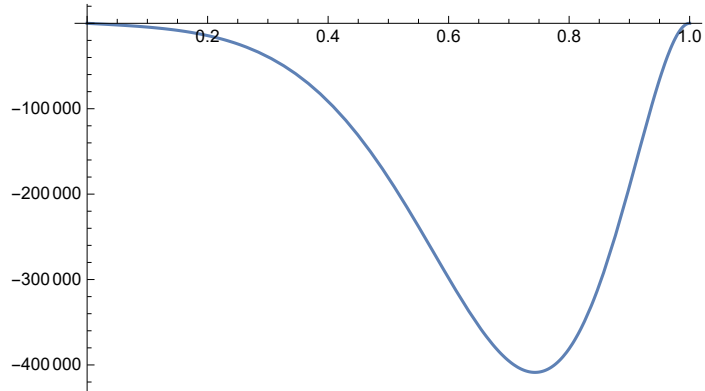

**Plot[Cf[3, 13, 7], {x, 0, 1}]**

[绘图](#)

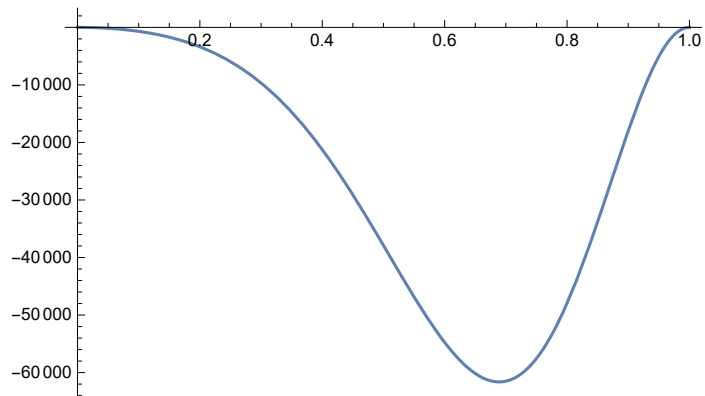

**Plot[Cf[3, 13, 6], {x, 0, 1}]**

[绘图](#)

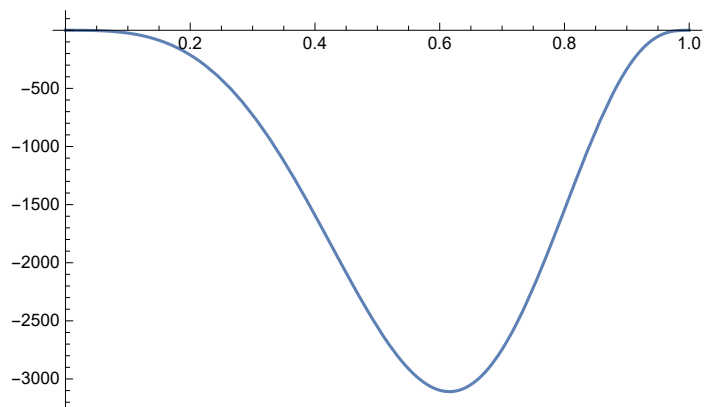

**Plot[Cf[3, 13, 5], {x, 0, 1}]**

[绘图](#)

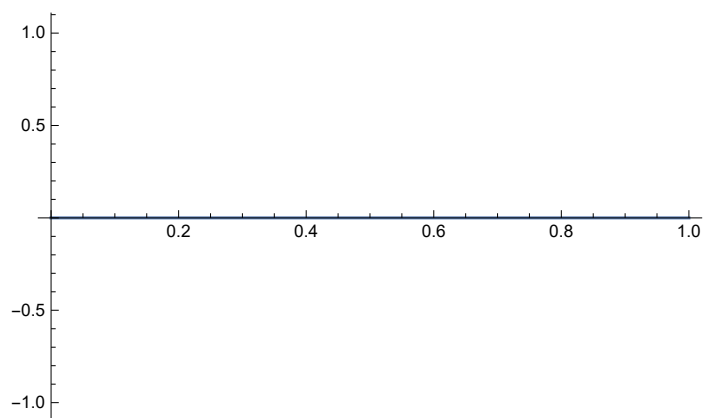

**(\*168th group coefficients r2^3r3^12\*)**

**Plot[Cf[3, 12, 14], {x, 0, 1}]**

[绘图](#)

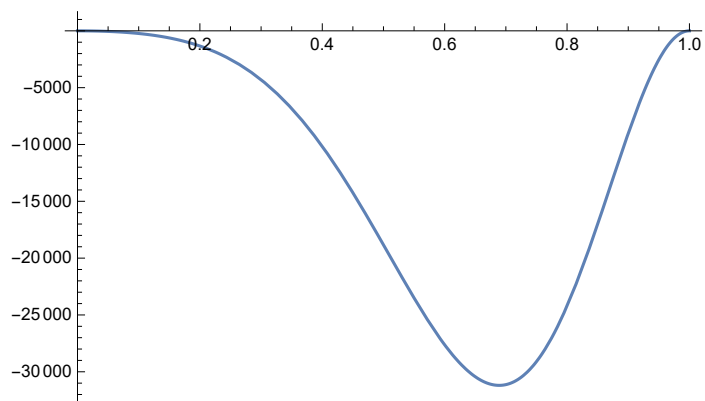



```
Plot[Cf[3, 12, 13], {x, 0, 1}]
```

[绘图](#)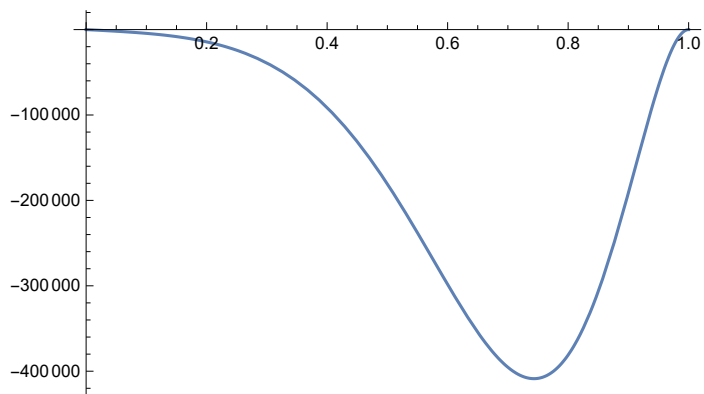

```
Plot[Cf[3, 12, 12], {x, 0, 1}]
```

[绘图](#)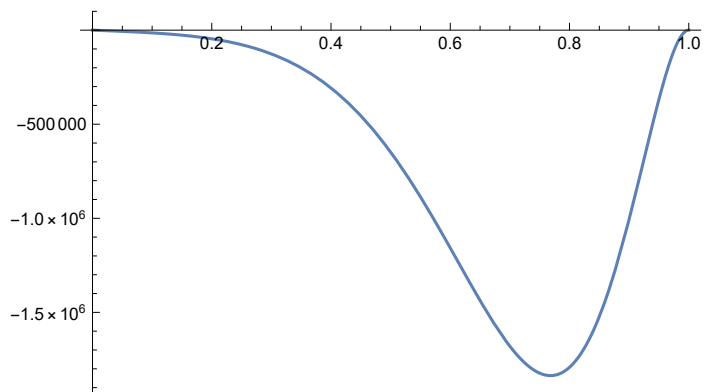

```
Plot[Cf[3, 12, 11], {x, 0, 1}]
```

[绘图](#)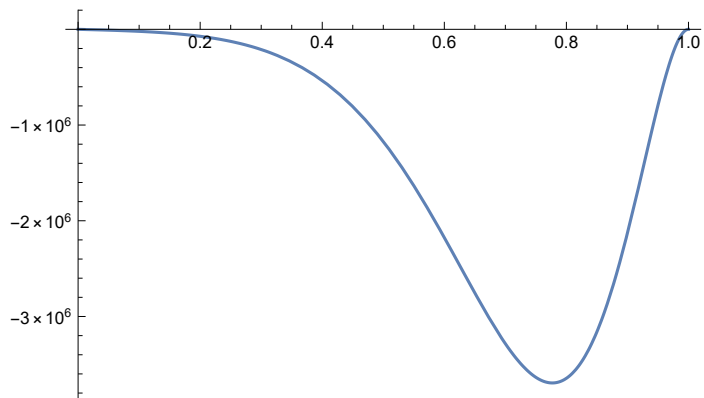

```
Plot[Cf[3, 12, 10], {x, 0, 1}]
```

[绘图](#)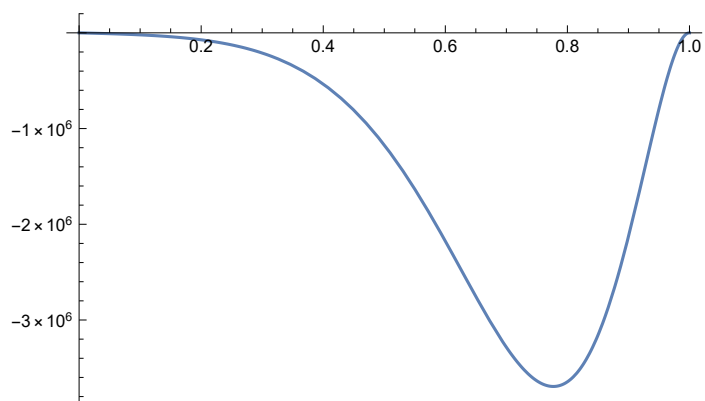

```
Plot[Cf[3, 12, 9], {x, 0, 1}]
```

[绘图](#)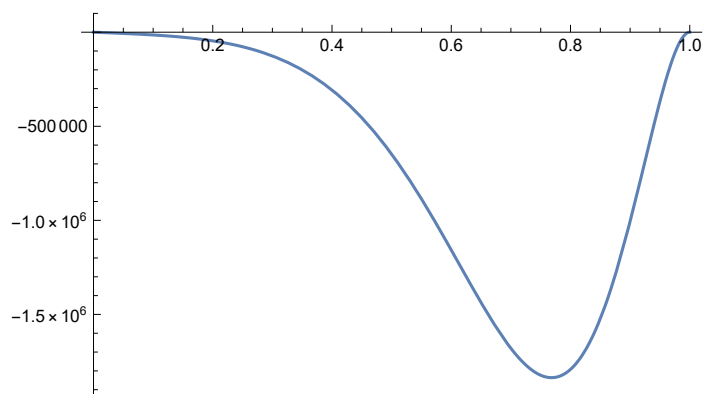

```
Plot[Cf[3, 12, 8], {x, 0, 1}]
```

[绘图](#)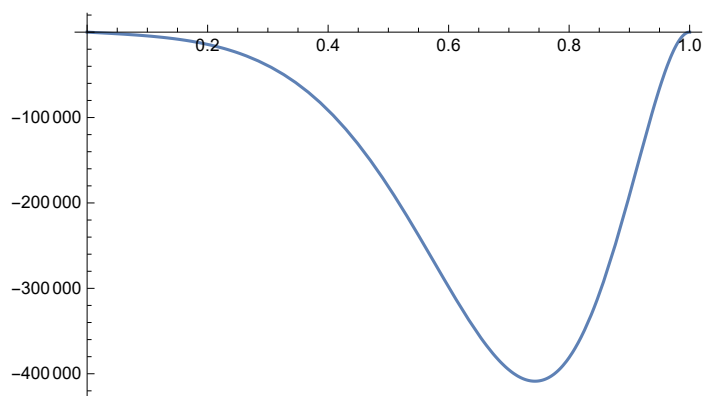

**Plot[Cf[3, 12, 7], {x, 0, 1}]**

[绘图](#)

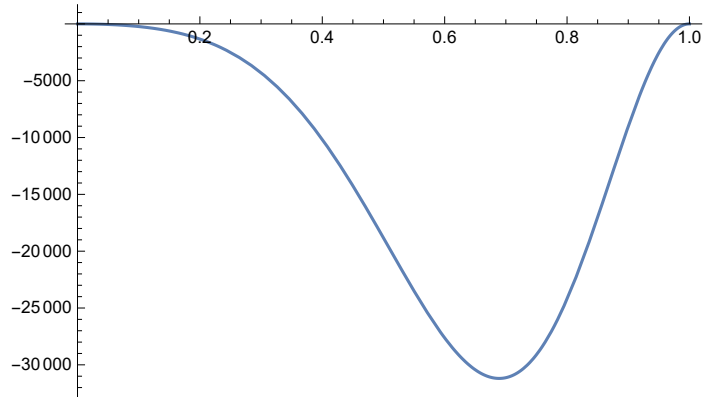

**Plot[Cf[3, 12, 6], {x, 0, 1}]**

[绘图](#)

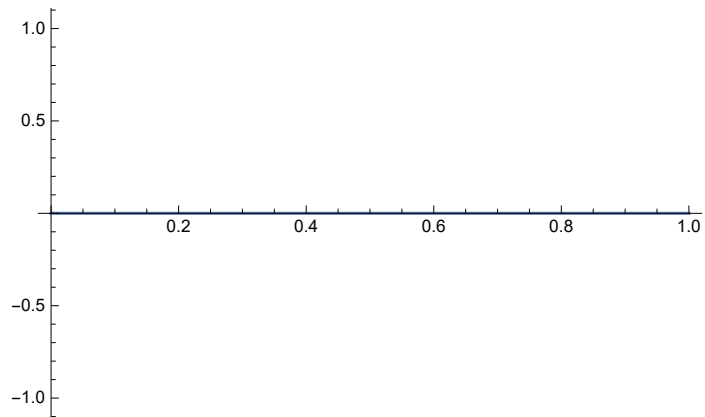

**(\*169th group coefficients r2^3r3^11\*)**

**Plot[Cf[3, 11, 14], {x, 0, 1}]**

[绘图](#)

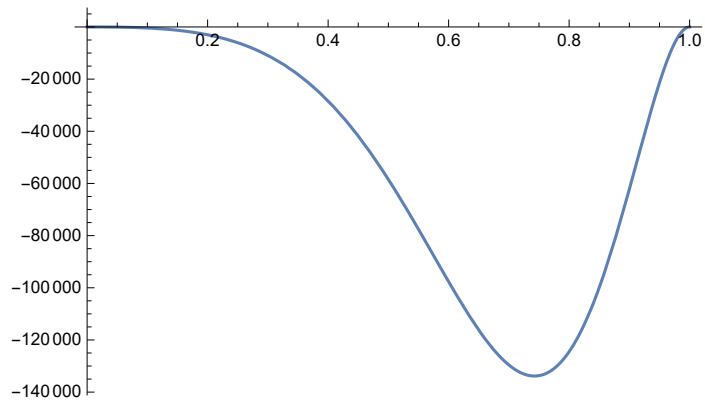

```
Plot[Cf[3, 11, 13], {x, 0, 1}]
```

[绘图](#)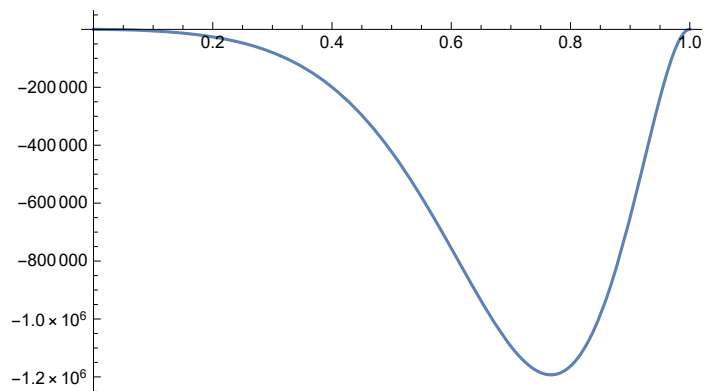

```
Plot[Cf[3, 11, 12], {x, 0, 1}]
```

[绘图](#)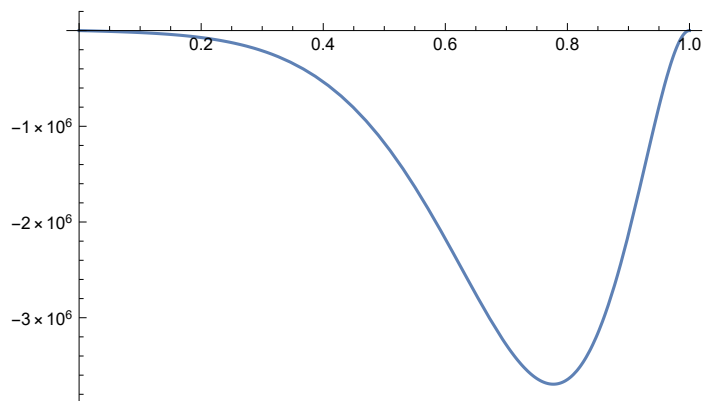

```
Plot[Cf[3, 11, 11], {x, 0, 1}]
```

[绘图](#)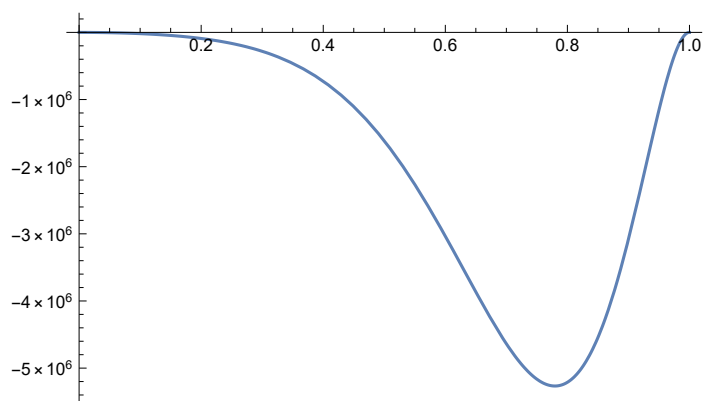

```
Plot[Cf[3, 11, 10], {x, 0, 1}]
```

[绘图](#)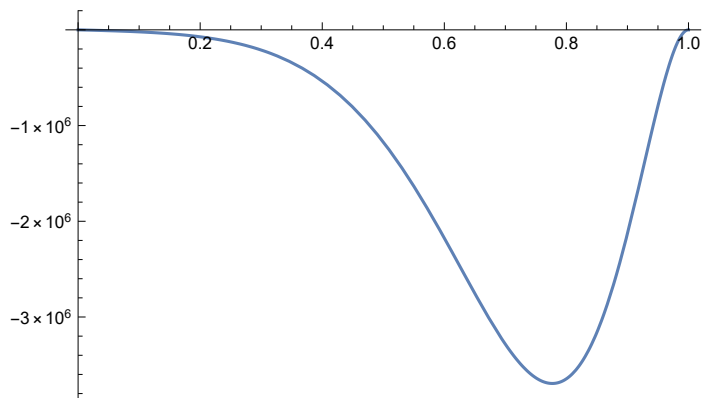

```
Plot[Cf[3, 11, 9], {x, 0, 1}]
```

[绘图](#)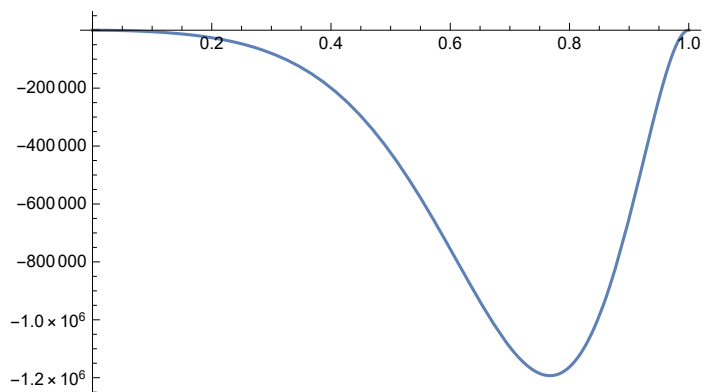

```
Plot[Cf[3, 11, 8], {x, 0, 1}]
```

[绘图](#)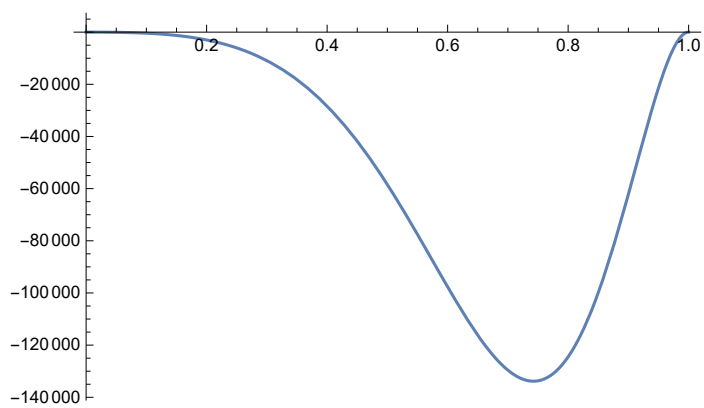

**Plot[Cf[3, 11, 7], {x, 0, 1}]**

[绘图](#)

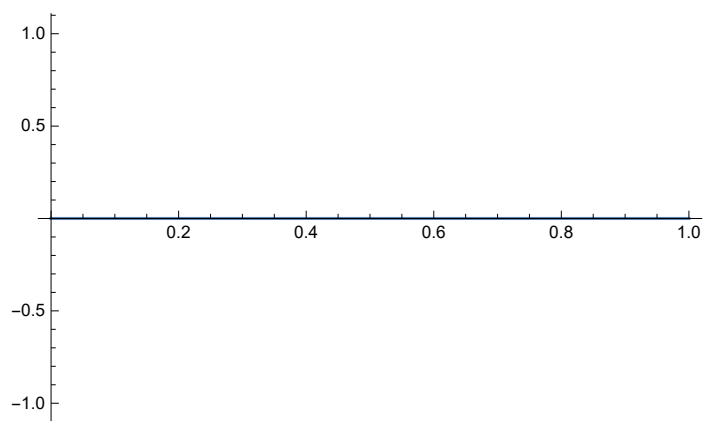

**(\*170th group coefficients r2^3r3^10\*)**

**Plot[Cf[3, 10, 14], {x, 0, 1}]**

[绘图](#)

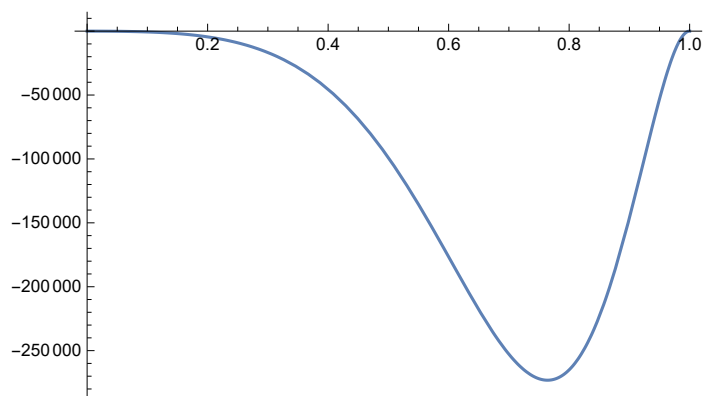

**Plot[Cf[3, 10, 13], {x, 0, 1}]**

[绘图](#)

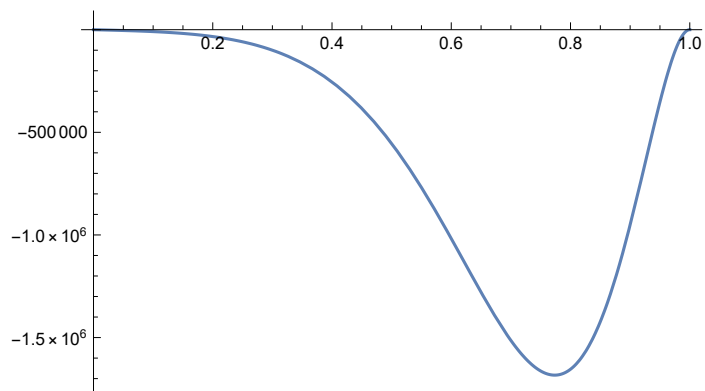

```
Plot[Cf[3, 10, 12], {x, 0, 1}]
```

[绘图](#)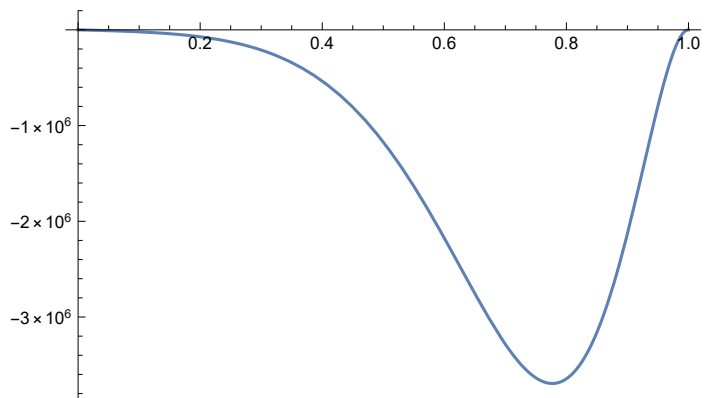

```
Plot[Cf[3, 10, 11], {x, 0, 1}]
```

[绘图](#)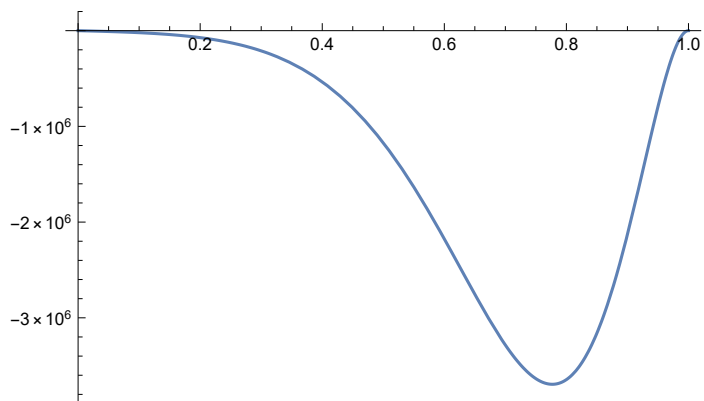

```
Plot[Cf[3, 10, 10], {x, 0, 1}]
```

[绘图](#)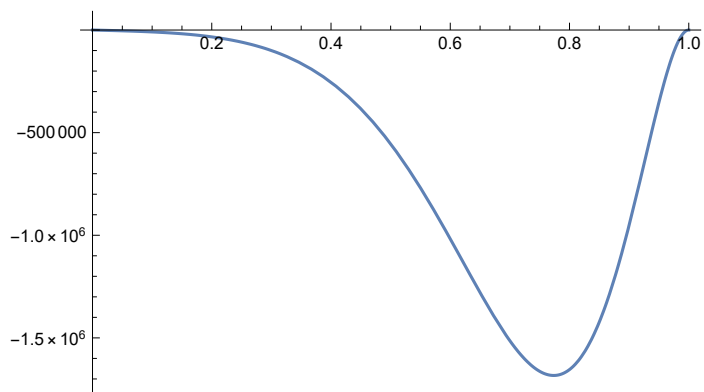

**Plot[Cf[3, 10, 9], {x, 0, 1}]**

[绘图](#)

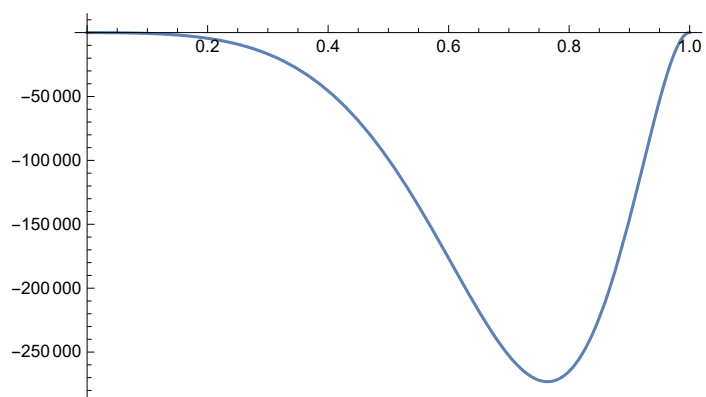

**Plot[Cf[3, 10, 8], {x, 0, 1}]**

[绘图](#)

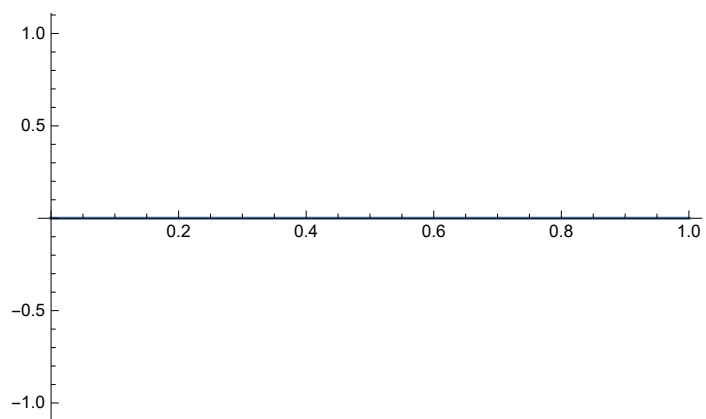

**(\*171th group coefficients r2^3r3^9\*)**

**Plot[Cf[3, 9, 14], {x, 0, 1}]**

[绘图](#)

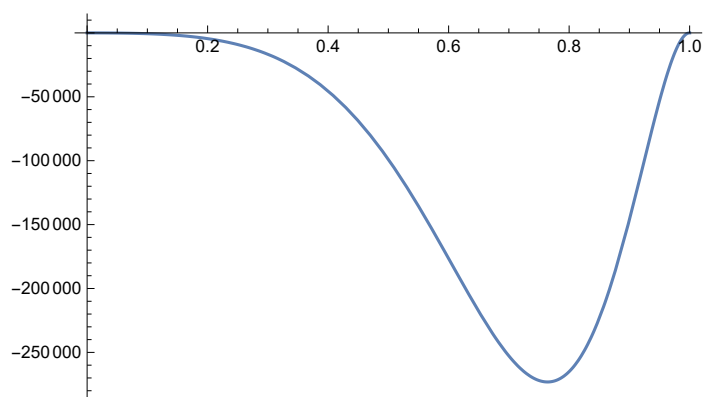



```
Plot[Cf[3, 9, 13], {x, 0, 1}]
```

[绘图](#)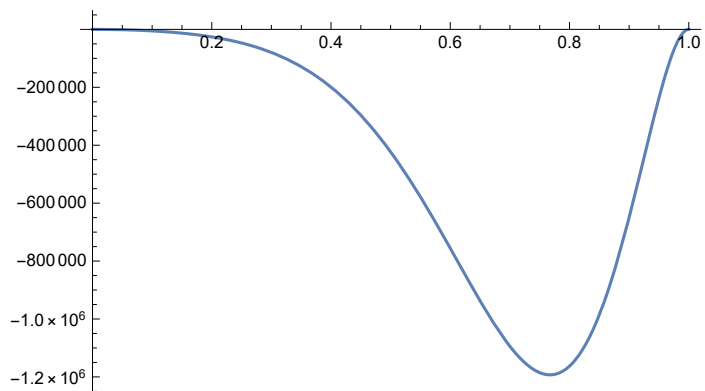

```
Plot[Cf[3, 9, 12], {x, 0, 1}]
```

[绘图](#)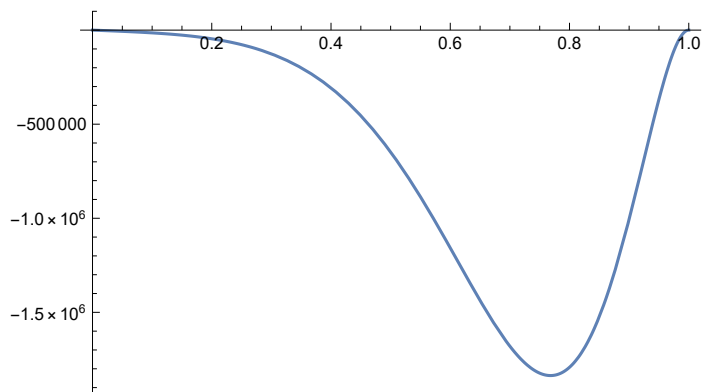

```
Plot[Cf[3, 9, 11], {x, 0, 1}]
```

[绘图](#)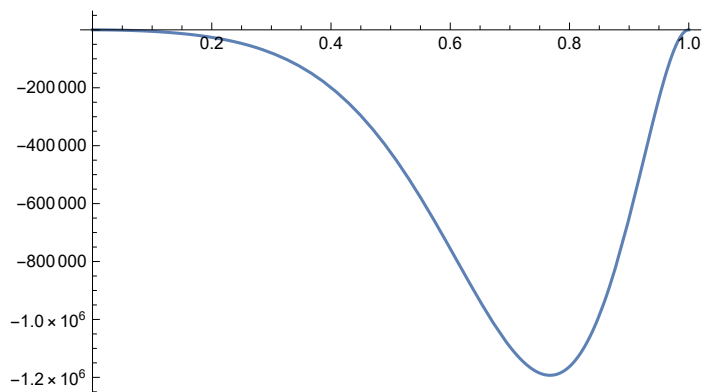

**Plot[Cf[3, 9, 10], {x, 0, 1}]**

[绘图](#)

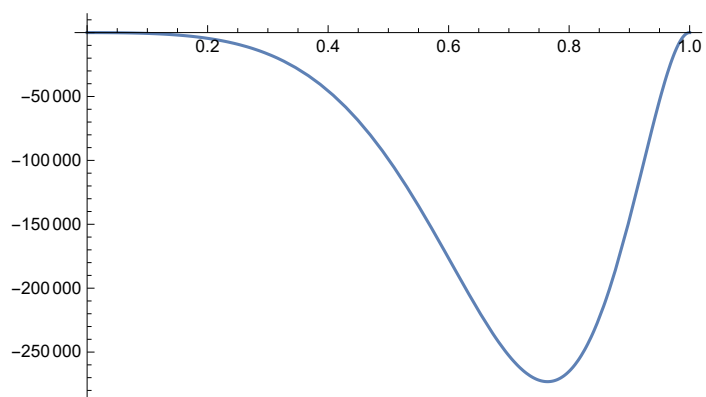

**Plot[Cf[3, 9, 9], {x, 0, 1}]**

[绘图](#)

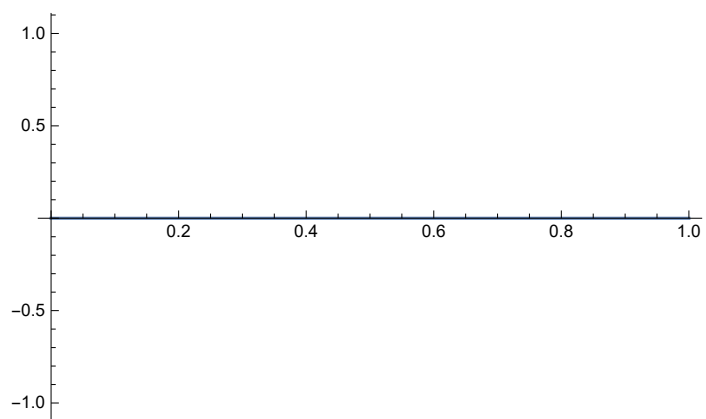

**(\*172th group coefficients r2^3r3^8\*)**

**Plot[Cf[3, 8, 14], {x, 0, 1}]**

[绘图](#)

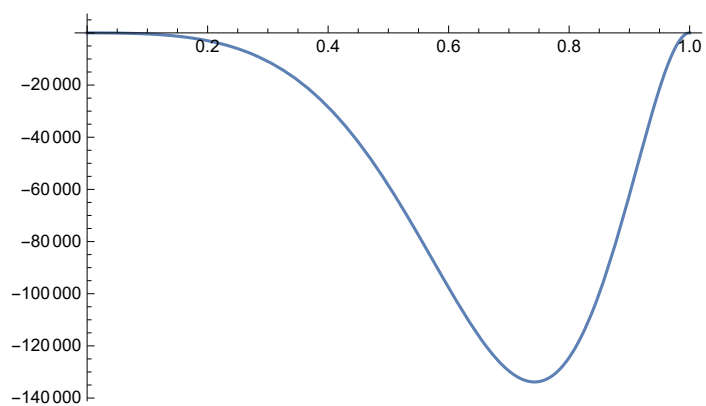

**Plot[Cf[3, 8, 13], {x, 0, 1}]**

[绘图](#)

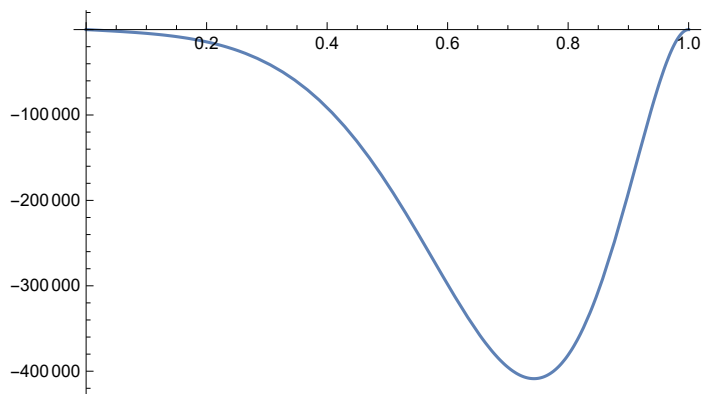

**Plot[Cf[3, 8, 12], {x, 0, 1}]**

[绘图](#)

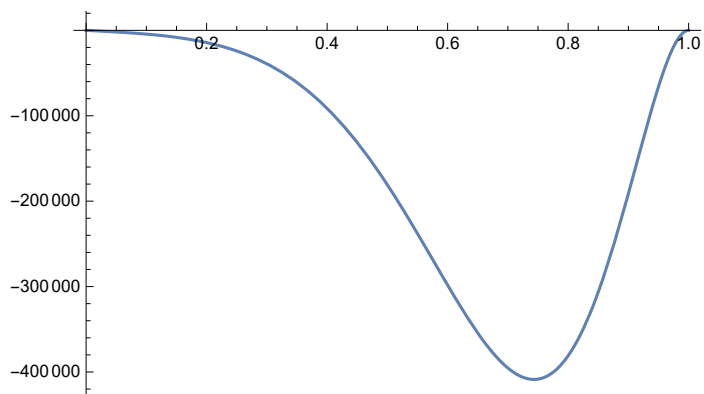

**Plot[Cf[3, 8, 11], {x, 0, 1}]**

[绘图](#)

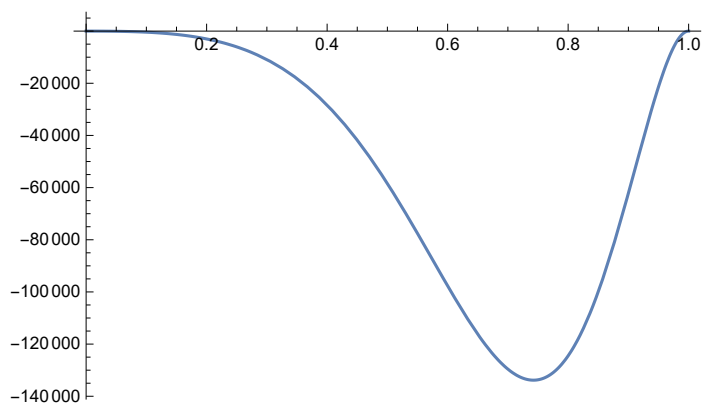

`Plot[Cf[3, 8, 10], {x, 0, 1}]`

[绘图](#)

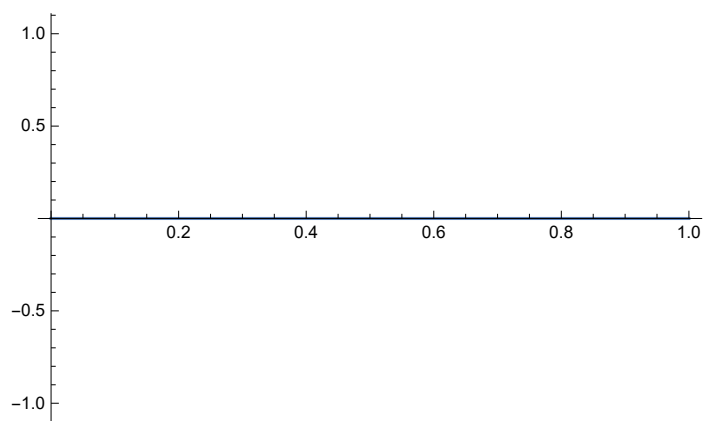

`Plot[Cf[3, 8, 9], {x, 0, 1}]`

[绘图](#)

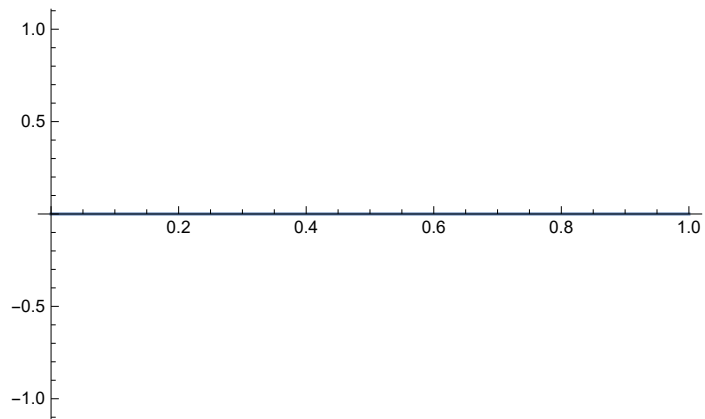

(\*173th group coefficients r2^3r3^7\*)

`Plot[Cf[3, 7, 14], {x, 0, 1}]`

[绘图](#)

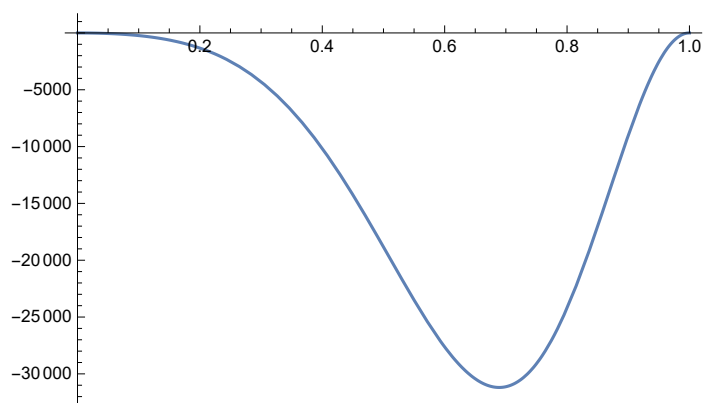

**Plot[Cf[3, 7, 13], {x, 0, 1}]**

[绘图](#)

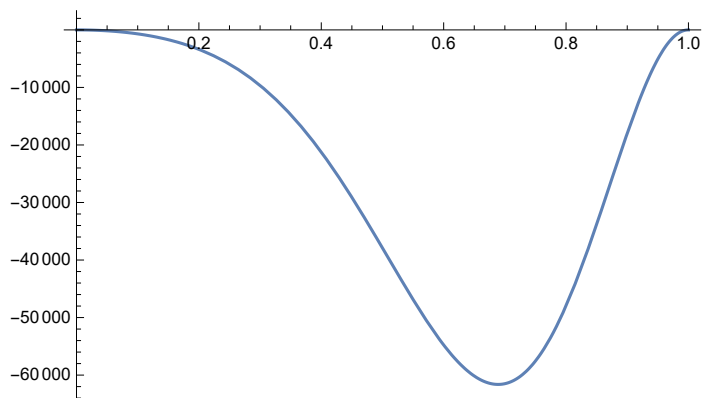

**Plot[Cf[3, 7, 12], {x, 0, 1}]**

[绘图](#)

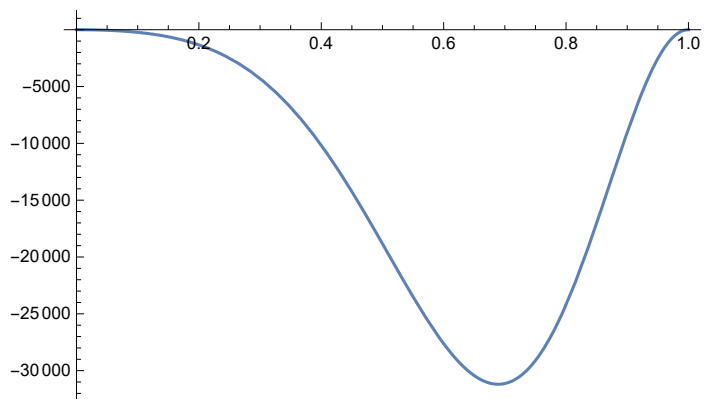

**Plot[Cf[3, 7, 11], {x, 0, 1}]**

[绘图](#)

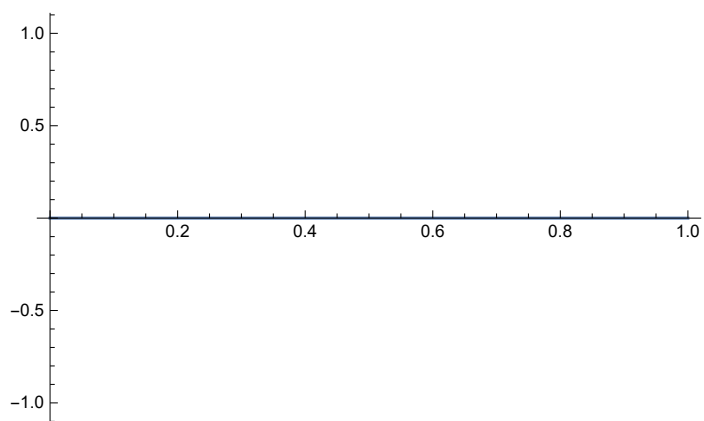

(\*174th group coefficients r2^3r3^6\*)

**Plot[Cf[3, 6, 14], {x, 0, 1}]**

[绘图](#)

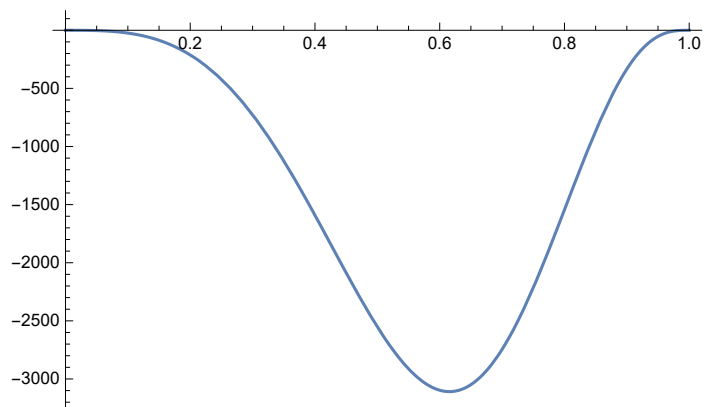

**Plot[Cf[3, 6, 13], {x, 0, 1}]**

[绘图](#)

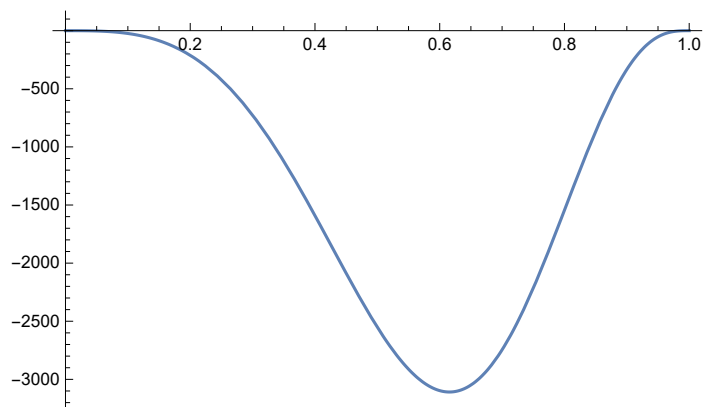

**Plot[Cf[3, 6, 12], {x, 0, 1}]**

[绘图](#)

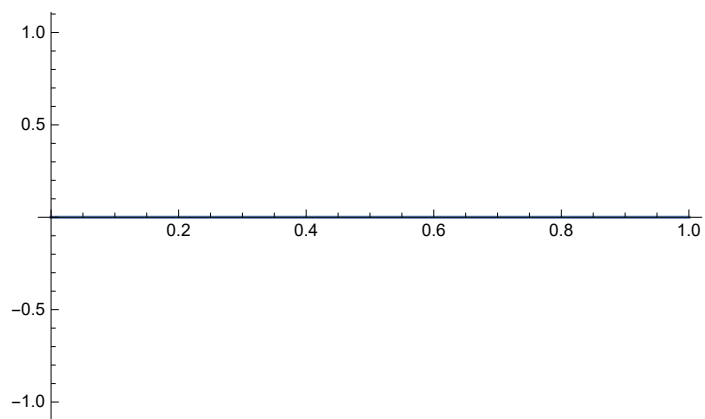

**(\*175th group coefficients r2^3r3^5\*)**

**Plot[Cf[3, 5, 14], {x, 0, 1}]**

[绘图](#)

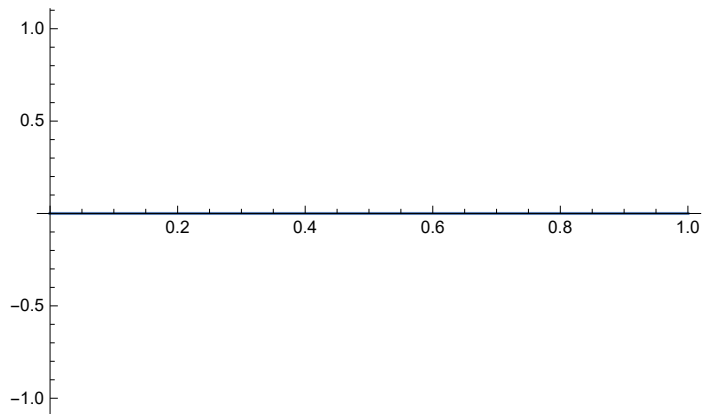

(\*176th group coefficients r2^3r3^4\*)

**Plot[Cf[3, 4, 14], {x, 0, 1}]**

[绘图](#)

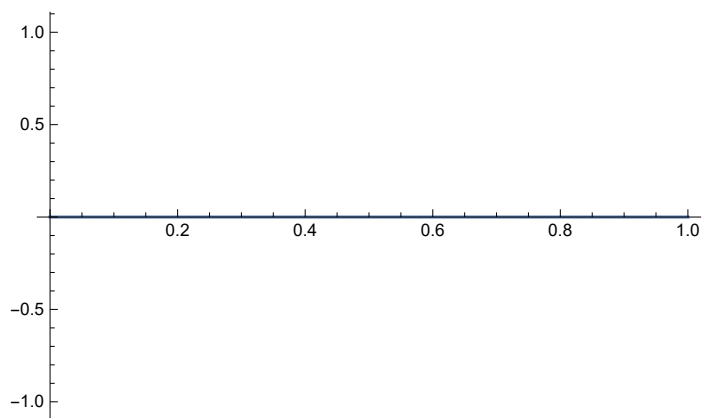

(\*177th group coefficients r2^3r3^3\*)

**Plot[Cf[3, 3, 14], {x, 0, 1}]**

[绘图](#)

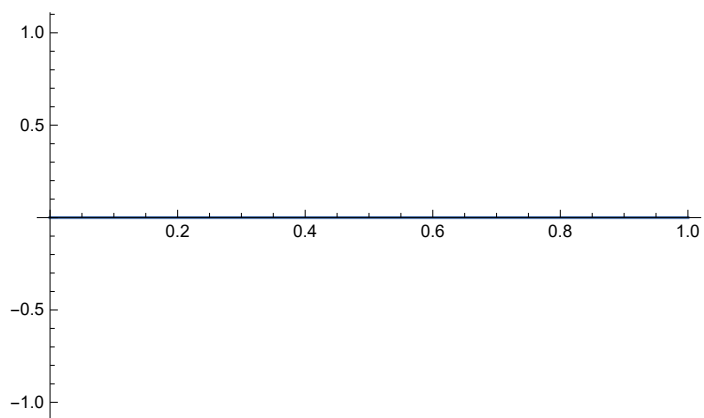

(\*178th group coefficients r2^3r3^2\*)

**Plot[Cf[3, 2, 14], {x, 0, 1}]**

[绘图](#)

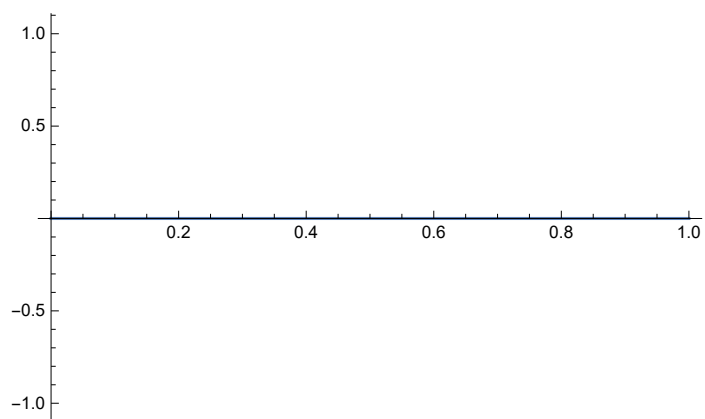

(\*179th group coefficients r2^3r3^1\*)

**Plot[Cf[3, 1, 14], {x, 0, 1}]**

[绘图](#)

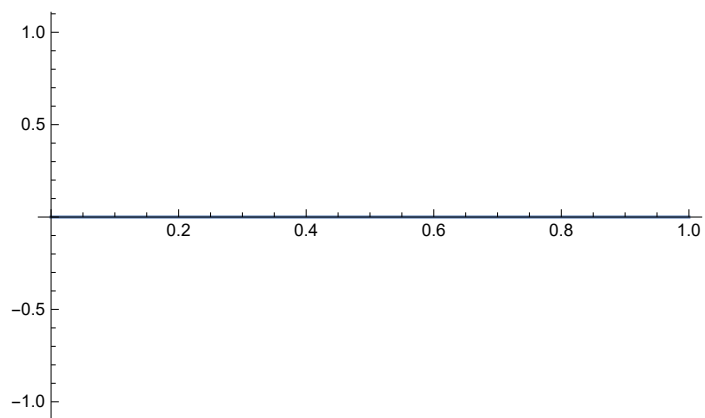

(\*180th group coefficients r2^3r3^0\*)

**Plot[Cf[3, 0, 14], {x, 0, 1}]**

[绘图](#)

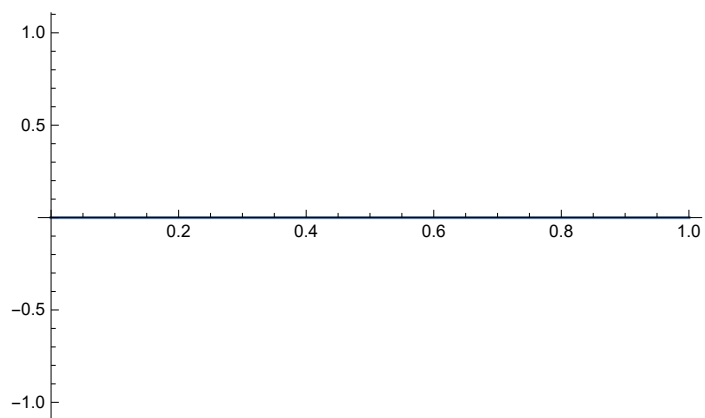

(\*181th group coefficients r2^2r3^14\*)



**Plot[Cf[2, 14, 14], {x, 0, 1}]**

[绘图](#)

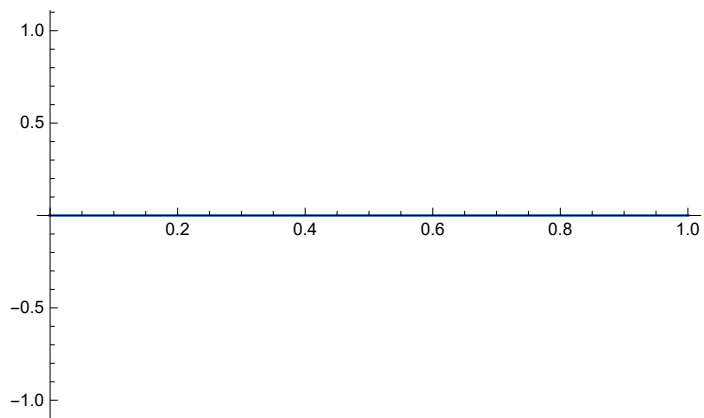

**Plot[Cf[2, 14, 13], {x, 0, 1}]**

[绘图](#)

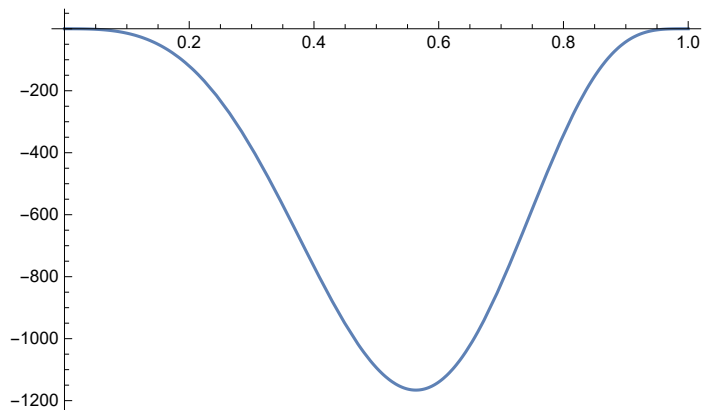

**Plot[Cf[2, 14, 12], {x, 0, 1}]**

[绘图](#)

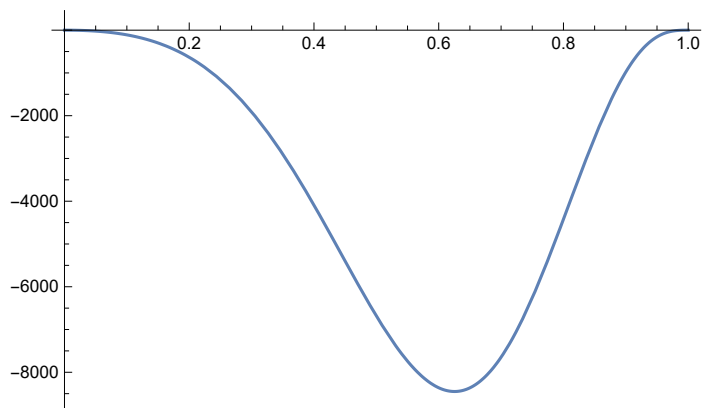

```
Plot[Cf[2, 14, 11], {x, 0, 1}]
```

[绘图](#)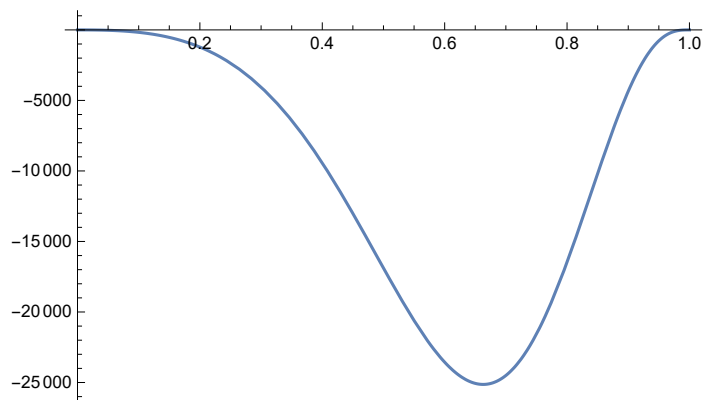

```
Plot[Cf[2, 14, 10], {x, 0, 1}]
```

[绘图](#)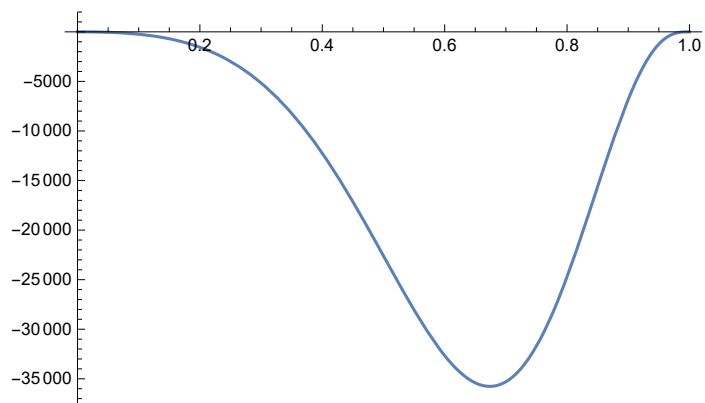

```
Plot[Cf[2, 14, 9], {x, 0, 1}]
```

[绘图](#)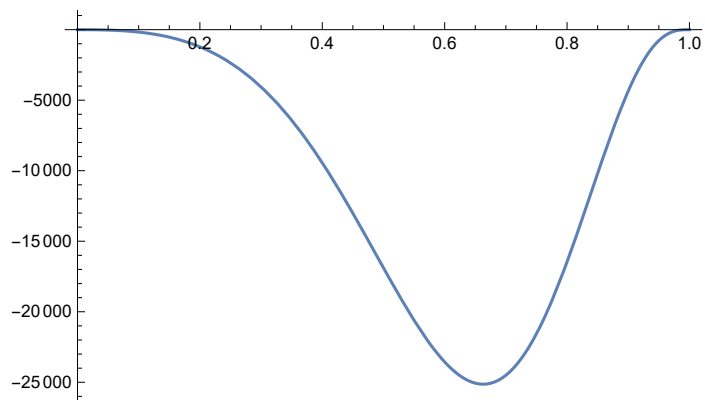

**Plot[Cf[2, 14, 8], {x, 0, 1}]**

[绘图](#)

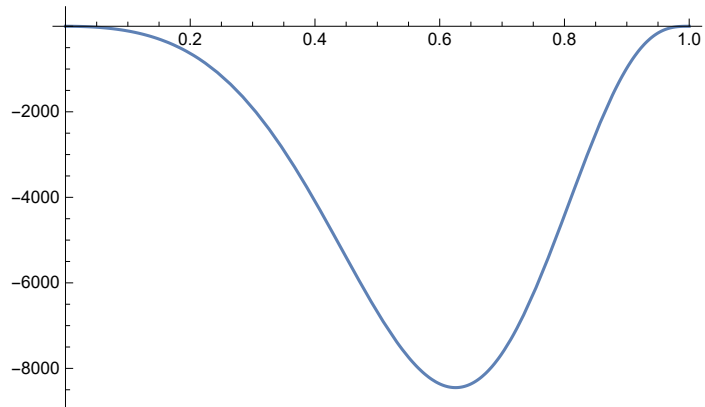

**Plot[Cf[2, 14, 7], {x, 0, 1}]**

[绘图](#)

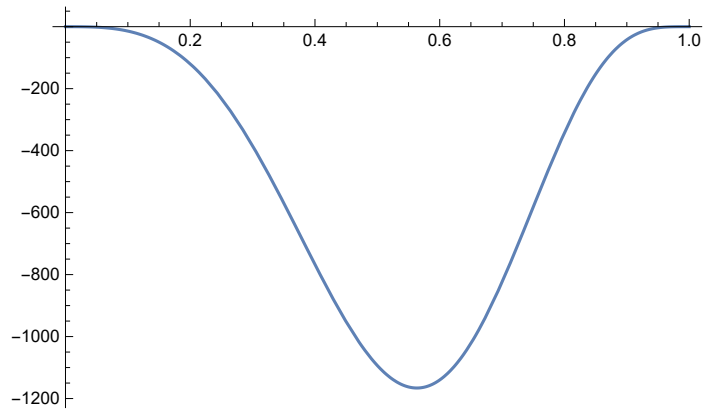

**Plot[Cf[2, 14, 6], {x, 0, 1}]**

[绘图](#)

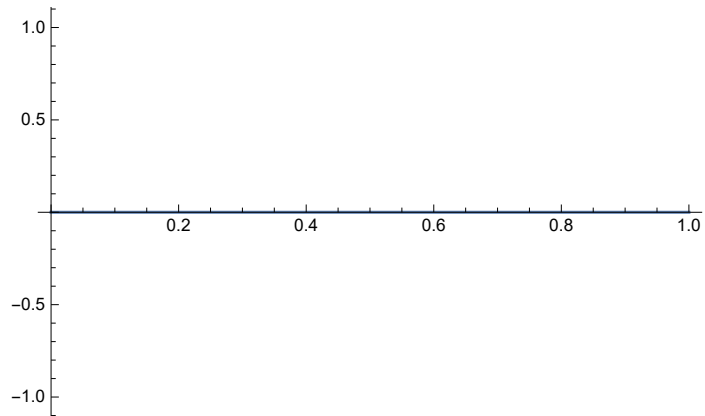

**(\*182th group coefficients r2^2r3^13\*)**

```
Plot[Cf[2, 13, 14], {x, 0, 1}]
```

[绘图](#)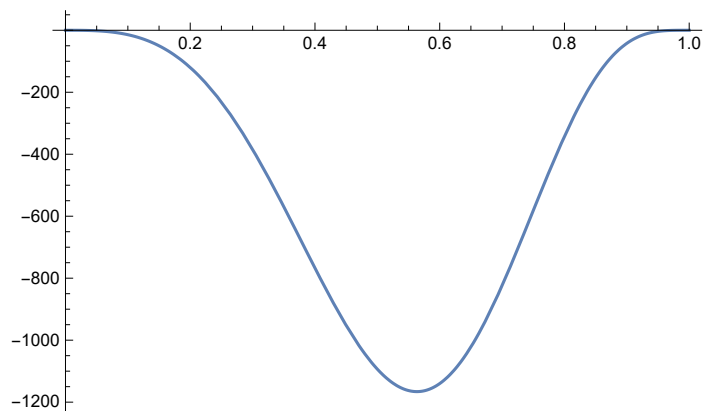

```
Plot[Cf[2, 13, 13], {x, 0, 1}]
```

[绘图](#)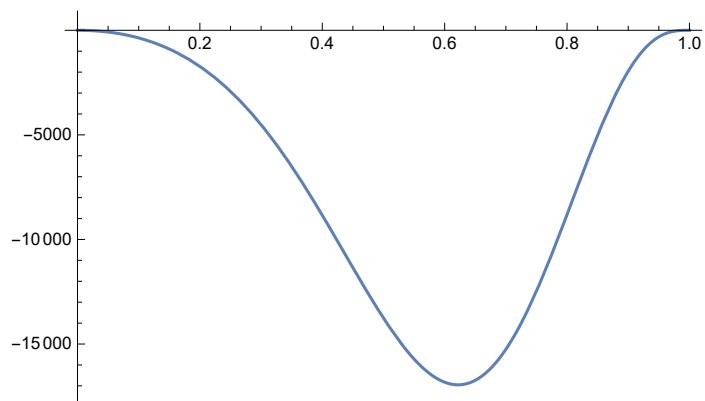

```
Plot[Cf[2, 13, 12], {x, 0, 1}]
```

[绘图](#)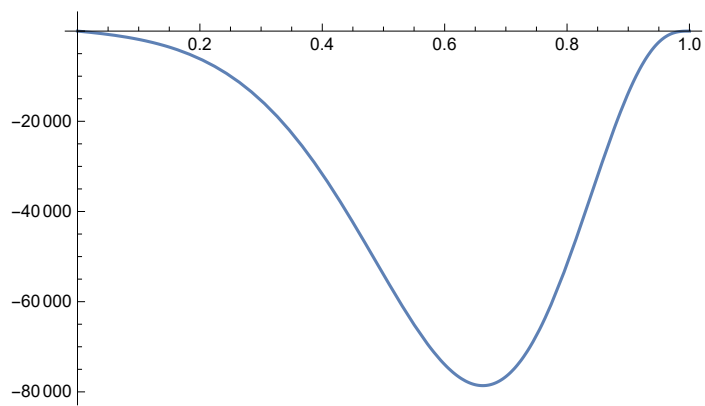

**Plot[Cf[2, 13, 11], {x, 0, 1}]**

[绘图](#)

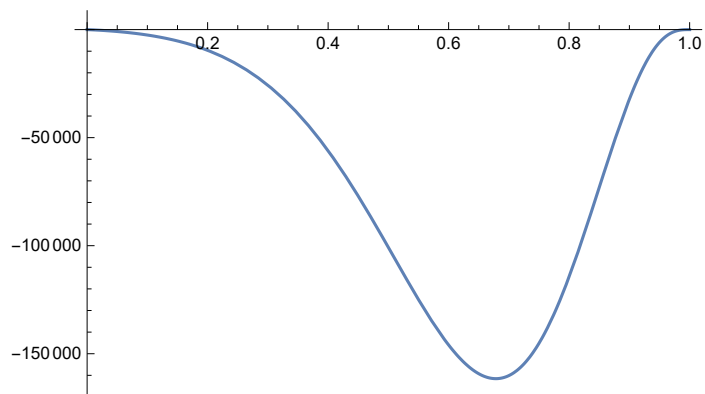

**Plot[Cf[2, 13, 10], {x, 0, 1}]**

[绘图](#)

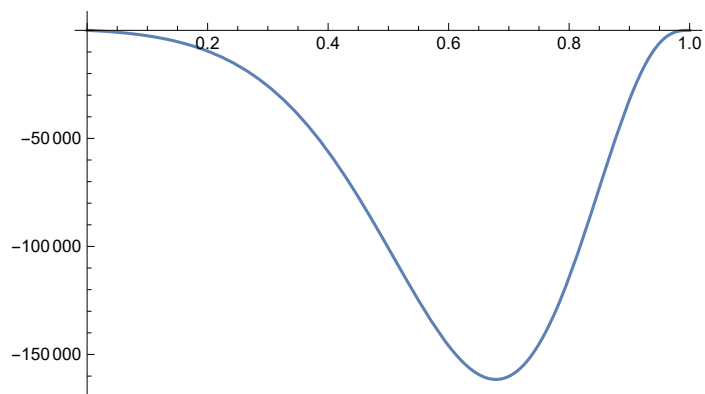

**Plot[Cf[2, 13, 9], {x, 0, 1}]**

[绘图](#)

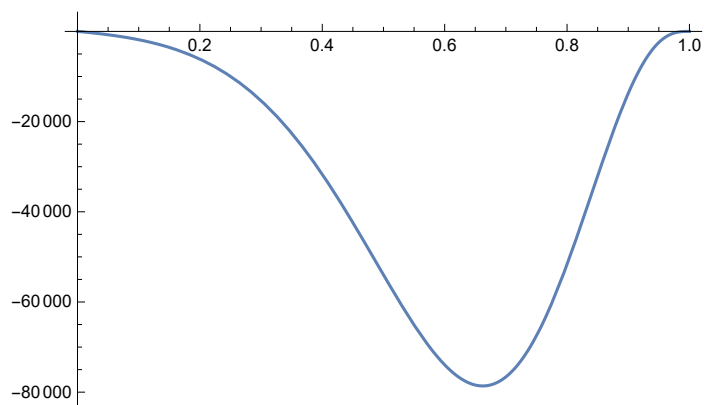

**Plot[Cf[2, 13, 8], {x, 0, 1}]**

[绘图](#)

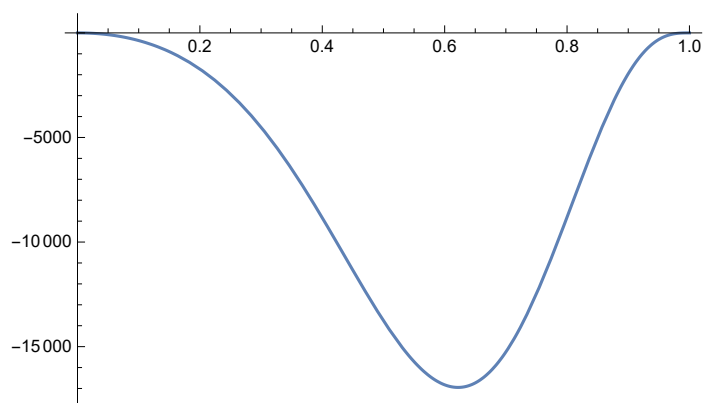

**Plot[Cf[2, 13, 7], {x, 0, 1}]**

[绘图](#)

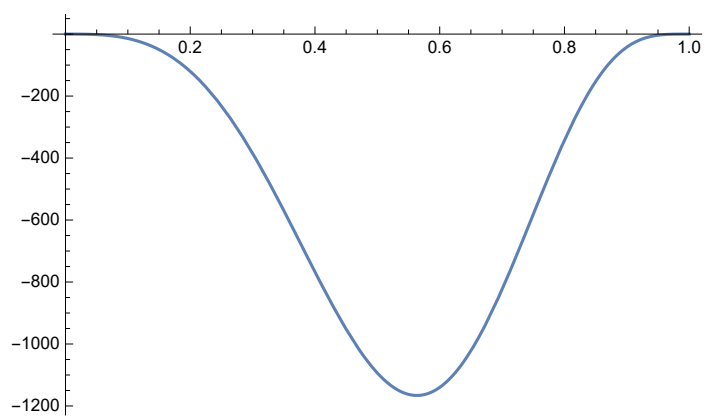

**Plot[Cf[2, 13, 6], {x, 0, 1}]**

[绘图](#)

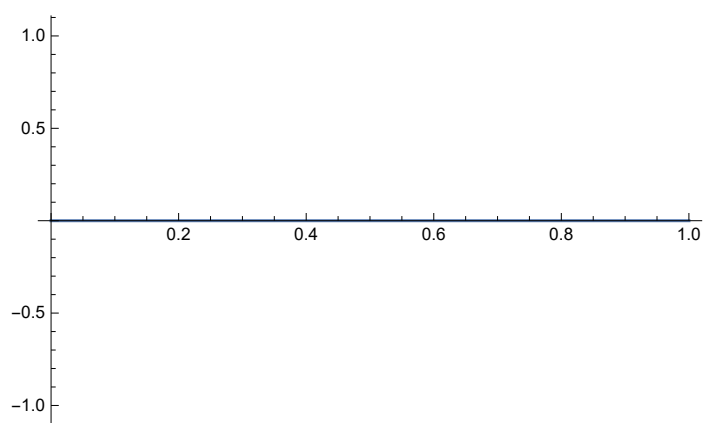

**(\*183th group coefficients r2^2r3^12\*)**

```
Plot[Cf[2, 12, 14], {x, 0, 1}]
```

[绘图](#)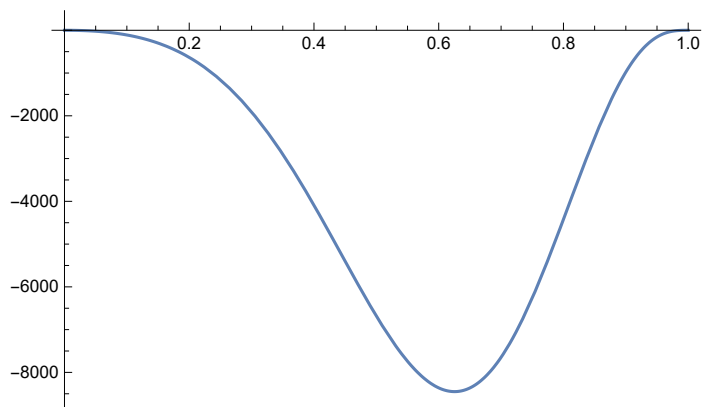

```
Plot[Cf[2, 12, 13], {x, 0, 1}]
```

[绘图](#)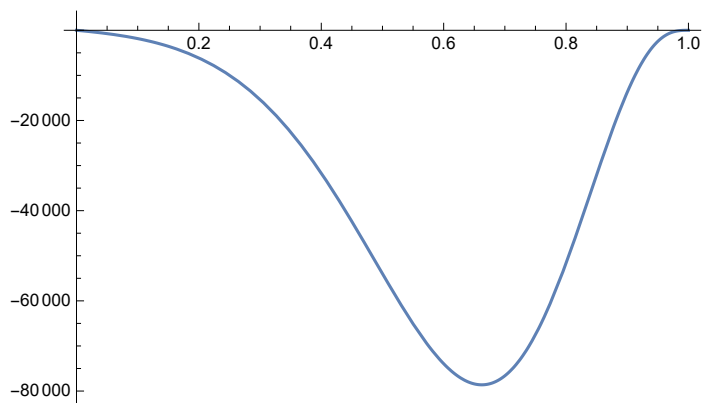

```
Plot[Cf[2, 12, 12], {x, 0, 1}]
```

[绘图](#)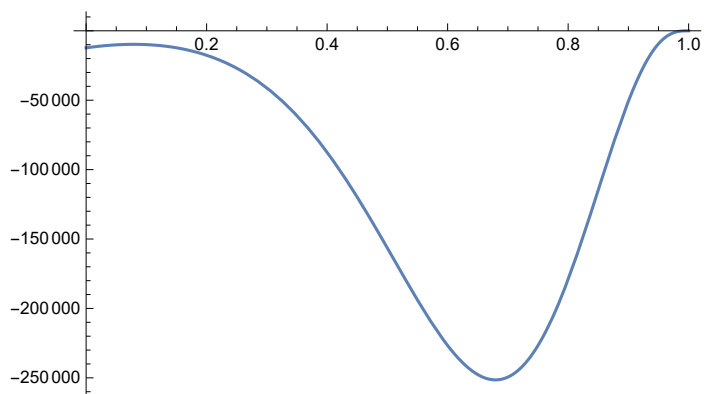

```
Plot[Cf[2, 12, 11], {x, 0, 1}]
```

[绘图](#)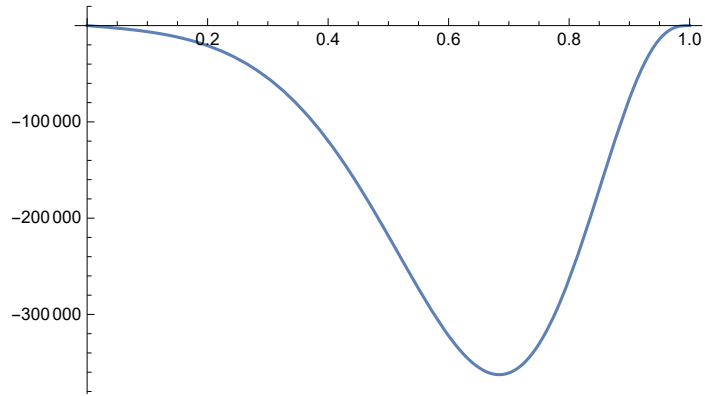

```
Plot[Cf[2, 12, 10], {x, 0, 1}]
```

[绘图](#)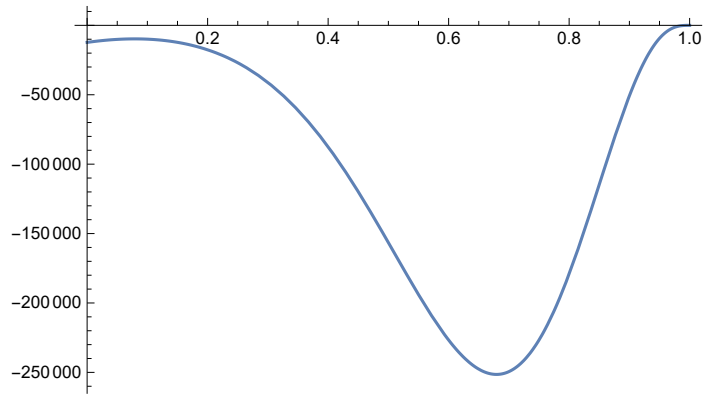

```
Plot[Cf[2, 12, 9], {x, 0, 1}]
```

[绘图](#)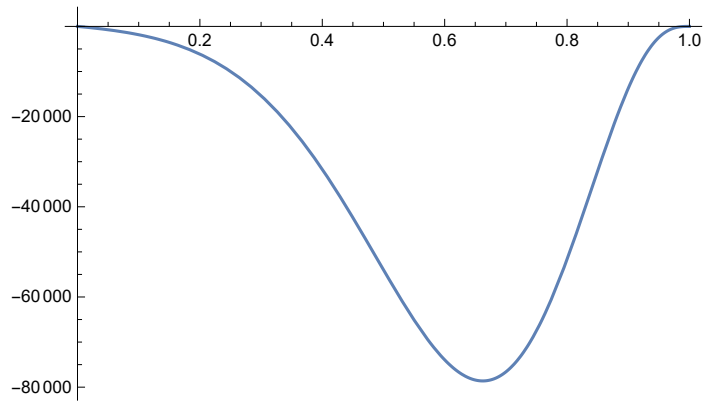



**Plot[Cf[2, 12, 8], {x, 0, 1}]**

[绘图](#)

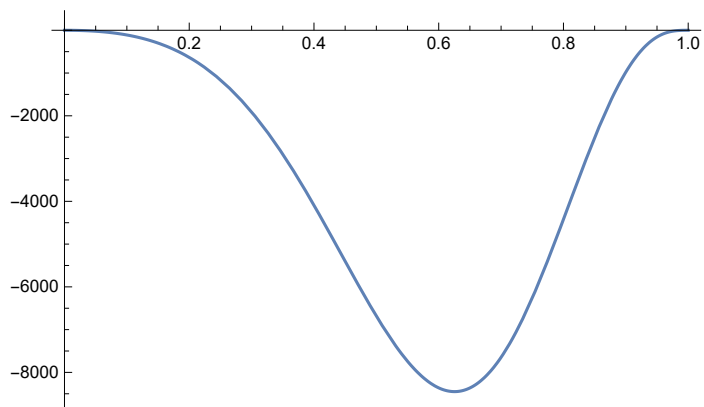

**Plot[Cf[2, 12, 7], {x, 0, 1}]**

[绘图](#)

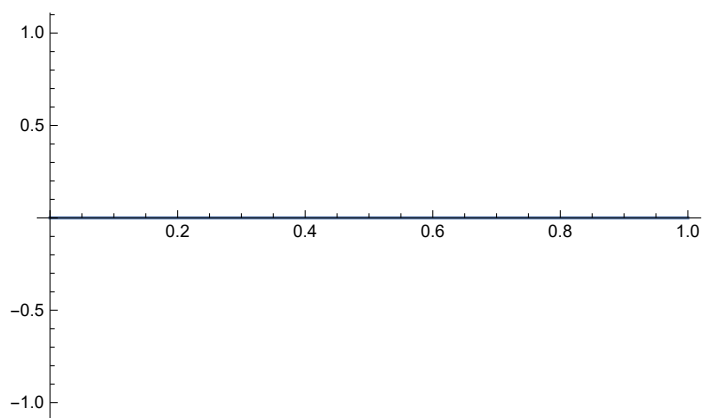

**(\*184th group coefficients r2^2r3^11\*)**

**Plot[Cf[2, 11, 14], {x, 0, 1}]**

[绘图](#)

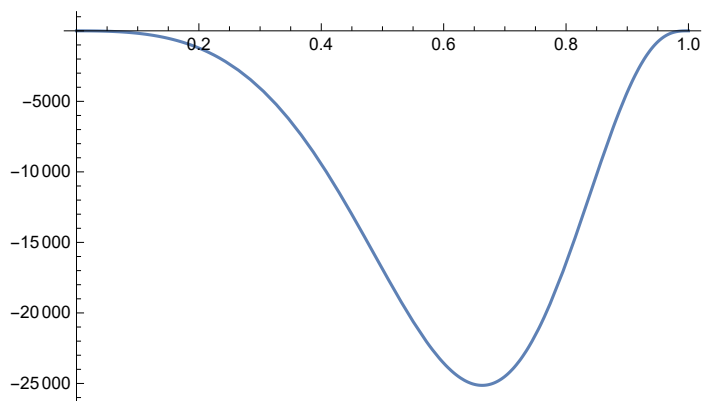

```
Plot[Cf[2, 11, 13], {x, 0, 1}]
```

[绘图](#)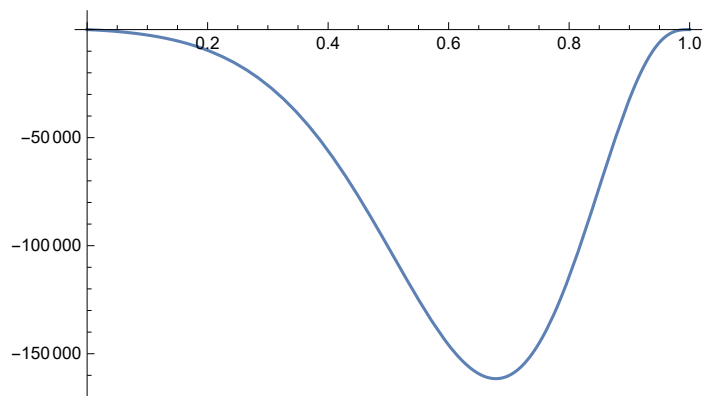

```
Plot[Cf[2, 11, 12], {x, 0, 1}]
```

[绘图](#)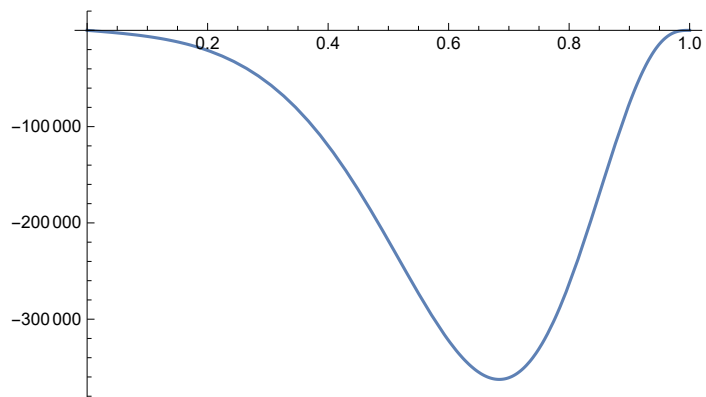

```
Plot[Cf[2, 11, 11], {x, 0, 1}]
```

[绘图](#)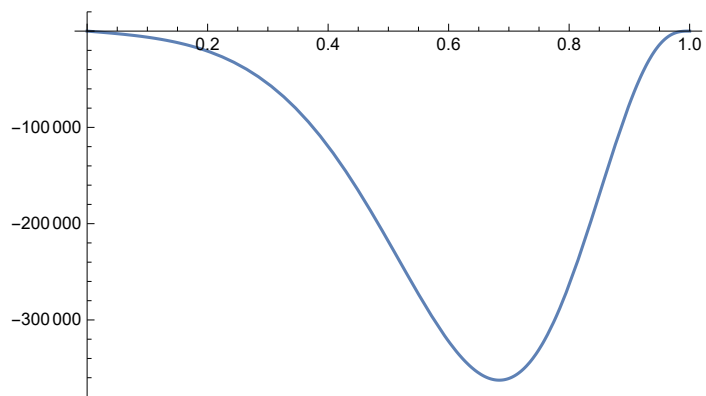

`Plot[Cf[2, 11, 10], {x, 0, 1}]`

[绘图](#)

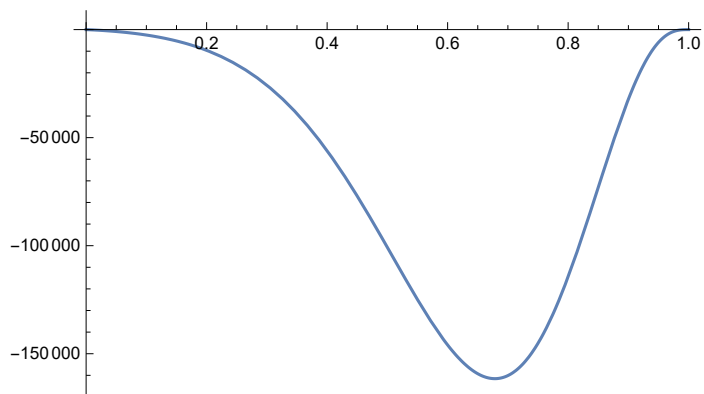

`Plot[Cf[2, 11, 9], {x, 0, 1}]`

[绘图](#)

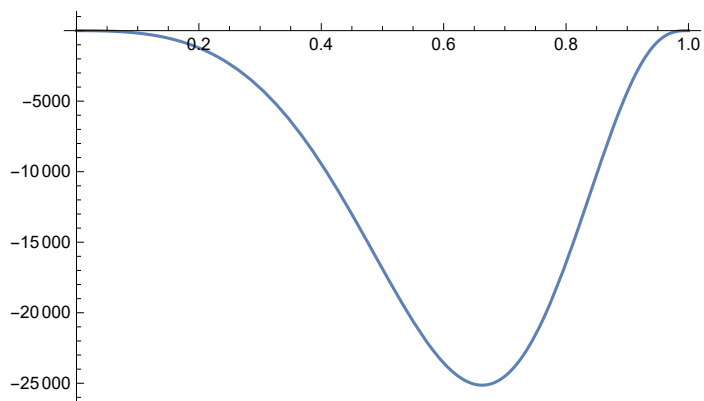

`Plot[Cf[2, 11, 8], {x, 0, 1}]`

[绘图](#)

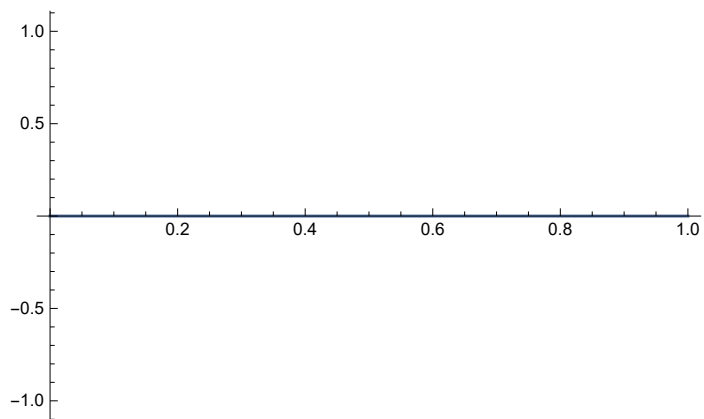

`(*185th group coefficients r2^2r3^10*)`

```
Plot[Cf[2, 10, 14], {x, 0, 1}]
```

[绘图](#)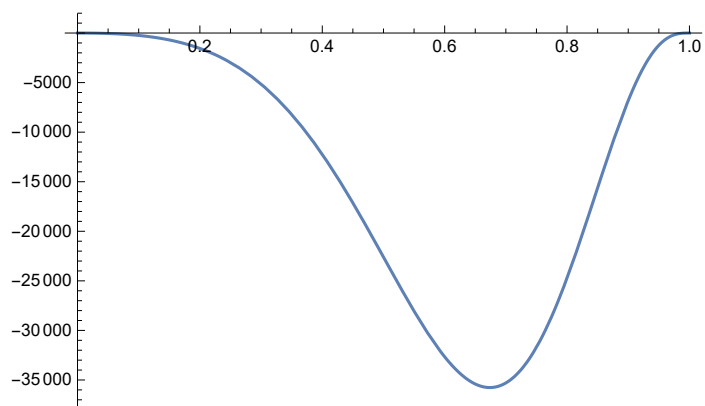

```
Plot[Cf[2, 10, 13], {x, 0, 1}]
```

[绘图](#)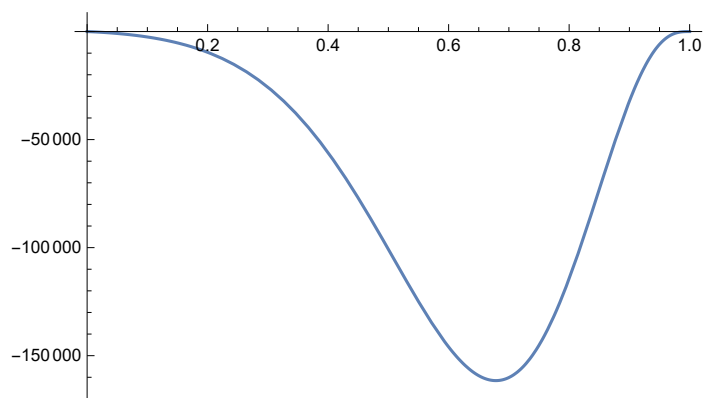

```
Plot[Cf[2, 10, 12], {x, 0, 1}]
```

[绘图](#)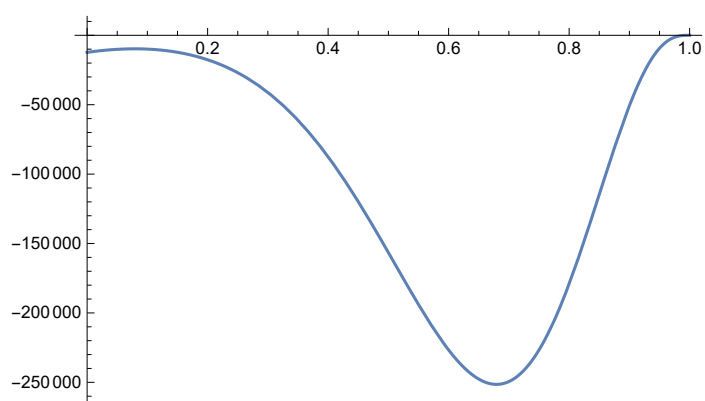

**Plot[Cf[2, 10, 11], {x, 0, 1}]**

[绘图](#)

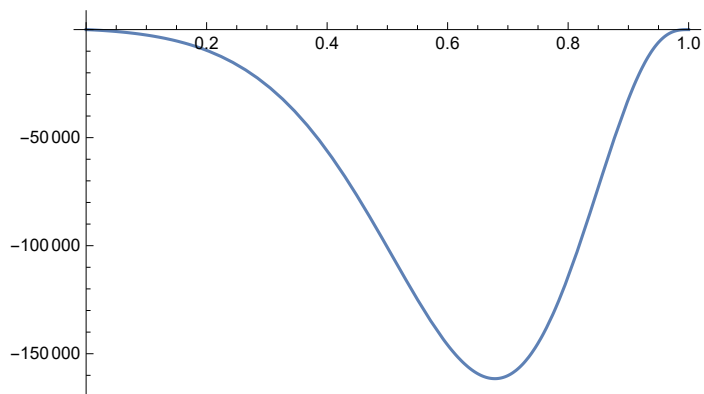

**Plot[Cf[2, 10, 10], {x, 0, 1}]**

[绘图](#)

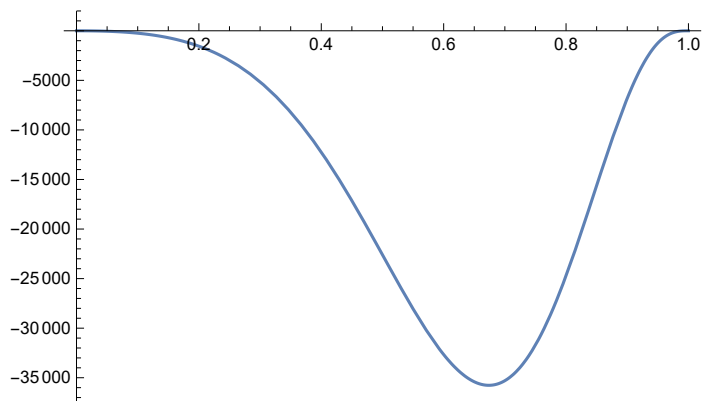

**Plot[Cf[2, 10, 9], {x, 0, 1}]**

[绘图](#)

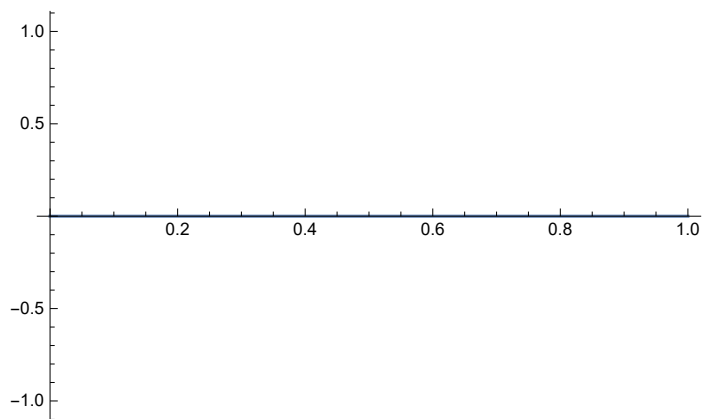

**(\*186th group coefficients r2^2r3^9\*)**

```
Plot[Cf[2, 9, 14], {x, 0, 1}]
```

[绘图](#)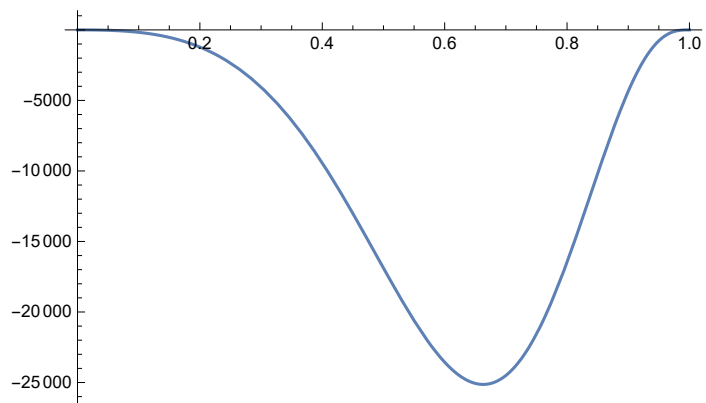

```
Plot[Cf[2, 9, 13], {x, 0, 1}]
```

[绘图](#)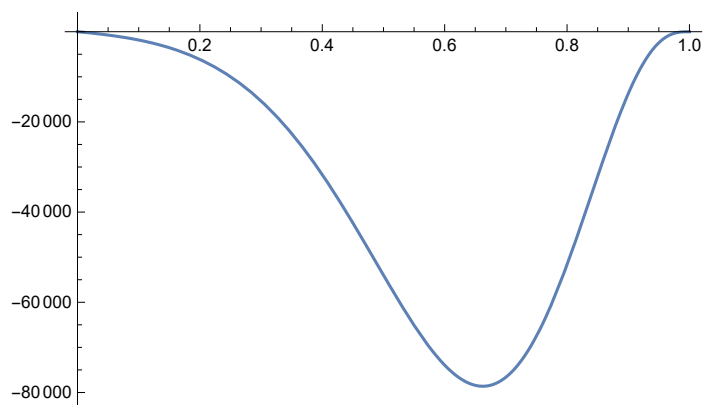

```
Plot[Cf[2, 9, 12], {x, 0, 1}]
```

[绘图](#)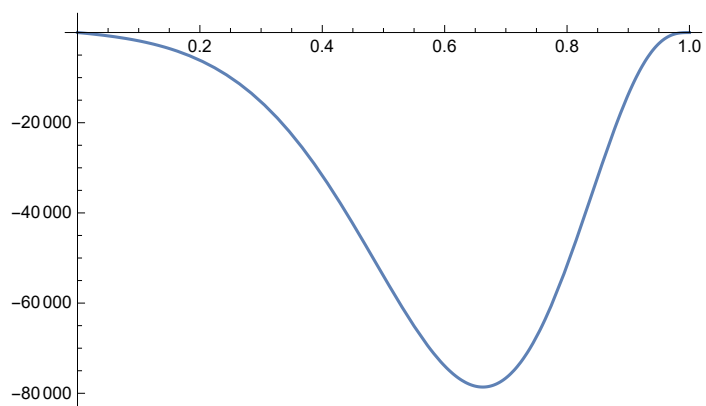

**Plot[Cf[2, 9, 11], {x, 0, 1}]**

[绘图](#)

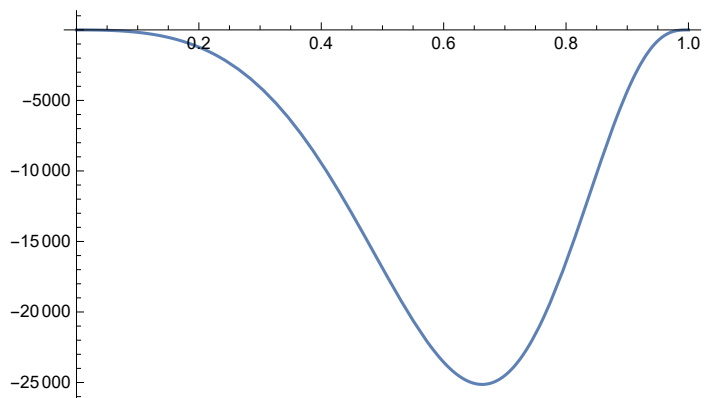

**Plot[Cf[2, 9, 10], {x, 0, 1}]**

[绘图](#)

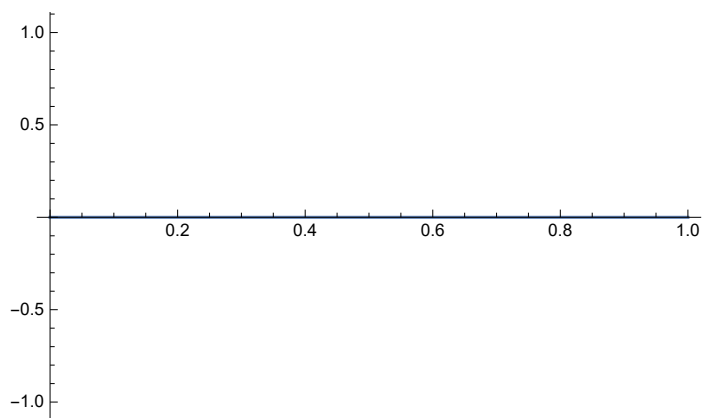

**(\*187th group coefficients r2^2r3^8\*)**

**Plot[Cf[2, 8, 14], {x, 0, 1}]**

[绘图](#)

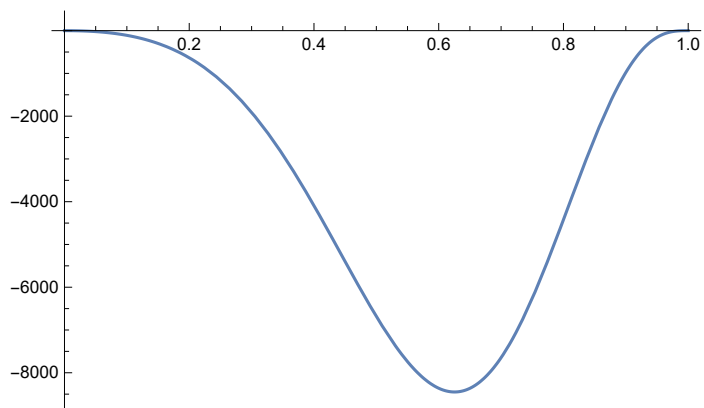

**Plot[Cf[2, 8, 13], {x, 0, 1}]**

[绘图](#)

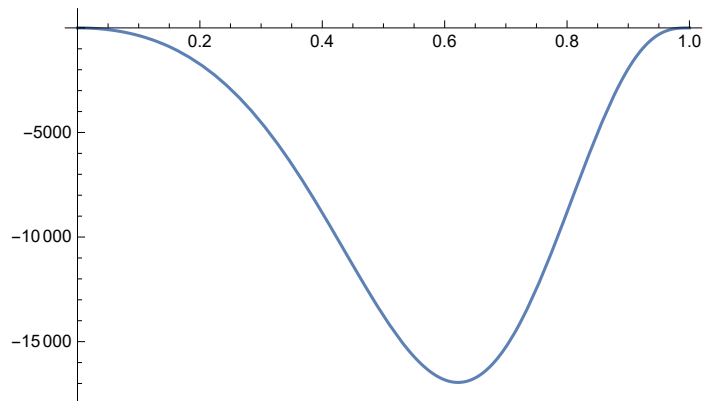

**Plot[Cf[2, 8, 12], {x, 0, 1}]**

[绘图](#)

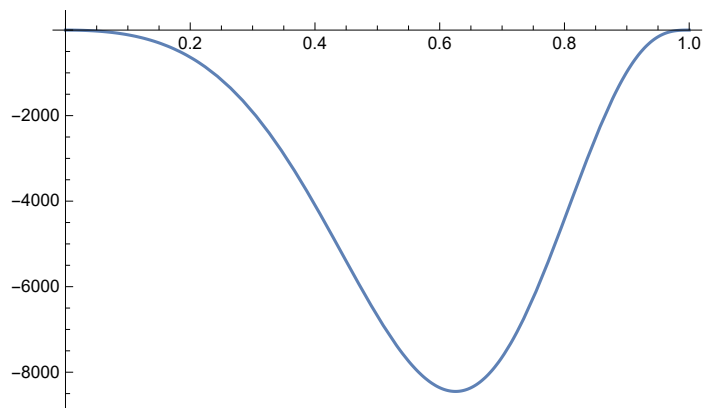

**Plot[Cf[2, 8, 11], {x, 0, 1}]**

[绘图](#)

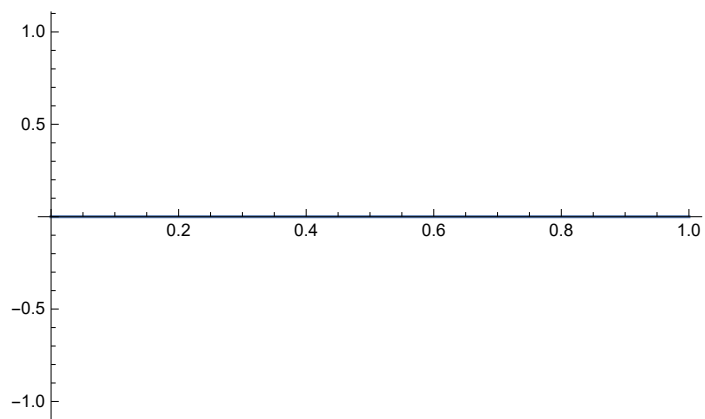

**(\*188th group coefficients r2^2r3^7\*)**



**Plot[Cf[2, 7, 14], {x, 0, 1}]**

[绘图](#)

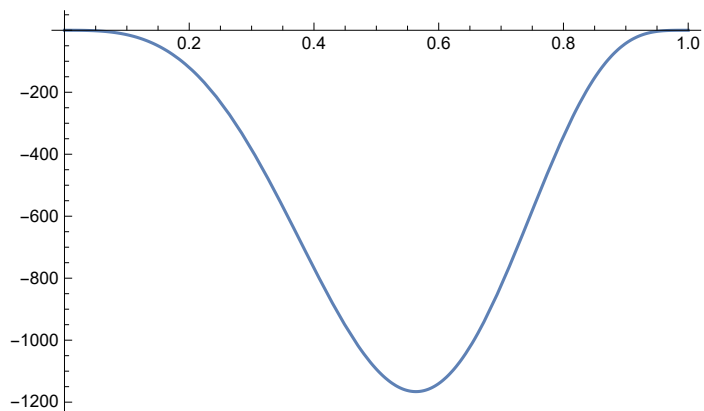

**Plot[Cf[2, 7, 13], {x, 0, 1}]**

[绘图](#)

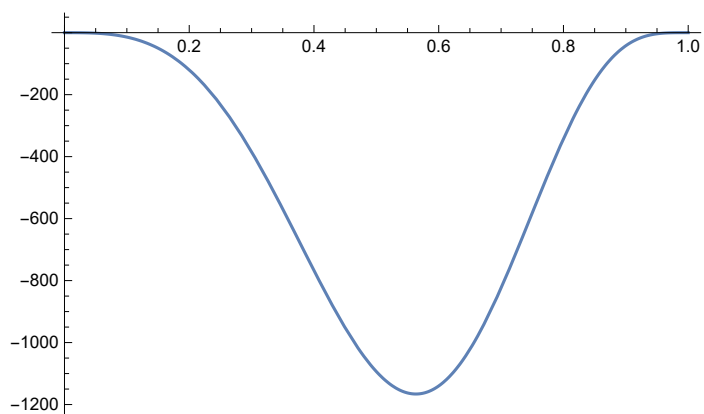

**Plot[Cf[2, 7, 12], {x, 0, 1}]**

[绘图](#)

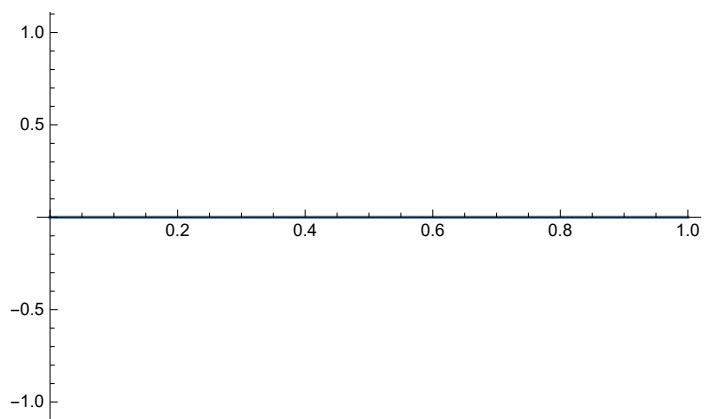

(\*189th group coefficients r2^2r3^6\*)

**Plot[Cf[2, 6, 14], {x, 0, 1}]**

[绘图](#)

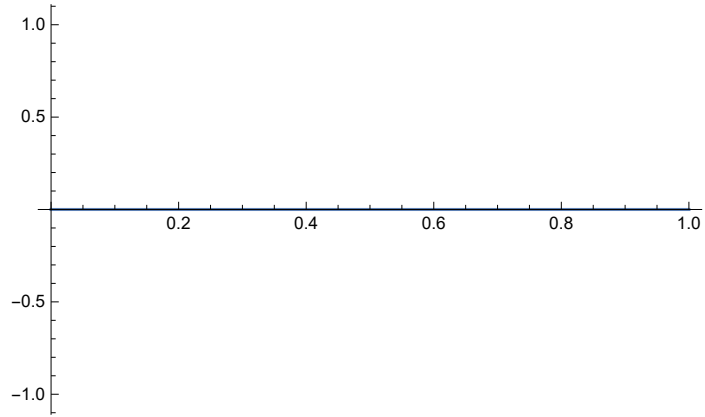

**(\*190th group coefficients r2^2r3^5\*)**

**Plot[Cf[2, 5, 14], {x, 0, 1}]**

[绘图](#)

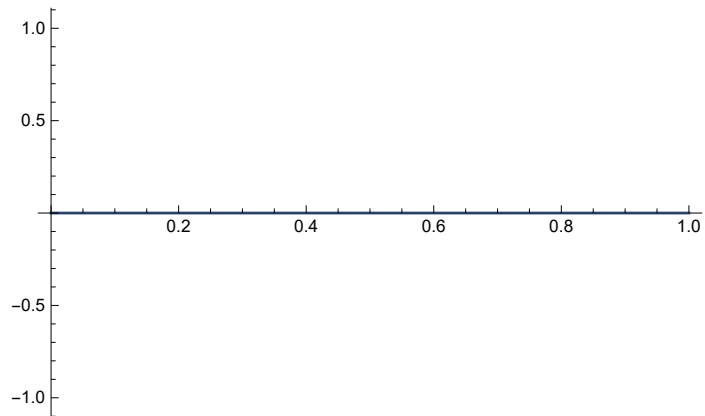

**(\*191th group coefficients r2^2r3^4\*)**

**Plot[Cf[2, 4, 14], {x, 0, 1}]**

[绘图](#)

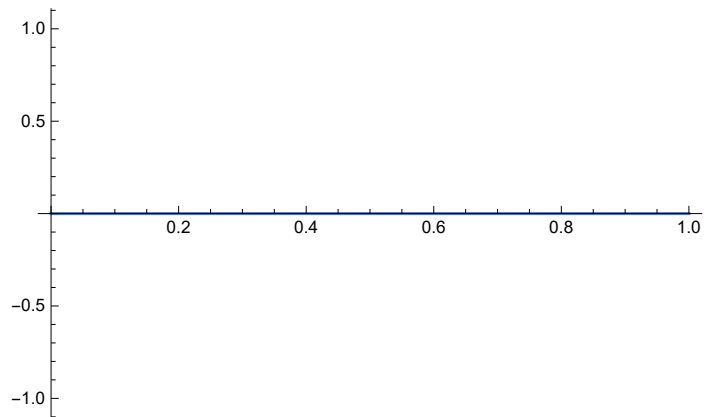

**(\*192th group coefficients r2^2r3^3\*)**

**Plot[Cf[2, 3, 14], {x, 0, 1}]**

[绘图](#)

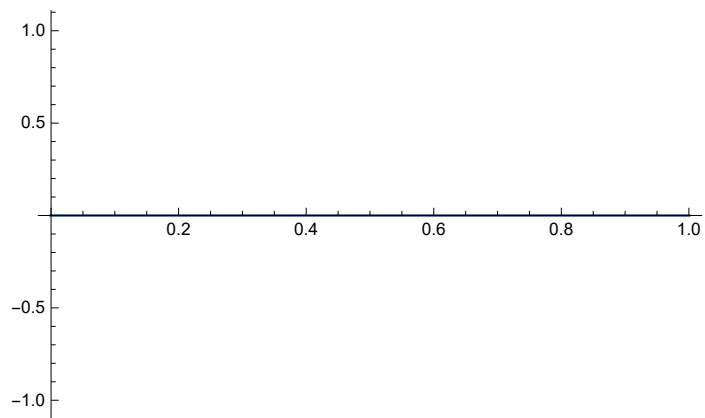

(\*193th group coefficients r2^2r3^2\*)

**Plot[Cf[2, 2, 14], {x, 0, 1}]**

[绘图](#)

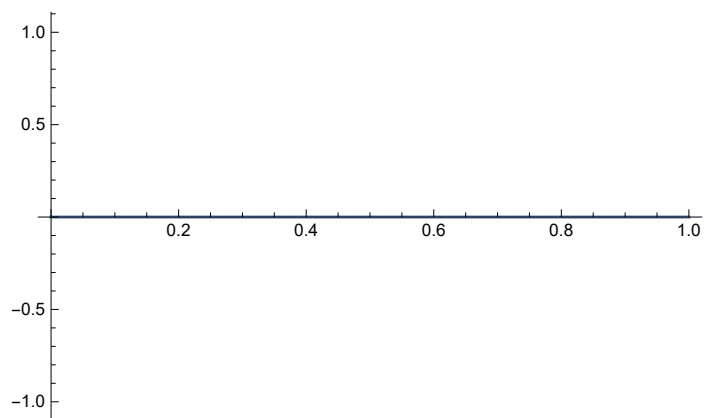

(\*194th group coefficients r2^2r3^1\*)

**Plot[Cf[2, 1, 14], {x, 0, 1}]**

[绘图](#)

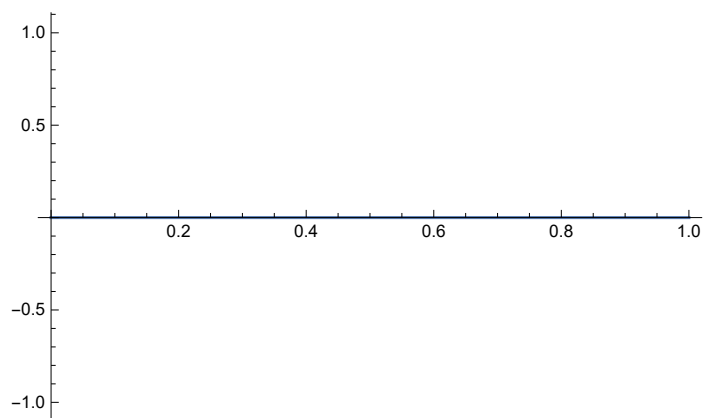

(\*195th group coefficients r2^2r3^0\*)

`Plot[Cf[2, 0, 14], {x, 0, 1}]`

[绘图](#)

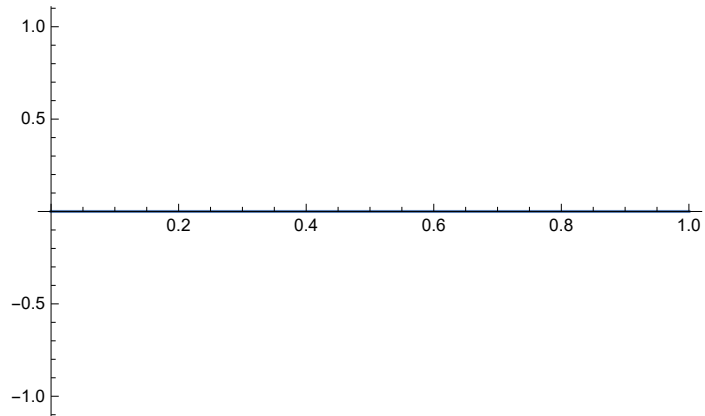

(\*196th group coefficients r2^1r3^14\*)

`Plot[Cf[1, 14, 14], {x, 0, 1}]`

[绘图](#)

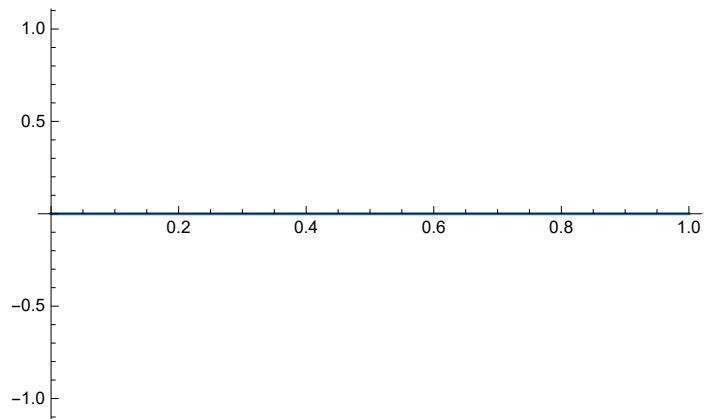

`Plot[Cf[1, 14, 13], {x, 0, 1}]`

[绘图](#)

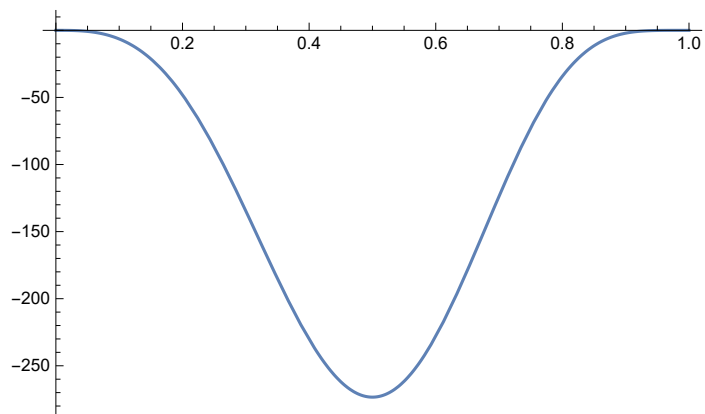

**Plot[Cf[1, 14, 12], {x, 0, 1}]**

[绘图](#)

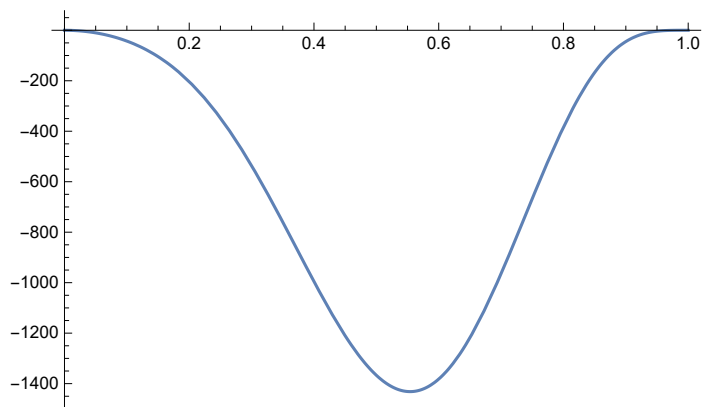

**Plot[Cf[1, 14, 11], {x, 0, 1}]**

[绘图](#)

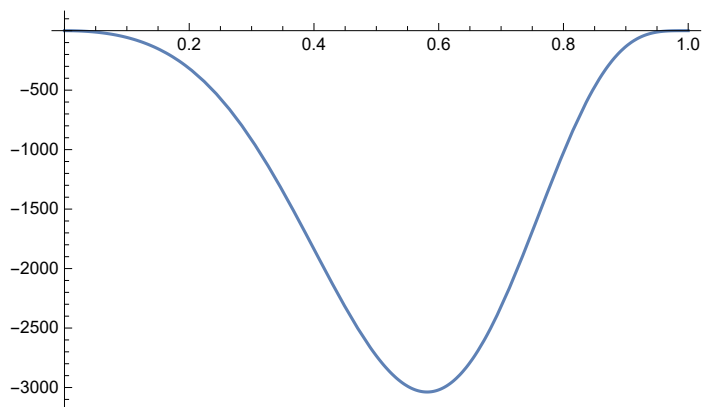

**Plot[Cf[1, 14, 10], {x, 0, 1}]**

[绘图](#)

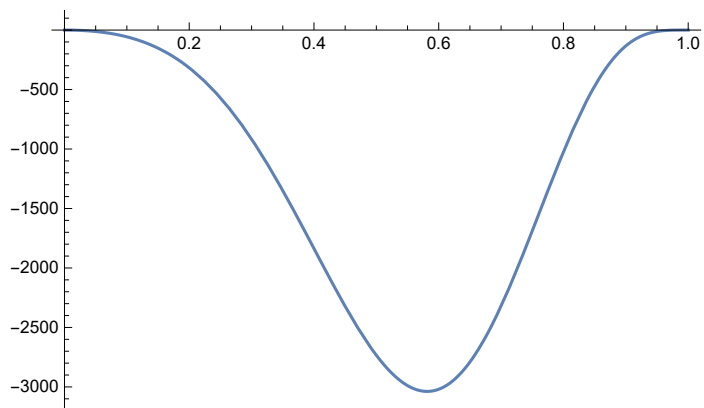

**Plot[Cf[1, 14, 9], {x, 0, 1}]**

[绘图](#)

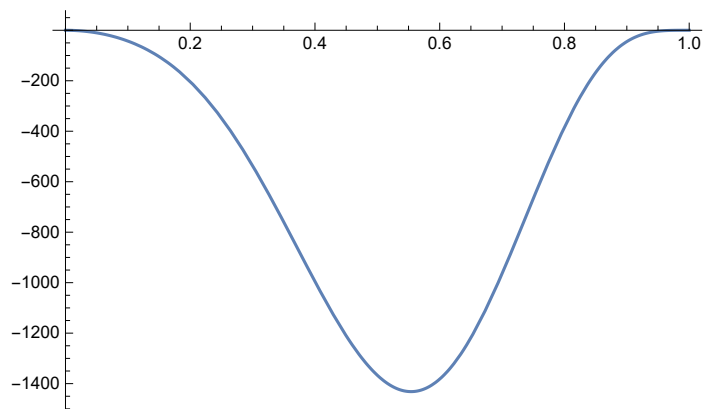

**Plot[Cf[1, 14, 8], {x, 0, 1}]**

[绘图](#)

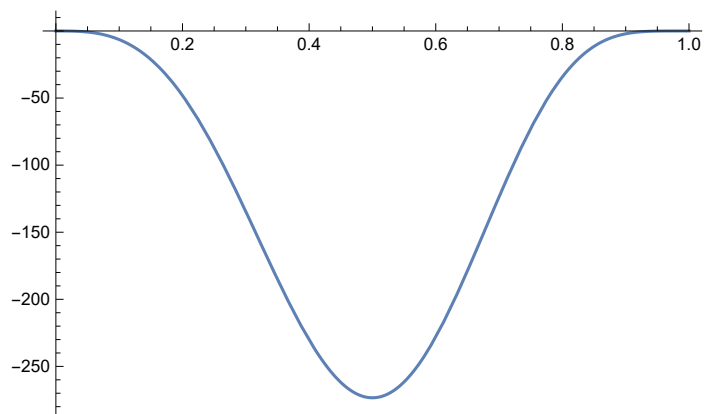

**Plot[Cf[1, 14, 7], {x, 0, 1}]**

[绘图](#)

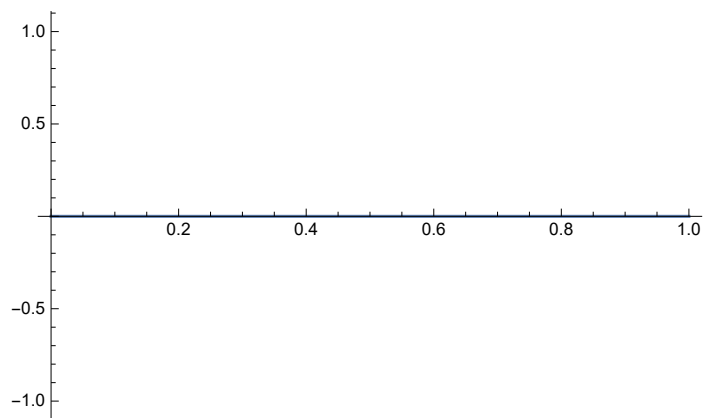

**(\*197th group coefficients r2^1r3^13\*)**

```
Plot[Cf[1, 13, 14], {x, 0, 1}]
```

[绘图](#)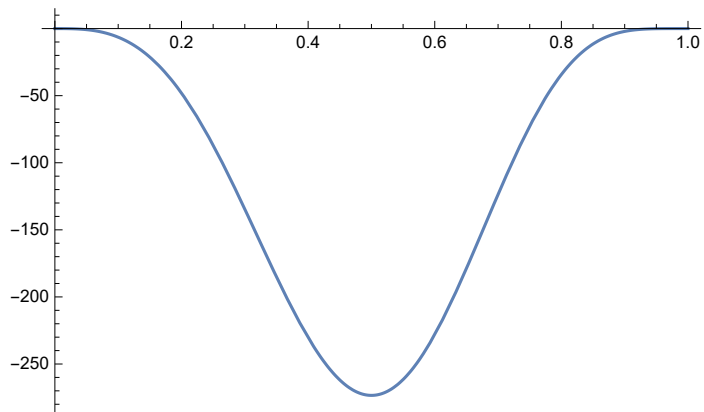

```
Plot[Cf[1, 13, 13], {x, 0, 1}]
```

[绘图](#)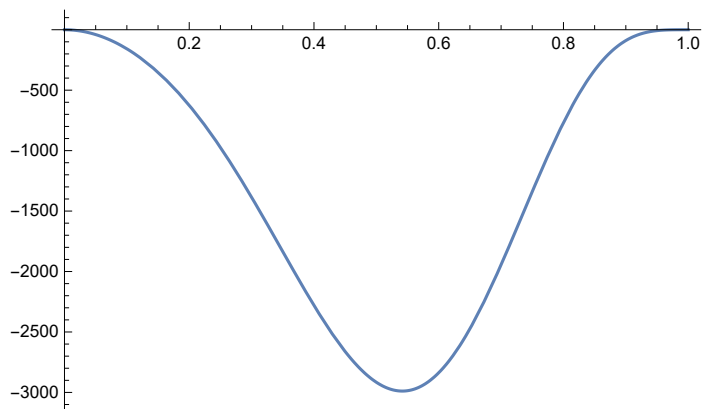

```
Plot[Cf[1, 13, 12], {x, 0, 1}]
```

[绘图](#)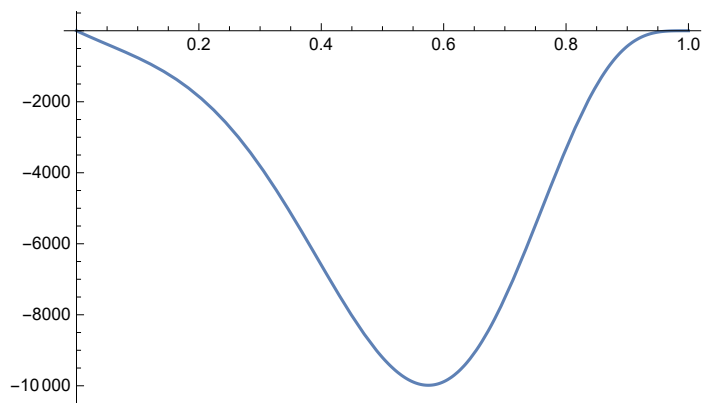

```
Plot[Cf[1, 13, 11], {x, 0, 1}]
```

[绘图](#)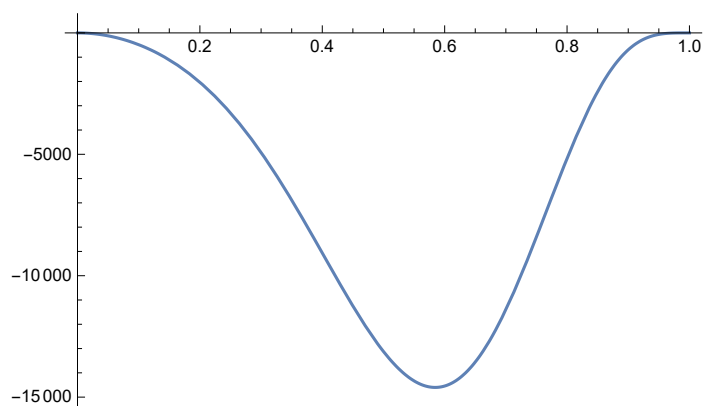

```
Plot[Cf[1, 13, 10], {x, 0, 1}]
```

[绘图](#)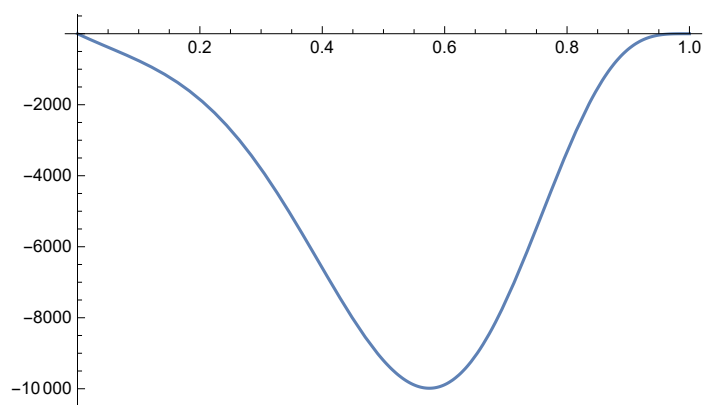

```
Plot[Cf[1, 13, 9], {x, 0, 1}]
```

[绘图](#)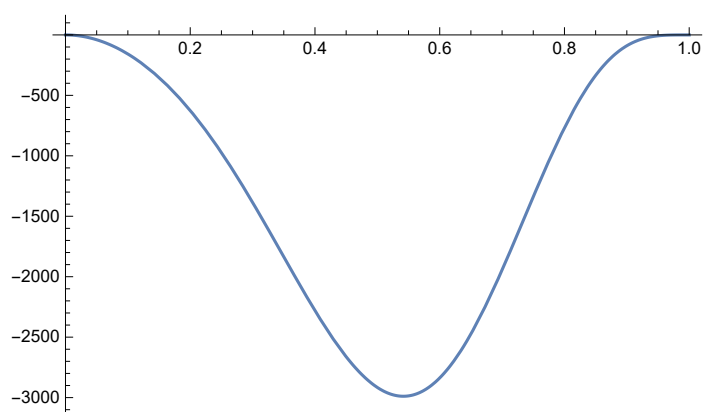



**Plot[Cf[1, 13, 8], {x, 0, 1}]**

[绘图](#)

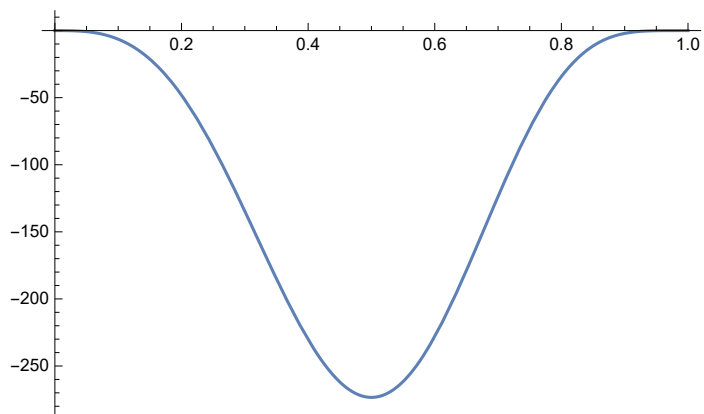

**Plot[Cf[1, 13, 7], {x, 0, 1}]**

[绘图](#)

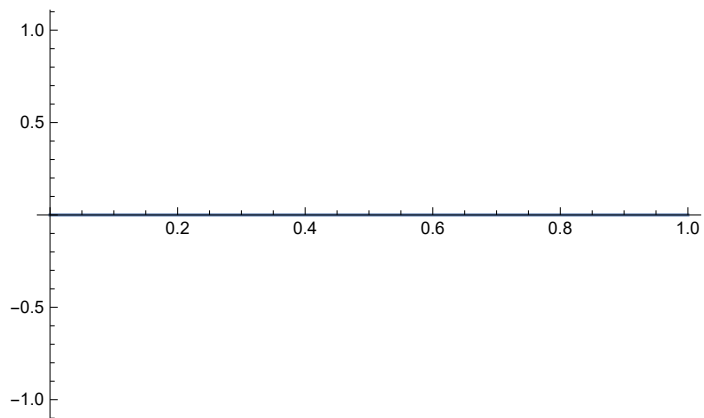

**(\*198th group coefficients r2^1r3^12\*)**

**Plot[Cf[1, 12, 14], {x, 0, 1}]**

[绘图](#)

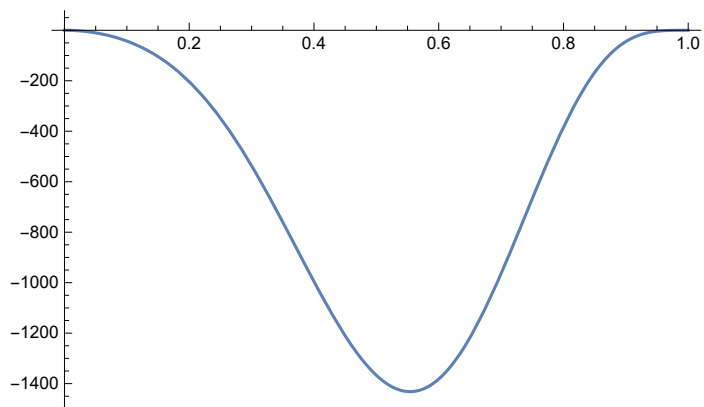

```
Plot[Cf[1, 12, 13], {x, 0, 1}]
```

[绘图](#)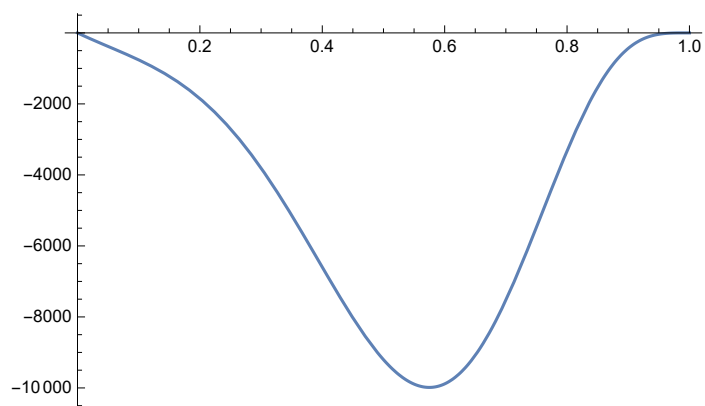

```
Plot[Cf[1, 12, 12], {x, 0, 1}]
```

[绘图](#)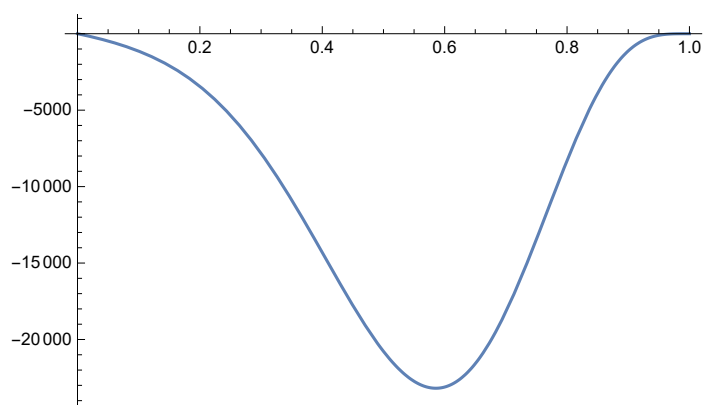

```
Plot[Cf[1, 12, 11], {x, 0, 1}]
```

[绘图](#)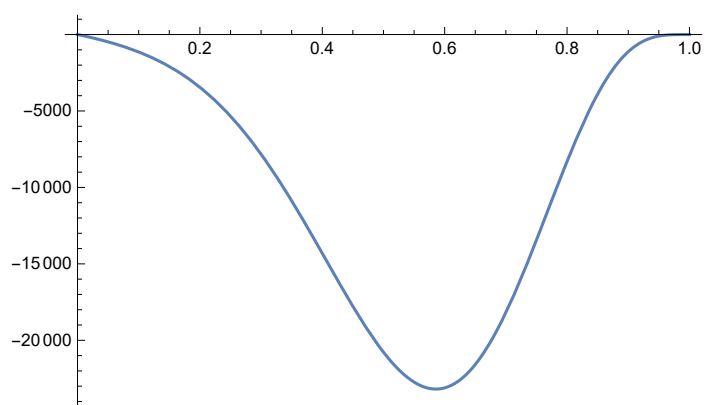

**Plot[Cf[1, 12, 10], {x, 0, 1}]**

[绘图](#)

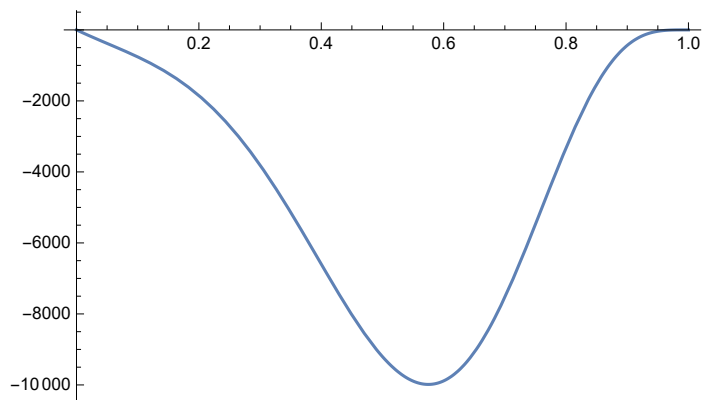

**Plot[Cf[1, 12, 9], {x, 0, 1}]**

[绘图](#)

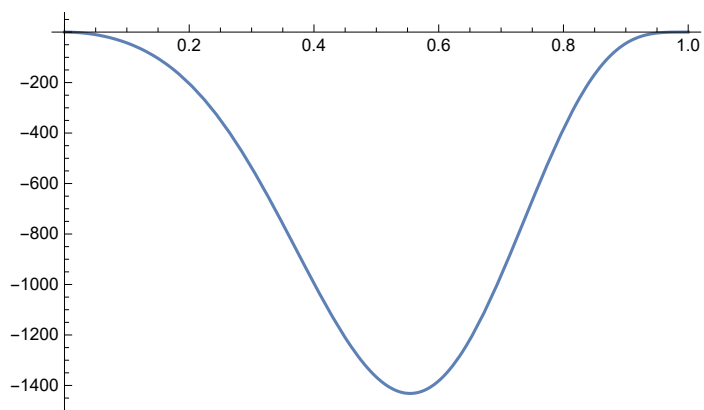

**Plot[Cf[1, 12, 8], {x, 0, 1}]**

[绘图](#)

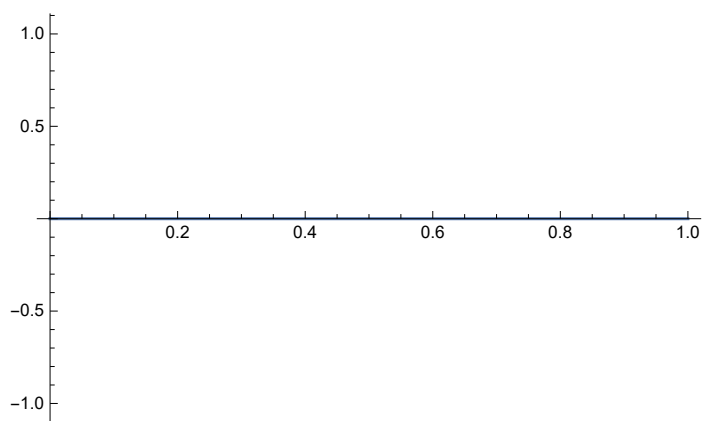

(\*199th group coefficients r2^1r3^11\*)

```
Plot[Cf[1, 11, 14], {x, 0, 1}]
```

[绘图](#)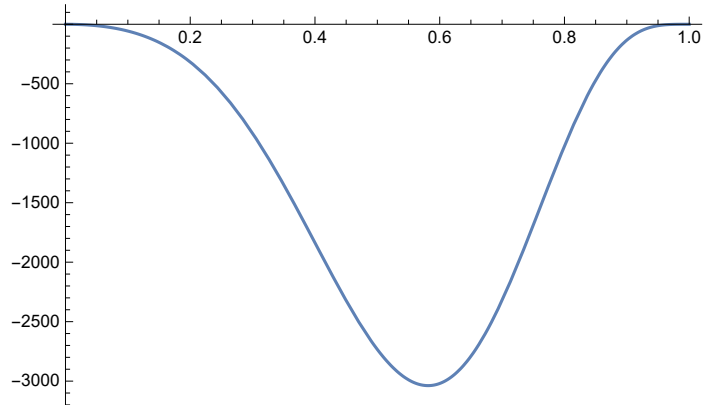

```
Plot[Cf[1, 11, 13], {x, 0, 1}]
```

[绘图](#)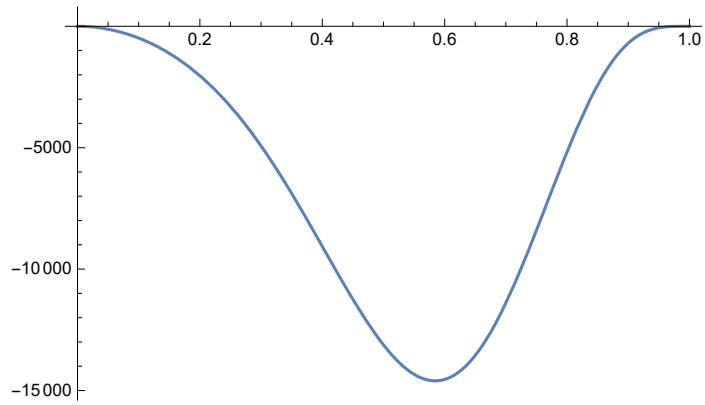

```
Plot[Cf[1, 11, 12], {x, 0, 1}]
```

[绘图](#)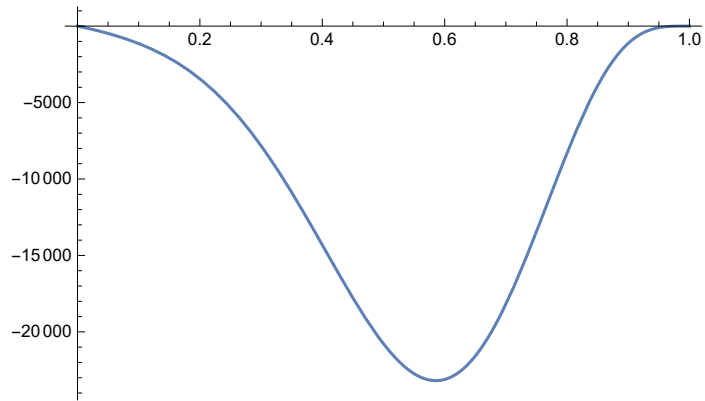

**Plot[Cf[1, 11, 11], {x, 0, 1}]**

[绘图](#)

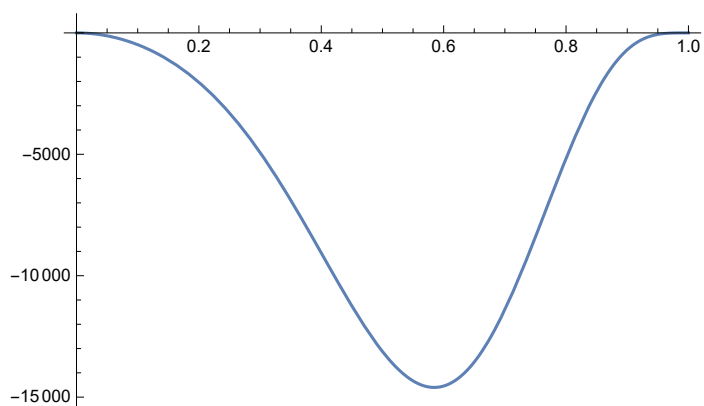

**Plot[Cf[1, 11, 10], {x, 0, 1}]**

[绘图](#)

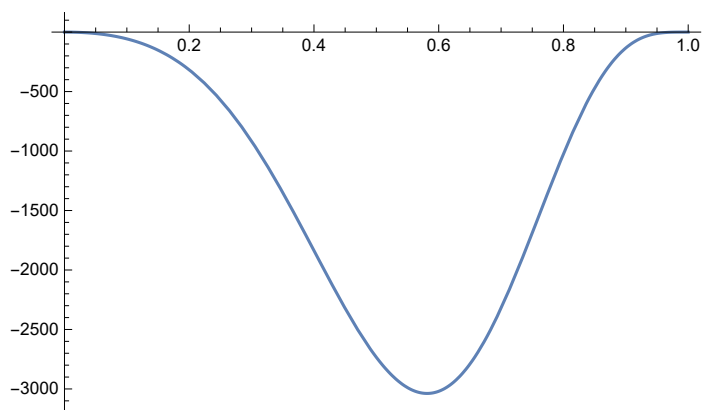

**Plot[Cf[1, 11, 9], {x, 0, 1}]**

[绘图](#)

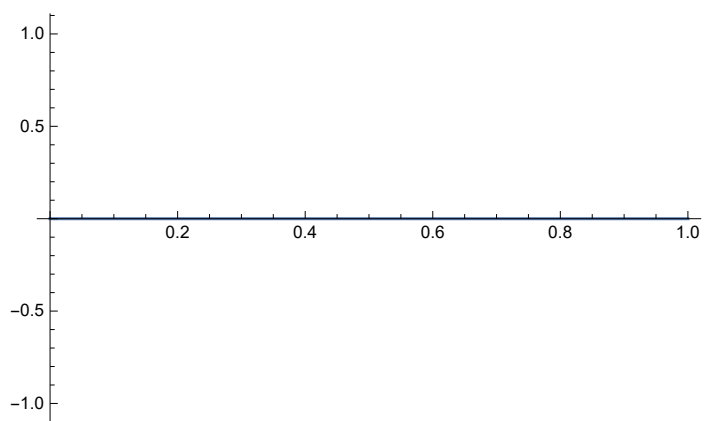

(\*200th group coefficients r2^1r3^10\*)

**Plot[Cf[1, 10, 14], {x, 0, 1}]**

[绘图](#)

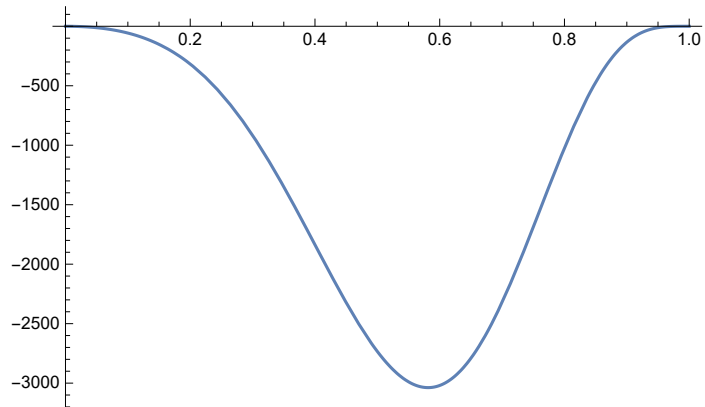

**Plot[Cf[1, 10, 13], {x, 0, 1}]**

[绘图](#)

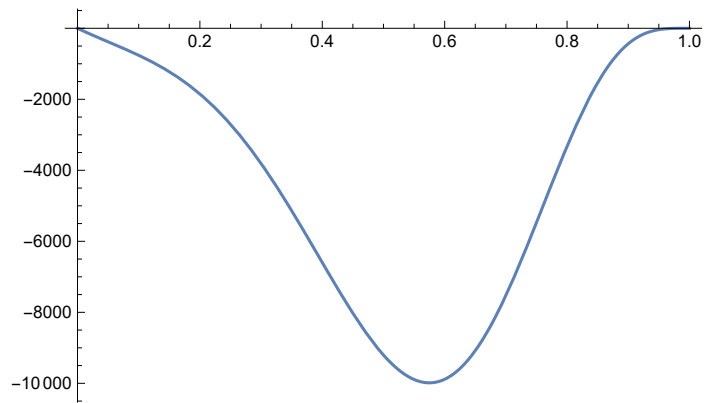

**Plot[Cf[1, 10, 12], {x, 0, 1}]**

[绘图](#)

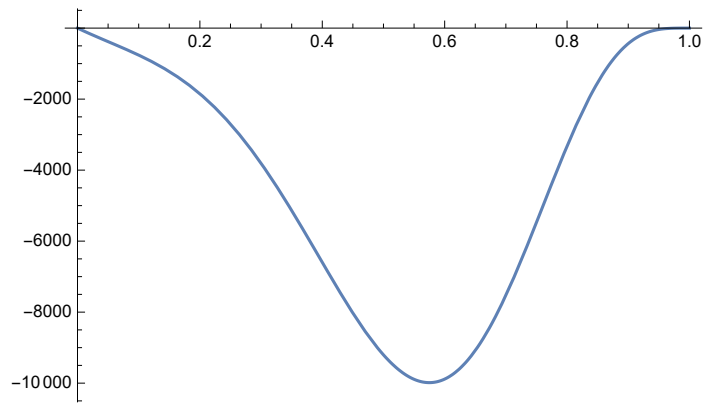

**Plot[Cf[1, 10, 11], {x, 0, 1}]**

[绘图](#)

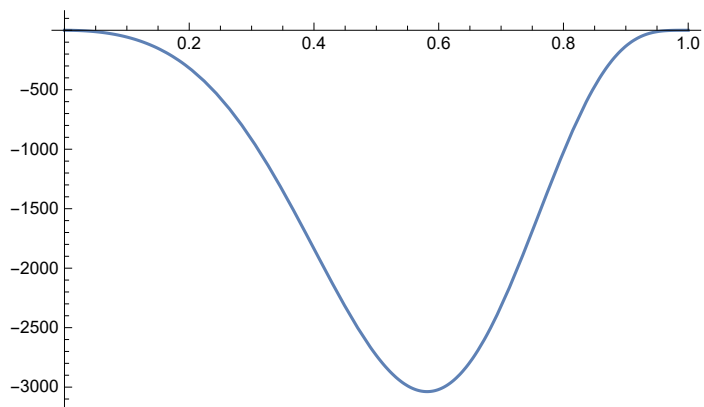

**Plot[Cf[1, 10, 10], {x, 0, 1}]**

[绘图](#)

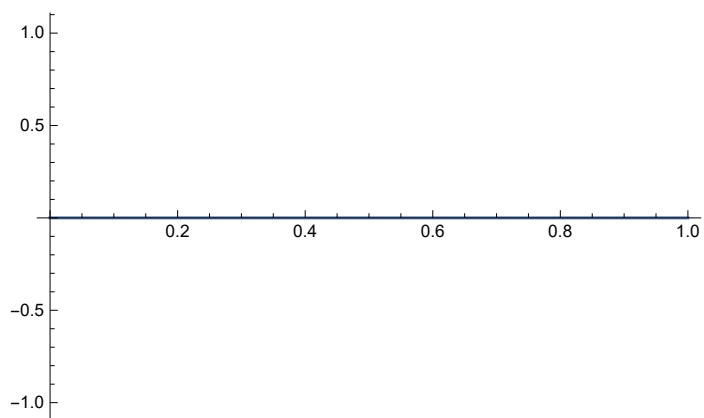

**Plot[Cf[1, 10, 9], {x, 0, 1}]**

[绘图](#)

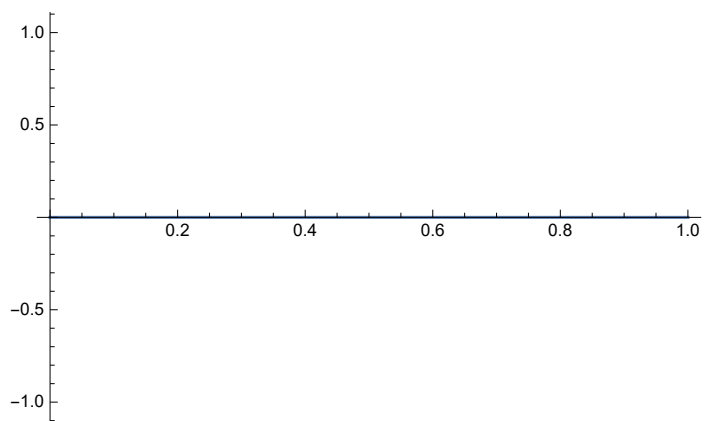

(\*201th group coefficients r2^1r3^9\*)

**Plot[Cf[1, 9, 14], {x, 0, 1}]**

[绘图](#)

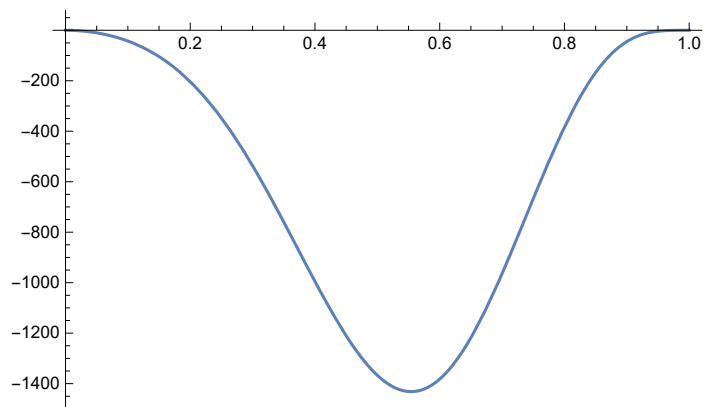

**Plot[Cf[1, 9, 13], {x, 0, 1}]**

[绘图](#)

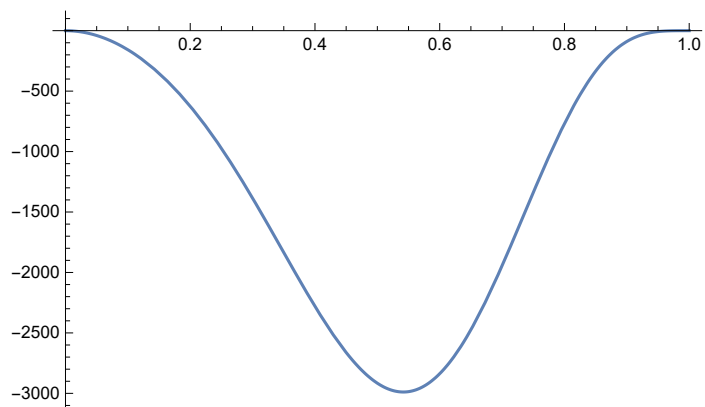

**Plot[Cf[1, 9, 12], {x, 0, 1}]**

[绘图](#)

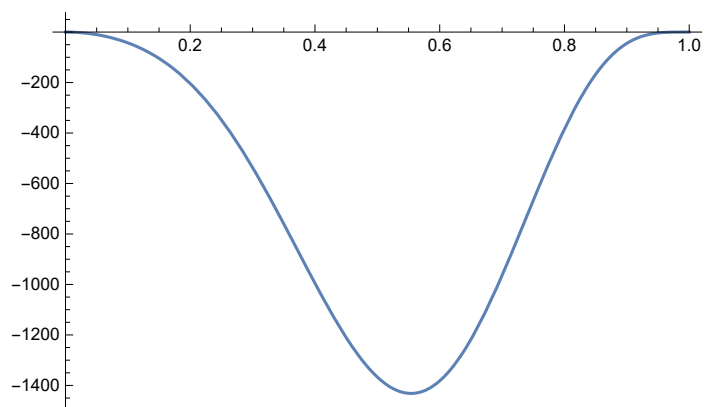



**Plot[Cf[1, 9, 11], {x, 0, 1}]**

[绘图](#)

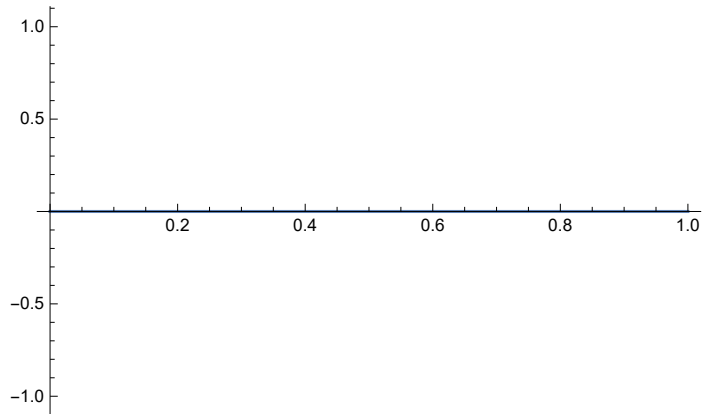

(\*202th group coefficients r2^1r3^8\*)

**Plot[Cf[1, 8, 14], {x, 0, 1}]**

[绘图](#)

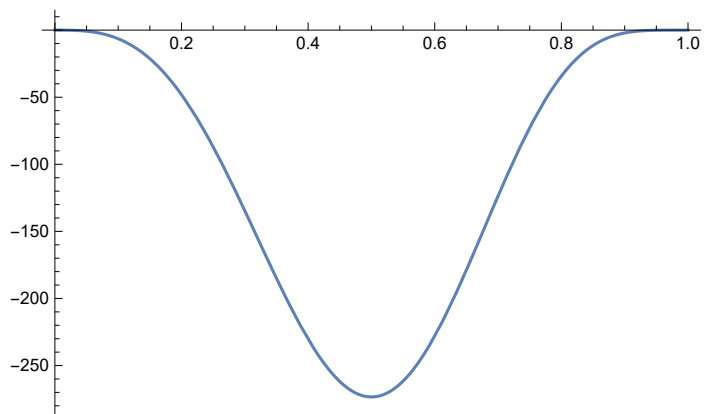

**Plot[Cf[1, 8, 13], {x, 0, 1}]**

[绘图](#)

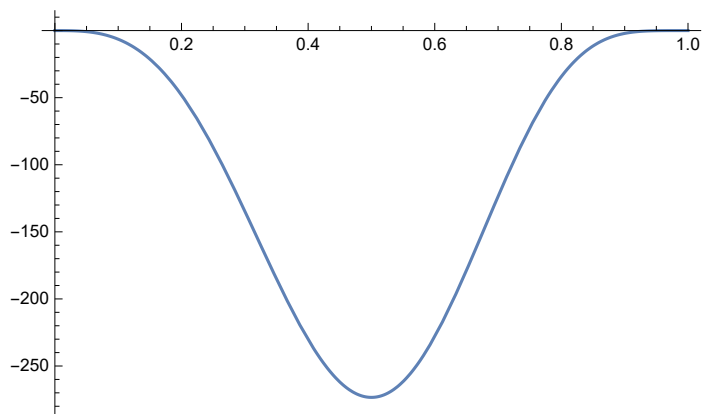

**Plot[Cf[1, 8, 12], {x, 0, 1}]**

[绘图](#)

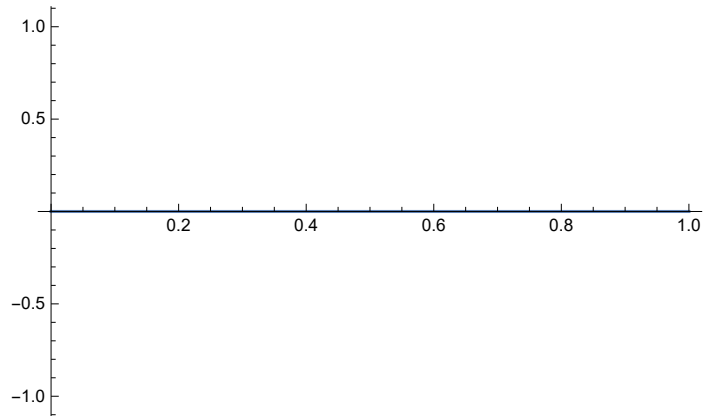

(\*203th group coefficients r2^1r3^7\*)

**Plot[Cf[1, 7, 14], {x, 0, 1}]**

[绘图](#)

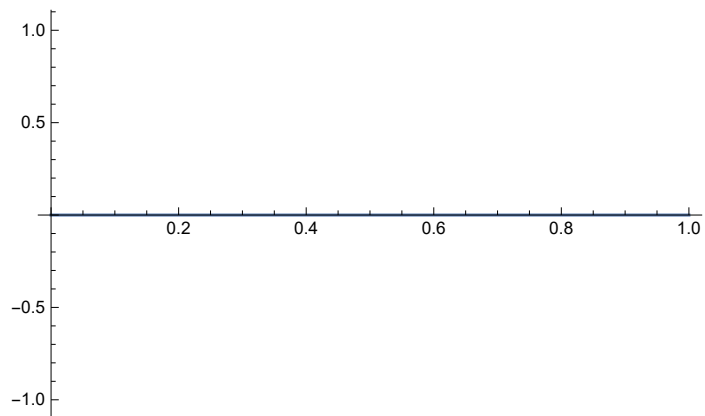

**Plot[Cf[1, 7, 13], {x, 0, 1}]**

[绘图](#)

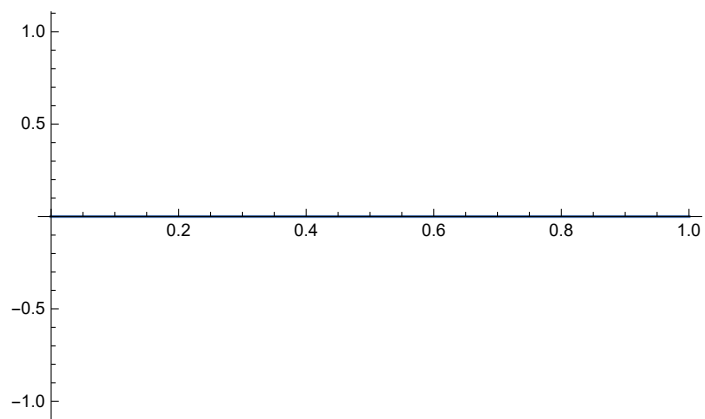

(\*204th group coefficients r2^1r3^6\*)

**Plot[Cf[1, 6, 14], {x, 0, 1}]**

[绘图](#)

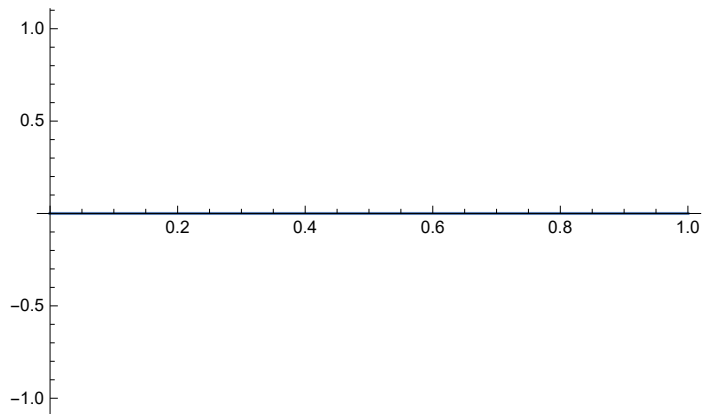

**(\*205th group coefficients r2^1r3^5\*)**

**Plot[Cf[1, 5, 14], {x, 0, 1}]**

[绘图](#)

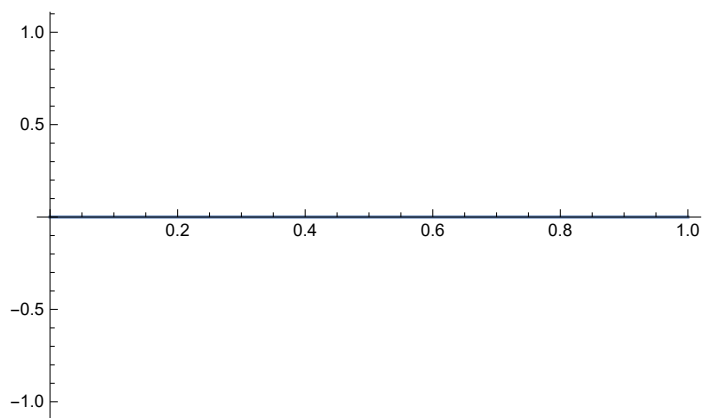

**(\*206th group coefficients r2^1r3^4\*)**

**Plot[Cf[1, 4, 14], {x, 0, 1}]**

[绘图](#)

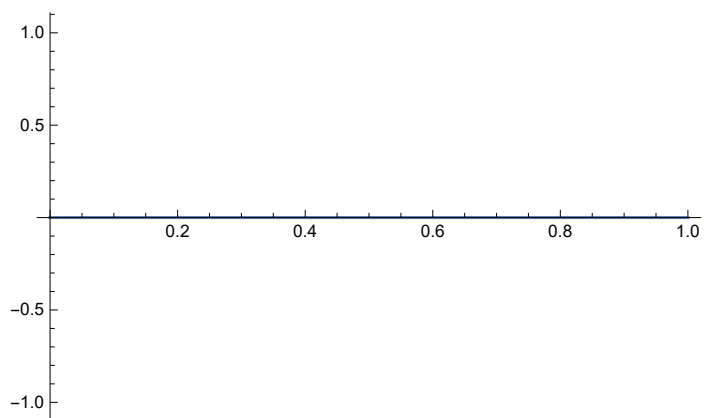

**(\*207th group coefficients r2^1r3^3\*)**

**Plot[Cf[1, 3, 14], {x, 0, 1}]**

[绘图](#)

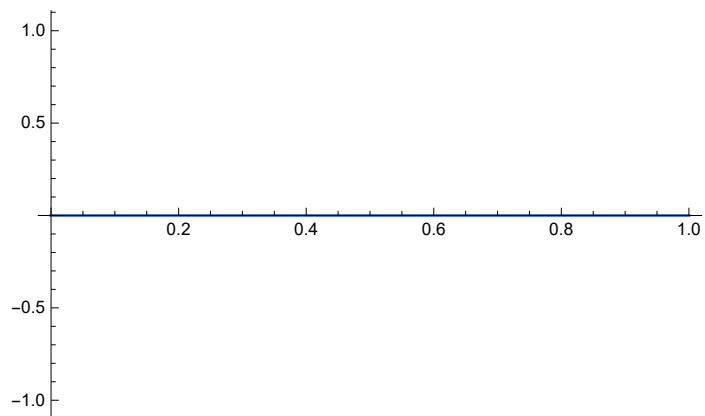

(\*208th group coefficients  $r^2 r^3^2$ \*)

**Plot[Cf[1, 2, 14], {x, 0, 1}]**

[绘图](#)

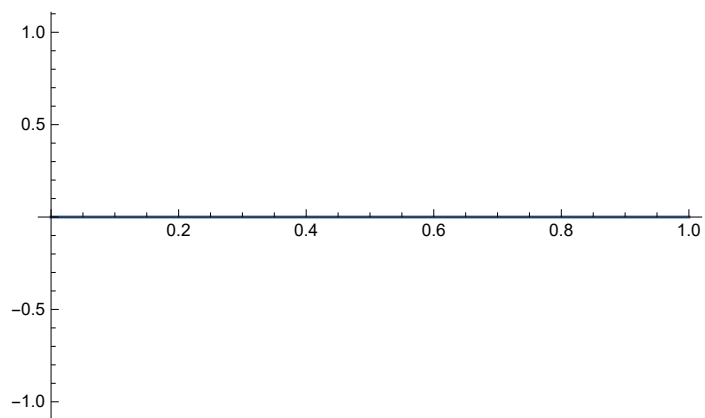

(\*209th group coefficients  $r^2 r^3^1$ \*)

**Plot[Cf[1, 1, 14], {x, 0, 1}]**

[绘图](#)

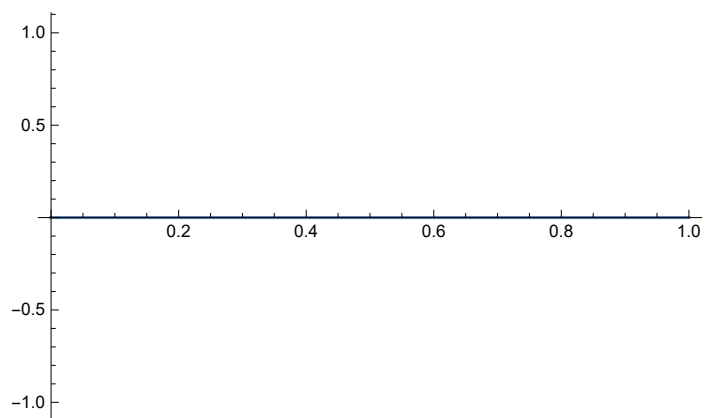

(\*210th group coefficients  $r^2 r^3^0$ \*)

`Plot[Cf[1, 0, 14], {x, 0, 1}]`

[绘图](#)

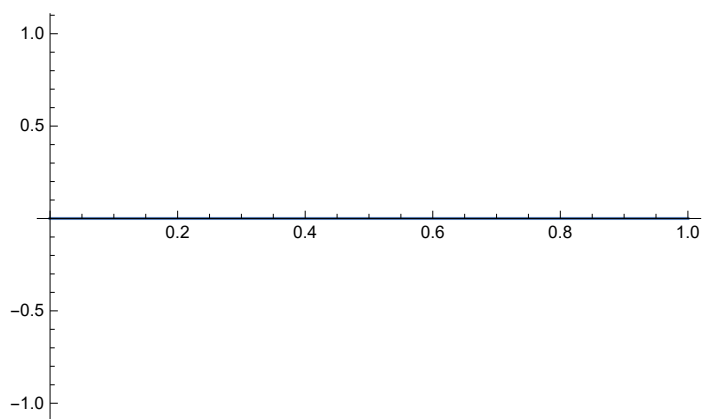

(\*211th group coefficients r2^0r3^14\*)

`Plot[Cf[0, 14, 14], {x, 0, 1}]`

[绘图](#)

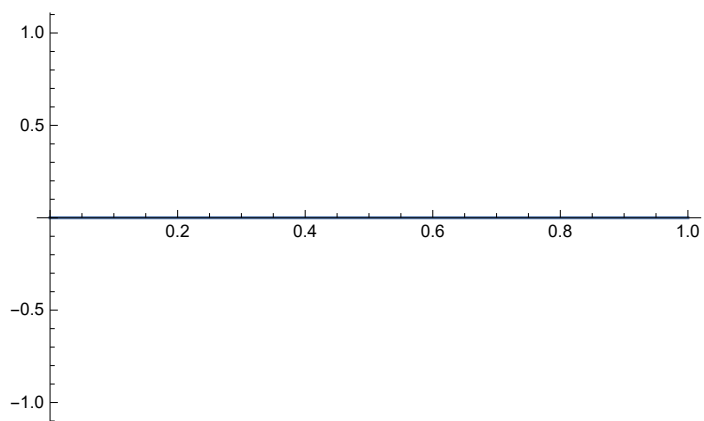

`Plot[Cf[0, 14, 13], {x, 0, 1}]`

[绘图](#)

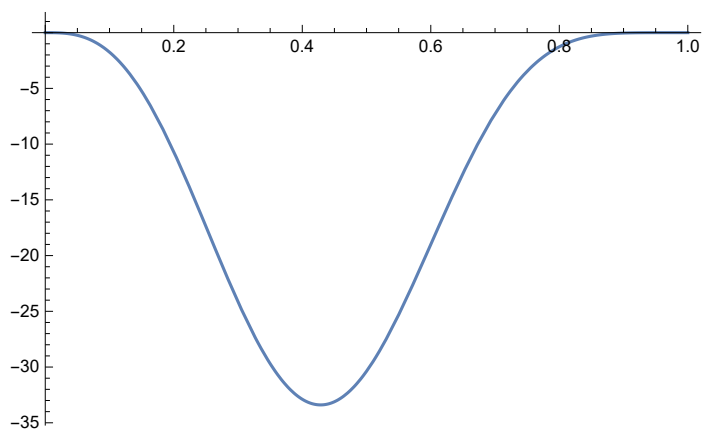

```
Plot[Cf[0, 14, 12], {x, 0, 1}]
```

[绘图](#)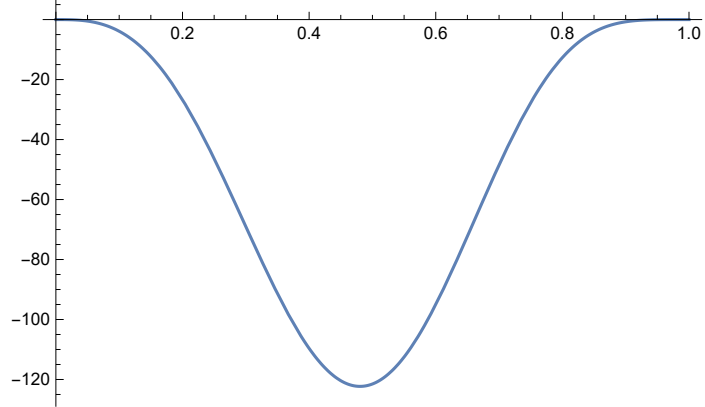

```
Plot[Cf[0, 14, 11], {x, 0, 1}]
```

[绘图](#)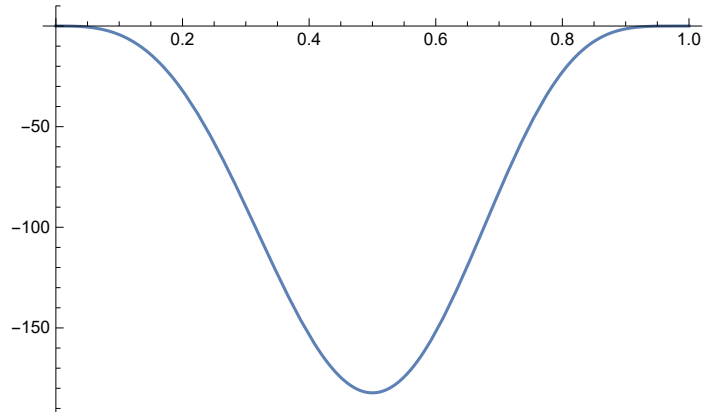

```
Plot[Cf[0, 14, 10], {x, 0, 1}]
```

[绘图](#)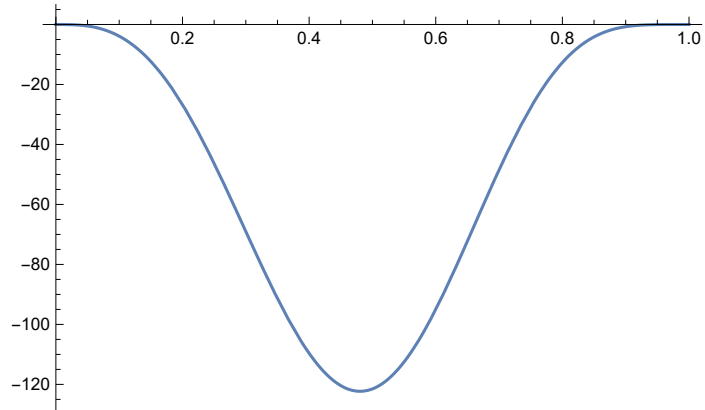

**Plot[Cf[0, 14, 9], {x, 0, 1}]**

[绘图](#)

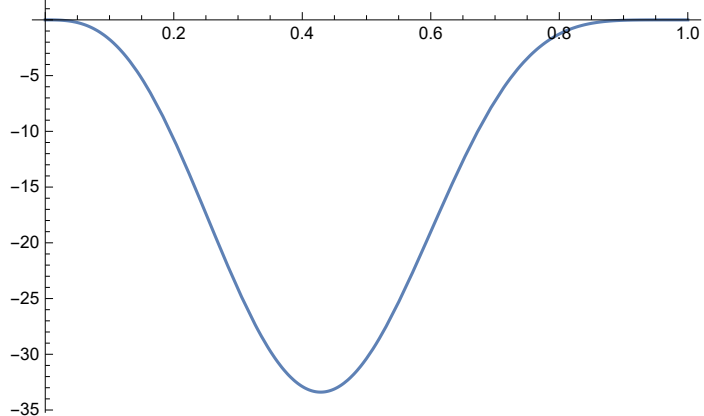

**Plot[Cf[0, 14, 8], {x, 0, 1}]**

[绘图](#)

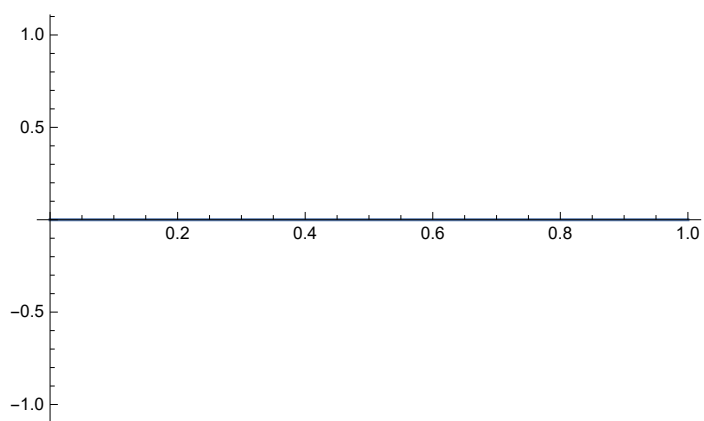

**(\*212th group coefficients r2^0r3^13\*)**

**Plot[Cf[0, 13, 14], {x, 0, 1}]**

[绘图](#)

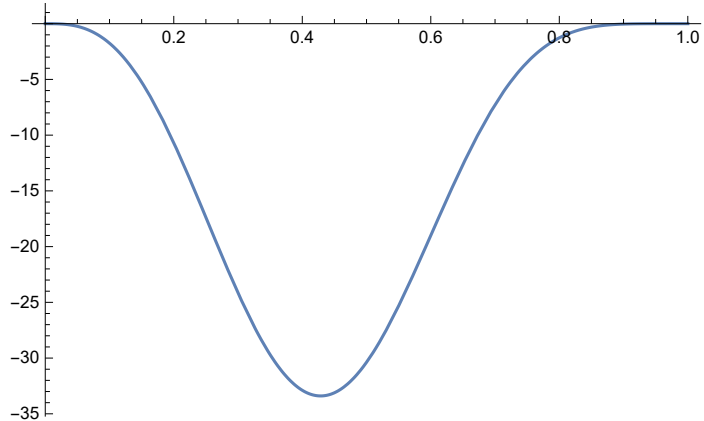

```
Plot[Cf[0, 13, 13], {x, 0, 1}]
```

[绘图](#)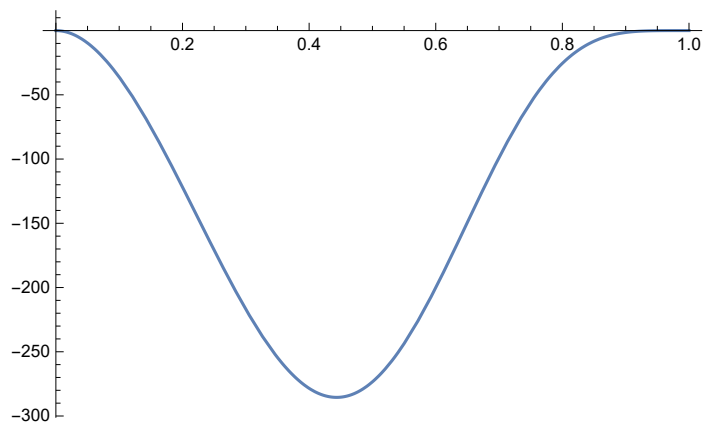

```
Plot[Cf[0, 13, 12], {x, 0, 1}]
```

[绘图](#)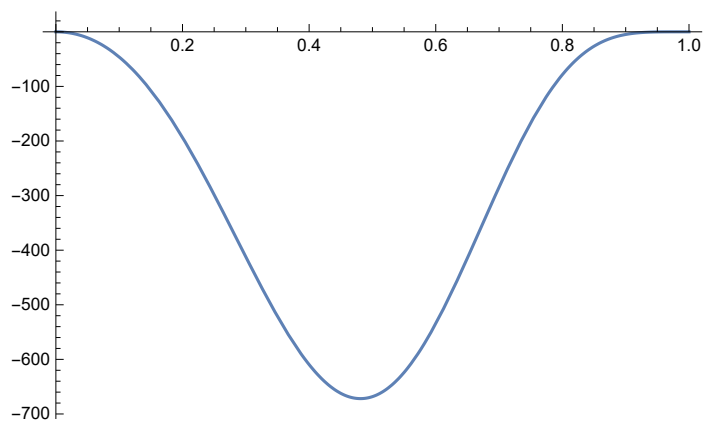

```
Plot[Cf[0, 13, 11], {x, 0, 1}]
```

[绘图](#)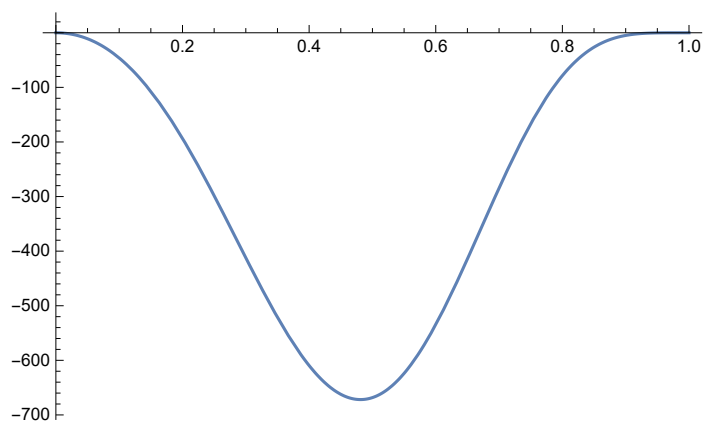



`Plot[Cf[0, 13, 10], {x, 0, 1}]`

[绘图](#)

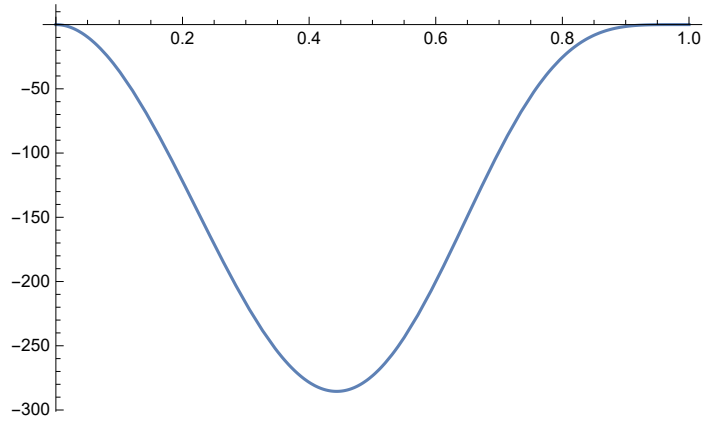

`Plot[Cf[0, 13, 9], {x, 0, 1}]`

[绘图](#)

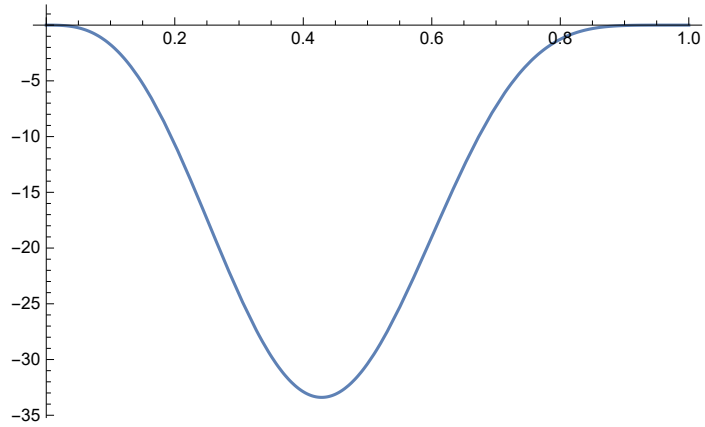

`Plot[Cf[0, 13, 8], {x, 0, 1}]`

[绘图](#)

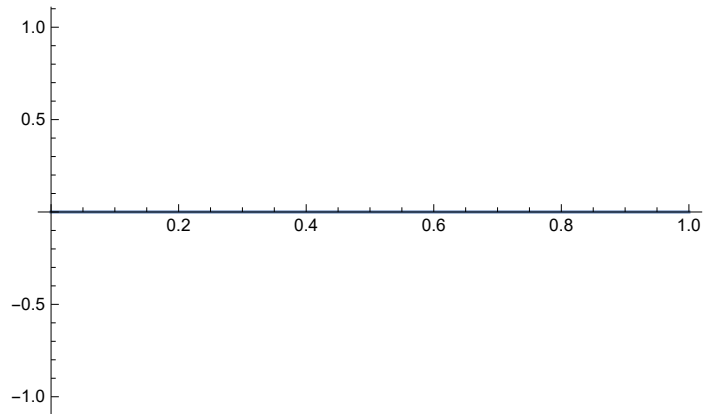

`(*213th group coefficients r2^0r3^12*)`

```
Plot[Cf[0, 12, 14], {x, 0, 1}]
```

[绘图](#)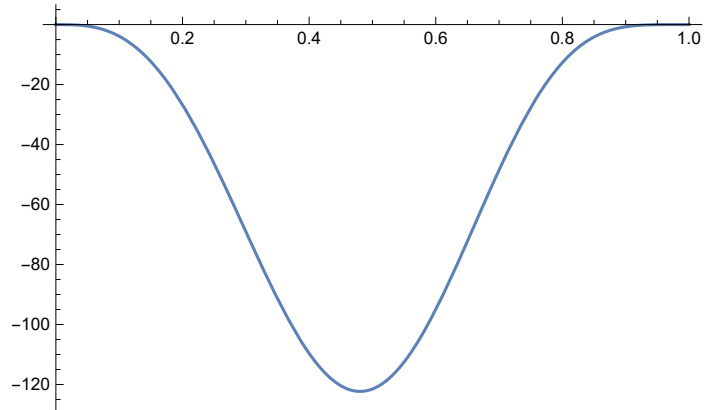

```
Plot[Cf[0, 12, 13], {x, 0, 1}]
```

[绘图](#)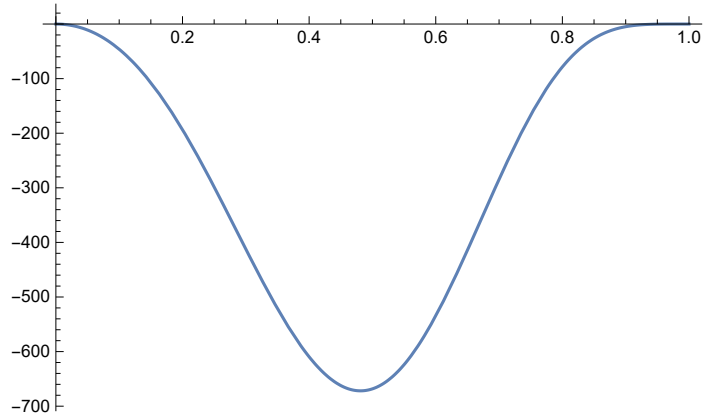

```
Plot[Cf[0, 12, 12], {x, 0, 1}]
```

[绘图](#)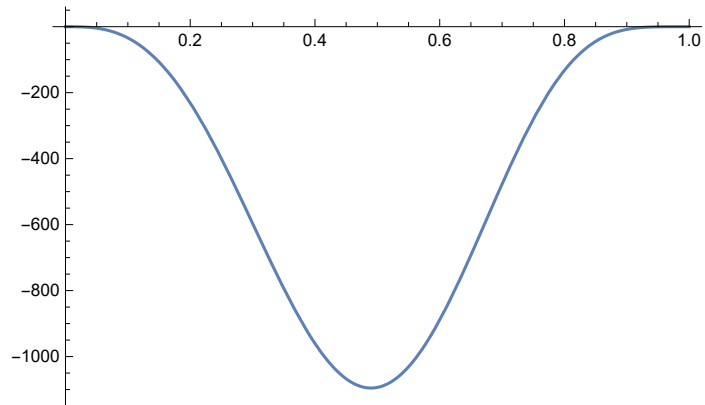

`Plot[Cf[0, 12, 11], {x, 0, 1}]`

[绘图](#)

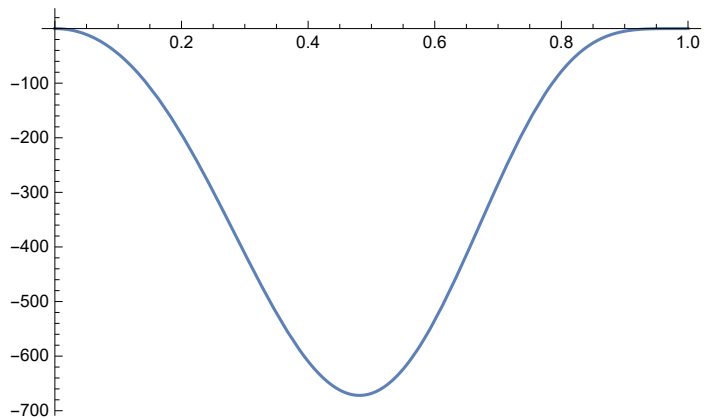

`Plot[Cf[0, 12, 10], {x, 0, 1}]`

[绘图](#)

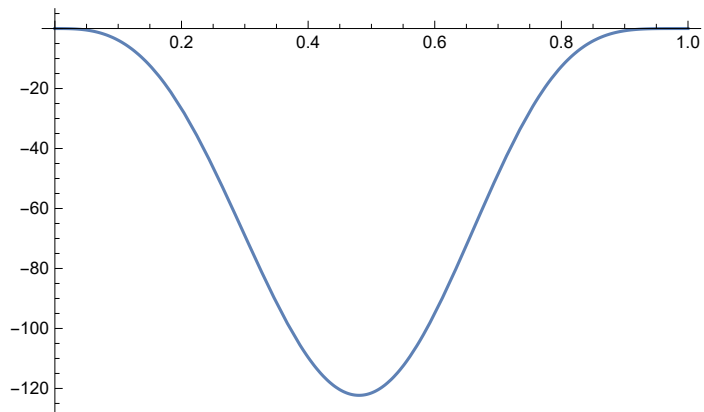

`Plot[Cf[0, 12, 9], {x, 0, 1}]`

[绘图](#)

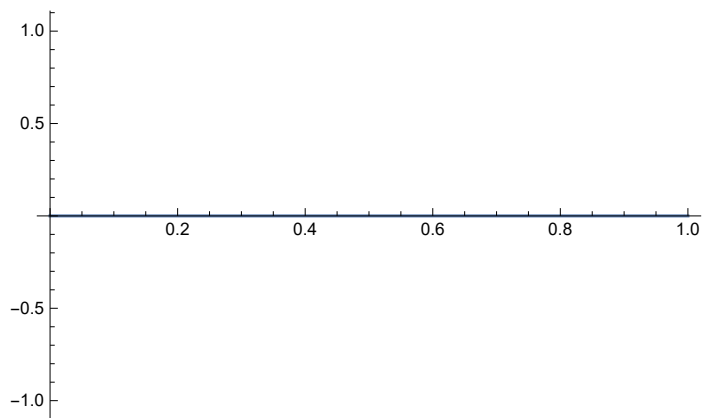

(\*214th group coefficients  $r^2 r^3^{11}$ \*)

```
Plot[Cf[0, 11, 14], {x, 0, 1}]
```

[绘图](#)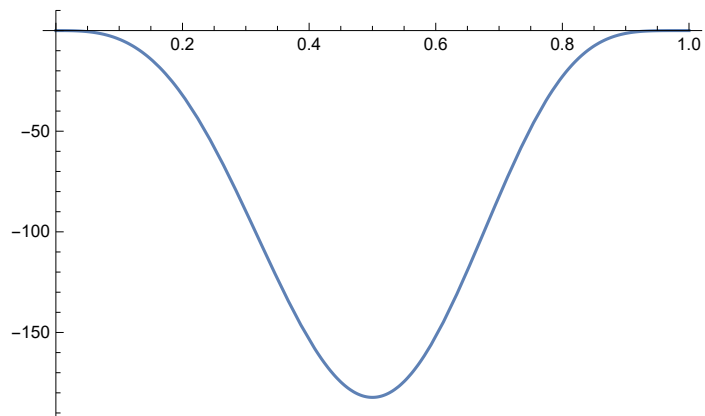

```
Plot[Cf[0, 11, 13], {x, 0, 1}]
```

[绘图](#)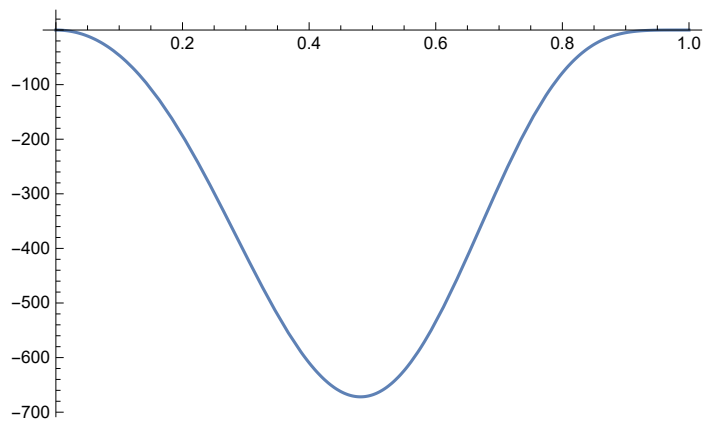

```
Plot[Cf[0, 11, 12], {x, 0, 1}]
```

[绘图](#)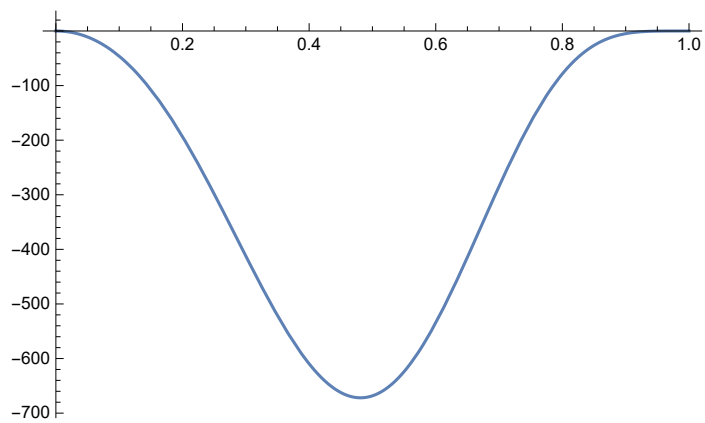

**Plot[Cf[0, 11, 11], {x, 0, 1}]**

[绘图](#)

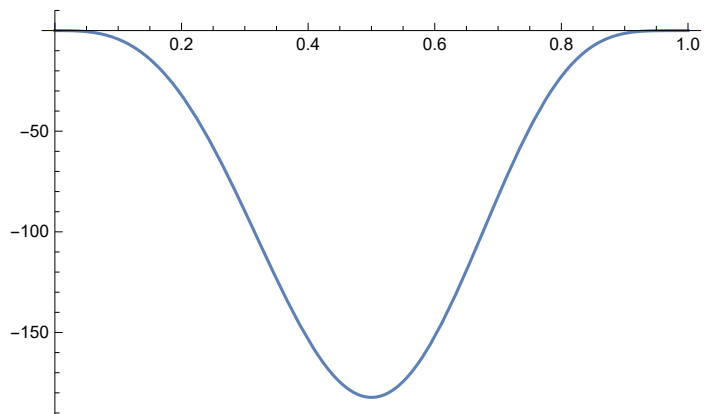

**Plot[Cf[0, 11, 10], {x, 0, 1}]**

[绘图](#)

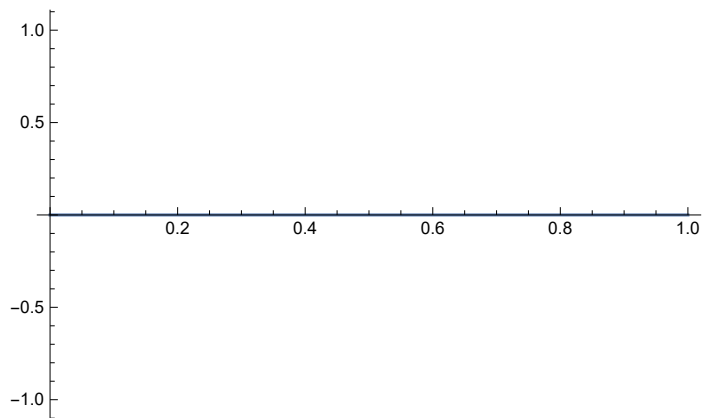

**(\*215th group coefficients r2^0r3^10\*)**

**Plot[Cf[0, 10, 14], {x, 0, 1}]**

[绘图](#)

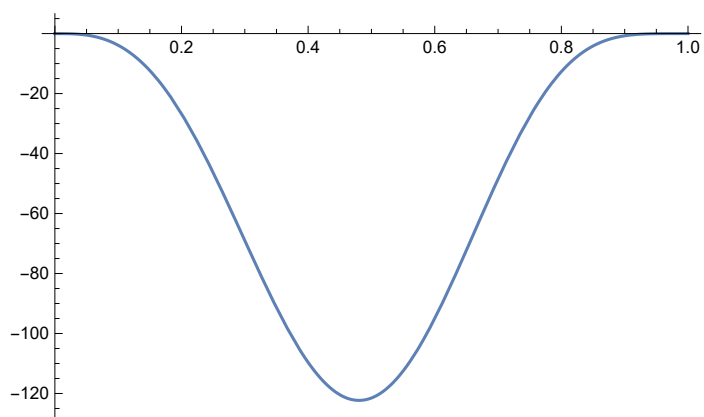

`Plot[Cf[0, 10, 13], {x, 0, 1}]`

[绘图](#)

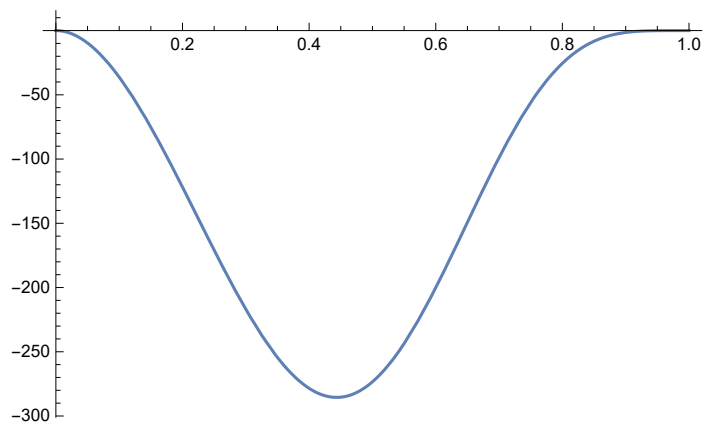

`Plot[Cf[0, 10, 12], {x, 0, 1}]`

[绘图](#)

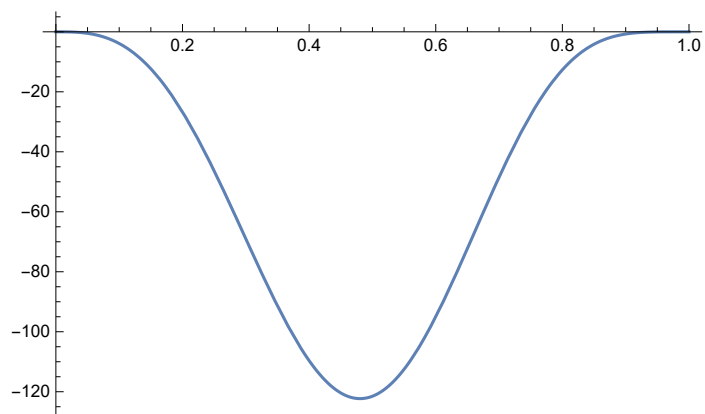

`Plot[Cf[0, 10, 11], {x, 0, 1}]`

[绘图](#)

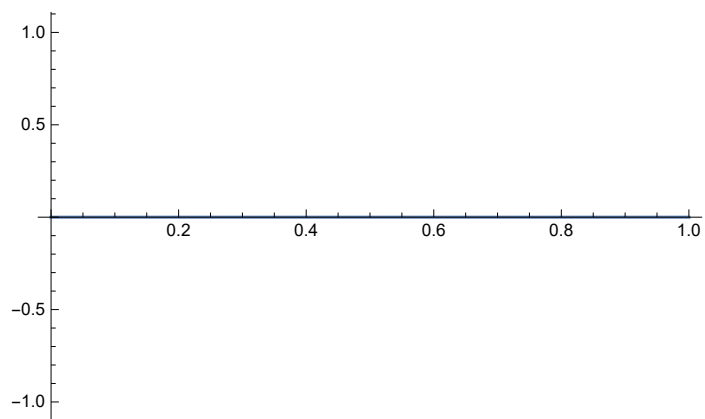

(\*216th group coefficients r2^0r3^9\*)

`Plot[Cf[0, 9, 14], {x, 0, 1}]`

[绘图](#)

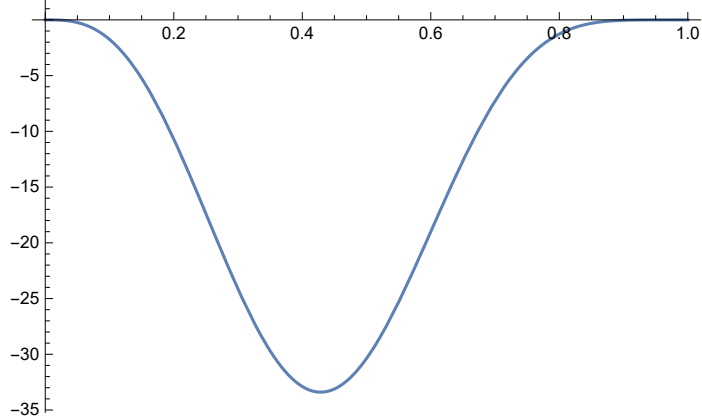

`Plot[Cf[0, 9, 13], {x, 0, 1}]`

[绘图](#)

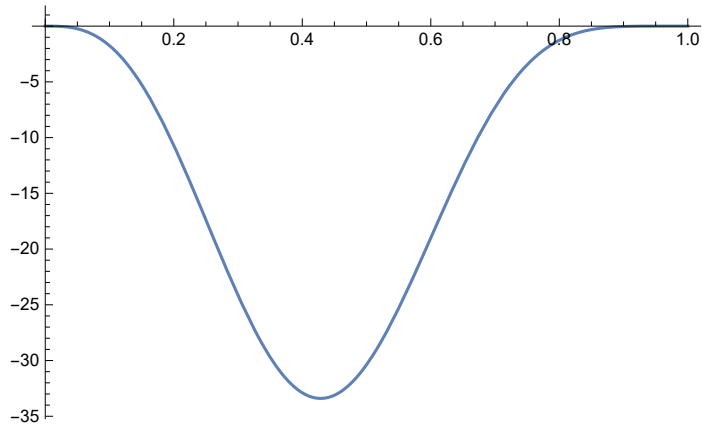

`Plot[Cf[0, 9, 12], {x, 0, 1}]`

[绘图](#)

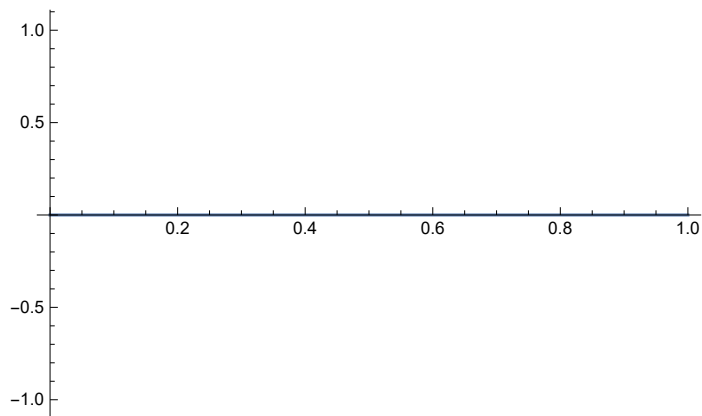

`(*217th group coefficients r2^0r3^8*)`

**Plot[Cf[0, 8, 14], {x, 0, 1}]**

[绘图](#)

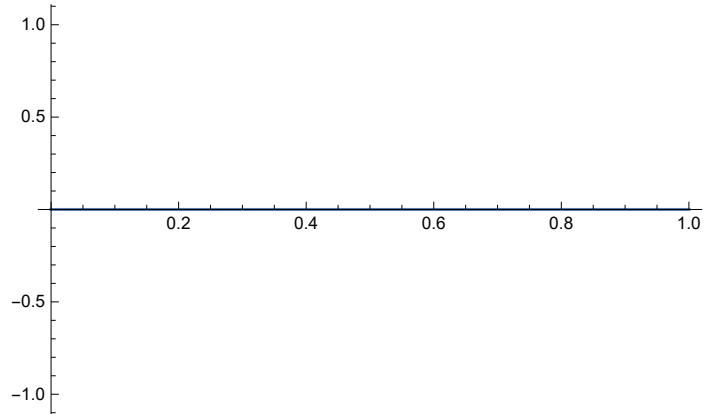

**(\*218th group coefficients r2^0r3^7\*)**

**Plot[Cf[0, 7, 14], {x, 0, 1}]**

[绘图](#)

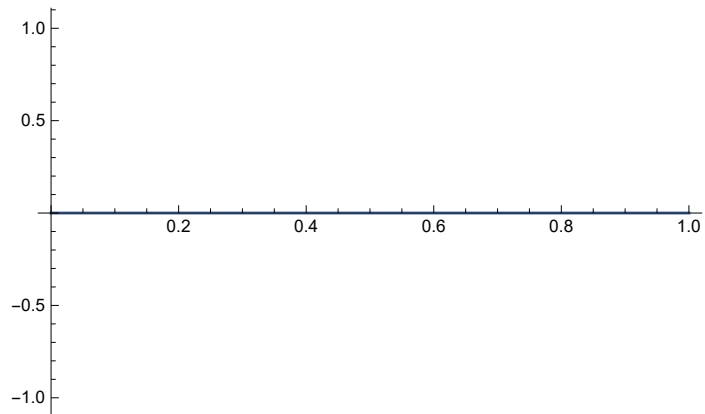

**(\*219th group coefficients r2^0r3^6\*)**

**Plot[Cf[0, 6, 14], {x, 0, 1}]**

[绘图](#)

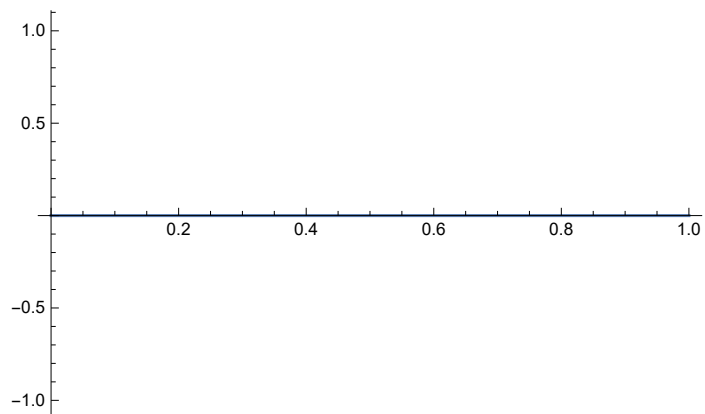

**(\*220th group coefficients r2^0r3^5\*)**



**Plot[Cf[0, 5, 14], {x, 0, 1}]**

[绘图](#)

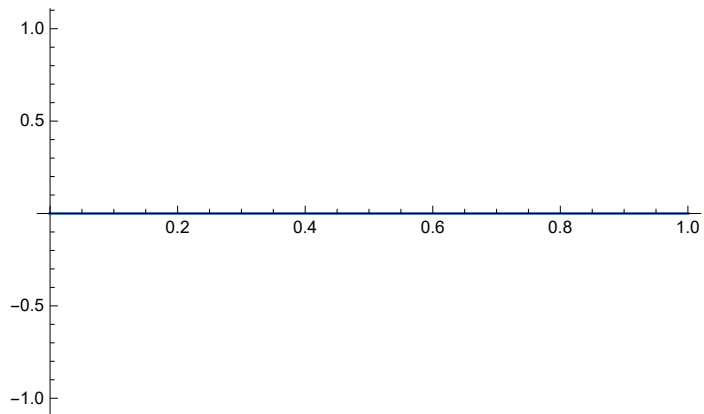

(\*221th group coefficients r2^0r3^4\*)

**Plot[Cf[0, 4, 14], {x, 0, 1}]**

[绘图](#)

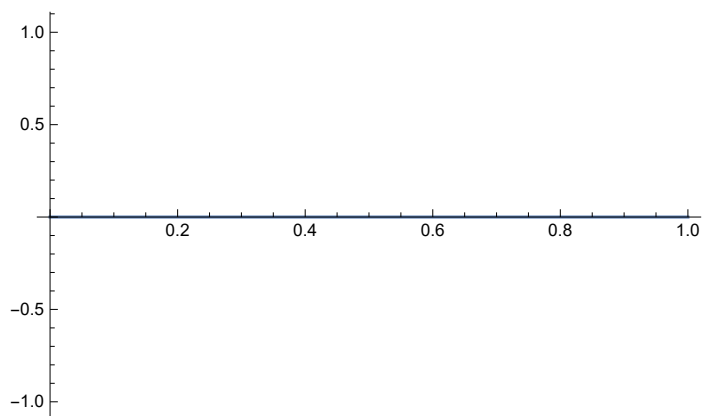

(\*222th group coefficients r2^0r3^3\*)

**Plot[Cf[0, 3, 14], {x, 0, 1}]**

[绘图](#)

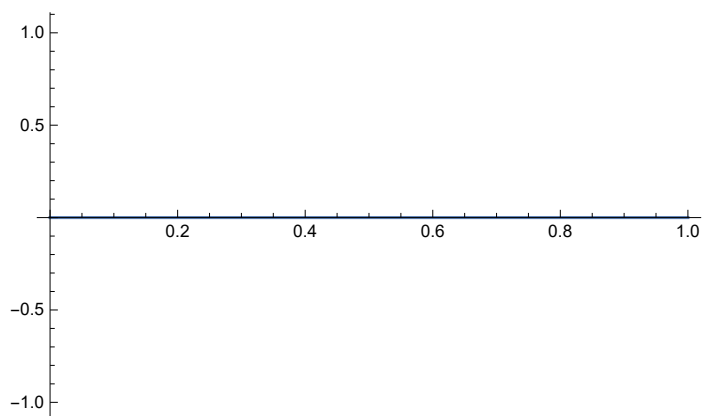

(\*223th group coefficients r2^0r3^2\*)

**Plot[Cf[0, 2, 14], {x, 0, 1}]**

[绘图](#)

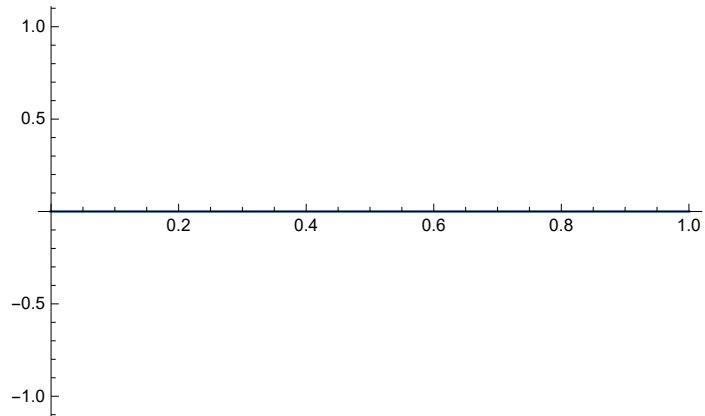

(\*224th group coefficients r2^0r3^1\*)

**Plot[Cf[0, 1, 14], {x, 0, 1}]**

[绘图](#)

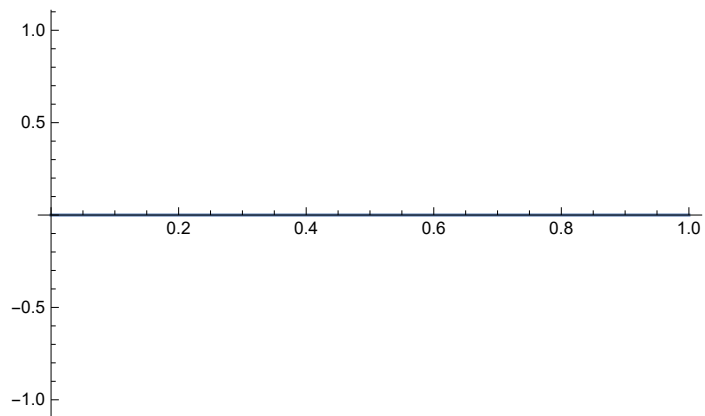

(\*225th group coefficients r2^0r3^0\*)

**Plot[Cf[0, 0, 14], {x, 0, 1}]**

[绘图](#)

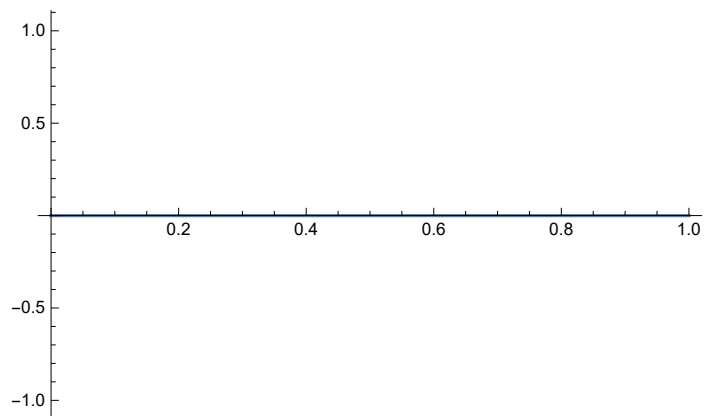

**Coefficient[q12new11, r2, 15]**

[系数](#)

{0, 0}

```
Coefficient[q12new11, r3, 15]
```

```
系数
```

```
{0, 0}
```

```
Coefficient[q12new11, r4, 15]
```

```
系数
```

```
{0, 0}
```

```
(*Now we will give the Explicit expression of coefficients Cf[i,j,k]*)
```

```
此刻
```

```
(*r2^0r^30*)
```

```
Simplify[Cf[0, 0, 0]]
```

```
化简
```

```
0
```

```
Simplify[Cf[0, 0, 1]]
```

```
化简
```

```
0
```

```
Simplify[Cf[0, 0, 2]]
```

```
化简
```

```
0
```

```
Simplify[Cf[0, 0, 3]]
```

```
化简
```

```
0
```

```
Simplify[Cf[0, 0, 4]]
```

```
化简
```

```
0
```

```
Simplify[Cf[0, 0, 5]]
```

```
化简
```

```
0
```

```
Simplify[Cf[0, 0, 6]]
```

```
化简
```

```
0
```

```
Simplify[Cf[0, 0, 7]]
```

```
化简
```

```
0
```

```
Simplify[Cf[0, 0, 8]]
```

```
化简
```

```
0
```

```
Simplify[Cf[0, 0, 9]]
```

```
化简
```

```
0
```

**Simplify[Cf[0, 0, 10]]**

[\[化简\]](#)

0

**Simplify[Cf[0, 0, 11]]**

[\[化简\]](#)

0

**Simplify[Cf[0, 0, 12]]**

[\[化简\]](#)

0

**Simplify[Cf[0, 0, 13]]**

[\[化简\]](#)

0

**Simplify[Cf[0, 0, 14]]**

[\[化简\]](#)

0

**(\*r2^0r3^1\*)**

**Simplify[Cf[0, 1, 0]]**

[\[化简\]](#)

0

**Simplify[Cf[0, 1, 1]]**

[\[化简\]](#)

0

**Simplify[Cf[0, 1, 2]]**

[\[化简\]](#)

0

**Simplify[Cf[0, 1, 3]]**

[\[化简\]](#)

0

**Simplify[Cf[0, 1, 4]]**

[\[化简\]](#)

0

**Simplify[Cf[0, 1, 5]]**

[\[化简\]](#)

0

**Simplify[Cf[0, 1, 6]]**

[\[化简\]](#)

0

**Simplify[Cf[0, 1, 7]]**

[\[化简\]](#)

0

**Simplify[Cf[0, 1, 8]]**

[化简]

0

**Simplify[Cf[0, 1, 9]]**

[化简]

0

**Simplify[Cf[0, 1, 10]]**

[化简]

0

**Simplify[Cf[0, 1, 11]]**

[化简]

0

**Simplify[Cf[0, 1, 12]]**

[化简]

0

**Simplify[Cf[0, 1, 13]]**

[化简]

0

**Simplify[Cf[0, 1, 14]]**

[化简]

0

**Simplify[Cf[0, 1, 15]]**

[化简]

0

**(\*r2^0r3^2\*)**

**Simplify[Cf[0, 2, 0]]**

[化简]

0

**Simplify[Cf[0, 2, 1]]**

[化简]

0

**Simplify[Cf[0, 2, 2]]**

[化简]

0

**Simplify[Cf[0, 2, 3]]**

[化简]

0

**Simplify[Cf[0, 2, 4]]**

[化简]

0

**Simplify[Cf[0, 2, 5]]**

[化简]

0

**Simplify[Cf[0, 2, 6]]**

[化简]

0

**Simplify[Cf[0, 2, 7]]**

[化简]

0

**Simplify[Cf[0, 2, 8]]**

[化简]

0

**Simplify[Cf[0, 2, 9]]**

[化简]

0

**Simplify[Cf[0, 2, 10]]**

[化简]

0

**Simplify[Cf[0, 2, 11]]**

[化简]

0

**Simplify[Cf[0, 2, 12]]**

[化简]

0

**Simplify[Cf[0, 2, 13]]**

[化简]

0

**Simplify[Cf[0, 2, 14]]**

[化简]

0

**(\*r2^0r3^3\*)**

**Simplify[Cf[0, 3, 0]]**

[化简]

0

**Simplify[Cf[0, 3, 1]]**

[化简]

0

**Simplify[Cf[0, 3, 2]]**

[化简]

0

**Simplify[Cf[0, 3, 3]]**

[化简]

0

**Simplify[Cf[0, 3, 4]]**

[化简]

0

**Simplify[Cf[0, 3, 5]]**

[化简]

0

**Simplify[Cf[0, 3, 6]]**

[化简]

0

**Simplify[Cf[0, 3, 7]]**

[化简]

0

**Simplify[Cf[0, 3, 8]]**

[化简]

0

**Simplify[Cf[0, 3, 9]]**

[化简]

0

**Simplify[Cf[0, 3, 10]]**

[化简]

0

**Simplify[Cf[0, 3, 11]]**

[化简]

0

**Simplify[Cf[0, 3, 12]]**

[化简]

0

**Simplify[Cf[0, 3, 13]]**

[化简]

0

**Simplify[Cf[0, 3, 14]]**

[化简]

0

**(\*r2^0r3^4\*)**

**Simplify[Cf[0, 4, 0]]**

[化简]

0

**Simplify[Cf[0, 4, 1]]**

[化简]

0

**Simplify[Cf[0, 4, 2]]**

[化简]

0

**Simplify[Cf[0, 4, 3]]**

[化简]

0

**Simplify[Cf[0, 4, 4]]**

[化简]

0

**Simplify[Cf[0, 4, 5]]**

[化简]

0

**Simplify[Cf[0, 4, 6]]**

[化简]

0

**Simplify[Cf[0, 4, 7]]**

[化简]

0

**Simplify[Cf[0, 4, 8]]**

[化简]

0

**Simplify[Cf[0, 4, 9]]**

[化简]

0

**Simplify[Cf[0, 4, 10]]**

[化简]

0

**Simplify[Cf[0, 4, 11]]**

[化简]

0

**Simplify[Cf[0, 4, 12]]**

[化简]

0

**Simplify[Cf[0, 4, 13]]**

[化简]

0



**Simplify[Cf[0, 4, 14]]**

[化简]

0

**(\*r2^0r3^5\*)**

**Simplify[Cf[0, 5, 0]]**

[化简]

0

**Simplify[Cf[0, 5, 1]]**

[化简]

0

**Simplify[Cf[0, 5, 2]]**

[化简]

0

**Simplify[Cf[0, 5, 3]]**

[化简]

0

**Simplify[Cf[0, 5, 4]]**

[化简]

0

**Simplify[Cf[0, 5, 5]]**

[化简]

0

**Simplify[Cf[0, 5, 6]]**

[化简]

0

**Simplify[Cf[0, 5, 7]]**

[化简]

0

**Simplify[Cf[0, 5, 8]]**

[化简]

0

**Simplify[Cf[0, 5, 9]]**

[化简]

0

**Simplify[Cf[0, 5, 10]]**

[化简]

0

**Simplify[Cf[0, 5, 11]]**

[化简]

0

**Simplify[Cf[0, 5, 12]]**

[化简]

0

**Simplify[Cf[0, 5, 13]]**

[化简]

0

**Simplify[Cf[0, 5, 14]]**

[化简]

0

**(\*r2^0r3^6\*)**

**Simplify[Cf[0, 6, 0]]**

[化简]

0

**Simplify[Cf[0, 6, 1]]**

[化简]

0

**Simplify[Cf[0, 6, 2]]**

[化简]

0

**Simplify[Cf[0, 6, 3]]**

[化简]

0

**Simplify[Cf[0, 6, 4]]**

[化简]

0

**Simplify[Cf[0, 6, 5]]**

[化简]

0

**Simplify[Cf[0, 6, 6]]**

[化简]

0

**Simplify[Cf[0, 6, 7]]**

[化简]

0

**Simplify[Cf[0, 6, 8]]**

[化简]

0

**Simplify[Cf[0, 6, 9]]**

[化简]

0

**Simplify[Cf[0, 6, 10]]**

[化简]

0

**Simplify[Cf[0, 6, 11]]**

[化简]

0

**Simplify[Cf[0, 6, 12]]**

[化简]

0

**Simplify[Cf[0, 6, 13]]**

[化简]

0

**Simplify[Cf[0, 6, 14]]**

[化简]

0

**(\*r2^0r3^7\*)**

**Simplify[Cf[0, 7, 0]]**

[化简]

0

**Simplify[Cf[0, 7, 1]]**

[化简]

0

**Simplify[Cf[0, 7, 2]]**

[化简]

0

**Simplify[Cf[0, 7, 3]]**

[化简]

0

**Simplify[Cf[0, 7, 4]]**

[化简]

0

**Simplify[Cf[0, 7, 5]]**

[化简]

0

**Simplify[Cf[0, 7, 6]]**

[化简]

0

**Simplify[Cf[0, 7, 7]]**

[化简]

0

**Simplify[Cf[0, 7, 8]]**

[化简]

0

**Simplify[Cf[0, 7, 9]]**

[化简]

0

**Simplify[Cf[0, 7, 10]]**

[化简]

0

**Simplify[Cf[0, 7, 11]]**

[化简]

0

**Simplify[Cf[0, 7, 12]]**

[化简]

0

**Simplify[Cf[0, 7, 13]]**

[化简]

0

**Simplify[Cf[0, 7, 14]]**

[化简]

0

**(\*r2^0r3^8\*)**

**Simplify[Cf[0, 8, 0]]**

[化简]

0

**Simplify[Cf[0, 8, 1]]**

[化简]

0

**Simplify[Cf[0, 8, 2]]**

[化简]

0

**Simplify[Cf[0, 8, 3]]**

[化简]

0

**Simplify[Cf[0, 8, 4]]**

[化简]

0

**Simplify[Cf[0, 8, 5]]**

[化简]

0

**Simplify[Cf[0, 8, 6]]**

[化简]

0

**Simplify[Cf[0, 8, 7]]**

[化简]

0

**Simplify[Cf[0, 8, 8]]**

[化简]

0

**Simplify[Cf[0, 8, 9]]**

[化简]

0

**Simplify[Cf[0, 8, 10]]**

[化简]

0

**Simplify[Cf[0, 8, 11]]**

[化简]

0

**Simplify[Cf[0, 8, 12]]**

[化简]

0

**Simplify[Cf[0, 8, 13]]**

[化简]

0

**Simplify[Cf[0, 8, 14]]**

[化简]

0

**(\*r2^0r3^9\*)**

**Simplify[Cf[0, 9, 0]]**

[化简]

0

**Simplify[Cf[0, 9, 1]]**

[化简]

0

**Simplify[Cf[0, 9, 2]]**

[化简]

0

**Simplify[Cf[0, 9, 3]]**

[化简]

0

**Simplify[Cf[0, 9, 4]]**

[化简]

0

**Simplify[Cf[0, 9, 5]]**

[化简]

0

**Simplify[Cf[0, 9, 6]]**

[化简]

0

**Simplify[Cf[0, 9, 7]]**

[化简]

0

**Simplify[Cf[0, 9, 8]]**

[化简]

0

**Simplify[Cf[0, 9, 9]]**

[化简]

0

**Simplify[Cf[0, 9, 10]]**

[化简]

0

**Simplify[Cf[0, 9, 11]]**

[化简]

0

**Simplify[Cf[0, 9, 12]]**

[化简]

0

**Simplify[Cf[0, 9, 13]]**

[化简]

$-2048 (-1+x) x^3 (-1+x^2)^5$

**Simplify[Cf[0, 9, 14]]**

[化简]

$-2048 (-1+x) x^3 (-1+x^2)^5$

(\*r2^0r3^10\*)

**Simplify[Cf[0, 10, 0]]**

[化简]

0

**Simplify[Cf[0, 10, 1]]**

[化简]

0

**Simplify[Cf[0, 10, 2]]**

[化简]

0

**Simplify[Cf[0, 10, 3]]**

[化简]

0

**Simplify[Cf[0, 10, 4]]**

[化简]

0

**Simplify[Cf[0, 10, 5]]**

[化简]

0

**Simplify[Cf[0, 10, 6]]**

[化简]

0

**Simplify[Cf[0, 10, 7]]**

[化简]

0

**Simplify[Cf[0, 10, 8]]**

[化简]

0

**Simplify[Cf[0, 10, 9]]**

[化简]

0

**Simplify[Cf[0, 10, 10]]**

[化简]

0

**Simplify[Cf[0, 10, 11]]**

[化简]

0

**Simplify[Cf[0, 10, 12]]**

[化简]

$4096 x^3 (-1 + x^2)^5$

**Simplify[Cf[0, 10, 13]]**

[化简]

$-4096 x^2 (-1 + x^2)^5 (-1 + x - 3 x^2 + x^3)$

**Simplify[Cf[0, 10, 14]]**

[化简]

$4096 x^3 (-1 + x^2)^5$

( $\ast r2^0 r3^{11}$ )

**Simplify[Cf[0, 11, 0]]**

[化简]

0

**Simplify[Cf[0, 11, 1]]**

[化简]

0

**Simplify[Cf[0, 11, 2]]**

[化简]

0

**Simplify[Cf[0, 11, 3]]**

[化简]

0

**Simplify[Cf[0, 11, 4]]**

[化简]

0

**Simplify[Cf[0, 11, 5]]**

[化简]

0

**Simplify[Cf[0, 11, 6]]**

[化简]

0

**Simplify[Cf[0, 11, 7]]**

[化简]

0

**Simplify[Cf[0, 11, 8]]**

[化简]

0

**Simplify[Cf[0, 11, 9]]**

[化简]

0

**Simplify[Cf[0, 11, 10]]**

[化简]

0

**Simplify[Cf[0, 11, 11]]**

[化简]

$4096 x^3 (1 + x) (-1 + x^2)^5$

**Simplify[Cf[0, 11, 12]]**

[化简]

$2048 x^2 (-1 + x^2)^5 (2 + 3 x + 7 x^2 + 2 x^3)$



**Simplify[Cf[0, 11, 13]]**

[化简]

$$2048 x^2 (-1 + x^2)^5 (2 + 3 x + 7 x^2 + 2 x^3)$$

**Simplify[Cf[0, 11, 14]]**

[化简]

$$4096 x^3 (1 + x) (-1 + x^2)^5$$

**(\*r2^0r3^12\*)**

**Simplify[Cf[0, 12, 0]]**

[化简]

0

**Simplify[Cf[0, 12, 1]]**

[化简]

0

**Simplify[Cf[0, 12, 2]]**

[化简]

0

**Simplify[Cf[0, 12, 3]]**

[化简]

0

**Simplify[Cf[0, 12, 4]]**

[化简]

0

**Simplify[Cf[0, 12, 5]]**

[化简]

0

**Simplify[Cf[0, 12, 6]]**

[化简]

0

**Simplify[Cf[0, 12, 7]]**

[化简]

0

**Simplify[Cf[0, 12, 8]]**

[化简]

0

**Simplify[Cf[0, 12, 9]]**

[化简]

0

**Simplify[Cf[0, 12, 10]]**

[\[化简\]](#)

$$4096 x^3 (-1 + x^2)^5$$

**Simplify[Cf[0, 12, 11]]**

[\[化简\]](#)

$$2048 x^2 (-1 + x^2)^5 (2 + 3 x + 7 x^2 + 2 x^3)$$

**Simplify[Cf[0, 12, 12]]**

[\[化简\]](#)

$$12288 x^3 (-1 + x^2)^5 (3 - x + 2 x^2)$$

**Simplify[Cf[0, 12, 13]]**

[\[化简\]](#)

$$2048 x^2 (-1 + x^2)^5 (2 + 3 x + 7 x^2 + 2 x^3)$$

**Simplify[Cf[0, 12, 14]]**

[\[化简\]](#)

$$4096 x^3 (-1 + x^2)^5$$

**(\*r2^0r3^13\*)**

**Simplify[Cf[0, 13, 0]]**

[\[化简\]](#)

0

**Simplify[Cf[0, 13, 1]]**

[\[化简\]](#)

0

**Simplify[Cf[0, 13, 2]]**

[\[化简\]](#)

0

**Simplify[Cf[0, 13, 3]]**

[\[化简\]](#)

0

**Simplify[Cf[0, 13, 4]]**

[\[化简\]](#)

0

**Simplify[Cf[0, 13, 5]]**

[\[化简\]](#)

0

**Simplify[Cf[0, 13, 6]]**

[\[化简\]](#)

0

**Simplify[Cf[0, 13, 7]]**

[\[化简\]](#)

0

**Simplify[Cf[0, 13, 8]]**

[\[化简\]](#)

0

**Simplify[Cf[0, 13, 9]]**

[\[化简\]](#)

$$-2048 (-1+x) x^3 (-1+x^2)^5$$

**Simplify[Cf[0, 13, 10]]**

[\[化简\]](#)

$$-4096 x^2 (-1+x^2)^5 (-1+x-3x^2+x^3)$$

**Simplify[Cf[0, 13, 11]]**

[\[化简\]](#)

$$2048 x^2 (-1+x^2)^5 (2+3x+7x^2+2x^3)$$

**Simplify[Cf[0, 13, 12]]**

[\[化简\]](#)

$$2048 x^2 (-1+x^2)^5 (2+3x+7x^2+2x^3)$$

**Simplify[Cf[0, 13, 13]]**

[\[化简\]](#)

$$-4096 x^2 (-1+x^2)^5 (-1+x-3x^2+x^3)$$

**Simplify[Cf[0, 13, 14]]**

[\[化简\]](#)

$$-2048 (-1+x) x^3 (-1+x^2)^5$$

**(\*r2^0r3^14\*)**

**Simplify[Cf[0, 14, 0]]**

[\[化简\]](#)

0

**Simplify[Cf[0, 14, 1]]**

[\[化简\]](#)

0

**Simplify[Cf[0, 14, 2]]**

[\[化简\]](#)

0

**Simplify[Cf[0, 14, 3]]**

[\[化简\]](#)

0

**Simplify[Cf[0, 14, 4]]**

[化简]

0

**Simplify[Cf[0, 14, 5]]**

[化简]

0

**Simplify[Cf[0, 14, 6]]**

[化简]

0

**Simplify[Cf[0, 14, 7]]**

[化简]

0

**Simplify[Cf[0, 14, 8]]**

[化简]

0

**Simplify[Cf[0, 14, 9]]**

[化简]

$-2048 (-1+x) x^3 (-1+x^2)^5$

**Simplify[Cf[0, 14, 10]]**

[化简]

$4096 x^3 (-1+x^2)^5$

**Simplify[Cf[0, 14, 11]]**

[化简]

$4096 x^3 (1+x) (-1+x^2)^5$

**Simplify[Cf[0, 14, 12]]**

[化简]

$4096 x^3 (-1+x^2)^5$

**Simplify[Cf[0, 14, 13]]**

[化简]

$-2048 (-1+x) x^3 (-1+x^2)^5$

**Simplify[Cf[0, 14, 14]]**

[化简]

0

**(\*r2^1r3^0\*)**

**Simplify[Cf[1, 0, 0]]**

[化简]

0

**Simplify[Cf[1, 0, 1]]**

[化简]

0

**Simplify[Cf[1, 0, 2]]**

[化简]

0

**Simplify[Cf[1, 0, 3]]**

[化简]

0

**Simplify[Cf[1, 0, 4]]**

[化简]

0

**Simplify[Cf[1, 0, 5]]**

[化简]

0

**Simplify[Cf[1, 0, 6]]**

[化简]

0

**Simplify[Cf[1, 0, 7]]**

[化简]

0

**Simplify[Cf[1, 0, 8]]**

[化简]

0

**Simplify[Cf[1, 0, 9]]**

[化简]

0

**Simplify[Cf[1, 0, 10]]**

[化简]

0

**Simplify[Cf[1, 0, 11]]**

[化简]

0

**Simplify[Cf[1, 0, 12]]**

[化简]

0

**Simplify[Cf[1, 0, 13]]**

[化简]

0

**Simplify[Cf[1, 0, 14]]**

[化简]

0

**(\*r2^1r3^1\*)**

**Simplify[Cf[1, 1, 0]]**

[化简]

0

**Simplify[Cf[1, 1, 1]]**

[化简]

0

**Simplify[Cf[1, 1, 2]]**

[化简]

0

**Simplify[Cf[1, 1, 3]]**

[化简]

0

**Simplify[Cf[1, 1, 4]]**

[化简]

0

**Simplify[Cf[1, 1, 5]]**

[化简]

0

**Simplify[Cf[1, 1, 6]]**

[化简]

0

**Simplify[Cf[1, 1, 7]]**

[化简]

0

**Simplify[Cf[1, 1, 8]]**

[化简]

0

**Simplify[Cf[1, 1, 9]]**

[化简]

0

**Simplify[Cf[1, 1, 10]]**

[化简]

0

**Simplify[Cf[1, 1, 11]]**

[化简]

0

**Simplify[Cf[1, 1, 12]]**

[化简]

0

**Simplify[Cf[1, 1, 13]]**

[化简]

0

**Simplify[Cf[1, 1, 14]]**

[化简]

0

**(\*r2^1r3^2\*)**

**Simplify[Cf[1, 2, 0]]**

[化简]

0

**Simplify[Cf[1, 2, 1]]**

[化简]

0

**Simplify[Cf[1, 2, 2]]**

[化简]

0

**Simplify[Cf[1, 2, 3]]**

[化简]

0

**Simplify[Cf[1, 2, 4]]**

[化简]

0

**Simplify[Cf[1, 2, 5]]**

[化简]

0

**Simplify[Cf[1, 2, 6]]**

[化简]

0

**Simplify[Cf[1, 2, 7]]**

[化简]

**Simplify[Cf[1, 2, 8]]**

[化简]

**Simplify[Cf[1, 2, 9]]**

[化简]

**Simplify[Cf[1, 2, 10]]**

[化简]

**Simplify[Cf[1, 2, 11]]**

[化简]

**Simplify[Cf[1, 2, 12]]**

[化简]

**Simplify[Cf[1, 2, 13]]**

[化简]

**Simplify[Cf[1, 2, 14]]**

[化简]

**(\*r2^1r3^3\*)**

**Simplify[Cf[1, 3, 0]]**

[化简]

0

**Simplify[Cf[1, 3, 1]]**

[化简]

0

**Simplify[Cf[1, 3, 2]]**

[化简]

0

**Simplify[Cf[1, 3, 3]]**

[化简]

0

**Simplify[Cf[1, 3, 4]]**

[化简]

0

**Simplify[Cf[1, 3, 5]]**

[化简]

0

**Simplify[Cf[1, 3, 6]]**

[化简]

0

**Simplify[Cf[1, 3, 7]]**

[化简]

0

**Simplify[Cf[1, 3, 8]]**

[化简]

0

**Simplify[Cf[1, 3, 9]]**

[化简]

0



**Simplify[Cf[1, 3, 10]]**

[化简]

0

**Simplify[Cf[1, 3, 11]]**

[化简]

0

**Simplify[Cf[1, 3, 12]]**

[化简]

0

**Simplify[Cf[1, 3, 13]]**

[化简]

0

**Simplify[Cf[1, 3, 14]]**

[化简]

0

**(\*r2^1r3^4\*)**

**Simplify[Cf[1, 4, 0]]**

[化简]

0

**Simplify[Cf[1, 4, 1]]**

[化简]

0

**Simplify[Cf[1, 4, 2]]**

[化简]

0

**Simplify[Cf[1, 4, 3]]**

[化简]

0

**Simplify[Cf[1, 4, 4]]**

[化简]

0

**Simplify[Cf[1, 4, 5]]**

[化简]

0

**Simplify[Cf[1, 4, 6]]**

[化简]

0

**Simplify[Cf[1, 4, 7]]**

[化简]

0

**Simplify[Cf[1, 4, 8]]**

[化简]

0

**Simplify[Cf[1, 4, 9]]**

[化简]

0

**Simplify[Cf[1, 4, 10]]**

[化简]

0

**Simplify[Cf[1, 4, 11]]**

[化简]

0

**Simplify[Cf[1, 4, 12]]**

[化简]

0

**Simplify[Cf[1, 4, 13]]**

[化简]

0

**Simplify[Cf[1, 4, 14]]**

[化简]

0

**(\*r2^1r3^5\*)**

**Simplify[Cf[1, 5, 0]]**

[化简]

0

**Simplify[Cf[1, 5, 1]]**

[化简]

0

**Simplify[Cf[1, 5, 2]]**

[化简]

0

**Simplify[Cf[1, 5, 3]]**

[化简]

0

**Simplify[Cf[1, 5, 4]]**

[化简]

0

**Simplify[Cf[1, 5, 5]]**

[化简]

0

**Simplify[Cf[1, 5, 6]]**

[化简]

0

**Simplify[Cf[1, 5, 7]]**

[化简]

0

**Simplify[Cf[1, 5, 8]]**

[化简]

0

**Simplify[Cf[1, 5, 9]]**

[化简]

0

**Simplify[Cf[1, 5, 10]]**

[化简]

0

**Simplify[Cf[1, 5, 11]]**

[化简]

0

**Simplify[Cf[1, 5, 12]]**

[化简]

0

**Simplify[Cf[1, 5, 13]]**

[化简]

0

**Simplify[Cf[1, 5, 14]]**

[化简]

0

**Simplify[Cf[1, 5, 15]]**

[化简]

0

**(\*r2^1r3^6\*)**

**Simplify[Cf[1, 6, 0]]**

[化简]

0

**Simplify[Cf[1, 6, 1]]**

[化简]

0

**Simplify[Cf[1, 6, 2]]**

[化简]

0

**Simplify[Cf[1, 6, 3]]**

[\[化简\]](#)

0

**Simplify[Cf[1, 6, 4]]**

[\[化简\]](#)

0

**Simplify[Cf[1, 6, 5]]**

[\[化简\]](#)

0

**Simplify[Cf[1, 6, 6]]**

[\[化简\]](#)

0

**Simplify[Cf[1, 6, 7]]**

[\[化简\]](#)

0

**Simplify[Cf[1, 6, 8]]**

[\[化简\]](#)

0

**Simplify[Cf[1, 6, 9]]**

[\[化简\]](#)

0

**Simplify[Cf[1, 6, 10]]**

[\[化简\]](#)

0

**Simplify[Cf[1, 6, 11]]**

[\[化简\]](#)

0

**Simplify[Cf[1, 6, 12]]**

[\[化简\]](#)

0

**Simplify[Cf[1, 6, 13]]**

[\[化简\]](#)

0

**Simplify[Cf[1, 6, 14]]**

[\[化简\]](#)

0

**(\*r2^1r3^7\*)**

**Simplify[Cf[1, 7, 0]]**

[\[化简\]](#)

0

**Simplify[Cf[1, 7, 1]]**

[化简]

0

**Simplify[Cf[1, 7, 2]]**

[化简]

0

**Simplify[Cf[1, 7, 3]]**

[化简]

0

**Simplify[Cf[1, 7, 4]]**

[化简]

0

**Simplify[Cf[1, 7, 5]]**

[化简]

0

**Simplify[Cf[1, 7, 6]]**

[化简]

0

**Simplify[Cf[1, 7, 7]]**

[化简]

0

**Simplify[Cf[1, 7, 8]]**

[化简]

0

**Simplify[Cf[1, 7, 9]]**

[化简]

0

**Simplify[Cf[1, 7, 10]]**

[化简]

0

**Simplify[Cf[1, 7, 11]]**

[化简]

0

**Simplify[Cf[1, 7, 12]]**

[化简]

0

**Simplify[Cf[1, 7, 13]]**

[化简]

0

**Simplify[Cf[1, 7, 14]]**

[化简]

0

**(\*r2^1r3^8\*)**

**Simplify[Cf[1, 8, 0]]**

[化简]

0

**Simplify[Cf[1, 8, 1]]**

[化简]

0

**Simplify[Cf[1, 8, 2]]**

[化简]

0

**Simplify[Cf[1, 8, 3]]**

[化简]

0

**Simplify[Cf[1, 8, 4]]**

[化简]

0

**Simplify[Cf[1, 8, 5]]**

[化简]

0

**Simplify[Cf[1, 8, 6]]**

[化简]

0

**Simplify[Cf[1, 8, 7]]**

[化简]

0

**Simplify[Cf[1, 8, 8]]**

[化简]

0

**Simplify[Cf[1, 8, 9]]**

[化简]

0

**Simplify[Cf[1, 8, 10]]**

[化简]

0

**Simplify[Cf[1, 8, 11]]**

[化简]

0

**Simplify[Cf[1, 8, 12]]**

[化简]

0

**Simplify[Cf[1, 8, 13]]**

[化简]

$6144 (-1 + x)^4 x^3 (1 + x)^5 (-1 + x^2)$

**Simplify[Cf[1, 8, 14]]**

[化简]

$6144 (-1 + x)^4 x^3 (1 + x)^5 (-1 + x^2)$

(\*r2^1r3^9\*)

**Simplify[Cf[1, 9, 0]]**

[化简]

0

**Simplify[Cf[1, 9, 1]]**

[化简]

0

**Simplify[Cf[1, 9, 2]]**

[化简]

0

**Simplify[Cf[1, 9, 3]]**

[化简]

0

**Simplify[Cf[1, 9, 4]]**

[化简]

0

**Simplify[Cf[1, 9, 5]]**

[化简]

0

**Simplify[Cf[1, 9, 6]]**

[化简]

0

**Simplify[Cf[1, 9, 7]]**

[化简]

0

**Simplify[Cf[1, 9, 8]]**

[化简]

0

**Simplify[Cf[1, 9, 9]]**

[化简]

0

**Simplify[Cf[1, 9, 10]]**

[化简]

0

**Simplify[Cf[1, 9, 11]]**

[化简]

0

**Simplify[Cf[1, 9, 12]]**

[化简]

$$-2048 (-1+x)^4 x^2 (1+x)^5 (2-3x+30x^2-21x^3+4x^4)$$

**Simplify[Cf[1, 9, 13]]**

[化简]

$$8192 (-1+x)^4 x^2 (1+x)^5 (-2+3x-13x^2+6x^3)$$

**Simplify[Cf[1, 9, 14]]**

[化简]

$$-2048 (-1+x)^4 x^2 (1+x)^5 (2-3x+30x^2-21x^3+4x^4)$$

**(\*r2^1r3^10\*)**

**Simplify[Cf[1, 10, 0]]**

[化简]

0

**Simplify[Cf[1, 10, 1]]**

[化简]

0

**Simplify[Cf[1, 10, 2]]**

[化简]

0

**Simplify[Cf[1, 10, 3]]**

[化简]

0

**Simplify[Cf[1, 10, 4]]**

[化简]

0

**Simplify[Cf[1, 10, 5]]**

[化简]

0

**Simplify[Cf[1, 10, 6]]**

[化简]

0

**Simplify[Cf[1, 10, 7]]**

[化简]

0



**Simplify[Cf[1, 10, 8]]**

[\[化简\]](#)

0

**Simplify[Cf[1, 10, 9]]**

[\[化简\]](#)

0

**Simplify[Cf[1, 10, 10]]**

[\[化简\]](#)

0

**Simplify[Cf[1, 10, 11]]**

[\[化简\]](#)

$$4096 (-1+x)^4 x^2 (1+x)^5 (-1-2x-11x^2-8x^3+2x^4)$$

**Simplify[Cf[1, 10, 12]]**

[\[化简\]](#)

$$-2048 (-1+x)^4 x (1+x)^5 (4-12x+75x^2-52x^3+165x^4-56x^5+8x^6)$$

**Simplify[Cf[1, 10, 13]]**

[\[化简\]](#)

$$-2048 (-1+x)^4 x (1+x)^5 (4-12x+75x^2-52x^3+165x^4-56x^5+8x^6)$$

**Simplify[Cf[1, 10, 14]]**

[\[化简\]](#)

$$4096 (-1+x)^4 x^2 (1+x)^5 (-1-2x-11x^2-8x^3+2x^4)$$

**(\*r2^1r3^11\*)**

**Simplify[Cf[1, 11, 0]]**

[\[化简\]](#)

0

**Simplify[Cf[1, 11, 1]]**

[\[化简\]](#)

0

**Simplify[Cf[1, 11, 2]]**

[\[化简\]](#)

0

**Simplify[Cf[1, 11, 3]]**

[\[化简\]](#)

0

**Simplify[Cf[1, 11, 4]]**

[\[化简\]](#)

0

**Simplify[Cf[1, 11, 5]]**

[\[化简\]](#)

0

**Simplify[Cf[1, 11, 6]]**

[\[化简\]](#)

0

**Simplify[Cf[1, 11, 7]]**

[\[化简\]](#)

0

**Simplify[Cf[1, 11, 8]]**

[\[化简\]](#)

0

**Simplify[Cf[1, 11, 9]]**

[\[化简\]](#)

0

**Simplify[Cf[1, 11, 10]]**

[\[化简\]](#)

$$4096 (-1+x)^4 x^2 (1+x)^5 (-1-2x-11x^2-8x^3+2x^4)$$

**Simplify[Cf[1, 11, 11]]**

[\[化简\]](#)

$$8192 (-1+x)^4 x^2 (1+x)^5 (-6+8x-41x^2-3x^3-16x^4+4x^5)$$

**Simplify[Cf[1, 11, 12]]**

[\[化简\]](#)

$$4096 (-1+x)^4 x (1+x)^5 (-2-4x-15x^2-84x^3-23x^4-60x^5+12x^6)$$

**Simplify[Cf[1, 11, 13]]**

[\[化简\]](#)

$$8192 (-1+x)^4 x^2 (1+x)^5 (-6+8x-41x^2-3x^3-16x^4+4x^5)$$

**Simplify[Cf[1, 11, 14]]**

[\[化简\]](#)

$$4096 (-1+x)^4 x^2 (1+x)^5 (-1-2x-11x^2-8x^3+2x^4)$$

**(\*r2^1r3^12\*)**

**Simplify[Cf[1, 12, 0]]**

[\[化简\]](#)

0

**Simplify[Cf[1, 12, 1]]**

[\[化简\]](#)

0

**Simplify[Cf[1, 12, 2]]**

[化简]

0

**Simplify[Cf[1, 12, 3]]**

[化简]

0

**Simplify[Cf[1, 12, 4]]**

[化简]

0

**Simplify[Cf[1, 12, 5]]**

[化简]

0

**Simplify[Cf[1, 12, 6]]**

[化简]

0

**Simplify[Cf[1, 12, 7]]**

[化简]

0

**Simplify[Cf[1, 12, 8]]**

[化简]

0

**Simplify[Cf[1, 12, 9]]**

[化简]

$$-2048 (-1+x)^4 x^2 (1+x)^5 (2-3x+30x^2-21x^3+4x^4)$$

**Simplify[Cf[1, 12, 10]]**

[化简]

$$-2048 (-1+x)^4 x (1+x)^5 (4-12x+75x^2-52x^3+165x^4-56x^5+8x^6)$$

**Simplify[Cf[1, 12, 11]]**

[化简]

$$4096 (-1+x)^4 x (1+x)^5 (-2-4x-15x^2-84x^3-23x^4-60x^5+12x^6)$$

**Simplify[Cf[1, 12, 12]]**

[化简]

$$4096 (-1+x)^4 x (1+x)^5 (-2-4x-15x^2-84x^3-23x^4-60x^5+12x^6)$$

**Simplify[Cf[1, 12, 13]]**

[化简]

$$-2048 (-1+x)^4 x (1+x)^5 (4-12x+75x^2-52x^3+165x^4-56x^5+8x^6)$$

**Simplify[Cf[1, 12, 14]]**

[化简]

$$-2048 (-1+x)^4 x^2 (1+x)^5 (2-3x+30x^2-21x^3+4x^4)$$

(**\*r2^1r3^13\***)

**Simplify[Cf[1, 13, 0]]**

[化简]

0

**Simplify[Cf[1, 13, 1]]**

[化简]

0

**Simplify[Cf[1, 13, 2]]**

[化简]

0

**Simplify[Cf[1, 13, 3]]**

[化简]

0

**Simplify[Cf[1, 13, 4]]**

[化简]

0

**Simplify[Cf[1, 13, 5]]**

[化简]

0

**Simplify[Cf[1, 13, 6]]**

[化简]

0

**Simplify[Cf[1, 13, 7]]**

[化简]

0

**Simplify[Cf[1, 13, 8]]**

[化简]

$6144 (-1+x)^4 x^3 (1+x)^5 (-1+x^2)$

**Simplify[Cf[1, 13, 9]]**

[化简]

$8192 (-1+x)^4 x^2 (1+x)^5 (-2+3x-13x^2+6x^3)$

**Simplify[Cf[1, 13, 10]]**

[化简]

$-2048 (-1+x)^4 x (1+x)^5 (4-12x+75x^2-52x^3+165x^4-56x^5+8x^6)$

**Simplify[Cf[1, 13, 11]]**

[化简]

$8192 (-1+x)^4 x^2 (1+x)^5 (-6+8x-41x^2-3x^3-16x^4+4x^5)$

**Simplify[Cf[1, 13, 12]]**

[化简]

$$-2048 (-1+x)^4 x (1+x)^5 (4-12x+75x^2-52x^3+165x^4-56x^5+8x^6)$$

**Simplify[Cf[1, 13, 13]]**

[化简]

$$8192 (-1+x)^4 x^2 (1+x)^5 (-2+3x-13x^2+6x^3)$$

**Simplify[Cf[1, 13, 14]]**

[化简]

$$6144 (-1+x)^4 x^3 (1+x)^5 (-1+x^2)$$

**(\*r2^1r3^14\*)**

**Simplify[Cf[1, 14, 0]]**

[化简]

0

**Simplify[Cf[1, 14, 1]]**

[化简]

0

**Simplify[Cf[1, 14, 2]]**

[化简]

0

**Simplify[Cf[1, 14, 3]]**

[化简]

0

**Simplify[Cf[1, 14, 4]]**

[化简]

0

**Simplify[Cf[1, 14, 5]]**

[化简]

0

**Simplify[Cf[1, 14, 6]]**

[化简]

0

**Simplify[Cf[1, 14, 7]]**

[化简]

0

**Simplify[Cf[1, 14, 8]]**

[化简]

$$6144 (-1+x)^4 x^3 (1+x)^5 (-1+x^2)$$

**Simplify[Cf[1, 14, 9]]**

[\[化简\]](#)

$$-2048 (-1+x)^4 x^2 (1+x)^5 (2-3x+30x^2-21x^3+4x^4)$$

**Simplify[Cf[1, 14, 10]]**

[\[化简\]](#)

$$4096 (-1+x)^4 x^2 (1+x)^5 (-1-2x-11x^2-8x^3+2x^4)$$

**Simplify[Cf[1, 14, 11]]**

[\[化简\]](#)

$$4096 (-1+x)^4 x^2 (1+x)^5 (-1-2x-11x^2-8x^3+2x^4)$$

**Simplify[Cf[1, 14, 12]]**

[\[化简\]](#)

$$-2048 (-1+x)^4 x^2 (1+x)^5 (2-3x+30x^2-21x^3+4x^4)$$

**Simplify[Cf[1, 14, 13]]**

[\[化简\]](#)

$$6144 (-1+x)^4 x^3 (1+x)^5 (-1+x^2)$$

**Simplify[Cf[1, 14, 14]]**

[\[化简\]](#)

0

**(\*r2^2r3^0\*)**

**Simplify[Cf[2, 0, 0]]**

[\[化简\]](#)

0

**Simplify[Cf[2, 0, 1]]**

[\[化简\]](#)

0

**Simplify[Cf[2, 0, 2]]**

[\[化简\]](#)

0

**Simplify[Cf[2, 0, 3]]**

[\[化简\]](#)

0

**Simplify[Cf[2, 0, 4]]**

[\[化简\]](#)

0

**Simplify[Cf[2, 0, 5]]**

[\[化简\]](#)

0

**Simplify[Cf[2, 0, 6]]**

[化简]

0

**Simplify[Cf[2, 0, 7]]**

[化简]

0

**Simplify[Cf[2, 0, 8]]**

[化简]

0

**Simplify[Cf[2, 0, 9]]**

[化简]

0

**Simplify[Cf[2, 0, 10]]**

[化简]

0

**Simplify[Cf[2, 0, 11]]**

[化简]

0

**Simplify[Cf[2, 0, 12]]**

[化简]

0

**Simplify[Cf[2, 0, 13]]**

[化简]

0

**Simplify[Cf[2, 0, 14]]**

[化简]

0

**(\*r2^2r3^1\*)**

**Simplify[Cf[2, 1, 0]]**

[化简]

0

**Simplify[Cf[2, 1, 1]]**

[化简]

0

**Simplify[Cf[2, 1, 2]]**

[化简]

0

**Simplify[Cf[2, 1, 3]]**

[化简]

0

**Simplify[Cf[2, 1, 4]]**

[化简]

0

**Simplify[Cf[2, 1, 5]]**

[化简]

0

**Simplify[Cf[2, 1, 6]]**

[化简]

0

**Simplify[Cf[2, 1, 7]]**

[化简]

0

**Simplify[Cf[2, 1, 8]]**

[化简]

0

**Simplify[Cf[2, 1, 9]]**

[化简]

0

**Simplify[Cf[2, 1, 10]]**

[化简]

0

**Simplify[Cf[2, 1, 11]]**

[化简]

0

**Simplify[Cf[2, 1, 12]]**

[化简]

0

**Simplify[Cf[2, 1, 13]]**

[化简]

0

**Simplify[Cf[2, 1, 14]]**

[化简]

0

**(\*r2^2r3^2\*)**

**Simplify[Cf[2, 2, 0]]**

[化简]

0

**Simplify[Cf[2, 2, 1]]**

[化简]

0



**Simplify[Cf[2, 2, 2]]**

[化简]

0

**Simplify[Cf[2, 2, 3]]**

[化简]

0

**Simplify[Cf[2, 2, 4]]**

[化简]

0

**Simplify[Cf[2, 2, 5]]**

[化简]

0

**Simplify[Cf[2, 2, 6]]**

[化简]

0

**Simplify[Cf[2, 2, 7]]**

[化简]

0

**Simplify[Cf[2, 2, 8]]**

[化简]

0

**Simplify[Cf[2, 2, 9]]**

[化简]

0

**Simplify[Cf[2, 2, 10]]**

[化简]

0

**Simplify[Cf[2, 2, 11]]**

[化简]

0

**Simplify[Cf[2, 2, 12]]**

[化简]

0

**Simplify[Cf[2, 2, 13]]**

[化简]

0

**Simplify[Cf[2, 2, 14]]**

[化简]

0

**(\*r2^2r3^3\*)**

**Simplify[Cf[2, 3, 0]]**

[化简]

0

**Simplify[Cf[2, 3, 1]]**

[化简]

0

**Simplify[Cf[2, 3, 2]]**

[化简]

0

**Simplify[Cf[2, 3, 3]]**

[化简]

0

**Simplify[Cf[2, 3, 4]]**

[化简]

0

**Simplify[Cf[2, 3, 5]]**

[化简]

0

**Simplify[Cf[2, 3, 6]]**

[化简]

0

**Simplify[Cf[2, 3, 7]]**

[化简]

0

**Simplify[Cf[2, 3, 8]]**

[化简]

0

**Simplify[Cf[2, 3, 9]]**

[化简]

0

**Simplify[Cf[2, 3, 10]]**

[化简]

0

**Simplify[Cf[2, 3, 11]]**

[化简]

0

**Simplify[Cf[2, 3, 12]]**

[化简]

0

**Simplify[Cf[2, 3, 13]]**

[化简]

0

**Simplify[Cf[2, 3, 14]]**

[化简]

0

**(\*r2^2r3^4\*)**

**Simplify[Cf[2, 4, 0]]**

[化简]

0

**Simplify[Cf[2, 4, 1]]**

[化简]

0

**Simplify[Cf[2, 4, 2]]**

[化简]

0

**Simplify[Cf[2, 4, 3]]**

[化简]

0

**Simplify[Cf[2, 4, 4]]**

[化简]

0

**Simplify[Cf[2, 4, 5]]**

[化简]

0

**Simplify[Cf[2, 4, 6]]**

[化简]

0

**Simplify[Cf[2, 4, 7]]**

[化简]

0

**Simplify[Cf[2, 4, 8]]**

[化简]

0

**Simplify[Cf[2, 4, 9]]**

[化简]

0

**Simplify[Cf[2, 4, 10]]**

[化简]

0

**Simplify[Cf[2, 4, 11]]**

[化简]

0

**Simplify[Cf[2, 4, 12]]**

[化简]

0

**Simplify[Cf[2, 4, 13]]**

[化简]

0

**Simplify[Cf[2, 4, 14]]**

[化简]

0

**(\*r2^2r3^5\*)**

**Simplify[Cf[2, 5, 0]]**

[化简]

0

**Simplify[Cf[2, 5, 1]]**

[化简]

0

**Simplify[Cf[2, 5, 2]]**

[化简]

0

**Simplify[Cf[2, 5, 3]]**

[化简]

0

**Simplify[Cf[2, 5, 4]]**

[化简]

0

**Simplify[Cf[2, 5, 5]]**

[化简]

0

**Simplify[Cf[2, 5, 6]]**

[化简]

0

**Simplify[Cf[2, 5, 7]]**

[化简]

0

**Simplify[Cf[2, 5, 8]]**

[化简]

0

**Simplify[Cf[2, 5, 9]]**

[化简]

0

**Simplify[Cf[2, 5, 10]]**

[化简]

0

**Simplify[Cf[2, 5, 11]]**

[化简]

0

**Simplify[Cf[2, 5, 12]]**

[化简]

0

**Simplify[Cf[2, 5, 13]]**

[化简]

0

**Simplify[Cf[2, 5, 14]]**

[化简]

0

(\*, r2^2r3^6\*)

**Simplify[Cf[2, 6, 0]]**

[化简]

0

**Simplify[Cf[2, 6, 1]]**

[化简]

0

**Simplify[Cf[2, 6, 2]]**

[化简]

0

**Simplify[Cf[2, 6, 3]]**

[化简]

0

**Simplify[Cf[2, 6, 4]]**

[化简]

0

**Simplify[Cf[2, 6, 5]]**

[化简]

0

**Simplify[Cf[2, 6, 6]]**

[化简]

0

**Simplify[Cf[2, 6, 7]]**

[化简]

0

**Simplify[Cf[2, 6, 8]]**

[化简]

0

**Simplify[Cf[2, 6, 9]]**

[化简]

0

**Simplify[Cf[2, 6, 10]]**

[化简]

0

**Simplify[Cf[2, 6, 11]]**

[化简]

0

**Simplify[Cf[2, 6, 12]]**

[化简]

0

**Simplify[Cf[2, 6, 13]]**

[化简]

0

**Simplify[Cf[2, 6, 14]]**

[化简]

0

**(\*, r2^2r3^7\*)**

**Simplify[Cf[2, 7, 0]]**

[化简]

0

**Simplify[Cf[2, 7, 1]]**

[化简]

0

**Simplify[Cf[2, 7, 2]]**

[化简]

0

**Simplify[Cf[2, 7, 3]]**

[化简]

0

**Simplify[Cf[2, 7, 4]]**

[化简]

0

**Simplify[Cf[2, 7, 5]]**

[化简]

0

**Simplify[Cf[2, 7, 6]]**

[化简]

0

**Simplify[Cf[2, 7, 7]]**

[化简]

0

**Simplify[Cf[2, 7, 8]]**

[化简]

0

**Simplify[Cf[2, 7, 9]]**

[化简]

0

**Simplify[Cf[2, 7, 10]]**

[化简]

0

**Simplify[Cf[2, 7, 11]]**

[化简]

0

**Simplify[Cf[2, 7, 12]]**

[化简]

0

**Simplify[Cf[2, 7, 13]]**

[化简]

$-12288 (-1+x)^3 x^3 (1+x)^5 (-1+x^2)$

**Simplify[Cf[2, 7, 14]]**

[化简]

$-12288 (-1+x)^3 x^3 (1+x)^5 (-1+x^2)$

(\*, r2^2r3^8\*)

**Simplify[Cf[2, 8, 0]]**

[化简]

0

**Simplify[Cf[2, 8, 1]]**

[化简]

0

**Simplify[Cf[2, 8, 2]]**

[化简]

0

**Simplify[Cf[2, 8, 3]]**

[化简]

0

**Simplify[Cf[2, 8, 4]]**

[化简]

0

**Simplify[Cf[2, 8, 5]]**

[化简]

0

**Simplify[Cf[2, 8, 6]]**

[化简]

0

**Simplify[Cf[2, 8, 7]]**

[化简]

0

**Simplify[Cf[2, 8, 8]]**

[化简]

0

**Simplify[Cf[2, 8, 9]]**

[化简]

0

**Simplify[Cf[2, 8, 10]]**

[化简]

0

**Simplify[Cf[2, 8, 11]]**

[化简]

0

**Simplify[Cf[2, 8, 12]]**

[化简]

$1024 (-1 + x)^3 x^2 (1 + x)^5 (7 + 19 x + 13 x^2 + 137 x^3 - 172 x^4 + 44 x^5)$

**Simplify[Cf[2, 8, 13]]**

[化简]

$2048 (-1 + x)^3 x^2 (1 + x)^5 (15 - x + 23 x^2 + 135 x^3 - 158 x^4 + 34 x^5)$

**Simplify[Cf[2, 8, 14]]**

[化简]

$1024 (-1 + x)^3 x^2 (1 + x)^5 (7 + 19 x + 13 x^2 + 137 x^3 - 172 x^4 + 44 x^5)$

(\*, r2^2r3^9\*)

**Simplify[Cf[2, 9, 0]]**

[化简]

0



**Simplify[Cf[2, 9, 1]]**

[化简]

0

**Simplify[Cf[2, 9, 2]]**

[化简]

0

**Simplify[Cf[2, 9, 3]]**

[化简]

0

**Simplify[Cf[2, 9, 4]]**

[化简]

0

**Simplify[Cf[2, 9, 5]]**

[化简]

0

**Simplify[Cf[2, 9, 6]]**

[化简]

0

**Simplify[Cf[2, 9, 7]]**

[化简]

0

**Simplify[Cf[2, 9, 8]]**

[化简]

0

**Simplify[Cf[2, 9, 9]]**

[化简]

0

**Simplify[Cf[2, 9, 10]]**

[化简]

0

**Simplify[Cf[2, 9, 11]]**

[化简]

$$-2048 (-1+x)^3 x^2 (1+x)^5 (-3-44x+37x^2-182x^3+60x^4)$$

**Simplify[Cf[2, 9, 12]]**

[化简]

$$2048 (-1+x)^3 x (1+x)^5 (6+7x+89x^2+50x^3+225x^4+197x^5-190x^6+36x^7)$$

**Simplify[Cf[2, 9, 13]]**

[化简]

$$2048 (-1+x)^3 x (1+x)^5 (6+7x+89x^2+50x^3+225x^4+197x^5-190x^6+36x^7)$$

**Simplify[Cf[2, 9, 14]]**

[化简]

$$-2048 (-1+x)^3 x^2 (1+x)^5 (-3-44x+37x^2-182x^3+60x^4)$$

**Simplify[Cf[2, 9, 15]]**

[化简]

0

**(\*, r2^2r3^10\*)**

**Simplify[Cf[2, 10, 0]]**

[化简]

0

**Simplify[Cf[2, 10, 1]]**

[化简]

0

**Simplify[Cf[2, 10, 2]]**

[化简]

0

**Simplify[Cf[2, 10, 3]]**

[化简]

0

**Simplify[Cf[2, 10, 4]]**

[化简]

0

**Simplify[Cf[2, 10, 5]]**

[化简]

0

**Simplify[Cf[2, 10, 6]]**

[化简]

0

**Simplify[Cf[2, 10, 7]]**

[化简]

0

**Simplify[Cf[2, 10, 8]]**

[化简]

0

**Simplify[Cf[2, 10, 9]]**

[化简]

0

**Simplify[Cf[2, 10, 10]]**

[化简]

$$-2048 (-1+x)^3 x^2 (1+x)^5 (-7-25x-57x^2-55x^3-116x^4+44x^5)$$

**Simplify[Cf[2, 10, 11]]**

[化简]

$$-2048 (-1+x)^3 x (1+x)^5 (-6-34x-84x^2-195x^3-332x^4-521x^5+92x^6+36x^7)$$

**Simplify[Cf[2, 10, 12]]**

[化简]

$$-4096 (-1+x)^3 (1+x)^5 (-3+21x-131x^2+203x^3-650x^4+431x^5-1014x^6+363x^7-60x^8+12x^9)$$

**Simplify[Cf[2, 10, 13]]**

[化简]

$$-2048 (-1+x)^3 x (1+x)^5 (-6-34x-84x^2-195x^3-332x^4-521x^5+92x^6+36x^7)$$

**Simplify[Cf[2, 10, 14]]**

[化简]

$$-2048 (-1+x)^3 x^2 (1+x)^5 (-7-25x-57x^2-55x^3-116x^4+44x^5)$$

**(\*, r2^2r3^11\*)**

**Simplify[Cf[2, 11, 0]]**

[化简]

0

**Simplify[Cf[2, 11, 1]]**

[化简]

0

**Simplify[Cf[2, 11, 2]]**

[化简]

0

**Simplify[Cf[2, 11, 3]]**

[化简]

0

**Simplify[Cf[2, 11, 4]]**

[化简]

0

**Simplify[Cf[2, 11, 5]]**

[化简]

0

**Simplify[Cf[2, 11, 6]]**

[化简]

0

**Simplify[Cf[2, 11, 7]]**

[化简]

0

**Simplify[Cf[2, 11, 8]]**

[\[化简\]](#)

0

**Simplify[Cf[2, 11, 9]]**

[\[化简\]](#)

$$-2048 (-1+x)^3 x^2 (1+x)^5 (-3-44x+37x^2-182x^3+60x^4)$$

**Simplify[Cf[2, 11, 10]]**

[\[化简\]](#)

$$-2048 (-1+x)^3 x (1+x)^5 (-6-34x-84x^2-195x^3-332x^4-521x^5+92x^6+36x^7)$$

**Simplify[Cf[2, 11, 11]]**

[\[化简\]](#)

$$2048 (-1+x)^3 x (1+x)^5 (24-31x+565x^2-483x^3+2171x^4-538x^5+1316x^6-552x^7+48x^8)$$

**Simplify[Cf[2, 11, 12]]**

[\[化简\]](#)

$$2048 (-1+x)^3 x (1+x)^5 (24-31x+565x^2-483x^3+2171x^4-538x^5+1316x^6-552x^7+48x^8)$$

**Simplify[Cf[2, 11, 13]]**

[\[化简\]](#)

$$-2048 (-1+x)^3 x (1+x)^5 (-6-34x-84x^2-195x^3-332x^4-521x^5+92x^6+36x^7)$$

**Simplify[Cf[2, 11, 14]]**

[\[化简\]](#)

$$-2048 (-1+x)^3 x^2 (1+x)^5 (-3-44x+37x^2-182x^3+60x^4)$$

**(\*, r2^2r3^12\*)**

**Simplify[Cf[2, 12, 0]]**

[\[化简\]](#)

0

**Simplify[Cf[2, 12, 1]]**

[\[化简\]](#)

0

**Simplify[Cf[2, 12, 2]]**

[\[化简\]](#)

0

**Simplify[Cf[2, 12, 3]]**

[\[化简\]](#)

0

**Simplify[Cf[2, 12, 4]]**

[\[化简\]](#)

0

**Simplify[Cf[2, 12, 5]]**

[\[化简\]](#)

0

**Simplify[Cf[2, 12, 6]]**

[\[化简\]](#)

0

**Simplify[Cf[2, 12, 7]]**

[\[化简\]](#)

0

**Simplify[Cf[2, 12, 8]]**

[\[化简\]](#)

$$1024 (-1+x)^3 x^2 (1+x)^5 (7+19x+13x^2+137x^3-172x^4+44x^5)$$

**Simplify[Cf[2, 12, 9]]**

[\[化简\]](#)

$$2048 (-1+x)^3 x (1+x)^5 (6+7x+89x^2+50x^3+225x^4+197x^5-190x^6+36x^7)$$

**Simplify[Cf[2, 12, 10]]**

[\[化简\]](#)

$$\begin{aligned} & -4096 (-1+x)^3 (1+x)^5 \\ & (-3+21x-131x^2+203x^3-650x^4+431x^5-1014x^6+363x^7-60x^8+12x^9) \end{aligned}$$

**Simplify[Cf[2, 12, 11]]**

[\[化简\]](#)

$$2048 (-1+x)^3 x (1+x)^5 (24-31x+565x^2-483x^3+2171x^4-538x^5+1316x^6-552x^7+48x^8)$$

**Simplify[Cf[2, 12, 12]]**

[\[化简\]](#)

$$\begin{aligned} & -4096 (-1+x)^3 (1+x)^5 \\ & (-3+21x-131x^2+203x^3-650x^4+431x^5-1014x^6+363x^7-60x^8+12x^9) \end{aligned}$$

**Simplify[Cf[2, 12, 13]]**

[\[化简\]](#)

$$2048 (-1+x)^3 x (1+x)^5 (6+7x+89x^2+50x^3+225x^4+197x^5-190x^6+36x^7)$$

**Simplify[Cf[2, 12, 14]]**

[\[化简\]](#)

$$1024 (-1+x)^3 x^2 (1+x)^5 (7+19x+13x^2+137x^3-172x^4+44x^5)$$

**(\*r2^2r3^13\*)**

**Simplify[Cf[2, 13, 0]]**

[\[化简\]](#)

0

**Simplify[Cf[2, 13, 1]]**

[\[化简\]](#)

0

**Simplify[Cf[2, 13, 2]]**

[化简]

0

**Simplify[Cf[2, 13, 3]]**

[化简]

0

**Simplify[Cf[2, 13, 4]]**

[化简]

0

**Simplify[Cf[2, 13, 5]]**

[化简]

0

**Simplify[Cf[2, 13, 6]]**

[化简]

0

**Simplify[Cf[2, 13, 7]]**

[化简]

$$-12288 (-1+x)^3 x^3 (1+x)^5 (-1+x^2)$$

**Simplify[Cf[2, 13, 8]]**

[化简]

$$2048 (-1+x)^3 x^2 (1+x)^5 (15-x+23x^2+135x^3-158x^4+34x^5)$$

**Simplify[Cf[2, 13, 9]]**

[化简]

$$2048 (-1+x)^3 x (1+x)^5 (6+7x+89x^2+50x^3+225x^4+197x^5-190x^6+36x^7)$$

**Simplify[Cf[2, 13, 10]]**

[化简]

$$-2048 (-1+x)^3 x (1+x)^5 (-6-34x-84x^2-195x^3-332x^4-521x^5+92x^6+36x^7)$$

**Simplify[Cf[2, 13, 11]]**

[化简]

$$-2048 (-1+x)^3 x (1+x)^5 (-6-34x-84x^2-195x^3-332x^4-521x^5+92x^6+36x^7)$$

**Simplify[Cf[2, 13, 12]]**

[化简]

$$2048 (-1+x)^3 x (1+x)^5 (6+7x+89x^2+50x^3+225x^4+197x^5-190x^6+36x^7)$$

**Simplify[Cf[2, 13, 13]]**

[化简]

$$2048 (-1+x)^3 x^2 (1+x)^5 (15-x+23x^2+135x^3-158x^4+34x^5)$$

**Simplify[Cf[2, 13, 14]]**

[化简]

$$-12288 (-1+x)^3 x^3 (1+x)^5 (-1+x^2)$$

(\*, r2^2r3^14\*)

**Simplify[Cf[2, 14, 0]]**

[化简]

0

**Simplify[Cf[2, 14, 1]]**

[化简]

0

**Simplify[Cf[2, 14, 2]]**

[化简]

0

**Simplify[Cf[2, 14, 3]]**

[化简]

0

**Simplify[Cf[2, 14, 4]]**

[化简]

0

**Simplify[Cf[2, 14, 5]]**

[化简]

0

**Simplify[Cf[2, 14, 6]]**

[化简]

0

**Simplify[Cf[2, 14, 7]]**

[化简]

$-12\,288\,(-1+x)^3 x^3 (1+x)^5 (-1+x^2)$

**Simplify[Cf[2, 14, 8]]**

[化简]

$1024\,(-1+x)^3 x^2 (1+x)^5 (7+19x+13x^2+137x^3-172x^4+44x^5)$

**Simplify[Cf[2, 14, 9]]**

[化简]

$-2048\,(-1+x)^3 x^2 (1+x)^5 (-3-44x+37x^2-182x^3+60x^4)$

**Simplify[Cf[2, 14, 10]]**

[化简]

$-2048\,(-1+x)^3 x^2 (1+x)^5 (-7-25x-57x^2-55x^3-116x^4+44x^5)$

**Simplify[Cf[2, 14, 11]]**

[化简]

$-2048\,(-1+x)^3 x^2 (1+x)^5 (-3-44x+37x^2-182x^3+60x^4)$

**Simplify[Cf[2, 14, 12]]**

[化简]

$$1024 (-1+x)^3 x^2 (1+x)^5 (7+19x+13x^2+137x^3-172x^4+44x^5)$$

**Simplify[Cf[2, 14, 13]]**

[化简]

$$-12288 (-1+x)^3 x^3 (1+x)^5 (-1+x^2)$$

**Simplify[Cf[2, 14, 14]]**

[化简]

0

**(\*r2^3r3^0\*)**

**Simplify[Cf[3, 0, 0]]**

[化简]

0

**Simplify[Cf[3, 0, 1]]**

[化简]

0

**Simplify[Cf[3, 0, 2]]**

[化简]

0

**Simplify[Cf[3, 0, 3]]**

[化简]

0

**Simplify[Cf[3, 0, 4]]**

[化简]

0

**Simplify[Cf[3, 0, 5]]**

[化简]

0

**Simplify[Cf[3, 0, 6]]**

[化简]

0

**Simplify[Cf[3, 0, 7]]**

[化简]

0

**Simplify[Cf[3, 0, 8]]**

[化简]

0



**Simplify[Cf[3, 0, 9]]**

[化简]

0

**Simplify[Cf[3, 0, 10]]**

[化简]

0

**Simplify[Cf[3, 0, 11]]**

[化简]

0

**Simplify[Cf[3, 0, 12]]**

[化简]

0

**Simplify[Cf[3, 0, 13]]**

[化简]

0

**Simplify[Cf[3, 0, 14]]**

[化简]

0

(\*, r2^3r3^1\*)

**Simplify[Cf[3, 1, 0]]**

[化简]

0

**Simplify[Cf[3, 1, 1]]**

[化简]

0

**Simplify[Cf[3, 1, 2]]**

[化简]

0

**Simplify[Cf[3, 1, 3]]**

[化简]

0

**Simplify[Cf[3, 1, 4]]**

[化简]

0

**Simplify[Cf[3, 1, 5]]**

[化简]

0

**Simplify[Cf[3, 1, 6]]**

[化简]

0

**Simplify[Cf[3, 1, 7]]**

[化简]

0

**Simplify[Cf[3, 1, 8]]**

[化简]

0

**Simplify[Cf[3, 1, 9]]**

[化简]

0

**Simplify[Cf[3, 1, 10]]**

[化简]

0

**Simplify[Cf[3, 1, 11]]**

[化简]

0

**Simplify[Cf[3, 1, 12]]**

[化简]

0

**Simplify[Cf[3, 1, 13]]**

[化简]

0

**Simplify[Cf[3, 1, 14]]**

[化简]

0

**(\*, r2^3r3^2\*)**

**Simplify[Cf[3, 2, 0]]**

[化简]

0

**Simplify[Cf[3, 2, 1]]**

[化简]

0

**Simplify[Cf[3, 2, 2]]**

[化简]

0

**Simplify[Cf[3, 2, 3]]**

[化简]

0

**Simplify[Cf[3, 2, 4]]**

[化简]

0

**Simplify[Cf[3, 2, 5]]**

[化简]

0

**Simplify[Cf[3, 2, 6]]**

[化简]

0

**Simplify[Cf[3, 2, 7]]**

[化简]

0

**Simplify[Cf[3, 2, 8]]**

[化简]

0

**Simplify[Cf[3, 2, 9]]**

[化简]

0

**Simplify[Cf[3, 2, 10]]**

[化简]

0

**Simplify[Cf[3, 2, 11]]**

[化简]

0

**Simplify[Cf[3, 2, 12]]**

[化简]

0

**Simplify[Cf[3, 2, 13]]**

[化简]

0

**Simplify[Cf[3, 2, 14]]**

[化简]

0

(\*, r2^3r3^3\*)

**Simplify[Cf[3, 3, 0]]**

[化简]

0

**Simplify[Cf[3, 3, 1]]**

[化简]

0

**Simplify[Cf[3, 3, 2]]**

[化简]

0

**Simplify[Cf[3, 3, 3]]**

[\[化简\]](#)

0

**Simplify[Cf[3, 3, 4]]**

[\[化简\]](#)

0

**Simplify[Cf[3, 3, 5]]**

[\[化简\]](#)

0

**Simplify[Cf[3, 3, 6]]**

[\[化简\]](#)

0

**Simplify[Cf[3, 3, 7]]**

[\[化简\]](#)

0

**Simplify[Cf[3, 3, 8]]**

[\[化简\]](#)

0

**Simplify[Cf[3, 3, 9]]**

[\[化简\]](#)

0

**Simplify[Cf[3, 3, 10]]**

[\[化简\]](#)

0

**Simplify[Cf[3, 3, 11]]**

[\[化简\]](#)

0

**Simplify[Cf[3, 3, 12]]**

[\[化简\]](#)

0

**Simplify[Cf[3, 3, 13]]**

[\[化简\]](#)

0

**Simplify[Cf[3, 3, 14]]**

[\[化简\]](#)

0

**(\*, r2^3r3^4\*)**

**Simplify[Cf[3, 4, 0]]**

[\[化简\]](#)

0

**Simplify[Cf[3, 4, 1]]**

[化简]

0

**Simplify[Cf[3, 4, 2]]**

[化简]

0

**Simplify[Cf[3, 4, 3]]**

[化简]

0

**Simplify[Cf[3, 4, 4]]**

[化简]

0

**Simplify[Cf[3, 4, 5]]**

[化简]

0

**Simplify[Cf[3, 4, 6]]**

[化简]

0

**Simplify[Cf[3, 4, 7]]**

[化简]

0

**Simplify[Cf[3, 4, 8]]**

[化简]

0

**Simplify[Cf[3, 4, 9]]**

[化简]

0

**Simplify[Cf[3, 4, 10]]**

[化简]

0

**Simplify[Cf[3, 4, 11]]**

[化简]

0

**Simplify[Cf[3, 4, 12]]**

[化简]

0

**Simplify[Cf[3, 4, 13]]**

[化简]

0

```
Simplify[Cf[3, 4, 14]]
```

```
[化简]
```

```
0
```

```
(*, r2^3r3^5*)
```

```
Simplify[Cf[3, 5, 0]]
```

```
[化简]
```

```
0
```

```
Simplify[Cf[3, 5, 1]]
```

```
[化简]
```

```
0
```

```
Simplify[Cf[3, 5, 2]]
```

```
[化简]
```

```
0
```

```
Simplify[Cf[3, 5, 3]]
```

```
[化简]
```

```
0
```

```
Simplify[Cf[3, 5, 4]]
```

```
[化简]
```

```
0
```

```
Simplify[Cf[3, 5, 5]]
```

```
[化简]
```

```
0
```

```
Simplify[Cf[3, 5, 6]]
```

```
[化简]
```

```
0
```

```
Simplify[Cf[3, 5, 7]]
```

```
[化简]
```

```
0
```

```
Simplify[Cf[3, 5, 8]]
```

```
[化简]
```

```
0
```

```
Simplify[Cf[3, 5, 9]]
```

```
[化简]
```

```
0
```

```
Simplify[Cf[3, 5, 10]]
```

```
[化简]
```

```
0
```

```
Simplify[Cf[3, 5, 11]]
```

```
[化简]
```

```
0
```

**Simplify[Cf[3, 5, 12]]**

[化简]

0

**Simplify[Cf[3, 5, 13]]**

[化简]

0

**Simplify[Cf[3, 5, 14]]**

[化简]

0

**(\*, r2^3r3^6\*)**

**Simplify[Cf[3, 6, 0]]**

[化简]

0

**Simplify[Cf[3, 6, 1]]**

[化简]

0

**Simplify[Cf[3, 6, 2]]**

[化简]

0

**Simplify[Cf[3, 6, 3]]**

[化简]

0

**Simplify[Cf[3, 6, 4]]**

[化简]

0

**Simplify[Cf[3, 6, 5]]**

[化简]

0

**Simplify[Cf[3, 6, 6]]**

[化简]

0

**Simplify[Cf[3, 6, 7]]**

[化简]

0

**Simplify[Cf[3, 6, 8]]**

[化简]

0

**Simplify[Cf[3, 6, 9]]**

[化简]

0

**Simplify[Cf[3, 6, 10]]**

[化简]

0

**Simplify[Cf[3, 6, 11]]**

[化简]

0

**Simplify[Cf[3, 6, 12]]**

[化简]

0

**Simplify[Cf[3, 6, 13]]**

[化简]

$-4096 (-1+x)^2 x^3 (1+x)^5 (5-5x+3x^2-7x^3+4x^4)$

**Simplify[Cf[3, 6, 14]]**

[化简]

$-4096 (-1+x)^2 x^3 (1+x)^5 (5-5x+3x^2-7x^3+4x^4)$

(\*, r2^3r3^7\*)

**Simplify[Cf[3, 7, 0]]**

[化简]

0

**Simplify[Cf[3, 7, 1]]**

[化简]

0

**Simplify[Cf[3, 7, 2]]**

[化简]

0

**Simplify[Cf[3, 7, 3]]**

[化简]

0

**Simplify[Cf[3, 7, 4]]**

[化简]

0

**Simplify[Cf[3, 7, 5]]**

[化简]

0

**Simplify[Cf[3, 7, 6]]**

[化简]

0

**Simplify[Cf[3, 7, 7]]**

[化简]

0



**Simplify[Cf[3, 7, 8]]**

[化简]

0

**Simplify[Cf[3, 7, 9]]**

[化简]

0

**Simplify[Cf[3, 7, 10]]**

[化简]

0

**Simplify[Cf[3, 7, 11]]**

[化简]

0

**Simplify[Cf[3, 7, 12]]**

[化简]

$-2048 (-1+x)^2 x^2 (1+x)^5 (9-14x+132x^2-190x^3+207x^4-180x^5+52x^6)$

**Simplify[Cf[3, 7, 13]]**

[化简]

$-4096 (-1+x)^2 x^2 (1+x)^5 (15-34x+152x^2-202x^3+221x^4-188x^5+52x^6)$

**Simplify[Cf[3, 7, 14]]**

[化简]

$-2048 (-1+x)^2 x^2 (1+x)^5 (9-14x+132x^2-190x^3+207x^4-180x^5+52x^6)$

(\*, r2^3r3^8\*)

**Simplify[Cf[3, 8, 0]]**

[化简]

0

**Simplify[Cf[3, 8, 1]]**

[化简]

0

**Simplify[Cf[3, 8, 2]]**

[化简]

0

**Simplify[Cf[3, 8, 3]]**

[化简]

0

**Simplify[Cf[3, 8, 4]]**

[化简]

0

**Simplify[Cf[3, 8, 5]]**

[化简]

0

**Simplify[Cf[3, 8, 6]]**

[化简]

0

**Simplify[Cf[3, 8, 7]]**

[化简]

0

**Simplify[Cf[3, 8, 8]]**

[化简]

0

**Simplify[Cf[3, 8, 9]]**

[化简]

0

**Simplify[Cf[3, 8, 10]]**

[化简]

0

**Simplify[Cf[3, 8, 11]]**

[化简]

$$-2048 (-1+x)^2 x^2 (1+x)^5 (9+60x+34x^2+56x^3+177x^4-188x^5+28x^6)$$

**Simplify[Cf[3, 8, 12]]**

[化简]

$$-2048 (-1+x)^2 x (1+x)^5 (18-53x+419x^2-464x^3+1070x^4-399x^5+121x^6-228x^7+60x^8)$$

**Simplify[Cf[3, 8, 13]]**

[化简]

$$-2048 (-1+x)^2 x (1+x)^5 (18-53x+419x^2-464x^3+1070x^4-399x^5+121x^6-228x^7+60x^8)$$

**Simplify[Cf[3, 8, 14]]**

[化简]

$$-2048 (-1+x)^2 x^2 (1+x)^5 (9+60x+34x^2+56x^3+177x^4-188x^5+28x^6)$$

(\*, r2^3r3^9\*)

**Simplify[Cf[3, 9, 0]]**

[化简]

0

**Simplify[Cf[3, 9, 1]]**

[化简]

0

**Simplify[Cf[3, 9, 2]]**

[化简]

0

**Simplify[Cf[3, 9, 3]]**

[化简]

0

**Simplify[Cf[3, 9, 4]]**

[化简]

0

**Simplify[Cf[3, 9, 5]]**

[化简]

0

**Simplify[Cf[3, 9, 6]]**

[化简]

0

**Simplify[Cf[3, 9, 7]]**

[化简]

0

**Simplify[Cf[3, 9, 8]]**

[化简]

0

**Simplify[Cf[3, 9, 9]]**

[化简]

0

**Simplify[Cf[3, 9, 10]]**

[化简]

$$4096 (-1+x)^2 x^2 (1+x)^5 (-9-18x-124x^2+82x^3-207x^4+4x^5+40x^6)$$

**Simplify[Cf[3, 9, 11]]**

[化简]

$$4096 (-1+x)^2 x^2 (1+x)^5 (-120+337x-1408x^2+1558x^3-2044x^4+597x^5+4x^6+36x^7)$$

**Simplify[Cf[3, 9, 12]]**

[化简]

$$4096 (-1+x)^2 x (1+x)^5 (-30+78x-535x^2+314x^3-1370x^4+916x^5-2281x^6+1676x^7-456x^8+72x^9)$$

**Simplify[Cf[3, 9, 13]]**

[化简]

$$4096 (-1+x)^2 x^2 (1+x)^5 (-120+337x-1408x^2+1558x^3-2044x^4+597x^5+4x^6+36x^7)$$

**Simplify[Cf[3, 9, 14]]**

[化简]

$$4096 (-1+x)^2 x^2 (1+x)^5 (-9-18x-124x^2+82x^3-207x^4+4x^5+40x^6)$$

(\*, r2^3r3^10\*)

**Simplify[Cf[3, 10, 0]]**

[\[化简\]](#)

0

**Simplify[Cf[3, 10, 1]]**

[\[化简\]](#)

0

**Simplify[Cf[3, 10, 2]]**

[\[化简\]](#)

0

**Simplify[Cf[3, 10, 3]]**

[\[化简\]](#)

0

**Simplify[Cf[3, 10, 4]]**

[\[化简\]](#)

0

**Simplify[Cf[3, 10, 5]]**

[\[化简\]](#)

0

**Simplify[Cf[3, 10, 6]]**

[\[化简\]](#)

0

**Simplify[Cf[3, 10, 7]]**

[\[化简\]](#)

0

**Simplify[Cf[3, 10, 8]]**

[\[化简\]](#)

0

**Simplify[Cf[3, 10, 9]]**

[\[化简\]](#)

$4096 (-1 + x)^2 x^2 (1 + x)^5 (-9 - 18 x - 124 x^2 + 82 x^3 - 207 x^4 + 4 x^5 + 40 x^6)$

**Simplify[Cf[3, 10, 10]]**

[\[化简\]](#)

$-4096 (-1 + x)^2 x (1 + x)^5 (18 - 53 x + 523 x^2 - 704 x^3 + 2078 x^4 - 1455 x^5 + 1921 x^6 - 772 x^7 + 12 x^8)$

**Simplify[Cf[3, 10, 11]]**

[\[化简\]](#)

$2048 (-1 + x)^2 x (1 + x)^5 (-78 + 134 x - 1447 x^2 + 514 x^3 - 4130 x^4 + 744 x^5 - 4349 x^6 + 600 x^7 + 1020 x^8 - 144 x^9)$

**Simplify[Cf[3, 10, 12]]**

[化简]

$$2048 (-1+x)^2 x (1+x)^5 (-78+134x-1447x^2+514x^3-4130x^4+744x^5-4349x^6+600x^7+1020x^8-144x^9)$$

**Simplify[Cf[3, 10, 13]]**

[化简]

$$-4096 (-1+x)^2 x (1+x)^5 (18-53x+523x^2-704x^3+2078x^4-1455x^5+1921x^6-772x^7+12x^8)$$

**Simplify[Cf[3, 10, 14]]**

[化简]

$$4096 (-1+x)^2 x^2 (1+x)^5 (-9-18x-124x^2+82x^3-207x^4+4x^5+40x^6)$$

(\*, r2^3r3^11\*)

**Simplify[Cf[3, 11, 0]]**

[化简]

0

**Simplify[Cf[3, 11, 1]]**

[化简]

0

**Simplify[Cf[3, 11, 2]]**

[化简]

0

**Simplify[Cf[3, 11, 3]]**

[化简]

0

**Simplify[Cf[3, 11, 4]]**

[化简]

0

**Simplify[Cf[3, 11, 5]]**

[化简]

0

**Simplify[Cf[3, 11, 6]]**

[化简]

0

**Simplify[Cf[3, 11, 7]]**

[化简]

0

**Simplify[Cf[3, 11, 8]]**

[化简]

$$-2048 (-1+x)^2 x^2 (1+x)^5 (9+60x+34x^2+56x^3+177x^4-188x^5+28x^6)$$

**Simplify[Cf[3, 11, 9]]**

[化简]

$$4096 (-1+x)^2 x^2 (1+x)^5 (-120+337x-1408x^2+1558x^3-2044x^4+597x^5+4x^6+36x^7)$$

**Simplify[Cf[3, 11, 10]]**

[化简]

$$2048 (-1+x)^2 x (1+x)^5 (-78+134x-1447x^2+514x^3-4130x^4+744x^5-4349x^6+600x^7+1020x^8-144x^9)$$

**Simplify[Cf[3, 11, 11]]**

[化简]

$$-12288 (-1+x)^2 x^2 (1+x)^5 (147-472x+1936x^2-2434x^3+3749x^4-2278x^5+1936x^6-984x^7+144x^8)$$

**Simplify[Cf[3, 11, 12]]**

[化简]

$$2048 (-1+x)^2 x (1+x)^5 (-78+134x-1447x^2+514x^3-4130x^4+744x^5-4349x^6+600x^7+1020x^8-144x^9)$$

**Simplify[Cf[3, 11, 13]]**

[化简]

$$4096 (-1+x)^2 x^2 (1+x)^5 (-120+337x-1408x^2+1558x^3-2044x^4+597x^5+4x^6+36x^7)$$

**Simplify[Cf[3, 11, 14]]**

[化简]

$$-2048 (-1+x)^2 x^2 (1+x)^5 (9+60x+34x^2+56x^3+177x^4-188x^5+28x^6)$$

**(\*, r2^3r3^12\*)**

**Simplify[Cf[3, 12, 0]]**

[化简]

0

**Simplify[Cf[3, 12, 1]]**

[化简]

0

**Simplify[Cf[3, 12, 2]]**

[化简]

0

**Simplify[Cf[3, 12, 3]]**

[化简]

0

**Simplify[Cf[3, 12, 4]]**

[化简]

0

**Simplify[Cf[3, 12, 5]]**

[化简]

0

**Simplify[Cf[3, 12, 6]]**

[化简]

0

**Simplify[Cf[3, 12, 7]]**

[化简]

$$-2048 (-1+x)^2 x^2 (1+x)^5 (9-14x+132x^2-190x^3+207x^4-180x^5+52x^6)$$

**Simplify[Cf[3, 12, 8]]**

[化简]

$$-2048 (-1+x)^2 x (1+x)^5 (18-53x+419x^2-464x^3+1070x^4-399x^5+121x^6-228x^7+60x^8)$$

**Simplify[Cf[3, 12, 9]]**

[化简]

$$4096 (-1+x)^2 x (1+x)^5 (-30+78x-535x^2+314x^3-1370x^4+916x^5-2281x^6+1676x^7-456x^8+72x^9)$$

**Simplify[Cf[3, 12, 10]]**

[化简]

$$2048 (-1+x)^2 x (1+x)^5 (-78+134x-1447x^2+514x^3-4130x^4+744x^5-4349x^6+600x^7+1020x^8-144x^9)$$

**Simplify[Cf[3, 12, 11]]**

[化简]

$$2048 (-1+x)^2 x (1+x)^5 (-78+134x-1447x^2+514x^3-4130x^4+744x^5-4349x^6+600x^7+1020x^8-144x^9)$$

**Simplify[Cf[3, 12, 12]]**

[化简]

$$4096 (-1+x)^2 x (1+x)^5 (-30+78x-535x^2+314x^3-1370x^4+916x^5-2281x^6+1676x^7-456x^8+72x^9)$$

**Simplify[Cf[3, 12, 13]]**

[化简]

$$-2048 (-1+x)^2 x (1+x)^5 (18-53x+419x^2-464x^3+1070x^4-399x^5+121x^6-228x^7+60x^8)$$

**Simplify[Cf[3, 12, 14]]**

[化简]

$$-2048 (-1+x)^2 x^2 (1+x)^5 (9-14x+132x^2-190x^3+207x^4-180x^5+52x^6)$$

**(\*, r2^3r3^13\*)****Simplify[Cf[3, 13, 0]]**

[化简]

0

**Simplify[Cf[3, 13, 1]]**

[化简]

0

**Simplify[Cf[3, 13, 2]]**

[化简]

0

**Simplify[Cf[3, 13, 3]]**

[化简]

0

**Simplify[Cf[3, 13, 4]]**

[化简]

0

**Simplify[Cf[3, 13, 5]]**

[化简]

0

**Simplify[Cf[3, 13, 6]]**

[化简]

$$-4096 (-1+x)^2 x^3 (1+x)^5 (5-5x+3x^2-7x^3+4x^4)$$

**Simplify[Cf[3, 13, 7]]**

[化简]

$$-4096 (-1+x)^2 x^2 (1+x)^5 (15-34x+152x^2-202x^3+221x^4-188x^5+52x^6)$$

**Simplify[Cf[3, 13, 8]]**

[化简]

$$-2048 (-1+x)^2 x (1+x)^5 (18-53x+419x^2-464x^3+1070x^4-399x^5+121x^6-228x^7+60x^8)$$

**Simplify[Cf[3, 13, 9]]**

[化简]

$$4096 (-1+x)^2 x^2 (1+x)^5 (-120+337x-1408x^2+1558x^3-2044x^4+597x^5+4x^6+36x^7)$$

**Simplify[Cf[3, 13, 10]]**

[化简]

$$-4096 (-1+x)^2 x (1+x)^5 (18-53x+523x^2-704x^3+2078x^4-1455x^5+1921x^6-772x^7+12x^8)$$

**Simplify[Cf[3, 13, 11]]**

[化简]

$$4096 (-1+x)^2 x^2 (1+x)^5 (-120+337x-1408x^2+1558x^3-2044x^4+597x^5+4x^6+36x^7)$$

**Simplify[Cf[3, 13, 12]]**

[化简]

$$-2048 (-1+x)^2 x (1+x)^5 (18-53x+419x^2-464x^3+1070x^4-399x^5+121x^6-228x^7+60x^8)$$

**Simplify[Cf[3, 13, 13]]**

[化简]

$$-4096 (-1+x)^2 x^2 (1+x)^5 (15-34x+152x^2-202x^3+221x^4-188x^5+52x^6)$$

**Simplify[Cf[3, 13, 14]]**

[化简]

$$-4096 (-1+x)^2 x^3 (1+x)^5 (5-5x+3x^2-7x^3+4x^4)$$



(\*, r2^3r3^14\*)

**Simplify[Cf[3, 14, 0]]**

[化简]

0

**Simplify[Cf[3, 14, 1]]**

[化简]

0

**Simplify[Cf[3, 14, 2]]**

[化简]

0

**Simplify[Cf[3, 14, 3]]**

[化简]

0

**Simplify[Cf[3, 14, 4]]**

[化简]

0

**Simplify[Cf[3, 14, 5]]**

[化简]

0

**Simplify[Cf[3, 14, 6]]**

[化简]

$-4096 (-1+x)^2 x^3 (1+x)^5 (5-5x+3x^2-7x^3+4x^4)$

**Simplify[Cf[3, 14, 7]]**

[化简]

$-2048 (-1+x)^2 x^2 (1+x)^5 (9-14x+132x^2-190x^3+207x^4-180x^5+52x^6)$

**Simplify[Cf[3, 14, 8]]**

[化简]

$-2048 (-1+x)^2 x^2 (1+x)^5 (9+60x+34x^2+56x^3+177x^4-188x^5+28x^6)$

**Simplify[Cf[3, 14, 9]]**

[化简]

$4096 (-1+x)^2 x^2 (1+x)^5 (-9-18x-124x^2+82x^3-207x^4+4x^5+40x^6)$

**Simplify[Cf[3, 14, 10]]**

[化简]

$4096 (-1+x)^2 x^2 (1+x)^5 (-9-18x-124x^2+82x^3-207x^4+4x^5+40x^6)$

**Simplify[Cf[3, 14, 11]]**

[化简]

$-2048 (-1+x)^2 x^2 (1+x)^5 (9+60x+34x^2+56x^3+177x^4-188x^5+28x^6)$

**Simplify[Cf[3, 14, 12]]**

[化简]

$$-2048 (-1+x)^2 x^2 (1+x)^5 (9-14x+132x^2-190x^3+207x^4-180x^5+52x^6)$$

**Simplify[Cf[3, 14, 13]]**

[化简]

$$-4096 (-1+x)^2 x^3 (1+x)^5 (5-5x+3x^2-7x^3+4x^4)$$

**Simplify[Cf[3, 14, 14]]**

[化简]

0

(\*, r2^4r3^0\*)

**Simplify[Cf[4, 0, 0]]**

[化简]

0

**Simplify[Cf[4, 0, 1]]**

[化简]

0

**Simplify[Cf[4, 0, 2]]**

[化简]

0

**Simplify[Cf[4, 0, 3]]**

[化简]

0

**Simplify[Cf[4, 0, 4]]**

[化简]

0

**Simplify[Cf[4, 0, 5]]**

[化简]

0

**Simplify[Cf[4, 0, 6]]**

[化简]

0

**Simplify[Cf[4, 0, 7]]**

[化简]

0

**Simplify[Cf[4, 0, 8]]**

[化简]

0

**Simplify[Cf[4, 0, 9]]**

[化简]

0

**Simplify[Cf[4, 0, 10]]**

[化简]

0

**Simplify[Cf[4, 0, 11]]**

[化简]

0

**Simplify[Cf[4, 0, 12]]**

[化简]

0

**Simplify[Cf[4, 0, 13]]**

[化简]

0

**Simplify[Cf[4, 0, 14]]**

[化简]

0

(\*, r2^4r3^1\*)

**Simplify[Cf[4, 1, 0]]**

[化简]

0

**Simplify[Cf[4, 1, 1]]**

[化简]

0

**Simplify[Cf[4, 1, 2]]**

[化简]

0

**Simplify[Cf[4, 1, 3]]**

[化简]

0

**Simplify[Cf[4, 1, 4]]**

[化简]

0

**Simplify[Cf[4, 1, 5]]**

[化简]

0

**Simplify[Cf[4, 1, 6]]**

[化简]

0

**Simplify[Cf[4, 1, 7]]**

[化简]

0

**Simplify[Cf[4, 1, 8]]**

[化简]

0

**Simplify[Cf[4, 1, 9]]**

[化简]

0

**Simplify[Cf[4, 1, 10]]**

[化简]

0

**Simplify[Cf[4, 1, 11]]**

[化简]

0

**Simplify[Cf[4, 1, 12]]**

[化简]

0

**Simplify[Cf[4, 1, 13]]**

[化简]

0

**Simplify[Cf[4, 1, 14]]**

[化简]

0

**(\*, r2^4r3^2\*)**

**Simplify[Cf[4, 2, 0]]**

[化简]

0

**Simplify[Cf[4, 2, 1]]**

[化简]

0

**Simplify[Cf[4, 2, 2]]**

[化简]

0

**Simplify[Cf[4, 2, 3]]**

[化简]

0

**Simplify[Cf[4, 2, 4]]**

[化简]

0

**Simplify[Cf[4, 2, 5]]**

[化简]

0

**Simplify[Cf[4, 2, 6]]**

[化简]

0

**Simplify[Cf[4, 2, 7]]**

[化简]

0

**Simplify[Cf[4, 2, 8]]**

[化简]

0

**Simplify[Cf[4, 2, 9]]**

[化简]

0

**Simplify[Cf[4, 2, 10]]**

[化简]

0

**Simplify[Cf[4, 2, 11]]**

[化简]

0

**Simplify[Cf[4, 2, 12]]**

[化简]

0

**Simplify[Cf[4, 2, 13]]**

[化简]

0

**Simplify[Cf[4, 2, 14]]**

[化简]

0

(\*, r2^4r3^3\*)

**Simplify[Cf[4, 3, 0]]**

[化简]

0

**Simplify[Cf[4, 3, 1]]**

[化简]

0

**Simplify[Cf[4, 3, 2]]**

[化简]

0

**Simplify[Cf[4, 3, 3]]**

[\[化简\]](#)

0

**Simplify[Cf[4, 3, 4]]**

[\[化简\]](#)

0

**Simplify[Cf[4, 3, 5]]**

[\[化简\]](#)

0

**Simplify[Cf[4, 3, 6]]**

[\[化简\]](#)

0

**Simplify[Cf[4, 3, 7]]**

[\[化简\]](#)

0

**Simplify[Cf[4, 3, 8]]**

[\[化简\]](#)

0

**Simplify[Cf[4, 3, 9]]**

[\[化简\]](#)

0

**Simplify[Cf[4, 3, 10]]**

[\[化简\]](#)

0

**Simplify[Cf[4, 3, 11]]**

[\[化简\]](#)

0

**Simplify[Cf[4, 3, 12]]**

[\[化简\]](#)

0

**Simplify[Cf[4, 3, 13]]**

[\[化简\]](#)

0

**Simplify[Cf[4, 3, 14]]**

[\[化简\]](#)

0

**(\*, r2^4r3^4\*)**

**Simplify[Cf[4, 4, 0]]**

[\[化简\]](#)

0

**Simplify[Cf[4, 4, 1]]**

[化简]

0

**Simplify[Cf[4, 4, 2]]**

[化简]

0

**Simplify[Cf[4, 4, 3]]**

[化简]

0

**Simplify[Cf[4, 4, 4]]**

[化简]

0

**Simplify[Cf[4, 4, 5]]**

[化简]

0

**Simplify[Cf[4, 4, 6]]**

[化简]

0

**Simplify[Cf[4, 4, 7]]**

[化简]

0

**Simplify[Cf[4, 4, 8]]**

[化简]

0

**Simplify[Cf[4, 4, 9]]**

[化简]

0

**Simplify[Cf[4, 4, 10]]**

[化简]

0

**Simplify[Cf[4, 4, 11]]**

[化简]

0

**Simplify[Cf[4, 4, 12]]**

[化简]

0

**Simplify[Cf[4, 4, 13]]**

[化简]

0

**Simplify[Cf[4, 4, 14]]**

[化简]

0

(\*, r2^4r3^5\*)

**Simplify[Cf[4, 5, 0]]**

[化简]

0

**Simplify[Cf[4, 5, 1]]**

[化简]

0

**Simplify[Cf[4, 5, 2]]**

[化简]

0

**Simplify[Cf[4, 5, 3]]**

[化简]

0

**Simplify[Cf[4, 5, 4]]**

[化简]

0

**Simplify[Cf[4, 5, 5]]**

[化简]

0

**Simplify[Cf[4, 5, 6]]**

[化简]

0

**Simplify[Cf[4, 5, 7]]**

[化简]

0

**Simplify[Cf[4, 5, 8]]**

[化简]

0

**Simplify[Cf[4, 5, 9]]**

[化简]

0

**Simplify[Cf[4, 5, 10]]**

[化简]

0

**Simplify[Cf[4, 5, 11]]**

[化简]

0



**Simplify[Cf[4, 5, 12]]**

[化简]

0

**Simplify[Cf[4, 5, 13]]**

[化简]

$12\,288 (-1+x)^3 x^3 (1+x)^5 (2+x+x^3)$

**Simplify[Cf[4, 5, 14]]**

[化简]

$12\,288 (-1+x)^3 x^3 (1+x)^5 (2+x+x^3)$

(\*, r2^4r3^6\*)

**Simplify[Cf[4, 6, 0]]**

[化简]

0

**Simplify[Cf[4, 6, 1]]**

[化简]

0

**Simplify[Cf[4, 6, 2]]**

[化简]

0

**Simplify[Cf[4, 6, 3]]**

[化简]

0

**Simplify[Cf[4, 6, 4]]**

[化简]

0

**Simplify[Cf[4, 6, 5]]**

[化简]

0

**Simplify[Cf[4, 6, 6]]**

[化简]

0

**Simplify[Cf[4, 6, 7]]**

[化简]

0

**Simplify[Cf[4, 6, 8]]**

[化简]

0

**Simplify[Cf[4, 6, 9]]**

[化简]

0

**Simplify[Cf[4, 6, 10]]**

[化简]

0

**Simplify[Cf[4, 6, 11]]**

[化简]

0

**Simplify[Cf[4, 6, 12]]**

[化简]

$$1024 (-1+x) x^2 (1+x)^5 (21+3x+54x^2+250x^3-879x^4+975x^5-572x^6+148x^7)$$

**Simplify[Cf[4, 6, 13]]**

[化简]

$$2048 (-1+x) x^2 (1+x)^5 (35-51x+106x^2+274x^3-961x^4+1057x^5-620x^6+160x^7)$$

**Simplify[Cf[4, 6, 14]]**

[化简]

$$1024 (-1+x) x^2 (1+x)^5 (21+3x+54x^2+250x^3-879x^4+975x^5-572x^6+148x^7)$$

(\*, r2^4r3^7\*)

**Simplify[Cf[4, 7, 0]]**

[化简]

0

**Simplify[Cf[4, 7, 1]]**

[化简]

0

**Simplify[Cf[4, 7, 2]]**

[化简]

0

**Simplify[Cf[4, 7, 3]]**

[化简]

0

**Simplify[Cf[4, 7, 4]]**

[化简]

0

**Simplify[Cf[4, 7, 5]]**

[化简]

0

**Simplify[Cf[4, 7, 6]]**

[化简]

0

**Simplify[Cf[4, 7, 7]]**

[化简]

0

**Simplify[Cf[4, 7, 8]]**

[\[化简\]](#)

0

**Simplify[Cf[4, 7, 9]]**

[\[化简\]](#)

0

**Simplify[Cf[4, 7, 10]]**

[\[化简\]](#)

0

**Simplify[Cf[4, 7, 11]]**

[\[化简\]](#)

$$2048 (-1 + x) x^2 (1 + x)^5 (11 + 127 x - 210 x^2 + 612 x^3 - 659 x^4 + 361 x^5 - 206 x^6 + 44 x^7)$$

**Simplify[Cf[4, 7, 12]]**

[\[化简\]](#)

$$2048 (-1 + x) x (1 + x)^5 (22 - 39 x + 425 x^2 - 474 x^3 + 1292 x^4 - 997 x^5 + 39 x^6 + 50 x^7 - 122 x^8 + 44 x^9)$$

**Simplify[Cf[4, 7, 13]]**

[\[化简\]](#)

$$2048 (-1 + x) x (1 + x)^5 (22 - 39 x + 425 x^2 - 474 x^3 + 1292 x^4 - 997 x^5 + 39 x^6 + 50 x^7 - 122 x^8 + 44 x^9)$$

**Simplify[Cf[4, 7, 14]]**

[\[化简\]](#)

$$2048 (-1 + x) x^2 (1 + x)^5 (11 + 127 x - 210 x^2 + 612 x^3 - 659 x^4 + 361 x^5 - 206 x^6 + 44 x^7)$$

(\*, r2^4r3^8\*)

**Simplify[Cf[4, 8, 0]]**

[\[化简\]](#)

0

**Simplify[Cf[4, 8, 1]]**

[\[化简\]](#)

0

**Simplify[Cf[4, 8, 2]]**

[\[化简\]](#)

0

**Simplify[Cf[4, 8, 3]]**

[\[化简\]](#)

0

**Simplify[Cf[4, 8, 4]]**

[\[化简\]](#)

0

**Simplify[Cf[4, 8, 5]]**

[\[化简\]](#)

0

**Simplify[Cf[4, 8, 6]]**

[\[化简\]](#)

0

**Simplify[Cf[4, 8, 7]]**

[\[化简\]](#)

0

**Simplify[Cf[4, 8, 8]]**

[\[化简\]](#)

0

**Simplify[Cf[4, 8, 9]]**

[\[化简\]](#)

0

**Simplify[Cf[4, 8, 10]]**

[\[化简\]](#)

$$-1024 (-1+x) x^2 (1+x)^5 (-67-69x-926x^2+1166x^3-1907x^4+1219x^5-476x^6+260x^7)$$

**Simplify[Cf[4, 8, 11]]**

[\[化简\]](#)

$$-2048 (-1+x) x (1+x)^5 (-24-95x-484x^2+687x^3-4880x^4+6533x^5-6898x^6+4467x^7-1274x^8+288x^9)$$

**Simplify[Cf[4, 8, 12]]**

[\[化简\]](#)

$$-2048 (-1+x) (1+x)^5 (-24+216x-1539x^2+4297x^3-11896x^4+17098x^5-23731x^6+22197x^7-15418x^8+8320x^9-2464x^{10}+384x^{11})$$

**Simplify[Cf[4, 8, 13]]**

[\[化简\]](#)

$$-2048 (-1+x) x (1+x)^5 (-24-95x-484x^2+687x^3-4880x^4+6533x^5-6898x^6+4467x^7-1274x^8+288x^9)$$

**Simplify[Cf[4, 8, 14]]**

[\[化简\]](#)

$$-1024 (-1+x) x^2 (1+x)^5 (-67-69x-926x^2+1166x^3-1907x^4+1219x^5-476x^6+260x^7)$$

(\*, r2^4r3^9\*)

**Simplify[Cf[4, 9, 0]]**

[\[化简\]](#)

0

**Simplify[Cf[4, 9, 1]]**

[\[化简\]](#)

0

**Simplify[Cf[4, 9, 2]]**

[化简]

0

**Simplify[Cf[4, 9, 3]]**

[化简]

0

**Simplify[Cf[4, 9, 4]]**

[化简]

0

**Simplify[Cf[4, 9, 5]]**

[化简]

0

**Simplify[Cf[4, 9, 6]]**

[化简]

0

**Simplify[Cf[4, 9, 7]]**

[化简]

0

**Simplify[Cf[4, 9, 8]]**

[化简]

0

**Simplify[Cf[4, 9, 9]]**

[化简]

$$4096 (-1 + x) x^2 (1 + x)^5 (11 + 117 x - 182 x^2 + 866 x^3 - 1189 x^4 + 1149 x^5 - 464 x^6 + 12 x^7)$$

**Simplify[Cf[4, 9, 10]]**

[化简]

$$2048 (-1 + x) x (1 + x)^5 (46 + 25 x + 996 x^2 - 651 x^3 + 4598 x^4 - 2185 x^5 + 960 x^6 + 2231 x^7 - 2424 x^8 + 244 x^9)$$

**Simplify[Cf[4, 9, 11]]**

[化简]

$$2048 (-1 + x) x (1 + x)^5 (142 - 283 x + 3407 x^2 - 5194 x^3 + 16796 x^4 - 14679 x^5 + 13931 x^6 - 4048 x^7 - 1260 x^8 - 612 x^9 + 120 x^{10})$$

**Simplify[Cf[4, 9, 12]]**

[化简]

$$2048 (-1 + x) x (1 + x)^5 (142 - 283 x + 3407 x^2 - 5194 x^3 + 16796 x^4 - 14679 x^5 + 13931 x^6 - 4048 x^7 - 1260 x^8 - 612 x^9 + 120 x^{10})$$

**Simplify[Cf[4, 9, 13]]**

[化简]

$$2048 (-1 + x) x (1 + x)^5 (46 + 25 x + 996 x^2 - 651 x^3 + 4598 x^4 - 2185 x^5 + 960 x^6 + 2231 x^7 - 2424 x^8 + 244 x^9)$$

**Simplify[Cf[4, 9, 14]]**

[化简]

$$4096 (-1+x) x^2 (1+x)^5 (11+117x-182x^2+866x^3-1189x^4+1149x^5-464x^6+12x^7)$$

(\*, r2^4r3^10\*)

**Simplify[Cf[4, 10, 0]]**

[化简]

0

**Simplify[Cf[4, 10, 1]]**

[化简]

0

**Simplify[Cf[4, 10, 2]]**

[化简]

0

**Simplify[Cf[4, 10, 3]]**

[化简]

0

**Simplify[Cf[4, 10, 4]]**

[化简]

0

**Simplify[Cf[4, 10, 5]]**

[化简]

0

**Simplify[Cf[4, 10, 6]]**

[化简]

0

**Simplify[Cf[4, 10, 7]]**

[化简]

0

**Simplify[Cf[4, 10, 8]]**

[化简]

$$-1024 (-1+x) x^2 (1+x)^5 (-67-69x-926x^2+1166x^3-1907x^4+1219x^5-476x^6+260x^7)$$

**Simplify[Cf[4, 10, 9]]**

[化简]

$$2048 (-1+x) x (1+x)^5 (46+25x+996x^2-651x^3+4598x^4-2185x^5+960x^6+2231x^7-2424x^8+244x^9)$$

**Simplify[Cf[4, 10, 10]]**

[化简]

$$2048 (-1+x) (1+x)^5 (48-432x+3123x^2-8215x^3+25074x^4-37250x^5+61579x^6-57639x^7+42128x^8-17232x^9+288x^{10}+528x^{11})$$

**Simplify[Cf[4, 10, 11]]**

[化简]

$$2048 (-1+x) x (1+x)^5 (168 - 27x + 4433x^2 - 7114x^3 + 29452x^4 - 29371x^5 + 37213x^6 - 25016x^7 + 17622x^8 - 12952x^9 + 2712x^{10})$$

**Simplify[Cf[4, 10, 12]]**

[化简]

$$2048 (-1+x) (1+x)^5 (48 - 432x + 3123x^2 - 8215x^3 + 25074x^4 - 37250x^5 + 61579x^6 - 57639x^7 + 42128x^8 - 17232x^9 + 288x^{10} + 528x^{11})$$

**Simplify[Cf[4, 10, 13]]**

[化简]

$$2048 (-1+x) x (1+x)^5 (46 + 25x + 996x^2 - 651x^3 + 4598x^4 - 2185x^5 + 960x^6 + 2231x^7 - 2424x^8 + 244x^9)$$

**Simplify[Cf[4, 10, 14]]**

[化简]

$$-1024 (-1+x) x^2 (1+x)^5 (-67 - 69x - 926x^2 + 1166x^3 - 1907x^4 + 1219x^5 - 476x^6 + 260x^7)$$

(\*r2^4r3^11\*)

**Simplify[Cf[4, 11, 0]]**

[化简]

0

**Simplify[Cf[4, 11, 1]]**

[化简]

0

**Simplify[Cf[4, 11, 2]]**

[化简]

0

**Simplify[Cf[4, 11, 3]]**

[化简]

0

**Simplify[Cf[4, 11, 4]]**

[化简]

0

**Simplify[Cf[4, 11, 5]]**

[化简]

0

**Simplify[Cf[4, 11, 6]]**

[化简]

0

**Simplify[Cf[4, 11, 7]]**

[化简]

$$2048 (-1+x) x^2 (1+x)^5 (11 + 127x - 210x^2 + 612x^3 - 659x^4 + 361x^5 - 206x^6 + 44x^7)$$

**Simplify[Cf[4, 11, 8]]**

[化简]

$$-2048 (-1+x) x (1+x)^5 \\ (-24 - 95x - 484x^2 + 687x^3 - 4880x^4 + 6533x^5 - 6898x^6 + 4467x^7 - 1274x^8 + 288x^9)$$

**Simplify[Cf[4, 11, 9]]**

[化简]

$$2048 (-1+x) x (1+x)^5 (142 - 283x + 3407x^2 - 5194x^3 + \\ 16796x^4 - 14679x^5 + 13931x^6 - 4048x^7 - 1260x^8 - 612x^9 + 120x^{10})$$

**Simplify[Cf[4, 11, 10]]**

[化简]

$$2048 (-1+x) x (1+x)^5 (168 - 27x + 4433x^2 - 7114x^3 + \\ 29452x^4 - 29371x^5 + 37213x^6 - 25016x^7 + 17622x^8 - 12952x^9 + 2712x^{10})$$

**Simplify[Cf[4, 11, 11]]**

[化简]

$$2048 (-1+x) x (1+x)^5 (168 - 27x + 4433x^2 - 7114x^3 + \\ 29452x^4 - 29371x^5 + 37213x^6 - 25016x^7 + 17622x^8 - 12952x^9 + 2712x^{10})$$

**Simplify[Cf[4, 11, 12]]**

[化简]

$$2048 (-1+x) x (1+x)^5 (142 - 283x + 3407x^2 - 5194x^3 + \\ 16796x^4 - 14679x^5 + 13931x^6 - 4048x^7 - 1260x^8 - 612x^9 + 120x^{10})$$

**Simplify[Cf[4, 11, 13]]**

[化简]

$$-2048 (-1+x) x (1+x)^5 \\ (-24 - 95x - 484x^2 + 687x^3 - 4880x^4 + 6533x^5 - 6898x^6 + 4467x^7 - 1274x^8 + 288x^9)$$

**Simplify[Cf[4, 11, 14]]**

[化简]

$$2048 (-1+x) x^2 (1+x)^5 (11 + 127x - 210x^2 + 612x^3 - 659x^4 + 361x^5 - 206x^6 + 44x^7)$$

**(\*, r2^4r3^12\*)****Simplify[Cf[4, 12, 0]]**

[化简]

0

**Simplify[Cf[4, 12, 1]]**

[化简]

0

**Simplify[Cf[4, 12, 2]]**

[化简]

0

**Simplify[Cf[4, 12, 3]]**

[化简]

0



**Simplify[Cf[4, 12, 4]]**

[化简]

0

**Simplify[Cf[4, 12, 5]]**

[化简]

0

**Simplify[Cf[4, 12, 6]]**

[化简]

$$1024 (-1+x) x^2 (1+x)^5 (21+3x+54x^2+250x^3-879x^4+975x^5-572x^6+148x^7)$$

**Simplify[Cf[4, 12, 7]]**

[化简]

$$2048 (-1+x) x (1+x)^5 (22-39x+425x^2-474x^3+1292x^4-997x^5+39x^6+50x^7-122x^8+44x^9)$$

**Simplify[Cf[4, 12, 8]]**

[化简]

$$-2048 (-1+x) (1+x)^5 (-24+216x-1539x^2+4297x^3-11896x^4+17098x^5-23731x^6+22197x^7-15418x^8+8320x^9-2464x^{10}+384x^{11})$$

**Simplify[Cf[4, 12, 9]]**

[化简]

$$2048 (-1+x) x (1+x)^5 (142-283x+3407x^2-5194x^3+16796x^4-14679x^5+13931x^6-4048x^7-1260x^8-612x^9+120x^{10})$$

**Simplify[Cf[4, 12, 10]]**

[化简]

$$2048 (-1+x) (1+x)^5 (48-432x+3123x^2-8215x^3+25074x^4-37250x^5+61579x^6-57639x^7+42128x^8-17232x^9+288x^{10}+528x^{11})$$

**Simplify[Cf[4, 12, 11]]**

[化简]

$$2048 (-1+x) x (1+x)^5 (142-283x+3407x^2-5194x^3+16796x^4-14679x^5+13931x^6-4048x^7-1260x^8-612x^9+120x^{10})$$

**Simplify[Cf[4, 12, 12]]**

[化简]

$$-2048 (-1+x) (1+x)^5 (-24+216x-1539x^2+4297x^3-11896x^4+17098x^5-23731x^6+22197x^7-15418x^8+8320x^9-2464x^{10}+384x^{11})$$

**Simplify[Cf[4, 12, 13]]**

[化简]

$$2048 (-1+x) x (1+x)^5 (22-39x+425x^2-474x^3+1292x^4-997x^5+39x^6+50x^7-122x^8+44x^9)$$

**Simplify[Cf[4, 12, 14]]**

[化简]

$$1024 (-1+x) x^2 (1+x)^5 (21+3x+54x^2+250x^3-879x^4+975x^5-572x^6+148x^7)$$

(\*, r2^4r3^13\*)

**Simplify[Cf[4, 13, 0]]**

|化简

0

**Simplify[Cf[4, 13, 1]]**

|化简

0

**Simplify[Cf[4, 13, 2]]**

|化简

0

**Simplify[Cf[4, 13, 3]]**

|化简

0

**Simplify[Cf[4, 13, 4]]**

|化简

0

**Simplify[Cf[4, 13, 5]]**

|化简

$$12\,288 (-1+x)^3 x^3 (1+x)^5 (2+x+x^3)$$

**Simplify[Cf[4, 13, 6]]**

|化简

$$2048 (-1+x) x^2 (1+x)^5 (35-51x+106x^2+274x^3-961x^4+1057x^5-620x^6+160x^7)$$

**Simplify[Cf[4, 13, 7]]**

|化简

$$2048 (-1+x) x (1+x)^5 (22-39x+425x^2-474x^3+1292x^4-997x^5+39x^6+50x^7-122x^8+44x^9)$$

**Simplify[Cf[4, 13, 8]]**

|化简

$$\begin{aligned} & -2048 (-1+x) x (1+x)^5 \\ & (-24-95x-484x^2+687x^3-4880x^4+6533x^5-6898x^6+4467x^7-1274x^8+288x^9) \end{aligned}$$

**Simplify[Cf[4, 13, 9]]**

|化简

$$\begin{aligned} & 2048 (-1+x) x (1+x)^5 \\ & (46+25x+996x^2-651x^3+4598x^4-2185x^5+960x^6+2231x^7-2424x^8+244x^9) \end{aligned}$$

**Simplify[Cf[4, 13, 10]]**

|化简

$$\begin{aligned} & 2048 (-1+x) x (1+x)^5 \\ & (46+25x+996x^2-651x^3+4598x^4-2185x^5+960x^6+2231x^7-2424x^8+244x^9) \end{aligned}$$

**Simplify[Cf[4, 13, 11]]**

|化简

$$\begin{aligned} & -2048 (-1+x) x (1+x)^5 \\ & (-24-95x-484x^2+687x^3-4880x^4+6533x^5-6898x^6+4467x^7-1274x^8+288x^9) \end{aligned}$$

**Simplify[Cf[4, 13, 12]]**

[化简]

$$2048 (-1+x) x (1+x)^5 (22-39x+425x^2-474x^3+1292x^4-997x^5+39x^6+50x^7-122x^8+44x^9)$$

**Simplify[Cf[4, 13, 13]]**

[化简]

$$2048 (-1+x) x^2 (1+x)^5 (35-51x+106x^2+274x^3-961x^4+1057x^5-620x^6+160x^7)$$

**Simplify[Cf[4, 13, 14]]**

[化简]

$$12288 (-1+x)^3 x^3 (1+x)^5 (2+x+x^3)$$

**(\*, r2^4r3^14\*)****Simplify[Cf[4, 14, 0]]**

[化简]

0

**Simplify[Cf[4, 14, 1]]**

[化简]

0

**Simplify[Cf[4, 14, 2]]**

[化简]

0

**Simplify[Cf[4, 14, 3]]**

[化简]

0

**Simplify[Cf[4, 14, 4]]**

[化简]

0

**Simplify[Cf[4, 14, 5]]**

[化简]

$$12288 (-1+x)^3 x^3 (1+x)^5 (2+x+x^3)$$

**Simplify[Cf[4, 14, 6]]**

[化简]

$$1024 (-1+x) x^2 (1+x)^5 (21+3x+54x^2+250x^3-879x^4+975x^5-572x^6+148x^7)$$

**Simplify[Cf[4, 14, 7]]**

[化简]

$$2048 (-1+x) x^2 (1+x)^5 (11+127x-210x^2+612x^3-659x^4+361x^5-206x^6+44x^7)$$

**Simplify[Cf[4, 14, 8]]**

[化简]

$$-1024 (-1+x) x^2 (1+x)^5 (-67-69x-926x^2+1166x^3-1907x^4+1219x^5-476x^6+260x^7)$$

**Simplify[Cf[4, 14, 9]]**

[化简]

$$4096 (-1+x) x^2 (1+x)^5 (11+117x-182x^2+866x^3-1189x^4+1149x^5-464x^6+12x^7)$$

**Simplify[Cf[4, 14, 10]]**

[化简]

$$-1024 (-1+x) x^2 (1+x)^5 (-67-69x-926x^2+1166x^3-1907x^4+1219x^5-476x^6+260x^7)$$

**Simplify[Cf[4, 14, 11]]**

[化简]

$$2048 (-1+x) x^2 (1+x)^5 (11+127x-210x^2+612x^3-659x^4+361x^5-206x^6+44x^7)$$

**Simplify[Cf[4, 14, 12]]**

[化简]

$$1024 (-1+x) x^2 (1+x)^5 (21+3x+54x^2+250x^3-879x^4+975x^5-572x^6+148x^7)$$

**Simplify[Cf[4, 14, 13]]**

[化简]

$$12288 (-1+x)^3 x^3 (1+x)^5 (2+x+x^3)$$

**Simplify[Cf[4, 14, 14]]**

[化简]

0

(\*, r2^5r3^0\*)

**Simplify[Cf[5, 0, 0]]**

[化简]

0

**Simplify[Cf[5, 0, 1]]**

[化简]

0

**Simplify[Cf[5, 0, 2]]**

[化简]

0

**Simplify[Cf[5, 0, 3]]**

[化简]

0

**Simplify[Cf[5, 0, 4]]**

[化简]

0

**Simplify[Cf[5, 0, 5]]**

[化简]

0

**Simplify[Cf[5, 0, 6]]**

[化简]

0

**Simplify[Cf[5, 0, 7]]**

[化简]

0

**Simplify[Cf[5, 0, 8]]**

[化简]

0

**Simplify[Cf[5, 0, 9]]**

[化简]

0

**Simplify[Cf[5, 0, 10]]**

[化简]

0

**Simplify[Cf[5, 0, 11]]**

[化简]

0

**Simplify[Cf[5, 0, 12]]**

[化简]

0

**Simplify[Cf[5, 0, 13]]**

[化简]

0

**Simplify[Cf[5, 0, 14]]**

[化简]

0

(\*, r2^5r3^1\*)

**Simplify[Cf[5, 1, 0]]**

[化简]

0

**Simplify[Cf[5, 1, 1]]**

[化简]

0

**Simplify[Cf[5, 1, 2]]**

[化简]

0

**Simplify[Cf[5, 1, 3]]**

[化简]

0

**Simplify[Cf[5, 1, 4]]**

[化简]

0

**Simplify[Cf[5, 1, 5]]**

[化简]

0

**Simplify[Cf[5, 1, 6]]**

[化简]

0

**Simplify[Cf[5, 1, 7]]**

[化简]

0

**Simplify[Cf[5, 1, 8]]**

[化简]

0

**Simplify[Cf[5, 1, 9]]**

[化简]

0

**Simplify[Cf[5, 1, 10]]**

[化简]

0

**Simplify[Cf[5, 1, 11]]**

[化简]

0

**Simplify[Cf[5, 1, 12]]**

[化简]

0

**Simplify[Cf[5, 1, 13]]**

[化简]

0

**Simplify[Cf[5, 1, 14]]**

[化简]

0

**(\*, r2^5r3^2\*)**

**Simplify[Cf[5, 2, 0]]**

[化简]

0

**Simplify[Cf[5, 2, 1]]**

[化简]

0

**Simplify[Cf[5, 2, 2]]**

[化简]

0

**Simplify[Cf[5, 2, 3]]**

[化简]

0

**Simplify[Cf[5, 2, 4]]**

[化简]

0

**Simplify[Cf[5, 2, 5]]**

[化简]

0

**Simplify[Cf[5, 2, 6]]**

[化简]

0

**Simplify[Cf[5, 2, 7]]**

[化简]

0

**Simplify[Cf[5, 2, 8]]**

[化简]

0

**Simplify[Cf[5, 2, 9]]**

[化简]

0

**Simplify[Cf[5, 2, 10]]**

[化简]

0

**Simplify[Cf[5, 2, 11]]**

[化简]

0

**Simplify[Cf[5, 2, 12]]**

[化简]

0

**Simplify[Cf[5, 2, 13]]**

[化简]

0

**Simplify[Cf[5, 2, 14]]**

[化简]

0

(\*, r2^5r3^3\*)

```
Simplify[Cf[5, 3, 0]]
```

```
[化简
```

```
0
```

```
Simplify[Cf[5, 3, 1]]
```

```
[化简
```

```
0
```

```
Simplify[Cf[5, 3, 2]]
```

```
[化简
```

```
0
```

```
Simplify[Cf[5, 3, 3]]
```

```
[化简
```

```
0
```

```
Simplify[Cf[5, 3, 4]]
```

```
[化简
```

```
0
```

```
Simplify[Cf[5, 3, 5]]
```

```
[化简
```

```
0
```

```
Simplify[Cf[5, 3, 6]]
```

```
[化简
```

```
0
```

```
Simplify[Cf[5, 3, 7]]
```

```
[化简
```

```
0
```

```
Simplify[Cf[5, 3, 8]]
```

```
[化简
```

```
0
```

```
Simplify[Cf[5, 3, 9]]
```

```
[化简
```

```
0
```

```
Simplify[Cf[5, 3, 10]]
```

```
[化简
```

```
0
```

```
Simplify[Cf[5, 3, 11]]
```

```
[化简
```

```
0
```

```
Simplify[Cf[5, 3, 12]]
```

```
[化简
```

```
0
```



**Simplify[Cf[5, 3, 13]]**

[化简]

0

**Simplify[Cf[5, 3, 14]]**

[化简]

0

**(\*, r2^5r3^4\*)**

**Simplify[Cf[5, 4, 0]]**

[化简]

0

**Simplify[Cf[5, 4, 1]]**

[化简]

0

**Simplify[Cf[5, 4, 2]]**

[化简]

0

**Simplify[Cf[5, 4, 3]]**

[化简]

0

**Simplify[Cf[5, 4, 4]]**

[化简]

0

**Simplify[Cf[5, 4, 5]]**

[化简]

0

**Simplify[Cf[5, 4, 6]]**

[化简]

0

**Simplify[Cf[5, 4, 7]]**

[化简]

0

**Simplify[Cf[5, 4, 8]]**

[化简]

0

**Simplify[Cf[5, 4, 9]]**

[化简]

0

**Simplify[Cf[5, 4, 10]]**

[\[化简\]](#)

0

**Simplify[Cf[5, 4, 11]]**

[\[化简\]](#)

0

**Simplify[Cf[5, 4, 12]]**

[\[化简\]](#)

0

**Simplify[Cf[5, 4, 13]]**

[\[化简\]](#)

$12\,288 \left(-1+x\right)^3 x^3 \left(1+x\right)^5 \left(2+x+x^3\right)$

**Simplify[Cf[5, 4, 14]]**

[\[化简\]](#)

$12\,288 \left(-1+x\right)^3 x^3 \left(1+x\right)^5 \left(2+x+x^3\right)$

(\*, r2^5r3^5\*)

**Simplify[Cf[5, 5, 0]]**

[\[化简\]](#)

0

**Simplify[Cf[5, 5, 1]]**

[\[化简\]](#)

0

**Simplify[Cf[5, 5, 2]]**

[\[化简\]](#)

0

**Simplify[Cf[5, 5, 3]]**

[\[化简\]](#)

0

**Simplify[Cf[5, 5, 4]]**

[\[化简\]](#)

0

**Simplify[Cf[5, 5, 5]]**

[\[化简\]](#)

0

**Simplify[Cf[5, 5, 6]]**

[\[化简\]](#)

0

**Simplify[Cf[5, 5, 7]]**

[\[化简\]](#)

0

**Simplify[Cf[5, 5, 8]]**

[\[化简\]](#)

0

**Simplify[Cf[5, 5, 9]]**

[\[化简\]](#)

0

**Simplify[Cf[5, 5, 10]]**

[\[化简\]](#)

0

**Simplify[Cf[5, 5, 11]]**

[\[化简\]](#)

0

**Simplify[Cf[5, 5, 12]]**

[\[化简\]](#)

$-4096 (-1+x)^2 x^2 (1+x)^5 (7-7x+96x^2-102x^3+149x^4-111x^5+40x^6)$

**Simplify[Cf[5, 5, 13]]**

[\[化简\]](#)

$-8192 (-1+x)^2 x^2 (1+x)^5 (11-20x+108x^2-112x^3+161x^4-120x^5+44x^6)$

**Simplify[Cf[5, 5, 14]]**

[\[化简\]](#)

$-4096 (-1+x)^2 x^2 (1+x)^5 (7-7x+96x^2-102x^3+149x^4-111x^5+40x^6)$

(\*, r2^5r3^6\*)

**Simplify[Cf[5, 6, 0]]**

[\[化简\]](#)

0

**Simplify[Cf[5, 6, 1]]**

[\[化简\]](#)

0

**Simplify[Cf[5, 6, 2]]**

[\[化简\]](#)

0

**Simplify[Cf[5, 6, 3]]**

[\[化简\]](#)

0

**Simplify[Cf[5, 6, 4]]**

[\[化简\]](#)

0

**Simplify[Cf[5, 6, 5]]**

[\[化简\]](#)

0

**Simplify[Cf[5, 6, 6]]**

[化简]

0

**Simplify[Cf[5, 6, 7]]**

[化简]

0

**Simplify[Cf[5, 6, 8]]**

[化简]

0

**Simplify[Cf[5, 6, 9]]**

[化简]

0

**Simplify[Cf[5, 6, 10]]**

[化简]

0

**Simplify[Cf[5, 6, 11]]**

[化简]

$$-2048 x^2 (1+x)^5 (15+129 x-276 x^2+570 x^3-597 x^4+37 x^5+198 x^6-96 x^7+20 x^8)$$

**Simplify[Cf[5, 6, 12]]**

[化简]

$$2048 x (1+x)^5 (-30+109 x-767 x^2+1588 x^3-3006 x^4+3343 x^5-1303 x^6+22 x^7+30 x^8+26 x^9-12 x^{10})$$

**Simplify[Cf[5, 6, 13]]**

[化简]

$$2048 x (1+x)^5 (-30+109 x-767 x^2+1588 x^3-3006 x^4+3343 x^5-1303 x^6+22 x^7+30 x^8+26 x^9-12 x^{10})$$

**Simplify[Cf[5, 6, 14]]**

[化简]

$$-2048 x^2 (1+x)^5 (15+129 x-276 x^2+570 x^3-597 x^4+37 x^5+198 x^6-96 x^7+20 x^8)$$

(\*, r2^5r3^7\*)

**Simplify[Cf[5, 7, 0]]**

[化简]

0

**Simplify[Cf[5, 7, 1]]**

[化简]

0

**Simplify[Cf[5, 7, 2]]**

[化简]

0

**Simplify[Cf[5, 7, 3]]**

[\[化简\]](#)

0

**Simplify[Cf[5, 7, 4]]**

[\[化简\]](#)

0

**Simplify[Cf[5, 7, 5]]**

[\[化简\]](#)

0

**Simplify[Cf[5, 7, 6]]**

[\[化简\]](#)

0

**Simplify[Cf[5, 7, 7]]**

[\[化简\]](#)

0

**Simplify[Cf[5, 7, 8]]**

[\[化简\]](#)

0

**Simplify[Cf[5, 7, 9]]**

[\[化简\]](#)

**Simplify[Cf[5, 7, 10]]**

[\[化简\]](#)

$2048 x^2 (1 + x)^5 (-45 - 33 x - 508 x^2 + 870 x^3 - 773 x^4 - 265 x^5 + 1450 x^6 - 1100 x^7 + 308 x^8)$

**Simplify[Cf[5, 7, 11]]**

[\[化简\]](#)

$4096 x^2 (1 + x)^5 (-299 + 1352 x - 5616 x^2 + 11877 x^3 - 18447 x^4 + 19478 x^5 - 12818 x^6 + 5737 x^7 - 1796 x^8 + 340 x^9)$

**Simplify[Cf[5, 7, 12]]**

[\[化简\]](#)

$4096 x (1 + x)^5 (-80 + 393 x - 2217 x^2 + 4730 x^3 - 9858 x^4 + 14329 x^5 - 18549 x^6 + 21468 x^7 - 16396 x^8 + 7712 x^9 - 2132 x^{10} + 312 x^{11})$

**Simplify[Cf[5, 7, 13]]**

[\[化简\]](#)

$4096 x^2 (1 + x)^5 (-299 + 1352 x - 5616 x^2 + 11877 x^3 - 18447 x^4 + 19478 x^5 - 12818 x^6 + 5737 x^7 - 1796 x^8 + 340 x^9)$

**Simplify[Cf[5, 7, 14]]**

[\[化简\]](#)

$2048 x^2 (1 + x)^5 (-45 - 33 x - 508 x^2 + 870 x^3 - 773 x^4 - 265 x^5 + 1450 x^6 - 1100 x^7 + 308 x^8)$

(\*, r2^5r3^8\*)

**Simplify[Cf[5, 8, 0]]**

[化简]

0

**Simplify[Cf[5, 8, 1]]**

[化简]

0

**Simplify[Cf[5, 8, 2]]**

[化简]

0

**Simplify[Cf[5, 8, 3]]**

[化简]

0

**Simplify[Cf[5, 8, 4]]**

[化简]

0

**Simplify[Cf[5, 8, 5]]**

[化简]

0

**Simplify[Cf[5, 8, 6]]**

[化简]

0

**Simplify[Cf[5, 8, 7]]**

[化简]

0

**Simplify[Cf[5, 8, 8]]**

[化简]

0

**Simplify[Cf[5, 8, 9]]**

[化简]

$$-4096 x^2 (1+x)^5 (23+98 x+26 x^2+194 x^3-51 x^4-384 x^5+674 x^6-540 x^7+104 x^8)$$

**Simplify[Cf[5, 8, 10]]**

[化简]

$$-2048 x (1+x)^5 (94-303 x+3119 x^2-6866 x^3+17814 x^4-22905 x^5+21615 x^6-15272 x^7+5986 x^8-1982 x^9+236 x^{10})$$

**Simplify[Cf[5, 8, 11]]**

[化简]

$$2048 x (1+x)^5 (-238+753 x-6036 x^2+11066 x^3-26967 x^4+30947 x^5-31826 x^6+26928 x^7-10617 x^8+2938 x^9-140 x^{10}+24 x^{11})$$

**Simplify[Cf[5, 8, 12]]**

[化简]

$$2048 x (1+x)^5 (-238 + 753 x - 6036 x^2 + 11066 x^3 - 26967 x^4 + 30947 x^5 - 31826 x^6 + 26928 x^7 - 10617 x^8 + 2938 x^9 - 140 x^{10} + 24 x^{11})$$

**Simplify[Cf[5, 8, 13]]**

[化简]

$$-2048 x (1+x)^5 (94 - 303 x + 3119 x^2 - 6866 x^3 + 17814 x^4 - 22905 x^5 + 21615 x^6 - 15272 x^7 + 5986 x^8 - 1982 x^9 + 236 x^{10})$$

**Simplify[Cf[5, 8, 14]]**

[化简]

$$-4096 x^2 (1+x)^5 (23 + 98 x + 26 x^2 + 194 x^3 - 51 x^4 - 384 x^5 + 674 x^6 - 540 x^7 + 104 x^8)$$

(\*, r2^5r3^9\*)

**Simplify[Cf[5, 9, 0]]**

[化简]

0

**Simplify[Cf[5, 9, 1]]**

[化简]

0

**Simplify[Cf[5, 9, 2]]**

[化简]

0

**Simplify[Cf[5, 9, 3]]**

[化简]

0

**Simplify[Cf[5, 9, 4]]**

[化简]

0

**Simplify[Cf[5, 9, 5]]**

[化简]

0

**Simplify[Cf[5, 9, 6]]**

[化简]

0

**Simplify[Cf[5, 9, 7]]**

[化简]

0

**Simplify[Cf[5, 9, 8]]**

[化简]

$$-4096 x^2 (1+x)^5 (23 + 98 x + 26 x^2 + 194 x^3 - 51 x^4 - 384 x^5 + 674 x^6 - 540 x^7 + 104 x^8)$$

**Simplify[Cf[5, 9, 9]]**

[化简]

$$-8192 x^2 (1+x)^5 (279 - 1252 x + 5397 x^2 - 10826 x^3 + 16897 x^4 - 16812 x^5 + 10319 x^6 - 3486 x^7 - 156 x^8 + 216 x^9)$$

**Simplify[Cf[5, 9, 10]]**

[化简]

$$-2048 x (1+x)^5 (368 - 1398 x + 9883 x^2 - 17514 x^3 + 44189 x^4 - 58954 x^5 + 85081 x^6 - 92946 x^7 + 62287 x^8 - 29148 x^9 + 4128 x^{10} + 648 x^{11})$$

**Simplify[Cf[5, 9, 11]]**

[化简]

$$-8192 x^2 (1+x)^5 (1015 - 4761 x + 20474 x^2 - 42830 x^3 + 70527 x^4 - 75961 x^5 + 60448 x^6 - 38664 x^7 + 16928 x^8 - 6072 x^9 + 1200 x^{10})$$

**Simplify[Cf[5, 9, 12]]**

[化简]

$$-2048 x (1+x)^5 (368 - 1398 x + 9883 x^2 - 17514 x^3 + 44189 x^4 - 58954 x^5 + 85081 x^6 - 92946 x^7 + 62287 x^8 - 29148 x^9 + 4128 x^{10} + 648 x^{11})$$

**Simplify[Cf[5, 9, 13]]**

[化简]

$$-8192 x^2 (1+x)^5 (279 - 1252 x + 5397 x^2 - 10826 x^3 + 16897 x^4 - 16812 x^5 + 10319 x^6 - 3486 x^7 - 156 x^8 + 216 x^9)$$

**Simplify[Cf[5, 9, 14]]**

[化简]

$$-4096 x^2 (1+x)^5 (23 + 98 x + 26 x^2 + 194 x^3 - 51 x^4 - 384 x^5 + 674 x^6 - 540 x^7 + 104 x^8)$$

**(\*, r2^5r3^10\*)****Simplify[Cf[5, 10, 0]]**

[化简]

0

**Simplify[Cf[5, 10, 1]]**

[化简]

0

**Simplify[Cf[5, 10, 2]]**

[化简]

0

**Simplify[Cf[5, 10, 3]]**

[化简]

0

**Simplify[Cf[5, 10, 4]]**

[化简]

0



**Simplify[Cf[5, 10, 5]]**

[化简]

0

**Simplify[Cf[5, 10, 6]]**

[化简]

0

**Simplify[Cf[5, 10, 7]]**

[化简]

$$2048 x^2 (1+x)^5 (-45 - 33 x - 508 x^2 + 870 x^3 - 773 x^4 - 265 x^5 + 1450 x^6 - 1100 x^7 + 308 x^8)$$

**Simplify[Cf[5, 10, 8]]**

[化简]

$$-2048 x (1+x)^5 (94 - 303 x + 3119 x^2 - 6866 x^3 + 17814 x^4 - 22905 x^5 + 21615 x^6 - 15272 x^7 + 5986 x^8 - 1982 x^9 + 236 x^{10})$$

**Simplify[Cf[5, 10, 9]]**

[化简]

$$-2048 x (1+x)^5 (368 - 1398 x + 9883 x^2 - 17514 x^3 + 44189 x^4 - 58954 x^5 + 85081 x^6 - 92946 x^7 + 62287 x^8 - 29148 x^9 + 4128 x^{10} + 648 x^{11})$$

**Simplify[Cf[5, 10, 10]]**

[化简]

$$-8192 x (1+x)^5 (120 - 360 x + 3492 x^2 - 6400 x^3 + 17918 x^4 - 21997 x^5 + 27966 x^6 - 23532 x^7 + 9060 x^8 - 1027 x^9 - 3428 x^{10} + 1404 x^{11})$$

**Simplify[Cf[5, 10, 11]]**

[化简]

$$-8192 x (1+x)^5 (120 - 360 x + 3492 x^2 - 6400 x^3 + 17918 x^4 - 21997 x^5 + 27966 x^6 - 23532 x^7 + 9060 x^8 - 1027 x^9 - 3428 x^{10} + 1404 x^{11})$$

**Simplify[Cf[5, 10, 12]]**

[化简]

$$-2048 x (1+x)^5 (368 - 1398 x + 9883 x^2 - 17514 x^3 + 44189 x^4 - 58954 x^5 + 85081 x^6 - 92946 x^7 + 62287 x^8 - 29148 x^9 + 4128 x^{10} + 648 x^{11})$$

**Simplify[Cf[5, 10, 13]]**

[化简]

$$-2048 x (1+x)^5 (94 - 303 x + 3119 x^2 - 6866 x^3 + 17814 x^4 - 22905 x^5 + 21615 x^6 - 15272 x^7 + 5986 x^8 - 1982 x^9 + 236 x^{10})$$

**Simplify[Cf[5, 10, 14]]**

[化简]

$$2048 x^2 (1+x)^5 (-45 - 33 x - 508 x^2 + 870 x^3 - 773 x^4 - 265 x^5 + 1450 x^6 - 1100 x^7 + 308 x^8)$$

(\*, r2^5r3^11\*)

**Simplify[Cf[5, 11, 0]]**

[化简]

0

**Simplify[Cf[5, 11, 1]]**

[化简]

0

**Simplify[Cf[5, 11, 2]]**

[化简]

0

**Simplify[Cf[5, 11, 3]]**

[化简]

0

**Simplify[Cf[5, 11, 4]]**

[化简]

0

**Simplify[Cf[5, 11, 5]]**

[化简]

0

**Simplify[Cf[5, 11, 6]]**

[化简]

$$-2048 x^2 (1+x)^5 (15+129 x-276 x^2+570 x^3-597 x^4+37 x^5+198 x^6-96 x^7+20 x^8)$$

**Simplify[Cf[5, 11, 7]]**

[化简]

$$4096 x^2 (1+x)^5 (-299+1352 x-5616 x^2+11877 x^3-18447 x^4+19478 x^5-12818 x^6+5737 x^7-1796 x^8+340 x^9)$$

**Simplify[Cf[5, 11, 8]]**

[化简]

$$2048 x (1+x)^5 (-238+753 x-6036 x^2+11066 x^3-26967 x^4+30947 x^5-31826 x^6+26928 x^7-10617 x^8+2938 x^9-140 x^{10}+24 x^{11})$$

**Simplify[Cf[5, 11, 9]]**

[化简]

$$-8192 x^2 (1+x)^5 (1015-4761 x+20474 x^2-42830 x^3+70527 x^4-75961 x^5+60448 x^6-38664 x^7+16928 x^8-6072 x^9+1200 x^{10})$$

**Simplify[Cf[5, 11, 10]]**

[化简]

$$-8192 x (1+x)^5 (120-360 x+3492 x^2-6400 x^3+17918 x^4-21997 x^5+27966 x^6-23532 x^7+9060 x^8-1027 x^9-3428 x^{10}+1404 x^{11})$$

**Simplify[Cf[5, 11, 11]]**

[化简]

$$-8192 x^2 (1+x)^5 (1015-4761 x+20474 x^2-42830 x^3+70527 x^4-75961 x^5+60448 x^6-38664 x^7+16928 x^8-6072 x^9+1200 x^{10})$$

**Simplify[Cf[5, 11, 12]]**

|化简

$$2048 x (1+x)^5 (-238 + 753 x - 6036 x^2 + 11066 x^3 - 26967 x^4 + 30947 x^5 - 31826 x^6 + 26928 x^7 - 10617 x^8 + 2938 x^9 - 140 x^{10} + 24 x^{11})$$

**Simplify[Cf[5, 11, 13]]**

|化简

$$4096 x^2 (1+x)^5 (-299 + 1352 x - 5616 x^2 + 11877 x^3 - 18447 x^4 + 19478 x^5 - 12818 x^6 + 5737 x^7 - 1796 x^8 + 340 x^9)$$

**Simplify[Cf[5, 11, 14]]**

|化简

$$-2048 x^2 (1+x)^5 (15 + 129 x - 276 x^2 + 570 x^3 - 597 x^4 + 37 x^5 + 198 x^6 - 96 x^7 + 20 x^8)$$

**(\*, r2^5r3^12\*)****Simplify[Cf[5, 12, 0]]**

|化简

0

**Simplify[Cf[5, 12, 1]]**

|化简

0

**Simplify[Cf[5, 12, 2]]**

|化简

0

**Simplify[Cf[5, 12, 3]]**

|化简

0

**Simplify[Cf[5, 12, 4]]**

|化简

0

**Simplify[Cf[5, 12, 5]]**

|化简

$$-4096 (-1+x)^2 x^2 (1+x)^5 (7 - 7 x + 96 x^2 - 102 x^3 + 149 x^4 - 111 x^5 + 40 x^6)$$

**Simplify[Cf[5, 12, 6]]**

|化简

$$2048 x (1+x)^5 (-30 + 109 x - 767 x^2 + 1588 x^3 - 3006 x^4 + 3343 x^5 - 1303 x^6 + 22 x^7 + 30 x^8 + 26 x^9 - 12 x^{10})$$

**Simplify[Cf[5, 12, 7]]**

|化简

$$4096 x (1+x)^5 (-80 + 393 x - 2217 x^2 + 4730 x^3 - 9858 x^4 + 14329 x^5 - 18549 x^6 + 21468 x^7 - 16396 x^8 + 7712 x^9 - 2132 x^{10} + 312 x^{11})$$

**Simplify[Cf[5, 12, 8]]**

[化简]

$$2048 x (1+x)^5 (-238 + 753 x - 6036 x^2 + 11066 x^3 - 26967 x^4 + 30947 x^5 - 31826 x^6 + 26928 x^7 - 10617 x^8 + 2938 x^9 - 140 x^{10} + 24 x^{11})$$

**Simplify[Cf[5, 12, 9]]**

[化简]

$$-2048 x (1+x)^5 (368 - 1398 x + 9883 x^2 - 17514 x^3 + 44189 x^4 - 58954 x^5 + 85081 x^6 - 92946 x^7 + 62287 x^8 - 29148 x^9 + 4128 x^{10} + 648 x^{11})$$

**Simplify[Cf[5, 12, 10]]**

[化简]

$$-2048 x (1+x)^5 (368 - 1398 x + 9883 x^2 - 17514 x^3 + 44189 x^4 - 58954 x^5 + 85081 x^6 - 92946 x^7 + 62287 x^8 - 29148 x^9 + 4128 x^{10} + 648 x^{11})$$

**Simplify[Cf[5, 12, 11]]**

[化简]

$$2048 x (1+x)^5 (-238 + 753 x - 6036 x^2 + 11066 x^3 - 26967 x^4 + 30947 x^5 - 31826 x^6 + 26928 x^7 - 10617 x^8 + 2938 x^9 - 140 x^{10} + 24 x^{11})$$

**Simplify[Cf[5, 12, 12]]**

[化简]

$$4096 x (1+x)^5 (-80 + 393 x - 2217 x^2 + 4730 x^3 - 9858 x^4 + 14329 x^5 - 18549 x^6 + 21468 x^7 - 16396 x^8 + 7712 x^9 - 2132 x^{10} + 312 x^{11})$$

**Simplify[Cf[5, 12, 13]]**

[化简]

$$2048 x (1+x)^5 (-30 + 109 x - 767 x^2 + 1588 x^3 - 3006 x^4 + 3343 x^5 - 1303 x^6 + 22 x^7 + 30 x^8 + 26 x^9 - 12 x^{10})$$

**Simplify[Cf[5, 12, 14]]**

[化简]

$$-4096 (-1+x)^2 x^2 (1+x)^5 (7 - 7 x + 96 x^2 - 102 x^3 + 149 x^4 - 111 x^5 + 40 x^6)$$

**(\*, r2^5r3^13\*)****Simplify[Cf[5, 13, 0]]**

[化简]

0

**Simplify[Cf[5, 13, 1]]**

[化简]

0

**Simplify[Cf[5, 13, 2]]**

[化简]

0

**Simplify[Cf[5, 13, 3]]**

[化简]

0

**Simplify[Cf[5, 13, 4]]**

[化简]

$$12\,288 (-1+x)^3 x^3 (1+x)^5 (2+x+x^3)$$

**Simplify[Cf[5, 13, 5]]**

[化简]

$$-8192 (-1+x)^2 x^2 (1+x)^5 (11-20x+108x^2-112x^3+161x^4-120x^5+44x^6)$$

**Simplify[Cf[5, 13, 6]]**

[化简]

$$2048 x (1+x)^5 (-30+109x-767x^2+1588x^3-3006x^4+3343x^5-1303x^6+22x^7+30x^8+26x^9-12x^{10})$$

**Simplify[Cf[5, 13, 7]]**

[化简]

$$4096 x^2 (1+x)^5 (-299+1352x-5616x^2+11877x^3-18447x^4+19478x^5-12818x^6+5737x^7-1796x^8+340x^9)$$

**Simplify[Cf[5, 13, 8]]**

[化简]

$$-2048 x (1+x)^5 (94-303x+3119x^2-6866x^3+17814x^4-22905x^5+21615x^6-15272x^7+5986x^8-1982x^9+236x^{10})$$

**Simplify[Cf[5, 13, 9]]**

[化简]

$$-8192 x^2 (1+x)^5 (279-1252x+5397x^2-10826x^3+16897x^4-16812x^5+10319x^6-3486x^7-156x^8+216x^9)$$

**Simplify[Cf[5, 13, 10]]**

[化简]

$$-2048 x (1+x)^5 (94-303x+3119x^2-6866x^3+17814x^4-22905x^5+21615x^6-15272x^7+5986x^8-1982x^9+236x^{10})$$

**Simplify[Cf[5, 13, 11]]**

[化简]

$$4096 x^2 (1+x)^5 (-299+1352x-5616x^2+11877x^3-18447x^4+19478x^5-12818x^6+5737x^7-1796x^8+340x^9)$$

**Simplify[Cf[5, 13, 12]]**

[化简]

$$2048 x (1+x)^5 (-30+109x-767x^2+1588x^3-3006x^4+3343x^5-1303x^6+22x^7+30x^8+26x^9-12x^{10})$$

**Simplify[Cf[5, 13, 13]]**

[化简]

$$-8192 (-1+x)^2 x^2 (1+x)^5 (11-20x+108x^2-112x^3+161x^4-120x^5+44x^6)$$

**Simplify[Cf[5, 13, 14]]**

[化简]

$$12\,288 (-1+x)^3 x^3 (1+x)^5 (2+x+x^3)$$

(\*, r2^5r3^14\*)

**Simplify[Cf[5, 14, 0]]**

[化简]

0

**Simplify[Cf[5, 14, 1]]**

[化简]

0

**Simplify[Cf[5, 14, 2]]**

[化简]

0

**Simplify[Cf[5, 14, 3]]**

[化简]

0

**Simplify[Cf[5, 14, 4]]**

[化简]

$12\,288 (-1+x)^3 x^3 (1+x)^5 (2+x+x^3)$

**Simplify[Cf[5, 14, 5]]**

[化简]

$-4096 (-1+x)^2 x^2 (1+x)^5 (7-7x+96x^2-102x^3+149x^4-111x^5+40x^6)$

**Simplify[Cf[5, 14, 6]]**

[化简]

$-2048 x^2 (1+x)^5 (15+129x-276x^2+570x^3-597x^4+37x^5+198x^6-96x^7+20x^8)$

**Simplify[Cf[5, 14, 7]]**

[化简]

$2048 x^2 (1+x)^5 (-45-33x-508x^2+870x^3-773x^4-265x^5+1450x^6-1100x^7+308x^8)$

**Simplify[Cf[5, 14, 8]]**

[化简]

$-4096 x^2 (1+x)^5 (23+98x+26x^2+194x^3-51x^4-384x^5+674x^6-540x^7+104x^8)$

**Simplify[Cf[5, 14, 9]]**

[化简]

$-4096 x^2 (1+x)^5 (23+98x+26x^2+194x^3-51x^4-384x^5+674x^6-540x^7+104x^8)$

**Simplify[Cf[5, 14, 10]]**

[化简]

$2048 x^2 (1+x)^5 (-45-33x-508x^2+870x^3-773x^4-265x^5+1450x^6-1100x^7+308x^8)$

**Simplify[Cf[5, 14, 11]]**

[化简]

$-2048 x^2 (1+x)^5 (15+129x-276x^2+570x^3-597x^4+37x^5+198x^6-96x^7+20x^8)$

**Simplify[Cf[5, 14, 12]]**

[化简]

$$-4096 (-1+x)^2 x^2 (1+x)^5 (7-7x+96x^2-102x^3+149x^4-111x^5+40x^6)$$

**Simplify[Cf[5, 14, 13]]**

[化简]

$$12288 (-1+x)^3 x^3 (1+x)^5 (2+x+x^3)$$

**Simplify[Cf[5, 14, 14]]**

[化简]

0

(\*, r2^6r3^0\*)

**Simplify[Cf[6, 0, 0]]**

[化简]

0

**Simplify[Cf[6, 0, 1]]**

[化简]

0

**Simplify[Cf[6, 0, 2]]**

[化简]

0

**Simplify[Cf[6, 0, 3]]**

[化简]

0

**Simplify[Cf[6, 0, 4]]**

[化简]

0

**Simplify[Cf[6, 0, 5]]**

[化简]

0

**Simplify[Cf[6, 0, 6]]**

[化简]

0

**Simplify[Cf[6, 0, 7]]**

[化简]

0

**Simplify[Cf[6, 0, 8]]**

[化简]

0

**Simplify[Cf[6, 0, 9]]**

[化简]

0

**Simplify[Cf[6, 0, 10]]**

[化简]

0

**Simplify[Cf[6, 0, 11]]**

[化简]

0

**Simplify[Cf[6, 0, 12]]**

[化简]

0

**Simplify[Cf[6, 0, 13]]**

[化简]

0

**Simplify[Cf[6, 0, 14]]**

[化简]

0

**(\*, r2^6r3^1\*)**

**Simplify[Cf[6, 1, 0]]**

[化简]

0

**Simplify[Cf[6, 1, 1]]**

[化简]

0

**Simplify[Cf[6, 1, 2]]**

[化简]

0

**Simplify[Cf[6, 1, 3]]**

[化简]

0

**Simplify[Cf[6, 1, 4]]**

[化简]

0

**Simplify[Cf[6, 1, 5]]**

[化简]

0

**Simplify[Cf[6, 1, 6]]**

[化简]

0



**Simplify[Cf[6, 1, 7]]**

[化简]

0

**Simplify[Cf[6, 1, 8]]**

[化简]

0

**Simplify[Cf[6, 1, 9]]**

[化简]

0

**Simplify[Cf[6, 1, 10]]**

[化简]

0

**Simplify[Cf[6, 1, 11]]**

[化简]

0

**Simplify[Cf[6, 1, 12]]**

[化简]

0

**Simplify[Cf[6, 1, 13]]**

[化简]

0

**Simplify[Cf[6, 1, 14]]**

[化简]

0

(\*, r2^6r3^2\*)

**Simplify[Cf[6, 2, 0]]**

[化简]

0

**Simplify[Cf[6, 2, 1]]**

[化简]

0

**Simplify[Cf[6, 2, 2]]**

[化简]

0

**Simplify[Cf[6, 2, 3]]**

[化简]

0

**Simplify[Cf[6, 2, 4]]**

[化简]

0

**Simplify[Cf[6, 2, 5]]**

[化简]

0

**Simplify[Cf[6, 2, 6]]**

[化简]

0

**Simplify[Cf[6, 2, 7]]**

[化简]

0

**Simplify[Cf[6, 2, 8]]**

[化简]

0

**Simplify[Cf[6, 2, 9]]**

[化简]

0

**Simplify[Cf[6, 2, 10]]**

[化简]

0

**Simplify[Cf[6, 2, 11]]**

[化简]

0

**Simplify[Cf[6, 2, 12]]**

[化简]

0

**Simplify[Cf[6, 2, 13]]**

[化简]

0

**Simplify[Cf[6, 2, 14]]**

[化简]

0

**(\*, r2^6r3^3\*)**

**Simplify[Cf[6, 3, 0]]**

[化简]

0

**Simplify[Cf[6, 3, 1]]**

[化简]

0

**Simplify[Cf[6, 3, 2]]**

[化简]

0

**Simplify[Cf[6, 3, 3]]**

[化简]

0

**Simplify[Cf[6, 3, 4]]**

[化简]

0

**Simplify[Cf[6, 3, 5]]**

[化简]

0

**Simplify[Cf[6, 3, 6]]**

[化简]

0

**Simplify[Cf[6, 3, 7]]**

[化简]

0

**Simplify[Cf[6, 3, 8]]**

[化简]

0

**Simplify[Cf[6, 3, 9]]**

[化简]

0

**Simplify[Cf[6, 3, 10]]**

[化简]

0

**Simplify[Cf[6, 3, 11]]**

[化简]

0

**Simplify[Cf[6, 3, 12]]**

[化简]

0

**Simplify[Cf[6, 3, 13]]**

[化简]

$-4096 (-1+x)^3 x^3 (1+x)^5 (-5-3x^2+4x^3)$

**Simplify[Cf[6, 3, 14]]**

[化简]

$-4096 (-1+x)^3 x^3 (1+x)^5 (-5-3x^2+4x^3)$

(\*, r2^6r3^4\*)

**Simplify[Cf[6, 4, 0]]**

[化简]

0

**Simplify[Cf[6, 4, 1]]**

[化简]

0

**Simplify[Cf[6, 4, 2]]**

[化简]

0

**Simplify[Cf[6, 4, 3]]**

[化简]

0

**Simplify[Cf[6, 4, 4]]**

[化简]

0

**Simplify[Cf[6, 4, 5]]**

[化简]

0

**Simplify[Cf[6, 4, 6]]**

[化简]

0

**Simplify[Cf[6, 4, 7]]**

[化简]

0

**Simplify[Cf[6, 4, 8]]**

[化简]

0

**Simplify[Cf[6, 4, 9]]**

[化简]

0

**Simplify[Cf[6, 4, 10]]**

[化简]

0

**Simplify[Cf[6, 4, 11]]**

[化简]

0

**Simplify[Cf[6, 4, 12]]**

[化简]

$1024 (-1 + x)^2 x^2 (1 + x)^5 (-21 - 24 x - 78 x^2 - 328 x^3 + 551 x^4 - 424 x^5 + 148 x^6)$

**Simplify[Cf[6, 4, 13]]**

[化简]

$$2048 (-1+x)^2 x^2 (1+x)^5 (-35+16x-90x^2-364x^3+597x^4-460x^5+160x^6)$$

**Simplify[Cf[6, 4, 14]]**

[化简]

$$1024 (-1+x)^2 x^2 (1+x)^5 (-21-24x-78x^2-328x^3+551x^4-424x^5+148x^6)$$

(\*, r2^6r3^5\*)

**Simplify[Cf[6, 5, 0]]**

[化简]

0

**Simplify[Cf[6, 5, 1]]**

[化简]

0

**Simplify[Cf[6, 5, 2]]**

[化简]

0

**Simplify[Cf[6, 5, 3]]**

[化简]

0

**Simplify[Cf[6, 5, 4]]**

[化简]

0

**Simplify[Cf[6, 5, 5]]**

[化简]

0

**Simplify[Cf[6, 5, 6]]**

[化简]

0

**Simplify[Cf[6, 5, 7]]**

[化简]

0

**Simplify[Cf[6, 5, 8]]**

[化简]

0

**Simplify[Cf[6, 5, 9]]**

[化简]

0

**Simplify[Cf[6, 5, 10]]**

[化简]

0

**Simplify[Cf[6, 5, 11]]**

[化简]

$$-2048 x^2 (1+x)^5 (15+129 x-276 x^2+570 x^3-597 x^4+37 x^5+198 x^6-96 x^7+20 x^8)$$

**Simplify[Cf[6, 5, 12]]**

[化简]

$$-2048 x (1+x)^5 (30-109 x+767 x^2-1588 x^3+3006 x^4-3343 x^5+1303 x^6-22 x^7-30 x^8-26 x^9+12 x^{10})$$

**Simplify[Cf[6, 5, 13]]**

[化简]

$$-2048 x (1+x)^5 (30-109 x+767 x^2-1588 x^3+3006 x^4-3343 x^5+1303 x^6-22 x^7-30 x^8-26 x^9+12 x^{10})$$

**Simplify[Cf[6, 5, 14]]**

[化简]

$$-2048 x^2 (1+x)^5 (15+129 x-276 x^2+570 x^3-597 x^4+37 x^5+198 x^6-96 x^7+20 x^8)$$

(\*, r2^6r3^6\*)

**Simplify[Cf[6, 6, 0]]**

[化简]

0

**Simplify[Cf[6, 6, 1]]**

[化简]

0

**Simplify[Cf[6, 6, 2]]**

[化简]

0

**Simplify[Cf[6, 6, 3]]**

[化简]

0

**Simplify[Cf[6, 6, 4]]**

[化简]

0

**Simplify[Cf[6, 6, 5]]**

[化简]

0

**Simplify[Cf[6, 6, 6]]**

[化简]

0

**Simplify[Cf[6, 6, 7]]**

[化简]

0

**Simplify[Cf[6, 6, 8]]**

[化简]

0

**Simplify[Cf[6, 6, 9]]**

[化简]

0

**Simplify[Cf[6, 6, 10]]**

[化简]

$$-2048 x^2 (1+x)^5 (53 + 837 x^2 - 1888 x^3 + 3187 x^4 - 3528 x^5 + 2623 x^6 - 1528 x^7 + 436 x^8)$$

**Simplify[Cf[6, 6, 11]]**

[化简]

$$-4096 x (1+x)^5 (18 + 57 x + 380 x^2 - 1128 x^3 + 5543 x^4 - 10971 x^5 + 14182 x^6 - 12722 x^7 + 6857 x^8 - 2276 x^9 + 444 x^{10})$$

**Simplify[Cf[6, 6, 12]]**

[化简]

$$-4096 (1+x)^5 (18 - 180 x + 1349 x^2 - 4492 x^3 + 12813 x^4 - 22478 x^5 + 32069 x^6 - 34832 x^7 + 28217 x^8 - 18466 x^9 + 8598 x^{10} - 2400 x^{11} + 360 x^{12})$$

**Simplify[Cf[6, 6, 13]]**

[化简]

$$-4096 x (1+x)^5 (18 + 57 x + 380 x^2 - 1128 x^3 + 5543 x^4 - 10971 x^5 + 14182 x^6 - 12722 x^7 + 6857 x^8 - 2276 x^9 + 444 x^{10})$$

**Simplify[Cf[6, 6, 14]]**

[化简]

$$-2048 x^2 (1+x)^5 (53 + 837 x^2 - 1888 x^3 + 3187 x^4 - 3528 x^5 + 2623 x^6 - 1528 x^7 + 436 x^8)$$

(\*, r2^6r3^7\*)

**Simplify[Cf[6, 7, 0]]**

[化简]

0

**Simplify[Cf[6, 7, 1]]**

[化简]

0

**Simplify[Cf[6, 7, 2]]**

[化简]

0

**Simplify[Cf[6, 7, 3]]**

[化简]

0

**Simplify[Cf[6, 7, 4]]**

[化简]

0

**Simplify[Cf[6, 7, 5]]**

[\[化简\]](#)

0

**Simplify[Cf[6, 7, 6]]**

[\[化简\]](#)

0

**Simplify[Cf[6, 7, 7]]**

[\[化简\]](#)

0

**Simplify[Cf[6, 7, 8]]**

[\[化简\]](#)

0

**Simplify[Cf[6, 7, 9]]**

[\[化简\]](#)

$$2048 x^2 (1 + x)^5 (-49 - 363 x + 500 x^2 - 2542 x^3 + 3875 x^4 - 3919 x^5 + 2046 x^6 - 520 x^7 + 108 x^8)$$

**Simplify[Cf[6, 7, 10]]**

[\[化简\]](#)

$$2048 x (1 + x)^5 (-102 + 188 x - 2949 x^2 + 5328 x^3 - 16599 x^4 + 19224 x^5 - 17363 x^6 + 8556 x^7 - 391 x^8 - 560 x^9 + 60 x^{10})$$

**Simplify[Cf[6, 7, 11]]**

[\[化简\]](#)

$$-2048 x (1 + x)^5 (282 - 791 x + 7232 x^2 - 13452 x^3 + 36789 x^4 - 41995 x^5 + 42522 x^6 - 25450 x^7 + 3219 x^8 + 1336 x^9 - 236 x^{10} + 48 x^{11})$$

**Simplify[Cf[6, 7, 12]]**

[\[化简\]](#)

$$-2048 x (1 + x)^5 (282 - 791 x + 7232 x^2 - 13452 x^3 + 36789 x^4 - 41995 x^5 + 42522 x^6 - 25450 x^7 + 3219 x^8 + 1336 x^9 - 236 x^{10} + 48 x^{11})$$

**Simplify[Cf[6, 7, 13]]**

[\[化简\]](#)

$$2048 x (1 + x)^5 (-102 + 188 x - 2949 x^2 + 5328 x^3 - 16599 x^4 + 19224 x^5 - 17363 x^6 + 8556 x^7 - 391 x^8 - 560 x^9 + 60 x^{10})$$

**Simplify[Cf[6, 7, 14]]**

[\[化简\]](#)

$$2048 x^2 (1 + x)^5 (-49 - 363 x + 500 x^2 - 2542 x^3 + 3875 x^4 - 3919 x^5 + 2046 x^6 - 520 x^7 + 108 x^8)$$

(\*, r2^6r3^8\*)

**Simplify[Cf[6, 8, 0]]**

[\[化简\]](#)

0



**Simplify[Cf[6, 8, 1]]**

[化简]

0

**Simplify[Cf[6, 8, 2]]**

[化简]

0

**Simplify[Cf[6, 8, 3]]**

[化简]

0

**Simplify[Cf[6, 8, 4]]**

[化简]

0

**Simplify[Cf[6, 8, 5]]**

[化简]

0

**Simplify[Cf[6, 8, 6]]**

[化简]

0

**Simplify[Cf[6, 8, 7]]**

[化简]

0

**Simplify[Cf[6, 8, 8]]**

[化简]

$$2048 x^2 (1+x)^5 (-85 - 26 x - 1639 x^2 + 3668 x^3 - 7407 x^4 + 7286 x^5 - 3481 x^6 - 208 x^7 + 548 x^8)$$

**Simplify[Cf[6, 8, 9]]**

[化简]

$$2048 x (1+x)^5 (-108 - 12 x - 3006 x^2 + 5481 x^3 - 23953 x^4 + 31960 x^5 - 38556 x^6 + 27749 x^7 - 12817 x^8 + 2438 x^9 + 840 x^{10})$$

**Simplify[Cf[6, 8, 10]]**

[化简]

$$1024 (1+x)^5 (-228 + 2280 x - 17657 x^2 + 55410 x^3 - 175923 x^4 + 316440 x^5 - 538591 x^6 + 605042 x^7 - 527289 x^8 + 312060 x^9 - 106312 x^{10} + 17792 x^{11} + 1104 x^{12})$$

**Simplify[Cf[6, 8, 11]]**

[化简]

$$2048 x (1+x)^5 (-384 + 9 x - 11414 x^2 + 26555 x^3 - 107046 x^4 + 159337 x^5 - 217282 x^6 + 182633 x^7 - 123402 x^8 + 75666 x^9 - 29528 x^{10} + 6264 x^{11})$$

**Simplify[Cf[6, 8, 12]]**

[化简]

$$1024 (1+x)^5 (-228 + 2280 x - 17657 x^2 + 55410 x^3 - 175923 x^4 + 316440 x^5 - 538591 x^6 + 605042 x^7 - 527289 x^8 + 312060 x^9 - 106312 x^{10} + 17792 x^{11} + 1104 x^{12})$$

**Simplify[Cf[6, 8, 13]]**

[化简]

$$2048 x (1+x)^5 (-108 - 12 x - 3006 x^2 + 5481 x^3 - 23953 x^4 + 31960 x^5 - 38556 x^6 + 27749 x^7 - 12817 x^8 + 2438 x^9 + 840 x^{10})$$

**Simplify[Cf[6, 8, 14]]**

[化简]

$$2048 x^2 (1+x)^5 (-85 - 26 x - 1639 x^2 + 3668 x^3 - 7407 x^4 + 7286 x^5 - 3481 x^6 - 208 x^7 + 548 x^8)$$

(\*, r2^6r3^9\*)

**Simplify[Cf[6, 9, 0]]**

[化简]

0

**Simplify[Cf[6, 9, 1]]**

[化简]

0

**Simplify[Cf[6, 9, 2]]**

[化简]

0

**Simplify[Cf[6, 9, 3]]**

[化简]

0

**Simplify[Cf[6, 9, 4]]**

[化简]

0

**Simplify[Cf[6, 9, 5]]**

[化简]

0

**Simplify[Cf[6, 9, 6]]**

[化简]

0

**Simplify[Cf[6, 9, 7]]**

[化简]

$$2048 x^2 (1+x)^5 (-49 - 363 x + 500 x^2 - 2542 x^3 + 3875 x^4 - 3919 x^5 + 2046 x^6 - 520 x^7 + 108 x^8)$$

**Simplify[Cf[6, 9, 8]]**

[化简]

$$2048 x (1+x)^5 (-108 - 12 x - 3006 x^2 + 5481 x^3 - 23953 x^4 + 31960 x^5 - 38556 x^6 + 27749 x^7 - 12817 x^8 + 2438 x^9 + 840 x^{10})$$

**Simplify[Cf[6, 9, 9]]**

[化简]

$$4096 x (1+x)^5 (-258 + 722 x - 6933 x^2 + 12092 x^3 - 38987 x^4 + 44434 x^5 - 55507 x^6 + 31712 x^7 - 7683 x^8 - 2296 x^9 + 2904 x^{10} + 216 x^{11})$$

**Simplify[Cf[6, 9, 10]]**

[化简]

$$2048 x (1+x)^5 (-648 + 1015 x - 19296 x^2 + 35793 x^3 - 134342 x^4 + 163415 x^5 - 221688 x^6 + 152143 x^7 - 93386 x^8 + 54714 x^9 - 17376 x^{10} + 6024 x^{11})$$

**Simplify[Cf[6, 9, 11]]**

[化简]

$$2048 x (1+x)^5 (-648 + 1015 x - 19296 x^2 + 35793 x^3 - 134342 x^4 + 163415 x^5 - 221688 x^6 + 152143 x^7 - 93386 x^8 + 54714 x^9 - 17376 x^{10} + 6024 x^{11})$$

**Simplify[Cf[6, 9, 12]]**

[化简]

$$4096 x (1+x)^5 (-258 + 722 x - 6933 x^2 + 12092 x^3 - 38987 x^4 + 44434 x^5 - 55507 x^6 + 31712 x^7 - 7683 x^8 - 2296 x^9 + 2904 x^{10} + 216 x^{11})$$

**Simplify[Cf[6, 9, 13]]**

[化简]

$$2048 x (1+x)^5 (-108 - 12 x - 3006 x^2 + 5481 x^3 - 23953 x^4 + 31960 x^5 - 38556 x^6 + 27749 x^7 - 12817 x^8 + 2438 x^9 + 840 x^{10})$$

**Simplify[Cf[6, 9, 14]]**

[化简]

$$2048 x^2 (1+x)^5 (-49 - 363 x + 500 x^2 - 2542 x^3 + 3875 x^4 - 3919 x^5 + 2046 x^6 - 520 x^7 + 108 x^8)$$

(\*, r2^6r3^10\*)

**Simplify[Cf[6, 10, 0]]**

[化简]

0

**Simplify[Cf[6, 10, 1]]**

[化简]

0

**Simplify[Cf[6, 10, 2]]**

[化简]

0

**Simplify[Cf[6, 10, 3]]**

[化简]

0

**Simplify[Cf[6, 10, 4]]**

[化简]

0

**Simplify[Cf[6, 10, 5]]**

[化简]

0

**Simplify[Cf[6, 10, 6]]**

|化简

$$-2048 x^2 (1+x)^5 (53 + 837 x^2 - 1888 x^3 + 3187 x^4 - 3528 x^5 + 2623 x^6 - 1528 x^7 + 436 x^8)$$

**Simplify[Cf[6, 10, 7]]**

|化简

$$2048 x (1+x)^5 (-102 + 188 x - 2949 x^2 + 5328 x^3 - 16599 x^4 + 19224 x^5 - 17363 x^6 + 8556 x^7 - 391 x^8 - 560 x^9 + 60 x^{10})$$

**Simplify[Cf[6, 10, 8]]**

|化简

$$1024 (1+x)^5 (-228 + 2280 x - 17657 x^2 + 55410 x^3 - 175923 x^4 + 316440 x^5 - 538591 x^6 + 605042 x^7 - 527289 x^8 + 312060 x^9 - 106312 x^{10} + 17792 x^{11} + 1104 x^{12})$$

**Simplify[Cf[6, 10, 9]]**

|化简

$$2048 x (1+x)^5 (-648 + 1015 x - 19296 x^2 + 35793 x^3 - 134342 x^4 + 163415 x^5 - 221688 x^6 + 152143 x^7 - 93386 x^8 + 54714 x^9 - 17376 x^{10} + 6024 x^{11})$$

**Simplify[Cf[6, 10, 10]]**

|化简

$$6144 (1+x)^5 (-78 + 780 x - 6133 x^2 + 18672 x^3 - 64249 x^4 + 119158 x^5 - 222889 x^6 + 256892 x^7 - 237145 x^8 + 136978 x^9 - 46442 x^{10} + 10496 x^{11} + 552 x^{12})$$

**Simplify[Cf[6, 10, 11]]**

|化简

$$2048 x (1+x)^5 (-648 + 1015 x - 19296 x^2 + 35793 x^3 - 134342 x^4 + 163415 x^5 - 221688 x^6 + 152143 x^7 - 93386 x^8 + 54714 x^9 - 17376 x^{10} + 6024 x^{11})$$

**Simplify[Cf[6, 10, 12]]**

|化简

$$1024 (1+x)^5 (-228 + 2280 x - 17657 x^2 + 55410 x^3 - 175923 x^4 + 316440 x^5 - 538591 x^6 + 605042 x^7 - 527289 x^8 + 312060 x^9 - 106312 x^{10} + 17792 x^{11} + 1104 x^{12})$$

**Simplify[Cf[6, 10, 13]]**

|化简

$$2048 x (1+x)^5 (-102 + 188 x - 2949 x^2 + 5328 x^3 - 16599 x^4 + 19224 x^5 - 17363 x^6 + 8556 x^7 - 391 x^8 - 560 x^9 + 60 x^{10})$$

**Simplify[Cf[6, 10, 14]]**

|化简

$$-2048 x^2 (1+x)^5 (53 + 837 x^2 - 1888 x^3 + 3187 x^4 - 3528 x^5 + 2623 x^6 - 1528 x^7 + 436 x^8)$$

**(\*, r2^6r3^11\*)****Simplify[Cf[6, 11, 0]]**

|化简

0

**Simplify[Cf[6, 11, 1]]**

[\[化简\]](#)

0

**Simplify[Cf[6, 11, 2]]**

[\[化简\]](#)

0

**Simplify[Cf[6, 11, 3]]**

[\[化简\]](#)

0

**Simplify[Cf[6, 11, 4]]**

[\[化简\]](#)

0

**Simplify[Cf[6, 11, 5]]**

[\[化简\]](#)

$$-2048 x^2 (1+x)^5 (15+129 x-276 x^2+570 x^3-597 x^4+37 x^5+198 x^6-96 x^7+20 x^8)$$

**Simplify[Cf[6, 11, 6]]**

[\[化简\]](#)

$$-4096 x (1+x)^5 (18+57 x+380 x^2-1128 x^3+5543 x^4-10971 x^5+14182 x^6-12722 x^7+6857 x^8-2276 x^9+444 x^{10})$$

**Simplify[Cf[6, 11, 7]]**

[\[化简\]](#)

$$-2048 x (1+x)^5 (282-791 x+7232 x^2-13452 x^3+36789 x^4-41995 x^5+42522 x^6-25450 x^7+3219 x^8+1336 x^9-236 x^{10}+48 x^{11})$$

**Simplify[Cf[6, 11, 8]]**

[\[化简\]](#)

$$2048 x (1+x)^5 (-384+9 x-11414 x^2+26555 x^3-107046 x^4+159337 x^5-217282 x^6+182633 x^7-123402 x^8+75666 x^9-29528 x^{10}+6264 x^{11})$$

**Simplify[Cf[6, 11, 9]]**

[\[化简\]](#)

$$2048 x (1+x)^5 (-648+1015 x-19296 x^2+35793 x^3-134342 x^4+163415 x^5-221688 x^6+152143 x^7-93386 x^8+54714 x^9-17376 x^{10}+6024 x^{11})$$

**Simplify[Cf[6, 11, 10]]**

[\[化简\]](#)

$$2048 x (1+x)^5 (-648+1015 x-19296 x^2+35793 x^3-134342 x^4+163415 x^5-221688 x^6+152143 x^7-93386 x^8+54714 x^9-17376 x^{10}+6024 x^{11})$$

**Simplify[Cf[6, 11, 11]]**

[\[化简\]](#)

$$2048 x (1+x)^5 (-384+9 x-11414 x^2+26555 x^3-107046 x^4+159337 x^5-217282 x^6+182633 x^7-123402 x^8+75666 x^9-29528 x^{10}+6264 x^{11})$$

**Simplify[Cf[6, 11, 12]]**

[化简]

$$-2048 x (1+x)^5 (282 - 791 x + 7232 x^2 - 13452 x^3 + 36789 x^4 - 41995 x^5 + 42522 x^6 - 25450 x^7 + 3219 x^8 + 1336 x^9 - 236 x^{10} + 48 x^{11})$$

**Simplify[Cf[6, 11, 13]]**

[化简]

$$-4096 x (1+x)^5 (18 + 57 x + 380 x^2 - 1128 x^3 + 5543 x^4 - 10971 x^5 + 14182 x^6 - 12722 x^7 + 6857 x^8 - 2276 x^9 + 444 x^{10})$$

**Simplify[Cf[6, 11, 14]]**

[化简]

$$-2048 x^2 (1+x)^5 (15 + 129 x - 276 x^2 + 570 x^3 - 597 x^4 + 37 x^5 + 198 x^6 - 96 x^7 + 20 x^8)$$

**(\*, r2^6r3^12\*)****Simplify[Cf[6, 12, 0]]**

[化简]

0

**Simplify[Cf[6, 12, 1]]**

[化简]

0

**Simplify[Cf[6, 12, 2]]**

[化简]

0

**Simplify[Cf[6, 12, 3]]**

[化简]

0

**Simplify[Cf[6, 12, 4]]**

[化简]

$$1024 (-1+x)^2 x^2 (1+x)^5 (-21 - 24 x - 78 x^2 - 328 x^3 + 551 x^4 - 424 x^5 + 148 x^6)$$

**Simplify[Cf[6, 12, 5]]**

[化简]

$$-2048 x (1+x)^5 (30 - 109 x + 767 x^2 - 1588 x^3 + 3006 x^4 - 3343 x^5 + 1303 x^6 - 22 x^7 - 30 x^8 - 26 x^9 + 12 x^{10})$$

**Simplify[Cf[6, 12, 6]]**

[化简]

$$-4096 (1+x)^5 (18 - 180 x + 1349 x^2 - 4492 x^3 + 12813 x^4 - 22478 x^5 + 32069 x^6 - 34832 x^7 + 28217 x^8 - 18466 x^9 + 8598 x^{10} - 2400 x^{11} + 360 x^{12})$$

**Simplify[Cf[6, 12, 7]]**

[化简]

$$-2048 x (1+x)^5 (282 - 791 x + 7232 x^2 - 13452 x^3 + 36789 x^4 - 41995 x^5 + 42522 x^6 - 25450 x^7 + 3219 x^8 + 1336 x^9 - 236 x^{10} + 48 x^{11})$$

**Simplify[Cf[6, 12, 8]]**

[化简]

$$1024 (1+x)^5 (-228 + 2280x - 17657x^2 + 55410x^3 - 175923x^4 + 316440x^5 - 538591x^6 + 605042x^7 - 527289x^8 + 312060x^9 - 106312x^{10} + 17792x^{11} + 1104x^{12})$$

**Simplify[Cf[6, 12, 9]]**

[化简]

$$4096x(1+x)^5 (-258 + 722x - 6933x^2 + 12092x^3 - 38987x^4 + 44434x^5 - 55507x^6 + 31712x^7 - 7683x^8 - 2296x^9 + 2904x^{10} + 216x^{11})$$

**Simplify[Cf[6, 12, 10]]**

[化简]

$$1024 (1+x)^5 (-228 + 2280x - 17657x^2 + 55410x^3 - 175923x^4 + 316440x^5 - 538591x^6 + 605042x^7 - 527289x^8 + 312060x^9 - 106312x^{10} + 17792x^{11} + 1104x^{12})$$

**Simplify[Cf[6, 12, 11]]**

[化简]

$$-2048x(1+x)^5 (282 - 791x + 7232x^2 - 13452x^3 + 36789x^4 - 41995x^5 + 42522x^6 - 25450x^7 + 3219x^8 + 1336x^9 - 236x^{10} + 48x^{11})$$

**Simplify[Cf[6, 12, 12]]**

[化简]

$$-4096(1+x)^5 (18 - 180x + 1349x^2 - 4492x^3 + 12813x^4 - 22478x^5 + 32069x^6 - 34832x^7 + 28217x^8 - 18466x^9 + 8598x^{10} - 2400x^{11} + 360x^{12})$$

**Simplify[Cf[6, 12, 13]]**

[化简]

$$-2048x(1+x)^5 (30 - 109x + 767x^2 - 1588x^3 + 3006x^4 - 3343x^5 + 1303x^6 - 22x^7 - 30x^8 - 26x^9 + 12x^{10})$$

**Simplify[Cf[6, 12, 14]]**

[化简]

$$1024(-1+x)^2x^2(1+x)^5(-21 - 24x - 78x^2 - 328x^3 + 551x^4 - 424x^5 + 148x^6)$$

**(\*, r2^6r3^13\*)****Simplify[Cf[6, 13, 0]]**

[化简]

0

**Simplify[Cf[6, 13, 1]]**

[化简]

0

**Simplify[Cf[6, 13, 2]]**

[化简]

0

**Simplify[Cf[6, 13, 3]]**

[化简]

$$-4096(-1+x)^3x^3(1+x)^5(-5 - 3x^2 + 4x^3)$$

**Simplify[Cf[6, 13, 4]]**

[化简]

$$2048 (-1+x)^2 x^2 (1+x)^5 (-35+16x-90x^2-364x^3+597x^4-460x^5+160x^6)$$

**Simplify[Cf[6, 13, 5]]**

[化简]

$$-2048x(1+x)^5 (30-109x+767x^2-1588x^3+3006x^4-3343x^5+1303x^6-22x^7-30x^8-26x^9+12x^{10})$$

**Simplify[Cf[6, 13, 6]]**

[化简]

$$-4096x(1+x)^5 (18+57x+380x^2-1128x^3+5543x^4-10971x^5+14182x^6-12722x^7+6857x^8-2276x^9+444x^{10})$$

**Simplify[Cf[6, 13, 7]]**

[化简]

$$2048x(1+x)^5 (-102+188x-2949x^2+5328x^3-16599x^4+19224x^5-17363x^6+8556x^7-391x^8-560x^9+60x^{10})$$

**Simplify[Cf[6, 13, 8]]**

[化简]

$$2048x(1+x)^5 (-108-12x-3006x^2+5481x^3-23953x^4+31960x^5-38556x^6+27749x^7-12817x^8+2438x^9+840x^{10})$$

**Simplify[Cf[6, 13, 9]]**

[化简]

$$2048x(1+x)^5 (-108-12x-3006x^2+5481x^3-23953x^4+31960x^5-38556x^6+27749x^7-12817x^8+2438x^9+840x^{10})$$

**Simplify[Cf[6, 13, 10]]**

[化简]

$$2048x(1+x)^5 (-102+188x-2949x^2+5328x^3-16599x^4+19224x^5-17363x^6+8556x^7-391x^8-560x^9+60x^{10})$$

**Simplify[Cf[6, 13, 11]]**

[化简]

$$-4096x(1+x)^5 (18+57x+380x^2-1128x^3+5543x^4-10971x^5+14182x^6-12722x^7+6857x^8-2276x^9+444x^{10})$$

**Simplify[Cf[6, 13, 12]]**

[化简]

$$-2048x(1+x)^5 (30-109x+767x^2-1588x^3+3006x^4-3343x^5+1303x^6-22x^7-30x^8-26x^9+12x^{10})$$

**Simplify[Cf[6, 13, 13]]**

[化简]

$$2048 (-1+x)^2 x^2 (1+x)^5 (-35+16x-90x^2-364x^3+597x^4-460x^5+160x^6)$$

**Simplify[Cf[6, 13, 14]]**

[化简]

$$-4096(-1+x)^3 x^3 (1+x)^5 (-5-3x^2+4x^3)$$



(\*, r2^6r3^14\*)

**Simplify[Cf[6, 14, 0]]**

[\[化简\]](#)

0

**Simplify[Cf[6, 14, 1]]**

[\[化简\]](#)

0

**Simplify[Cf[6, 14, 2]]**

[\[化简\]](#)

0

**Simplify[Cf[6, 14, 3]]**

[\[化简\]](#)

$-4096 (-1+x)^3 x^3 (1+x)^5 (-5-3x^2+4x^3)$

**Simplify[Cf[6, 14, 4]]**

[\[化简\]](#)

$1024 (-1+x)^2 x^2 (1+x)^5 (-21-24x-78x^2-328x^3+551x^4-424x^5+148x^6)$

**Simplify[Cf[6, 14, 5]]**

[\[化简\]](#)

$-2048 x^2 (1+x)^5 (15+129x-276x^2+570x^3-597x^4+37x^5+198x^6-96x^7+20x^8)$

**Simplify[Cf[6, 14, 6]]**

[\[化简\]](#)

$-2048 x^2 (1+x)^5 (53+837x^2-1888x^3+3187x^4-3528x^5+2623x^6-1528x^7+436x^8)$

**Simplify[Cf[6, 14, 7]]**

[\[化简\]](#)

$2048 x^2 (1+x)^5 (-49-363x+500x^2-2542x^3+3875x^4-3919x^5+2046x^6-520x^7+108x^8)$

**Simplify[Cf[6, 14, 8]]**

[\[化简\]](#)

$2048 x^2 (1+x)^5 (-85-26x-1639x^2+3668x^3-7407x^4+7286x^5-3481x^6-208x^7+548x^8)$

**Simplify[Cf[6, 14, 9]]**

[\[化简\]](#)

$2048 x^2 (1+x)^5 (-49-363x+500x^2-2542x^3+3875x^4-3919x^5+2046x^6-520x^7+108x^8)$

**Simplify[Cf[6, 14, 10]]**

[\[化简\]](#)

$-2048 x^2 (1+x)^5 (53+837x^2-1888x^3+3187x^4-3528x^5+2623x^6-1528x^7+436x^8)$

**Simplify[Cf[6, 14, 11]]**

[\[化简\]](#)

$-2048 x^2 (1+x)^5 (15+129x-276x^2+570x^3-597x^4+37x^5+198x^6-96x^7+20x^8)$

**Simplify[Cf[6, 14, 12]]**

[化简]

$$1024 (-1 + x)^2 x^2 (1 + x)^5 (-21 - 24 x - 78 x^2 - 328 x^3 + 551 x^4 - 424 x^5 + 148 x^6)$$

**Simplify[Cf[6, 14, 13]]**

[化简]

$$-4096 (-1 + x)^3 x^3 (1 + x)^5 (-5 - 3 x^2 + 4 x^3)$$

**Simplify[Cf[6, 14, 14]]**

[化简]

0

(\*, r2^7r3^0\*)

**Simplify[Cf[7, 0, 0]]**

[化简]

0

**Simplify[Cf[7, 0, 1]]**

[化简]

0

**Simplify[Cf[7, 0, 2]]**

[化简]

0

**Simplify[Cf[7, 0, 3]]**

[化简]

0

**Simplify[Cf[7, 0, 4]]**

[化简]

0

**Simplify[Cf[7, 0, 5]]**

[化简]

0

**Simplify[Cf[7, 0, 6]]**

[化简]

0

**Simplify[Cf[7, 0, 7]]**

[化简]

0

**Simplify[Cf[7, 0, 8]]**

[化简]

0

**Simplify[Cf[7, 0, 9]]**

[化简]

0

**Simplify[Cf[7, 0, 10]]**

[化简]

0

**Simplify[Cf[7, 0, 11]]**

[化简]

0

**Simplify[Cf[7, 0, 12]]**

[化简]

0

**Simplify[Cf[7, 0, 13]]**

[化简]

0

**Simplify[Cf[7, 0, 14]]**

[化简]

0

(\*, r2^7r3^1\*)

**Simplify[Cf[7, 1, 0]]**

[化简]

0

**Simplify[Cf[7, 1, 1]]**

[化简]

0

**Simplify[Cf[7, 1, 2]]**

[化简]

0

**Simplify[Cf[7, 1, 3]]**

[化简]

0

**Simplify[Cf[7, 1, 4]]**

[化简]

0

**Simplify[Cf[7, 1, 5]]**

[化简]

0

**Simplify[Cf[7, 1, 6]]**

[化简]

0

**Simplify[Cf[7, 1, 7]]**

[化简]

0

**Simplify[Cf[7, 1, 8]]**

[化简]

0

**Simplify[Cf[7, 1, 9]]**

[化简]

0

**Simplify[Cf[7, 1, 10]]**

[化简]

0

**Simplify[Cf[7, 1, 11]]**

[化简]

0

**Simplify[Cf[7, 1, 12]]**

[化简]

0

**Simplify[Cf[7, 1, 13]]**

[化简]

0

**Simplify[Cf[7, 1, 14]]**

[化简]

0

**(\*, r2^7r3^2\*)**

**Simplify[Cf[7, 2, 0]]**

[化简]

0

**Simplify[Cf[7, 2, 1]]**

[化简]

0

**Simplify[Cf[7, 2, 2]]**

[化简]

0

**Simplify[Cf[7, 2, 3]]**

[化简]

0

**Simplify[Cf[7, 2, 4]]**

[化简]

0

**Simplify[Cf[7, 2, 5]]**

[化简]

0

**Simplify[Cf[7, 2, 6]]**

[化简]

0

**Simplify[Cf[7, 2, 7]]**

[化简]

0

**Simplify[Cf[7, 2, 8]]**

[化简]

0

**Simplify[Cf[7, 2, 9]]**

[化简]

0

**Simplify[Cf[7, 2, 10]]**

[化简]

0

**Simplify[Cf[7, 2, 11]]**

[化简]

0

**Simplify[Cf[7, 2, 12]]**

[化简]

0

**Simplify[Cf[7, 2, 13]]**

[化简]

$-12288 (-1+x)^4 x^3 (1+x)^6$

**Simplify[Cf[7, 2, 14]]**

[化简]

$-12288 (-1+x)^4 x^3 (1+x)^6$

(\*, r2^7r3^3\*)

**Simplify[Cf[7, 3, 0]]**

[化简]

0

**Simplify[Cf[7, 3, 1]]**

[化简]

0

**Simplify[Cf[7, 3, 2]]**

[化简]

0

**Simplify[Cf[7, 3, 3]]**

[化简]

0

**Simplify[Cf[7, 3, 4]]**

[化简]

0

**Simplify[Cf[7, 3, 5]]**

[化简]

0

**Simplify[Cf[7, 3, 6]]**

[化简]

0

**Simplify[Cf[7, 3, 7]]**

[化简]

0

**Simplify[Cf[7, 3, 8]]**

[化简]

0

**Simplify[Cf[7, 3, 9]]**

[化简]

0

**Simplify[Cf[7, 3, 10]]**

[化简]

0

**Simplify[Cf[7, 3, 11]]**

[化简]

0

**Simplify[Cf[7, 3, 12]]**

[化简]

$-2048 (-1+x)^2 x^2 (1+x)^5 (9-14x+132x^2-190x^3+207x^4-180x^5+52x^6)$

**Simplify[Cf[7, 3, 13]]**

[化简]

$-4096 (-1+x)^2 x^2 (1+x)^5 (15-34x+152x^2-202x^3+221x^4-188x^5+52x^6)$

**Simplify[Cf[7, 3, 14]]**

[化简]

$-2048 (-1+x)^2 x^2 (1+x)^5 (9-14x+132x^2-190x^3+207x^4-180x^5+52x^6)$

(\*, r2^7r3^4\*)

**Simplify[Cf[7, 4, 0]]**

[化简]

0

**Simplify[Cf[7, 4, 1]]**

[化简]

0

**Simplify[Cf[7, 4, 2]]**

[化简]

0

**Simplify[Cf[7, 4, 3]]**

[化简]

0

**Simplify[Cf[7, 4, 4]]**

[化简]

0

**Simplify[Cf[7, 4, 5]]**

[化简]

0

**Simplify[Cf[7, 4, 6]]**

[化简]

0

**Simplify[Cf[7, 4, 7]]**

[化简]

0

**Simplify[Cf[7, 4, 8]]**

[化简]

0

**Simplify[Cf[7, 4, 9]]**

[化简]

0

**Simplify[Cf[7, 4, 10]]**

[化简]

0

**Simplify[Cf[7, 4, 11]]**

[化简]

$2048 x^2 (1 + x)^5 (-11 - 116 x + 337 x^2 - 822 x^3 + 1271 x^4 - 1020 x^5 + 567 x^6 - 250 x^7 + 44 x^8)$

**Simplify[Cf[7, 4, 12]]**

[化简]

$2048 x (1 + x)^5 (-22 + 61 x - 464 x^2 + 899 x^3 - 1766 x^4 + 2289 x^5 - 1036 x^6 - 11 x^7 + 172 x^8 - 166 x^9 + 44 x^{10})$

**Simplify[Cf[7, 4, 13]]**

[化简]

$$2048 x (1 + x)^5 (-22 + 61 x - 464 x^2 + 899 x^3 - 1766 x^4 + 2289 x^5 - 1036 x^6 - 11 x^7 + 172 x^8 - 166 x^9 + 44 x^{10})$$

**Simplify[Cf[7, 4, 14]]**

[化简]

$$2048 x^2 (1 + x)^5 (-11 - 116 x + 337 x^2 - 822 x^3 + 1271 x^4 - 1020 x^5 + 567 x^6 - 250 x^7 + 44 x^8)$$

(\*, r2^7r3^5\*)

**Simplify[Cf[7, 5, 0]]**

[化简]

0

**Simplify[Cf[7, 5, 1]]**

[化简]

0

**Simplify[Cf[7, 5, 2]]**

[化简]

0

**Simplify[Cf[7, 5, 3]]**

[化简]

0

**Simplify[Cf[7, 5, 4]]**

[化简]

0

**Simplify[Cf[7, 5, 5]]**

[化简]

0

**Simplify[Cf[7, 5, 6]]**

[化简]

0

**Simplify[Cf[7, 5, 7]]**

[化简]

0

**Simplify[Cf[7, 5, 8]]**

[化简]

0

**Simplify[Cf[7, 5, 9]]**

[化简]

0



**Simplify[Cf[7, 5, 10]]**

[化简]

$$-2048 x^2 (1+x)^5 (45+33 x+508 x^2-870 x^3+773 x^4+265 x^5-1450 x^6+1100 x^7-308 x^8)$$

**Simplify[Cf[7, 5, 11]]**

[化简]

$$4096 x^2 (1+x)^5 (-299+1352 x-5616 x^2+11877 x^3-18447 x^4+19478 x^5-12818 x^6+5737 x^7-1796 x^8+340 x^9)$$

**Simplify[Cf[7, 5, 12]]**

[化简]

$$4096 x (1+x)^5 (-80+393 x-2217 x^2+4730 x^3-9858 x^4+14329 x^5-18549 x^6+21468 x^7-16396 x^8+7712 x^9-2132 x^{10}+312 x^{11})$$

**Simplify[Cf[7, 5, 13]]**

[化简]

$$4096 x^2 (1+x)^5 (-299+1352 x-5616 x^2+11877 x^3-18447 x^4+19478 x^5-12818 x^6+5737 x^7-1796 x^8+340 x^9)$$

**Simplify[Cf[7, 5, 14]]**

[化简]

$$-2048 x^2 (1+x)^5 (45+33 x+508 x^2-870 x^3+773 x^4+265 x^5-1450 x^6+1100 x^7-308 x^8)$$

**(\*, r2^7r3^6\*)****Simplify[Cf[7, 6, 0]]**

[化简]

0

**Simplify[Cf[7, 6, 1]]**

[化简]

0

**Simplify[Cf[7, 6, 2]]**

[化简]

0

**Simplify[Cf[7, 6, 3]]**

[化简]

0

**Simplify[Cf[7, 6, 4]]**

[化简]

0

**Simplify[Cf[7, 6, 5]]**

[化简]

0

**Simplify[Cf[7, 6, 6]]**

[化简]

0

**Simplify[Cf[7, 6, 7]]**

[化简]

0

**Simplify[Cf[7, 6, 8]]**

[化简]

0

**Simplify[Cf[7, 6, 9]]**

[化简]

$$2048 x^2 (1+x)^5 (-49 - 363 x + 500 x^2 - 2542 x^3 + 3875 x^4 - 3919 x^5 + 2046 x^6 - 520 x^7 + 108 x^8)$$

**Simplify[Cf[7, 6, 10]]**

[化简]

$$2048 x (1+x)^5 (-102 + 188 x - 2949 x^2 + 5328 x^3 - 16599 x^4 + 19224 x^5 - 17363 x^6 + 8556 x^7 - 391 x^8 - 560 x^9 + 60 x^{10})$$

**Simplify[Cf[7, 6, 11]]**

[化简]

$$-2048 x (1+x)^5 (282 - 791 x + 7232 x^2 - 13452 x^3 + 36789 x^4 - 41995 x^5 + 42522 x^6 - 25450 x^7 + 3219 x^8 + 1336 x^9 - 236 x^{10} + 48 x^{11})$$

**Simplify[Cf[7, 6, 12]]**

[化简]

$$-2048 x (1+x)^5 (282 - 791 x + 7232 x^2 - 13452 x^3 + 36789 x^4 - 41995 x^5 + 42522 x^6 - 25450 x^7 + 3219 x^8 + 1336 x^9 - 236 x^{10} + 48 x^{11})$$

**Simplify[Cf[7, 6, 13]]**

[化简]

$$2048 x (1+x)^5 (-102 + 188 x - 2949 x^2 + 5328 x^3 - 16599 x^4 + 19224 x^5 - 17363 x^6 + 8556 x^7 - 391 x^8 - 560 x^9 + 60 x^{10})$$

**Simplify[Cf[7, 6, 14]]**

[化简]

$$2048 x^2 (1+x)^5 (-49 - 363 x + 500 x^2 - 2542 x^3 + 3875 x^4 - 3919 x^5 + 2046 x^6 - 520 x^7 + 108 x^8)$$

(\*, r2^7r3^7\*)

**Simplify[Cf[7, 7, 0]]**

[化简]

0

**Simplify[Cf[7, 7, 1]]**

[化简]

0

**Simplify[Cf[7, 7, 2]]**

[化简]

0

**Simplify[Cf[7, 7, 3]]**

[化简]

0

**Simplify[Cf[7, 7, 4]]**

[化简]

0

**Simplify[Cf[7, 7, 5]]**

[化简]

0

**Simplify[Cf[7, 7, 6]]**

[化简]

0

**Simplify[Cf[7, 7, 7]]**

[化简]

0

**Simplify[Cf[7, 7, 8]]**

[化简]

$$-4096 x^2 (1+x)^5 (37 + 159 x + 117 x^2 + 585 x^3 - 685 x^4 + 1145 x^5 - 489 x^6 - 17 x^7 + 204 x^8)$$

**Simplify[Cf[7, 7, 9]]**

[化简]

$$-8192 x^2 (1+x)^5 (442 - 1939 x + 8752 x^2 - 17217 x^3 + 28770 x^4 - 28765 x^5 + 20384 x^6 - 8115 x^7 + 1364 x^8 + 164 x^9)$$

**Simplify[Cf[7, 7, 10]]**

[化简]

$$-2048 x (1+x)^5 (588 - 2271 x + 16628 x^2 - 28673 x^3 + 79818 x^4 - 101037 x^5 + 162376 x^6 - 160663 x^7 + 117606 x^8 - 52908 x^9 + 10632 x^{10} + 528 x^{11})$$

**Simplify[Cf[7, 7, 11]]**

[化简]

$$-4096 x^2 (1+x)^5 (3201 - 14506 x + 64639 x^2 - 131240 x^3 + 223947 x^4 - 230882 x^5 + 190569 x^6 - 112108 x^7 + 48140 x^8 - 15744 x^9 + 3360 x^{10})$$

**Simplify[Cf[7, 7, 12]]**

[化简]

$$-2048 x (1+x)^5 (588 - 2271 x + 16628 x^2 - 28673 x^3 + 79818 x^4 - 101037 x^5 + 162376 x^6 - 160663 x^7 + 117606 x^8 - 52908 x^9 + 10632 x^{10} + 528 x^{11})$$

**Simplify[Cf[7, 7, 13]]**

[化简]

$$-8192 x^2 (1+x)^5 (442 - 1939 x + 8752 x^2 - 17217 x^3 + 28770 x^4 - 28765 x^5 + 20384 x^6 - 8115 x^7 + 1364 x^8 + 164 x^9)$$

**Simplify[Cf[7, 7, 14]]**

[\[化简\]](#)

$$-4096 x^2 (1+x)^5 (37+159 x+117 x^2+585 x^3-685 x^4+1145 x^5-489 x^6-17 x^7+204 x^8)$$

(\*, r2^7r3^8\*)

**Simplify[Cf[7, 8, 0]]**

[\[化简\]](#)

0

**Simplify[Cf[7, 8, 1]]**

[\[化简\]](#)

0

**Simplify[Cf[7, 8, 2]]**

[\[化简\]](#)

0

**Simplify[Cf[7, 8, 3]]**

[\[化简\]](#)

0

**Simplify[Cf[7, 8, 4]]**

[\[化简\]](#)

0

**Simplify[Cf[7, 8, 5]]**

[\[化简\]](#)

0

**Simplify[Cf[7, 8, 6]]**

[\[化简\]](#)

0

**Simplify[Cf[7, 8, 7]]**

[\[化简\]](#)

$$-4096 x^2 (1+x)^5 (37+159 x+117 x^2+585 x^3-685 x^4+1145 x^5-489 x^6-17 x^7+204 x^8)$$

**Simplify[Cf[7, 8, 8]]**

[\[化简\]](#)

$$-4096 x (1+x)^5 (80-127 x+2587 x^2-4727 x^3+17005 x^4-19163 x^5+23373 x^6-13825 x^7+6171 x^8-366 x^9+128 x^{10})$$

**Simplify[Cf[7, 8, 9]]**

[\[化简\]](#)

$$-2048 x (1+x)^5 (688-2146 x+18920 x^2-30213 x^3+98031 x^4-105466 x^5+166870 x^6-122025 x^7+79547 x^8-24214 x^9+4344 x^{10}+48 x^{11})$$

**Simplify[Cf[7, 8, 10]]**

[\[化简\]](#)

$$-2048 x (1+x)^5 (888-1940 x+27259 x^2-45307 x^3+164672 x^4-170926 x^5+259107 x^6-149199 x^7+94290 x^8-21764 x^9-3096 x^{10}+2592 x^{11})$$

**Simplify[Cf[7, 8, 11]]**

[化简]

$$-2048 x (1+x)^5 (888 - 1940 x + 27259 x^2 - 45307 x^3 + 164672 x^4 - 170926 x^5 + 259107 x^6 - 149199 x^7 + 94290 x^8 - 21764 x^9 - 3096 x^{10} + 2592 x^{11})$$

**Simplify[Cf[7, 8, 12]]**

[化简]

$$-2048 x (1+x)^5 (688 - 2146 x + 18920 x^2 - 30213 x^3 + 98031 x^4 - 105466 x^5 + 166870 x^6 - 122025 x^7 + 79547 x^8 - 24214 x^9 + 4344 x^{10} + 48 x^{11})$$

**Simplify[Cf[7, 8, 13]]**

[化简]

$$-4096 x (1+x)^5 (80 - 127 x + 2587 x^2 - 4727 x^3 + 17005 x^4 - 19163 x^5 + 23373 x^6 - 13825 x^7 + 6171 x^8 - 366 x^9 + 128 x^{10})$$

**Simplify[Cf[7, 8, 14]]**

[化简]

$$-4096 x^2 (1+x)^5 (37 + 159 x + 117 x^2 + 585 x^3 - 685 x^4 + 1145 x^5 - 489 x^6 - 17 x^7 + 204 x^8)$$

**Simplify[Cf[7, 8, 15]]**

[化简]

0

(\*, r2^7r3^9\*)

**Simplify[Cf[7, 9, 0]]**

[化简]

0

**Simplify[Cf[7, 9, 1]]**

[化简]

0

**Simplify[Cf[7, 9, 2]]**

[化简]

0

**Simplify[Cf[7, 9, 3]]**

[化简]

0

**Simplify[Cf[7, 9, 4]]**

[化简]

0

**Simplify[Cf[7, 9, 5]]**

[化简]

0

**Simplify[Cf[7, 9, 6]]**

[化简]

$$2048 x^2 (1+x)^5 (-49 - 363 x + 500 x^2 - 2542 x^3 + 3875 x^4 - 3919 x^5 + 2046 x^6 - 520 x^7 + 108 x^8)$$

**Simplify[Cf[7, 9, 7]]**

[化简]

$$-8192 x^2 (1+x)^5 (442 - 1939 x + 8752 x^2 - 17217 x^3 + 28770 x^4 - 28765 x^5 + 20384 x^6 - 8115 x^7 + 1364 x^8 + 164 x^9)$$

**Simplify[Cf[7, 9, 8]]**

[化简]

$$-2048 x (1+x)^5 (688 - 2146 x + 18920 x^2 - 30213 x^3 + 98031 x^4 - 105466 x^5 + 166870 x^6 - 122025 x^7 + 79547 x^8 - 24214 x^9 + 4344 x^{10} + 48 x^{11})$$

**Simplify[Cf[7, 9, 9]]**

[化简]

$$-8192 x^2 (1+x)^5 (2970 - 13299 x + 61532 x^2 - 120459 x^3 + 216260 x^4 - 218797 x^5 + 199684 x^6 - 115401 x^7 + 54586 x^8 - 15068 x^9 + 1464 x^{10})$$

**Simplify[Cf[7, 9, 10]]**

[化简]

$$4096 x (1+x)^5 (-702 + 2041 x - 21456 x^2 + 32433 x^3 - 121166 x^4 + 130121 x^5 - 240420 x^6 + 179135 x^7 - 144600 x^8 + 47206 x^9 - 8872 x^{10} + 2280 x^{11})$$

**Simplify[Cf[7, 9, 11]]**

[化简]

$$-8192 x^2 (1+x)^5 (2970 - 13299 x + 61532 x^2 - 120459 x^3 + 216260 x^4 - 218797 x^5 + 199684 x^6 - 115401 x^7 + 54586 x^8 - 15068 x^9 + 1464 x^{10})$$

**Simplify[Cf[7, 9, 12]]**

[化简]

$$-2048 x (1+x)^5 (688 - 2146 x + 18920 x^2 - 30213 x^3 + 98031 x^4 - 105466 x^5 + 166870 x^6 - 122025 x^7 + 79547 x^8 - 24214 x^9 + 4344 x^{10} + 48 x^{11})$$

**Simplify[Cf[7, 9, 13]]**

[化简]

$$-8192 x^2 (1+x)^5 (442 - 1939 x + 8752 x^2 - 17217 x^3 + 28770 x^4 - 28765 x^5 + 20384 x^6 - 8115 x^7 + 1364 x^8 + 164 x^9)$$

**Simplify[Cf[7, 9, 14]]**

[化简]

$$2048 x^2 (1+x)^5 (-49 - 363 x + 500 x^2 - 2542 x^3 + 3875 x^4 - 3919 x^5 + 2046 x^6 - 520 x^7 + 108 x^8)$$

**(\*, r2^7r3^10\*)****Simplify[Cf[7, 10, 0]]**

[化简]

0

**Simplify[Cf[7, 10, 1]]**

[化简]

0

**Simplify[Cf[7, 10, 2]]**

[化简]

0

**Simplify[Cf[7, 10, 3]]**

[化简]

0

**Simplify[Cf[7, 10, 4]]**

[化简]

0

**Simplify[Cf[7, 10, 5]]**

[化简]

$$-2048 x^2 (1+x)^5 (45 + 33 x + 508 x^2 - 870 x^3 + 773 x^4 + 265 x^5 - 1450 x^6 + 1100 x^7 - 308 x^8)$$

**Simplify[Cf[7, 10, 6]]**

[化简]

$$2048 x (1+x)^5 (-102 + 188 x - 2949 x^2 + 5328 x^3 - 16599 x^4 + 19224 x^5 - 17363 x^6 + 8556 x^7 - 391 x^8 - 560 x^9 + 60 x^{10})$$

**Simplify[Cf[7, 10, 7]]**

[化简]

$$-2048 x (1+x)^5 (588 - 2271 x + 16628 x^2 - 28673 x^3 + 79818 x^4 - 101037 x^5 + 162376 x^6 - 160663 x^7 + 117606 x^8 - 52908 x^9 + 10632 x^{10} + 528 x^{11})$$

**Simplify[Cf[7, 10, 8]]**

[化简]

$$-2048 x (1+x)^5 (888 - 1940 x + 27259 x^2 - 45307 x^3 + 164672 x^4 - 170926 x^5 + 259107 x^6 - 149199 x^7 + 94290 x^8 - 21764 x^9 - 3096 x^{10} + 2592 x^{11})$$

**Simplify[Cf[7, 10, 9]]**

[化简]

$$4096 x (1+x)^5 (-702 + 2041 x - 21456 x^2 + 32433 x^3 - 121166 x^4 + 130121 x^5 - 240420 x^6 + 179135 x^7 - 144600 x^8 + 47206 x^9 - 8872 x^{10} + 2280 x^{11})$$

**Simplify[Cf[7, 10, 10]]**

[化简]

$$4096 x (1+x)^5 (-702 + 2041 x - 21456 x^2 + 32433 x^3 - 121166 x^4 + 130121 x^5 - 240420 x^6 + 179135 x^7 - 144600 x^8 + 47206 x^9 - 8872 x^{10} + 2280 x^{11})$$

**Simplify[Cf[7, 10, 11]]**

[化简]

$$-2048 x (1+x)^5 (888 - 1940 x + 27259 x^2 - 45307 x^3 + 164672 x^4 - 170926 x^5 + 259107 x^6 - 149199 x^7 + 94290 x^8 - 21764 x^9 - 3096 x^{10} + 2592 x^{11})$$

**Simplify[Cf[7, 10, 12]]**

[化简]

$$-2048 x (1+x)^5 (588 - 2271 x + 16628 x^2 - 28673 x^3 + 79818 x^4 - 101037 x^5 + 162376 x^6 - 160663 x^7 + 117606 x^8 - 52908 x^9 + 10632 x^{10} + 528 x^{11})$$

**Simplify[Cf[7, 10, 13]]**

[化简]

$$2048 x (1+x)^5 (-102 + 188 x - 2949 x^2 + 5328 x^3 - 16599 x^4 + 19224 x^5 - 17363 x^6 + 8556 x^7 - 391 x^8 - 560 x^9 + 60 x^{10})$$

**Simplify[Cf[7, 10, 14]]**

[化简]

$$-2048 x^2 (1+x)^5 (45 + 33 x + 508 x^2 - 870 x^3 + 773 x^4 + 265 x^5 - 1450 x^6 + 1100 x^7 - 308 x^8)$$

(\*, r2^7r3^11\*)

**Simplify[Cf[7, 11, 0]]**

[化简]

0

**Simplify[Cf[7, 11, 1]]**

[化简]

0

**Simplify[Cf[7, 11, 2]]**

[化简]

0

**Simplify[Cf[7, 11, 3]]**

[化简]

0

**Simplify[Cf[7, 11, 4]]**

[化简]

$$2048 x^2 (1+x)^5 (-11 - 116 x + 337 x^2 - 822 x^3 + 1271 x^4 - 1020 x^5 + 567 x^6 - 250 x^7 + 44 x^8)$$

**Simplify[Cf[7, 11, 5]]**

[化简]

$$4096 x^2 (1+x)^5 (-299 + 1352 x - 5616 x^2 + 11877 x^3 - 18447 x^4 + 19478 x^5 - 12818 x^6 + 5737 x^7 - 1796 x^8 + 340 x^9)$$

**Simplify[Cf[7, 11, 6]]**

[化简]

$$-2048 x (1+x)^5 (282 - 791 x + 7232 x^2 - 13452 x^3 + 36789 x^4 - 41995 x^5 + 42522 x^6 - 25450 x^7 + 3219 x^8 + 1336 x^9 - 236 x^{10} + 48 x^{11})$$

**Simplify[Cf[7, 11, 7]]**

[化简]

$$-4096 x^2 (1+x)^5 (3201 - 14506 x + 64639 x^2 - 131240 x^3 + 223947 x^4 - 230882 x^5 + 190569 x^6 - 112108 x^7 + 48140 x^8 - 15744 x^9 + 3360 x^{10})$$

**Simplify[Cf[7, 11, 8]]**

[化简]

$$-2048 x (1+x)^5 (888 - 1940 x + 27259 x^2 - 45307 x^3 + 164672 x^4 - 170926 x^5 + 259107 x^6 - 149199 x^7 + 94290 x^8 - 21764 x^9 - 3096 x^{10} + 2592 x^{11})$$

**Simplify[Cf[7, 11, 9]]**

[化简]

$$-8192 x^2 (1+x)^5 (2970 - 13299 x + 61532 x^2 - 120459 x^3 + 216260 x^4 - 218797 x^5 + 199684 x^6 - 115401 x^7 + 54586 x^8 - 15068 x^9 + 1464 x^{10})$$



**Simplify[Cf[7, 11, 10]]**

[化简]

$$-2048 x (1+x)^5 (888 - 1940 x + 27259 x^2 - 45307 x^3 + 164672 x^4 - 170926 x^5 + 259107 x^6 - 149199 x^7 + 94290 x^8 - 21764 x^9 - 3096 x^{10} + 2592 x^{11})$$

**Simplify[Cf[7, 11, 11]]**

[化简]

$$-4096 x^2 (1+x)^5 (3201 - 14506 x + 64639 x^2 - 131240 x^3 + 223947 x^4 - 230882 x^5 + 190569 x^6 - 112108 x^7 + 48140 x^8 - 15744 x^9 + 3360 x^{10})$$

**Simplify[Cf[7, 11, 12]]**

[化简]

$$-2048 x (1+x)^5 (282 - 791 x + 7232 x^2 - 13452 x^3 + 36789 x^4 - 41995 x^5 + 42522 x^6 - 25450 x^7 + 3219 x^8 + 1336 x^9 - 236 x^{10} + 48 x^{11})$$

**Simplify[Cf[7, 11, 13]]**

[化简]

$$4096 x^2 (1+x)^5 (-299 + 1352 x - 5616 x^2 + 11877 x^3 - 18447 x^4 + 19478 x^5 - 12818 x^6 + 5737 x^7 - 1796 x^8 + 340 x^9)$$

**Simplify[Cf[7, 11, 14]]**

[化简]

$$2048 x^2 (1+x)^5 (-11 - 116 x + 337 x^2 - 822 x^3 + 1271 x^4 - 1020 x^5 + 567 x^6 - 250 x^7 + 44 x^8)$$

**(\*, r2^7r3^12\*)****Simplify[Cf[7, 12, 0]]**

[化简]

0

**Simplify[Cf[7, 12, 1]]**

[化简]

0

**Simplify[Cf[7, 12, 2]]**

[化简]

0

**Simplify[Cf[7, 12, 3]]**

[化简]

$$-2048 (-1+x)^2 x^2 (1+x)^5 (9 - 14 x + 132 x^2 - 190 x^3 + 207 x^4 - 180 x^5 + 52 x^6)$$

**Simplify[Cf[7, 12, 4]]**

[化简]

$$2048 x (1+x)^5 (-22 + 61 x - 464 x^2 + 899 x^3 - 1766 x^4 + 2289 x^5 - 1036 x^6 - 11 x^7 + 172 x^8 - 166 x^9 + 44 x^{10})$$

**Simplify[Cf[7, 12, 5]]**

[化简]

$$4096 x (1+x)^5 (-80 + 393 x - 2217 x^2 + 4730 x^3 - 9858 x^4 + 14329 x^5 - 18549 x^6 + 21468 x^7 - 16396 x^8 + 7712 x^9 - 2132 x^{10} + 312 x^{11})$$

**Simplify[Cf[7, 12, 6]]**

[化简]

$$-2048 x (1+x)^5 (282 - 791 x + 7232 x^2 - 13452 x^3 + 36789 x^4 - 41995 x^5 + 42522 x^6 - 25450 x^7 + 3219 x^8 + 1336 x^9 - 236 x^{10} + 48 x^{11})$$

**Simplify[Cf[7, 12, 7]]**

[化简]

$$-2048 x (1+x)^5 (588 - 2271 x + 16628 x^2 - 28673 x^3 + 79818 x^4 - 101037 x^5 + 162376 x^6 - 160663 x^7 + 117606 x^8 - 52908 x^9 + 10632 x^{10} + 528 x^{11})$$

**Simplify[Cf[7, 12, 8]]**

[化简]

$$-2048 x (1+x)^5 (688 - 2146 x + 18920 x^2 - 30213 x^3 + 98031 x^4 - 105466 x^5 + 166870 x^6 - 122025 x^7 + 79547 x^8 - 24214 x^9 + 4344 x^{10} + 48 x^{11})$$

**Simplify[Cf[7, 12, 9]]**

[化简]

$$-2048 x (1+x)^5 (688 - 2146 x + 18920 x^2 - 30213 x^3 + 98031 x^4 - 105466 x^5 + 166870 x^6 - 122025 x^7 + 79547 x^8 - 24214 x^9 + 4344 x^{10} + 48 x^{11})$$

**Simplify[Cf[7, 12, 10]]**

[化简]

$$-2048 x (1+x)^5 (588 - 2271 x + 16628 x^2 - 28673 x^3 + 79818 x^4 - 101037 x^5 + 162376 x^6 - 160663 x^7 + 117606 x^8 - 52908 x^9 + 10632 x^{10} + 528 x^{11})$$

**Simplify[Cf[7, 12, 11]]**

[化简]

$$-2048 x (1+x)^5 (282 - 791 x + 7232 x^2 - 13452 x^3 + 36789 x^4 - 41995 x^5 + 42522 x^6 - 25450 x^7 + 3219 x^8 + 1336 x^9 - 236 x^{10} + 48 x^{11})$$

**Simplify[Cf[7, 12, 12]]**

[化简]

$$4096 x (1+x)^5 (-80 + 393 x - 2217 x^2 + 4730 x^3 - 9858 x^4 + 14329 x^5 - 18549 x^6 + 21468 x^7 - 16396 x^8 + 7712 x^9 - 2132 x^{10} + 312 x^{11})$$

**Simplify[Cf[7, 12, 13]]**

[化简]

$$2048 x (1+x)^5 (-22 + 61 x - 464 x^2 + 899 x^3 - 1766 x^4 + 2289 x^5 - 1036 x^6 - 11 x^7 + 172 x^8 - 166 x^9 + 44 x^{10})$$

**Simplify[Cf[7, 12, 14]]**

[化简]

$$-2048 (-1+x)^2 x^2 (1+x)^5 (9 - 14 x + 132 x^2 - 190 x^3 + 207 x^4 - 180 x^5 + 52 x^6)$$

**(\*, r2^7r3^13\*)****Simplify[Cf[7, 13, 0]]**

[化简]

0

**Simplify[Cf[7, 13, 1]]**

[化简]

0

**Simplify[Cf[7, 13, 2]]**

[化简]

$$-12\,288 (-1+x)^4 x^3 (1+x)^6$$

**Simplify[Cf[7, 13, 3]]**

[化简]

$$-4096 (-1+x)^2 x^2 (1+x)^5 (15-34x+152x^2-202x^3+221x^4-188x^5+52x^6)$$

**Simplify[Cf[7, 13, 4]]**

[化简]

$$2048 x (1+x)^5 (-22+61x-464x^2+899x^3-1766x^4+2289x^5-1036x^6-11x^7+172x^8-166x^9+44x^{10})$$

**Simplify[Cf[7, 13, 5]]**

[化简]

$$4096 x^2 (1+x)^5 (-299+1352x-5616x^2+11877x^3-18447x^4+19478x^5-12818x^6+5737x^7-1796x^8+340x^9)$$

**Simplify[Cf[7, 13, 6]]**

[化简]

$$2048 x (1+x)^5 (-102+188x-2949x^2+5328x^3-16599x^4+19224x^5-17363x^6+8556x^7-391x^8-560x^9+60x^{10})$$

**Simplify[Cf[7, 13, 7]]**

[化简]

$$-8192 x^2 (1+x)^5 (442-1939x+8752x^2-17217x^3+28770x^4-28765x^5+20384x^6-8115x^7+1364x^8+164x^9)$$

**Simplify[Cf[7, 13, 8]]**

[化简]

$$-4096 x (1+x)^5 (80-127x+2587x^2-4727x^3+17005x^4-19163x^5+23373x^6-13825x^7+6171x^8-366x^9+128x^{10})$$

**Simplify[Cf[7, 13, 9]]**

[化简]

$$-8192 x^2 (1+x)^5 (442-1939x+8752x^2-17217x^3+28770x^4-28765x^5+20384x^6-8115x^7+1364x^8+164x^9)$$

**Simplify[Cf[7, 13, 10]]**

[化简]

$$2048 x (1+x)^5 (-102+188x-2949x^2+5328x^3-16599x^4+19224x^5-17363x^6+8556x^7-391x^8-560x^9+60x^{10})$$

**Simplify[Cf[7, 13, 11]]**

[化简]

$$4096 x^2 (1+x)^5 (-299+1352x-5616x^2+11877x^3-18447x^4+19478x^5-12818x^6+5737x^7-1796x^8+340x^9)$$

**Simplify[Cf[7, 13, 12]]**

[化简]

$$2048 x (1+x)^5 (-22 + 61 x - 464 x^2 + 899 x^3 - 1766 x^4 + 2289 x^5 - 1036 x^6 - 11 x^7 + 172 x^8 - 166 x^9 + 44 x^{10})$$

**Simplify[Cf[7, 13, 13]]**

[化简]

$$-4096 (-1+x)^2 x^2 (1+x)^5 (15 - 34 x + 152 x^2 - 202 x^3 + 221 x^4 - 188 x^5 + 52 x^6)$$

**Simplify[Cf[7, 13, 14]]**

[化简]

$$-12288 (-1+x)^4 x^3 (1+x)^6$$

**(\*, r2^7r3^14\*)****Simplify[Cf[7, 14, 0]]**

[化简]

0

**Simplify[Cf[7, 14, 1]]**

[化简]

0

**Simplify[Cf[7, 14, 2]]**

[化简]

$$-12288 (-1+x)^4 x^3 (1+x)^6$$

**Simplify[Cf[7, 14, 3]]**

[化简]

$$-2048 (-1+x)^2 x^2 (1+x)^5 (9 - 14 x + 132 x^2 - 190 x^3 + 207 x^4 - 180 x^5 + 52 x^6)$$

**Simplify[Cf[7, 14, 4]]**

[化简]

$$2048 x^2 (1+x)^5 (-11 - 116 x + 337 x^2 - 822 x^3 + 1271 x^4 - 1020 x^5 + 567 x^6 - 250 x^7 + 44 x^8)$$

**Simplify[Cf[7, 14, 5]]**

[化简]

$$-2048 x^2 (1+x)^5 (45 + 33 x + 508 x^2 - 870 x^3 + 773 x^4 + 265 x^5 - 1450 x^6 + 1100 x^7 - 308 x^8)$$

**Simplify[Cf[7, 14, 6]]**

[化简]

$$2048 x^2 (1+x)^5 (-49 - 363 x + 500 x^2 - 2542 x^3 + 3875 x^4 - 3919 x^5 + 2046 x^6 - 520 x^7 + 108 x^8)$$

**Simplify[Cf[7, 14, 7]]**

[化简]

$$-4096 x^2 (1+x)^5 (37 + 159 x + 117 x^2 + 585 x^3 - 685 x^4 + 1145 x^5 - 489 x^6 - 17 x^7 + 204 x^8)$$

**Simplify[Cf[7, 14, 8]]**

[化简]

$$-4096 x^2 (1+x)^5 (37 + 159 x + 117 x^2 + 585 x^3 - 685 x^4 + 1145 x^5 - 489 x^6 - 17 x^7 + 204 x^8)$$

**Simplify[Cf[7, 14, 9]]**

[化简]

$$2048 x^2 (1+x)^5 (-49 - 363 x + 500 x^2 - 2542 x^3 + 3875 x^4 - 3919 x^5 + 2046 x^6 - 520 x^7 + 108 x^8)$$

**Simplify[Cf[7, 14, 10]]**

[化简]

$$-2048 x^2 (1+x)^5 (45 + 33 x + 508 x^2 - 870 x^3 + 773 x^4 + 265 x^5 - 1450 x^6 + 1100 x^7 - 308 x^8)$$

**Simplify[Cf[7, 14, 11]]**

[化简]

$$2048 x^2 (1+x)^5 (-11 - 116 x + 337 x^2 - 822 x^3 + 1271 x^4 - 1020 x^5 + 567 x^6 - 250 x^7 + 44 x^8)$$

**Simplify[Cf[7, 14, 12]]**

[化简]

$$-2048 (-1+x)^2 x^2 (1+x)^5 (9 - 14 x + 132 x^2 - 190 x^3 + 207 x^4 - 180 x^5 + 52 x^6)$$

**Simplify[Cf[7, 14, 13]]**

[化简]

$$-12288 (-1+x)^4 x^3 (1+x)^6$$

**Simplify[Cf[7, 14, 14]]**

[化简]

0

(\*, r2^8r3^0\*)

**Simplify[Cf[8, 0, 0]]**

[化简]

0

**Simplify[Cf[8, 0, 1]]**

[化简]

0

**Simplify[Cf[8, 0, 2]]**

[化简]

0

**Simplify[Cf[8, 0, 3]]**

[化简]

0

**Simplify[Cf[8, 0, 4]]**

[化简]

0

**Simplify[Cf[8, 0, 5]]**

[化简]

0

**Simplify[Cf[8, 0, 6]]**

[化简]

0

**Simplify[Cf[8, 0, 7]]**

[化简]

0

**Simplify[Cf[8, 0, 8]]**

[化简]

0

**Simplify[Cf[8, 0, 9]]**

[化简]

0

**Simplify[Cf[8, 0, 10]]**

[化简]

0

**Simplify[Cf[8, 0, 11]]**

[化简]

0

**Simplify[Cf[8, 0, 12]]**

[化简]

0

**Simplify[Cf[8, 0, 13]]**

[化简]

0

**Simplify[Cf[8, 0, 14]]**

[化简]

0

(\*, r2^8r3^1\*)

**Simplify[Cf[8, 1, 0]]**

[化简]

0

**Simplify[Cf[8, 1, 1]]**

[化简]

0

**Simplify[Cf[8, 1, 2]]**

[化简]

0

**Simplify[Cf[8, 1, 3]]**

[化简]

0

**Simplify[Cf[8, 1, 4]]**

[化简]

0

**Simplify[Cf[8, 1, 5]]**

[化简]

0

**Simplify[Cf[8, 1, 6]]**

[化简]

0

**Simplify[Cf[8, 1, 7]]**

[化简]

0

**Simplify[Cf[8, 1, 8]]**

[化简]

0

**Simplify[Cf[8, 1, 9]]**

[化简]

0

**Simplify[Cf[8, 1, 10]]**

[化简]

0

**Simplify[Cf[8, 1, 11]]**

[化简]

0

**Simplify[Cf[8, 1, 12]]**

[化简]

0

**Simplify[Cf[8, 1, 13]]**

[化简]

$6144 (-1 + x)^5 x^3 (1 + x)^6$

**Simplify[Cf[8, 1, 14]]**

[化简]

$6144 (-1 + x)^5 x^3 (1 + x)^6$

(\*, r2^8r3^2\*)

**Simplify[Cf[8, 2, 0]]**

[化简]

0

**Simplify[Cf[8, 2, 1]]**

[化简]

0

**Simplify[Cf[8, 2, 2]]**

[化简]

0

**Simplify[Cf[8, 2, 3]]**

[化简]

0

**Simplify[Cf[8, 2, 4]]**

[化简]

0

**Simplify[Cf[8, 2, 5]]**

[化简]

0

**Simplify[Cf[8, 2, 6]]**

[化简]

0

**Simplify[Cf[8, 2, 7]]**

[化简]

0

**Simplify[Cf[8, 2, 8]]**

[化简]

0

**Simplify[Cf[8, 2, 9]]**

[化简]

0

**Simplify[Cf[8, 2, 10]]**

[化简]

0

**Simplify[Cf[8, 2, 11]]**

[化简]

0

**Simplify[Cf[8, 2, 12]]**

[化简]

$1024 (-1 + x)^3 x^2 (1 + x)^5 (7 + 19 x + 13 x^2 + 137 x^3 - 172 x^4 + 44 x^5)$

**Simplify[Cf[8, 2, 13]]**

[化简]

$2048 (-1 + x)^3 x^2 (1 + x)^5 (15 - x + 23 x^2 + 135 x^3 - 158 x^4 + 34 x^5)$

**Simplify[Cf[8, 2, 14]]**

[化简]

$1024 (-1 + x)^3 x^2 (1 + x)^5 (7 + 19 x + 13 x^2 + 137 x^3 - 172 x^4 + 44 x^5)$

(\*, r2^8r3^3\*)



**Simplify[Cf[8, 3, 0]]**

[化简]

0

**Simplify[Cf[8, 3, 1]]**

[化简]

0

**Simplify[Cf[8, 3, 2]]**

[化简]

0

**Simplify[Cf[8, 3, 3]]**

[化简]

0

**Simplify[Cf[8, 3, 4]]**

[化简]

0

**Simplify[Cf[8, 3, 5]]**

[化简]

0

**Simplify[Cf[8, 3, 6]]**

[化简]

0

**Simplify[Cf[8, 3, 7]]**

[化简]

0

**Simplify[Cf[8, 3, 8]]**

[化简]

0

**Simplify[Cf[8, 3, 9]]**

[化简]

0

**Simplify[Cf[8, 3, 10]]**

[化简]

0

**Simplify[Cf[8, 3, 11]]**

[化简]

$-2048 (-1+x)^2 x^2 (1+x)^5 (9+60x+34x^2+56x^3+177x^4-188x^5+28x^6)$

**Simplify[Cf[8, 3, 12]]**

[化简]

$-2048 (-1+x)^2 x (1+x)^5 (18-53x+419x^2-464x^3+1070x^4-399x^5+121x^6-228x^7+60x^8)$

**Simplify[Cf[8, 3, 13]]**

[\[化简\]](#)

$$-2048 (-1+x)^2 x (1+x)^5 (18-53x+419x^2-464x^3+1070x^4-399x^5+121x^6-228x^7+60x^8)$$

**Simplify[Cf[8, 3, 14]]**

[\[化简\]](#)

$$-2048 (-1+x)^2 x^2 (1+x)^5 (9+60x+34x^2+56x^3+177x^4-188x^5+28x^6)$$

**(\*, r2^8r3^4\*)**

**Simplify[Cf[8, 4, 0]]**

[\[化简\]](#)

0

**Simplify[Cf[8, 4, 1]]**

[\[化简\]](#)

0

**Simplify[Cf[8, 4, 2]]**

[\[化简\]](#)

0

**Simplify[Cf[8, 4, 3]]**

[\[化简\]](#)

0

**Simplify[Cf[8, 4, 4]]**

[\[化简\]](#)

0

**Simplify[Cf[8, 4, 5]]**

[\[化简\]](#)

0

**Simplify[Cf[8, 4, 6]]**

[\[化简\]](#)

0

**Simplify[Cf[8, 4, 7]]**

[\[化简\]](#)

0

**Simplify[Cf[8, 4, 8]]**

[\[化简\]](#)

0

**Simplify[Cf[8, 4, 9]]**

[\[化简\]](#)

0

**Simplify[Cf[8, 4, 10]]**

[\[化简\]](#)

$$-1024 x^2 (1+x)^5 (67+2x+857x^2-2092x^3+3073x^4-3126x^5+1695x^6-736x^7+260x^8)$$

**Simplify[Cf[8, 4, 11]]**

[化简]

$$-2048 x (1+x)^5 (24 + 71 x + 389 x^2 - 1171 x^3 + 5567 x^4 - 11413 x^5 + 13431 x^6 - 11365 x^7 + 5741 x^8 - 1562 x^9 + 288 x^{10})$$

**Simplify[Cf[8, 4, 12]]**

[化简]

$$-2048 (1+x)^5 (24 - 240 x + 1755 x^2 - 5836 x^3 + 16193 x^4 - 28994 x^5 + 40829 x^6 - 45928 x^7 + 37615 x^8 - 23738 x^9 + 10784 x^{10} - 2848 x^{11} + 384 x^{12})$$

**Simplify[Cf[8, 4, 13]]**

[化简]

$$-2048 x (1+x)^5 (24 + 71 x + 389 x^2 - 1171 x^3 + 5567 x^4 - 11413 x^5 + 13431 x^6 - 11365 x^7 + 5741 x^8 - 1562 x^9 + 288 x^{10})$$

**Simplify[Cf[8, 4, 14]]**

[化简]

$$-1024 x^2 (1+x)^5 (67 + 2 x + 857 x^2 - 2092 x^3 + 3073 x^4 - 3126 x^5 + 1695 x^6 - 736 x^7 + 260 x^8)$$

(\*, r2^8r3^5\*)

**Simplify[Cf[8, 5, 0]]**

[化简]

0

**Simplify[Cf[8, 5, 1]]**

[化简]

0

**Simplify[Cf[8, 5, 2]]**

[化简]

0

**Simplify[Cf[8, 5, 3]]**

[化简]

0

**Simplify[Cf[8, 5, 4]]**

[化简]

0

**Simplify[Cf[8, 5, 5]]**

[化简]

0

**Simplify[Cf[8, 5, 6]]**

[化简]

0

**Simplify[Cf[8, 5, 7]]**

[化简]

0

**Simplify[Cf[8, 5, 8]]**

[\[化简\]](#)

0

**Simplify[Cf[8, 5, 9]]**

[\[化简\]](#)

$$-4096 x^2 (1+x)^5 (23+98 x+26 x^2+194 x^3-51 x^4-384 x^5+674 x^6-540 x^7+104 x^8)$$

**Simplify[Cf[8, 5, 10]]**

[\[化简\]](#)

$$-2048 x (1+x)^5 (94-303 x+3119 x^2-6866 x^3+17814 x^4-22905 x^5+21615 x^6-15272 x^7+5986 x^8-1982 x^9+236 x^{10})$$

**Simplify[Cf[8, 5, 11]]**

[\[化简\]](#)

$$2048 x (1+x)^5 (-238+753 x-6036 x^2+11066 x^3-26967 x^4+30947 x^5-31826 x^6+26928 x^7-10617 x^8+2938 x^9-140 x^{10}+24 x^{11})$$

**Simplify[Cf[8, 5, 12]]**

[\[化简\]](#)

$$2048 x (1+x)^5 (-238+753 x-6036 x^2+11066 x^3-26967 x^4+30947 x^5-31826 x^6+26928 x^7-10617 x^8+2938 x^9-140 x^{10}+24 x^{11})$$

**Simplify[Cf[8, 5, 13]]**

[\[化简\]](#)

$$-2048 x (1+x)^5 (94-303 x+3119 x^2-6866 x^3+17814 x^4-22905 x^5+21615 x^6-15272 x^7+5986 x^8-1982 x^9+236 x^{10})$$

**Simplify[Cf[8, 5, 14]]**

[\[化简\]](#)

$$-4096 x^2 (1+x)^5 (23+98 x+26 x^2+194 x^3-51 x^4-384 x^5+674 x^6-540 x^7+104 x^8)$$

(\*, r2^8r3^6\*)

**Simplify[Cf[8, 6, 0]]**

[\[化简\]](#)

0

**Simplify[Cf[8, 6, 1]]**

[\[化简\]](#)

0

**Simplify[Cf[8, 6, 2]]**

[\[化简\]](#)

0

**Simplify[Cf[8, 6, 3]]**

[\[化简\]](#)

0

**Simplify[Cf[8, 6, 4]]**[\[化简\]](#)

0

**Simplify[Cf[8, 6, 5]]**[\[化简\]](#)

0

**Simplify[Cf[8, 6, 6]]**[\[化简\]](#)

0

**Simplify[Cf[8, 6, 7]]**[\[化简\]](#)

0

**Simplify[Cf[8, 6, 8]]**[\[化简\]](#)

$$2048 x^2 (1+x)^5 (-85 - 26 x - 1639 x^2 + 3668 x^3 - 7407 x^4 + 7286 x^5 - 3481 x^6 - 208 x^7 + 548 x^8)$$

**Simplify[Cf[8, 6, 9]]**[\[化简\]](#)

$$2048 x (1+x)^5 (-108 - 12 x - 3006 x^2 + 5481 x^3 - 23953 x^4 + 31960 x^5 - 38556 x^6 + 27749 x^7 - 12817 x^8 + 2438 x^9 + 840 x^{10})$$

**Simplify[Cf[8, 6, 10]]**[\[化简\]](#)

$$1024 (1+x)^5 (-228 + 2280 x - 17657 x^2 + 55410 x^3 - 175923 x^4 + 316440 x^5 - 538591 x^6 + 605042 x^7 - 527289 x^8 + 312060 x^9 - 106312 x^{10} + 17792 x^{11} + 1104 x^{12})$$

**Simplify[Cf[8, 6, 11]]**[\[化简\]](#)

$$2048 x (1+x)^5 (-384 + 9 x - 11414 x^2 + 26555 x^3 - 107046 x^4 + 159337 x^5 - 217282 x^6 + 182633 x^7 - 123402 x^8 + 75666 x^9 - 29528 x^{10} + 6264 x^{11})$$

**Simplify[Cf[8, 6, 12]]**[\[化简\]](#)

$$1024 (1+x)^5 (-228 + 2280 x - 17657 x^2 + 55410 x^3 - 175923 x^4 + 316440 x^5 - 538591 x^6 + 605042 x^7 - 527289 x^8 + 312060 x^9 - 106312 x^{10} + 17792 x^{11} + 1104 x^{12})$$

**Simplify[Cf[8, 6, 13]]**[\[化简\]](#)

$$2048 x (1+x)^5 (-108 - 12 x - 3006 x^2 + 5481 x^3 - 23953 x^4 + 31960 x^5 - 38556 x^6 + 27749 x^7 - 12817 x^8 + 2438 x^9 + 840 x^{10})$$

**Simplify[Cf[8, 6, 14]]**[\[化简\]](#)

$$2048 x^2 (1+x)^5 (-85 - 26 x - 1639 x^2 + 3668 x^3 - 7407 x^4 + 7286 x^5 - 3481 x^6 - 208 x^7 + 548 x^8)$$

(\*, r2^8r3^7\*)

**Simplify[Cf[8, 7, 0]]**

[\[化简\]](#)

0

**Simplify[Cf[8, 7, 1]]**

[\[化简\]](#)

0

**Simplify[Cf[8, 7, 2]]**

[\[化简\]](#)

0

**Simplify[Cf[8, 7, 3]]**

[\[化简\]](#)

0

**Simplify[Cf[8, 7, 4]]**

[\[化简\]](#)

0

**Simplify[Cf[8, 7, 5]]**

[\[化简\]](#)

0

**Simplify[Cf[8, 7, 6]]**

[\[化简\]](#)

0

**Simplify[Cf[8, 7, 7]]**

[\[化简\]](#)

$$-4096 x^2 (1+x)^5 (37+159 x+117 x^2+585 x^3-685 x^4+1145 x^5-489 x^6-17 x^7+204 x^8)$$

**Simplify[Cf[8, 7, 8]]**

[\[化简\]](#)

$$-4096 x (1+x)^5 (80-127 x+2587 x^2-4727 x^3+17005 x^4-19163 x^5+23373 x^6-13825 x^7+6171 x^8-366 x^9+128 x^{10})$$

**Simplify[Cf[8, 7, 9]]**

[\[化简\]](#)

$$-2048 x (1+x)^5 (688-2146 x+18920 x^2-30213 x^3+98031 x^4-105466 x^5+166870 x^6-122025 x^7+79547 x^8-24214 x^9+4344 x^{10}+48 x^{11})$$

**Simplify[Cf[8, 7, 10]]**

[\[化简\]](#)

$$-2048 x (1+x)^5 (888-1940 x+27259 x^2-45307 x^3+164672 x^4-170926 x^5+259107 x^6-149199 x^7+94290 x^8-21764 x^9-3096 x^{10}+2592 x^{11})$$

**Simplify[Cf[8, 7, 11]]**

[\[化简\]](#)

$$-2048 x (1+x)^5 (888-1940 x+27259 x^2-45307 x^3+164672 x^4-170926 x^5+259107 x^6-149199 x^7+94290 x^8-21764 x^9-3096 x^{10}+2592 x^{11})$$

**Simplify[Cf[8, 7, 12]]**

[化简]

$$-2048 x (1+x)^5 (688 - 2146 x + 18920 x^2 - 30213 x^3 + 98031 x^4 - 105466 x^5 + 166870 x^6 - 122025 x^7 + 79547 x^8 - 24214 x^9 + 4344 x^{10} + 48 x^{11})$$

**Simplify[Cf[8, 7, 13]]**

[化简]

$$-4096 x (1+x)^5 (80 - 127 x + 2587 x^2 - 4727 x^3 + 17005 x^4 - 19163 x^5 + 23373 x^6 - 13825 x^7 + 6171 x^8 - 366 x^9 + 128 x^{10})$$

**Simplify[Cf[8, 7, 14]]**

[化简]

$$-4096 x^2 (1+x)^5 (37 + 159 x + 117 x^2 + 585 x^3 - 685 x^4 + 1145 x^5 - 489 x^6 - 17 x^7 + 204 x^8)$$

**(\*, r2^8r3^8\*)****Simplify[Cf[8, 8, 0]]**

[化简]

0

**Simplify[Cf[8, 8, 1]]**

[化简]

0

**Simplify[Cf[8, 8, 2]]**

[化简]

0

**Simplify[Cf[8, 8, 3]]**

[化简]

0

**Simplify[Cf[8, 8, 4]]**

[化简]

0

**Simplify[Cf[8, 8, 5]]**

[化简]

0

**Simplify[Cf[8, 8, 6]]**

[化简]

$$2048 x^2 (1+x)^5 (-85 - 26 x - 1639 x^2 + 3668 x^3 - 7407 x^4 + 7286 x^5 - 3481 x^6 - 208 x^7 + 548 x^8)$$

**Simplify[Cf[8, 8, 7]]**

[化简]

$$-4096 x (1+x)^5 (80 - 127 x + 2587 x^2 - 4727 x^3 + 17005 x^4 - 19163 x^5 + 23373 x^6 - 13825 x^7 + 6171 x^8 - 366 x^9 + 128 x^{10})$$

**Simplify[Cf[8, 8, 8]]**

[化简]

$$-12\,288 (1+x)^5 (30 - 300x + 2370x^2 - 7303x^3 + 24\,342x^4 - 43\,183x^5 + 79\,252x^6 - 86\,093x^7 + 80\,456x^8 - 44\,489x^9 + 16\,526x^{10} - 1784x^{11} + 48x^{12})$$

**Simplify[Cf[8, 8, 9]]**

[化简]

$$4096x (1+x)^5 (-506 + 573x - 16\,189x^2 + 28\,202x^3 - 122\,602x^4 + 136\,419x^5 - 225\,173x^6 + 140\,452x^7 - 121\,230x^8 + 50\,018x^9 - 21\,356x^{10} + 1920x^{11})$$

**Simplify[Cf[8, 8, 10]]**

[化简]

$$-4096 (1+x)^5 (186 - 1860x + 14\,925x^2 - 44\,680x^3 + 161\,887x^4 - 293\,128x^5 + 584\,285x^6 - 635\,584x^7 + 623\,747x^8 - 322\,396x^9 + 135\,154x^{10} - 26\,672x^{11} + 4776x^{12})$$

**Simplify[Cf[8, 8, 11]]**

[化简]

$$4096x (1+x)^5 (-506 + 573x - 16\,189x^2 + 28\,202x^3 - 122\,602x^4 + 136\,419x^5 - 225\,173x^6 + 140\,452x^7 - 121\,230x^8 + 50\,018x^9 - 21\,356x^{10} + 1920x^{11})$$

**Simplify[Cf[8, 8, 12]]**

[化简]

$$-12\,288 (1+x)^5 (30 - 300x + 2370x^2 - 7303x^3 + 24\,342x^4 - 43\,183x^5 + 79\,252x^6 - 86\,093x^7 + 80\,456x^8 - 44\,489x^9 + 16\,526x^{10} - 1784x^{11} + 48x^{12})$$

**Simplify[Cf[8, 8, 13]]**

[化简]

$$-4096x (1+x)^5 (80 - 127x + 2587x^2 - 4727x^3 + 17\,005x^4 - 19\,163x^5 + 23\,373x^6 - 13\,825x^7 + 6171x^8 - 366x^9 + 128x^{10})$$

**Simplify[Cf[8, 8, 14]]**

[化简]

$$2048x^2 (1+x)^5 (-85 - 26x - 1639x^2 + 3668x^3 - 7407x^4 + 7286x^5 - 3481x^6 - 208x^7 + 548x^8)$$

**(\*, r2^8r3^9\*)****Simplify[Cf[8, 9, 0]]**

[化简]

0

**Simplify[Cf[8, 9, 1]]**

[化简]

0

**Simplify[Cf[8, 9, 2]]**

[化简]

0

**Simplify[Cf[8, 9, 3]]**

[化简]

0



**Simplify[Cf[8, 9, 4]]**

[化简]

0

**Simplify[Cf[8, 9, 5]]**

[化简]

$$-4096 x^2 (1+x)^5 (23+98 x+26 x^2+194 x^3-51 x^4-384 x^5+674 x^6-540 x^7+104 x^8)$$

**Simplify[Cf[8, 9, 6]]**

[化简]

$$2048 x (1+x)^5 (-108-12 x-3006 x^2+5481 x^3-23953 x^4+31960 x^5-38556 x^6+27749 x^7-12817 x^8+2438 x^9+840 x^{10})$$

**Simplify[Cf[8, 9, 7]]**

[化简]

$$-2048 x (1+x)^5 (688-2146 x+18920 x^2-30213 x^3+98031 x^4-105466 x^5+166870 x^6-122025 x^7+79547 x^8-24214 x^9+4344 x^{10}+48 x^{11})$$

**Simplify[Cf[8, 9, 8]]**

[化简]

$$4096 x (1+x)^5 (-506+573 x-16189 x^2+28202 x^3-122602 x^4+136419 x^5-225173 x^6+140452 x^7-121230 x^8+50018 x^9-21356 x^{10}+1920 x^{11})$$

**Simplify[Cf[8, 9, 9]]**

[化简]

$$8192 x (1+x)^5 (-410+870 x-12862 x^2+19133 x^3-83657 x^4+81396 x^5-153656 x^6+82967 x^7-76651 x^8+15660 x^9-8444 x^{10}+102 x^{11})$$

**Simplify[Cf[8, 9, 10]]**

[化简]

$$8192 x (1+x)^5 (-410+870 x-12862 x^2+19133 x^3-83657 x^4+81396 x^5-153656 x^6+82967 x^7-76651 x^8+15660 x^9-8444 x^{10}+102 x^{11})$$

**Simplify[Cf[8, 9, 11]]**

[化简]

$$4096 x (1+x)^5 (-506+573 x-16189 x^2+28202 x^3-122602 x^4+136419 x^5-225173 x^6+140452 x^7-121230 x^8+50018 x^9-21356 x^{10}+1920 x^{11})$$

**Simplify[Cf[8, 9, 12]]**

[化简]

$$-2048 x (1+x)^5 (688-2146 x+18920 x^2-30213 x^3+98031 x^4-105466 x^5+166870 x^6-122025 x^7+79547 x^8-24214 x^9+4344 x^{10}+48 x^{11})$$

**Simplify[Cf[8, 9, 13]]**

[化简]

$$2048 x (1+x)^5 (-108-12 x-3006 x^2+5481 x^3-23953 x^4+31960 x^5-38556 x^6+27749 x^7-12817 x^8+2438 x^9+840 x^{10})$$

**Simplify[Cf[8, 9, 14]]**

[化简]

$$-4096 x^2 (1+x)^5 (23+98 x+26 x^2+194 x^3-51 x^4-384 x^5+674 x^6-540 x^7+104 x^8)$$

(\*, r2^8r3^10\*)

**Simplify[Cf[8, 10, 0]]**

[化简]

0

**Simplify[Cf[8, 10, 1]]**

[化简]

0

**Simplify[Cf[8, 10, 2]]**

[化简]

0

**Simplify[Cf[8, 10, 3]]**

[化简]

0

**Simplify[Cf[8, 10, 4]]**

[化简]

$$-1024 x^2 (1+x)^5 (67+2 x+857 x^2-2092 x^3+3073 x^4-3126 x^5+1695 x^6-736 x^7+260 x^8)$$

**Simplify[Cf[8, 10, 5]]**

[化简]

$$-2048 x (1+x)^5 (94-303 x+3119 x^2-6866 x^3+17814 x^4-22905 x^5+21615 x^6-15272 x^7+5986 x^8-1982 x^9+236 x^{10})$$

**Simplify[Cf[8, 10, 6]]**

[化简]

$$1024 (1+x)^5 (-228+2280 x-17657 x^2+55410 x^3-175923 x^4+316440 x^5-538591 x^6+605042 x^7-527289 x^8+312060 x^9-106312 x^{10}+17792 x^{11}+1104 x^{12})$$

**Simplify[Cf[8, 10, 7]]**

[化简]

$$-2048 x (1+x)^5 (888-1940 x+27259 x^2-45307 x^3+164672 x^4-170926 x^5+259107 x^6-149199 x^7+94290 x^8-21764 x^9-3096 x^{10}+2592 x^{11})$$

**Simplify[Cf[8, 10, 8]]**

[化简]

$$-4096 (1+x)^5 (186-1860 x+14925 x^2-44680 x^3+161887 x^4-293128 x^5+584285 x^6-635584 x^7+623747 x^8-322396 x^9+135154 x^{10}-26672 x^{11}+4776 x^{12})$$

**Simplify[Cf[8, 10, 9]]**

[化简]

$$8192 x (1+x)^5 (-410+870 x-12862 x^2+19133 x^3-83657 x^4+81396 x^5-153656 x^6+82967 x^7-76651 x^8+15660 x^9-8444 x^{10}+102 x^{11})$$

**Simplify[Cf[8, 10, 10]]**

[化简]

$$-4096 (1+x)^5 (186-1860 x+14925 x^2-44680 x^3+161887 x^4-293128 x^5+584285 x^6-635584 x^7+623747 x^8-322396 x^9+135154 x^{10}-26672 x^{11}+4776 x^{12})$$

**Simplify[Cf[8, 10, 11]]**

[化简]

$$-2048 x (1+x)^5 (888 - 1940 x + 27259 x^2 - 45307 x^3 + 164672 x^4 - 170926 x^5 + 259107 x^6 - 149199 x^7 + 94290 x^8 - 21764 x^9 - 3096 x^{10} + 2592 x^{11})$$

**Simplify[Cf[8, 10, 12]]**

[化简]

$$1024 (1+x)^5 (-228 + 2280 x - 17657 x^2 + 55410 x^3 - 175923 x^4 + 316440 x^5 - 538591 x^6 + 605042 x^7 - 527289 x^8 + 312060 x^9 - 106312 x^{10} + 17792 x^{11} + 1104 x^{12})$$

**Simplify[Cf[8, 10, 13]]**

[化简]

$$-2048 x (1+x)^5 (94 - 303 x + 3119 x^2 - 6866 x^3 + 17814 x^4 - 22905 x^5 + 21615 x^6 - 15272 x^7 + 5986 x^8 - 1982 x^9 + 236 x^{10})$$

**Simplify[Cf[8, 10, 14]]**

[化简]

$$-1024 x^2 (1+x)^5 (67 + 2 x + 857 x^2 - 2092 x^3 + 3073 x^4 - 3126 x^5 + 1695 x^6 - 736 x^7 + 260 x^8)$$

**(\*, r2^8r3^11\*)****Simplify[Cf[8, 11, 0]]**

[化简]

0

**Simplify[Cf[8, 11, 1]]**

[化简]

0

**Simplify[Cf[8, 11, 2]]**

[化简]

0

**Simplify[Cf[8, 11, 3]]**

[化简]

$$-2048 (-1+x)^2 x^2 (1+x)^5 (9 + 60 x + 34 x^2 + 56 x^3 + 177 x^4 - 188 x^5 + 28 x^6)$$

**Simplify[Cf[8, 11, 4]]**

[化简]

$$-2048 x (1+x)^5 (24 + 71 x + 389 x^2 - 1171 x^3 + 5567 x^4 - 11413 x^5 + 13431 x^6 - 11365 x^7 + 5741 x^8 - 1562 x^9 + 288 x^{10})$$

**Simplify[Cf[8, 11, 5]]**

[化简]

$$2048 x (1+x)^5 (-238 + 753 x - 6036 x^2 + 11066 x^3 - 26967 x^4 + 30947 x^5 - 31826 x^6 + 26928 x^7 - 10617 x^8 + 2938 x^9 - 140 x^{10} + 24 x^{11})$$

**Simplify[Cf[8, 11, 6]]**

[化简]

$$2048 x (1+x)^5 (-384 + 9 x - 11414 x^2 + 26555 x^3 - 107046 x^4 + 159337 x^5 - 217282 x^6 + 182633 x^7 - 123402 x^8 + 75666 x^9 - 29528 x^{10} + 6264 x^{11})$$

**Simplify[Cf[8, 11, 7]]**

[化简]

$$-2048 x (1+x)^5 (888 - 1940 x + 27259 x^2 - 45307 x^3 + 164672 x^4 - 170926 x^5 + 259107 x^6 - 149199 x^7 + 94290 x^8 - 21764 x^9 - 3096 x^{10} + 2592 x^{11})$$

**Simplify[Cf[8, 11, 8]]**

[化简]

$$4096 x (1+x)^5 (-506 + 573 x - 16189 x^2 + 28202 x^3 - 122602 x^4 + 136419 x^5 - 225173 x^6 + 140452 x^7 - 121230 x^8 + 50018 x^9 - 21356 x^{10} + 1920 x^{11})$$

**Simplify[Cf[8, 11, 9]]**

[化简]

$$4096 x (1+x)^5 (-506 + 573 x - 16189 x^2 + 28202 x^3 - 122602 x^4 + 136419 x^5 - 225173 x^6 + 140452 x^7 - 121230 x^8 + 50018 x^9 - 21356 x^{10} + 1920 x^{11})$$

**Simplify[Cf[8, 11, 10]]**

[化简]

$$-2048 x (1+x)^5 (888 - 1940 x + 27259 x^2 - 45307 x^3 + 164672 x^4 - 170926 x^5 + 259107 x^6 - 149199 x^7 + 94290 x^8 - 21764 x^9 - 3096 x^{10} + 2592 x^{11})$$

**Simplify[Cf[8, 11, 11]]**

[化简]

$$2048 x (1+x)^5 (-384 + 9 x - 11414 x^2 + 26555 x^3 - 107046 x^4 + 159337 x^5 - 217282 x^6 + 182633 x^7 - 123402 x^8 + 75666 x^9 - 29528 x^{10} + 6264 x^{11})$$

**Simplify[Cf[8, 11, 12]]**

[化简]

$$2048 x (1+x)^5 (-238 + 753 x - 6036 x^2 + 11066 x^3 - 26967 x^4 + 30947 x^5 - 31826 x^6 + 26928 x^7 - 10617 x^8 + 2938 x^9 - 140 x^{10} + 24 x^{11})$$

**Simplify[Cf[8, 11, 13]]**

[化简]

$$-2048 x (1+x)^5 (24 + 71 x + 389 x^2 - 1171 x^3 + 5567 x^4 - 11413 x^5 + 13431 x^6 - 11365 x^7 + 5741 x^8 - 1562 x^9 + 288 x^{10})$$

**Simplify[Cf[8, 11, 14]]**

[化简]

$$-2048 (-1+x)^2 x^2 (1+x)^5 (9 + 60 x + 34 x^2 + 56 x^3 + 177 x^4 - 188 x^5 + 28 x^6)$$

**(\*, r2^8r3^12\*)****Simplify[Cf[8, 12, 0]]**

[化简]

0

**Simplify[Cf[8, 12, 1]]**

[化简]

0

**Simplify[Cf[8, 12, 2]]**

[化简]

$$1024 (-1+x)^3 x^2 (1+x)^5 (7+19x+13x^2+137x^3-172x^4+44x^5)$$

**Simplify[Cf[8, 12, 3]]**

[化简]

$$-2048 (-1+x)^2 x (1+x)^5 (18-53x+419x^2-464x^3+1070x^4-399x^5+121x^6-228x^7+60x^8)$$

**Simplify[Cf[8, 12, 4]]**

[化简]

$$-2048 (1+x)^5 (24-240x+1755x^2-5836x^3+16193x^4-28994x^5+40829x^6-45928x^7+37615x^8-23738x^9+10784x^{10}-2848x^{11}+384x^{12})$$

**Simplify[Cf[8, 12, 5]]**

[化简]

$$2048 x (1+x)^5 (-238+753x-6036x^2+11066x^3-26967x^4+30947x^5-31826x^6+26928x^7-10617x^8+2938x^9-140x^{10}+24x^{11})$$

**Simplify[Cf[8, 12, 6]]**

[化简]

$$1024 (1+x)^5 (-228+2280x-17657x^2+55410x^3-175923x^4+316440x^5-538591x^6+605042x^7-527289x^8+312060x^9-106312x^{10}+17792x^{11}+1104x^{12})$$

**Simplify[Cf[8, 12, 7]]**

[化简]

$$-2048 x (1+x)^5 (688-2146x+18920x^2-30213x^3+98031x^4-105466x^5+166870x^6-122025x^7+79547x^8-24214x^9+4344x^{10}+48x^{11})$$

**Simplify[Cf[8, 12, 8]]**

[化简]

$$-12288 (1+x)^5 (30-300x+2370x^2-7303x^3+24342x^4-43183x^5+79252x^6-86093x^7+80456x^8-44489x^9+16526x^{10}-1784x^{11}+48x^{12})$$

**Simplify[Cf[8, 12, 9]]**

[化简]

$$-2048 x (1+x)^5 (688-2146x+18920x^2-30213x^3+98031x^4-105466x^5+166870x^6-122025x^7+79547x^8-24214x^9+4344x^{10}+48x^{11})$$

**Simplify[Cf[8, 12, 10]]**

[化简]

$$1024 (1+x)^5 (-228+2280x-17657x^2+55410x^3-175923x^4+316440x^5-538591x^6+605042x^7-527289x^8+312060x^9-106312x^{10}+17792x^{11}+1104x^{12})$$

**Simplify[Cf[8, 12, 11]]**

[化简]

$$2048 x (1+x)^5 (-238+753x-6036x^2+11066x^3-26967x^4+30947x^5-31826x^6+26928x^7-10617x^8+2938x^9-140x^{10}+24x^{11})$$

**Simplify[Cf[8, 12, 12]]**

[化简]

$$-2048 (1+x)^5 (24 - 240x + 1755x^2 - 5836x^3 + 16193x^4 - 28994x^5 + 40829x^6 - 45928x^7 + 37615x^8 - 23738x^9 + 10784x^{10} - 2848x^{11} + 384x^{12})$$

**Simplify[Cf[8, 12, 13]]**

[化简]

$$-2048 (-1+x)^2 x (1+x)^5 (18 - 53x + 419x^2 - 464x^3 + 1070x^4 - 399x^5 + 121x^6 - 228x^7 + 60x^8)$$

**Simplify[Cf[8, 12, 14]]**

[化简]

$$1024 (-1+x)^3 x^2 (1+x)^5 (7 + 19x + 13x^2 + 137x^3 - 172x^4 + 44x^5)$$

**(\*, r2^8r3^13\*)****Simplify[Cf[8, 13, 0]]**

[化简]

0

**Simplify[Cf[8, 13, 1]]**

[化简]

$$6144 (-1+x)^5 x^3 (1+x)^6$$

**Simplify[Cf[8, 13, 2]]**

[化简]

$$2048 (-1+x)^3 x^2 (1+x)^5 (15 - x + 23x^2 + 135x^3 - 158x^4 + 34x^5)$$

**Simplify[Cf[8, 13, 3]]**

[化简]

$$-2048 (-1+x)^2 x (1+x)^5 (18 - 53x + 419x^2 - 464x^3 + 1070x^4 - 399x^5 + 121x^6 - 228x^7 + 60x^8)$$

**Simplify[Cf[8, 13, 4]]**

[化简]

$$-2048 x (1+x)^5 (24 + 71x + 389x^2 - 1171x^3 + 5567x^4 - 11413x^5 + 13431x^6 - 11365x^7 + 5741x^8 - 1562x^9 + 288x^{10})$$

**Simplify[Cf[8, 13, 5]]**

[化简]

$$-2048 x (1+x)^5 (94 - 303x + 3119x^2 - 6866x^3 + 17814x^4 - 22905x^5 + 21615x^6 - 15272x^7 + 5986x^8 - 1982x^9 + 236x^{10})$$

**Simplify[Cf[8, 13, 6]]**

[化简]

$$2048 x (1+x)^5 (-108 - 12x - 3006x^2 + 5481x^3 - 23953x^4 + 31960x^5 - 38556x^6 + 27749x^7 - 12817x^8 + 2438x^9 + 840x^{10})$$

**Simplify[Cf[8, 13, 7]]**

[化简]

$$-4096 x (1+x)^5 (80 - 127x + 2587x^2 - 4727x^3 + 17005x^4 - 19163x^5 + 23373x^6 - 13825x^7 + 6171x^8 - 366x^9 + 128x^{10})$$

**Simplify[Cf[8, 13, 8]]**

[化简]

$$-4096 x (1+x)^5 (80 - 127 x + 2587 x^2 - 4727 x^3 + 17005 x^4 - 19163 x^5 + 23373 x^6 - 13825 x^7 + 6171 x^8 - 366 x^9 + 128 x^{10})$$

**Simplify[Cf[8, 13, 9]]**

[化简]

$$2048 x (1+x)^5 (-108 - 12 x - 3006 x^2 + 5481 x^3 - 23953 x^4 + 31960 x^5 - 38556 x^6 + 27749 x^7 - 12817 x^8 + 2438 x^9 + 840 x^{10})$$

**Simplify[Cf[8, 13, 10]]**

[化简]

$$-2048 x (1+x)^5 (94 - 303 x + 3119 x^2 - 6866 x^3 + 17814 x^4 - 22905 x^5 + 21615 x^6 - 15272 x^7 + 5986 x^8 - 1982 x^9 + 236 x^{10})$$

**Simplify[Cf[8, 13, 11]]**

[化简]

$$-2048 x (1+x)^5 (24 + 71 x + 389 x^2 - 1171 x^3 + 5567 x^4 - 11413 x^5 + 13431 x^6 - 11365 x^7 + 5741 x^8 - 1562 x^9 + 288 x^{10})$$

**Simplify[Cf[8, 13, 12]]**

[化简]

$$-2048 (-1+x)^2 x (1+x)^5 (18 - 53 x + 419 x^2 - 464 x^3 + 1070 x^4 - 399 x^5 + 121 x^6 - 228 x^7 + 60 x^8)$$

**Simplify[Cf[8, 13, 13]]**

[化简]

$$2048 (-1+x)^3 x^2 (1+x)^5 (15 - x + 23 x^2 + 135 x^3 - 158 x^4 + 34 x^5)$$

**Simplify[Cf[8, 13, 14]]**

[化简]

$$6144 (-1+x)^5 x^3 (1+x)^6$$

**(\*, r2^8r3^14\*)****Simplify[Cf[8, 14, 0]]**

[化简]

0

**Simplify[Cf[8, 14, 1]]**

[化简]

$$6144 (-1+x)^5 x^3 (1+x)^6$$

**Simplify[Cf[8, 14, 2]]**

[化简]

$$1024 (-1+x)^3 x^2 (1+x)^5 (7 + 19 x + 13 x^2 + 137 x^3 - 172 x^4 + 44 x^5)$$

**Simplify[Cf[8, 14, 3]]**

[化简]

$$-2048 (-1+x)^2 x^2 (1+x)^5 (9 + 60 x + 34 x^2 + 56 x^3 + 177 x^4 - 188 x^5 + 28 x^6)$$

**Simplify[Cf[8, 14, 4]]**

[\[化简\]](#)

$$-1024 x^2 (1+x)^5 (67+2x+857x^2-2092x^3+3073x^4-3126x^5+1695x^6-736x^7+260x^8)$$

**Simplify[Cf[8, 14, 5]]**

[\[化简\]](#)

$$-4096 x^2 (1+x)^5 (23+98x+26x^2+194x^3-51x^4-384x^5+674x^6-540x^7+104x^8)$$

**Simplify[Cf[8, 14, 6]]**

[\[化简\]](#)

$$2048 x^2 (1+x)^5 (-85-26x-1639x^2+3668x^3-7407x^4+7286x^5-3481x^6-208x^7+548x^8)$$

**Simplify[Cf[8, 14, 7]]**

[\[化简\]](#)

$$-4096 x^2 (1+x)^5 (37+159x+117x^2+585x^3-685x^4+1145x^5-489x^6-17x^7+204x^8)$$

**Simplify[Cf[8, 14, 8]]**

[\[化简\]](#)

$$2048 x^2 (1+x)^5 (-85-26x-1639x^2+3668x^3-7407x^4+7286x^5-3481x^6-208x^7+548x^8)$$

**Simplify[Cf[8, 14, 9]]**

[\[化简\]](#)

$$-4096 x^2 (1+x)^5 (23+98x+26x^2+194x^3-51x^4-384x^5+674x^6-540x^7+104x^8)$$

**Simplify[Cf[8, 14, 10]]**

[\[化简\]](#)

$$-1024 x^2 (1+x)^5 (67+2x+857x^2-2092x^3+3073x^4-3126x^5+1695x^6-736x^7+260x^8)$$

**Simplify[Cf[8, 14, 11]]**

[\[化简\]](#)

$$-2048 (-1+x)^2 x^2 (1+x)^5 (9+60x+34x^2+56x^3+177x^4-188x^5+28x^6)$$

**Simplify[Cf[8, 14, 12]]**

[\[化简\]](#)

$$1024 (-1+x)^3 x^2 (1+x)^5 (7+19x+13x^2+137x^3-172x^4+44x^5)$$

**Simplify[Cf[8, 14, 13]]**

[\[化简\]](#)

$$6144 (-1+x)^5 x^3 (1+x)^6$$

**Simplify[Cf[8, 14, 14]]**

[\[化简\]](#)

0

(\*, r2^9r3^0\*)

**Simplify[Cf[9, 0, 0]]**

[\[化简\]](#)

0



**Simplify[Cf[9, 0, 1]]**

[化简]

0

**Simplify[Cf[9, 0, 2]]**

[化简]

0

**Simplify[Cf[9, 0, 3]]**

[化简]

0

**Simplify[Cf[9, 0, 4]]**

[化简]

0

**Simplify[Cf[9, 0, 5]]**

[化简]

0

**Simplify[Cf[9, 0, 6]]**

[化简]

0

**Simplify[Cf[9, 0, 7]]**

[化简]

0

**Simplify[Cf[9, 0, 8]]**

[化简]

0

**Simplify[Cf[9, 0, 9]]**

[化简]

0

**Simplify[Cf[9, 0, 10]]**

[化简]

0

**Simplify[Cf[9, 0, 11]]**

[化简]

0

**Simplify[Cf[9, 0, 12]]**

[化简]

0

**Simplify[Cf[9, 0, 13]]**

[化简]

$-2048 (-1+x)^6 x^3 (1+x)^5$

**Simplify[Cf[9, 0, 14]]**

[化简]

$$-2048 (-1+x)^6 x^3 (1+x)^5$$

(\*, r2^9r3^1\*)

**Simplify[Cf[9, 1, 0]]**

[化简]

0

**Simplify[Cf[9, 1, 1]]**

[化简]

0

**Simplify[Cf[9, 1, 2]]**

[化简]

0

**Simplify[Cf[9, 1, 3]]**

[化简]

0

**Simplify[Cf[9, 1, 4]]**

[化简]

0

**Simplify[Cf[9, 1, 5]]**

[化简]

0

**Simplify[Cf[9, 1, 6]]**

[化简]

0

**Simplify[Cf[9, 1, 7]]**

[化简]

0

**Simplify[Cf[9, 1, 8]]**

[化简]

0

**Simplify[Cf[9, 1, 9]]**

[化简]

0

**Simplify[Cf[9, 1, 10]]**

[化简]

0

**Simplify[Cf[9, 1, 11]]**

[化简]

0

**Simplify[Cf[9, 1, 12]]**

[化简]

$$-2048 (-1+x)^4 x^2 (1+x)^5 (2-3x+30x^2-21x^3+4x^4)$$

**Simplify[Cf[9, 1, 13]]**

[化简]

$$8192 (-1+x)^4 x^2 (1+x)^5 (-2+3x-13x^2+6x^3)$$

**Simplify[Cf[9, 1, 14]]**

[化简]

$$-2048 (-1+x)^4 x^2 (1+x)^5 (2-3x+30x^2-21x^3+4x^4)$$

**(\*, r2^9r3^2\*)**

**Simplify[Cf[9, 2, 0]]**

[化简]

0

**Simplify[Cf[9, 2, 1]]**

[化简]

0

**Simplify[Cf[9, 2, 2]]**

[化简]

0

**Simplify[Cf[9, 2, 3]]**

[化简]

0

**Simplify[Cf[9, 2, 4]]**

[化简]

0

**Simplify[Cf[9, 2, 5]]**

[化简]

0

**Simplify[Cf[9, 2, 6]]**

[化简]

0

**Simplify[Cf[9, 2, 7]]**

[化简]

0

**Simplify[Cf[9, 2, 8]]**

[化简]

0

**Simplify[Cf[9, 2, 9]]**

[化简]

0

**Simplify[Cf[9, 2, 10]]**

[\[化简\]](#)

0

**Simplify[Cf[9, 2, 11]]**

[\[化简\]](#)

$-2048 (-1+x)^3 x^2 (1+x)^5 (-3-44x+37x^2-182x^3+60x^4)$

**Simplify[Cf[9, 2, 12]]**

[\[化简\]](#)

$2048 (-1+x)^3 x (1+x)^5 (6+7x+89x^2+50x^3+225x^4+197x^5-190x^6+36x^7)$

**Simplify[Cf[9, 2, 13]]**

[\[化简\]](#)

$2048 (-1+x)^3 x (1+x)^5 (6+7x+89x^2+50x^3+225x^4+197x^5-190x^6+36x^7)$

**Simplify[Cf[9, 2, 14]]**

[\[化简\]](#)

$-2048 (-1+x)^3 x^2 (1+x)^5 (-3-44x+37x^2-182x^3+60x^4)$

(\*, r2^9r3^3\*)

**Simplify[Cf[9, 3, 0]]**

[\[化简\]](#)

0

**Simplify[Cf[9, 3, 1]]**

[\[化简\]](#)

0

**Simplify[Cf[9, 3, 2]]**

[\[化简\]](#)

0

**Simplify[Cf[9, 3, 3]]**

[\[化简\]](#)

0

**Simplify[Cf[9, 3, 4]]**

[\[化简\]](#)

0

**Simplify[Cf[9, 3, 5]]**

[\[化简\]](#)

0

**Simplify[Cf[9, 3, 6]]**

[\[化简\]](#)

0

**Simplify[Cf[9, 3, 7]]**

[化简]

0

**Simplify[Cf[9, 3, 8]]**

[化简]

0

**Simplify[Cf[9, 3, 9]]**

[化简]

0

**Simplify[Cf[9, 3, 10]]**

[化简]

$$4096 (-1+x)^2 x^2 (1+x)^5 (-9-18x-124x^2+82x^3-207x^4+4x^5+40x^6)$$

**Simplify[Cf[9, 3, 11]]**

[化简]

$$4096 (-1+x)^2 x^2 (1+x)^5 (-120+337x-1408x^2+1558x^3-2044x^4+597x^5+4x^6+36x^7)$$

**Simplify[Cf[9, 3, 12]]**

[化简]

$$4096 (-1+x)^2 x (1+x)^5 (-30+78x-535x^2+314x^3-1370x^4+916x^5-2281x^6+1676x^7-456x^8+72x^9)$$

**Simplify[Cf[9, 3, 13]]**

[化简]

$$4096 (-1+x)^2 x^2 (1+x)^5 (-120+337x-1408x^2+1558x^3-2044x^4+597x^5+4x^6+36x^7)$$

**Simplify[Cf[9, 3, 14]]**

[化简]

$$4096 (-1+x)^2 x^2 (1+x)^5 (-9-18x-124x^2+82x^3-207x^4+4x^5+40x^6)$$

**(\*, r2^9r3^4\*)****Simplify[Cf[9, 4, 0]]**

[化简]

0

**Simplify[Cf[9, 4, 1]]**

[化简]

0

**Simplify[Cf[9, 4, 2]]**

[化简]

0

**Simplify[Cf[9, 4, 3]]**

[化简]

0

**Simplify[Cf[9, 4, 4]]**

[化简]

0

**Simplify[Cf[9, 4, 5]]**

[化简]

0

**Simplify[Cf[9, 4, 6]]**

[化简]

0

**Simplify[Cf[9, 4, 7]]**

[化简]

0

**Simplify[Cf[9, 4, 8]]**

[化简]

0

**Simplify[Cf[9, 4, 9]]**

[化简]

$$4096 x^2 (1+x)^5 (-11 - 106 x + 299 x^2 - 1048 x^3 + 2055 x^4 - 2338 x^5 + 1613 x^6 - 476 x^7 + 12 x^8)$$

**Simplify[Cf[9, 4, 10]]**

[化简]

$$2048 x (1+x)^5 (-46 + 21 x - 971 x^2 + 1647 x^3 - 5249 x^4 + 6783 x^5 - 3145 x^6 - 1271 x^7 + 4655 x^8 - 2668 x^9 + 244 x^{10})$$

**Simplify[Cf[9, 4, 11]]**

[化简]

$$2048 x (1+x)^5 (-142 + 425 x - 3690 x^2 + 8601 x^3 - 21990 x^4 + 31475 x^5 - 28610 x^6 + 17979 x^7 - 2788 x^8 - 648 x^9 - 732 x^{10} + 120 x^{11})$$

**Simplify[Cf[9, 4, 12]]**

[化简]

$$2048 x (1+x)^5 (-142 + 425 x - 3690 x^2 + 8601 x^3 - 21990 x^4 + 31475 x^5 - 28610 x^6 + 17979 x^7 - 2788 x^8 - 648 x^9 - 732 x^{10} + 120 x^{11})$$

**Simplify[Cf[9, 4, 13]]**

[化简]

$$2048 x (1+x)^5 (-46 + 21 x - 971 x^2 + 1647 x^3 - 5249 x^4 + 6783 x^5 - 3145 x^6 - 1271 x^7 + 4655 x^8 - 2668 x^9 + 244 x^{10})$$

**Simplify[Cf[9, 4, 14]]**

[化简]

$$4096 x^2 (1+x)^5 (-11 - 106 x + 299 x^2 - 1048 x^3 + 2055 x^4 - 2338 x^5 + 1613 x^6 - 476 x^7 + 12 x^8)$$

(\*, r2^9r3^5\*)

**Simplify[Cf[9, 5, 0]]**

[化简]

0

**Simplify[Cf[9, 5, 1]]**

[化简]

0

**Simplify[Cf[9, 5, 2]]**

[化简]

0

**Simplify[Cf[9, 5, 3]]**

[化简]

0

**Simplify[Cf[9, 5, 4]]**

[化简]

0

**Simplify[Cf[9, 5, 5]]**

[化简]

0

**Simplify[Cf[9, 5, 6]]**

[化简]

0

**Simplify[Cf[9, 5, 7]]**

[化简]

0

**Simplify[Cf[9, 5, 8]]**

[化简]

$$-4096 x^2 (1+x)^5 (23+98 x+26 x^2+194 x^3-51 x^4-384 x^5+674 x^6-540 x^7+104 x^8)$$

**Simplify[Cf[9, 5, 9]]**

[化简]

$$-8192 x^2 (1+x)^5 (279-1252 x+5397 x^2-10826 x^3+16897 x^4-16812 x^5+10319 x^6-3486 x^7-156 x^8+216 x^9)$$

**Simplify[Cf[9, 5, 10]]**

[化简]

$$-2048 x (1+x)^5 (368-1398 x+9883 x^2-17514 x^3+44189 x^4-58954 x^5+85081 x^6-92946 x^7+62287 x^8-29148 x^9+4128 x^{10}+648 x^{11})$$

**Simplify[Cf[9, 5, 11]]**

[化简]

$$-8192 x^2 (1+x)^5 (1015-4761 x+20474 x^2-42830 x^3+70527 x^4-75961 x^5+60448 x^6-38664 x^7+16928 x^8-6072 x^9+1200 x^{10})$$

**Simplify[Cf[9, 5, 12]]**

[化简]

$$-2048 x (1+x)^5 (368 - 1398 x + 9883 x^2 - 17514 x^3 + 44189 x^4 - 58954 x^5 + 85081 x^6 - 92946 x^7 + 62287 x^8 - 29148 x^9 + 4128 x^{10} + 648 x^{11})$$

**Simplify[Cf[9, 5, 13]]**

[化简]

$$-8192 x^2 (1+x)^5 (279 - 1252 x + 5397 x^2 - 10826 x^3 + 16897 x^4 - 16812 x^5 + 10319 x^6 - 3486 x^7 - 156 x^8 + 216 x^9)$$

**Simplify[Cf[9, 5, 14]]**

[化简]

$$-4096 x^2 (1+x)^5 (23 + 98 x + 26 x^2 + 194 x^3 - 51 x^4 - 384 x^5 + 674 x^6 - 540 x^7 + 104 x^8)$$

(\*, r2^9r3^6\*)

**Simplify[Cf[9, 6, 0]]**

[化简]

0

**Simplify[Cf[9, 6, 1]]**

[化简]

0

**Simplify[Cf[9, 6, 2]]**

[化简]

0

**Simplify[Cf[9, 6, 3]]**

[化简]

0

**Simplify[Cf[9, 6, 4]]**

[化简]

0

**Simplify[Cf[9, 6, 5]]**

[化简]

0

**Simplify[Cf[9, 6, 6]]**

[化简]

0

**Simplify[Cf[9, 6, 7]]**

[化简]

$$2048 x^2 (1+x)^5 (-49 - 363 x + 500 x^2 - 2542 x^3 + 3875 x^4 - 3919 x^5 + 2046 x^6 - 520 x^7 + 108 x^8)$$

**Simplify[Cf[9, 6, 8]]**

[化简]

$$2048 x (1+x)^5 (-108 - 12 x - 3006 x^2 + 5481 x^3 - 23953 x^4 + 31960 x^5 - 38556 x^6 + 27749 x^7 - 12817 x^8 + 2438 x^9 + 840 x^{10})$$



**Simplify[Cf[9, 6, 9]]**

[化简]

$$4096 x (1+x)^5 (-258 + 722 x - 6933 x^2 + 12092 x^3 - 38987 x^4 + 44434 x^5 - 55507 x^6 + 31712 x^7 - 7683 x^8 - 2296 x^9 + 2904 x^{10} + 216 x^{11})$$

**Simplify[Cf[9, 6, 10]]**

[化简]

$$2048 x (1+x)^5 (-648 + 1015 x - 19296 x^2 + 35793 x^3 - 134342 x^4 + 163415 x^5 - 221688 x^6 + 152143 x^7 - 93386 x^8 + 54714 x^9 - 17376 x^{10} + 6024 x^{11})$$

**Simplify[Cf[9, 6, 11]]**

[化简]

$$2048 x (1+x)^5 (-648 + 1015 x - 19296 x^2 + 35793 x^3 - 134342 x^4 + 163415 x^5 - 221688 x^6 + 152143 x^7 - 93386 x^8 + 54714 x^9 - 17376 x^{10} + 6024 x^{11})$$

**Simplify[Cf[9, 6, 12]]**

[化简]

$$4096 x (1+x)^5 (-258 + 722 x - 6933 x^2 + 12092 x^3 - 38987 x^4 + 44434 x^5 - 55507 x^6 + 31712 x^7 - 7683 x^8 - 2296 x^9 + 2904 x^{10} + 216 x^{11})$$

**Simplify[Cf[9, 6, 13]]**

[化简]

$$2048 x (1+x)^5 (-108 - 12 x - 3006 x^2 + 5481 x^3 - 23953 x^4 + 31960 x^5 - 38556 x^6 + 27749 x^7 - 12817 x^8 + 2438 x^9 + 840 x^{10})$$

**Simplify[Cf[9, 6, 14]]**

[化简]

$$2048 x^2 (1+x)^5 (-49 - 363 x + 500 x^2 - 2542 x^3 + 3875 x^4 - 3919 x^5 + 2046 x^6 - 520 x^7 + 108 x^8)$$

**(\*, r2^9r3^7\*)****Simplify[Cf[9, 7, 0]]**

[化简]

0

**Simplify[Cf[9, 7, 1]]**

[化简]

0

**Simplify[Cf[9, 7, 2]]**

[化简]

0

**Simplify[Cf[9, 7, 3]]**

[化简]

0

**Simplify[Cf[9, 7, 4]]**

[化简]

0

**Simplify[Cf[9, 7, 5]]**

[化简]

0

**Simplify[Cf[9, 7, 6]]**

[化简]

$$2048 x^2 (1+x)^5 (-49 - 363 x + 500 x^2 - 2542 x^3 + 3875 x^4 - 3919 x^5 + 2046 x^6 - 520 x^7 + 108 x^8)$$

**Simplify[Cf[9, 7, 7]]**

[化简]

$$-8192 x^2 (1+x)^5 (442 - 1939 x + 8752 x^2 - 17217 x^3 + 28770 x^4 - 28765 x^5 + 20384 x^6 - 8115 x^7 + 1364 x^8 + 164 x^9)$$

**Simplify[Cf[9, 7, 8]]**

[化简]

$$-2048 x (1+x)^5 (688 - 2146 x + 18920 x^2 - 30213 x^3 + 98031 x^4 - 105466 x^5 + 166870 x^6 - 122025 x^7 + 79547 x^8 - 24214 x^9 + 4344 x^{10} + 48 x^{11})$$

**Simplify[Cf[9, 7, 9]]**

[化简]

$$-8192 x^2 (1+x)^5 (2970 - 13299 x + 61532 x^2 - 120459 x^3 + 216260 x^4 - 218797 x^5 + 199684 x^6 - 115401 x^7 + 54586 x^8 - 15068 x^9 + 1464 x^{10})$$

**Simplify[Cf[9, 7, 10]]**

[化简]

$$4096 x (1+x)^5 (-702 + 2041 x - 21456 x^2 + 32433 x^3 - 121166 x^4 + 130121 x^5 - 240420 x^6 + 179135 x^7 - 144600 x^8 + 47206 x^9 - 8872 x^{10} + 2280 x^{11})$$

**Simplify[Cf[9, 7, 11]]**

[化简]

$$-8192 x^2 (1+x)^5 (2970 - 13299 x + 61532 x^2 - 120459 x^3 + 216260 x^4 - 218797 x^5 + 199684 x^6 - 115401 x^7 + 54586 x^8 - 15068 x^9 + 1464 x^{10})$$

**Simplify[Cf[9, 7, 12]]**

[化简]

$$-2048 x (1+x)^5 (688 - 2146 x + 18920 x^2 - 30213 x^3 + 98031 x^4 - 105466 x^5 + 166870 x^6 - 122025 x^7 + 79547 x^8 - 24214 x^9 + 4344 x^{10} + 48 x^{11})$$

**Simplify[Cf[9, 7, 13]]**

[化简]

$$-8192 x^2 (1+x)^5 (442 - 1939 x + 8752 x^2 - 17217 x^3 + 28770 x^4 - 28765 x^5 + 20384 x^6 - 8115 x^7 + 1364 x^8 + 164 x^9)$$

**Simplify[Cf[9, 7, 14]]**

[化简]

$$2048 x^2 (1+x)^5 (-49 - 363 x + 500 x^2 - 2542 x^3 + 3875 x^4 - 3919 x^5 + 2046 x^6 - 520 x^7 + 108 x^8)$$

(\*, r2^9r3^8\*)

**Simplify[Cf[9, 8, 0]]**

[化简]

0

**Simplify[Cf[9, 8, 1]]**

[化简]

0

**Simplify[Cf[9, 8, 2]]**

[化简]

0

**Simplify[Cf[9, 8, 3]]**

[化简]

0

**Simplify[Cf[9, 8, 4]]**

[化简]

0

**Simplify[Cf[9, 8, 5]]**

[化简]

$$-4096 x^2 (1+x)^5 (23+98 x+26 x^2+194 x^3-51 x^4-384 x^5+674 x^6-540 x^7+104 x^8)$$

**Simplify[Cf[9, 8, 6]]**

[化简]

$$2048 x (1+x)^5 (-108-12 x-3006 x^2+5481 x^3-23953 x^4+31960 x^5-38556 x^6+27749 x^7-12817 x^8+2438 x^9+840 x^{10})$$

**Simplify[Cf[9, 8, 7]]**

[化简]

$$-2048 x (1+x)^5 (688-2146 x+18920 x^2-30213 x^3+98031 x^4-105466 x^5+166870 x^6-122025 x^7+79547 x^8-24214 x^9+4344 x^{10}+48 x^{11})$$

**Simplify[Cf[9, 8, 8]]**

[化简]

$$4096 x (1+x)^5 (-506+573 x-16189 x^2+28202 x^3-122602 x^4+136419 x^5-225173 x^6+140452 x^7-121230 x^8+50018 x^9-21356 x^{10}+1920 x^{11})$$

**Simplify[Cf[9, 8, 9]]**

[化简]

$$8192 x (1+x)^5 (-410+870 x-12862 x^2+19133 x^3-83657 x^4+81396 x^5-153656 x^6+82967 x^7-76651 x^8+15660 x^9-8444 x^{10}+102 x^{11})$$

**Simplify[Cf[9, 8, 10]]**

[化简]

$$8192 x (1+x)^5 (-410+870 x-12862 x^2+19133 x^3-83657 x^4+81396 x^5-153656 x^6+82967 x^7-76651 x^8+15660 x^9-8444 x^{10}+102 x^{11})$$

**Simplify[Cf[9, 8, 11]]**

[化简]

$$4096 x (1+x)^5 (-506 + 573 x - 16189 x^2 + 28202 x^3 - 122602 x^4 + 136419 x^5 - 225173 x^6 + 140452 x^7 - 121230 x^8 + 50018 x^9 - 21356 x^{10} + 1920 x^{11})$$

**Simplify[Cf[9, 8, 12]]**

[化简]

$$-2048 x (1+x)^5 (688 - 2146 x + 18920 x^2 - 30213 x^3 + 98031 x^4 - 105466 x^5 + 166870 x^6 - 122025 x^7 + 79547 x^8 - 24214 x^9 + 4344 x^{10} + 48 x^{11})$$

**Simplify[Cf[9, 8, 13]]**

[化简]

$$2048 x (1+x)^5 (-108 - 12 x - 3006 x^2 + 5481 x^3 - 23953 x^4 + 31960 x^5 - 38556 x^6 + 27749 x^7 - 12817 x^8 + 2438 x^9 + 840 x^{10})$$

**Simplify[Cf[9, 8, 14]]**

[化简]

$$-4096 x^2 (1+x)^5 (23 + 98 x + 26 x^2 + 194 x^3 - 51 x^4 - 384 x^5 + 674 x^6 - 540 x^7 + 104 x^8)$$

**(\*, r2^9r3^9\*)****Simplify[Cf[9, 9, 0]]**

[化简]

0

**Simplify[Cf[9, 9, 1]]**

[化简]

0

**Simplify[Cf[9, 9, 2]]**

[化简]

0

**Simplify[Cf[9, 9, 3]]**

[化简]

0

**Simplify[Cf[9, 9, 4]]**

[化简]

$$4096 x^2 (1+x)^5 (-11 - 106 x + 299 x^2 - 1048 x^3 + 2055 x^4 - 2338 x^5 + 1613 x^6 - 476 x^7 + 12 x^8)$$

**Simplify[Cf[9, 9, 5]]**

[化简]

$$-8192 x^2 (1+x)^5 (279 - 1252 x + 5397 x^2 - 10826 x^3 + 16897 x^4 - 16812 x^5 + 10319 x^6 - 3486 x^7 - 156 x^8 + 216 x^9)$$

**Simplify[Cf[9, 9, 6]]**

[化简]

$$4096 x (1+x)^5 (-258 + 722 x - 6933 x^2 + 12092 x^3 - 38987 x^4 + 44434 x^5 - 55507 x^6 + 31712 x^7 - 7683 x^8 - 2296 x^9 + 2904 x^{10} + 216 x^{11})$$

**Simplify[Cf[9, 9, 7]]**

[化简]

$$-8192 x^2 (1+x)^5 (2970 - 13299 x + 61532 x^2 - 120459 x^3 + 216260 x^4 - 218797 x^5 + 199684 x^6 - 115401 x^7 + 54586 x^8 - 15068 x^9 + 1464 x^{10})$$

**Simplify[Cf[9, 9, 8]]**

[化简]

$$8192 x (1+x)^5 (-410 + 870 x - 12862 x^2 + 19133 x^3 - 83657 x^4 + 81396 x^5 - 153656 x^6 + 82967 x^7 - 76651 x^8 + 15660 x^9 - 8444 x^{10} + 102 x^{11})$$

**Simplify[Cf[9, 9, 9]]**

[化简]

$$-24576 x^2 (1+x)^5 (1841 - 8122 x + 38987 x^2 - 73344 x^3 + 139539 x^4 - 135874 x^5 + 137573 x^6 - 73684 x^7 + 39276 x^8 - 6480 x^9 + 1152 x^{10})$$

**Simplify[Cf[9, 9, 10]]**

[化简]

$$8192 x (1+x)^5 (-410 + 870 x - 12862 x^2 + 19133 x^3 - 83657 x^4 + 81396 x^5 - 153656 x^6 + 82967 x^7 - 76651 x^8 + 15660 x^9 - 8444 x^{10} + 102 x^{11})$$

**Simplify[Cf[9, 9, 11]]**

[化简]

$$-8192 x^2 (1+x)^5 (2970 - 13299 x + 61532 x^2 - 120459 x^3 + 216260 x^4 - 218797 x^5 + 199684 x^6 - 115401 x^7 + 54586 x^8 - 15068 x^9 + 1464 x^{10})$$

**Simplify[Cf[9, 9, 12]]**

[化简]

$$4096 x (1+x)^5 (-258 + 722 x - 6933 x^2 + 12092 x^3 - 38987 x^4 + 44434 x^5 - 55507 x^6 + 31712 x^7 - 7683 x^8 - 2296 x^9 + 2904 x^{10} + 216 x^{11})$$

**Simplify[Cf[9, 9, 13]]**

[化简]

$$-8192 x^2 (1+x)^5 (279 - 1252 x + 5397 x^2 - 10826 x^3 + 16897 x^4 - 16812 x^5 + 10319 x^6 - 3486 x^7 - 156 x^8 + 216 x^9)$$

**Simplify[Cf[9, 9, 14]]**

[化简]

$$4096 x^2 (1+x)^5 (-11 - 106 x + 299 x^2 - 1048 x^3 + 2055 x^4 - 2338 x^5 + 1613 x^6 - 476 x^7 + 12 x^8)$$

**(\*, r2^9r3^10\*)****Simplify[Cf[9, 10, 0]]**

[化简]

0

**Simplify[Cf[9, 10, 1]]**

[化简]

0

**Simplify[Cf[9, 10, 2]]**

[化简]

0

**Simplify[Cf[9, 10, 3]]**

[化简]

$$4096 (-1 + x)^2 x^2 (1 + x)^5 (-9 - 18x - 124x^2 + 82x^3 - 207x^4 + 4x^5 + 40x^6)$$

**Simplify[Cf[9, 10, 4]]**

[化简]

$$2048x(1+x)^5 (-46 + 21x - 971x^2 + 1647x^3 - 5249x^4 + 6783x^5 - 3145x^6 - 1271x^7 + 4655x^8 - 2668x^9 + 244x^{10})$$

**Simplify[Cf[9, 10, 5]]**

[化简]

$$-2048x(1+x)^5 (368 - 1398x + 9883x^2 - 17514x^3 + 44189x^4 - 58954x^5 + 85081x^6 - 92946x^7 + 62287x^8 - 29148x^9 + 4128x^{10} + 648x^{11})$$

**Simplify[Cf[9, 10, 6]]**

[化简]

$$2048x(1+x)^5 (-648 + 1015x - 19296x^2 + 35793x^3 - 134342x^4 + 163415x^5 - 221688x^6 + 152143x^7 - 93386x^8 + 54714x^9 - 17376x^{10} + 6024x^{11})$$

**Simplify[Cf[9, 10, 7]]**

[化简]

$$4096x(1+x)^5 (-702 + 2041x - 21456x^2 + 32433x^3 - 121166x^4 + 130121x^5 - 240420x^6 + 179135x^7 - 144600x^8 + 47206x^9 - 8872x^{10} + 2280x^{11})$$

**Simplify[Cf[9, 10, 8]]**

[化简]

$$8192x(1+x)^5 (-410 + 870x - 12862x^2 + 19133x^3 - 83657x^4 + 81396x^5 - 153656x^6 + 82967x^7 - 76651x^8 + 15660x^9 - 8444x^{10} + 102x^{11})$$

**Simplify[Cf[9, 10, 9]]**

[化简]

$$8192x(1+x)^5 (-410 + 870x - 12862x^2 + 19133x^3 - 83657x^4 + 81396x^5 - 153656x^6 + 82967x^7 - 76651x^8 + 15660x^9 - 8444x^{10} + 102x^{11})$$

**Simplify[Cf[9, 10, 10]]**

[化简]

$$4096x(1+x)^5 (-702 + 2041x - 21456x^2 + 32433x^3 - 121166x^4 + 130121x^5 - 240420x^6 + 179135x^7 - 144600x^8 + 47206x^9 - 8872x^{10} + 2280x^{11})$$

**Simplify[Cf[9, 10, 11]]**

[化简]

$$2048x(1+x)^5 (-648 + 1015x - 19296x^2 + 35793x^3 - 134342x^4 + 163415x^5 - 221688x^6 + 152143x^7 - 93386x^8 + 54714x^9 - 17376x^{10} + 6024x^{11})$$

**Simplify[Cf[9, 10, 12]]**

[化简]

$$-2048x(1+x)^5 (368 - 1398x + 9883x^2 - 17514x^3 + 44189x^4 - 58954x^5 + 85081x^6 - 92946x^7 + 62287x^8 - 29148x^9 + 4128x^{10} + 648x^{11})$$

**Simplify[Cf[9, 10, 13]]**

[化简]

$$2048 x (1+x)^5 (-46 + 21 x - 971 x^2 + 1647 x^3 - 5249 x^4 + 6783 x^5 - 3145 x^6 - 1271 x^7 + 4655 x^8 - 2668 x^9 + 244 x^{10})$$

**Simplify[Cf[9, 10, 14]]**

[化简]

$$4096 (-1+x)^2 x^2 (1+x)^5 (-9 - 18 x - 124 x^2 + 82 x^3 - 207 x^4 + 4 x^5 + 40 x^6)$$

(\*, r2^9r3^11\*)

**Simplify[Cf[9, 11, 0]]**

[化简]

0

**Simplify[Cf[9, 11, 1]]**

[化简]

0

**Simplify[Cf[9, 11, 2]]**

[化简]

$$-2048 (-1+x)^3 x^2 (1+x)^5 (-3 - 44 x + 37 x^2 - 182 x^3 + 60 x^4)$$

**Simplify[Cf[9, 11, 3]]**

[化简]

$$4096 (-1+x)^2 x^2 (1+x)^5 (-120 + 337 x - 1408 x^2 + 1558 x^3 - 2044 x^4 + 597 x^5 + 4 x^6 + 36 x^7)$$

**Simplify[Cf[9, 11, 4]]**

[化简]

$$2048 x (1+x)^5 (-142 + 425 x - 3690 x^2 + 8601 x^3 - 21990 x^4 + 31475 x^5 - 28610 x^6 + 17979 x^7 - 2788 x^8 - 648 x^9 - 732 x^{10} + 120 x^{11})$$

**Simplify[Cf[9, 11, 5]]**

[化简]

$$-8192 x^2 (1+x)^5 (1015 - 4761 x + 20474 x^2 - 42830 x^3 + 70527 x^4 - 75961 x^5 + 60448 x^6 - 38664 x^7 + 16928 x^8 - 6072 x^9 + 1200 x^{10})$$

**Simplify[Cf[9, 11, 6]]**

[化简]

$$2048 x (1+x)^5 (-648 + 1015 x - 19296 x^2 + 35793 x^3 - 134342 x^4 + 163415 x^5 - 221688 x^6 + 152143 x^7 - 93386 x^8 + 54714 x^9 - 17376 x^{10} + 6024 x^{11})$$

**Simplify[Cf[9, 11, 7]]**

[化简]

$$-8192 x^2 (1+x)^5 (2970 - 13299 x + 61532 x^2 - 120459 x^3 + 216260 x^4 - 218797 x^5 + 199684 x^6 - 115401 x^7 + 54586 x^8 - 15068 x^9 + 1464 x^{10})$$

**Simplify[Cf[9, 11, 8]]**

[化简]

$$4096 x (1+x)^5 (-506 + 573 x - 16189 x^2 + 28202 x^3 - 122602 x^4 + 136419 x^5 - 225173 x^6 + 140452 x^7 - 121230 x^8 + 50018 x^9 - 21356 x^{10} + 1920 x^{11})$$

**Simplify[Cf[9, 11, 9]]**

[化简]

$$-8192 x^2 (1+x)^5 (2970 - 13299 x + 61532 x^2 - 120459 x^3 + 216260 x^4 - 218797 x^5 + 199684 x^6 - 115401 x^7 + 54586 x^8 - 15068 x^9 + 1464 x^{10})$$

**Simplify[Cf[9, 11, 10]]**

[化简]

$$2048 x (1+x)^5 (-648 + 1015 x - 19296 x^2 + 35793 x^3 - 134342 x^4 + 163415 x^5 - 221688 x^6 + 152143 x^7 - 93386 x^8 + 54714 x^9 - 17376 x^{10} + 6024 x^{11})$$

**Simplify[Cf[9, 11, 11]]**

[化简]

$$-8192 x^2 (1+x)^5 (1015 - 4761 x + 20474 x^2 - 42830 x^3 + 70527 x^4 - 75961 x^5 + 60448 x^6 - 38664 x^7 + 16928 x^8 - 6072 x^9 + 1200 x^{10})$$

**Simplify[Cf[9, 11, 12]]**

[化简]

$$2048 x (1+x)^5 (-142 + 425 x - 3690 x^2 + 8601 x^3 - 21990 x^4 + 31475 x^5 - 28610 x^6 + 17979 x^7 - 2788 x^8 - 648 x^9 - 732 x^{10} + 120 x^{11})$$

**Simplify[Cf[9, 11, 13]]**

[化简]

$$4096 (-1+x)^2 x^2 (1+x)^5 (-120 + 337 x - 1408 x^2 + 1558 x^3 - 2044 x^4 + 597 x^5 + 4 x^6 + 36 x^7)$$

**Simplify[Cf[9, 11, 14]]**

[化简]

$$-2048 (-1+x)^3 x^2 (1+x)^5 (-3 - 44 x + 37 x^2 - 182 x^3 + 60 x^4)$$

**(\*, r2^9r3^12\*)****Simplify[Cf[9, 12, 0]]**

[化简]

0

**Simplify[Cf[9, 12, 1]]**

[化简]

$$-2048 (-1+x)^4 x^2 (1+x)^5 (2 - 3 x + 30 x^2 - 21 x^3 + 4 x^4)$$

**Simplify[Cf[9, 12, 2]]**

[化简]

$$2048 (-1+x)^3 x (1+x)^5 (6 + 7 x + 89 x^2 + 50 x^3 + 225 x^4 + 197 x^5 - 190 x^6 + 36 x^7)$$

**Simplify[Cf[9, 12, 3]]**

[化简]

$$4096 (-1+x)^2 x (1+x)^5 (-30 + 78 x - 535 x^2 + 314 x^3 - 1370 x^4 + 916 x^5 - 2281 x^6 + 1676 x^7 - 456 x^8 + 72 x^9)$$

**Simplify[Cf[9, 12, 4]]**

[化简]

$$2048 x (1+x)^5 (-142 + 425 x - 3690 x^2 + 8601 x^3 - 21990 x^4 + 31475 x^5 - 28610 x^6 + 17979 x^7 - 2788 x^8 - 648 x^9 - 732 x^{10} + 120 x^{11})$$



**Simplify[Cf[9, 12, 5]]**

|化简

$$-2048 x (1+x)^5 (368 - 1398 x + 9883 x^2 - 17514 x^3 + 44189 x^4 - 58954 x^5 + 85081 x^6 - 92946 x^7 + 62287 x^8 - 29148 x^9 + 4128 x^{10} + 648 x^{11})$$

**Simplify[Cf[9, 12, 6]]**

|化简

$$4096 x (1+x)^5 (-258 + 722 x - 6933 x^2 + 12092 x^3 - 38987 x^4 + 44434 x^5 - 55507 x^6 + 31712 x^7 - 7683 x^8 - 2296 x^9 + 2904 x^{10} + 216 x^{11})$$

**Simplify[Cf[9, 12, 7]]**

|化简

$$-2048 x (1+x)^5 (688 - 2146 x + 18920 x^2 - 30213 x^3 + 98031 x^4 - 105466 x^5 + 166870 x^6 - 122025 x^7 + 79547 x^8 - 24214 x^9 + 4344 x^{10} + 48 x^{11})$$

**Simplify[Cf[9, 12, 8]]**

|化简

$$-2048 x (1+x)^5 (688 - 2146 x + 18920 x^2 - 30213 x^3 + 98031 x^4 - 105466 x^5 + 166870 x^6 - 122025 x^7 + 79547 x^8 - 24214 x^9 + 4344 x^{10} + 48 x^{11})$$

**Simplify[Cf[9, 12, 9]]**

|化简

$$4096 x (1+x)^5 (-258 + 722 x - 6933 x^2 + 12092 x^3 - 38987 x^4 + 44434 x^5 - 55507 x^6 + 31712 x^7 - 7683 x^8 - 2296 x^9 + 2904 x^{10} + 216 x^{11})$$

**Simplify[Cf[9, 12, 10]]**

|化简

$$-2048 x (1+x)^5 (368 - 1398 x + 9883 x^2 - 17514 x^3 + 44189 x^4 - 58954 x^5 + 85081 x^6 - 92946 x^7 + 62287 x^8 - 29148 x^9 + 4128 x^{10} + 648 x^{11})$$

**Simplify[Cf[9, 12, 11]]**

|化简

$$2048 x (1+x)^5 (-142 + 425 x - 3690 x^2 + 8601 x^3 - 21990 x^4 + 31475 x^5 - 28610 x^6 + 17979 x^7 - 2788 x^8 - 648 x^9 - 732 x^{10} + 120 x^{11})$$

**Simplify[Cf[9, 12, 12]]**

|化简

$$4096 (-1+x)^2 x (1+x)^5 (-30 + 78 x - 535 x^2 + 314 x^3 - 1370 x^4 + 916 x^5 - 2281 x^6 + 1676 x^7 - 456 x^8 + 72 x^9)$$

**Simplify[Cf[9, 12, 13]]**

|化简

$$2048 (-1+x)^3 x (1+x)^5 (6 + 7 x + 89 x^2 + 50 x^3 + 225 x^4 + 197 x^5 - 190 x^6 + 36 x^7)$$

**Simplify[Cf[9, 12, 14]]**

|化简

$$-2048 (-1+x)^4 x^2 (1+x)^5 (2 - 3 x + 30 x^2 - 21 x^3 + 4 x^4)$$

**(\*, r2^9r3^13\*)**

**Simplify[Cf[9, 13, 0]]**

[化简]

$$-2048 (-1+x)^6 x^3 (1+x)^5$$

**Simplify[Cf[9, 13, 1]]**

[化简]

$$8192 (-1+x)^4 x^2 (1+x)^5 (-2+3x-13x^2+6x^3)$$

**Simplify[Cf[9, 13, 2]]**

[化简]

$$2048 (-1+x)^3 x (1+x)^5 (6+7x+89x^2+50x^3+225x^4+197x^5-190x^6+36x^7)$$

**Simplify[Cf[9, 13, 3]]**

[化简]

$$4096 (-1+x)^2 x^2 (1+x)^5 (-120+337x-1408x^2+1558x^3-2044x^4+597x^5+4x^6+36x^7)$$

**Simplify[Cf[9, 13, 4]]**

[化简]

$$2048 x (1+x)^5 (-46+21x-971x^2+1647x^3-5249x^4+6783x^5-3145x^6-1271x^7+4655x^8-2668x^9+244x^{10})$$

**Simplify[Cf[9, 13, 5]]**

[化简]

$$-8192 x^2 (1+x)^5 (279-1252x+5397x^2-10826x^3+16897x^4-16812x^5+10319x^6-3486x^7-156x^8+216x^9)$$

**Simplify[Cf[9, 13, 6]]**

[化简]

$$2048 x (1+x)^5 (-108-12x-3006x^2+5481x^3-23953x^4+31960x^5-38556x^6+27749x^7-12817x^8+2438x^9+840x^{10})$$

**Simplify[Cf[9, 13, 7]]**

[化简]

$$-8192 x^2 (1+x)^5 (442-1939x+8752x^2-17217x^3+28770x^4-28765x^5+20384x^6-8115x^7+1364x^8+164x^9)$$

**Simplify[Cf[9, 13, 8]]**

[化简]

$$2048 x (1+x)^5 (-108-12x-3006x^2+5481x^3-23953x^4+31960x^5-38556x^6+27749x^7-12817x^8+2438x^9+840x^{10})$$

**Simplify[Cf[9, 13, 9]]**

[化简]

$$-8192 x^2 (1+x)^5 (279-1252x+5397x^2-10826x^3+16897x^4-16812x^5+10319x^6-3486x^7-156x^8+216x^9)$$

**Simplify[Cf[9, 13, 10]]**

[化简]

$$2048 x (1+x)^5 (-46+21x-971x^2+1647x^3-5249x^4+6783x^5-3145x^6-1271x^7+4655x^8-2668x^9+244x^{10})$$

**Simplify[Cf[9, 13, 11]]**

[\[化简\]](#)

$$4096 (-1+x)^2 x^2 (1+x)^5 (-120+337x-1408x^2+1558x^3-2044x^4+597x^5+4x^6+36x^7)$$

**Simplify[Cf[9, 13, 12]]**

[\[化简\]](#)

$$2048 (-1+x)^3 x (1+x)^5 (6+7x+89x^2+50x^3+225x^4+197x^5-190x^6+36x^7)$$

**Simplify[Cf[9, 13, 13]]**

[\[化简\]](#)

$$8192 (-1+x)^4 x^2 (1+x)^5 (-2+3x-13x^2+6x^3)$$

**Simplify[Cf[9, 13, 14]]**

[\[化简\]](#)

$$-2048 (-1+x)^6 x^3 (1+x)^5$$

**(\*, r2^9r3^14\*)**

**Simplify[Cf[9, 14, 0]]**

[\[化简\]](#)

$$-2048 (-1+x)^6 x^3 (1+x)^5$$

**Simplify[Cf[9, 14, 1]]**

[\[化简\]](#)

$$-2048 (-1+x)^4 x^2 (1+x)^5 (2-3x+30x^2-21x^3+4x^4)$$

**Simplify[Cf[9, 14, 2]]**

[\[化简\]](#)

$$-2048 (-1+x)^3 x^2 (1+x)^5 (-3-44x+37x^2-182x^3+60x^4)$$

**Simplify[Cf[9, 14, 3]]**

[\[化简\]](#)

$$4096 (-1+x)^2 x^2 (1+x)^5 (-9-18x-124x^2+82x^3-207x^4+4x^5+40x^6)$$

**Simplify[Cf[9, 14, 4]]**

[\[化简\]](#)

$$4096 x^2 (1+x)^5 (-11-106x+299x^2-1048x^3+2055x^4-2338x^5+1613x^6-476x^7+12x^8)$$

**Simplify[Cf[9, 14, 5]]**

[\[化简\]](#)

$$-4096 x^2 (1+x)^5 (23+98x+26x^2+194x^3-51x^4-384x^5+674x^6-540x^7+104x^8)$$

**Simplify[Cf[9, 14, 6]]**

[\[化简\]](#)

$$2048 x^2 (1+x)^5 (-49-363x+500x^2-2542x^3+3875x^4-3919x^5+2046x^6-520x^7+108x^8)$$

**Simplify[Cf[9, 14, 7]]**

[\[化简\]](#)

$$2048 x^2 (1+x)^5 (-49-363x+500x^2-2542x^3+3875x^4-3919x^5+2046x^6-520x^7+108x^8)$$

**Simplify[Cf[9, 14, 8]]**

[\[化简\]](#)

$$-4096 x^2 (1+x)^5 (23+98 x+26 x^2+194 x^3-51 x^4-384 x^5+674 x^6-540 x^7+104 x^8)$$

**Simplify[Cf[9, 14, 9]]**

[\[化简\]](#)

$$4096 x^2 (1+x)^5 (-11-106 x+299 x^2-1048 x^3+2055 x^4-2338 x^5+1613 x^6-476 x^7+12 x^8)$$

**Simplify[Cf[9, 14, 10]]**

[\[化简\]](#)

$$4096 (-1+x)^2 x^2 (1+x)^5 (-9-18 x-124 x^2+82 x^3-207 x^4+4 x^5+40 x^6)$$

**Simplify[Cf[9, 14, 11]]**

[\[化简\]](#)

$$-2048 (-1+x)^3 x^2 (1+x)^5 (-3-44 x+37 x^2-182 x^3+60 x^4)$$

**Simplify[Cf[9, 14, 12]]**

[\[化简\]](#)

$$-2048 (-1+x)^4 x^2 (1+x)^5 (2-3 x+30 x^2-21 x^3+4 x^4)$$

**Simplify[Cf[9, 14, 13]]**

[\[化简\]](#)

$$-2048 (-1+x)^6 x^3 (1+x)^5$$

**Simplify[Cf[9, 14, 14]]**

[\[化简\]](#)

0

**(\*, r2^10r3^0\*)**

**Simplify[Cf[10, 0, 0]]**

[\[化简\]](#)

0

**Simplify[Cf[10, 0, 1]]**

[\[化简\]](#)

0

**Simplify[Cf[10, 0, 2]]**

[\[化简\]](#)

0

**Simplify[Cf[10, 0, 3]]**

[\[化简\]](#)

0

**Simplify[Cf[10, 0, 4]]**

[\[化简\]](#)

0

**Simplify[Cf[10, 0, 5]]**

[化简]

0

**Simplify[Cf[10, 0, 6]]**

[化简]

0

**Simplify[Cf[10, 0, 7]]**

[化简]

0

**Simplify[Cf[10, 0, 8]]**

[化简]

0

**Simplify[Cf[10, 0, 9]]**

[化简]

0

**Simplify[Cf[10, 0, 10]]**

[化简]

0

**Simplify[Cf[10, 0, 11]]**

[化简]

0

**Simplify[Cf[10, 0, 12]]**

[化简]

$4096 x^3 (-1 + x^2)^5$

**Simplify[Cf[10, 0, 13]]**

[化简]

$-4096 x^2 (-1 + x^2)^5 (-1 + x - 3 x^2 + x^3)$

**Simplify[Cf[10, 0, 14]]**

[化简]

$4096 x^3 (-1 + x^2)^5$

(\*, r2^10r3^1\*)

**Simplify[Cf[10, 1, 0]]**

[化简]

0

**Simplify[Cf[10, 1, 1]]**

[化简]

0

**Simplify[Cf[10, 1, 2]]**

[化简]

0

**Simplify[Cf[10, 1, 3]]**

[化简]

0

**Simplify[Cf[10, 1, 4]]**

[化简]

0

**Simplify[Cf[10, 1, 5]]**

[化简]

0

**Simplify[Cf[10, 1, 6]]**

[化简]

0

**Simplify[Cf[10, 1, 7]]**

[化简]

0

**Simplify[Cf[10, 1, 8]]**

[化简]

0

**Simplify[Cf[10, 1, 9]]**

[化简]

0

**Simplify[Cf[10, 1, 10]]**

[化简]

0

**Simplify[Cf[10, 1, 11]]**

[化简]

$$4096 (-1+x)^4 x^2 (1+x)^5 (-1-2x-11x^2-8x^3+2x^4)$$

**Simplify[Cf[10, 1, 12]]**

[化简]

$$-2048 (-1+x)^4 x (1+x)^5 (4-12x+75x^2-52x^3+165x^4-56x^5+8x^6)$$

**Simplify[Cf[10, 1, 13]]**

[化简]

$$-2048 (-1+x)^4 x (1+x)^5 (4-12x+75x^2-52x^3+165x^4-56x^5+8x^6)$$

**Simplify[Cf[10, 1, 14]]**

[化简]

$$4096 (-1+x)^4 x^2 (1+x)^5 (-1-2x-11x^2-8x^3+2x^4)$$

(\*, r2^10r3^2\*)

**Simplify[Cf[10, 2, 0]]**

[化简]

0

**Simplify[Cf[10, 2, 1]]**

[化简]

0

**Simplify[Cf[10, 2, 2]]**

[化简]

0

**Simplify[Cf[10, 2, 3]]**

[化简]

0

**Simplify[Cf[10, 2, 4]]**

[化简]

0

**Simplify[Cf[10, 2, 5]]**

[化简]

0

**Simplify[Cf[10, 2, 6]]**

[化简]

0

**Simplify[Cf[10, 2, 7]]**

[化简]

0

**Simplify[Cf[10, 2, 8]]**

[化简]

0

**Simplify[Cf[10, 2, 9]]**

[化简]

0

**Simplify[Cf[10, 2, 10]]**

[化简]

$-2048 (-1+x)^3 x^2 (1+x)^5 (-7-25x-57x^2-55x^3-116x^4+44x^5)$

**Simplify[Cf[10, 2, 11]]**

[化简]

$-2048 (-1+x)^3 x (1+x)^5 (-6-34x-84x^2-195x^3-332x^4-521x^5+92x^6+36x^7)$

**Simplify[Cf[10, 2, 12]]**

[化简]

$$-4096 (-1+x)^3 (1+x)^5 (-3+21x-131x^2+203x^3-650x^4+431x^5-1014x^6+363x^7-60x^8+12x^9)$$

**Simplify[Cf[10, 2, 13]]**

[化简]

$$-2048 (-1+x)^3 x (1+x)^5 (-6-34x-84x^2-195x^3-332x^4-521x^5+92x^6+36x^7)$$

**Simplify[Cf[10, 2, 14]]**

[化简]

$$-2048 (-1+x)^3 x^2 (1+x)^5 (-7-25x-57x^2-55x^3-116x^4+44x^5)$$

(\*, r2^10r3^3\*)

**Simplify[Cf[10, 3, 0]]**

[化简]

0

**Simplify[Cf[10, 3, 1]]**

[化简]

0

**Simplify[Cf[10, 3, 2]]**

[化简]

0

**Simplify[Cf[10, 3, 3]]**

[化简]

0

**Simplify[Cf[10, 3, 4]]**

[化简]

0

**Simplify[Cf[10, 3, 5]]**

[化简]

0

**Simplify[Cf[10, 3, 6]]**

[化简]

0

**Simplify[Cf[10, 3, 7]]**

[化简]

0

**Simplify[Cf[10, 3, 8]]**

[化简]

0



**Simplify[Cf[10, 3, 9]]**

[化简]

$$4096 (-1+x)^2 x^2 (1+x)^5 (-9-18x-124x^2+82x^3-207x^4+4x^5+40x^6)$$

**Simplify[Cf[10, 3, 10]]**

[化简]

$$-4096 (-1+x)^2 x (1+x)^5 (18-53x+523x^2-704x^3+2078x^4-1455x^5+1921x^6-772x^7+12x^8)$$

**Simplify[Cf[10, 3, 11]]**

[化简]

$$-2048 (-1+x)^2 x (1+x)^5 (78-134x+1447x^2-514x^3+4130x^4-744x^5+4349x^6-600x^7-1020x^8+144x^9)$$

**Simplify[Cf[10, 3, 12]]**

[化简]

$$-2048 (-1+x)^2 x (1+x)^5 (78-134x+1447x^2-514x^3+4130x^4-744x^5+4349x^6-600x^7-1020x^8+144x^9)$$

**Simplify[Cf[10, 3, 13]]**

[化简]

$$-4096 (-1+x)^2 x (1+x)^5 (18-53x+523x^2-704x^3+2078x^4-1455x^5+1921x^6-772x^7+12x^8)$$

**Simplify[Cf[10, 3, 14]]**

[化简]

$$4096 (-1+x)^2 x^2 (1+x)^5 (-9-18x-124x^2+82x^3-207x^4+4x^5+40x^6)$$

**(\*, r2^10r3^4\*)****Simplify[Cf[10, 4, 0]]**

[化简]

0

**Simplify[Cf[10, 4, 1]]**

[化简]

0

**Simplify[Cf[10, 4, 2]]**

[化简]

0

**Simplify[Cf[10, 4, 3]]**

[化简]

0

**Simplify[Cf[10, 4, 4]]**

[化简]

0

**Simplify[Cf[10, 4, 5]]**

[化简]

0

**Simplify[Cf[10, 4, 6]]**

[化简]

0

**Simplify[Cf[10, 4, 7]]**

[化简]

0

**Simplify[Cf[10, 4, 8]]**

[化简]

$$-1024 x^2 (1+x)^5 (67+2x+857x^2-2092x^3+3073x^4-3126x^5+1695x^6-736x^7+260x^8)$$

**Simplify[Cf[10, 4, 9]]**

[化简]

$$2048 x (1+x)^5 (-46+21x-971x^2+1647x^3-5249x^4+6783x^5-3145x^6-1271x^7+4655x^8-2668x^9+244x^{10})$$

**Simplify[Cf[10, 4, 10]]**

[化简]

$$2048 (1+x)^5 (-48+480x-3555x^2+11338x^3-33289x^4+62324x^5-98829x^6+119218x^7-99767x^8+59360x^9-17520x^{10}-240x^{11}+528x^{12})$$

**Simplify[Cf[10, 4, 11]]**

[化简]

$$2048 x (1+x)^5 (-168+195x-4460x^2+11547x^3-36566x^4+58823x^5-66584x^6+62229x^7-42638x^8+30574x^9-15664x^{10}+2712x^{11})$$

**Simplify[Cf[10, 4, 12]]**

[化简]

$$2048 (1+x)^5 (-48+480x-3555x^2+11338x^3-33289x^4+62324x^5-98829x^6+119218x^7-99767x^8+59360x^9-17520x^{10}-240x^{11}+528x^{12})$$

**Simplify[Cf[10, 4, 13]]**

[化简]

$$2048 x (1+x)^5 (-46+21x-971x^2+1647x^3-5249x^4+6783x^5-3145x^6-1271x^7+4655x^8-2668x^9+244x^{10})$$

**Simplify[Cf[10, 4, 14]]**

[化简]

$$-1024 x^2 (1+x)^5 (67+2x+857x^2-2092x^3+3073x^4-3126x^5+1695x^6-736x^7+260x^8)$$

**(\*, r2^10r3^5\*)****Simplify[Cf[10, 5, 0]]**

[化简]

0

**Simplify[Cf[10, 5, 1]]**

[化简]

0

**Simplify[Cf[10, 5, 2]]**

[化简]

0

**Simplify[Cf[10, 5, 3]]**

[化简]

0

**Simplify[Cf[10, 5, 4]]**

[化简]

0

**Simplify[Cf[10, 5, 5]]**

[化简]

0

**Simplify[Cf[10, 5, 6]]**

[化简]

0

**Simplify[Cf[10, 5, 7]]**

[化简]

$$2048 x^2 (1+x)^5 (-45 - 33 x - 508 x^2 + 870 x^3 - 773 x^4 - 265 x^5 + 1450 x^6 - 1100 x^7 + 308 x^8)$$

**Simplify[Cf[10, 5, 8]]**

[化简]

$$-2048 x (1+x)^5 (94 - 303 x + 3119 x^2 - 6866 x^3 + 17814 x^4 - 22905 x^5 + 21615 x^6 - 15272 x^7 + 5986 x^8 - 1982 x^9 + 236 x^{10})$$

**Simplify[Cf[10, 5, 9]]**

[化简]

$$-2048 x (1+x)^5 (368 - 1398 x + 9883 x^2 - 17514 x^3 + 44189 x^4 - 58954 x^5 + 85081 x^6 - 92946 x^7 + 62287 x^8 - 29148 x^9 + 4128 x^{10} + 648 x^{11})$$

**Simplify[Cf[10, 5, 10]]**

[化简]

$$-8192 x (1+x)^5 (120 - 360 x + 3492 x^2 - 6400 x^3 + 17918 x^4 - 21997 x^5 + 27966 x^6 - 23532 x^7 + 9060 x^8 - 1027 x^9 - 3428 x^{10} + 1404 x^{11})$$

**Simplify[Cf[10, 5, 11]]**

[化简]

$$-8192 x (1+x)^5 (120 - 360 x + 3492 x^2 - 6400 x^3 + 17918 x^4 - 21997 x^5 + 27966 x^6 - 23532 x^7 + 9060 x^8 - 1027 x^9 - 3428 x^{10} + 1404 x^{11})$$

**Simplify[Cf[10, 5, 12]]**

[化简]

$$-2048 x (1+x)^5 (368 - 1398 x + 9883 x^2 - 17514 x^3 + 44189 x^4 - 58954 x^5 + 85081 x^6 - 92946 x^7 + 62287 x^8 - 29148 x^9 + 4128 x^{10} + 648 x^{11})$$

**Simplify[Cf[10, 5, 13]]**

[化简]

$$-2048 x (1+x)^5 (94 - 303 x + 3119 x^2 - 6866 x^3 + 17814 x^4 - 22905 x^5 + 21615 x^6 - 15272 x^7 + 5986 x^8 - 1982 x^9 + 236 x^{10})$$

**Simplify[Cf[10, 5, 14]]**

[化简]

$$2048 x^2 (1+x)^5 (-45 - 33 x - 508 x^2 + 870 x^3 - 773 x^4 - 265 x^5 + 1450 x^6 - 1100 x^7 + 308 x^8)$$

(\*, r2^10r3^6\*)

**Simplify[Cf[10, 6, 0]]**

[化简]

0

**Simplify[Cf[10, 6, 1]]**

[化简]

0

**Simplify[Cf[10, 6, 2]]**

[化简]

0

**Simplify[Cf[10, 6, 3]]**

[化简]

0

**Simplify[Cf[10, 6, 4]]**

[化简]

0

**Simplify[Cf[10, 6, 5]]**

[化简]

0

**Simplify[Cf[10, 6, 6]]**

[化简]

$$-2048 x^2 (1+x)^5 (53 + 837 x^2 - 1888 x^3 + 3187 x^4 - 3528 x^5 + 2623 x^6 - 1528 x^7 + 436 x^8)$$

**Simplify[Cf[10, 6, 7]]**

[化简]

$$2048 x (1+x)^5 (-102 + 188 x - 2949 x^2 + 5328 x^3 - 16599 x^4 + 19224 x^5 - 17363 x^6 + 8556 x^7 - 391 x^8 - 560 x^9 + 60 x^{10})$$

**Simplify[Cf[10, 6, 8]]**

[化简]

$$1024 (1+x)^5 (-228 + 2280 x - 17657 x^2 + 55410 x^3 - 175923 x^4 + 316440 x^5 - 538591 x^6 + 605042 x^7 - 527289 x^8 + 312060 x^9 - 106312 x^{10} + 17792 x^{11} + 1104 x^{12})$$

**Simplify[Cf[10, 6, 9]]**

[化简]

$$2048 x (1+x)^5 (-648 + 1015 x - 19296 x^2 + 35793 x^3 - 134342 x^4 + 163415 x^5 - 221688 x^6 + 152143 x^7 - 93386 x^8 + 54714 x^9 - 17376 x^{10} + 6024 x^{11})$$

**Simplify[Cf[10, 6, 10]]**

[化简]

$$6144 (1+x)^5 (-78 + 780 x - 6133 x^2 + 18672 x^3 - 64249 x^4 + 119158 x^5 - 222889 x^6 + 256892 x^7 - 237145 x^8 + 136978 x^9 - 46442 x^{10} + 10496 x^{11} + 552 x^{12})$$

**Simplify[Cf[10, 6, 11]]**

[化简]

$$2048 x (1+x)^5 (-648 + 1015 x - 19296 x^2 + 35793 x^3 - 134342 x^4 + 163415 x^5 - 221688 x^6 + 152143 x^7 - 93386 x^8 + 54714 x^9 - 17376 x^{10} + 6024 x^{11})$$

**Simplify[Cf[10, 6, 12]]**

[化简]

$$1024 (1+x)^5 (-228 + 2280 x - 17657 x^2 + 55410 x^3 - 175923 x^4 + 316440 x^5 - 538591 x^6 + 605042 x^7 - 527289 x^8 + 312060 x^9 - 106312 x^{10} + 17792 x^{11} + 1104 x^{12})$$

**Simplify[Cf[10, 6, 13]]**

[化简]

$$2048 x (1+x)^5 (-102 + 188 x - 2949 x^2 + 5328 x^3 - 16599 x^4 + 19224 x^5 - 17363 x^6 + 8556 x^7 - 391 x^8 - 560 x^9 + 60 x^{10})$$

**Simplify[Cf[10, 6, 14]]**

[化简]

$$-2048 x^2 (1+x)^5 (53 + 837 x^2 - 1888 x^3 + 3187 x^4 - 3528 x^5 + 2623 x^6 - 1528 x^7 + 436 x^8)$$

**(\*, r2^10r3^7\*)****Simplify[Cf[10, 7, 0]]**

[化简]

0

**Simplify[Cf[10, 7, 1]]**

[化简]

0

**Simplify[Cf[10, 7, 2]]**

[化简]

0

**Simplify[Cf[10, 7, 3]]**

[化简]

0

**Simplify[Cf[10, 7, 4]]**

[化简]

0

**Simplify[Cf[10, 7, 5]]**

[化简]

$$2048 x^2 (1+x)^5 (-45 - 33 x - 508 x^2 + 870 x^3 - 773 x^4 - 265 x^5 + 1450 x^6 - 1100 x^7 + 308 x^8)$$

**Simplify[Cf[10, 7, 6]]**

[化简]

$$2048 x (1+x)^5 (-102 + 188 x - 2949 x^2 + 5328 x^3 - 16599 x^4 + 19224 x^5 - 17363 x^6 + 8556 x^7 - 391 x^8 - 560 x^9 + 60 x^{10})$$

**Simplify[Cf[10, 7, 7]]**

[化简]

$$-2048 x (1+x)^5 (588 - 2271 x + 16628 x^2 - 28673 x^3 + 79818 x^4 - 101037 x^5 + 162376 x^6 - 160663 x^7 + 117606 x^8 - 52908 x^9 + 10632 x^{10} + 528 x^{11})$$

**Simplify[Cf[10, 7, 8]]**

[化简]

$$-2048 x (1+x)^5 (888 - 1940 x + 27259 x^2 - 45307 x^3 + 164672 x^4 - 170926 x^5 + 259107 x^6 - 149199 x^7 + 94290 x^8 - 21764 x^9 - 3096 x^{10} + 2592 x^{11})$$

**Simplify[Cf[10, 7, 9]]**

[化简]

$$4096 x (1+x)^5 (-702 + 2041 x - 21456 x^2 + 32433 x^3 - 121166 x^4 + 130121 x^5 - 240420 x^6 + 179135 x^7 - 144600 x^8 + 47206 x^9 - 8872 x^{10} + 2280 x^{11})$$

**Simplify[Cf[10, 7, 10]]**

[化简]

$$4096 x (1+x)^5 (-702 + 2041 x - 21456 x^2 + 32433 x^3 - 121166 x^4 + 130121 x^5 - 240420 x^6 + 179135 x^7 - 144600 x^8 + 47206 x^9 - 8872 x^{10} + 2280 x^{11})$$

**Simplify[Cf[10, 7, 11]]**

[化简]

$$-2048 x (1+x)^5 (888 - 1940 x + 27259 x^2 - 45307 x^3 + 164672 x^4 - 170926 x^5 + 259107 x^6 - 149199 x^7 + 94290 x^8 - 21764 x^9 - 3096 x^{10} + 2592 x^{11})$$

**Simplify[Cf[10, 7, 12]]**

[化简]

$$-2048 x (1+x)^5 (588 - 2271 x + 16628 x^2 - 28673 x^3 + 79818 x^4 - 101037 x^5 + 162376 x^6 - 160663 x^7 + 117606 x^8 - 52908 x^9 + 10632 x^{10} + 528 x^{11})$$

**Simplify[Cf[10, 7, 13]]**

[化简]

$$2048 x (1+x)^5 (-102 + 188 x - 2949 x^2 + 5328 x^3 - 16599 x^4 + 19224 x^5 - 17363 x^6 + 8556 x^7 - 391 x^8 - 560 x^9 + 60 x^{10})$$

**Simplify[Cf[10, 7, 14]]**

[化简]

$$2048 x^2 (1+x)^5 (-45 - 33 x - 508 x^2 + 870 x^3 - 773 x^4 - 265 x^5 + 1450 x^6 - 1100 x^7 + 308 x^8)$$

**(\*, r2^10r3^8\*)**

**Simplify[Cf[10, 8, 0]]**

[化简]

0

**Simplify[Cf[10, 8, 1]]**

[化简]

0

**Simplify[Cf[10, 8, 2]]**

[化简]

0

**Simplify[Cf[10, 8, 3]]**

[化简]

0

**Simplify[Cf[10, 8, 4]]**

[化简]

$$-1024 x^2 (1+x)^5 (67+2 x+857 x^2-2092 x^3+3073 x^4-3126 x^5+1695 x^6-736 x^7+260 x^8)$$

**Simplify[Cf[10, 8, 5]]**

[化简]

$$-2048 x (1+x)^5 (94-303 x+3119 x^2-6866 x^3+17814 x^4-22905 x^5+21615 x^6-15272 x^7+5986 x^8-1982 x^9+236 x^{10})$$

**Simplify[Cf[10, 8, 6]]**

[化简]

$$1024 (1+x)^5 (-228+2280 x-17657 x^2+55410 x^3-175923 x^4+316440 x^5-538591 x^6+605042 x^7-527289 x^8+312060 x^9-106312 x^{10}+17792 x^{11}+1104 x^{12})$$

**Simplify[Cf[10, 8, 7]]**

[化简]

$$-2048 x (1+x)^5 (888-1940 x+27259 x^2-45307 x^3+164672 x^4-170926 x^5+259107 x^6-149199 x^7+94290 x^8-21764 x^9-3096 x^{10}+2592 x^{11})$$

**Simplify[Cf[10, 8, 8]]**

[化简]

$$-4096 (1+x)^5 (186-1860 x+14925 x^2-44680 x^3+161887 x^4-293128 x^5+584285 x^6-635584 x^7+623747 x^8-322396 x^9+135154 x^{10}-26672 x^{11}+4776 x^{12})$$

**Simplify[Cf[10, 8, 9]]**

[化简]

$$8192 x (1+x)^5 (-410+870 x-12862 x^2+19133 x^3-83657 x^4+81396 x^5-153656 x^6+82967 x^7-76651 x^8+15660 x^9-8444 x^{10}+102 x^{11})$$

**Simplify[Cf[10, 8, 10]]**

[化简]

$$-4096 (1+x)^5 (186-1860 x+14925 x^2-44680 x^3+161887 x^4-293128 x^5+584285 x^6-635584 x^7+623747 x^8-322396 x^9+135154 x^{10}-26672 x^{11}+4776 x^{12})$$

**Simplify[Cf[10, 8, 11]]**

[化简]

$$-2048 x (1+x)^5 (888 - 1940 x + 27259 x^2 - 45307 x^3 + 164672 x^4 - 170926 x^5 + 259107 x^6 - 149199 x^7 + 94290 x^8 - 21764 x^9 - 3096 x^{10} + 2592 x^{11})$$

**Simplify[Cf[10, 8, 12]]**

[化简]

$$1024 (1+x)^5 (-228 + 2280 x - 17657 x^2 + 55410 x^3 - 175923 x^4 + 316440 x^5 - 538591 x^6 + 605042 x^7 - 527289 x^8 + 312060 x^9 - 106312 x^{10} + 17792 x^{11} + 1104 x^{12})$$

**Simplify[Cf[10, 8, 13]]**

[化简]

$$-2048 x (1+x)^5 (94 - 303 x + 3119 x^2 - 6866 x^3 + 17814 x^4 - 22905 x^5 + 21615 x^6 - 15272 x^7 + 5986 x^8 - 1982 x^9 + 236 x^{10})$$

**Simplify[Cf[10, 8, 14]]**

[化简]

$$-1024 x^2 (1+x)^5 (67 + 2 x + 857 x^2 - 2092 x^3 + 3073 x^4 - 3126 x^5 + 1695 x^6 - 736 x^7 + 260 x^8)$$

**(\*, r2^10r3^9\*)****Simplify[Cf[10, 9, 0]]**

[化简]

0

**Simplify[Cf[10, 9, 1]]**

[化简]

0

**Simplify[Cf[10, 9, 2]]**

[化简]

0

**Simplify[Cf[10, 9, 3]]**

[化简]

$$4096 (-1+x)^2 x^2 (1+x)^5 (-9 - 18 x - 124 x^2 + 82 x^3 - 207 x^4 + 4 x^5 + 40 x^6)$$

**Simplify[Cf[10, 9, 4]]**

[化简]

$$2048 x (1+x)^5 (-46 + 21 x - 971 x^2 + 1647 x^3 - 5249 x^4 + 6783 x^5 - 3145 x^6 - 1271 x^7 + 4655 x^8 - 2668 x^9 + 244 x^{10})$$

**Simplify[Cf[10, 9, 5]]**

[化简]

$$-2048 x (1+x)^5 (368 - 1398 x + 9883 x^2 - 17514 x^3 + 44189 x^4 - 58954 x^5 + 85081 x^6 - 92946 x^7 + 62287 x^8 - 29148 x^9 + 4128 x^{10} + 648 x^{11})$$

**Simplify[Cf[10, 9, 6]]**

[化简]

$$2048 x (1+x)^5 (-648 + 1015 x - 19296 x^2 + 35793 x^3 - 134342 x^4 + 163415 x^5 - 221688 x^6 + 152143 x^7 - 93386 x^8 + 54714 x^9 - 17376 x^{10} + 6024 x^{11})$$



**Simplify[Cf[10, 9, 7]]**

[\[化简\]](#)

$$4096 x (1+x)^5 (-702 + 2041 x - 21456 x^2 + 32433 x^3 - 121166 x^4 + 130121 x^5 - 240420 x^6 + 179135 x^7 - 144600 x^8 + 47206 x^9 - 8872 x^{10} + 2280 x^{11})$$

**Simplify[Cf[10, 9, 8]]**

[\[化简\]](#)

$$8192 x (1+x)^5 (-410 + 870 x - 12862 x^2 + 19133 x^3 - 83657 x^4 + 81396 x^5 - 153656 x^6 + 82967 x^7 - 76651 x^8 + 15660 x^9 - 8444 x^{10} + 102 x^{11})$$

**Simplify[Cf[10, 9, 9]]**

[\[化简\]](#)

$$8192 x (1+x)^5 (-410 + 870 x - 12862 x^2 + 19133 x^3 - 83657 x^4 + 81396 x^5 - 153656 x^6 + 82967 x^7 - 76651 x^8 + 15660 x^9 - 8444 x^{10} + 102 x^{11})$$

**Simplify[Cf[10, 9, 10]]**

[\[化简\]](#)

$$4096 x (1+x)^5 (-702 + 2041 x - 21456 x^2 + 32433 x^3 - 121166 x^4 + 130121 x^5 - 240420 x^6 + 179135 x^7 - 144600 x^8 + 47206 x^9 - 8872 x^{10} + 2280 x^{11})$$

**Simplify[Cf[10, 9, 11]]**

[\[化简\]](#)

$$2048 x (1+x)^5 (-648 + 1015 x - 19296 x^2 + 35793 x^3 - 134342 x^4 + 163415 x^5 - 221688 x^6 + 152143 x^7 - 93386 x^8 + 54714 x^9 - 17376 x^{10} + 6024 x^{11})$$

**Simplify[Cf[10, 9, 12]]**

[\[化简\]](#)

$$-2048 x (1+x)^5 (368 - 1398 x + 9883 x^2 - 17514 x^3 + 44189 x^4 - 58954 x^5 + 85081 x^6 - 92946 x^7 + 62287 x^8 - 29148 x^9 + 4128 x^{10} + 648 x^{11})$$

**Simplify[Cf[10, 9, 13]]**

[\[化简\]](#)

$$2048 x (1+x)^5 (-46 + 21 x - 971 x^2 + 1647 x^3 - 5249 x^4 + 6783 x^5 - 3145 x^6 - 1271 x^7 + 4655 x^8 - 2668 x^9 + 244 x^{10})$$

**Simplify[Cf[10, 9, 14]]**

[\[化简\]](#)

$$4096 (-1+x)^2 x^2 (1+x)^5 (-9 - 18 x - 124 x^2 + 82 x^3 - 207 x^4 + 4 x^5 + 40 x^6)$$

**(\*, r2^10r3^10\*)**

**Simplify[Cf[10, 10, 0]]**

[\[化简\]](#)

0

**Simplify[Cf[10, 10, 1]]**

[\[化简\]](#)

0

**Simplify[Cf[10, 10, 2]]**

[化简]

$$-2048 (-1+x)^3 x^2 (1+x)^5 (-7-25x-57x^2-55x^3-116x^4+44x^5)$$

**Simplify[Cf[10, 10, 3]]**

[化简]

$$-4096 (-1+x)^2 x (1+x)^5 (18-53x+523x^2-704x^3+2078x^4-1455x^5+1921x^6-772x^7+12x^8)$$

**Simplify[Cf[10, 10, 4]]**

[化简]

$$2048 (1+x)^5 (-48+480x-3555x^2+11338x^3-33289x^4+62324x^5-98829x^6+119218x^7-99767x^8+59360x^9-17520x^{10}-240x^{11}+528x^{12})$$

**Simplify[Cf[10, 10, 5]]**

[化简]

$$-8192 x (1+x)^5 (120-360x+3492x^2-6400x^3+17918x^4-21997x^5+27966x^6-23532x^7+9060x^8-1027x^9-3428x^{10}+1404x^{11})$$

**Simplify[Cf[10, 10, 6]]**

[化简]

$$6144 (1+x)^5 (-78+780x-6133x^2+18672x^3-64249x^4+119158x^5-222889x^6+256892x^7-237145x^8+136978x^9-46442x^{10}+10496x^{11}+552x^{12})$$

**Simplify[Cf[10, 10, 7]]**

[化简]

$$4096 x (1+x)^5 (-702+2041x-21456x^2+32433x^3-121166x^4+130121x^5-240420x^6+179135x^7-144600x^8+47206x^9-8872x^{10}+2280x^{11})$$

**Simplify[Cf[10, 10, 8]]**

[化简]

$$-4096 (1+x)^5 (186-1860x+14925x^2-44680x^3+161887x^4-293128x^5+584285x^6-635584x^7+623747x^8-322396x^9+135154x^{10}-26672x^{11}+4776x^{12})$$

**Simplify[Cf[10, 10, 9]]**

[化简]

$$4096 x (1+x)^5 (-702+2041x-21456x^2+32433x^3-121166x^4+130121x^5-240420x^6+179135x^7-144600x^8+47206x^9-8872x^{10}+2280x^{11})$$

**Simplify[Cf[10, 10, 10]]**

[化简]

$$6144 (1+x)^5 (-78+780x-6133x^2+18672x^3-64249x^4+119158x^5-222889x^6+256892x^7-237145x^8+136978x^9-46442x^{10}+10496x^{11}+552x^{12})$$

**Simplify[Cf[10, 10, 11]]**

[化简]

$$-8192 x (1+x)^5 (120-360x+3492x^2-6400x^3+17918x^4-21997x^5+27966x^6-23532x^7+9060x^8-1027x^9-3428x^{10}+1404x^{11})$$

**Simplify[Cf[10, 10, 12]]**

[化简]

$$2048 (1+x)^5 (-48 + 480x - 3555x^2 + 11338x^3 - 33289x^4 + 62324x^5 - 98829x^6 + 119218x^7 - 99767x^8 + 59360x^9 - 17520x^{10} - 240x^{11} + 528x^{12})$$

**Simplify[Cf[10, 10, 13]]**

[化简]

$$-4096 (-1+x)^2 x (1+x)^5 (18 - 53x + 523x^2 - 704x^3 + 2078x^4 - 1455x^5 + 1921x^6 - 772x^7 + 12x^8)$$

**Simplify[Cf[10, 10, 14]]**

[化简]

$$-2048 (-1+x)^3 x^2 (1+x)^5 (-7 - 25x - 57x^2 - 55x^3 - 116x^4 + 44x^5)$$

**(\*, r2^10r3^11\*)****Simplify[Cf[10, 11, 0]]**

[化简]

0

**Simplify[Cf[10, 11, 1]]**

[化简]

$$4096 (-1+x)^4 x^2 (1+x)^5 (-1 - 2x - 11x^2 - 8x^3 + 2x^4)$$

**Simplify[Cf[10, 11, 2]]**

[化简]

$$-2048 (-1+x)^3 x (1+x)^5 (-6 - 34x - 84x^2 - 195x^3 - 332x^4 - 521x^5 + 92x^6 + 36x^7)$$

**Simplify[Cf[10, 11, 3]]**

[化简]

$$-2048 (-1+x)^2 x (1+x)^5 (78 - 134x + 1447x^2 - 514x^3 + 4130x^4 - 744x^5 + 4349x^6 - 600x^7 - 1020x^8 + 144x^9)$$

**Simplify[Cf[10, 11, 4]]**

[化简]

$$2048 x (1+x)^5 (-168 + 195x - 4460x^2 + 11547x^3 - 36566x^4 + 58823x^5 - 66584x^6 + 62229x^7 - 42638x^8 + 30574x^9 - 15664x^{10} + 2712x^{11})$$

**Simplify[Cf[10, 11, 5]]**

[化简]

$$-8192 x (1+x)^5 (120 - 360x + 3492x^2 - 6400x^3 + 17918x^4 - 21997x^5 + 27966x^6 - 23532x^7 + 9060x^8 - 1027x^9 - 3428x^{10} + 1404x^{11})$$

**Simplify[Cf[10, 11, 6]]**

[化简]

$$2048 x (1+x)^5 (-648 + 1015x - 19296x^2 + 35793x^3 - 134342x^4 + 163415x^5 - 221688x^6 + 152143x^7 - 93386x^8 + 54714x^9 - 17376x^{10} + 6024x^{11})$$

**Simplify[Cf[10, 11, 7]]**

[化简]

$$-2048 x (1+x)^5 (888 - 1940x + 27259x^2 - 45307x^3 + 164672x^4 - 170926x^5 + 259107x^6 - 149199x^7 + 94290x^8 - 21764x^9 - 3096x^{10} + 2592x^{11})$$

**Simplify[Cf[10, 11, 8]]**

[化简]

$$-2048 x (1+x)^5 (888 - 1940 x + 27259 x^2 - 45307 x^3 + 164672 x^4 - 170926 x^5 + 259107 x^6 - 149199 x^7 + 94290 x^8 - 21764 x^9 - 3096 x^{10} + 2592 x^{11})$$

**Simplify[Cf[10, 11, 9]]**

[化简]

$$2048 x (1+x)^5 (-648 + 1015 x - 19296 x^2 + 35793 x^3 - 134342 x^4 + 163415 x^5 - 221688 x^6 + 152143 x^7 - 93386 x^8 + 54714 x^9 - 17376 x^{10} + 6024 x^{11})$$

**Simplify[Cf[10, 11, 10]]**

[化简]

$$-8192 x (1+x)^5 (120 - 360 x + 3492 x^2 - 6400 x^3 + 17918 x^4 - 21997 x^5 + 27966 x^6 - 23532 x^7 + 9060 x^8 - 1027 x^9 - 3428 x^{10} + 1404 x^{11})$$

**Simplify[Cf[10, 11, 11]]**

[化简]

$$2048 x (1+x)^5 (-168 + 195 x - 4460 x^2 + 11547 x^3 - 36566 x^4 + 58823 x^5 - 66584 x^6 + 62229 x^7 - 42638 x^8 + 30574 x^9 - 15664 x^{10} + 2712 x^{11})$$

**Simplify[Cf[10, 11, 12]]**

[化简]

$$-2048 (-1+x)^2 x (1+x)^5 (78 - 134 x + 1447 x^2 - 514 x^3 + 4130 x^4 - 744 x^5 + 4349 x^6 - 600 x^7 - 1020 x^8 + 144 x^9)$$

**Simplify[Cf[10, 11, 13]]**

[化简]

$$-2048 (-1+x)^3 x (1+x)^5 (-6 - 34 x - 84 x^2 - 195 x^3 - 332 x^4 - 521 x^5 + 92 x^6 + 36 x^7)$$

**Simplify[Cf[10, 11, 14]]**

[化简]

$$4096 (-1+x)^4 x^2 (1+x)^5 (-1 - 2 x - 11 x^2 - 8 x^3 + 2 x^4)$$

**(\*, r2^10r3^12\*)****Simplify[Cf[10, 12, 0]]**

[化简]

$$4096 x^3 (-1+x^2)^5$$

**Simplify[Cf[10, 12, 1]]**

[化简]

$$-2048 (-1+x)^4 x (1+x)^5 (4 - 12 x + 75 x^2 - 52 x^3 + 165 x^4 - 56 x^5 + 8 x^6)$$

**Simplify[Cf[10, 12, 2]]**

[化简]

$$-4096 (-1+x)^3 (1+x)^5 (-3 + 21 x - 131 x^2 + 203 x^3 - 650 x^4 + 431 x^5 - 1014 x^6 + 363 x^7 - 60 x^8 + 12 x^9)$$

**Simplify[Cf[10, 12, 3]]**

|化简

$$-2048 (-1+x)^2 x (1+x)^5 \\ (78 - 134x + 1447x^2 - 514x^3 + 4130x^4 - 744x^5 + 4349x^6 - 600x^7 - 1020x^8 + 144x^9)$$

**Simplify[Cf[10, 12, 4]]**

|化简

$$2048 (1+x)^5 (-48 + 480x - 3555x^2 + 11338x^3 - 33289x^4 + 62324x^5 - \\ 98829x^6 + 119218x^7 - 99767x^8 + 59360x^9 - 17520x^{10} - 240x^{11} + 528x^{12})$$

**Simplify[Cf[10, 12, 5]]**

|化简

$$-2048 x (1+x)^5 (368 - 1398x + 9883x^2 - 17514x^3 + 44189x^4 - \\ 58954x^5 + 85081x^6 - 92946x^7 + 62287x^8 - 29148x^9 + 4128x^{10} + 648x^{11})$$

**Simplify[Cf[10, 12, 6]]**

|化简

$$1024 (1+x)^5 (-228 + 2280x - 17657x^2 + 55410x^3 - 175923x^4 + 316440x^5 - \\ 538591x^6 + 605042x^7 - 527289x^8 + 312060x^9 - 106312x^{10} + 17792x^{11} + 1104x^{12})$$

**Simplify[Cf[10, 12, 7]]**

|化简

$$-2048 x (1+x)^5 (588 - 2271x + 16628x^2 - 28673x^3 + 79818x^4 - \\ 101037x^5 + 162376x^6 - 160663x^7 + 117606x^8 - 52908x^9 + 10632x^{10} + 528x^{11})$$

**Simplify[Cf[10, 12, 8]]**

|化简

$$1024 (1+x)^5 (-228 + 2280x - 17657x^2 + 55410x^3 - 175923x^4 + 316440x^5 - \\ 538591x^6 + 605042x^7 - 527289x^8 + 312060x^9 - 106312x^{10} + 17792x^{11} + 1104x^{12})$$

**Simplify[Cf[10, 12, 9]]**

|化简

$$-2048 x (1+x)^5 (368 - 1398x + 9883x^2 - 17514x^3 + 44189x^4 - \\ 58954x^5 + 85081x^6 - 92946x^7 + 62287x^8 - 29148x^9 + 4128x^{10} + 648x^{11})$$

**Simplify[Cf[10, 12, 10]]**

|化简

$$2048 (1+x)^5 (-48 + 480x - 3555x^2 + 11338x^3 - 33289x^4 + 62324x^5 - \\ 98829x^6 + 119218x^7 - 99767x^8 + 59360x^9 - 17520x^{10} - 240x^{11} + 528x^{12})$$

**Simplify[Cf[10, 12, 11]]**

|化简

$$-2048 (-1+x)^2 x (1+x)^5 \\ (78 - 134x + 1447x^2 - 514x^3 + 4130x^4 - 744x^5 + 4349x^6 - 600x^7 - 1020x^8 + 144x^9)$$

**Simplify[Cf[10, 12, 12]]**

|化简

$$-4096 (-1+x)^3 (1+x)^5 \\ (-3 + 21x - 131x^2 + 203x^3 - 650x^4 + 431x^5 - 1014x^6 + 363x^7 - 60x^8 + 12x^9)$$

**Simplify[Cf[10, 12, 13]]**

[化简]

$$-2048 (-1+x)^4 x (1+x)^5 (4-12x+75x^2-52x^3+165x^4-56x^5+8x^6)$$

**Simplify[Cf[10, 12, 14]]**

[化简]

$$4096 x^3 (-1+x^2)^5$$

**(\*, r2^10r3^13\*)****Simplify[Cf[10, 13, 0]]**

[化简]

$$-4096 x^2 (-1+x^2)^5 (-1+x-3x^2+x^3)$$

**Simplify[Cf[10, 13, 1]]**

[化简]

$$-2048 (-1+x)^4 x (1+x)^5 (4-12x+75x^2-52x^3+165x^4-56x^5+8x^6)$$

**Simplify[Cf[10, 13, 2]]**

[化简]

$$-2048 (-1+x)^3 x (1+x)^5 (-6-34x-84x^2-195x^3-332x^4-521x^5+92x^6+36x^7)$$

**Simplify[Cf[10, 13, 3]]**

[化简]

$$-4096 (-1+x)^2 x (1+x)^5 (18-53x+523x^2-704x^3+2078x^4-1455x^5+1921x^6-772x^7+12x^8)$$

**Simplify[Cf[10, 13, 4]]**

[化简]

$$2048 x (1+x)^5 (-46+21x-971x^2+1647x^3-5249x^4+6783x^5-3145x^6-1271x^7+4655x^8-2668x^9+244x^{10})$$

**Simplify[Cf[10, 13, 5]]**

[化简]

$$-2048 x (1+x)^5 (94-303x+3119x^2-6866x^3+17814x^4-22905x^5+21615x^6-15272x^7+5986x^8-1982x^9+236x^{10})$$

**Simplify[Cf[10, 13, 6]]**

[化简]

$$2048 x (1+x)^5 (-102+188x-2949x^2+5328x^3-16599x^4+19224x^5-17363x^6+8556x^7-391x^8-560x^9+60x^{10})$$

**Simplify[Cf[10, 13, 7]]**

[化简]

$$2048 x (1+x)^5 (-102+188x-2949x^2+5328x^3-16599x^4+19224x^5-17363x^6+8556x^7-391x^8-560x^9+60x^{10})$$

**Simplify[Cf[10, 13, 8]]**

[化简]

$$-2048 x (1+x)^5 (94-303x+3119x^2-6866x^3+17814x^4-22905x^5+21615x^6-15272x^7+5986x^8-1982x^9+236x^{10})$$

**Simplify[Cf[10, 13, 9]]**

[化简]

$$2048 x (1+x)^5 (-46 + 21 x - 971 x^2 + 1647 x^3 - 5249 x^4 + 6783 x^5 - 3145 x^6 - 1271 x^7 + 4655 x^8 - 2668 x^9 + 244 x^{10})$$

**Simplify[Cf[10, 13, 10]]**

[化简]

$$-4096 (-1+x)^2 x (1+x)^5 (18 - 53 x + 523 x^2 - 704 x^3 + 2078 x^4 - 1455 x^5 + 1921 x^6 - 772 x^7 + 12 x^8)$$

**Simplify[Cf[10, 13, 11]]**

[化简]

$$-2048 (-1+x)^3 x (1+x)^5 (-6 - 34 x - 84 x^2 - 195 x^3 - 332 x^4 - 521 x^5 + 92 x^6 + 36 x^7)$$

**Simplify[Cf[10, 13, 12]]**

[化简]

$$-2048 (-1+x)^4 x (1+x)^5 (4 - 12 x + 75 x^2 - 52 x^3 + 165 x^4 - 56 x^5 + 8 x^6)$$

**Simplify[Cf[10, 13, 13]]**

[化简]

$$-4096 x^2 (-1+x^2)^5 (-1+x-3 x^2+x^3)$$

**Simplify[Cf[10, 13, 14]]**

[化简]

0

**(\*, r2^10r3^14\*)****Simplify[Cf[10, 14, 0]]**

[化简]

$$4096 x^3 (-1+x^2)^5$$

**Simplify[Cf[10, 14, 1]]**

[化简]

$$4096 (-1+x)^4 x^2 (1+x)^5 (-1-2 x-11 x^2-8 x^3+2 x^4)$$

**Simplify[Cf[10, 14, 2]]**

[化简]

$$-2048 (-1+x)^3 x^2 (1+x)^5 (-7-25 x-57 x^2-55 x^3-116 x^4+44 x^5)$$

**Simplify[Cf[10, 14, 3]]**

[化简]

$$4096 (-1+x)^2 x^2 (1+x)^5 (-9-18 x-124 x^2+82 x^3-207 x^4+4 x^5+40 x^6)$$

**Simplify[Cf[10, 14, 4]]**

[化简]

$$-1024 x^2 (1+x)^5 (67+2 x+857 x^2-2092 x^3+3073 x^4-3126 x^5+1695 x^6-736 x^7+260 x^8)$$

**Simplify[Cf[10, 14, 5]]**

[化简]

$$2048 x^2 (1+x)^5 (-45-33 x-508 x^2+870 x^3-773 x^4-265 x^5+1450 x^6-1100 x^7+308 x^8)$$

**Simplify[Cf[10, 14, 6]]**

[化简]

$$-2048 x^2 (1+x)^5 (53 + 837 x^2 - 1888 x^3 + 3187 x^4 - 3528 x^5 + 2623 x^6 - 1528 x^7 + 436 x^8)$$

**Simplify[Cf[10, 14, 7]]**

[化简]

$$2048 x^2 (1+x)^5 (-45 - 33 x - 508 x^2 + 870 x^3 - 773 x^4 - 265 x^5 + 1450 x^6 - 1100 x^7 + 308 x^8)$$

**Simplify[Cf[10, 14, 8]]**

[化简]

$$-1024 x^2 (1+x)^5 (67 + 2 x + 857 x^2 - 2092 x^3 + 3073 x^4 - 3126 x^5 + 1695 x^6 - 736 x^7 + 260 x^8)$$

**Simplify[Cf[10, 14, 9]]**

[化简]

$$4096 (-1+x)^2 x^2 (1+x)^5 (-9 - 18 x - 124 x^2 + 82 x^3 - 207 x^4 + 4 x^5 + 40 x^6)$$

**Simplify[Cf[10, 14, 10]]**

[化简]

$$-2048 (-1+x)^3 x^2 (1+x)^5 (-7 - 25 x - 57 x^2 - 55 x^3 - 116 x^4 + 44 x^5)$$

**Simplify[Cf[10, 14, 11]]**

[化简]

$$4096 (-1+x)^4 x^2 (1+x)^5 (-1 - 2 x - 11 x^2 - 8 x^3 + 2 x^4)$$

**Simplify[Cf[10, 14, 12]]**

[化简]

$$4096 x^3 (-1+x^2)^5$$

**Simplify[Cf[10, 14, 13]]**

[化简]

0

**Simplify[Cf[10, 14, 14]]**

[化简]

0

(\*, r2^11r3^0\*)

**Simplify[Cf[11, 0, 0]]**

[化简]

0

**Simplify[Cf[11, 0, 1]]**

[化简]

0

**Simplify[Cf[11, 0, 2]]**

[化简]

0



**Simplify[Cf[11, 0, 3]]**

[化简]

0

**Simplify[Cf[11, 0, 4]]**

[化简]

0

**Simplify[Cf[11, 0, 5]]**

[化简]

0

**Simplify[Cf[11, 0, 6]]**

[化简]

0

**Simplify[Cf[11, 0, 7]]**

[化简]

0

**Simplify[Cf[11, 0, 8]]**

[化简]

0

**Simplify[Cf[11, 0, 9]]**

[化简]

0

**Simplify[Cf[11, 0, 10]]**

[化简]

0

**Simplify[Cf[11, 0, 11]]**

[化简]

$4096 x^3 (1 + x) (-1 + x^2)^5$

**Simplify[Cf[11, 0, 12]]**

[化简]

$2048 x^2 (-1 + x^2)^5 (2 + 3 x + 7 x^2 + 2 x^3)$

**Simplify[Cf[11, 0, 13]]**

[化简]

$2048 x^2 (-1 + x^2)^5 (2 + 3 x + 7 x^2 + 2 x^3)$

**Simplify[Cf[11, 0, 14]]**

[化简]

$4096 x^3 (1 + x) (-1 + x^2)^5$

(\*, r2^11r3^1\*)

**Simplify[Cf[11, 1, 0]]**

[化简]

0

**Simplify[Cf[11, 1, 1]]**

[化简]

0

**Simplify[Cf[11, 1, 2]]**

[化简]

0

**Simplify[Cf[11, 1, 3]]**

[化简]

0

**Simplify[Cf[11, 1, 4]]**

[化简]

0

**Simplify[Cf[11, 1, 5]]**

[化简]

0

**Simplify[Cf[11, 1, 6]]**

[化简]

0

**Simplify[Cf[11, 1, 7]]**

[化简]

0

**Simplify[Cf[11, 1, 8]]**

[化简]

0

**Simplify[Cf[11, 1, 9]]**

[化简]

0

**Simplify[Cf[11, 1, 10]]**

[化简]

$$4096 (-1+x)^4 x^2 (1+x)^5 (-1-2x-11x^2-8x^3+2x^4)$$

**Simplify[Cf[11, 1, 11]]**

[化简]

$$8192 (-1+x)^4 x^2 (1+x)^5 (-6+8x-41x^2-3x^3-16x^4+4x^5)$$

**Simplify[Cf[11, 1, 12]]**

[化简]

$$4096 (-1+x)^4 x (1+x)^5 (-2-4x-15x^2-84x^3-23x^4-60x^5+12x^6)$$

**Simplify[Cf[11, 1, 13]]**

[化简]

$$8192 (-1+x)^4 x^2 (1+x)^5 (-6+8x-41x^2-3x^3-16x^4+4x^5)$$

**Simplify[Cf[11, 1, 14]]**

[化简]

$$4096 (-1+x)^4 x^2 (1+x)^5 (-1-2x-11x^2-8x^3+2x^4)$$

**(\*, r2^11r3^2\*)**

**Simplify[Cf[11, 2, 0]]**

[化简]

0

**Simplify[Cf[11, 2, 1]]**

[化简]

0

**Simplify[Cf[11, 2, 2]]**

[化简]

0

**Simplify[Cf[11, 2, 3]]**

[化简]

0

**Simplify[Cf[11, 2, 4]]**

[化简]

0

**Simplify[Cf[11, 2, 5]]**

[化简]

0

**Simplify[Cf[11, 2, 6]]**

[化简]

0

**Simplify[Cf[11, 2, 7]]**

[化简]

0

**Simplify[Cf[11, 2, 8]]**

[化简]

0

**Simplify[Cf[11, 2, 9]]**

[化简]

$$-2048 (-1+x)^3 x^2 (1+x)^5 (-3-44x+37x^2-182x^3+60x^4)$$

**Simplify[Cf[11, 2, 10]]**

[\[化简\]](#)

$$-2048 (-1+x)^3 x (1+x)^5 (-6-34x-84x^2-195x^3-332x^4-521x^5+92x^6+36x^7)$$

**Simplify[Cf[11, 2, 11]]**

[\[化简\]](#)

$$2048 (-1+x)^3 x (1+x)^5 (24-31x+565x^2-483x^3+2171x^4-538x^5+1316x^6-552x^7+48x^8)$$

**Simplify[Cf[11, 2, 12]]**

[\[化简\]](#)

$$2048 (-1+x)^3 x (1+x)^5 (24-31x+565x^2-483x^3+2171x^4-538x^5+1316x^6-552x^7+48x^8)$$

**Simplify[Cf[11, 2, 13]]**

[\[化简\]](#)

$$-2048 (-1+x)^3 x (1+x)^5 (-6-34x-84x^2-195x^3-332x^4-521x^5+92x^6+36x^7)$$

**Simplify[Cf[11, 2, 14]]**

[\[化简\]](#)

$$-2048 (-1+x)^3 x^2 (1+x)^5 (-3-44x+37x^2-182x^3+60x^4)$$

**(\*, r2^11r3^3\*)**

**Simplify[Cf[11, 3, 0]]**

[\[化简\]](#)

0

**Simplify[Cf[11, 3, 1]]**

[\[化简\]](#)

0

**Simplify[Cf[11, 3, 2]]**

[\[化简\]](#)

0

**Simplify[Cf[11, 3, 3]]**

[\[化简\]](#)

0

**Simplify[Cf[11, 3, 4]]**

[\[化简\]](#)

0

**Simplify[Cf[11, 3, 5]]**

[\[化简\]](#)

0

**Simplify[Cf[11, 3, 6]]**

[\[化简\]](#)

0

**Simplify[Cf[11, 3, 7]]**

[化简]

0

**Simplify[Cf[11, 3, 8]]**

[化简]

$$-2048 (-1+x)^2 x^2 (1+x)^5 (9+60x+34x^2+56x^3+177x^4-188x^5+28x^6)$$

**Simplify[Cf[11, 3, 9]]**

[化简]

$$4096 (-1+x)^2 x^2 (1+x)^5 (-120+337x-1408x^2+1558x^3-2044x^4+597x^5+4x^6+36x^7)$$

**Simplify[Cf[11, 3, 10]]**

[化简]

$$-2048 (-1+x)^2 x (1+x)^5 (78-134x+1447x^2-514x^3+4130x^4-744x^5+4349x^6-600x^7-1020x^8+144x^9)$$

**Simplify[Cf[11, 3, 11]]**

[化简]

$$-12288 (-1+x)^2 x^2 (1+x)^5 (147-472x+1936x^2-2434x^3+3749x^4-2278x^5+1936x^6-984x^7+144x^8)$$

**Simplify[Cf[11, 3, 12]]**

[化简]

$$-2048 (-1+x)^2 x (1+x)^5 (78-134x+1447x^2-514x^3+4130x^4-744x^5+4349x^6-600x^7-1020x^8+144x^9)$$

**Simplify[Cf[11, 3, 13]]**

[化简]

$$4096 (-1+x)^2 x^2 (1+x)^5 (-120+337x-1408x^2+1558x^3-2044x^4+597x^5+4x^6+36x^7)$$

**Simplify[Cf[11, 3, 14]]**

[化简]

$$-2048 (-1+x)^2 x^2 (1+x)^5 (9+60x+34x^2+56x^3+177x^4-188x^5+28x^6)$$

**(\*, r2^11r3^4\*)****Simplify[Cf[11, 4, 0]]**

[化简]

0

**Simplify[Cf[11, 4, 1]]**

[化简]

0

**Simplify[Cf[11, 4, 2]]**

[化简]

0

**Simplify[Cf[11, 4, 3]]**

[化简]

0

**Simplify[Cf[11, 4, 4]]**

[\[化简\]](#)

0

**Simplify[Cf[11, 4, 5]]**

[\[化简\]](#)

0

**Simplify[Cf[11, 4, 6]]**

[\[化简\]](#)

0

**Simplify[Cf[11, 4, 7]]**

[\[化简\]](#)

$$2048 x^2 (1+x)^5 (-11-116 x+337 x^2-822 x^3+1271 x^4-1020 x^5+567 x^6-250 x^7+44 x^8)$$

**Simplify[Cf[11, 4, 8]]**

[\[化简\]](#)

$$\begin{aligned} & -2048 x (1+x)^5 \\ & (24+71 x+389 x^2-1171 x^3+5567 x^4-11413 x^5+13431 x^6-11365 x^7+5741 x^8-1562 x^9+288 x^{10}) \end{aligned}$$

**Simplify[Cf[11, 4, 9]]**

[\[化简\]](#)

$$\begin{aligned} & 2048 x (1+x)^5 (-142+425 x-3690 x^2+8601 x^3-21990 x^4+ \\ & 31475 x^5-28610 x^6+17979 x^7-2788 x^8-648 x^9-732 x^{10}+120 x^{11}) \end{aligned}$$

**Simplify[Cf[11, 4, 10]]**

[\[化简\]](#)

$$\begin{aligned} & 2048 x (1+x)^5 (-168+195 x-4460 x^2+11547 x^3-36566 x^4+ \\ & 58823 x^5-66584 x^6+62229 x^7-42638 x^8+30574 x^9-15664 x^{10}+2712 x^{11}) \end{aligned}$$

**Simplify[Cf[11, 4, 11]]**

[\[化简\]](#)

$$\begin{aligned} & 2048 x (1+x)^5 (-168+195 x-4460 x^2+11547 x^3-36566 x^4+ \\ & 58823 x^5-66584 x^6+62229 x^7-42638 x^8+30574 x^9-15664 x^{10}+2712 x^{11}) \end{aligned}$$

**Simplify[Cf[11, 4, 12]]**

[\[化简\]](#)

$$\begin{aligned} & 2048 x (1+x)^5 (-142+425 x-3690 x^2+8601 x^3-21990 x^4+ \\ & 31475 x^5-28610 x^6+17979 x^7-2788 x^8-648 x^9-732 x^{10}+120 x^{11}) \end{aligned}$$

**Simplify[Cf[11, 4, 13]]**

[\[化简\]](#)

$$\begin{aligned} & -2048 x (1+x)^5 \\ & (24+71 x+389 x^2-1171 x^3+5567 x^4-11413 x^5+13431 x^6-11365 x^7+5741 x^8-1562 x^9+288 x^{10}) \end{aligned}$$

**Simplify[Cf[11, 4, 14]]**

[\[化简\]](#)

$$2048 x^2 (1+x)^5 (-11-116 x+337 x^2-822 x^3+1271 x^4-1020 x^5+567 x^6-250 x^7+44 x^8)$$

(\*, r2^11r3^5\*)

**Simplify[Cf[11, 5, 0]]**

[\[化简\]](#)

0

**Simplify[Cf[11, 5, 1]]**

[\[化简\]](#)

0

**Simplify[Cf[11, 5, 2]]**

[\[化简\]](#)

0

**Simplify[Cf[11, 5, 3]]**

[\[化简\]](#)

0

**Simplify[Cf[11, 5, 4]]**

[\[化简\]](#)

0

**Simplify[Cf[11, 5, 5]]**

[\[化简\]](#)

0

**Simplify[Cf[11, 5, 6]]**

[\[化简\]](#)

$$-2048 x^2 (1+x)^5 (15+129 x-276 x^2+570 x^3-597 x^4+37 x^5+198 x^6-96 x^7+20 x^8)$$

**Simplify[Cf[11, 5, 7]]**

[\[化简\]](#)

$$4096 x^2 (1+x)^5 (-299+1352 x-5616 x^2+11877 x^3-18447 x^4+19478 x^5-12818 x^6+5737 x^7-1796 x^8+340 x^9)$$

**Simplify[Cf[11, 5, 8]]**

[\[化简\]](#)

$$2048 x (1+x)^5 (-238+753 x-6036 x^2+11066 x^3-26967 x^4+30947 x^5-31826 x^6+26928 x^7-10617 x^8+2938 x^9-140 x^{10}+24 x^{11})$$

**Simplify[Cf[11, 5, 9]]**

[\[化简\]](#)

$$-8192 x^2 (1+x)^5 (1015-4761 x+20474 x^2-42830 x^3+70527 x^4-75961 x^5+60448 x^6-38664 x^7+16928 x^8-6072 x^9+1200 x^{10})$$

**Simplify[Cf[11, 5, 10]]**

[\[化简\]](#)

$$-8192 x (1+x)^5 (120-360 x+3492 x^2-6400 x^3+17918 x^4-21997 x^5+27966 x^6-23532 x^7+9060 x^8-1027 x^9-3428 x^{10}+1404 x^{11})$$

**Simplify[Cf[11, 5, 11]]**

[\[化简\]](#)

$$-8192 x^2 (1+x)^5 (1015-4761 x+20474 x^2-42830 x^3+70527 x^4-75961 x^5+60448 x^6-38664 x^7+16928 x^8-6072 x^9+1200 x^{10})$$

**Simplify[Cf[11, 5, 12]]**

[化简]

$$2048 x (1+x)^5 (-238 + 753 x - 6036 x^2 + 11066 x^3 - 26967 x^4 + 30947 x^5 - 31826 x^6 + 26928 x^7 - 10617 x^8 + 2938 x^9 - 140 x^{10} + 24 x^{11})$$

**Simplify[Cf[11, 5, 13]]**

[化简]

$$4096 x^2 (1+x)^5 (-299 + 1352 x - 5616 x^2 + 11877 x^3 - 18447 x^4 + 19478 x^5 - 12818 x^6 + 5737 x^7 - 1796 x^8 + 340 x^9)$$

**Simplify[Cf[11, 5, 14]]**

[化简]

$$-2048 x^2 (1+x)^5 (15 + 129 x - 276 x^2 + 570 x^3 - 597 x^4 + 37 x^5 + 198 x^6 - 96 x^7 + 20 x^8)$$

**(\*, r2^11r3^6\*)****Simplify[Cf[11, 6, 0]]**

[化简]

0

**Simplify[Cf[11, 6, 1]]**

[化简]

0

**Simplify[Cf[11, 6, 2]]**

[化简]

0

**Simplify[Cf[11, 6, 3]]**

[化简]

0

**Simplify[Cf[11, 6, 4]]**

[化简]

0

**Simplify[Cf[11, 6, 5]]**

[化简]

$$-2048 x^2 (1+x)^5 (15 + 129 x - 276 x^2 + 570 x^3 - 597 x^4 + 37 x^5 + 198 x^6 - 96 x^7 + 20 x^8)$$

**Simplify[Cf[11, 6, 6]]**

[化简]

$$-4096 x (1+x)^5 (18 + 57 x + 380 x^2 - 1128 x^3 + 5543 x^4 - 10971 x^5 + 14182 x^6 - 12722 x^7 + 6857 x^8 - 2276 x^9 + 444 x^{10})$$

**Simplify[Cf[11, 6, 7]]**

[化简]

$$-2048 x (1+x)^5 (282 - 791 x + 7232 x^2 - 13452 x^3 + 36789 x^4 - 41995 x^5 + 42522 x^6 - 25450 x^7 + 3219 x^8 + 1336 x^9 - 236 x^{10} + 48 x^{11})$$



**Simplify[Cf[11, 6, 8]]**

[化简]

$$2048 x (1+x)^5 (-384 + 9x - 11414x^2 + 26555x^3 - 107046x^4 + 159337x^5 - 217282x^6 + 182633x^7 - 123402x^8 + 75666x^9 - 29528x^{10} + 6264x^{11})$$

**Simplify[Cf[11, 6, 9]]**

[化简]

$$2048 x (1+x)^5 (-648 + 1015x - 19296x^2 + 35793x^3 - 134342x^4 + 163415x^5 - 221688x^6 + 152143x^7 - 93386x^8 + 54714x^9 - 17376x^{10} + 6024x^{11})$$

**Simplify[Cf[11, 6, 10]]**

[化简]

$$2048 x (1+x)^5 (-648 + 1015x - 19296x^2 + 35793x^3 - 134342x^4 + 163415x^5 - 221688x^6 + 152143x^7 - 93386x^8 + 54714x^9 - 17376x^{10} + 6024x^{11})$$

**Simplify[Cf[11, 6, 11]]**

[化简]

$$2048 x (1+x)^5 (-384 + 9x - 11414x^2 + 26555x^3 - 107046x^4 + 159337x^5 - 217282x^6 + 182633x^7 - 123402x^8 + 75666x^9 - 29528x^{10} + 6264x^{11})$$

**Simplify[Cf[11, 6, 12]]**

[化简]

$$-2048 x (1+x)^5 (282 - 791x + 7232x^2 - 13452x^3 + 36789x^4 - 41995x^5 + 42522x^6 - 25450x^7 + 3219x^8 + 1336x^9 - 236x^{10} + 48x^{11})$$

**Simplify[Cf[11, 6, 13]]**

[化简]

$$-4096 x (1+x)^5 (18 + 57x + 380x^2 - 1128x^3 + 5543x^4 - 10971x^5 + 14182x^6 - 12722x^7 + 6857x^8 - 2276x^9 + 444x^{10})$$

**Simplify[Cf[11, 6, 14]]**

[化简]

$$-2048 x^2 (1+x)^5 (15 + 129x - 276x^2 + 570x^3 - 597x^4 + 37x^5 + 198x^6 - 96x^7 + 20x^8)$$

**(\*, r2^11r3^7\*)****Simplify[Cf[11, 7, 0]]**

[化简]

0

**Simplify[Cf[11, 7, 1]]**

[化简]

0

**Simplify[Cf[11, 7, 2]]**

[化简]

0

**Simplify[Cf[11, 7, 3]]**

[化简]

0

**Simplify[Cf[11, 7, 4]]**

[化简]

$$2048 x^2 (1+x)^5 (-11 - 116 x + 337 x^2 - 822 x^3 + 1271 x^4 - 1020 x^5 + 567 x^6 - 250 x^7 + 44 x^8)$$

**Simplify[Cf[11, 7, 5]]**

[化简]

$$4096 x^2 (1+x)^5 (-299 + 1352 x - 5616 x^2 + 11877 x^3 - 18447 x^4 + 19478 x^5 - 12818 x^6 + 5737 x^7 - 1796 x^8 + 340 x^9)$$

**Simplify[Cf[11, 7, 6]]**

[化简]

$$-2048 x (1+x)^5 (282 - 791 x + 7232 x^2 - 13452 x^3 + 36789 x^4 - 41995 x^5 + 42522 x^6 - 25450 x^7 + 3219 x^8 + 1336 x^9 - 236 x^{10} + 48 x^{11})$$

**Simplify[Cf[11, 7, 7]]**

[化简]

$$-4096 x^2 (1+x)^5 (3201 - 14506 x + 64639 x^2 - 131240 x^3 + 223947 x^4 - 230882 x^5 + 190569 x^6 - 112108 x^7 + 48140 x^8 - 15744 x^9 + 3360 x^{10})$$

**Simplify[Cf[11, 7, 8]]**

[化简]

$$2048 x (1+x)^5 (-888 + 1940 x - 27259 x^2 + 45307 x^3 - 164672 x^4 + 170926 x^5 - 259107 x^6 + 149199 x^7 - 94290 x^8 + 21764 x^9 + 3096 x^{10} - 2592 x^{11})$$

**Simplify[Cf[11, 7, 9]]**

[化简]

$$-8192 x^2 (1+x)^5 (2970 - 13299 x + 61532 x^2 - 120459 x^3 + 216260 x^4 - 218797 x^5 + 199684 x^6 - 115401 x^7 + 54586 x^8 - 15068 x^9 + 1464 x^{10})$$

**Simplify[Cf[11, 7, 10]]**

[化简]

$$2048 x (1+x)^5 (-888 + 1940 x - 27259 x^2 + 45307 x^3 - 164672 x^4 + 170926 x^5 - 259107 x^6 + 149199 x^7 - 94290 x^8 + 21764 x^9 + 3096 x^{10} - 2592 x^{11})$$

**Simplify[Cf[11, 7, 11]]**

[化简]

$$-4096 x^2 (1+x)^5 (3201 - 14506 x + 64639 x^2 - 131240 x^3 + 223947 x^4 - 230882 x^5 + 190569 x^6 - 112108 x^7 + 48140 x^8 - 15744 x^9 + 3360 x^{10})$$

**Simplify[Cf[11, 7, 12]]**

[化简]

$$-2048 x (1+x)^5 (282 - 791 x + 7232 x^2 - 13452 x^3 + 36789 x^4 - 41995 x^5 + 42522 x^6 - 25450 x^7 + 3219 x^8 + 1336 x^9 - 236 x^{10} + 48 x^{11})$$

**Simplify[Cf[11, 7, 13]]**

[化简]

$$4096 x^2 (1+x)^5 (-299 + 1352 x - 5616 x^2 + 11877 x^3 - 18447 x^4 + 19478 x^5 - 12818 x^6 + 5737 x^7 - 1796 x^8 + 340 x^9)$$

**Simplify[Cf[11, 7, 14]]**

[化简]

$$2048 x^2 (1+x)^5 (-11 - 116 x + 337 x^2 - 822 x^3 + 1271 x^4 - 1020 x^5 + 567 x^6 - 250 x^7 + 44 x^8)$$

(\*, r2^11r3^8\*)

**Simplify[Cf[11, 8, 0]]**

[化简]

0

**Simplify[Cf[11, 8, 1]]**

[化简]

0

**Simplify[Cf[11, 8, 2]]**

[化简]

0

**Simplify[Cf[11, 8, 3]]**

[化简]

$$-2048 (-1+x)^2 x^2 (1+x)^5 (9 + 60 x + 34 x^2 + 56 x^3 + 177 x^4 - 188 x^5 + 28 x^6)$$

**Simplify[Cf[11, 8, 4]]**

[化简]

$$-2048 x (1+x)^5 (24 + 71 x + 389 x^2 - 1171 x^3 + 5567 x^4 - 11413 x^5 + 13431 x^6 - 11365 x^7 + 5741 x^8 - 1562 x^9 + 288 x^{10})$$

**Simplify[Cf[11, 8, 5]]**

[化简]

$$2048 x (1+x)^5 (-238 + 753 x - 6036 x^2 + 11066 x^3 - 26967 x^4 + 30947 x^5 - 31826 x^6 + 26928 x^7 - 10617 x^8 + 2938 x^9 - 140 x^{10} + 24 x^{11})$$

**Simplify[Cf[11, 8, 6]]**

[化简]

$$2048 x (1+x)^5 (-384 + 9 x - 11414 x^2 + 26555 x^3 - 107046 x^4 + 159337 x^5 - 217282 x^6 + 182633 x^7 - 123402 x^8 + 75666 x^9 - 29528 x^{10} + 6264 x^{11})$$

**Simplify[Cf[11, 8, 7]]**

[化简]

$$2048 x (1+x)^5 (-888 + 1940 x - 27259 x^2 + 45307 x^3 - 164672 x^4 + 170926 x^5 - 259107 x^6 + 149199 x^7 - 94290 x^8 + 21764 x^9 + 3096 x^{10} - 2592 x^{11})$$

**Simplify[Cf[11, 8, 8]]**

[化简]

$$4096 x (1+x)^5 (-506 + 573 x - 16189 x^2 + 28202 x^3 - 122602 x^4 + 136419 x^5 - 225173 x^6 + 140452 x^7 - 121230 x^8 + 50018 x^9 - 21356 x^{10} + 1920 x^{11})$$

**Simplify[Cf[11, 8, 9]]**

[化简]

$$4096 x (1+x)^5 (-506 + 573 x - 16189 x^2 + 28202 x^3 - 122602 x^4 + 136419 x^5 - 225173 x^6 + 140452 x^7 - 121230 x^8 + 50018 x^9 - 21356 x^{10} + 1920 x^{11})$$

**Simplify[Cf[11, 8, 10]]**

[化简]

$$2048 x (1+x)^5 (-888 + 1940 x - 27259 x^2 + 45307 x^3 - 164672 x^4 + 170926 x^5 - 259107 x^6 + 149199 x^7 - 94290 x^8 + 21764 x^9 + 3096 x^{10} - 2592 x^{11})$$

**Simplify[Cf[11, 8, 11]]**

[化简]

$$2048 x (1+x)^5 (-384 + 9 x - 11414 x^2 + 26555 x^3 - 107046 x^4 + 159337 x^5 - 217282 x^6 + 182633 x^7 - 123402 x^8 + 75666 x^9 - 29528 x^{10} + 6264 x^{11})$$

**Simplify[Cf[11, 8, 12]]**

[化简]

$$2048 x (1+x)^5 (-238 + 753 x - 6036 x^2 + 11066 x^3 - 26967 x^4 + 30947 x^5 - 31826 x^6 + 26928 x^7 - 10617 x^8 + 2938 x^9 - 140 x^{10} + 24 x^{11})$$

**Simplify[Cf[11, 8, 13]]**

[化简]

$$-2048 x (1+x)^5 (24 + 71 x + 389 x^2 - 1171 x^3 + 5567 x^4 - 11413 x^5 + 13431 x^6 - 11365 x^7 + 5741 x^8 - 1562 x^9 + 288 x^{10})$$

**Simplify[Cf[11, 8, 14]]**

[化简]

$$-2048 (-1+x)^2 x^2 (1+x)^5 (9 + 60 x + 34 x^2 + 56 x^3 + 177 x^4 - 188 x^5 + 28 x^6)$$

**(\*, r2^11r3^9\*)****Simplify[Cf[11, 9, 0]]**

[化简]

0

**Simplify[Cf[11, 9, 1]]**

[化简]

0

**Simplify[Cf[11, 9, 2]]**

[化简]

$$-2048 (-1+x)^3 x^2 (1+x)^5 (-3 - 44 x + 37 x^2 - 182 x^3 + 60 x^4)$$

**Simplify[Cf[11, 9, 3]]**

[化简]

$$4096 (-1+x)^2 x^2 (1+x)^5 (-120 + 337 x - 1408 x^2 + 1558 x^3 - 2044 x^4 + 597 x^5 + 4 x^6 + 36 x^7)$$

**Simplify[Cf[11, 9, 4]]**

[化简]

$$2048 x (1+x)^5 (-142 + 425 x - 3690 x^2 + 8601 x^3 - 21990 x^4 + 31475 x^5 - 28610 x^6 + 17979 x^7 - 2788 x^8 - 648 x^9 - 732 x^{10} + 120 x^{11})$$

**Simplify[Cf[11, 9, 5]]**

[化简]

$$-8192 x^2 (1+x)^5 (1015 - 4761 x + 20474 x^2 - 42830 x^3 + 70527 x^4 - 75961 x^5 + 60448 x^6 - 38664 x^7 + 16928 x^8 - 6072 x^9 + 1200 x^{10})$$

**Simplify[Cf[11, 9, 6]]**

[化简]

$$2048 x (1+x)^5 (-648 + 1015 x - 19296 x^2 + 35793 x^3 - 134342 x^4 + 163415 x^5 - 221688 x^6 + 152143 x^7 - 93386 x^8 + 54714 x^9 - 17376 x^{10} + 6024 x^{11})$$

**Simplify[Cf[11, 9, 7]]**

[化简]

$$-8192 x^2 (1+x)^5 (2970 - 13299 x + 61532 x^2 - 120459 x^3 + 216260 x^4 - 218797 x^5 + 199684 x^6 - 115401 x^7 + 54586 x^8 - 15068 x^9 + 1464 x^{10})$$

**Simplify[Cf[11, 9, 8]]**

[化简]

$$4096 x (1+x)^5 (-506 + 573 x - 16189 x^2 + 28202 x^3 - 122602 x^4 + 136419 x^5 - 225173 x^6 + 140452 x^7 - 121230 x^8 + 50018 x^9 - 21356 x^{10} + 1920 x^{11})$$

**Simplify[Cf[11, 9, 9]]**

[化简]

$$-8192 x^2 (1+x)^5 (2970 - 13299 x + 61532 x^2 - 120459 x^3 + 216260 x^4 - 218797 x^5 + 199684 x^6 - 115401 x^7 + 54586 x^8 - 15068 x^9 + 1464 x^{10})$$

**Simplify[Cf[11, 9, 10]]**

[化简]

$$2048 x (1+x)^5 (-648 + 1015 x - 19296 x^2 + 35793 x^3 - 134342 x^4 + 163415 x^5 - 221688 x^6 + 152143 x^7 - 93386 x^8 + 54714 x^9 - 17376 x^{10} + 6024 x^{11})$$

**Simplify[Cf[11, 9, 11]]**

[化简]

$$-8192 x^2 (1+x)^5 (1015 - 4761 x + 20474 x^2 - 42830 x^3 + 70527 x^4 - 75961 x^5 + 60448 x^6 - 38664 x^7 + 16928 x^8 - 6072 x^9 + 1200 x^{10})$$

**Simplify[Cf[11, 9, 12]]**

[化简]

$$2048 x (1+x)^5 (-142 + 425 x - 3690 x^2 + 8601 x^3 - 21990 x^4 + 31475 x^5 - 28610 x^6 + 17979 x^7 - 2788 x^8 - 648 x^9 - 732 x^{10} + 120 x^{11})$$

**Simplify[Cf[11, 9, 13]]**

[化简]

$$4096 (-1+x)^2 x^2 (1+x)^5 (-120 + 337 x - 1408 x^2 + 1558 x^3 - 2044 x^4 + 597 x^5 + 4 x^6 + 36 x^7)$$

**Simplify[Cf[11, 9, 14]]**

[化简]

$$-2048 (-1+x)^3 x^2 (1+x)^5 (-3 - 44 x + 37 x^2 - 182 x^3 + 60 x^4)$$

**(\*, r2^11r3^10\*)****Simplify[Cf[11, 10, 0]]**

[化简]

0

**Simplify[Cf[11, 10, 1]]**

化简

$$4096 (-1+x)^4 x^2 (1+x)^5 (-1-2x-11x^2-8x^3+2x^4)$$

**Simplify[Cf[11, 10, 2]]**

化简

$$-2048 (-1+x)^3 x (1+x)^5 (-6-34x-84x^2-195x^3-332x^4-521x^5+92x^6+36x^7)$$

**Simplify[Cf[11, 10, 3]]**

化简

$$-2048 (-1+x)^2 x (1+x)^5 (78-134x+1447x^2-514x^3+4130x^4-744x^5+4349x^6-600x^7-1020x^8+144x^9)$$

**Simplify[Cf[11, 10, 4]]**

化简

$$2048 x (1+x)^5 (-168+195x-4460x^2+11547x^3-36566x^4+58823x^5-66584x^6+62229x^7-42638x^8+30574x^9-15664x^{10}+2712x^{11})$$

**Simplify[Cf[11, 10, 5]]**

化简

$$-8192 x (1+x)^5 (120-360x+3492x^2-6400x^3+17918x^4-21997x^5+27966x^6-23532x^7+9060x^8-1027x^9-3428x^{10}+1404x^{11})$$

**Simplify[Cf[11, 10, 6]]**

化简

$$2048 x (1+x)^5 (-648+1015x-19296x^2+35793x^3-134342x^4+163415x^5-221688x^6+152143x^7-93386x^8+54714x^9-17376x^{10}+6024x^{11})$$

**Simplify[Cf[11, 10, 7]]**

化简

$$2048 x (1+x)^5 (-888+1940x-27259x^2+45307x^3-164672x^4+170926x^5-259107x^6+149199x^7-94290x^8+21764x^9+3096x^{10}-2592x^{11})$$

**Simplify[Cf[11, 10, 8]]**

化简

$$2048 x (1+x)^5 (-888+1940x-27259x^2+45307x^3-164672x^4+170926x^5-259107x^6+149199x^7-94290x^8+21764x^9+3096x^{10}-2592x^{11})$$

**Simplify[Cf[11, 10, 9]]**

化简

$$2048 x (1+x)^5 (-648+1015x-19296x^2+35793x^3-134342x^4+163415x^5-221688x^6+152143x^7-93386x^8+54714x^9-17376x^{10}+6024x^{11})$$

**Simplify[Cf[11, 10, 10]]**

化简

$$-8192 x (1+x)^5 (120-360x+3492x^2-6400x^3+17918x^4-21997x^5+27966x^6-23532x^7+9060x^8-1027x^9-3428x^{10}+1404x^{11})$$

**Simplify[Cf[11, 10, 11]]**

| 化简

$$2048 x (1+x)^5 (-168 + 195 x - 4460 x^2 + 11547 x^3 - 36566 x^4 + 58823 x^5 - 66584 x^6 + 62229 x^7 - 42638 x^8 + 30574 x^9 - 15664 x^{10} + 2712 x^{11})$$

**Simplify[Cf[11, 10, 12]]**

| 化简

$$-2048 (-1+x)^2 x (1+x)^5 (78 - 134 x + 1447 x^2 - 514 x^3 + 4130 x^4 - 744 x^5 + 4349 x^6 - 600 x^7 - 1020 x^8 + 144 x^9)$$

**Simplify[Cf[11, 10, 13]]**

| 化简

$$-2048 (-1+x)^3 x (1+x)^5 (-6 - 34 x - 84 x^2 - 195 x^3 - 332 x^4 - 521 x^5 + 92 x^6 + 36 x^7)$$

**Simplify[Cf[11, 10, 14]]**

| 化简

$$4096 (-1+x)^4 x^2 (1+x)^5 (-1 - 2 x - 11 x^2 - 8 x^3 + 2 x^4)$$

**(\*, r2^11r3^11\*)****Simplify[Cf[11, 11, 0]]**

| 化简

$$4096 (-1+x)^5 x^3 (1+x)^6$$

**Simplify[Cf[11, 11, 1]]**

| 化简

$$8192 (-1+x)^4 x^2 (1+x)^5 (-6 + 8 x - 41 x^2 - 3 x^3 - 16 x^4 + 4 x^5)$$

**Simplify[Cf[11, 11, 2]]**

| 化简

$$2048 (-1+x)^3 x (1+x)^5 (24 - 31 x + 565 x^2 - 483 x^3 + 2171 x^4 - 538 x^5 + 1316 x^6 - 552 x^7 + 48 x^8)$$

**Simplify[Cf[11, 11, 3]]**

| 化简

$$-12288 (-1+x)^2 x^2 (1+x)^5 (147 - 472 x + 1936 x^2 - 2434 x^3 + 3749 x^4 - 2278 x^5 + 1936 x^6 - 984 x^7 + 144 x^8)$$

**Simplify[Cf[11, 11, 4]]**

| 化简

$$2048 x (1+x)^5 (-168 + 195 x - 4460 x^2 + 11547 x^3 - 36566 x^4 + 58823 x^5 - 66584 x^6 + 62229 x^7 - 42638 x^8 + 30574 x^9 - 15664 x^{10} + 2712 x^{11})$$

**Simplify[Cf[11, 11, 5]]**

| 化简

$$-8192 x^2 (1+x)^5 (1015 - 4761 x + 20474 x^2 - 42830 x^3 + 70527 x^4 - 75961 x^5 + 60448 x^6 - 38664 x^7 + 16928 x^8 - 6072 x^9 + 1200 x^{10})$$

**Simplify[Cf[11, 11, 6]]**

| 化简

$$2048 x (1+x)^5 (-384 + 9 x - 11414 x^2 + 26555 x^3 - 107046 x^4 + 159337 x^5 - 217282 x^6 + 182633 x^7 - 123402 x^8 + 75666 x^9 - 29528 x^{10} + 6264 x^{11})$$

**Simplify[Cf[11, 11, 7]]**

[化简]

$$-4096 x^2 (1+x)^5 (3201 - 14506 x + 64639 x^2 - 131240 x^3 + 223947 x^4 - 230882 x^5 + 190569 x^6 - 112108 x^7 + 48140 x^8 - 15744 x^9 + 3360 x^{10})$$

**Simplify[Cf[11, 11, 8]]**

[化简]

$$2048 x (1+x)^5 (-384 + 9 x - 11414 x^2 + 26555 x^3 - 107046 x^4 + 159337 x^5 - 217282 x^6 + 182633 x^7 - 123402 x^8 + 75666 x^9 - 29528 x^{10} + 6264 x^{11})$$

**Simplify[Cf[11, 11, 9]]**

[化简]

$$-8192 x^2 (1+x)^5 (1015 - 4761 x + 20474 x^2 - 42830 x^3 + 70527 x^4 - 75961 x^5 + 60448 x^6 - 38664 x^7 + 16928 x^8 - 6072 x^9 + 1200 x^{10})$$

**Simplify[Cf[11, 11, 10]]**

[化简]

$$2048 x (1+x)^5 (-168 + 195 x - 4460 x^2 + 11547 x^3 - 36566 x^4 + 58823 x^5 - 66584 x^6 + 62229 x^7 - 42638 x^8 + 30574 x^9 - 15664 x^{10} + 2712 x^{11})$$

**Simplify[Cf[11, 11, 11]]**

[化简]

$$-12288 (-1+x)^2 x^2 (1+x)^5 (147 - 472 x + 1936 x^2 - 2434 x^3 + 3749 x^4 - 2278 x^5 + 1936 x^6 - 984 x^7 + 144 x^8)$$

**Simplify[Cf[11, 11, 12]]**

[化简]

$$2048 (-1+x)^3 x (1+x)^5 (24 - 31 x + 565 x^2 - 483 x^3 + 2171 x^4 - 538 x^5 + 1316 x^6 - 552 x^7 + 48 x^8)$$

**Simplify[Cf[11, 11, 13]]**

[化简]

$$8192 (-1+x)^4 x^2 (1+x)^5 (-6 + 8 x - 41 x^2 - 3 x^3 - 16 x^4 + 4 x^5)$$

**Simplify[Cf[11, 11, 14]]**

[化简]

$$4096 (-1+x)^5 x^3 (1+x)^6$$

**(\*, r2^11r3^12\*)****Simplify[Cf[11, 12, 0]]**

[化简]

$$2048 x^2 (-1+x^2)^5 (2 + 3 x + 7 x^2 + 2 x^3)$$

**Simplify[Cf[11, 12, 1]]**

[化简]

$$4096 (-1+x)^4 x (1+x)^5 (-2 - 4 x - 15 x^2 - 84 x^3 - 23 x^4 - 60 x^5 + 12 x^6)$$

**Simplify[Cf[11, 12, 2]]**

[化简]

$$2048 (-1+x)^3 x (1+x)^5 (24 - 31 x + 565 x^2 - 483 x^3 + 2171 x^4 - 538 x^5 + 1316 x^6 - 552 x^7 + 48 x^8)$$



**Simplify[Cf[11, 12, 3]]**

[化简]

$$-2048 (-1+x)^2 x (1+x)^5 (78-134x+1447x^2-514x^3+4130x^4-744x^5+4349x^6-600x^7-1020x^8+144x^9)$$

**Simplify[Cf[11, 12, 4]]**

[化简]

$$2048x(1+x)^5(-142+425x-3690x^2+8601x^3-21990x^4+31475x^5-28610x^6+17979x^7-2788x^8-648x^9-732x^{10}+120x^{11})$$

**Simplify[Cf[11, 12, 5]]**

[化简]

$$2048x(1+x)^5(-238+753x-6036x^2+11066x^3-26967x^4+30947x^5-31826x^6+26928x^7-10617x^8+2938x^9-140x^{10}+24x^{11})$$

**Simplify[Cf[11, 12, 6]]**

[化简]

$$-2048x(1+x)^5(282-791x+7232x^2-13452x^3+36789x^4-41995x^5+42522x^6-25450x^7+3219x^8+1336x^9-236x^{10}+48x^{11})$$

**Simplify[Cf[11, 12, 7]]**

[化简]

$$-2048x(1+x)^5(282-791x+7232x^2-13452x^3+36789x^4-41995x^5+42522x^6-25450x^7+3219x^8+1336x^9-236x^{10}+48x^{11})$$

**Simplify[Cf[11, 12, 8]]**

[化简]

$$2048x(1+x)^5(-238+753x-6036x^2+11066x^3-26967x^4+30947x^5-31826x^6+26928x^7-10617x^8+2938x^9-140x^{10}+24x^{11})$$

**Simplify[Cf[11, 12, 9]]**

[化简]

$$2048x(1+x)^5(-142+425x-3690x^2+8601x^3-21990x^4+31475x^5-28610x^6+17979x^7-2788x^8-648x^9-732x^{10}+120x^{11})$$

**Simplify[Cf[11, 12, 10]]**

[化简]

$$-2048 (-1+x)^2 x (1+x)^5 (78-134x+1447x^2-514x^3+4130x^4-744x^5+4349x^6-600x^7-1020x^8+144x^9)$$

**Simplify[Cf[11, 12, 11]]**

[化简]

$$2048 (-1+x)^3 x (1+x)^5 (24-31x+565x^2-483x^3+2171x^4-538x^5+1316x^6-552x^7+48x^8)$$

**Simplify[Cf[11, 12, 12]]**

[化简]

$$4096 (-1+x)^4 x (1+x)^5 (-2-4x-15x^2-84x^3-23x^4-60x^5+12x^6)$$

**Simplify[Cf[11, 12, 13]]**

[化简]

$$2048x^2(-1+x^2)^5(2+3x+7x^2+2x^3)$$

**Simplify[Cf[11, 12, 14]]**

[\[化简\]](#)

0

**(\*, r2^11r3^13\*)**

**Simplify[Cf[11, 13, 0]]**

[\[化简\]](#)

$2048 x^2 (-1 + x^2)^5 (2 + 3x + 7x^2 + 2x^3)$

**Simplify[Cf[11, 13, 1]]**

[\[化简\]](#)

$8192 (-1 + x)^4 x^2 (1 + x)^5 (-6 + 8x - 41x^2 - 3x^3 - 16x^4 + 4x^5)$

**Simplify[Cf[11, 13, 2]]**

[\[化简\]](#)

$-2048 (-1 + x)^3 x (1 + x)^5 (-6 - 34x - 84x^2 - 195x^3 - 332x^4 - 521x^5 + 92x^6 + 36x^7)$

**Simplify[Cf[11, 13, 3]]**

[\[化简\]](#)

$4096 (-1 + x)^2 x^2 (1 + x)^5 (-120 + 337x - 1408x^2 + 1558x^3 - 2044x^4 + 597x^5 + 4x^6 + 36x^7)$

**Simplify[Cf[11, 13, 4]]**

[\[化简\]](#)

$-2048 x (1 + x)^5 (24 + 71x + 389x^2 - 1171x^3 + 5567x^4 - 11413x^5 + 13431x^6 - 11365x^7 + 5741x^8 - 1562x^9 + 288x^{10})$

**Simplify[Cf[11, 13, 5]]**

[\[化简\]](#)

$4096 x^2 (1 + x)^5 (-299 + 1352x - 5616x^2 + 11877x^3 - 18447x^4 + 19478x^5 - 12818x^6 + 5737x^7 - 1796x^8 + 340x^9)$

**Simplify[Cf[11, 13, 6]]**

[\[化简\]](#)

$-4096 x (1 + x)^5 (18 + 57x + 380x^2 - 1128x^3 + 5543x^4 - 10971x^5 + 14182x^6 - 12722x^7 + 6857x^8 - 2276x^9 + 444x^{10})$

**Simplify[Cf[11, 13, 7]]**

[\[化简\]](#)

$4096 x^2 (1 + x)^5 (-299 + 1352x - 5616x^2 + 11877x^3 - 18447x^4 + 19478x^5 - 12818x^6 + 5737x^7 - 1796x^8 + 340x^9)$

**Simplify[Cf[11, 13, 8]]**

[\[化简\]](#)

$-2048 x (1 + x)^5 (24 + 71x + 389x^2 - 1171x^3 + 5567x^4 - 11413x^5 + 13431x^6 - 11365x^7 + 5741x^8 - 1562x^9 + 288x^{10})$

**Simplify[Cf[11, 13, 9]]**

[\[化简\]](#)

$4096 (-1 + x)^2 x^2 (1 + x)^5 (-120 + 337x - 1408x^2 + 1558x^3 - 2044x^4 + 597x^5 + 4x^6 + 36x^7)$

**Simplify[Cf[11, 13, 10]]**

[\[化简\]](#)

$$-2048 (-1+x)^3 x (1+x)^5 (-6-34x-84x^2-195x^3-332x^4-521x^5+92x^6+36x^7)$$

**Simplify[Cf[11, 13, 11]]**

[\[化简\]](#)

$$8192 (-1+x)^4 x^2 (1+x)^5 (-6+8x-41x^2-3x^3-16x^4+4x^5)$$

**Simplify[Cf[11, 13, 12]]**

[\[化简\]](#)

$$2048 x^2 (-1+x^2)^5 (2+3x+7x^2+2x^3)$$

**Simplify[Cf[11, 13, 13]]**

[\[化简\]](#)

0

**Simplify[Cf[11, 13, 14]]**

[\[化简\]](#)

0

**(\*, r2^11r3^14\*)**

**Simplify[Cf[11, 14, 0]]**

[\[化简\]](#)

$$4096 (-1+x)^5 x^3 (1+x)^6$$

**Simplify[Cf[11, 14, 1]]**

[\[化简\]](#)

$$4096 (-1+x)^4 x^2 (1+x)^5 (-1-2x-11x^2-8x^3+2x^4)$$

**Simplify[Cf[11, 14, 2]]**

[\[化简\]](#)

$$-2048 (-1+x)^3 x^2 (1+x)^5 (-3-44x+37x^2-182x^3+60x^4)$$

**Simplify[Cf[11, 14, 3]]**

[\[化简\]](#)

$$-2048 (-1+x)^2 x^2 (1+x)^5 (9+60x+34x^2+56x^3+177x^4-188x^5+28x^6)$$

**Simplify[Cf[11, 14, 4]]**

[\[化简\]](#)

$$2048 x^2 (1+x)^5 (-11-116x+337x^2-822x^3+1271x^4-1020x^5+567x^6-250x^7+44x^8)$$

**Simplify[Cf[11, 14, 5]]**

[\[化简\]](#)

$$-2048 x^2 (1+x)^5 (15+129x-276x^2+570x^3-597x^4+37x^5+198x^6-96x^7+20x^8)$$

**Simplify[Cf[11, 14, 6]]**

[\[化简\]](#)

$$-2048 x^2 (1+x)^5 (15+129x-276x^2+570x^3-597x^4+37x^5+198x^6-96x^7+20x^8)$$

**Simplify[Cf[11, 14, 7]]**

[化简]

$$2048 x^2 (1+x)^5 (-11 - 116 x + 337 x^2 - 822 x^3 + 1271 x^4 - 1020 x^5 + 567 x^6 - 250 x^7 + 44 x^8)$$

**Simplify[Cf[11, 14, 8]]**

[化简]

$$-2048 (-1+x)^2 x^2 (1+x)^5 (9 + 60 x + 34 x^2 + 56 x^3 + 177 x^4 - 188 x^5 + 28 x^6)$$

**Simplify[Cf[11, 14, 9]]**

[化简]

$$-2048 (-1+x)^3 x^2 (1+x)^5 (-3 - 44 x + 37 x^2 - 182 x^3 + 60 x^4)$$

**Simplify[Cf[11, 14, 10]]**

[化简]

$$4096 (-1+x)^4 x^2 (1+x)^5 (-1 - 2 x - 11 x^2 - 8 x^3 + 2 x^4)$$

**Simplify[Cf[11, 14, 11]]**

[化简]

$$4096 (-1+x)^5 x^3 (1+x)^6$$

**Simplify[Cf[11, 14, 12]]**

[化简]

0

**Simplify[Cf[11, 14, 13]]**

[化简]

0

**Simplify[Cf[11, 14, 14]]**

[化简]

0

**(\*, r2^12r3^0\*)**

**Simplify[Cf[12, 0, 0]]**

[化简]

0

**Simplify[Cf[12, 0, 1]]**

[化简]

0

**Simplify[Cf[12, 0, 2]]**

[化简]

0

**Simplify[Cf[12, 0, 3]]**

[化简]

0

**Simplify[Cf[12, 0, 4]]**

[化简]

0

**Simplify[Cf[12, 0, 5]]**

[化简]

0

**Simplify[Cf[12, 0, 6]]**

[化简]

0

**Simplify[Cf[12, 0, 7]]**

[化简]

0

**Simplify[Cf[12, 0, 8]]**

[化简]

0

**Simplify[Cf[12, 0, 9]]**

[化简]

0

**Simplify[Cf[12, 0, 10]]**

[化简]

$4096 x^3 (-1 + x^2)^5$

**Simplify[Cf[12, 0, 11]]**

[化简]

$2048 x^2 (-1 + x^2)^5 (2 + 3 x + 7 x^2 + 2 x^3)$

**Simplify[Cf[12, 0, 12]]**

[化简]

$12288 x^3 (-1 + x^2)^5 (3 - x + 2 x^2)$

**Simplify[Cf[12, 0, 13]]**

[化简]

$2048 x^2 (-1 + x^2)^5 (2 + 3 x + 7 x^2 + 2 x^3)$

**Simplify[Cf[12, 0, 14]]**

[化简]

$4096 x^3 (-1 + x^2)^5$

(\*, r2^12r3^1\*)

**Simplify[Cf[12, 1, 0]]**

[化简]

0

**Simplify[Cf[12, 1, 1]]**

[化简]

0

**Simplify[Cf[12, 1, 2]]**

[化简]

0

**Simplify[Cf[12, 1, 3]]**

[化简]

0

**Simplify[Cf[12, 1, 4]]**

[化简]

0

**Simplify[Cf[12, 1, 5]]**

[化简]

0

**Simplify[Cf[12, 1, 6]]**

[化简]

0

**Simplify[Cf[12, 1, 7]]**

[化简]

0

**Simplify[Cf[12, 1, 8]]**

[化简]

0

**Simplify[Cf[12, 1, 9]]**

[化简]

$$-2048 (-1+x)^4 x^2 (1+x)^5 (2-3x+30x^2-21x^3+4x^4)$$

**Simplify[Cf[12, 1, 10]]**

[化简]

$$-2048 (-1+x)^4 x (1+x)^5 (4-12x+75x^2-52x^3+165x^4-56x^5+8x^6)$$

**Simplify[Cf[12, 1, 11]]**

[化简]

$$4096 (-1+x)^4 x (1+x)^5 (-2-4x-15x^2-84x^3-23x^4-60x^5+12x^6)$$

**Simplify[Cf[12, 1, 12]]**

[化简]

$$4096 (-1+x)^4 x (1+x)^5 (-2-4x-15x^2-84x^3-23x^4-60x^5+12x^6)$$

**Simplify[Cf[12, 1, 13]]**

[化简]

$$-2048 (-1+x)^4 x (1+x)^5 (4-12x+75x^2-52x^3+165x^4-56x^5+8x^6)$$

**Simplify[Cf[12, 1, 14]]**

[\[化简\]](#)

$$-2048 (-1+x)^4 x^2 (1+x)^5 (2-3x+30x^2-21x^3+4x^4)$$

**(\*, r2^12r3^2\*)**

**Simplify[Cf[12, 2, 0]]**

[\[化简\]](#)

0

**Simplify[Cf[12, 2, 1]]**

[\[化简\]](#)

0

**Simplify[Cf[12, 2, 2]]**

[\[化简\]](#)

0

**Simplify[Cf[12, 2, 3]]**

[\[化简\]](#)

0

**Simplify[Cf[12, 2, 4]]**

[\[化简\]](#)

0

**Simplify[Cf[12, 2, 5]]**

[\[化简\]](#)

0

**Simplify[Cf[12, 2, 6]]**

[\[化简\]](#)

0

**Simplify[Cf[12, 2, 7]]**

[\[化简\]](#)

0

**Simplify[Cf[12, 2, 8]]**

[\[化简\]](#)

$$1024 (-1+x)^3 x^2 (1+x)^5 (7+19x+13x^2+137x^3-172x^4+44x^5)$$

**Simplify[Cf[12, 2, 9]]**

[\[化简\]](#)

$$2048 (-1+x)^3 x (1+x)^5 (6+7x+89x^2+50x^3+225x^4+197x^5-190x^6+36x^7)$$

**Simplify[Cf[12, 2, 10]]**

[\[化简\]](#)

$$-4096 (-1+x)^3 (1+x)^5 (-3+21x-131x^2+203x^3-650x^4+431x^5-1014x^6+363x^7-60x^8+12x^9)$$

**Simplify[Cf[12, 2, 11]]**

[\[化简\]](#)

$$2048 (-1+x)^3 x (1+x)^5 (24 - 31x + 565x^2 - 483x^3 + 2171x^4 - 538x^5 + 1316x^6 - 552x^7 + 48x^8)$$

**Simplify[Cf[12, 2, 12]]**

[\[化简\]](#)

$$-4096 (-1+x)^3 (1+x)^5 (-3 + 21x - 131x^2 + 203x^3 - 650x^4 + 431x^5 - 1014x^6 + 363x^7 - 60x^8 + 12x^9)$$

**Simplify[Cf[12, 2, 13]]**

[\[化简\]](#)

$$2048 (-1+x)^3 x (1+x)^5 (6 + 7x + 89x^2 + 50x^3 + 225x^4 + 197x^5 - 190x^6 + 36x^7)$$

**Simplify[Cf[12, 2, 14]]**

[\[化简\]](#)

$$1024 (-1+x)^3 x^2 (1+x)^5 (7 + 19x + 13x^2 + 137x^3 - 172x^4 + 44x^5)$$

**(\*, r2^12r3^3\*)**

**Simplify[Cf[12, 3, 0]]**

[\[化简\]](#)

0

**Simplify[Cf[12, 3, 1]]**

[\[化简\]](#)

0

**Simplify[Cf[12, 3, 2]]**

[\[化简\]](#)

0

**Simplify[Cf[12, 3, 4]]**

[\[化简\]](#)

0

**Simplify[Cf[12, 3, 5]]**

[\[化简\]](#)

0

**Simplify[Cf[12, 3, 6]]**

[\[化简\]](#)

0

**Simplify[Cf[12, 3, 7]]**

[\[化简\]](#)

$$-2048 (-1+x)^2 x^2 (1+x)^5 (9 - 14x + 132x^2 - 190x^3 + 207x^4 - 180x^5 + 52x^6)$$

**Simplify[Cf[12, 3, 8]]**

[\[化简\]](#)

$$-2048 (-1+x)^2 x (1+x)^5 (18 - 53x + 419x^2 - 464x^3 + 1070x^4 - 399x^5 + 121x^6 - 228x^7 + 60x^8)$$



**Simplify[Cf[12, 3, 9]]**

[\[化简\]](#)

$$4096 (-1+x)^2 x (1+x)^5 \\ (-30+78x-535x^2+314x^3-1370x^4+916x^5-2281x^6+1676x^7-456x^8+72x^9)$$

**Simplify[Cf[12, 3, 10]]**

[\[化简\]](#)

$$-2048 (-1+x)^2 x (1+x)^5 \\ (78-134x+1447x^2-514x^3+4130x^4-744x^5+4349x^6-600x^7-1020x^8+144x^9)$$

**Simplify[Cf[12, 3, 11]]**

[\[化简\]](#)

$$-2048 (-1+x)^2 x (1+x)^5 \\ (78-134x+1447x^2-514x^3+4130x^4-744x^5+4349x^6-600x^7-1020x^8+144x^9)$$

**Simplify[Cf[12, 3, 12]]**

[\[化简\]](#)

$$4096 (-1+x)^2 x (1+x)^5 \\ (-30+78x-535x^2+314x^3-1370x^4+916x^5-2281x^6+1676x^7-456x^8+72x^9)$$

**Simplify[Cf[12, 3, 13]]**

[\[化简\]](#)

$$-2048 (-1+x)^2 x (1+x)^5 (18-53x+419x^2-464x^3+1070x^4-399x^5+121x^6-228x^7+60x^8)$$

**Simplify[Cf[12, 3, 14]]**

[\[化简\]](#)

$$-2048 (-1+x)^2 x^2 (1+x)^5 (9-14x+132x^2-190x^3+207x^4-180x^5+52x^6)$$

**(\*, r2^12r3^4\*)**

**Simplify[Cf[12, 4, 0]]**

[\[化简\]](#)

0

**Simplify[Cf[12, 4, 1]]**

[\[化简\]](#)

0

**Simplify[Cf[12, 4, 2]]**

[\[化简\]](#)

0

**Simplify[Cf[12, 4, 3]]**

[\[化简\]](#)

0

**Simplify[Cf[12, 4, 4]]**

[\[化简\]](#)

0

**Simplify[Cf[12, 4, 5]]**

[化简]

0

**Simplify[Cf[12, 4, 6]]**

[化简]

$$1024 (-1+x)^2 x^2 (1+x)^5 (-21-24x-78x^2-328x^3+551x^4-424x^5+148x^6)$$

**Simplify[Cf[12, 4, 7]]**

[化简]

$$2048x(1+x)^5 (-22+61x-464x^2+899x^3-1766x^4+2289x^5-1036x^6-11x^7+172x^8-166x^9+44x^{10})$$

**Simplify[Cf[12, 4, 8]]**

[化简]

$$-2048(1+x)^5 (24-240x+1755x^2-5836x^3+16193x^4-28994x^5+40829x^6-45928x^7+37615x^8-23738x^9+10784x^{10}-2848x^{11}+384x^{12})$$

**Simplify[Cf[12, 4, 9]]**

[化简]

$$2048x(1+x)^5 (-142+425x-3690x^2+8601x^3-21990x^4+31475x^5-28610x^6+17979x^7-2788x^8-648x^9-732x^{10}+120x^{11})$$

**Simplify[Cf[12, 4, 10]]**

[化简]

$$2048(1+x)^5 (-48+480x-3555x^2+11338x^3-33289x^4+62324x^5-98829x^6+119218x^7-99767x^8+59360x^9-17520x^{10}-240x^{11}+528x^{12})$$

**Simplify[Cf[12, 4, 11]]**

[化简]

$$2048x(1+x)^5 (-142+425x-3690x^2+8601x^3-21990x^4+31475x^5-28610x^6+17979x^7-2788x^8-648x^9-732x^{10}+120x^{11})$$

**Simplify[Cf[12, 4, 12]]**

[化简]

$$-2048(1+x)^5 (24-240x+1755x^2-5836x^3+16193x^4-28994x^5+40829x^6-45928x^7+37615x^8-23738x^9+10784x^{10}-2848x^{11}+384x^{12})$$

**Simplify[Cf[12, 4, 13]]**

[化简]

$$2048x(1+x)^5 (-22+61x-464x^2+899x^3-1766x^4+2289x^5-1036x^6-11x^7+172x^8-166x^9+44x^{10})$$

**Simplify[Cf[12, 4, 14]]**

[化简]

$$1024 (-1+x)^2 x^2 (1+x)^5 (-21-24x-78x^2-328x^3+551x^4-424x^5+148x^6)$$

(\*, r2^12r3^5\*)

**Simplify[Cf[12, 5, 0]]**

[化简]

0

**Simplify[Cf[12, 5, 1]]**

[化简]

0

**Simplify[Cf[12, 5, 2]]**

[化简]

0

**Simplify[Cf[12, 5, 3]]**

[化简]

0

**Simplify[Cf[12, 5, 4]]**

[化简]

0

**Simplify[Cf[12, 5, 5]]**

[化简]

$$-4096 (-1+x)^2 x^2 (1+x)^5 (7-7x+96x^2-102x^3+149x^4-111x^5+40x^6)$$

**Simplify[Cf[12, 5, 6]]**

[化简]

$$-2048 x (1+x)^5 (30-109x+767x^2-1588x^3+3006x^4-3343x^5+1303x^6-22x^7-30x^8-26x^9+12x^{10})$$

**Simplify[Cf[12, 5, 7]]**

[化简]

$$4096 x (1+x)^5 (-80+393x-2217x^2+4730x^3-9858x^4+14329x^5-18549x^6+21468x^7-16396x^8+7712x^9-2132x^{10}+312x^{11})$$

**Simplify[Cf[12, 5, 8]]**

[化简]

$$2048 x (1+x)^5 (-238+753x-6036x^2+11066x^3-26967x^4+30947x^5-31826x^6+26928x^7-10617x^8+2938x^9-140x^{10}+24x^{11})$$

**Simplify[Cf[12, 5, 9]]**

[化简]

$$-2048 x (1+x)^5 (368-1398x+9883x^2-17514x^3+44189x^4-58954x^5+85081x^6-92946x^7+62287x^8-29148x^9+4128x^{10}+648x^{11})$$

**Simplify[Cf[12, 5, 10]]**

[化简]

$$-2048 x (1+x)^5 (368-1398x+9883x^2-17514x^3+44189x^4-58954x^5+85081x^6-92946x^7+62287x^8-29148x^9+4128x^{10}+648x^{11})$$

**Simplify[Cf[12, 5, 11]]**

[化简]

$$2048 x (1+x)^5 (-238 + 753 x - 6036 x^2 + 11066 x^3 - 26967 x^4 + 30947 x^5 - 31826 x^6 + 26928 x^7 - 10617 x^8 + 2938 x^9 - 140 x^{10} + 24 x^{11})$$

**Simplify[Cf[12, 5, 12]]**

[化简]

$$4096 x (1+x)^5 (-80 + 393 x - 2217 x^2 + 4730 x^3 - 9858 x^4 + 14329 x^5 - 18549 x^6 + 21468 x^7 - 16396 x^8 + 7712 x^9 - 2132 x^{10} + 312 x^{11})$$

**Simplify[Cf[12, 5, 13]]**

[化简]

$$-2048 x (1+x)^5 (30 - 109 x + 767 x^2 - 1588 x^3 + 3006 x^4 - 3343 x^5 + 1303 x^6 - 22 x^7 - 30 x^8 - 26 x^9 + 12 x^{10})$$

**Simplify[Cf[12, 5, 14]]**

[化简]

$$-4096 (-1+x)^2 x^2 (1+x)^5 (7 - 7 x + 96 x^2 - 102 x^3 + 149 x^4 - 111 x^5 + 40 x^6)$$

**(\*, r2^12r3^6\*)****Simplify[Cf[12, 6, 0]]**

[化简]

0

**Simplify[Cf[12, 6, 1]]**

[化简]

0

**Simplify[Cf[12, 6, 2]]**

[化简]

0

**Simplify[Cf[12, 6, 3]]**

[化简]

0

**Simplify[Cf[12, 6, 4]]**

[化简]

$$1024 (-1+x)^2 x^2 (1+x)^5 (-21 - 24 x - 78 x^2 - 328 x^3 + 551 x^4 - 424 x^5 + 148 x^6)$$

**Simplify[Cf[12, 6, 5]]**

[化简]

$$-2048 x (1+x)^5 (30 - 109 x + 767 x^2 - 1588 x^3 + 3006 x^4 - 3343 x^5 + 1303 x^6 - 22 x^7 - 30 x^8 - 26 x^9 + 12 x^{10})$$

**Simplify[Cf[12, 6, 6]]**

[化简]

$$-4096 (1+x)^5 (18 - 180 x + 1349 x^2 - 4492 x^3 + 12813 x^4 - 22478 x^5 + 32069 x^6 - 34832 x^7 + 28217 x^8 - 18466 x^9 + 8598 x^{10} - 2400 x^{11} + 360 x^{12})$$

**Simplify[Cf[12, 6, 7]]**

[化简]

$$-2048 x (1+x)^5 (282 - 791 x + 7232 x^2 - 13452 x^3 + 36789 x^4 - 41995 x^5 + 42522 x^6 - 25450 x^7 + 3219 x^8 + 1336 x^9 - 236 x^{10} + 48 x^{11})$$

**Simplify[Cf[12, 6, 8]]**

[化简]

$$1024 (1+x)^5 (-228 + 2280 x - 17657 x^2 + 55410 x^3 - 175923 x^4 + 316440 x^5 - 538591 x^6 + 605042 x^7 - 527289 x^8 + 312060 x^9 - 106312 x^{10} + 17792 x^{11} + 1104 x^{12})$$

**Simplify[Cf[12, 6, 9]]**

[化简]

$$4096 x (1+x)^5 (-258 + 722 x - 6933 x^2 + 12092 x^3 - 38987 x^4 + 44434 x^5 - 55507 x^6 + 31712 x^7 - 7683 x^8 - 2296 x^9 + 2904 x^{10} + 216 x^{11})$$

**Simplify[Cf[12, 6, 10]]**

[化简]

$$1024 (1+x)^5 (-228 + 2280 x - 17657 x^2 + 55410 x^3 - 175923 x^4 + 316440 x^5 - 538591 x^6 + 605042 x^7 - 527289 x^8 + 312060 x^9 - 106312 x^{10} + 17792 x^{11} + 1104 x^{12})$$

**Simplify[Cf[12, 6, 11]]**

[化简]

$$-2048 x (1+x)^5 (282 - 791 x + 7232 x^2 - 13452 x^3 + 36789 x^4 - 41995 x^5 + 42522 x^6 - 25450 x^7 + 3219 x^8 + 1336 x^9 - 236 x^{10} + 48 x^{11})$$

**Simplify[Cf[12, 6, 12]]**

[化简]

$$-4096 (1+x)^5 (18 - 180 x + 1349 x^2 - 4492 x^3 + 12813 x^4 - 22478 x^5 + 32069 x^6 - 34832 x^7 + 28217 x^8 - 18466 x^9 + 8598 x^{10} - 2400 x^{11} + 360 x^{12})$$

**Simplify[Cf[12, 6, 13]]**

[化简]

$$-2048 x (1+x)^5 (30 - 109 x + 767 x^2 - 1588 x^3 + 3006 x^4 - 3343 x^5 + 1303 x^6 - 22 x^7 - 30 x^8 - 26 x^9 + 12 x^{10})$$

**Simplify[Cf[12, 6, 14]]**

[化简]

$$1024 (-1+x)^2 x^2 (1+x)^5 (-21 - 24 x - 78 x^2 - 328 x^3 + 551 x^4 - 424 x^5 + 148 x^6)$$

**(\*, r2^12r3^7\*)****Simplify[Cf[12, 7, 0]]**

[化简]

0

**Simplify[Cf[12, 7, 1]]**

[化简]

0

**Simplify[Cf[12, 7, 2]]**

[化简]

0

**Simplify[Cf[12, 7, 3]]**

[化简]

$$-2048 (-1+x)^2 x^2 (1+x)^5 (9-14x+132x^2-190x^3+207x^4-180x^5+52x^6)$$

**Simplify[Cf[12, 7, 4]]**

[化简]

$$2048x(1+x)^5 (-22+61x-464x^2+899x^3-1766x^4+2289x^5-1036x^6-11x^7+172x^8-166x^9+44x^{10})$$

**Simplify[Cf[12, 7, 5]]**

[化简]

$$4096x(1+x)^5 (-80+393x-2217x^2+4730x^3-9858x^4+14329x^5-18549x^6+21468x^7-16396x^8+7712x^9-2132x^{10}+312x^{11})$$

**Simplify[Cf[12, 7, 6]]**

[化简]

$$-2048x(1+x)^5 (282-791x+7232x^2-13452x^3+36789x^4-41995x^5+42522x^6-25450x^7+3219x^8+1336x^9-236x^{10}+48x^{11})$$

**Simplify[Cf[12, 7, 7]]**

[化简]

$$-2048x(1+x)^5 (588-2271x+16628x^2-28673x^3+79818x^4-101037x^5+162376x^6-160663x^7+117606x^8-52908x^9+10632x^{10}+528x^{11})$$

**Simplify[Cf[12, 7, 8]]**

[化简]

$$-2048x(1+x)^5 (688-2146x+18920x^2-30213x^3+98031x^4-105466x^5+166870x^6-122025x^7+79547x^8-24214x^9+4344x^{10}+48x^{11})$$

**Simplify[Cf[12, 7, 9]]**

[化简]

$$-2048x(1+x)^5 (688-2146x+18920x^2-30213x^3+98031x^4-105466x^5+166870x^6-122025x^7+79547x^8-24214x^9+4344x^{10}+48x^{11})$$

**Simplify[Cf[12, 7, 10]]**

[化简]

$$-2048x(1+x)^5 (588-2271x+16628x^2-28673x^3+79818x^4-101037x^5+162376x^6-160663x^7+117606x^8-52908x^9+10632x^{10}+528x^{11})$$

**Simplify[Cf[12, 7, 11]]**

[化简]

$$-2048x(1+x)^5 (282-791x+7232x^2-13452x^3+36789x^4-41995x^5+42522x^6-25450x^7+3219x^8+1336x^9-236x^{10}+48x^{11})$$

**Simplify[Cf[12, 7, 12]]**

[化简]

$$4096x(1+x)^5 (-80+393x-2217x^2+4730x^3-9858x^4+14329x^5-18549x^6+21468x^7-16396x^8+7712x^9-2132x^{10}+312x^{11})$$

**Simplify[Cf[12, 7, 13]]**

[化简]

$$2048 x (1+x)^5 (-22 + 61 x - 464 x^2 + 899 x^3 - 1766 x^4 + 2289 x^5 - 1036 x^6 - 11 x^7 + 172 x^8 - 166 x^9 + 44 x^{10})$$

**Simplify[Cf[12, 7, 14]]**

[化简]

$$-2048 (-1+x)^2 x^2 (1+x)^5 (9 - 14 x + 132 x^2 - 190 x^3 + 207 x^4 - 180 x^5 + 52 x^6)$$

(\*, r2^12r3^8\*)

**Simplify[Cf[12, 8, 0]]**

[化简]

0

**Simplify[Cf[12, 8, 1]]**

[化简]

0

**Simplify[Cf[12, 8, 2]]**

[化简]

$$1024 (-1+x)^3 x^2 (1+x)^5 (7 + 19 x + 13 x^2 + 137 x^3 - 172 x^4 + 44 x^5)$$

**Simplify[Cf[12, 8, 3]]**

[化简]

$$-2048 (-1+x)^2 x (1+x)^5 (18 - 53 x + 419 x^2 - 464 x^3 + 1070 x^4 - 399 x^5 + 121 x^6 - 228 x^7 + 60 x^8)$$

**Simplify[Cf[12, 8, 4]]**

[化简]

$$-2048 (1+x)^5 (24 - 240 x + 1755 x^2 - 5836 x^3 + 16193 x^4 - 28994 x^5 + 40829 x^6 - 45928 x^7 + 37615 x^8 - 23738 x^9 + 10784 x^{10} - 2848 x^{11} + 384 x^{12})$$

**Simplify[Cf[12, 8, 5]]**

[化简]

$$2048 x (1+x)^5 (-238 + 753 x - 6036 x^2 + 11066 x^3 - 26967 x^4 + 30947 x^5 - 31826 x^6 + 26928 x^7 - 10617 x^8 + 2938 x^9 - 140 x^{10} + 24 x^{11})$$

**Simplify[Cf[12, 8, 6]]**

[化简]

$$1024 (1+x)^5 (-228 + 2280 x - 17657 x^2 + 55410 x^3 - 175923 x^4 + 316440 x^5 - 538591 x^6 + 605042 x^7 - 527289 x^8 + 312060 x^9 - 106312 x^{10} + 17792 x^{11} + 1104 x^{12})$$

**Simplify[Cf[12, 8, 7]]**

[化简]

$$-2048 x (1+x)^5 (688 - 2146 x + 18920 x^2 - 30213 x^3 + 98031 x^4 - 105466 x^5 + 166870 x^6 - 122025 x^7 + 79547 x^8 - 24214 x^9 + 4344 x^{10} + 48 x^{11})$$

**Simplify[Cf[12, 8, 8]]**

[化简]

$$-12288 (1+x)^5 (30 - 300 x + 2370 x^2 - 7303 x^3 + 24342 x^4 - 43183 x^5 + 79252 x^6 - 86093 x^7 + 80456 x^8 - 44489 x^9 + 16526 x^{10} - 1784 x^{11} + 48 x^{12})$$

**Simplify[Cf[12, 8, 9]]**

[化简]

$$-2048 x (1+x)^5 (688 - 2146 x + 18920 x^2 - 30213 x^3 + 98031 x^4 - 105466 x^5 + 166870 x^6 - 122025 x^7 + 79547 x^8 - 24214 x^9 + 4344 x^{10} + 48 x^{11})$$

**Simplify[Cf[12, 8, 10]]**

[化简]

$$1024 (1+x)^5 (-228 + 2280 x - 17657 x^2 + 55410 x^3 - 175923 x^4 + 316440 x^5 - 538591 x^6 + 605042 x^7 - 527289 x^8 + 312060 x^9 - 106312 x^{10} + 17792 x^{11} + 1104 x^{12})$$

**Simplify[Cf[12, 8, 11]]**

[化简]

$$2048 x (1+x)^5 (-238 + 753 x - 6036 x^2 + 11066 x^3 - 26967 x^4 + 30947 x^5 - 31826 x^6 + 26928 x^7 - 10617 x^8 + 2938 x^9 - 140 x^{10} + 24 x^{11})$$

**Simplify[Cf[12, 8, 12]]**

[化简]

$$-2048 (1+x)^5 (24 - 240 x + 1755 x^2 - 5836 x^3 + 16193 x^4 - 28994 x^5 + 40829 x^6 - 45928 x^7 + 37615 x^8 - 23738 x^9 + 10784 x^{10} - 2848 x^{11} + 384 x^{12})$$

**Simplify[Cf[12, 8, 13]]**

[化简]

$$-2048 (-1+x)^2 x (1+x)^5 (18 - 53 x + 419 x^2 - 464 x^3 + 1070 x^4 - 399 x^5 + 121 x^6 - 228 x^7 + 60 x^8)$$

**Simplify[Cf[12, 8, 14]]**

[化简]

$$1024 (-1+x)^3 x^2 (1+x)^5 (7 + 19 x + 13 x^2 + 137 x^3 - 172 x^4 + 44 x^5)$$

**(\*, r2^12r3^9\*)****Simplify[Cf[12, 9, 0]]**

[化简]

0

**Simplify[Cf[12, 9, 1]]**

[化简]

$$-2048 (-1+x)^4 x^2 (1+x)^5 (2 - 3 x + 30 x^2 - 21 x^3 + 4 x^4)$$

**Simplify[Cf[12, 9, 2]]**

[化简]

$$2048 (-1+x)^3 x (1+x)^5 (6 + 7 x + 89 x^2 + 50 x^3 + 225 x^4 + 197 x^5 - 190 x^6 + 36 x^7)$$

**Simplify[Cf[12, 9, 3]]**

[化简]

$$4096 (-1+x)^2 x (1+x)^5 (-30 + 78 x - 535 x^2 + 314 x^3 - 1370 x^4 + 916 x^5 - 2281 x^6 + 1676 x^7 - 456 x^8 + 72 x^9)$$

**Simplify[Cf[12, 9, 4]]**

[化简]

$$2048 x (1+x)^5 (-142 + 425 x - 3690 x^2 + 8601 x^3 - 21990 x^4 + 31475 x^5 - 28610 x^6 + 17979 x^7 - 2788 x^8 - 648 x^9 - 732 x^{10} + 120 x^{11})$$



**Simplify[Cf[12, 9, 5]]**

|化简

$$-2048 x (1+x)^5 (368 - 1398 x + 9883 x^2 - 17514 x^3 + 44189 x^4 - 58954 x^5 + 85081 x^6 - 92946 x^7 + 62287 x^8 - 29148 x^9 + 4128 x^{10} + 648 x^{11})$$

**Simplify[Cf[12, 9, 6]]**

|化简

$$4096 x (1+x)^5 (-258 + 722 x - 6933 x^2 + 12092 x^3 - 38987 x^4 + 44434 x^5 - 55507 x^6 + 31712 x^7 - 7683 x^8 - 2296 x^9 + 2904 x^{10} + 216 x^{11})$$

**Simplify[Cf[12, 9, 7]]**

|化简

$$-2048 x (1+x)^5 (688 - 2146 x + 18920 x^2 - 30213 x^3 + 98031 x^4 - 105466 x^5 + 166870 x^6 - 122025 x^7 + 79547 x^8 - 24214 x^9 + 4344 x^{10} + 48 x^{11})$$

**Simplify[Cf[12, 9, 8]]**

|化简

$$-2048 x (1+x)^5 (688 - 2146 x + 18920 x^2 - 30213 x^3 + 98031 x^4 - 105466 x^5 + 166870 x^6 - 122025 x^7 + 79547 x^8 - 24214 x^9 + 4344 x^{10} + 48 x^{11})$$

**Simplify[Cf[12, 9, 9]]**

|化简

$$4096 x (1+x)^5 (-258 + 722 x - 6933 x^2 + 12092 x^3 - 38987 x^4 + 44434 x^5 - 55507 x^6 + 31712 x^7 - 7683 x^8 - 2296 x^9 + 2904 x^{10} + 216 x^{11})$$

**Simplify[Cf[12, 9, 10]]**

|化简

$$-2048 x (1+x)^5 (368 - 1398 x + 9883 x^2 - 17514 x^3 + 44189 x^4 - 58954 x^5 + 85081 x^6 - 92946 x^7 + 62287 x^8 - 29148 x^9 + 4128 x^{10} + 648 x^{11})$$

**Simplify[Cf[12, 9, 11]]**

|化简

$$2048 x (1+x)^5 (-142 + 425 x - 3690 x^2 + 8601 x^3 - 21990 x^4 + 31475 x^5 - 28610 x^6 + 17979 x^7 - 2788 x^8 - 648 x^9 - 732 x^{10} + 120 x^{11})$$

**Simplify[Cf[12, 9, 12]]**

|化简

$$4096 (-1+x)^2 x (1+x)^5 (-30 + 78 x - 535 x^2 + 314 x^3 - 1370 x^4 + 916 x^5 - 2281 x^6 + 1676 x^7 - 456 x^8 + 72 x^9)$$

**Simplify[Cf[12, 9, 13]]**

|化简

$$2048 (-1+x)^3 x (1+x)^5 (6 + 7 x + 89 x^2 + 50 x^3 + 225 x^4 + 197 x^5 - 190 x^6 + 36 x^7)$$

**Simplify[Cf[12, 9, 14]]**

|化简

$$-2048 (-1+x)^4 x^2 (1+x)^5 (2 - 3 x + 30 x^2 - 21 x^3 + 4 x^4)$$

**(\*, r2^12r3^10\*)**

**Simplify[Cf[12, 10, 0]]**

[化简]

$$4096 x^3 (-1 + x^2)^5$$

**Simplify[Cf[12, 10, 1]]**

[化简]

$$-2048 (-1 + x)^4 x (1 + x)^5 (4 - 12x + 75x^2 - 52x^3 + 165x^4 - 56x^5 + 8x^6)$$

**Simplify[Cf[12, 10, 2]]**

[化简]

$$-4096 (-1 + x)^3 (1 + x)^5 (-3 + 21x - 131x^2 + 203x^3 - 650x^4 + 431x^5 - 1014x^6 + 363x^7 - 60x^8 + 12x^9)$$

**Simplify[Cf[12, 10, 3]]**

[化简]

$$-2048 (-1 + x)^2 x (1 + x)^5 (78 - 134x + 1447x^2 - 514x^3 + 4130x^4 - 744x^5 + 4349x^6 - 600x^7 - 1020x^8 + 144x^9)$$

**Simplify[Cf[12, 10, 4]]**

[化简]

$$2048 (1 + x)^5 (-48 + 480x - 3555x^2 + 11338x^3 - 33289x^4 + 62324x^5 - 98829x^6 + 119218x^7 - 99767x^8 + 59360x^9 - 17520x^{10} - 240x^{11} + 528x^{12})$$

**Simplify[Cf[12, 10, 5]]**

[化简]

$$-2048 x (1 + x)^5 (368 - 1398x + 9883x^2 - 17514x^3 + 44189x^4 - 58954x^5 + 85081x^6 - 92946x^7 + 62287x^8 - 29148x^9 + 4128x^{10} + 648x^{11})$$

**Simplify[Cf[12, 10, 6]]**

[化简]

$$1024 (1 + x)^5 (-228 + 2280x - 17657x^2 + 55410x^3 - 175923x^4 + 316440x^5 - 538591x^6 + 605042x^7 - 527289x^8 + 312060x^9 - 106312x^{10} + 17792x^{11} + 1104x^{12})$$

**Simplify[Cf[12, 10, 7]]**

[化简]

$$-2048 x (1 + x)^5 (588 - 2271x + 16628x^2 - 28673x^3 + 79818x^4 - 101037x^5 + 162376x^6 - 160663x^7 + 117606x^8 - 52908x^9 + 10632x^{10} + 528x^{11})$$

**Simplify[Cf[12, 10, 8]]**

[化简]

$$1024 (1 + x)^5 (-228 + 2280x - 17657x^2 + 55410x^3 - 175923x^4 + 316440x^5 - 538591x^6 + 605042x^7 - 527289x^8 + 312060x^9 - 106312x^{10} + 17792x^{11} + 1104x^{12})$$

**Simplify[Cf[12, 10, 9]]**

[化简]

$$-2048 x (1 + x)^5 (368 - 1398x + 9883x^2 - 17514x^3 + 44189x^4 - 58954x^5 + 85081x^6 - 92946x^7 + 62287x^8 - 29148x^9 + 4128x^{10} + 648x^{11})$$

**Simplify[Cf[12, 10, 10]]**

[化简]

$$2048 (1+x)^5 (-48 + 480x - 3555x^2 + 11338x^3 - 33289x^4 + 62324x^5 - 98829x^6 + 119218x^7 - 99767x^8 + 59360x^9 - 17520x^{10} - 240x^{11} + 528x^{12})$$

**Simplify[Cf[12, 10, 11]]**

[化简]

$$-2048 (-1+x)^2 x (1+x)^5 (78 - 134x + 1447x^2 - 514x^3 + 4130x^4 - 744x^5 + 4349x^6 - 600x^7 - 1020x^8 + 144x^9)$$

**Simplify[Cf[12, 10, 12]]**

[化简]

$$-4096 (-1+x)^3 (1+x)^5 (-3 + 21x - 131x^2 + 203x^3 - 650x^4 + 431x^5 - 1014x^6 + 363x^7 - 60x^8 + 12x^9)$$

**Simplify[Cf[12, 10, 13]]**

[化简]

$$-2048 (-1+x)^4 x (1+x)^5 (4 - 12x + 75x^2 - 52x^3 + 165x^4 - 56x^5 + 8x^6)$$

**Simplify[Cf[12, 10, 14]]**

[化简]

$$4096 x^3 (-1+x^2)^5$$

**(\*, r2^12r3^11\*)****Simplify[Cf[12, 11, 0]]**

[化简]

$$2048 x^2 (-1+x^2)^5 (2 + 3x + 7x^2 + 2x^3)$$

**Simplify[Cf[12, 11, 1]]**

[化简]

$$4096 (-1+x)^4 x (1+x)^5 (-2 - 4x - 15x^2 - 84x^3 - 23x^4 - 60x^5 + 12x^6)$$

**Simplify[Cf[12, 11, 2]]**

[化简]

$$2048 (-1+x)^3 x (1+x)^5 (24 - 31x + 565x^2 - 483x^3 + 2171x^4 - 538x^5 + 1316x^6 - 552x^7 + 48x^8)$$

**Simplify[Cf[12, 11, 3]]**

[化简]

$$-2048 (-1+x)^2 x (1+x)^5 (78 - 134x + 1447x^2 - 514x^3 + 4130x^4 - 744x^5 + 4349x^6 - 600x^7 - 1020x^8 + 144x^9)$$

**Simplify[Cf[12, 11, 4]]**

[化简]

$$2048 x (1+x)^5 (-142 + 425x - 3690x^2 + 8601x^3 - 21990x^4 + 31475x^5 - 28610x^6 + 17979x^7 - 2788x^8 - 648x^9 - 732x^{10} + 120x^{11})$$

**Simplify[Cf[12, 11, 5]]**

[化简]

$$2048 x (1+x)^5 (-238 + 753x - 6036x^2 + 11066x^3 - 26967x^4 + 30947x^5 - 31826x^6 + 26928x^7 - 10617x^8 + 2938x^9 - 140x^{10} + 24x^{11})$$

**Simplify[Cf[12, 11, 6]]**

[化简]

$$-2048 x (1+x)^5 (282 - 791 x + 7232 x^2 - 13452 x^3 + 36789 x^4 - 41995 x^5 + 42522 x^6 - 25450 x^7 + 3219 x^8 + 1336 x^9 - 236 x^{10} + 48 x^{11})$$

**Simplify[Cf[12, 11, 7]]**

[化简]

$$-2048 x (1+x)^5 (282 - 791 x + 7232 x^2 - 13452 x^3 + 36789 x^4 - 41995 x^5 + 42522 x^6 - 25450 x^7 + 3219 x^8 + 1336 x^9 - 236 x^{10} + 48 x^{11})$$

**Simplify[Cf[12, 11, 8]]**

[化简]

$$2048 x (1+x)^5 (-238 + 753 x - 6036 x^2 + 11066 x^3 - 26967 x^4 + 30947 x^5 - 31826 x^6 + 26928 x^7 - 10617 x^8 + 2938 x^9 - 140 x^{10} + 24 x^{11})$$

**Simplify[Cf[12, 11, 9]]**

[化简]

$$2048 x (1+x)^5 (-142 + 425 x - 3690 x^2 + 8601 x^3 - 21990 x^4 + 31475 x^5 - 28610 x^6 + 17979 x^7 - 2788 x^8 - 648 x^9 - 732 x^{10} + 120 x^{11})$$

**Simplify[Cf[12, 11, 10]]**

[化简]

$$-2048 (-1+x)^2 x (1+x)^5 (78 - 134 x + 1447 x^2 - 514 x^3 + 4130 x^4 - 744 x^5 + 4349 x^6 - 600 x^7 - 1020 x^8 + 144 x^9)$$

**Simplify[Cf[12, 11, 11]]**

[化简]

$$2048 (-1+x)^3 x (1+x)^5 (24 - 31 x + 565 x^2 - 483 x^3 + 2171 x^4 - 538 x^5 + 1316 x^6 - 552 x^7 + 48 x^8)$$

**Simplify[Cf[12, 11, 12]]**

[化简]

$$4096 (-1+x)^4 x (1+x)^5 (-2 - 4 x - 15 x^2 - 84 x^3 - 23 x^4 - 60 x^5 + 12 x^6)$$

**Simplify[Cf[12, 11, 13]]**

[化简]

$$2048 x^2 (-1+x^2)^5 (2 + 3 x + 7 x^2 + 2 x^3)$$

**Simplify[Cf[12, 11, 14]]**

[化简]

0

**(\*, r2^12r3^12\*)****Simplify[Cf[12, 12, 0]]**

[化简]

$$12288 x^3 (-1+x^2)^5 (3 - x + 2 x^2)$$

**Simplify[Cf[12, 12, 1]]**

[化简]

$$4096 (-1+x)^4 x (1+x)^5 (-2 - 4 x - 15 x^2 - 84 x^3 - 23 x^4 - 60 x^5 + 12 x^6)$$

**Simplify[Cf[12, 12, 2]]**

[化简]

$$-4096 (-1+x)^3 (1+x)^5 \\ (-3+21x-131x^2+203x^3-650x^4+431x^5-1014x^6+363x^7-60x^8+12x^9)$$

**Simplify[Cf[12, 12, 3]]**

[化简]

$$4096 (-1+x)^2 x (1+x)^5 \\ (-30+78x-535x^2+314x^3-1370x^4+916x^5-2281x^6+1676x^7-456x^8+72x^9)$$

**Simplify[Cf[12, 12, 4]]**

[化简]

$$-2048 (1+x)^5 (24-240x+1755x^2-5836x^3+16193x^4-28994x^5+ \\ 40829x^6-45928x^7+37615x^8-23738x^9+10784x^{10}-2848x^{11}+384x^{12})$$

**Simplify[Cf[12, 12, 5]]**

[化简]

$$4096 x (1+x)^5 (-80+393x-2217x^2+4730x^3-9858x^4+ \\ 14329x^5-18549x^6+21468x^7-16396x^8+7712x^9-2132x^{10}+312x^{11})$$

**Simplify[Cf[12, 12, 6]]**

[化简]

$$-4096 (1+x)^5 (18-180x+1349x^2-4492x^3+12813x^4-22478x^5+ \\ 32069x^6-34832x^7+28217x^8-18466x^9+8598x^{10}-2400x^{11}+360x^{12})$$

**Simplify[Cf[12, 12, 7]]**

[化简]

$$4096 x (1+x)^5 (-80+393x-2217x^2+4730x^3-9858x^4+ \\ 14329x^5-18549x^6+21468x^7-16396x^8+7712x^9-2132x^{10}+312x^{11})$$

**Simplify[Cf[12, 12, 8]]**

[化简]

$$-2048 (1+x)^5 (24-240x+1755x^2-5836x^3+16193x^4-28994x^5+ \\ 40829x^6-45928x^7+37615x^8-23738x^9+10784x^{10}-2848x^{11}+384x^{12})$$

**Simplify[Cf[12, 12, 9]]**

[化简]

$$4096 (-1+x)^2 x (1+x)^5 \\ (-30+78x-535x^2+314x^3-1370x^4+916x^5-2281x^6+1676x^7-456x^8+72x^9)$$

**Simplify[Cf[12, 12, 10]]**

[化简]

$$-4096 (-1+x)^3 (1+x)^5 \\ (-3+21x-131x^2+203x^3-650x^4+431x^5-1014x^6+363x^7-60x^8+12x^9)$$

**Simplify[Cf[12, 12, 11]]**

[化简]

$$4096 (-1+x)^4 x (1+x)^5 (-2-4x-15x^2-84x^3-23x^4-60x^5+12x^6)$$

**Simplify[Cf[12, 12, 12]]**

[化简]

$$12\,288\,x^3\left(-1+x^2\right)^5\left(3-x+2\,x^2\right)$$

**Simplify[Cf[12, 12, 13]]**

[化简]

$$0$$

**Simplify[Cf[12, 12, 14]]**

[化简]

$$0$$

**(\*, r2^12r3^13\*)**

**Simplify[Cf[12, 13, 0]]**

[化简]

$$2048\,x^2\left(-1+x^2\right)^5\left(2+3\,x+7\,x^2+2\,x^3\right)$$

**Simplify[Cf[12, 13, 1]]**

[化简]

$$-2048\left(-1+x\right)^4x\left(1+x\right)^5\left(4-12\,x+75\,x^2-52\,x^3+165\,x^4-56\,x^5+8\,x^6\right)$$

**Simplify[Cf[12, 13, 2]]**

[化简]

$$2048\left(-1+x\right)^3x\left(1+x\right)^5\left(6+7\,x+89\,x^2+50\,x^3+225\,x^4+197\,x^5-190\,x^6+36\,x^7\right)$$

**Simplify[Cf[12, 13, 3]]**

[化简]

$$-2048\left(-1+x\right)^2x\left(1+x\right)^5\left(18-53\,x+419\,x^2-464\,x^3+1070\,x^4-399\,x^5+121\,x^6-228\,x^7+60\,x^8\right)$$

**Simplify[Cf[12, 13, 4]]**

[化简]

$$2048\,x\left(1+x\right)^5\left(-22+61\,x-464\,x^2+899\,x^3-1766\,x^4+2289\,x^5-1036\,x^6-11\,x^7+172\,x^8-166\,x^9+44\,x^{10}\right)$$

**Simplify[Cf[12, 13, 5]]**

[化简]

$$-2048\,x\left(1+x\right)^5\left(30-109\,x+767\,x^2-1588\,x^3+3006\,x^4-3343\,x^5+1303\,x^6-22\,x^7-30\,x^8-26\,x^9+12\,x^{10}\right)$$

**Simplify[Cf[12, 13, 6]]**

[化简]

$$-2048\,x\left(1+x\right)^5\left(30-109\,x+767\,x^2-1588\,x^3+3006\,x^4-3343\,x^5+1303\,x^6-22\,x^7-30\,x^8-26\,x^9+12\,x^{10}\right)$$

**Simplify[Cf[12, 13, 7]]**

[化简]

$$2048\,x\left(1+x\right)^5\left(-22+61\,x-464\,x^2+899\,x^3-1766\,x^4+2289\,x^5-1036\,x^6-11\,x^7+172\,x^8-166\,x^9+44\,x^{10}\right)$$

**Simplify[Cf[12, 13, 8]]**

[化简]

$$-2048 (-1+x)^2 x (1+x)^5 (18-53x+419x^2-464x^3+1070x^4-399x^5+121x^6-228x^7+60x^8)$$

**Simplify[Cf[12, 13, 9]]**

[化简]

$$2048 (-1+x)^3 x (1+x)^5 (6+7x+89x^2+50x^3+225x^4+197x^5-190x^6+36x^7)$$

**Simplify[Cf[12, 13, 10]]**

[化简]

$$-2048 (-1+x)^4 x (1+x)^5 (4-12x+75x^2-52x^3+165x^4-56x^5+8x^6)$$

**Simplify[Cf[12, 13, 11]]**

[化简]

$$2048 x^2 (-1+x^2)^5 (2+3x+7x^2+2x^3)$$

**Simplify[Cf[12, 13, 12]]**

[化简]

0

**Simplify[Cf[12, 13, 13]]**

[化简]

0

**Simplify[Cf[12, 13, 14]]**

[化简]

0

**(\*, r2^12r3^14\*)****Simplify[Cf[12, 14, 0]]**

[化简]

$$4096 x^3 (-1+x^2)^5$$

**Simplify[Cf[12, 14, 1]]**

[化简]

$$-2048 (-1+x)^4 x^2 (1+x)^5 (2-3x+30x^2-21x^3+4x^4)$$

**Simplify[Cf[12, 14, 2]]**

[化简]

$$1024 (-1+x)^2 x^2 (1+x)^5 (-7-12x+6x^2-124x^3+309x^4-216x^5+44x^6)$$

**Simplify[Cf[12, 14, 3]]**

[化简]

$$-2048 (-1+x)^2 x^2 (1+x)^5 (9-14x+132x^2-190x^3+207x^4-180x^5+52x^6)$$

**Simplify[Cf[12, 14, 4]]**

[化简]

$$1024 (-1+x)^2 x^2 (1+x)^5 (-21-24x-78x^2-328x^3+551x^4-424x^5+148x^6)$$

**Simplify[Cf[12, 14, 5]]**

[\[化简\]](#)

$$-4096 (-1+x)^2 x^2 (1+x)^5 (7-7x+96x^2-102x^3+149x^4-111x^5+40x^6)$$

**Simplify[Cf[12, 14, 6]]**

[\[化简\]](#)

$$1024 (-1+x)^2 x^2 (1+x)^5 (-21-24x-78x^2-328x^3+551x^4-424x^5+148x^6)$$

**Simplify[Cf[12, 14, 7]]**

[\[化简\]](#)

$$-2048 (-1+x)^2 x^2 (1+x)^5 (9-14x+132x^2-190x^3+207x^4-180x^5+52x^6)$$

**Simplify[Cf[12, 14, 8]]**

[\[化简\]](#)

$$1024 (-1+x)^2 x^2 (1+x)^5 (-7-12x+6x^2-124x^3+309x^4-216x^5+44x^6)$$

**Simplify[Cf[12, 14, 9]]**

[\[化简\]](#)

$$-2048 (-1+x)^4 x^2 (1+x)^5 (2-3x+30x^2-21x^3+4x^4)$$

**Simplify[Cf[12, 14, 10]]**

[\[化简\]](#)

$$4096 x^3 (-1+x^2)^5$$

**Simplify[Cf[12, 14, 11]]**

[\[化简\]](#)

0

**Simplify[Cf[12, 14, 12]]**

[\[化简\]](#)

0

**Simplify[Cf[12, 14, 13]]**

[\[化简\]](#)

0

**Simplify[Cf[12, 14, 14]]**

[\[化简\]](#)

0

**(\*, r2^13r3^0\*)**

**Simplify[Cf[13, 0, 0]]**

[\[化简\]](#)

0

**Simplify[Cf[13, 0, 1]]**

[\[化简\]](#)

0



**Simplify[Cf[13, 0, 2]]**

[化简]

0

**Simplify[Cf[13, 0, 3]]**

[化简]

0

**Simplify[Cf[13, 0, 4]]**

[化简]

0

**Simplify[Cf[13, 0, 5]]**

[化简]

0

**Simplify[Cf[13, 0, 6]]**

[化简]

0

**Simplify[Cf[13, 0, 7]]**

[化简]

0

**Simplify[Cf[13, 0, 8]]**

[化简]

0

**Simplify[Cf[13, 0, 9]]**

[化简]

$-2048 (-1 + x) x^3 (-1 + x^2)^5$

**Simplify[Cf[13, 0, 10]]**

[化简]

$-4096 x^2 (-1 + x^2)^5 (-1 + x - 3 x^2 + x^3)$

**Simplify[Cf[13, 0, 11]]**

[化简]

$2048 x^2 (-1 + x^2)^5 (2 + 3 x + 7 x^2 + 2 x^3)$

**Simplify[Cf[13, 0, 12]]**

[化简]

$2048 x^2 (-1 + x^2)^5 (2 + 3 x + 7 x^2 + 2 x^3)$

**Simplify[Cf[13, 0, 13]]**

[化简]

$-4096 x^2 (-1 + x^2)^5 (-1 + x - 3 x^2 + x^3)$

**Simplify[Cf[13, 0, 14]]**

[化简]

$-2048 (-1 + x) x^3 (-1 + x^2)^5$

(\*, r2^13r3^1\*)

**Simplify**[Cf[13, 1, 0]]

[化简]

0

**Simplify**[Cf[13, 1, 1]]

[化简]

0

**Simplify**[Cf[13, 1, 2]]

[化简]

0

**Simplify**[Cf[13, 1, 3]]

[化简]

0

**Simplify**[Cf[13, 1, 4]]

[化简]

0

**Simplify**[Cf[13, 1, 5]]

[化简]

0

**Simplify**[Cf[13, 1, 6]]

[化简]

0

**Simplify**[Cf[13, 1, 7]]

[化简]

0

**Simplify**[Cf[13, 1, 8]]

[化简]

$6144 (-1 + x)^5 x^3 (1 + x)^6$

**Simplify**[Cf[13, 1, 9]]

[化简]

$8192 (-1 + x)^4 x^2 (1 + x)^5 (-2 + 3x - 13x^2 + 6x^3)$

**Simplify**[Cf[13, 1, 10]]

[化简]

$-2048 (-1 + x)^4 x (1 + x)^5 (4 - 12x + 75x^2 - 52x^3 + 165x^4 - 56x^5 + 8x^6)$

**Simplify**[Cf[13, 1, 11]]

[化简]

$8192 (-1 + x)^4 x^2 (1 + x)^5 (-6 + 8x - 41x^2 - 3x^3 - 16x^4 + 4x^5)$

**Simplify[Cf[13, 1, 12]]**

[化简]

$$-2048 (-1+x)^4 x (1+x)^5 (4-12x+75x^2-52x^3+165x^4-56x^5+8x^6)$$

**Simplify[Cf[13, 1, 13]]**

[化简]

$$8192 (-1+x)^4 x^2 (1+x)^5 (-2+3x-13x^2+6x^3)$$

**Simplify[Cf[13, 1, 14]]**

[化简]

$$6144 (-1+x)^5 x^3 (1+x)^6$$

**(\*, r2^13r3^2\*)**

**Simplify[Cf[13, 2, 0]]**

[化简]

0

**Simplify[Cf[13, 2, 1]]**

[化简]

0

**Simplify[Cf[13, 2, 2]]**

[化简]

0

**Simplify[Cf[13, 2, 3]]**

[化简]

0

**Simplify[Cf[13, 2, 4]]**

[化简]

0

**Simplify[Cf[13, 2, 3]]**

[化简]

0

**Simplify[Cf[13, 2, 4]]**

[化简]

0

**Simplify[Cf[13, 2, 5]]**

[化简]

0

**Simplify[Cf[13, 2, 6]]**

[化简]

0

**Simplify[Cf[13, 2, 7]]**

[\[化简\]](#)

$$-12288 (-1+x)^4 x^3 (1+x)^6$$

**Simplify[Cf[13, 2, 8]]**

[\[化简\]](#)

$$2048 (-1+x)^3 x^2 (1+x)^5 (15-x+23x^2+135x^3-158x^4+34x^5)$$

**Simplify[Cf[13, 2, 9]]**

[\[化简\]](#)

$$2048 (-1+x)^3 x (1+x)^5 (6+7x+89x^2+50x^3+225x^4+197x^5-190x^6+36x^7)$$

**Simplify[Cf[13, 2, 10]]**

[\[化简\]](#)

$$-2048 (-1+x)^3 x (1+x)^5 (-6-34x-84x^2-195x^3-332x^4-521x^5+92x^6+36x^7)$$

**Simplify[Cf[13, 2, 11]]**

[\[化简\]](#)

$$-2048 (-1+x)^3 x (1+x)^5 (-6-34x-84x^2-195x^3-332x^4-521x^5+92x^6+36x^7)$$

**Simplify[Cf[13, 2, 12]]**

[\[化简\]](#)

$$2048 (-1+x)^3 x (1+x)^5 (6+7x+89x^2+50x^3+225x^4+197x^5-190x^6+36x^7)$$

**Simplify[Cf[13, 2, 13]]**

[\[化简\]](#)

$$2048 (-1+x)^3 x^2 (1+x)^5 (15-x+23x^2+135x^3-158x^4+34x^5)$$

**Simplify[Cf[13, 2, 14]]**

[\[化简\]](#)

$$-12288 (-1+x)^4 x^3 (1+x)^6$$

**(\*, r2^13r3^3\*)**

**Simplify[Cf[13, 3, 0]]**

[\[化简\]](#)

0

**Simplify[Cf[13, 3, 1]]**

[\[化简\]](#)

0

**Simplify[Cf[13, 3, 2]]**

[\[化简\]](#)

0

**Simplify[Cf[13, 3, 3]]**

[\[化简\]](#)

0

**Simplify[Cf[13, 3, 4]]**

[\[化简\]](#)

0

**Simplify[Cf[13, 3, 5]]**

[\[化简\]](#)

0

**Simplify[Cf[13, 3, 6]]**

[\[化简\]](#)

$$-4096 (-1+x)^3 x^3 (1+x)^5 (-5-3x^2+4x^3)$$

**Simplify[Cf[13, 3, 7]]**

[\[化简\]](#)

$$-4096 (-1+x)^2 x^2 (1+x)^5 (15-34x+152x^2-202x^3+221x^4-188x^5+52x^6)$$

**Simplify[Cf[13, 3, 8]]**

[\[化简\]](#)

$$-2048 (-1+x)^2 x (1+x)^5 (18-53x+419x^2-464x^3+1070x^4-399x^5+121x^6-228x^7+60x^8)$$

**Simplify[Cf[13, 3, 9]]**

[\[化简\]](#)

$$4096 (-1+x)^2 x^2 (1+x)^5 (-120+337x-1408x^2+1558x^3-2044x^4+597x^5+4x^6+36x^7)$$

**Simplify[Cf[13, 3, 10]]**

[\[化简\]](#)

$$-4096 (-1+x)^2 x (1+x)^5 (18-53x+523x^2-704x^3+2078x^4-1455x^5+1921x^6-772x^7+12x^8)$$

**Simplify[Cf[13, 3, 11]]**

[\[化简\]](#)

$$4096 (-1+x)^2 x^2 (1+x)^5 (-120+337x-1408x^2+1558x^3-2044x^4+597x^5+4x^6+36x^7)$$

**Simplify[Cf[13, 3, 12]]**

[\[化简\]](#)

$$-2048 (-1+x)^2 x (1+x)^5 (18-53x+419x^2-464x^3+1070x^4-399x^5+121x^6-228x^7+60x^8)$$

**Simplify[Cf[13, 3, 13]]**

[\[化简\]](#)

$$-4096 (-1+x)^2 x^2 (1+x)^5 (15-34x+152x^2-202x^3+221x^4-188x^5+52x^6)$$

**Simplify[Cf[13, 3, 14]]**

[\[化简\]](#)

$$-4096 (-1+x)^3 x^3 (1+x)^5 (-5-3x^2+4x^3)$$

**(\*, r2^13r3^4\*)**

**Simplify[Cf[13, 4, 0]]**

[\[化简\]](#)

0

**Simplify[Cf[13, 4, 1]]**

[\[化简\]](#)

0

**Simplify[Cf[13, 4, 2]]**

[\[化简\]](#)

0

**Simplify[Cf[13, 4, 3]]**

[\[化简\]](#)

0

**Simplify[Cf[13, 4, 4]]**

[\[化简\]](#)

0

**Simplify[Cf[13, 4, 5]]**

[\[化简\]](#)

$$12\,288 \left(-1+x\right)^3 x^3 \left(1+x\right)^5 \left(2+x+x^3\right)$$

**Simplify[Cf[13, 4, 6]]**

[\[化简\]](#)

$$2048 \left(-1+x\right)^2 x^2 \left(1+x\right)^5 \left(-35+16 x-90 x^2-364 x^3+597 x^4-460 x^5+160 x^6\right)$$

**Simplify[Cf[13, 4, 7]]**

[\[化简\]](#)

$$2048 x \left(1+x\right)^5 \left(-22+61 x-464 x^2+899 x^3-1766 x^4+2289 x^5-1036 x^6-11 x^7+172 x^8-166 x^9+44 x^{10}\right)$$

**Simplify[Cf[13, 4, 8]]**

[\[化简\]](#)

$$-2048 x \left(1+x\right)^5 \left(24+71 x+389 x^2-1171 x^3+5567 x^4-11\,413 x^5+13\,431 x^6-11\,365 x^7+5741 x^8-1562 x^9+288 x^{10}\right)$$

**Simplify[Cf[13, 4, 9]]**

[\[化简\]](#)

$$2048 x \left(1+x\right)^5 \left(-46+21 x-971 x^2+1647 x^3-5249 x^4+6783 x^5-3145 x^6-1271 x^7+4655 x^8-2668 x^9+244 x^{10}\right)$$

**Simplify[Cf[13, 4, 10]]**

[\[化简\]](#)

$$2048 x \left(1+x\right)^5 \left(-46+21 x-971 x^2+1647 x^3-5249 x^4+6783 x^5-3145 x^6-1271 x^7+4655 x^8-2668 x^9+244 x^{10}\right)$$

**Simplify[Cf[13, 4, 11]]**

[\[化简\]](#)

$$-2048 x \left(1+x\right)^5 \left(24+71 x+389 x^2-1171 x^3+5567 x^4-11\,413 x^5+13\,431 x^6-11\,365 x^7+5741 x^8-1562 x^9+288 x^{10}\right)$$

**Simplify[Cf[13, 4, 12]]**

[化简]

$$2048 x (1+x)^5 (-22 + 61 x - 464 x^2 + 899 x^3 - 1766 x^4 + 2289 x^5 - 1036 x^6 - 11 x^7 + 172 x^8 - 166 x^9 + 44 x^{10})$$

**Simplify[Cf[13, 4, 13]]**

[化简]

$$2048 (-1+x)^2 x^2 (1+x)^5 (-35 + 16 x - 90 x^2 - 364 x^3 + 597 x^4 - 460 x^5 + 160 x^6)$$

**Simplify[Cf[13, 4, 14]]**

[化简]

$$12288 (-1+x)^3 x^3 (1+x)^5 (2+x+x^3)$$

(\*, r2^13r3^5\*)

**Simplify[Cf[13, 5, 0]]**

[化简]

0

**Simplify[Cf[13, 5, 1]]**

[化简]

0

**Simplify[Cf[13, 5, 2]]**

[化简]

0

**Simplify[Cf[13, 5, 3]]**

[化简]

0

**Simplify[Cf[13, 5, 4]]**

[化简]

$$12288 (-1+x)^3 x^3 (1+x)^5 (2+x+x^3)$$

**Simplify[Cf[13, 5, 5]]**

[化简]

$$-8192 (-1+x)^2 x^2 (1+x)^5 (11 - 20 x + 108 x^2 - 112 x^3 + 161 x^4 - 120 x^5 + 44 x^6)$$

**Simplify[Cf[13, 5, 6]]**

[化简]

$$-2048 x (1+x)^5 (30 - 109 x + 767 x^2 - 1588 x^3 + 3006 x^4 - 3343 x^5 + 1303 x^6 - 22 x^7 - 30 x^8 - 26 x^9 + 12 x^{10})$$

**Simplify[Cf[13, 5, 7]]**

[化简]

$$4096 x^2 (1+x)^5 (-299 + 1352 x - 5616 x^2 + 11877 x^3 - 18447 x^4 + 19478 x^5 - 12818 x^6 + 5737 x^7 - 1796 x^8 + 340 x^9)$$

**Simplify[Cf[13, 5, 8]]**

[化简]

$$-2048 x (1+x)^5 (94 - 303 x + 3119 x^2 - 6866 x^3 + 17814 x^4 - 22905 x^5 + 21615 x^6 - 15272 x^7 + 5986 x^8 - 1982 x^9 + 236 x^{10})$$

**Simplify[Cf[13, 5, 9]]**

[化简]

$$-8192 x^2 (1+x)^5 (279 - 1252 x + 5397 x^2 - 10826 x^3 + 16897 x^4 - 16812 x^5 + 10319 x^6 - 3486 x^7 - 156 x^8 + 216 x^9)$$

**Simplify[Cf[13, 5, 10]]**

[化简]

$$-2048 x (1+x)^5 (94 - 303 x + 3119 x^2 - 6866 x^3 + 17814 x^4 - 22905 x^5 + 21615 x^6 - 15272 x^7 + 5986 x^8 - 1982 x^9 + 236 x^{10})$$

**Simplify[Cf[13, 5, 11]]**

[化简]

$$4096 x^2 (1+x)^5 (-299 + 1352 x - 5616 x^2 + 11877 x^3 - 18447 x^4 + 19478 x^5 - 12818 x^6 + 5737 x^7 - 1796 x^8 + 340 x^9)$$

**Simplify[Cf[13, 5, 12]]**

[化简]

$$-2048 x (1+x)^5 (30 - 109 x + 767 x^2 - 1588 x^3 + 3006 x^4 - 3343 x^5 + 1303 x^6 - 22 x^7 - 30 x^8 - 26 x^9 + 12 x^{10})$$

**Simplify[Cf[13, 5, 13]]**

[化简]

$$-8192 (-1+x)^2 x^2 (1+x)^5 (11 - 20 x + 108 x^2 - 112 x^3 + 161 x^4 - 120 x^5 + 44 x^6)$$

**Simplify[Cf[13, 5, 14]]**

[化简]

$$12288 (-1+x)^3 x^3 (1+x)^5 (2+x+x^3)$$

**(\*, r2^13r3^6\*)****Simplify[Cf[13, 6, 0]]**

[化简]

0

**Simplify[Cf[13, 6, 1]]**

[化简]

0

**Simplify[Cf[13, 6, 2]]**

[化简]

0

**Simplify[Cf[13, 6, 3]]**

[化简]

$$-4096 (-1+x)^3 x^3 (1+x)^5 (-5 - 3 x^2 + 4 x^3)$$



**Simplify[Cf[13, 6, 4]]**

[化简]

$$2048 (-1+x)^2 x^2 (1+x)^5 (-35+16x-90x^2-364x^3+597x^4-460x^5+160x^6)$$

**Simplify[Cf[13, 6, 5]]**

[化简]

$$-2048x(1+x)^5 (30-109x+767x^2-1588x^3+3006x^4-3343x^5+1303x^6-22x^7-30x^8-26x^9+12x^{10})$$

**Simplify[Cf[13, 6, 6]]**

[化简]

$$-4096x(1+x)^5 (18+57x+380x^2-1128x^3+5543x^4-10971x^5+14182x^6-12722x^7+6857x^8-2276x^9+444x^{10})$$

**Simplify[Cf[13, 6, 7]]**

[化简]

$$2048x(1+x)^5 (-102+188x-2949x^2+5328x^3-16599x^4+19224x^5-17363x^6+8556x^7-391x^8-560x^9+60x^{10})$$

**Simplify[Cf[13, 6, 8]]**

[化简]

$$2048x(1+x)^5 (-108-12x-3006x^2+5481x^3-23953x^4+31960x^5-38556x^6+27749x^7-12817x^8+2438x^9+840x^{10})$$

**Simplify[Cf[13, 6, 9]]**

[化简]

$$2048x(1+x)^5 (-108-12x-3006x^2+5481x^3-23953x^4+31960x^5-38556x^6+27749x^7-12817x^8+2438x^9+840x^{10})$$

**Simplify[Cf[13, 6, 10]]**

[化简]

$$2048x(1+x)^5 (-102+188x-2949x^2+5328x^3-16599x^4+19224x^5-17363x^6+8556x^7-391x^8-560x^9+60x^{10})$$

**Simplify[Cf[13, 6, 11]]**

[化简]

$$-4096x(1+x)^5 (18+57x+380x^2-1128x^3+5543x^4-10971x^5+14182x^6-12722x^7+6857x^8-2276x^9+444x^{10})$$

**Simplify[Cf[13, 6, 12]]**

[化简]

$$-2048x(1+x)^5 (30-109x+767x^2-1588x^3+3006x^4-3343x^5+1303x^6-22x^7-30x^8-26x^9+12x^{10})$$

**Simplify[Cf[13, 6, 13]]**

[化简]

$$2048 (-1+x)^2 x^2 (1+x)^5 (-35+16x-90x^2-364x^3+597x^4-460x^5+160x^6)$$

**Simplify[Cf[13, 6, 14]]**

[化简]

$$-4096(-1+x)^3 x^3 (1+x)^5 (-5-3x^2+4x^3)$$

(\*, r2^13r3^7\*)

**Simplify[Cf[13, 7, 0]]**

[\[化简\]](#)

0

**Simplify[Cf[13, 7, 1]]**

[\[化简\]](#)

0

**Simplify[Cf[13, 7, 2]]**

[\[化简\]](#)

$$-12\,288 (-1+x)^4 x^3 (1+x)^6$$

**Simplify[Cf[13, 7, 3]]**

[\[化简\]](#)

$$-4096 (-1+x)^2 x^2 (1+x)^5 (15-34x+152x^2-202x^3+221x^4-188x^5+52x^6)$$

**Simplify[Cf[13, 7, 4]]**

[\[化简\]](#)

$$2048 x (1+x)^5 (-22+61x-464x^2+899x^3-1766x^4+2289x^5-1036x^6-11x^7+172x^8-166x^9+44x^{10})$$

**Simplify[Cf[13, 7, 5]]**

[\[化简\]](#)

$$4096 x^2 (1+x)^5 (-299+1352x-5616x^2+11877x^3-18447x^4+19478x^5-12818x^6+5737x^7-1796x^8+340x^9)$$

**Simplify[Cf[13, 7, 6]]**

[\[化简\]](#)

$$2048 x (1+x)^5 (-102+188x-2949x^2+5328x^3-16599x^4+19224x^5-17363x^6+8556x^7-391x^8-560x^9+60x^{10})$$

**Simplify[Cf[13, 7, 7]]**

[\[化简\]](#)

$$-8192 x^2 (1+x)^5 (442-1939x+8752x^2-17217x^3+28770x^4-28765x^5+20384x^6-8115x^7+1364x^8+164x^9)$$

**Simplify[Cf[13, 7, 8]]**

[\[化简\]](#)

$$-4096 x (1+x)^5 (80-127x+2587x^2-4727x^3+17005x^4-19163x^5+23373x^6-13825x^7+6171x^8-366x^9+128x^{10})$$

**Simplify[Cf[13, 7, 9]]**

[\[化简\]](#)

$$-8192 x^2 (1+x)^5 (442-1939x+8752x^2-17217x^3+28770x^4-28765x^5+20384x^6-8115x^7+1364x^8+164x^9)$$

**Simplify[Cf[13, 7, 10]]**

化简

$$2048 x (1+x)^5 (-102 + 188 x - 2949 x^2 + 5328 x^3 - 16599 x^4 + 19224 x^5 - 17363 x^6 + 8556 x^7 - 391 x^8 - 560 x^9 + 60 x^{10})$$

**Simplify[Cf[13, 7, 11]]**

化简

$$4096 x^2 (1+x)^5 (-299 + 1352 x - 5616 x^2 + 11877 x^3 - 18447 x^4 + 19478 x^5 - 12818 x^6 + 5737 x^7 - 1796 x^8 + 340 x^9)$$

**Simplify[Cf[13, 7, 12]]**

化简

$$2048 x (1+x)^5 (-22 + 61 x - 464 x^2 + 899 x^3 - 1766 x^4 + 2289 x^5 - 1036 x^6 - 11 x^7 + 172 x^8 - 166 x^9 + 44 x^{10})$$

**Simplify[Cf[13, 7, 13]]**

化简

$$-4096 (-1+x)^2 x^2 (1+x)^5 (15 - 34 x + 152 x^2 - 202 x^3 + 221 x^4 - 188 x^5 + 52 x^6)$$

**Simplify[Cf[13, 7, 14]]**

化简

$$-12288 (-1+x)^4 x^3 (1+x)^6$$

**(\*, r2^13r3^8\*)****Simplify[Cf[13, 8, 0]]**

化简

0

**Simplify[Cf[13, 8, 1]]**

化简

$$6144 (-1+x)^5 x^3 (1+x)^6$$

**Simplify[Cf[13, 8, 2]]**

化简

$$2048 (-1+x)^3 x^2 (1+x)^5 (15 - x + 23 x^2 + 135 x^3 - 158 x^4 + 34 x^5)$$

**Simplify[Cf[13, 8, 3]]**

化简

$$-2048 (-1+x)^2 x (1+x)^5 (18 - 53 x + 419 x^2 - 464 x^3 + 1070 x^4 - 399 x^5 + 121 x^6 - 228 x^7 + 60 x^8)$$

**Simplify[Cf[13, 8, 4]]**

化简

$$-2048 x (1+x)^5 (24 + 71 x + 389 x^2 - 1171 x^3 + 5567 x^4 - 11413 x^5 + 13431 x^6 - 11365 x^7 + 5741 x^8 - 1562 x^9 + 288 x^{10})$$

**Simplify[Cf[13, 8, 5]]**

化简

$$-2048 x (1+x)^5 (94 - 303 x + 3119 x^2 - 6866 x^3 + 17814 x^4 - 22905 x^5 + 21615 x^6 - 15272 x^7 + 5986 x^8 - 1982 x^9 + 236 x^{10})$$

**Simplify[Cf[13, 8, 6]]**

[化简]

$$2048 x (1+x)^5 (-108 - 12 x - 3006 x^2 + 5481 x^3 - 23953 x^4 + 31960 x^5 - 38556 x^6 + 27749 x^7 - 12817 x^8 + 2438 x^9 + 840 x^{10})$$

**Simplify[Cf[13, 8, 7]]**

[化简]

$$-4096 x (1+x)^5 (80 - 127 x + 2587 x^2 - 4727 x^3 + 17005 x^4 - 19163 x^5 + 23373 x^6 - 13825 x^7 + 6171 x^8 - 366 x^9 + 128 x^{10})$$

**Simplify[Cf[13, 8, 8]]**

[化简]

$$-4096 x (1+x)^5 (80 - 127 x + 2587 x^2 - 4727 x^3 + 17005 x^4 - 19163 x^5 + 23373 x^6 - 13825 x^7 + 6171 x^8 - 366 x^9 + 128 x^{10})$$

**Simplify[Cf[13, 8, 9]]**

[化简]

$$2048 x (1+x)^5 (-108 - 12 x - 3006 x^2 + 5481 x^3 - 23953 x^4 + 31960 x^5 - 38556 x^6 + 27749 x^7 - 12817 x^8 + 2438 x^9 + 840 x^{10})$$

**Simplify[Cf[13, 8, 10]]**

[化简]

$$-2048 x (1+x)^5 (94 - 303 x + 3119 x^2 - 6866 x^3 + 17814 x^4 - 22905 x^5 + 21615 x^6 - 15272 x^7 + 5986 x^8 - 1982 x^9 + 236 x^{10})$$

**Simplify[Cf[13, 8, 11]]**

[化简]

$$-2048 x (1+x)^5 (24 + 71 x + 389 x^2 - 1171 x^3 + 5567 x^4 - 11413 x^5 + 13431 x^6 - 11365 x^7 + 5741 x^8 - 1562 x^9 + 288 x^{10})$$

**Simplify[Cf[13, 8, 12]]**

[化简]

$$-2048 (-1+x)^2 x (1+x)^5 (18 - 53 x + 419 x^2 - 464 x^3 + 1070 x^4 - 399 x^5 + 121 x^6 - 228 x^7 + 60 x^8)$$

**Simplify[Cf[13, 8, 13]]**

[化简]

$$2048 (-1+x)^3 x^2 (1+x)^5 (15 - x + 23 x^2 + 135 x^3 - 158 x^4 + 34 x^5)$$

**Simplify[Cf[13, 8, 14]]**

[化简]

$$6144 (-1+x)^5 x^3 (1+x)^6$$

**(\*, r2^13r3^9\*)****Simplify[Cf[13, 9, 0]]**

[化简]

$$-2048 (-1+x)^6 x^3 (1+x)^5$$

**Simplify[Cf[13, 9, 1]]**

[化简]

$$8192 (-1+x)^4 x^2 (1+x)^5 (-2 + 3 x - 13 x^2 + 6 x^3)$$

**Simplify[Cf[13, 9, 2]]**

[化简]

$$2048 (-1+x)^3 x (1+x)^5 (6+7x+89x^2+50x^3+225x^4+197x^5-190x^6+36x^7)$$

**Simplify[Cf[13, 9, 3]]**

[化简]

$$4096 (-1+x)^2 x^2 (1+x)^5 (-120+337x-1408x^2+1558x^3-2044x^4+597x^5+4x^6+36x^7)$$

**Simplify[Cf[13, 9, 4]]**

[化简]

$$2048 x (1+x)^5 (-46+21x-971x^2+1647x^3-5249x^4+6783x^5-3145x^6-1271x^7+4655x^8-2668x^9+244x^{10})$$

**Simplify[Cf[13, 9, 5]]**

[化简]

$$-8192 x^2 (1+x)^5 (279-1252x+5397x^2-10826x^3+16897x^4-16812x^5+10319x^6-3486x^7-156x^8+216x^9)$$

**Simplify[Cf[13, 9, 6]]**

[化简]

$$2048 x (1+x)^5 (-108-12x-3006x^2+5481x^3-23953x^4+31960x^5-38556x^6+27749x^7-12817x^8+2438x^9+840x^{10})$$

**Simplify[Cf[13, 9, 7]]**

[化简]

$$-8192 x^2 (1+x)^5 (442-1939x+8752x^2-17217x^3+28770x^4-28765x^5+20384x^6-8115x^7+1364x^8+164x^9)$$

**Simplify[Cf[13, 9, 8]]**

[化简]

$$2048 x (1+x)^5 (-108-12x-3006x^2+5481x^3-23953x^4+31960x^5-38556x^6+27749x^7-12817x^8+2438x^9+840x^{10})$$

**Simplify[Cf[13, 9, 9]]**

[化简]

$$-8192 x^2 (1+x)^5 (279-1252x+5397x^2-10826x^3+16897x^4-16812x^5+10319x^6-3486x^7-156x^8+216x^9)$$

**Simplify[Cf[13, 9, 10]]**

[化简]

$$2048 x (1+x)^5 (-46+21x-971x^2+1647x^3-5249x^4+6783x^5-3145x^6-1271x^7+4655x^8-2668x^9+244x^{10})$$

**Simplify[Cf[13, 9, 11]]**

[化简]

$$4096 (-1+x)^2 x^2 (1+x)^5 (-120+337x-1408x^2+1558x^3-2044x^4+597x^5+4x^6+36x^7)$$

**Simplify[Cf[13, 9, 12]]**

[化简]

$$2048 (-1+x)^3 x (1+x)^5 (6+7x+89x^2+50x^3+225x^4+197x^5-190x^6+36x^7)$$

**Simplify[Cf[13, 9, 13]]**

[化简]

$$8192 (-1+x)^4 x^2 (1+x)^5 (-2+3x-13x^2+6x^3)$$

**Simplify[Cf[13, 9, 14]]**

[化简]

$$-2048 (-1+x)^6 x^3 (1+x)^5$$

**(\*, r2^13r3^10\*)****Simplify[Cf[13, 10, 0]]**

[化简]

$$-4096 x^2 (-1+x^2)^5 (-1+x-3x^2+x^3)$$

**Simplify[Cf[13, 10, 1]]**

[化简]

$$-2048 (-1+x)^4 x (1+x)^5 (4-12x+75x^2-52x^3+165x^4-56x^5+8x^6)$$

**Simplify[Cf[13, 10, 2]]**

[化简]

$$-2048 (-1+x)^3 x (1+x)^5 (-6-34x-84x^2-195x^3-332x^4-521x^5+92x^6+36x^7)$$

**Simplify[Cf[13, 10, 3]]**

[化简]

$$-4096 (-1+x)^2 x (1+x)^5 (18-53x+523x^2-704x^3+2078x^4-1455x^5+1921x^6-772x^7+12x^8)$$

**Simplify[Cf[13, 10, 4]]**

[化简]

$$2048 x (1+x)^5 (-46+21x-971x^2+1647x^3-5249x^4+6783x^5-3145x^6-1271x^7+4655x^8-2668x^9+244x^{10})$$

**Simplify[Cf[13, 10, 5]]**

[化简]

$$-2048 x (1+x)^5 (94-303x+3119x^2-6866x^3+17814x^4-22905x^5+21615x^6-15272x^7+5986x^8-1982x^9+236x^{10})$$

**Simplify[Cf[13, 10, 6]]**

[化简]

$$2048 x (1+x)^5 (-102+188x-2949x^2+5328x^3-16599x^4+19224x^5-17363x^6+8556x^7-391x^8-560x^9+60x^{10})$$

**Simplify[Cf[13, 10, 7]]**

[化简]

$$2048 x (1+x)^5 (-102+188x-2949x^2+5328x^3-16599x^4+19224x^5-17363x^6+8556x^7-391x^8-560x^9+60x^{10})$$

**Simplify[Cf[13, 10, 8]]**

[化简]

$$-2048 x (1+x)^5 (94-303x+3119x^2-6866x^3+17814x^4-22905x^5+21615x^6-15272x^7+5986x^8-1982x^9+236x^{10})$$

**Simplify[Cf[13, 10, 9]]**

[化简]

$$2048 x (1+x)^5 (-46 + 21 x - 971 x^2 + 1647 x^3 - 5249 x^4 + 6783 x^5 - 3145 x^6 - 1271 x^7 + 4655 x^8 - 2668 x^9 + 244 x^{10})$$

**Simplify[Cf[13, 10, 10]]**

[化简]

$$-4096 (-1+x)^2 x (1+x)^5 (18 - 53 x + 523 x^2 - 704 x^3 + 2078 x^4 - 1455 x^5 + 1921 x^6 - 772 x^7 + 12 x^8)$$

**Simplify[Cf[13, 10, 11]]**

[化简]

$$-2048 (-1+x)^3 x (1+x)^5 (-6 - 34 x - 84 x^2 - 195 x^3 - 332 x^4 - 521 x^5 + 92 x^6 + 36 x^7)$$

**Simplify[Cf[13, 10, 12]]**

[化简]

$$-2048 (-1+x)^4 x (1+x)^5 (4 - 12 x + 75 x^2 - 52 x^3 + 165 x^4 - 56 x^5 + 8 x^6)$$

**Simplify[Cf[13, 10, 13]]**

[化简]

$$-4096 x^2 (-1+x^2)^5 (-1+x - 3 x^2 + x^3)$$

**Simplify[Cf[13, 10, 14]]**

[化简]

0

**(\*, r2^13r3^11\*)****Simplify[Cf[13, 11, 0]]**

[化简]

$$2048 x^2 (-1+x^2)^5 (2 + 3 x + 7 x^2 + 2 x^3)$$

**Simplify[Cf[13, 11, 1]]**

[化简]

$$8192 (-1+x)^4 x^2 (1+x)^5 (-6 + 8 x - 41 x^2 - 3 x^3 - 16 x^4 + 4 x^5)$$

**Simplify[Cf[13, 11, 2]]**

[化简]

$$-2048 (-1+x)^3 x (1+x)^5 (-6 - 34 x - 84 x^2 - 195 x^3 - 332 x^4 - 521 x^5 + 92 x^6 + 36 x^7)$$

**Simplify[Cf[13, 11, 3]]**

[化简]

$$4096 (-1+x)^2 x^2 (1+x)^5 (-120 + 337 x - 1408 x^2 + 1558 x^3 - 2044 x^4 + 597 x^5 + 4 x^6 + 36 x^7)$$

**Simplify[Cf[13, 11, 4]]**

[化简]

$$-2048 x (1+x)^5 (24 + 71 x + 389 x^2 - 1171 x^3 + 5567 x^4 - 11413 x^5 + 13431 x^6 - 11365 x^7 + 5741 x^8 - 1562 x^9 + 288 x^{10})$$

**Simplify[Cf[13, 11, 5]]**

[化简]

$$4096 x^2 (1+x)^5 (-299 + 1352 x - 5616 x^2 + 11877 x^3 - 18447 x^4 + 19478 x^5 - 12818 x^6 + 5737 x^7 - 1796 x^8 + 340 x^9)$$

**Simplify[Cf[13, 11, 6]]**

[化简]

$$-4096 x (1+x)^5 (18 + 57 x + 380 x^2 - 1128 x^3 + 5543 x^4 - 10971 x^5 + 14182 x^6 - 12722 x^7 + 6857 x^8 - 2276 x^9 + 444 x^{10})$$

**Simplify[Cf[13, 11, 7]]**

[化简]

$$4096 x^2 (1+x)^5 (-299 + 1352 x - 5616 x^2 + 11877 x^3 - 18447 x^4 + 19478 x^5 - 12818 x^6 + 5737 x^7 - 1796 x^8 + 340 x^9)$$

**Simplify[Cf[13, 11, 8]]**

[化简]

$$-2048 x (1+x)^5 (24 + 71 x + 389 x^2 - 1171 x^3 + 5567 x^4 - 11413 x^5 + 13431 x^6 - 11365 x^7 + 5741 x^8 - 1562 x^9 + 288 x^{10})$$

**Simplify[Cf[13, 11, 9]]**

[化简]

$$4096 (-1+x)^2 x^2 (1+x)^5 (-120 + 337 x - 1408 x^2 + 1558 x^3 - 2044 x^4 + 597 x^5 + 4 x^6 + 36 x^7)$$

**Simplify[Cf[13, 11, 10]]**

[化简]

$$-2048 (-1+x)^3 x (1+x)^5 (-6 - 34 x - 84 x^2 - 195 x^3 - 332 x^4 - 521 x^5 + 92 x^6 + 36 x^7)$$

**Simplify[Cf[13, 11, 11]]**

[化简]

$$8192 (-1+x)^4 x^2 (1+x)^5 (-6 + 8 x - 41 x^2 - 3 x^3 - 16 x^4 + 4 x^5)$$

**Simplify[Cf[13, 11, 12]]**

[化简]

$$2048 x^2 (-1+x^2)^5 (2 + 3 x + 7 x^2 + 2 x^3)$$

**Simplify[Cf[13, 11, 13]]**

[化简]

0

**Simplify[Cf[13, 11, 14]]**

[化简]

0

**(\*, r2^13r3^12\*)****Simplify[Cf[13, 12, 0]]**

[化简]

$$2048 x^2 (-1+x^2)^5 (2 + 3 x + 7 x^2 + 2 x^3)$$



**Simplify[Cf[13, 12, 1]]**

化简

$$-2048 (-1+x)^4 x (1+x)^5 (4-12x+75x^2-52x^3+165x^4-56x^5+8x^6)$$

**Simplify[Cf[13, 12, 2]]**

化简

$$2048 (-1+x)^3 x (1+x)^5 (6+7x+89x^2+50x^3+225x^4+197x^5-190x^6+36x^7)$$

**Simplify[Cf[13, 12, 3]]**

化简

$$-2048 (-1+x)^2 x (1+x)^5 (18-53x+419x^2-464x^3+1070x^4-399x^5+121x^6-228x^7+60x^8)$$

**Simplify[Cf[13, 12, 4]]**

化简

$$2048 x (1+x)^5 (-22+61x-464x^2+899x^3-1766x^4+2289x^5-1036x^6-11x^7+172x^8-166x^9+44x^{10})$$

**Simplify[Cf[13, 12, 5]]**

化简

$$-2048 x (1+x)^5 (30-109x+767x^2-1588x^3+3006x^4-3343x^5+1303x^6-22x^7-30x^8-26x^9+12x^{10})$$

**Simplify[Cf[13, 12, 6]]**

化简

$$-2048 x (1+x)^5 (30-109x+767x^2-1588x^3+3006x^4-3343x^5+1303x^6-22x^7-30x^8-26x^9+12x^{10})$$

**Simplify[Cf[13, 12, 7]]**

化简

$$2048 x (1+x)^5 (-22+61x-464x^2+899x^3-1766x^4+2289x^5-1036x^6-11x^7+172x^8-166x^9+44x^{10})$$

**Simplify[Cf[13, 12, 8]]**

化简

$$-2048 (-1+x)^2 x (1+x)^5 (18-53x+419x^2-464x^3+1070x^4-399x^5+121x^6-228x^7+60x^8)$$

**Simplify[Cf[13, 12, 9]]**

化简

$$2048 (-1+x)^3 x (1+x)^5 (6+7x+89x^2+50x^3+225x^4+197x^5-190x^6+36x^7)$$

**Simplify[Cf[13, 12, 10]]**

化简

$$-2048 (-1+x)^4 x (1+x)^5 (4-12x+75x^2-52x^3+165x^4-56x^5+8x^6)$$

**Simplify[Cf[13, 12, 11]]**

化简

$$2048 x^2 (-1+x^2)^5 (2+3x+7x^2+2x^3)$$

**Simplify[Cf[13, 12, 12]]**

化简

0

**Simplify[Cf[13, 12, 13]]**[\[化简\]](#)

0

**Simplify[Cf[13, 12, 14]]**[\[化简\]](#)

0

**(\*, r2^13r3^13\*)****Simplify[Cf[13, 13, 0]]**[\[化简\]](#)

$$-4096 x^2 (-1 + x^2)^5 (-1 + x - 3 x^2 + x^3)$$

**Simplify[Cf[13, 13, 1]]**[\[化简\]](#)

$$8192 (-1 + x)^4 x^2 (1 + x)^5 (-2 + 3 x - 13 x^2 + 6 x^3)$$

**Simplify[Cf[13, 13, 2]]**[\[化简\]](#)

$$2048 (-1 + x)^3 x^2 (1 + x)^5 (15 - x + 23 x^2 + 135 x^3 - 158 x^4 + 34 x^5)$$

**Simplify[Cf[13, 13, 3]]**[\[化简\]](#)

$$-4096 (-1 + x)^2 x^2 (1 + x)^5 (15 - 34 x + 152 x^2 - 202 x^3 + 221 x^4 - 188 x^5 + 52 x^6)$$

**Simplify[Cf[13, 13, 4]]**[\[化简\]](#)

$$2048 (-1 + x)^2 x^2 (1 + x)^5 (-35 + 16 x - 90 x^2 - 364 x^3 + 597 x^4 - 460 x^5 + 160 x^6)$$

**Simplify[Cf[13, 13, 5]]**[\[化简\]](#)

$$-8192 (-1 + x)^2 x^2 (1 + x)^5 (11 - 20 x + 108 x^2 - 112 x^3 + 161 x^4 - 120 x^5 + 44 x^6)$$

**Simplify[Cf[13, 13, 6]]**[\[化简\]](#)

$$2048 (-1 + x)^2 x^2 (1 + x)^5 (-35 + 16 x - 90 x^2 - 364 x^3 + 597 x^4 - 460 x^5 + 160 x^6)$$

**Simplify[Cf[13, 13, 7]]**[\[化简\]](#)

$$-4096 (-1 + x)^2 x^2 (1 + x)^5 (15 - 34 x + 152 x^2 - 202 x^3 + 221 x^4 - 188 x^5 + 52 x^6)$$

**Simplify[Cf[13, 13, 8]]**[\[化简\]](#)

$$2048 (-1 + x)^3 x^2 (1 + x)^5 (15 - x + 23 x^2 + 135 x^3 - 158 x^4 + 34 x^5)$$

**Simplify[Cf[13, 13, 9]]**[\[化简\]](#)

$$8192 (-1 + x)^4 x^2 (1 + x)^5 (-2 + 3 x - 13 x^2 + 6 x^3)$$

**Simplify[Cf[13, 13, 10]]**

[化简]

$$-4096 x^2 (-1 + x^2)^5 (-1 + x - 3 x^2 + x^3)$$

**Simplify[Cf[13, 13, 11]]**

[化简]

0

**Simplify[Cf[13, 13, 12]]**

[化简]

0

**Simplify[Cf[13, 13, 13]]**

[化简]

0

**Simplify[Cf[13, 13, 14]]**

[化简]

0

**(\*, r2^13r3^14\*)**

**Simplify[Cf[13, 14, 0]]**

[化简]

$$-2048 (-1 + x)^6 x^3 (1 + x)^5$$

**Simplify[Cf[13, 14, 1]]**

[化简]

$$6144 (-1 + x)^5 x^3 (1 + x)^6$$

**Simplify[Cf[13, 14, 2]]**

[化简]

$$-12288 (-1 + x)^3 x^3 (1 + x)^5 (-1 + x^2)$$

**Simplify[Cf[13, 14, 3]]**

[化简]

$$-4096 (-1 + x)^3 x^3 (1 + x)^5 (-5 - 3 x^2 + 4 x^3)$$

**Simplify[Cf[13, 14, 4]]**

[化简]

$$12288 (-1 + x)^3 x^3 (1 + x)^5 (2 + x + x^3)$$

**Simplify[Cf[13, 14, 5]]**

[化简]

$$12288 (-1 + x)^3 x^3 (1 + x)^5 (2 + x + x^3)$$

**Simplify[Cf[13, 14, 6]]**

[化简]

$$-4096 (-1 + x)^3 x^3 (1 + x)^5 (-5 - 3 x^2 + 4 x^3)$$

**Simplify[Cf[13, 14, 7]]**

[\[化简\]](#)

$$-12288 (-1+x)^3 x^3 (1+x)^5 (-1+x^2)$$

**Simplify[Cf[13, 14, 8]]**

[\[化简\]](#)

$$6144 (-1+x)^5 x^3 (1+x)^6$$

**Simplify[Cf[13, 14, 9]]**

[\[化简\]](#)

$$-2048 (-1+x)^6 x^3 (1+x)^5$$

**Simplify[Cf[13, 14, 10]]**

[\[化简\]](#)

0

**Simplify[Cf[13, 14, 11]]**

[\[化简\]](#)

0

**Simplify[Cf[13, 14, 12]]**

[\[化简\]](#)

0

**Simplify[Cf[13, 14, 13]]**

[\[化简\]](#)

0

**Simplify[Cf[13, 14, 14]]**

[\[化简\]](#)

0

**(\*, r2^14r3^0\*)**

**Simplify[Cf[14, 0, 0]]**

[\[化简\]](#)

0

**Simplify[Cf[14, 0, 1]]**

[\[化简\]](#)

0

**Simplify[Cf[14, 0, 2]]**

[\[化简\]](#)

0

**Simplify[Cf[14, 0, 3]]**

[\[化简\]](#)

0

**Simplify[Cf[14, 0, 4]]**

[\[化简\]](#)

0

**Simplify[Cf[14, 0, 5]]**

[\[化简\]](#)

0

**Simplify[Cf[14, 0, 6]]**

[\[化简\]](#)

0

**Simplify[Cf[14, 0, 7]]**

[\[化简\]](#)

0

**Simplify[Cf[14, 0, 8]]**

[\[化简\]](#)

0

**Simplify[Cf[14, 0, 9]]**

[\[化简\]](#)

$-2048 (-1+x)^6 x^3 (1+x)^5$

**Simplify[Cf[14, 0, 10]]**

[\[化简\]](#)

$4096 x^3 (-1+x^2)^5$

**Simplify[Cf[14, 0, 11]]**

[\[化简\]](#)

$4096 (-1+x)^5 x^3 (1+x)^6$

**Simplify[Cf[14, 0, 12]]**

[\[化简\]](#)

$4096 x^3 (-1+x^2)^5$

**Simplify[Cf[14, 0, 13]]**

[\[化简\]](#)

$-2048 (-1+x)^6 x^3 (1+x)^5$

**Simplify[Cf[14, 0, 14]]**

[\[化简\]](#)

0

**(\*, r2^14r3^1\*)**

**Simplify[Cf[14, 1, 0]]**

[\[化简\]](#)

0

**Simplify[Cf[14, 1, 1]]**

[\[化简\]](#)

0

**Simplify[Cf[14, 1, 2]]**

[\[化简\]](#)

0

**Simplify[Cf[14, 1, 3]]**

[\[化简\]](#)

0

**Simplify[Cf[14, 1, 4]]**

[\[化简\]](#)

0

**Simplify[Cf[14, 1, 5]]**

[\[化简\]](#)

0

**Simplify[Cf[14, 1, 6]]**

[\[化简\]](#)

0

**Simplify[Cf[14, 1, 7]]**

[\[化简\]](#)

0

**Simplify[Cf[14, 1, 8]]**

[\[化简\]](#)

$6144 (-1 + x)^5 x^3 (1 + x)^6$

**Simplify[Cf[14, 1, 9]]**

[\[化简\]](#)

$-2048 (-1 + x)^4 x^2 (1 + x)^5 (2 - 3x + 30x^2 - 21x^3 + 4x^4)$

**Simplify[Cf[14, 1, 10]]**

[\[化简\]](#)

$4096 (-1 + x)^4 x^2 (1 + x)^5 (-1 - 2x - 11x^2 - 8x^3 + 2x^4)$

**Simplify[Cf[14, 1, 11]]**

[\[化简\]](#)

$4096 (-1 + x)^4 x^2 (1 + x)^5 (-1 - 2x - 11x^2 - 8x^3 + 2x^4)$

**Simplify[Cf[14, 1, 12]]**

[\[化简\]](#)

$-2048 (-1 + x)^4 x^2 (1 + x)^5 (2 - 3x + 30x^2 - 21x^3 + 4x^4)$

**Simplify[Cf[14, 1, 13]]**

[\[化简\]](#)

$6144 (-1 + x)^5 x^3 (1 + x)^6$

**Simplify[Cf[14, 1, 14]]**

[化简]

0

(\*, r2^14r3^2\*)

**Simplify[Cf[14, 2, 0]]**

[化简]

0

**Simplify[Cf[14, 2, 1]]**

[化简]

0

**Simplify[Cf[14, 2, 2]]**

[化简]

0

**Simplify[Cf[14, 2, 3]]**

[化简]

0

**Simplify[Cf[14, 2, 4]]**

[化简]

0

**Simplify[Cf[14, 2, 5]]**

[化简]

0

**Simplify[Cf[14, 2, 6]]**

[化简]

0

**Simplify[Cf[14, 2, 7]]**

[化简]

$-12\,288 (-1+x)^4 x^3 (1+x)^6$

**Simplify[Cf[14, 2, 8]]**

[化简]

$1024 (-1+x)^3 x^2 (1+x)^5 (7+19x+13x^2+137x^3-172x^4+44x^5)$

**Simplify[Cf[14, 2, 9]]**

[化简]

$-2048 (-1+x)^3 x^2 (1+x)^5 (-3-44x+37x^2-182x^3+60x^4)$

**Simplify[Cf[14, 2, 10]]**

[化简]

$-2048 (-1+x)^3 x^2 (1+x)^5 (-7-25x-57x^2-55x^3-116x^4+44x^5)$

**Simplify[Cf[14, 2, 11]]**

[\[化简\]](#)

$$-2048 (-1+x)^3 x^2 (1+x)^5 (-3-44x+37x^2-182x^3+60x^4)$$

**Simplify[Cf[14, 2, 12]]**

[\[化简\]](#)

$$1024 (-1+x)^3 x^2 (1+x)^5 (7+19x+13x^2+137x^3-172x^4+44x^5)$$

**Simplify[Cf[14, 2, 13]]**

[\[化简\]](#)

$$-12288 (-1+x)^4 x^3 (1+x)^6$$

**Simplify[Cf[14, 2, 14]]**

[\[化简\]](#)

0

(\*, r2^14r3^3\*)

**Simplify[Cf[14, 3, 0]]**

[\[化简\]](#)

0

**Simplify[Cf[14, 3, 1]]**

[\[化简\]](#)

0

**Simplify[Cf[14, 3, 2]]**

[\[化简\]](#)

0

**Simplify[Cf[14, 3, 3]]**

[\[化简\]](#)

0

**Simplify[Cf[14, 3, 4]]**

[\[化简\]](#)

0

**Simplify[Cf[14, 3, 5]]**

[\[化简\]](#)

0

**Simplify[Cf[14, 3, 6]]**

[\[化简\]](#)

$$-4096 (-1+x)^3 x^3 (1+x)^5 (-5-3x^2+4x^3)$$

**Simplify[Cf[14, 3, 7]]**

[\[化简\]](#)

$$-2048 (-1+x)^2 x^2 (1+x)^5 (9-14x+132x^2-190x^3+207x^4-180x^5+52x^6)$$



**Simplify[Cf[14, 3, 8]]**

[\[化简\]](#)

$$-2048 (-1+x)^2 x^2 (1+x)^5 (9+60x+34x^2+56x^3+177x^4-188x^5+28x^6)$$

**Simplify[Cf[14, 3, 9]]**

[\[化简\]](#)

$$4096 (-1+x)^2 x^2 (1+x)^5 (-9-18x-124x^2+82x^3-207x^4+4x^5+40x^6)$$

**Simplify[Cf[14, 3, 10]]**

[\[化简\]](#)

$$4096 (-1+x)^2 x^2 (1+x)^5 (-9-18x-124x^2+82x^3-207x^4+4x^5+40x^6)$$

**Simplify[Cf[14, 3, 11]]**

[\[化简\]](#)

$$-2048 (-1+x)^2 x^2 (1+x)^5 (9+60x+34x^2+56x^3+177x^4-188x^5+28x^6)$$

**Simplify[Cf[14, 3, 12]]**

[\[化简\]](#)

$$-2048 (-1+x)^2 x^2 (1+x)^5 (9-14x+132x^2-190x^3+207x^4-180x^5+52x^6)$$

**Simplify[Cf[14, 3, 13]]**

[\[化简\]](#)

$$-4096 (-1+x)^3 x^3 (1+x)^5 (-5-3x^2+4x^3)$$

**Simplify[Cf[14, 3, 14]]**

[\[化简\]](#)

0

(\*, r2^14r3^4\*)

**Simplify[Cf[14, 4, 0]]**

[\[化简\]](#)

0

**Simplify[Cf[14, 4, 1]]**

[\[化简\]](#)

0

**Simplify[Cf[14, 4, 2]]**

[\[化简\]](#)

0

**Simplify[Cf[14, 4, 3]]**

[\[化简\]](#)

0

**Simplify[Cf[14, 4, 4]]**

[\[化简\]](#)

0

**Simplify[Cf[14, 4, 5]]**[\[化简\]](#)

$$12\,288 \left(-1+x\right)^3 x^3 \left(1+x\right)^5 \left(2+x+x^3\right)$$

**Simplify[Cf[14, 4, 6]]**[\[化简\]](#)

$$1024 \left(-1+x\right)^2 x^2 \left(1+x\right)^5 \left(-21-24x-78x^2-328x^3+551x^4-424x^5+148x^6\right)$$

**Simplify[Cf[14, 4, 7]]**[\[化简\]](#)

$$2048 x^2 \left(1+x\right)^5 \left(-11-116x+337x^2-822x^3+1271x^4-1020x^5+567x^6-250x^7+44x^8\right)$$

**Simplify[Cf[14, 4, 8]]**[\[化简\]](#)

$$-1024 x^2 \left(1+x\right)^5 \left(67+2x+857x^2-2092x^3+3073x^4-3126x^5+1695x^6-736x^7+260x^8\right)$$

**Simplify[Cf[14, 4, 9]]**[\[化简\]](#)

$$4096 x^2 \left(1+x\right)^5 \left(-11-106x+299x^2-1048x^3+2055x^4-2338x^5+1613x^6-476x^7+12x^8\right)$$

**Simplify[Cf[14, 4, 10]]**[\[化简\]](#)

$$-1024 x^2 \left(1+x\right)^5 \left(67+2x+857x^2-2092x^3+3073x^4-3126x^5+1695x^6-736x^7+260x^8\right)$$

**Simplify[Cf[14, 4, 11]]**[\[化简\]](#)

$$2048 x^2 \left(1+x\right)^5 \left(-11-116x+337x^2-822x^3+1271x^4-1020x^5+567x^6-250x^7+44x^8\right)$$

**Simplify[Cf[14, 4, 12]]**[\[化简\]](#)

$$1024 \left(-1+x\right)^2 x^2 \left(1+x\right)^5 \left(-21-24x-78x^2-328x^3+551x^4-424x^5+148x^6\right)$$

**Simplify[Cf[14, 4, 13]]**[\[化简\]](#)

$$12\,288 \left(-1+x\right)^3 x^3 \left(1+x\right)^5 \left(2+x+x^3\right)$$

**Simplify[Cf[14, 4, 14]]**[\[化简\]](#)

0

**(\*, r2^14r3^5\*)****Simplify[Cf[14, 5, 0]]**[\[化简\]](#)

0

**Simplify[Cf[14, 5, 1]]**[\[化简\]](#)

0

**Simplify[Cf[14, 5, 2]]**

[化简]

0

**Simplify[Cf[14, 5, 3]]**

[化简]

0

**Simplify[Cf[14, 5, 4]]**

[化简]

$$12\,288 (-1+x)^3 x^3 (1+x)^5 (2+x+x^3)$$

**Simplify[Cf[14, 5, 5]]**

[化简]

$$-4096 (-1+x)^2 x^2 (1+x)^5 (7-7x+96x^2-102x^3+149x^4-111x^5+40x^6)$$

**Simplify[Cf[14, 5, 6]]**

[化简]

$$-2048 x^2 (1+x)^5 (15+129x-276x^2+570x^3-597x^4+37x^5+198x^6-96x^7+20x^8)$$

**Simplify[Cf[14, 5, 7]]**

[化简]

$$2048 x^2 (1+x)^5 (-45-33x-508x^2+870x^3-773x^4-265x^5+1450x^6-1100x^7+308x^8)$$

**Simplify[Cf[14, 5, 8]]**

[化简]

$$-4096 x^2 (1+x)^5 (23+98x+26x^2+194x^3-51x^4-384x^5+674x^6-540x^7+104x^8)$$

**Simplify[Cf[14, 5, 9]]**

[化简]

$$-4096 x^2 (1+x)^5 (23+98x+26x^2+194x^3-51x^4-384x^5+674x^6-540x^7+104x^8)$$

**Simplify[Cf[14, 5, 10]]**

[化简]

$$2048 x^2 (1+x)^5 (-45-33x-508x^2+870x^3-773x^4-265x^5+1450x^6-1100x^7+308x^8)$$

**Simplify[Cf[14, 5, 11]]**

[化简]

$$-2048 x^2 (1+x)^5 (15+129x-276x^2+570x^3-597x^4+37x^5+198x^6-96x^7+20x^8)$$

**Simplify[Cf[14, 5, 12]]**

[化简]

$$-4096 (-1+x)^2 x^2 (1+x)^5 (7-7x+96x^2-102x^3+149x^4-111x^5+40x^6)$$

**Simplify[Cf[14, 5, 13]]**

[化简]

$$12\,288 (-1+x)^3 x^3 (1+x)^5 (2+x+x^3)$$

**Simplify[Cf[14, 5, 14]]**

[化简]

0

(\*, r2^14r3^6\*)

**Simplify[Cf[14, 6, 0]]**

[\[化简\]](#)

0

**Simplify[Cf[14, 6, 1]]**

[\[化简\]](#)

0

**Simplify[Cf[14, 6, 2]]**

[\[化简\]](#)

0

**Simplify[Cf[14, 6, 3]]**

[\[化简\]](#)

$-4096 (-1+x)^3 x^3 (1+x)^5 (-5-3x^2+4x^3)$

**Simplify[Cf[14, 6, 4]]**

[\[化简\]](#)

$1024 (-1+x)^2 x^2 (1+x)^5 (-21-24x-78x^2-328x^3+551x^4-424x^5+148x^6)$

**Simplify[Cf[14, 6, 5]]**

[\[化简\]](#)

$-2048 x^2 (1+x)^5 (15+129x-276x^2+570x^3-597x^4+37x^5+198x^6-96x^7+20x^8)$

**Simplify[Cf[14, 6, 6]]**

[\[化简\]](#)

$-2048 x^2 (1+x)^5 (53+837x^2-1888x^3+3187x^4-3528x^5+2623x^6-1528x^7+436x^8)$

**Simplify[Cf[14, 6, 7]]**

[\[化简\]](#)

$2048 x^2 (1+x)^5 (-49-363x+500x^2-2542x^3+3875x^4-3919x^5+2046x^6-520x^7+108x^8)$

**Simplify[Cf[14, 6, 8]]**

[\[化简\]](#)

$2048 x^2 (1+x)^5 (-85-26x-1639x^2+3668x^3-7407x^4+7286x^5-3481x^6-208x^7+548x^8)$

**Simplify[Cf[14, 6, 9]]**

[\[化简\]](#)

$2048 x^2 (1+x)^5 (-49-363x+500x^2-2542x^3+3875x^4-3919x^5+2046x^6-520x^7+108x^8)$

**Simplify[Cf[14, 6, 10]]**

[\[化简\]](#)

$-2048 x^2 (1+x)^5 (53+837x^2-1888x^3+3187x^4-3528x^5+2623x^6-1528x^7+436x^8)$

**Simplify[Cf[14, 6, 11]]**

[\[化简\]](#)

$-2048 x^2 (1+x)^5 (15+129x-276x^2+570x^3-597x^4+37x^5+198x^6-96x^7+20x^8)$

**Simplify[Cf[14, 6, 12]]**

[\[化简\]](#)

$$1024 (-1+x)^2 x^2 (1+x)^5 (-21-24x-78x^2-328x^3+551x^4-424x^5+148x^6)$$

**Simplify[Cf[14, 6, 13]]**

[\[化简\]](#)

$$-4096 (-1+x)^3 x^3 (1+x)^5 (-5-3x^2+4x^3)$$

**Simplify[Cf[14, 6, 14]]**

[\[化简\]](#)

0

(\*, r2^14r3^7\*)

**Simplify[Cf[14, 7, 0]]**

[\[化简\]](#)

0

**Simplify[Cf[14, 7, 1]]**

[\[化简\]](#)

0

**Simplify[Cf[14, 7, 2]]**

[\[化简\]](#)

$$-12288 (-1+x)^4 x^3 (1+x)^6$$

**Simplify[Cf[14, 7, 3]]**

[\[化简\]](#)

$$-2048 (-1+x)^2 x^2 (1+x)^5 (9-14x+132x^2-190x^3+207x^4-180x^5+52x^6)$$

**Simplify[Cf[14, 7, 4]]**

[\[化简\]](#)

$$2048 x^2 (1+x)^5 (-11-116x+337x^2-822x^3+1271x^4-1020x^5+567x^6-250x^7+44x^8)$$

**Simplify[Cf[14, 7, 5]]**

[\[化简\]](#)

$$2048 x^2 (1+x)^5 (-45-33x-508x^2+870x^3-773x^4-265x^5+1450x^6-1100x^7+308x^8)$$

**Simplify[Cf[14, 7, 6]]**

[\[化简\]](#)

$$2048 x^2 (1+x)^5 (-49-363x+500x^2-2542x^3+3875x^4-3919x^5+2046x^6-520x^7+108x^8)$$

**Simplify[Cf[14, 7, 7]]**

[\[化简\]](#)

$$-4096 x^2 (1+x)^5 (37+159x+117x^2+585x^3-685x^4+1145x^5-489x^6-17x^7+204x^8)$$

**Simplify[Cf[14, 7, 8]]**

[\[化简\]](#)

$$-4096 x^2 (1+x)^5 (37+159x+117x^2+585x^3-685x^4+1145x^5-489x^6-17x^7+204x^8)$$

**Simplify[Cf[14, 7, 9]]**

[化简]

$$2048 x^2 (1+x)^5 (-49 - 363 x + 500 x^2 - 2542 x^3 + 3875 x^4 - 3919 x^5 + 2046 x^6 - 520 x^7 + 108 x^8)$$

**Simplify[Cf[14, 7, 10]]**

[化简]

$$2048 x^2 (1+x)^5 (-45 - 33 x - 508 x^2 + 870 x^3 - 773 x^4 - 265 x^5 + 1450 x^6 - 1100 x^7 + 308 x^8)$$

**Simplify[Cf[14, 7, 11]]**

[化简]

$$2048 x^2 (1+x)^5 (-11 - 116 x + 337 x^2 - 822 x^3 + 1271 x^4 - 1020 x^5 + 567 x^6 - 250 x^7 + 44 x^8)$$

**Simplify[Cf[14, 7, 12]]**

[化简]

$$-2048 (-1+x)^2 x^2 (1+x)^5 (9 - 14 x + 132 x^2 - 190 x^3 + 207 x^4 - 180 x^5 + 52 x^6)$$

**Simplify[Cf[14, 7, 13]]**

[化简]

$$-12288 (-1+x)^4 x^3 (1+x)^6$$

**Simplify[Cf[14, 7, 14]]**

[化简]

0

**(\*, r2^14r3^8\*)****Simplify[Cf[14, 8, 0]]**

[化简]

0

**Simplify[Cf[14, 8, 1]]**

[化简]

$$6144 (-1+x)^5 x^3 (1+x)^6$$

**Simplify[Cf[14, 8, 2]]**

[化简]

$$1024 (-1+x)^3 x^2 (1+x)^5 (7 + 19 x + 13 x^2 + 137 x^3 - 172 x^4 + 44 x^5)$$

**Simplify[Cf[14, 8, 3]]**

[化简]

$$-2048 (-1+x)^2 x^2 (1+x)^5 (9 + 60 x + 34 x^2 + 56 x^3 + 177 x^4 - 188 x^5 + 28 x^6)$$

**Simplify[Cf[14, 8, 4]]**

[化简]

$$-1024 x^2 (1+x)^5 (67 + 2 x + 857 x^2 - 2092 x^3 + 3073 x^4 - 3126 x^5 + 1695 x^6 - 736 x^7 + 260 x^8)$$

**Simplify[Cf[14, 8, 5]]**

[化简]

$$-4096 x^2 (1+x)^5 (23 + 98 x + 26 x^2 + 194 x^3 - 51 x^4 - 384 x^5 + 674 x^6 - 540 x^7 + 104 x^8)$$

**Simplify[Cf[14, 8, 6]]**

[化简]

$$2048 x^2 (1+x)^5 (-85 - 26 x - 1639 x^2 + 3668 x^3 - 7407 x^4 + 7286 x^5 - 3481 x^6 - 208 x^7 + 548 x^8)$$

**Simplify[Cf[14, 8, 7]]**

[化简]

$$-4096 x^2 (1+x)^5 (37 + 159 x + 117 x^2 + 585 x^3 - 685 x^4 + 1145 x^5 - 489 x^6 - 17 x^7 + 204 x^8)$$

**Simplify[Cf[14, 8, 8]]**

[化简]

$$2048 x^2 (1+x)^5 (-85 - 26 x - 1639 x^2 + 3668 x^3 - 7407 x^4 + 7286 x^5 - 3481 x^6 - 208 x^7 + 548 x^8)$$

**Simplify[Cf[14, 8, 9]]**

[化简]

$$-4096 x^2 (1+x)^5 (23 + 98 x + 26 x^2 + 194 x^3 - 51 x^4 - 384 x^5 + 674 x^6 - 540 x^7 + 104 x^8)$$

**Simplify[Cf[14, 8, 10]]**

[化简]

$$-1024 x^2 (1+x)^5 (67 + 2 x + 857 x^2 - 2092 x^3 + 3073 x^4 - 3126 x^5 + 1695 x^6 - 736 x^7 + 260 x^8)$$

**Simplify[Cf[14, 8, 11]]**

[化简]

$$-2048 (-1+x)^2 x^2 (1+x)^5 (9 + 60 x + 34 x^2 + 56 x^3 + 177 x^4 - 188 x^5 + 28 x^6)$$

**Simplify[Cf[14, 8, 12]]**

[化简]

$$1024 (-1+x)^3 x^2 (1+x)^5 (7 + 19 x + 13 x^2 + 137 x^3 - 172 x^4 + 44 x^5)$$

**Simplify[Cf[14, 8, 13]]**

[化简]

$$6144 (-1+x)^5 x^3 (1+x)^6$$

**Simplify[Cf[14, 8, 14]]**

[化简]

0

**(\*, r2^14r3^9\*)****Simplify[Cf[14, 9, 0]]**

[化简]

$$-2048 (-1+x)^6 x^3 (1+x)^5$$

**Simplify[Cf[14, 9, 1]]**

[化简]

$$-2048 (-1+x)^4 x^2 (1+x)^5 (2 - 3 x + 30 x^2 - 21 x^3 + 4 x^4)$$

**Simplify[Cf[14, 9, 2]]**

[化简]

$$-2048 (-1+x)^3 x^2 (1+x)^5 (-3 - 44 x + 37 x^2 - 182 x^3 + 60 x^4)$$

**Simplify[Cf[14, 9, 3]]**[\[化简\]](#)

$$4096 (-1+x)^2 x^2 (1+x)^5 (-9-18x-124x^2+82x^3-207x^4+4x^5+40x^6)$$

**Simplify[Cf[14, 9, 4]]**[\[化简\]](#)

$$4096 x^2 (1+x)^5 (-11-106x+299x^2-1048x^3+2055x^4-2338x^5+1613x^6-476x^7+12x^8)$$

**Simplify[Cf[14, 9, 5]]**[\[化简\]](#)

$$-4096 x^2 (1+x)^5 (23+98x+26x^2+194x^3-51x^4-384x^5+674x^6-540x^7+104x^8)$$

**Simplify[Cf[14, 9, 6]]**[\[化简\]](#)

$$2048 x^2 (1+x)^5 (-49-363x+500x^2-2542x^3+3875x^4-3919x^5+2046x^6-520x^7+108x^8)$$

**Simplify[Cf[14, 9, 7]]**[\[化简\]](#)

$$2048 x^2 (1+x)^5 (-49-363x+500x^2-2542x^3+3875x^4-3919x^5+2046x^6-520x^7+108x^8)$$

**Simplify[Cf[14, 9, 8]]**[\[化简\]](#)

$$-4096 x^2 (1+x)^5 (23+98x+26x^2+194x^3-51x^4-384x^5+674x^6-540x^7+104x^8)$$

**Simplify[Cf[14, 9, 9]]**[\[化简\]](#)

$$4096 x^2 (1+x)^5 (-11-106x+299x^2-1048x^3+2055x^4-2338x^5+1613x^6-476x^7+12x^8)$$

**Simplify[Cf[14, 9, 10]]**[\[化简\]](#)

$$4096 (-1+x)^2 x^2 (1+x)^5 (-9-18x-124x^2+82x^3-207x^4+4x^5+40x^6)$$

**Simplify[Cf[14, 9, 11]]**[\[化简\]](#)

$$-2048 (-1+x)^3 x^2 (1+x)^5 (-3-44x+37x^2-182x^3+60x^4)$$

**Simplify[Cf[14, 9, 12]]**[\[化简\]](#)

$$-2048 (-1+x)^4 x^2 (1+x)^5 (2-3x+30x^2-21x^3+4x^4)$$

**Simplify[Cf[14, 9, 13]]**[\[化简\]](#)

$$-2048 (-1+x)^6 x^3 (1+x)^5$$

**Simplify[Cf[14, 9, 14]]**[\[化简\]](#)

0

(\*, r2^14r3^10\*)



**Simplify[Cf[14, 10, 0]]**

[化简]

$$4096 x^3 (-1 + x^2)^5$$

**Simplify[Cf[14, 10, 1]]**

[化简]

$$4096 (-1 + x)^4 x^2 (1 + x)^5 (-1 - 2x - 11x^2 - 8x^3 + 2x^4)$$

**Simplify[Cf[14, 10, 2]]**

[化简]

$$-2048 (-1 + x)^3 x^2 (1 + x)^5 (-7 - 25x - 57x^2 - 55x^3 - 116x^4 + 44x^5)$$

**Simplify[Cf[14, 10, 3]]**

[化简]

$$4096 (-1 + x)^2 x^2 (1 + x)^5 (-9 - 18x - 124x^2 + 82x^3 - 207x^4 + 4x^5 + 40x^6)$$

**Simplify[Cf[14, 10, 4]]**

[化简]

$$-1024 x^2 (1 + x)^5 (67 + 2x + 857x^2 - 2092x^3 + 3073x^4 - 3126x^5 + 1695x^6 - 736x^7 + 260x^8)$$

**Simplify[Cf[14, 10, 5]]**

[化简]

$$2048 x^2 (1 + x)^5 (-45 - 33x - 508x^2 + 870x^3 - 773x^4 - 265x^5 + 1450x^6 - 1100x^7 + 308x^8)$$

**Simplify[Cf[14, 10, 6]]**

[化简]

$$-2048 x^2 (1 + x)^5 (53 + 837x^2 - 1888x^3 + 3187x^4 - 3528x^5 + 2623x^6 - 1528x^7 + 436x^8)$$

**Simplify[Cf[14, 10, 7]]**

[化简]

$$2048 x^2 (1 + x)^5 (-45 - 33x - 508x^2 + 870x^3 - 773x^4 - 265x^5 + 1450x^6 - 1100x^7 + 308x^8)$$

**Simplify[Cf[14, 10, 8]]**

[化简]

$$-1024 x^2 (1 + x)^5 (67 + 2x + 857x^2 - 2092x^3 + 3073x^4 - 3126x^5 + 1695x^6 - 736x^7 + 260x^8)$$

**Simplify[Cf[14, 10, 9]]**

[化简]

$$4096 (-1 + x)^2 x^2 (1 + x)^5 (-9 - 18x - 124x^2 + 82x^3 - 207x^4 + 4x^5 + 40x^6)$$

**Simplify[Cf[14, 10, 10]]**

[化简]

$$-2048 (-1 + x)^3 x^2 (1 + x)^5 (-7 - 25x - 57x^2 - 55x^3 - 116x^4 + 44x^5)$$

**Simplify[Cf[14, 10, 11]]**

[化简]

$$4096 (-1 + x)^4 x^2 (1 + x)^5 (-1 - 2x - 11x^2 - 8x^3 + 2x^4)$$

**Simplify[Cf[14, 10, 12]]**

[化简]

$$4096 x^3 (-1 + x^2)^5$$

**Simplify[Cf[14, 10, 13]]**

[\[化简\]](#)

0

**Simplify[Cf[14, 10, 14]]**

[\[化简\]](#)

0

**(\*, r2^14r3^11\*)**

**Simplify[Cf[14, 11, 0]]**

[\[化简\]](#)

$4096 (-1+x)^5 x^3 (1+x)^6$

**Simplify[Cf[14, 11, 1]]**

[\[化简\]](#)

$4096 (-1+x)^4 x^2 (1+x)^5 (-1-2x-11x^2-8x^3+2x^4)$

**Simplify[Cf[14, 11, 2]]**

[\[化简\]](#)

$-2048 (-1+x)^3 x^2 (1+x)^5 (-3-44x+37x^2-182x^3+60x^4)$

**Simplify[Cf[14, 11, 3]]**

[\[化简\]](#)

$-2048 (-1+x)^2 x^2 (1+x)^5 (9+60x+34x^2+56x^3+177x^4-188x^5+28x^6)$

**Simplify[Cf[14, 11, 4]]**

[\[化简\]](#)

$2048 x^2 (1+x)^5 (-11-116x+337x^2-822x^3+1271x^4-1020x^5+567x^6-250x^7+44x^8)$

**Simplify[Cf[14, 11, 5]]**

[\[化简\]](#)

$-2048 x^2 (1+x)^5 (15+129x-276x^2+570x^3-597x^4+37x^5+198x^6-96x^7+20x^8)$

**Simplify[Cf[14, 11, 6]]**

[\[化简\]](#)

$-2048 x^2 (1+x)^5 (15+129x-276x^2+570x^3-597x^4+37x^5+198x^6-96x^7+20x^8)$

**Simplify[Cf[14, 11, 7]]**

[\[化简\]](#)

$2048 x^2 (1+x)^5 (-11-116x+337x^2-822x^3+1271x^4-1020x^5+567x^6-250x^7+44x^8)$

**Simplify[Cf[14, 11, 8]]**

[\[化简\]](#)

$-2048 (-1+x)^2 x^2 (1+x)^5 (9+60x+34x^2+56x^3+177x^4-188x^5+28x^6)$

**Simplify[Cf[14, 11, 9]]**

[\[化简\]](#)

$-2048 (-1+x)^3 x^2 (1+x)^5 (-3-44x+37x^2-182x^3+60x^4)$

**Simplify[Cf[14, 11, 10]]**

[化简]

$$4096 (-1+x)^4 x^2 (1+x)^5 (-1-2x-11x^2-8x^3+2x^4)$$

**Simplify[Cf[14, 11, 11]]**

[化简]

$$4096 (-1+x)^5 x^3 (1+x)^6$$

**Simplify[Cf[14, 11, 12]]**

[化简]

0

**Simplify[Cf[14, 11, 13]]**

[化简]

0

**Simplify[Cf[14, 11, 14]]**

[化简]

0

(\*, r2^14r3^12\*)

**Simplify[Cf[14, 12, 0]]**

[化简]

$$4096 x^3 (-1+x^2)^5$$

**Simplify[Cf[14, 12, 1]]**

[化简]

$$-2048 (-1+x)^4 x^2 (1+x)^5 (2-3x+30x^2-21x^3+4x^4)$$

**Simplify[Cf[14, 12, 2]]**

[化简]

$$1024 (-1+x)^3 x^2 (1+x)^5 (7+19x+13x^2+137x^3-172x^4+44x^5)$$

**Simplify[Cf[14, 12, 3]]**

[化简]

$$-2048 (-1+x)^2 x^2 (1+x)^5 (9-14x+132x^2-190x^3+207x^4-180x^5+52x^6)$$

**Simplify[Cf[14, 12, 4]]**

[化简]

$$1024 (-1+x)^2 x^2 (1+x)^5 (-21-24x-78x^2-328x^3+551x^4-424x^5+148x^6)$$

**Simplify[Cf[14, 12, 5]]**

[化简]

$$-4096 (-1+x)^2 x^2 (1+x)^5 (7-7x+96x^2-102x^3+149x^4-111x^5+40x^6)$$

**Simplify[Cf[14, 12, 6]]**

[化简]

$$1024 (-1+x)^2 x^2 (1+x)^5 (-21-24x-78x^2-328x^3+551x^4-424x^5+148x^6)$$

**Simplify[Cf[14, 12, 7]]**[\[化简\]](#)

$$-2048 (-1+x)^2 x^2 (1+x)^5 (9-14x+132x^2-190x^3+207x^4-180x^5+52x^6)$$

**Simplify[Cf[14, 12, 8]]**[\[化简\]](#)

$$1024 (-1+x)^3 x^2 (1+x)^5 (7+19x+13x^2+137x^3-172x^4+44x^5)$$

**Simplify[Cf[14, 12, 9]]**[\[化简\]](#)

$$-2048 (-1+x)^4 x^2 (1+x)^5 (2-3x+30x^2-21x^3+4x^4)$$

**Simplify[Cf[14, 12, 10]]**[\[化简\]](#)

$$4096 x^3 (-1+x^2)^5$$

**Simplify[Cf[14, 12, 11]]**[\[化简\]](#)

$$0$$

**Simplify[Cf[14, 12, 12]]**[\[化简\]](#)

$$0$$

**Simplify[Cf[14, 12, 13]]**[\[化简\]](#)

$$0$$

**Simplify[Cf[14, 12, 14]]**[\[化简\]](#)

$$0$$

**(\*, r2^14r3^13\*)****Simplify[Cf[14, 13, 0]]**[\[化简\]](#)

$$-2048 (-1+x)^6 x^3 (1+x)^5$$

**Simplify[Cf[14, 13, 1]]**[\[化简\]](#)

$$6144 (-1+x)^5 x^3 (1+x)^6$$

**Simplify[Cf[14, 13, 2]]**[\[化简\]](#)

$$-12288 (-1+x)^3 x^3 (1+x)^5 (-1+x^2)$$

**Simplify[Cf[14, 13, 3]]**[\[化简\]](#)

$$-4096 (-1+x)^3 x^3 (1+x)^5 (-5-3x^2+4x^3)$$

**Simplify[Cf[14, 13, 4]]**

[化简]

$$12\,288 (-1+x)^3 x^3 (1+x)^5 (2+x+x^3)$$

**Simplify[Cf[14, 13, 5]]**

[化简]

$$12\,288 (-1+x)^3 x^3 (1+x)^5 (2+x+x^3)$$

**Simplify[Cf[14, 13, 6]]**

[化简]

$$-4096 (-1+x)^3 x^3 (1+x)^5 (-5-3x^2+4x^3)$$

**Simplify[Cf[14, 13, 7]]**

[化简]

$$-12\,288 (-1+x)^3 x^3 (1+x)^5 (-1+x^2)$$

**Simplify[Cf[14, 13, 8]]**

[化简]

$$6144 (-1+x)^5 x^3 (1+x)^6$$

**Simplify[Cf[14, 13, 9]]**

[化简]

$$-2048 (-1+x)^6 x^3 (1+x)^5$$

**Simplify[Cf[14, 13, 10]]**

[化简]

0

**Simplify[Cf[14, 13, 11]]**

[化简]

0

**Simplify[Cf[14, 13, 12]]**

[化简]

0

**Simplify[Cf[14, 13, 13]]**

[化简]

0

**Simplify[Cf[14, 13, 14]]**

[化简]

0

(\*, r2^14r3^14\*)

**Simplify[Cf[14, 14, 0]]**

[化简]

0

**Simplify[Cf[14, 14, 1]]**

[化简]

0

**Simplify[Cf[14, 14, 2]]**

[化简]

0

**Simplify[Cf[14, 14, 3]]**

[化简]

0

**Simplify[Cf[14, 14, 4]]**

[化简]

0

**Simplify[Cf[14, 14, 5]]**

[化简]

0

**Simplify[Cf[14, 14, 6]]**

[化简]

0

**Simplify[Cf[14, 14, 7]]**

[化简]

0

**Simplify[Cf[14, 14, 8]]**

[化简]

0

**Simplify[Cf[14, 14, 9]]**

[化简]

0

**Simplify[Cf[14, 14, 10]]**

[化简]

0

**Simplify[Cf[14, 14, 11]]**

[化简]

0

**Simplify[Cf[14, 14, 12]]**

[化简]

0

**Simplify[Cf[14, 14, 13]]**

[化简]

0

```
Simplify[Cf[14, 14, 14]]
```

[化简]

```
0
```
